# Supplementary material for: The diversity of rotation curves of simulated galaxies with cusps and cores
Source: arXiv:2203.16652 source file (2024-06-07)
Supplement: Supplementary file 1 [file appendices.tex]

\documentclass[fleqn,usenatbib]{mnras}
\usepackage{newtxtext,newtxmath}
\usepackage[T1]{fontenc}

\DeclareRobustCommand{\VAN}[3]{#2}
\let\VANthebibliography\thebibliography
\def\thebibliography{\DeclareRobustCommand{\VAN}[3]{##3}\VANthebibliography}

\usepackage{graphicx}
\usepackage{amsmath}
\usepackage{bm}
\usepackage{xr-hyper}

\newcommand{\sgn}{\text{sgn}}

\makeatletter
\newcommand*{\addFileDependency}[1]{%
  \typeout{(#1)}%
  \@addtofilelist{#1}%
  \IfFileExists{#1}{}{\typeout{No file #1.}}%
}
\makeatother

\newcommand*{\myexternaldocument}[1]{%
    \externaldocument{#1}%
    \addFileDependency{#1.tex}%
    \addFileDependency{#1.aux}%
}

\myexternaldocument{../paper}

\usepackage{caption}
\DeclareCaptionLabelFormat{supfig}{Supplementary~Figure~#2}
\captionsetup[figure]{labelformat=supfig}
\DeclareCaptionLabelFormat{suptab}{Supplementary~Table~#2}
\captionsetup[table]{labelformat=suptab}

\newcommand{\appropto}{\mathrel{\vcenter{
  \offinterlineskip\halign{\hfil$##$\cr
    \propto\cr\noalign{\kern2pt}\sim\cr\noalign{\kern-2pt}}}}}

\defcitealias{NFW96}{NFW}
\defcitealias{Oman+19}{O19}
\defcitealias{SantosSantos+20}{SS20}

\usepackage{hyperref}
\usepackage{float}
\usepackage{pdflscape}

\title[Supplementary materials]{The diversity of rotation curves of simulated galaxies with cusps and cores: Appendices}

\author[F. A. Roper et al.]{\newauthor
Finn A. Roper$^{1,2,3}$\footnotemark[1]{},
Kyle A. Oman$^{2,3}$\footnotemark[1]{},
Carlos S. Frenk$^{2,3}$,
Alejandro Ben{\'i}tez-Llambay$^{4}$,
Julio F. Navarro$^{5}$,\newauthor
and Isabel M.E. Santos-Santos$^{2,3,5}$
\\
$^{1}$ Institute for Astronomy, University of Edinburgh, Royal Observatory, Blackford Hill, Edinburgh EH9 3HJ, United Kingdom\\
$^{2}$ Institute for Computational Cosmology, Durham University, South Road, Durham DH1 3LE, United Kingdom\\
$^{3}$ Department of Physics, Durham University, South Road, Durham DH1 3LE, United Kingdom\\
$^{4}$ University of Milano-Bicocca, Piazza della Scienza, 3, 20126 Milano MI, Italy\\
$^{5}$ Department of Physics and Astronomy, University of Victoria, Victoria, BC, Canada V8P 5C2\\
}

\date{\today}

\pubyear{\the\year}

\begin{document}
\label{firstpage-appendix}
\pagerange{\pageref{firstpage-appendix}--\pageref{lastpage-appendix}}
\onecolumn
\maketitle

\footnotetext[1]{E-mail: finn.roper@ed.ac.uk, kyle.a.oman@durham.ac.uk}

\noindent These appendices include:

\smallskip

\textbf{Appendix A.} Comparisons with observed velocity dispersion profiles and surface density profiles.

\textbf{Appendix B.} Tables listing properties of galaxies selected for kinematic analysis, and detailing reasons some galaxies were excluded from this analysis.

\textbf{Appendix C.} A full listing of our $^{\mathrm{3D}}${\sc barolo} configuration.

\textbf{Appendix D.} A description of the algorithm used to define $V_\mathrm{\lowercase{\phi,max}}$ for rotation curves from simulation.

\textbf{Appendix E.} Summaries of the kinematic analysis of each individual galaxy, including figures similar to Figs.~\ref{fig:visualisations}, \ref{fig:rot_curves}, and \ref{fig:loops}.

\appendix

\clearpage
\section{\texorpdfstring{Comparison with observed velocity dispersion profiles and surface density profiles}{Comparison with observed velocity dispersion profiles and surface density profiles}}
\label{appendix:extra_figures}

We provide additional figures to supplement the discussion of the realism of our simulated galaxies in Sec.~\ref{sec:realism}. Supplementary~Figs.~\ref{fig:dispersion_profiles}~and~\ref{fig:surface_density_profiles} show velocity dispersion and surface density profiles, both important when considering disc thicknesses and kinematic modelling, from mock observations of simulated dwarfs galaxies used in this work and compares them to dispersion profiles from observations of nearby dwarfs.

\clearpage

\begin{figure*}
\centering
\includegraphics[width=\textwidth]{../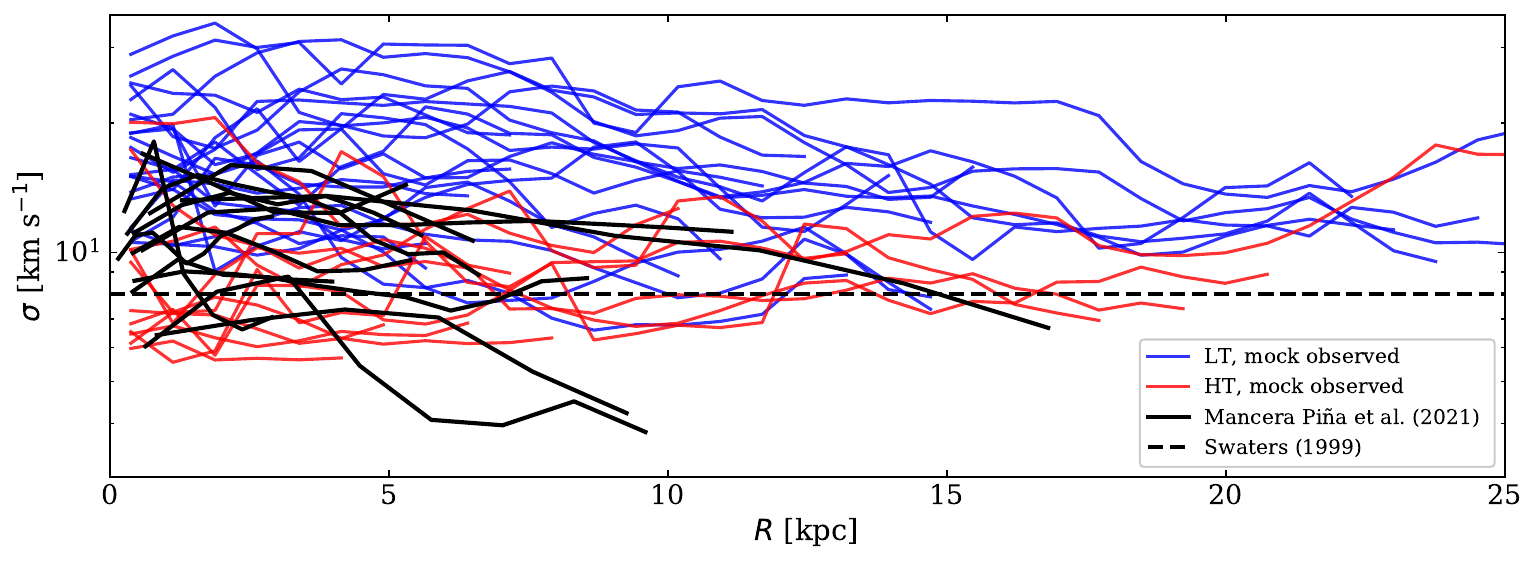}
\caption{Velocity dispersion profiles from mock observations of LT and HT galaxies selected for kinematic analysis (blue and red lines, respectively) with comparison to measurements from selected late-type dwarfs, also with ${50 < V_\mathrm{c,max} / \mathrm{km \, s}^{-1} < 120}$, from LVHIS \citep{Koribalski+18} and WHISP \citep{vanderHulst+01} observations and analysed by \citet[][solid black lines]{ManceraPina+21}, and an estimated constant value of $8 \, \mathrm{km \, s}^{-1}$ found by \citet[][dashed line]{Swaters99}. For visual clarity, only dispersion profiles corresponding to mock observations of LT and HT galaxies at $\Phi = 0\degr$ are shown (see Supplementary~Figs.~\ref{fig:S1}--\ref{fig:S21} and \ref{fig:S47}--\ref{fig:S89}, panels (l), for dispersion profiles from all mock observations and from simulations). HT galaxies follow the observed profiles well, however several LT galaxies are seen to have somewhat greater velocity dispersions at all radii.}
\label{fig:dispersion_profiles}
\end{figure*}

\begin{figure*}
\centering
\includegraphics[width=0.8\textwidth]{../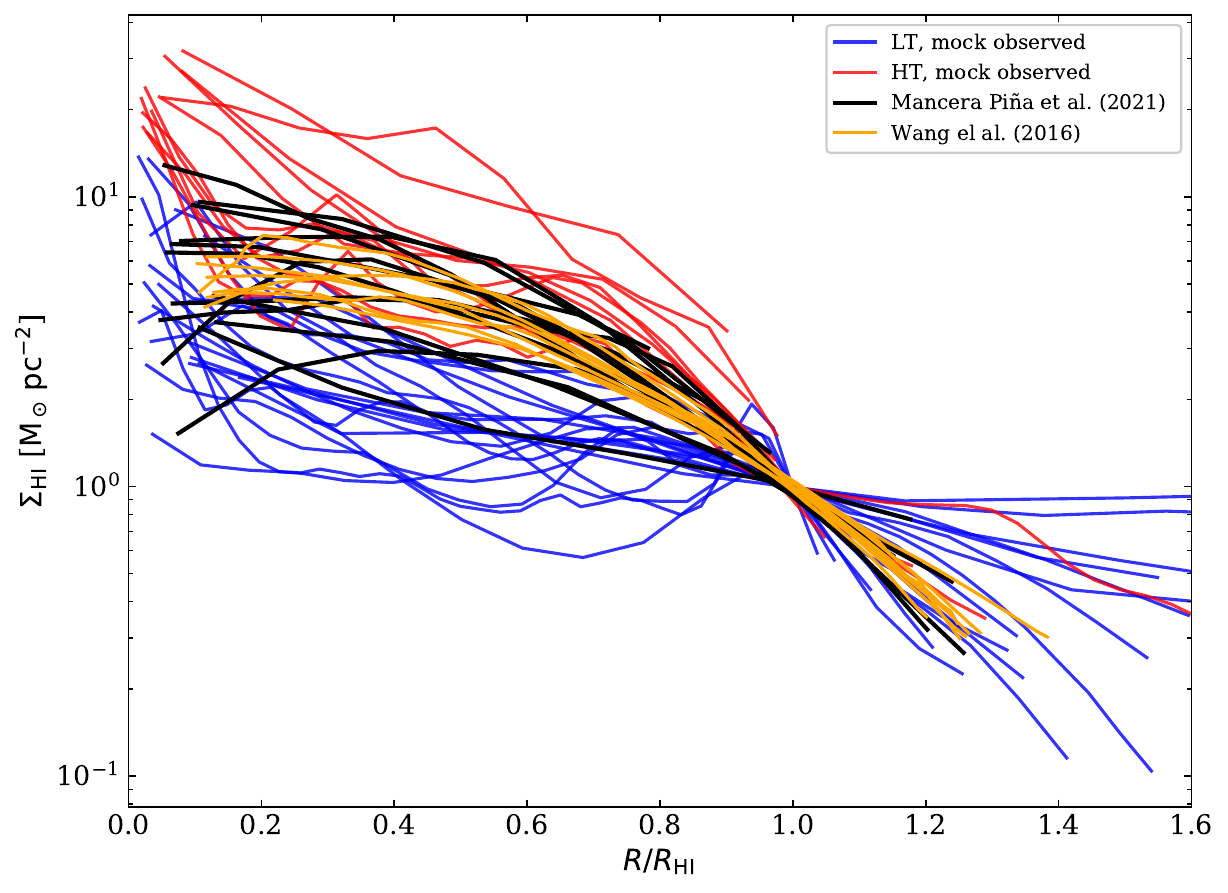}
\caption{Face-on (inclination-corrected) \ion{H}{i} surface density profiles from mock observations of LT and HT galaxies selected for kinematic analysis (blue and red lines, respectively) with comparison to measurements from selected late-type dwarfs, also with ${50 < V_\mathrm{c,max} / \mathrm{km \, s}^{-1} < 120}$, from LVHIS \citep{Koribalski+18} and WHISP \citep{vanderHulst+01} observations and analysed by \citet[][black lines]{ManceraPina+21}, and median profiles from samples of galaxies from WHISP (separate profiles for S and Sa galaxies), VIVA, LVHIS, Bluedisk, THINGS, LITTLE~THINGS, and FIGGS surveys \citep[][and references therein, orange lines]{Wang+16}. Here, ${R_\mathrm{HI} \equiv R(\Sigma_\mathrm{HI} = 1 \, \mathrm{M}_{\sun} \, \mathrm{pc}^{-2})}$ is found using (mock) observations; for profiles that do not fall to ${1 \, \mathrm{M}_{\sun} \, \mathrm{pc}^{-2}}$, $R_\mathrm{HI}$ is found from extrapolation. For visual clarity, only surface density profiles corresponding to mock observations of LT and HT galaxies at $\Phi = 0\degr$ are shown (see Supplementary~Figs.~\ref{fig:S1}--\ref{fig:S21} and \ref{fig:S47}--\ref{fig:S89}, panels (n), for surface density profiles from all mock observations and from simulations). The ranges of $\Sigma_\mathrm{HI}$ within $R_\mathrm{HI}$ of both LT and HT selected samples significantly overlap with that of the \citet{ManceraPina+21} sample, however are on average approximately ${0.3 \, \mathrm{dex}}$ higher and lower, respectively. LT and HT profiles are generally more irregular, primarily due to automated and therefore imperfect model fitting (see Sec.~\ref{subsubsec:model_optimisation} for further discussion).}
\label{fig:surface_density_profiles}
\end{figure*}

\clearpage
\section{Simulated galaxy sample selection}
\label{appendix:sample}

Supplementary~Table~\ref{tab:selected} lists galaxies from the LT and HT simulations selected for kinematic analysis, along with some of their key properties. Supplementary~Tables~\ref{tab:excludedLT}~and~\ref{tab:excludedHT} respectively list LT and HT galaxies excluded from our sample for kinematic analysis after visual inspection of \ion{H}{i} surface density maps and velocity fields along all projection angles. Individual reasons for exclusion are also listed. We label galaxies by the simulation model (LT or HT) and their FoF group number as recorded in the simulation outputs (recalling that all galaxies which we consider are centrals, and so have sub-group numbers of $0$, such that these labels are sufficient to uniquely specify each object).
\clearpage

\begin{table*}
  \caption{Galaxies selected for mock kinematic analysis. The initial sample is selected to have $50<V_\mathrm{c,max}/\mathrm{km}\,\mathrm{s}^{-1}<120$, $M_\mathrm{HI}>10^{8}\,\mathrm{M}_{\sun}$, yielding $49$~LT and $45$~HT galaxies. These were visually inspected to determine which were suitable for automated kinematic analysis, leaving $21$~LT and $11$~HT galaxies. Details of the galaxies omitted after visual inspection are given in Supplementary~Tables~\ref{tab:excludedLT}~and~\ref{tab:excludedHT}. Columns: {\bf (1)} simulation from which galaxy is drawn; {\bf (2)} friends-of-friend identifier as recorded by {\sc subfind}; {\bf (3)} friends-of-friends identifier of subhalo in opposite sample corresponding to the same initial system evolved with different SF density threshold; {\bf (4)} maximum circular velocity; {\bf (5)} `fiducial radius' $R_\mathrm{c,fid}/\mathrm{kpc}=V_\mathrm{c,max}/35\,\mathrm{km}\,\mathrm{s}^{-1}$; {\bf (6)} circular velocity at $R_\mathrm{c,fid}$; {\bf (7)} stellar mass; {\bf (8)} atomic hydrogen mass; {\bf (9)} radius where atomic hydrogen surface density drops below $1\mathrm{M}_{\sun}\,\mathrm{pc}^{-2}$; {\bf (10)} $\eta_\mathrm{rot}=V_\mathrm{c,fid}/V_\mathrm{c,max}$, tracing how steeply rising the circular velocity curve is; {\bf (11)} $\eta_\mathrm{bar}=(V_\mathrm{b,fid}/V_\mathrm{c,fid})^2$, tracing how centrally baryon-dominated the galaxy is.}
  \label{tab:selected}
  \begin{tabular}{crrrrrrrrr}
    \hline
    Simulation &
    &
    \multicolumn{1}{c}{$V_\mathrm{c,max}$} &
    \multicolumn{1}{c}{$R_\mathrm{c,fid}$} &
    \multicolumn{1}{c}{$V_\mathrm{c,fid}$} &
    \multicolumn{1}{c}{$M_\star$} &
    \multicolumn{1}{c}{$M_\mathrm{HI}$} &
    \multicolumn{1}{c}{$R_\mathrm{HI}$} &
    &
    \\
    model &
    \multicolumn{1}{c}{FoF} &
    \multicolumn{1}{c}{$[{\rm km}\,{\rm s}^{-1}]$} &
    \multicolumn{1}{c}{$[\mathrm{kpc}]$} &
    \multicolumn{1}{c}{$[{\rm km}\,{\rm s}^{-1}]$} &
    \multicolumn{1}{c}{$[\mathrm{M}_{\sun}]$} &
    \multicolumn{1}{c}{$[\mathrm{M}_{\sun}]$} &
    \multicolumn{1}{c}{$[\mathrm{kpc}]$} &
    \multicolumn{1}{c}{$\eta_\mathrm{rot}$} &
    \multicolumn{1}{c}{$\eta_\mathrm{bar}$} \\
    \hline
    LT & $11$ & $110$ & $3.1$ & $77$ & $2.2 \times 10^{9}$ & $3.8 \times 10^{9}$ & $25.4$ & $0.70$ & $0.22$ \\
    LT & $14$ & $99$ & $2.8$ & $63$ & $2.1 \times 10^{9}$ & $3.1 \times 10^{9}$ & $24.8$ & $0.64$ & $0.25$ \\
    LT & $16$ & $93$ & $2.7$ & $80$ & $1.7 \times 10^{9}$ & $2.5 \times 10^{8}$ & $5.4$ & $0.86$ & $0.23$ \\
    LT & $17$ & $89$ & $2.5$ & $62$ & $7.9 \times 10^{8}$ & $2.7 \times 10^{9}$ & $24.1$ & $0.69$ & $0.15$ \\
    LT & $18$ & $95$ & $2.7$ & $67$ & $2.1 \times 10^{9}$ & $2.0 \times 10^{9}$ & $18.2$ & $0.71$ & $0.27$ \\
    LT & $19$ & $102$ & $2.9$ & $88$ & $2.6 \times 10^{9}$ & $8.1 \times 10^{8}$ & $10.0$ & $0.86$ & $0.27$ \\
    LT & $22$ & $80$ & $2.3$ & $50$ & $6.6 \times 10^{8}$ & $1.5 \times 10^{9}$ & $16.4$ & $0.62$ & $0.14$ \\
    LT & $24$ & $89$ & $2.5$ & $64$ & $1.5 \times 10^{9}$ & $1.4 \times 10^{9}$ & $15.9$ & $0.72$ & $0.21$ \\
    LT & $26$ & $68$ & $2.0$ & $49$ & $3.0 \times 10^{8}$ & $8.1 \times 10^{8}$ & $10.2$ & $0.72$ & $0.13$ \\
    LT & $29$ & $73$ & $2.1$ & $47$ & $4.2 \times 10^{8}$ & $1.4 \times 10^{9}$ & $13.7$ & $0.64$ & $0.17$ \\
    LT & $35$ & $76$ & $2.2$ & $51$ & $1.0 \times 10^{9}$ & $8.5 \times 10^{8}$ & $12.0$ & $0.68$ & $0.18$ \\
    LT & $38$ & $56$ & $1.6$ & $31$ & $2.7 \times 10^{7}$ & $1.2 \times 10^{9}$ & $12.5$ & $0.56$ & $0.08$ \\
    LT & $41$ & $72$ & $2.1$ & $45$ & $4.1 \times 10^{8}$ & $6.0 \times 10^{8}$ & $9.8$ & $0.62$ & $0.10$ \\
    LT & $44$ & $70$ & $2.0$ & $40$ & $1.4 \times 10^{8}$ & $9.7 \times 10^{8}$ & $13.8$ & $0.57$ & $0.09$ \\
    LT & $46$ & $74$ & $2.1$ & $50$ & $3.8 \times 10^{8}$ & $3.2 \times 10^{8}$ & $2.7$ & $0.68$ & $0.14$ \\
    LT & $47$ & $58$ & $1.7$ & $33$ & $2.0 \times 10^{8}$ & $4.2 \times 10^{8}$ & $7.9$ & $0.56$ & $0.10$ \\
    LT & $51$ & $66$ & $1.9$ & $45$ & $2.2 \times 10^{8}$ & $3.9 \times 10^{8}$ & $1.8$ & $0.68$ & $0.10$ \\
    LT & $54$ & $65$ & $1.9$ & $47$ & $1.3 \times 10^{8}$ & $1.8 \times 10^{8}$ & $1.7$ & $0.72$ & $0.10$ \\
    LT & $60$ & $57$ & $1.6$ & $37$ & $7.6 \times 10^{7}$ & $1.1 \times 10^{8}$ & $3.8$ & $0.65$ & $0.09$ \\
    LT & $70$ & $51$ & $1.5$ & $36$ & $9.3 \times 10^{7}$ & $1.3 \times 10^{8}$ & $4.4$ & $0.71$ & $0.08$ \\
    LT & $72$ & $51$ & $1.4$ & $33$ & $4.4 \times 10^{7}$ & $2.5 \times 10^{8}$ & $5.9$ & $0.65$ & $0.16$ \\
    \hline
    HT & $12$ & $101$ & $2.9$ & $37$ & $8.5 \times 10^{8}$ & $5.9 \times 10^{9}$ & $21.1$ & $0.37$ & $0.43$ \\
    HT & $23$ & $83$ & $2.4$ & $30$ & $2.3 \times 10^{8}$ & $3.4 \times 10^{9}$ & $18.4$ & $0.36$ & $0.43$ \\
    HT & $24$ & $88$ & $2.5$ & $37$ & $4.7 \times 10^{8}$ & $2.4 \times 10^{9}$ & $14.4$ & $0.42$ & $0.40$ \\
    HT & $26$ & $71$ & $2.0$ & $44$ & $8.8 \times 10^{7}$ & $1.4 \times 10^{9}$ & $8.4$ & $0.62$ & $0.37$ \\
    HT & $28$ & $75$ & $2.1$ & $29$ & $3.4 \times 10^{8}$ & $1.4 \times 10^{9}$ & $11.3$ & $0.39$ & $0.42$ \\
    HT & $29$ & $80$ & $2.3$ & $41$ & $1.2 \times 10^{8}$ & $3.5 \times 10^{9}$ & $20.2$ & $0.51$ & $0.30$ \\
    HT & $39$ & $75$ & $2.1$ & $36$ & $7.3 \times 10^{7}$ & $2.8 \times 10^{9}$ & $15.8$ & $0.48$ & $0.39$ \\
    HT & $40$ & $55$ & $1.6$ & $35$ & $1.2 \times 10^{7}$ & $1.1 \times 10^{9}$ & $8.7$ & $0.63$ & $0.39$ \\
    HT & $55$ & $52$ & $1.5$ & $32$ & $2.9 \times 10^{7}$ & $6.1 \times 10^{8}$ & $5.5$ & $0.62$ & $0.57$ \\
    HT & $60$ & $52$ & $1.5$ & $32$ & $2.1 \times 10^{7}$ & $3.8 \times 10^{8}$ & $5.0$ & $0.61$ & $0.44$ \\
    HT & $86$ & $52$ & $1.5$ & $29$ & $2.1 \times 10^{7}$ & $8.8 \times 10^{8}$ & $7.8$ & $0.56$ & $0.64$ \\
    \hline
  \end{tabular}
\end{table*}

\begin{table*}
  \caption{Galaxies from the LT simulation excluded from kinematic analysis after visual inspection (see Supplementary~Table~\ref{tab:selected} for details of initial selection). Columns: {\bf (1)} simulation from which galaxy is drawn; {\bf (2)} friends-of-friends identifier as recorded by {\sc subfind}; {\bf (3)} whether galaxy was excluded based on inspection of particle distribution and moment maps (tick mark), or on the basis of kinematic modelling failure (no tick mark); {\bf (4)} reason the galaxy was excluded from kinematic analysis. For modelling failures, the probable reason is given. A brief explanation of common reasons for exclusion follows. No clear disc: viewing atomic hydrogen distribution from various angles revealed no morphological disc structure. Unclear rotation axis: severe misalignment between kinematic and morphological major axes; extreme warps; strong radial bulk flows within disc; or absence or any rotation pattern whatsoever. Merger or close companion: a companion system within ${100 \, \mathrm{kpc}}$ not satisfying cuts in Sec.~\ref{subsubsec:sim_samples} yet clearly gravitationally interacting. Galaxies from the HT simulation excluded from kinematic analysis after visual inspection are listed in Supplementary~Table~\ref{tab:excludedHT}.}
  \label{tab:excludedLT}
  \begin{tabular}{crcl}
    \hline
    Simulation &
    &
    Excluded before &
    \\
    model &
    FoF &
    kin. modelling? &
    Reason for exclusion \\
    \hline
    LT & 12 & \checkmark & No clear disc. \\
    LT & 13 & \checkmark & Counter-rotating central disc. \\
    LT & 15 & \checkmark & Unclear rotation axis. \\
    LT & 20 &            & Obvious tidal interaction. \\
    LT & 21 & \checkmark & No clear disc. \\
    LT & 23 & \checkmark & No clear disc. \\
    LT & 25 & \checkmark & No clear disc. \\
    LT & 27 &            & One side of disc disrupted. \\
    LT & 28 &            & One side of disc disrupted. \\
    LT & 30 & \checkmark & No clear disc. \\
    LT & 31 & \checkmark & Merger. \\
    LT & 32 &            & One side of disc disrupted. \\
    LT & 33 & \checkmark & No clear disc. \\
    LT & 36 & \checkmark & Merger. \\
    LT & 37 & \checkmark & No clear disc. \\
    LT & 39 & \checkmark & Unclear rotation axis. \\
    LT & 40 &            & Obvious tidal interaction. \\
    LT & 43 & \checkmark & Unclear rotation axis. \\
    LT & 45 & \checkmark & No clear disc. \\
    LT & 48 & \checkmark & Unclear rotation axis. \\
    LT & 49 & \checkmark & No clear disc. \\
    LT & 50 & \checkmark & Unclear rotation axis. \\
    LT & 62 & \checkmark & No clear disc. \\
    LT & 63 & \checkmark & No clear disc. \\
    LT & 67 & \checkmark & Unclear rotation axis. \\
    \hline
  \end{tabular}
\end{table*}

\begin{table*}
  \caption{As Supplementary~Table~\ref{tab:excludedLT}, but for galaxies from the HT simulation.}
  \label{tab:excludedHT}
  \begin{tabular}{crcl}
    \hline
    Simulation &
    &
    Excluded before &
    \\
    model &
    FoF &
    kin. modelling? &
    Reason for exclusion \\
    \hline
    HT & 10 & \checkmark & Merger. \\
    HT & 11 & \checkmark & No clear disc. \\
    HT & 13 & \checkmark & Unclear rotation axis. \\
    HT & 14 & \checkmark & Unclear rotation axis. \\
    HT & 15 & \checkmark & Unclear rotation axis. \\
    HT & 16 & \checkmark & Unclear rotation axis. \\
    HT & 17 & \checkmark & Extreme outer warp. \\
    HT & 18 &            & Supernova bubbles near centre. \\
    HT & 19 & \checkmark & Unclear rotation axis. \\
    HT & 20 & \checkmark & No clear disc. \\
    HT & 21 & \checkmark & No clear disc. \\
    HT & 22 & \checkmark & Unclear rotation axis. \\
    HT & 25 & \checkmark & No clear disc. \\
    HT & 27 & \checkmark & No clear disc. \\
    HT & 30 & \checkmark & No clear disc. \\
    HT & 31 & \checkmark & Merger. \\
    HT & 32 & \checkmark & Unclear rotation axis. \\
    HT & 33 & \checkmark & No clear disc. \\
    HT & 34 & \checkmark & Unclear rotation axis. \\
    HT & 36 & \checkmark & Merger. \\
    HT & 38 & \checkmark & Merger. \\
    HT & 41 & \checkmark & Unclear rotation axis. \\
    HT & 43 & \checkmark & Unclear rotation axis. \\
    HT & 44 & \checkmark & Close companion. \\
    HT & 46 & \checkmark & No clear disc. \\
    HT & 47 & \checkmark & Close companion. \\
    HT & 48 &            & Incorrect systemic velocity. \\
    HT & 50 &            & Incorrect systemic velocity. \\
    HT & 54 & \checkmark & Unclear rotation axis. \\
    HT & 62 & \checkmark & No clear disc. \\
    HT & 64 & \checkmark & No clear disc. \\
    HT & 67 &            & Incorrect systemic velocity. \\
    \hline
  \end{tabular}
\end{table*}

\clearpage
\section{\texorpdfstring{$^\mathrm{3D}${\sc barolo} configuration}{3DBarolo configuration}} 
\label{Appendix3DB}

Supplementary~Table~\ref{tab:3DBconfig} lists the full configuration of $^{\mathrm{3D}}${\sc barolo} used for all tilted-ring kinematic modelling of simulated systems in this work. We omit parameters such as file paths, flags to enable optional visualisation outputs, etc.
\clearpage

\begin{table*}
  \caption{Parameters used to configure the tilted-ring modelling tool, $^{\mathrm{3D}}${\sc barolo}, omitting parameters such as file paths, flags to enable optional outputs, etc. Configuration is based on that used in \citetalias{Oman+19} and \citet{Iorio+17}. See the $^{\mathrm{3D}}${\sc barolo}’s release paper (\citealt{DiTeodoro&Fraternali15}, see also \citealt{Iorio+17}) for further discussion of the parameters.}
  \label{tab:3DBconfig}
  \begin{tabular}{lrll}
    \hline
    Parameter & Value & Unit & Description \\
    \hline
    NRADII & \textit{varies} & - & Number of rings in the model; equal to the minimum number needed to enclose $R_{\mathrm{last}}$, \\
     & & & usually the radius of a sphere enclosing $90$~per~cent of the subhalo’s \ion{H}{i} mass. \\
    RADSEP & 12.0 & $\mathrm{arcsec}$ & Separation between rings. \\
    XPOS & \textit{varies} & px & Ring centre $x$-coordinate in the data cube; corresponds to the gravitational potential \\
     & & & minimum of the subhalo. \\
    YPOS & \textit{varies} & px & Similar to XPOS. \\
    VSYS & 907.57 & $\mathrm{km}\,\mathrm{s}^{-1}$ & Line-of-sight systemic velocity. \\
    VROT & 30 & $\mathrm{km}\,\mathrm{s}^{-1}$ & Initial value for rotational velocity \\
    VDISP & 8 & $\mathrm{km}\,\mathrm{s}^{-1}$ & Initial value for velocity dispersion. \\
    VRAD & 0 & $\mathrm{km}\,\mathrm{s}^{-1}$ & Initial value for radial velocity. \\
    INC & 60.00 & $\degr$ & Initial value for inclination. \\
    PA & 270.00 & $\degr$ & Initial value for position angle. \\
    Z0 & 1.6000 & $\mathrm{arcsec}$ & Scale-height of the disc. \\
    DELTAINC & 15 & $\degr$ & Allowed deviation in inclination from initial value. \\
    DELTAPA & 20 & $\degr$ & Allowed deviation in position angle from initial value. \\
    FREE & VROT INC VDISP PA & - & Free ring parameters to fit. \\
    FTYPE & 2 & - & Specifies the function to be minimised when fitting as the absolute difference \\
    & & & between model and data cube, $\lvert \mathrm{mod} - \mathrm{obs} \lvert$. \\
    WFUNC & 1 & - & Specifies the azimuthal weighting function used when fitting as $\lvert \cos \theta \lvert$, where \\
     & & & ${\theta=0}$ corresponds to the major axis. \\
    LTYPE & 1 & - & Specifies the layer type along $z$ as Gaussian. \\
    CDENS & 10 & $10^{20} \, \mathrm{cm}^{-2}$ & Surface density of atoms in clouds in the plane of the rings per pixel area. \\
    SIDE & B & - & Both sides of the galaxy are fitted. \\
    MASK & SMOOTH & - & The data cube is smoothed the factor specified by BLANKCUT and a signal-to-noise \\
    & & & cut is used to define a mask. \\
    BLANKCUT & 2.5 & - & See MASK description. \\
    NORM & LOCAL & - & Specifies pixel-by-pixel normalization of the model. \\
    TWOSTAGE & TRUE & - & Enables the second fitting stage after parameter regularisation. \\
    POLYN & bezier & - & Inclination and the position angle are regularised to a B\'{e}zier function in the second \\
    & & & fitting stage. \\
    BWEIGHT & 1 & - & Exponent of weight for blank pixels. \\
    FLAGERRORS & FALSE & - & Errors are not calculated to greatly decrease run times. \\
    LINEAR & 0.425 & channels & Standard deviation of instrumental spectral broadening. \\
    ADRIFT & TRUE & - & Calculate the asymmetric drift correction. \\
    BADOUT & TRUE & - & Also writes un-converged/bad rings in the output ringfile for debugging. \\
    FLAGROBUSTSTATS & TRUE & - & Uses robust statistics. \\
    NV & 200 & - & Number of sub-clouds in the velocity profile of a single cloud. \\
    NORMALCUBE & TRUE & - & The input cube is normalized before the fit. \\
    TOL & 0.001 & - & Minimisation tolerance. \\
    \hline
  \end{tabular}
\end{table*}

\clearpage
\section{\texorpdfstring{Description of algorithm used to define $V_\mathrm{\lowercase{\phi,max}}$}{Description of algorithm used to define Vphi,max}} \label{app:algorithm}

The algorithm used to find $V_{\mathrm{\phi,max}}$ for a single rotation curve is as follows:
\begin{enumerate}
\item Find the rotation velocity $V$ for which the highest number of data that define the rotation curve -- i.e. ($R$, $V_{\mathrm{\phi}}$) coordinates from $^{\mathrm{3D}}${\sc barolo} -- is contained by ${V \pm a_{n}V}$, for any $V$ and small ${a_{n} = a_{0}}$. The number of data contained is $N_{\mathrm{flat}}$.
\item If $N_{\mathrm{flat}}$ is less than one fifth of all velocity data or if ${N_{\mathrm{flat}} \leq 2}$, then ${V_{\mathrm{\phi,max}} \equiv V_{\mathrm{\phi}}(10 \, \mathrm{kpc})}$ (or ${V_{\mathrm{\phi}}(R_{\mathrm{last}})}$, if $R_{\mathrm{last}} < 10 \, \mathrm{kpc}$) and end here.
\item Increment $n$ by $1$ and find $V$ for which the highest number of data is contained by ${V \pm a_{n}V}$, using the recursive formula ${a_{n} = (1-b)a_{n-1}}$ for any $V$ and small $b$. The number of data contained is $N$.
\item If ${N < N_{\mathrm{flat}}}$ or ${n = n_{\mathrm{max}}}$, then ${V_{\mathrm{\phi,max}} \equiv V}$ using the last value of $V$ for which ${N = N_{\mathrm{flat}}}$. Else, if ${N = N_{\mathrm{flat}}}$, go to (iii). 
\end{enumerate}
We adopt the values ${a_{0} = 0.05}$; ${b = 0.002}$; and ${n_{\mathrm{max}} = 1000}$.

\clearpage

\clearpage
\section{Summaries of kinematic analyses of individual galaxies}
\label{app:supplementary}

We provide a set of summary figures (Supplementary~Figs.~\ref{fig:S1}--\ref{fig:S89}) for each mock observed galaxy listed in Supplementary~Tables~\ref{tab:selected}, \ref{tab:excludedLT} and \ref{tab:excludedHT}. Supplementary~Figs.~\ref{fig:S1}--\ref{fig:S21} show LT galaxies selected for kinematic analysis and Supplementary~Figs.~\ref{fig:S22}--\ref{fig:S46} show LT galaxies that are excluded. Likewise, Supplementary~Figs.~\ref{fig:S47}--\ref{fig:S57} show HT galaxies selected and Supplementary~Figs.~\ref{fig:S58}--\ref{fig:S89} show HT galaxies excluded. Figures include example moment maps for two orientations (panels (a)--(f); similar to Fig.~\ref{fig:visualisations}), a summary of the parameters $V_\mathrm{fid}$, $V_\mathrm{max}$, $\eta_\mathrm{rot}$, and $\eta_\mathrm{bar}$ (panels (g)--(j); similar to Fig.~\ref{fig:loops}), and a summary of the rotation curve analysis from $24$ viewing angles (panels (k)--(n); similar to Fig.~\ref{fig:rot_curves}). The individual panels are as follows:
\begin{itemize}
\item Panels \textbf{(a)} and \textbf{(d)} show a \ion{H}{i} surface density, $\Sigma_{\mathrm{HI}}$, calculated directly from the simulation particle distribution at projection angles ${\Phi = 0\degr}$~and~$90\degr$, respectively. Spatial resolution in panels is chosen for visual clarity. 
\item Panels \textbf{(b)} and \textbf{(e)} show 21-cm flux density $S_\mathrm{HI}$, from mock observed data cubes at ${\Phi = 0\degr}$~and~$90\degr$, respectively, using a ${12 \, \mathrm{arcsec}}$ (${750 \, \mathrm{pc}}$) FWHM circular Gaussian beam. 
\item Panels \textbf{(c)} and \textbf{(f)} show intensity-weighted mean velocity, from mock observed data cubes at $\Phi = 0\degr$~and~$90\degr$, respectively. These velocity maps are masked to show only pixels where the flux density exceeds $10^{-3} \, \mathrm{Jy} \, \mathrm{beam}^{-1}$ (indicated by the magenta contour in $S_\mathrm{HI}$; approximately $\Sigma_{\mathrm{HI}} = {1 \, \mathrm{M}_{\sun} \, \mathrm{pc}^{-2}} \approx 10^{20} \, \mathrm{atoms} \, \mathrm{cm}^{-2}$).  Velocity contours correspond to tick locations on the colour bar. All systems are mock observed at an inclination of $i=60\degr$, position angle of $270\degr$, and assuming a distance of $12.9 \, \mathrm{Mpc}$.
\item Panel \textbf{(g)} shows the inner `fiducial' velocity (see Eq.~\ref{eq:fiducial_things} and Fig.~\ref{fig:rot_curves}) as a function of outer `max' velocity (see Appendix~\ref{app:algorithm}). The square markers show the values from the circular velocity curves. The blue and red points show the values from each of the $24$ rotation curves obtained from mock observations. The measurement for projection angle ${\Phi=0\degr}$, shown in panels (a)--(c), is shown as an enlarged point (with error bars included for galaxies selected for kinematic analysis). This is connected to all measurements for values of $\Phi$ in $15\degr$ increments by solid lines. The solid black line shows the relation for an average NFW halo model assuming the mass-concentration relation of \citet{Ludlow+16}, and the shaded band illustrates the $10^\mathrm{th}$--$90^\mathrm{th}$ percentile scatter around this relation. The dashed black line shows ${V_{\mathrm{fid}} = V_{\mathrm{max}}}$.
\item Panel \textbf{(h)} shows the rotation curve shape parameter, $\eta_{\mathrm{rot}}$, as a function of central baryon-to-total mass fraction $\eta_{\mathrm{bar}}$ (see Sec.~\ref{subsubsec:baryon_dom}). The solid black line shows the average $\eta_{\mathrm{rot}}$ expected of NFW cusps and the grey band shows the approximate $10^\mathrm{th}$--$90^\mathrm{th}$~percentile scatter around this value. Symbol shapes and colours, and connecting lines, are as in panel \textbf{(g)}.
\item Panels \textbf{(i)} and \textbf{(j)} show $\eta_{\mathrm{bar}}$ and $\eta_{\mathrm{rot}}$, respectively, as functions of viewing angle $\Phi$. Symbols and the solid lines have the same meaning as in the panels (g) and (h). Dashed lines show best-fitting sinusoidal functions with a $180\degr$ period.
\item Panel \textbf{(k)} shows orbital velocities as a function of radius for the gas discs of simulated galaxies. The circular velocity, ${V_{\mathrm{circ}}(R) = \sgn(a_{r}(R))\sqrt{R|a_{r}(R)|}}$, where $a_{r}$ is the radial component of the gravitational acceleration field in the disc midplane, is shown in solid black. The baryonic contribution to the circular velocity, $V_{\mathrm{bar}}$, calculated in the same way, is shown in dotted black. The median azimuthal velocity of \ion{H}{i}-bearing particles, $V_\mathrm{az}$, reflecting the actual motion of the gas, is shown in green. The $24$ blue and magenta curves show the rotation velocity, $V_{\mathrm{\phi}}$, obtained by modelling mock observation of the galaxies seen along $24$ different sight lines at fixed overall inclination ($60\degr$). These have been corrected for pressure support. The mock observations for the projection angle ${\Phi=0\degr}$, corresponding to the images shown in panels (a)--(c), are shown in solid magenta, with uncertainty shown by the magenta shading, and mock observations at $\Phi=90\degr$, see panels (d)--(f), are shown in dashed magenta. The rotation velocity without pressure support-correction for $\Phi=0\degr$ mock observations is shown in dotted magenta.
\item Panel \textbf{(l)} shows velocity dispersions as a function of radius for the gas discs of simulated galaxies. The median velocity dispersion of \ion{H}{i}-bearing particles, $\sigma = \sqrt{(\sigma_\mathrm{az}^2 + \sigma_\mathrm{rad}^2 + \sigma_\mathrm{z}^2) / 3}$, reflecting the bulk motion of the gas (without contribution from thermal pressure), is shown in green. The $24$ blue and magenta curves show the velocity dispersion, $\sigma$, obtained by modelling mock observation of the galaxies seen along $24$ different sight lines at fixed overall inclination ($60\degr$). Similar to panel (k), solid magenta lines and dashed magenta lines correspond to mock observations for $\Phi=0\degr$~and~$90\degr$, respectively.
\item Panel \textbf{(m)} shows inclination angle as a function of radius for the gas discs of simulated galaxies. The $24$ blue and magenta curves show the inclination, $i$, obtained by modelling mock observation of the galaxies seen along $24$ different sight lines at fixed overall inclination ($60\degr$). Similar to panels (k) and (l), solid magenta lines and dashed magenta lines correspond to mock observations for ${\Phi=0\degr}$~and~$90\degr$, respectively. The green line shows the nominal value of ${i=60\degr}$.
\item Panel \textbf{(n)} shows face-on \ion{H}{i} surface density, $\Sigma_\mathrm{HI}$, as a function of radius for the gas discs. Each particle contributes flux proportionally to its \ion{H}{i} mass, with the gas assumed to be optically thin. $\Sigma_\mathrm{HI}$ calculated directly from simulation is shown in green. The $24$ blue and magenta curves show the inclination-corrected $\Sigma_\mathrm{HI}$, derived from mock observations. As in panel (k), solid magenta and dashed magenta lines correspond to mock observations for $\Phi=0\degr$~and~$90\degr$, respectively.

\end{itemize}

\clearpage

\begin{landscape}

\begin{figure}
\begin{minipage}{.9\textwidth}
\includegraphics[width=\textwidth]{../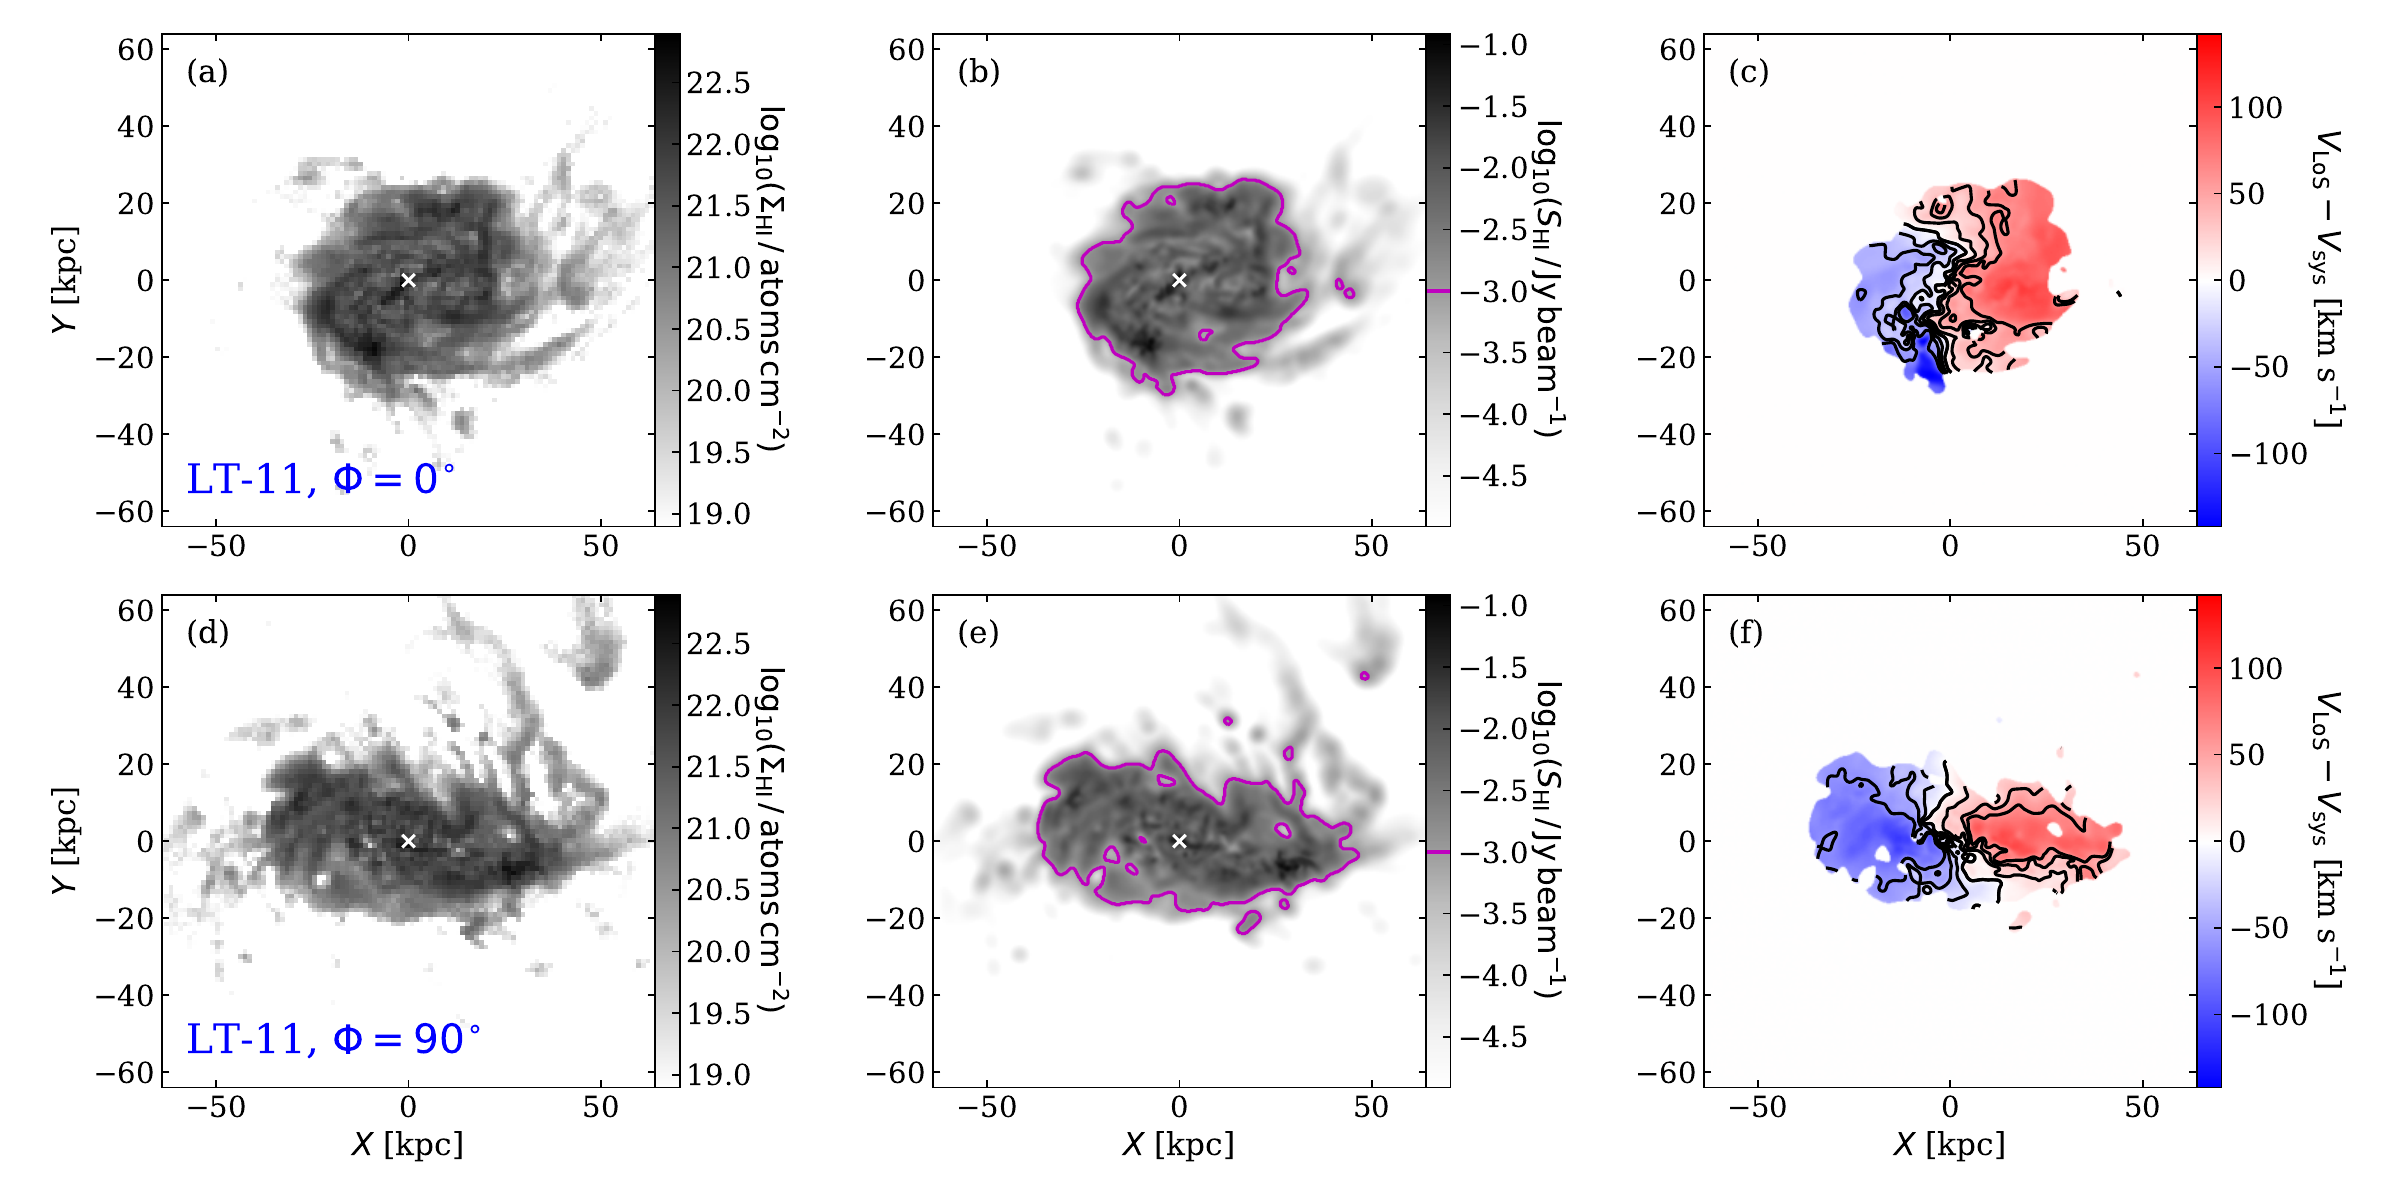}
\includegraphics[width=\textwidth]{../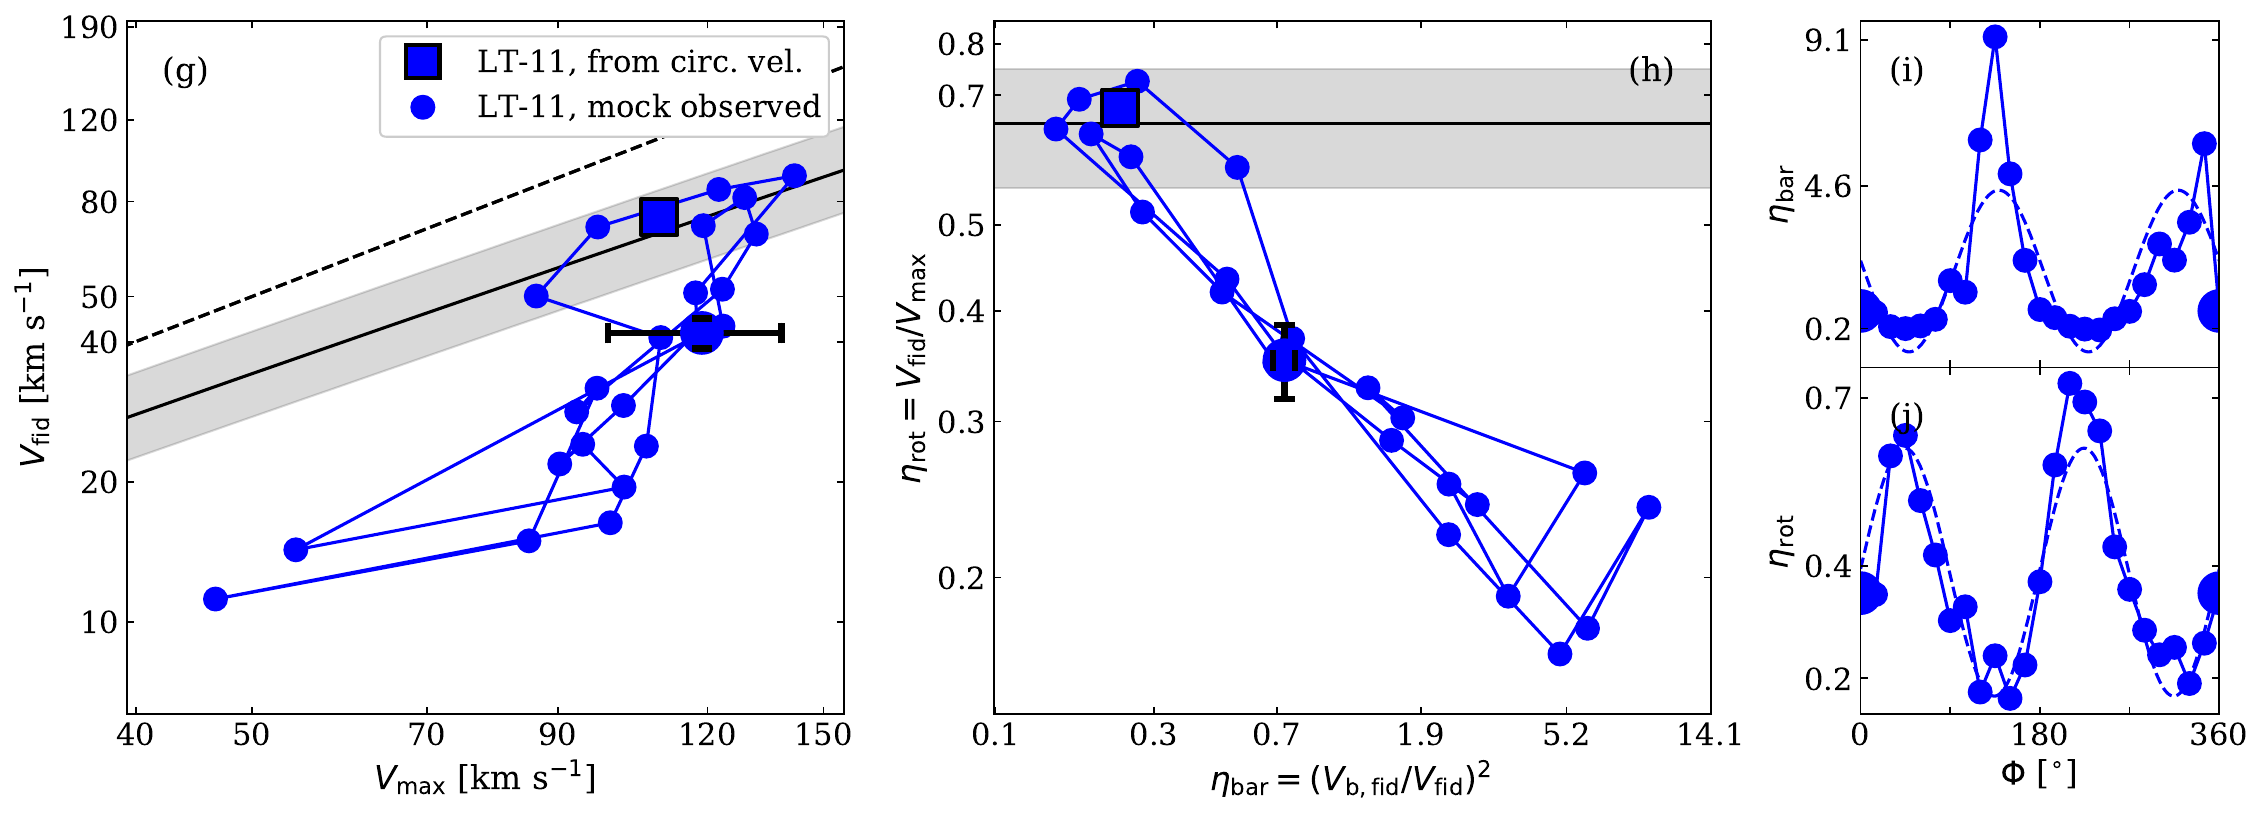}
\end{minipage}
\begin{minipage}{.4\textwidth}
\includegraphics[width=\textwidth]{../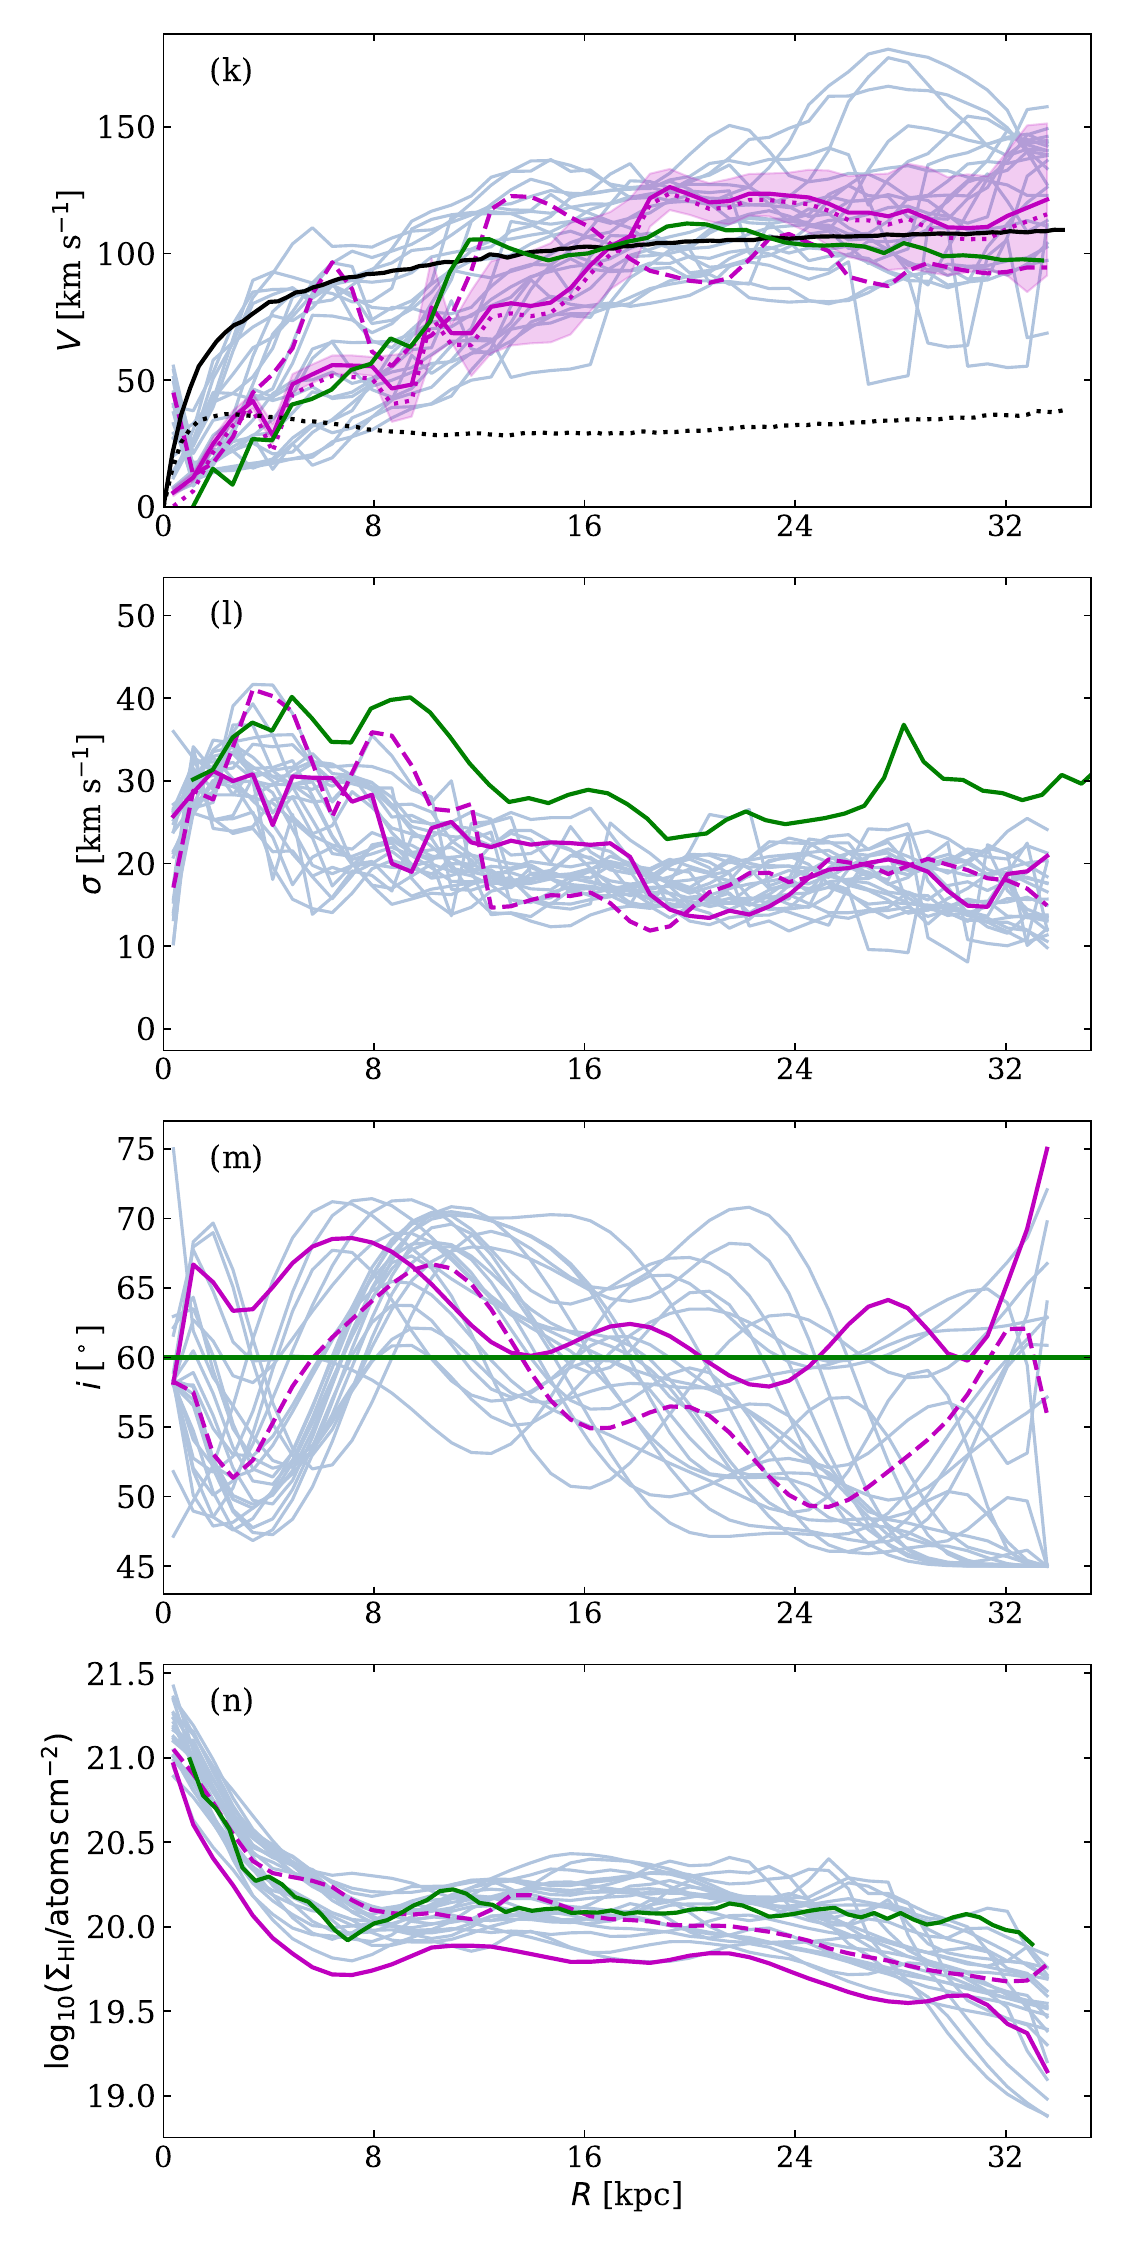}
\end{minipage}
\caption{A set of summary figures for galaxy LT-11, selected for kinematic analysis. These include example moment maps for two orientations (panels (a)--(f); similar to Fig.~\ref{fig:visualisations}), a summary of the parameters $V_\mathrm{fid}$, $V_\mathrm{max}$, $\eta_\mathrm{rot}$, and $\eta_\mathrm{bar}$ (panels (g)--(j); similar to Fig.~\ref{fig:loops}), and a summary of the rotation curve analysis from $24$ viewing angles (panels (k)--(n); similar to Fig.~\ref{fig:rot_curves}). See description of Appendix~\ref{app:supplementary} for details.}
\label{fig:S1}
\end{figure}
\clearpage

\begin{figure}
\begin{minipage}{.9\textwidth}
\includegraphics[width=\textwidth]{../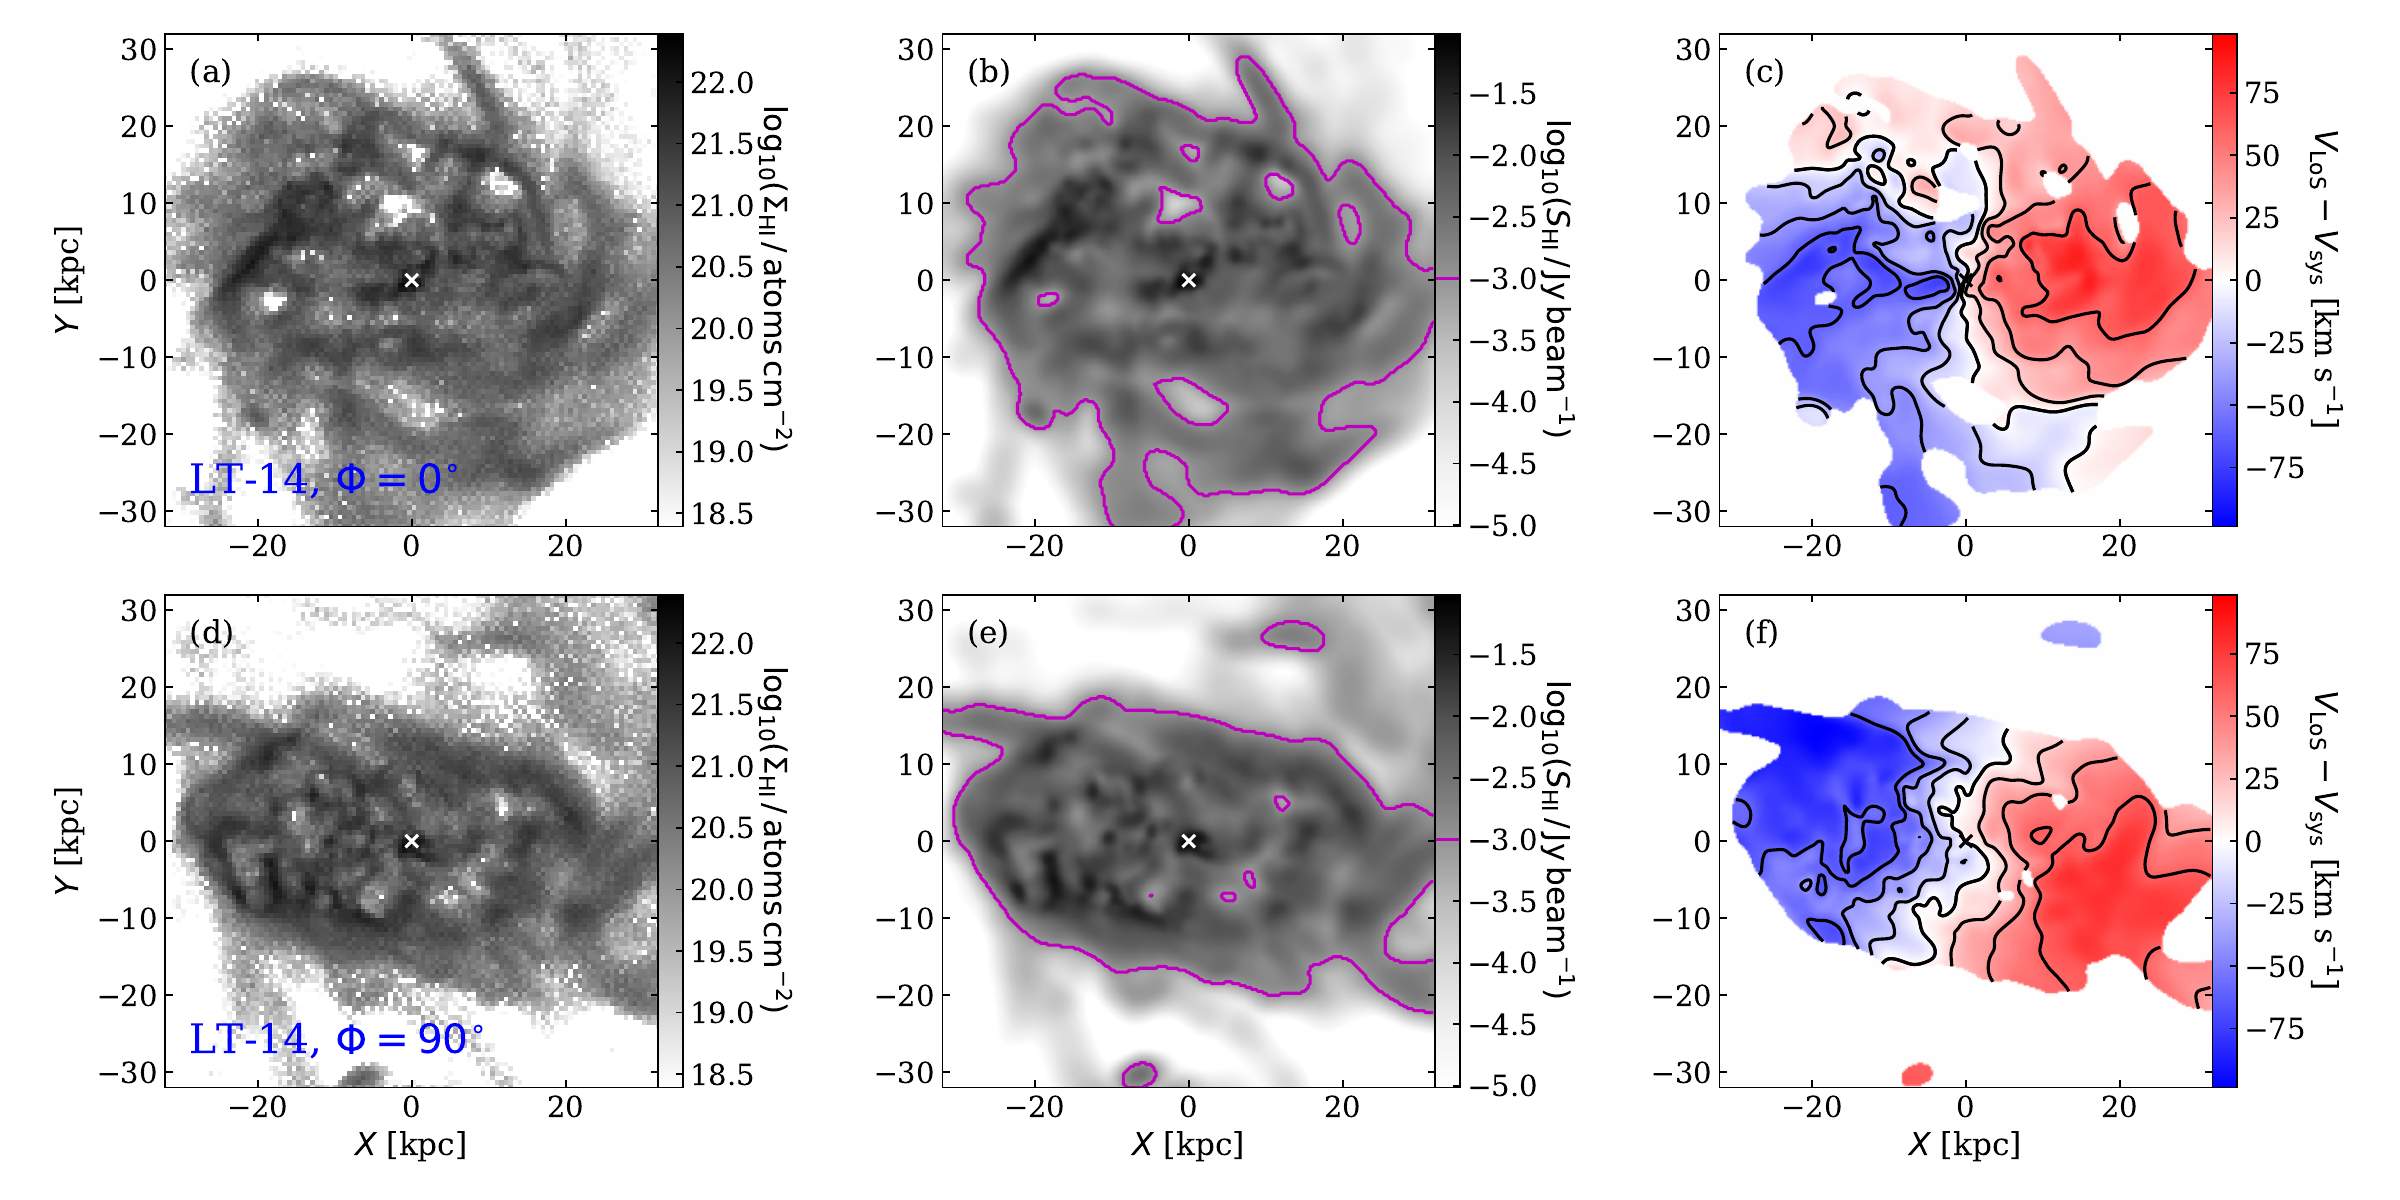}
\includegraphics[width=\textwidth]{../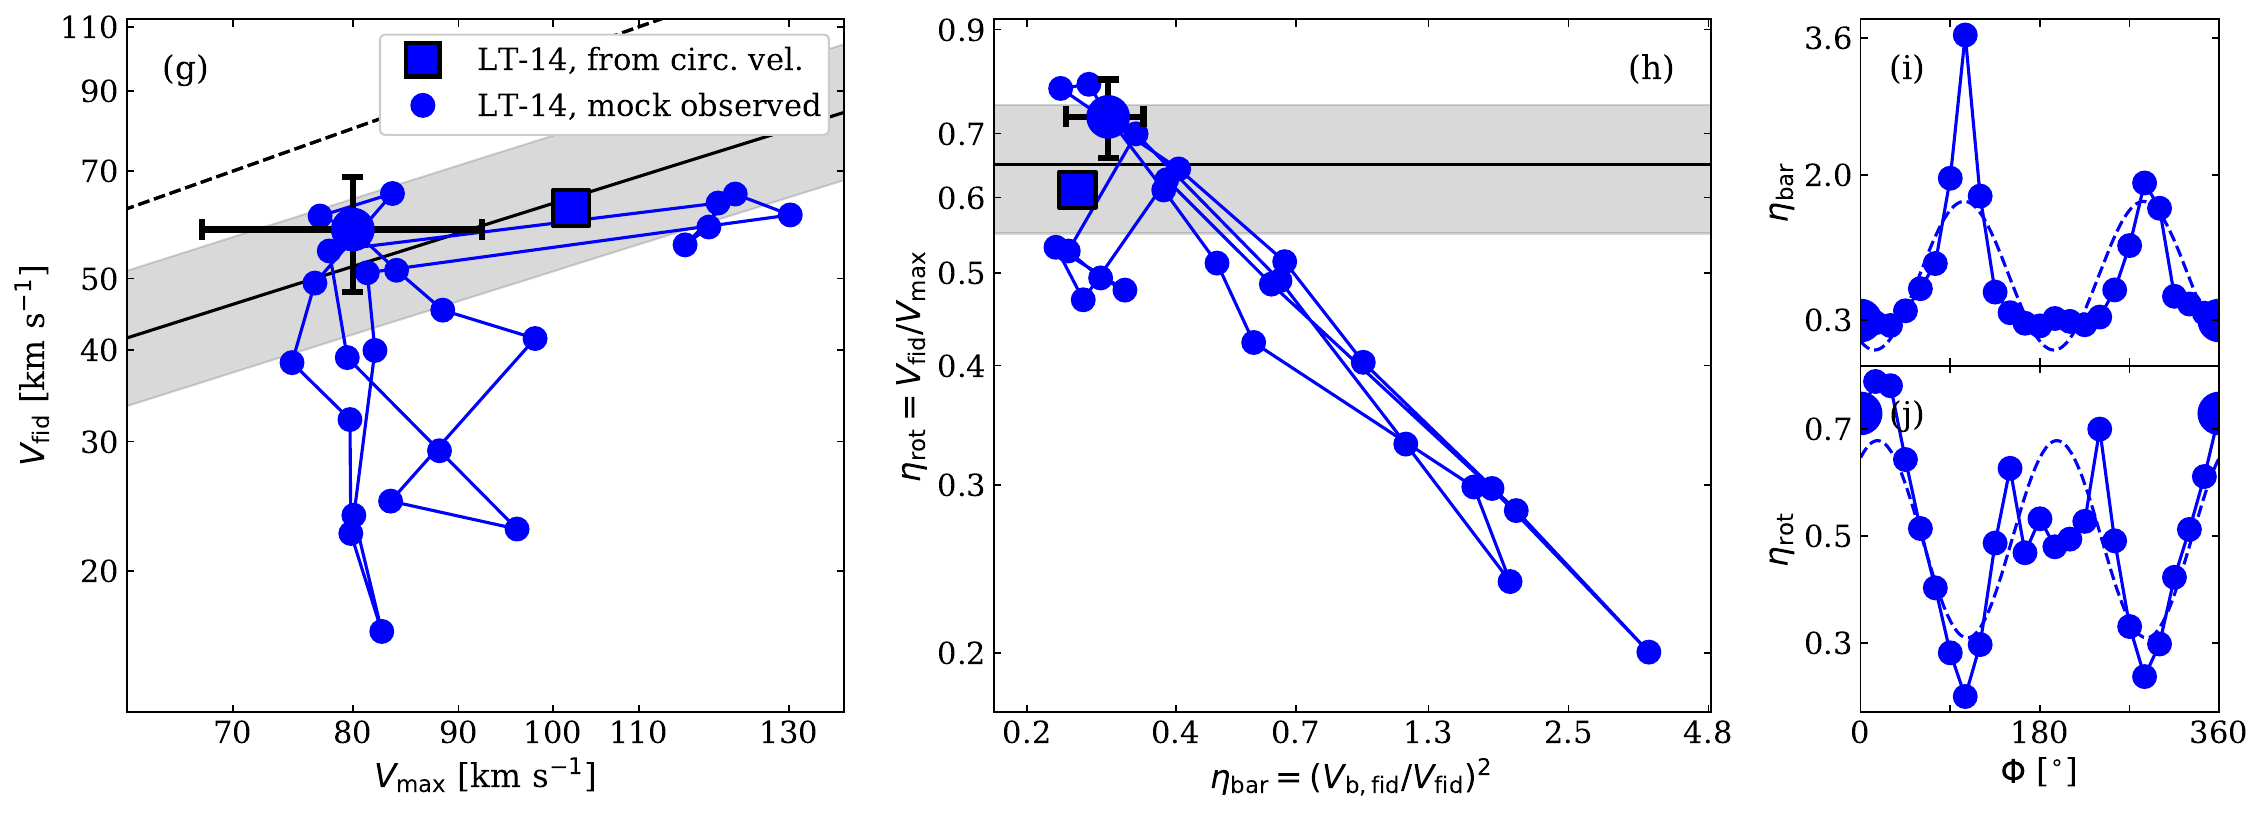}
\end{minipage}
\begin{minipage}{.4\textwidth}
\includegraphics[width=\textwidth]{../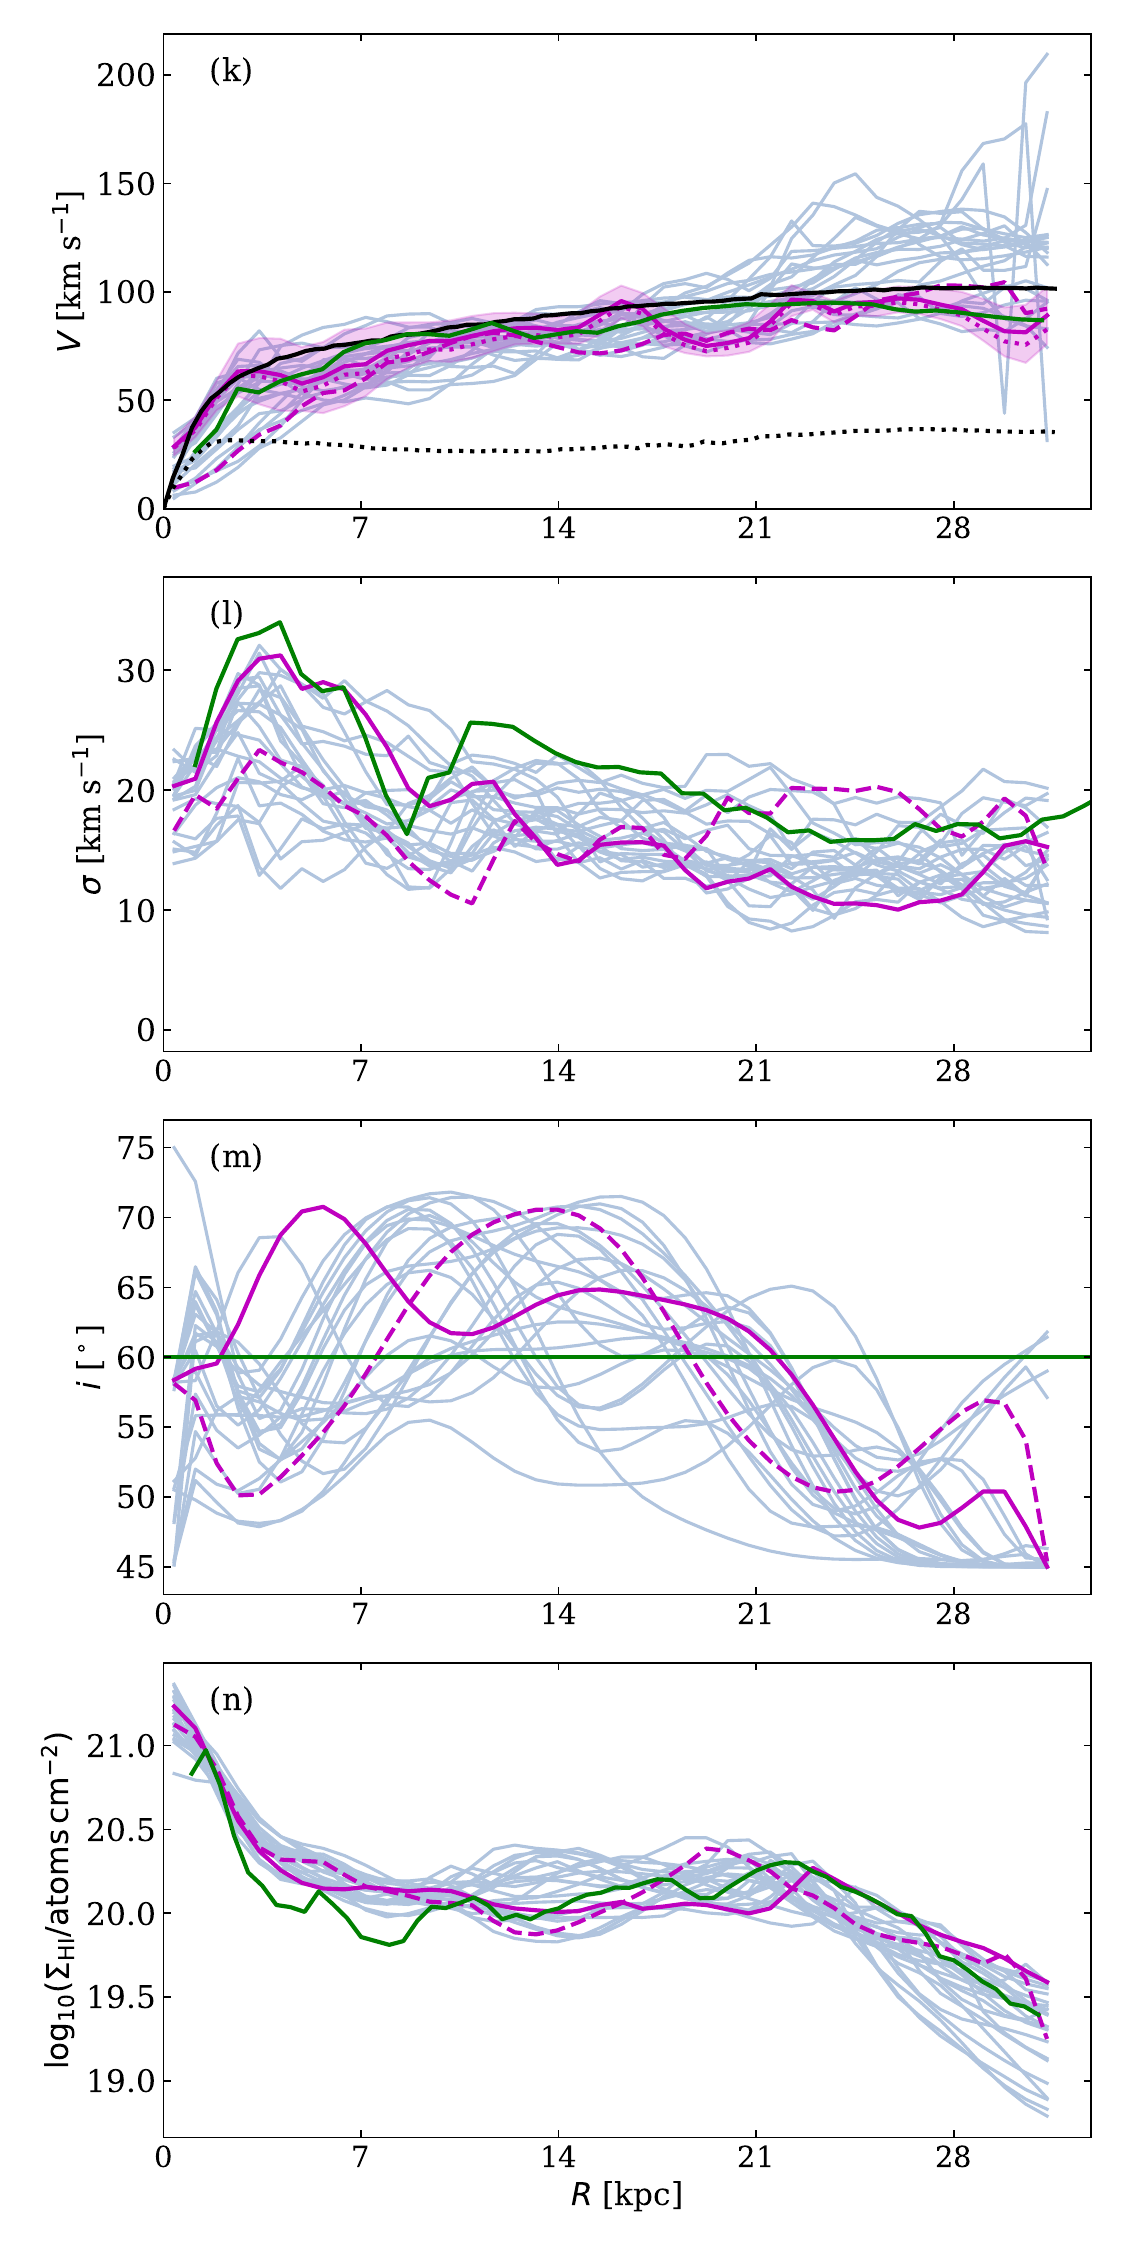}
\end{minipage}
\caption{A set of summary figures for galaxy LT-14, selected for kinematic analysis. These include example moment maps for two orientations (panels (a)--(f); similar to Fig.~\ref{fig:visualisations}), a summary of the parameters $V_\mathrm{fid}$, $V_\mathrm{max}$, $\eta_\mathrm{rot}$, and $\eta_\mathrm{bar}$ (panels (g)--(j); similar to Fig.~\ref{fig:loops}), and a summary of the rotation curve analysis from $24$ viewing angles (panels (k)--(n); similar to Fig.~\ref{fig:rot_curves}). See description of Appendix~\ref{app:supplementary} for details.}
\label{fig:S2}
\end{figure}
\clearpage

\begin{figure}
\begin{minipage}{.9\textwidth}
\includegraphics[width=\textwidth]{../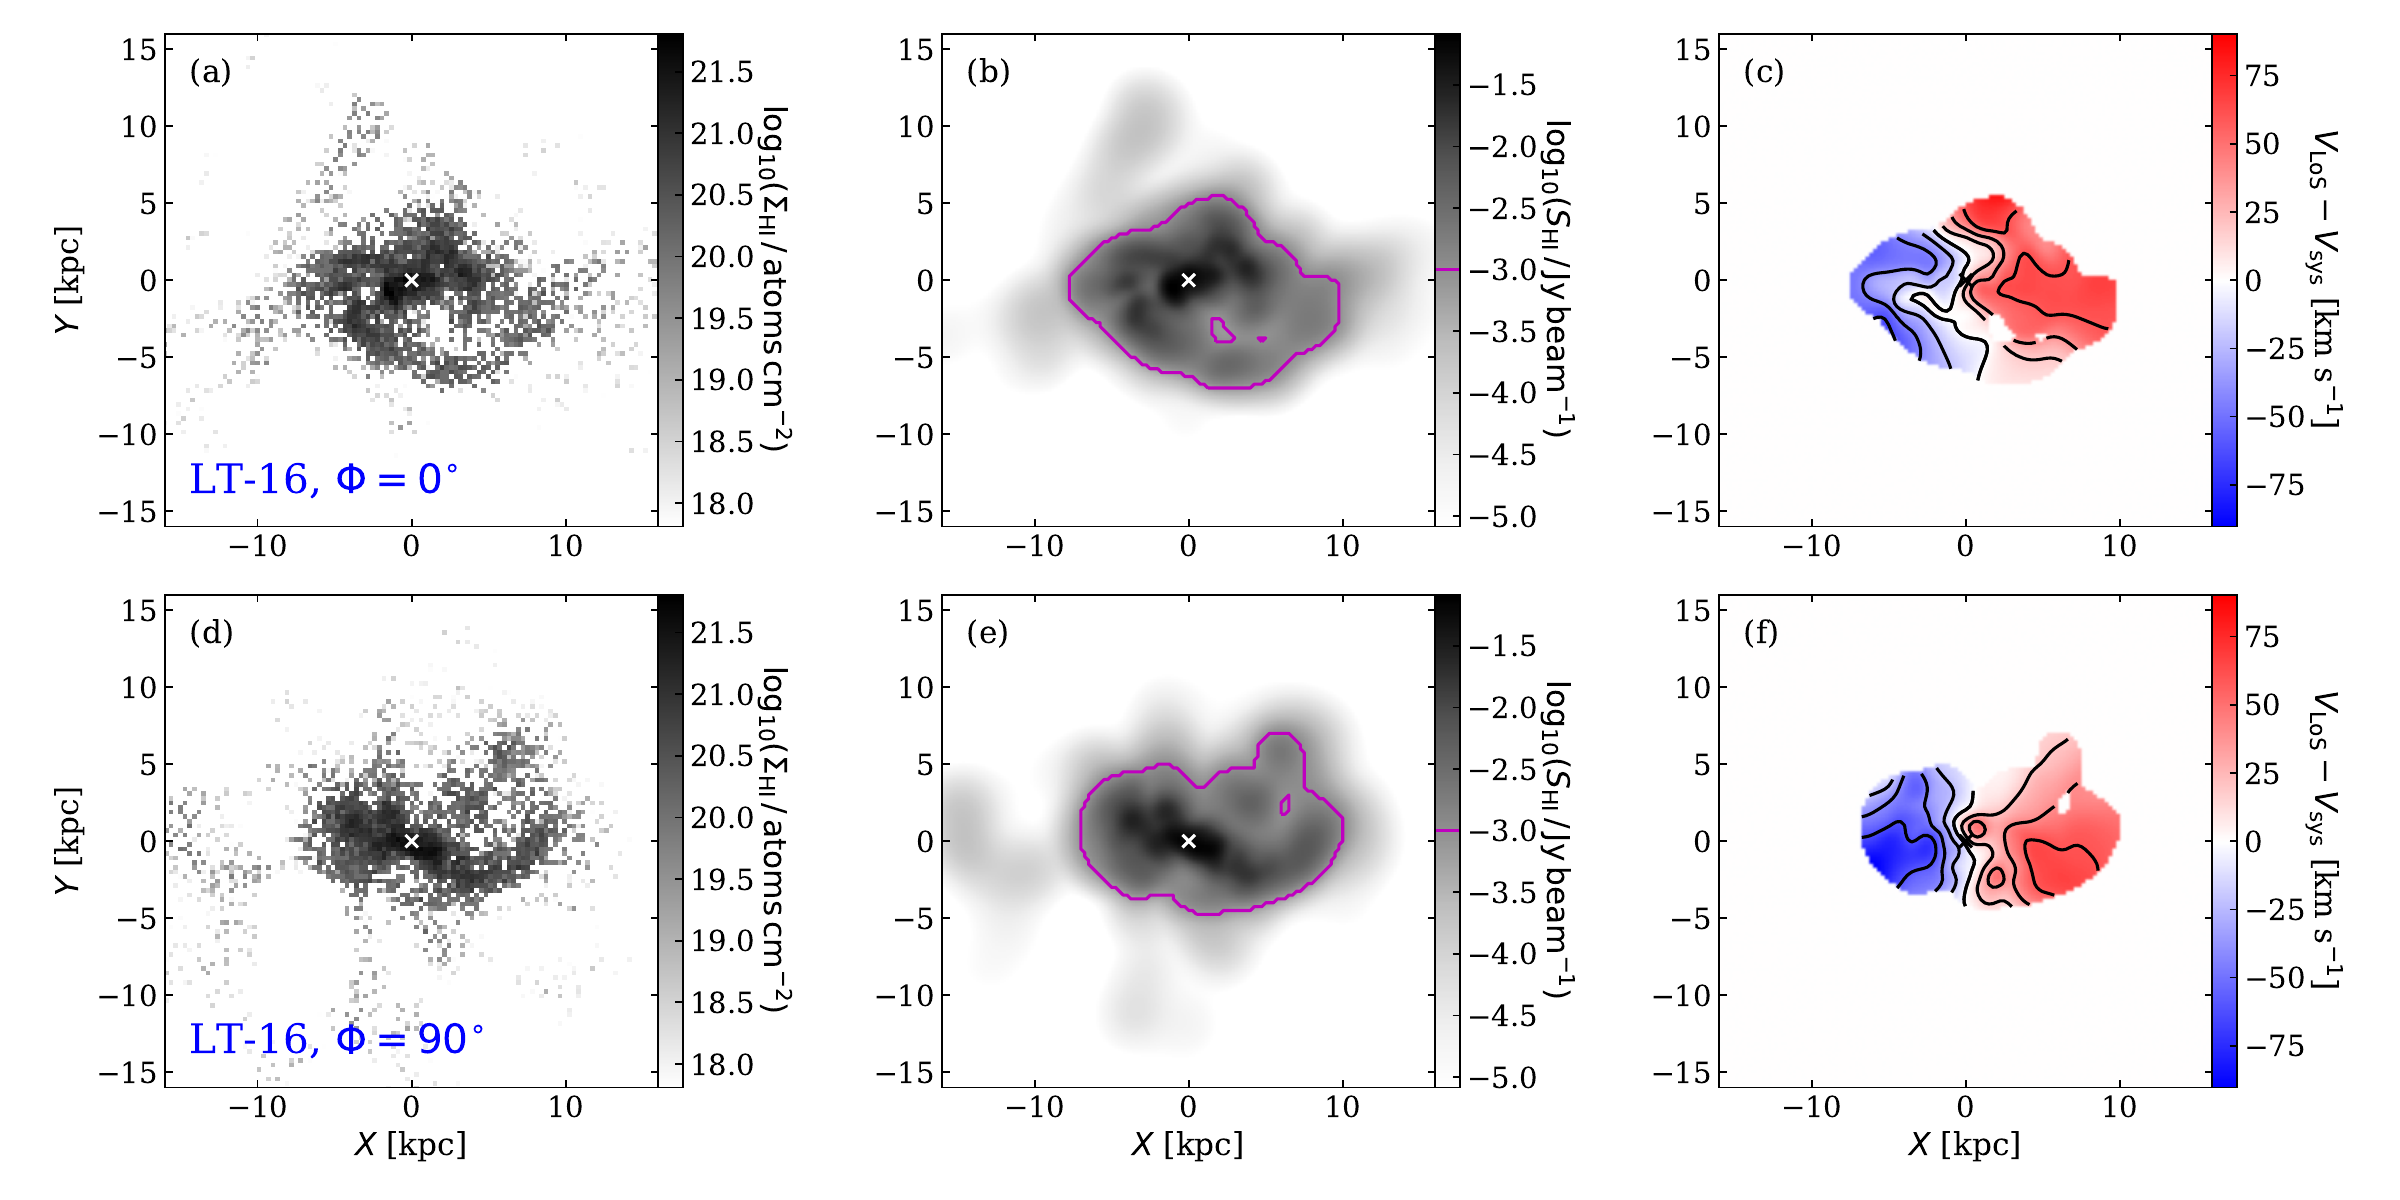}
\includegraphics[width=\textwidth]{../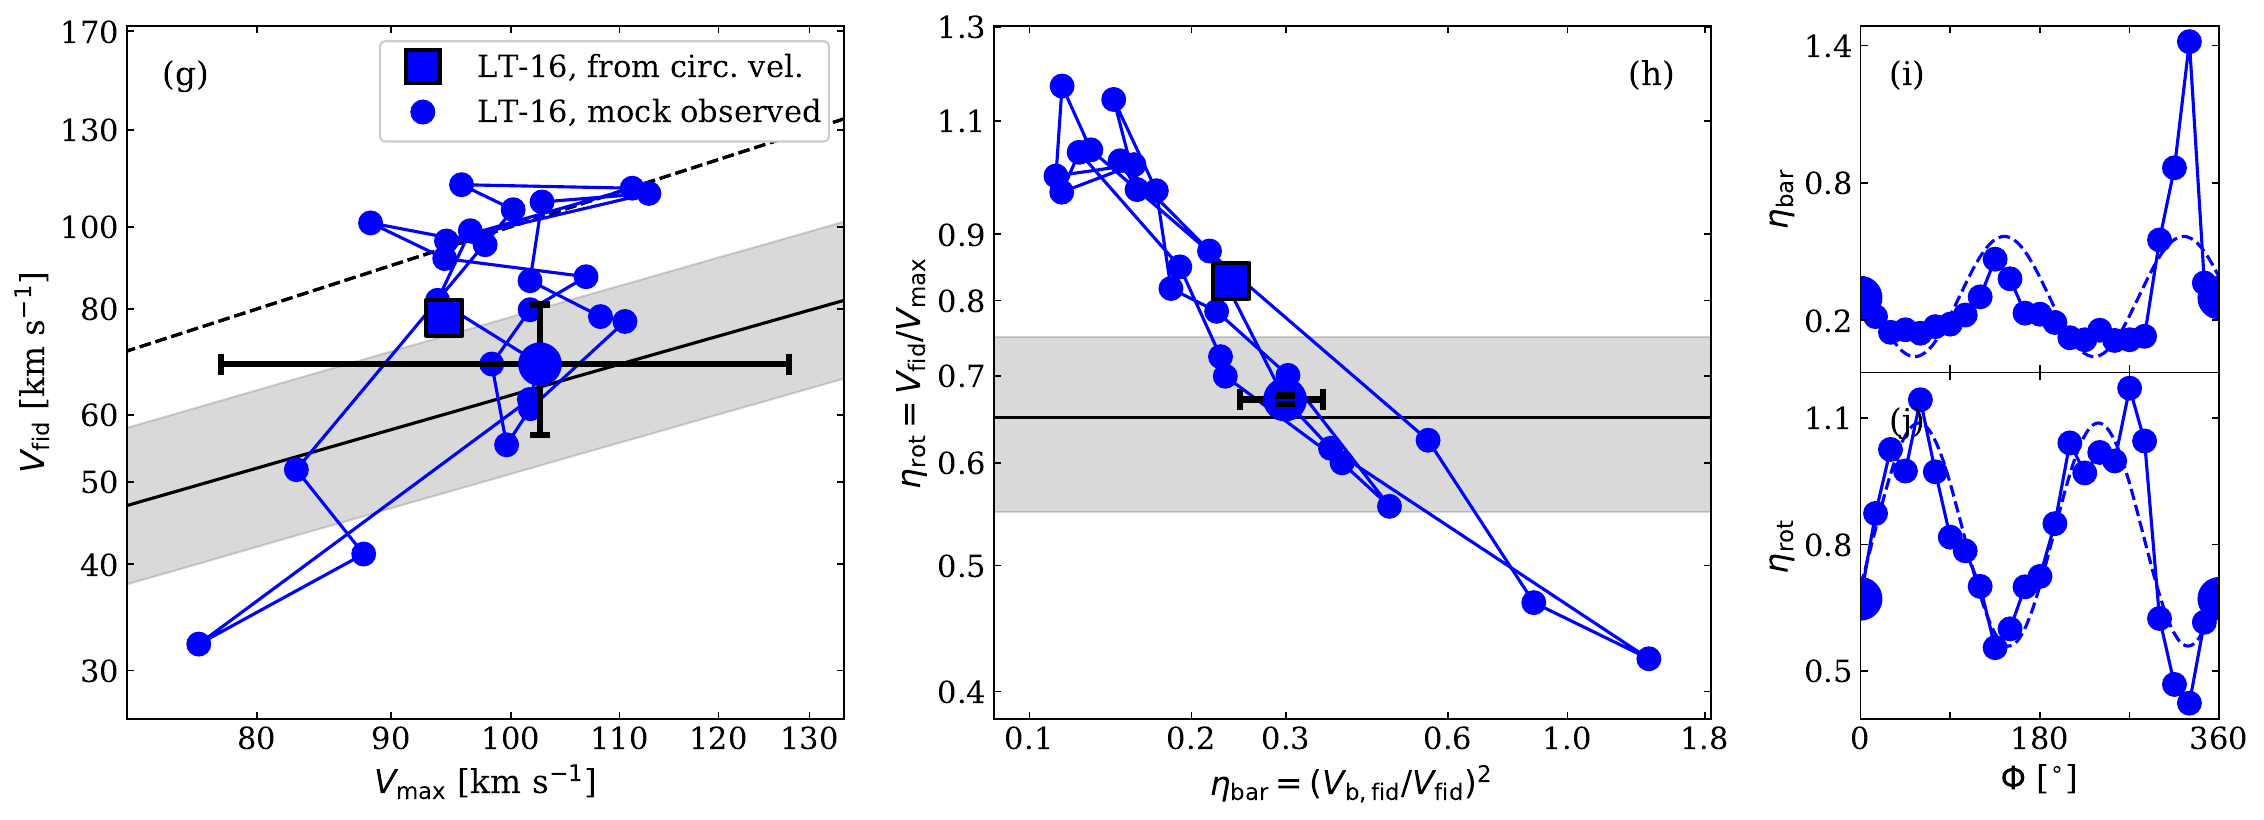}
\end{minipage}
\begin{minipage}{.4\textwidth}
\includegraphics[width=\textwidth]{../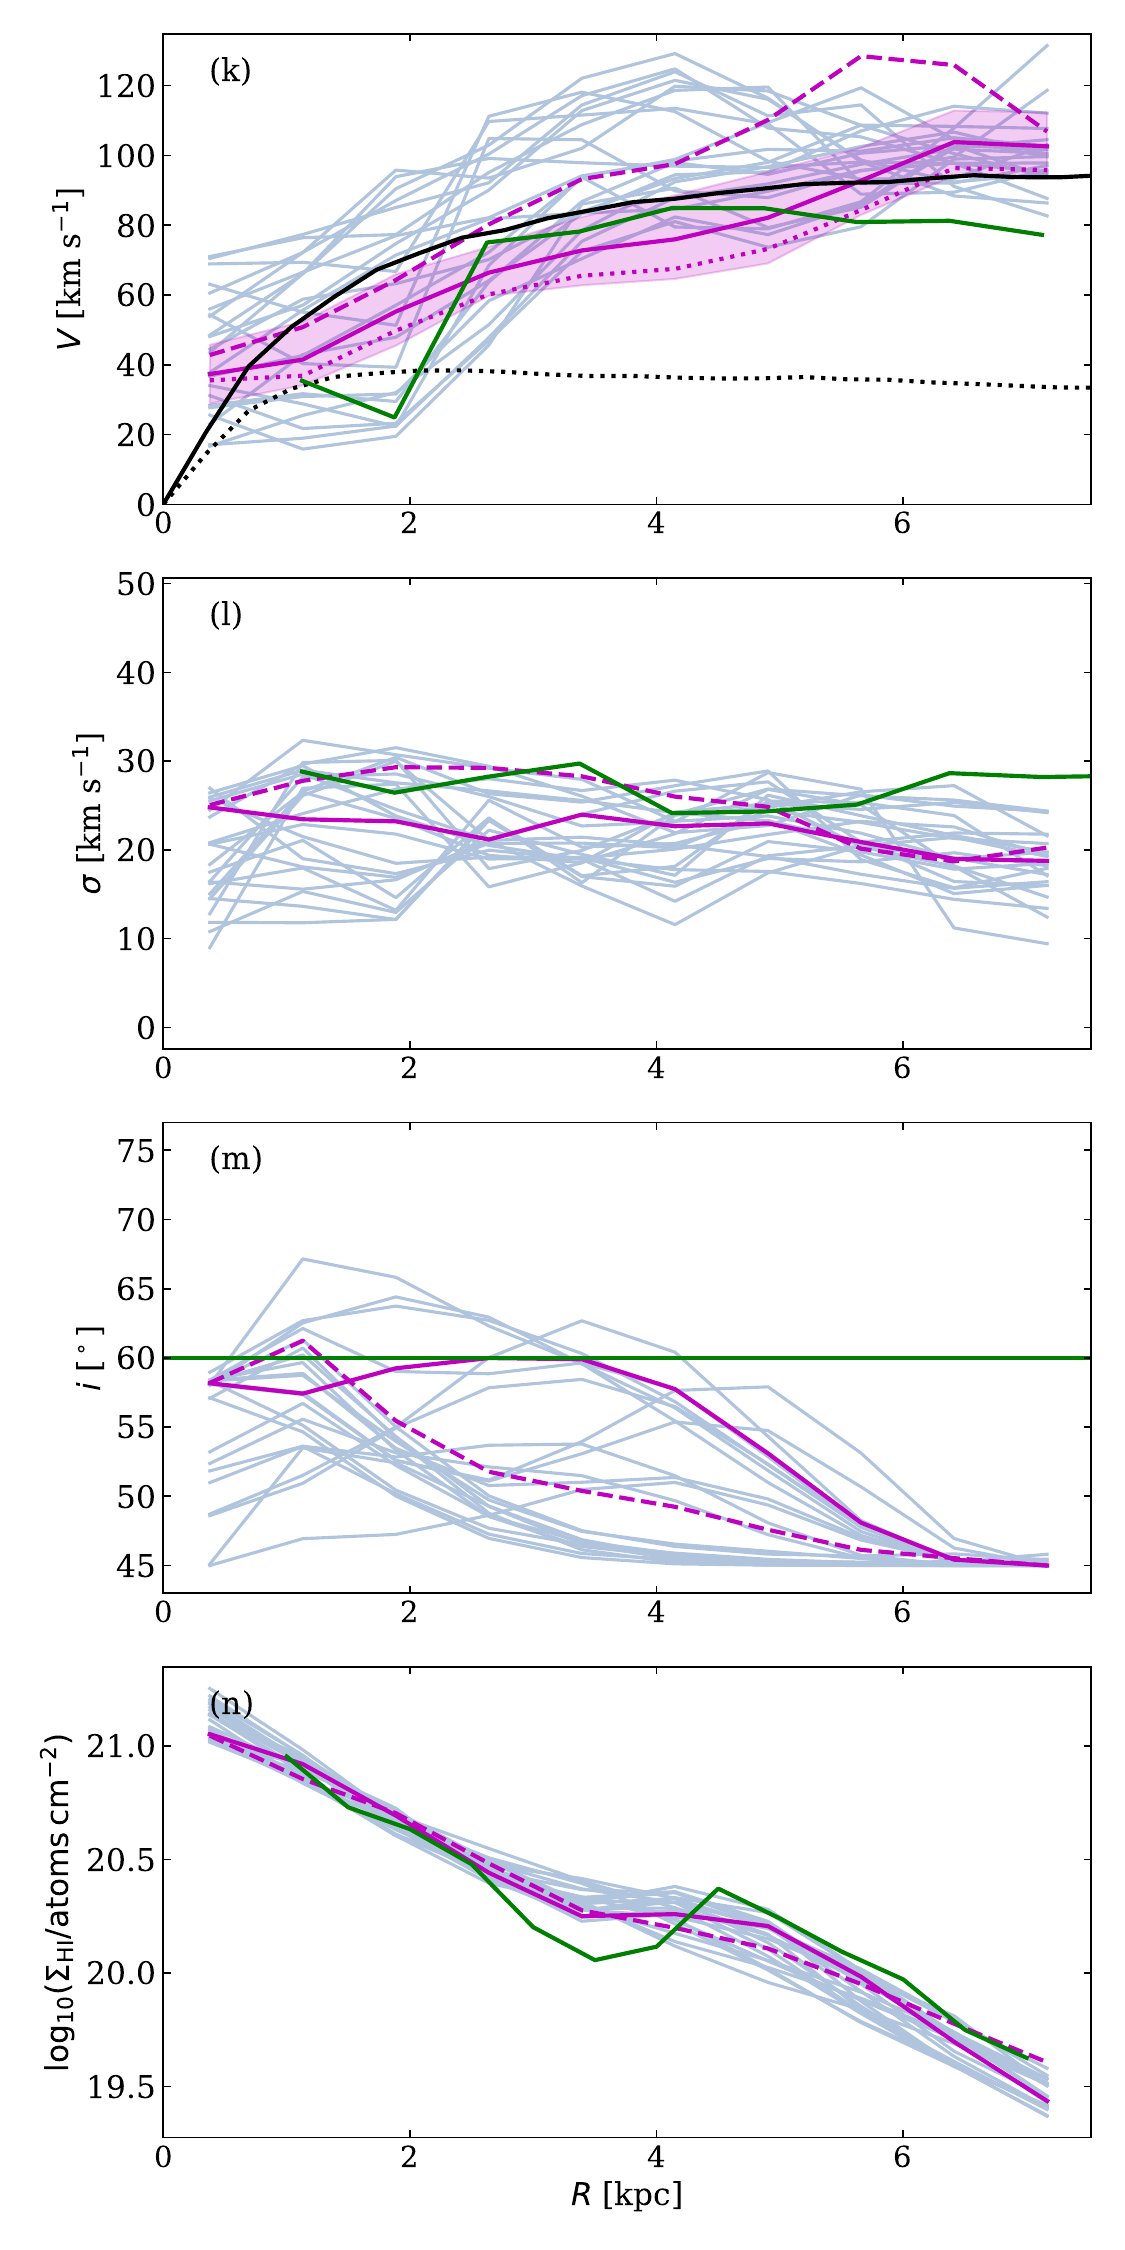}
\end{minipage}
\caption{A set of summary figures for galaxy LT-16, selected for kinematic analysis. These include example moment maps for two orientations (panels (a)--(f); similar to Fig.~\ref{fig:visualisations}), a summary of the parameters $V_\mathrm{fid}$, $V_\mathrm{max}$, $\eta_\mathrm{rot}$, and $\eta_\mathrm{bar}$ (panels (g)--(j); similar to Fig.~\ref{fig:loops}), and a summary of the rotation curve analysis from $24$ viewing angles (panels (k)--(n); similar to Fig.~\ref{fig:rot_curves}). See description of Appendix~\ref{app:supplementary} for details.}
\label{fig:S3}
\end{figure}
\clearpage

\begin{figure}
\begin{minipage}{.9\textwidth}
\includegraphics[width=\textwidth]{../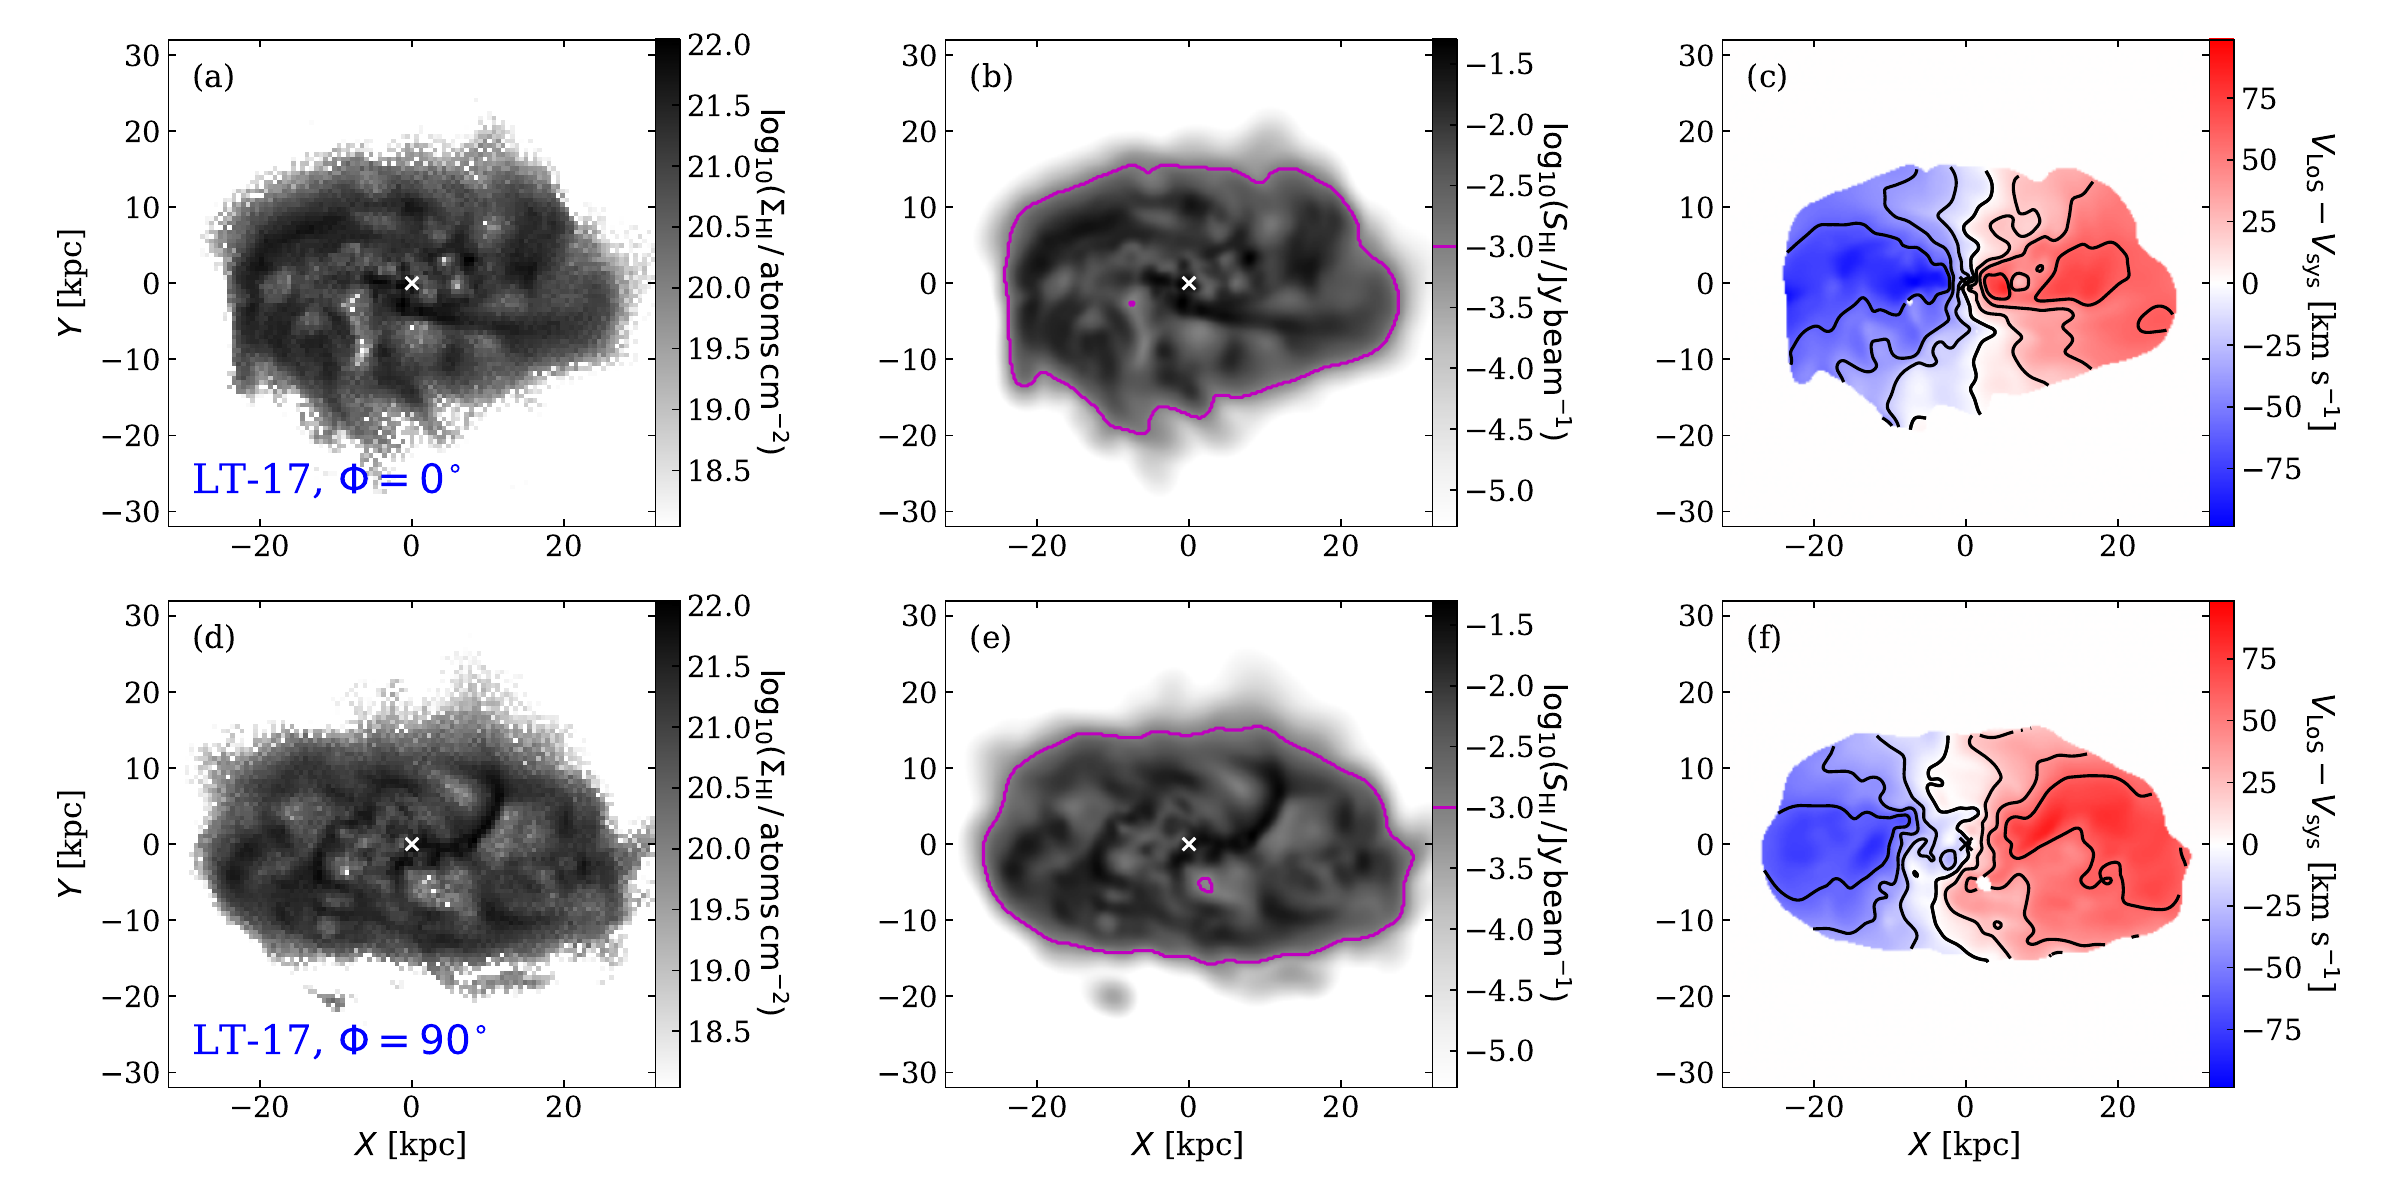}
\includegraphics[width=\textwidth]{../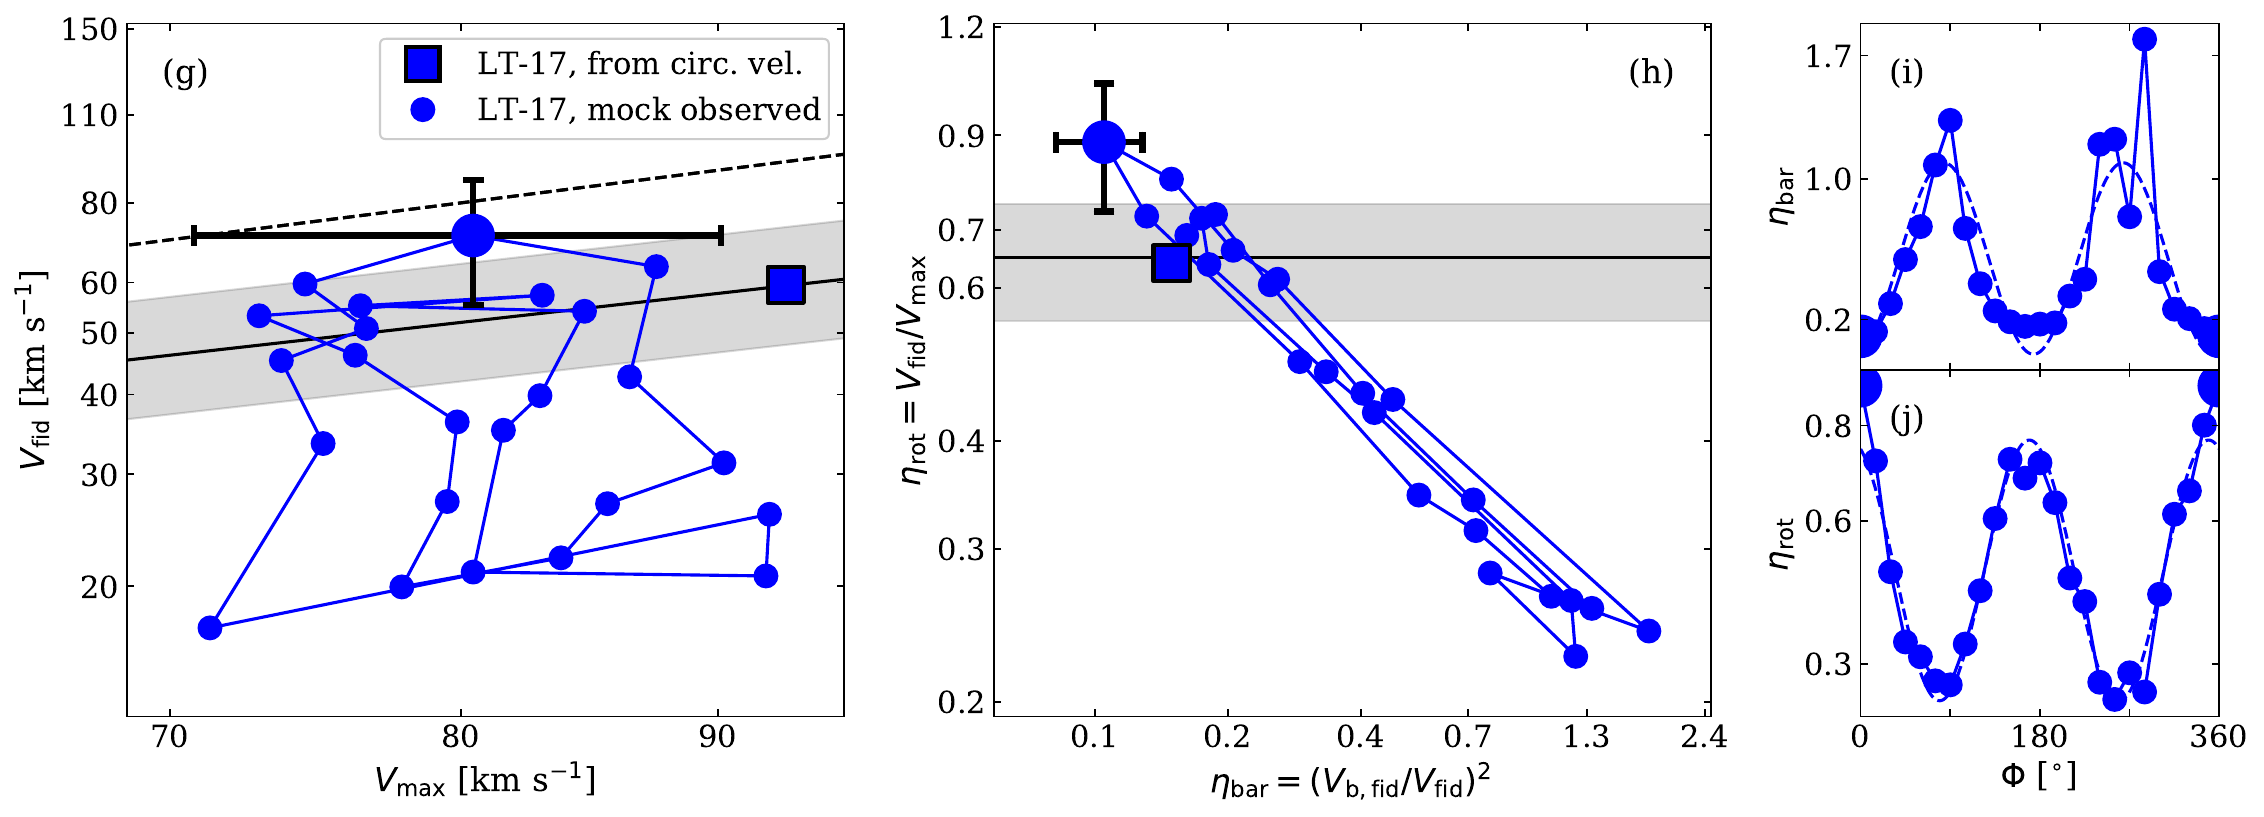}
\end{minipage}
\begin{minipage}{.4\textwidth}
\includegraphics[width=\textwidth]{../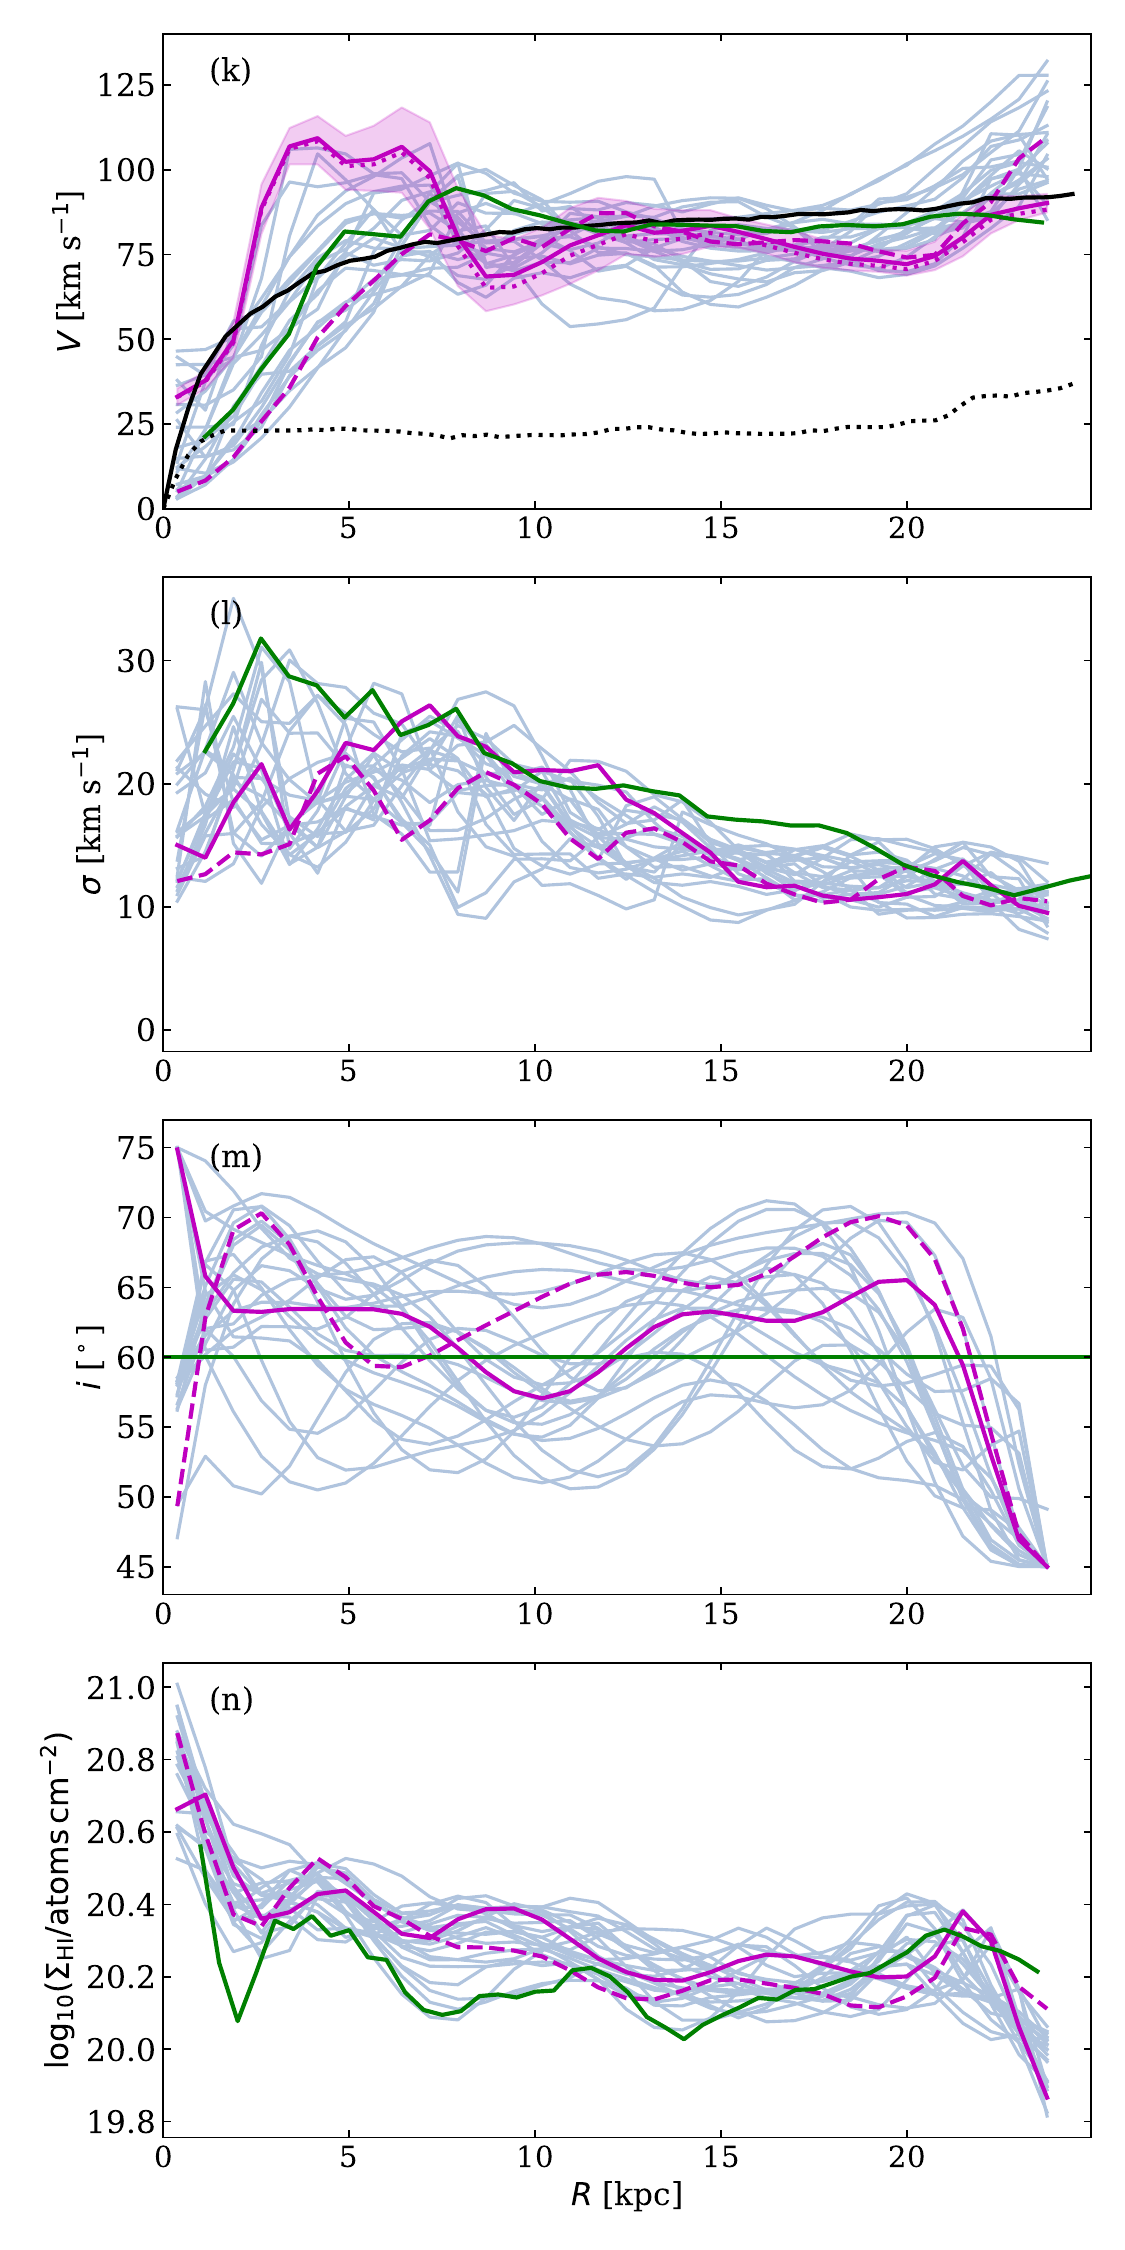}
\end{minipage}
\caption{A set of summary figures for galaxy LT-17, selected for kinematic analysis. These include example moment maps for two orientations (panels (a)--(f); similar to Fig.~\ref{fig:visualisations}), a summary of the parameters $V_\mathrm{fid}$, $V_\mathrm{max}$, $\eta_\mathrm{rot}$, and $\eta_\mathrm{bar}$ (panels (g)--(j); similar to Fig.~\ref{fig:loops}), and a summary of the rotation curve analysis from $24$ viewing angles (panels (k)--(n); similar to Fig.~\ref{fig:rot_curves}). See description of Appendix~\ref{app:supplementary} for details.}
\label{fig:S4}
\end{figure}
\clearpage

\begin{figure}
\begin{minipage}{.9\textwidth}
\includegraphics[width=\textwidth]{../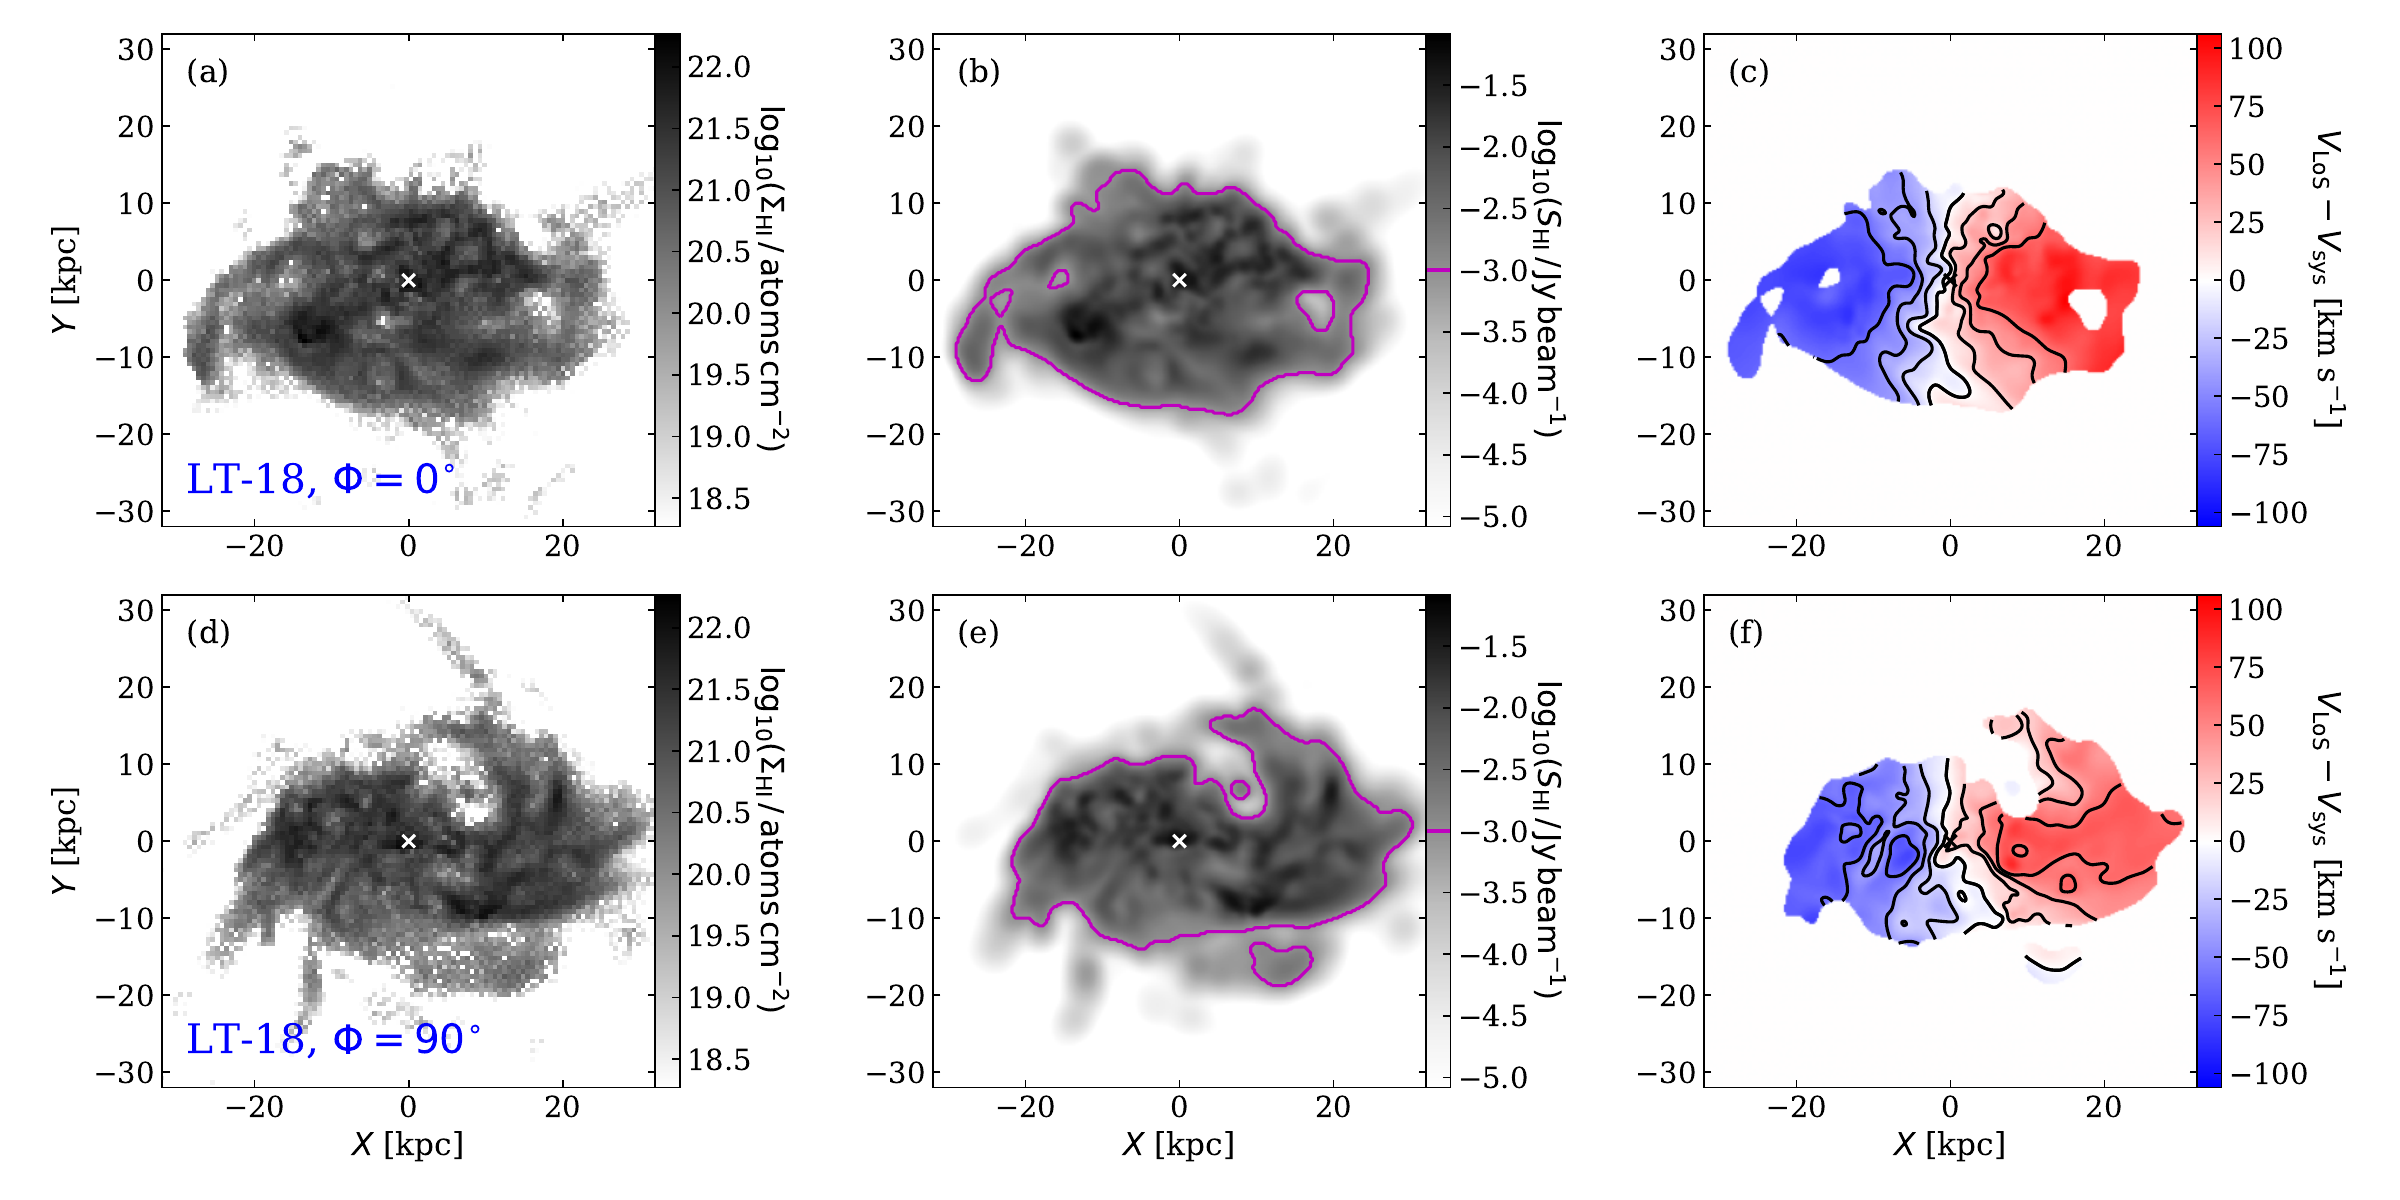}
\includegraphics[width=\textwidth]{../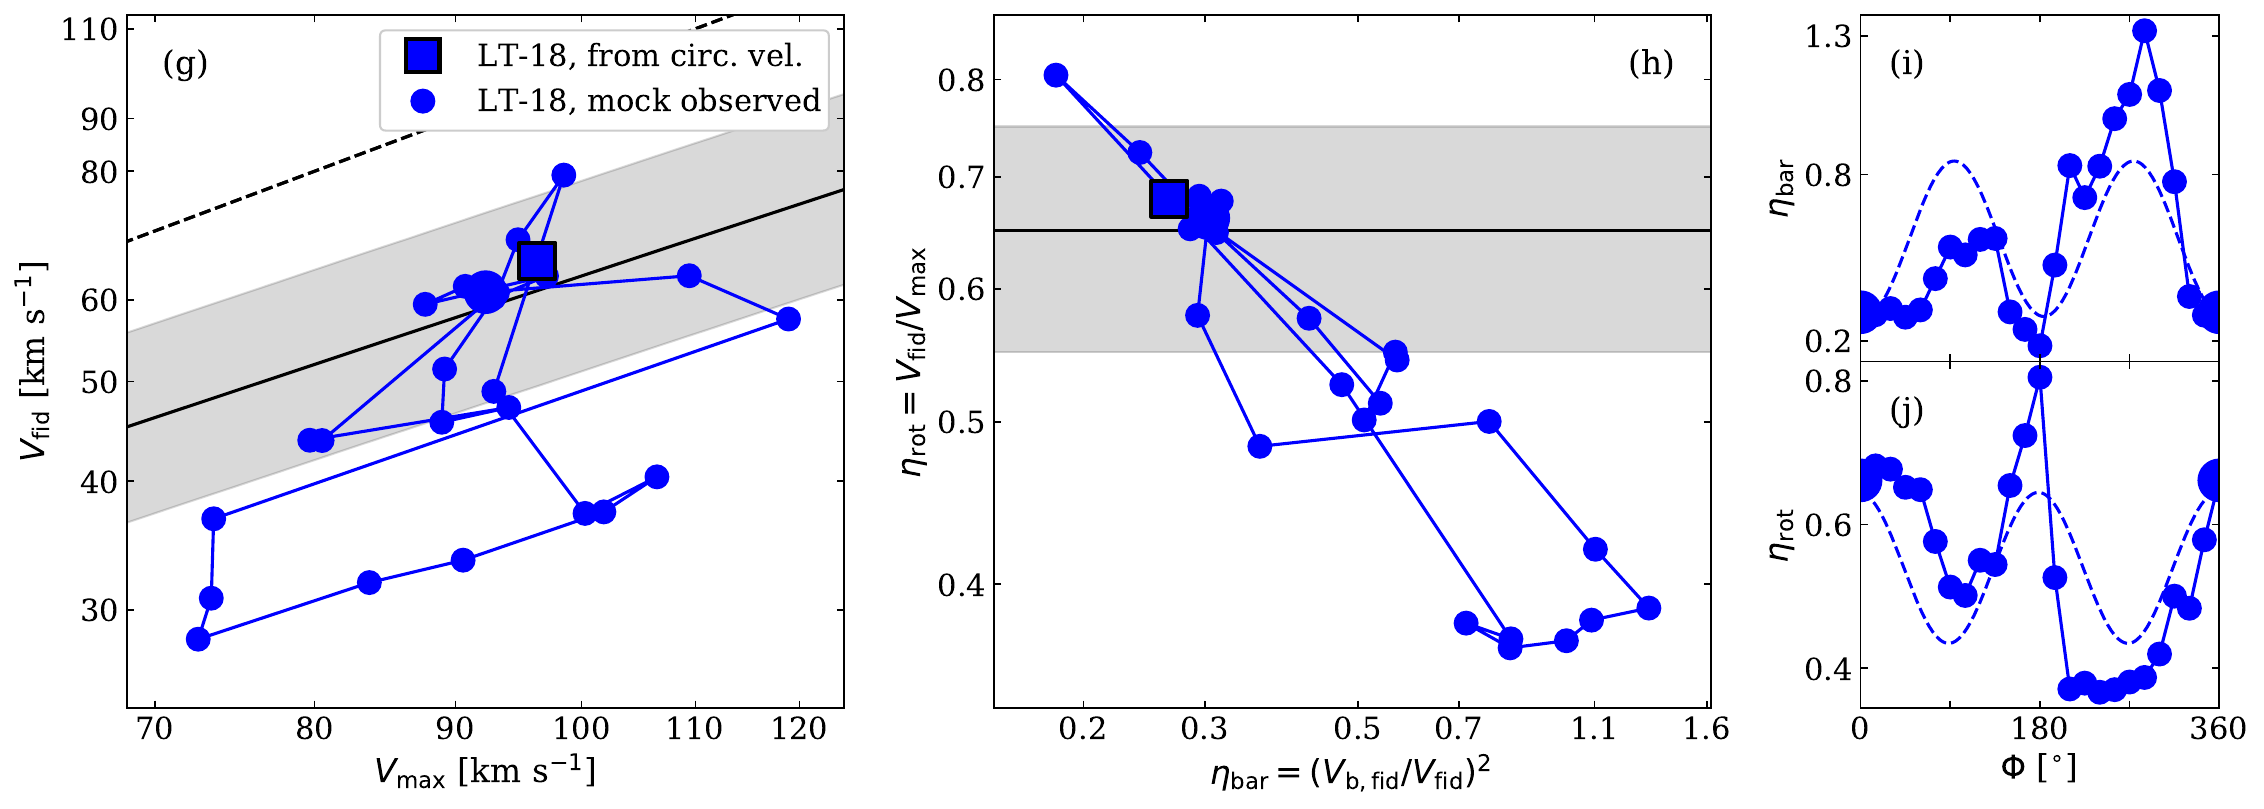}
\end{minipage}
\begin{minipage}{.4\textwidth}
\includegraphics[width=\textwidth]{../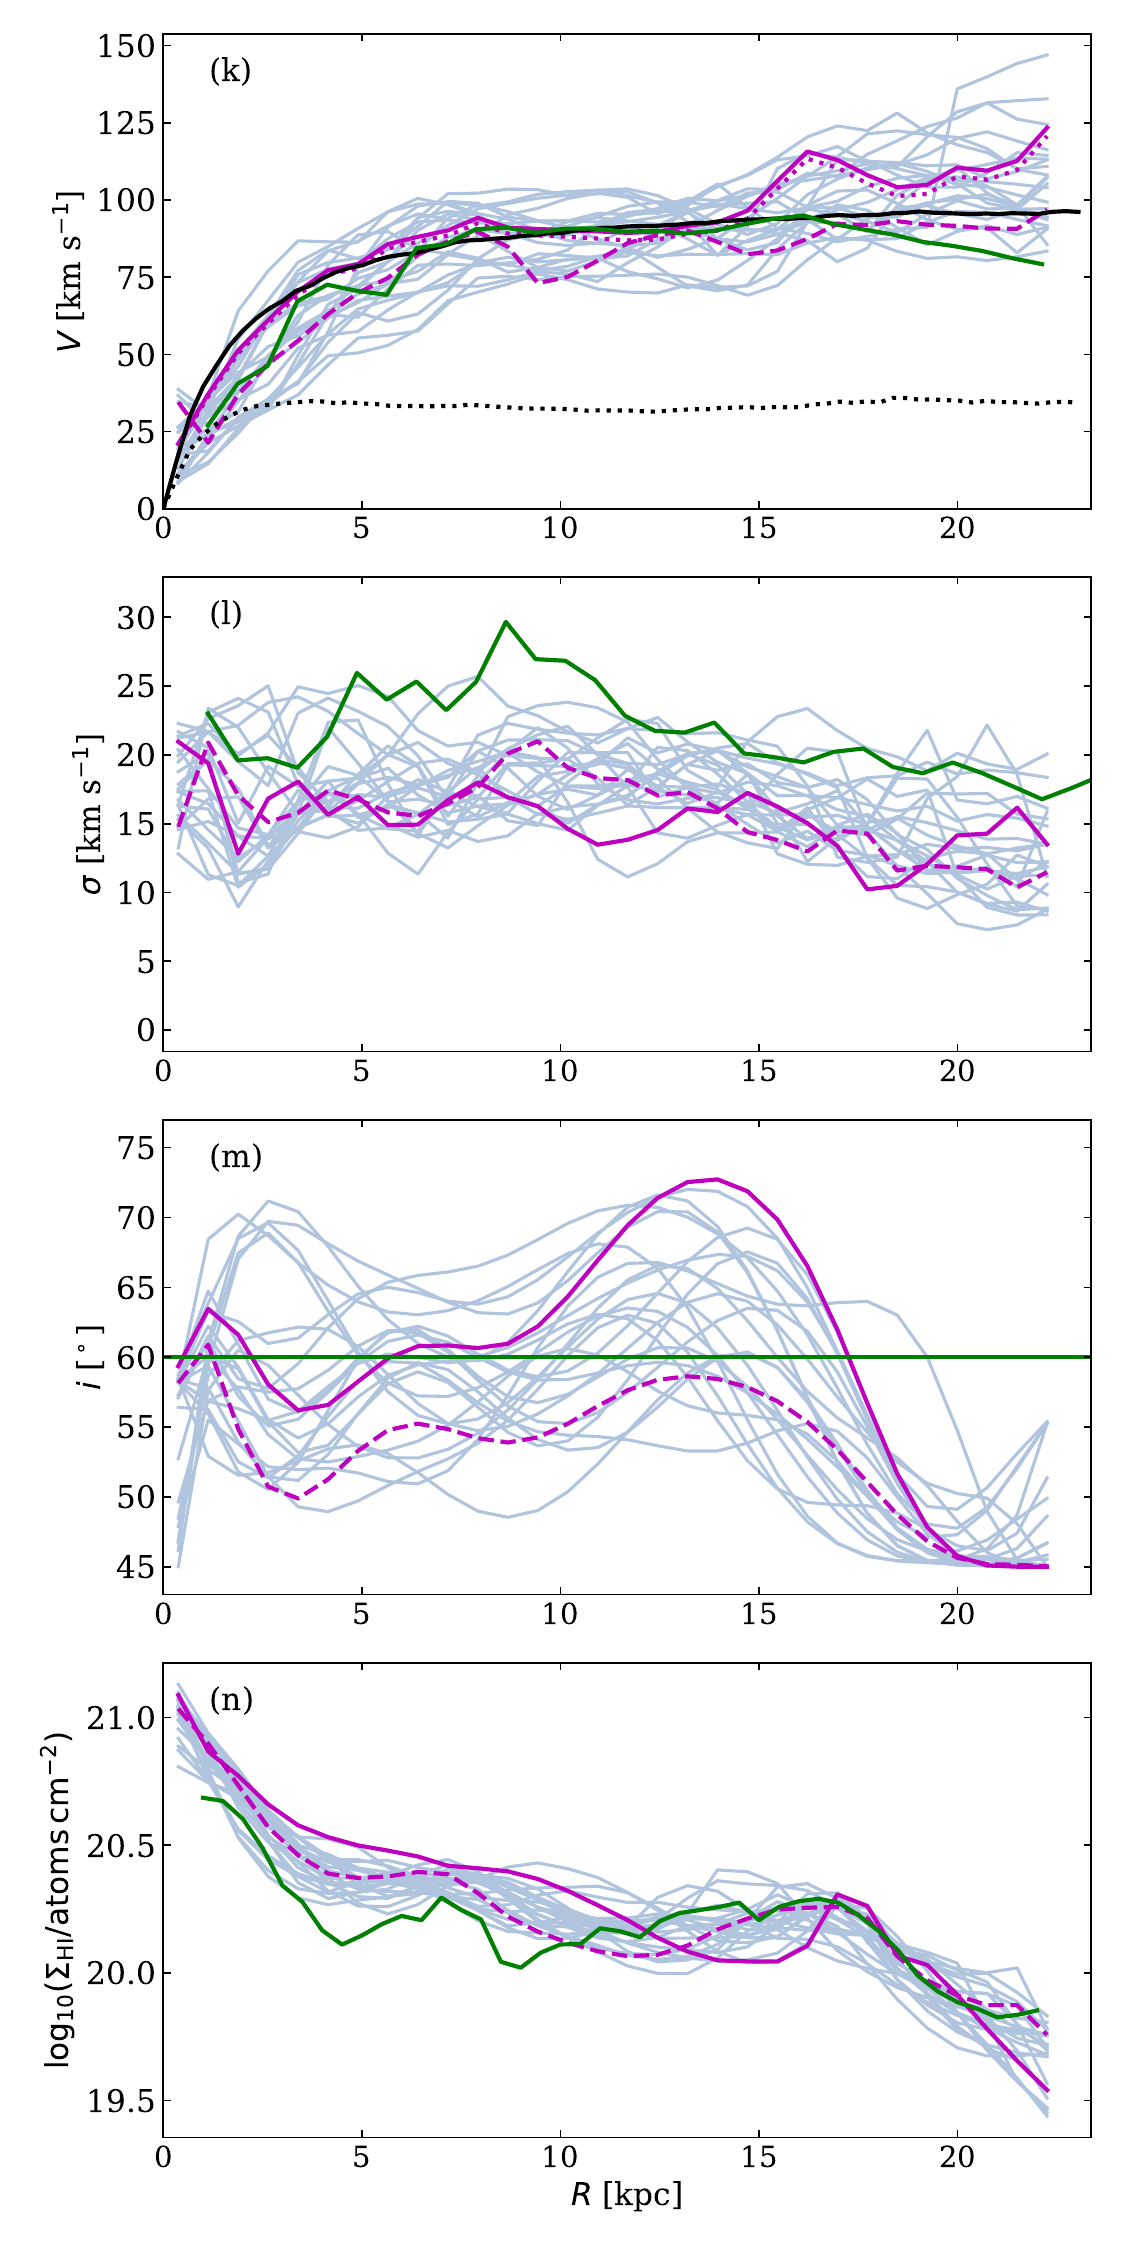}
\end{minipage}
\caption{A set of summary figures for galaxy LT-18, selected for kinematic analysis. These include example moment maps for two orientations (panels (a)--(f); similar to Fig.~\ref{fig:visualisations}), a summary of the parameters $V_\mathrm{fid}$, $V_\mathrm{max}$, $\eta_\mathrm{rot}$, and $\eta_\mathrm{bar}$ (panels (g)--(j); similar to Fig.~\ref{fig:loops}), and a summary of the rotation curve analysis from $24$ viewing angles (panels (k)--(n); similar to Fig.~\ref{fig:rot_curves}). See description of Appendix~\ref{app:supplementary} for details.}
\label{fig:S5}
\end{figure}
\clearpage

\begin{figure}
\begin{minipage}{.9\textwidth}
\includegraphics[width=\textwidth]{../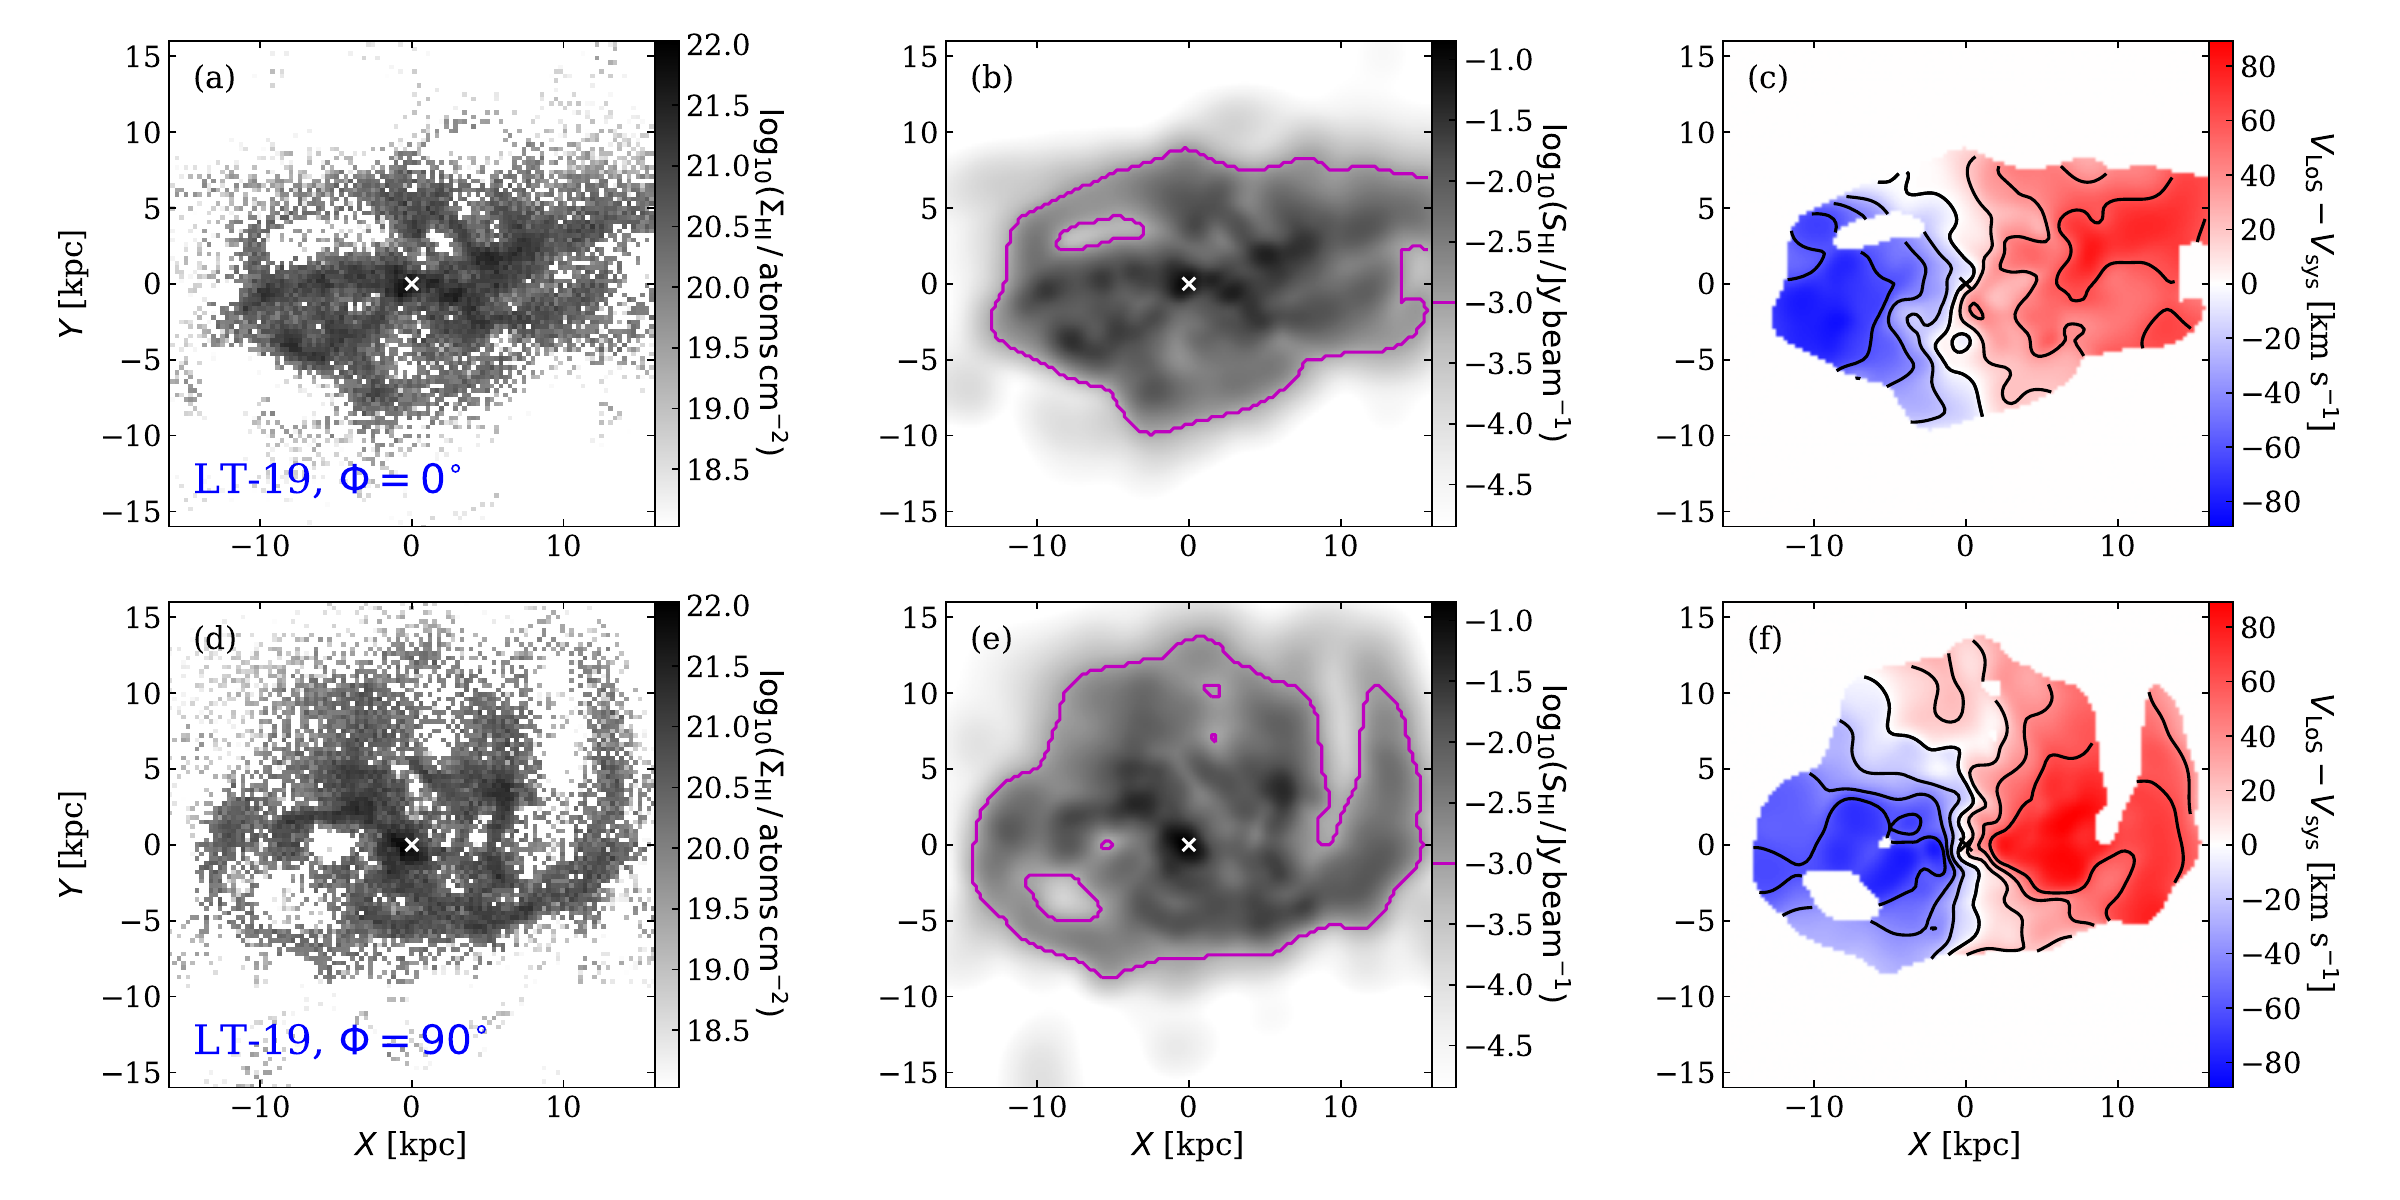}
\includegraphics[width=\textwidth]{../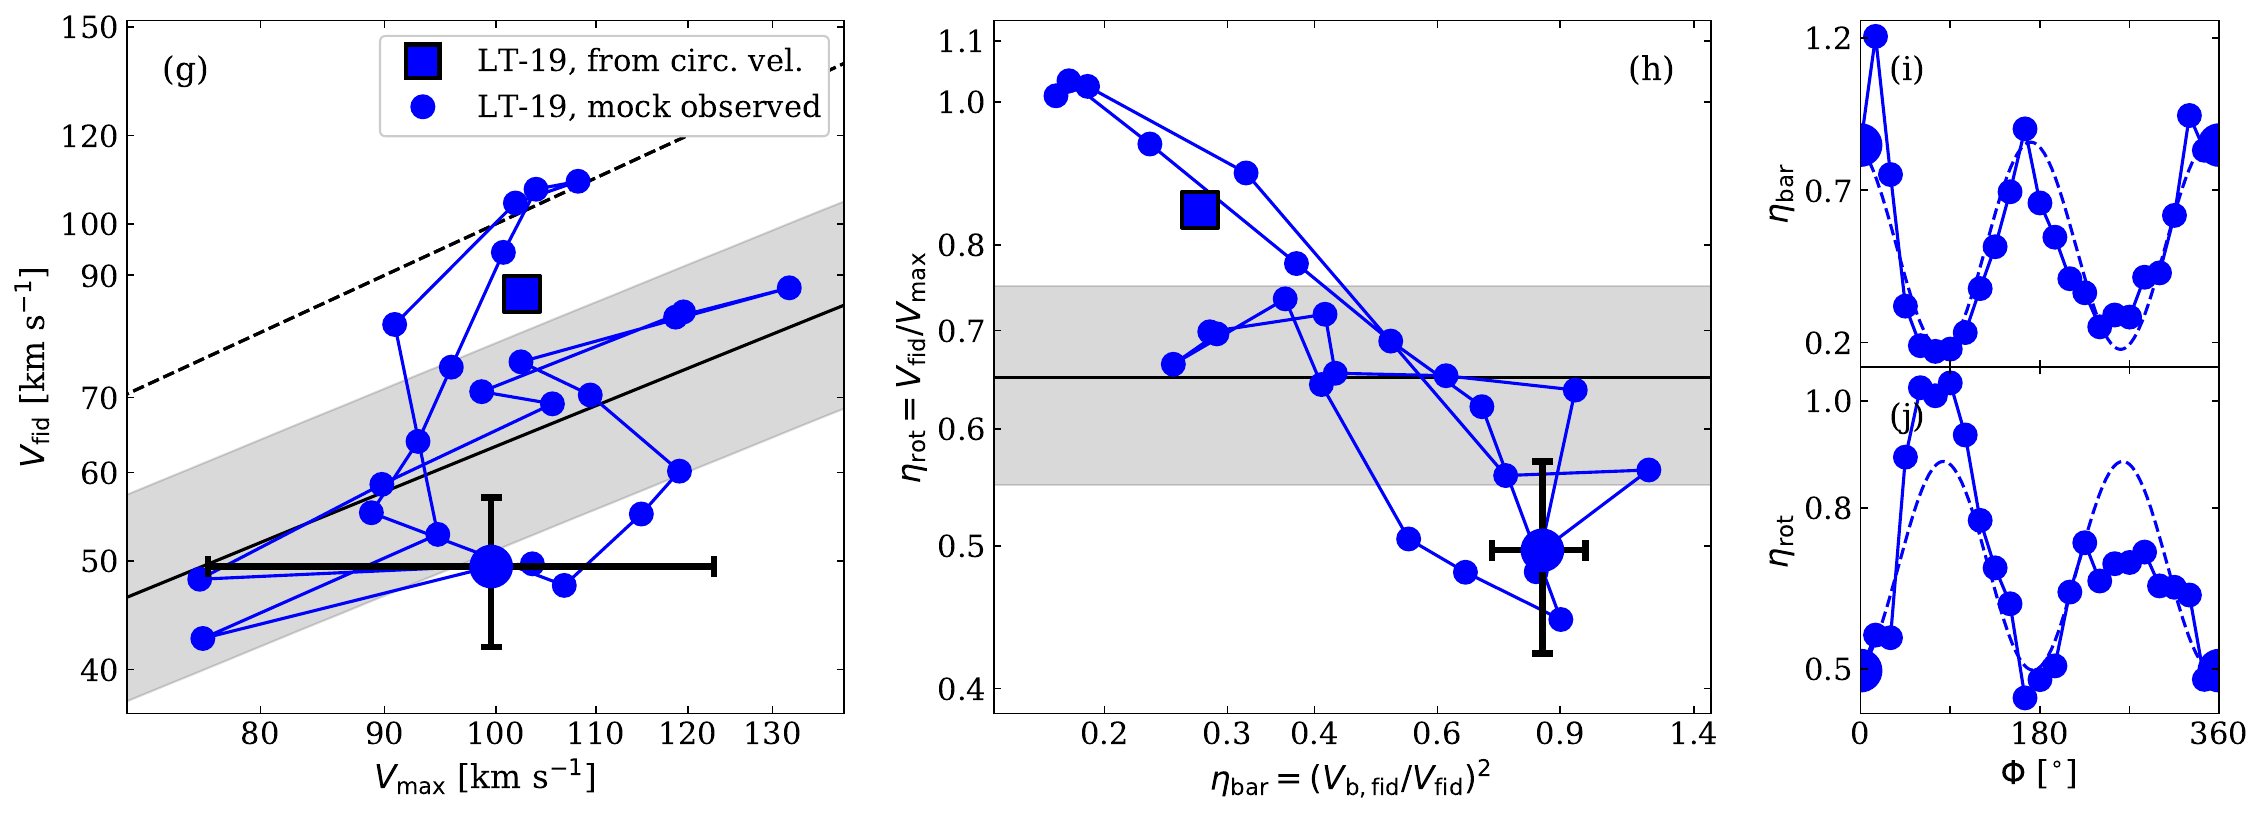}
\end{minipage}
\begin{minipage}{.4\textwidth}
\includegraphics[width=\textwidth]{../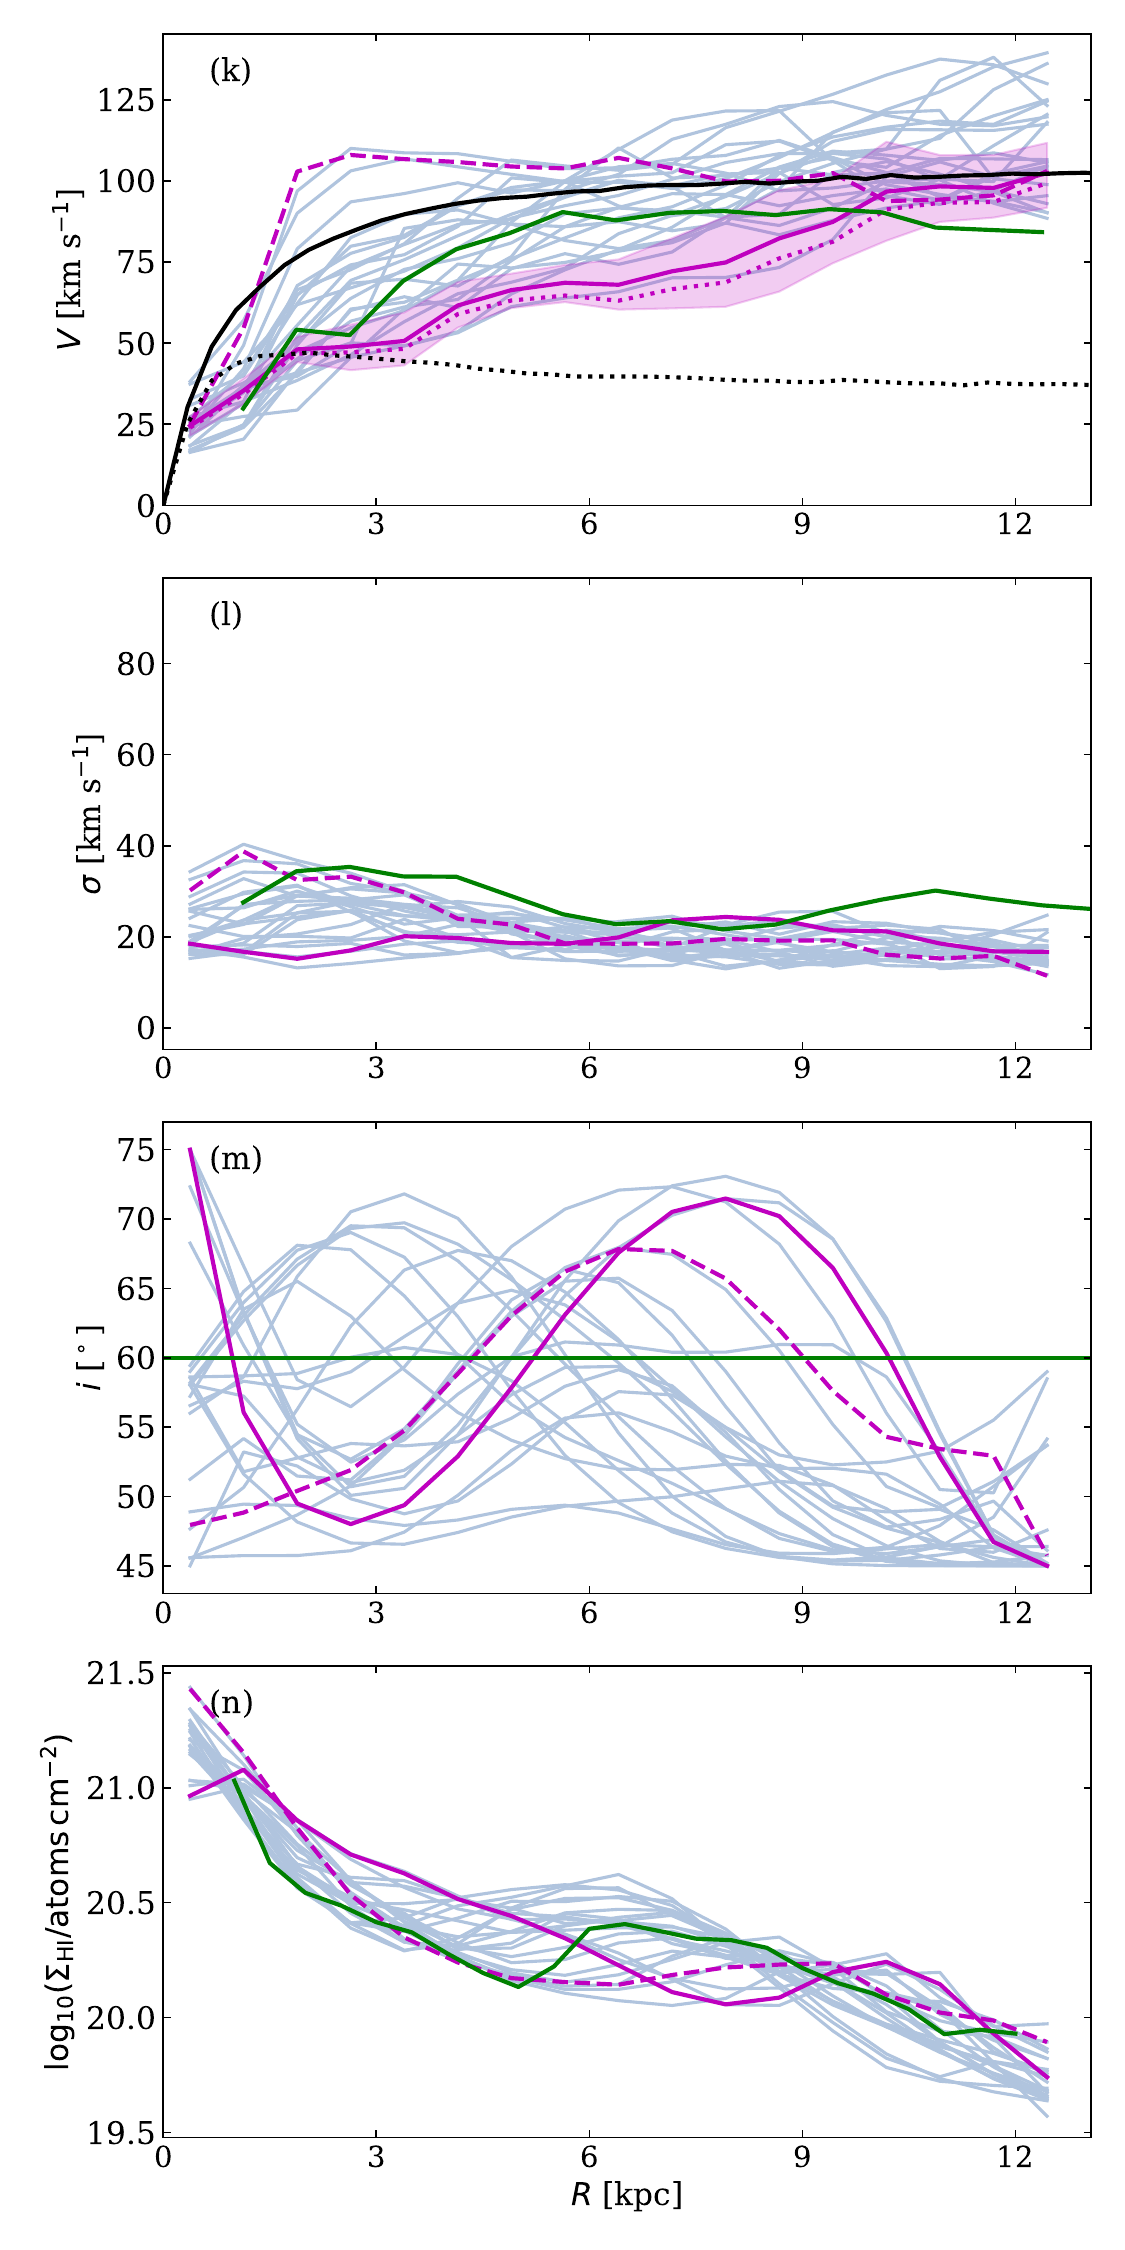}
\end{minipage}
\caption{A set of summary figures for galaxy LT-19, selected for kinematic analysis. These include example moment maps for two orientations (panels (a)--(f); similar to Fig.~\ref{fig:visualisations}), a summary of the parameters $V_\mathrm{fid}$, $V_\mathrm{max}$, $\eta_\mathrm{rot}$, and $\eta_\mathrm{bar}$ (panels (g)--(j); similar to Fig.~\ref{fig:loops}), and a summary of the rotation curve analysis from $24$ viewing angles (panels (k)--(n); similar to Fig.~\ref{fig:rot_curves}). See description of Appendix~\ref{app:supplementary} for details.}
\label{fig:S6}
\end{figure}
\clearpage

\begin{figure}
\begin{minipage}{.9\textwidth}
\includegraphics[width=\textwidth]{../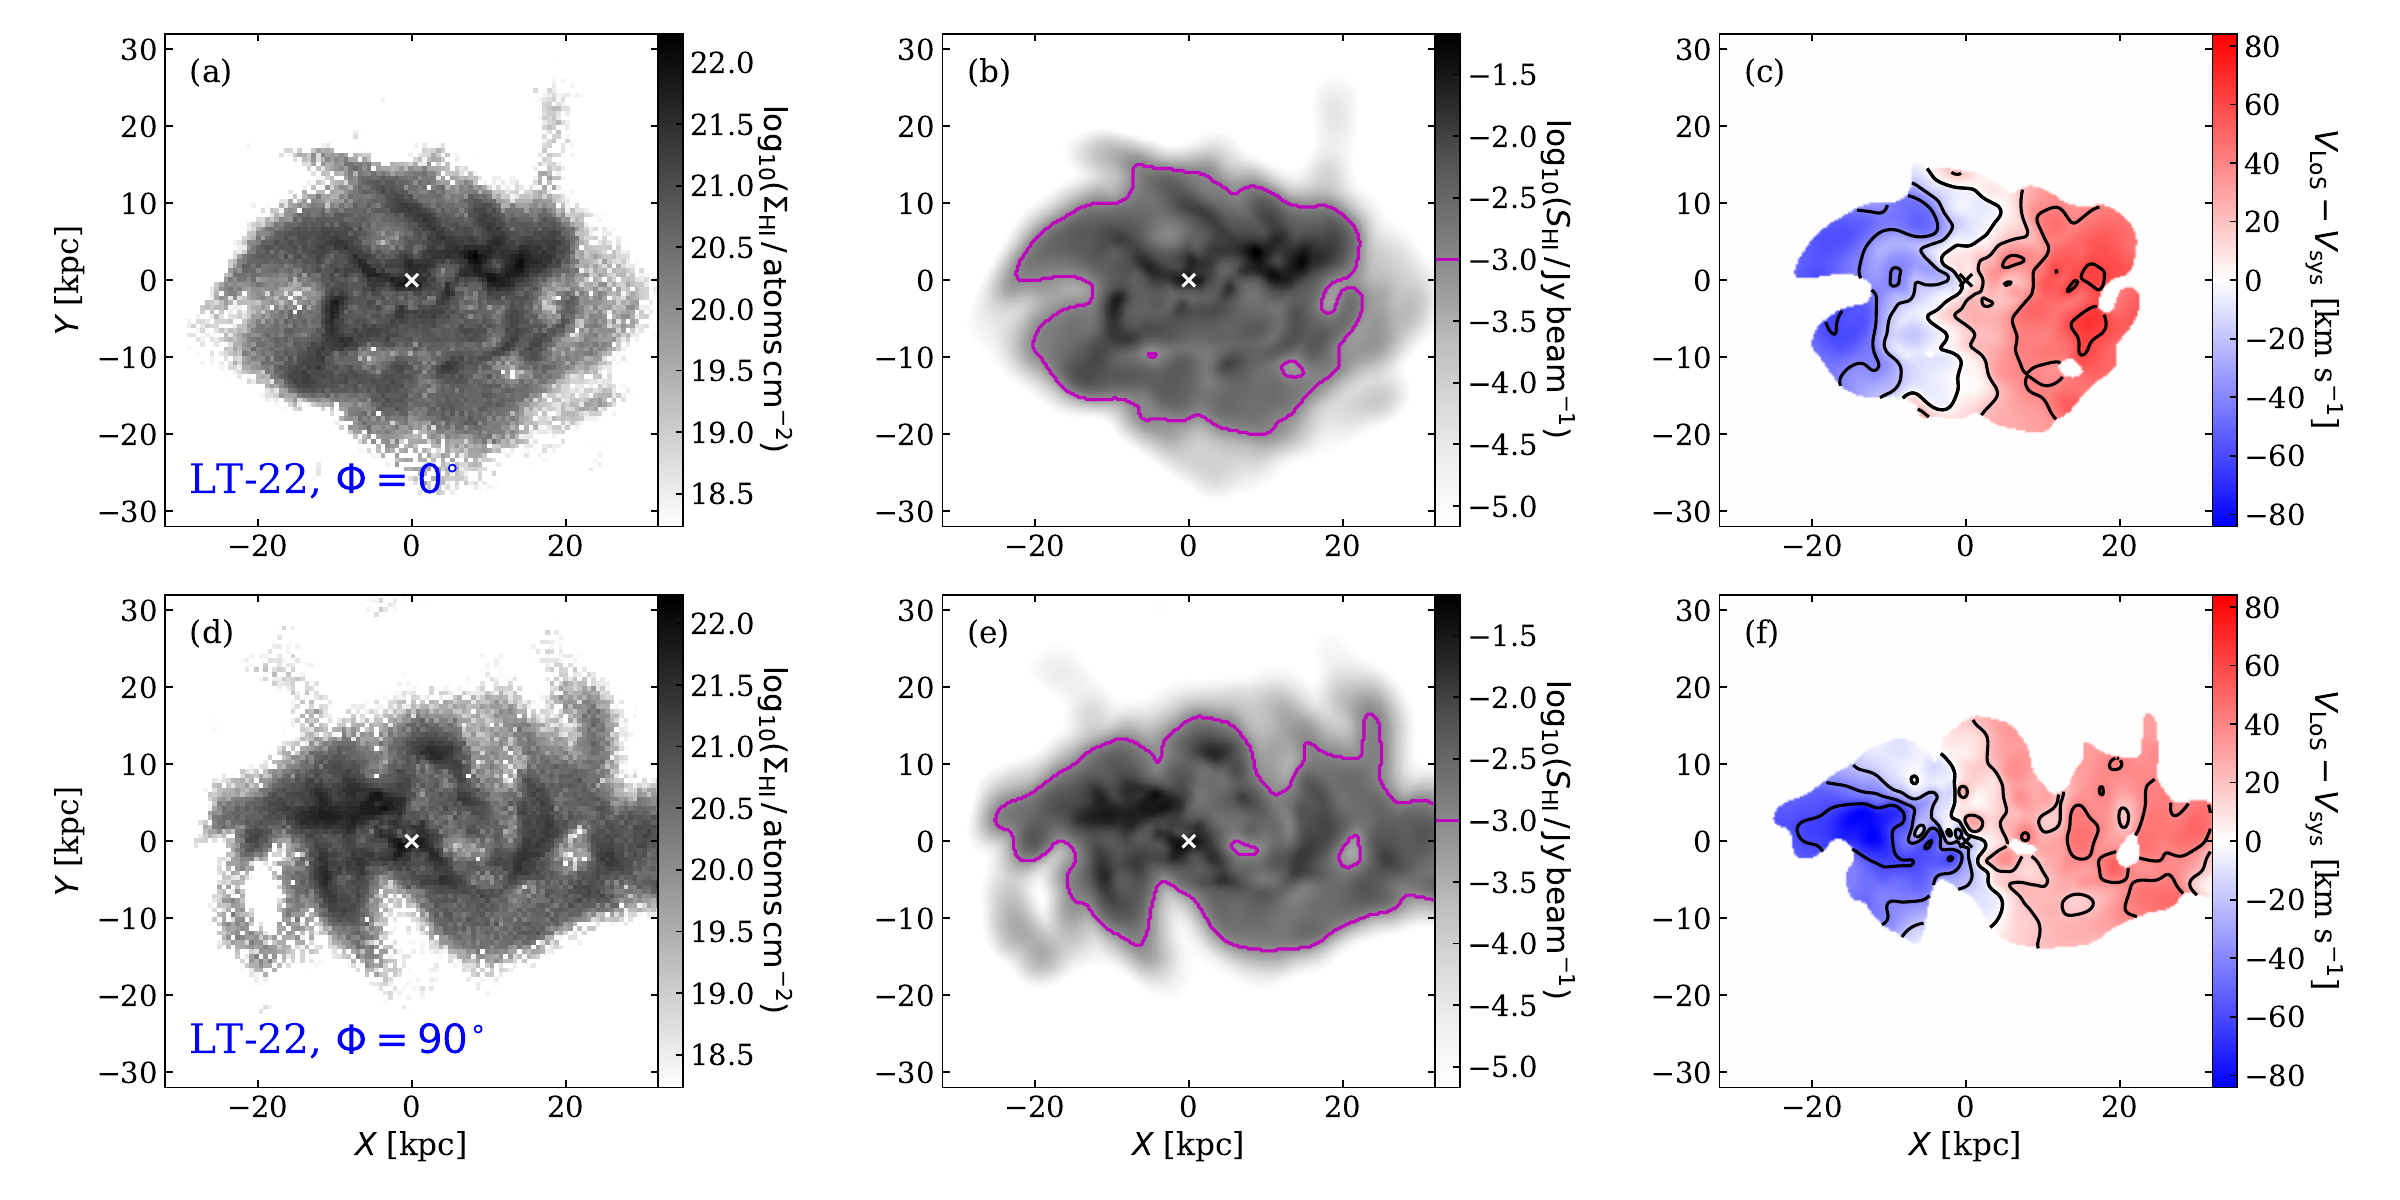}
\includegraphics[width=\textwidth]{../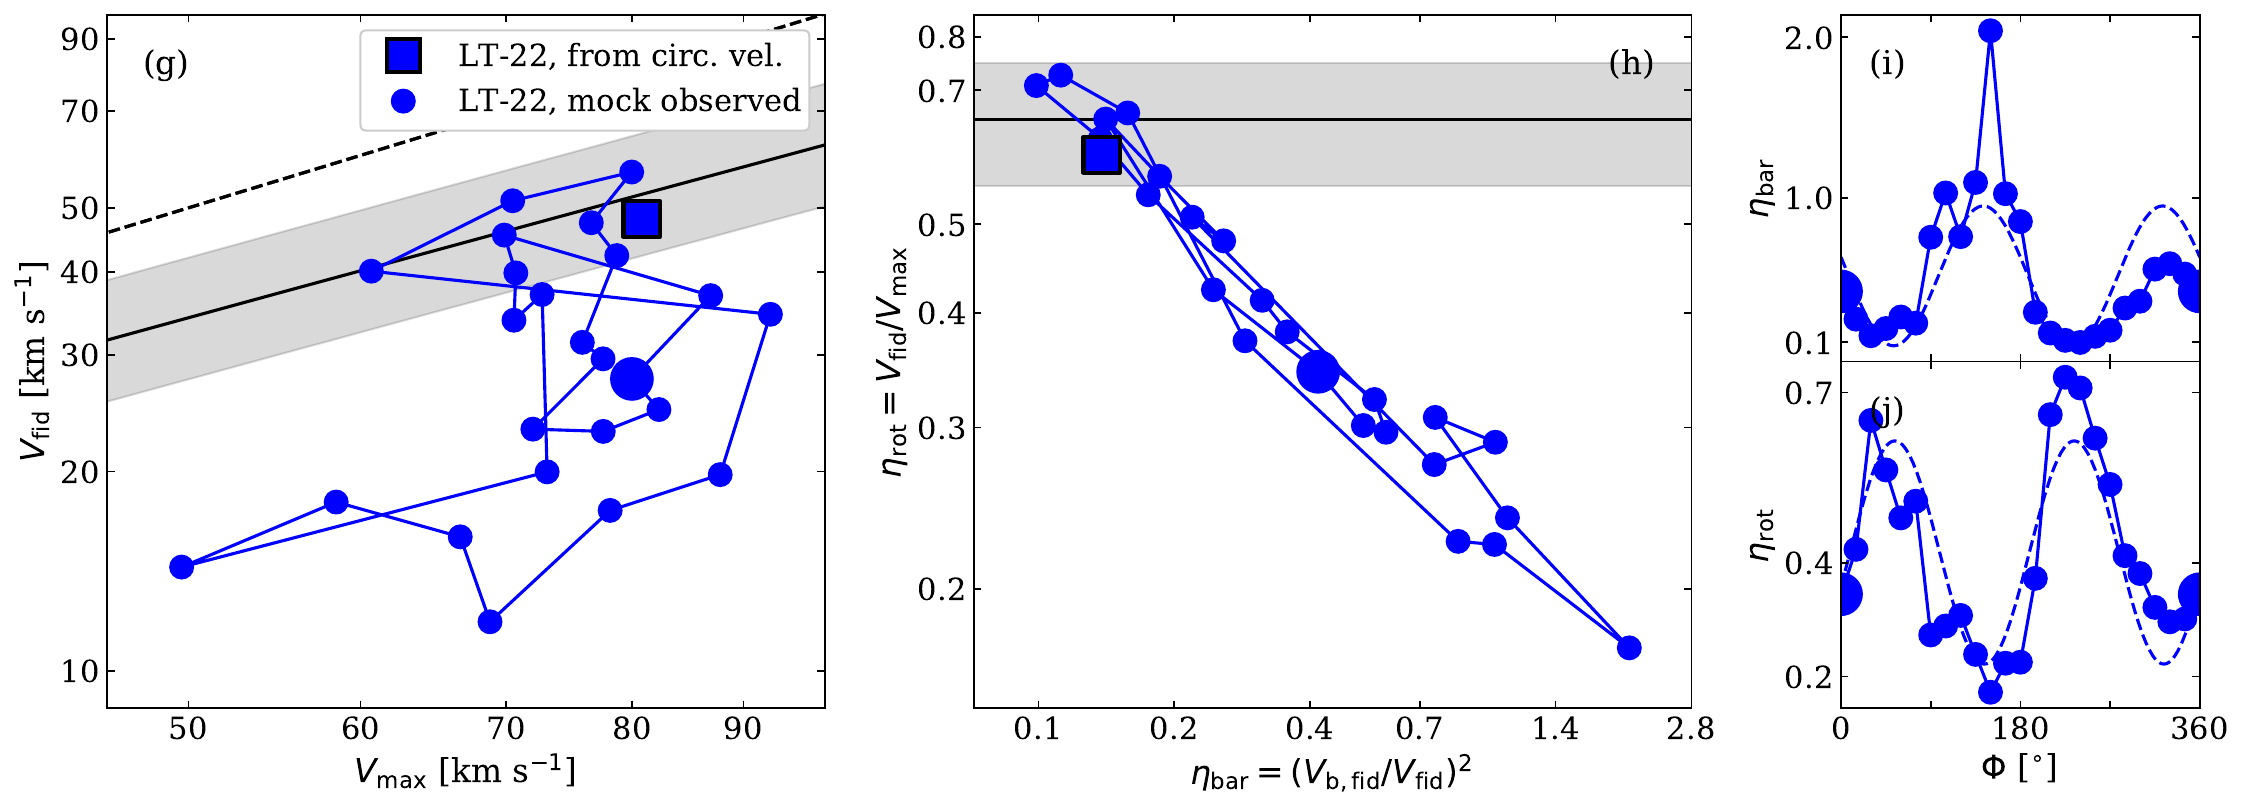}
\end{minipage}
\begin{minipage}{.4\textwidth}
\includegraphics[width=\textwidth]{../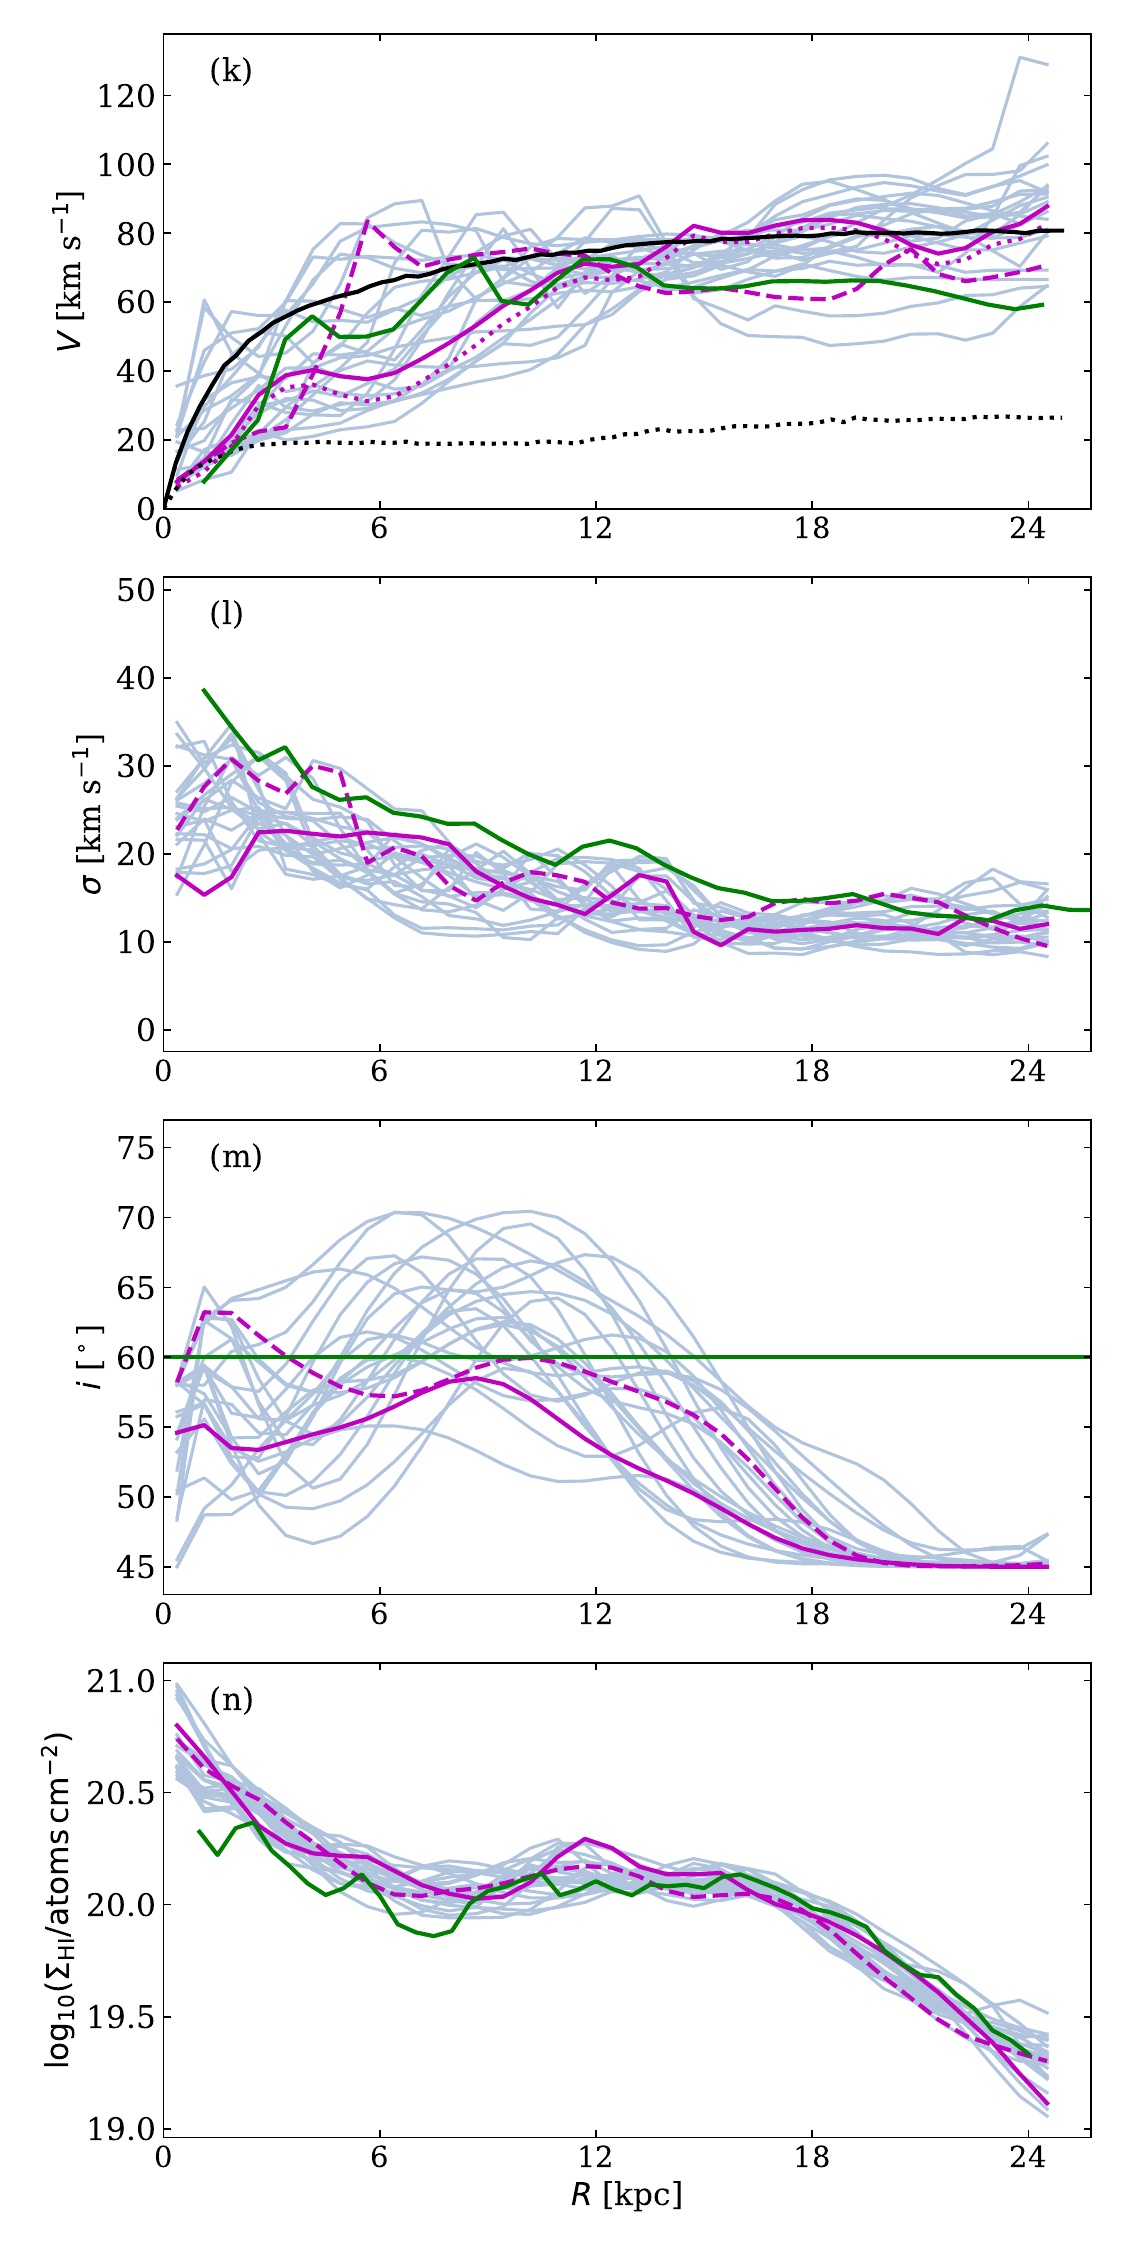}
\end{minipage}
\caption{A set of summary figures for galaxy LT-22, selected for kinematic analysis. These include example moment maps for two orientations (panels (a)--(f); similar to Fig.~\ref{fig:visualisations}), a summary of the parameters $V_\mathrm{fid}$, $V_\mathrm{max}$, $\eta_\mathrm{rot}$, and $\eta_\mathrm{bar}$ (panels (g)--(j); similar to Fig.~\ref{fig:loops}), and a summary of the rotation curve analysis from $24$ viewing angles (panels (k)--(n); similar to Fig.~\ref{fig:rot_curves}). See description of Appendix~\ref{app:supplementary} for details.}
\label{fig:S7}
\end{figure}
\clearpage

\begin{figure}
\begin{minipage}{.9\textwidth}
\includegraphics[width=\textwidth]{../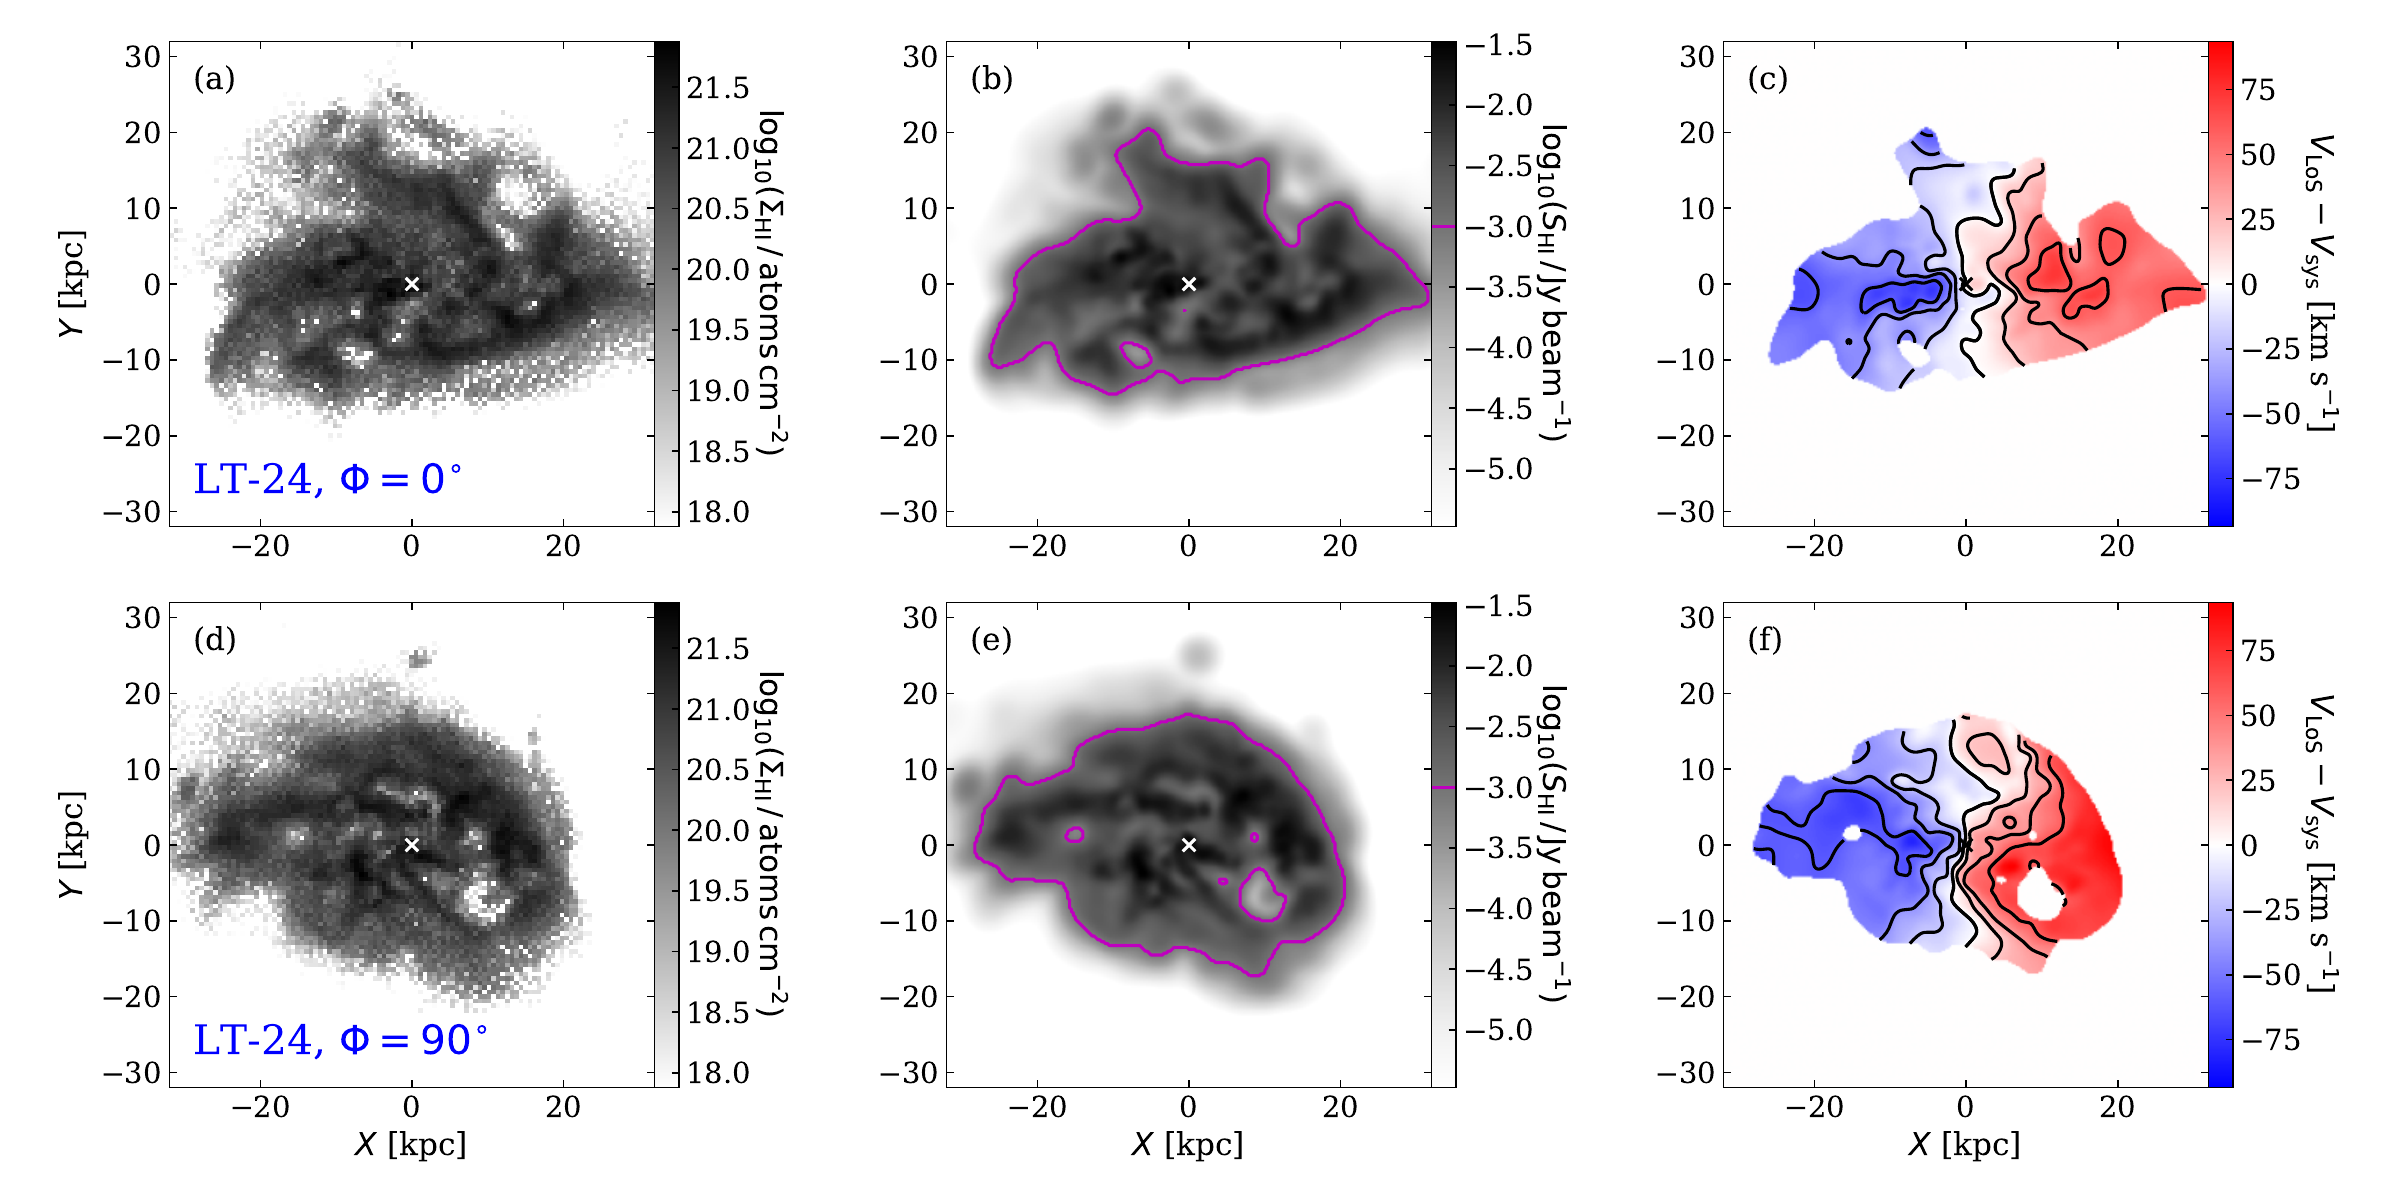}
\includegraphics[width=\textwidth]{../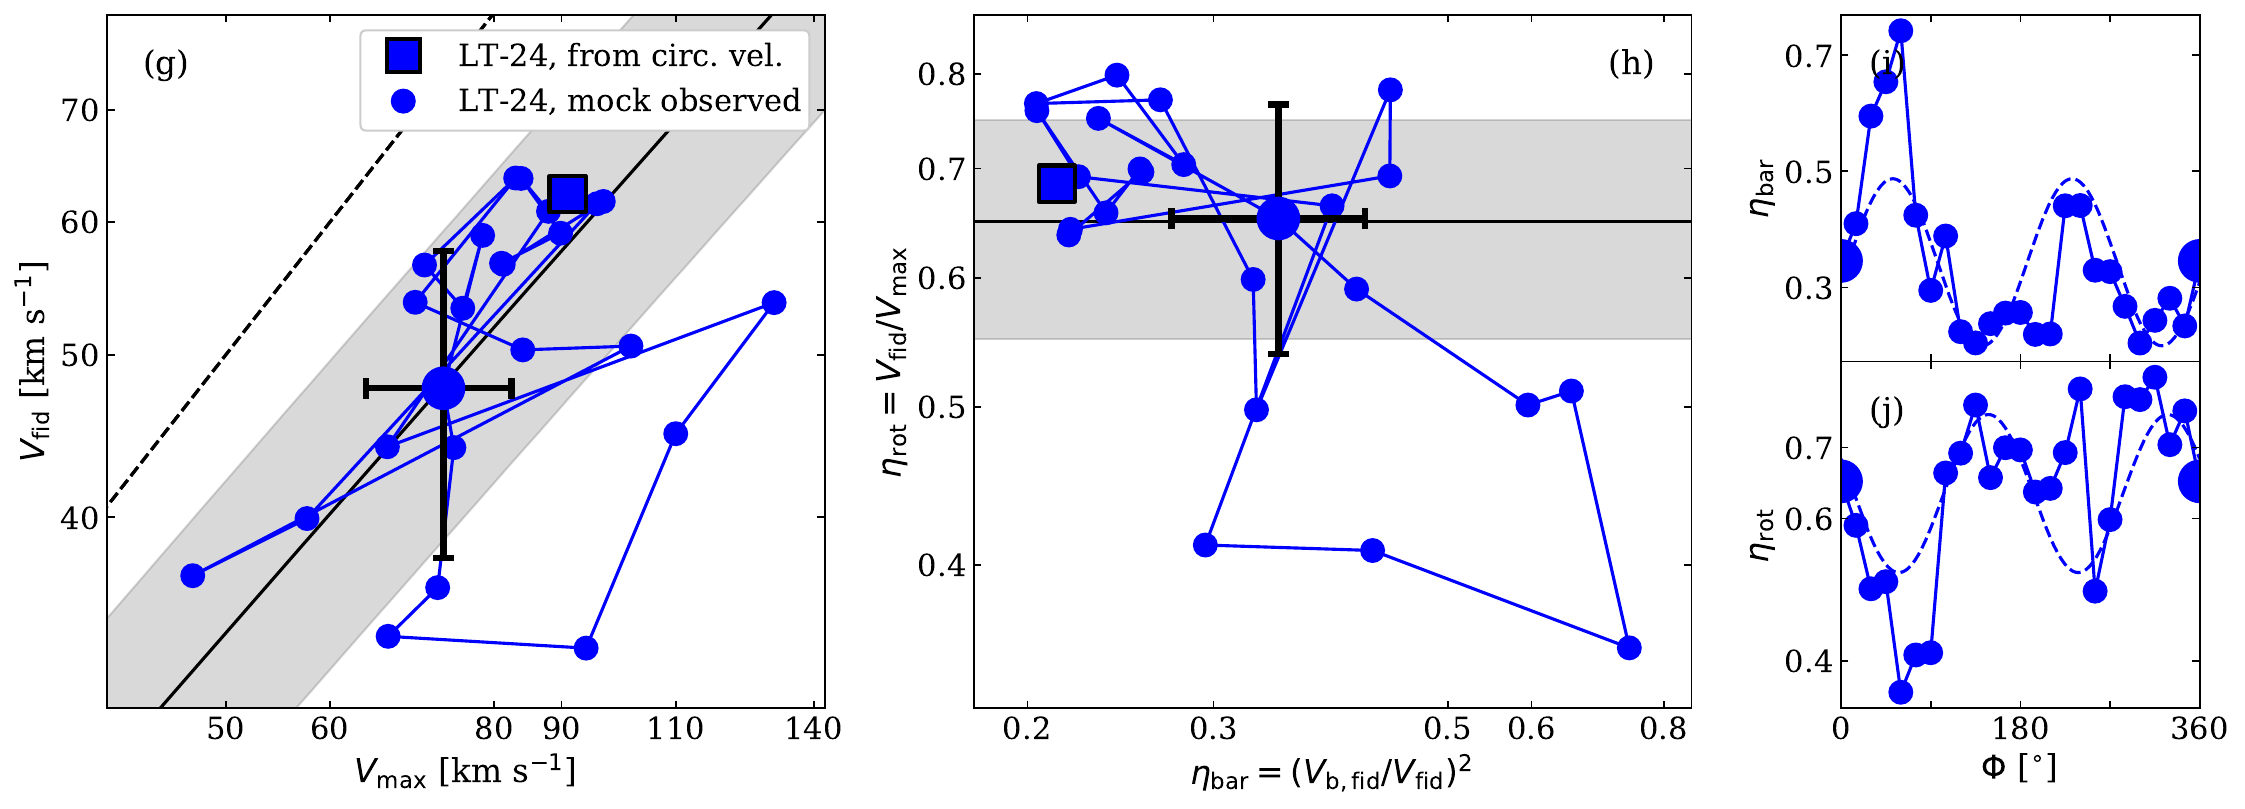}
\end{minipage}
\begin{minipage}{.4\textwidth}
\includegraphics[width=\textwidth]{../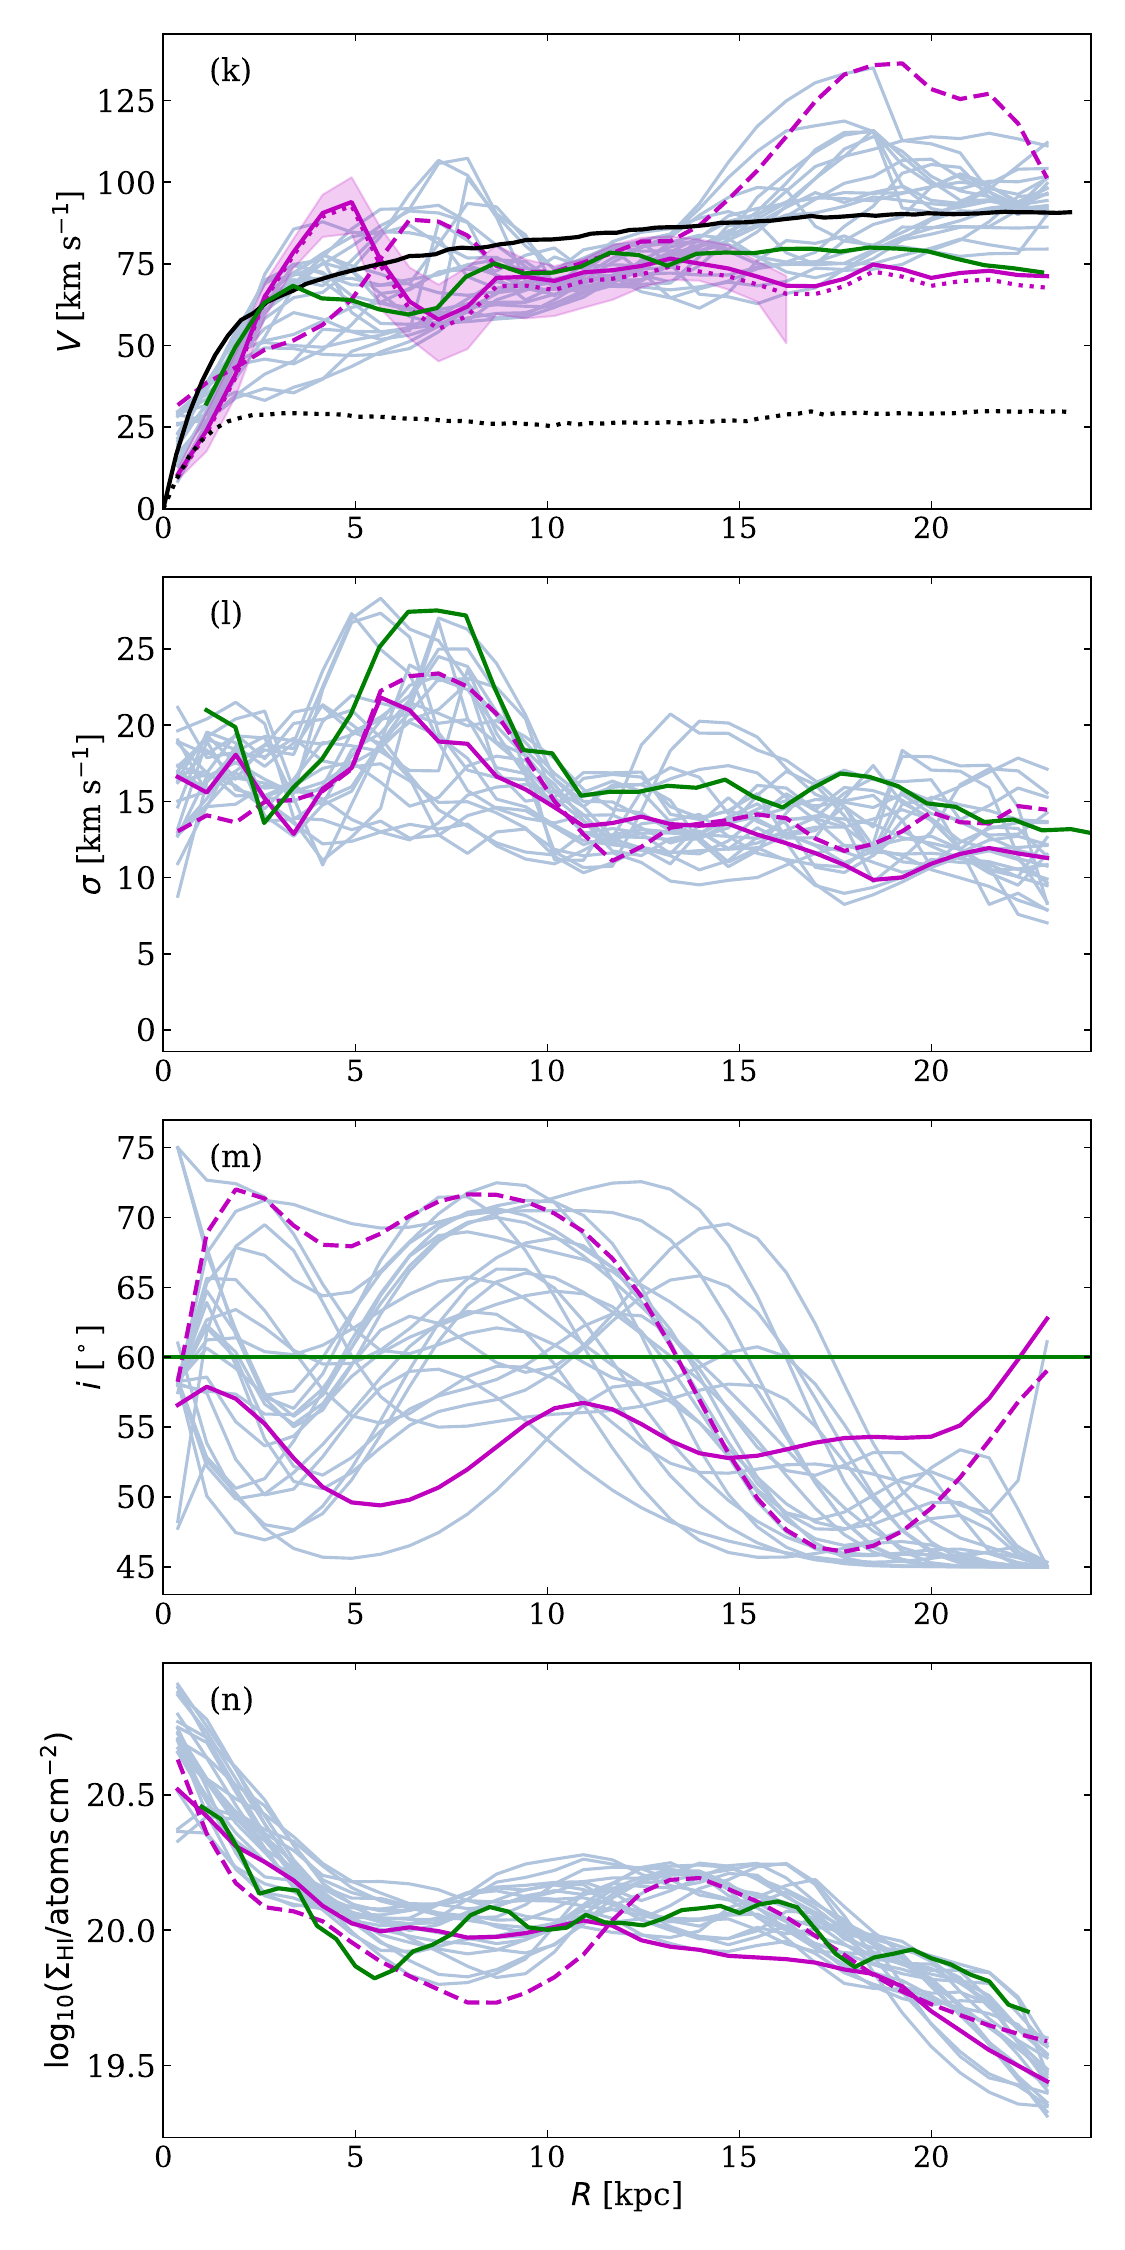}
\end{minipage}
\caption{A set of summary figures for galaxy LT-24, selected for kinematic analysis. These include example moment maps for two orientations (panels (a)--(f); similar to Fig.~\ref{fig:visualisations}), a summary of the parameters $V_\mathrm{fid}$, $V_\mathrm{max}$, $\eta_\mathrm{rot}$, and $\eta_\mathrm{bar}$ (panels (g)--(j); similar to Fig.~\ref{fig:loops}), and a summary of the rotation curve analysis from $24$ viewing angles (panels (k)--(n); similar to Fig.~\ref{fig:rot_curves}). See description of Appendix~\ref{app:supplementary} for details.}
\label{fig:S8}
\end{figure}
\clearpage

\begin{figure}
\begin{minipage}{.9\textwidth}
\includegraphics[width=\textwidth]{../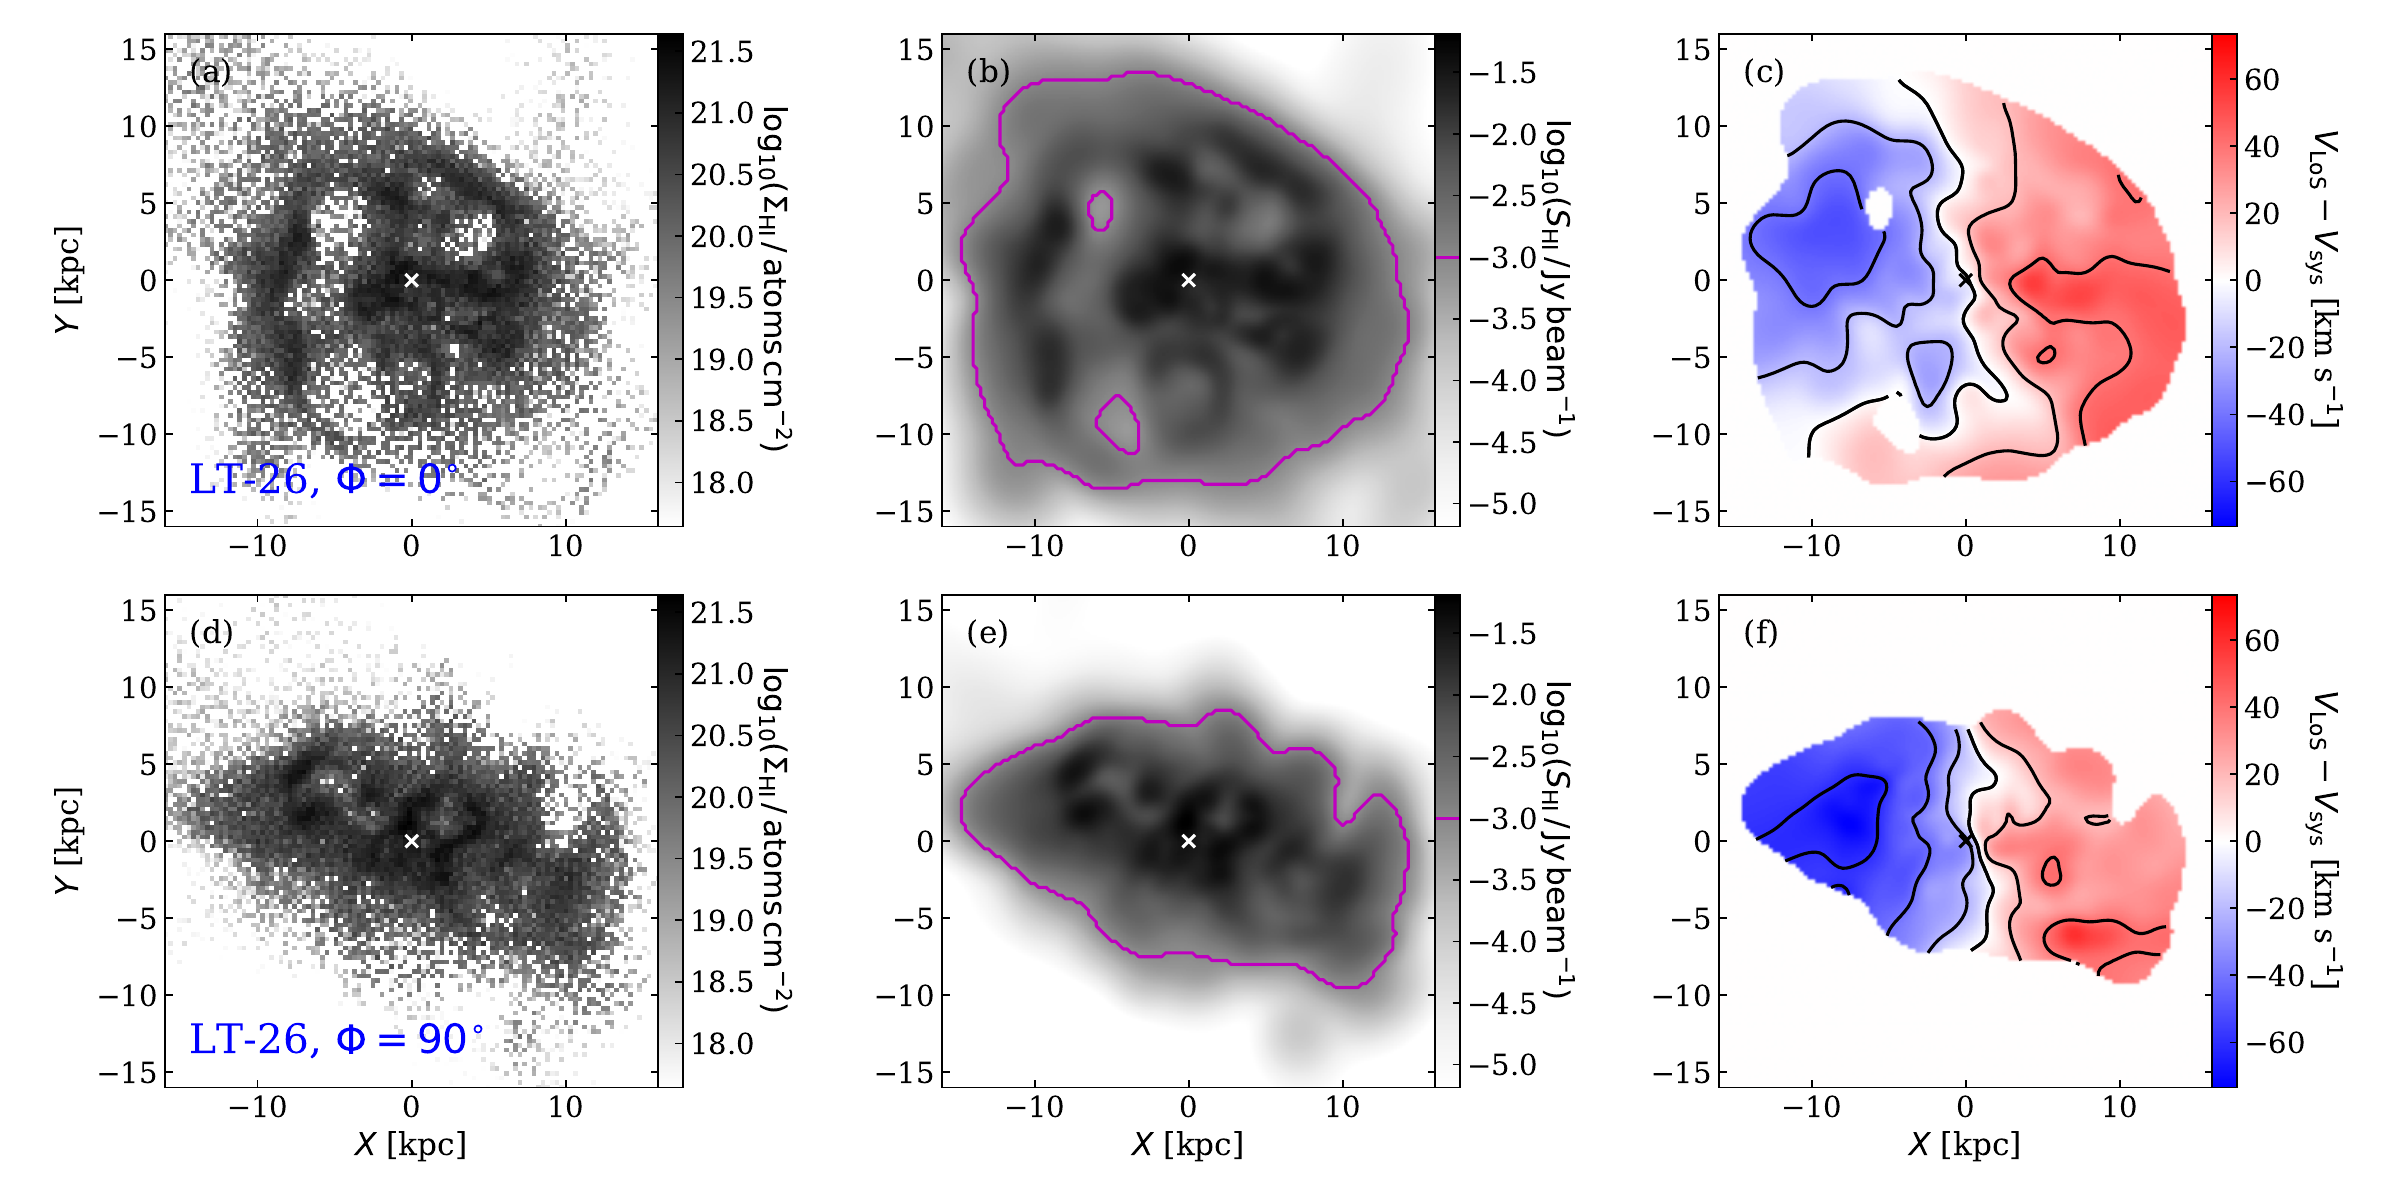}
\includegraphics[width=\textwidth]{../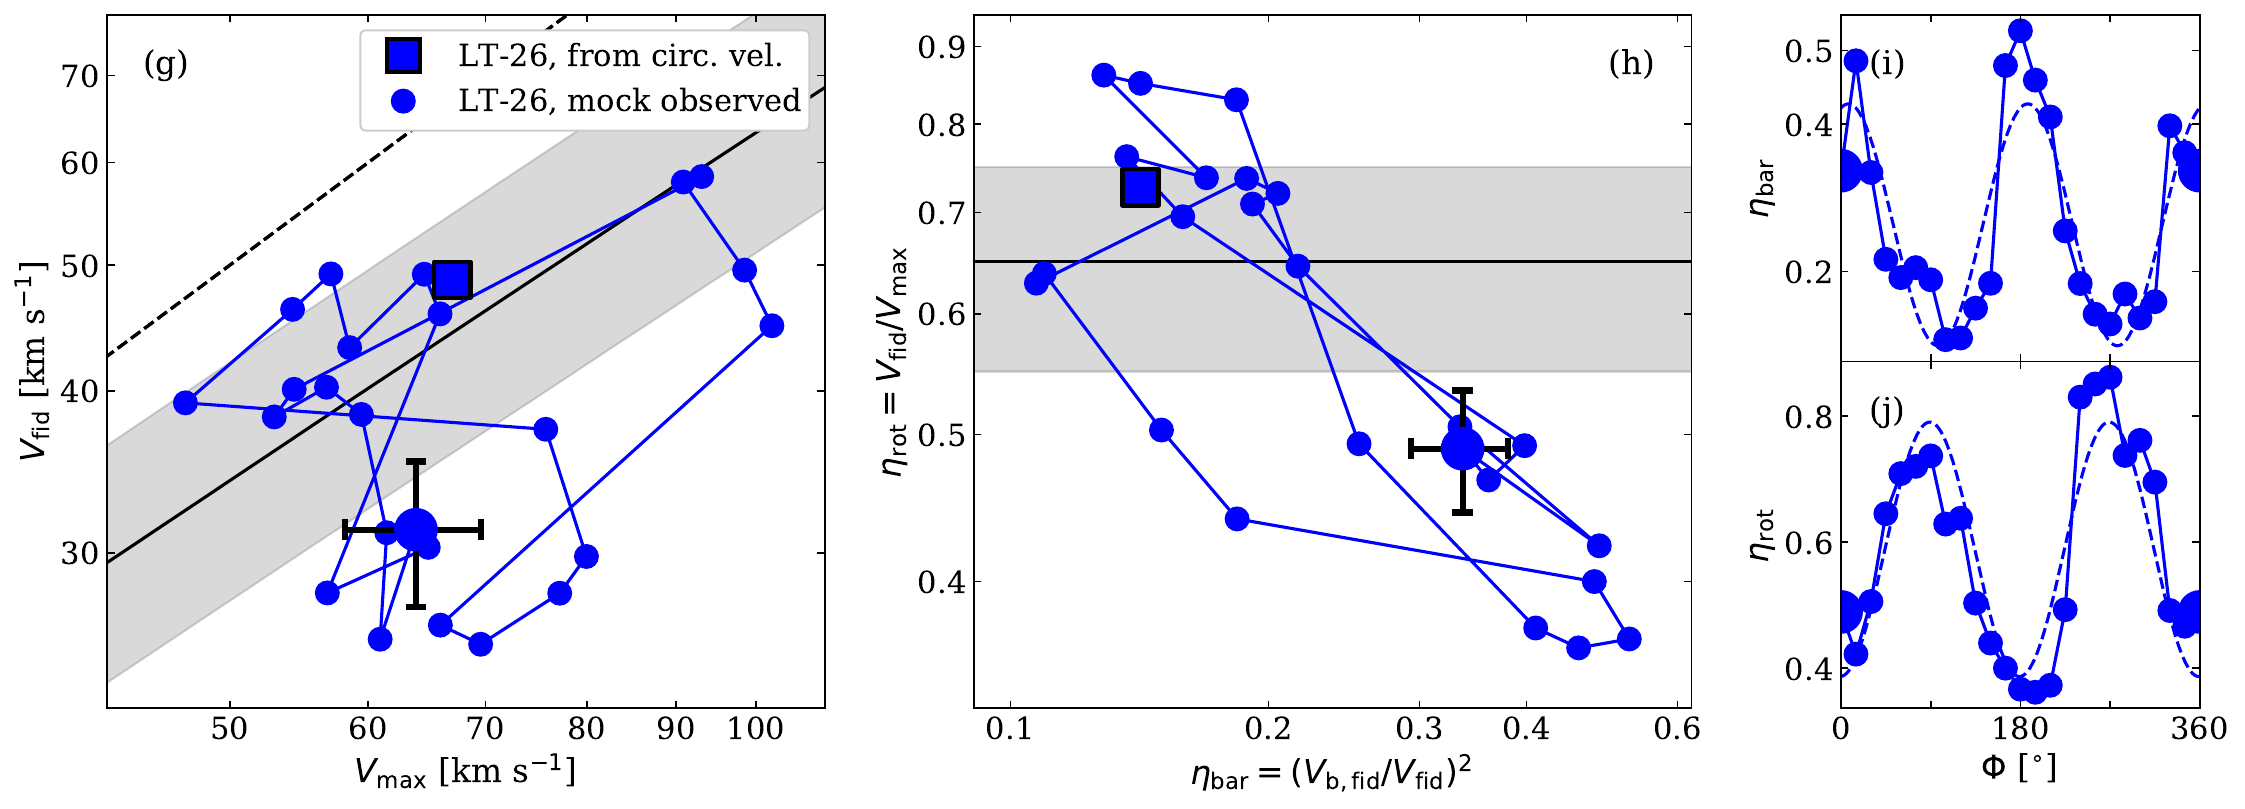}
\end{minipage}
\begin{minipage}{.4\textwidth}
\includegraphics[width=\textwidth]{../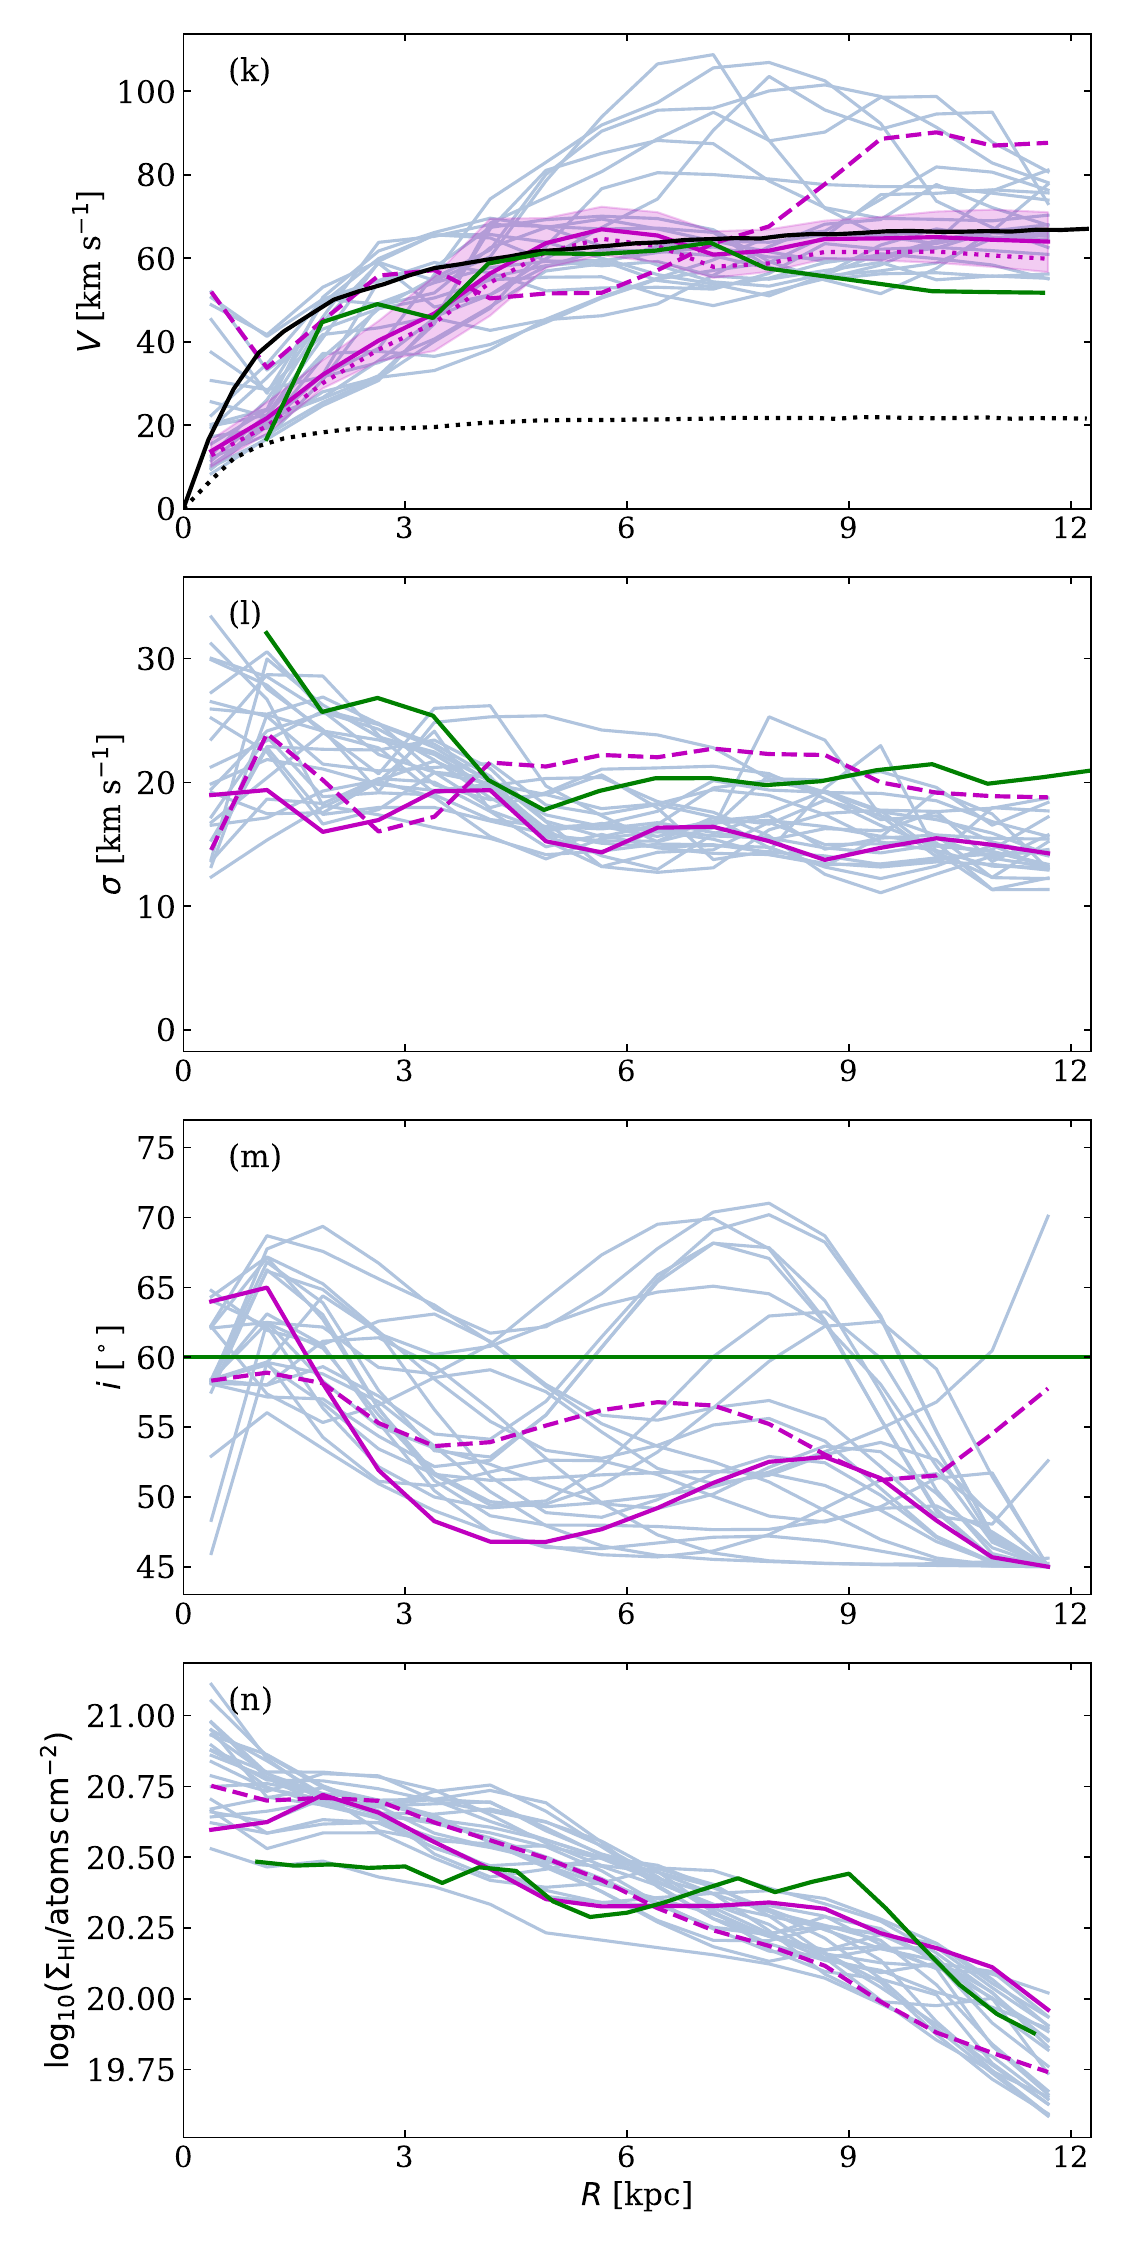}
\end{minipage}
\caption{A set of summary figures for galaxy LT-26, selected for kinematic analysis. These include example moment maps for two orientations (panels (a)--(f); similar to Fig.~\ref{fig:visualisations}), a summary of the parameters $V_\mathrm{fid}$, $V_\mathrm{max}$, $\eta_\mathrm{rot}$, and $\eta_\mathrm{bar}$ (panels (g)--(j); similar to Fig.~\ref{fig:loops}), and a summary of the rotation curve analysis from $24$ viewing angles (panels (k)--(n); similar to Fig.~\ref{fig:rot_curves}). See description of Appendix~\ref{app:supplementary} for details.}
\label{fig:S9}
\end{figure}
\clearpage

\begin{figure}
\begin{minipage}{.9\textwidth}
\includegraphics[width=\textwidth]{../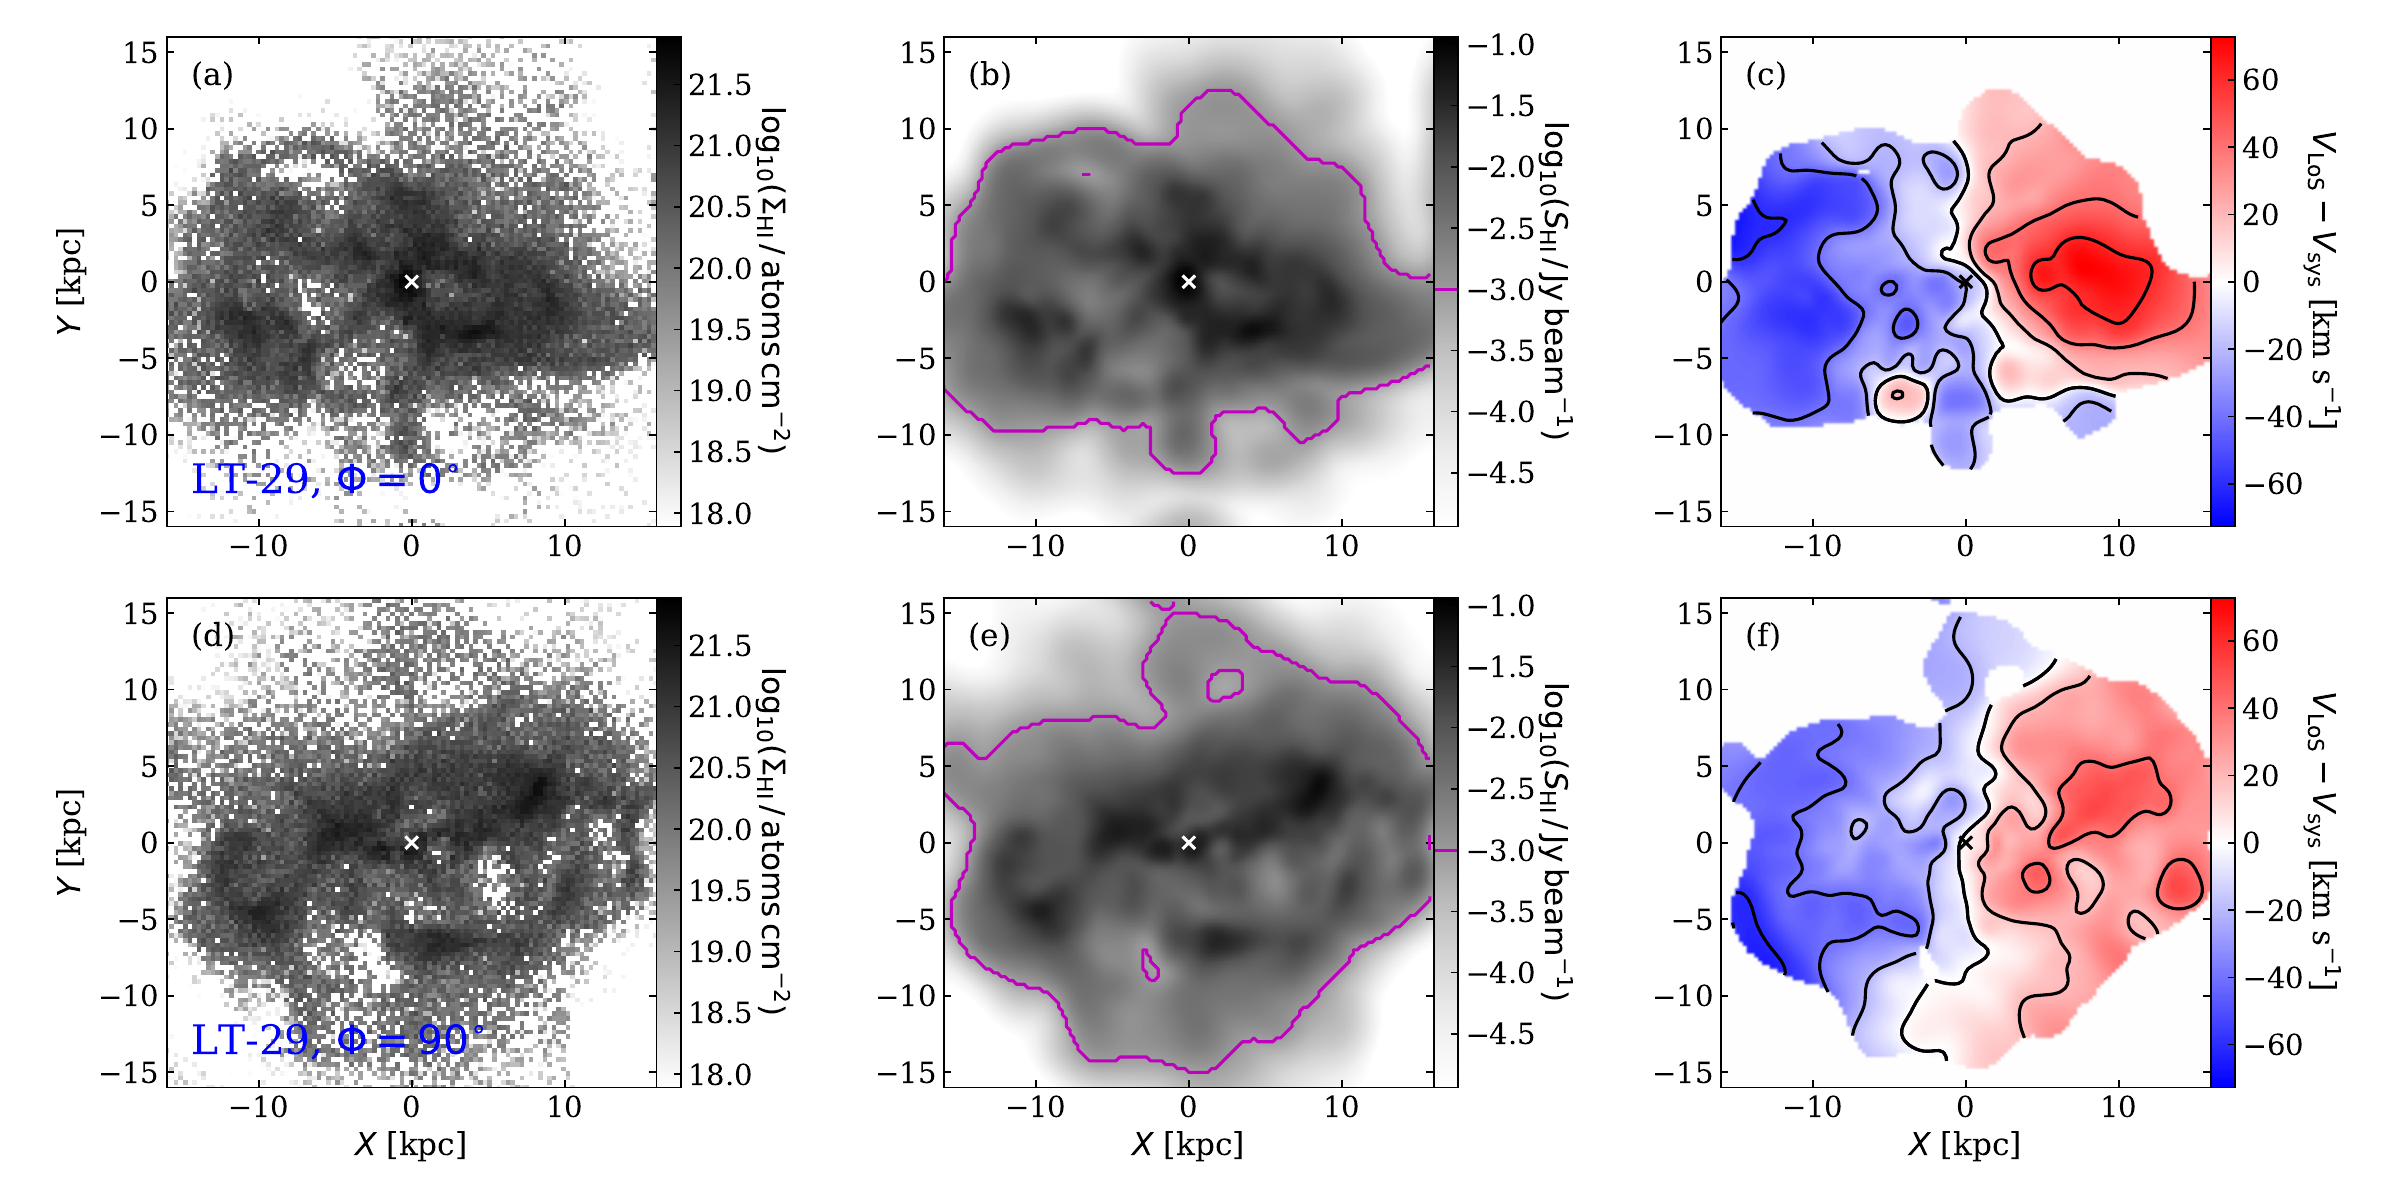}
\includegraphics[width=\textwidth]{../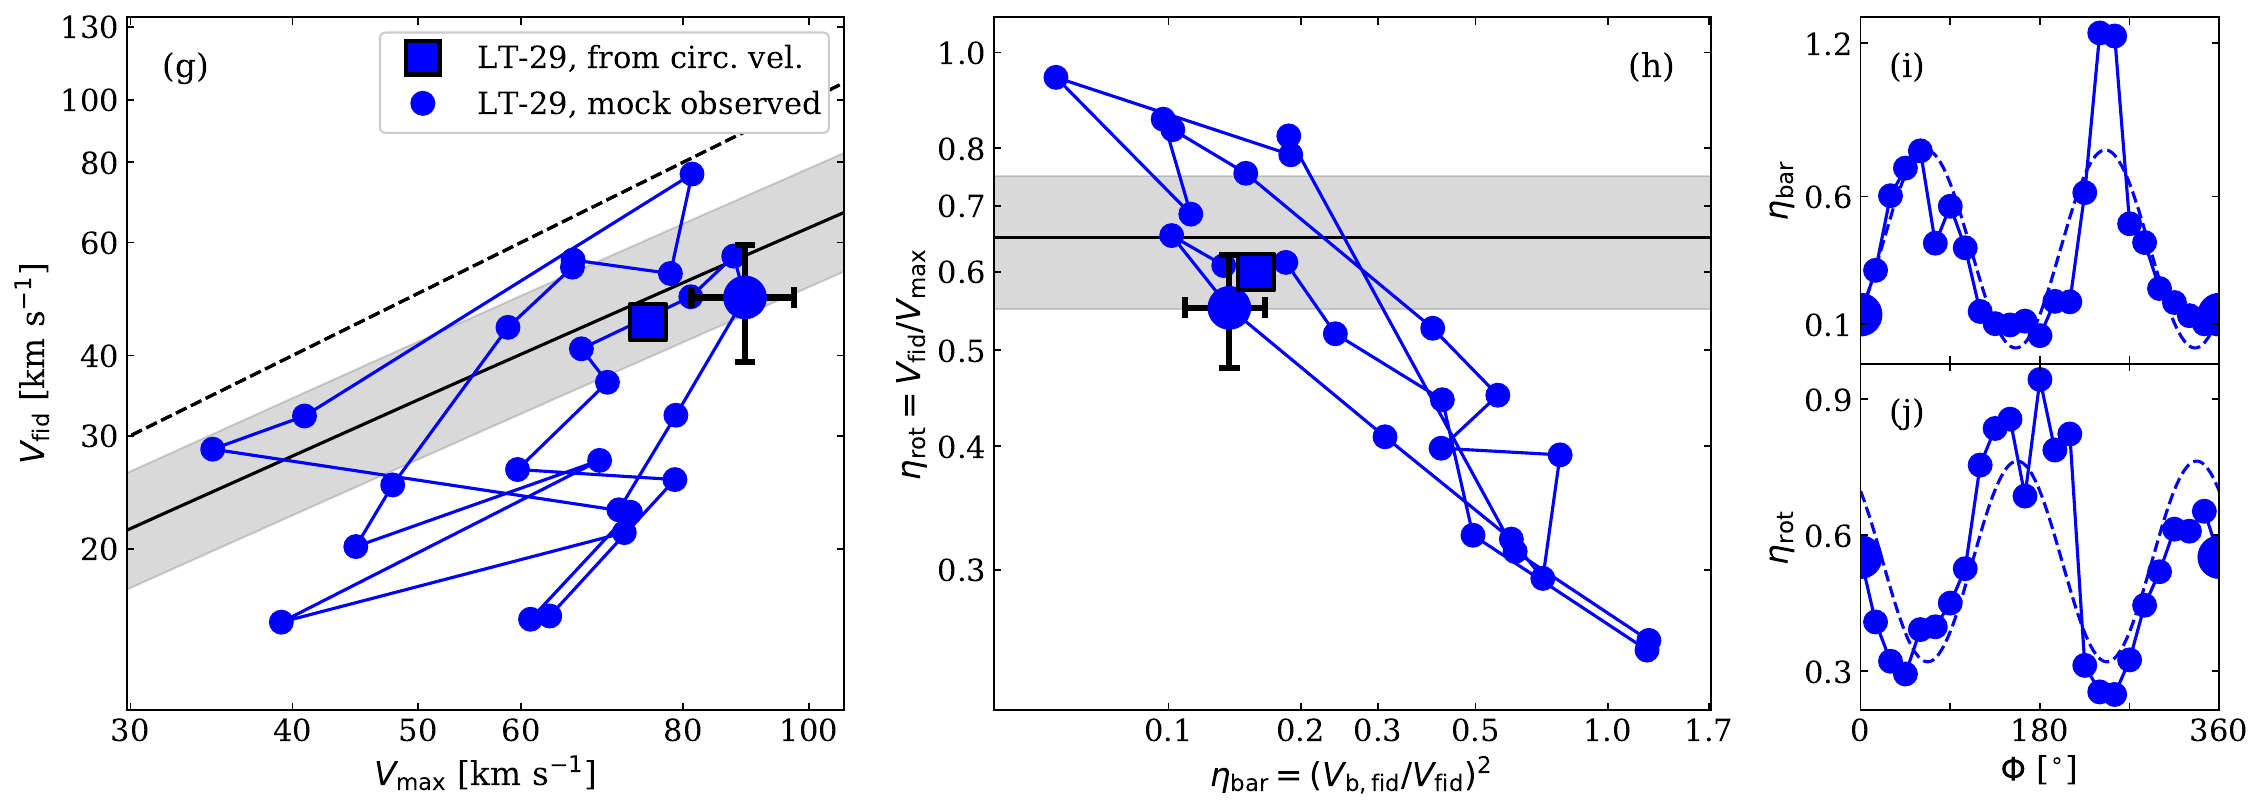}
\end{minipage}
\begin{minipage}{.4\textwidth}
\includegraphics[width=\textwidth]{../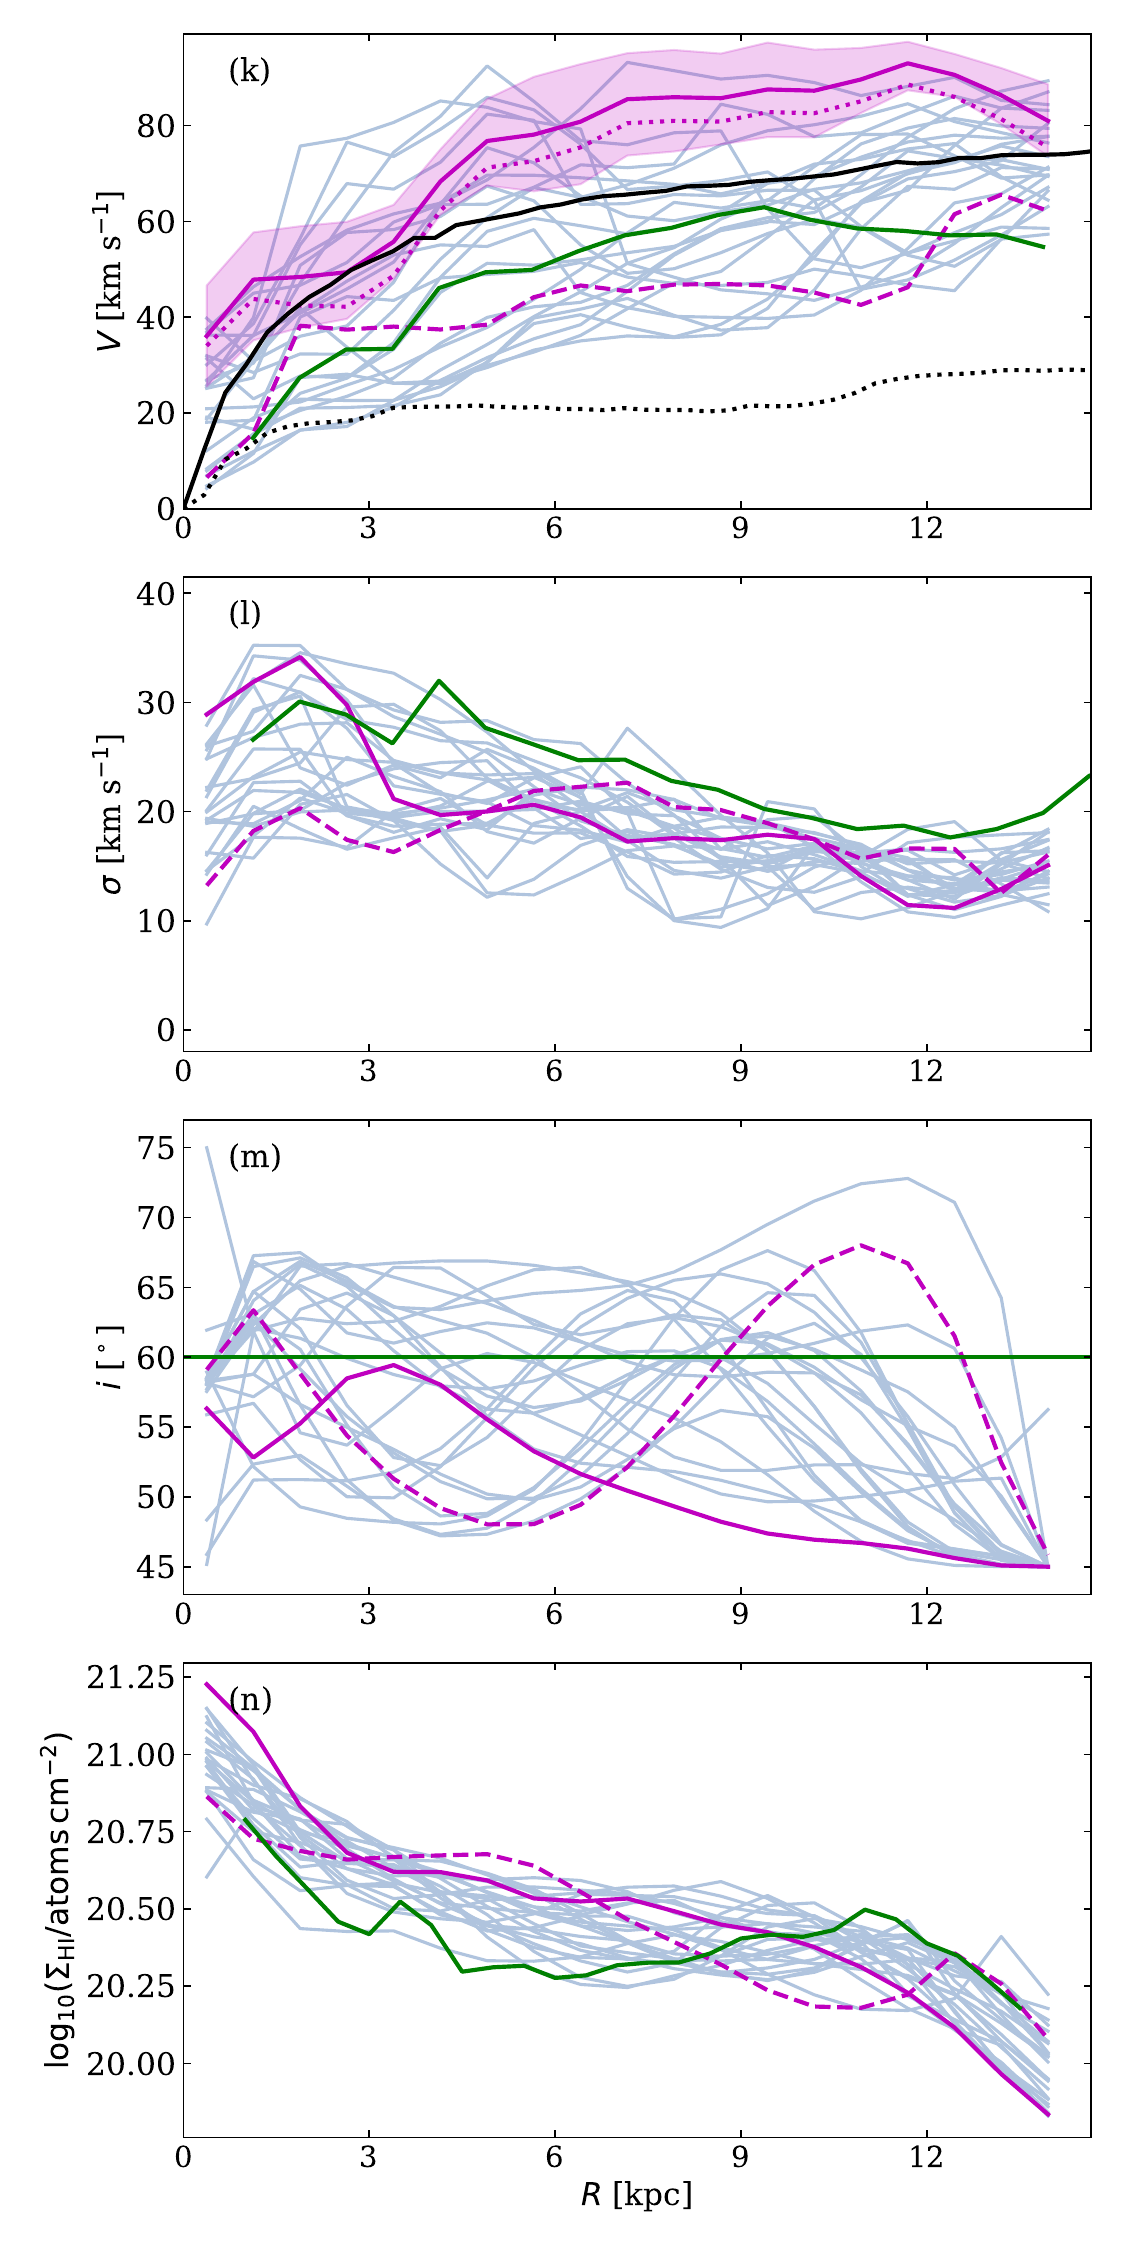}
\end{minipage}
\caption{A set of summary figures for galaxy LT-29, selected for kinematic analysis. These include example moment maps for two orientations (panels (a)--(f); similar to Fig.~\ref{fig:visualisations}), a summary of the parameters $V_\mathrm{fid}$, $V_\mathrm{max}$, $\eta_\mathrm{rot}$, and $\eta_\mathrm{bar}$ (panels (g)--(j); similar to Fig.~\ref{fig:loops}), and a summary of the rotation curve analysis from $24$ viewing angles (panels (k)--(n); similar to Fig.~\ref{fig:rot_curves}). See description of Appendix~\ref{app:supplementary} for details.}
\label{fig:S10}
\end{figure}
\clearpage

\begin{figure}
\begin{minipage}{.9\textwidth}
\includegraphics[width=\textwidth]{../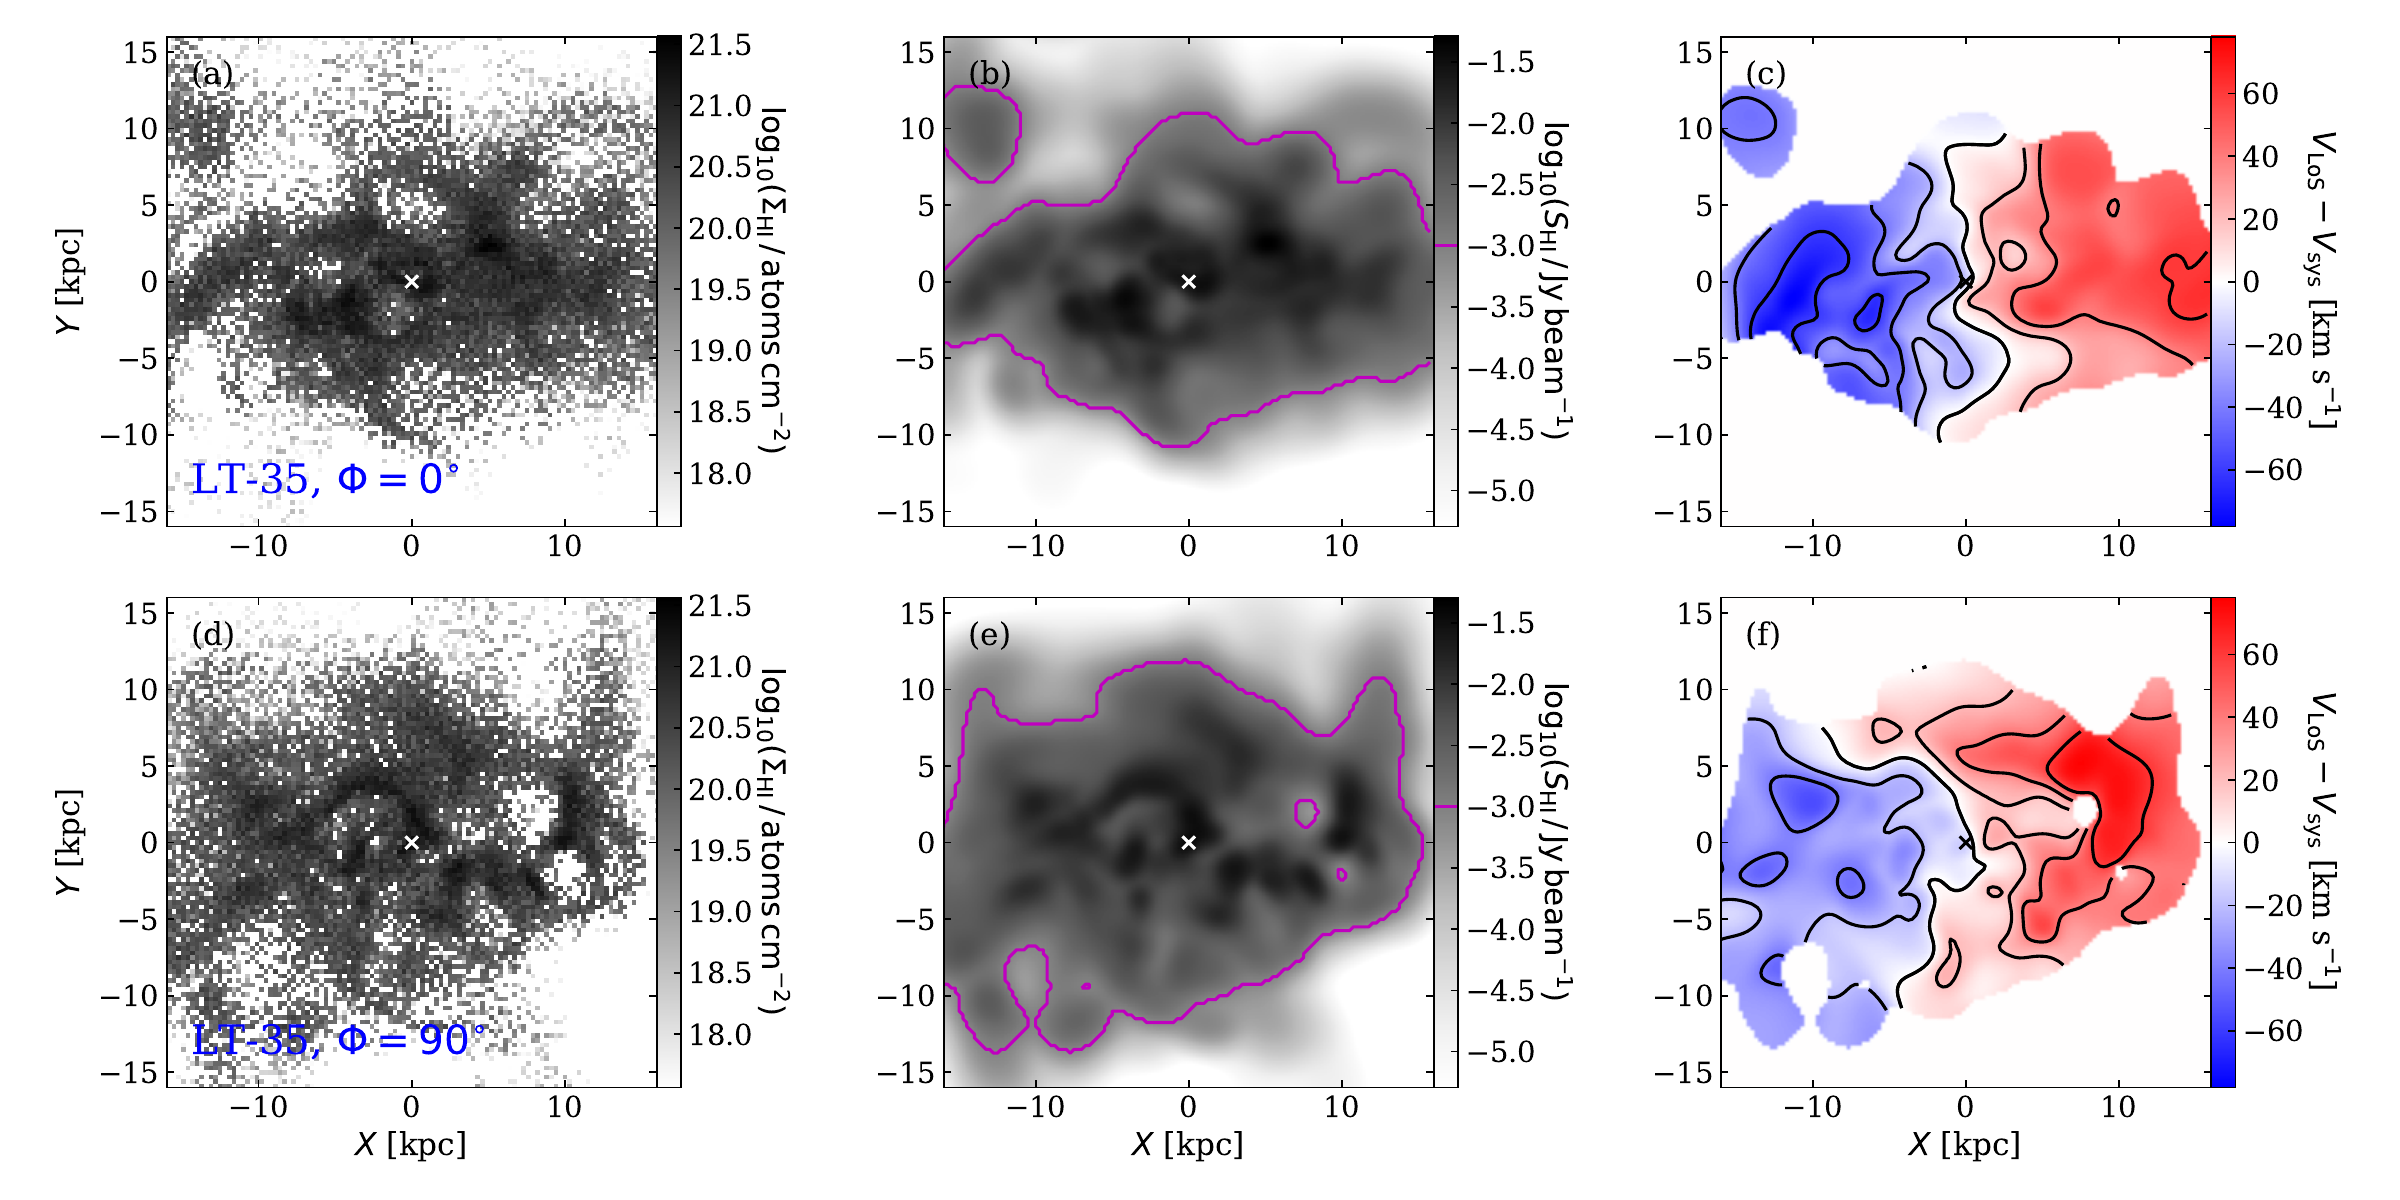}
\includegraphics[width=\textwidth]{../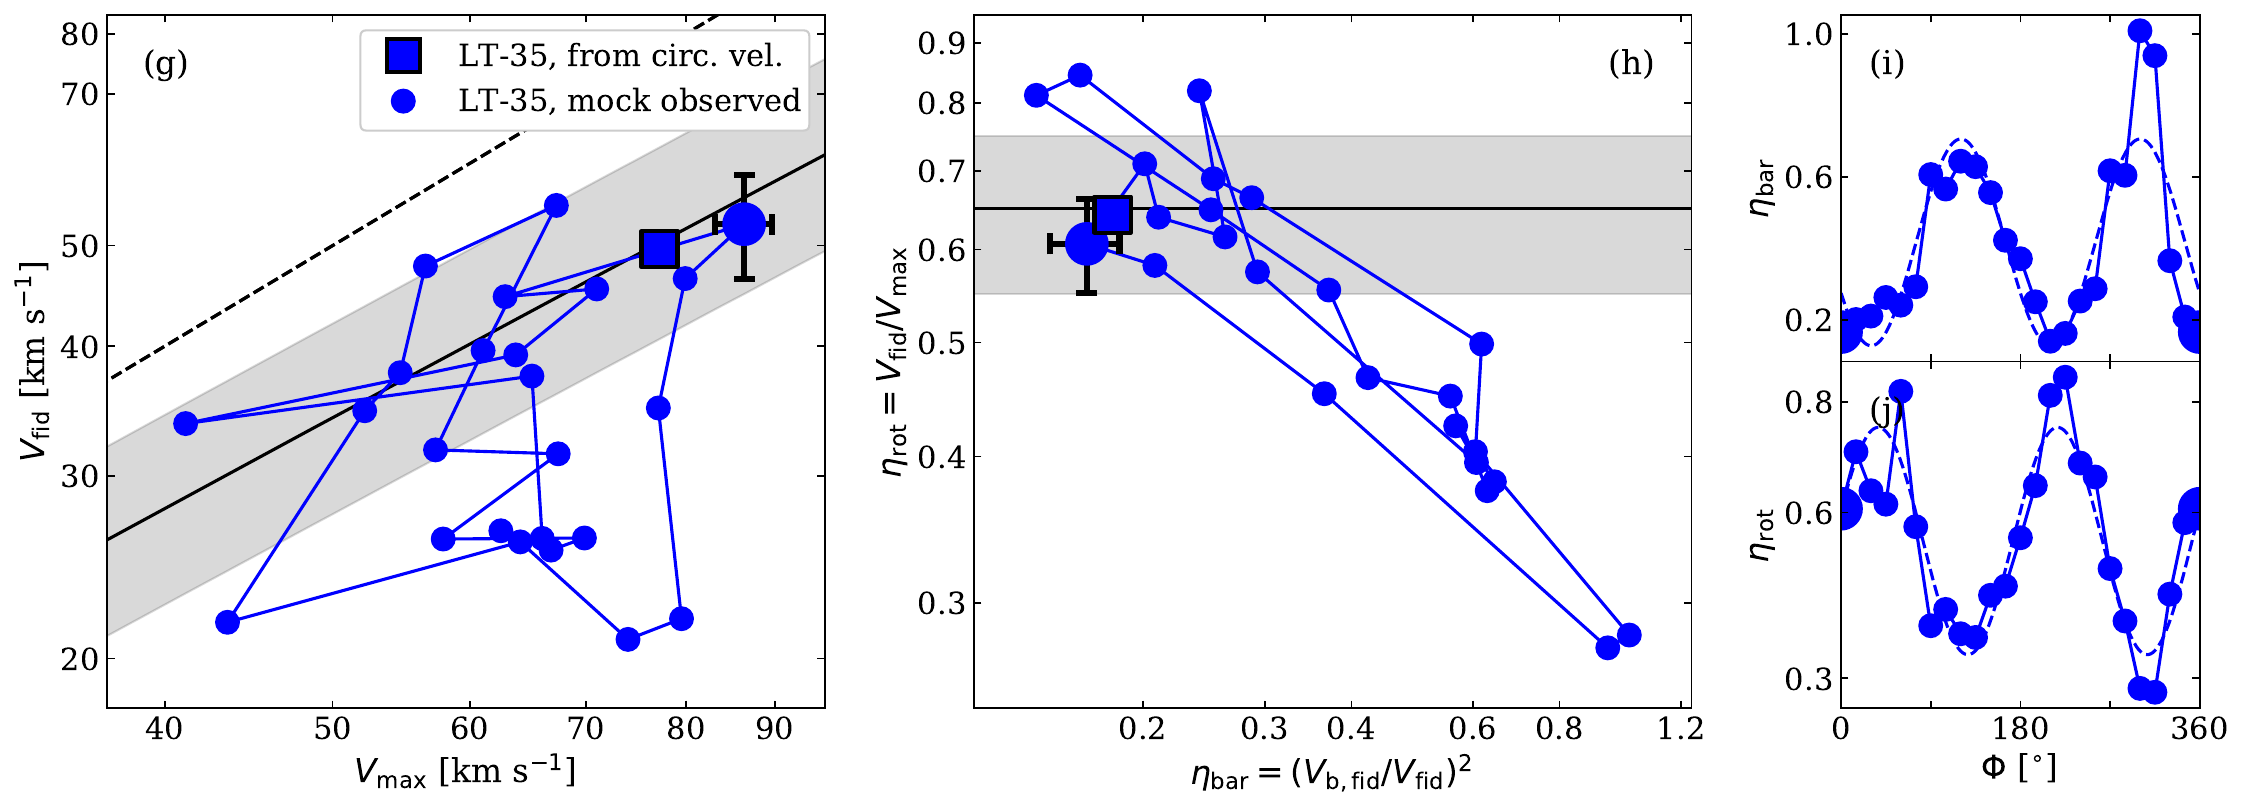}
\end{minipage}
\begin{minipage}{.4\textwidth}
\includegraphics[width=\textwidth]{../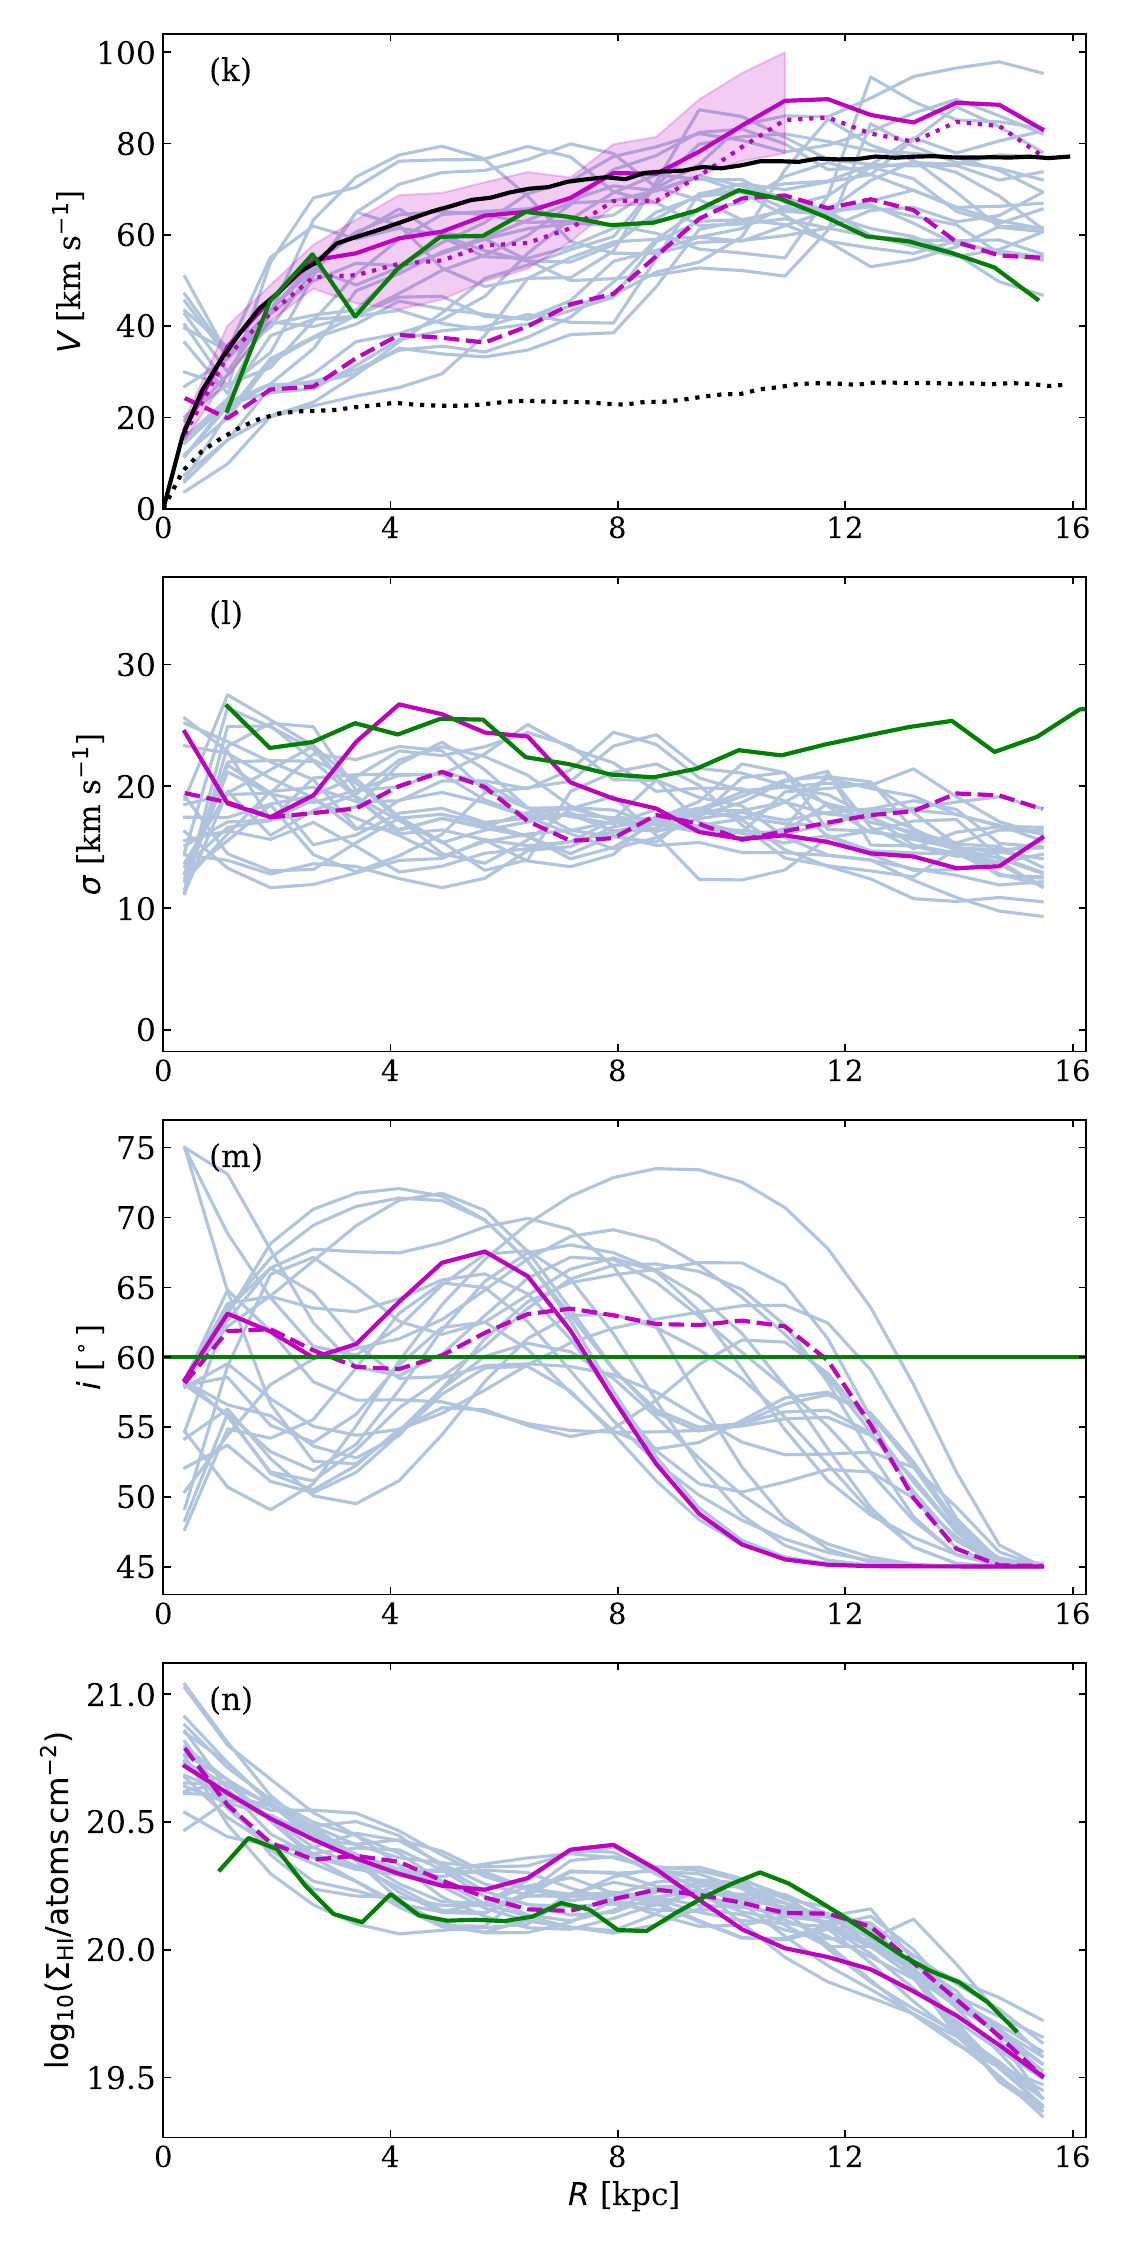}
\end{minipage}
\caption{A set of summary figures for galaxy LT-35, selected for kinematic analysis. These include example moment maps for two orientations (panels (a)--(f); similar to Fig.~\ref{fig:visualisations}), a summary of the parameters $V_\mathrm{fid}$, $V_\mathrm{max}$, $\eta_\mathrm{rot}$, and $\eta_\mathrm{bar}$ (panels (g)--(j); similar to Fig.~\ref{fig:loops}), and a summary of the rotation curve analysis from $24$ viewing angles (panels (k)--(n); similar to Fig.~\ref{fig:rot_curves}). See description of Appendix~\ref{app:supplementary} for details.}
\label{fig:S11}
\end{figure}
\clearpage

\begin{figure}
\begin{minipage}{.9\textwidth}
\includegraphics[width=\textwidth]{../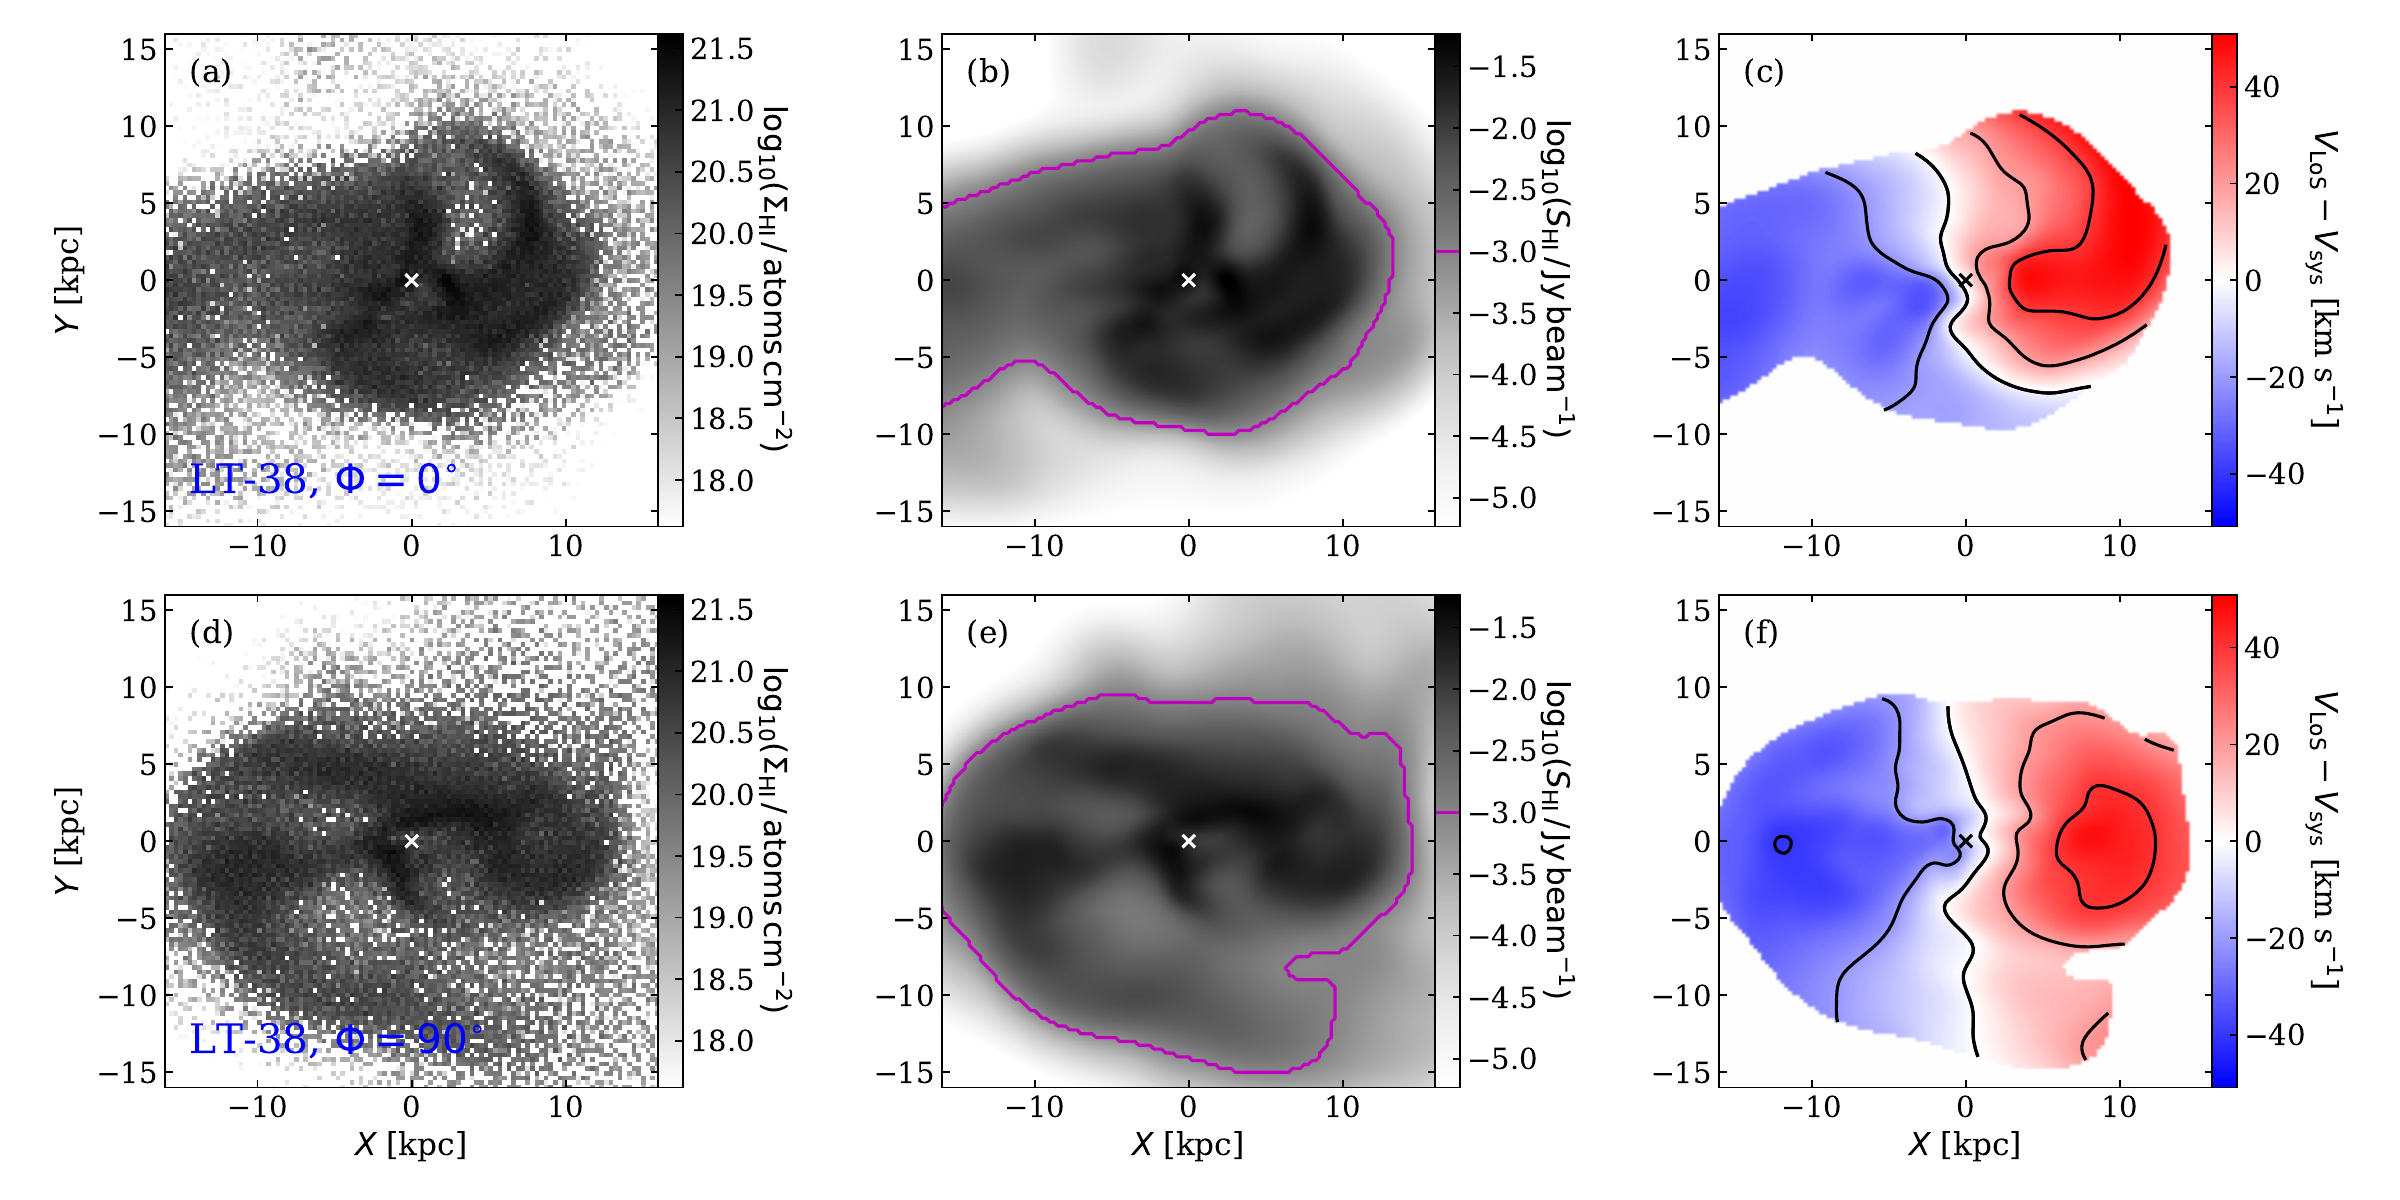}
\includegraphics[width=\textwidth]{../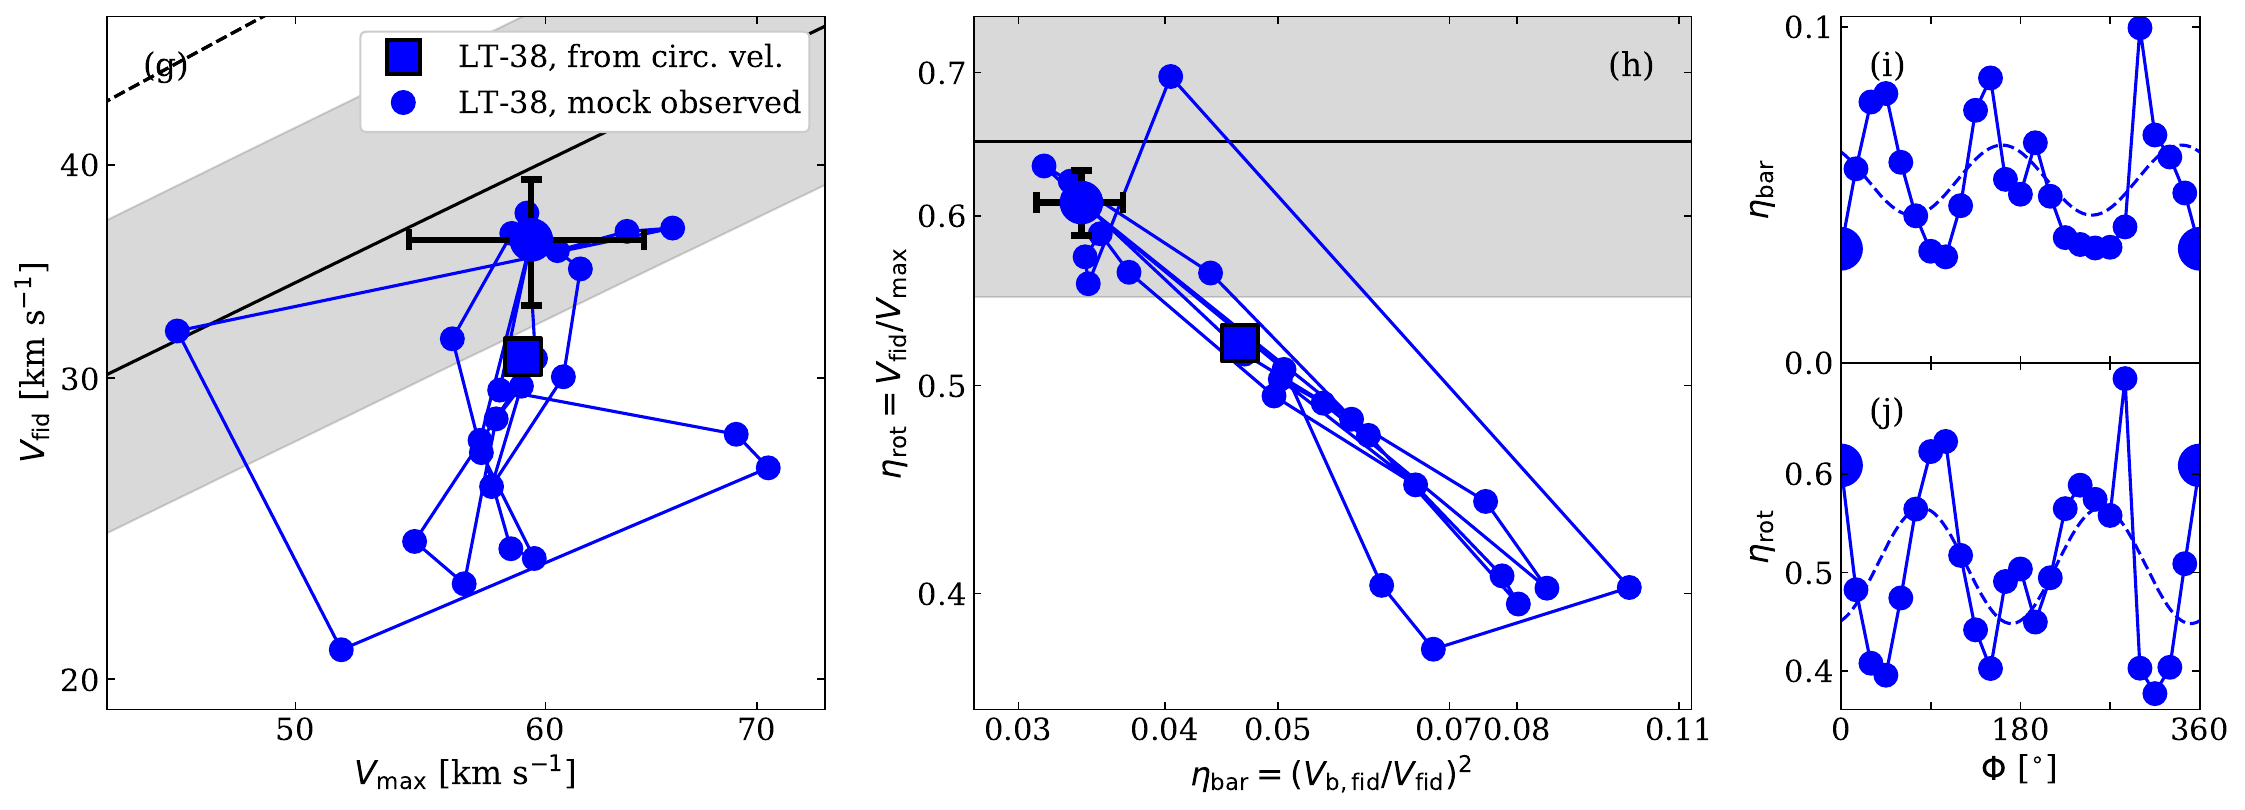}
\end{minipage}
\begin{minipage}{.4\textwidth}
\includegraphics[width=\textwidth]{../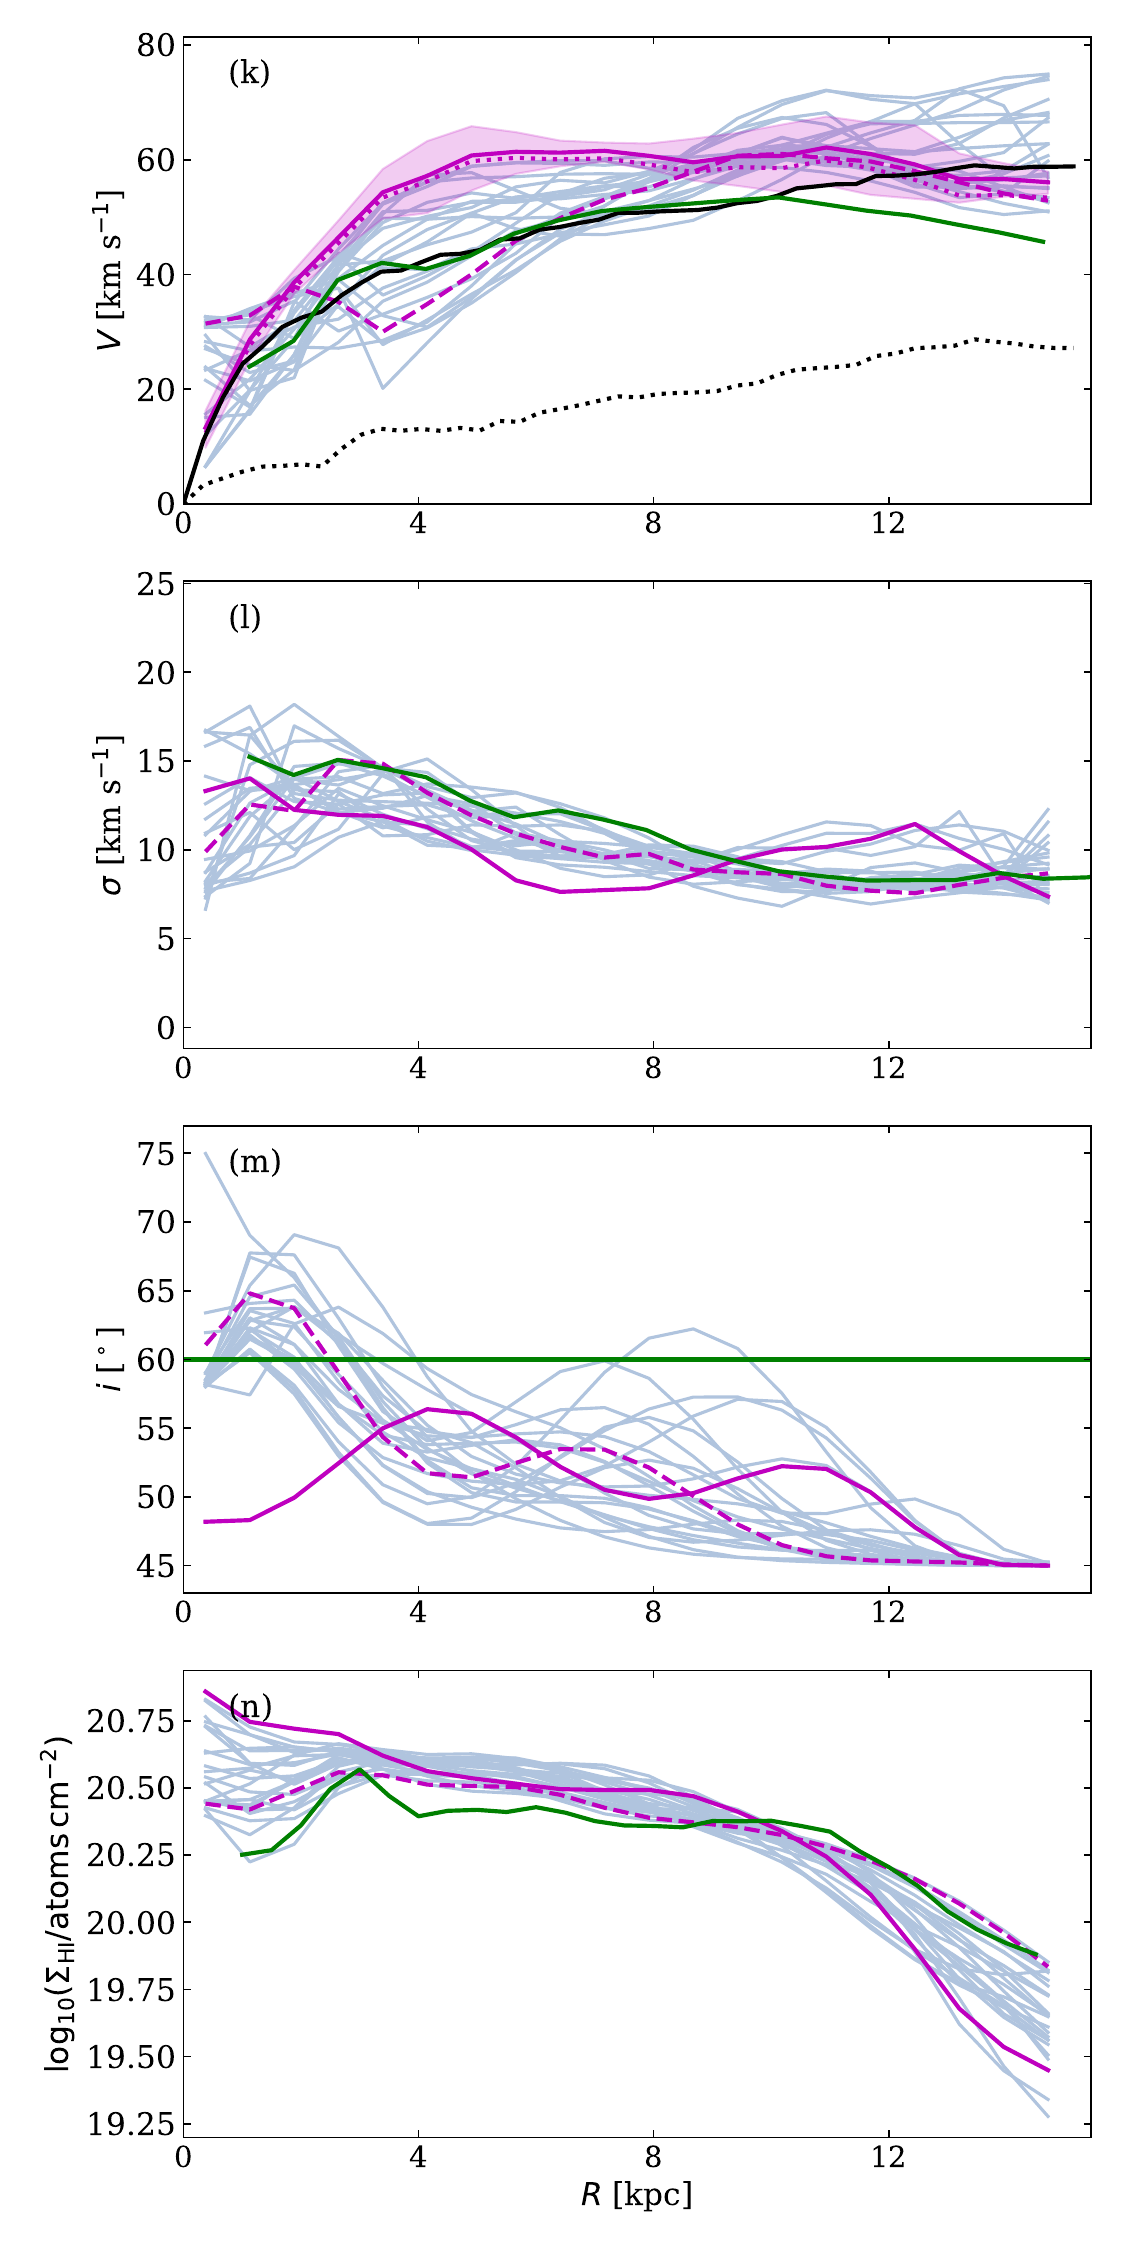}
\end{minipage}
\caption{A set of summary figures for galaxy LT-38, selected for kinematic analysis. These include example moment maps for two orientations (panels (a)--(f); similar to Fig.~\ref{fig:visualisations}), a summary of the parameters $V_\mathrm{fid}$, $V_\mathrm{max}$, $\eta_\mathrm{rot}$, and $\eta_\mathrm{bar}$ (panels (g)--(j); similar to Fig.~\ref{fig:loops}), and a summary of the rotation curve analysis from $24$ viewing angles (panels (k)--(n); similar to Fig.~\ref{fig:rot_curves}). See description of Appendix~\ref{app:supplementary} for details.}
\label{fig:S12}
\end{figure}
\clearpage

\begin{figure}
\begin{minipage}{.9\textwidth}
\includegraphics[width=\textwidth]{../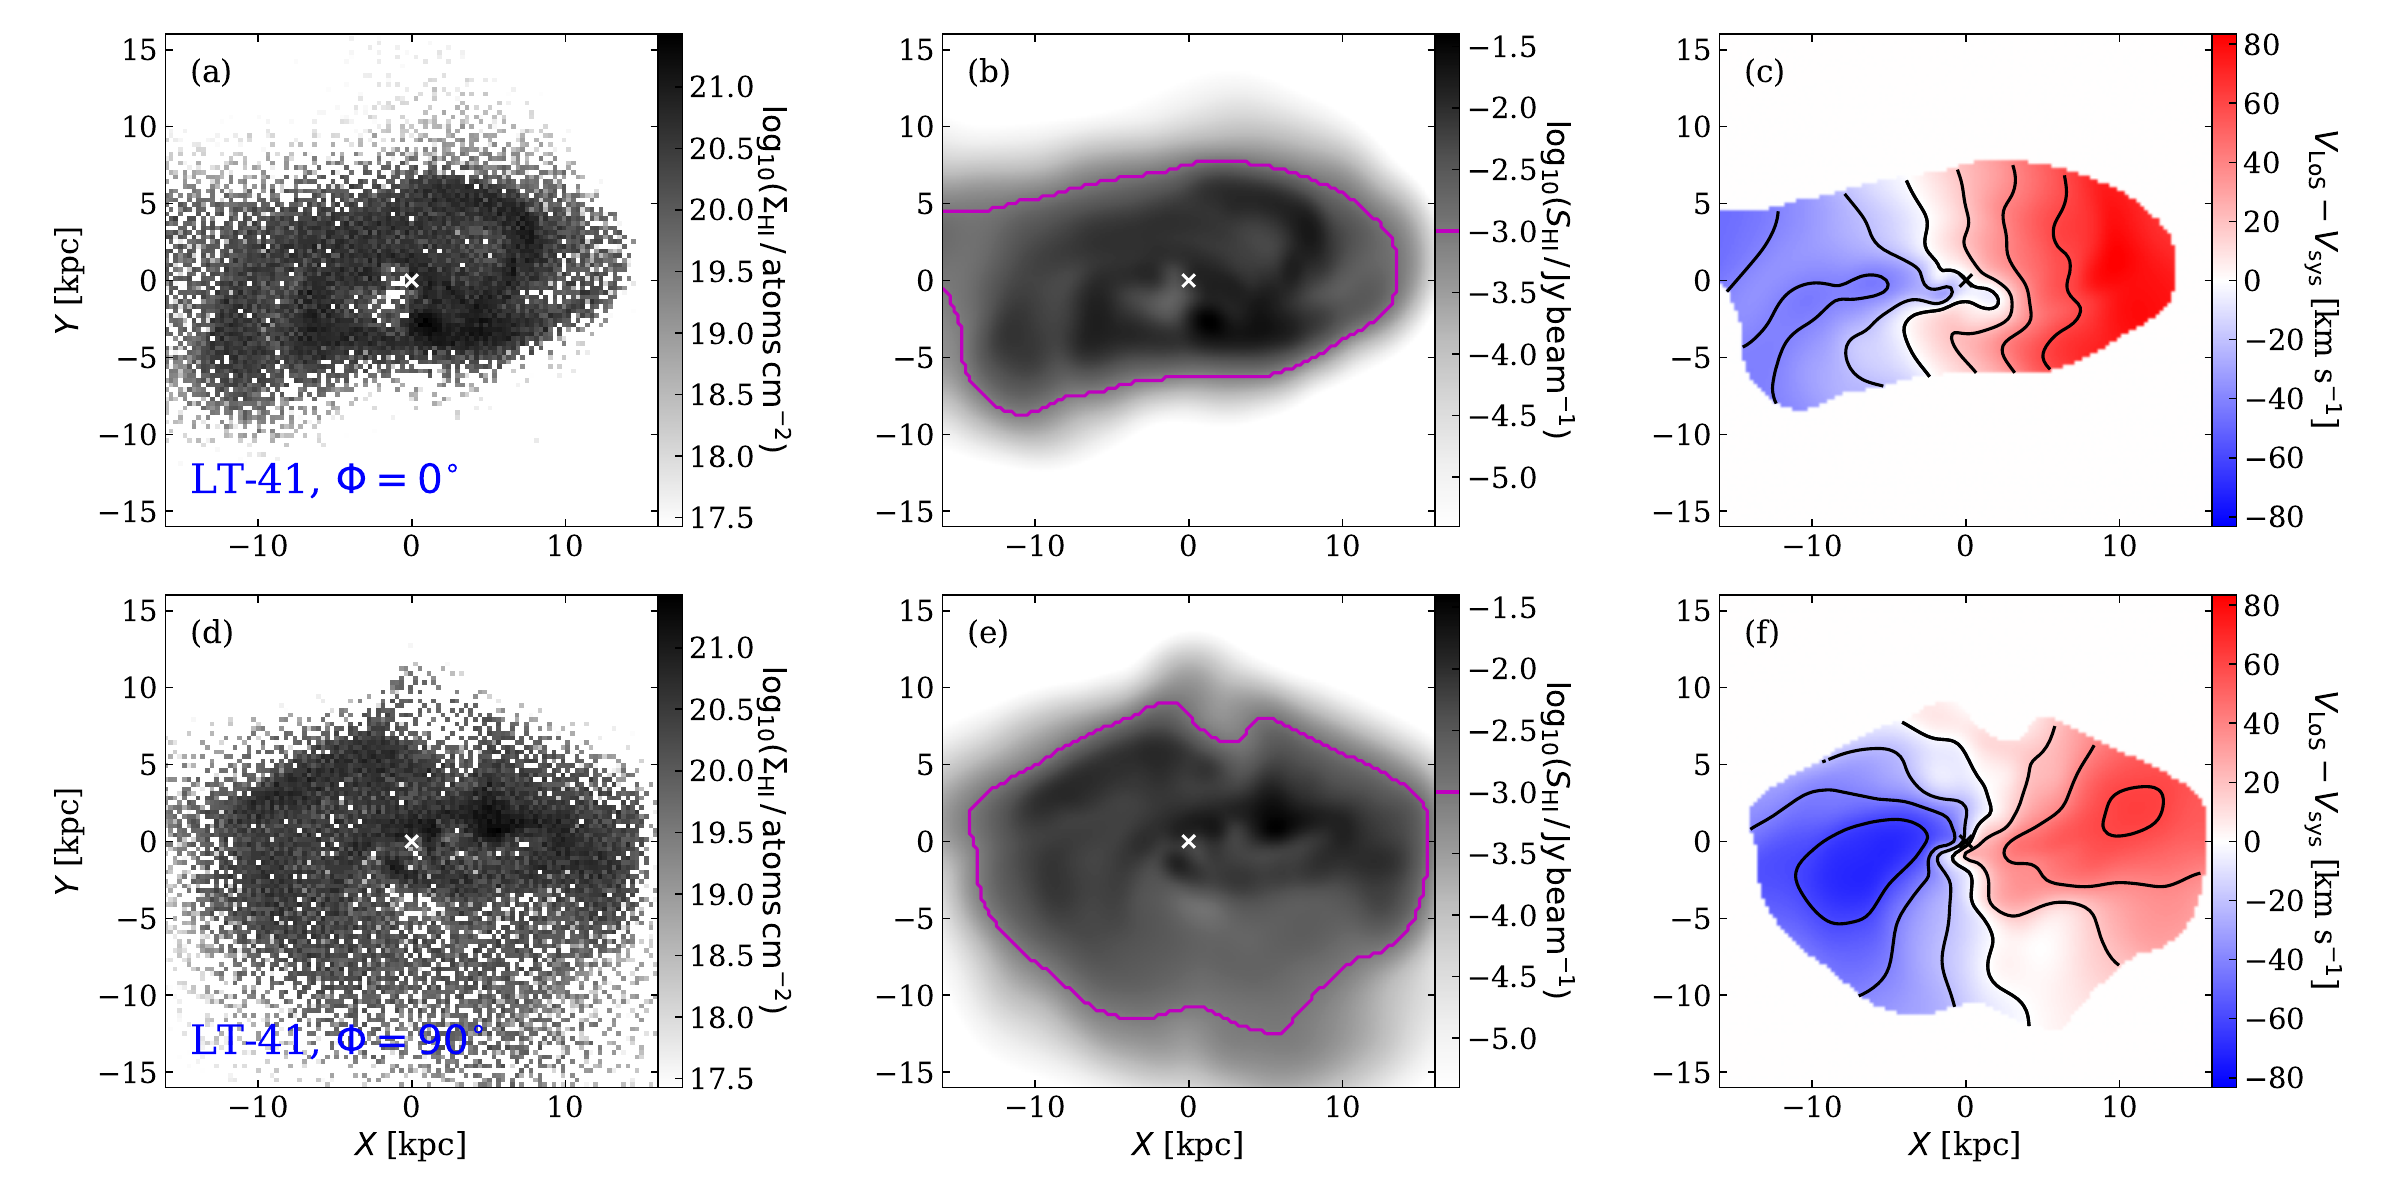}
\includegraphics[width=\textwidth]{../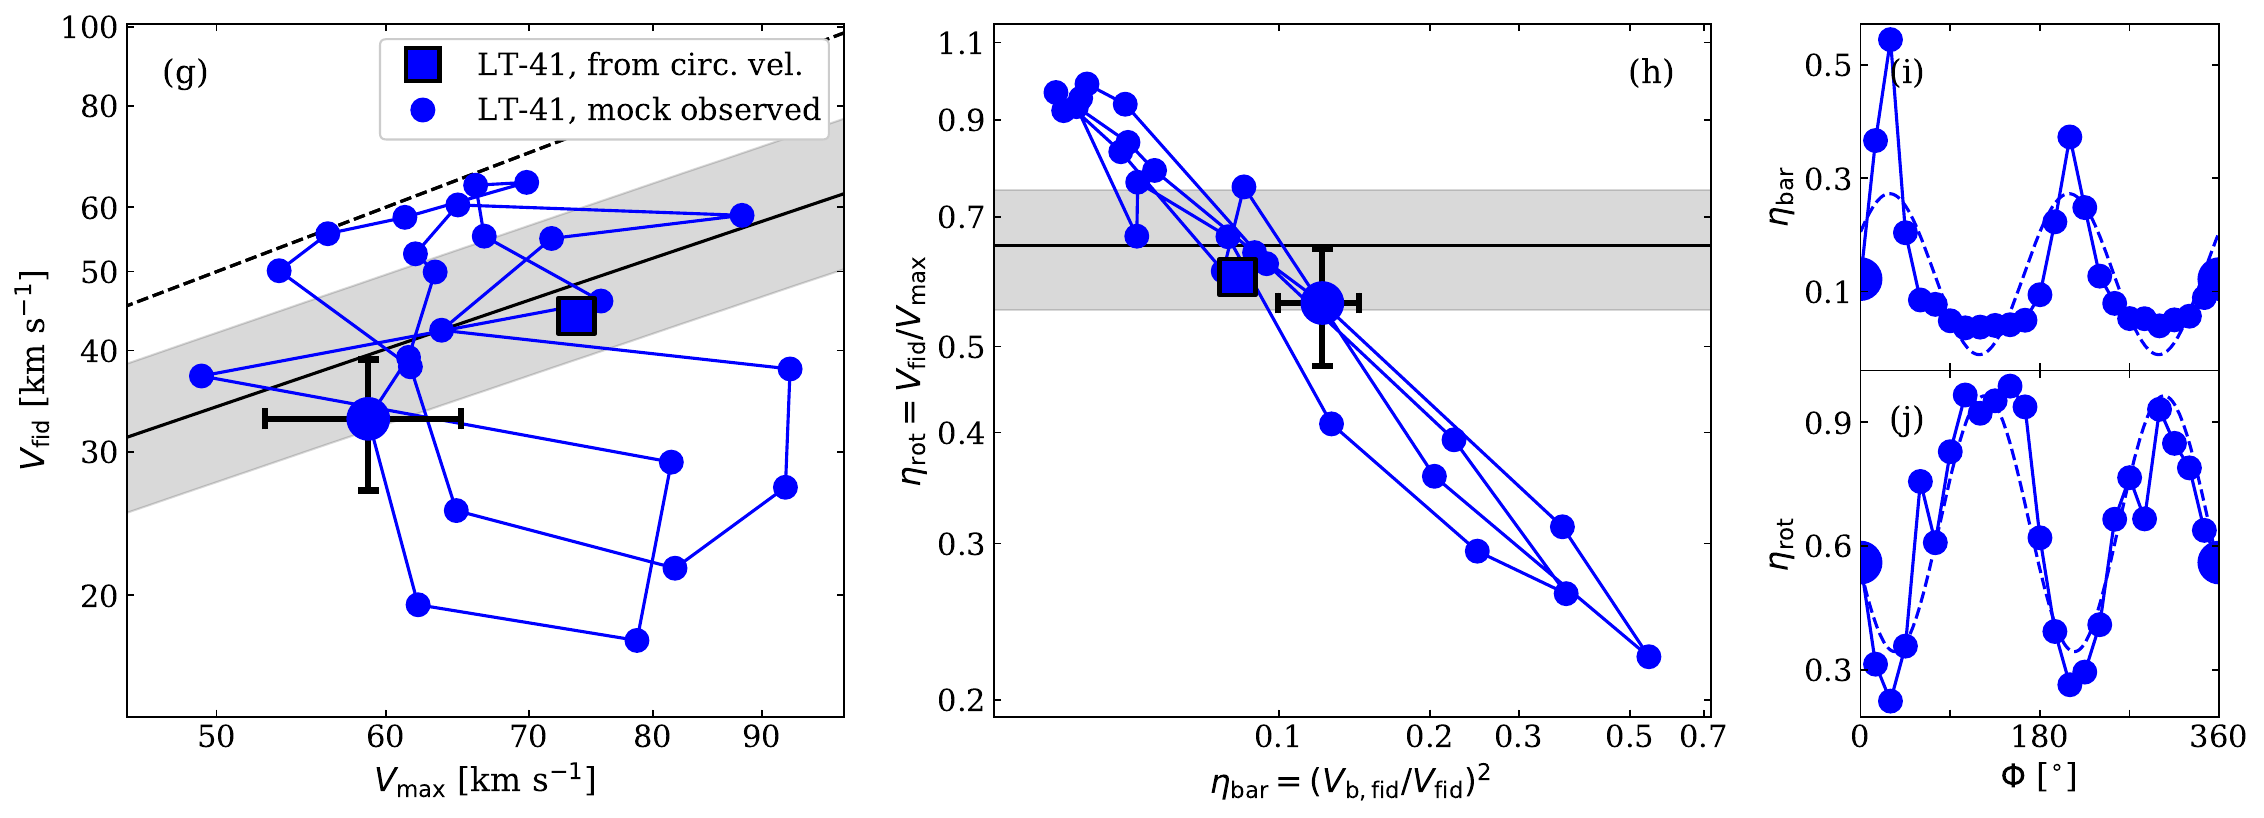}
\end{minipage}
\begin{minipage}{.4\textwidth}
\includegraphics[width=\textwidth]{../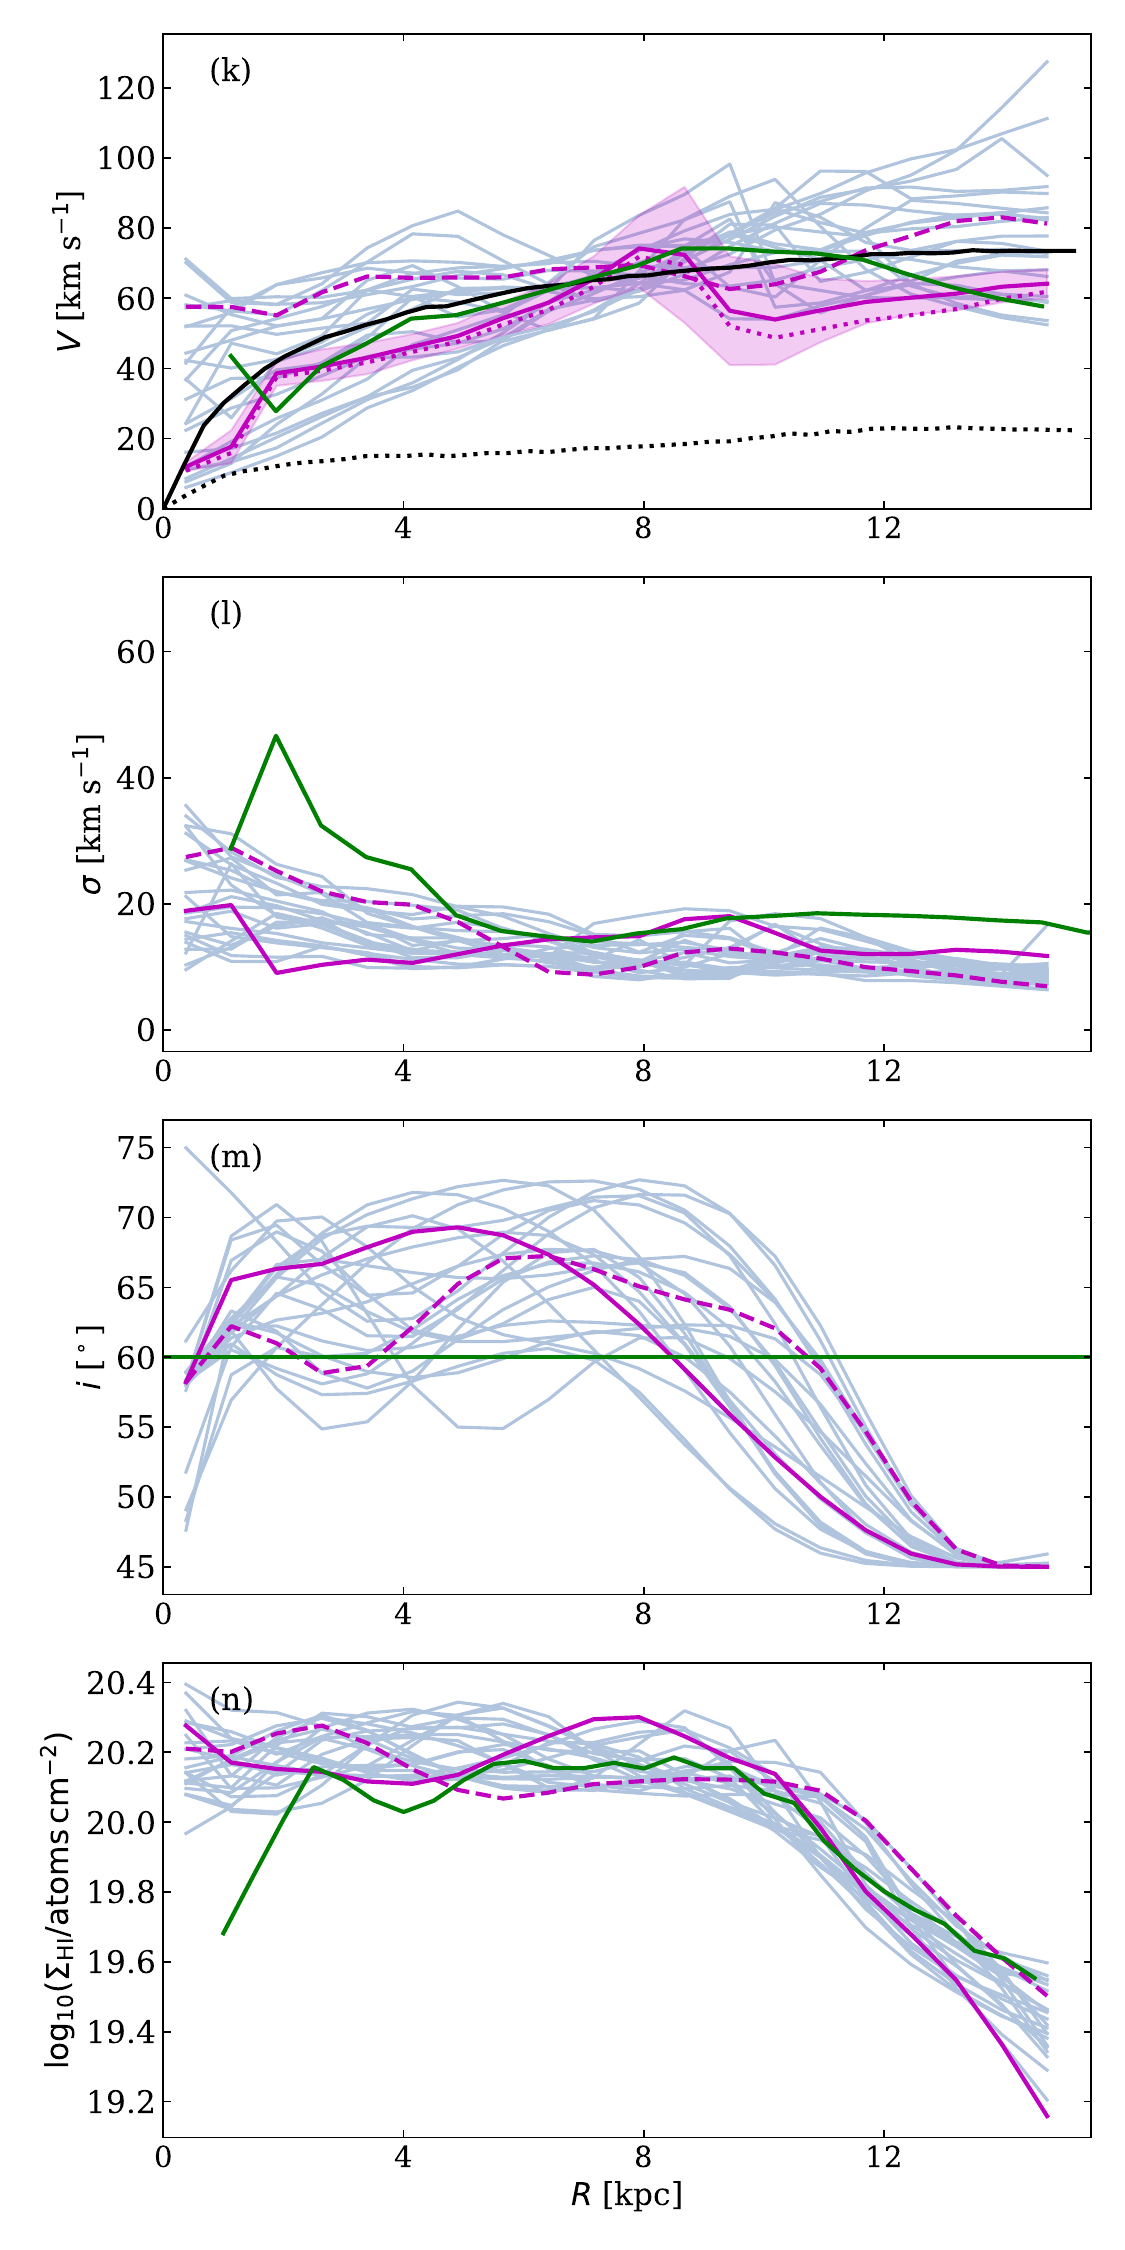}
\end{minipage}
\caption{A set of summary figures for galaxy LT-41, selected for kinematic analysis. These include example moment maps for two orientations (panels (a)--(f); similar to Fig.~\ref{fig:visualisations}), a summary of the parameters $V_\mathrm{fid}$, $V_\mathrm{max}$, $\eta_\mathrm{rot}$, and $\eta_\mathrm{bar}$ (panels (g)--(j); similar to Fig.~\ref{fig:loops}), and a summary of the rotation curve analysis from $24$ viewing angles (panels (k)--(n); similar to Fig.~\ref{fig:rot_curves}). See description of Appendix~\ref{app:supplementary} for details.}
\label{fig:S13}
\end{figure}
\clearpage

\begin{figure}
\begin{minipage}{.9\textwidth}
\includegraphics[width=\textwidth]{../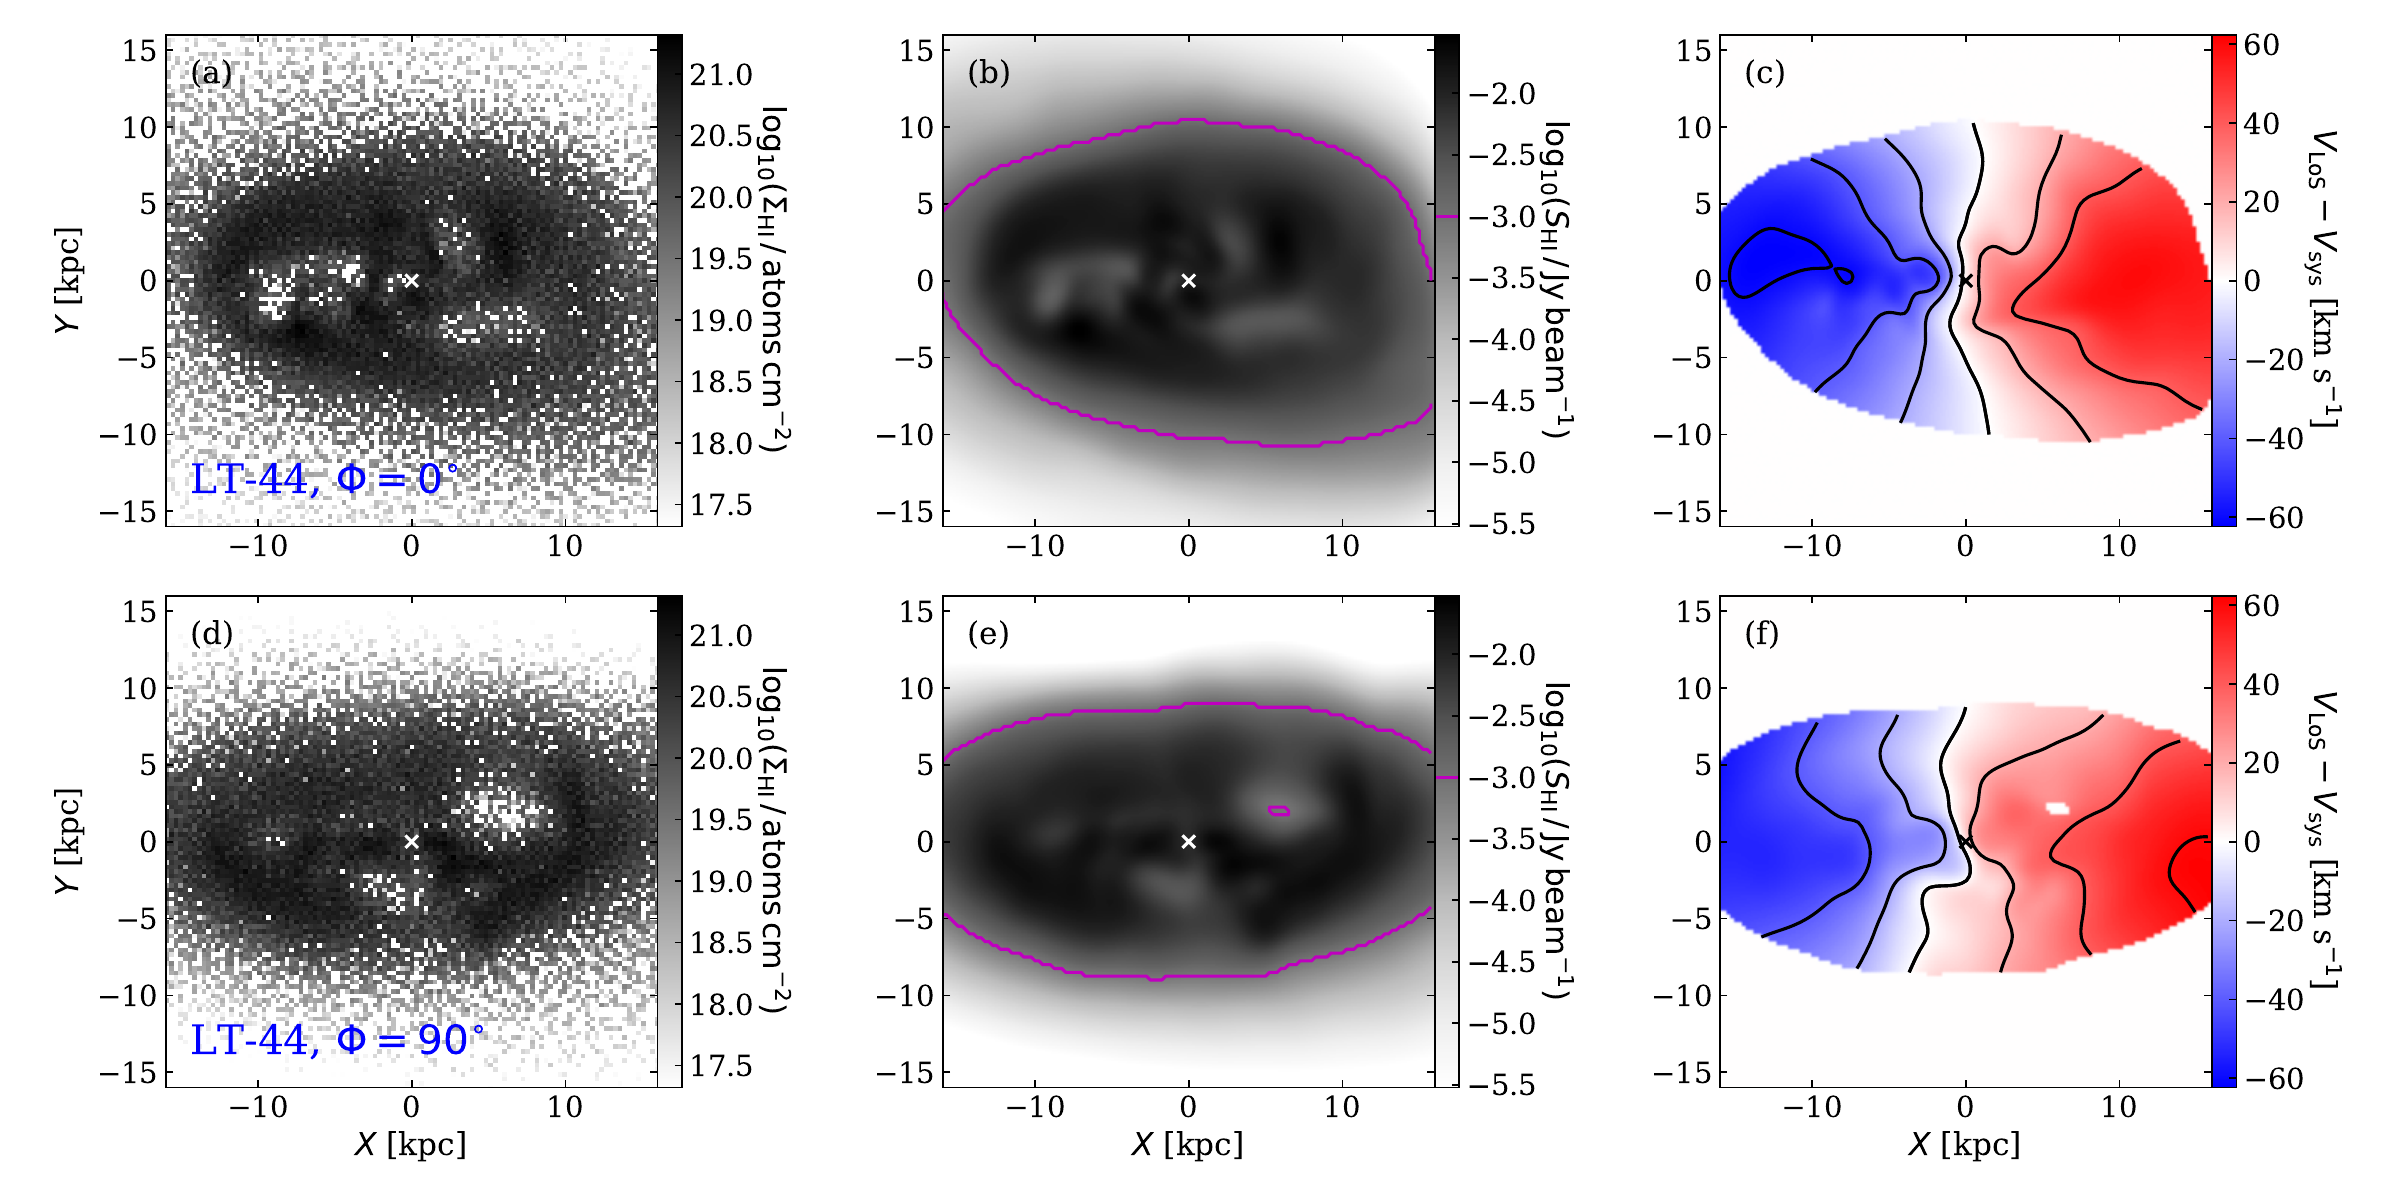}
\includegraphics[width=\textwidth]{../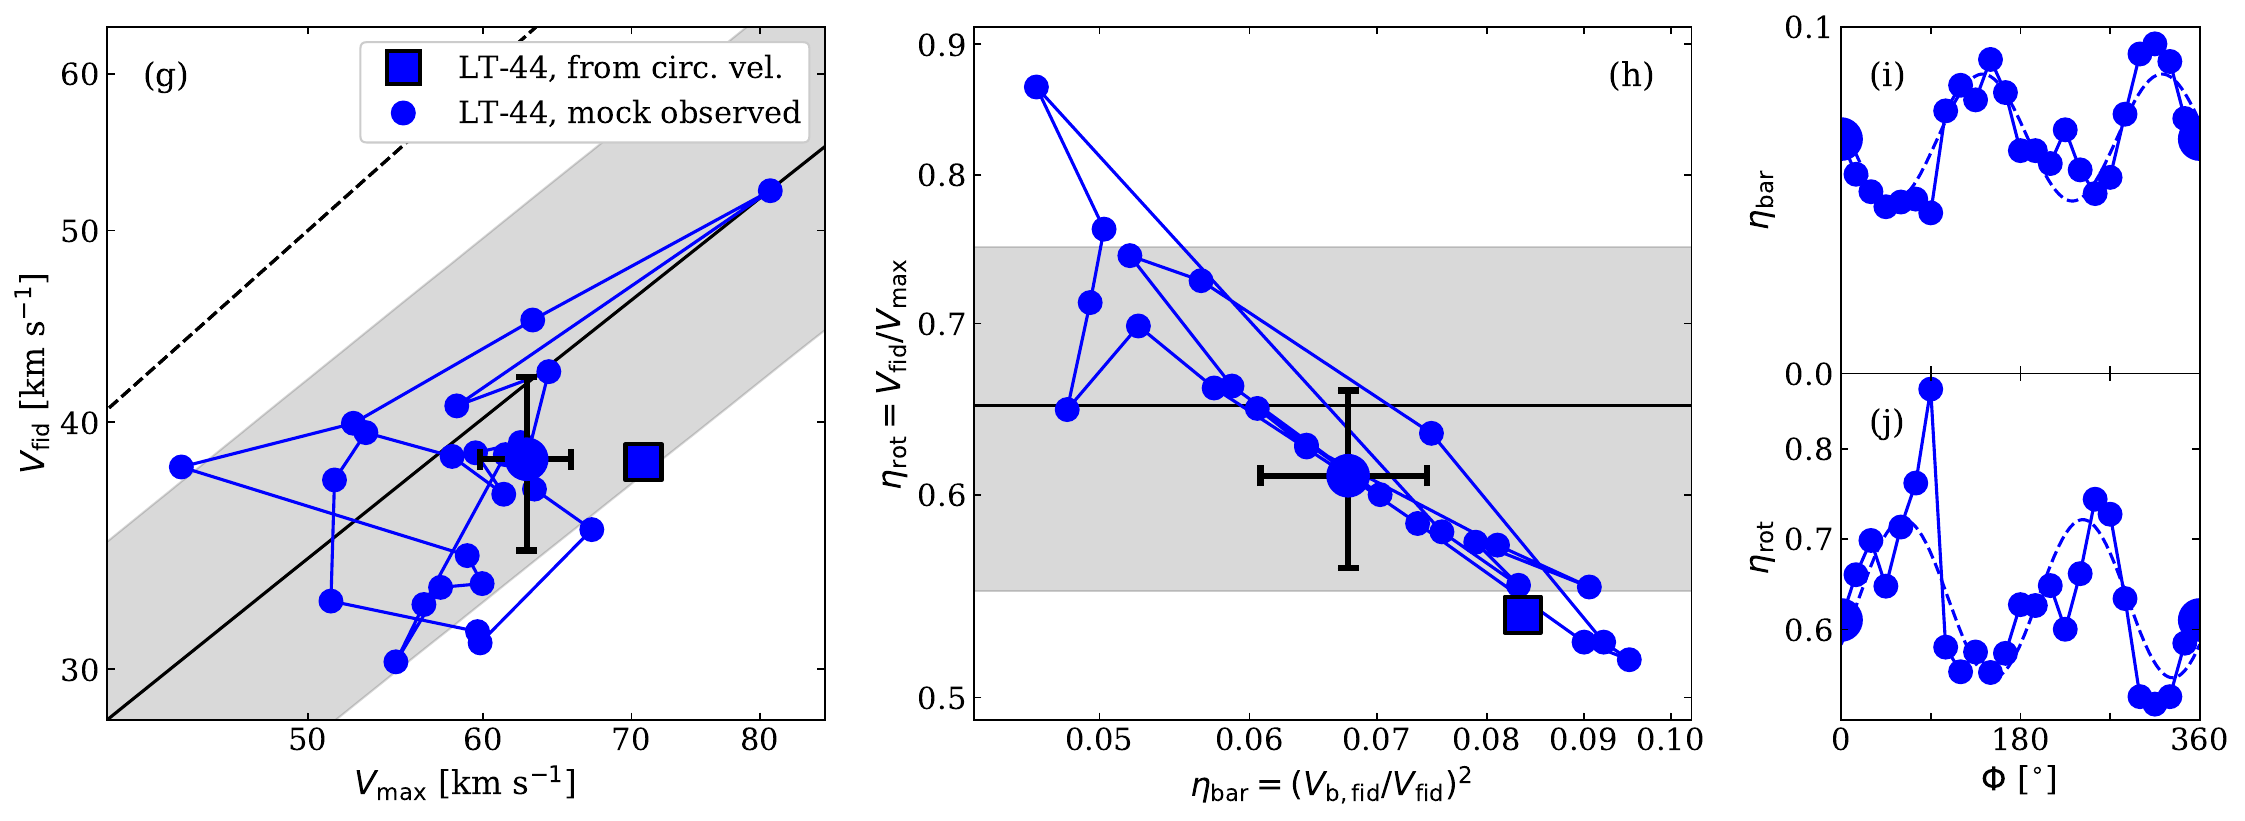}
\end{minipage}
\begin{minipage}{.4\textwidth}
\includegraphics[width=\textwidth]{../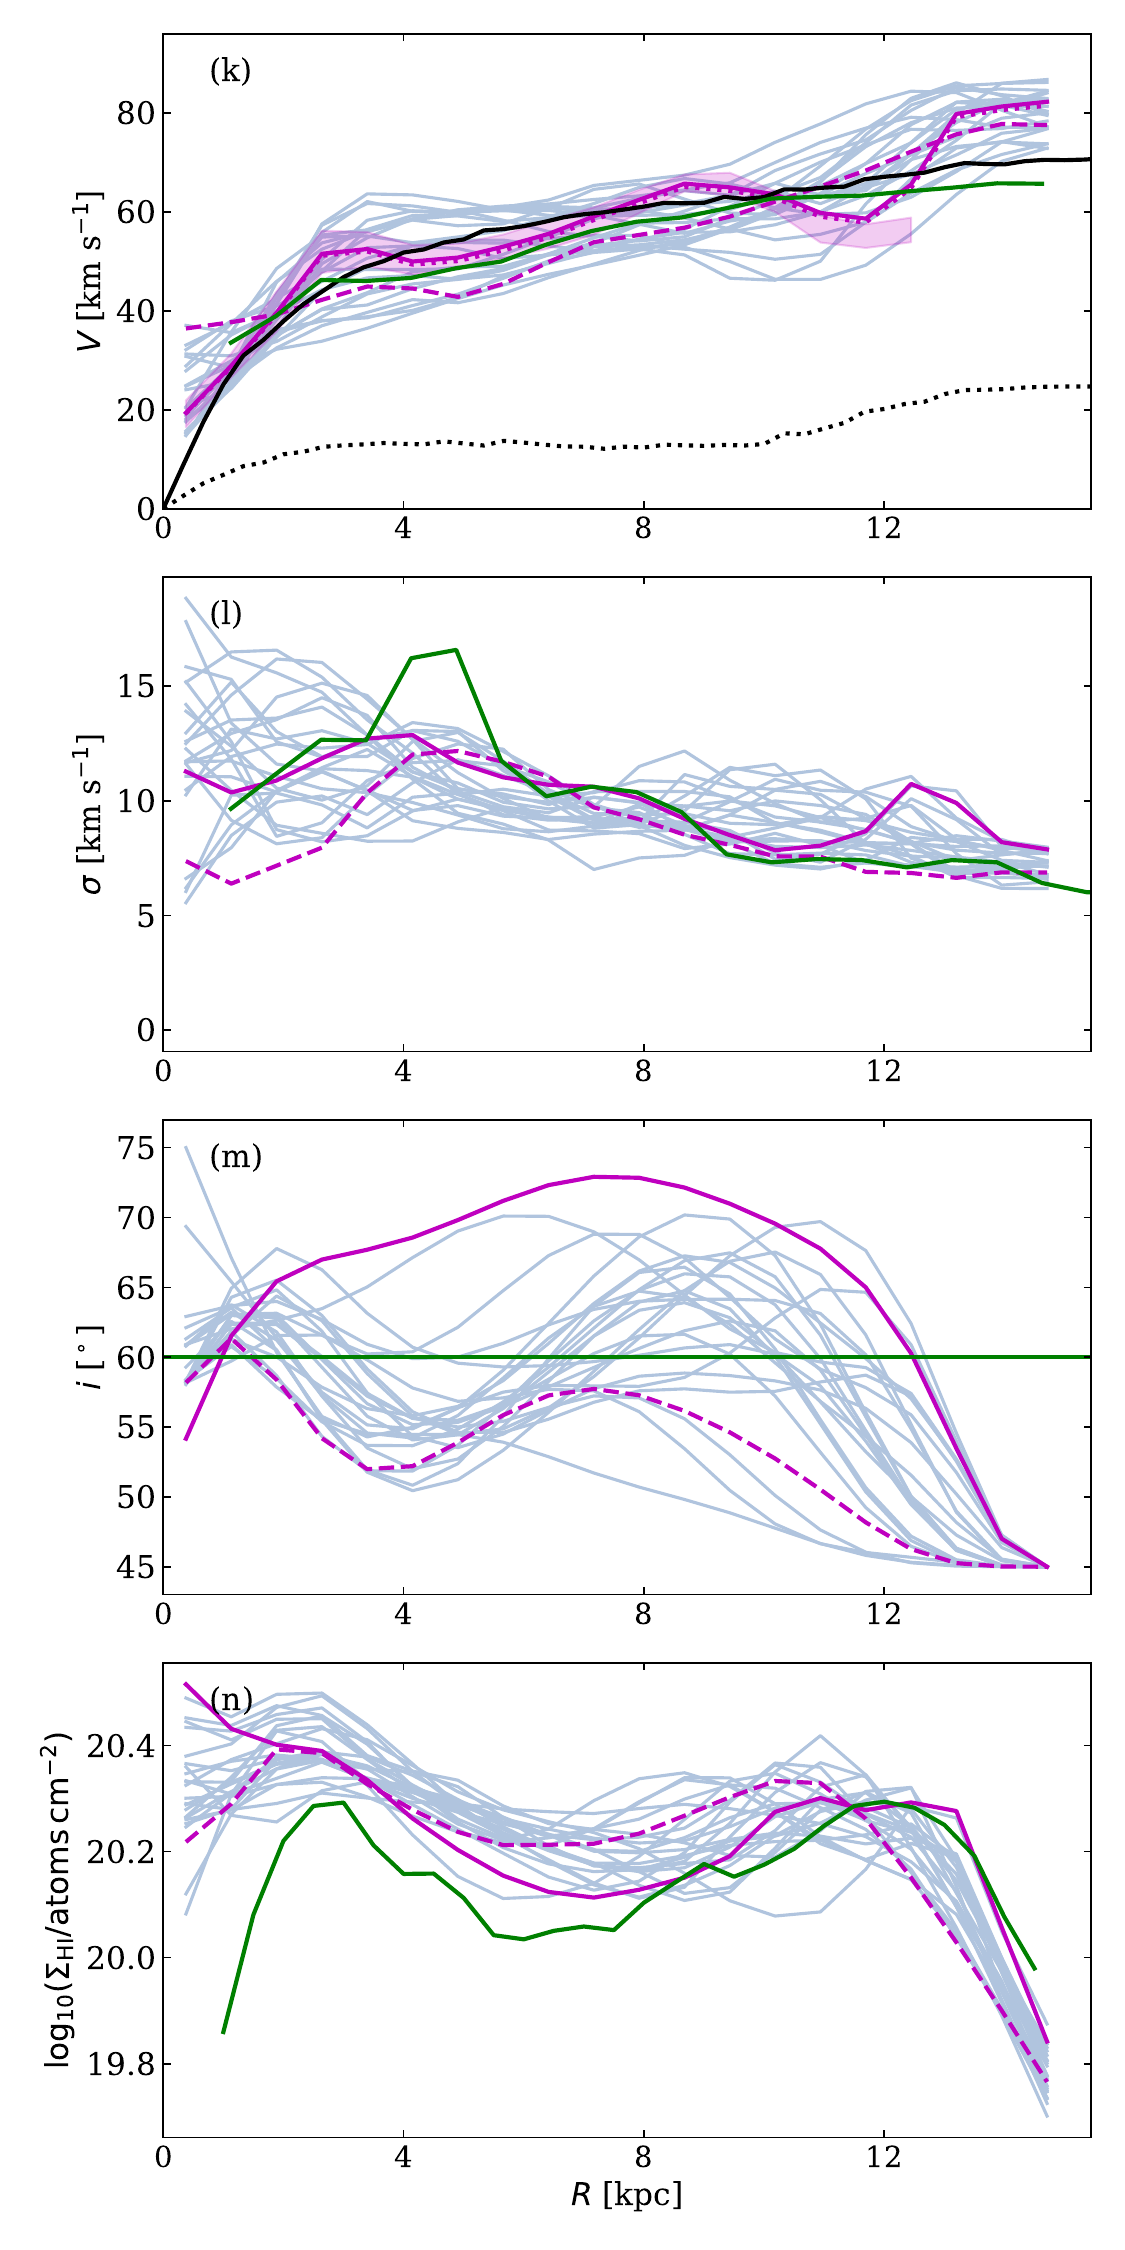}
\end{minipage}
\caption{A set of summary figures for galaxy LT-44, selected for kinematic analysis. These include example moment maps for two orientations (panels (a)--(f); similar to Fig.~\ref{fig:visualisations}), a summary of the parameters $V_\mathrm{fid}$, $V_\mathrm{max}$, $\eta_\mathrm{rot}$, and $\eta_\mathrm{bar}$ (panels (g)--(j); similar to Fig.~\ref{fig:loops}), and a summary of the rotation curve analysis from $24$ viewing angles (panels (k)--(n); similar to Fig.~\ref{fig:rot_curves}). See description of Appendix~\ref{app:supplementary} for details.}
\label{fig:S14}
\end{figure}
\clearpage

\begin{figure}
\begin{minipage}{.9\textwidth}
\includegraphics[width=\textwidth]{../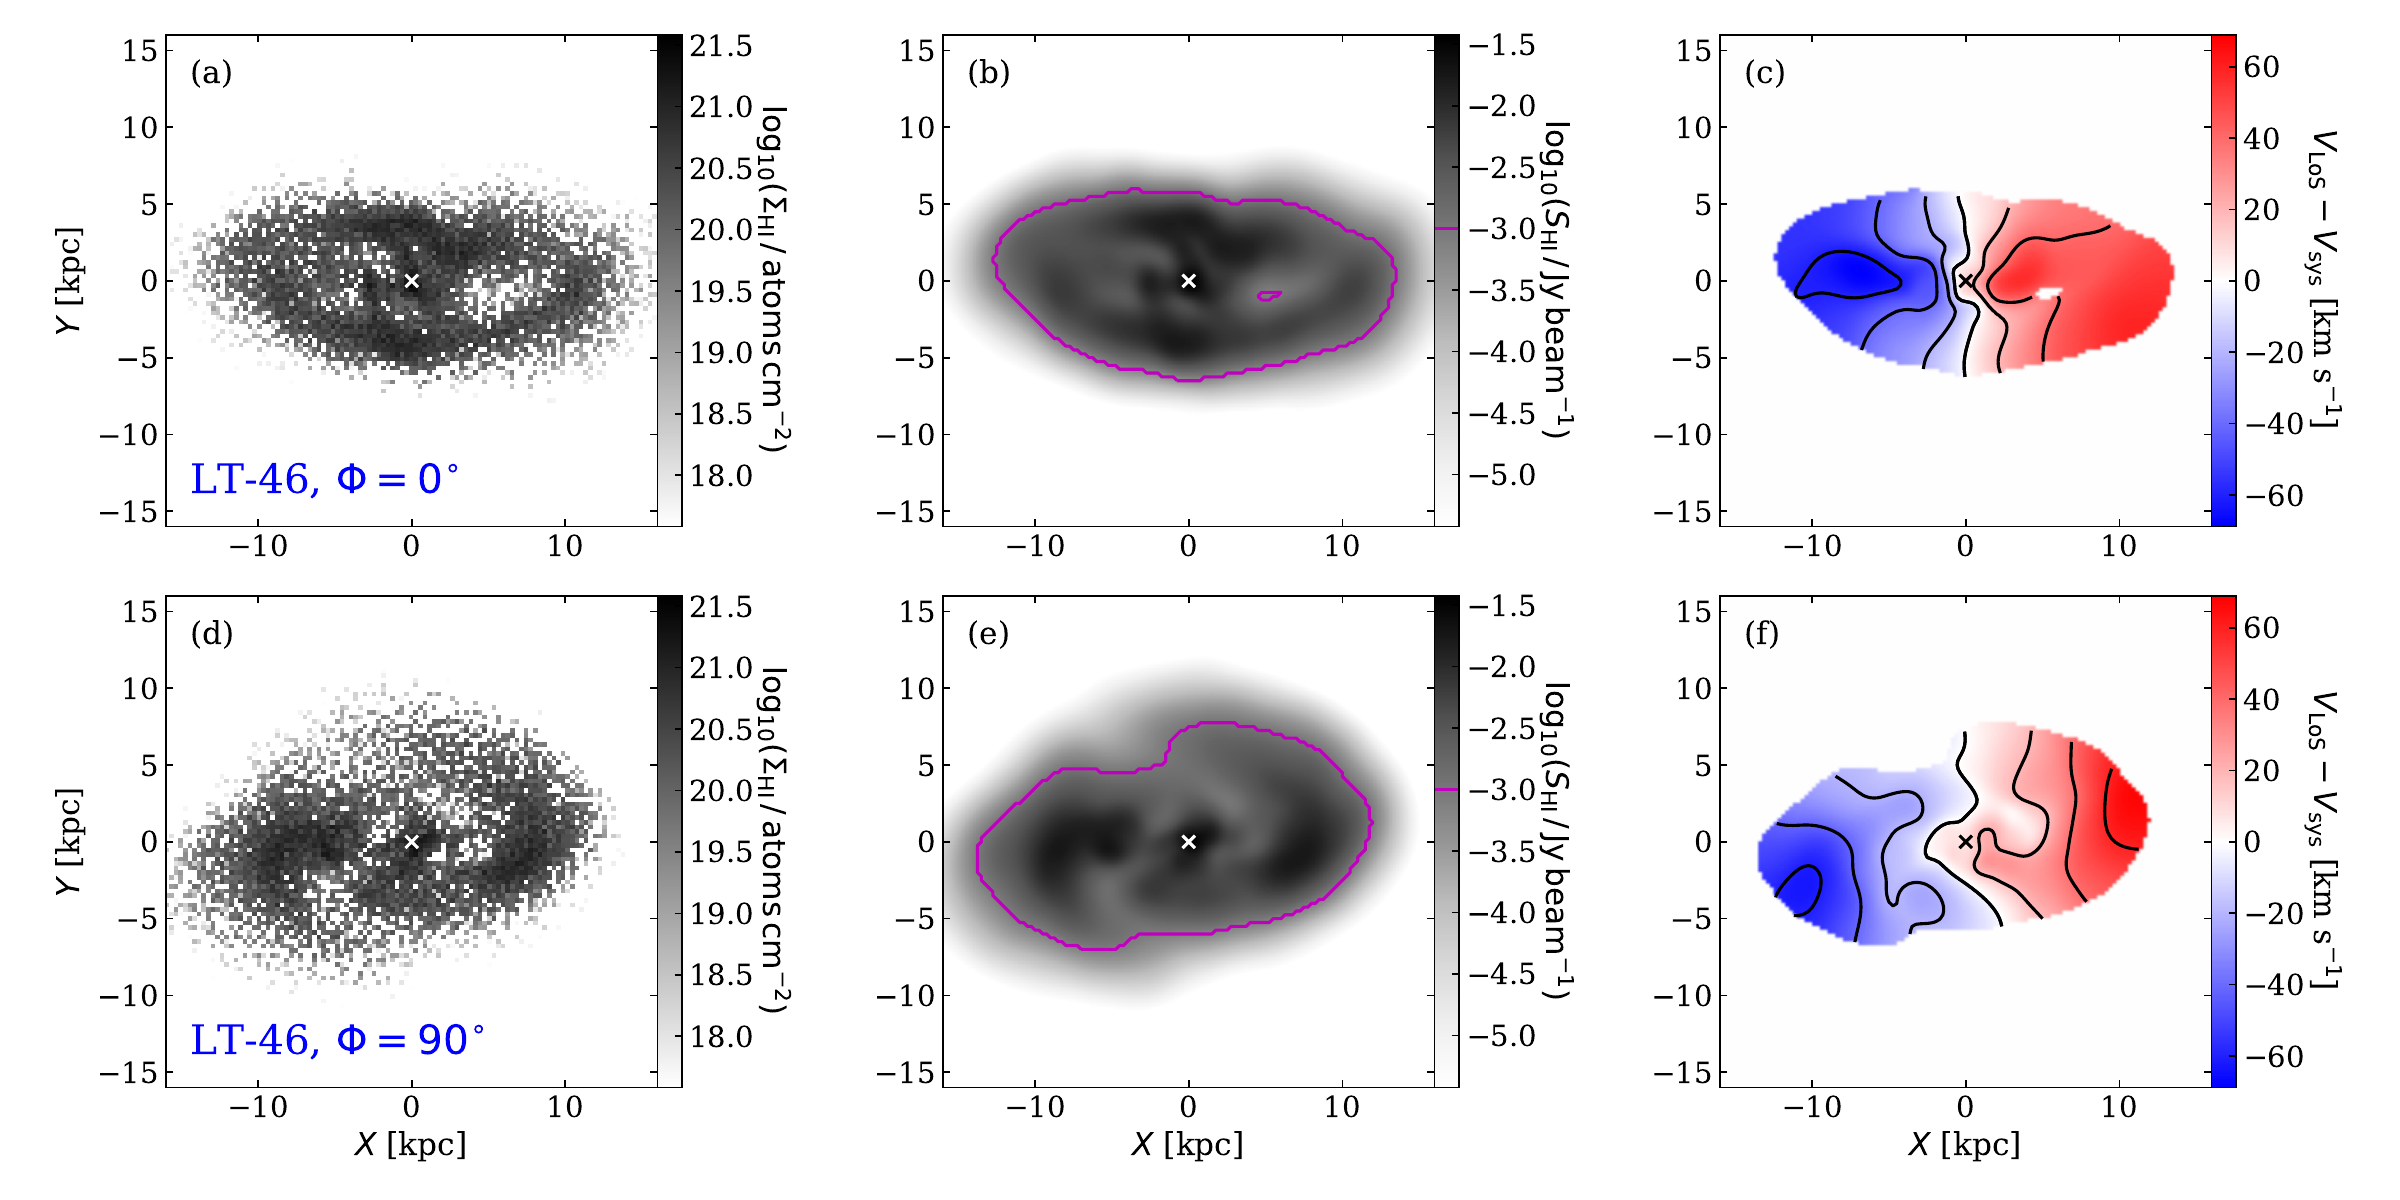}
\includegraphics[width=\textwidth]{../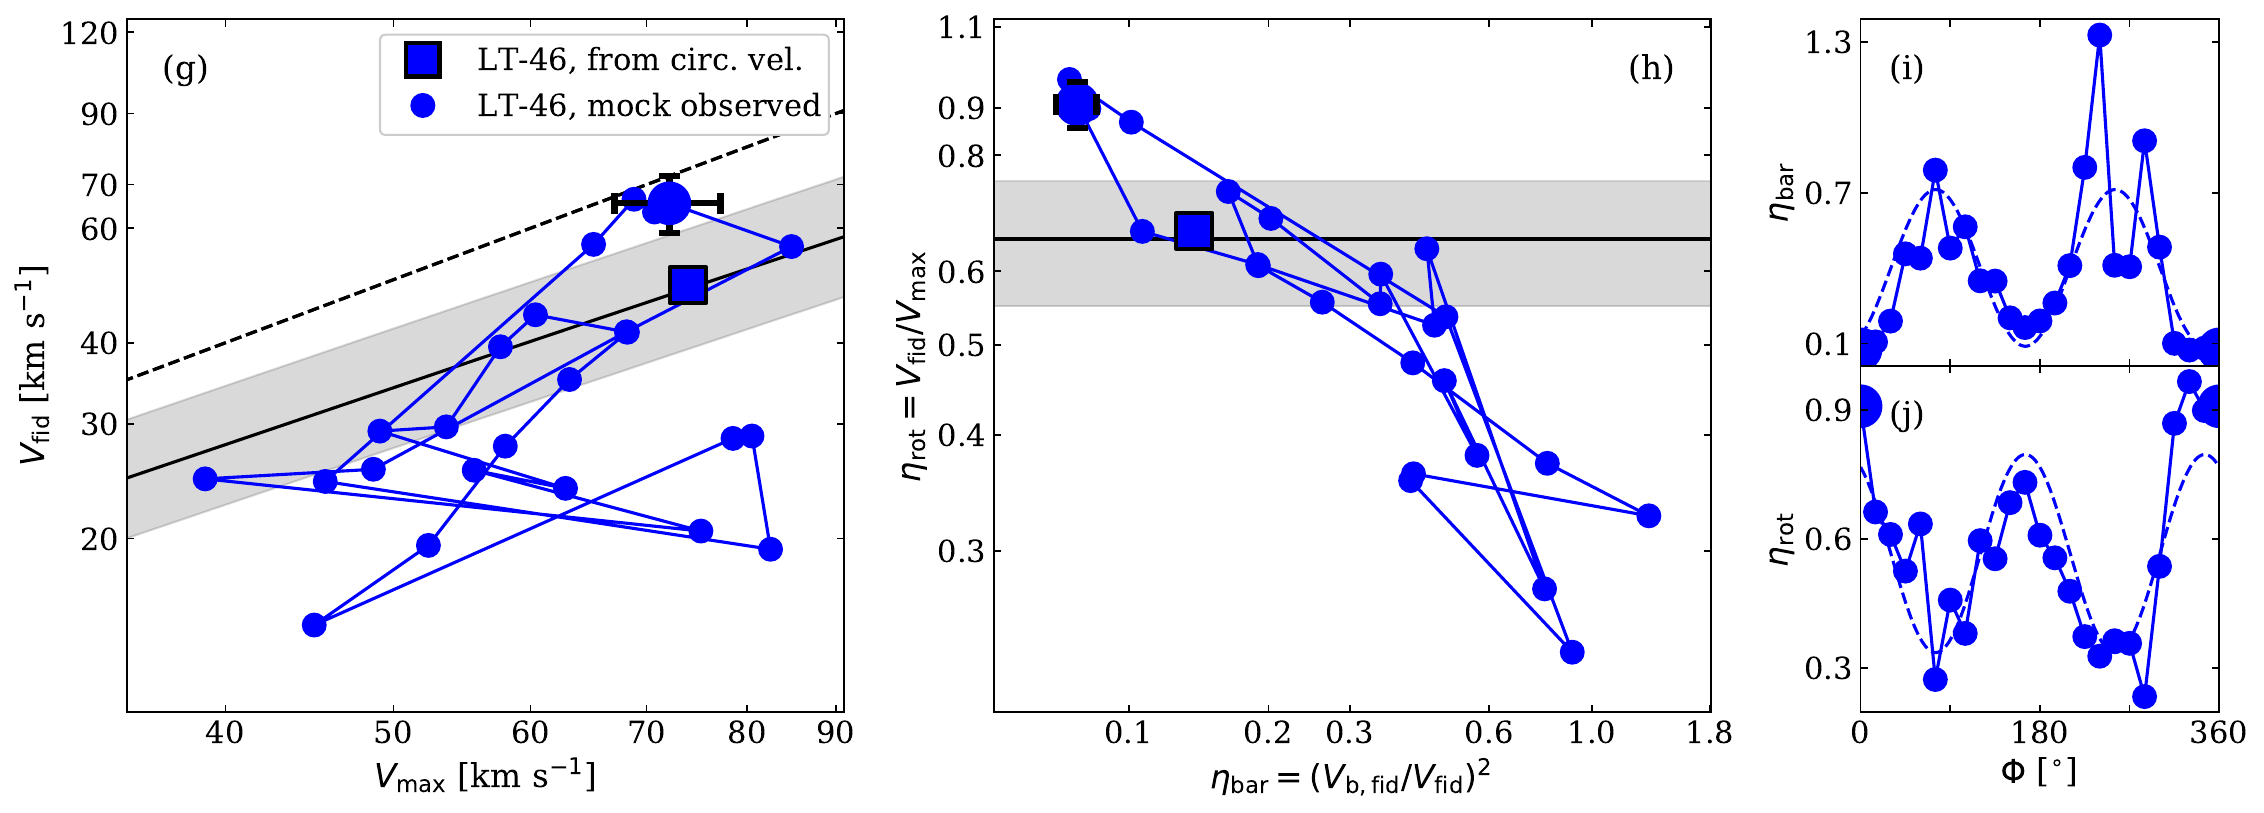}
\end{minipage}
\begin{minipage}{.4\textwidth}
\includegraphics[width=\textwidth]{../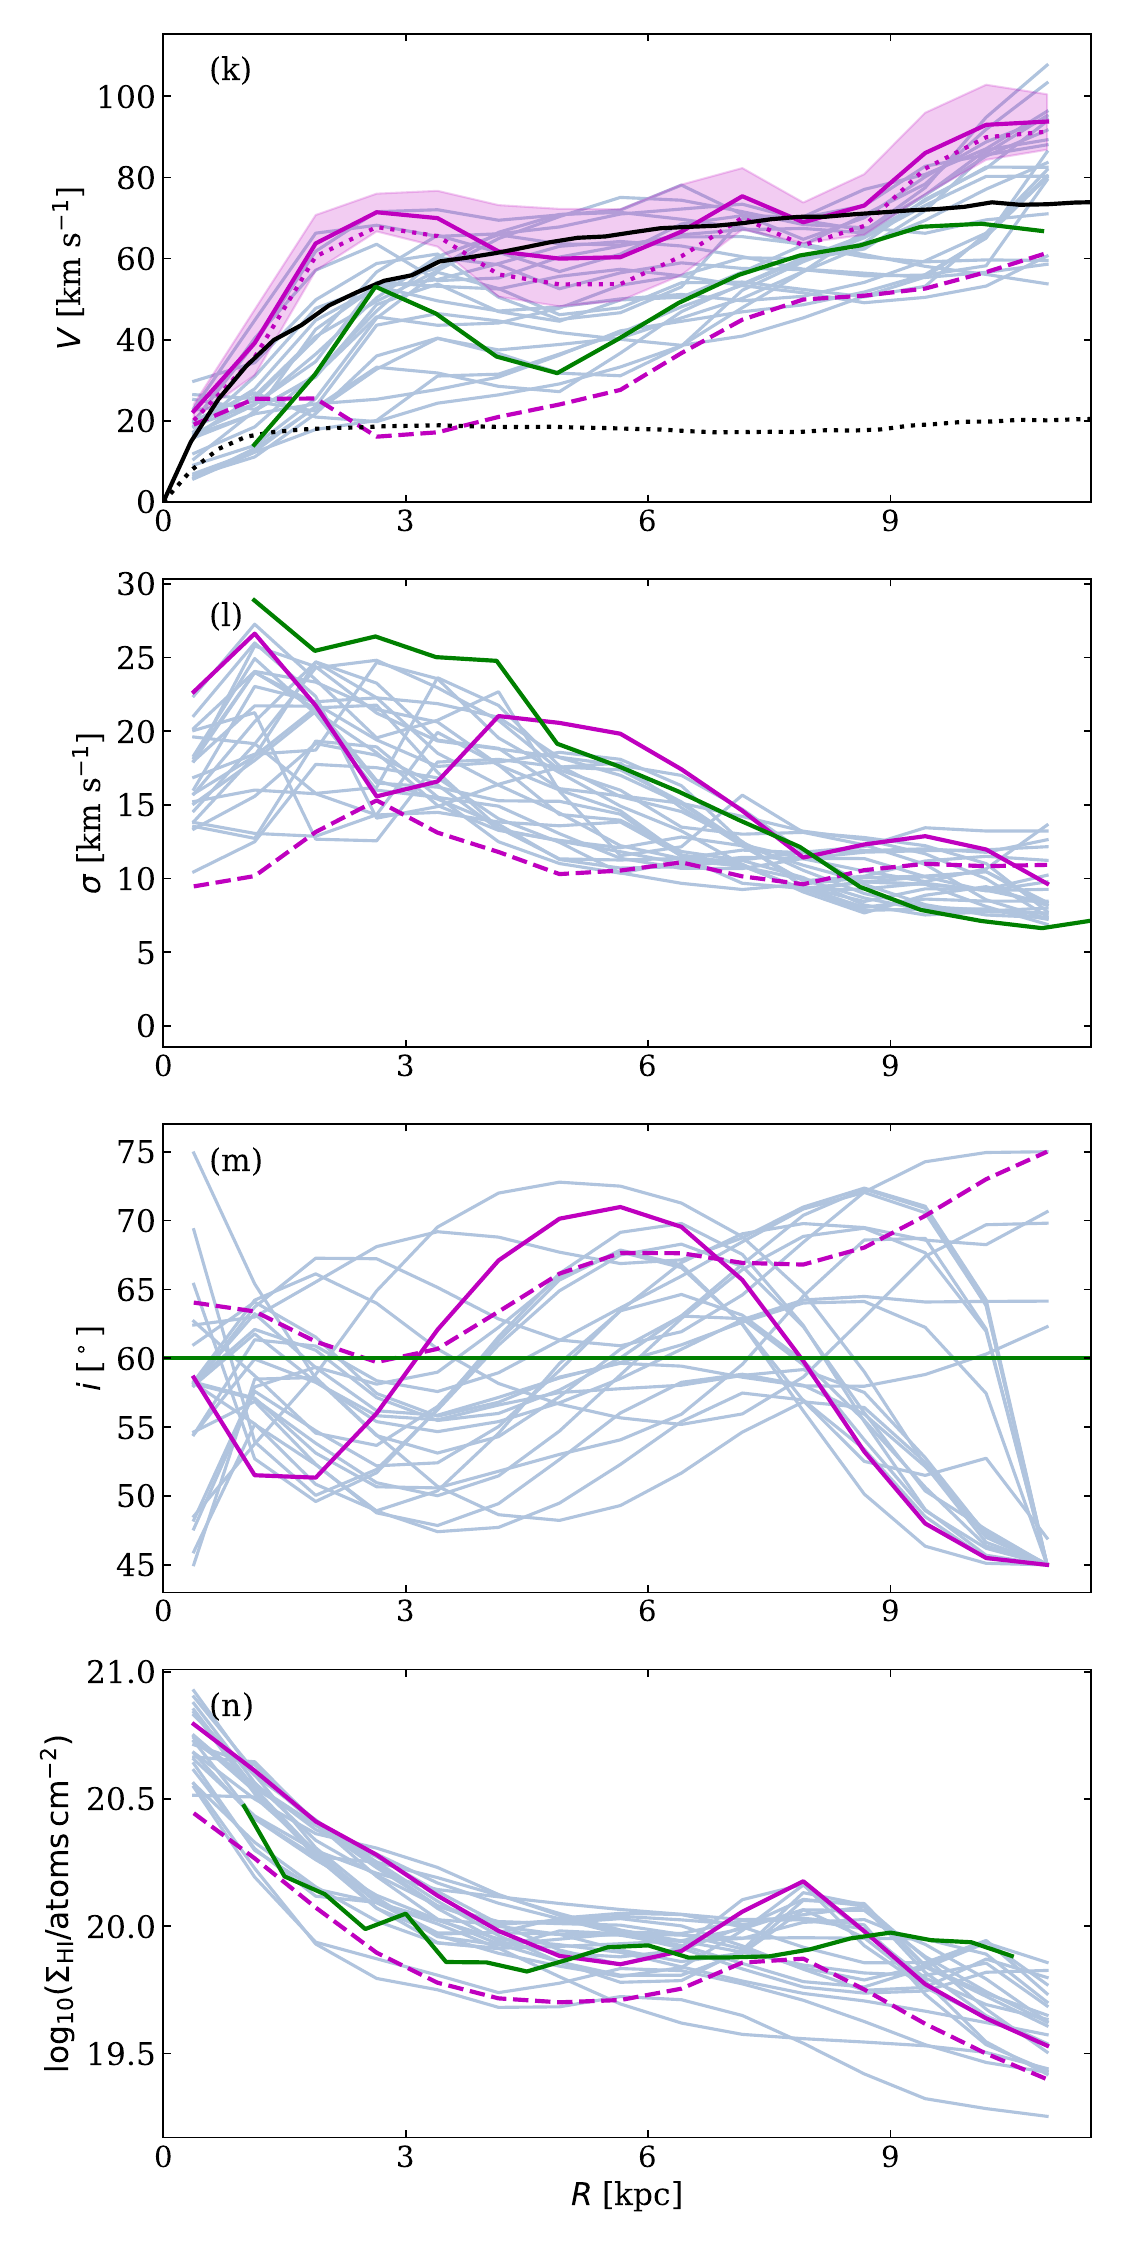}
\end{minipage}
\caption{A set of summary figures for galaxy LT-46, selected for kinematic analysis. These include example moment maps for two orientations (panels (a)--(f); similar to Fig.~\ref{fig:visualisations}), a summary of the parameters $V_\mathrm{fid}$, $V_\mathrm{max}$, $\eta_\mathrm{rot}$, and $\eta_\mathrm{bar}$ (panels (g)--(j); similar to Fig.~\ref{fig:loops}), and a summary of the rotation curve analysis from $24$ viewing angles (panels (k)--(n); similar to Fig.~\ref{fig:rot_curves}). See description of Appendix~\ref{app:supplementary} for details.}
\label{fig:S15}
\end{figure}
\clearpage

\begin{figure}
\begin{minipage}{.9\textwidth}
\includegraphics[width=\textwidth]{../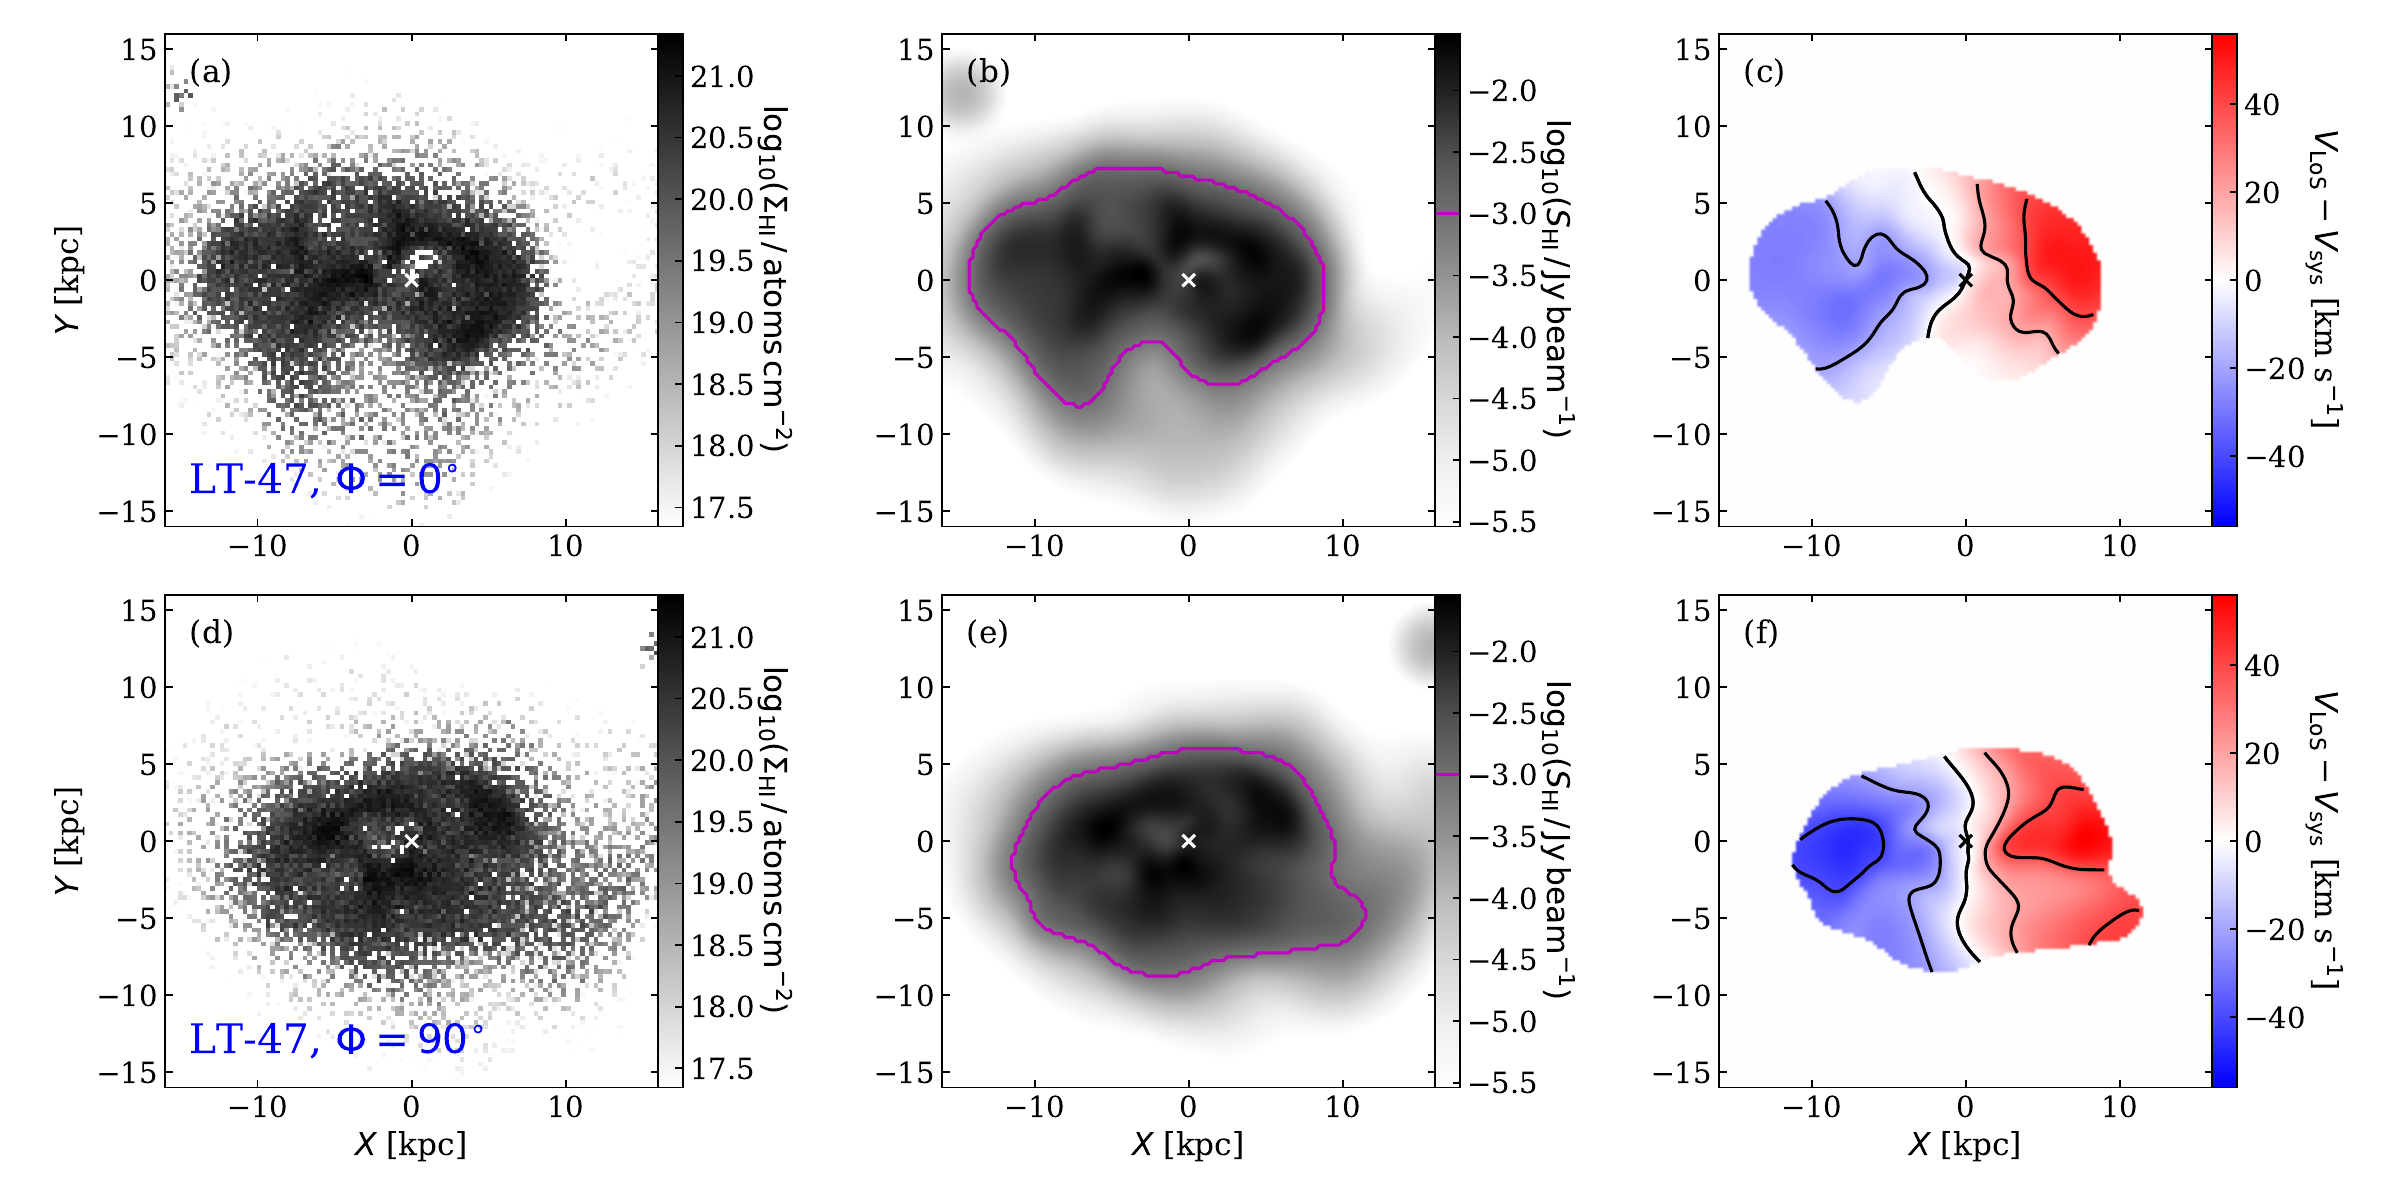}
\includegraphics[width=\textwidth]{../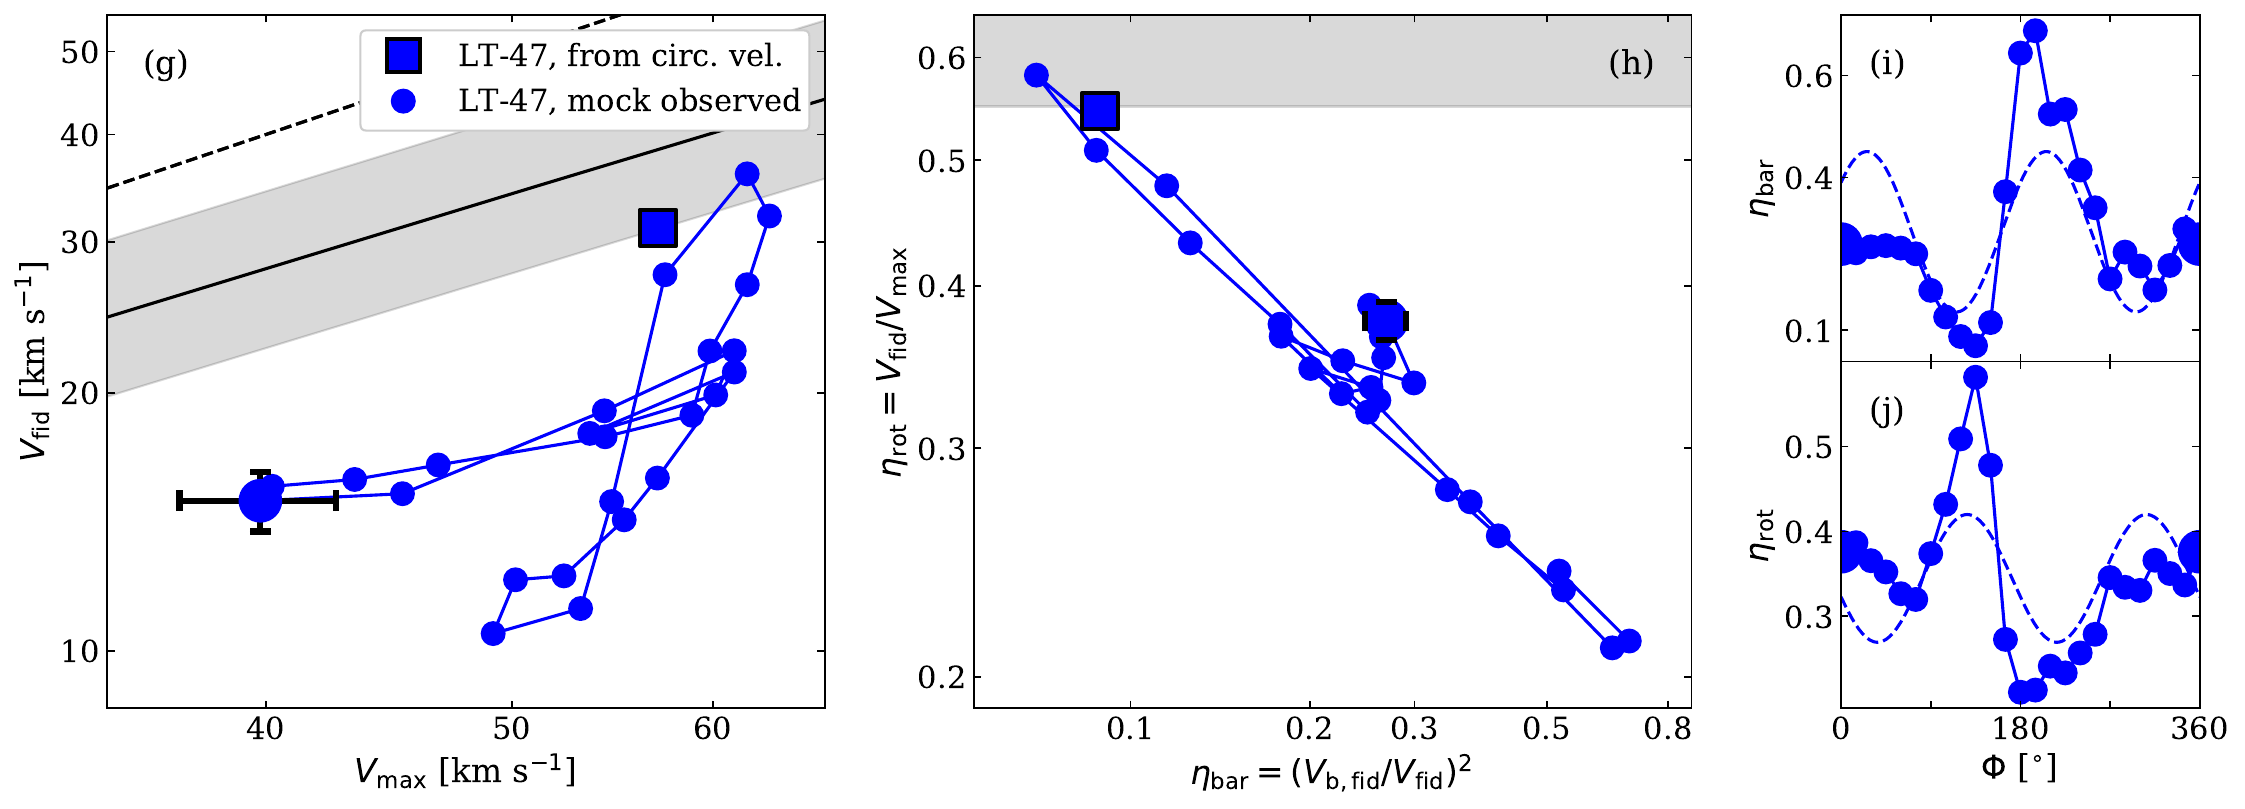}
\end{minipage}
\begin{minipage}{.4\textwidth}
\includegraphics[width=\textwidth]{../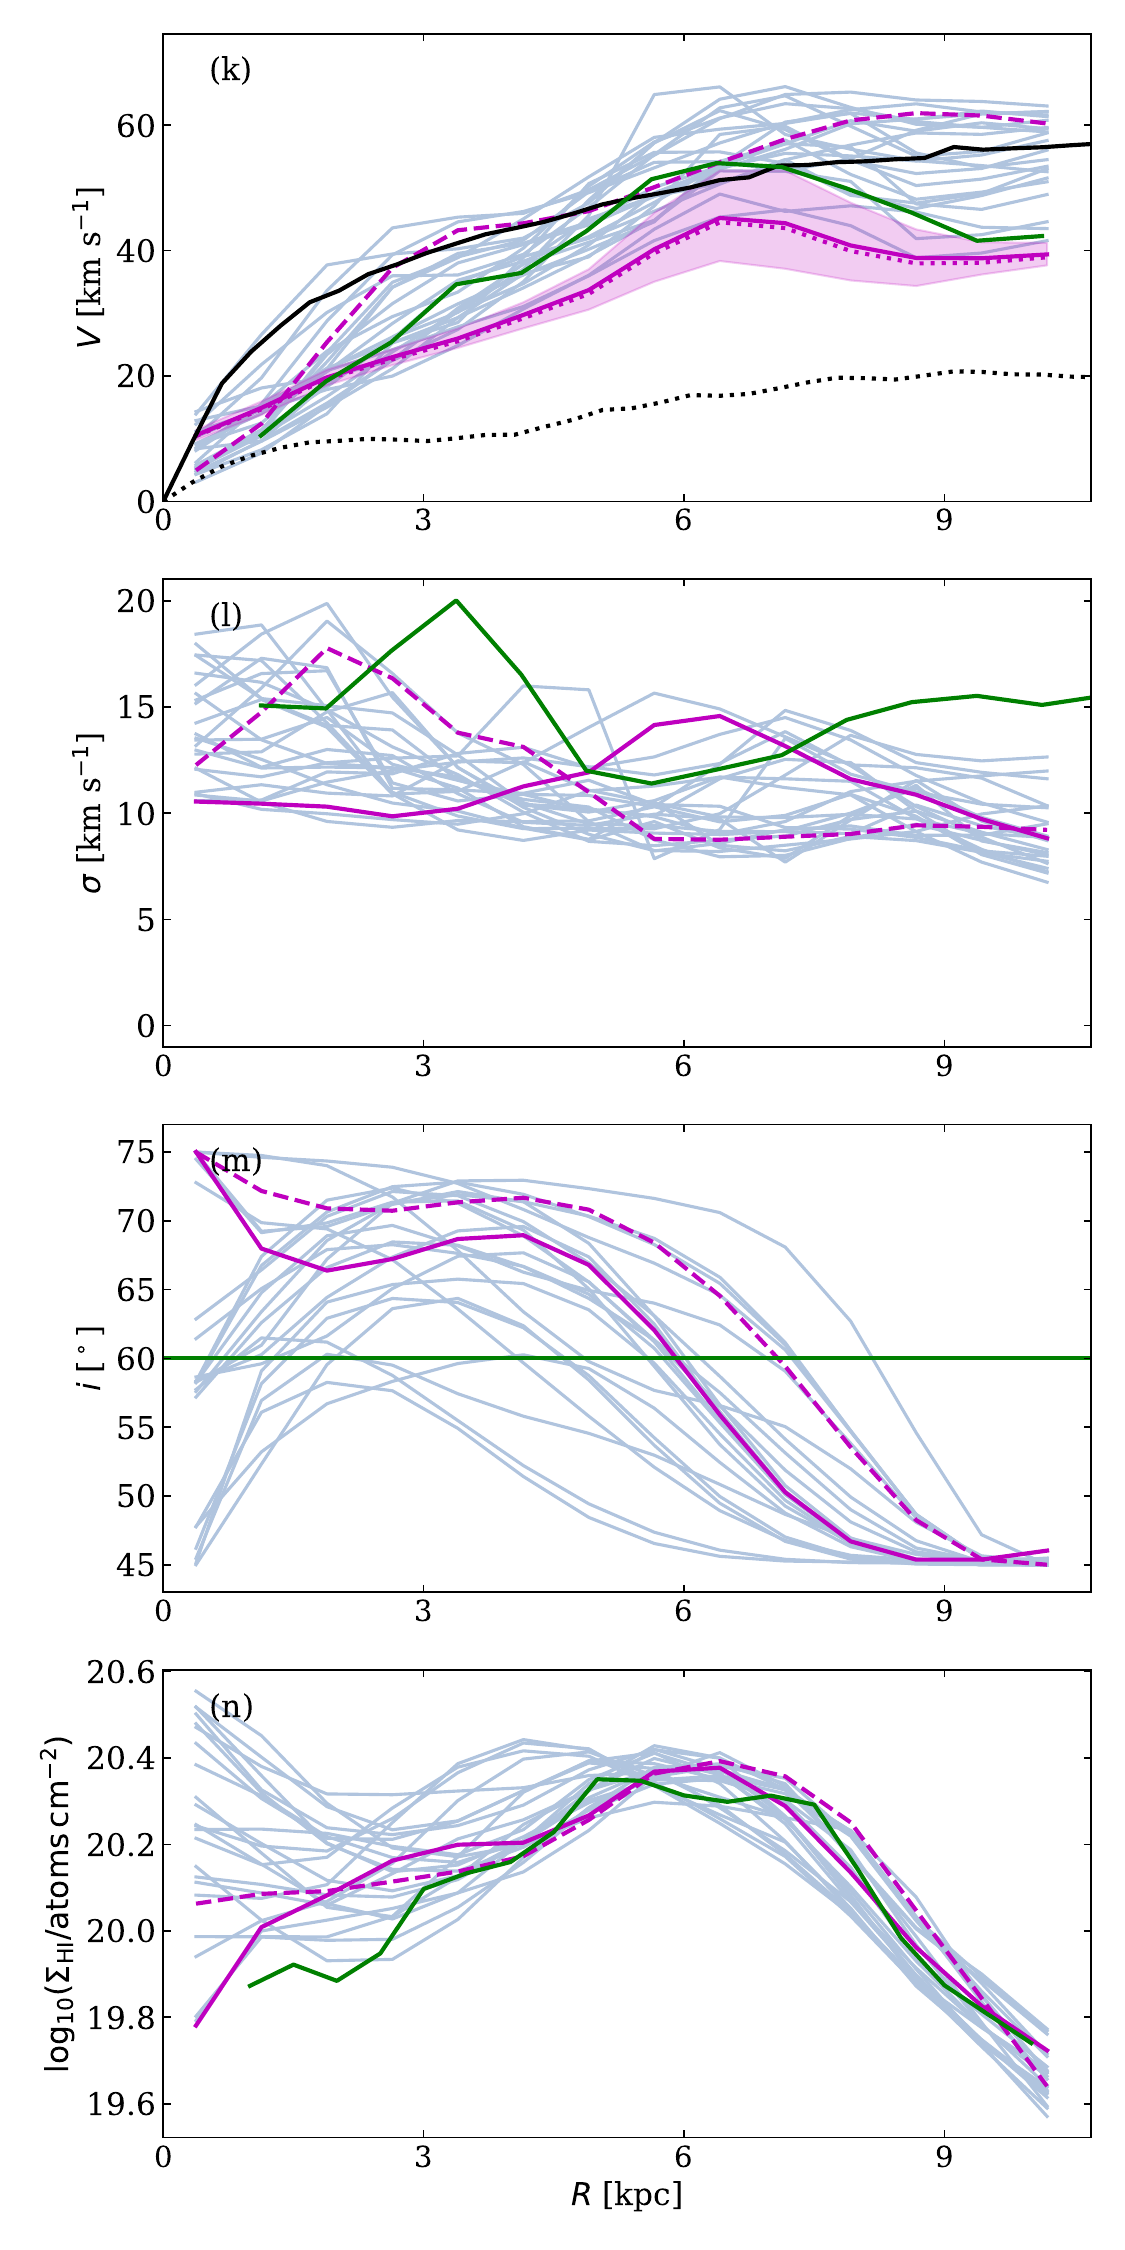}
\end{minipage}
\caption{A set of summary figures for galaxy LT-47, selected for kinematic analysis. These include example moment maps for two orientations (panels (a)--(f); similar to Fig.~\ref{fig:visualisations}), a summary of the parameters $V_\mathrm{fid}$, $V_\mathrm{max}$, $\eta_\mathrm{rot}$, and $\eta_\mathrm{bar}$ (panels (g)--(j); similar to Fig.~\ref{fig:loops}), and a summary of the rotation curve analysis from $24$ viewing angles (panels (k)--(n); similar to Fig.~\ref{fig:rot_curves}). See description of Appendix~\ref{app:supplementary} for details.}
\label{fig:S16}
\end{figure}
\clearpage

\begin{figure}
\begin{minipage}{.9\textwidth}
\includegraphics[width=\textwidth]{../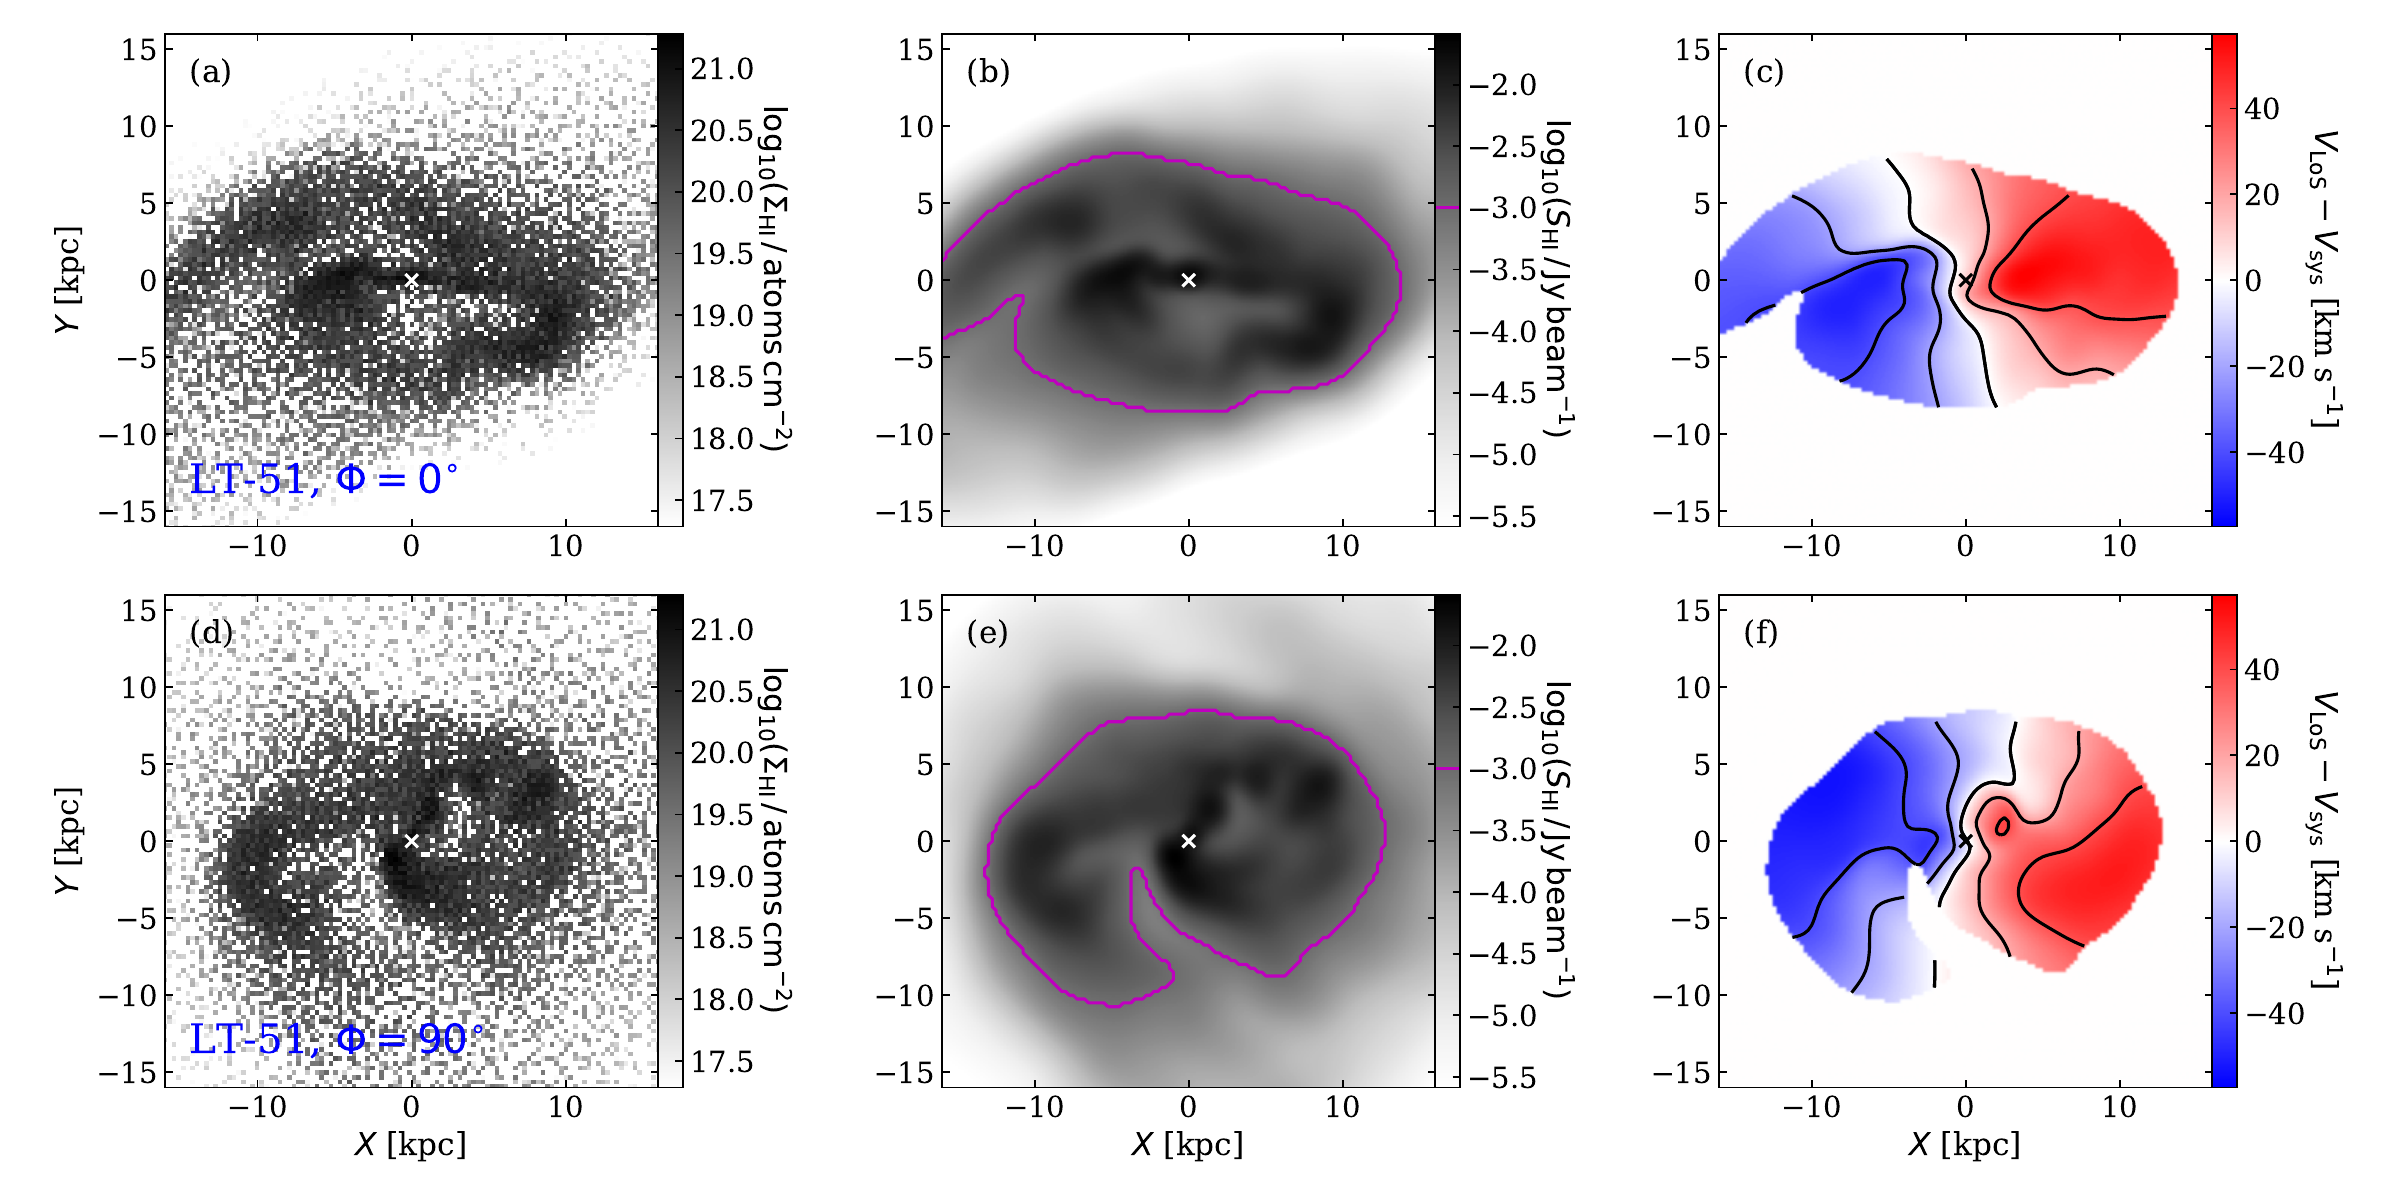}
\includegraphics[width=\textwidth]{../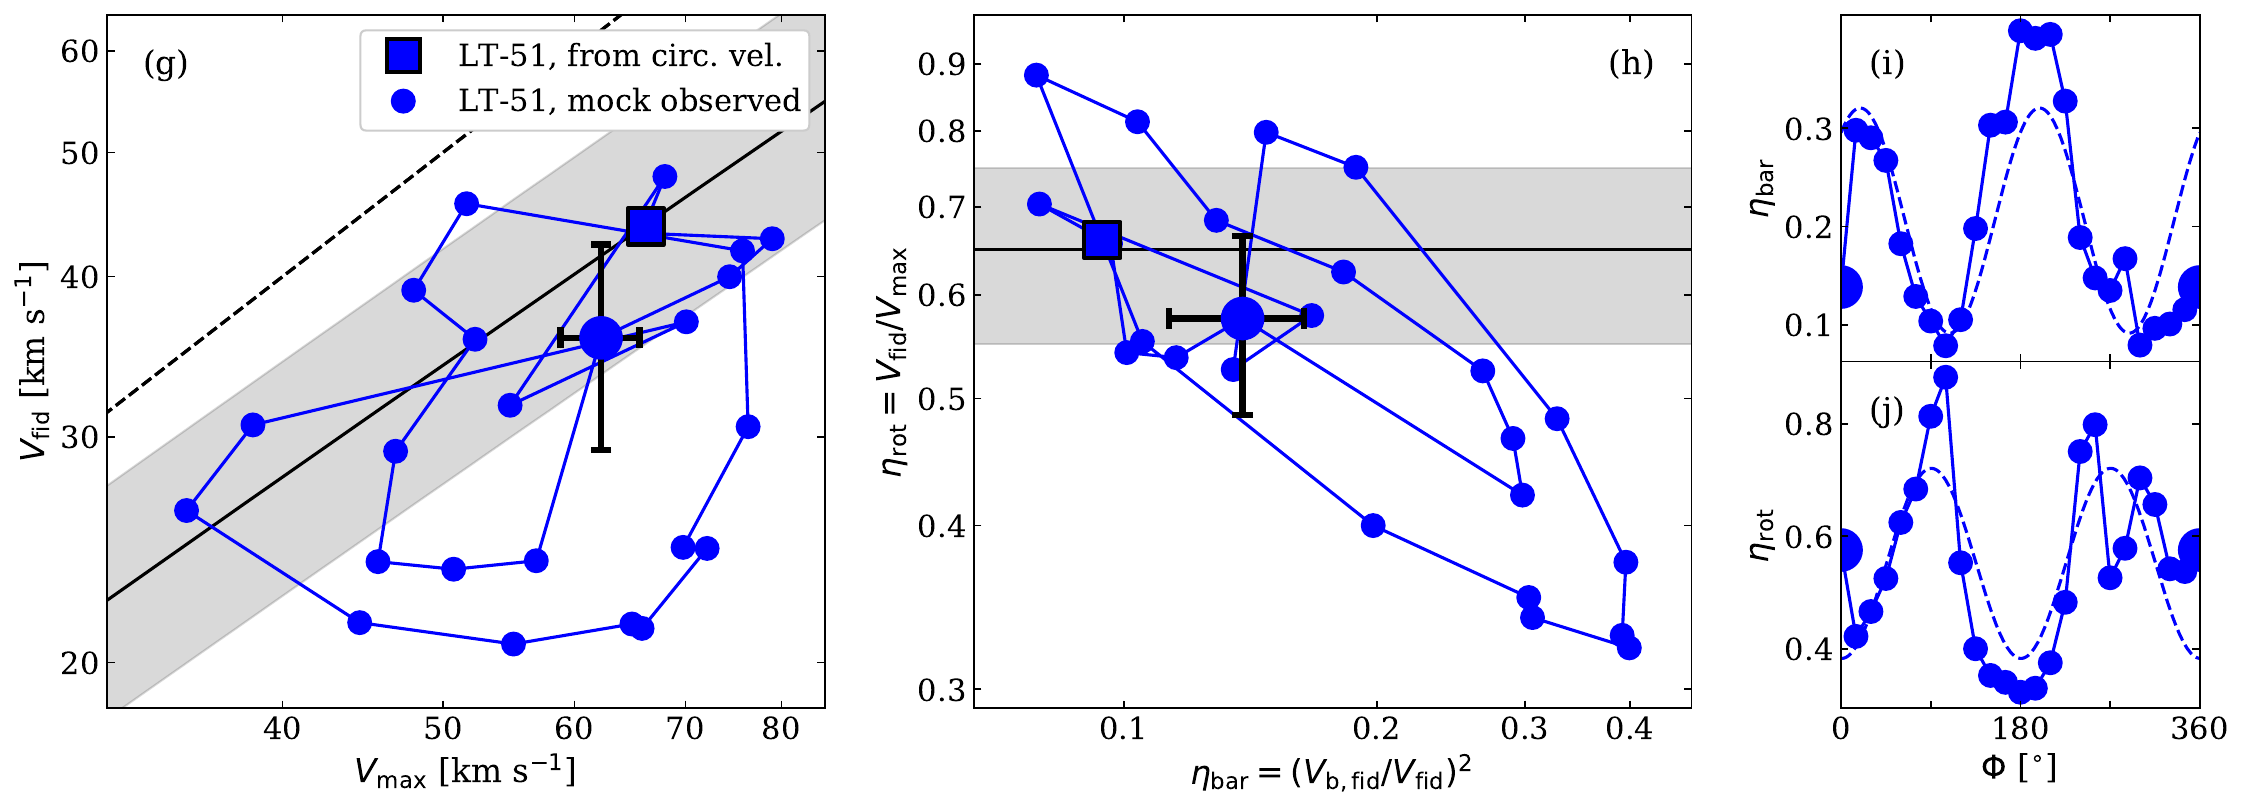}
\end{minipage}
\begin{minipage}{.4\textwidth}
\includegraphics[width=\textwidth]{../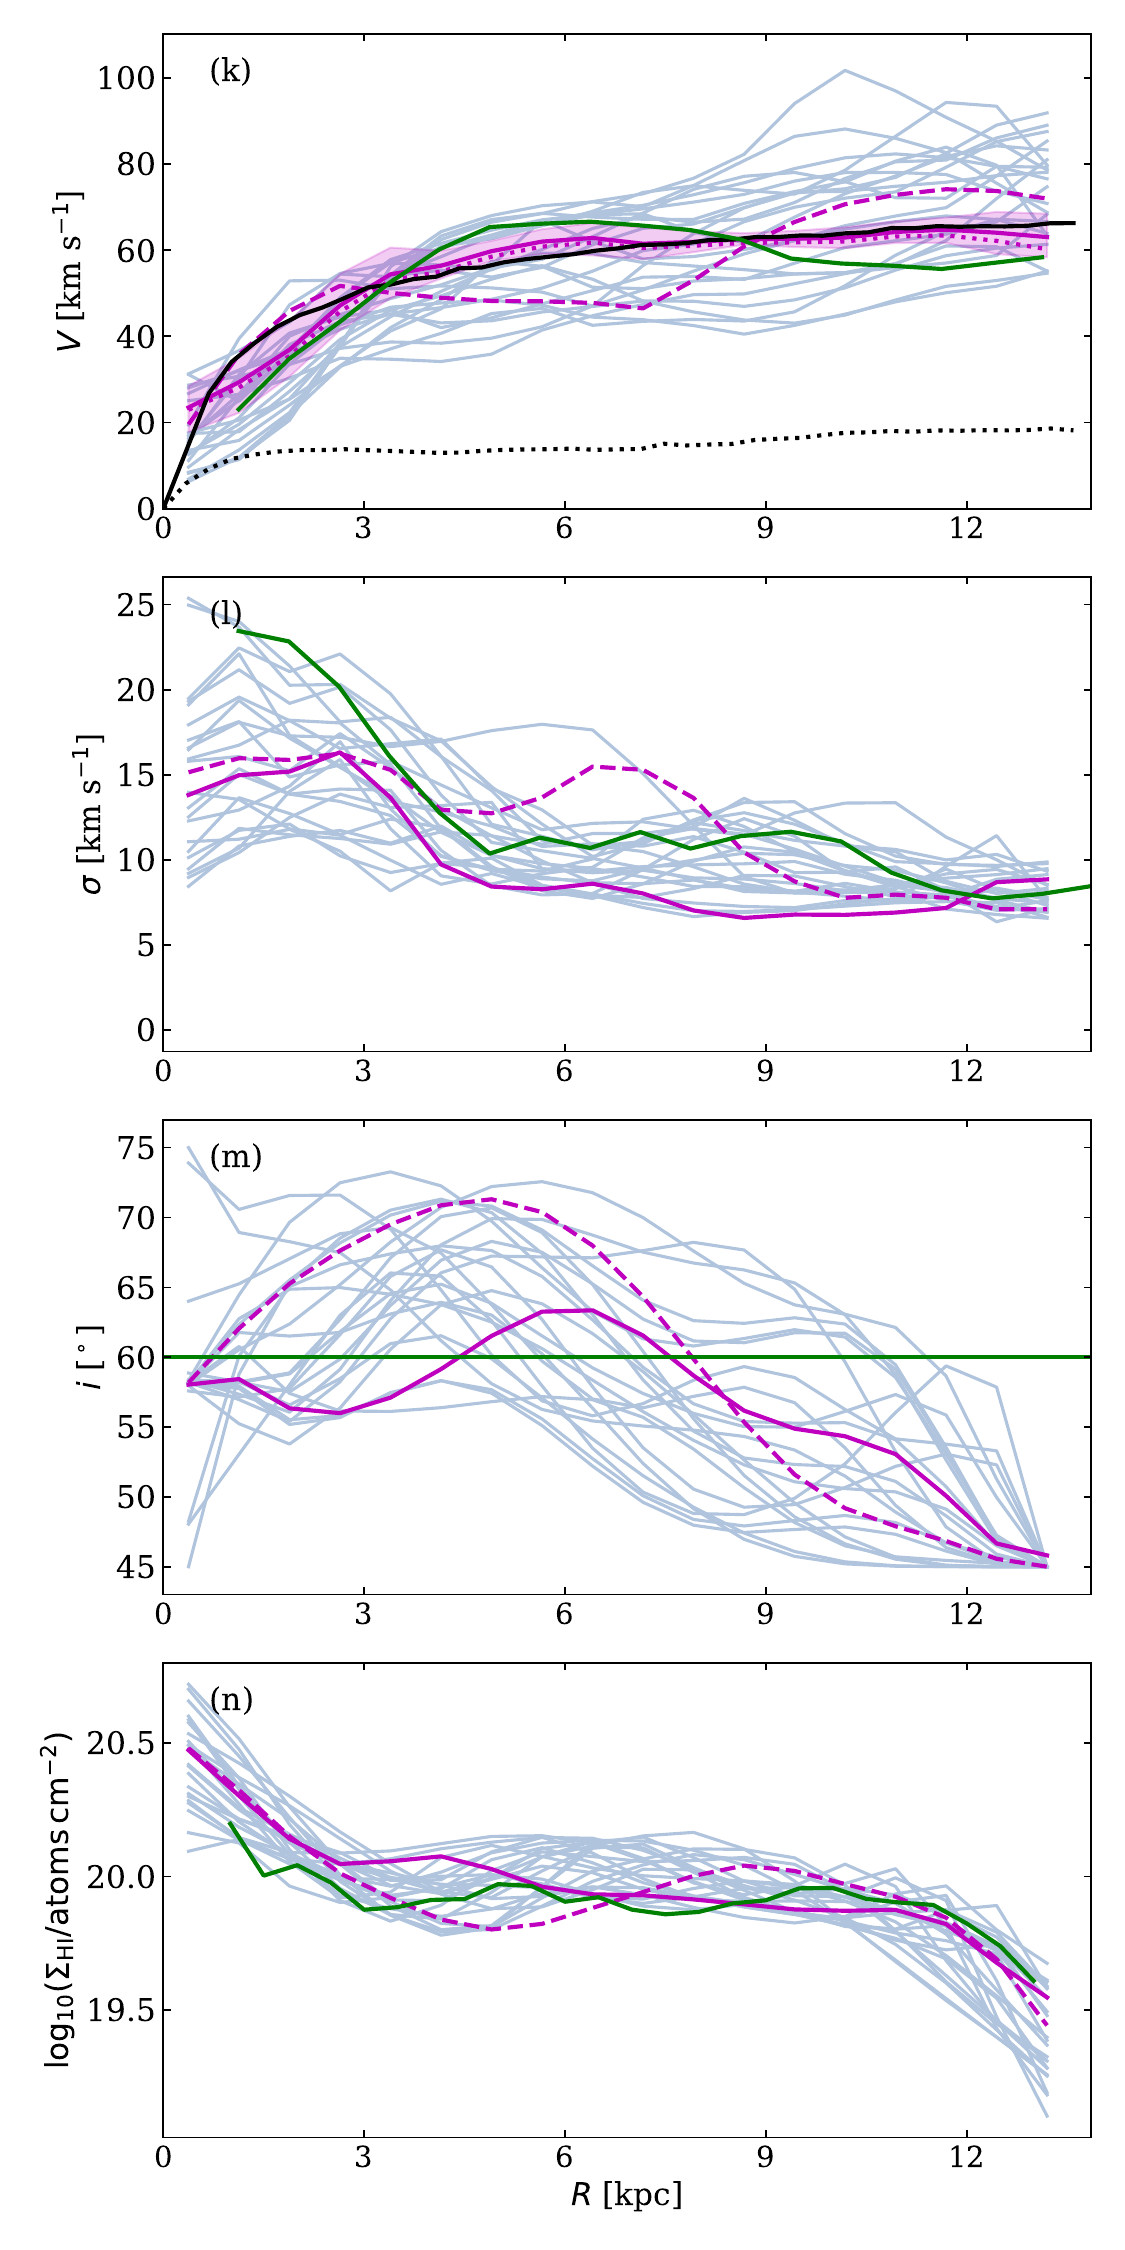}
\end{minipage}
\caption{A set of summary figures for galaxy LT-51, selected for kinematic analysis. These include example moment maps for two orientations (panels (a)--(f); similar to Fig.~\ref{fig:visualisations}), a summary of the parameters $V_\mathrm{fid}$, $V_\mathrm{max}$, $\eta_\mathrm{rot}$, and $\eta_\mathrm{bar}$ (panels (g)--(j); similar to Fig.~\ref{fig:loops}), and a summary of the rotation curve analysis from $24$ viewing angles (panels (k)--(n); similar to Fig.~\ref{fig:rot_curves}). See description of Appendix~\ref{app:supplementary} for details.}
\label{fig:S17}
\end{figure}
\clearpage

\begin{figure}
\begin{minipage}{.9\textwidth}
\includegraphics[width=\textwidth]{../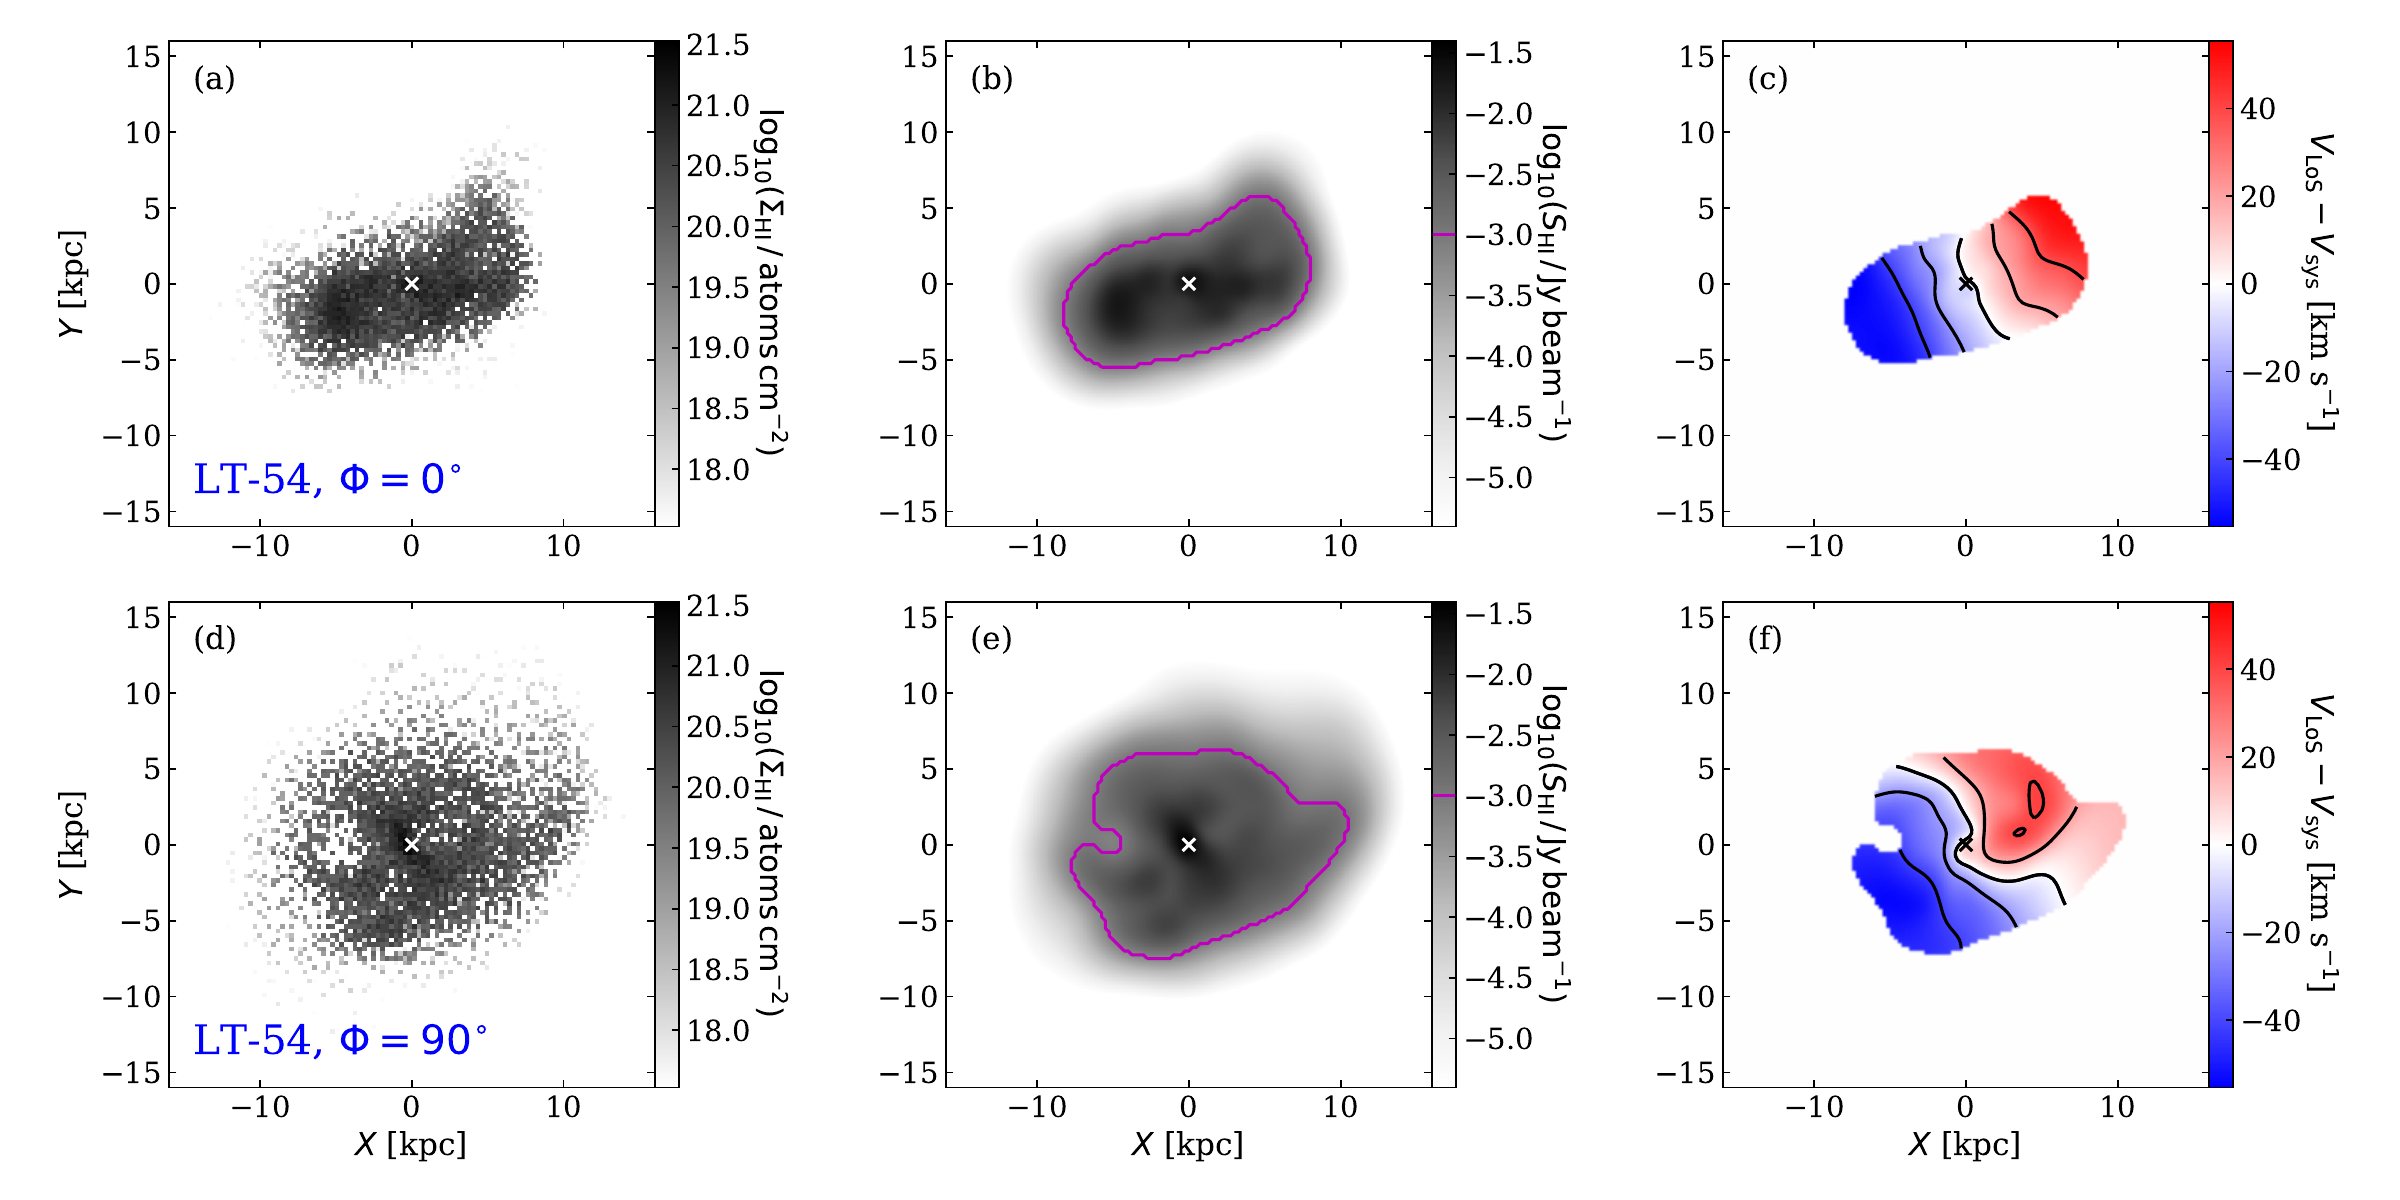}
\includegraphics[width=\textwidth]{../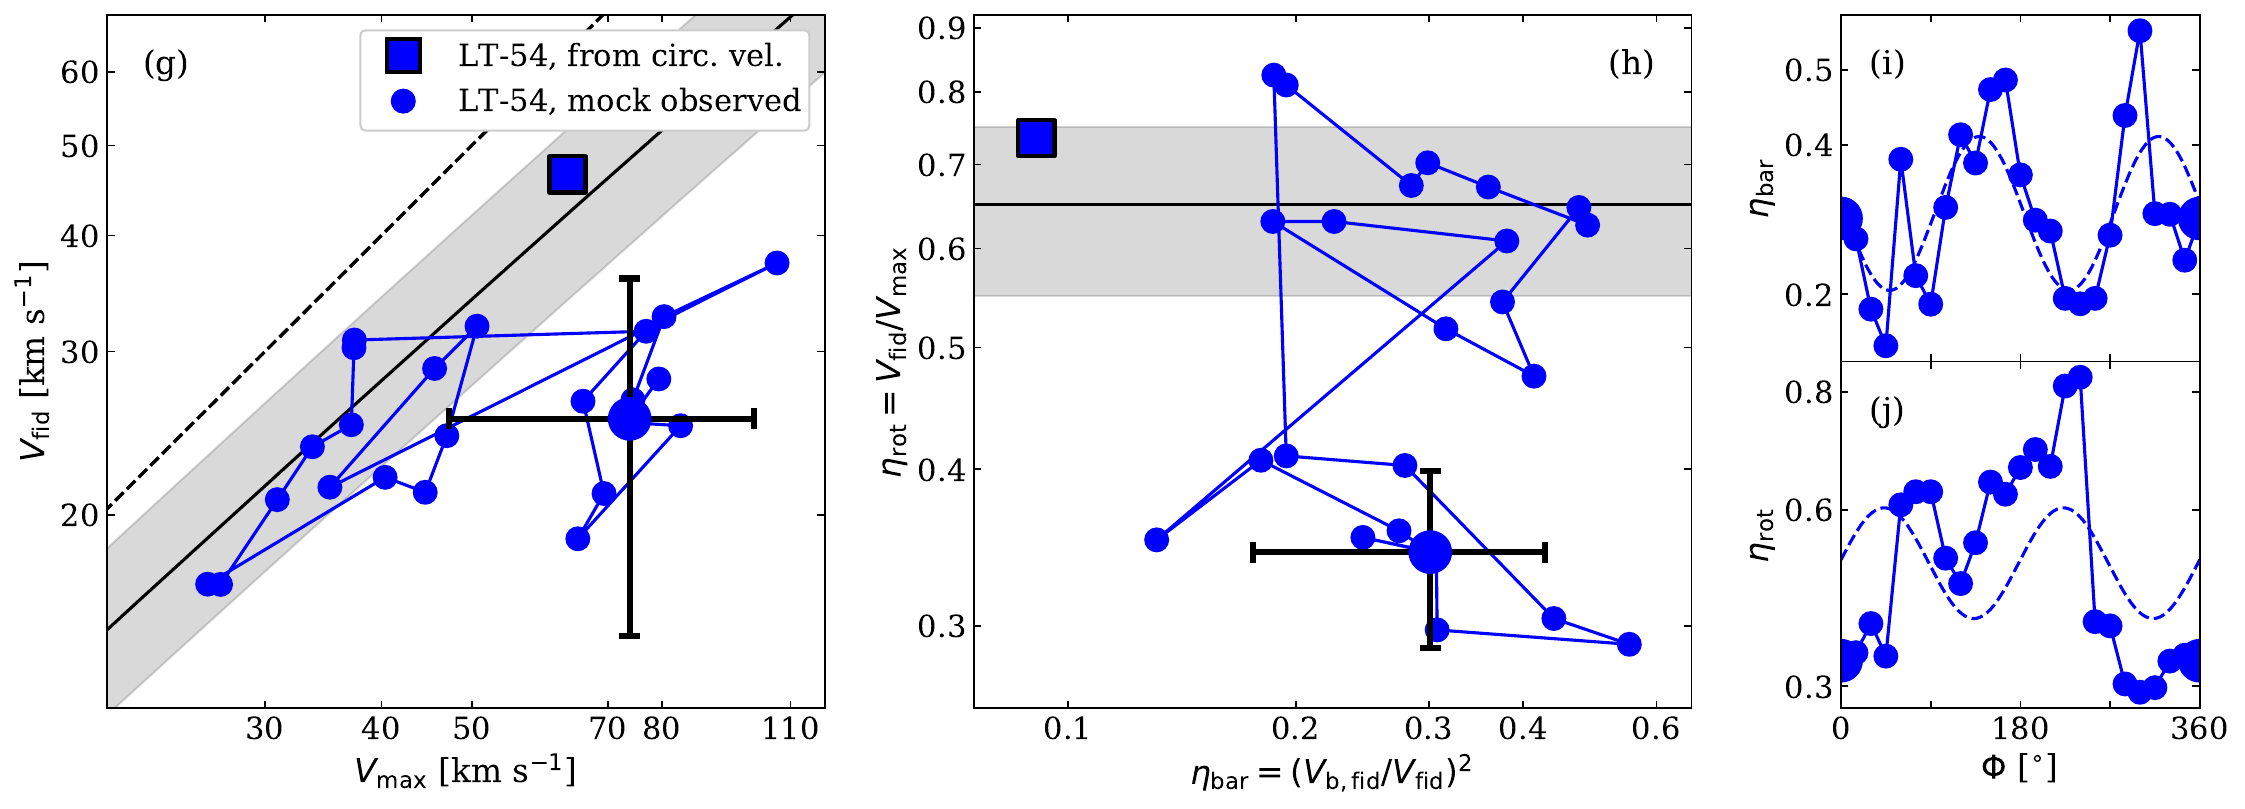}
\end{minipage}
\begin{minipage}{.4\textwidth}
\includegraphics[width=\textwidth]{../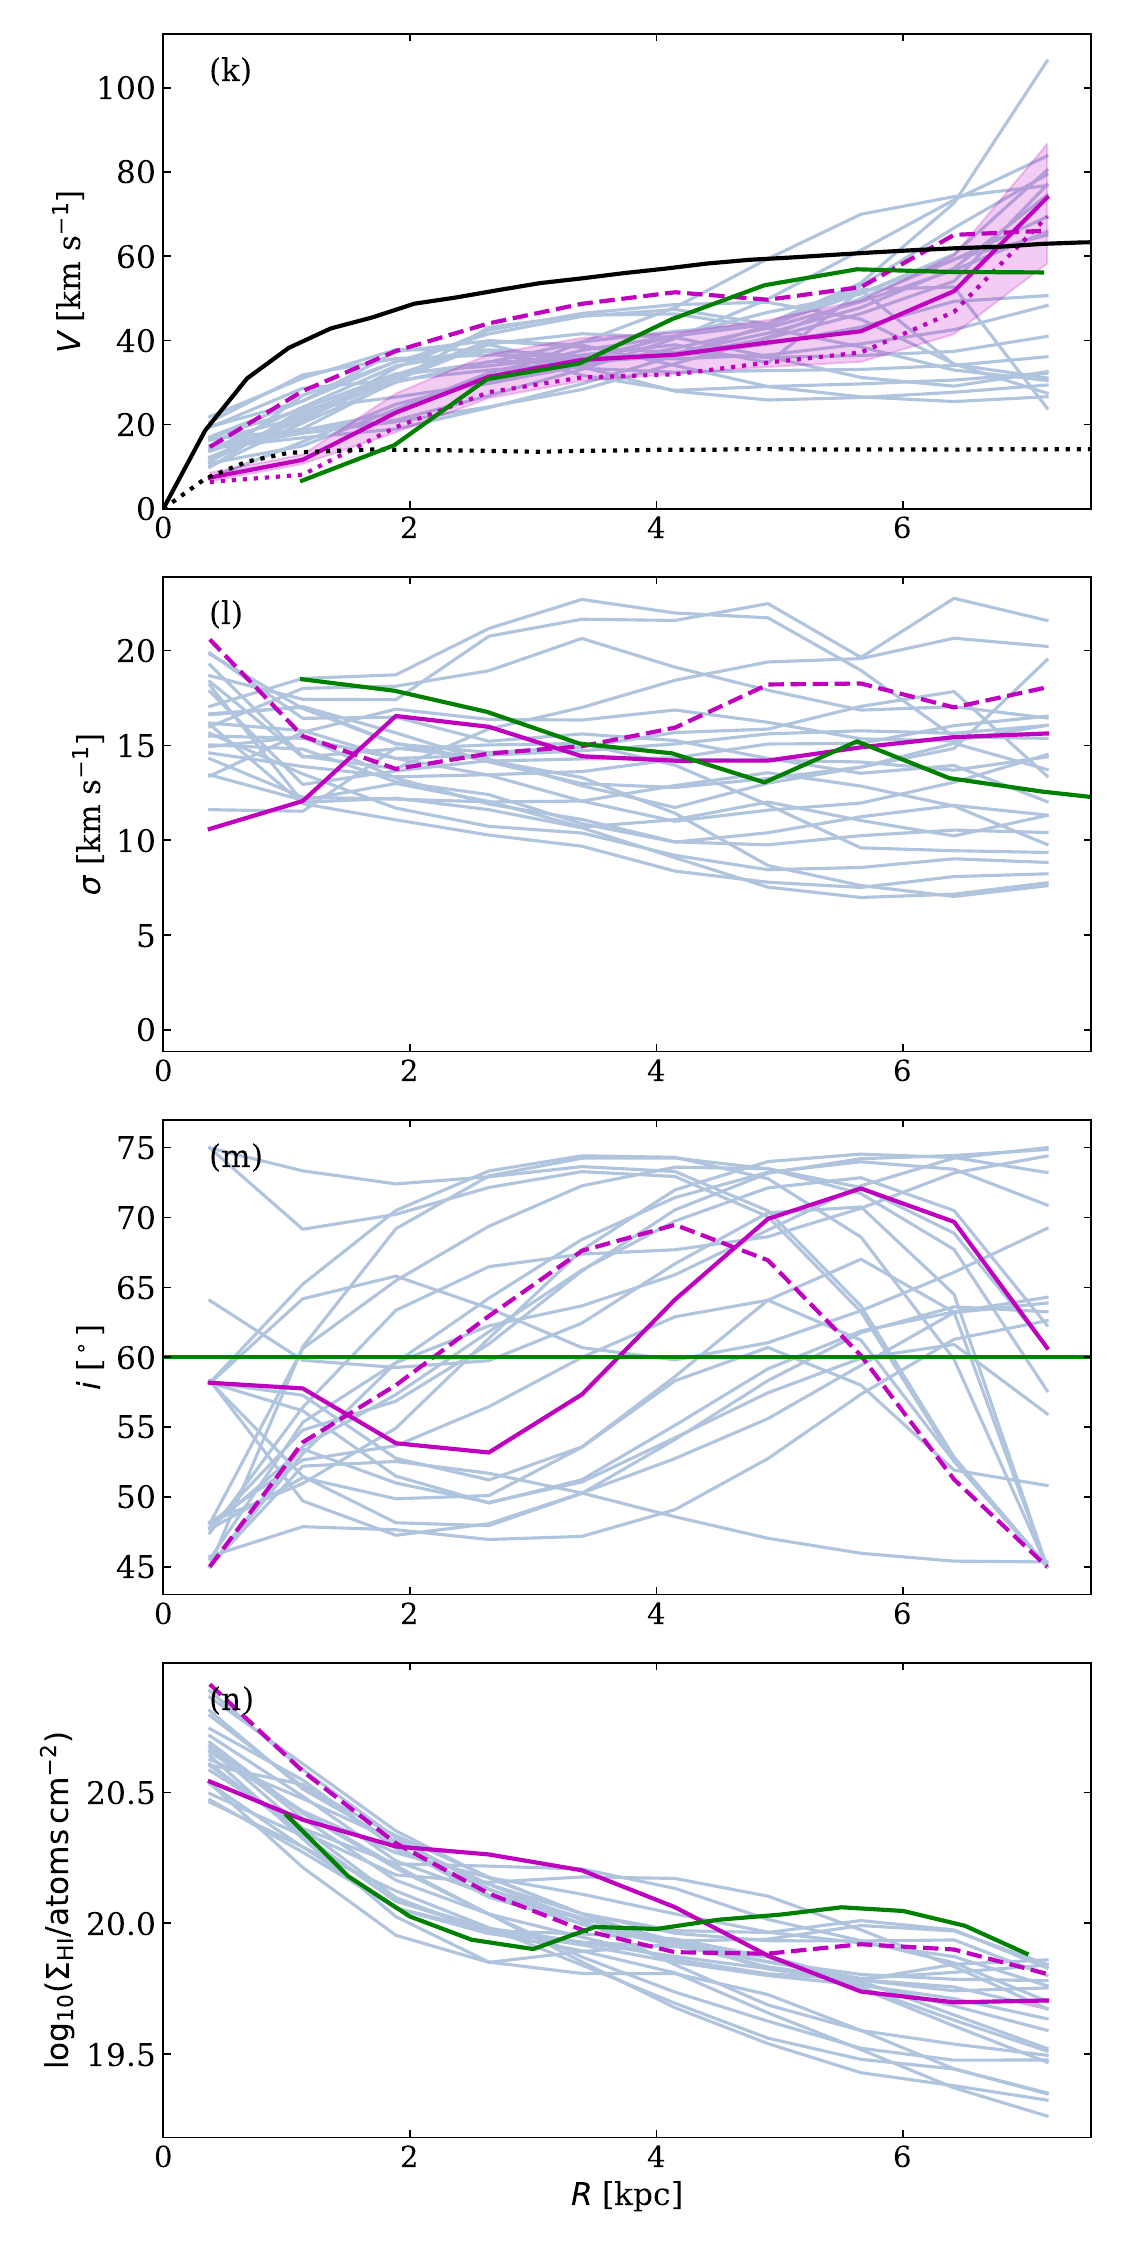}
\end{minipage}
\caption{A set of summary figures for galaxy LT-54, selected for kinematic analysis. These include example moment maps for two orientations (panels (a)--(f); similar to Fig.~\ref{fig:visualisations}), a summary of the parameters $V_\mathrm{fid}$, $V_\mathrm{max}$, $\eta_\mathrm{rot}$, and $\eta_\mathrm{bar}$ (panels (g)--(j); similar to Fig.~\ref{fig:loops}), and a summary of the rotation curve analysis from $24$ viewing angles (panels (k)--(n); similar to Fig.~\ref{fig:rot_curves}). See description of Appendix~\ref{app:supplementary} for details.}
\label{fig:S18}
\end{figure}
\clearpage

\begin{figure}
\begin{minipage}{.9\textwidth}
\includegraphics[width=\textwidth]{../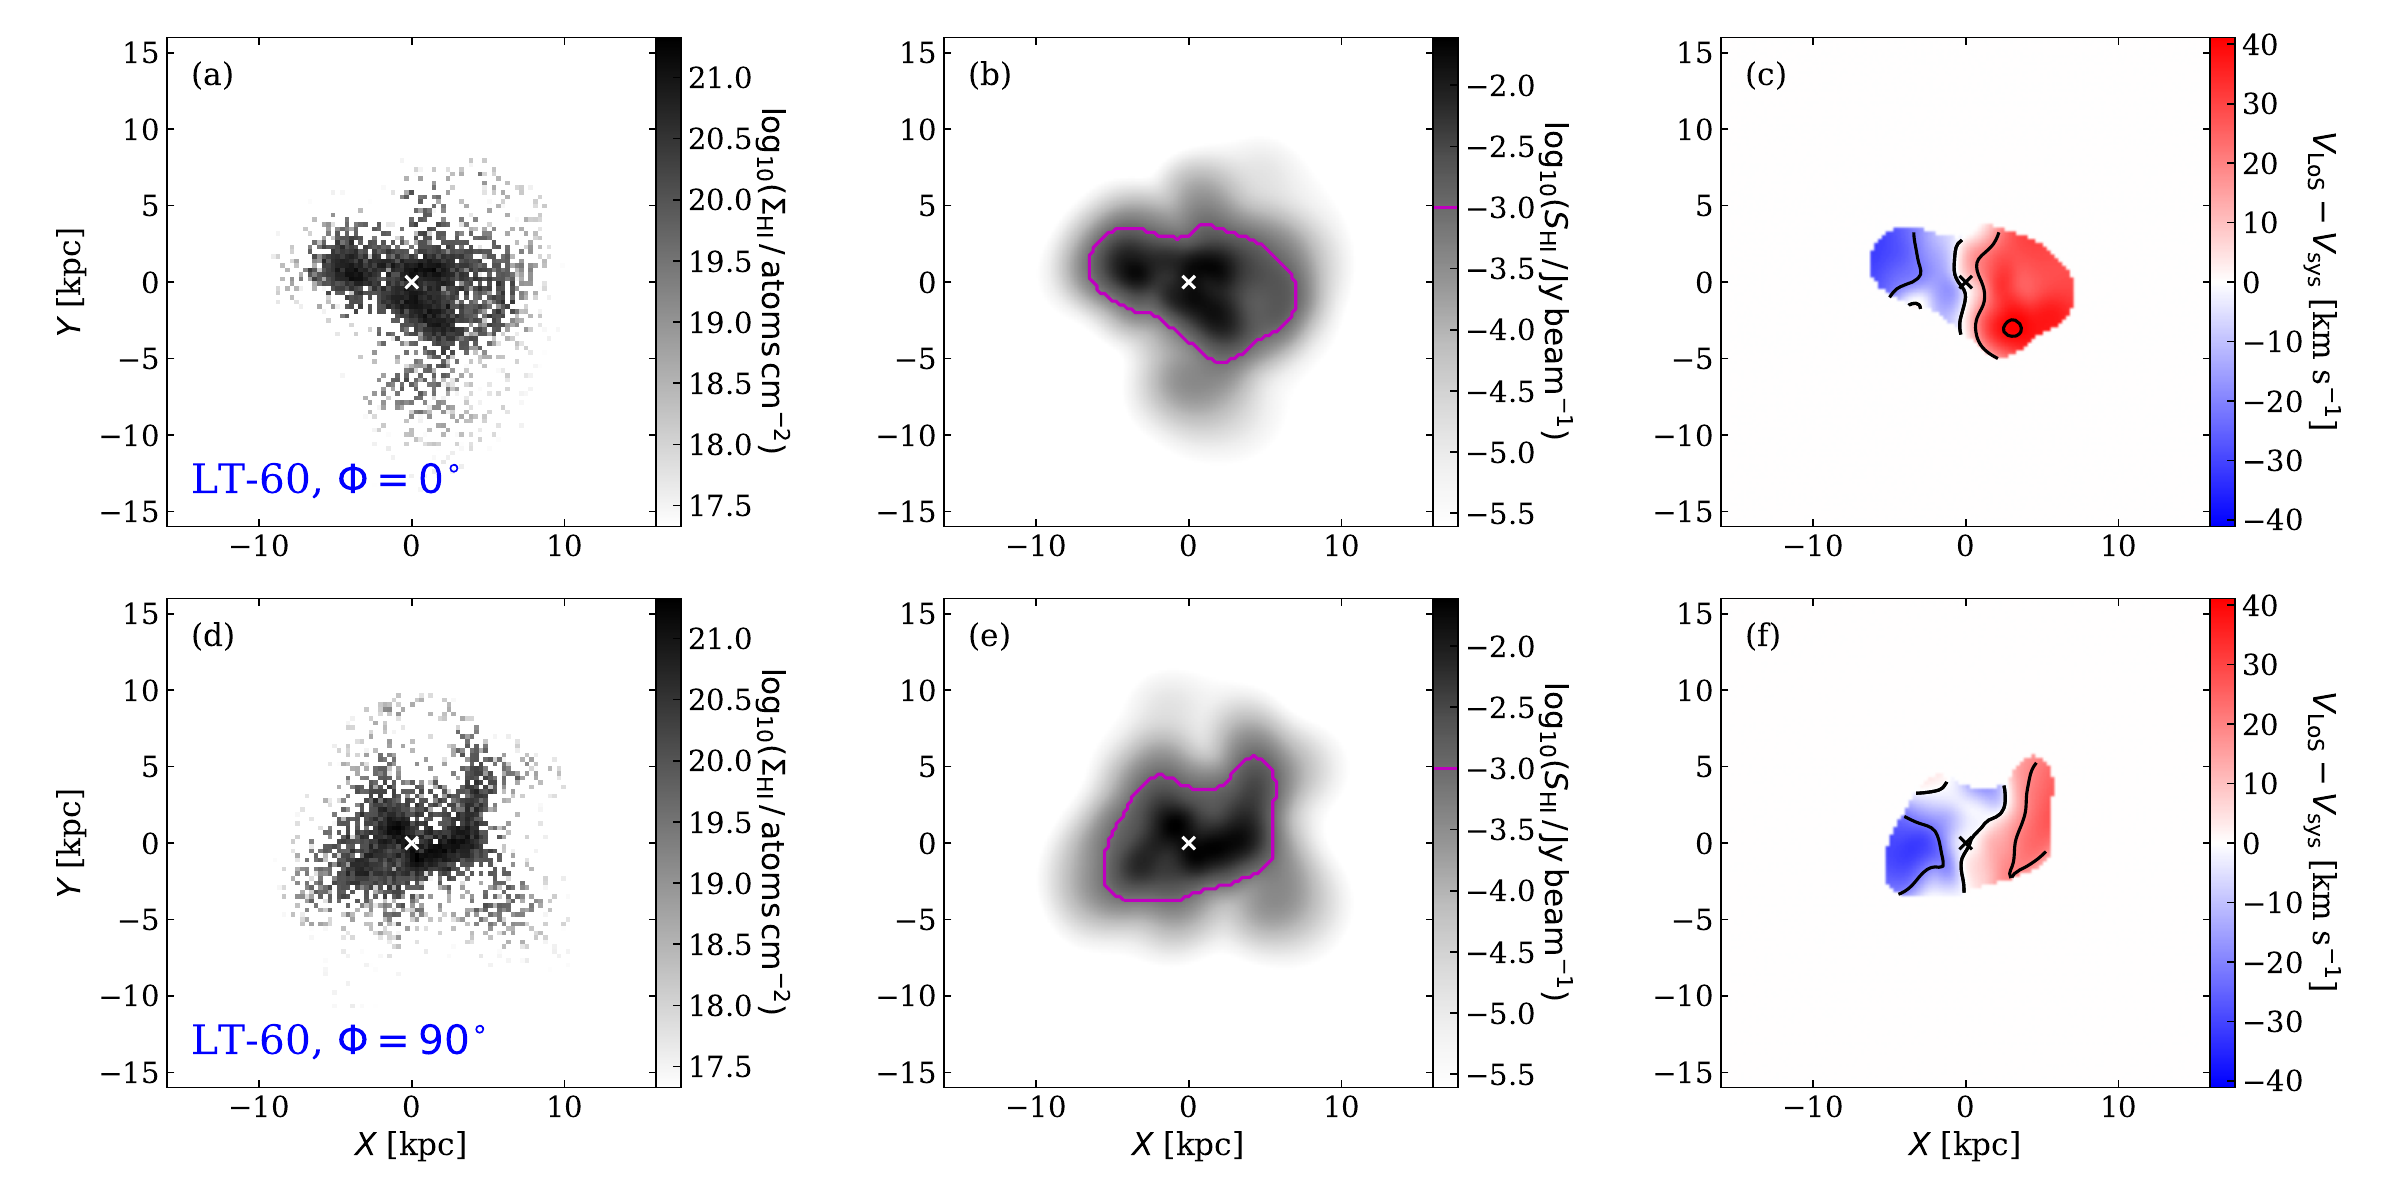}
\includegraphics[width=\textwidth]{../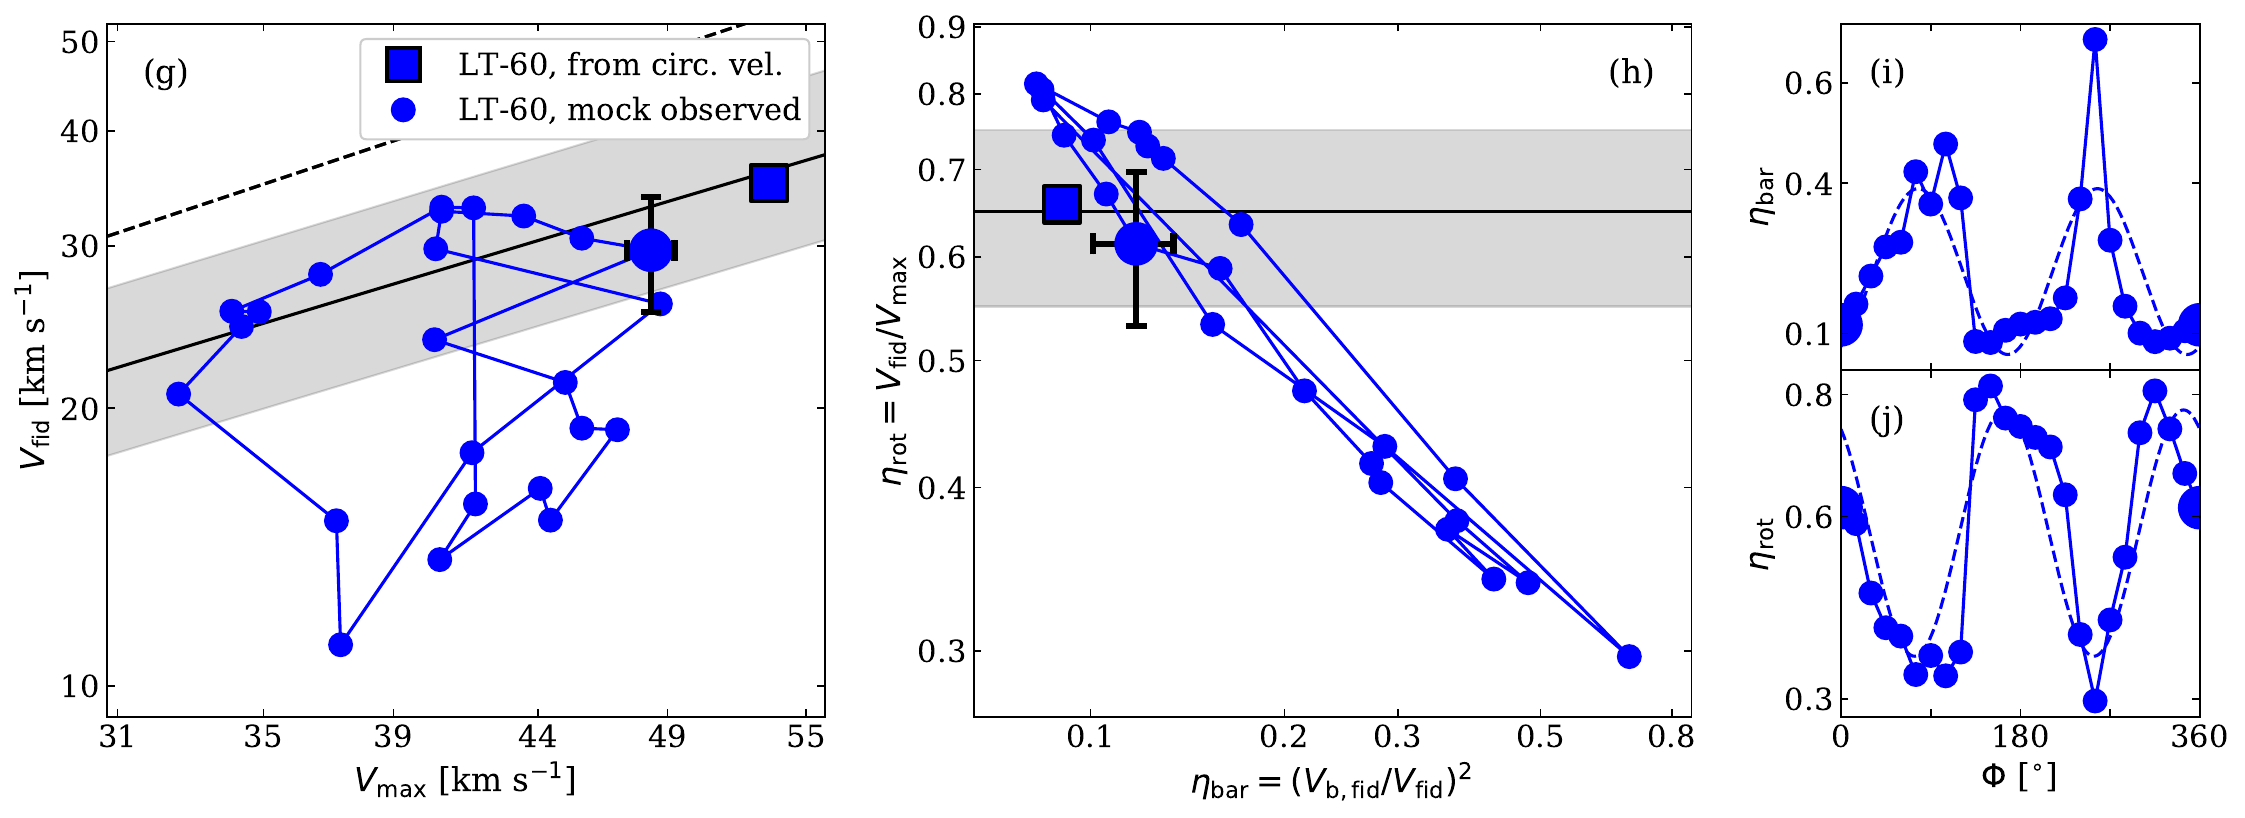}
\end{minipage}
\begin{minipage}{.4\textwidth}
\includegraphics[width=\textwidth]{../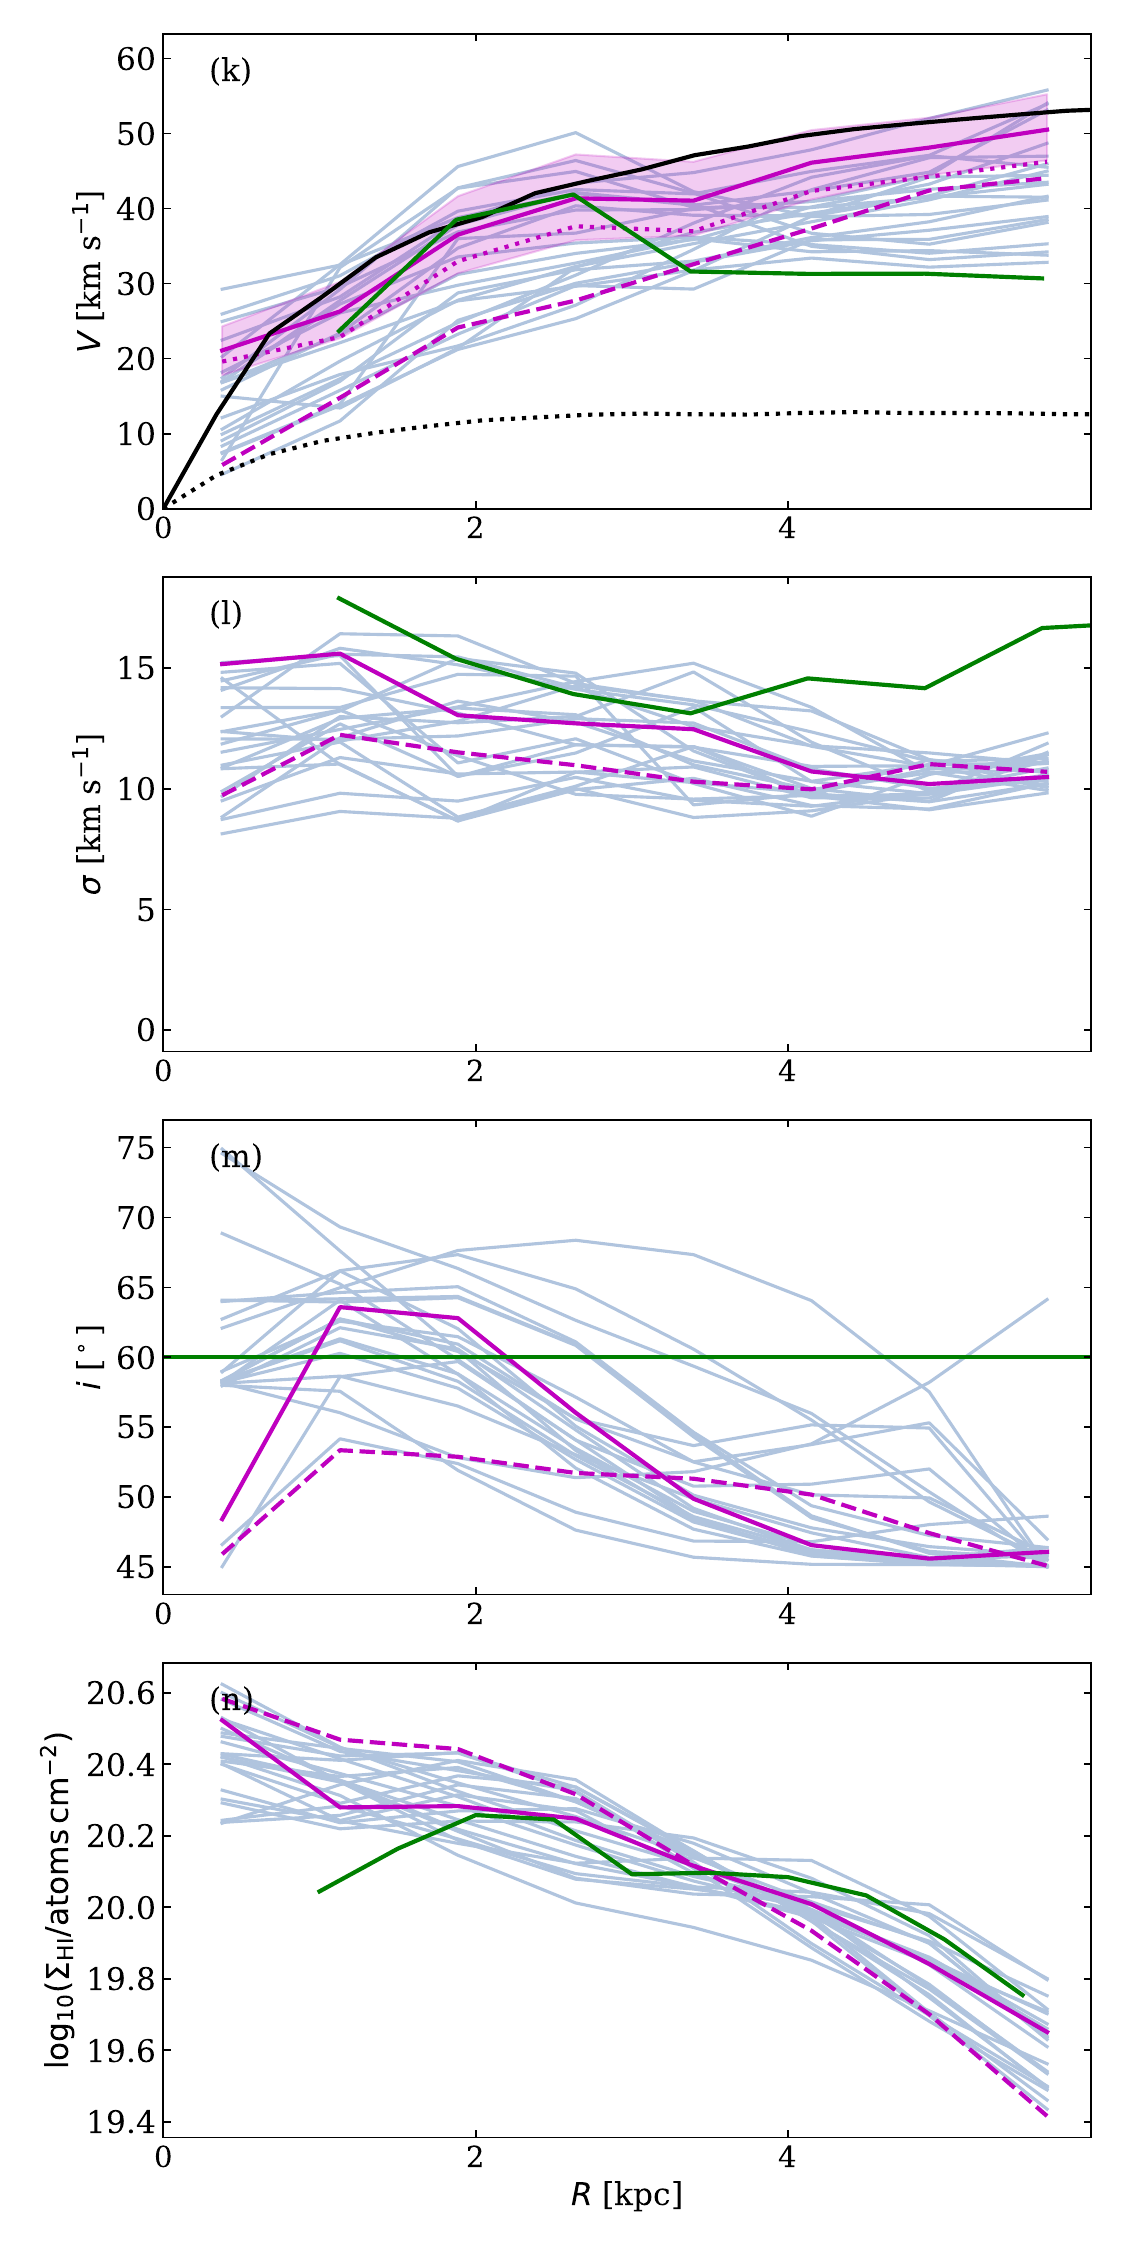}
\end{minipage}
\caption{A set of summary figures for galaxy LT-60, selected for kinematic analysis. These include example moment maps for two orientations (panels (a)--(f); similar to Fig.~\ref{fig:visualisations}), a summary of the parameters $V_\mathrm{fid}$, $V_\mathrm{max}$, $\eta_\mathrm{rot}$, and $\eta_\mathrm{bar}$ (panels (g)--(j); similar to Fig.~\ref{fig:loops}), and a summary of the rotation curve analysis from $24$ viewing angles (panels (k)--(n); similar to Fig.~\ref{fig:rot_curves}). See description of Appendix~\ref{app:supplementary} for details.}
\label{fig:S19}
\end{figure}
\clearpage

\begin{figure}
\begin{minipage}{.9\textwidth}
\includegraphics[width=\textwidth]{../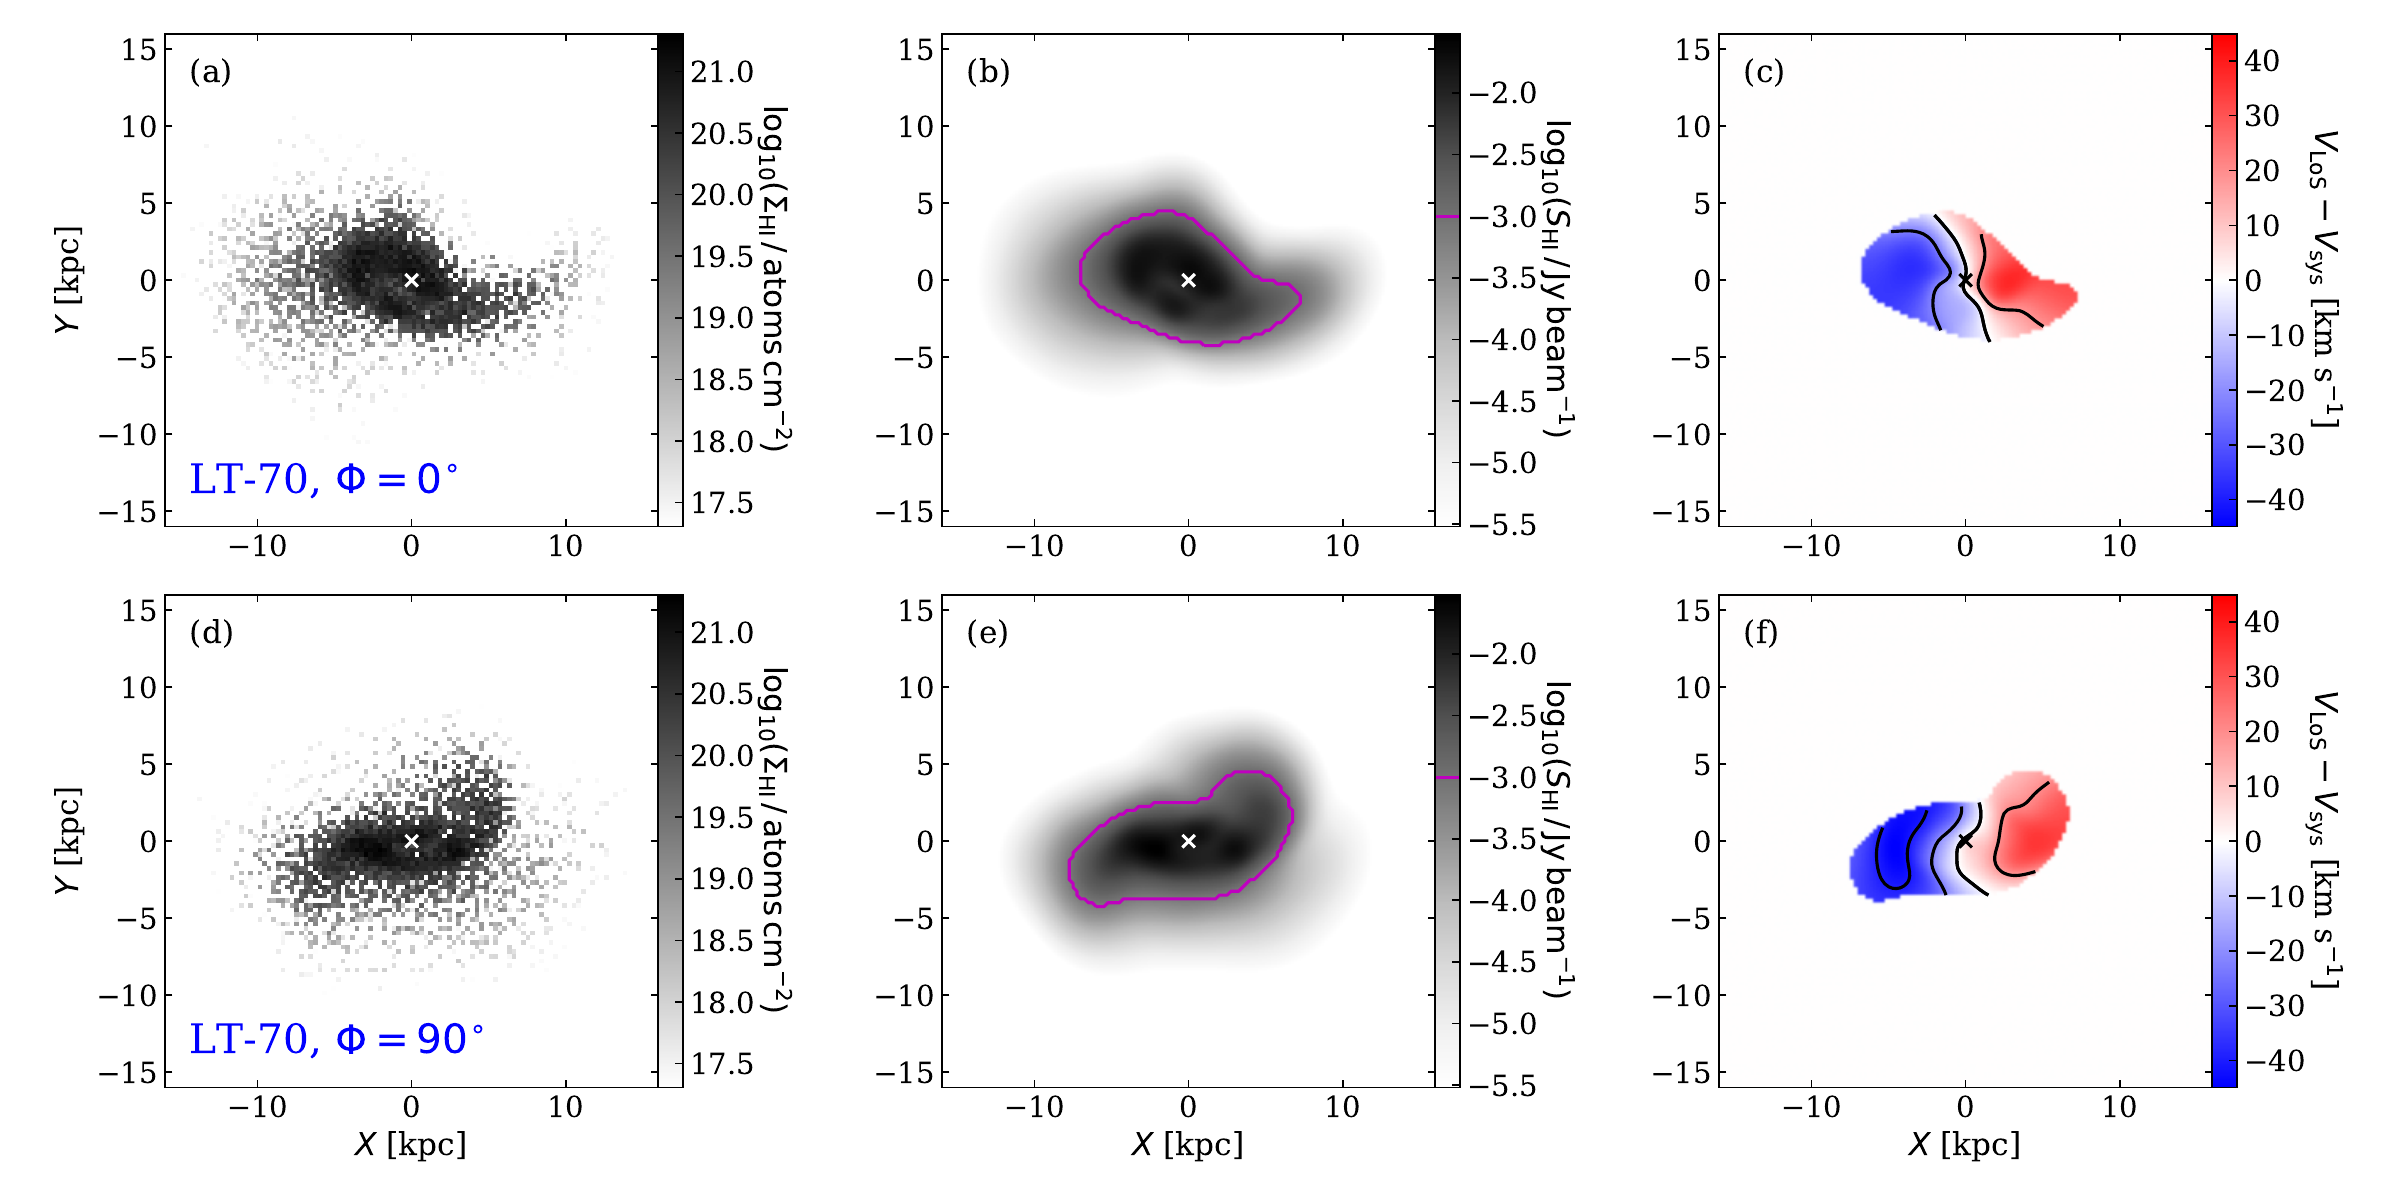}
\includegraphics[width=\textwidth]{../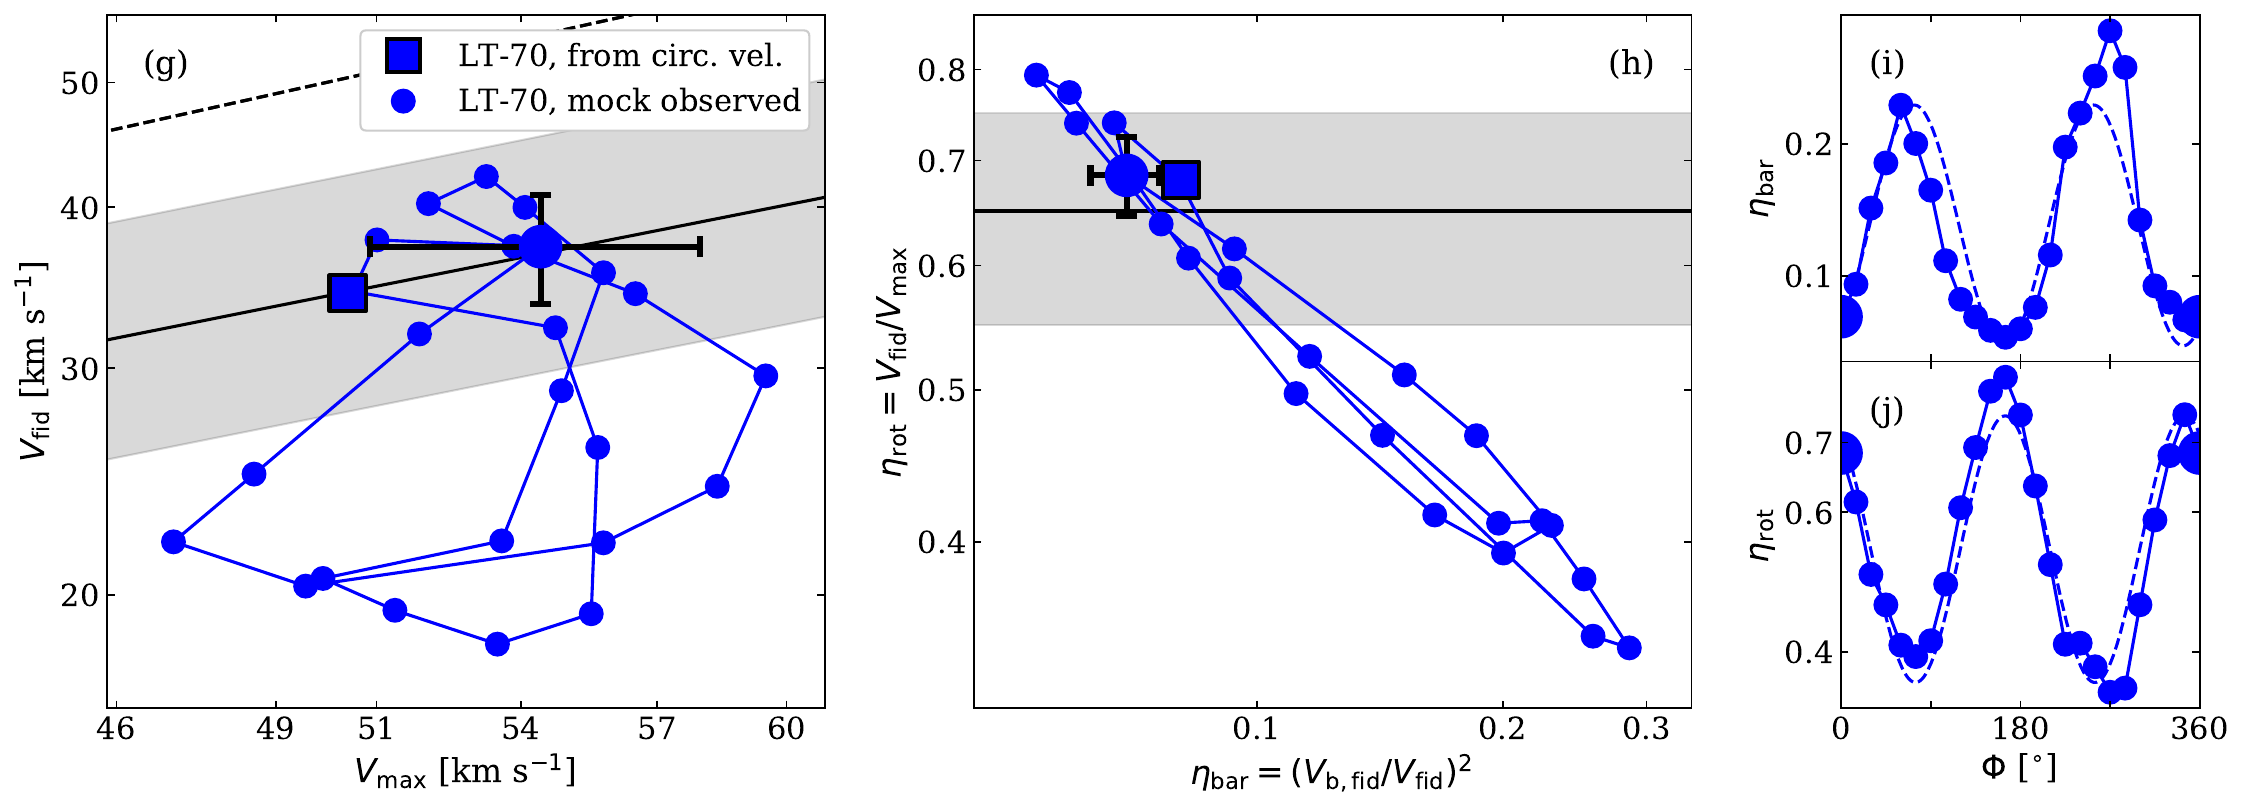}
\end{minipage}
\begin{minipage}{.4\textwidth}
\includegraphics[width=\textwidth]{../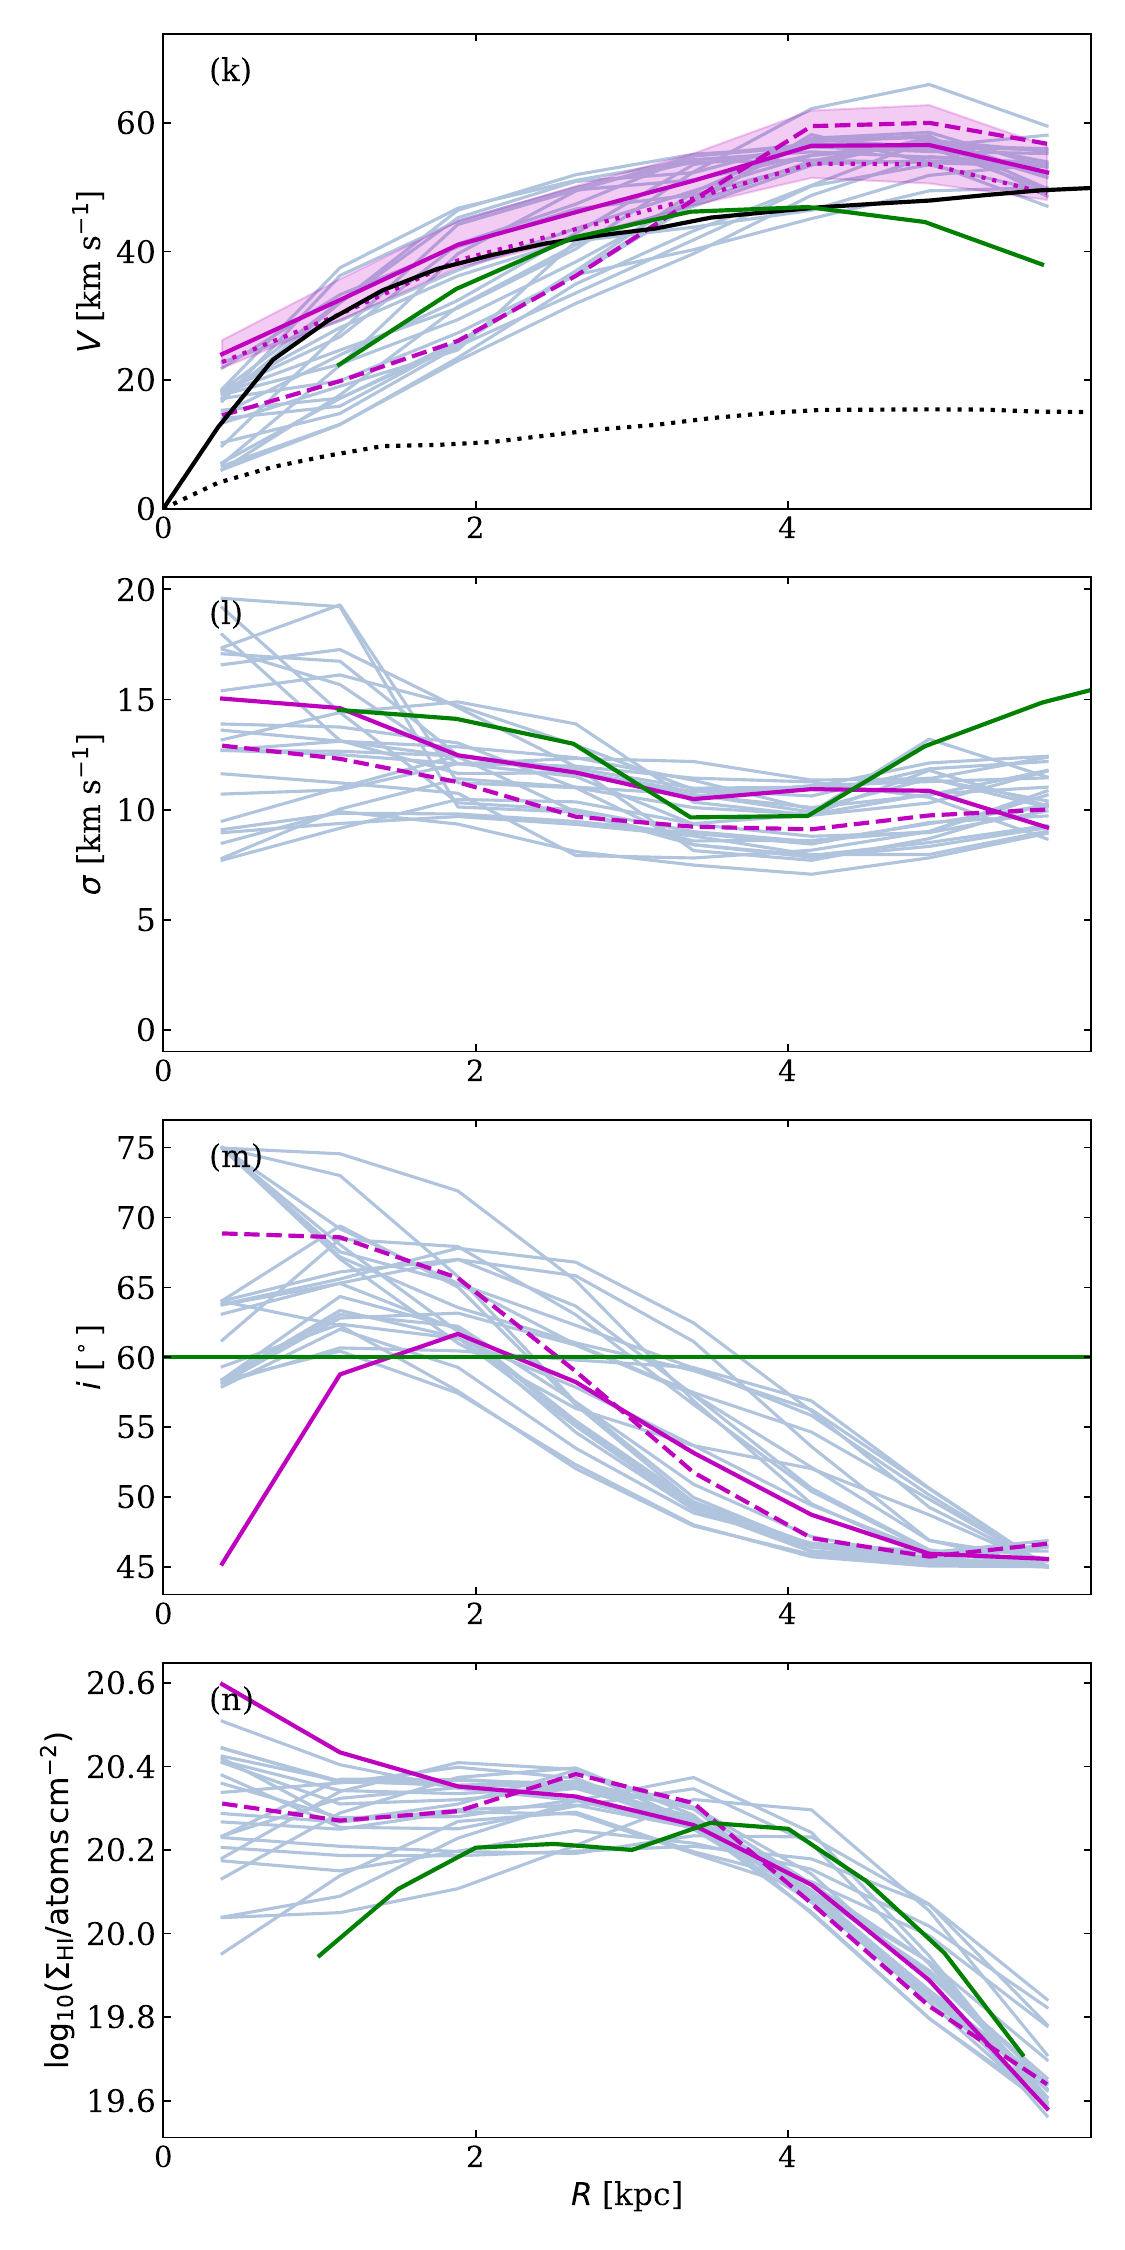}
\end{minipage}
\caption{A set of summary figures for galaxy LT-70, selected for kinematic analysis. These include example moment maps for two orientations (panels (a)--(f); similar to Fig.~\ref{fig:visualisations}), a summary of the parameters $V_\mathrm{fid}$, $V_\mathrm{max}$, $\eta_\mathrm{rot}$, and $\eta_\mathrm{bar}$ (panels (g)--(j); similar to Fig.~\ref{fig:loops}), and a summary of the rotation curve analysis from $24$ viewing angles (panels (k)--(n); similar to Fig.~\ref{fig:rot_curves}). See description of Appendix~\ref{app:supplementary} for details.}
\label{fig:S20}
\end{figure}
\clearpage

\begin{figure}
\begin{minipage}{.9\textwidth}
\includegraphics[width=\textwidth]{../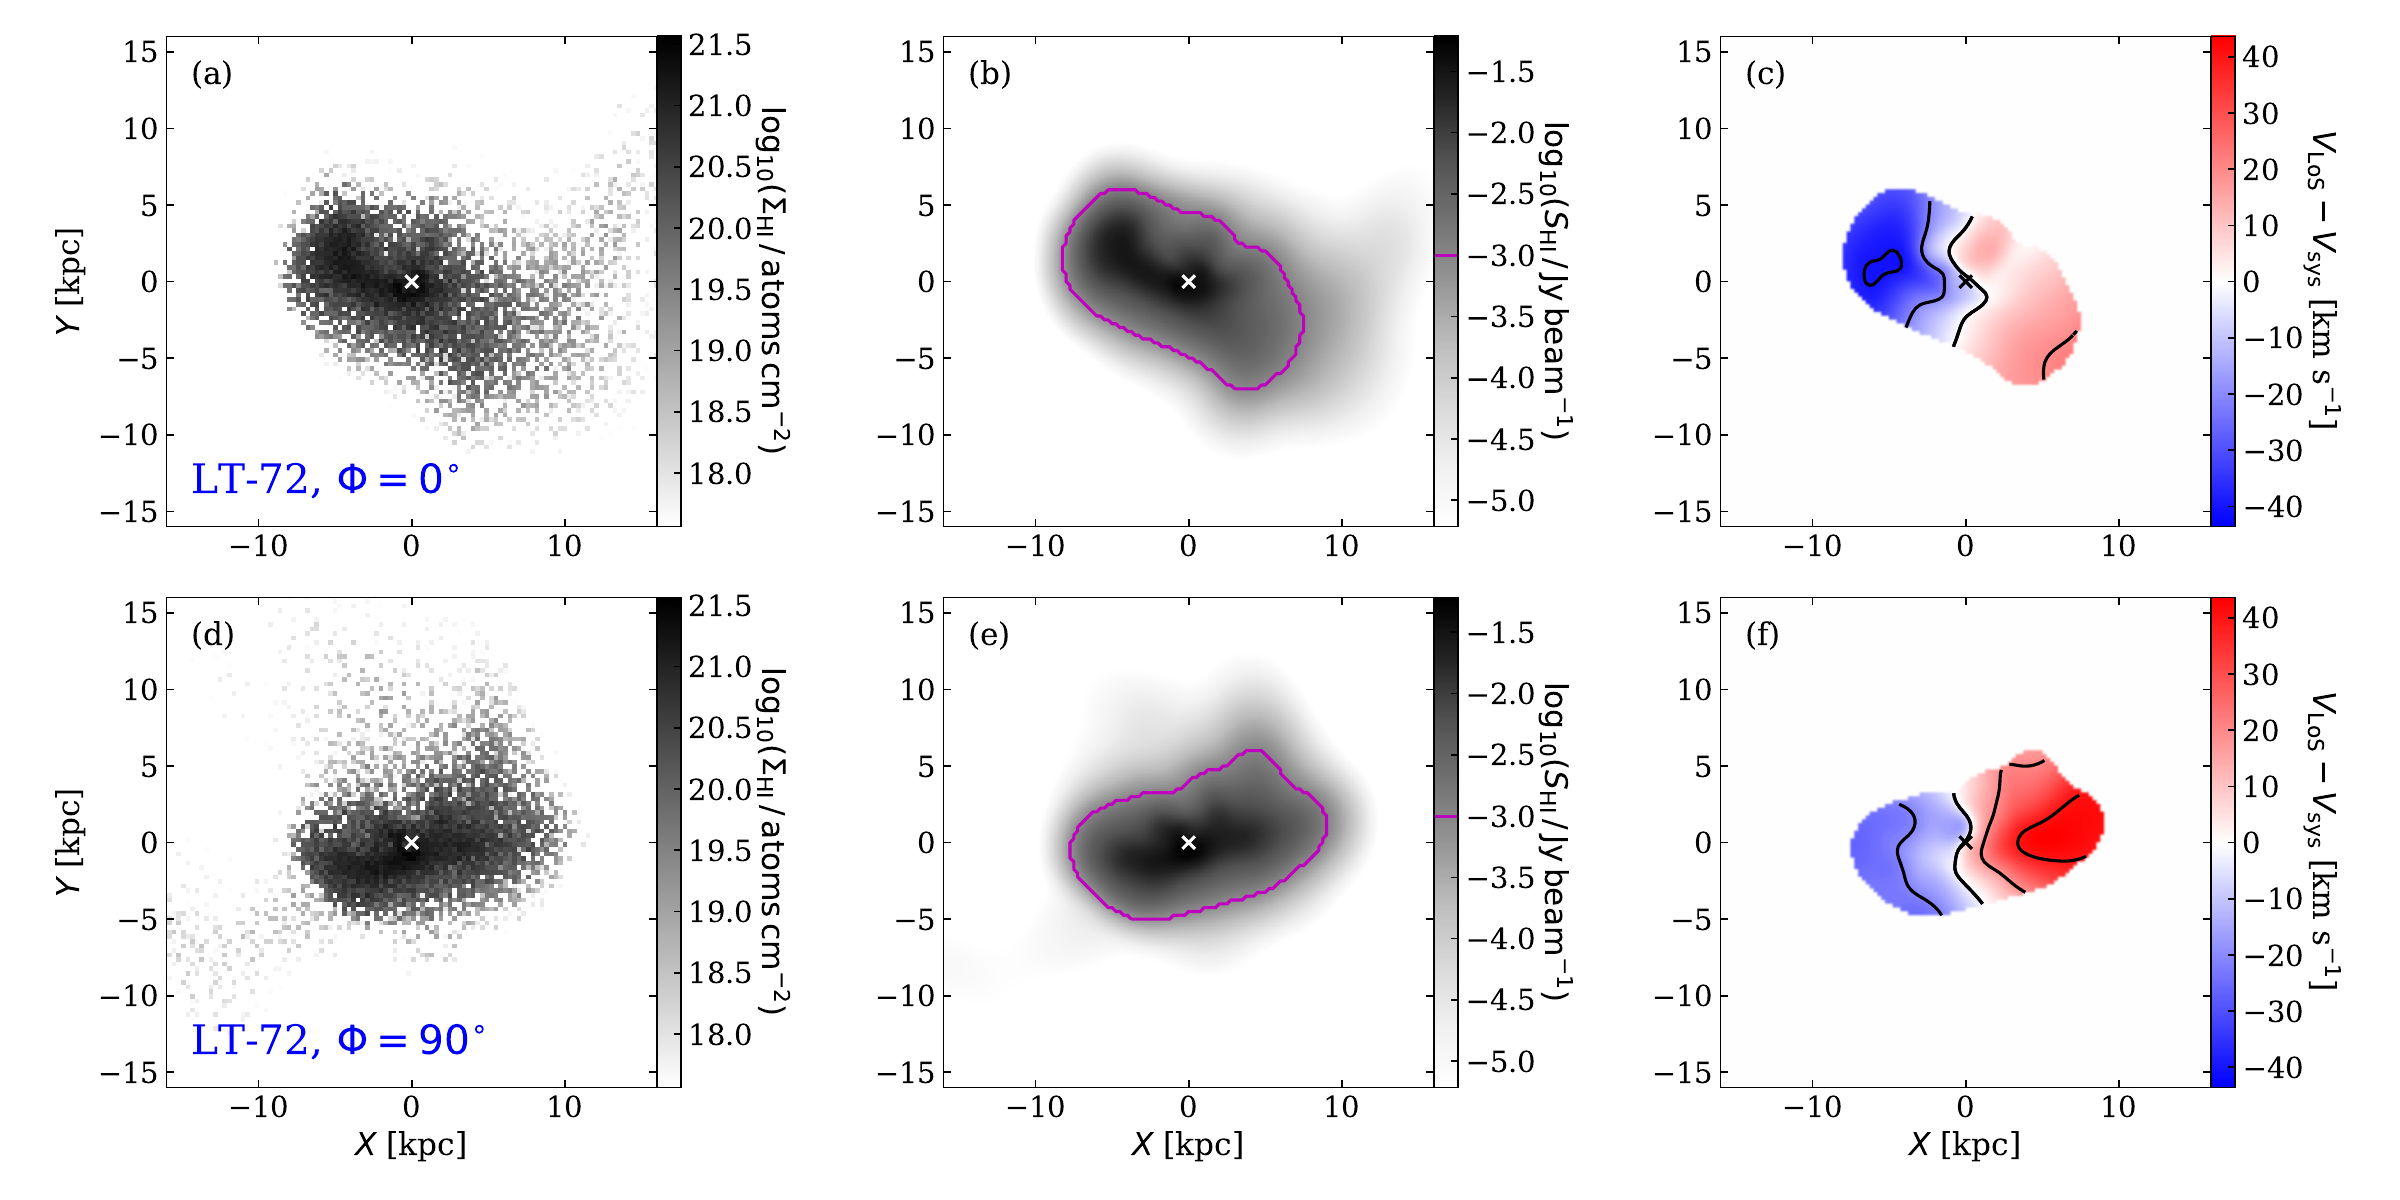}
\includegraphics[width=\textwidth]{../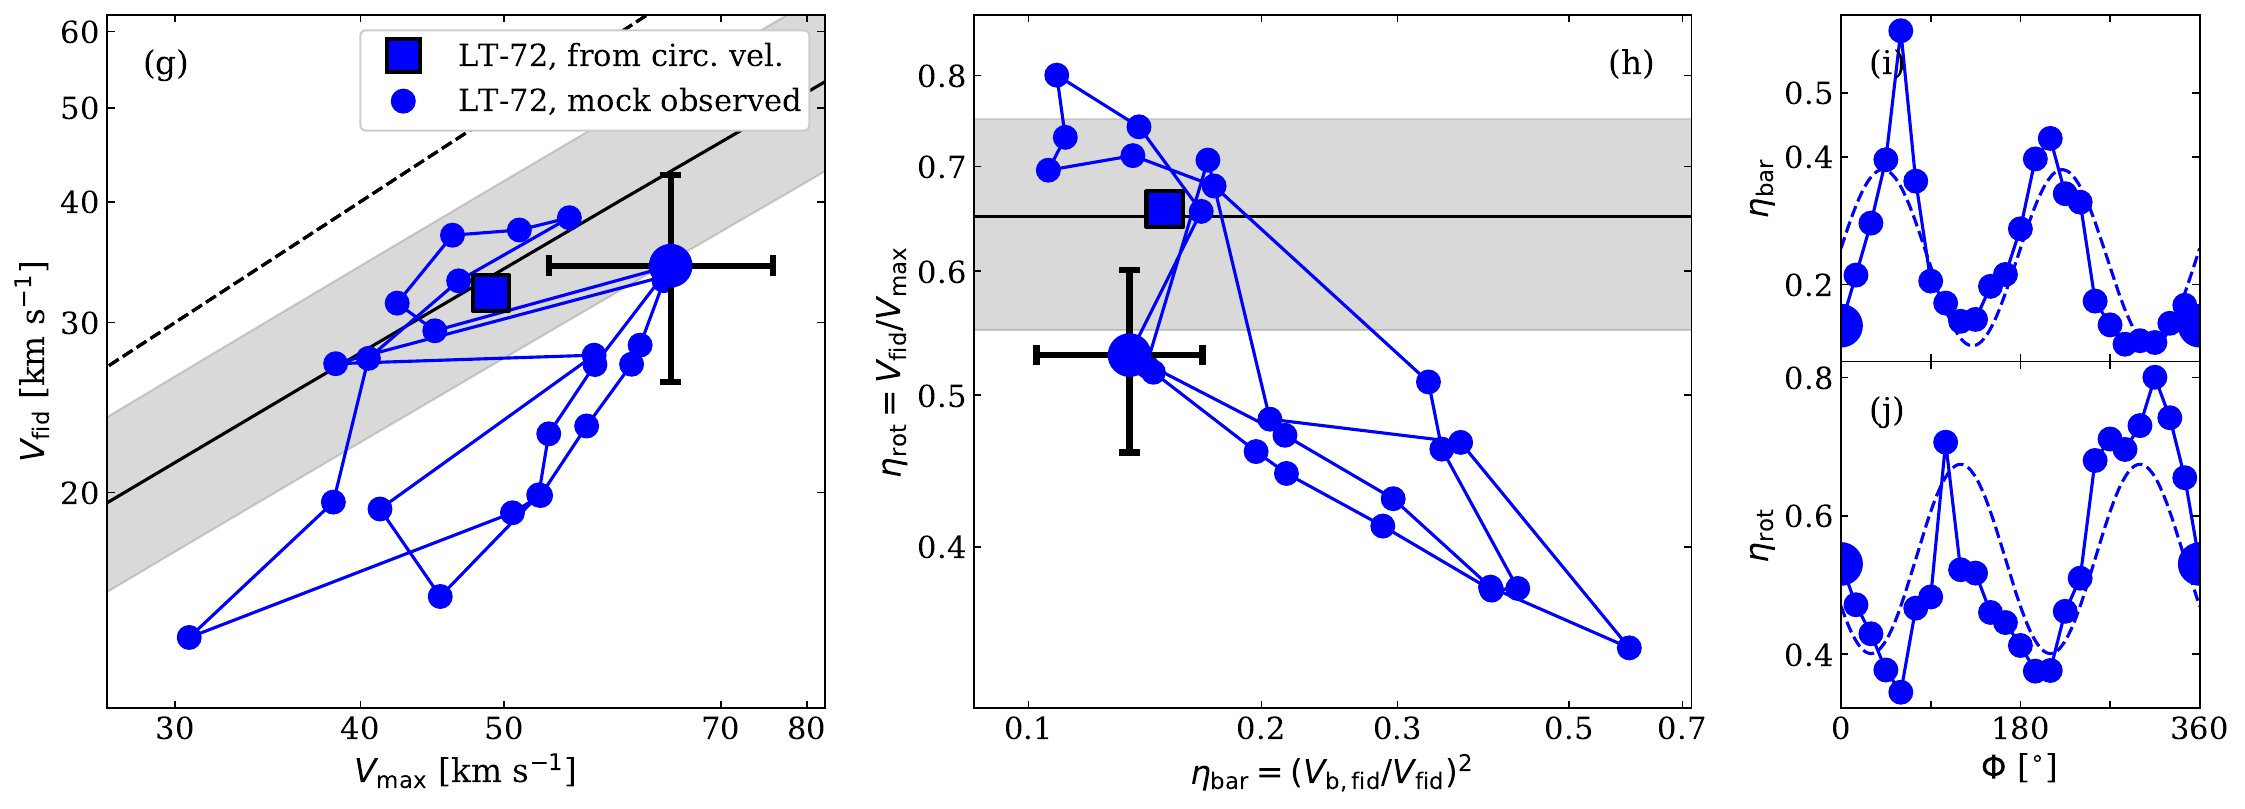}
\end{minipage}
\begin{minipage}{.4\textwidth}
\includegraphics[width=\textwidth]{../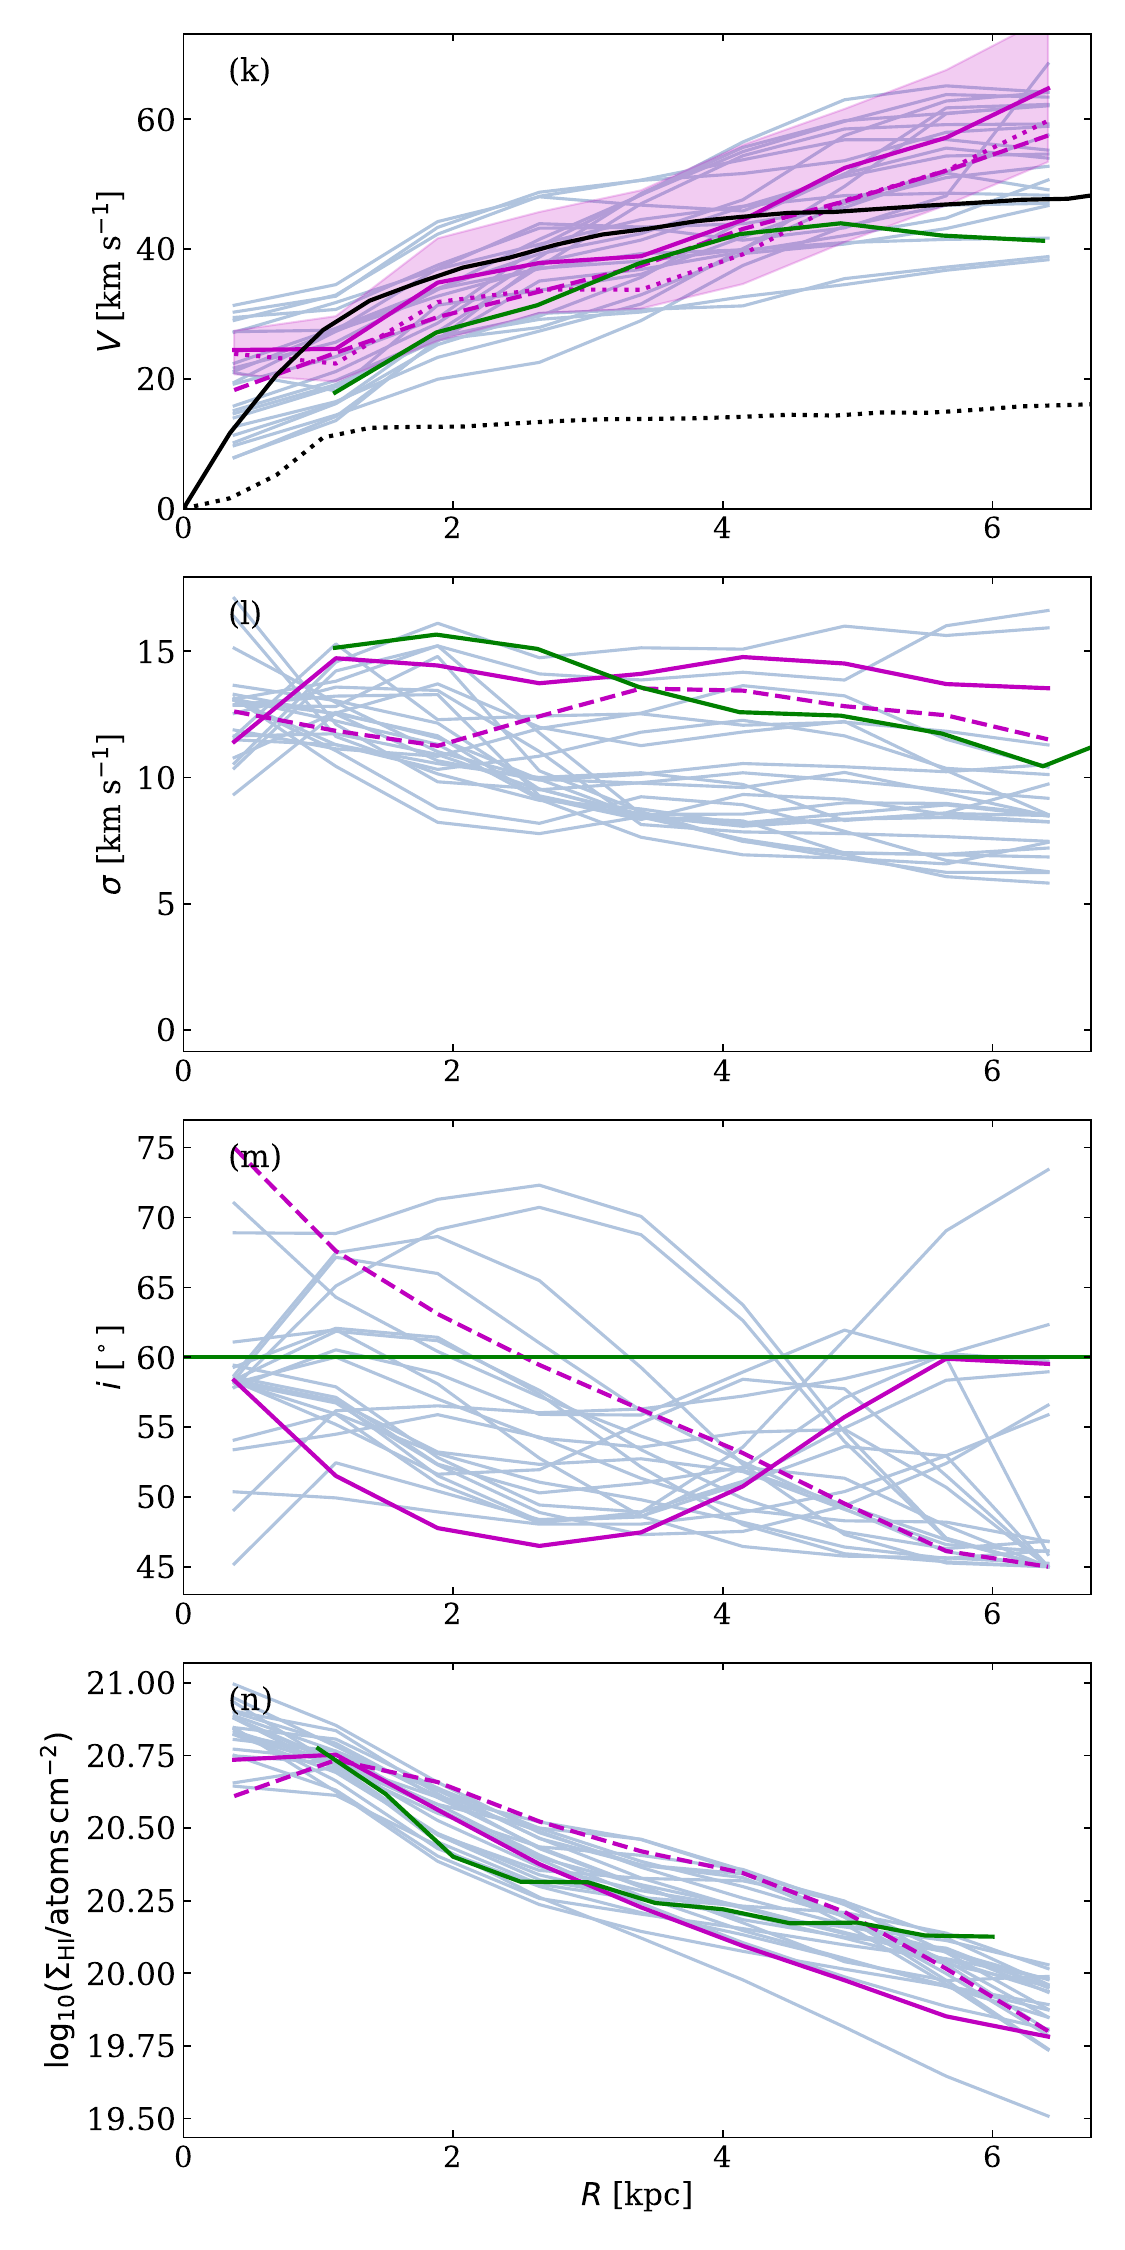}
\end{minipage}
\caption{A set of summary figures for galaxy LT-72, selected for kinematic analysis. These include example moment maps for two orientations (panels (a)--(f); similar to Fig.~\ref{fig:visualisations}), a summary of the parameters $V_\mathrm{fid}$, $V_\mathrm{max}$, $\eta_\mathrm{rot}$, and $\eta_\mathrm{bar}$ (panels (g)--(j); similar to Fig.~\ref{fig:loops}), and a summary of the rotation curve analysis from $24$ viewing angles (panels (k)--(n); similar to Fig.~\ref{fig:rot_curves}). See description of Appendix~\ref{app:supplementary} for details.}
\label{fig:S21}
\end{figure}
\clearpage

\begin{figure}
\begin{minipage}{.9\textwidth}
\includegraphics[width=\textwidth]{../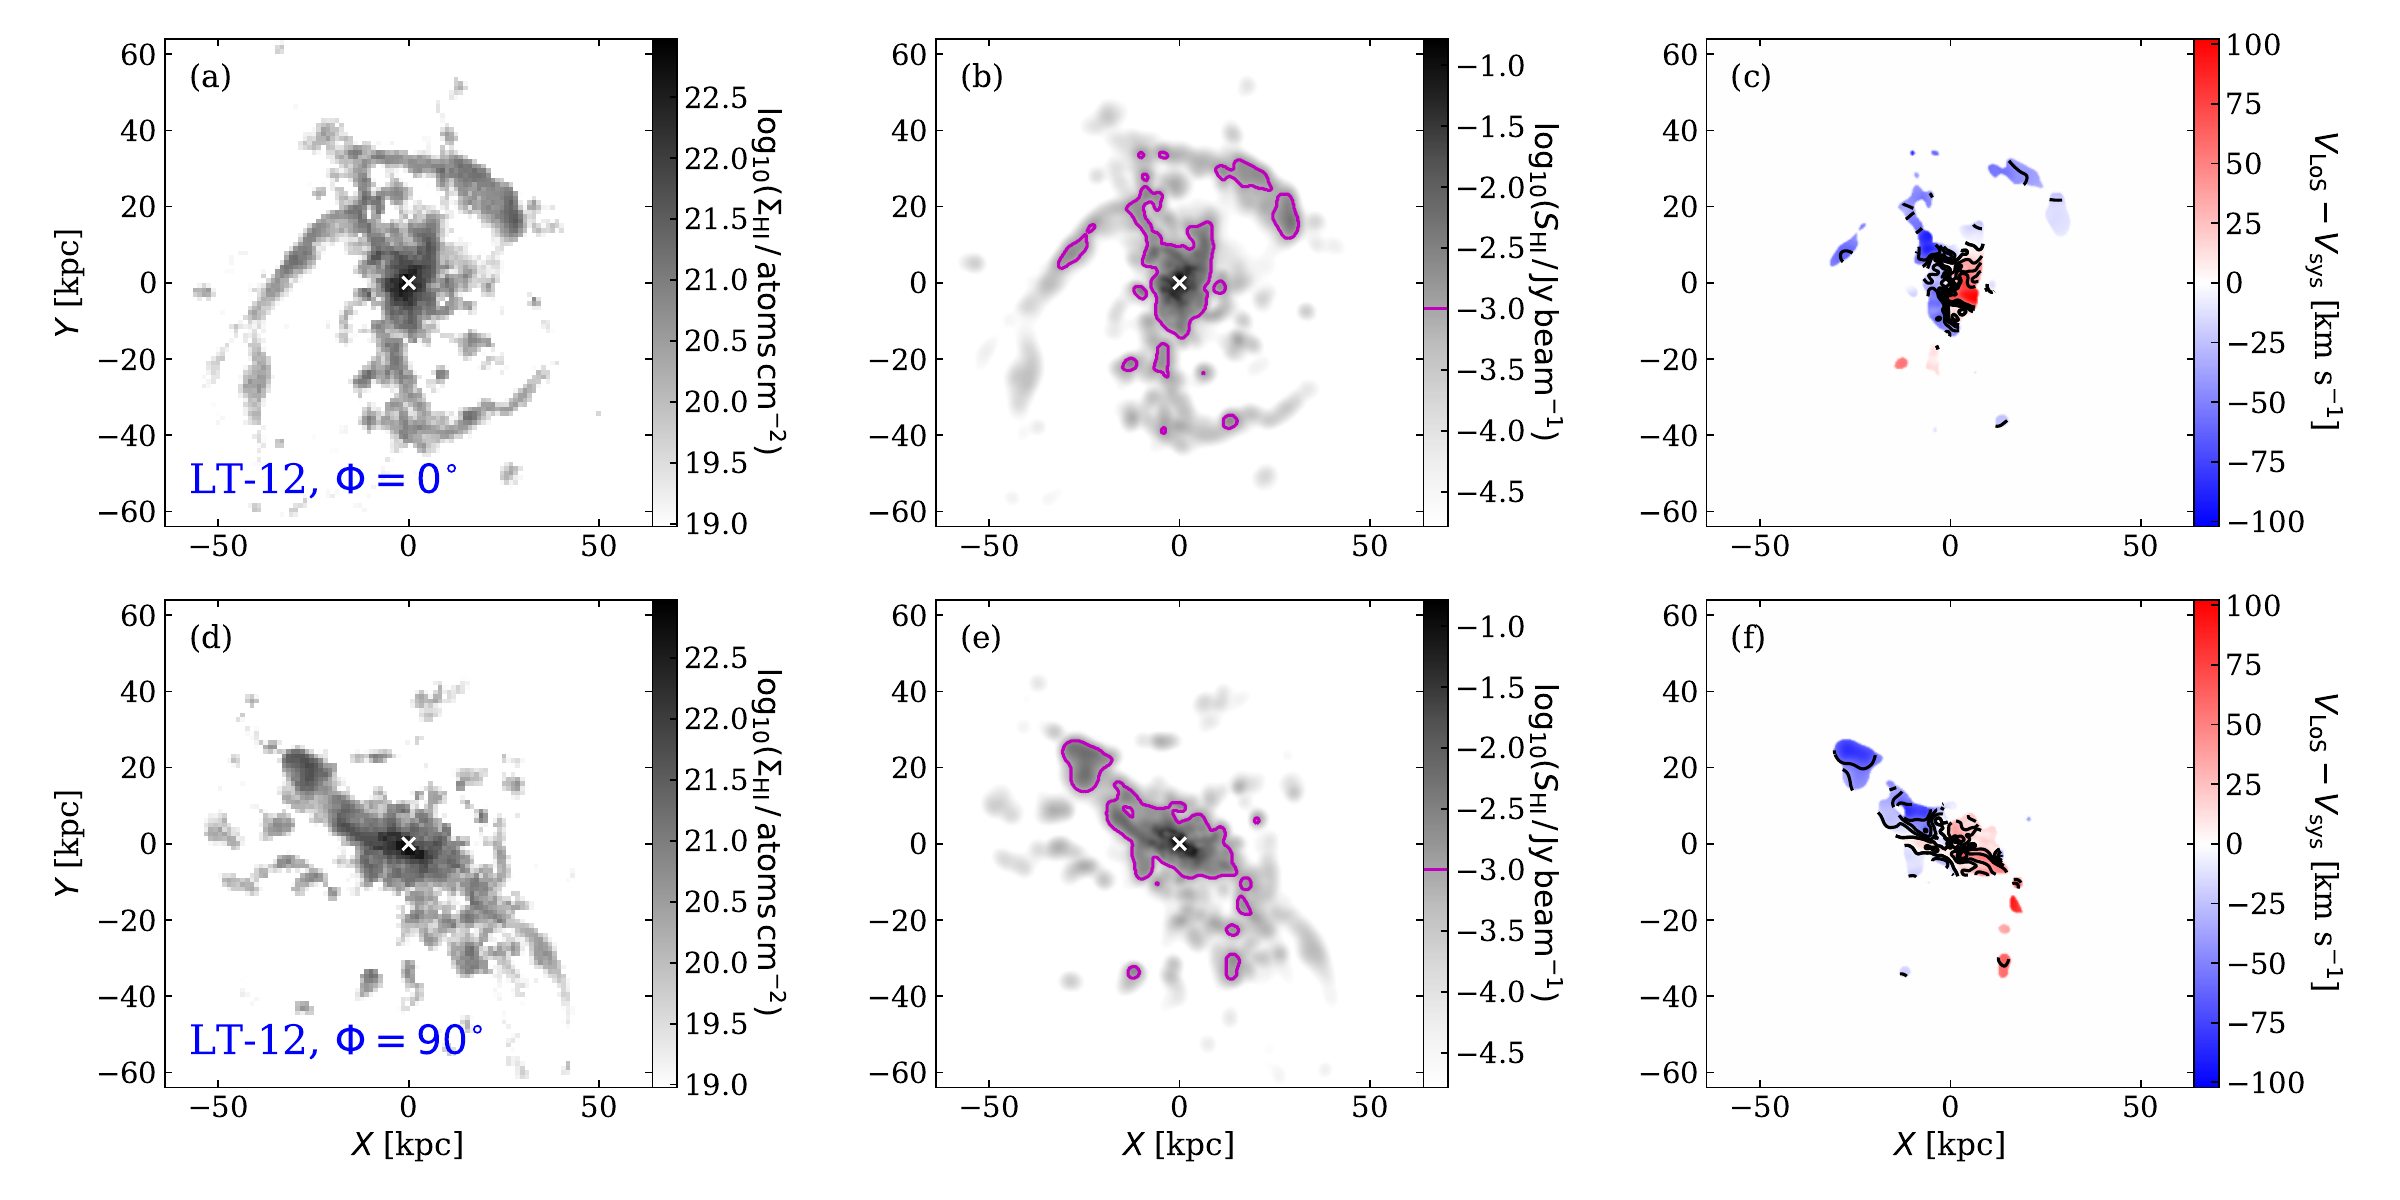}
\includegraphics[width=\textwidth]{../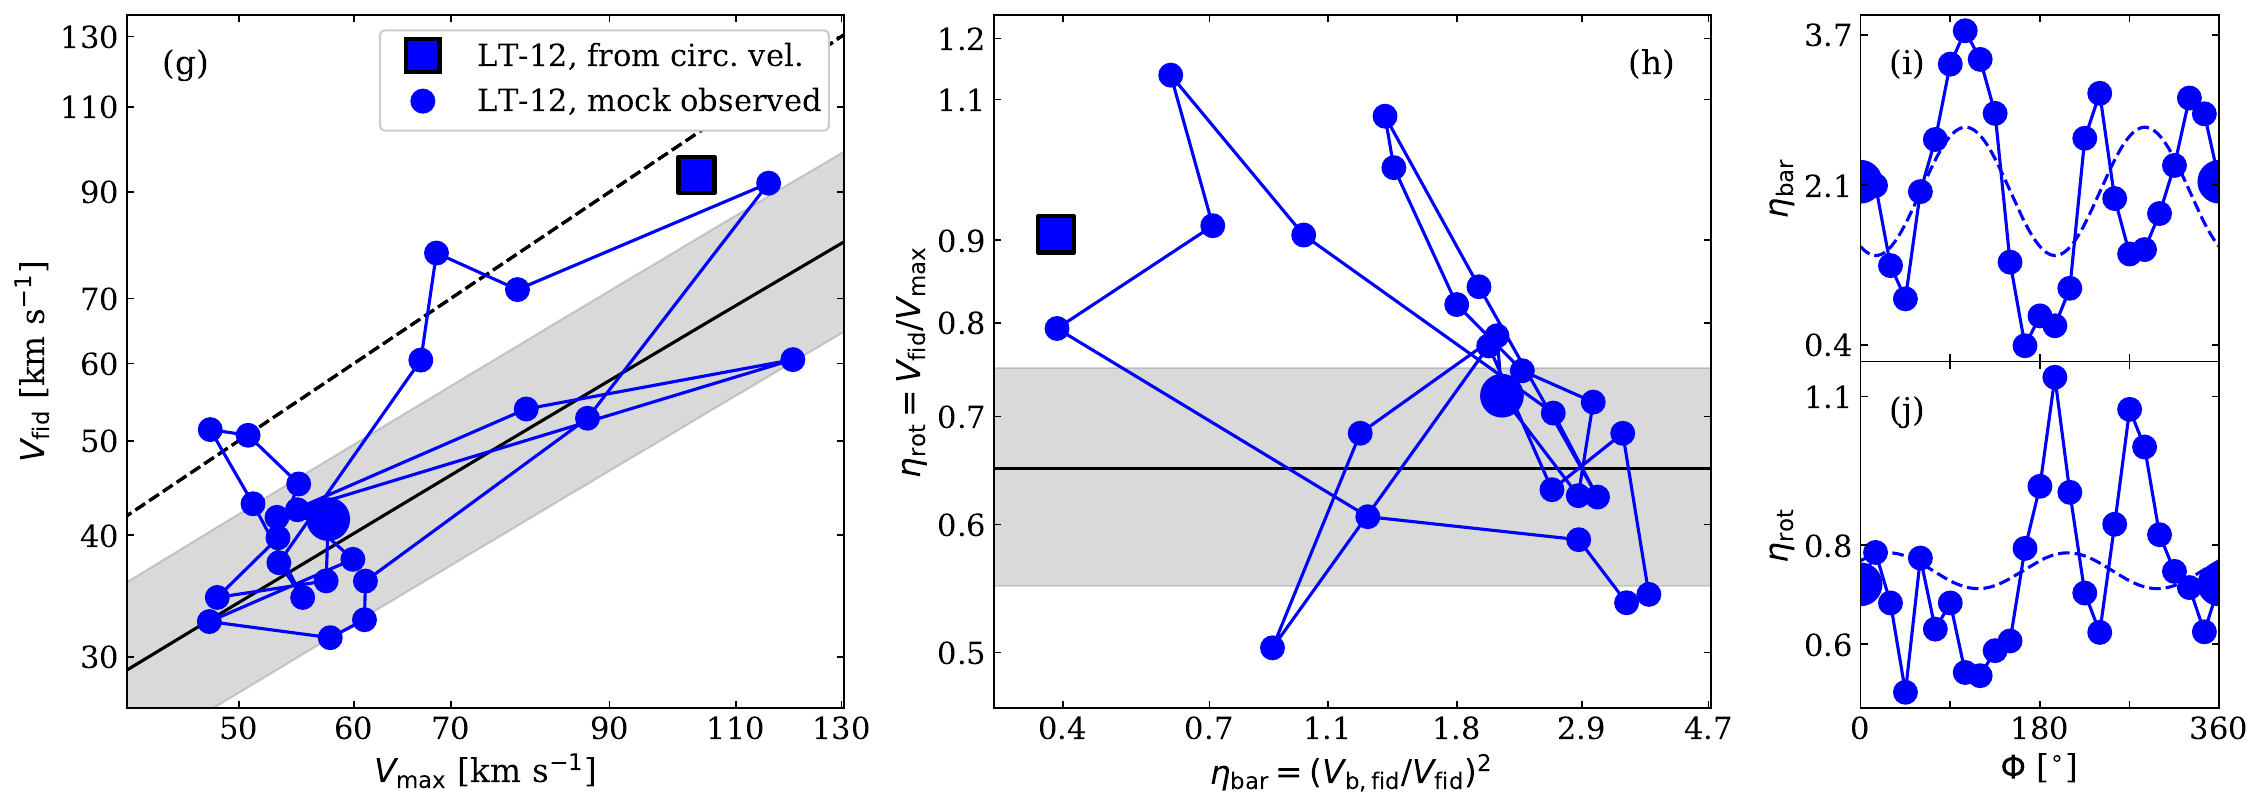}
\end{minipage}
\begin{minipage}{.4\textwidth}
\includegraphics[width=\textwidth]{../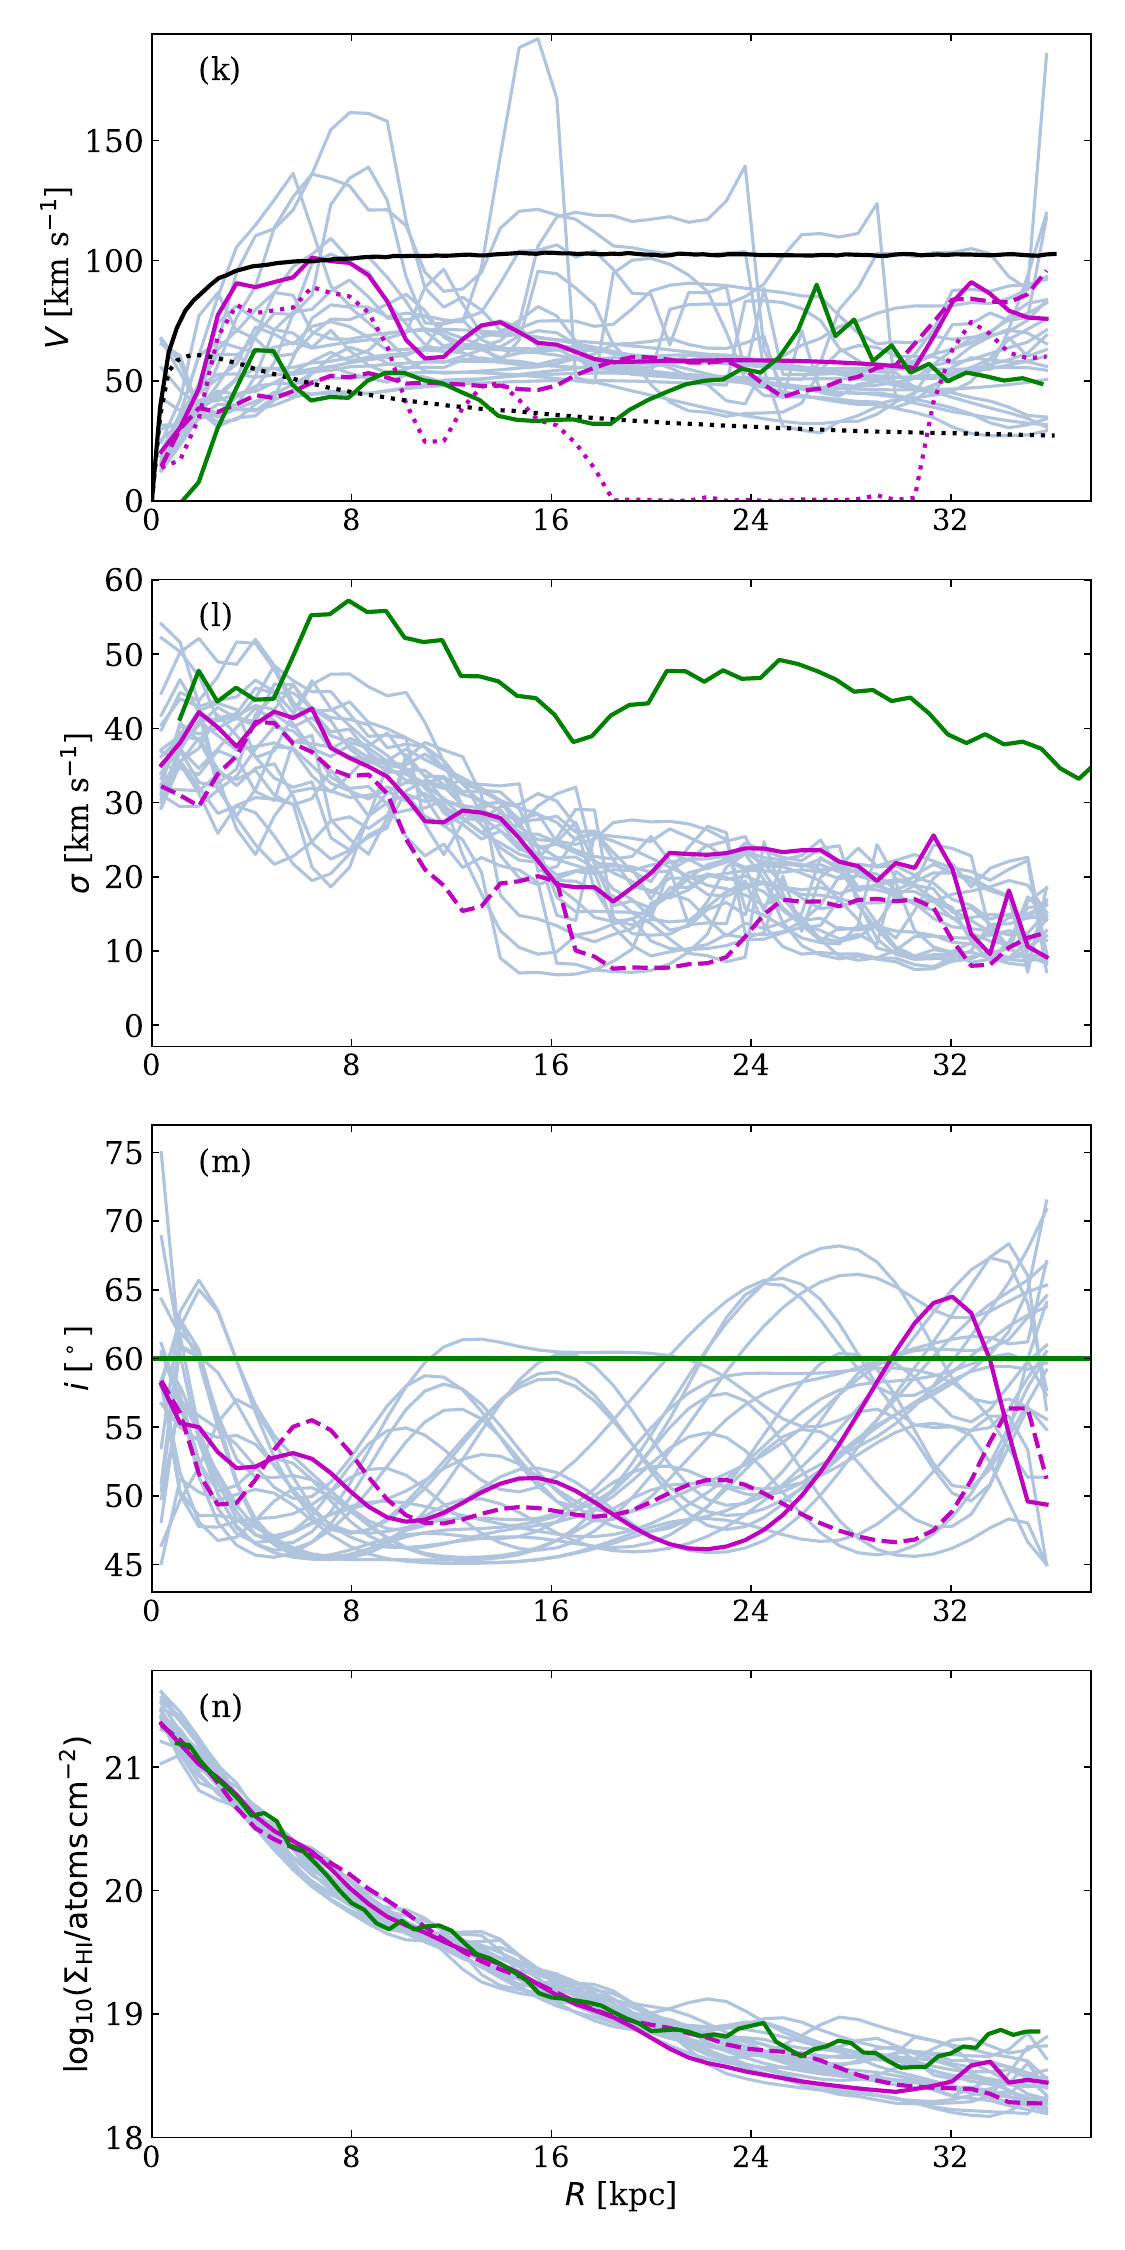}
\end{minipage}
\caption{A set of summary figures for galaxy LT-12, excluded from kinematic analysis. These include example moment maps for two orientations (panels (a)--(f); similar to Fig.~\ref{fig:visualisations}), a summary of the parameters $V_\mathrm{fid}$, $V_\mathrm{max}$, $\eta_\mathrm{rot}$, and $\eta_\mathrm{bar}$ (panels (g)--(j); similar to Fig.~\ref{fig:loops}), and a summary of the rotation curve analysis from $24$ viewing angles (panels (k)--(n); similar to Fig.~\ref{fig:rot_curves}). See description of Appendix~\ref{app:supplementary} for details.}
\label{fig:S22}
\end{figure}
\clearpage

\begin{figure}
\begin{minipage}{.9\textwidth}
\includegraphics[width=\textwidth]{../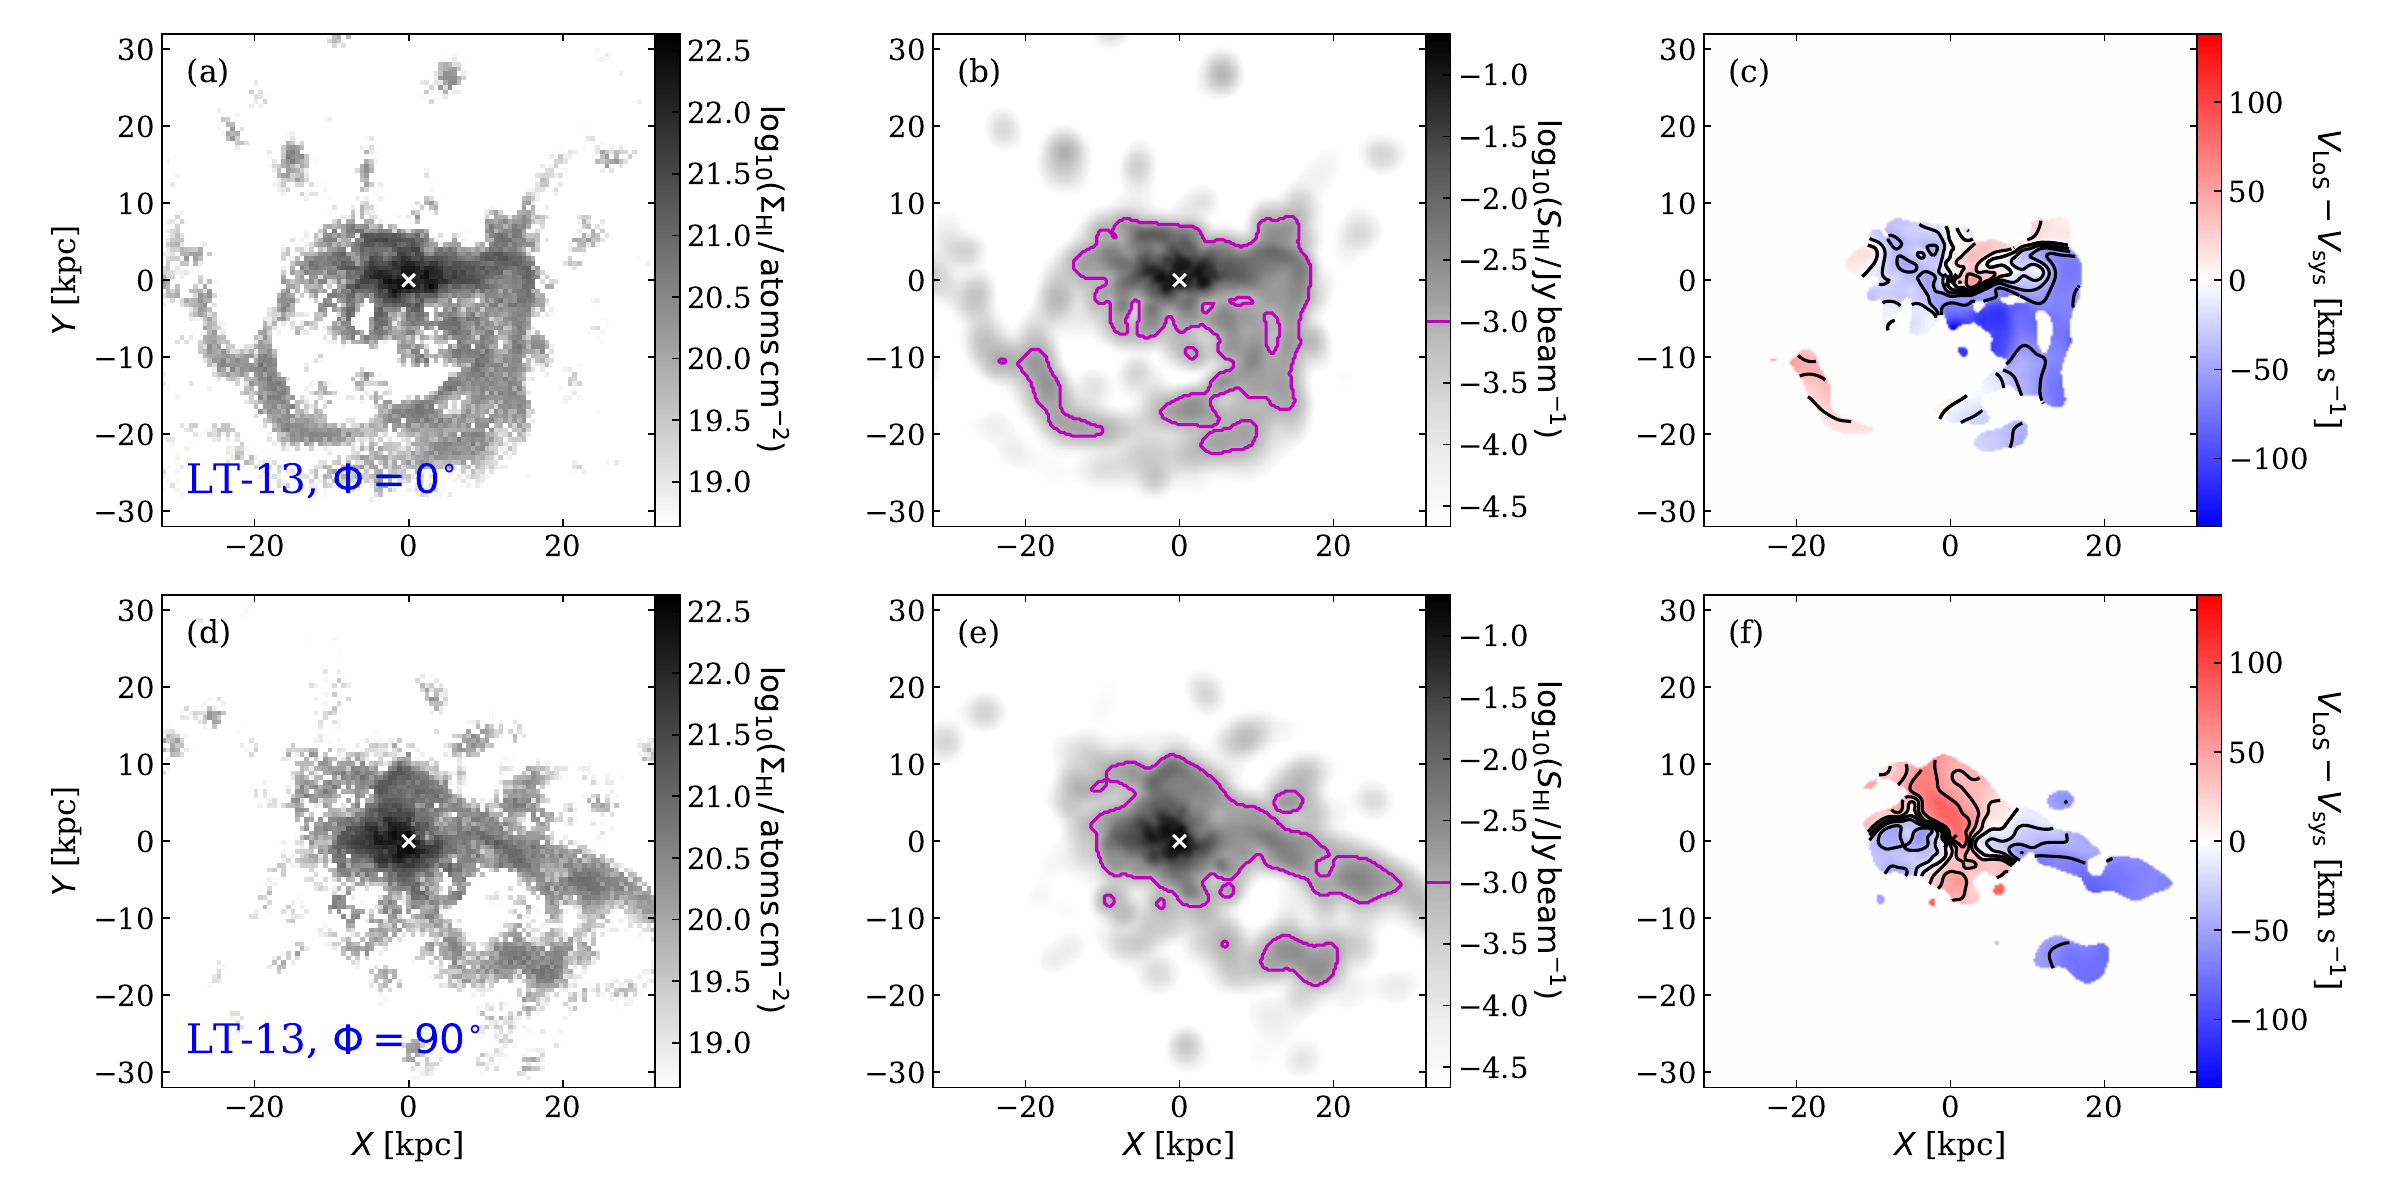}
\includegraphics[width=\textwidth]{../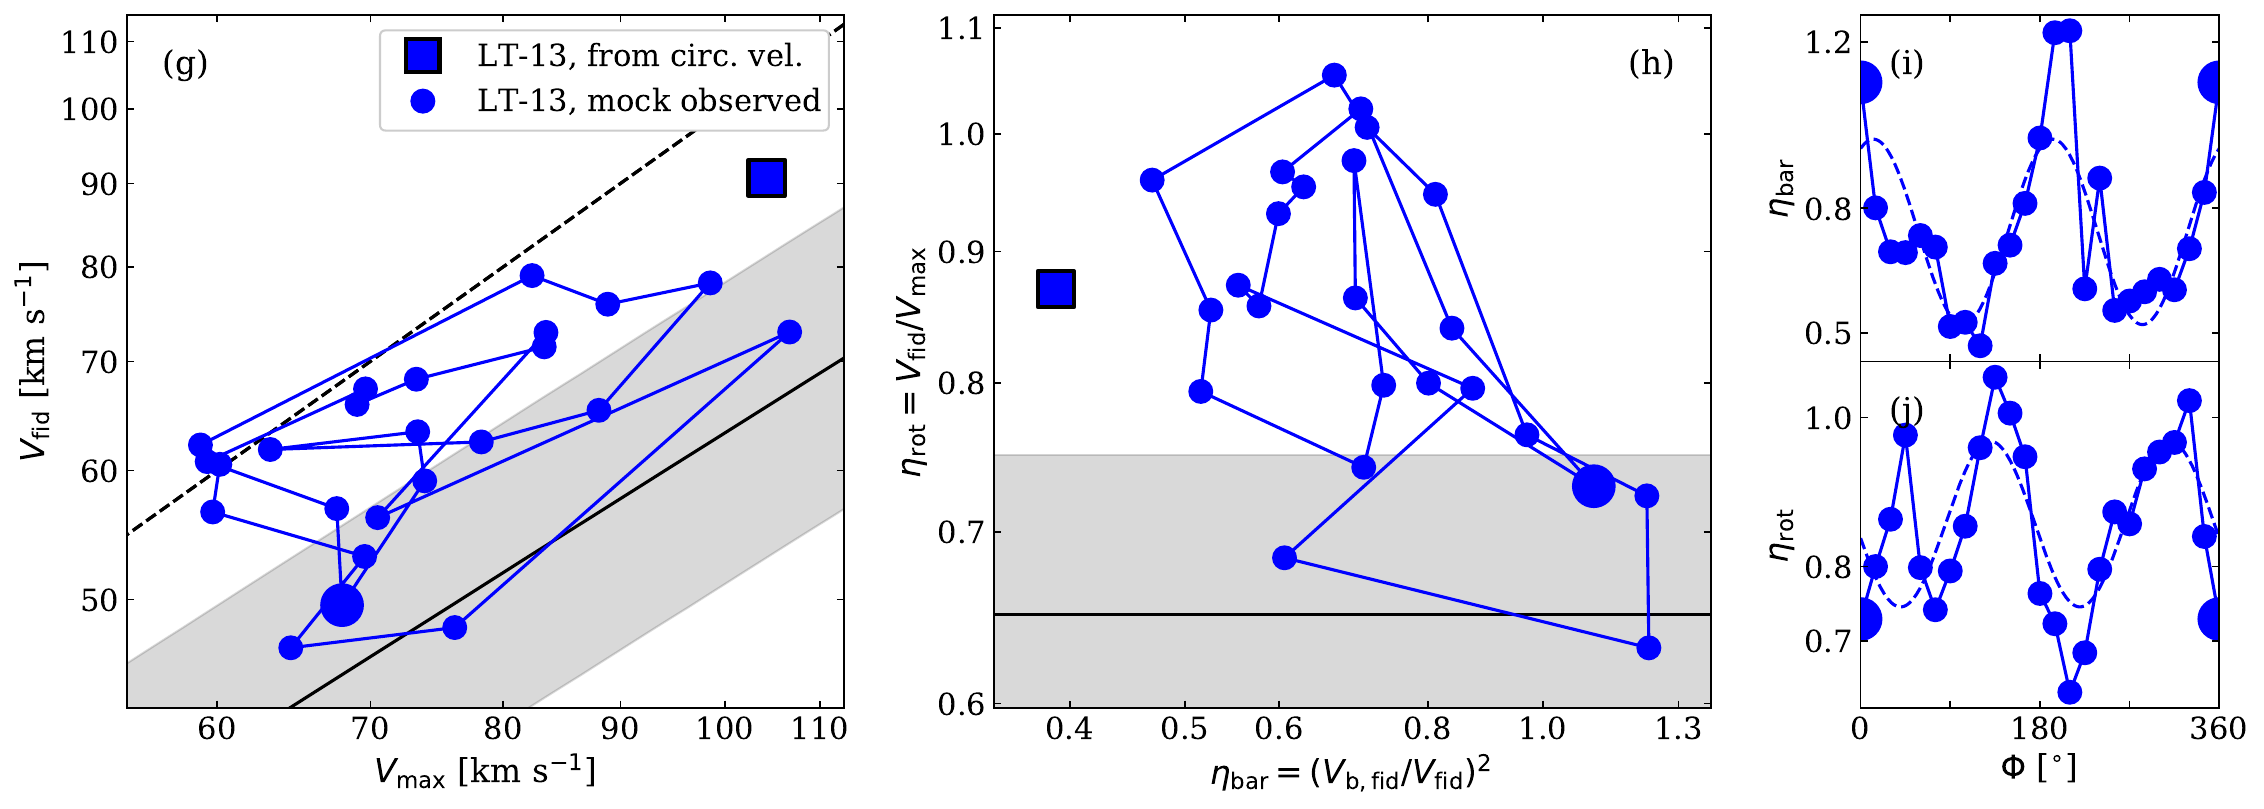}
\end{minipage}
\begin{minipage}{.4\textwidth}
\includegraphics[width=\textwidth]{../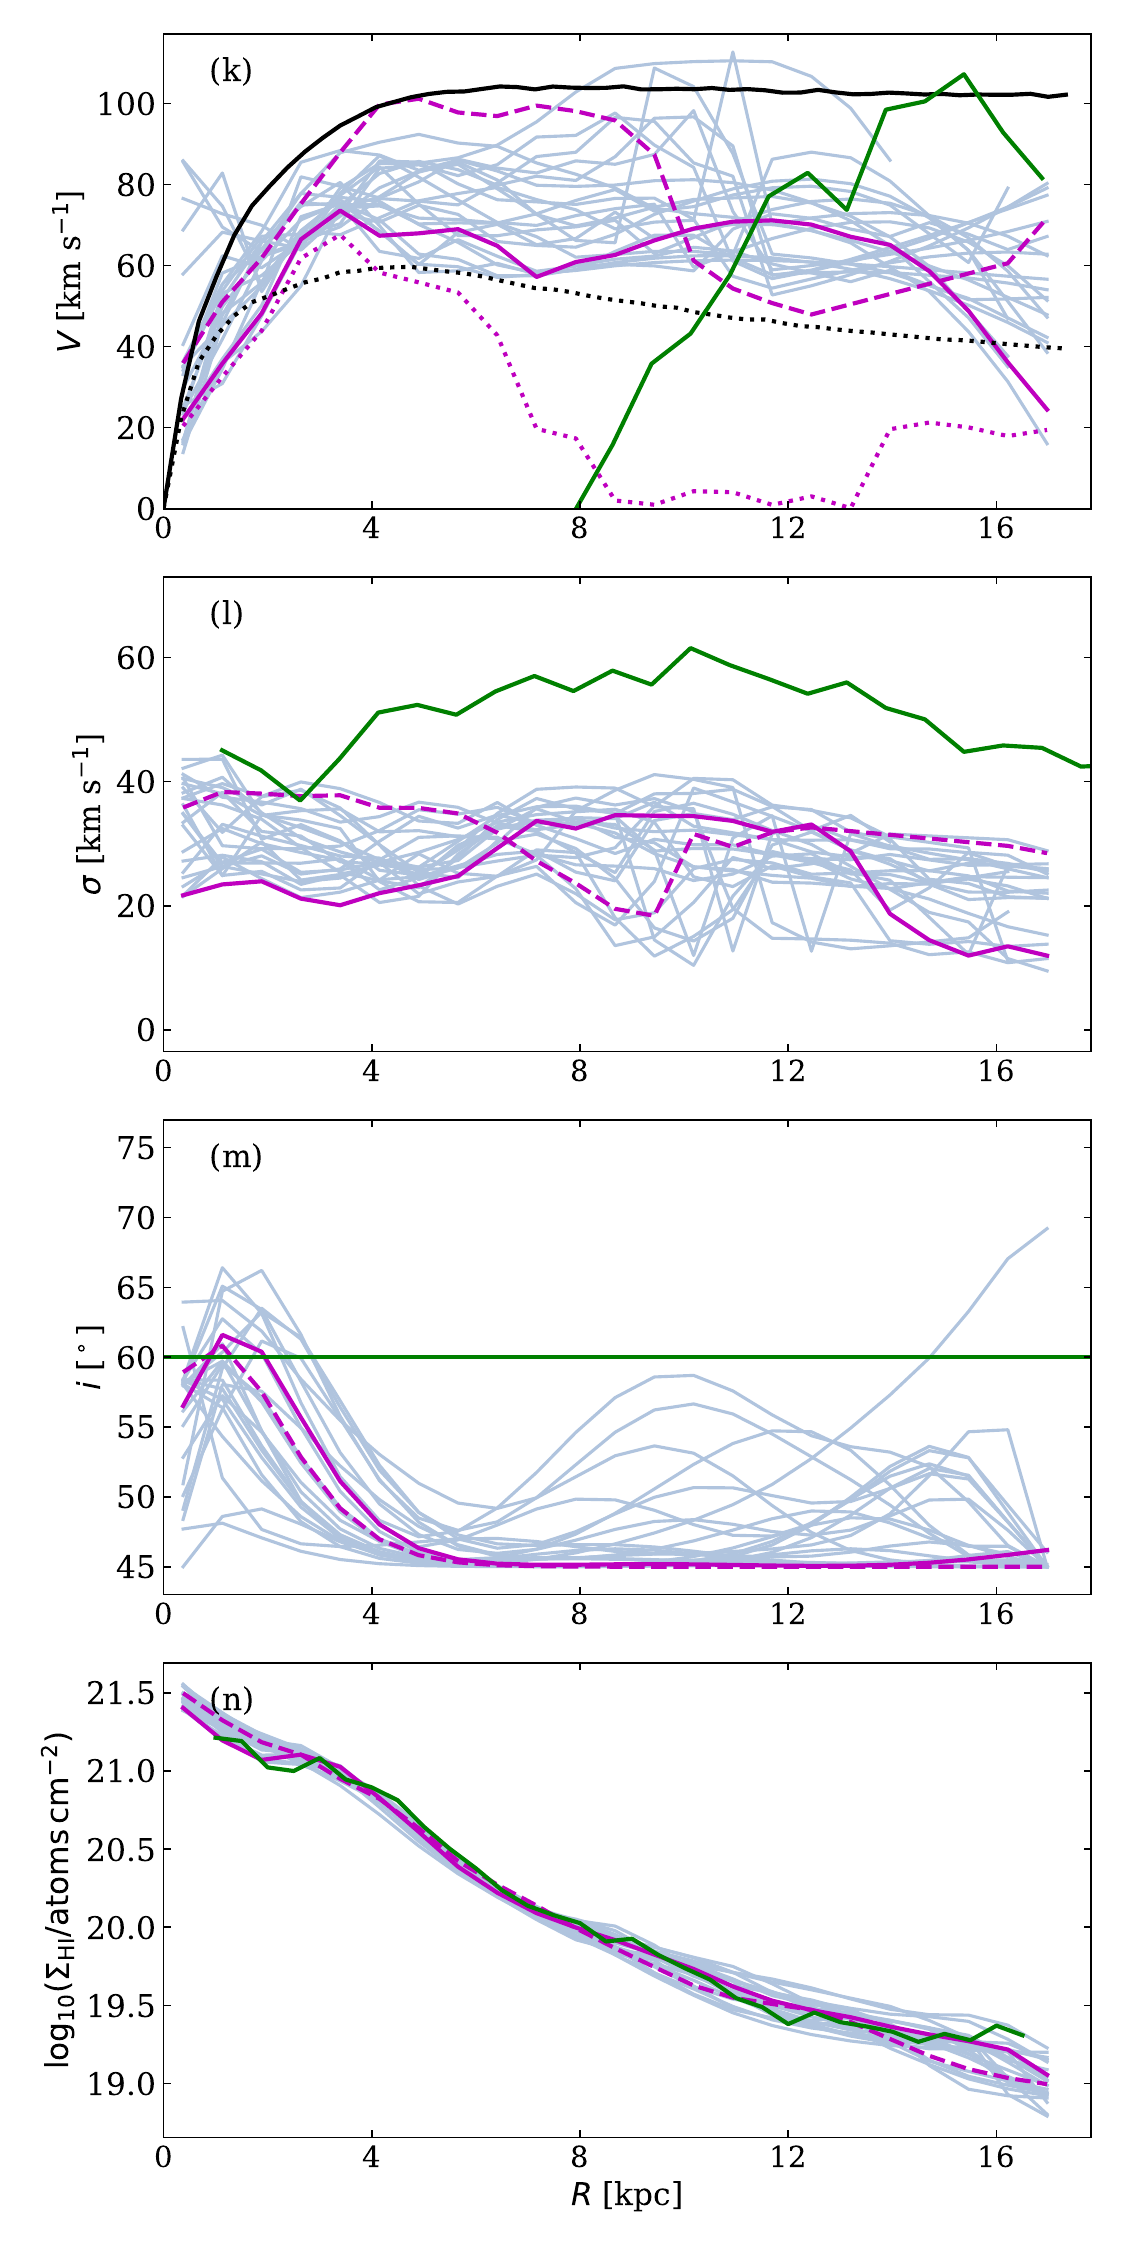}
\end{minipage}
\caption{A set of summary figures for galaxy LT-13, excluded from kinematic analysis. These include example moment maps for two orientations (panels (a)--(f); similar to Fig.~\ref{fig:visualisations}), a summary of the parameters $V_\mathrm{fid}$, $V_\mathrm{max}$, $\eta_\mathrm{rot}$, and $\eta_\mathrm{bar}$ (panels (g)--(j); similar to Fig.~\ref{fig:loops}), and a summary of the rotation curve analysis from $24$ viewing angles (panels (k)--(n); similar to Fig.~\ref{fig:rot_curves}). See description of Appendix~\ref{app:supplementary} for details.}
\label{fig:S23}
\end{figure}
\clearpage

\begin{figure}
\begin{minipage}{.9\textwidth}
\includegraphics[width=\textwidth]{../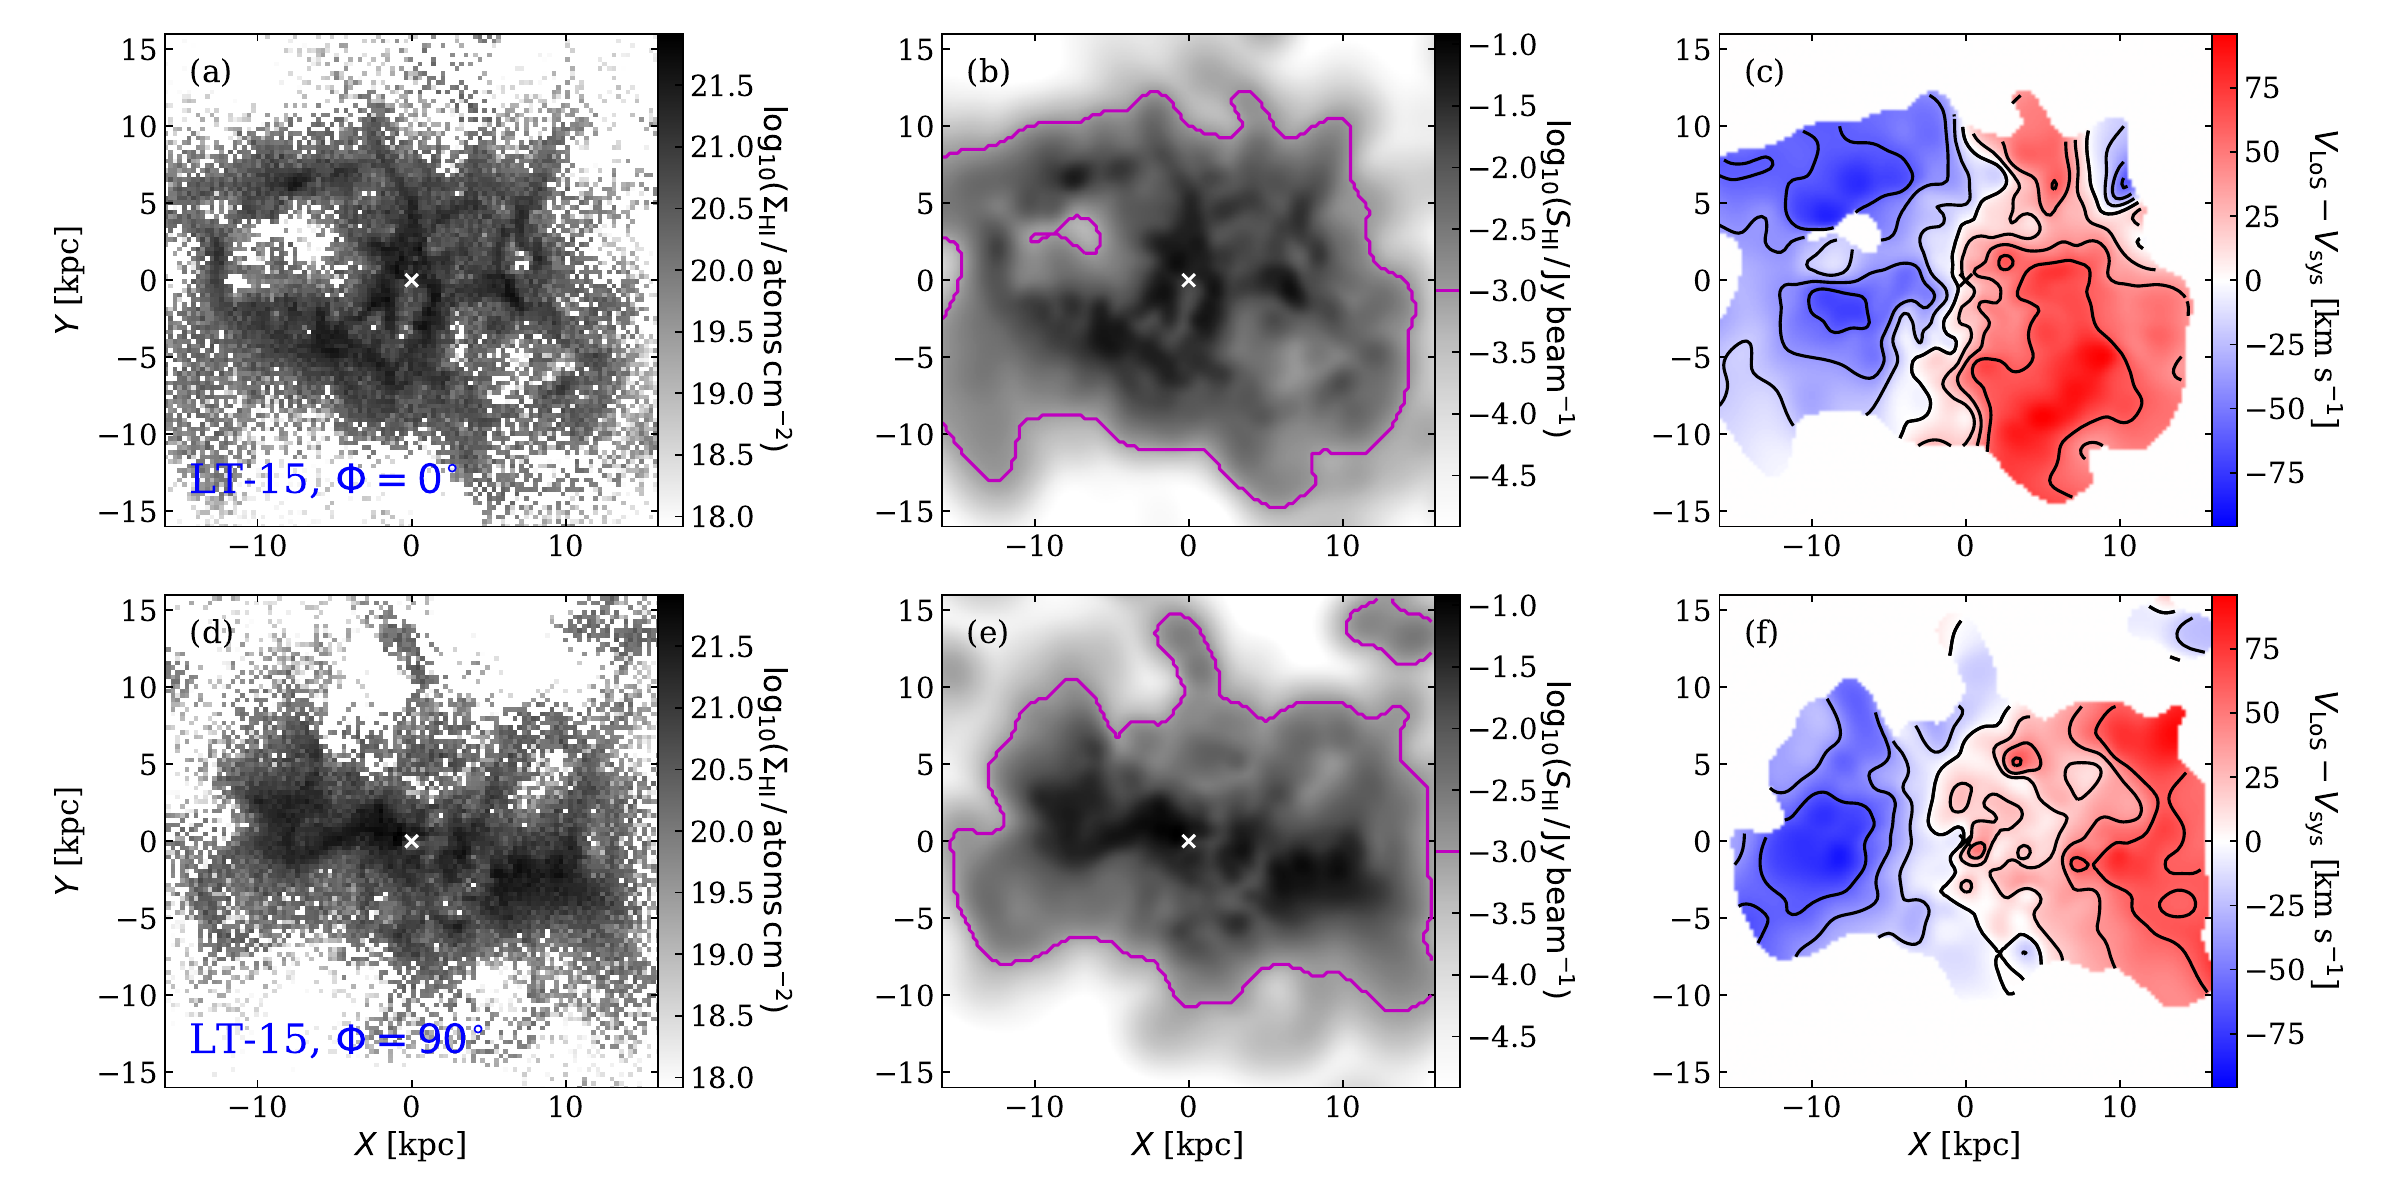}
\includegraphics[width=\textwidth]{../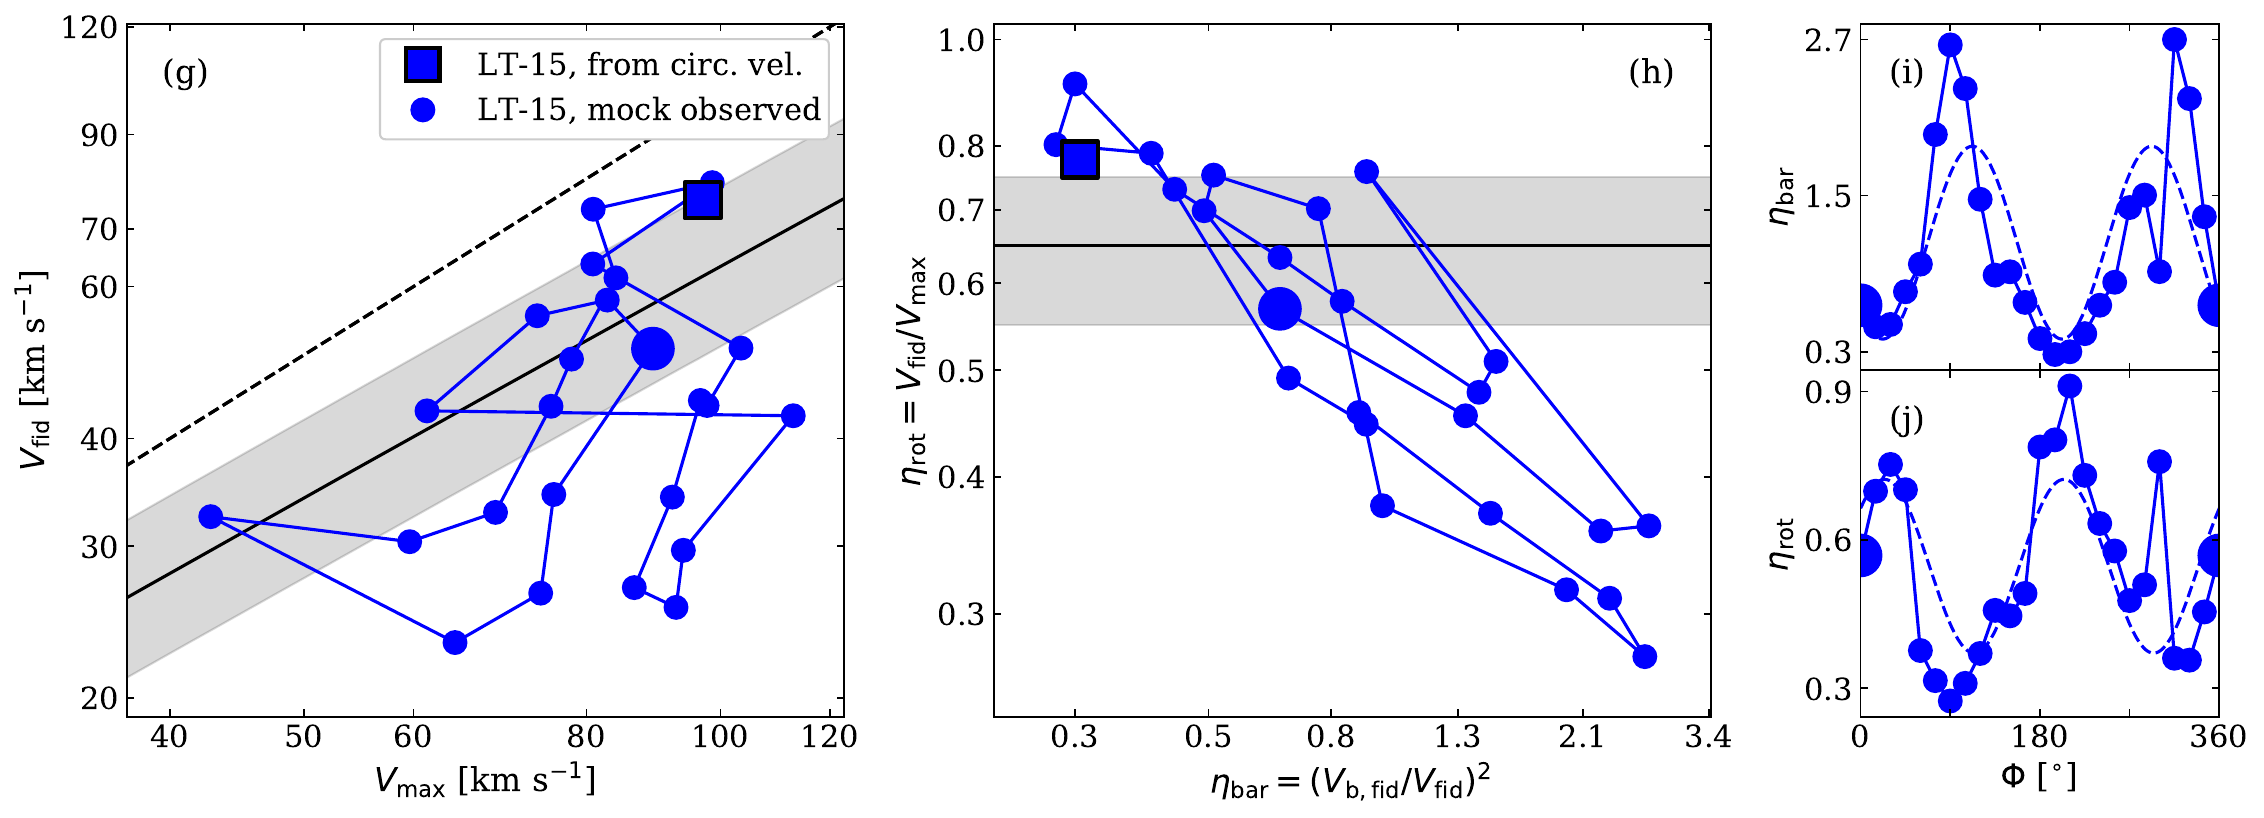}
\end{minipage}
\begin{minipage}{.4\textwidth}
\includegraphics[width=\textwidth]{../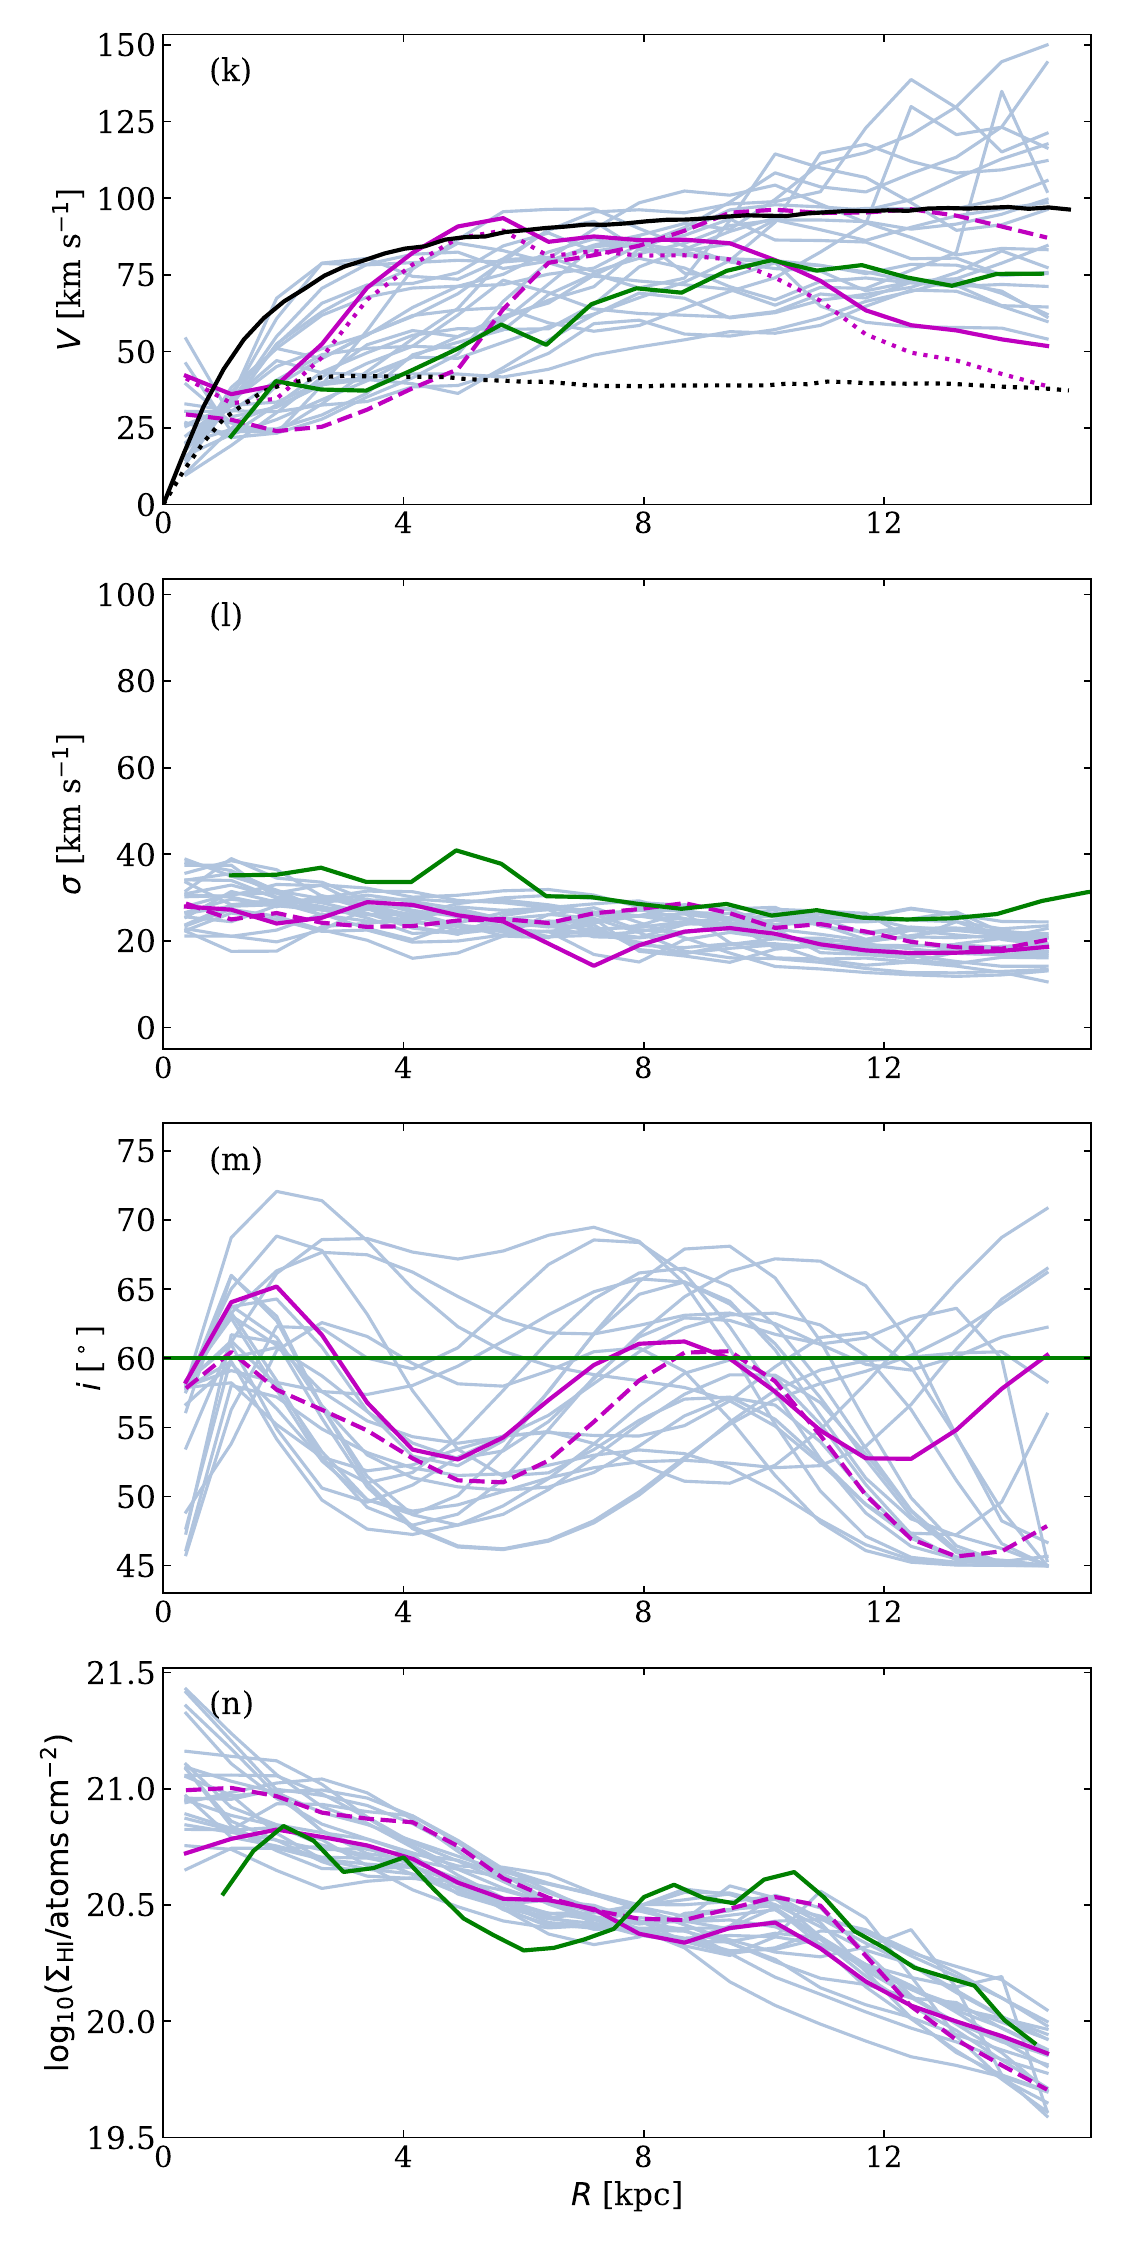}
\end{minipage}
\caption{A set of summary figures for galaxy LT-15, excluded from kinematic analysis. These include example moment maps for two orientations (panels (a)--(f); similar to Fig.~\ref{fig:visualisations}), a summary of the parameters $V_\mathrm{fid}$, $V_\mathrm{max}$, $\eta_\mathrm{rot}$, and $\eta_\mathrm{bar}$ (panels (g)--(j); similar to Fig.~\ref{fig:loops}), and a summary of the rotation curve analysis from $24$ viewing angles (panels (k)--(n); similar to Fig.~\ref{fig:rot_curves}). See description of Appendix~\ref{app:supplementary} for details.}
\label{fig:S24}
\end{figure}
\clearpage

\begin{figure}
\begin{minipage}{.9\textwidth}
\includegraphics[width=\textwidth]{../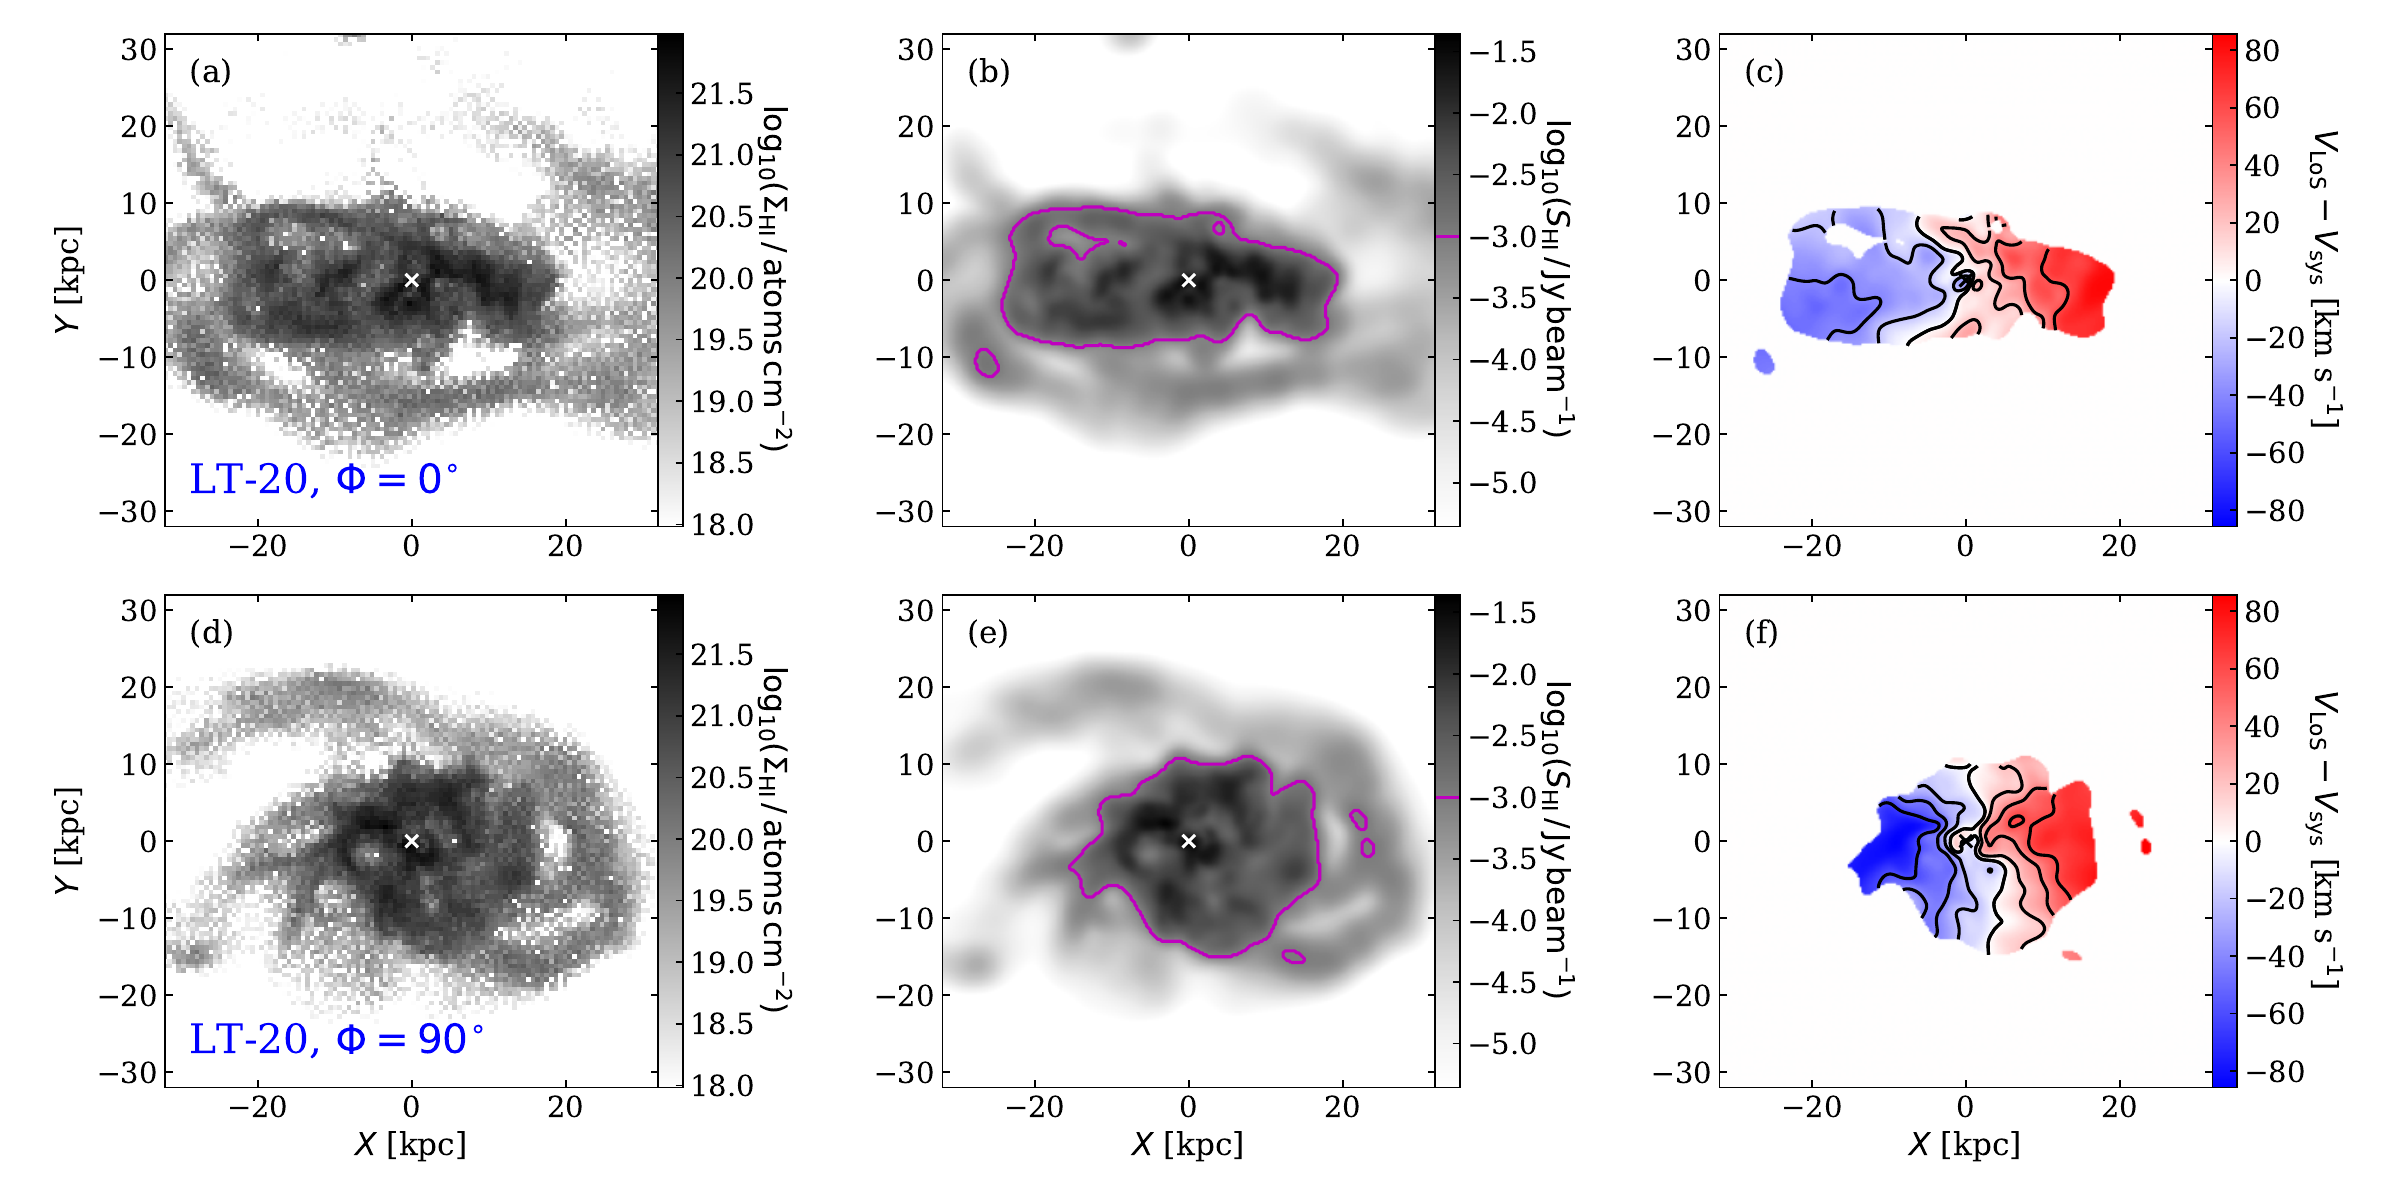}
\includegraphics[width=\textwidth]{../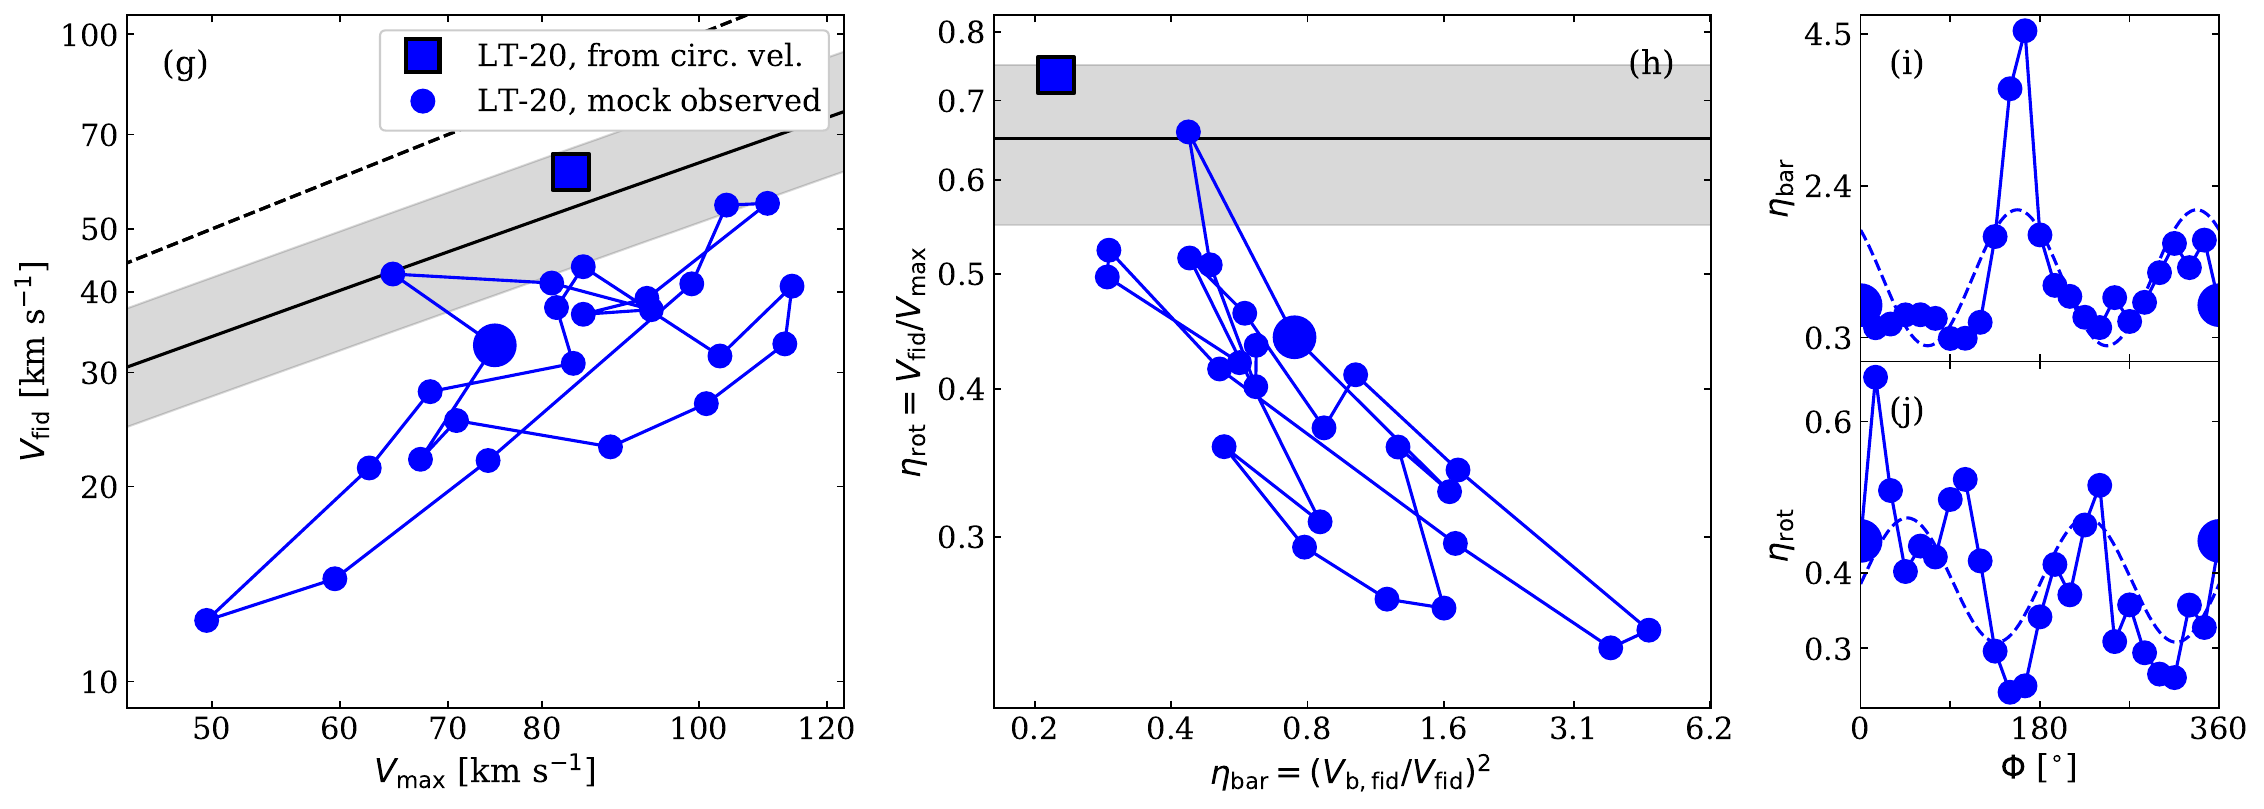}
\end{minipage}
\begin{minipage}{.4\textwidth}
\includegraphics[width=\textwidth]{../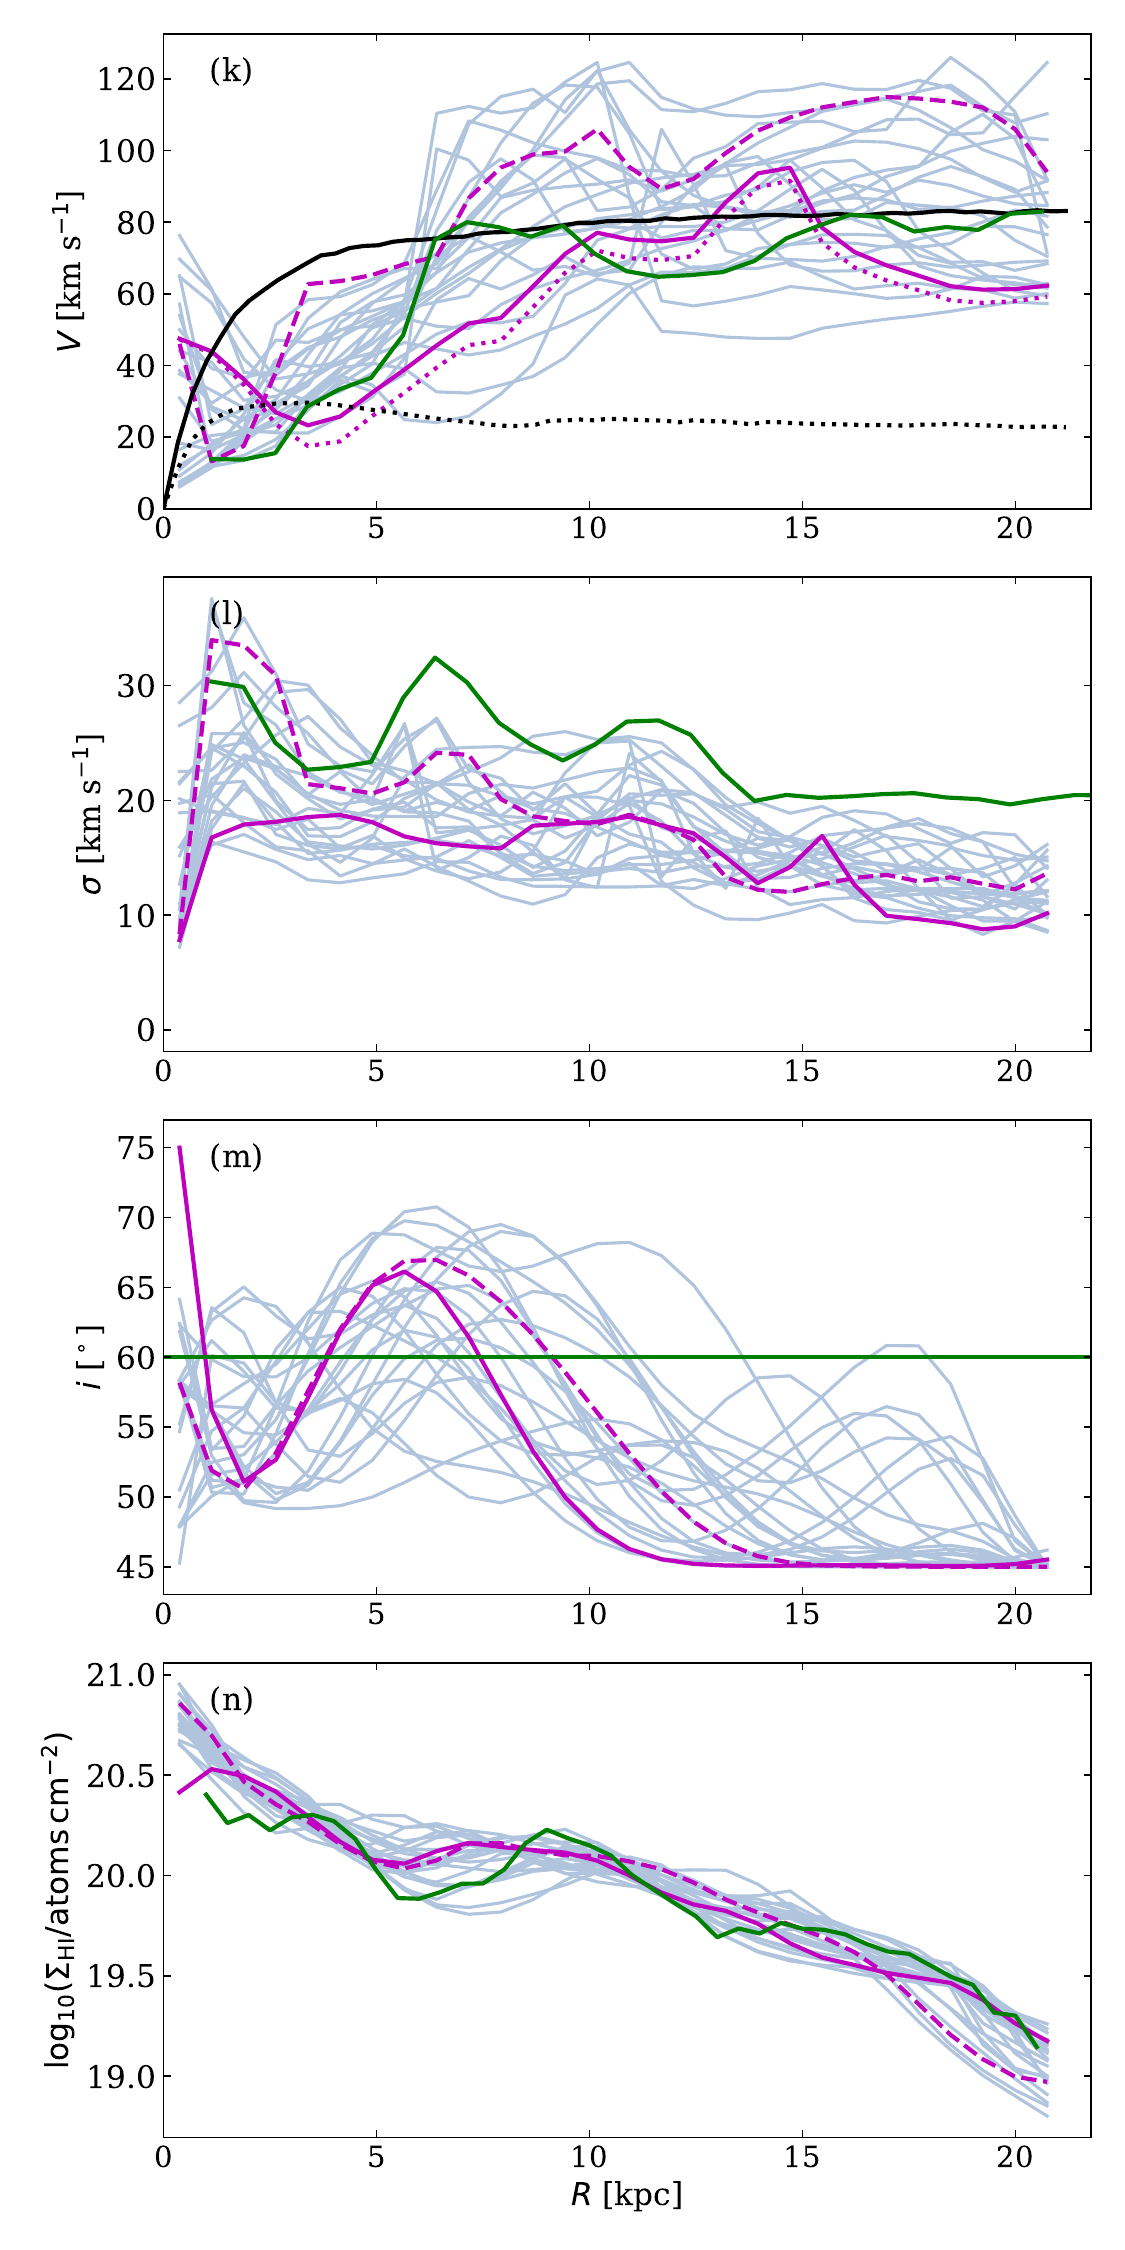}
\end{minipage}
\caption{A set of summary figures for galaxy LT-20, excluded from kinematic analysis. These include example moment maps for two orientations (panels (a)--(f); similar to Fig.~\ref{fig:visualisations}), a summary of the parameters $V_\mathrm{fid}$, $V_\mathrm{max}$, $\eta_\mathrm{rot}$, and $\eta_\mathrm{bar}$ (panels (g)--(j); similar to Fig.~\ref{fig:loops}), and a summary of the rotation curve analysis from $24$ viewing angles (panels (k)--(n); similar to Fig.~\ref{fig:rot_curves}). See description of Appendix~\ref{app:supplementary} for details.}
\label{fig:S25}
\end{figure}
\clearpage

\begin{figure}
\begin{minipage}{.9\textwidth}
\includegraphics[width=\textwidth]{../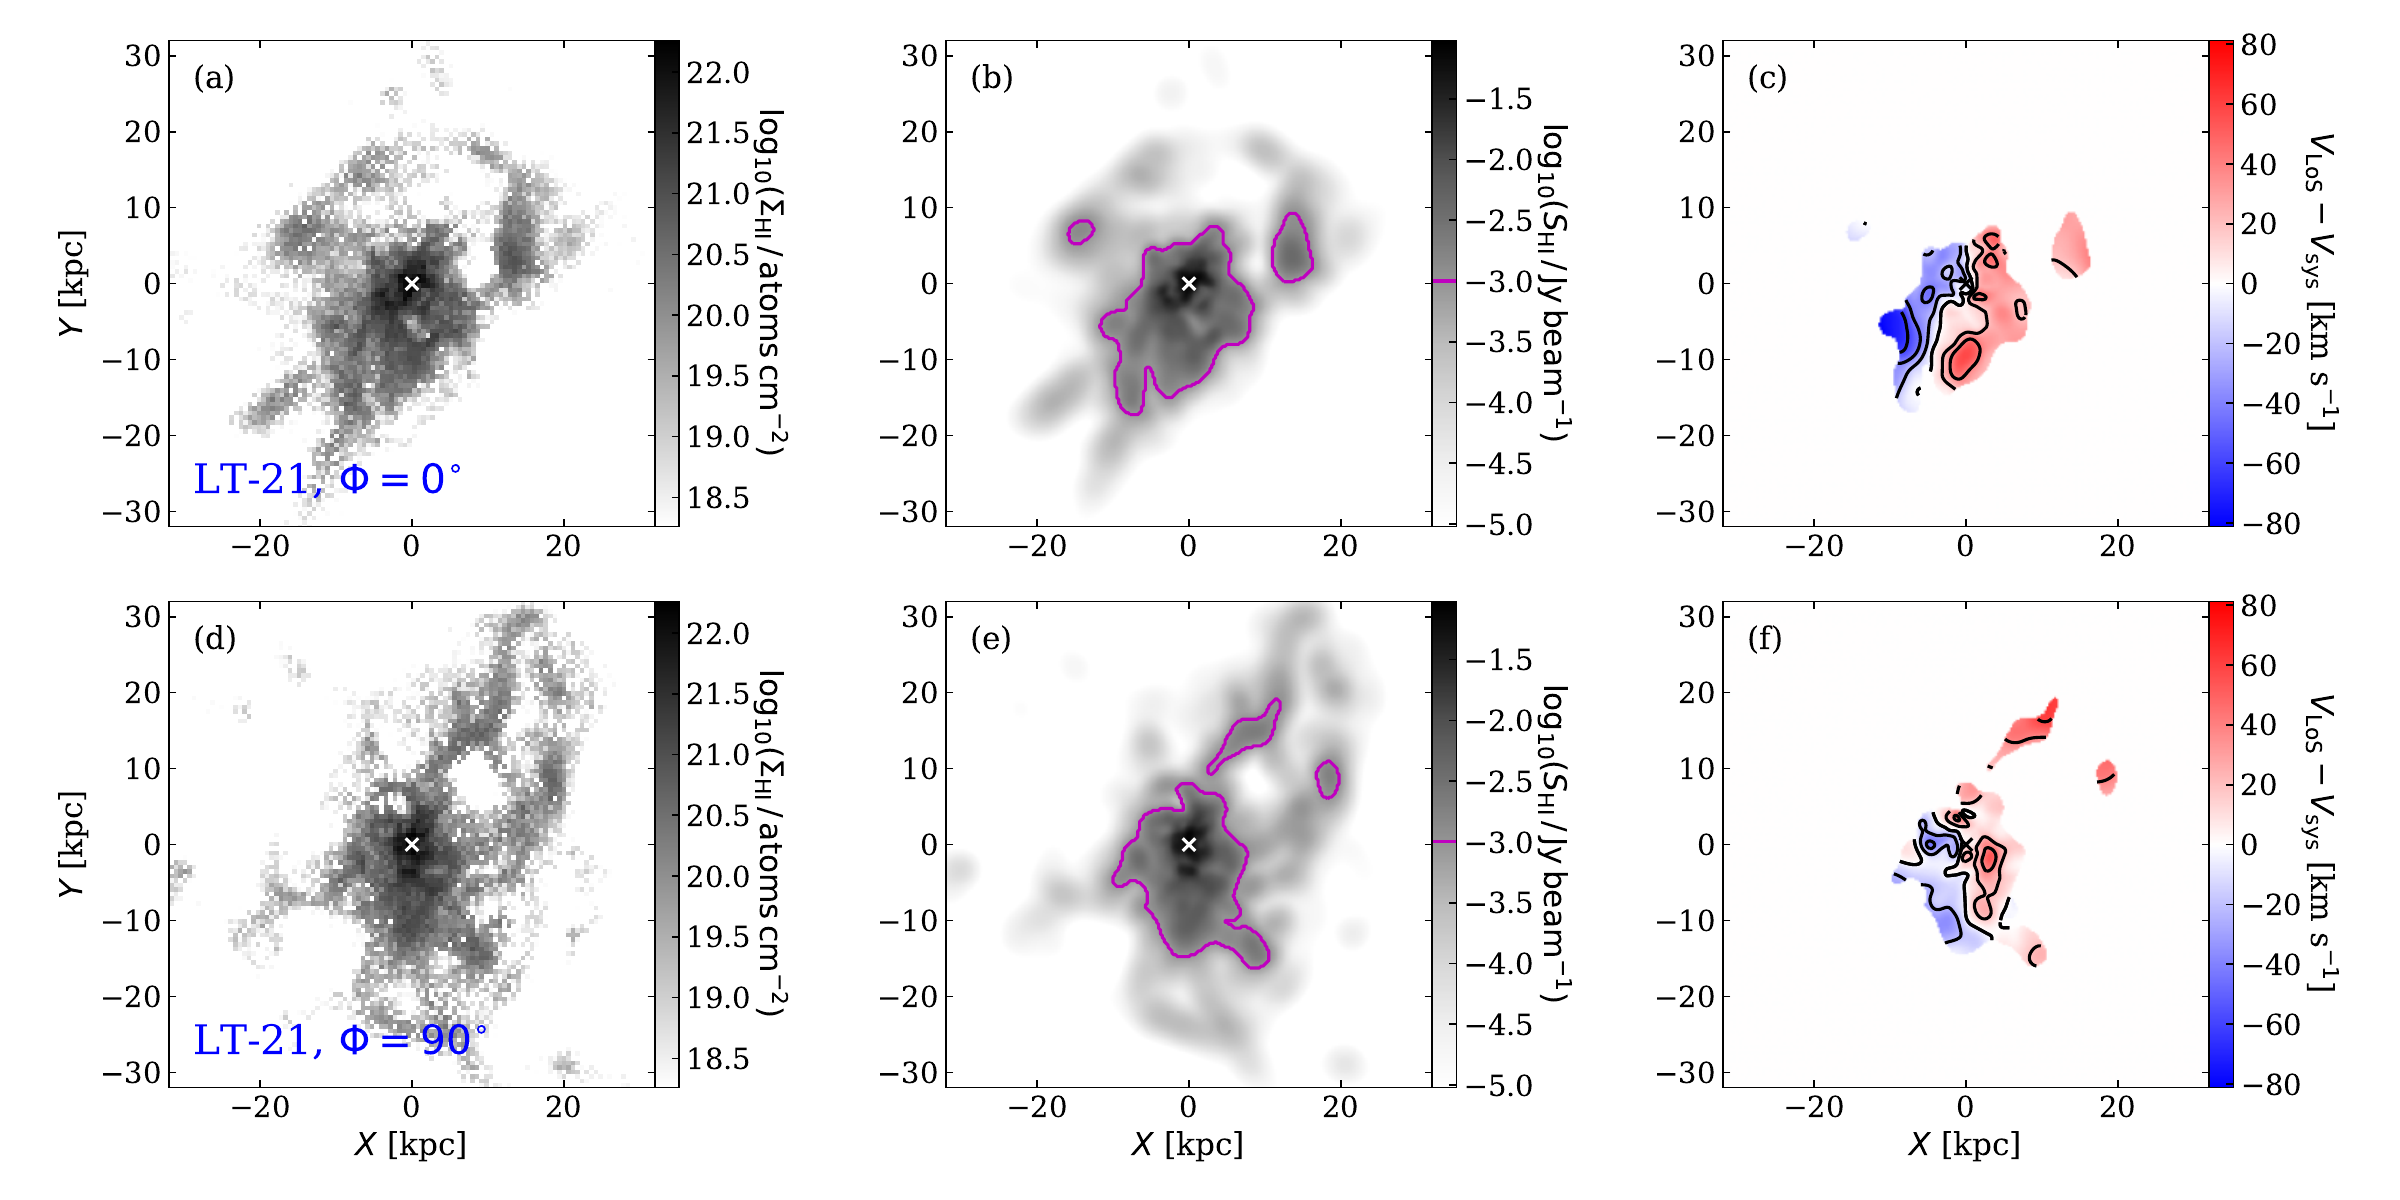}
\includegraphics[width=\textwidth]{../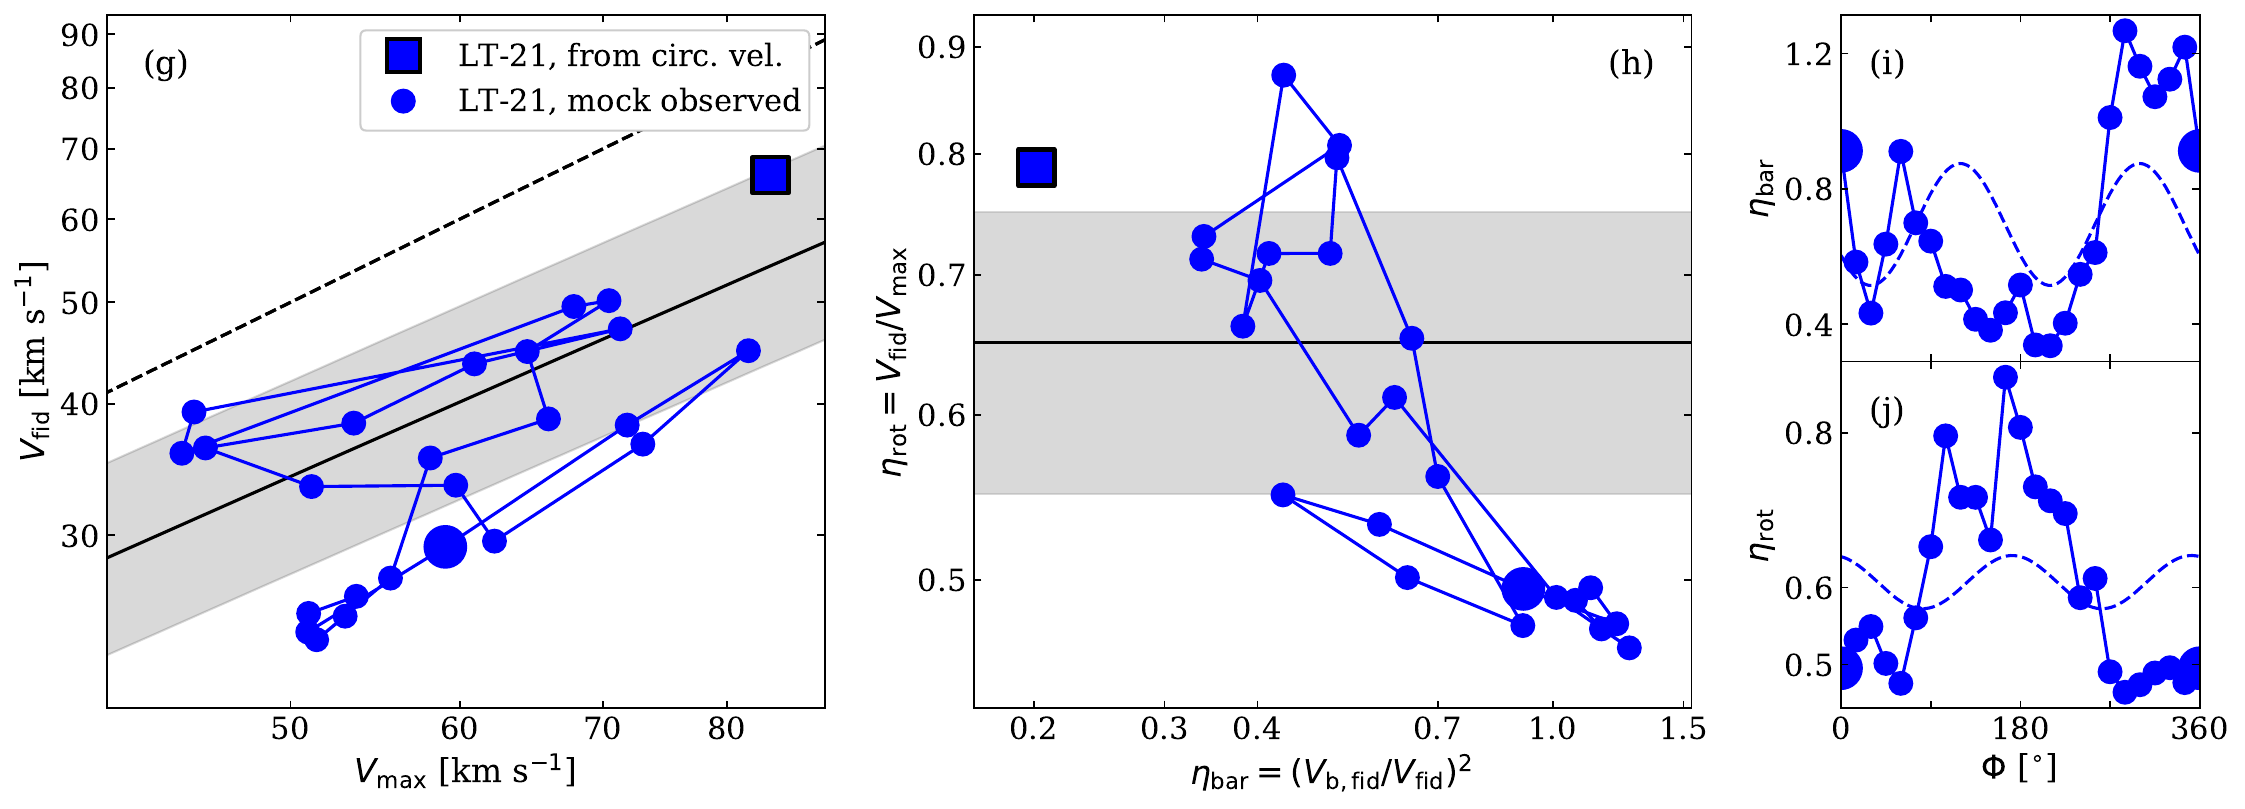}
\end{minipage}
\begin{minipage}{.4\textwidth}
\includegraphics[width=\textwidth]{../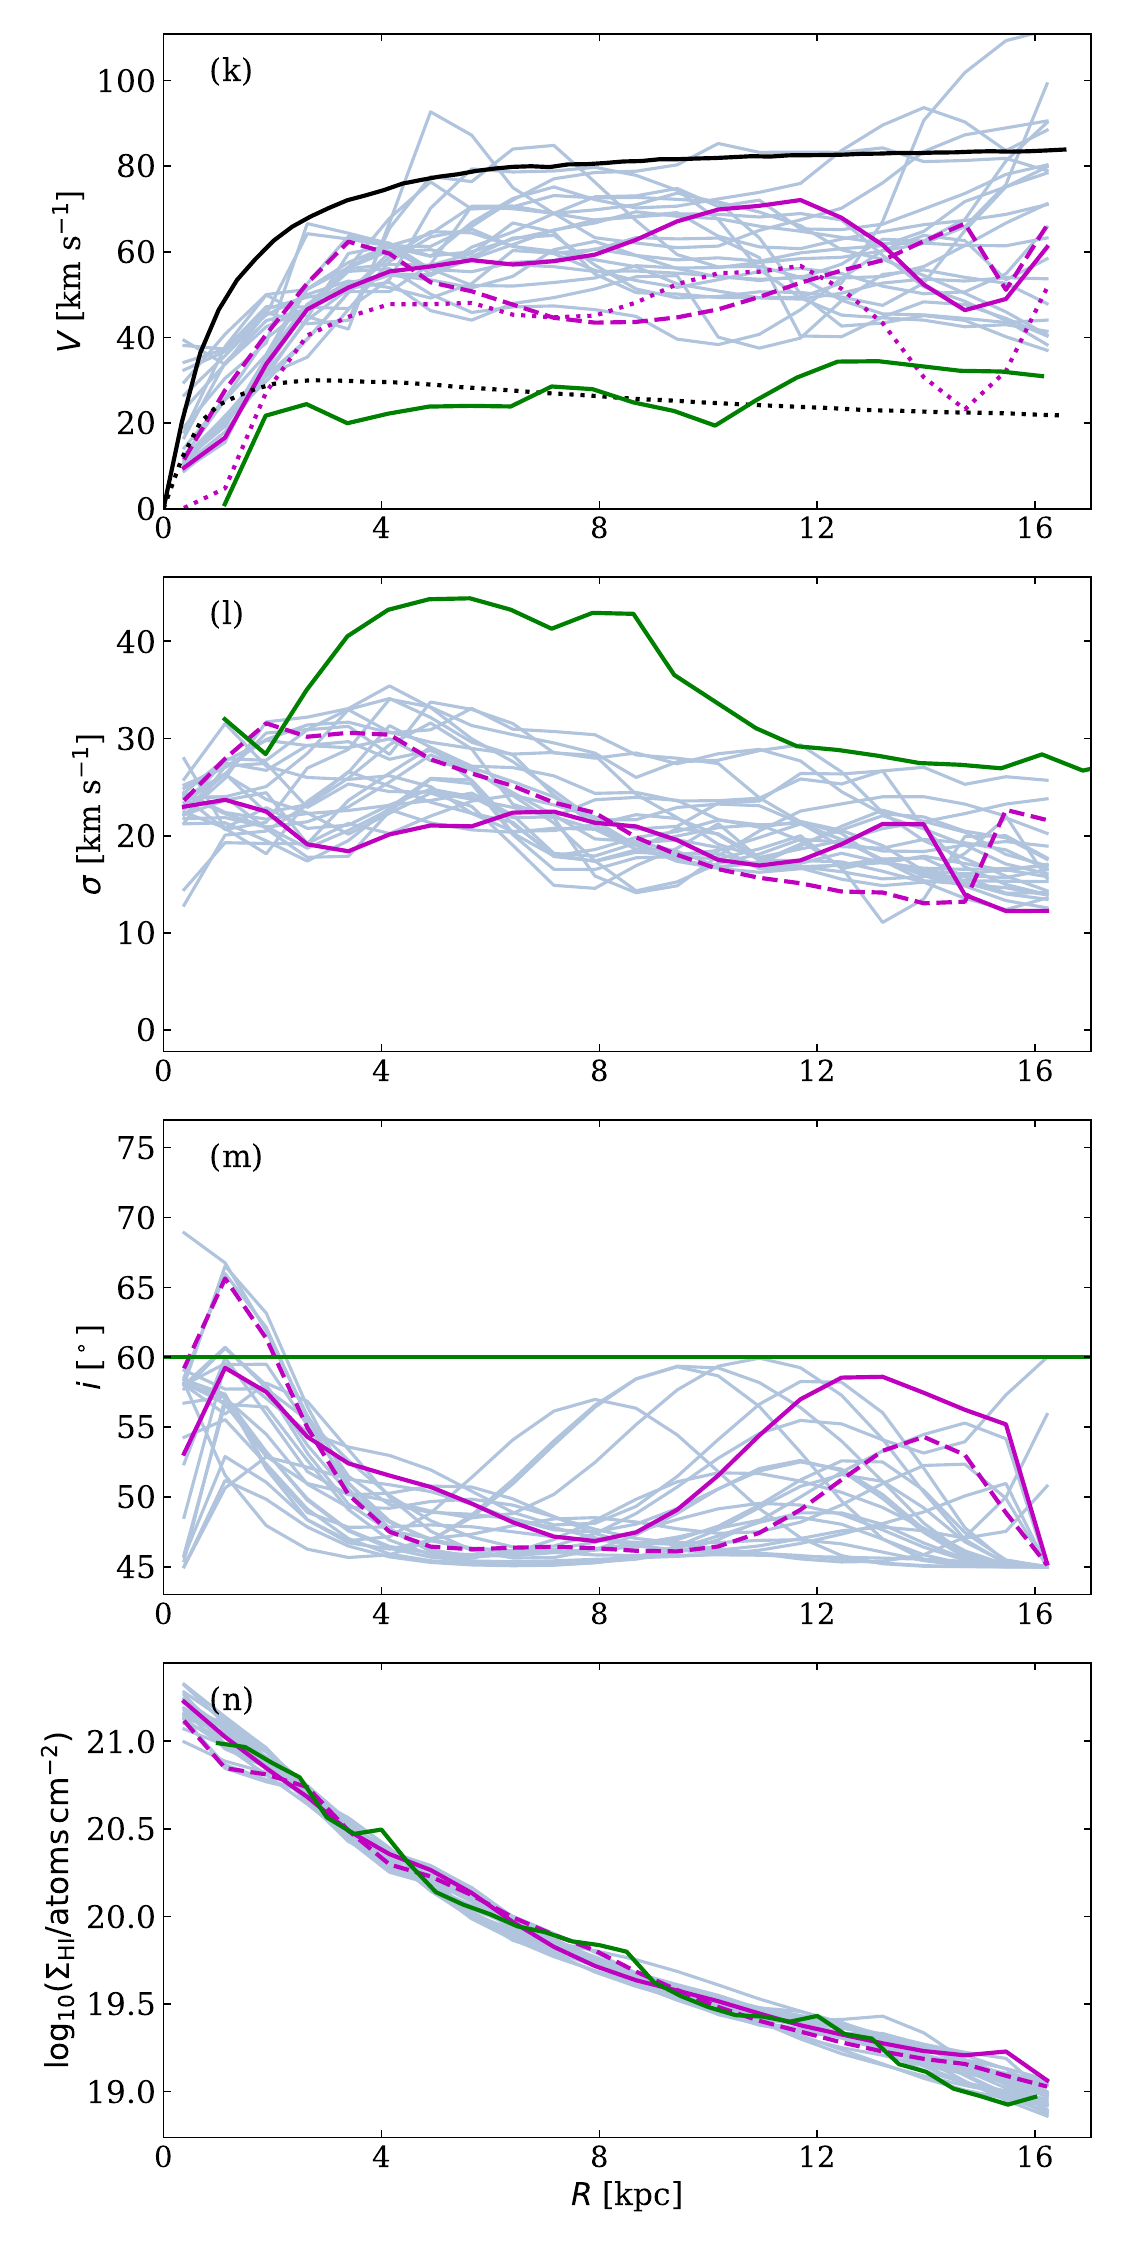}
\end{minipage}
\caption{A set of summary figures for galaxy LT-21, excluded from kinematic analysis. These include example moment maps for two orientations (panels (a)--(f); similar to Fig.~\ref{fig:visualisations}), a summary of the parameters $V_\mathrm{fid}$, $V_\mathrm{max}$, $\eta_\mathrm{rot}$, and $\eta_\mathrm{bar}$ (panels (g)--(j); similar to Fig.~\ref{fig:loops}), and a summary of the rotation curve analysis from $24$ viewing angles (panels (k)--(n); similar to Fig.~\ref{fig:rot_curves}). See description of Appendix~\ref{app:supplementary} for details.}
\label{fig:S26}
\end{figure}
\clearpage

\begin{figure}
\begin{minipage}{.9\textwidth}
\includegraphics[width=\textwidth]{../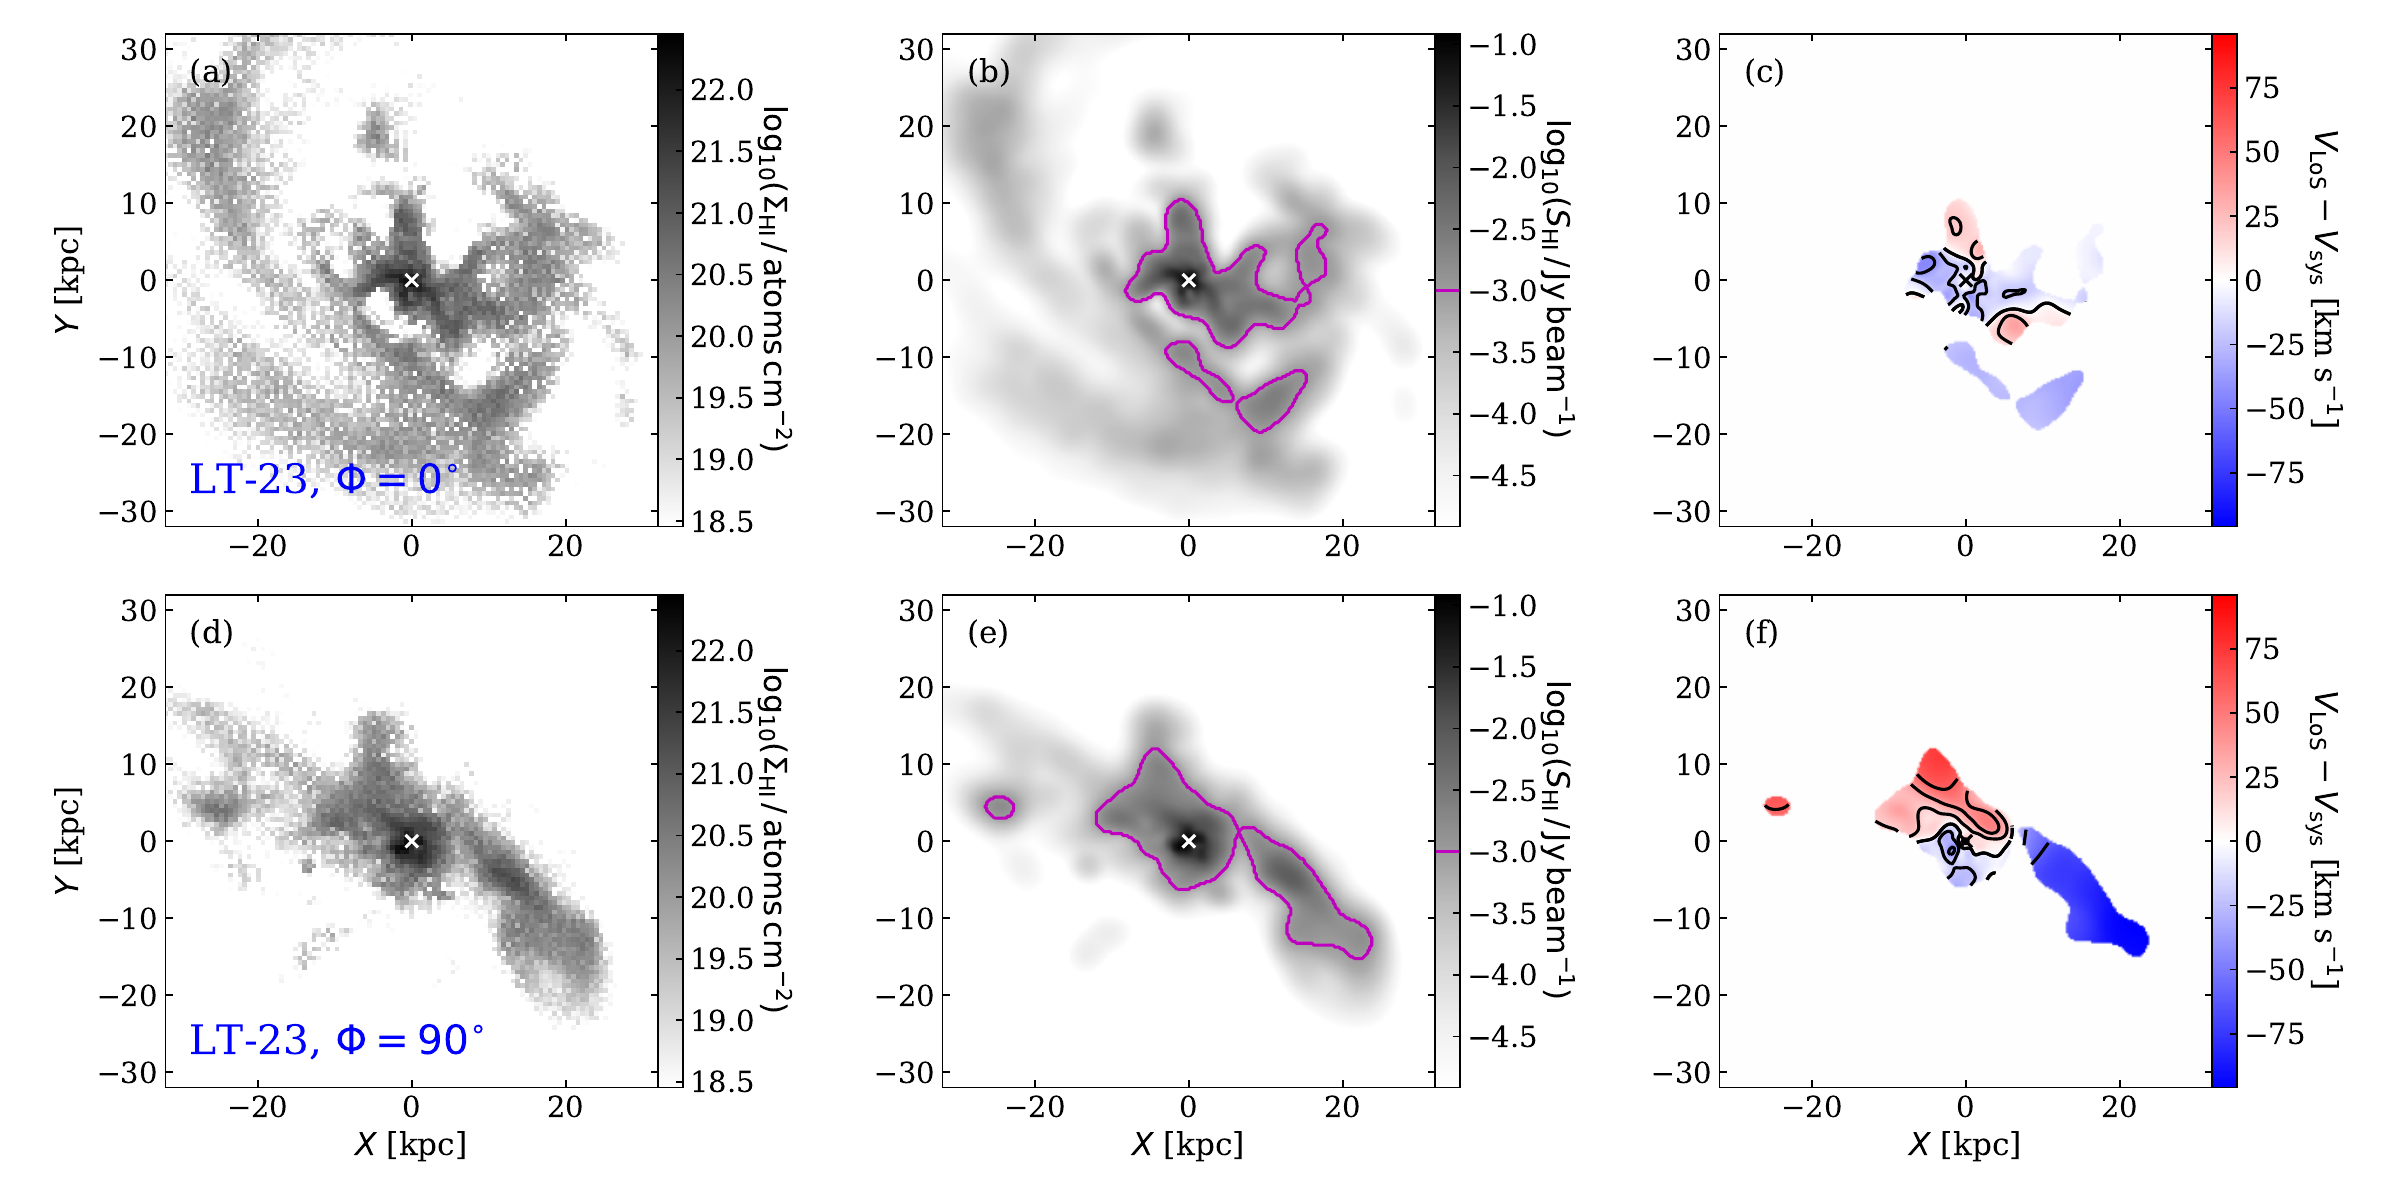}
\includegraphics[width=\textwidth]{../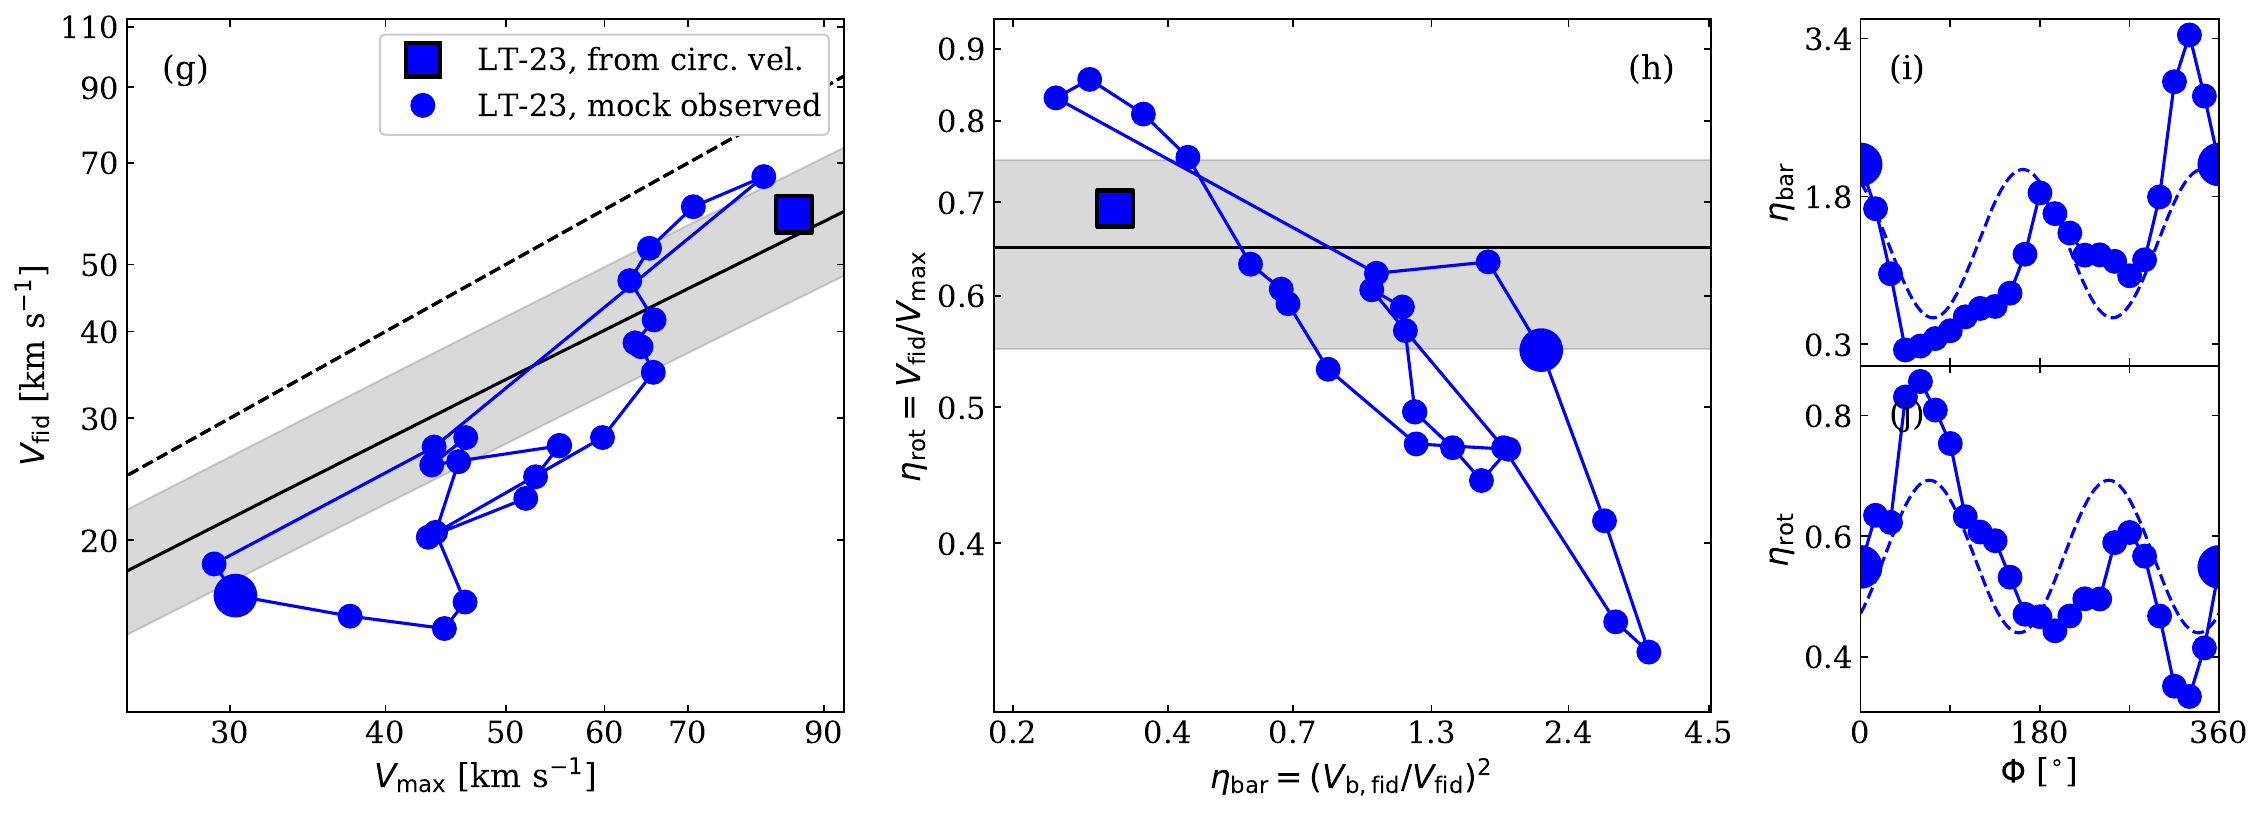}
\end{minipage}
\begin{minipage}{.4\textwidth}
\includegraphics[width=\textwidth]{../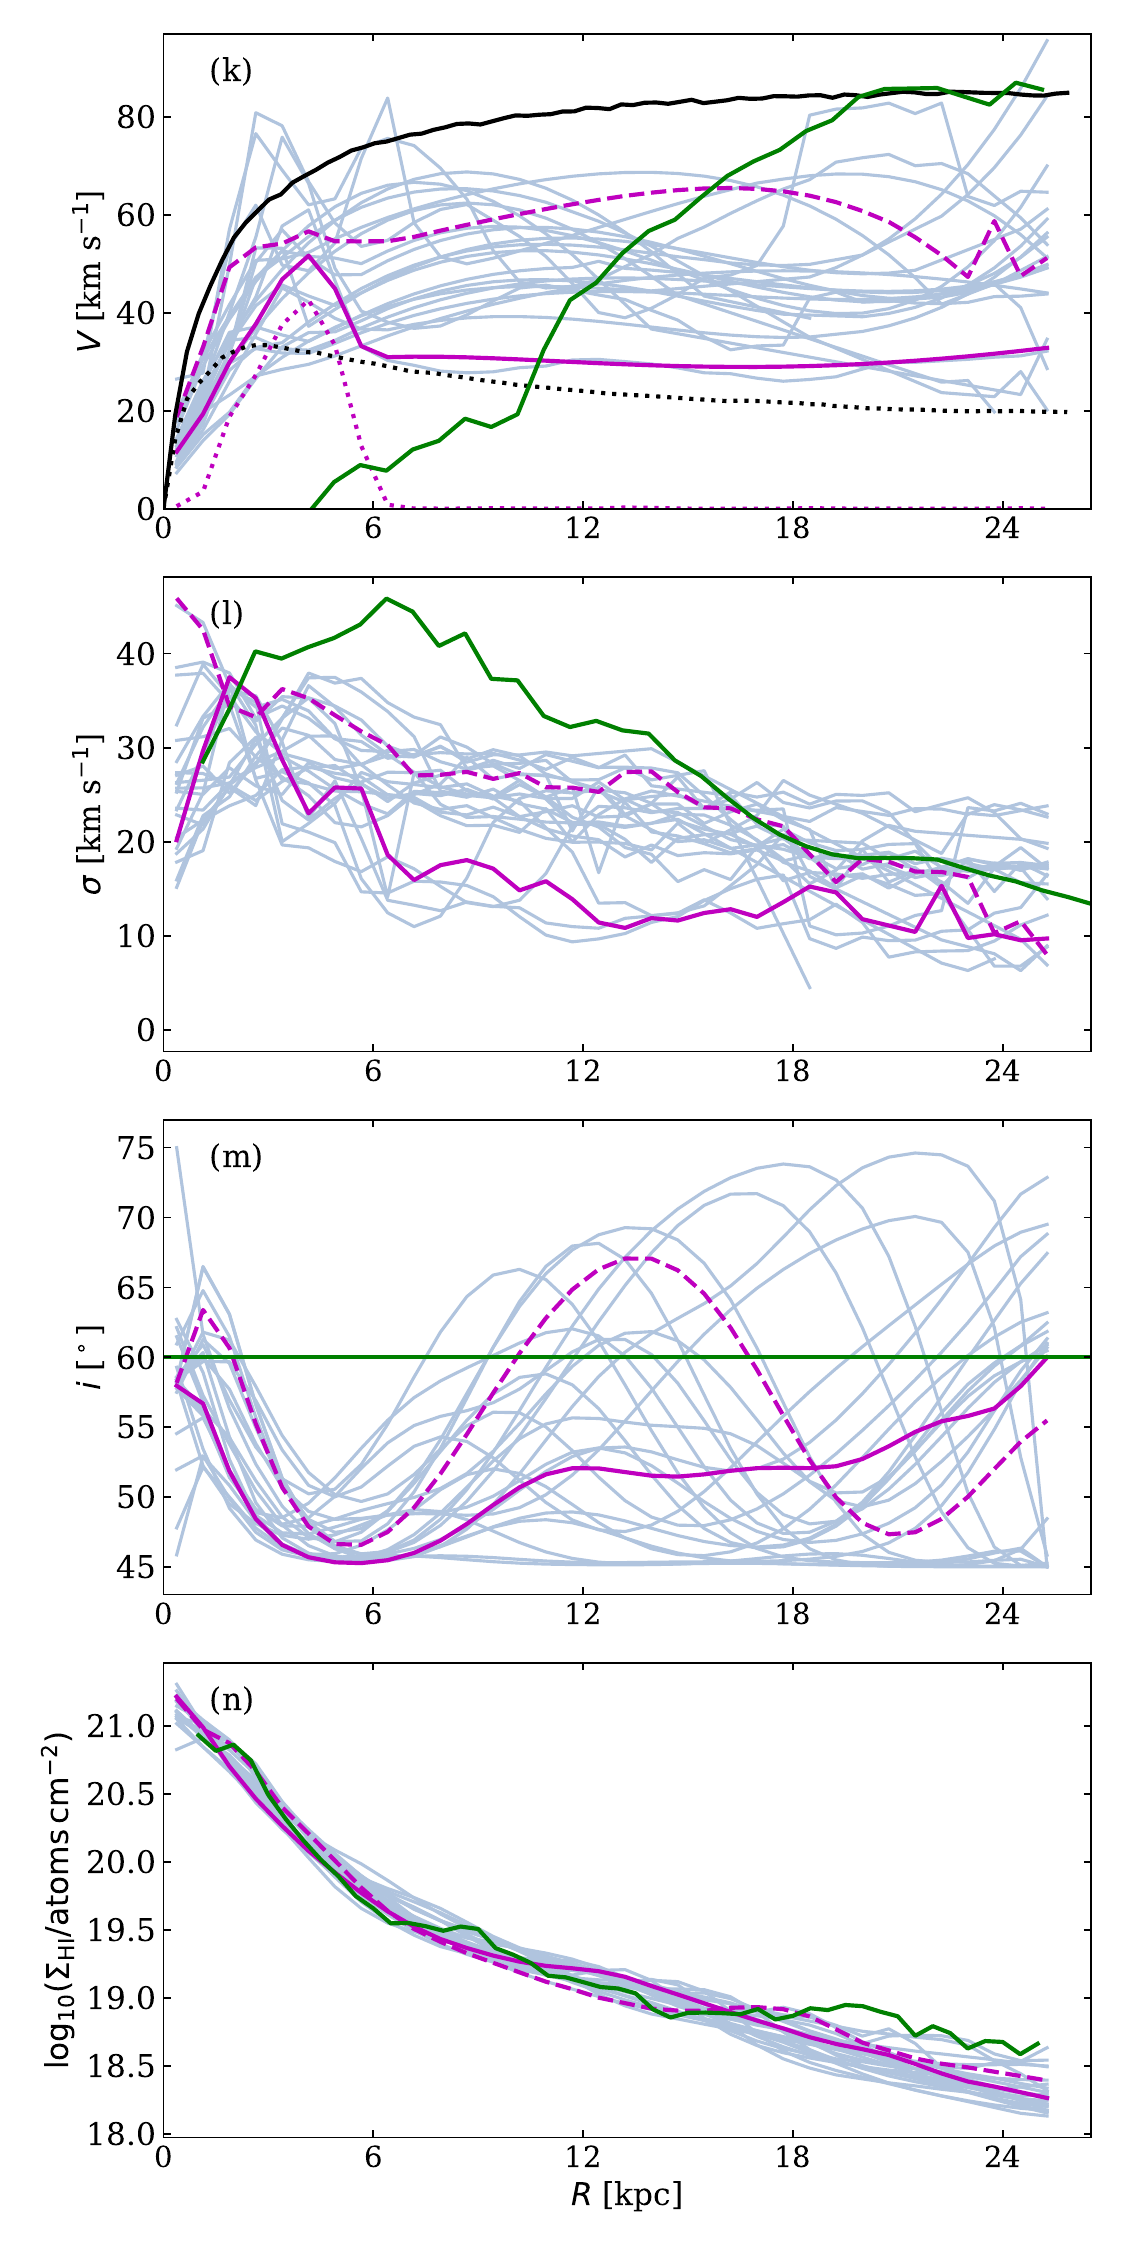}
\end{minipage}
\caption{A set of summary figures for galaxy LT-23, excluded from kinematic analysis. These include example moment maps for two orientations (panels (a)--(f); similar to Fig.~\ref{fig:visualisations}), a summary of the parameters $V_\mathrm{fid}$, $V_\mathrm{max}$, $\eta_\mathrm{rot}$, and $\eta_\mathrm{bar}$ (panels (g)--(j); similar to Fig.~\ref{fig:loops}), and a summary of the rotation curve analysis from $24$ viewing angles (panels (k)--(n); similar to Fig.~\ref{fig:rot_curves}). See description of Appendix~\ref{app:supplementary} for details.}
\label{fig:S27}
\end{figure}
\clearpage

\begin{figure}
\begin{minipage}{.9\textwidth}
\includegraphics[width=\textwidth]{../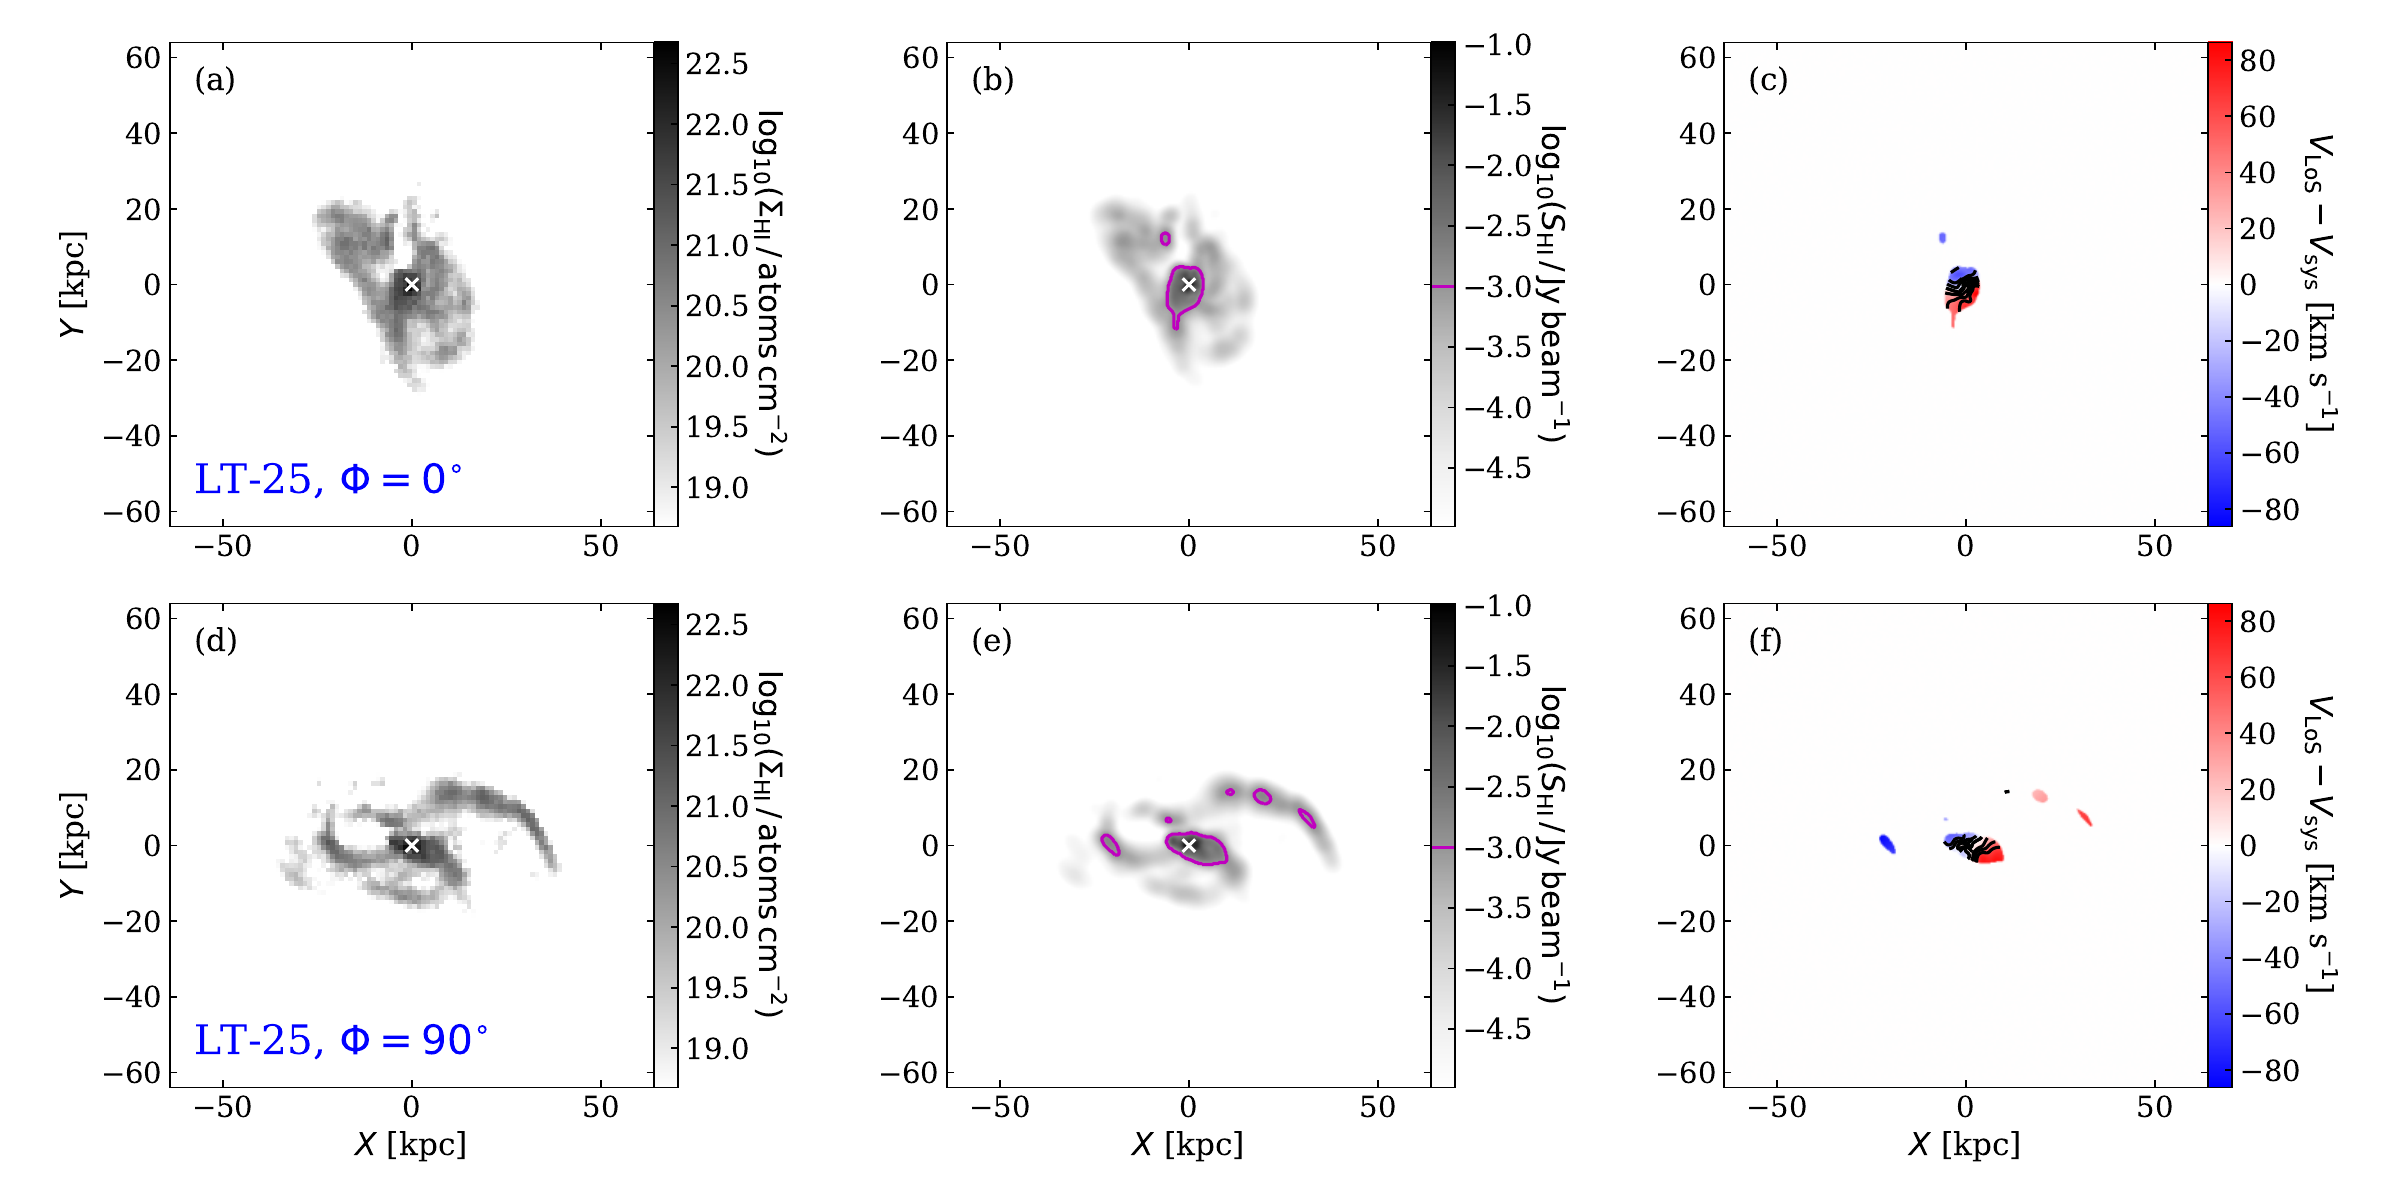}
\includegraphics[width=\textwidth]{../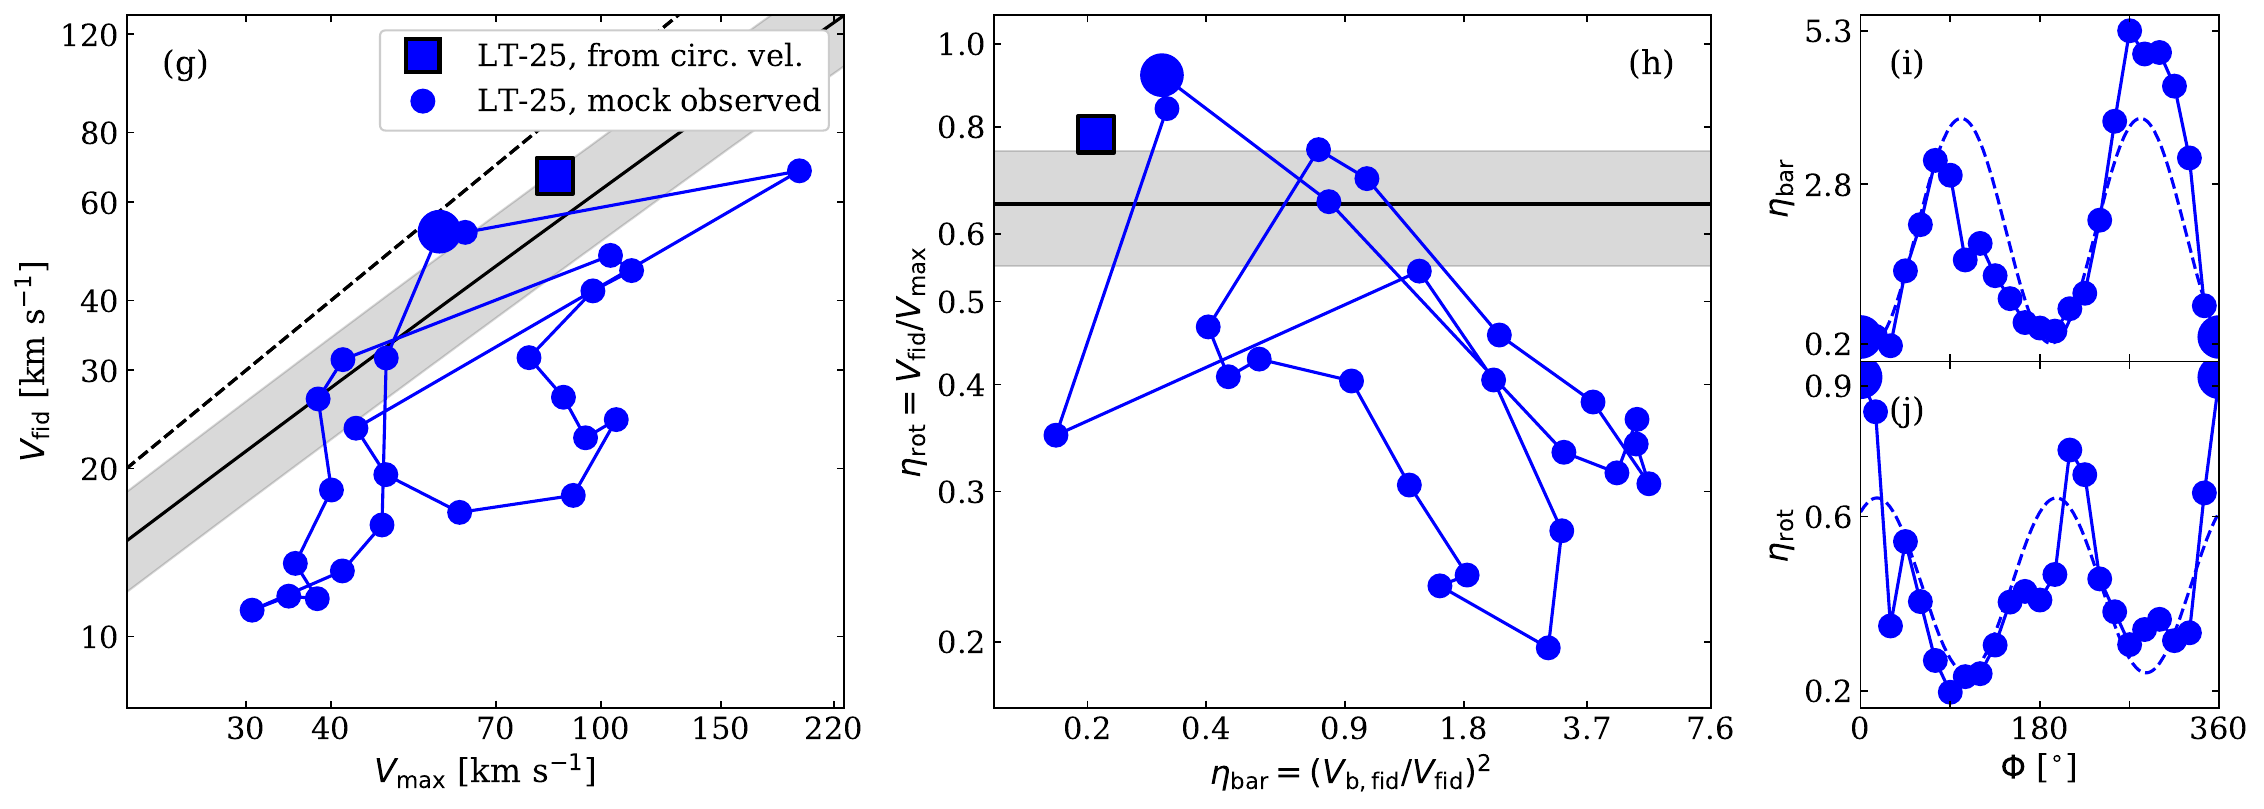}
\end{minipage}
\begin{minipage}{.4\textwidth}
\includegraphics[width=\textwidth]{../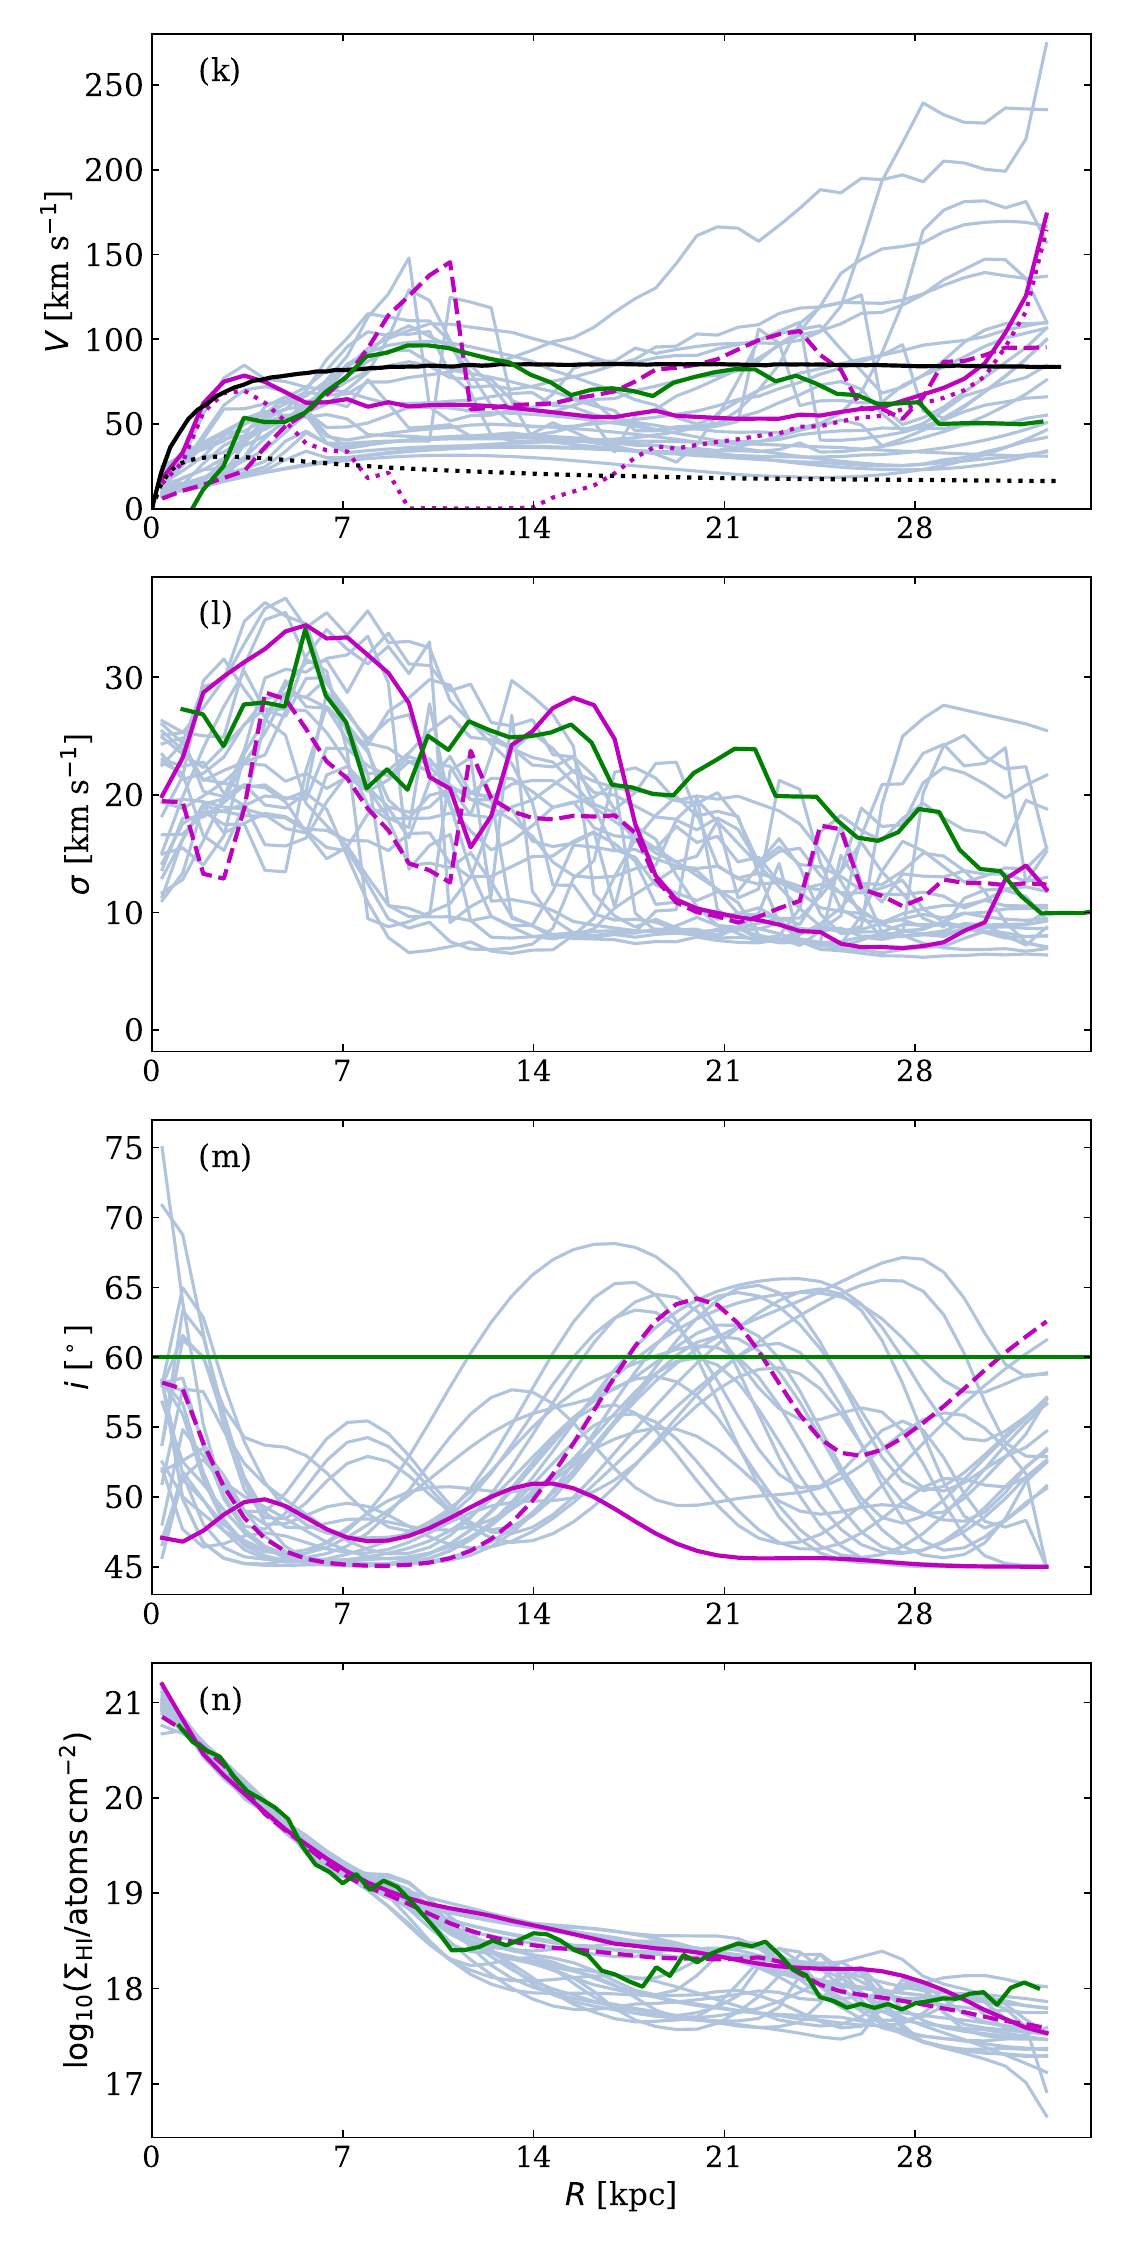}
\end{minipage}
\caption{A set of summary figures for galaxy LT-25, excluded from kinematic analysis. These include example moment maps for two orientations (panels (a)--(f); similar to Fig.~\ref{fig:visualisations}), a summary of the parameters $V_\mathrm{fid}$, $V_\mathrm{max}$, $\eta_\mathrm{rot}$, and $\eta_\mathrm{bar}$ (panels (g)--(j); similar to Fig.~\ref{fig:loops}), and a summary of the rotation curve analysis from $24$ viewing angles (panels (k)--(n); similar to Fig.~\ref{fig:rot_curves}). See description of Appendix~\ref{app:supplementary} for details.}
\label{fig:S28}
\end{figure}
\clearpage

\begin{figure}
\begin{minipage}{.9\textwidth}
\includegraphics[width=\textwidth]{../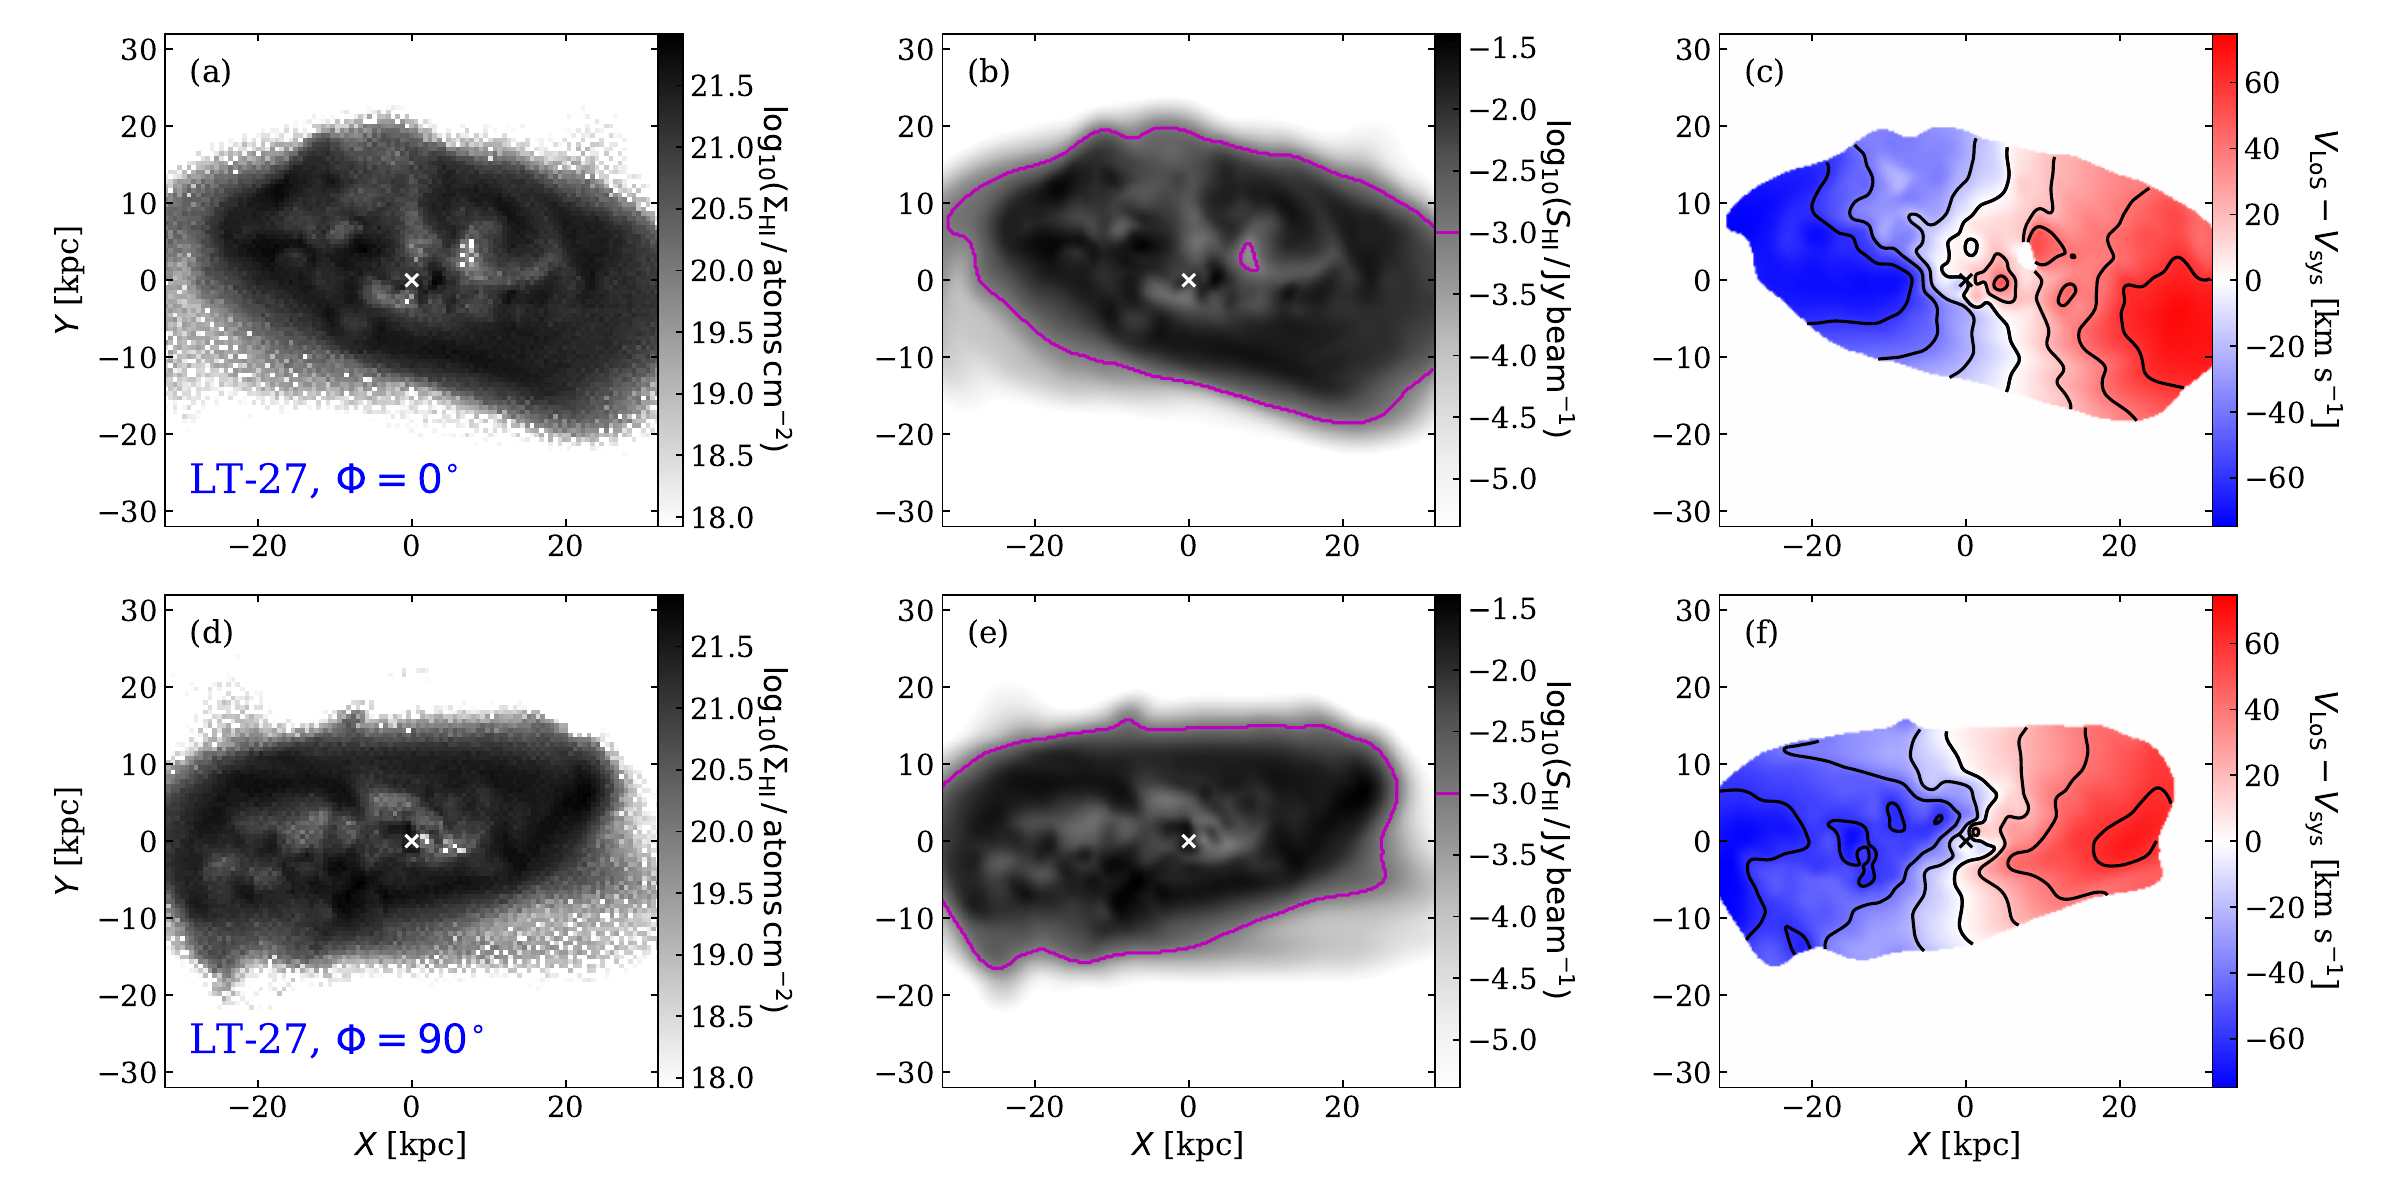}
\includegraphics[width=\textwidth]{../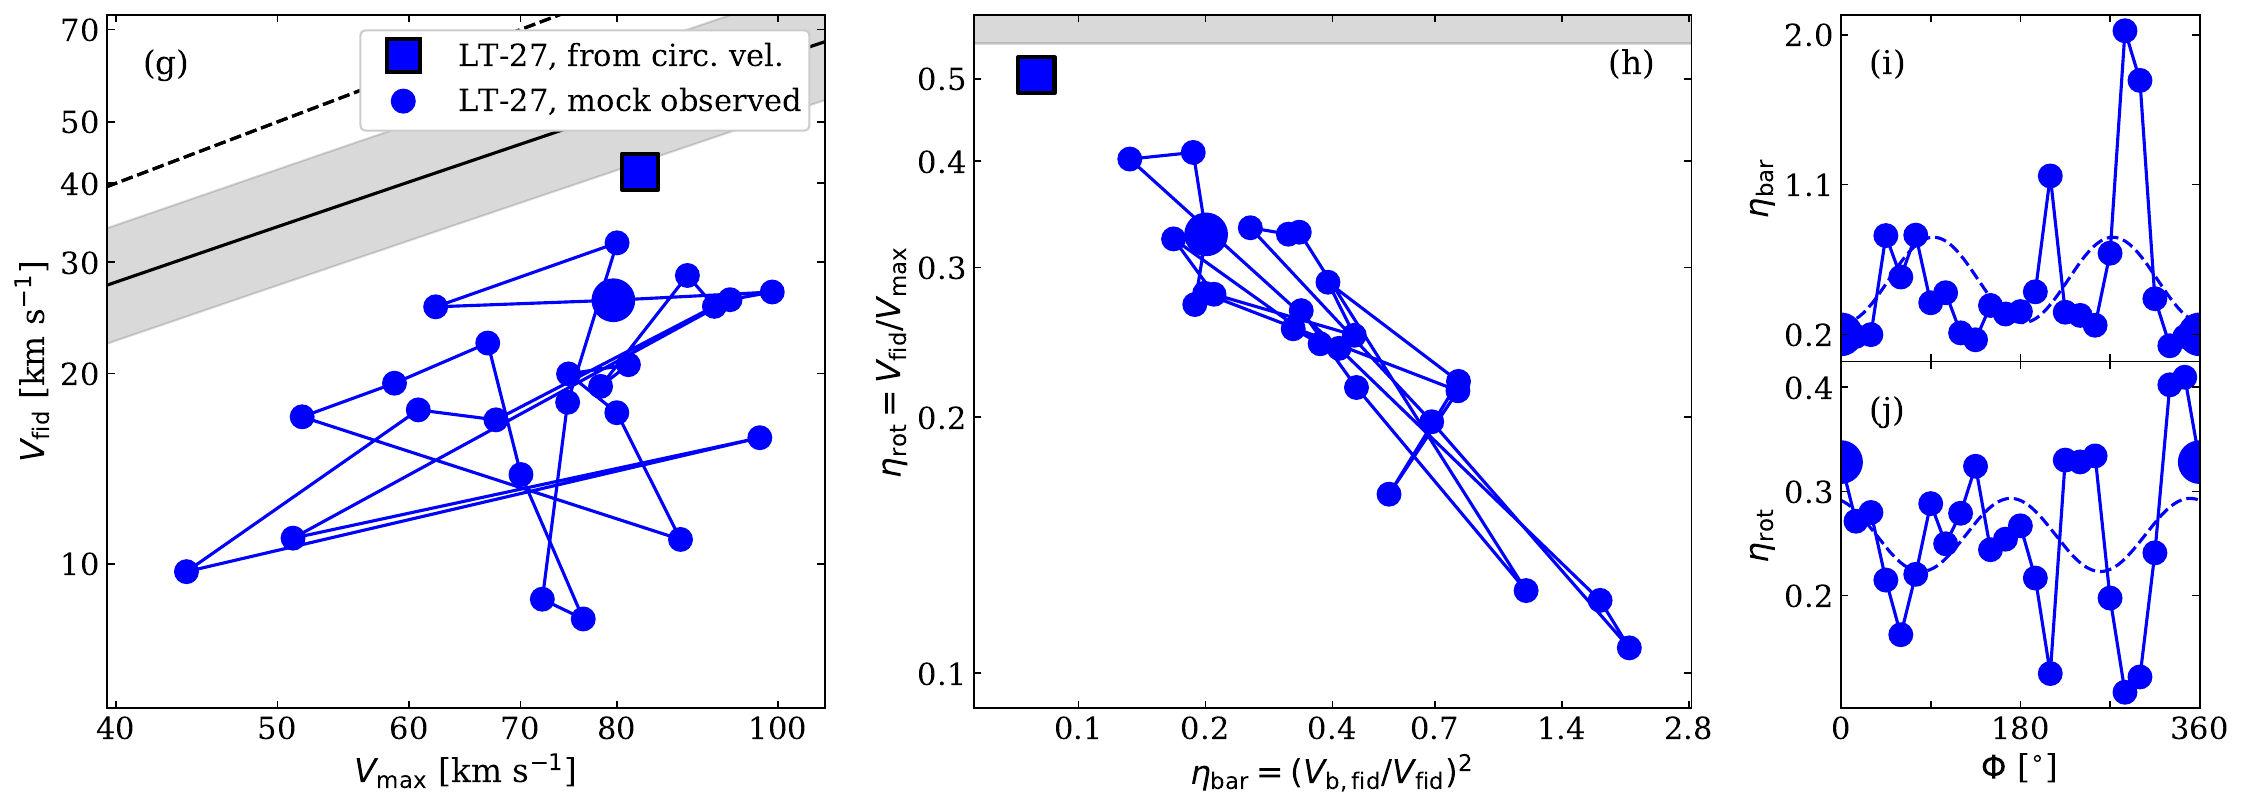}
\end{minipage}
\begin{minipage}{.4\textwidth}
\includegraphics[width=\textwidth]{../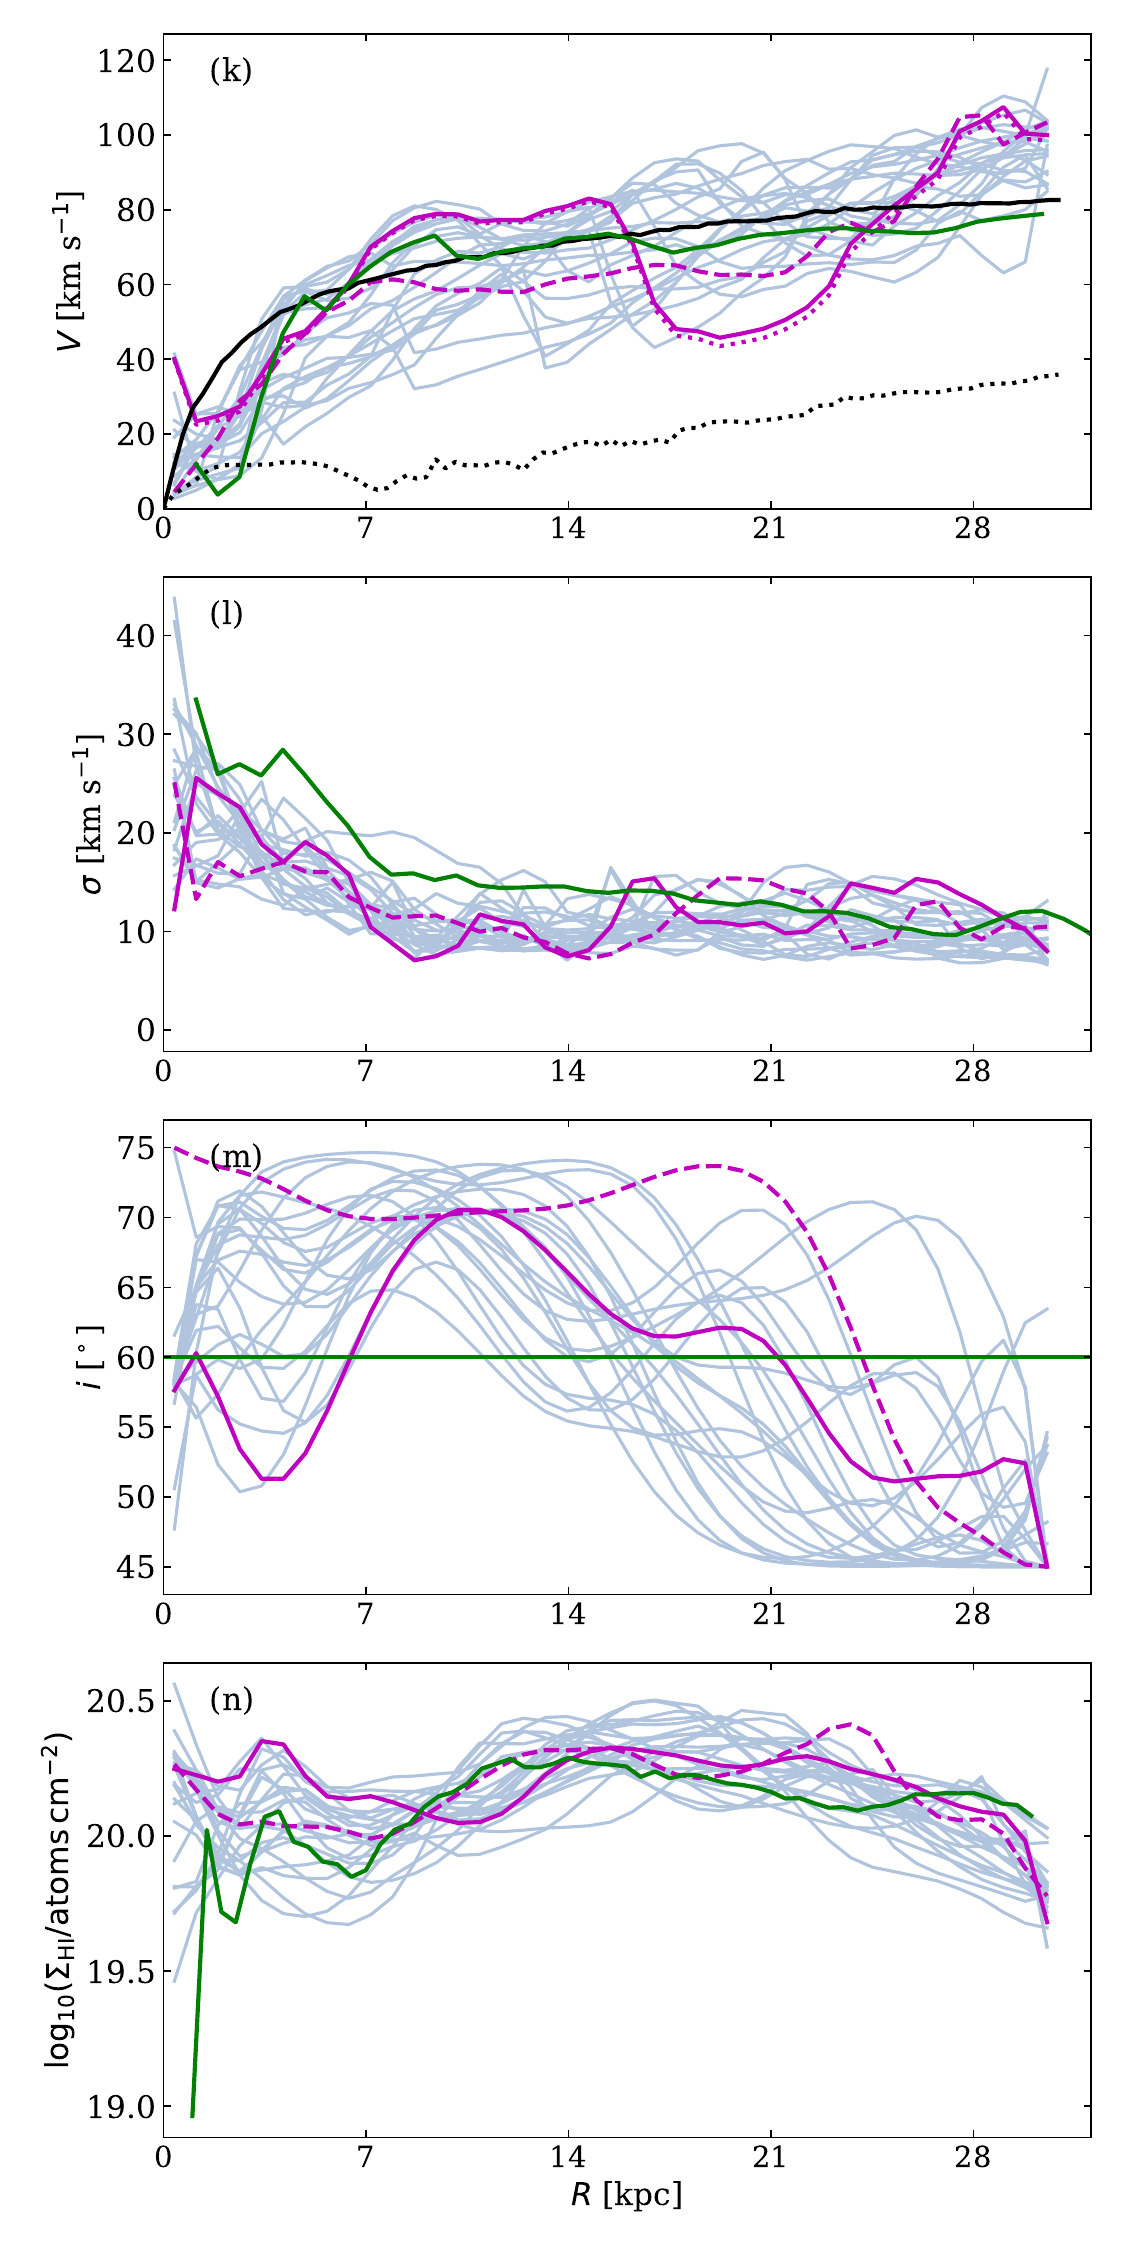}
\end{minipage}
\caption{A set of summary figures for galaxy LT-27, excluded from kinematic analysis. These include example moment maps for two orientations (panels (a)--(f); similar to Fig.~\ref{fig:visualisations}), a summary of the parameters $V_\mathrm{fid}$, $V_\mathrm{max}$, $\eta_\mathrm{rot}$, and $\eta_\mathrm{bar}$ (panels (g)--(j); similar to Fig.~\ref{fig:loops}), and a summary of the rotation curve analysis from $24$ viewing angles (panels (k)--(n); similar to Fig.~\ref{fig:rot_curves}). See description of Appendix~\ref{app:supplementary} for details.}
\label{fig:S29}
\end{figure}
\clearpage

\begin{figure}
\begin{minipage}{.9\textwidth}
\includegraphics[width=\textwidth]{../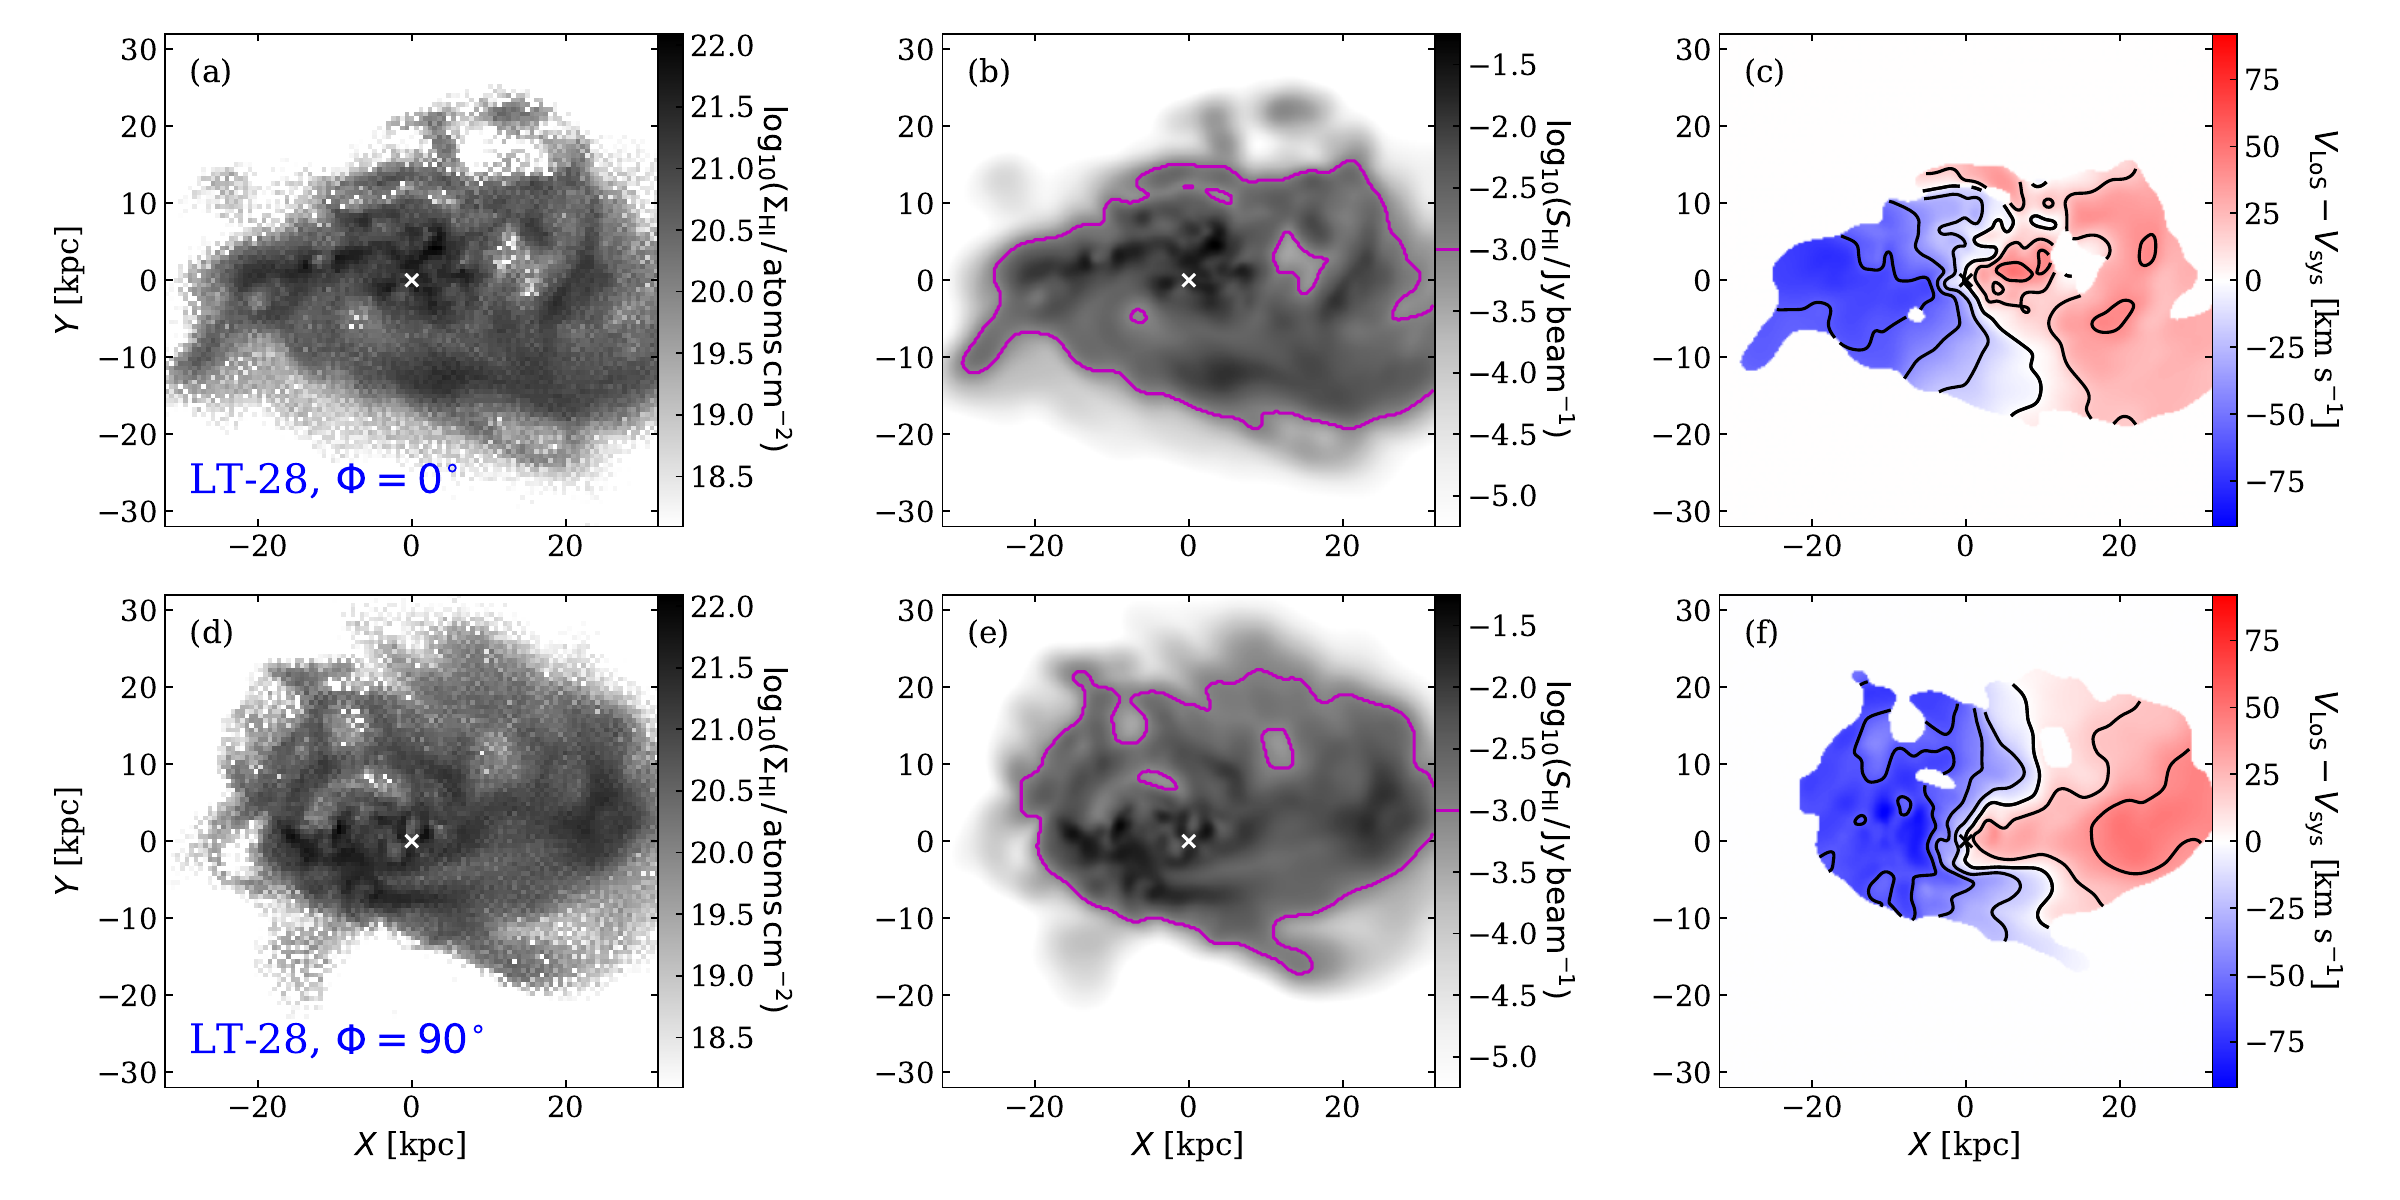}
\includegraphics[width=\textwidth]{../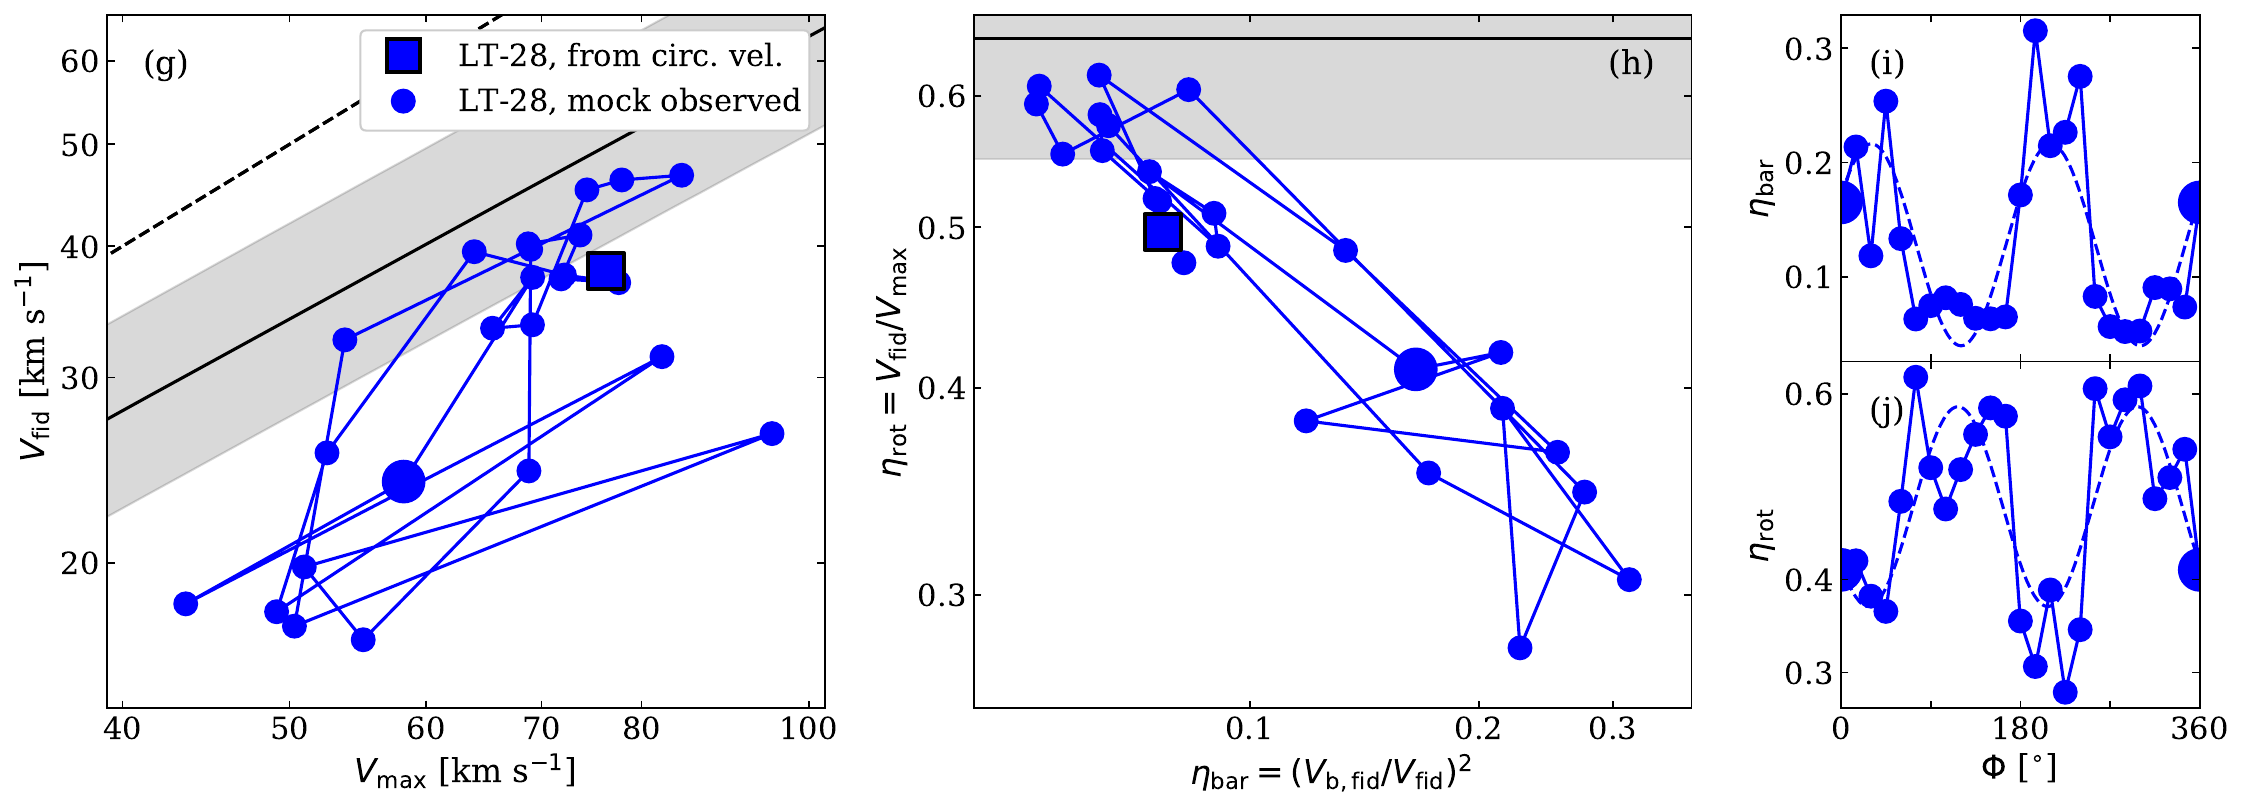}
\end{minipage}
\begin{minipage}{.4\textwidth}
\includegraphics[width=\textwidth]{../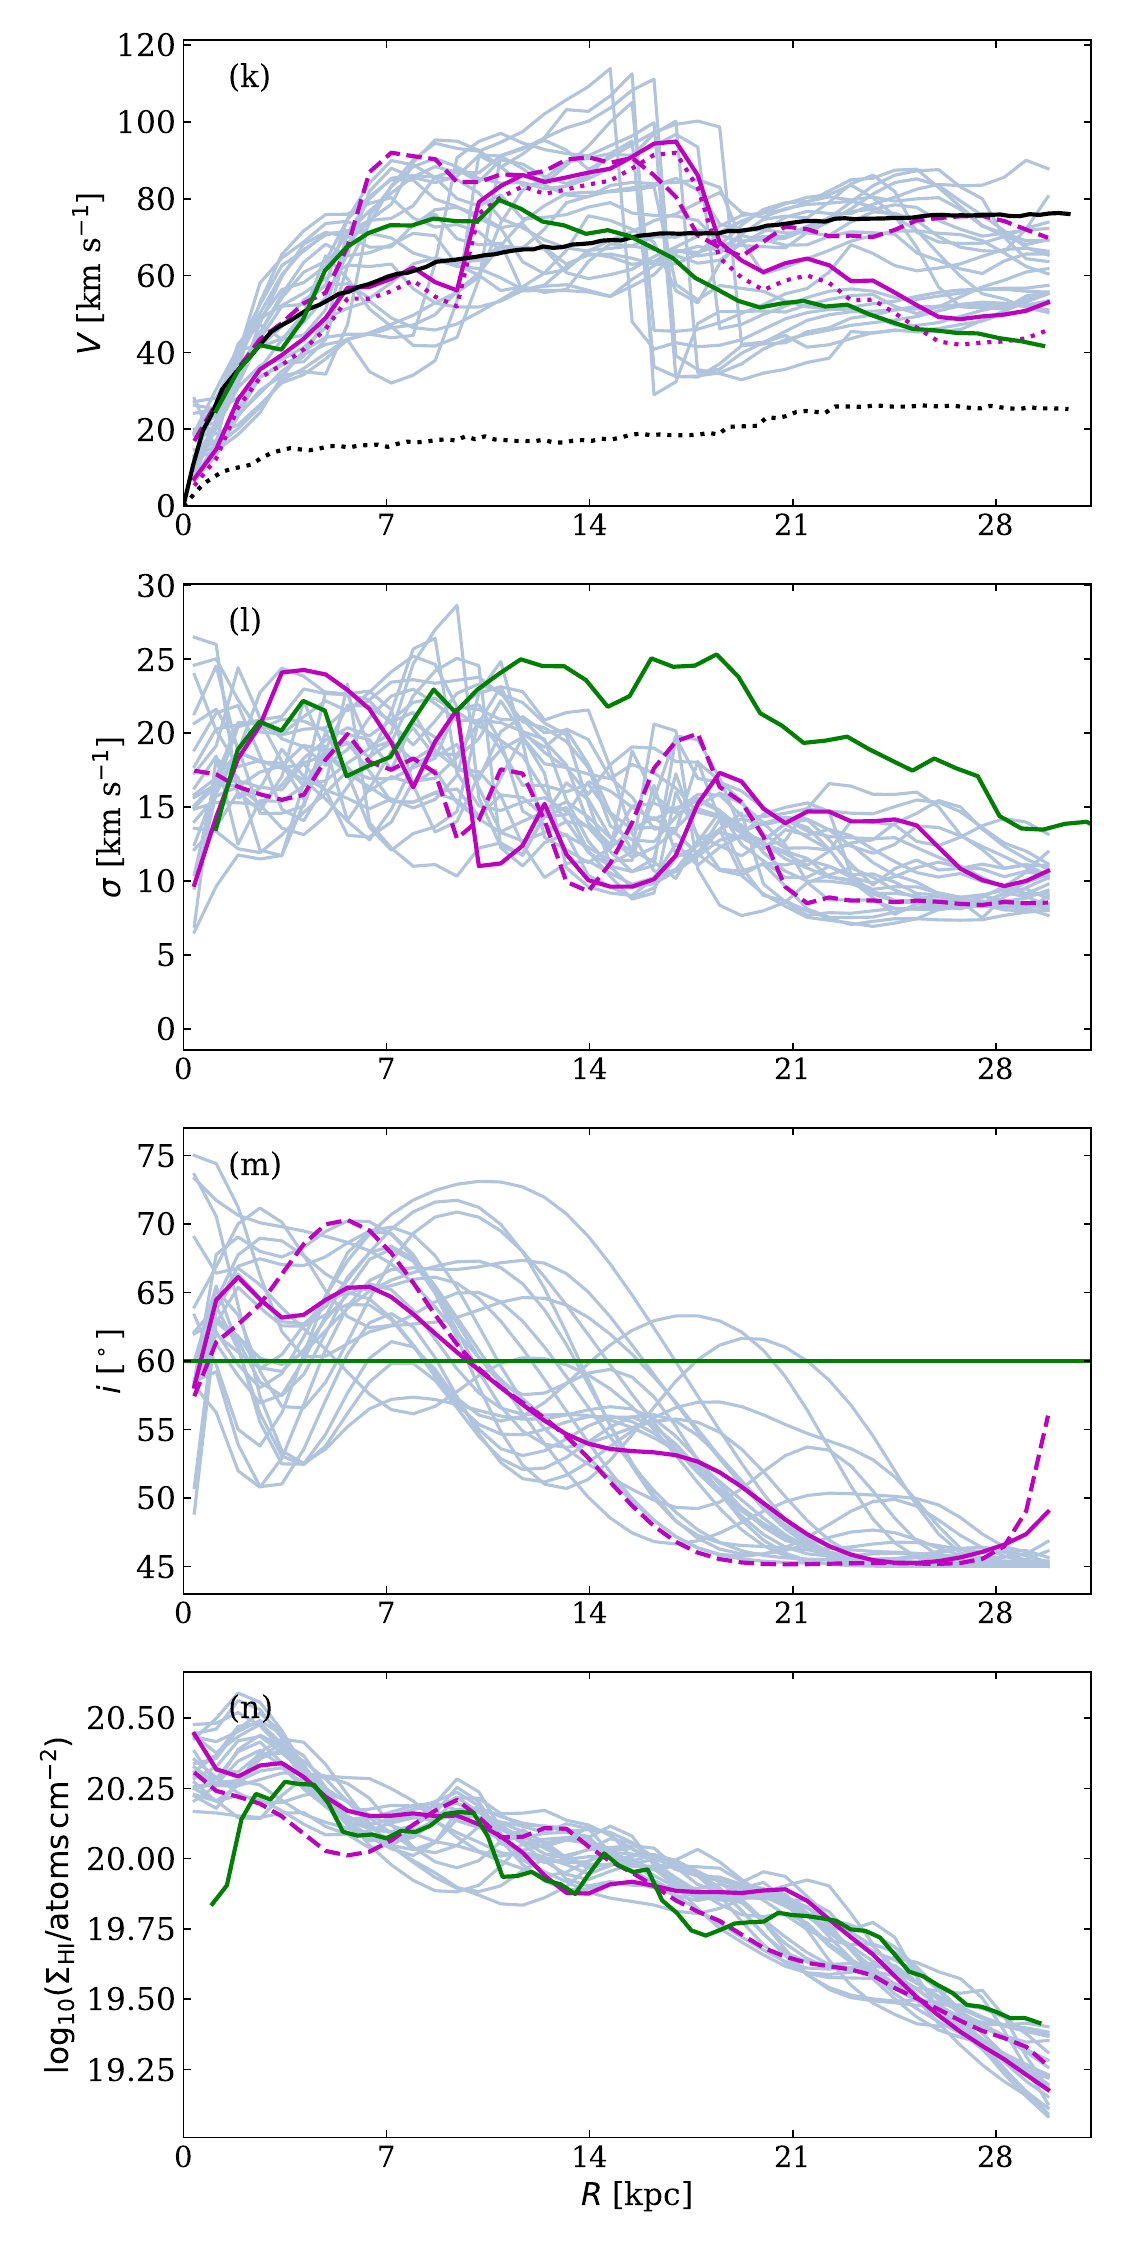}
\end{minipage}
\caption{A set of summary figures for galaxy LT-28, excluded from kinematic analysis. These include example moment maps for two orientations (panels (a)--(f); similar to Fig.~\ref{fig:visualisations}), a summary of the parameters $V_\mathrm{fid}$, $V_\mathrm{max}$, $\eta_\mathrm{rot}$, and $\eta_\mathrm{bar}$ (panels (g)--(j); similar to Fig.~\ref{fig:loops}), and a summary of the rotation curve analysis from $24$ viewing angles (panels (k)--(n); similar to Fig.~\ref{fig:rot_curves}). See description of Appendix~\ref{app:supplementary} for details.}
\label{fig:S30}
\end{figure}
\clearpage

\begin{figure}
\begin{minipage}{.9\textwidth}
\includegraphics[width=\textwidth]{../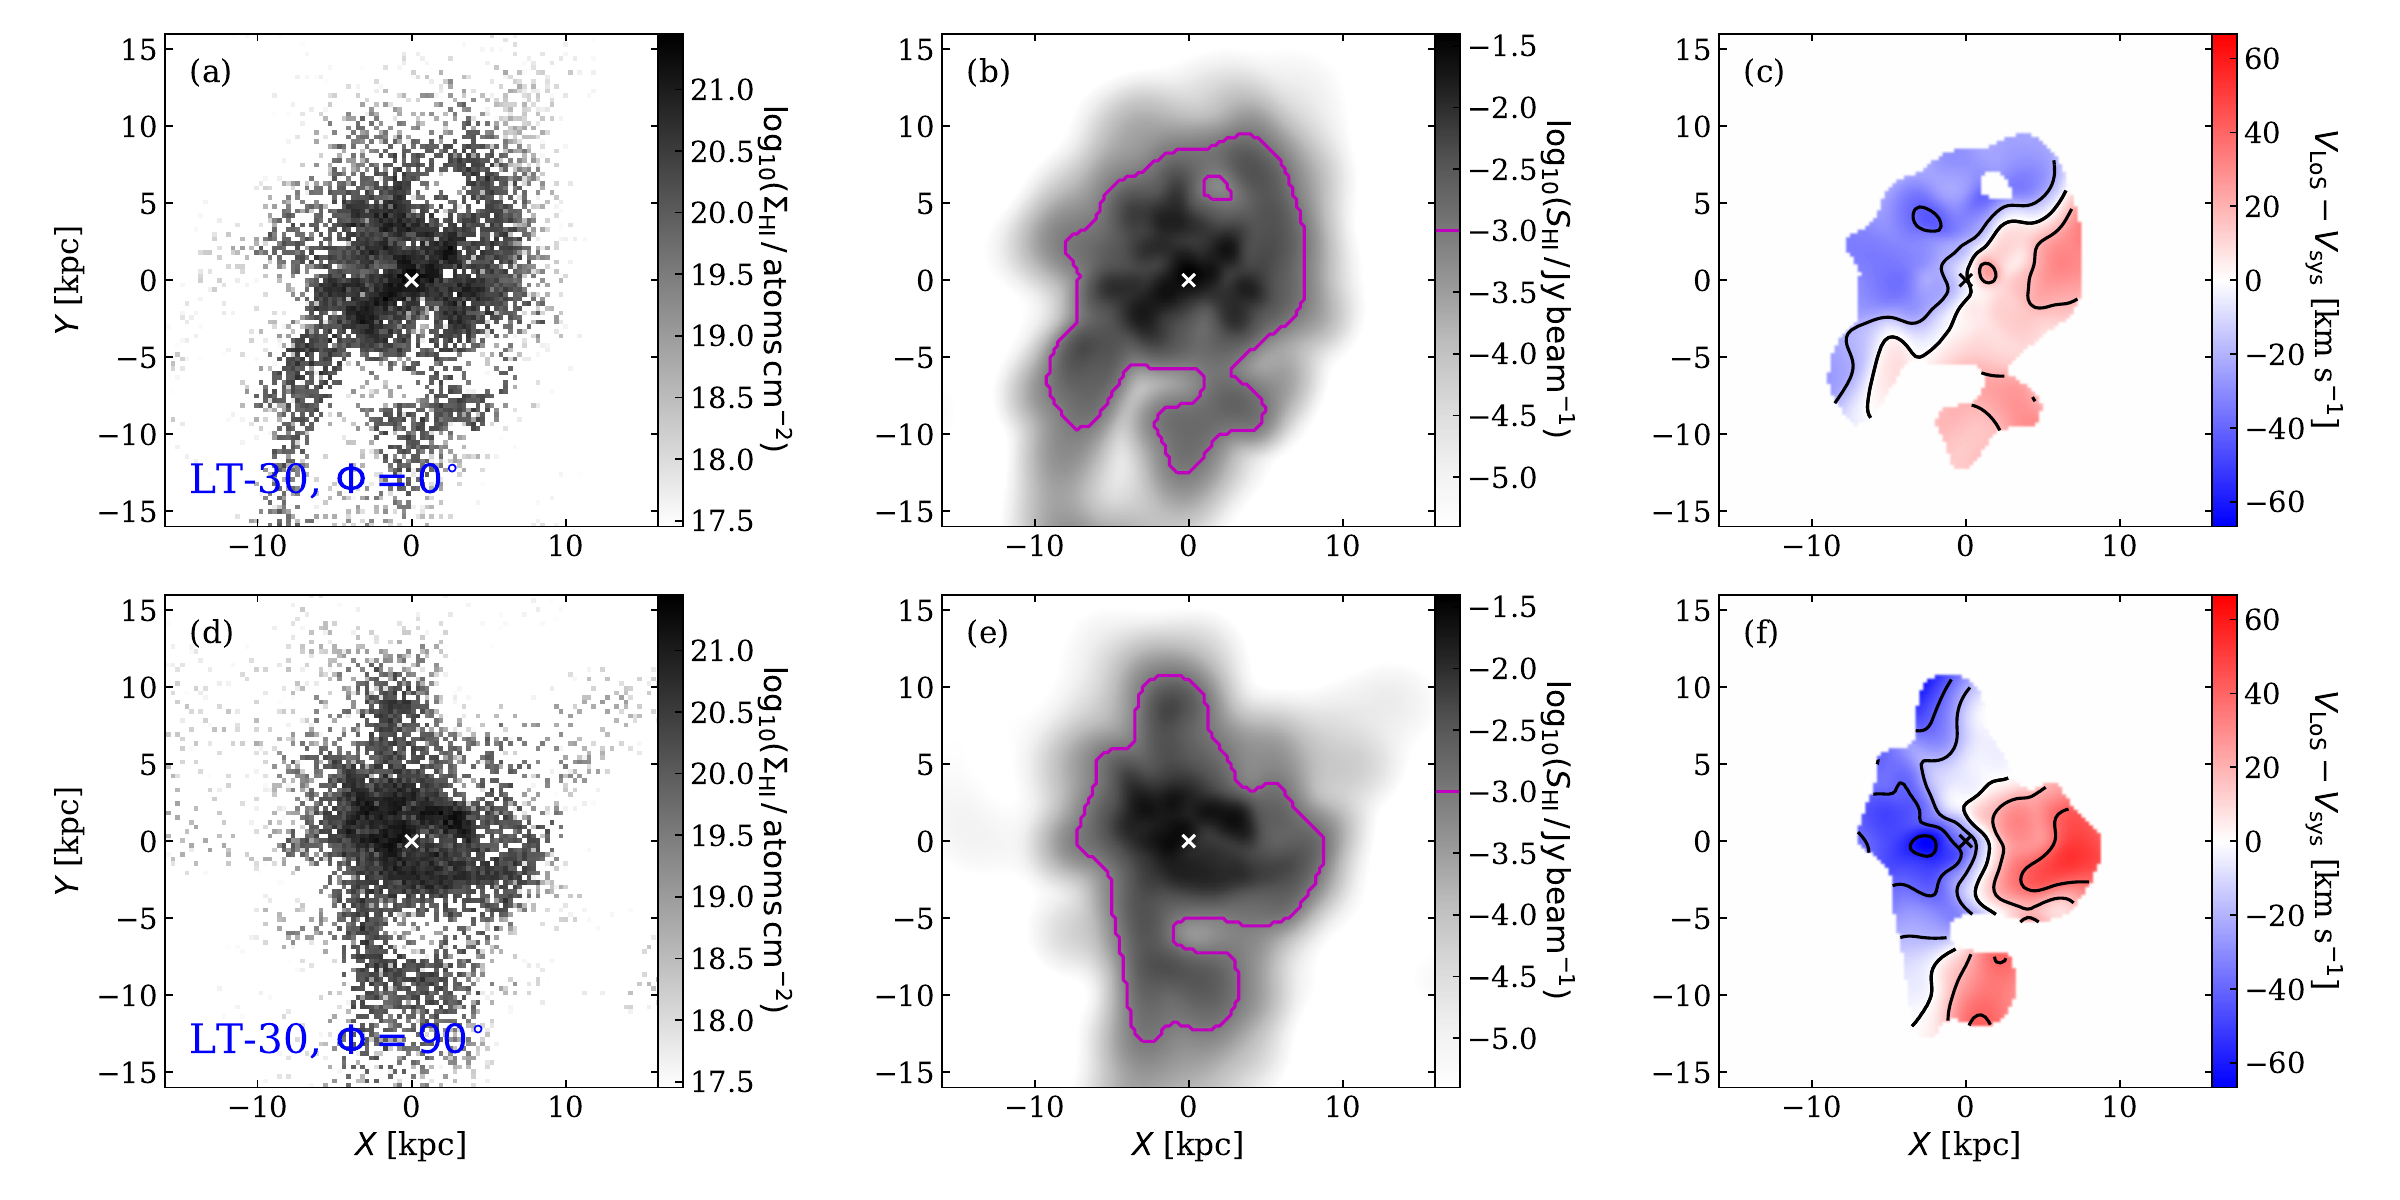}
\includegraphics[width=\textwidth]{../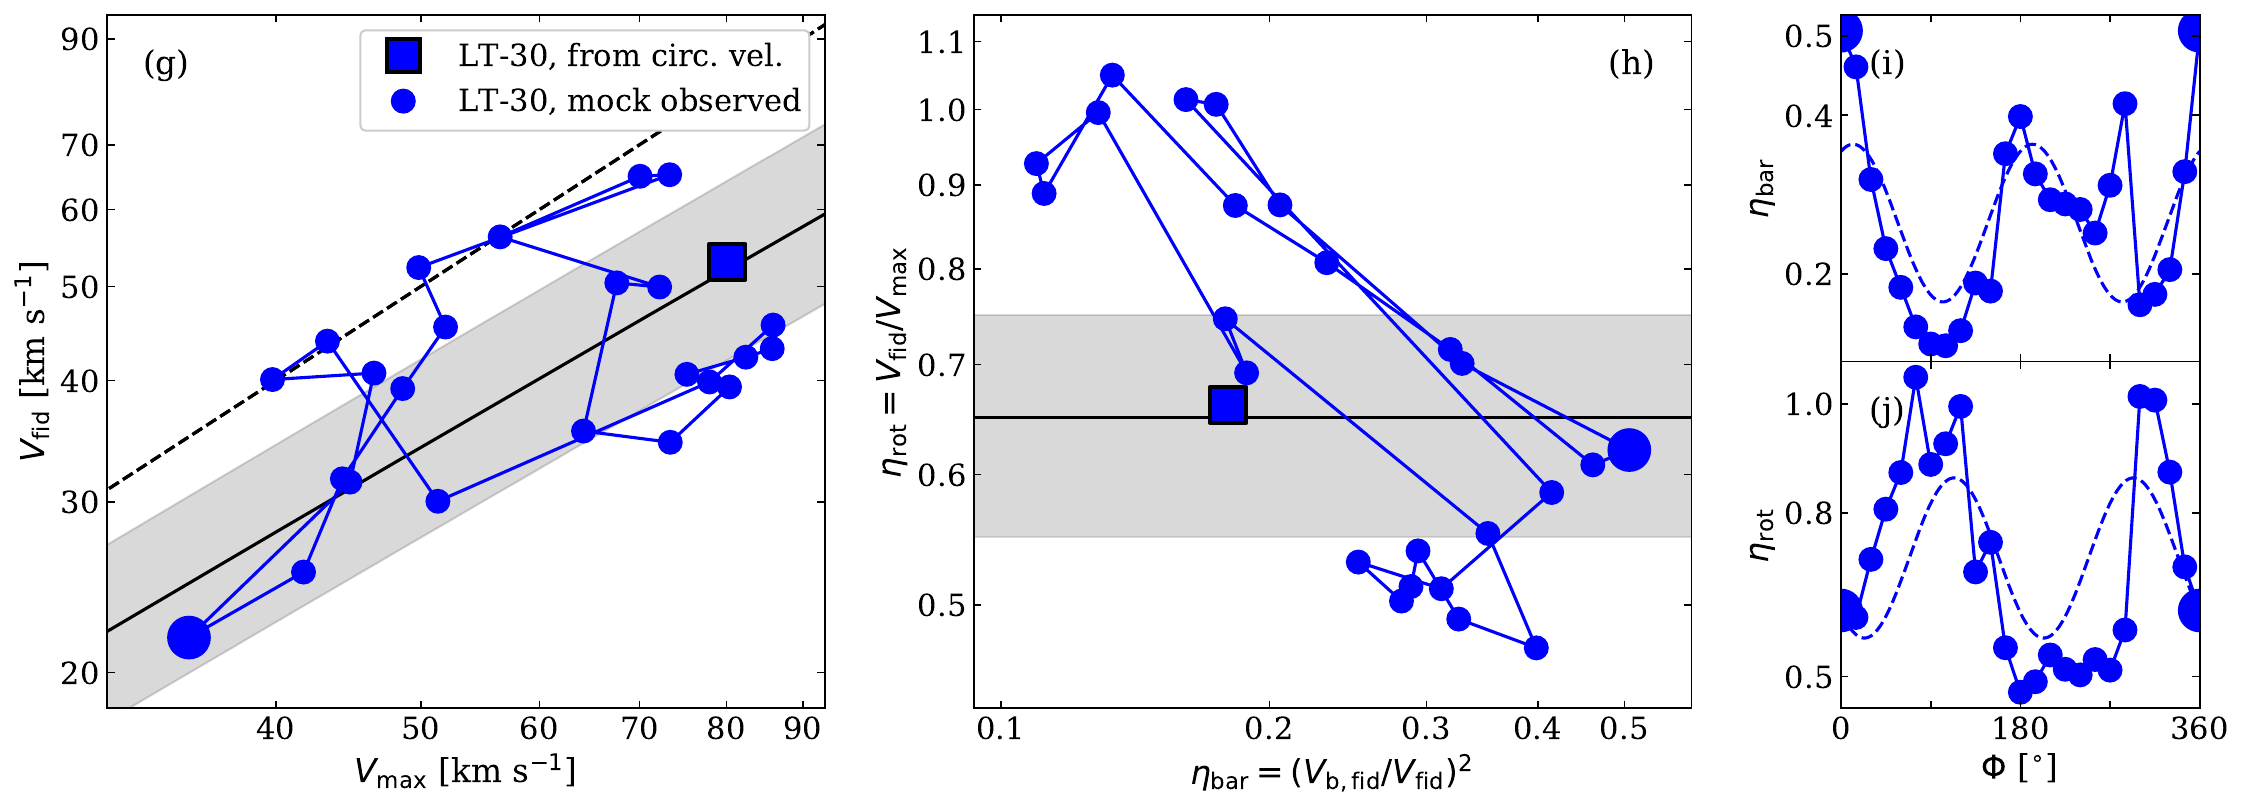}
\end{minipage}
\begin{minipage}{.4\textwidth}
\includegraphics[width=\textwidth]{../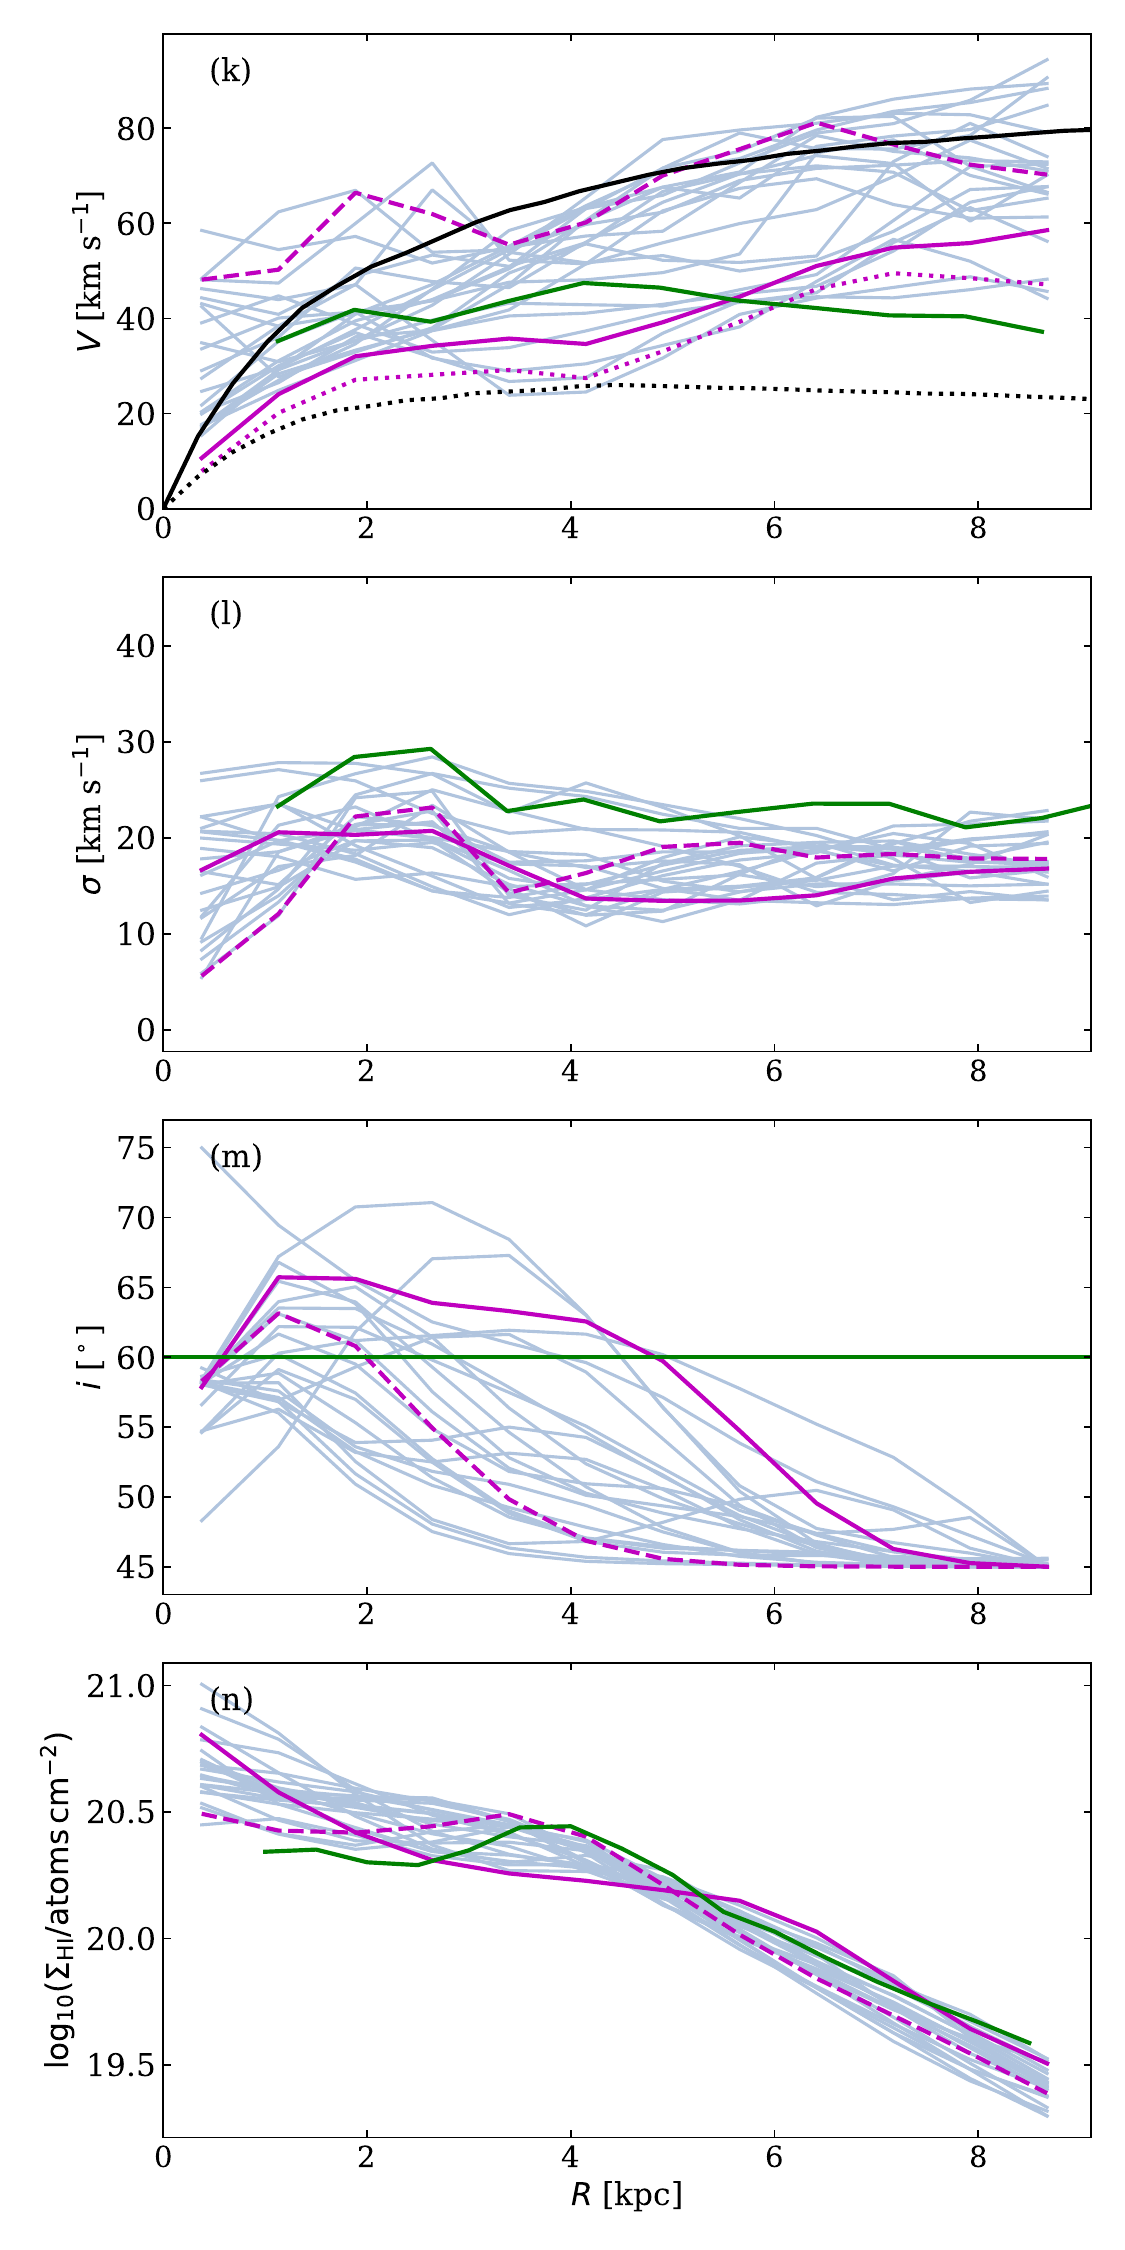}
\end{minipage}
\caption{A set of summary figures for galaxy LT-30, excluded from kinematic analysis. These include example moment maps for two orientations (panels (a)--(f); similar to Fig.~\ref{fig:visualisations}), a summary of the parameters $V_\mathrm{fid}$, $V_\mathrm{max}$, $\eta_\mathrm{rot}$, and $\eta_\mathrm{bar}$ (panels (g)--(j); similar to Fig.~\ref{fig:loops}), and a summary of the rotation curve analysis from $24$ viewing angles (panels (k)--(n); similar to Fig.~\ref{fig:rot_curves}). See description of Appendix~\ref{app:supplementary} for details.}
\label{fig:S31}
\end{figure}
\clearpage

\begin{figure}
\begin{minipage}{.9\textwidth}
\includegraphics[width=\textwidth]{../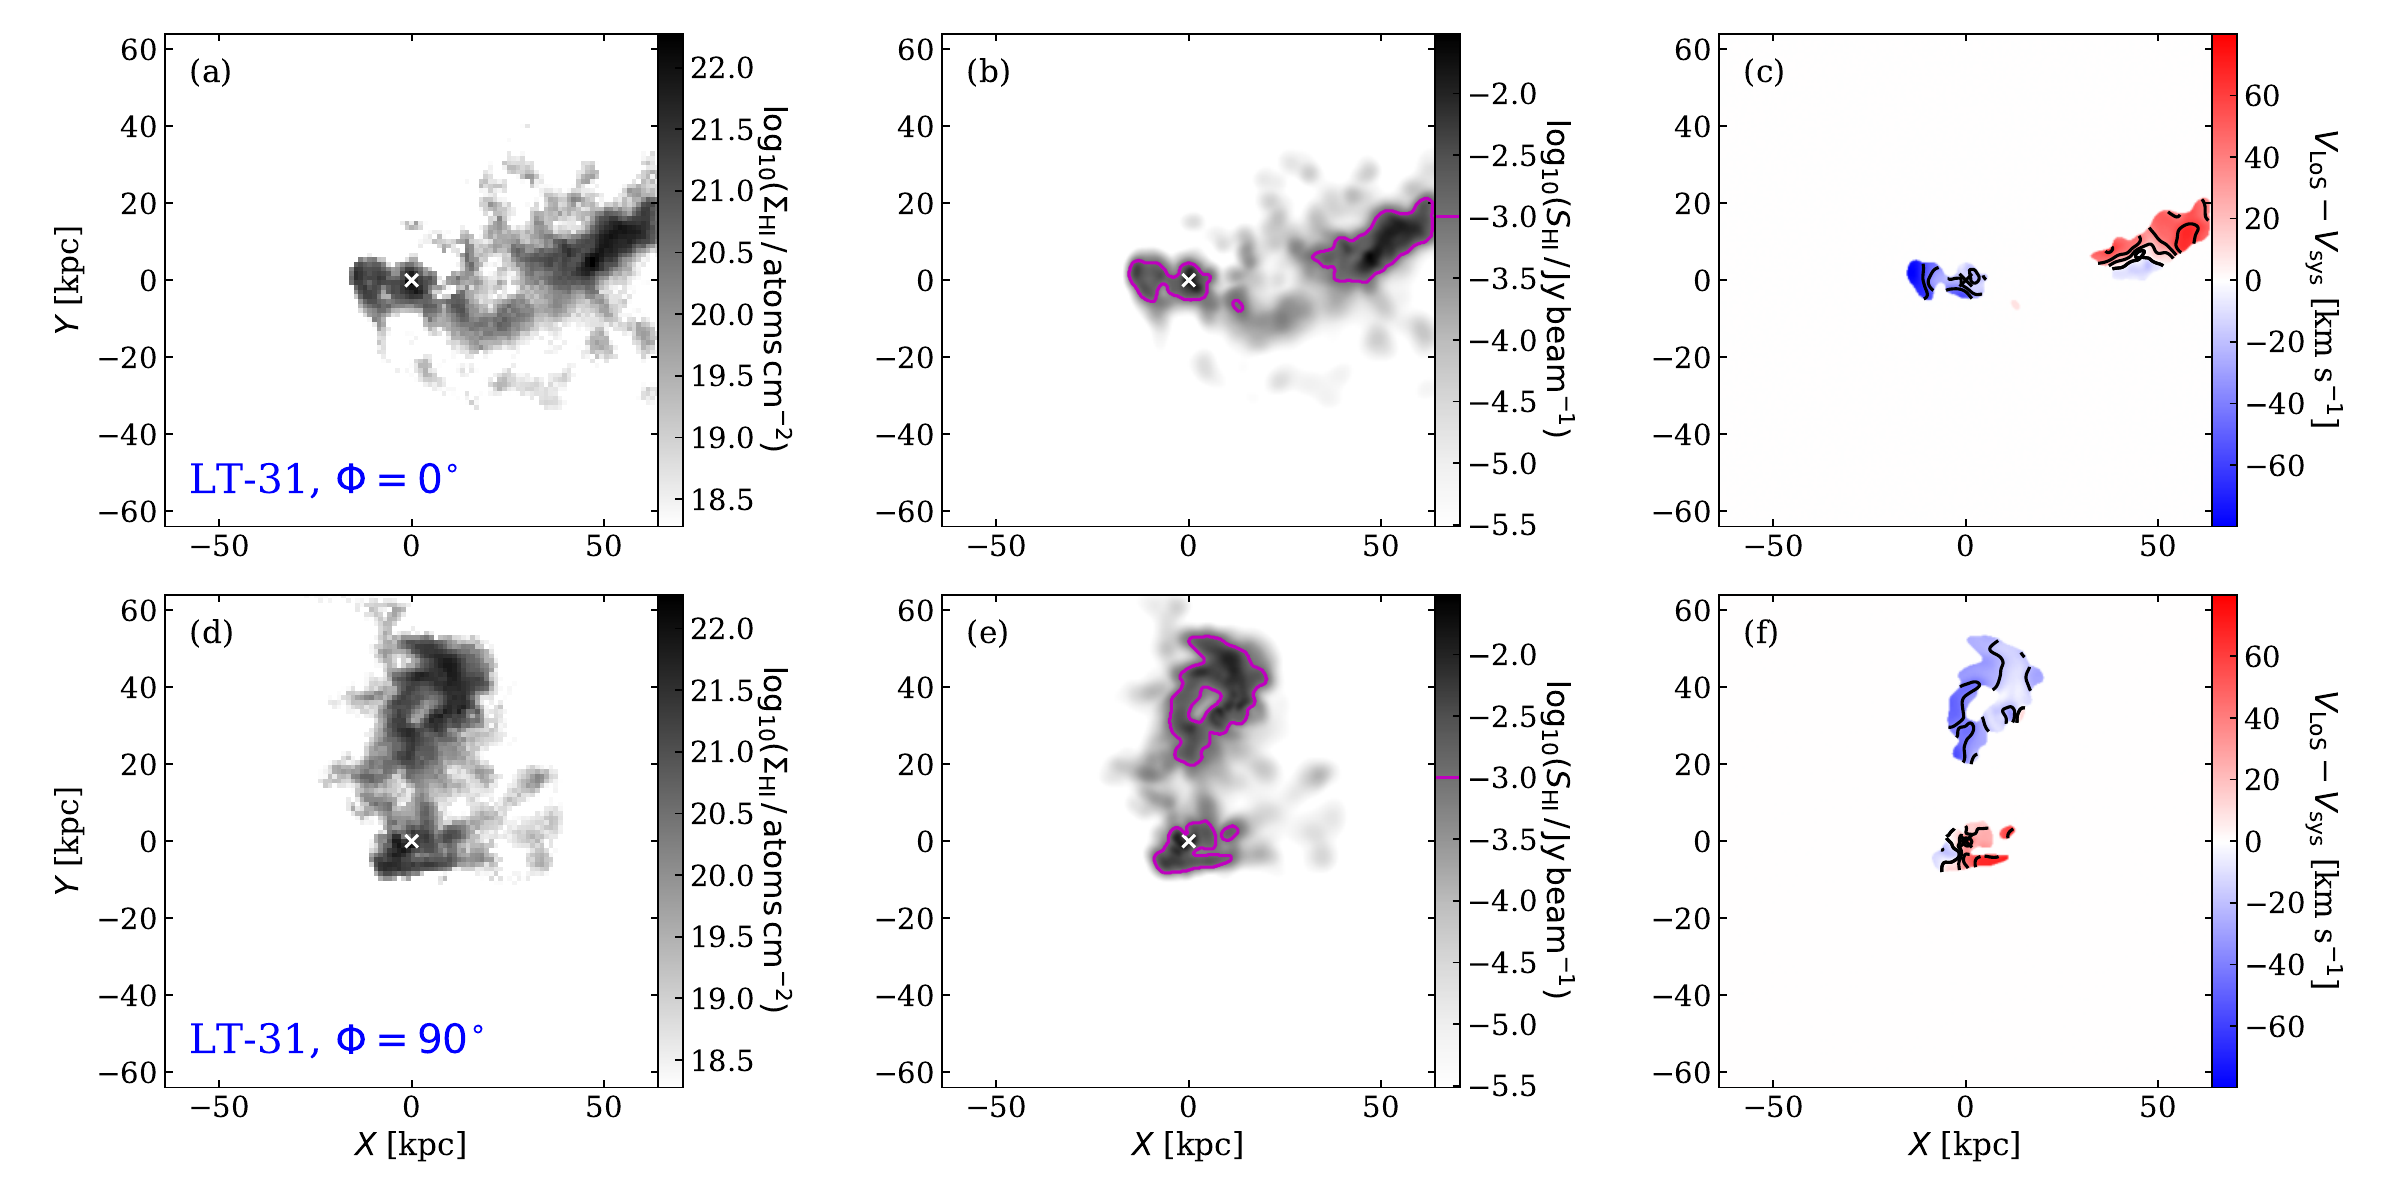}
\includegraphics[width=\textwidth]{../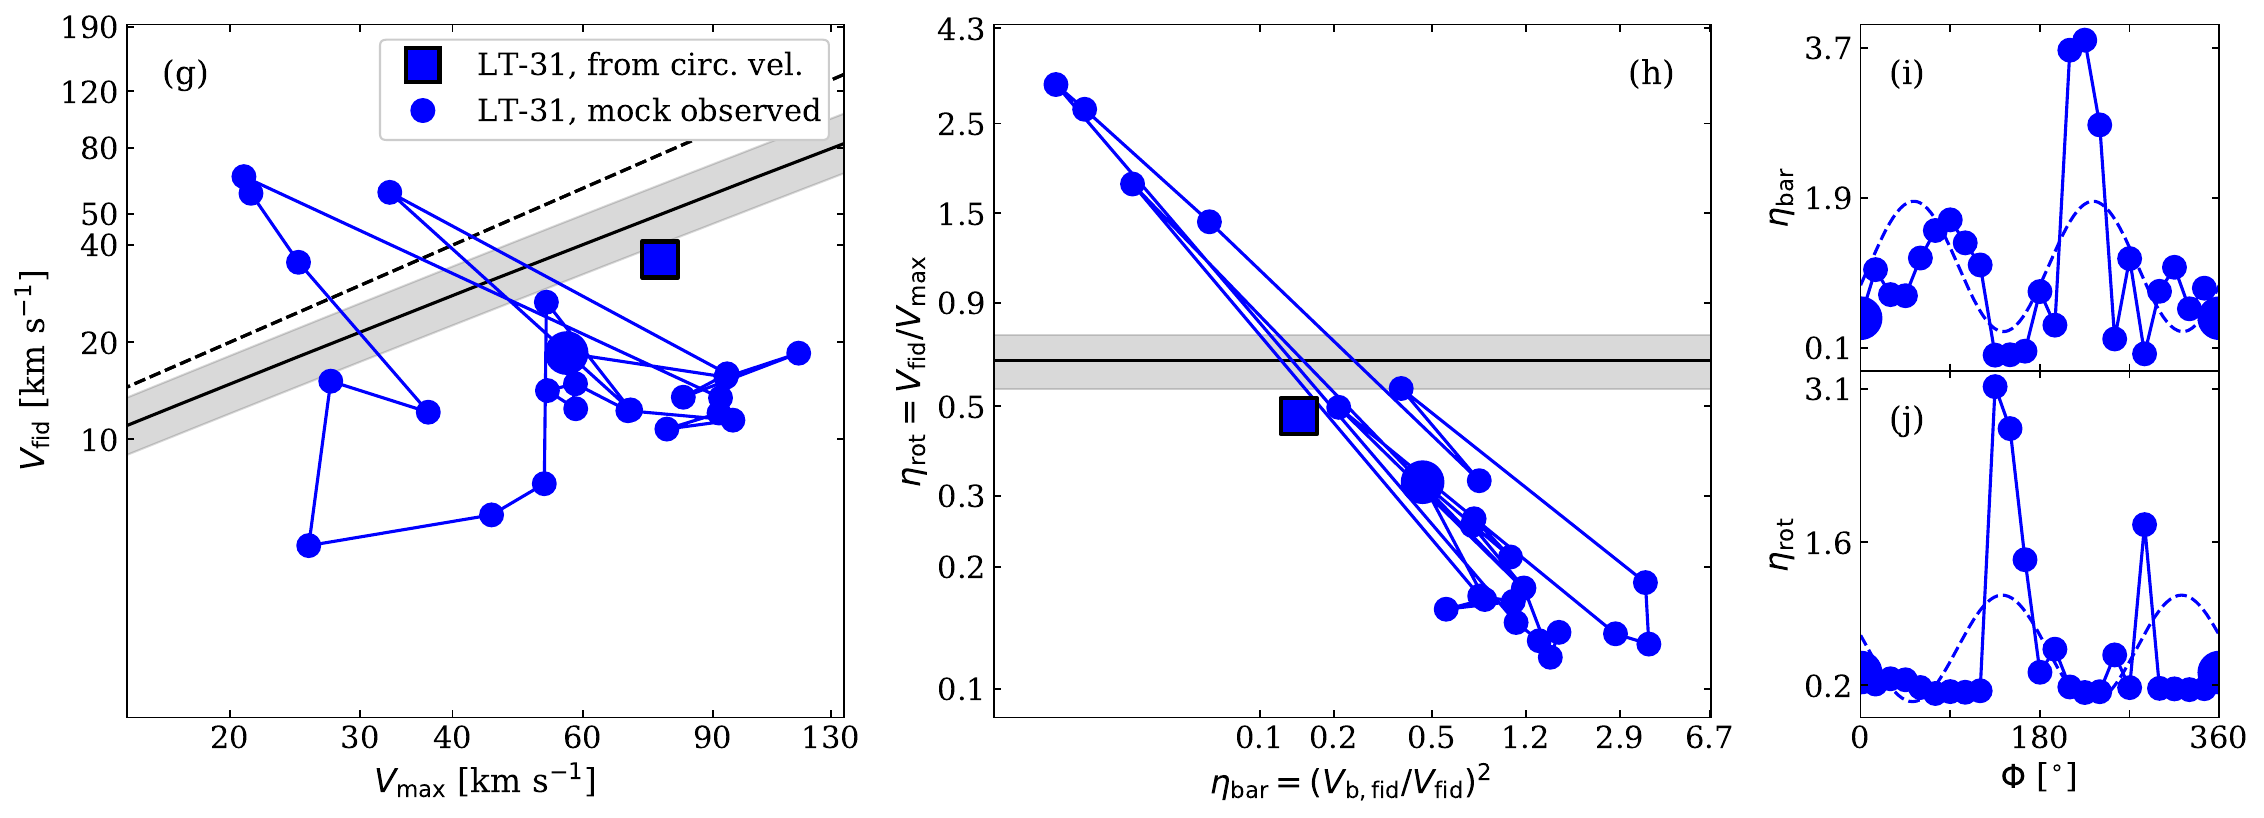}
\end{minipage}
\begin{minipage}{.4\textwidth}
\includegraphics[width=\textwidth]{../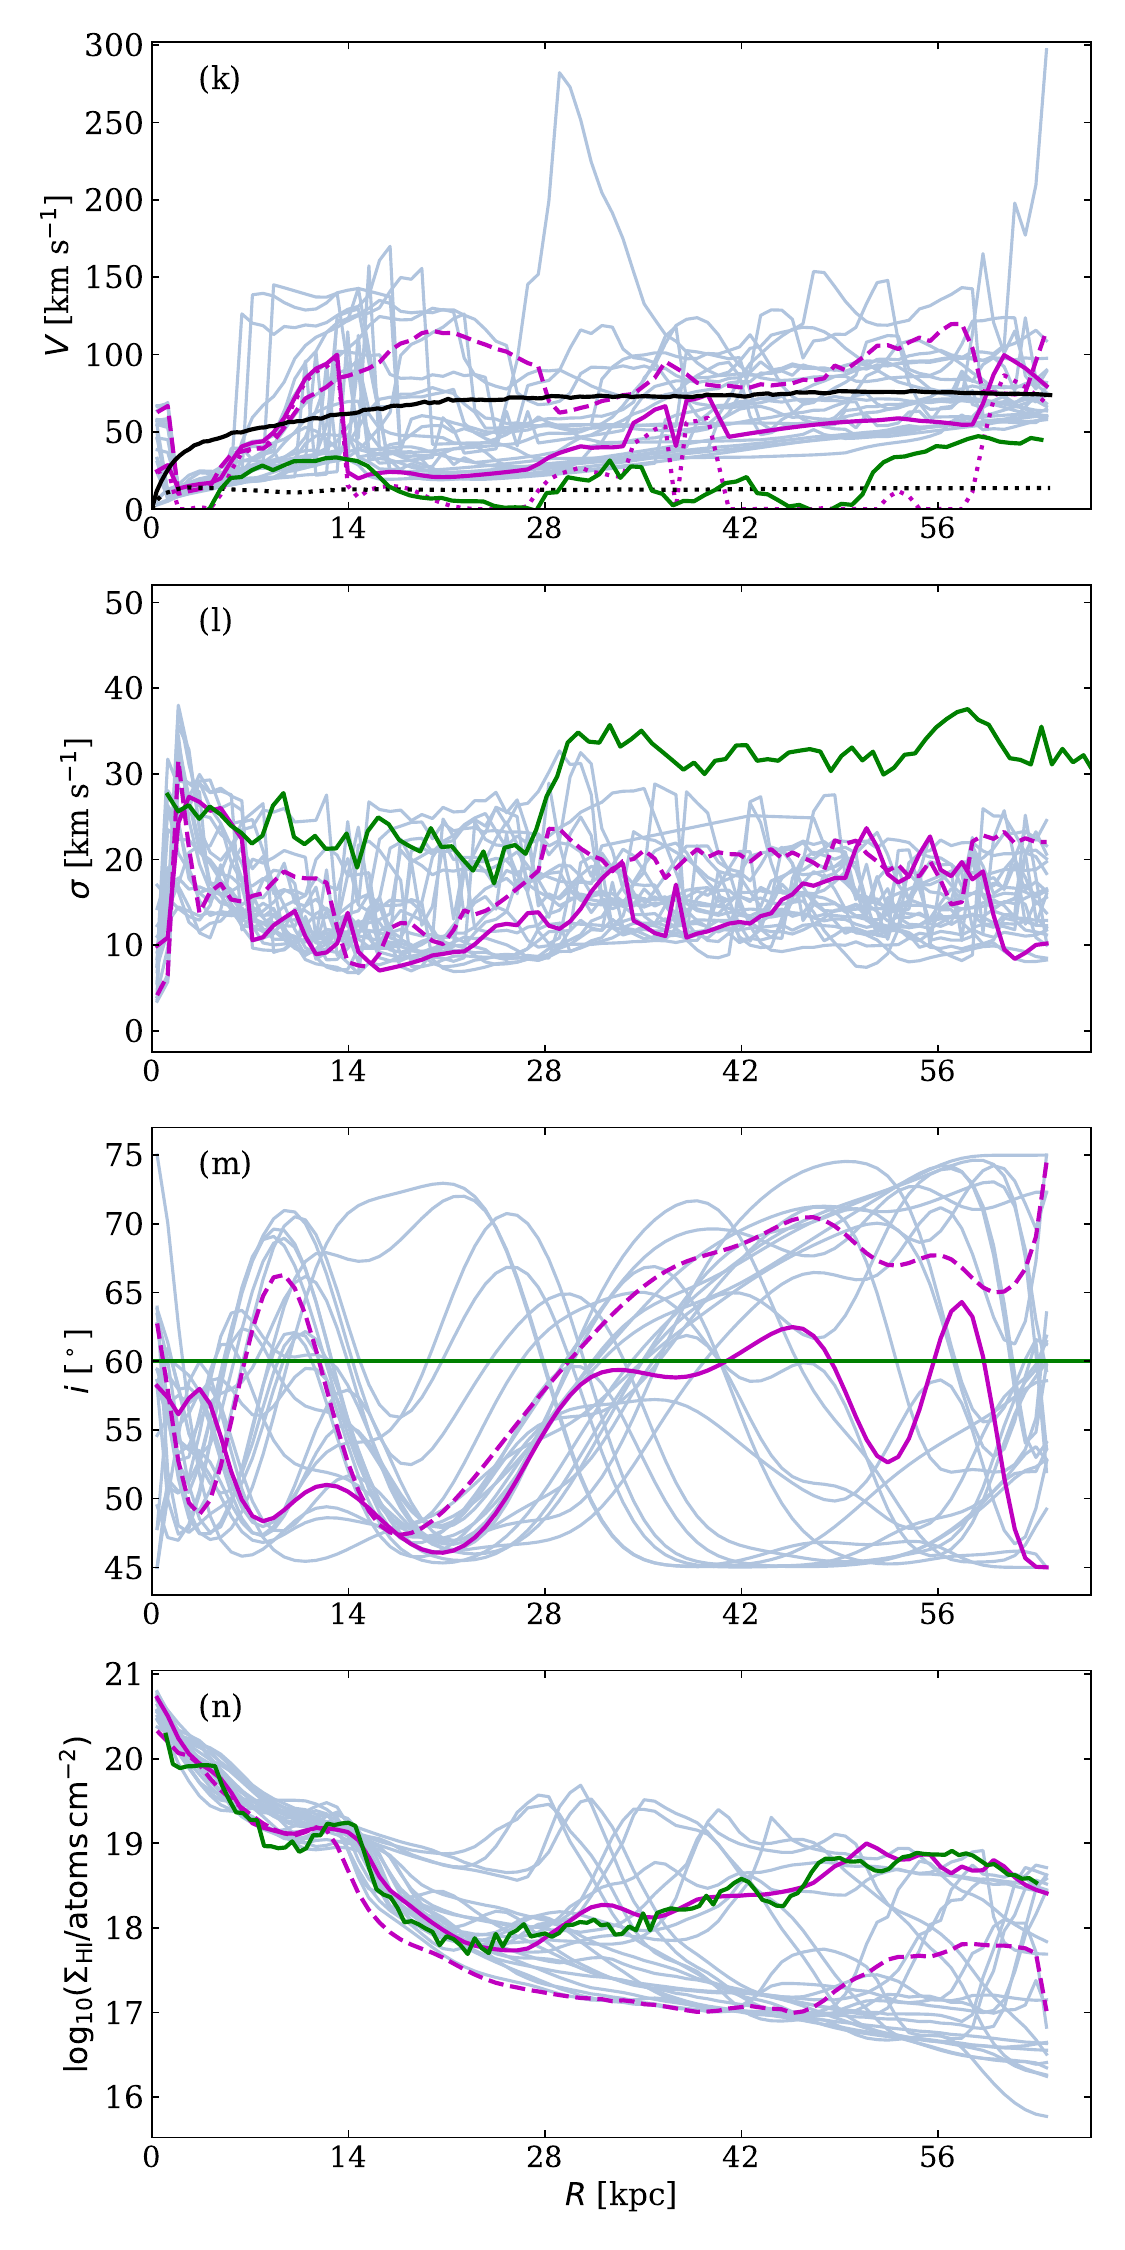}
\end{minipage}
\caption{A set of summary figures for galaxy LT-31, excluded from kinematic analysis. These include example moment maps for two orientations (panels (a)--(f); similar to Fig.~\ref{fig:visualisations}), a summary of the parameters $V_\mathrm{fid}$, $V_\mathrm{max}$, $\eta_\mathrm{rot}$, and $\eta_\mathrm{bar}$ (panels (g)--(j); similar to Fig.~\ref{fig:loops}), and a summary of the rotation curve analysis from $24$ viewing angles (panels (k)--(n); similar to Fig.~\ref{fig:rot_curves}). See description of Appendix~\ref{app:supplementary} for details.}
\label{fig:S32}
\end{figure}
\clearpage

\begin{figure}
\begin{minipage}{.9\textwidth}
\includegraphics[width=\textwidth]{../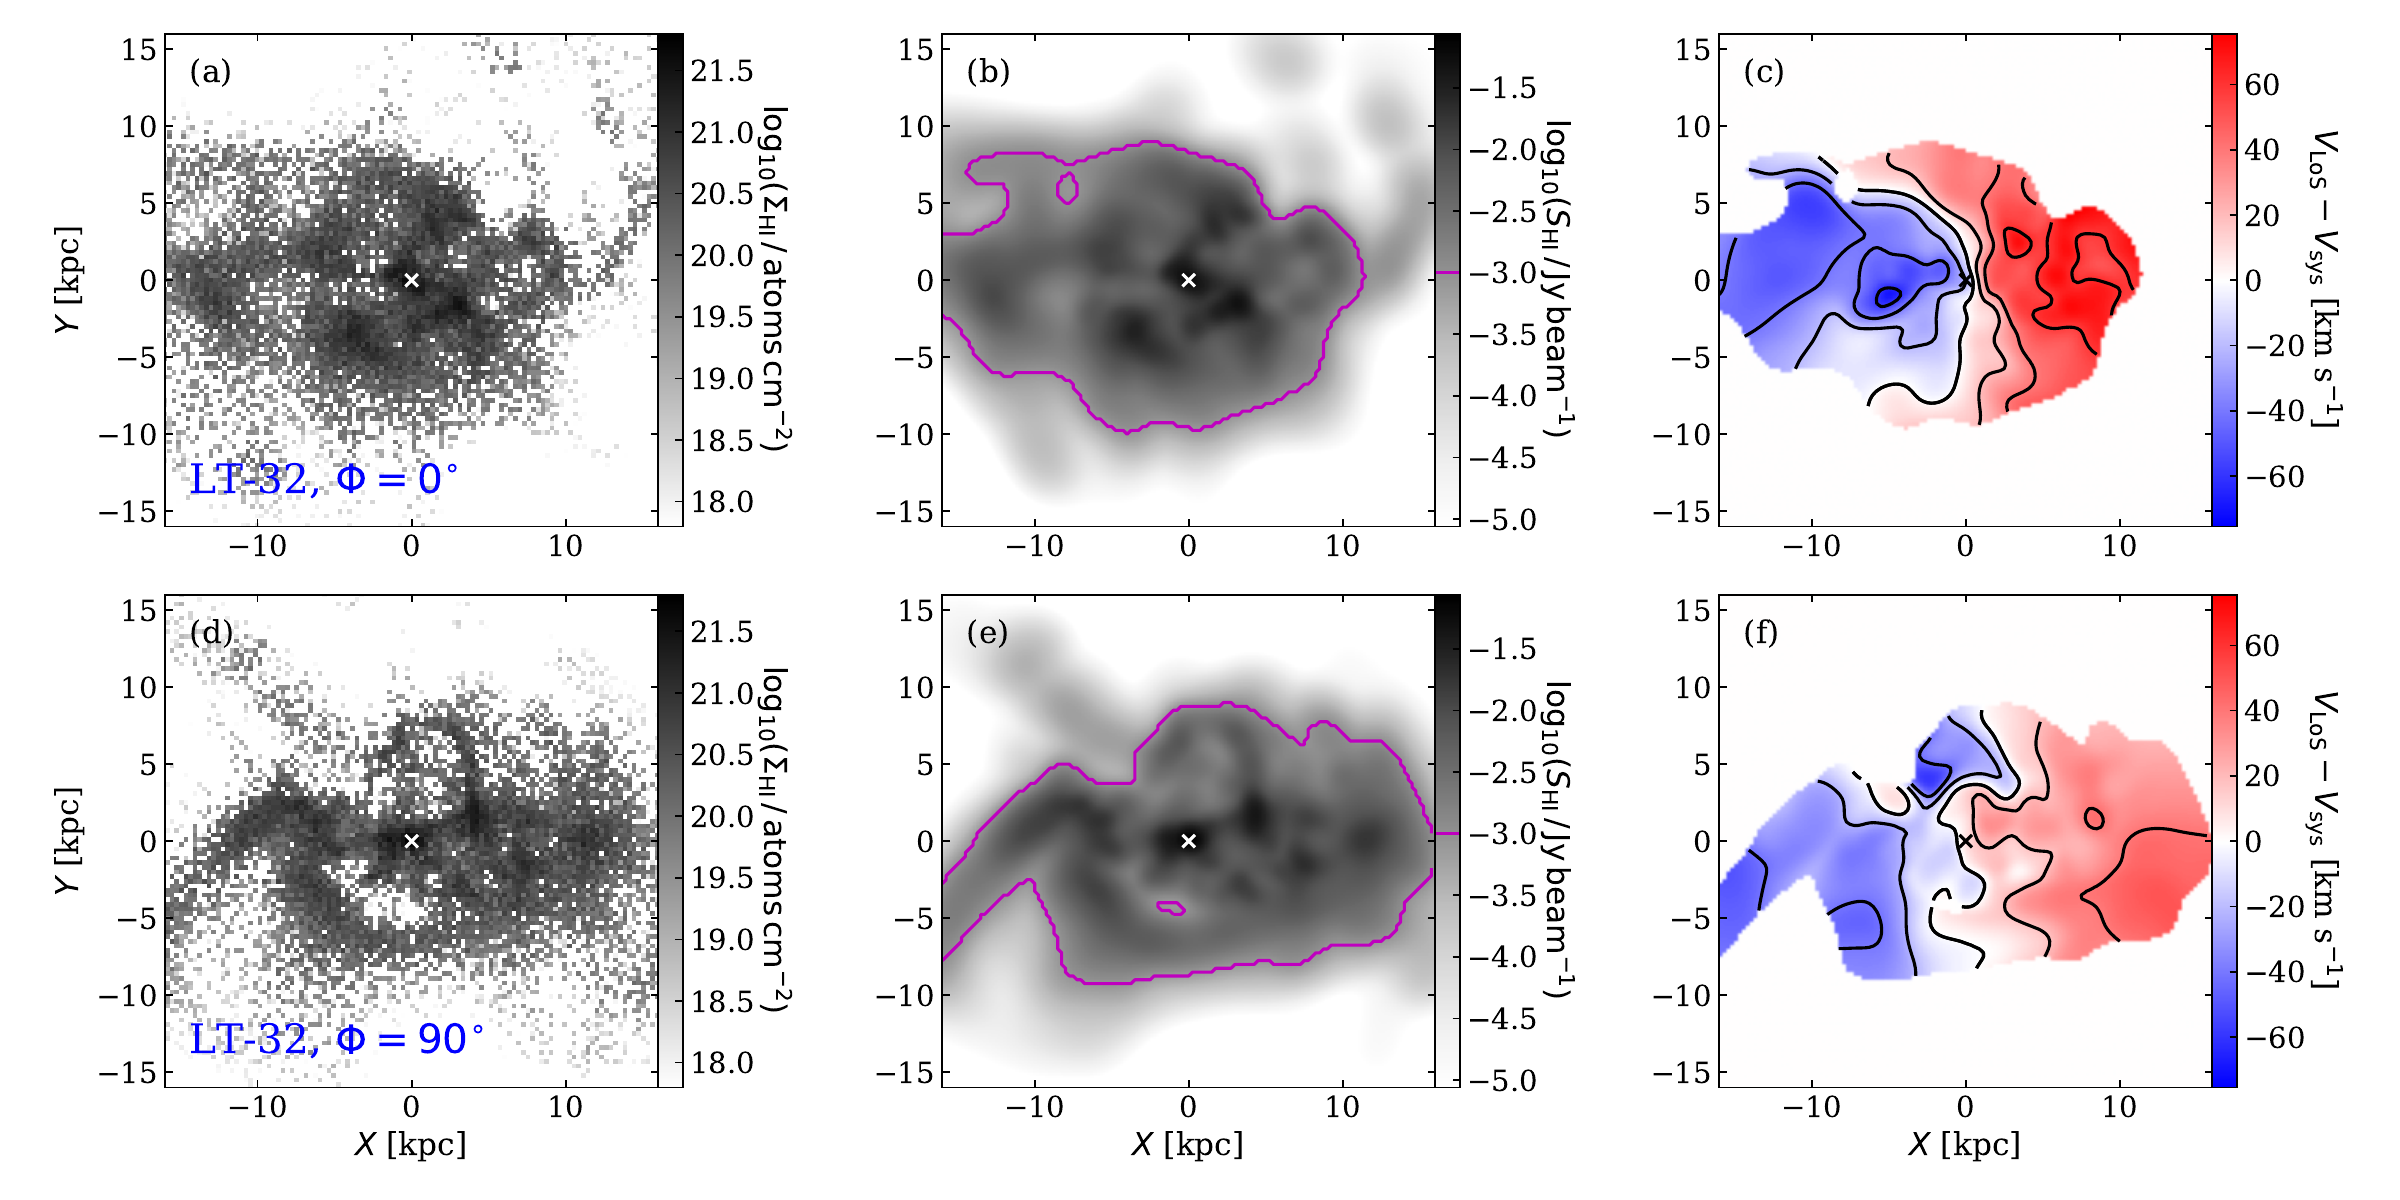}
\includegraphics[width=\textwidth]{../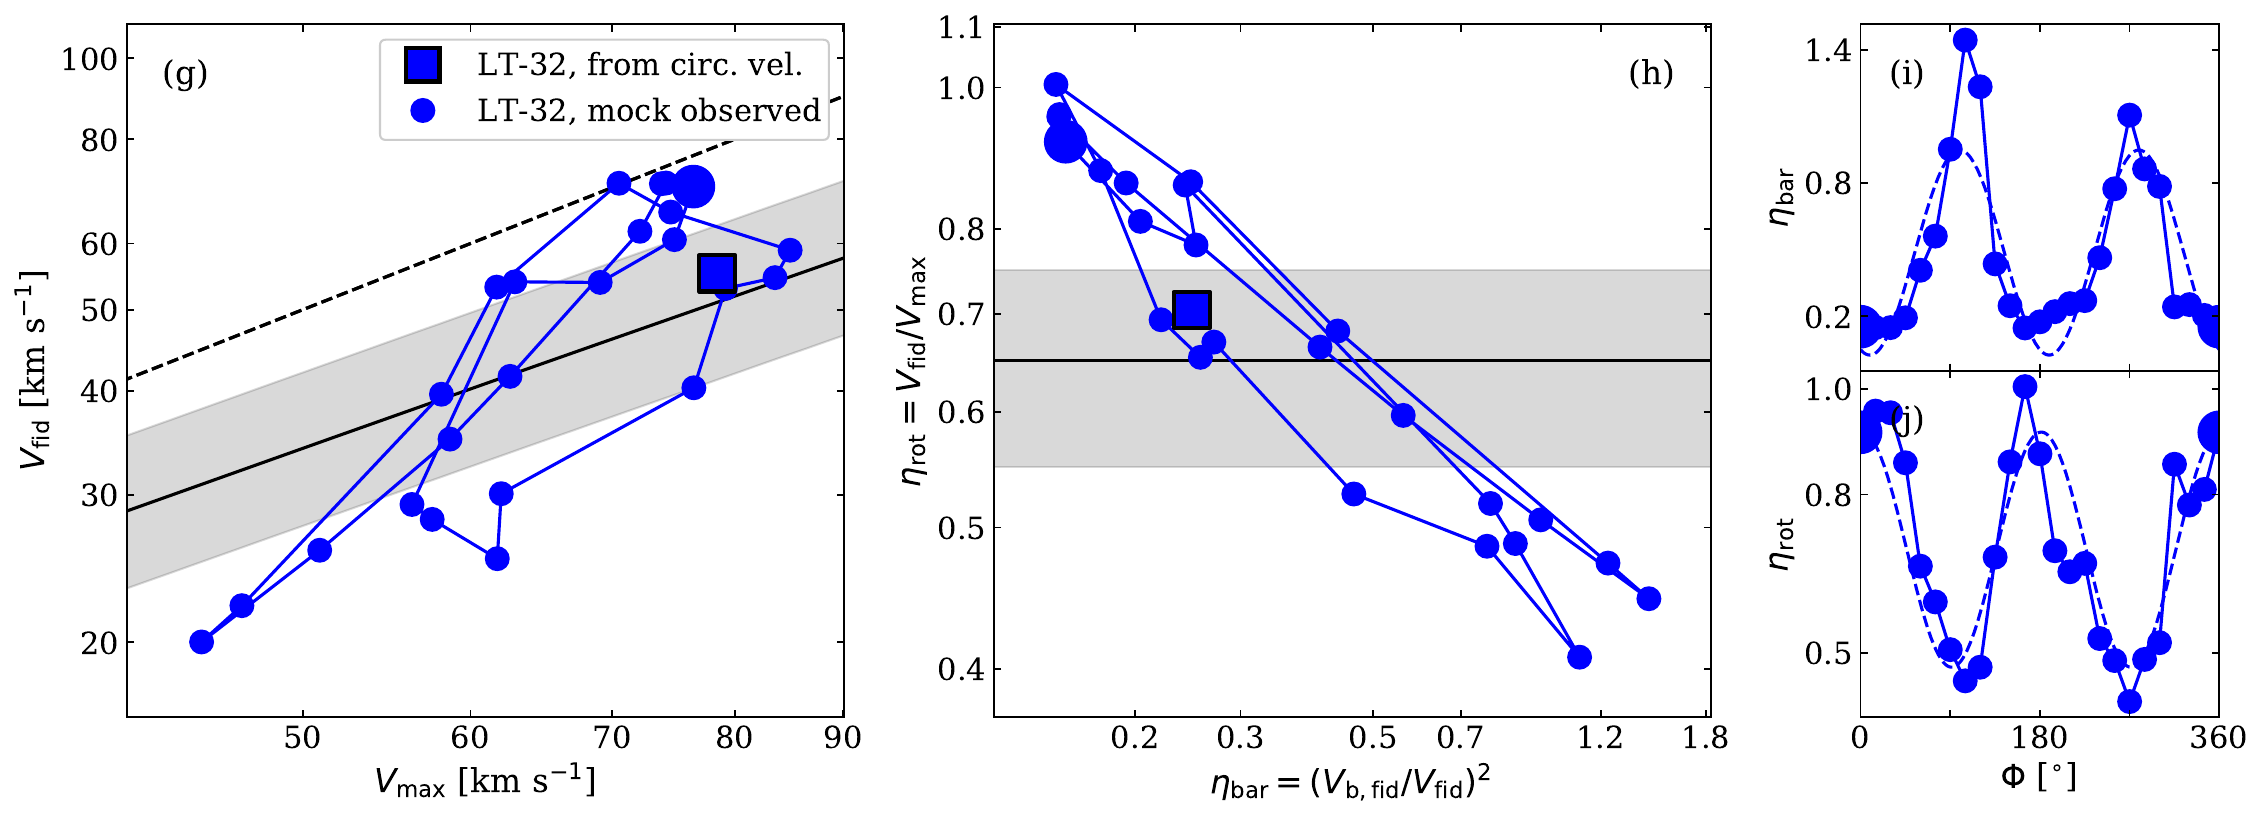}
\end{minipage}
\begin{minipage}{.4\textwidth}
\includegraphics[width=\textwidth]{../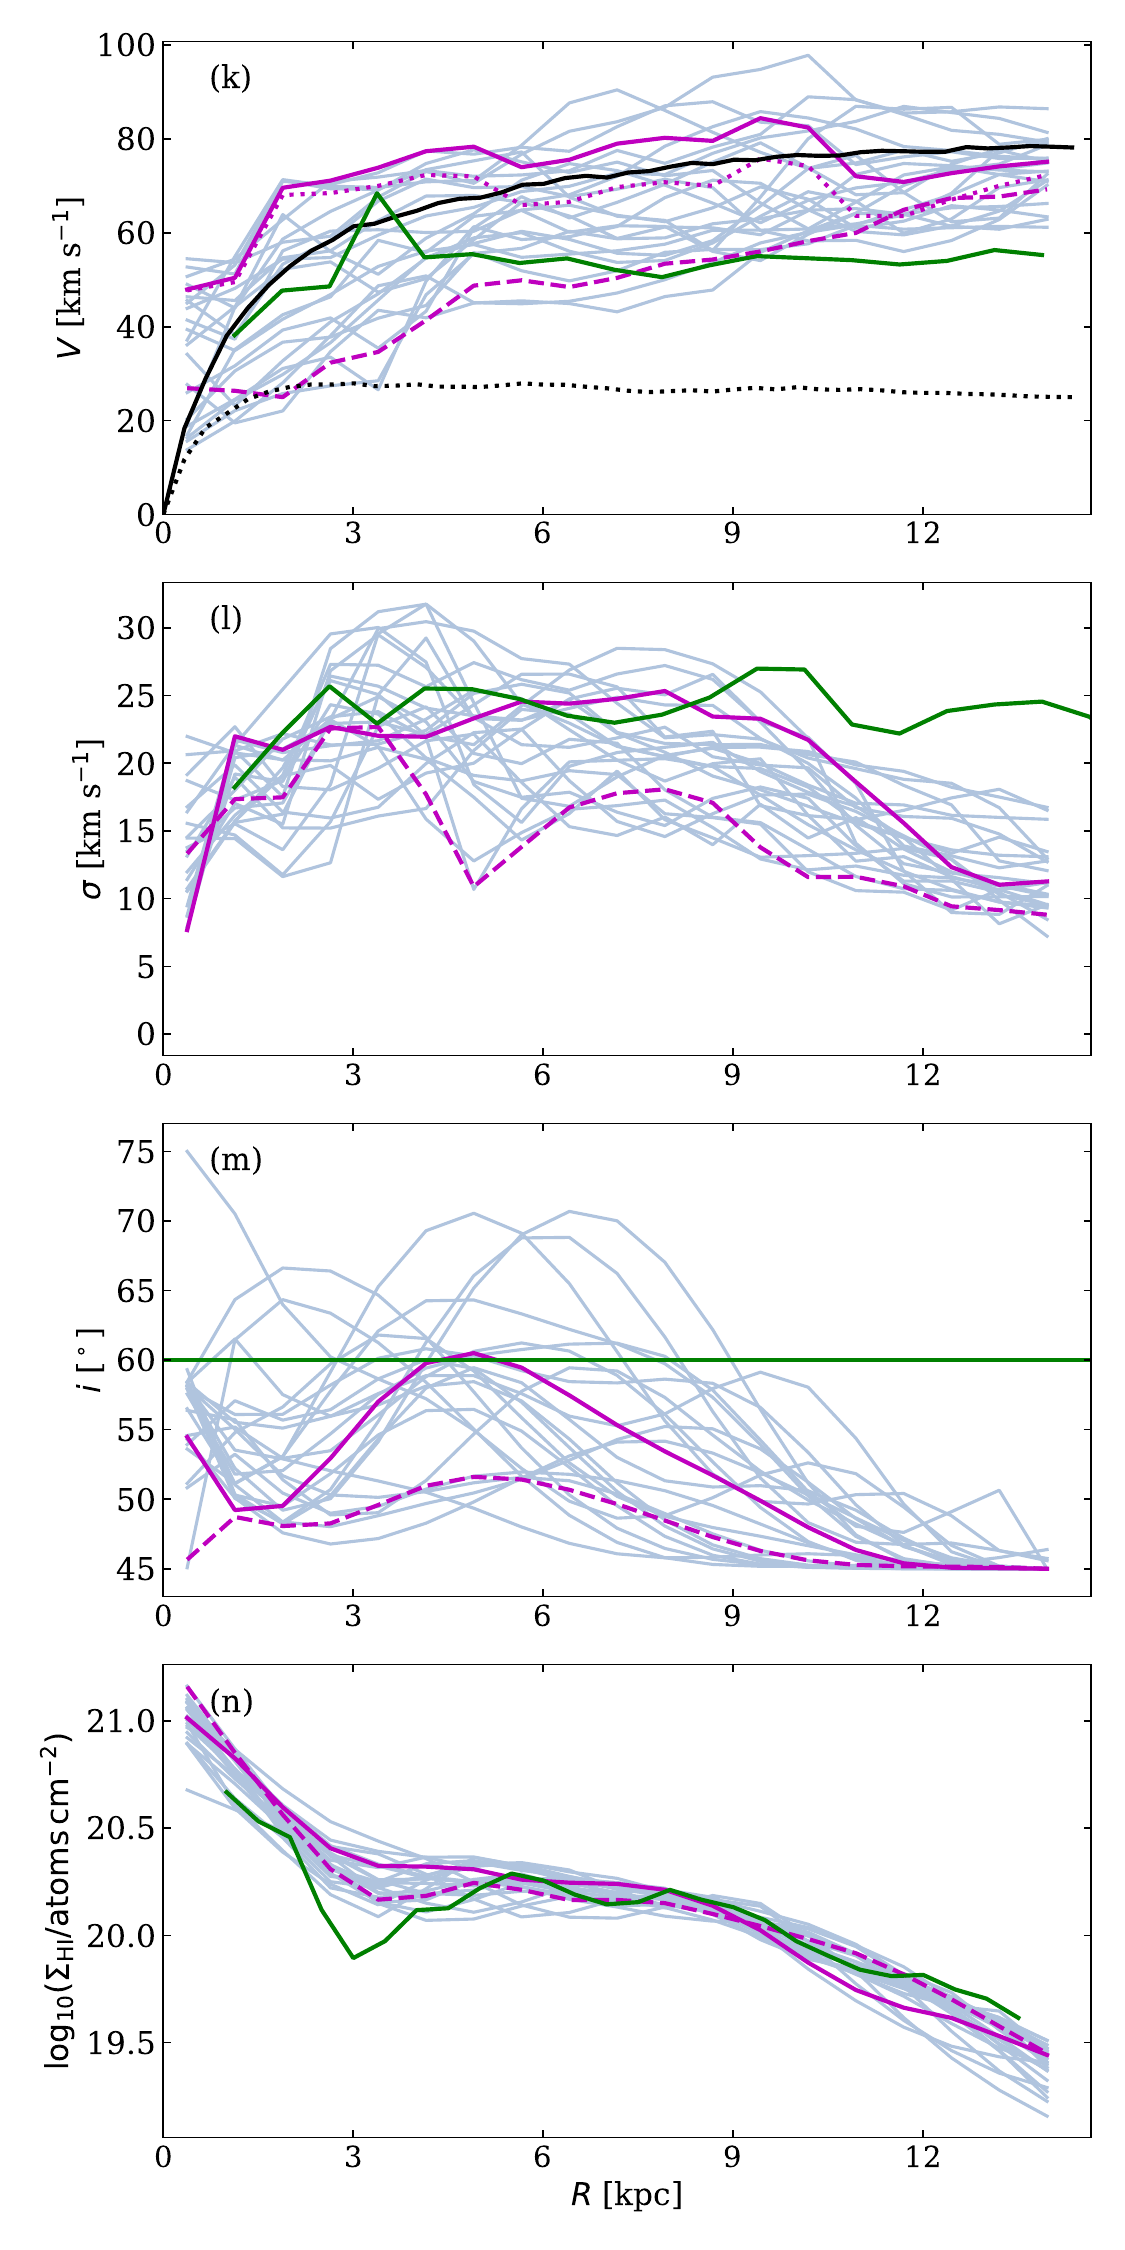}
\end{minipage}
\caption{A set of summary figures for galaxy LT-32, excluded from kinematic analysis. These include example moment maps for two orientations (panels (a)--(f); similar to Fig.~\ref{fig:visualisations}), a summary of the parameters $V_\mathrm{fid}$, $V_\mathrm{max}$, $\eta_\mathrm{rot}$, and $\eta_\mathrm{bar}$ (panels (g)--(j); similar to Fig.~\ref{fig:loops}), and a summary of the rotation curve analysis from $24$ viewing angles (panels (k)--(n); similar to Fig.~\ref{fig:rot_curves}). See description of Appendix~\ref{app:supplementary} for details.}
\label{fig:S33}
\end{figure}
\clearpage

\begin{figure}
\begin{minipage}{.9\textwidth}
\includegraphics[width=\textwidth]{../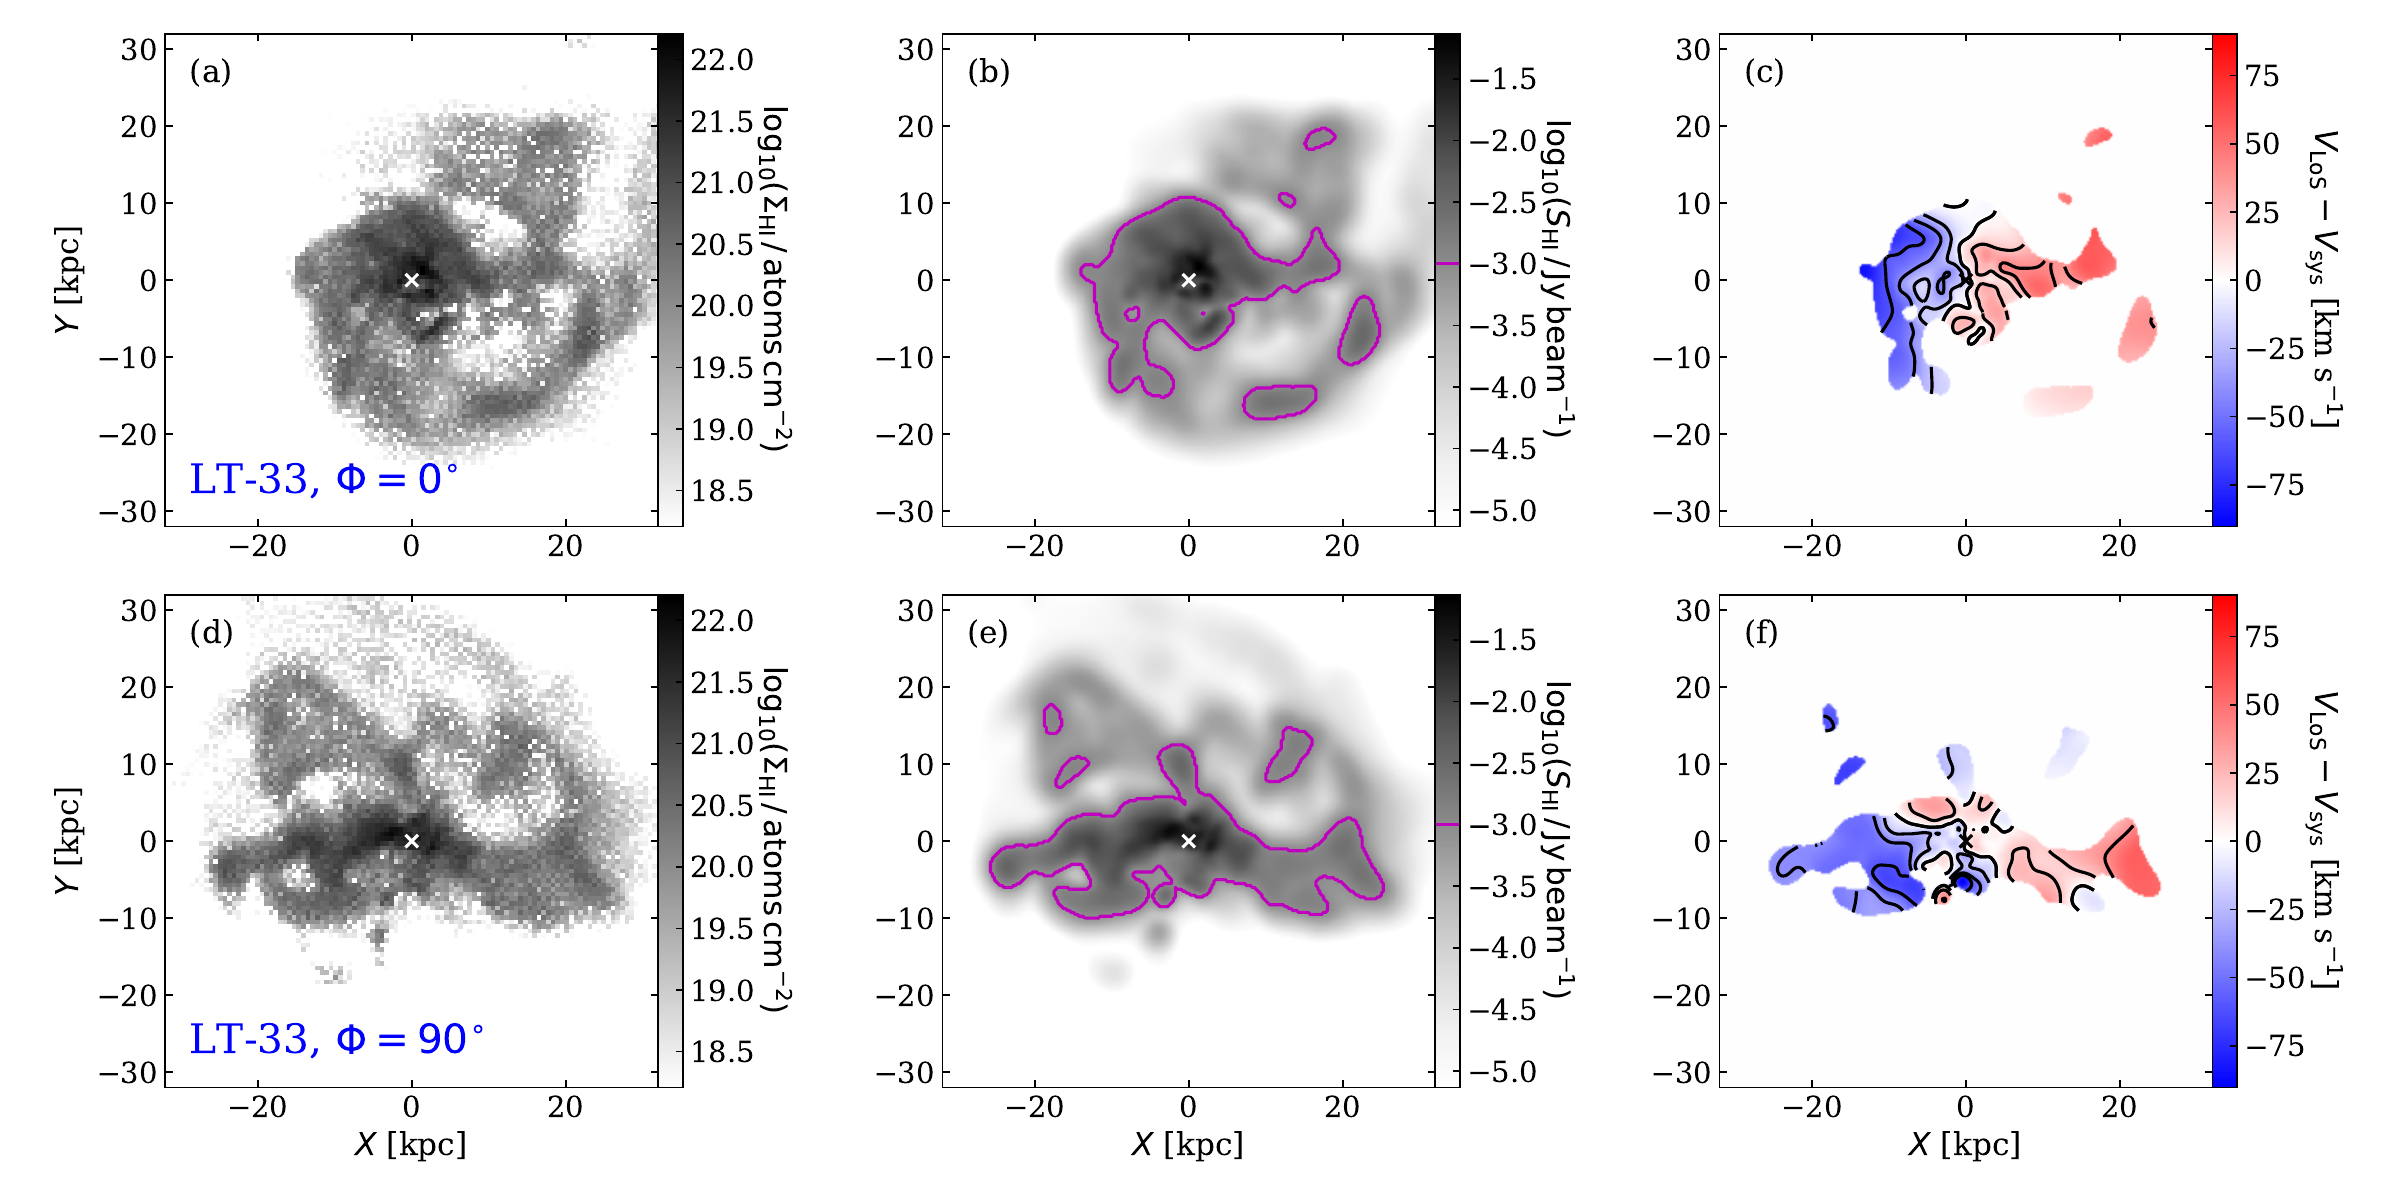}
\includegraphics[width=\textwidth]{../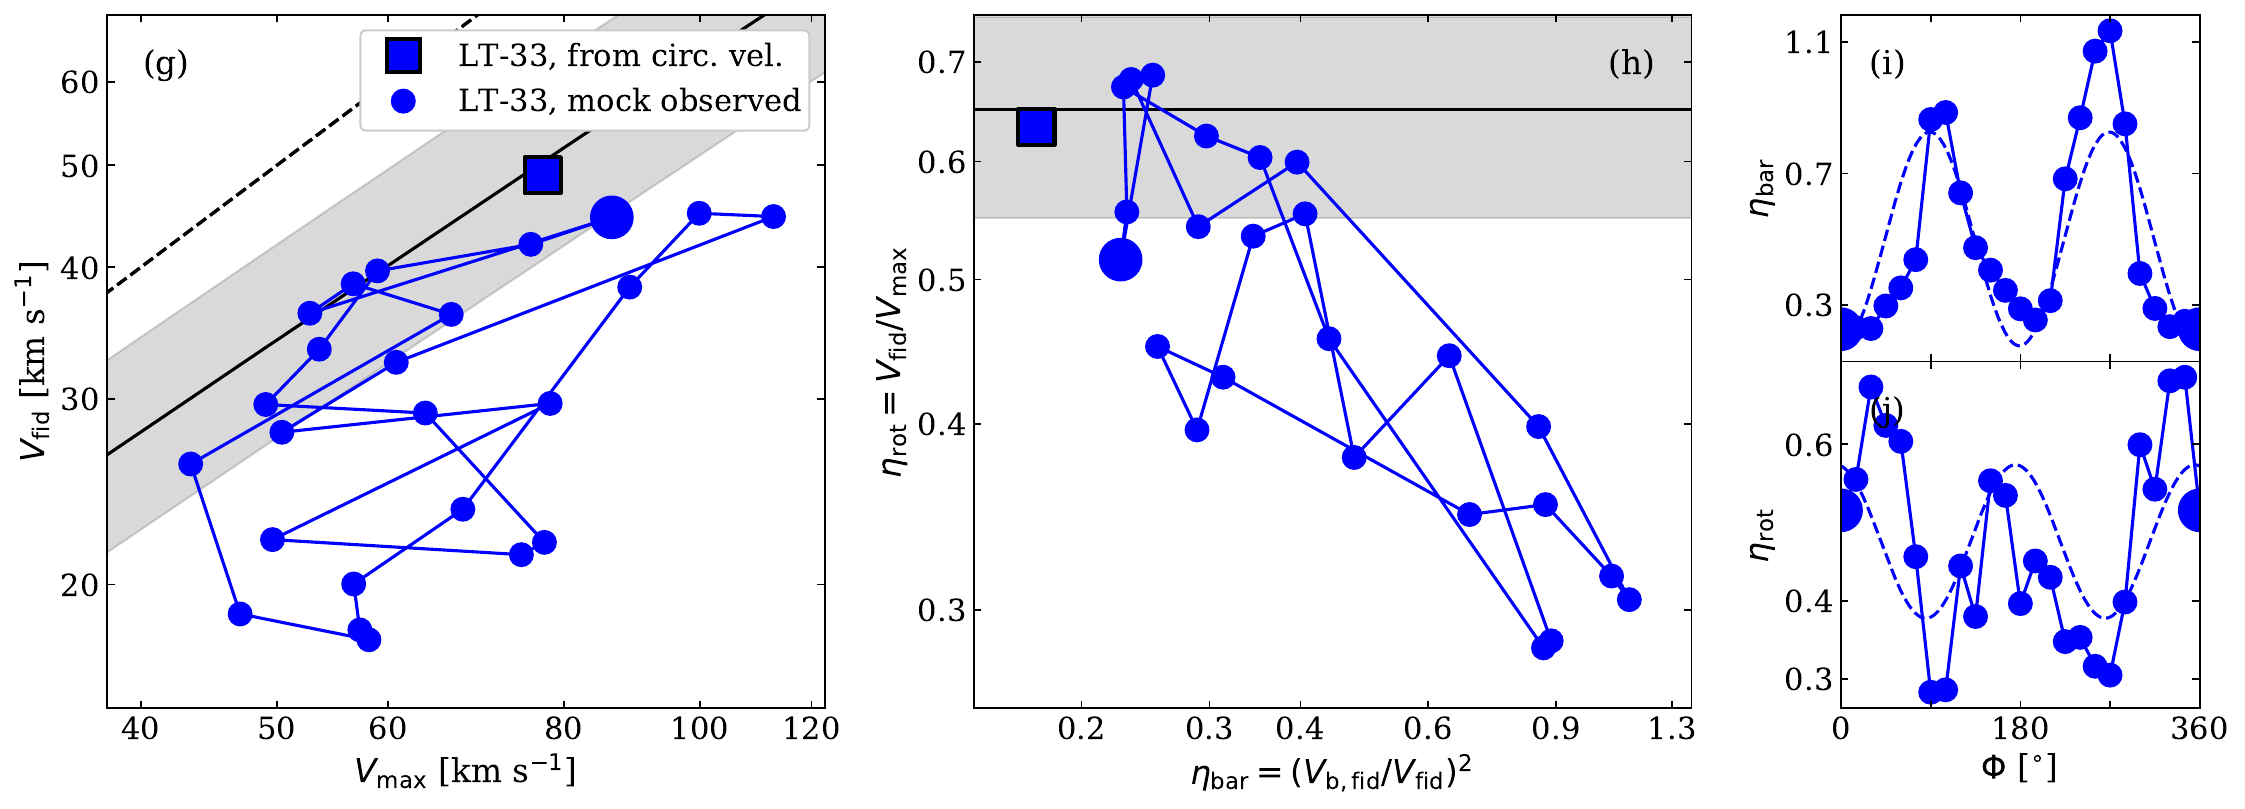}
\end{minipage}
\begin{minipage}{.4\textwidth}
\includegraphics[width=\textwidth]{../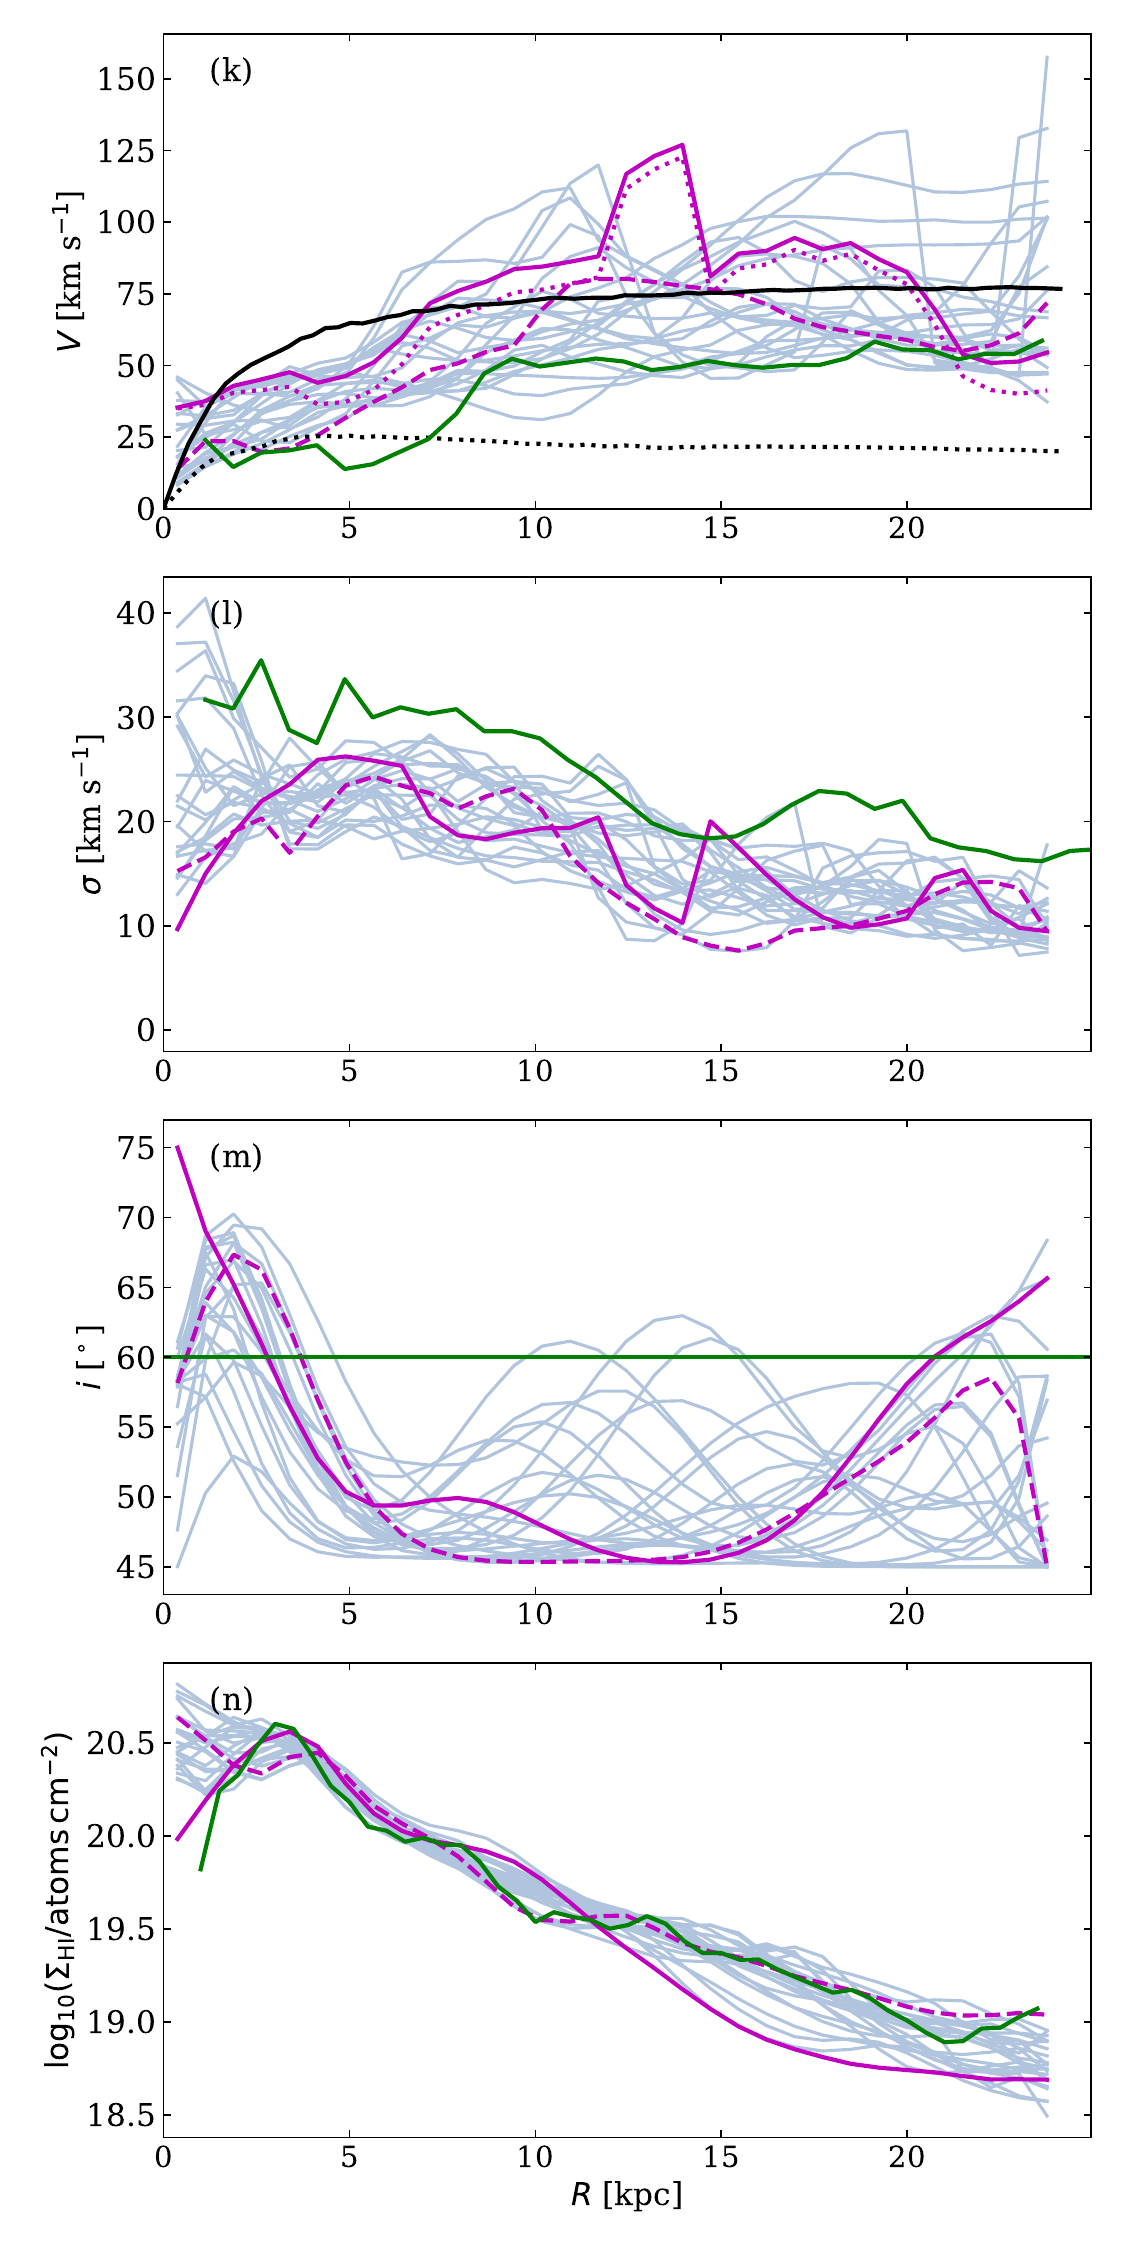}
\end{minipage}
\caption{A set of summary figures for galaxy LT-33, excluded from kinematic analysis. These include example moment maps for two orientations (panels (a)--(f); similar to Fig.~\ref{fig:visualisations}), a summary of the parameters $V_\mathrm{fid}$, $V_\mathrm{max}$, $\eta_\mathrm{rot}$, and $\eta_\mathrm{bar}$ (panels (g)--(j); similar to Fig.~\ref{fig:loops}), and a summary of the rotation curve analysis from $24$ viewing angles (panels (k)--(n); similar to Fig.~\ref{fig:rot_curves}). See description of Appendix~\ref{app:supplementary} for details.}
\label{fig:S34}
\end{figure}
\clearpage

\begin{figure}
\begin{minipage}{.9\textwidth}
\includegraphics[width=\textwidth]{../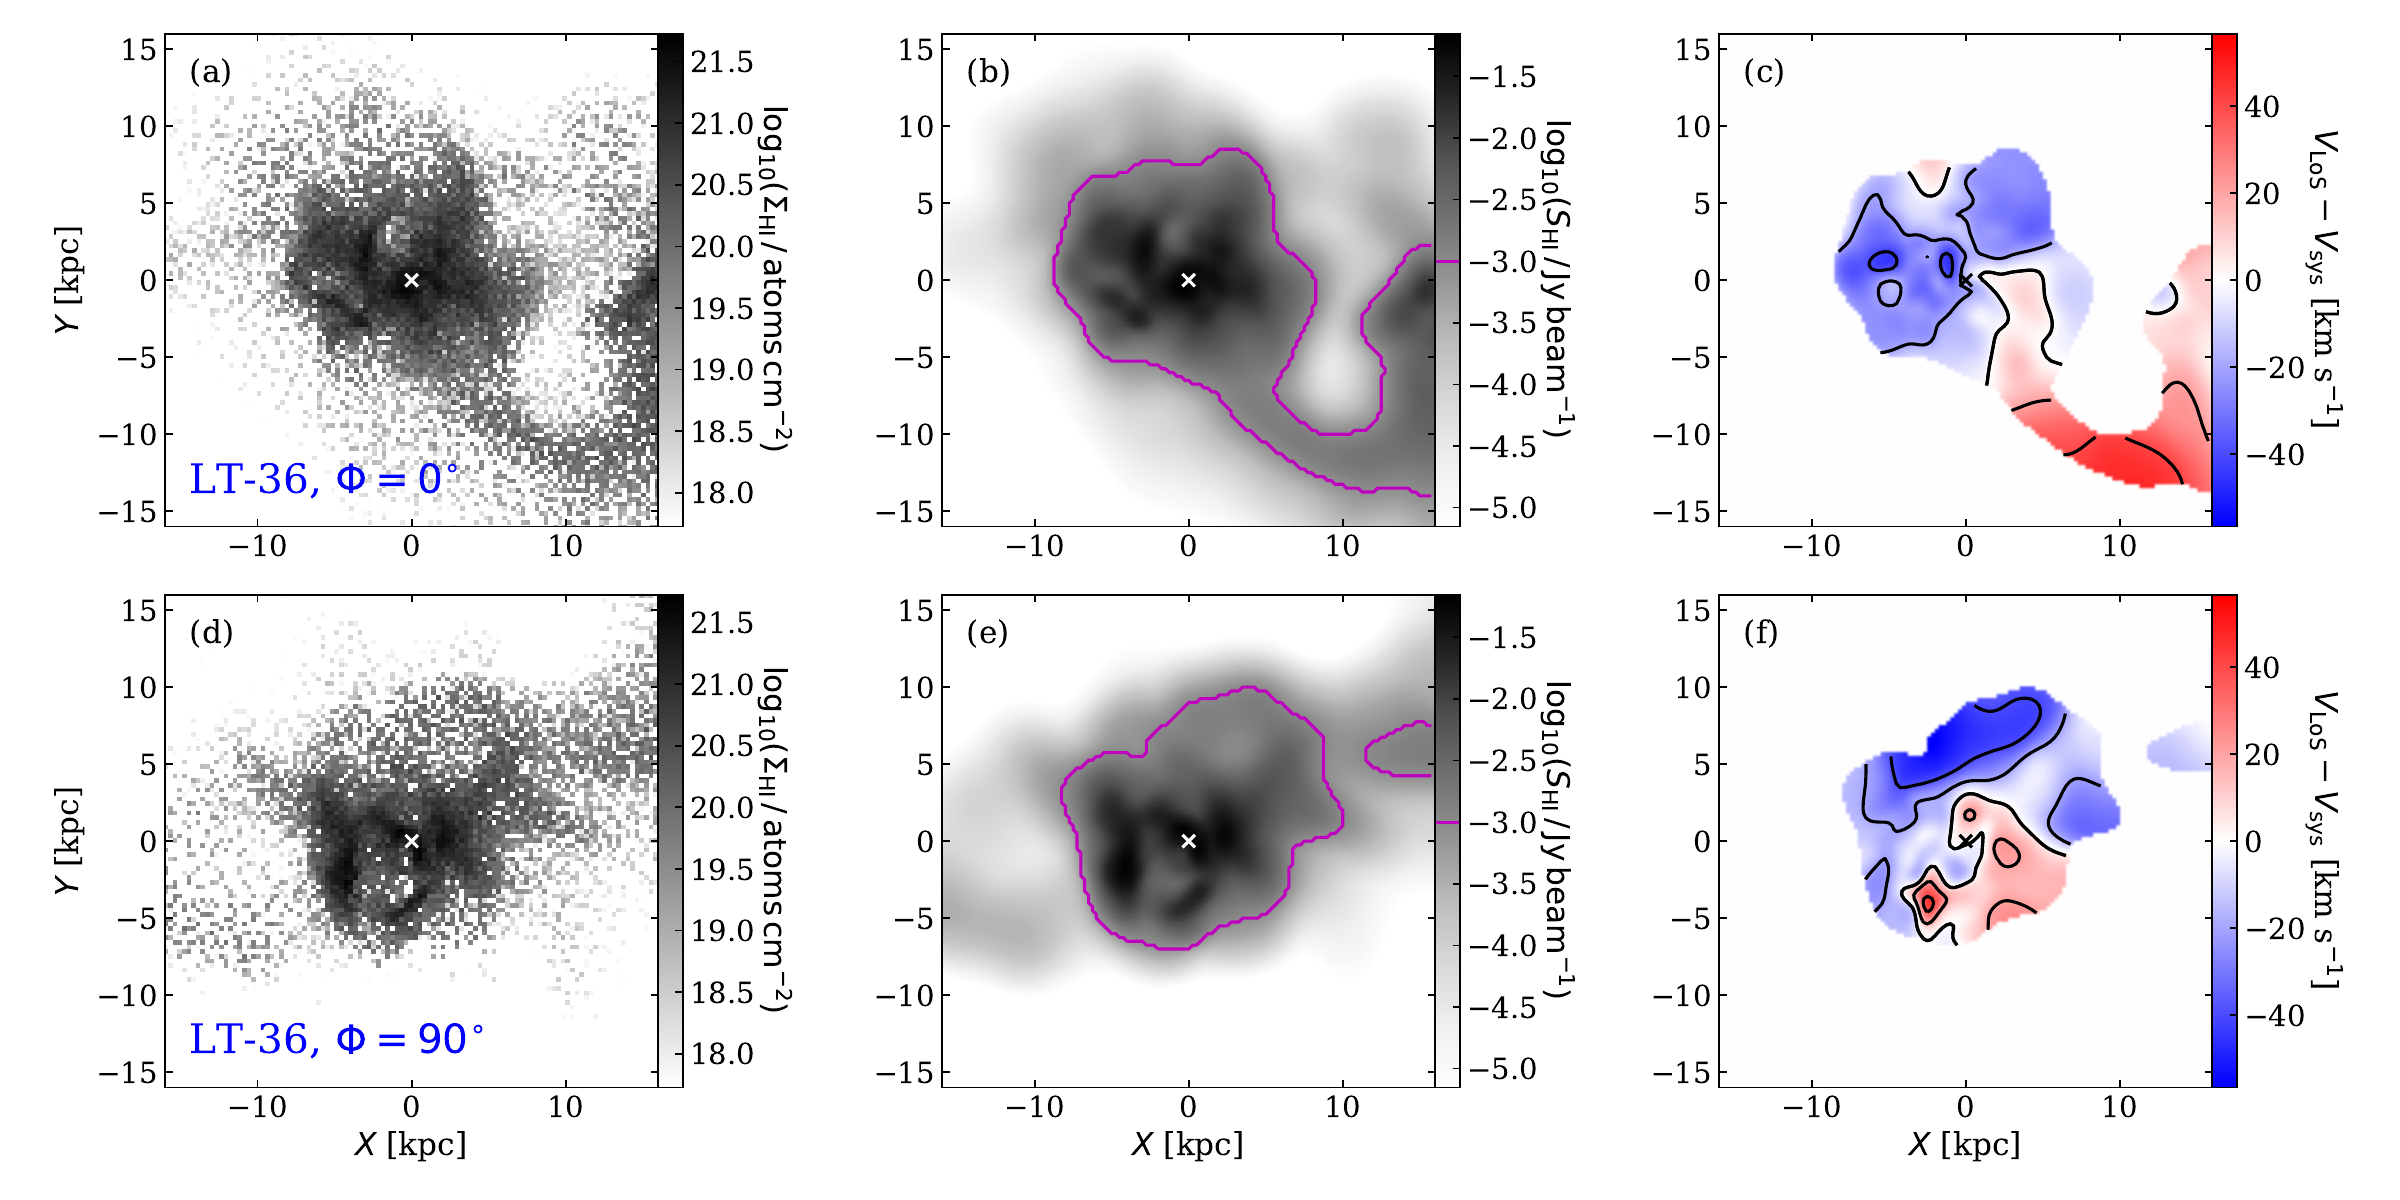}
\includegraphics[width=\textwidth]{../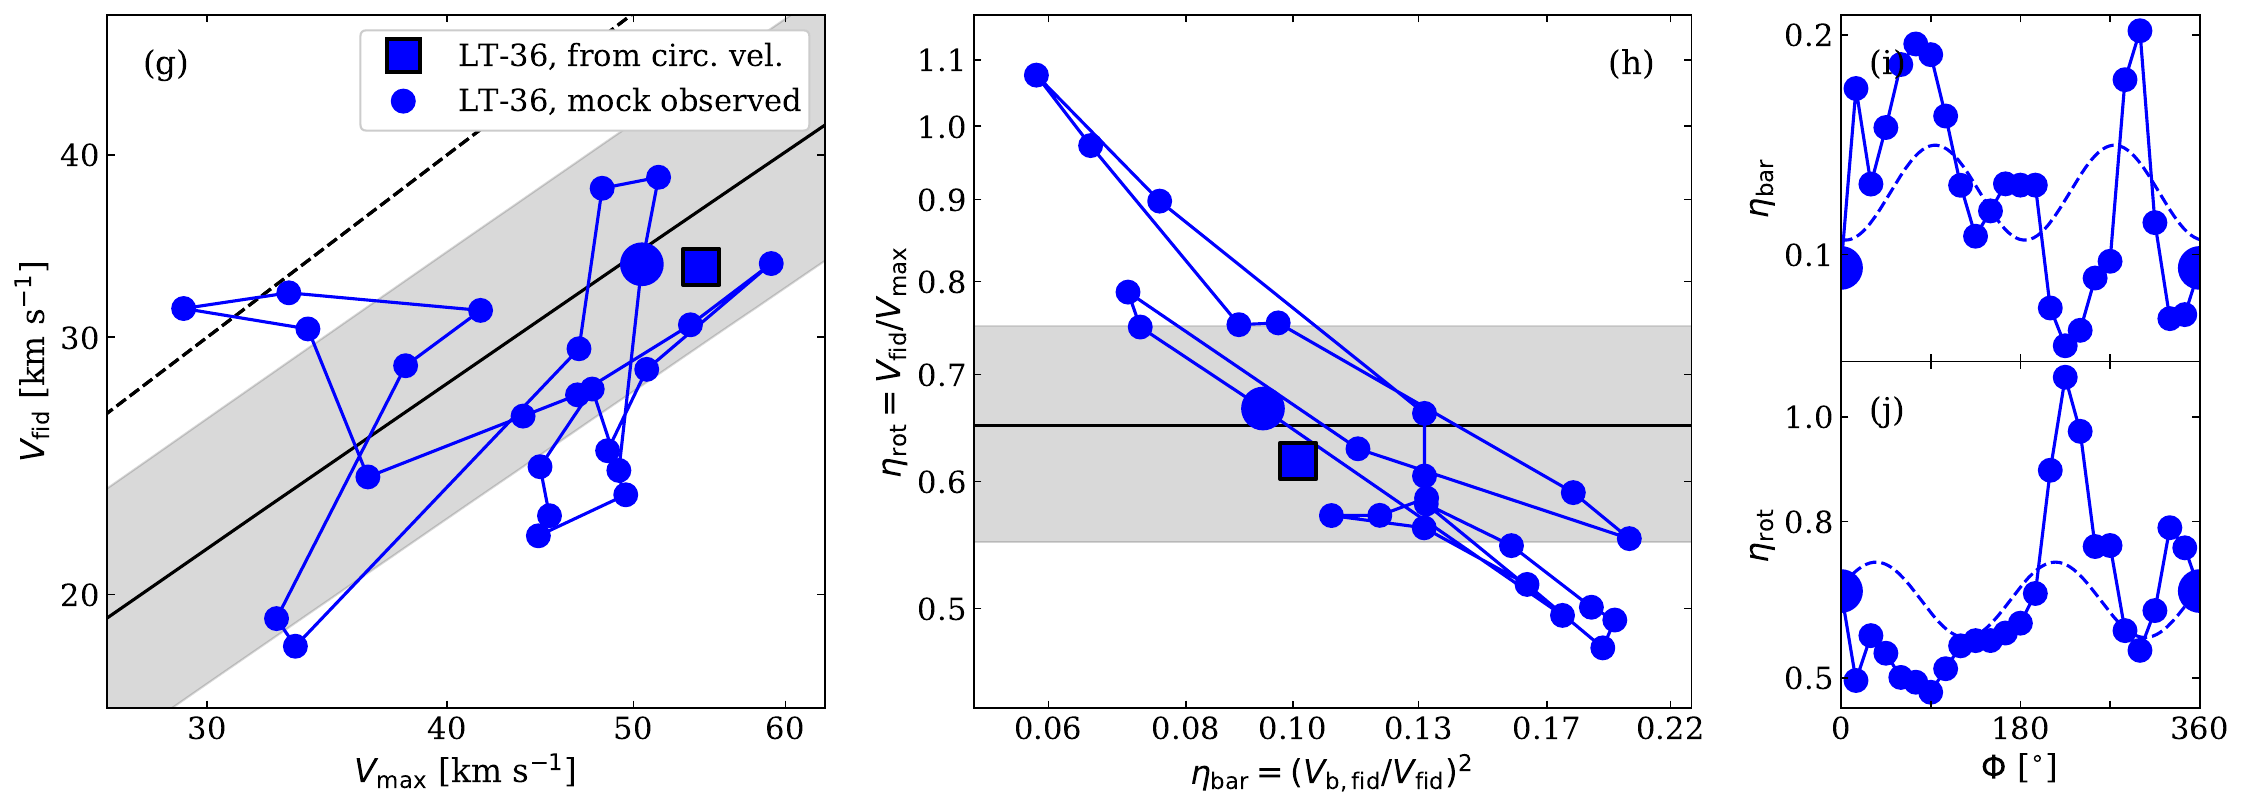}
\end{minipage}
\begin{minipage}{.4\textwidth}
\includegraphics[width=\textwidth]{../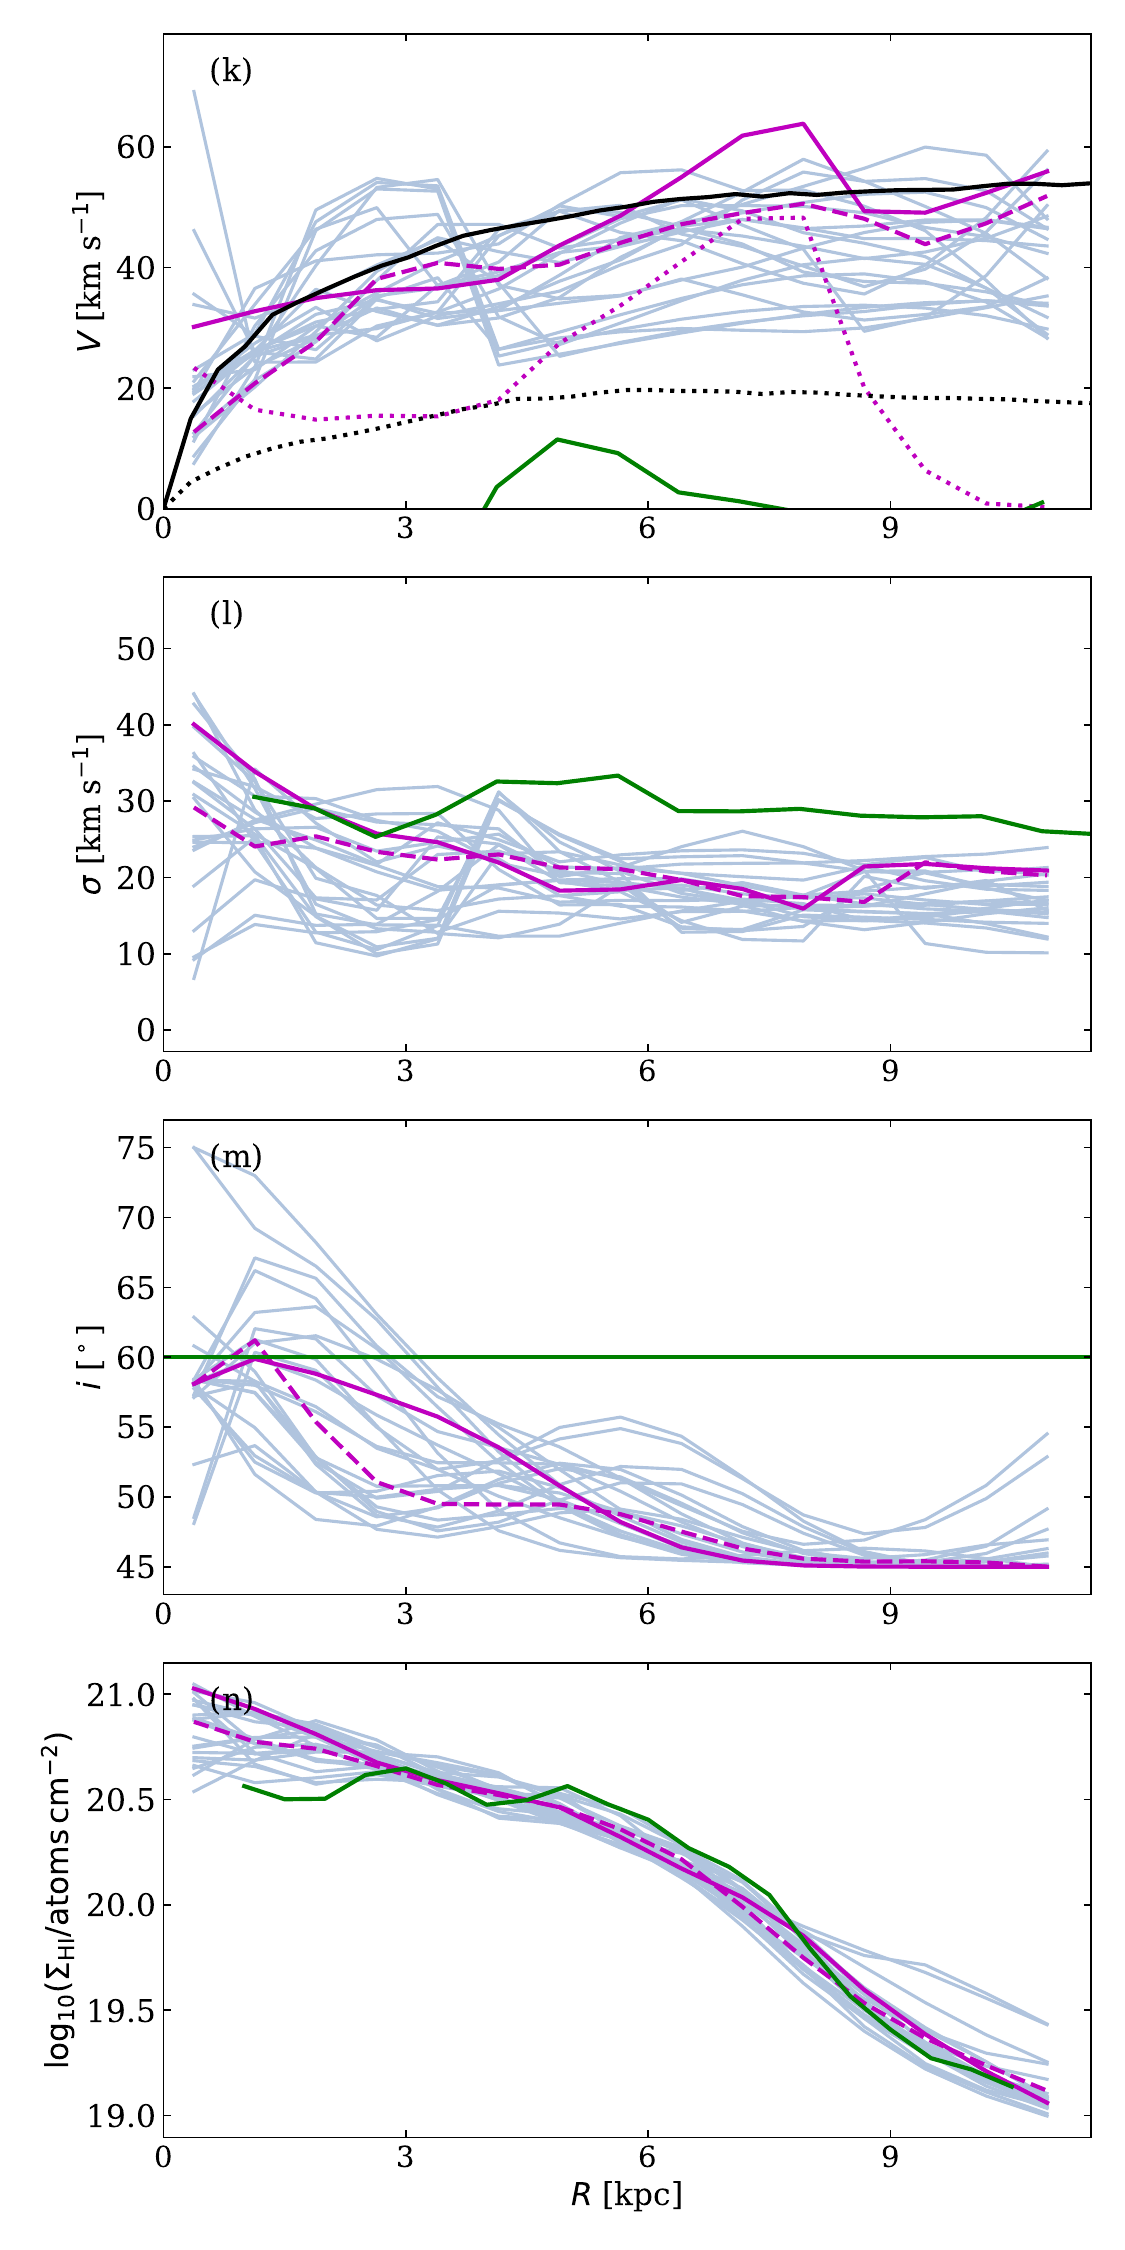}
\end{minipage}
\caption{A set of summary figures for galaxy LT-36, excluded from kinematic analysis. These include example moment maps for two orientations (panels (a)--(f); similar to Fig.~\ref{fig:visualisations}), a summary of the parameters $V_\mathrm{fid}$, $V_\mathrm{max}$, $\eta_\mathrm{rot}$, and $\eta_\mathrm{bar}$ (panels (g)--(j); similar to Fig.~\ref{fig:loops}), and a summary of the rotation curve analysis from $24$ viewing angles (panels (k)--(n); similar to Fig.~\ref{fig:rot_curves}). See description of Appendix~\ref{app:supplementary} for details.}
\label{fig:S35}
\end{figure}
\clearpage

\begin{figure}
\begin{minipage}{.9\textwidth}
\includegraphics[width=\textwidth]{../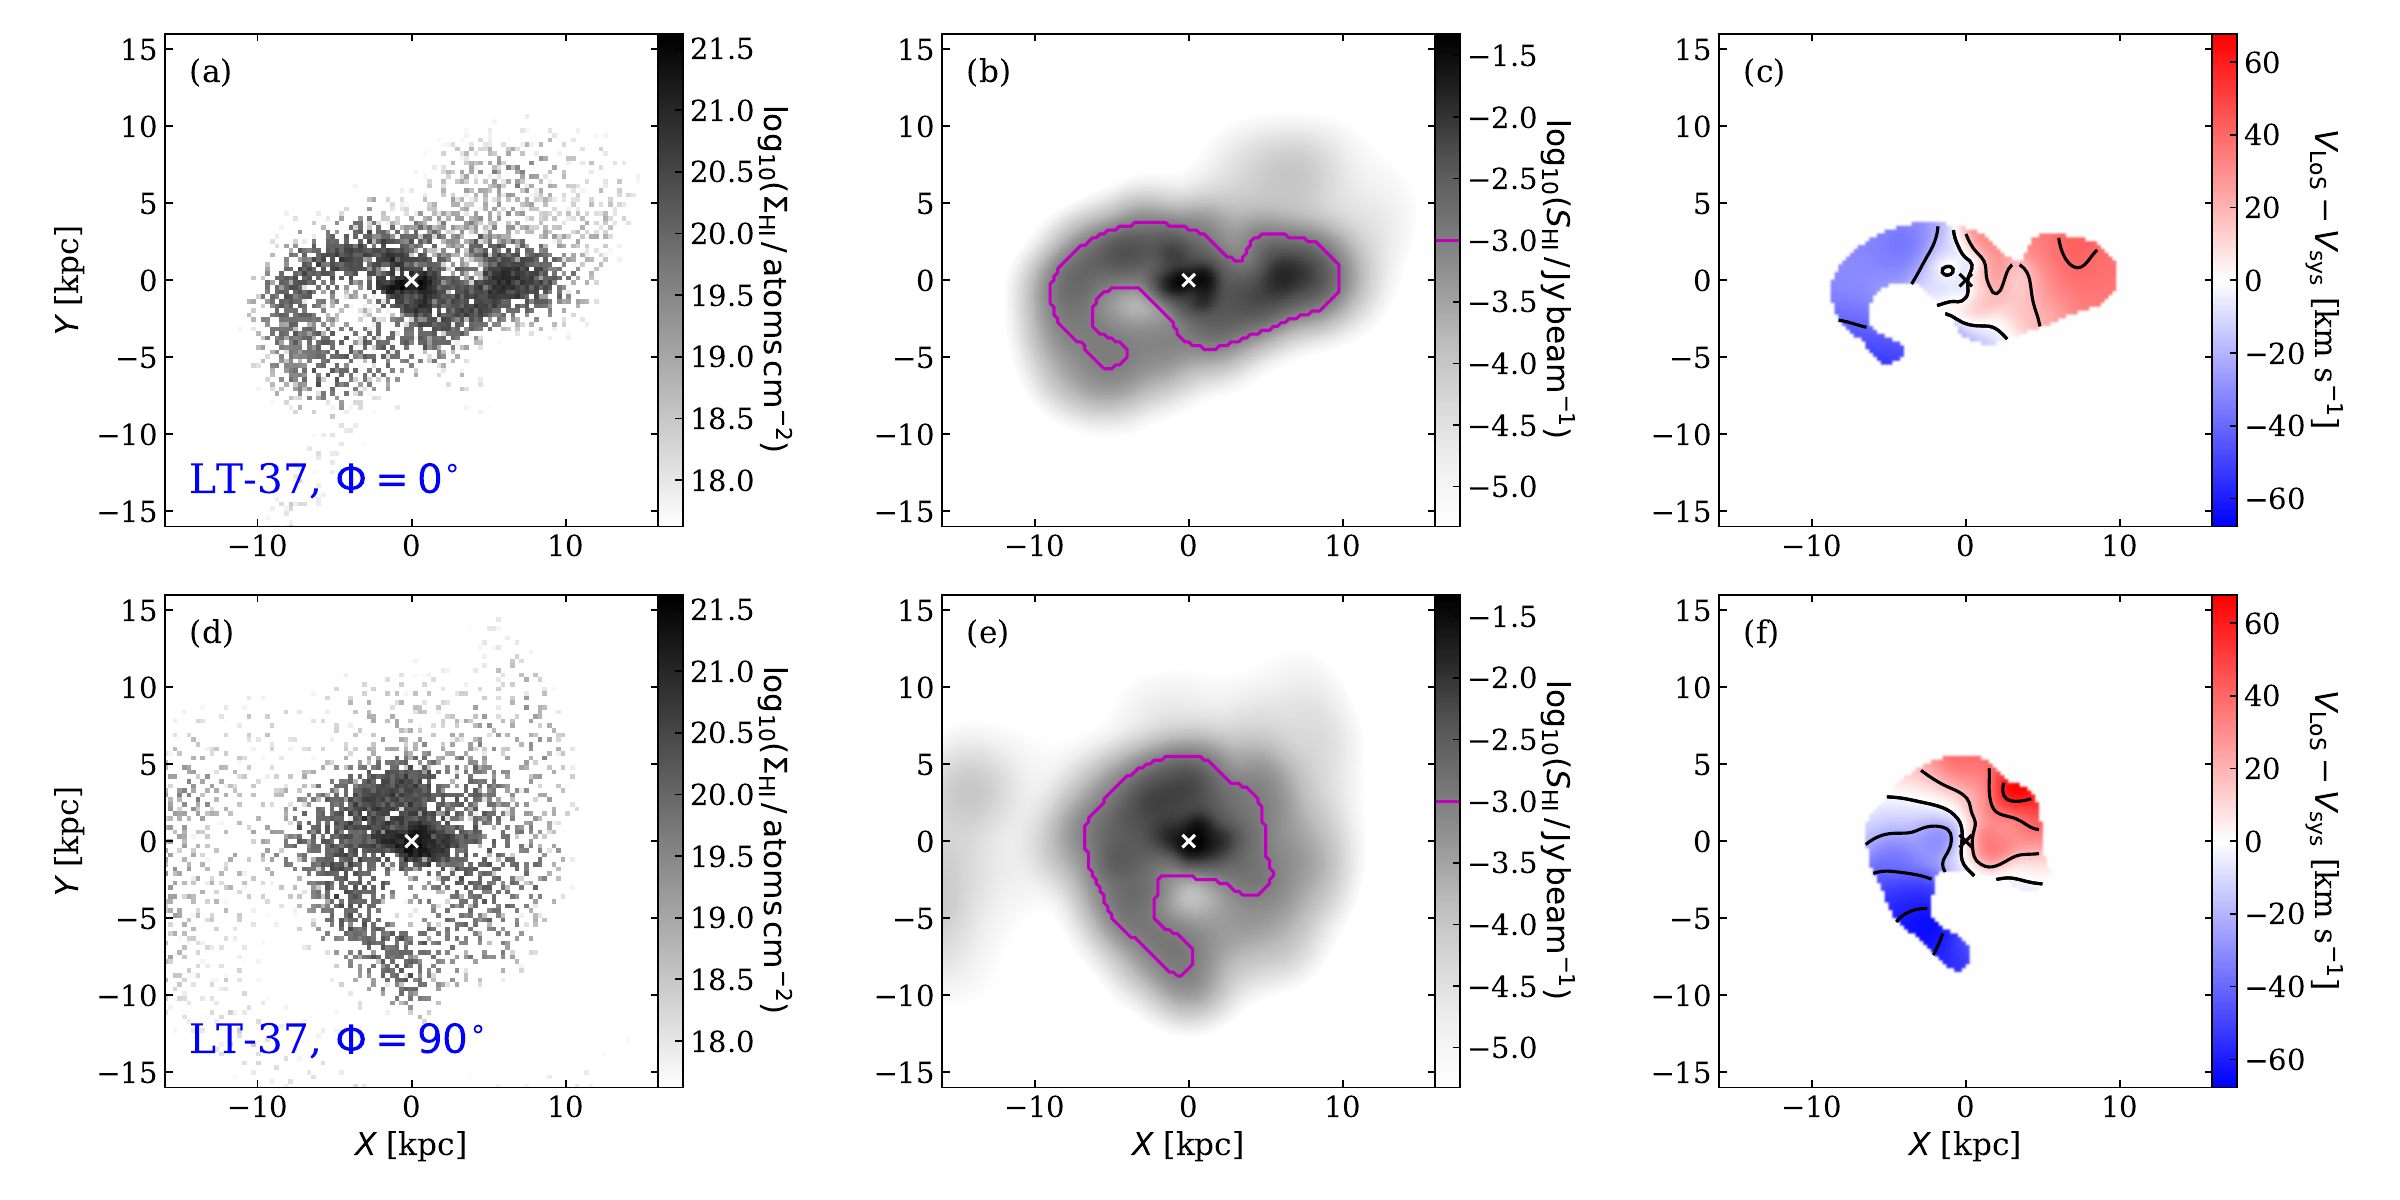}
\includegraphics[width=\textwidth]{../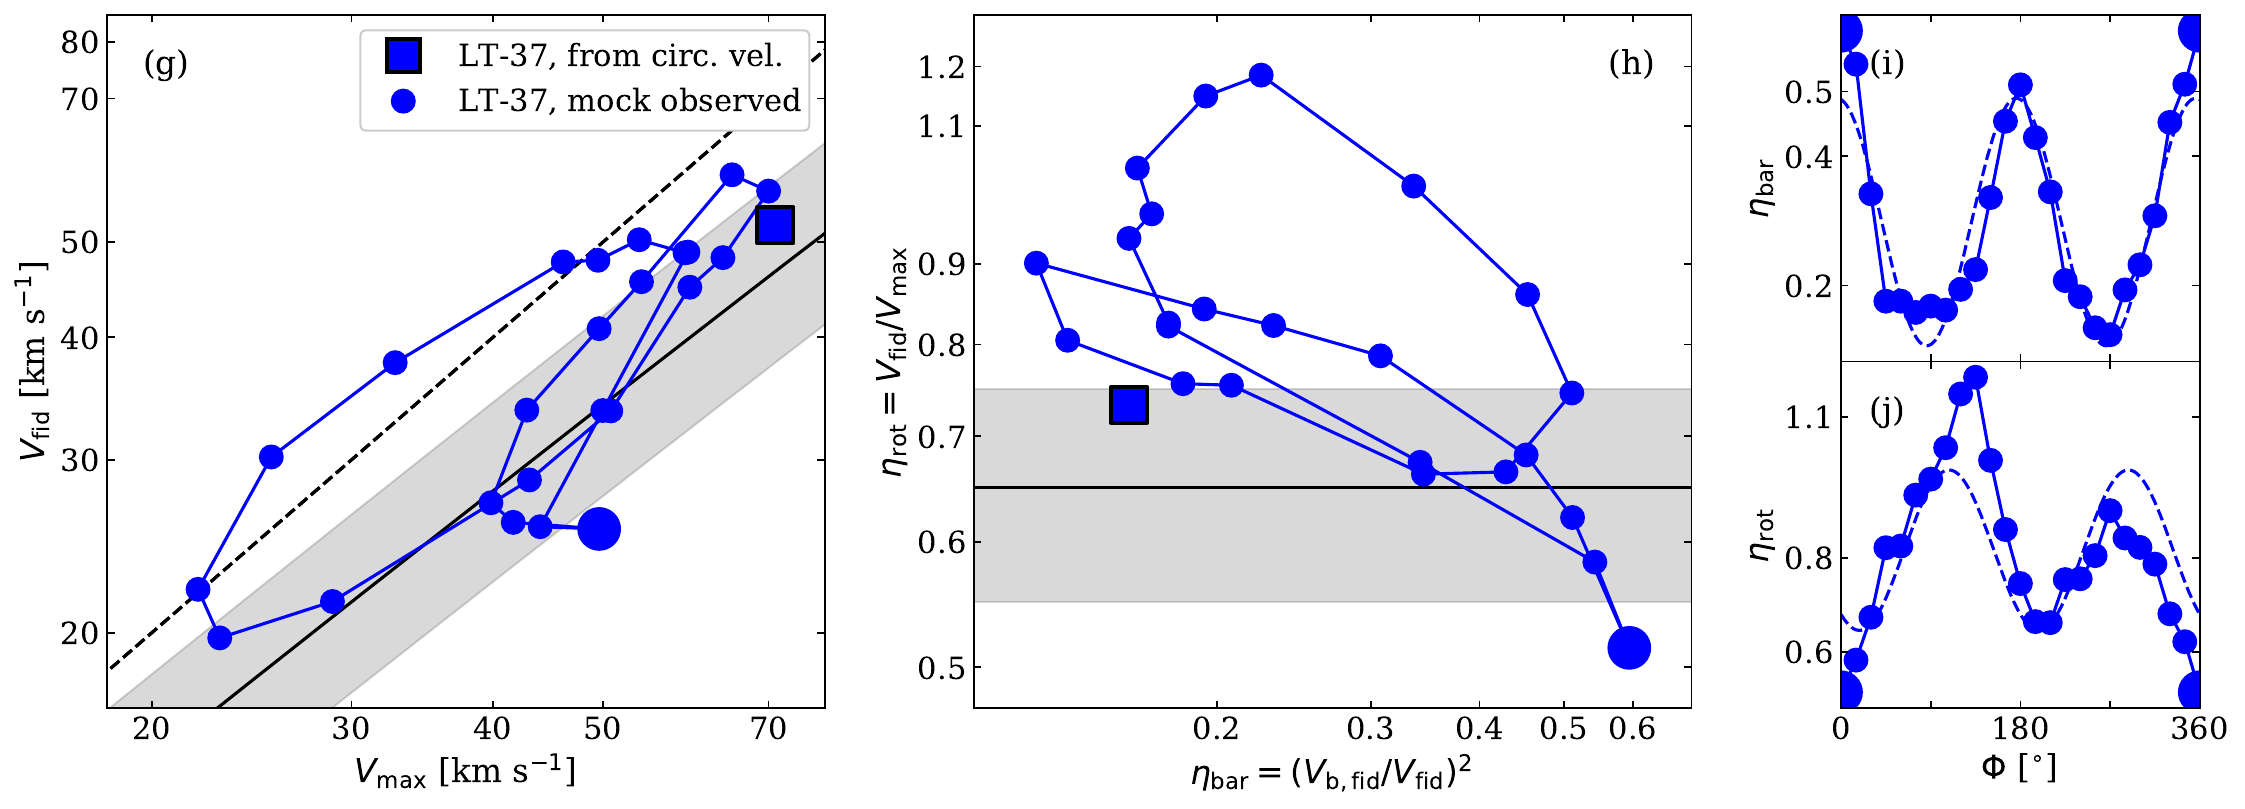}
\end{minipage}
\begin{minipage}{.4\textwidth}
\includegraphics[width=\textwidth]{../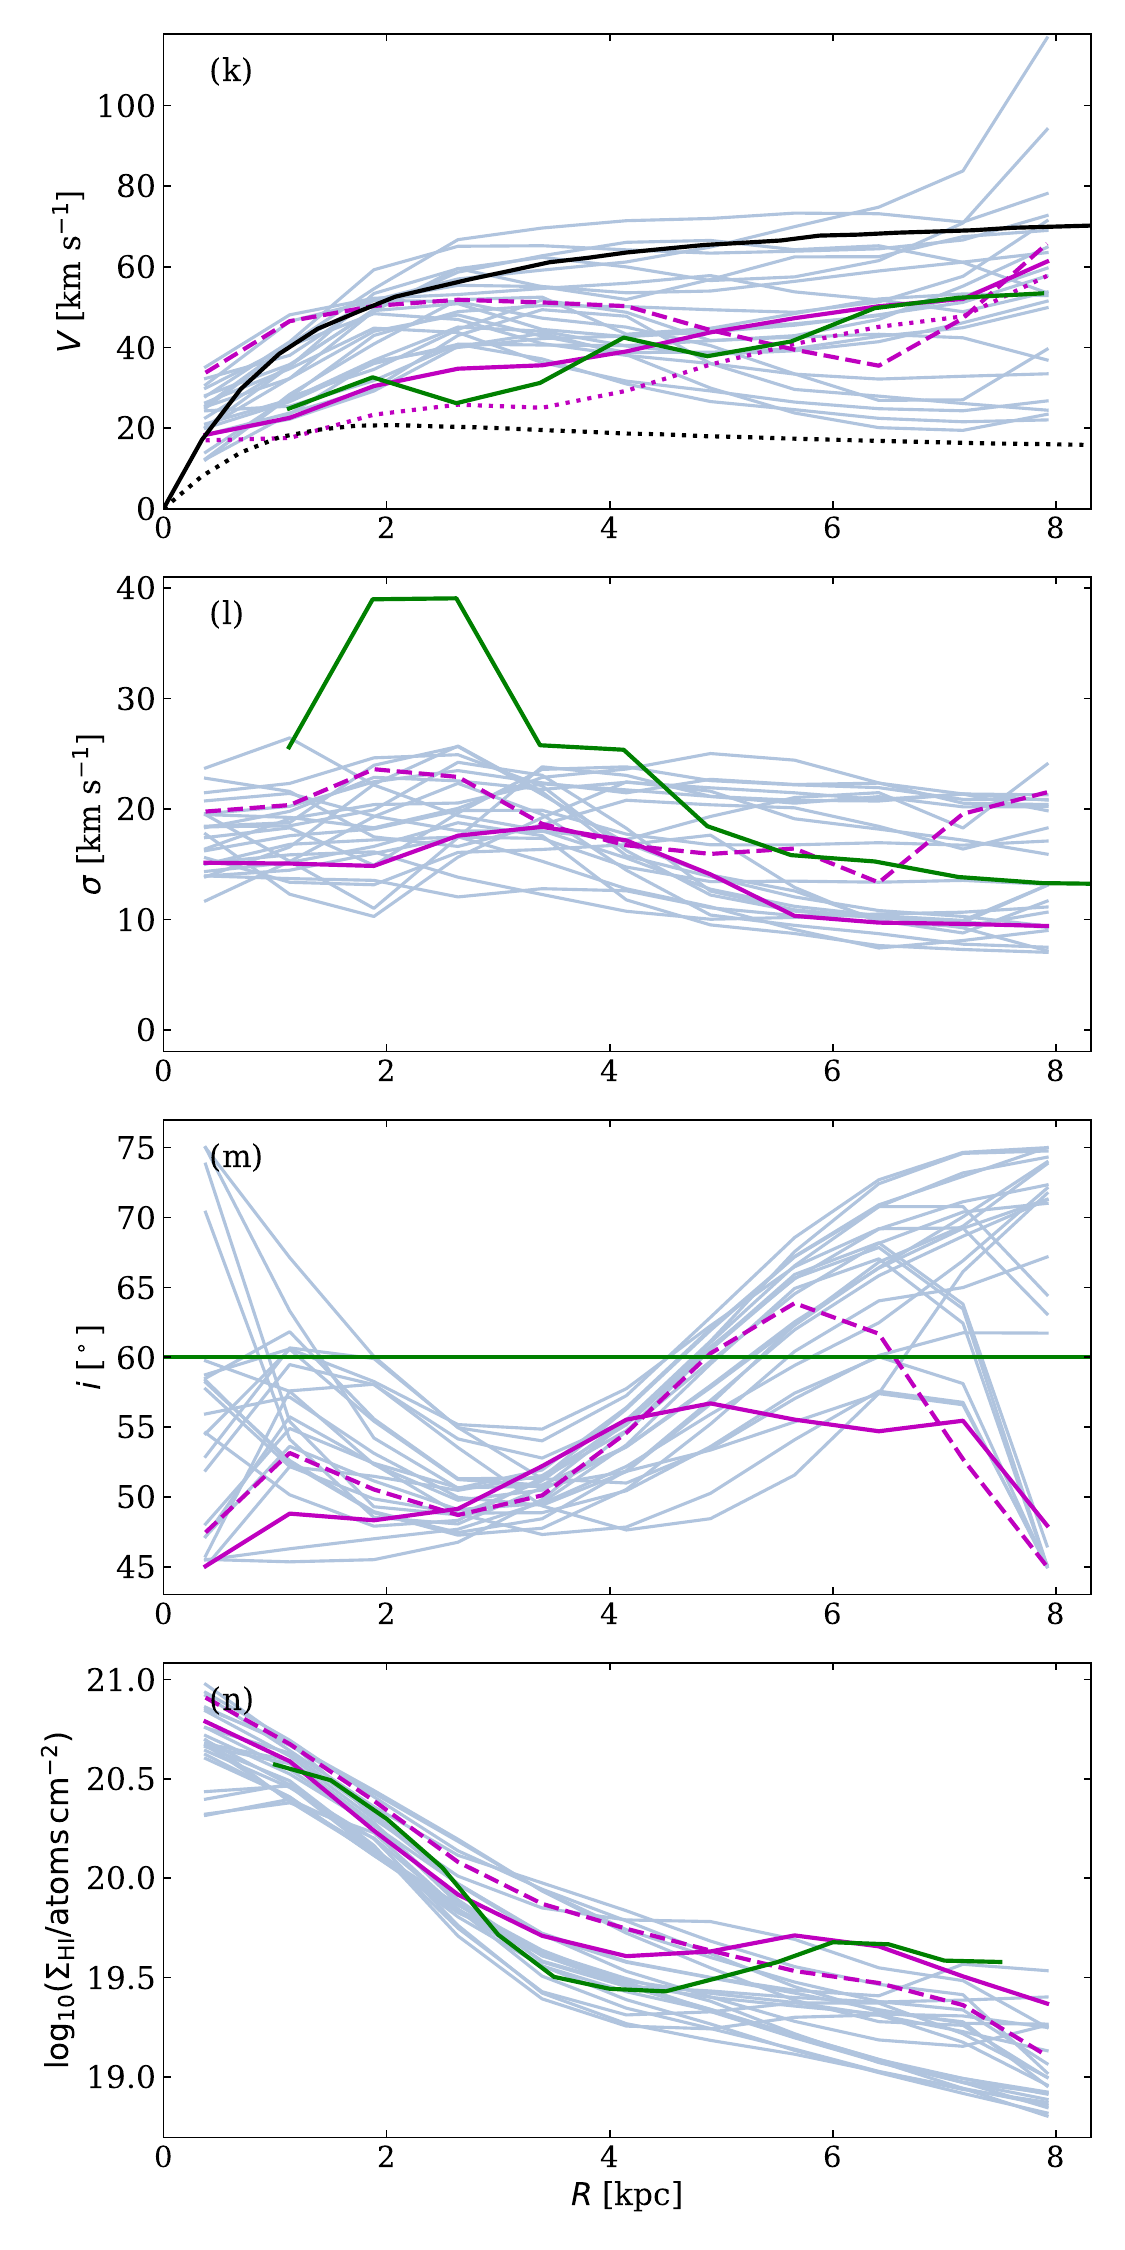}
\end{minipage}
\caption{A set of summary figures for galaxy LT-37, excluded from kinematic analysis. These include example moment maps for two orientations (panels (a)--(f); similar to Fig.~\ref{fig:visualisations}), a summary of the parameters $V_\mathrm{fid}$, $V_\mathrm{max}$, $\eta_\mathrm{rot}$, and $\eta_\mathrm{bar}$ (panels (g)--(j); similar to Fig.~\ref{fig:loops}), and a summary of the rotation curve analysis from $24$ viewing angles (panels (k)--(n); similar to Fig.~\ref{fig:rot_curves}). See description of Appendix~\ref{app:supplementary} for details.}
\label{fig:S36}
\end{figure}
\clearpage

\begin{figure}
\begin{minipage}{.9\textwidth}
\includegraphics[width=\textwidth]{../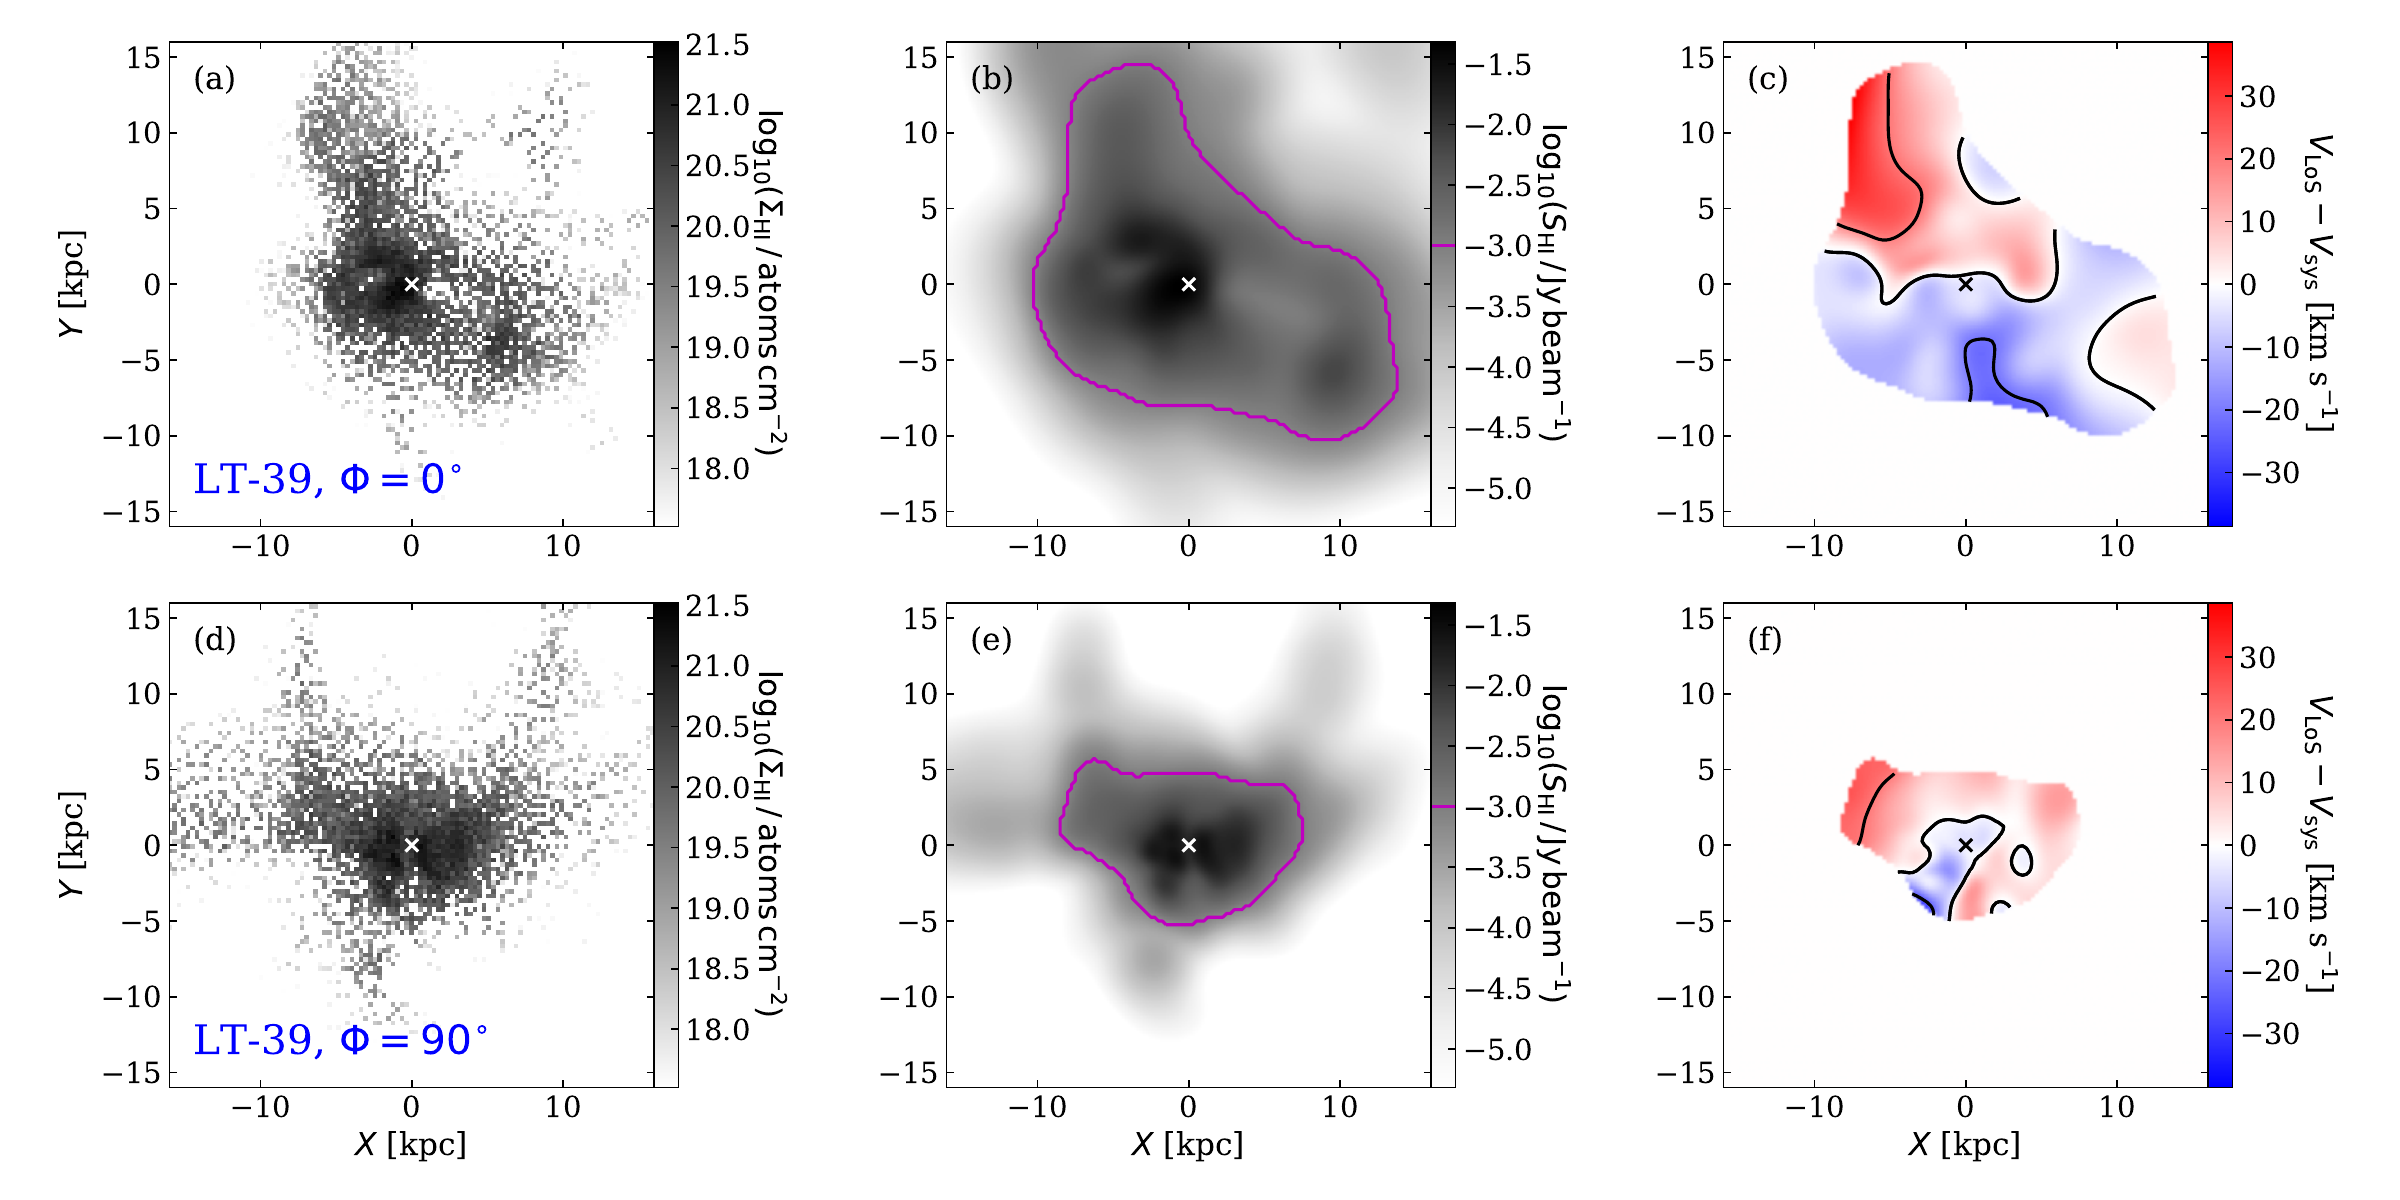}
\includegraphics[width=\textwidth]{../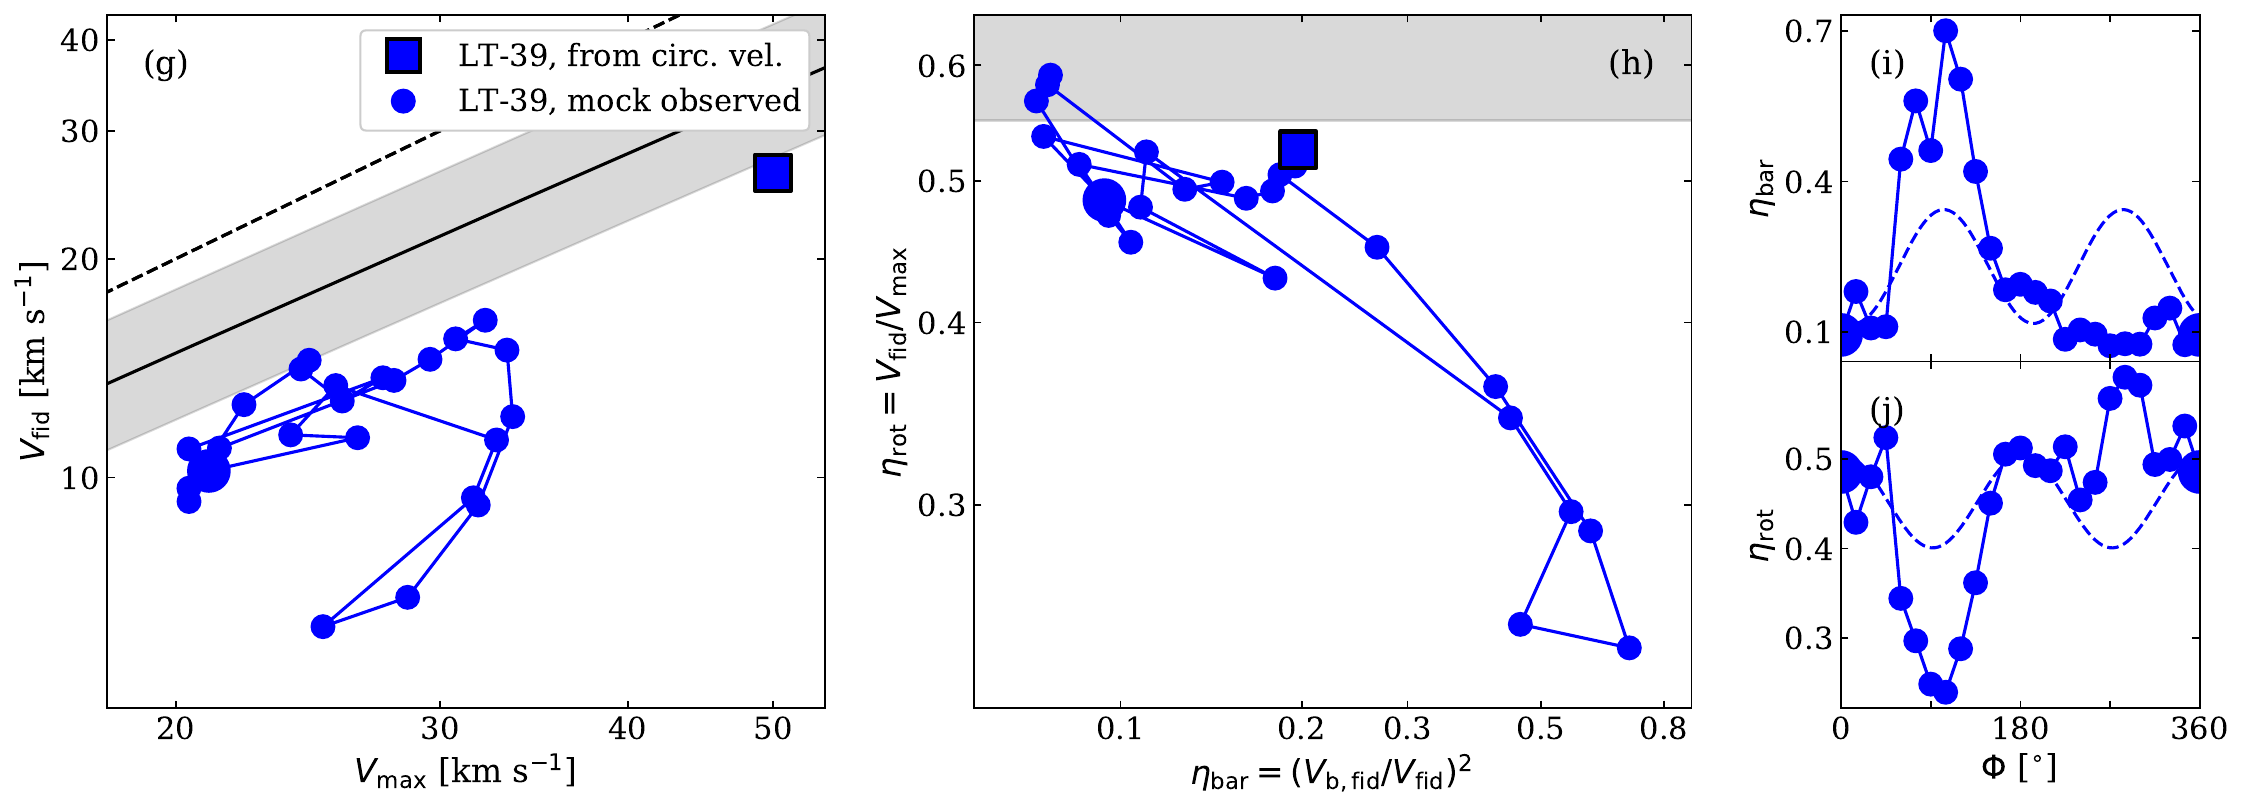}
\end{minipage}
\begin{minipage}{.4\textwidth}
\includegraphics[width=\textwidth]{../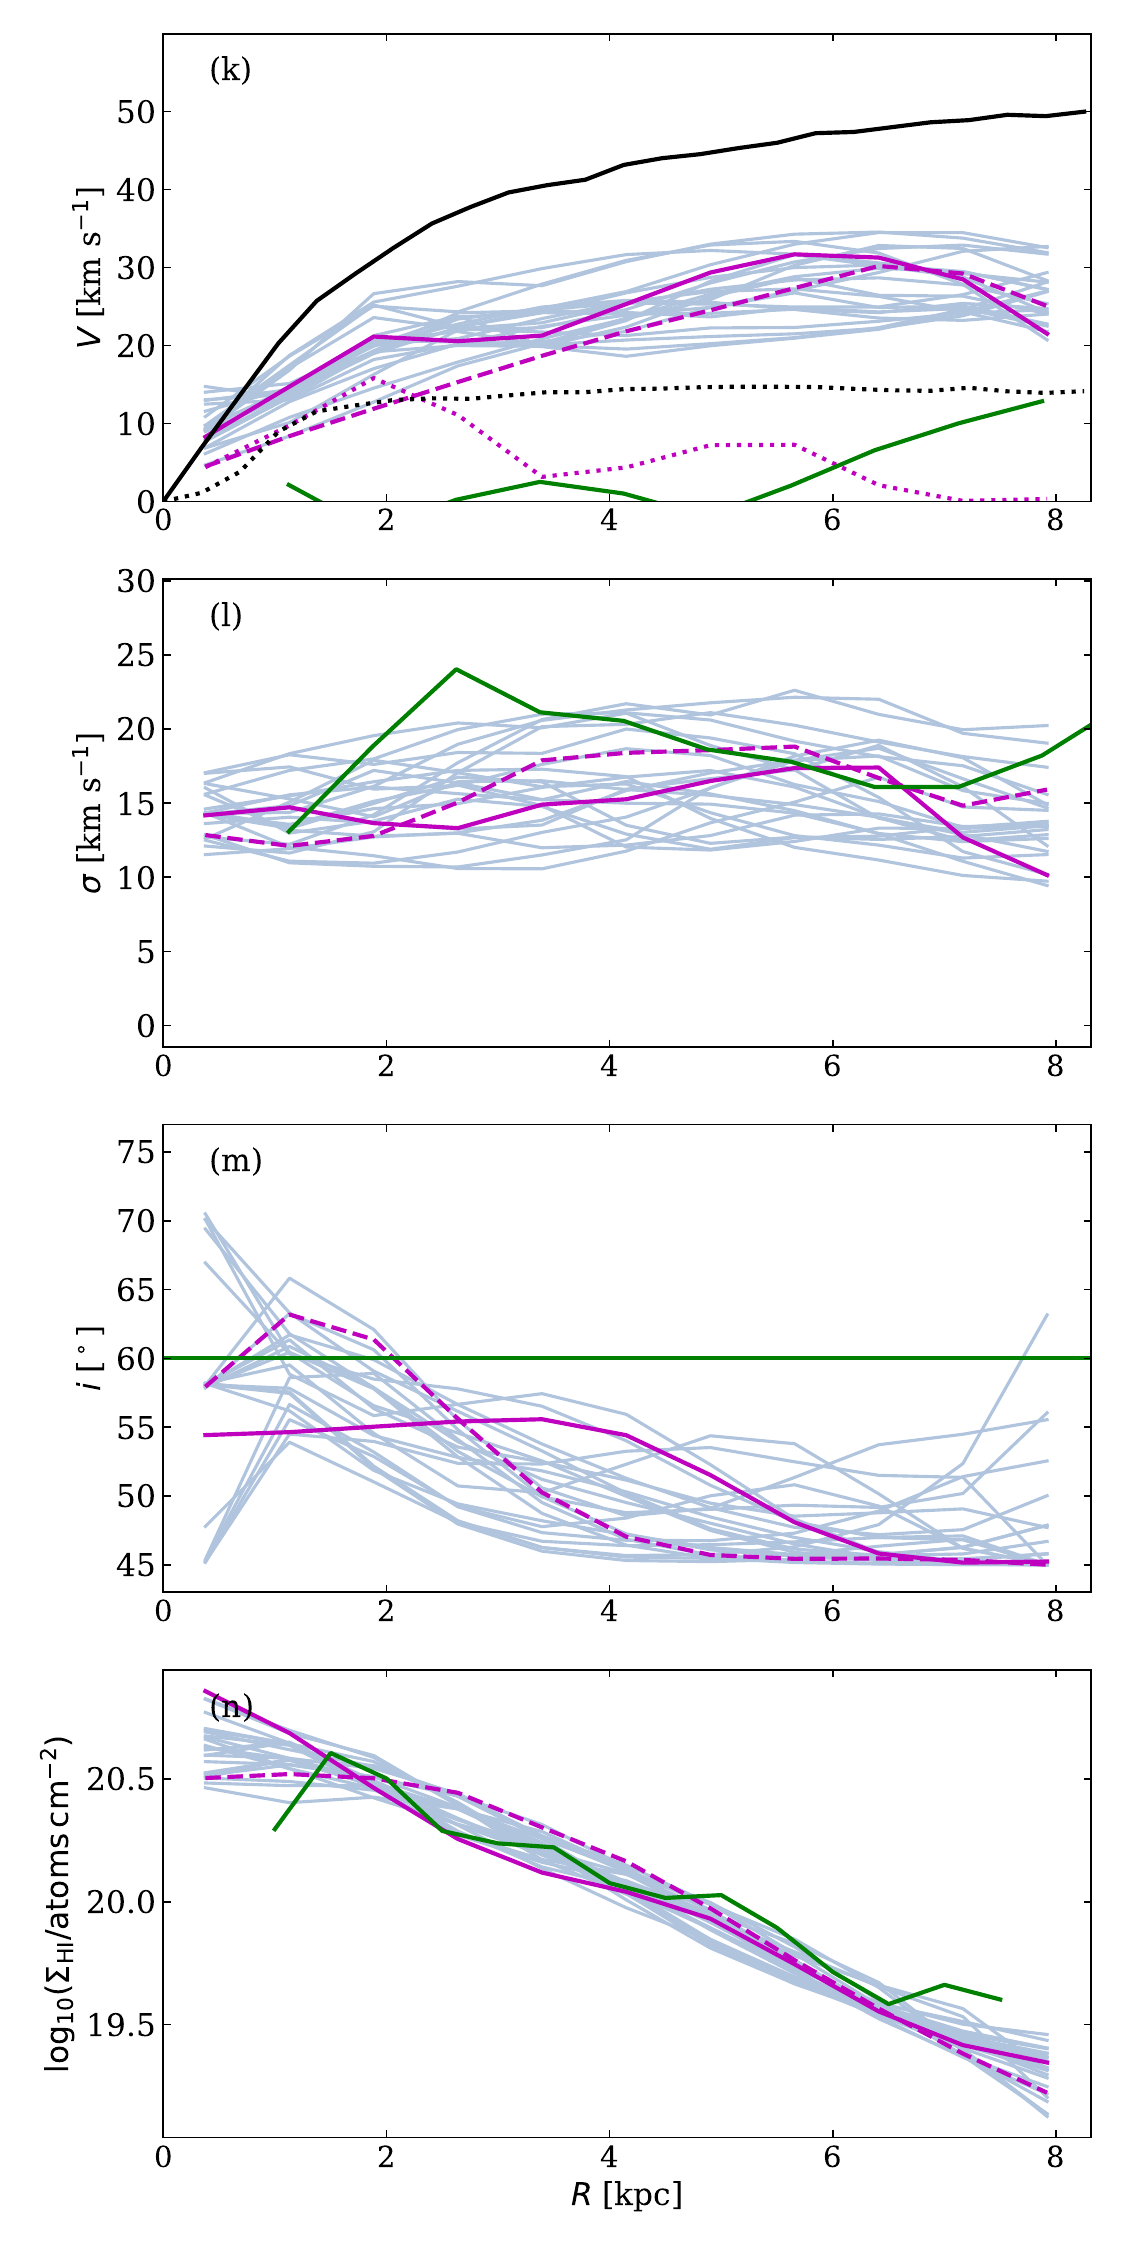}
\end{minipage}
\caption{A set of summary figures for galaxy LT-39, excluded from kinematic analysis. These include example moment maps for two orientations (panels (a)--(f); similar to Fig.~\ref{fig:visualisations}), a summary of the parameters $V_\mathrm{fid}$, $V_\mathrm{max}$, $\eta_\mathrm{rot}$, and $\eta_\mathrm{bar}$ (panels (g)--(j); similar to Fig.~\ref{fig:loops}), and a summary of the rotation curve analysis from $24$ viewing angles (panels (k)--(n); similar to Fig.~\ref{fig:rot_curves}). See description of Appendix~\ref{app:supplementary} for details.}
\label{fig:S37}
\end{figure}
\clearpage

\begin{figure}
\begin{minipage}{.9\textwidth}
\includegraphics[width=\textwidth]{../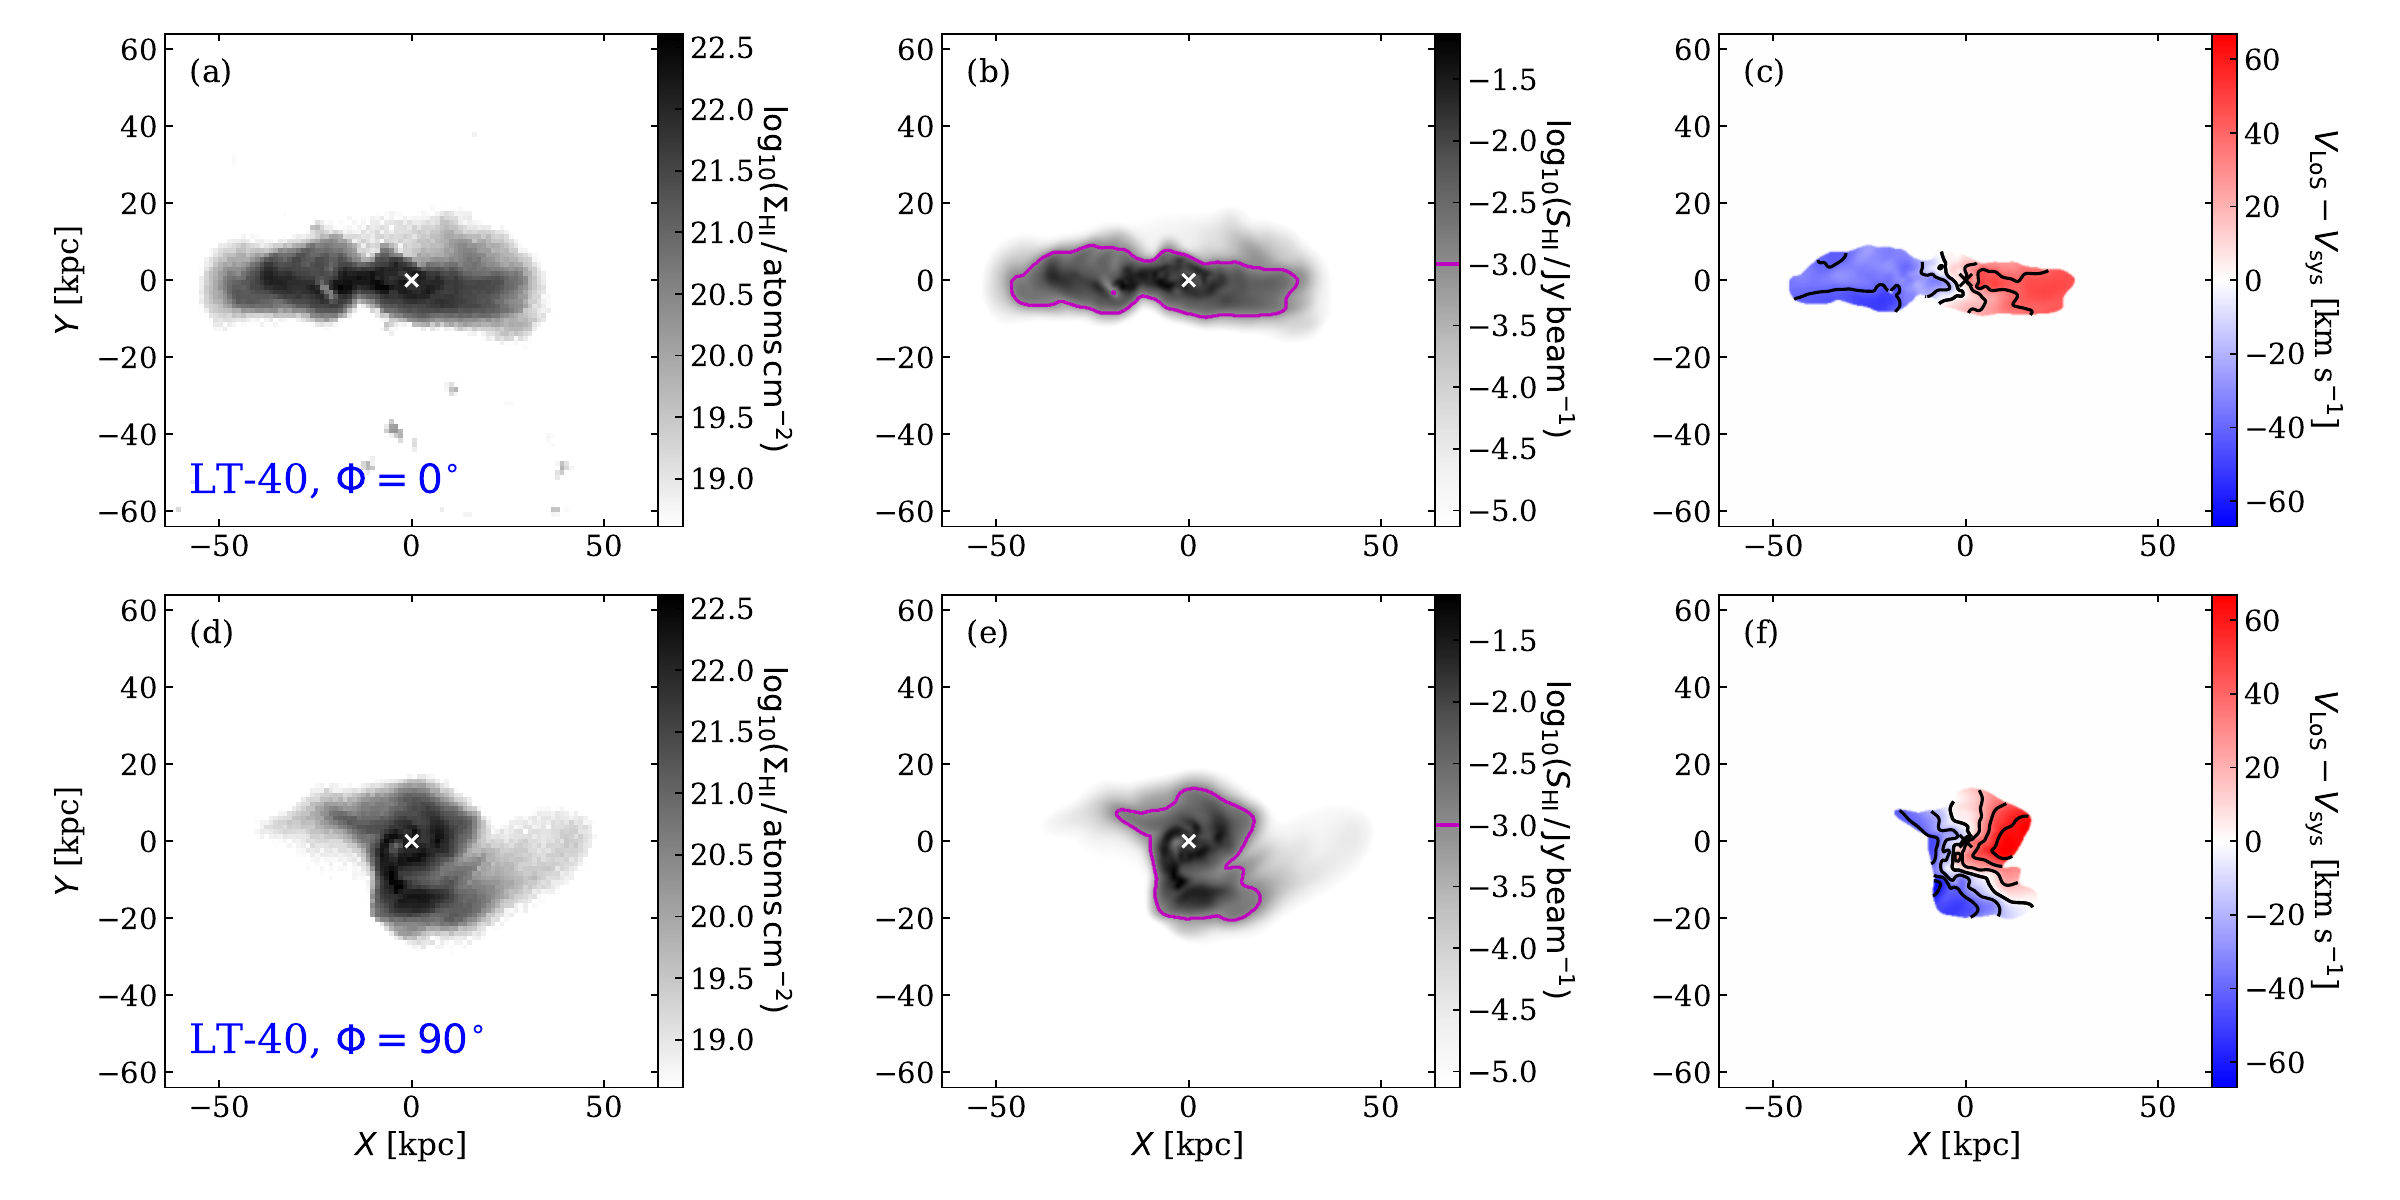}
\includegraphics[width=\textwidth]{../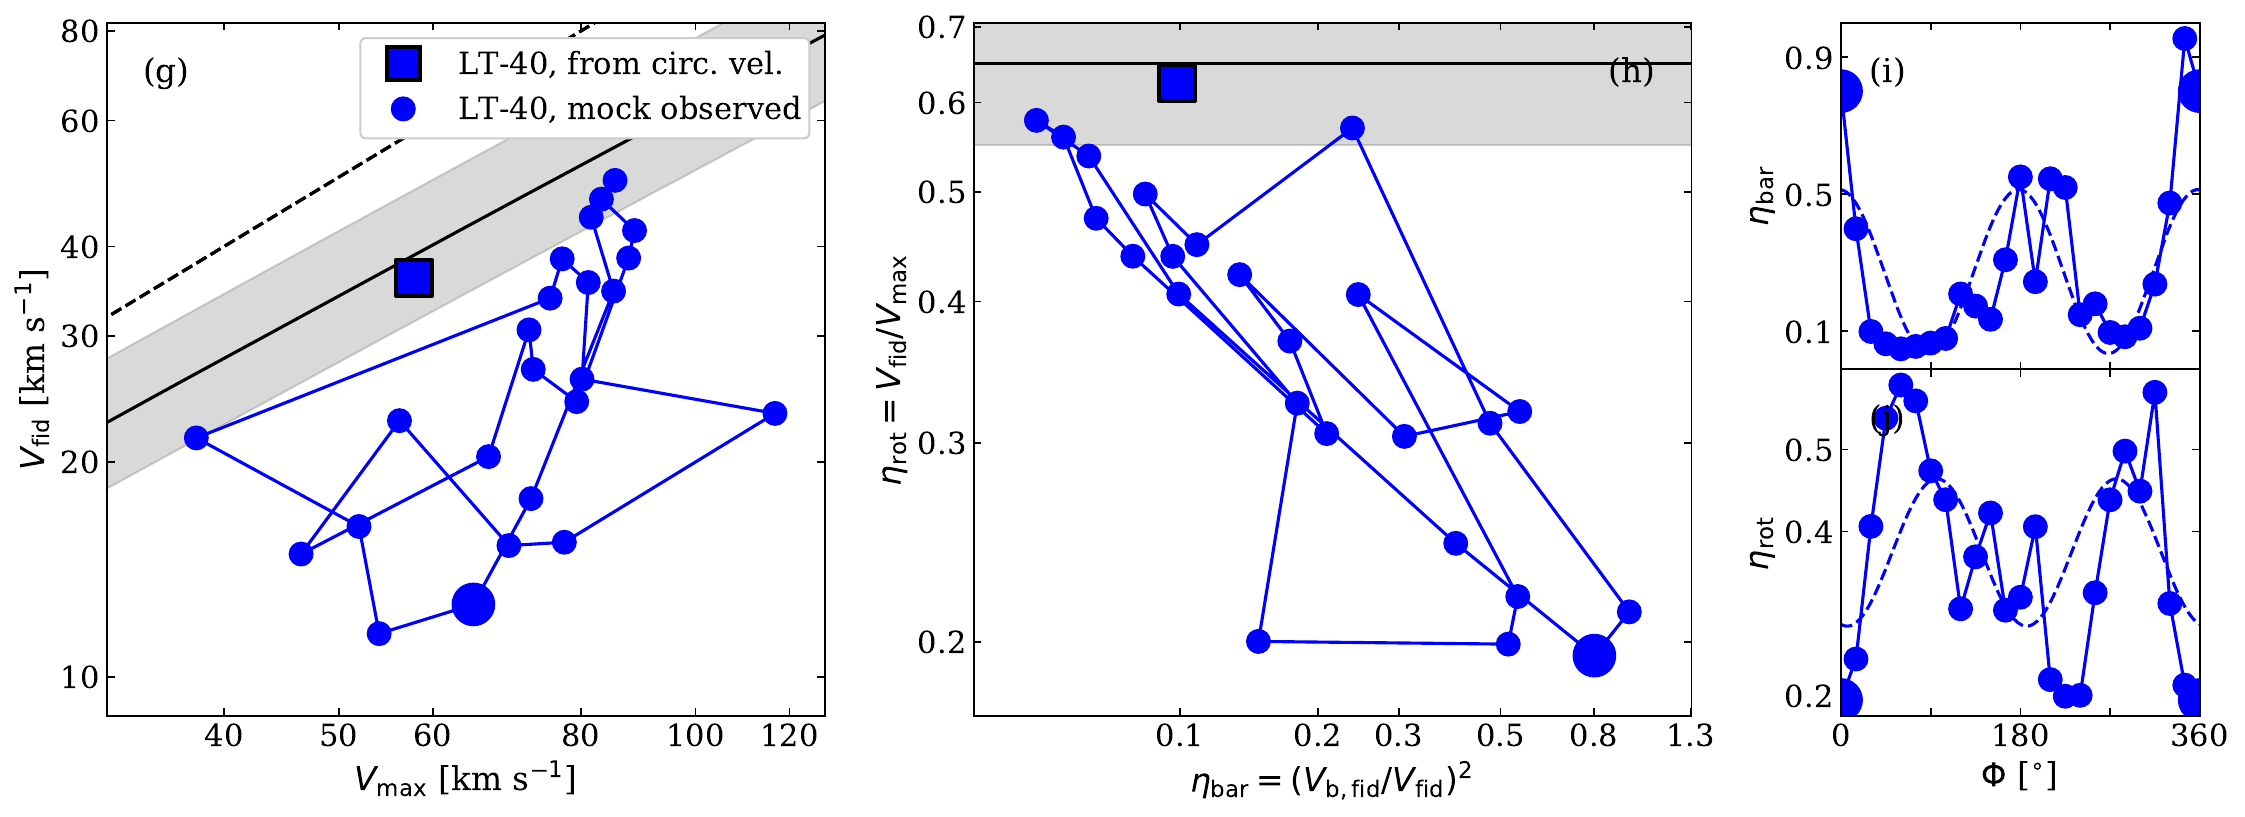}
\end{minipage}
\begin{minipage}{.4\textwidth}
\includegraphics[width=\textwidth]{../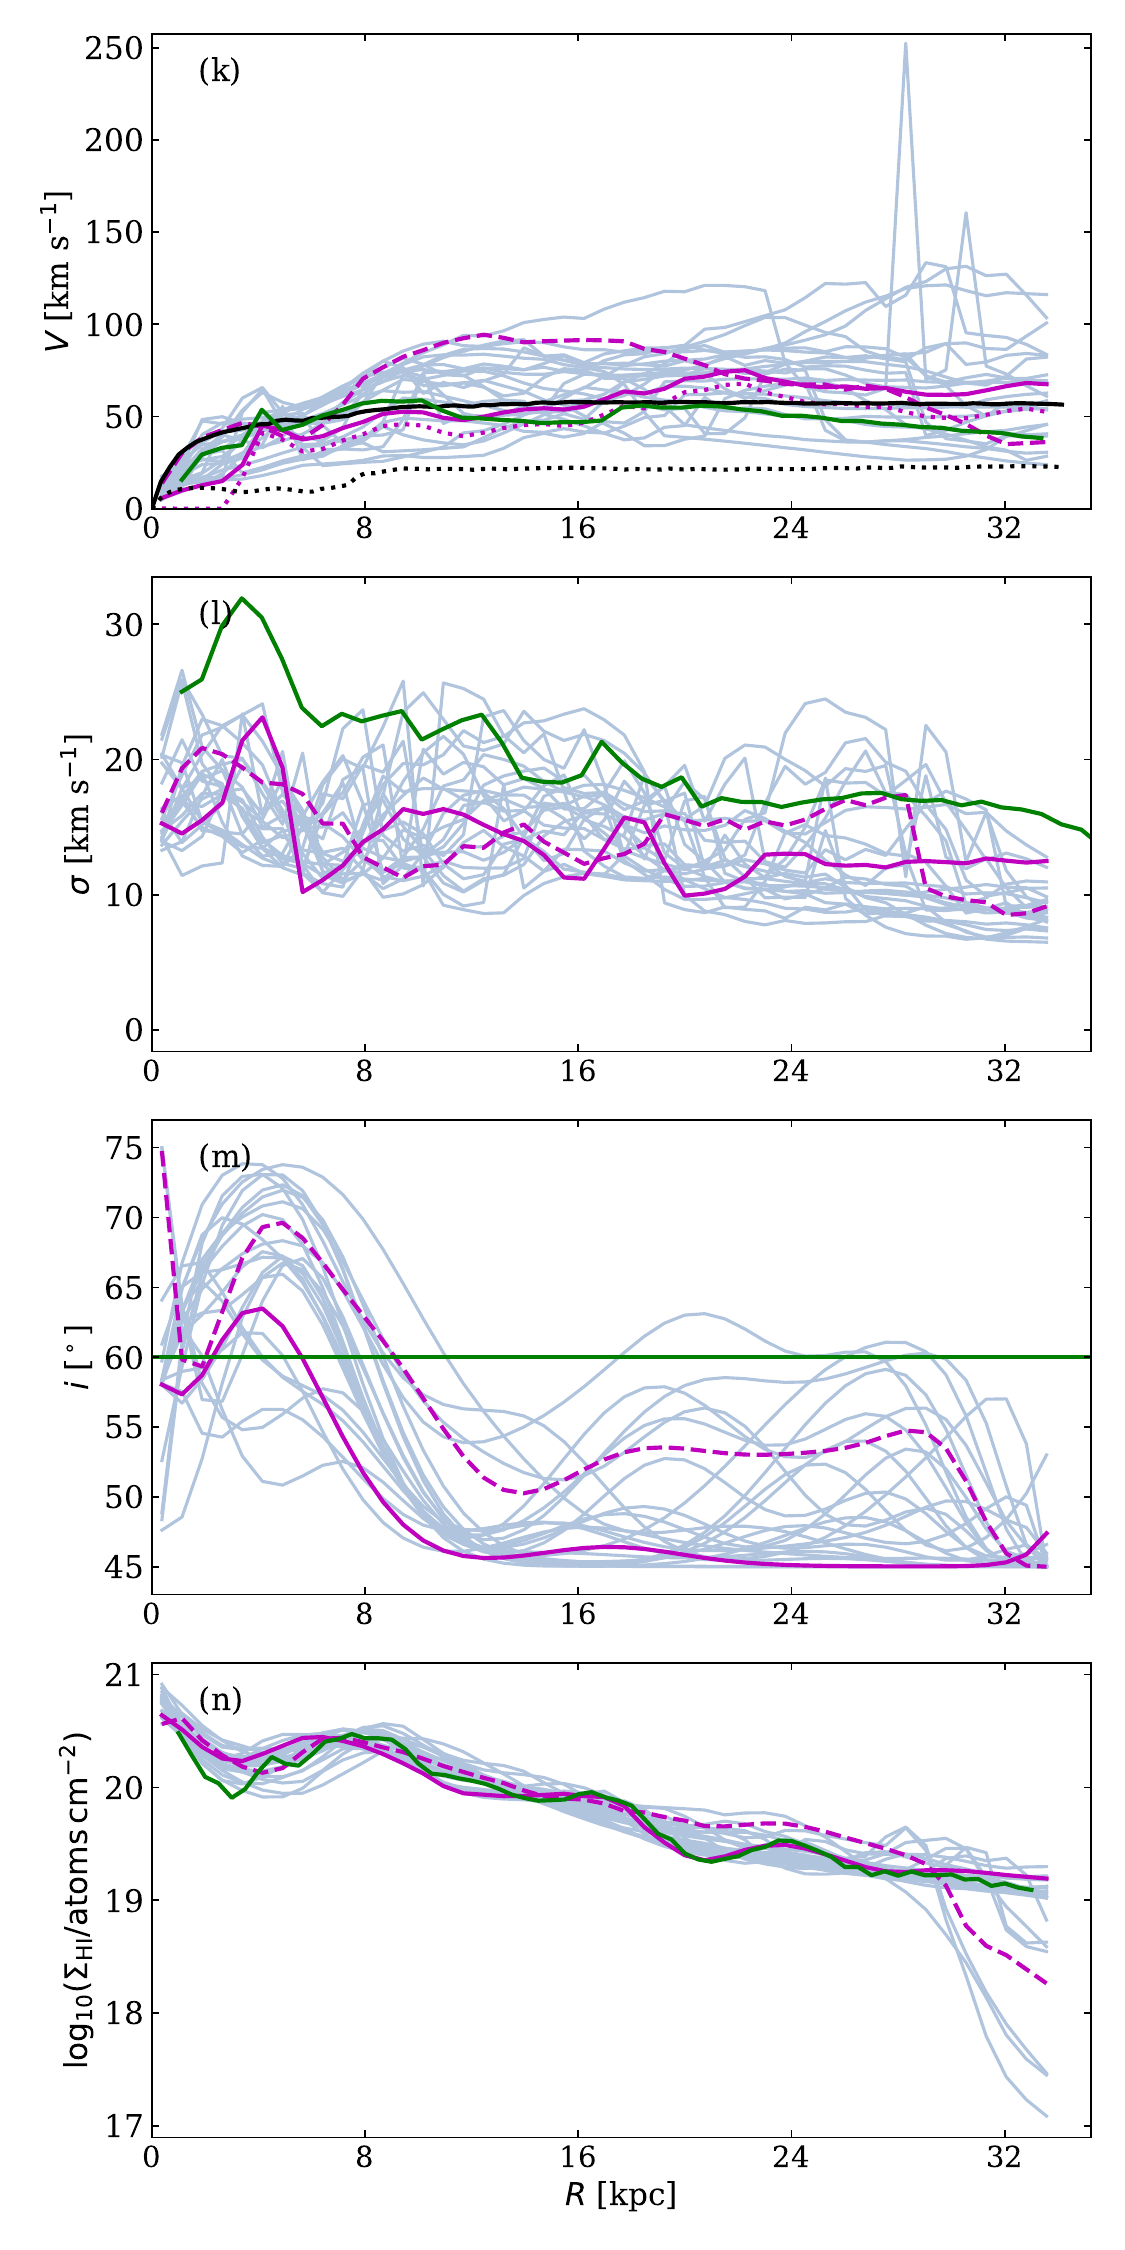}
\end{minipage}
\caption{A set of summary figures for galaxy LT-40, excluded from kinematic analysis. These include example moment maps for two orientations (panels (a)--(f); similar to Fig.~\ref{fig:visualisations}), a summary of the parameters $V_\mathrm{fid}$, $V_\mathrm{max}$, $\eta_\mathrm{rot}$, and $\eta_\mathrm{bar}$ (panels (g)--(j); similar to Fig.~\ref{fig:loops}), and a summary of the rotation curve analysis from $24$ viewing angles (panels (k)--(n); similar to Fig.~\ref{fig:rot_curves}). See description of Appendix~\ref{app:supplementary} for details.}
\label{fig:S38}
\end{figure}
\clearpage

\begin{figure}
\begin{minipage}{.9\textwidth}
\includegraphics[width=\textwidth]{../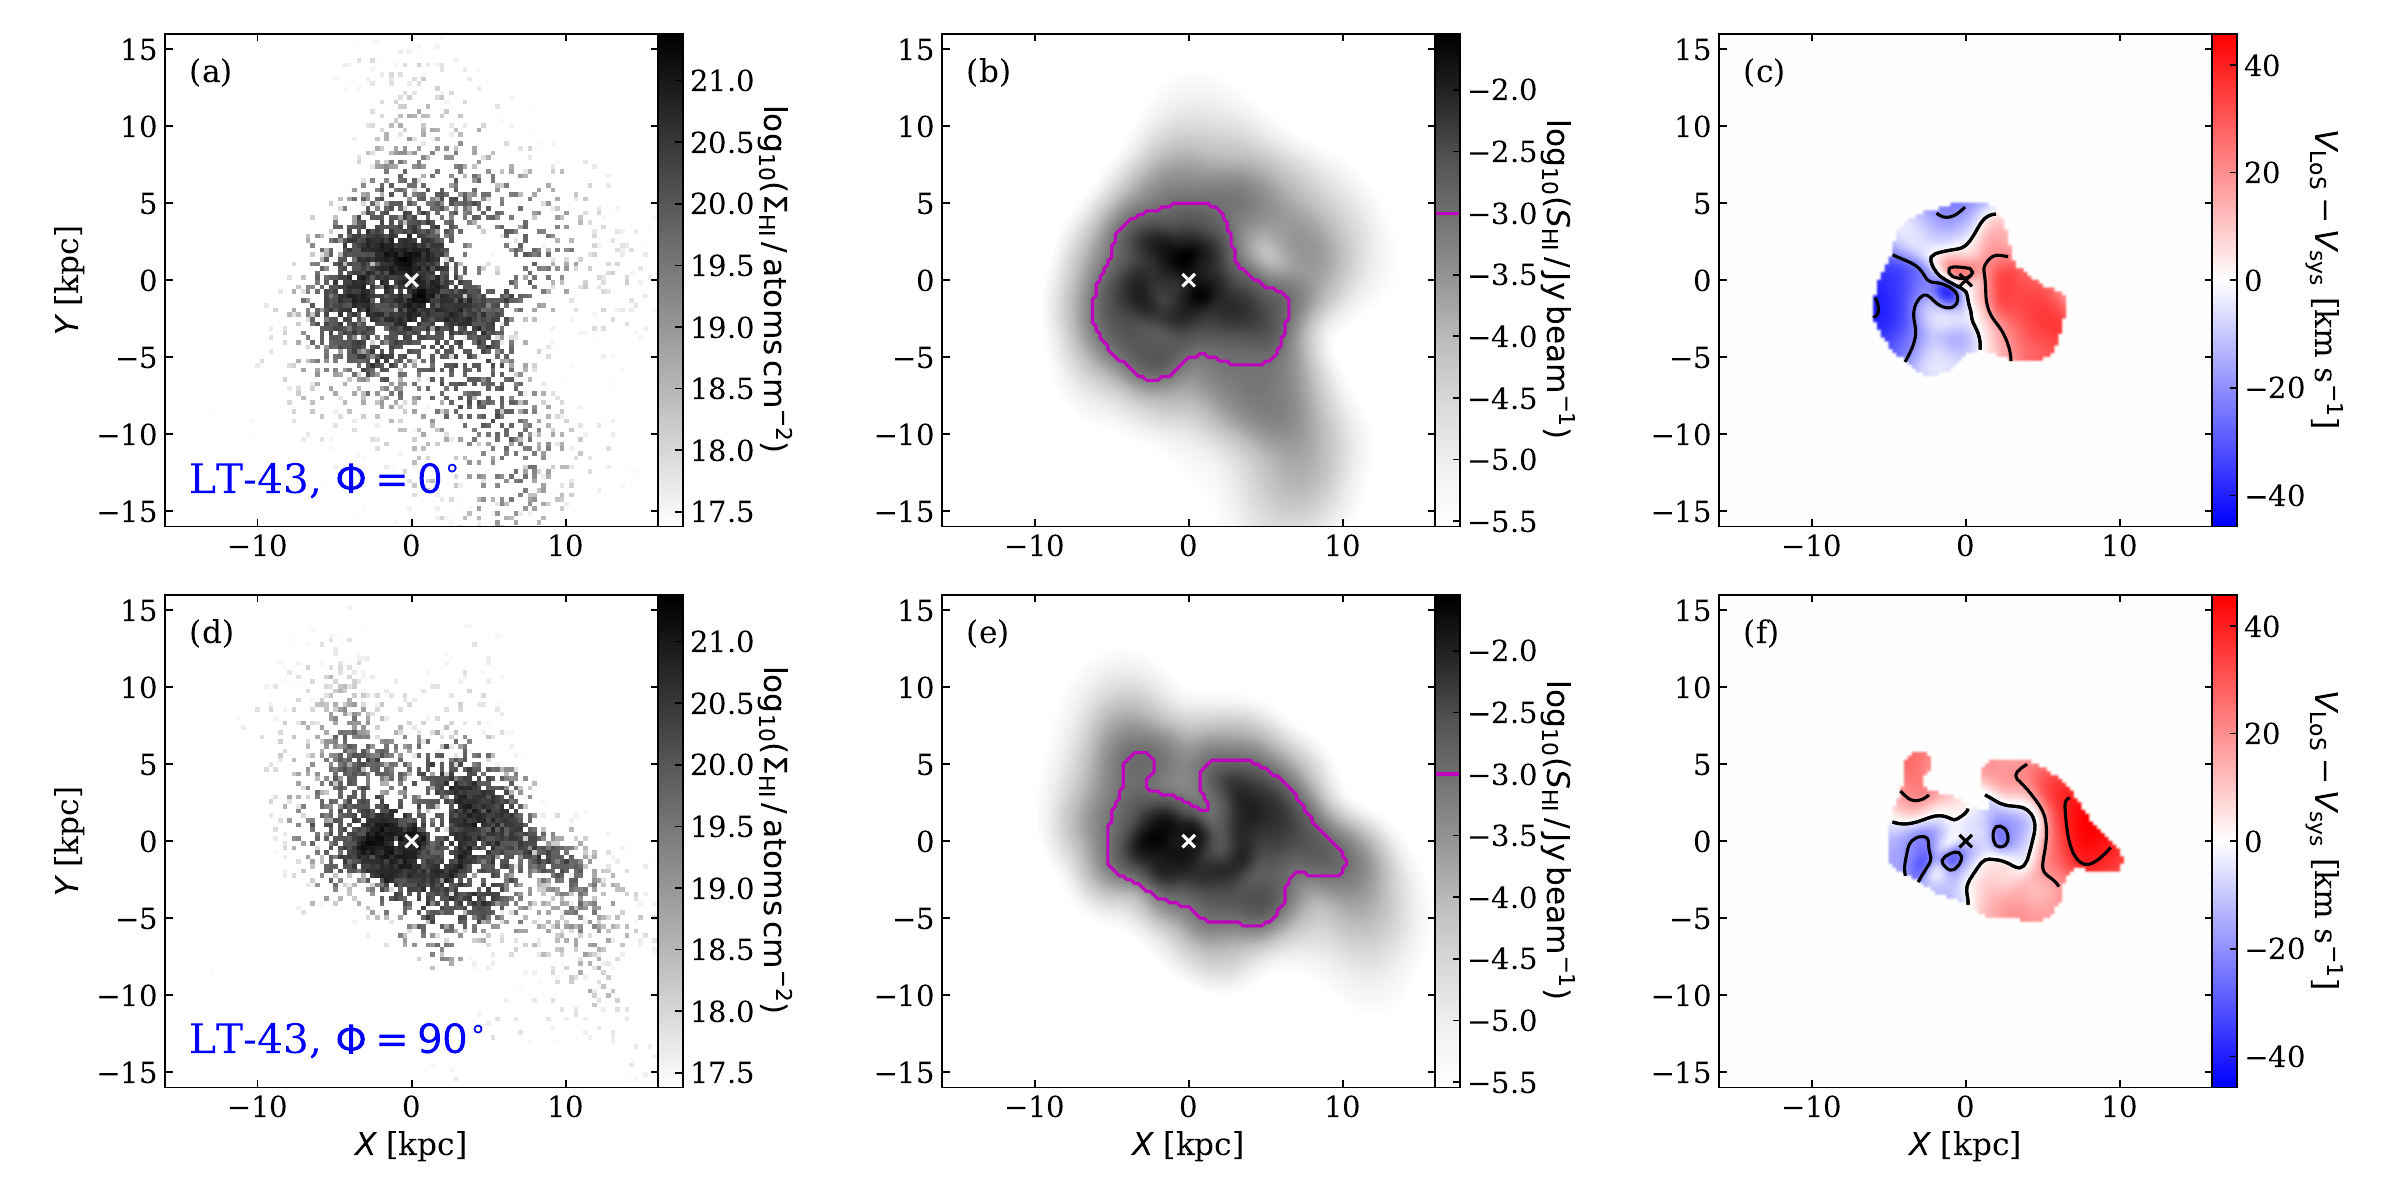}
\includegraphics[width=\textwidth]{../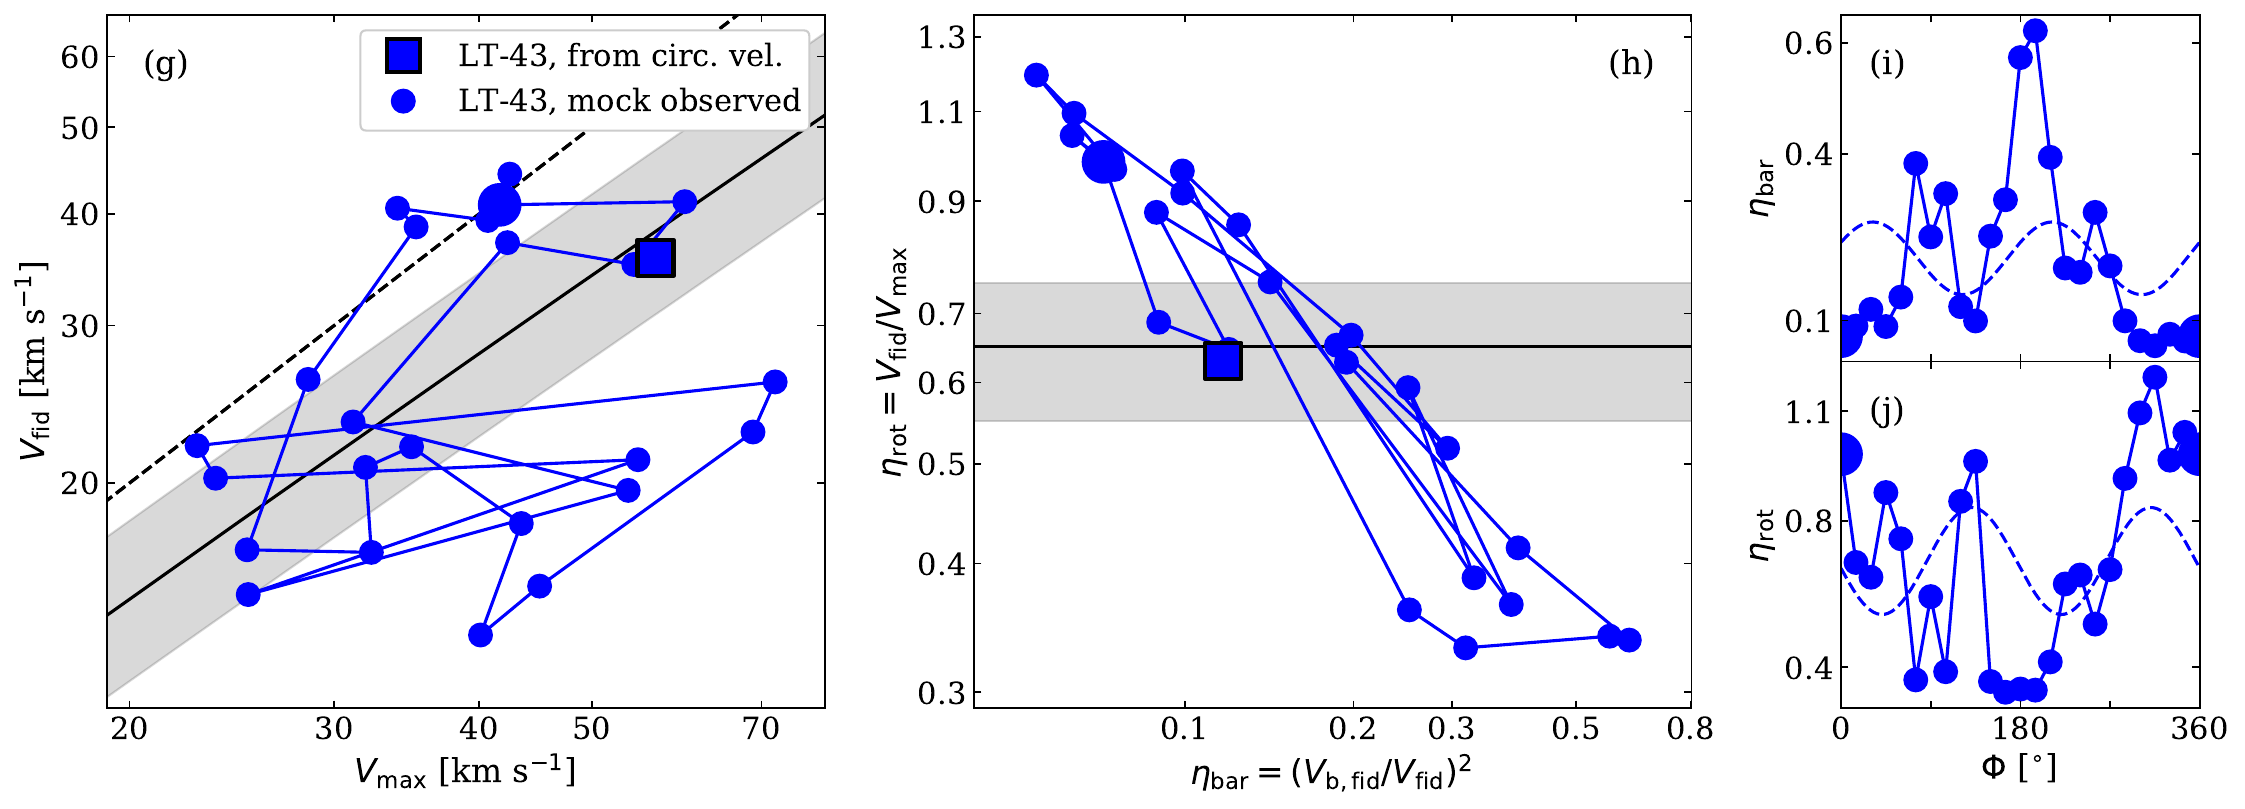}
\end{minipage}
\begin{minipage}{.4\textwidth}
\includegraphics[width=\textwidth]{../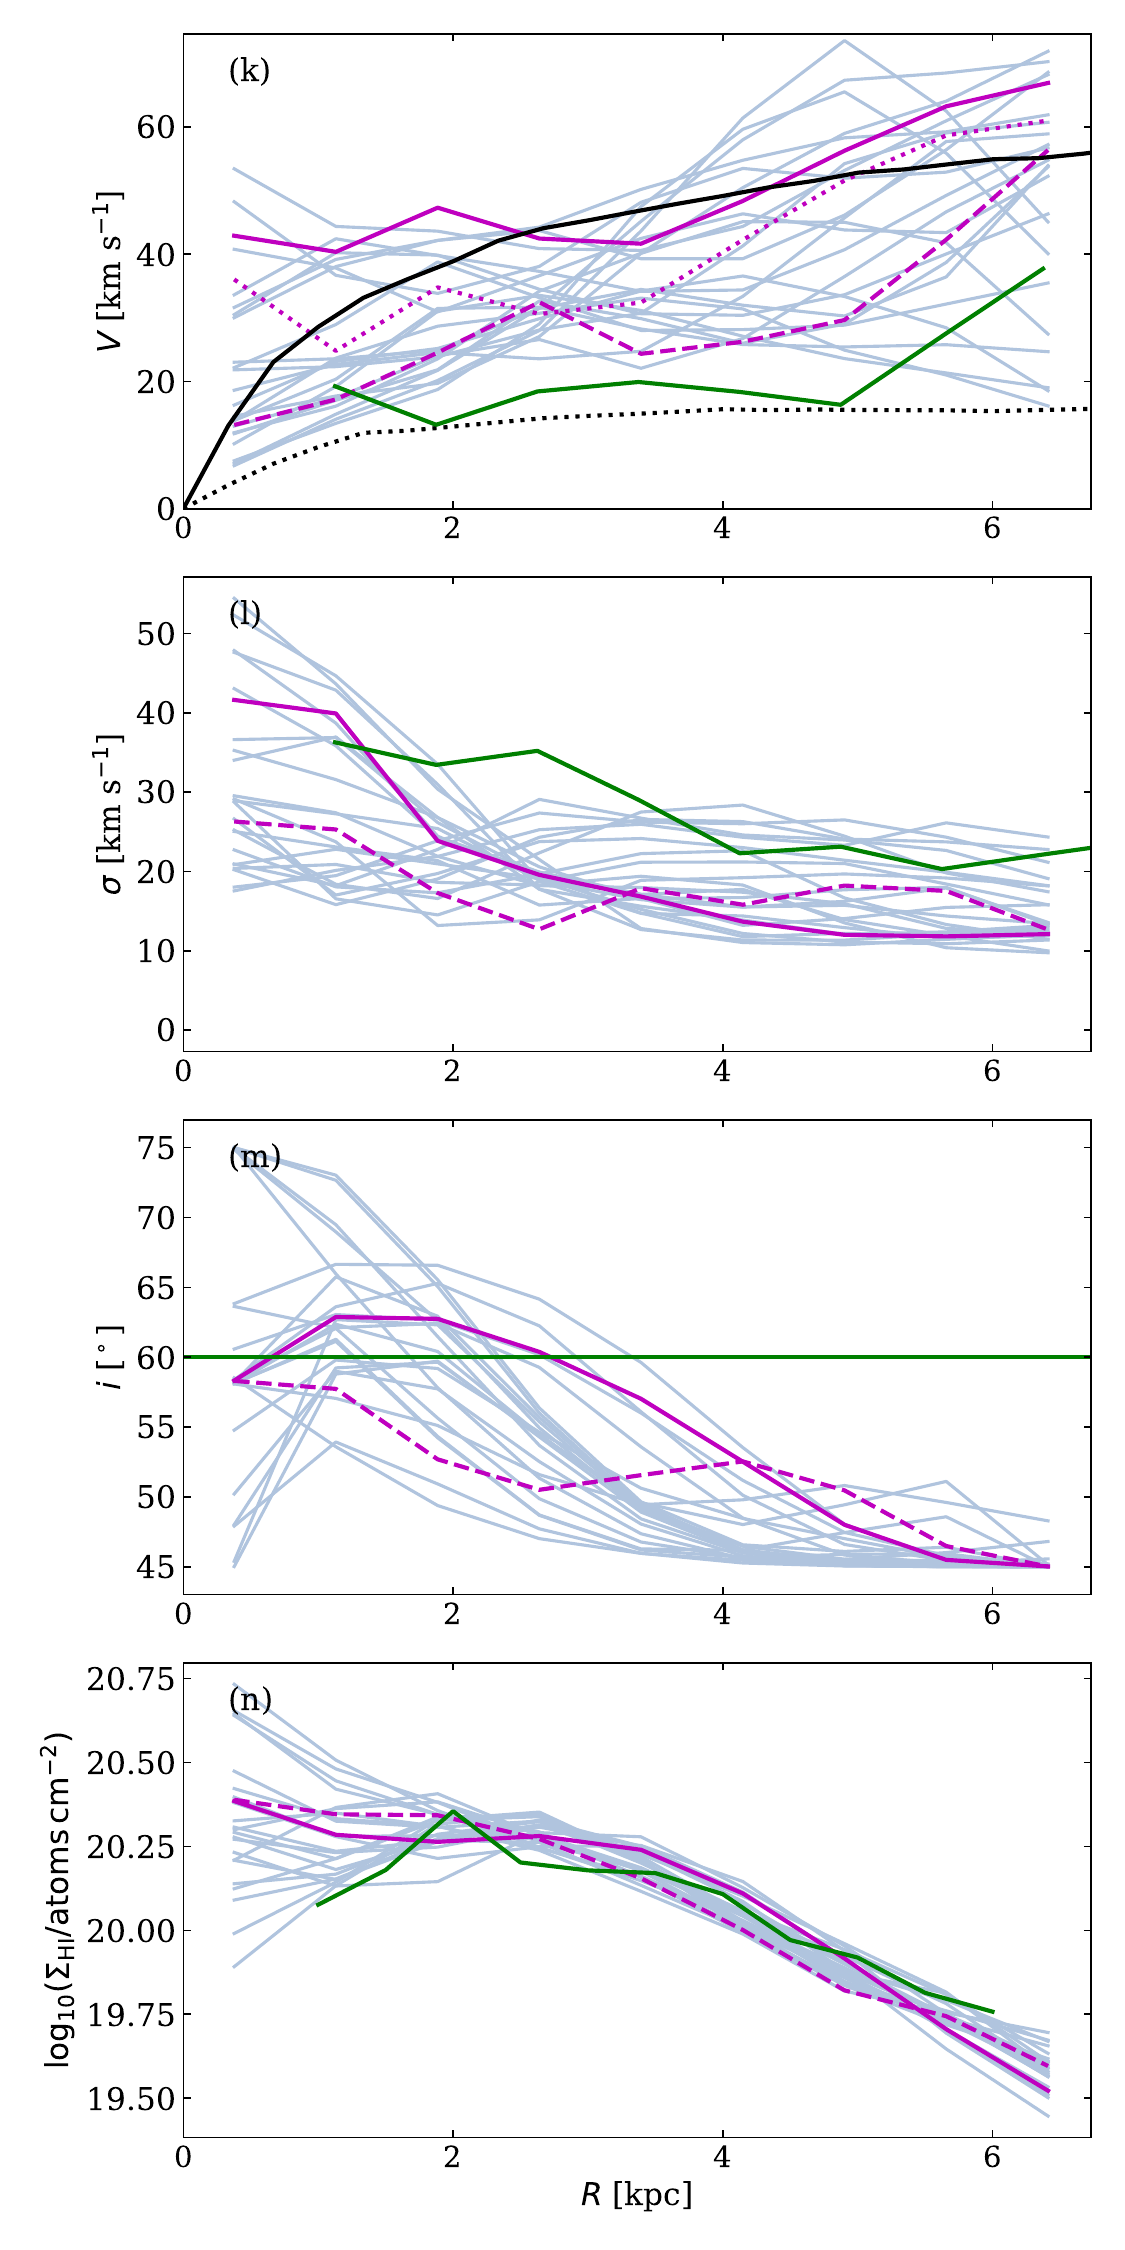}
\end{minipage}
\caption{A set of summary figures for galaxy LT-43, excluded from kinematic analysis. These include example moment maps for two orientations (panels (a)--(f); similar to Fig.~\ref{fig:visualisations}), a summary of the parameters $V_\mathrm{fid}$, $V_\mathrm{max}$, $\eta_\mathrm{rot}$, and $\eta_\mathrm{bar}$ (panels (g)--(j); similar to Fig.~\ref{fig:loops}), and a summary of the rotation curve analysis from $24$ viewing angles (panels (k)--(n); similar to Fig.~\ref{fig:rot_curves}). See description of Appendix~\ref{app:supplementary} for details.}
\label{fig:S39}
\end{figure}
\clearpage

\begin{figure}
\begin{minipage}{.9\textwidth}
\includegraphics[width=\textwidth]{../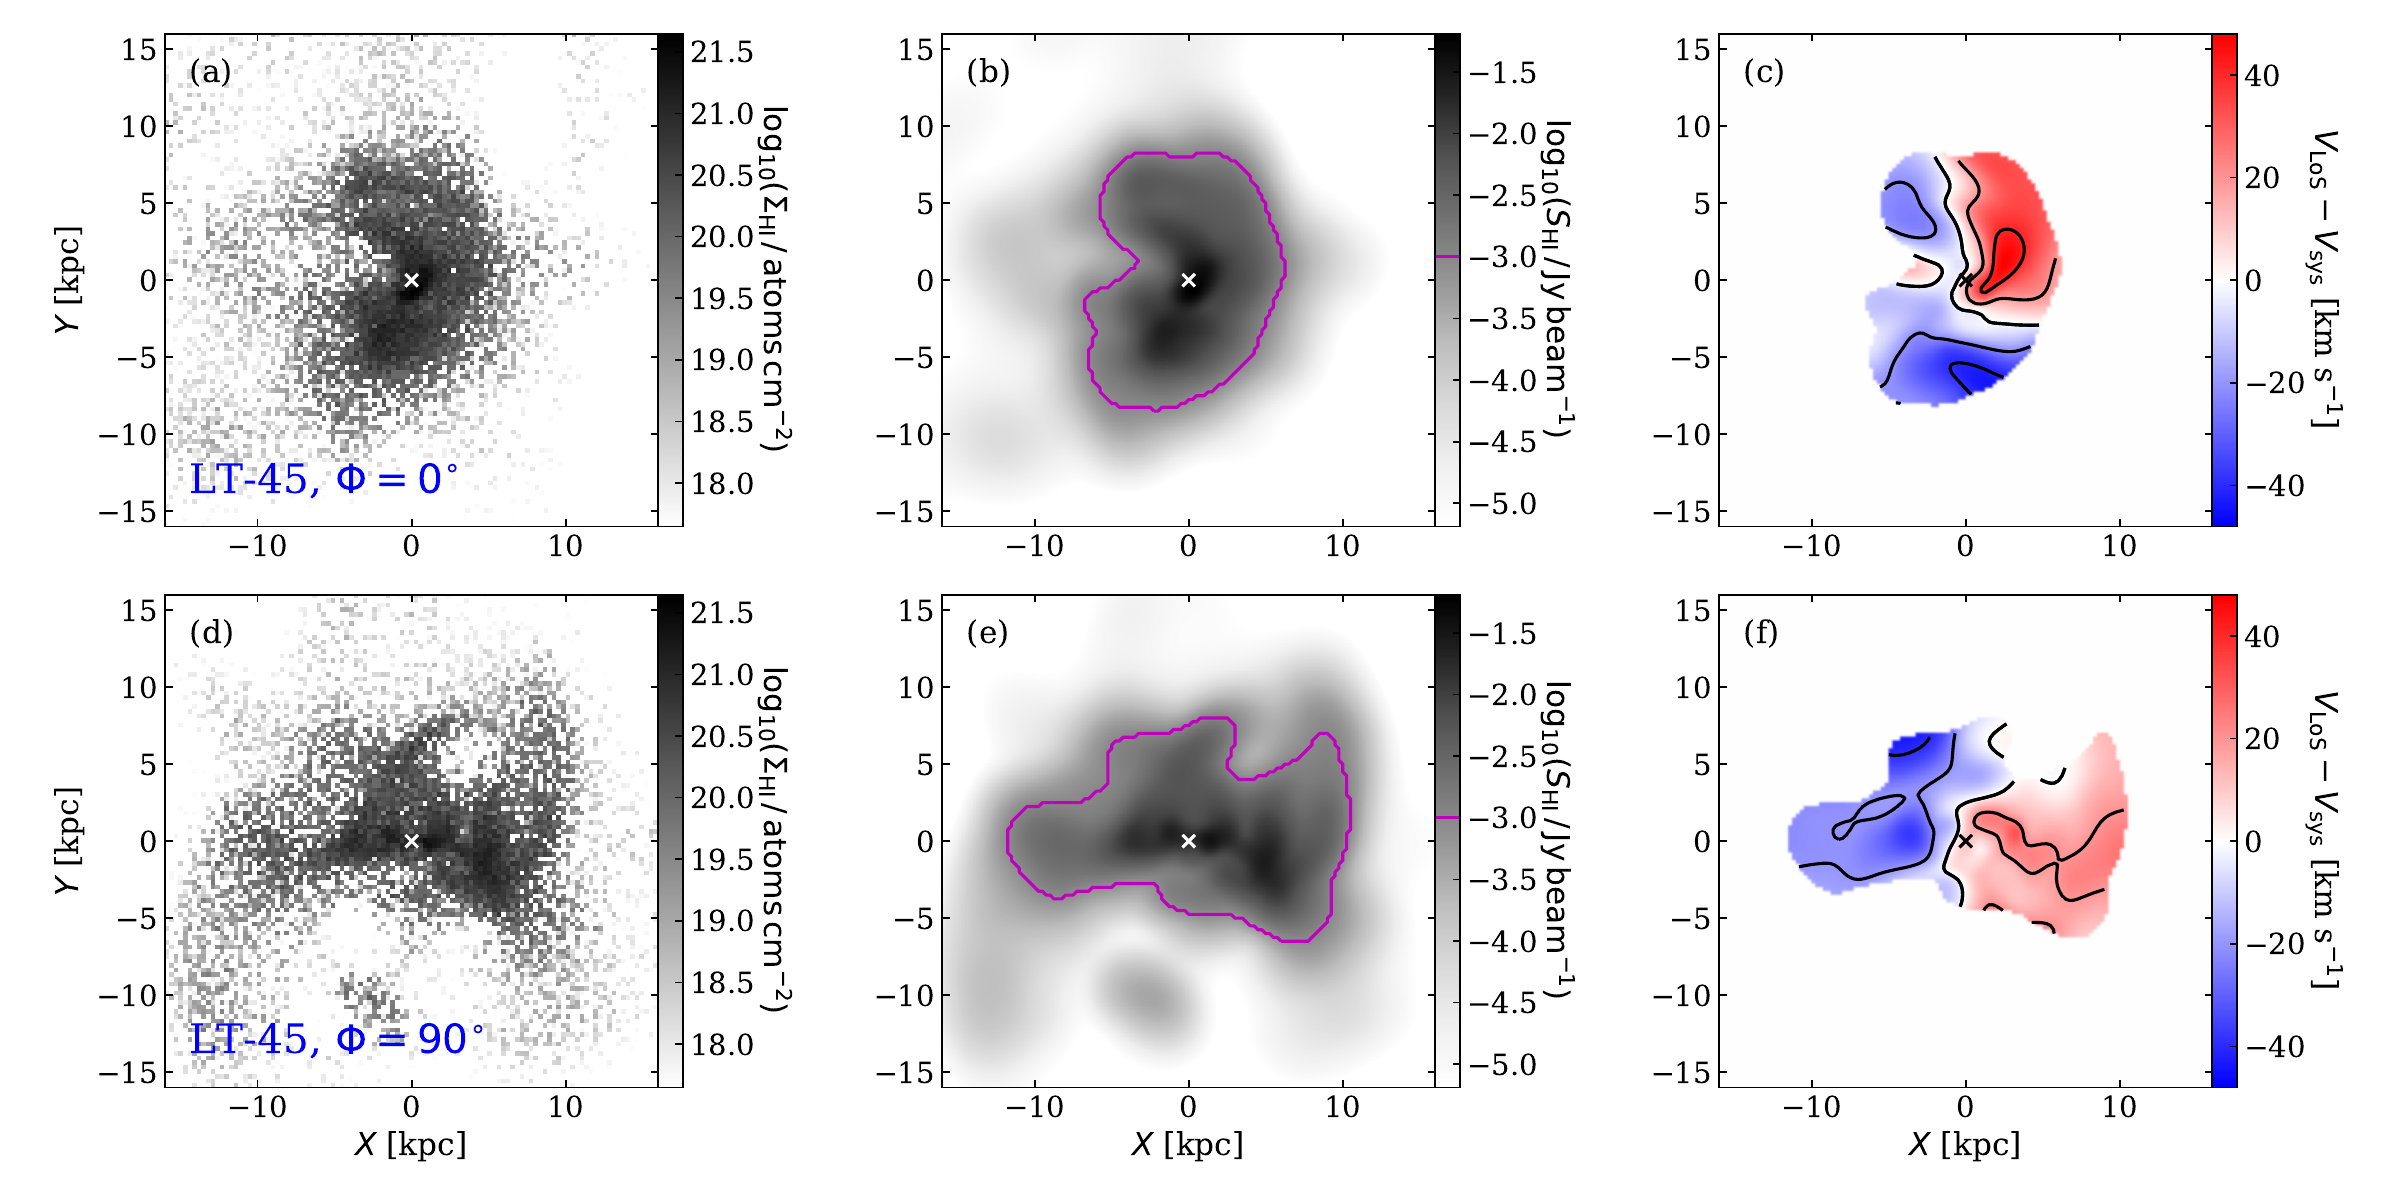}
\includegraphics[width=\textwidth]{../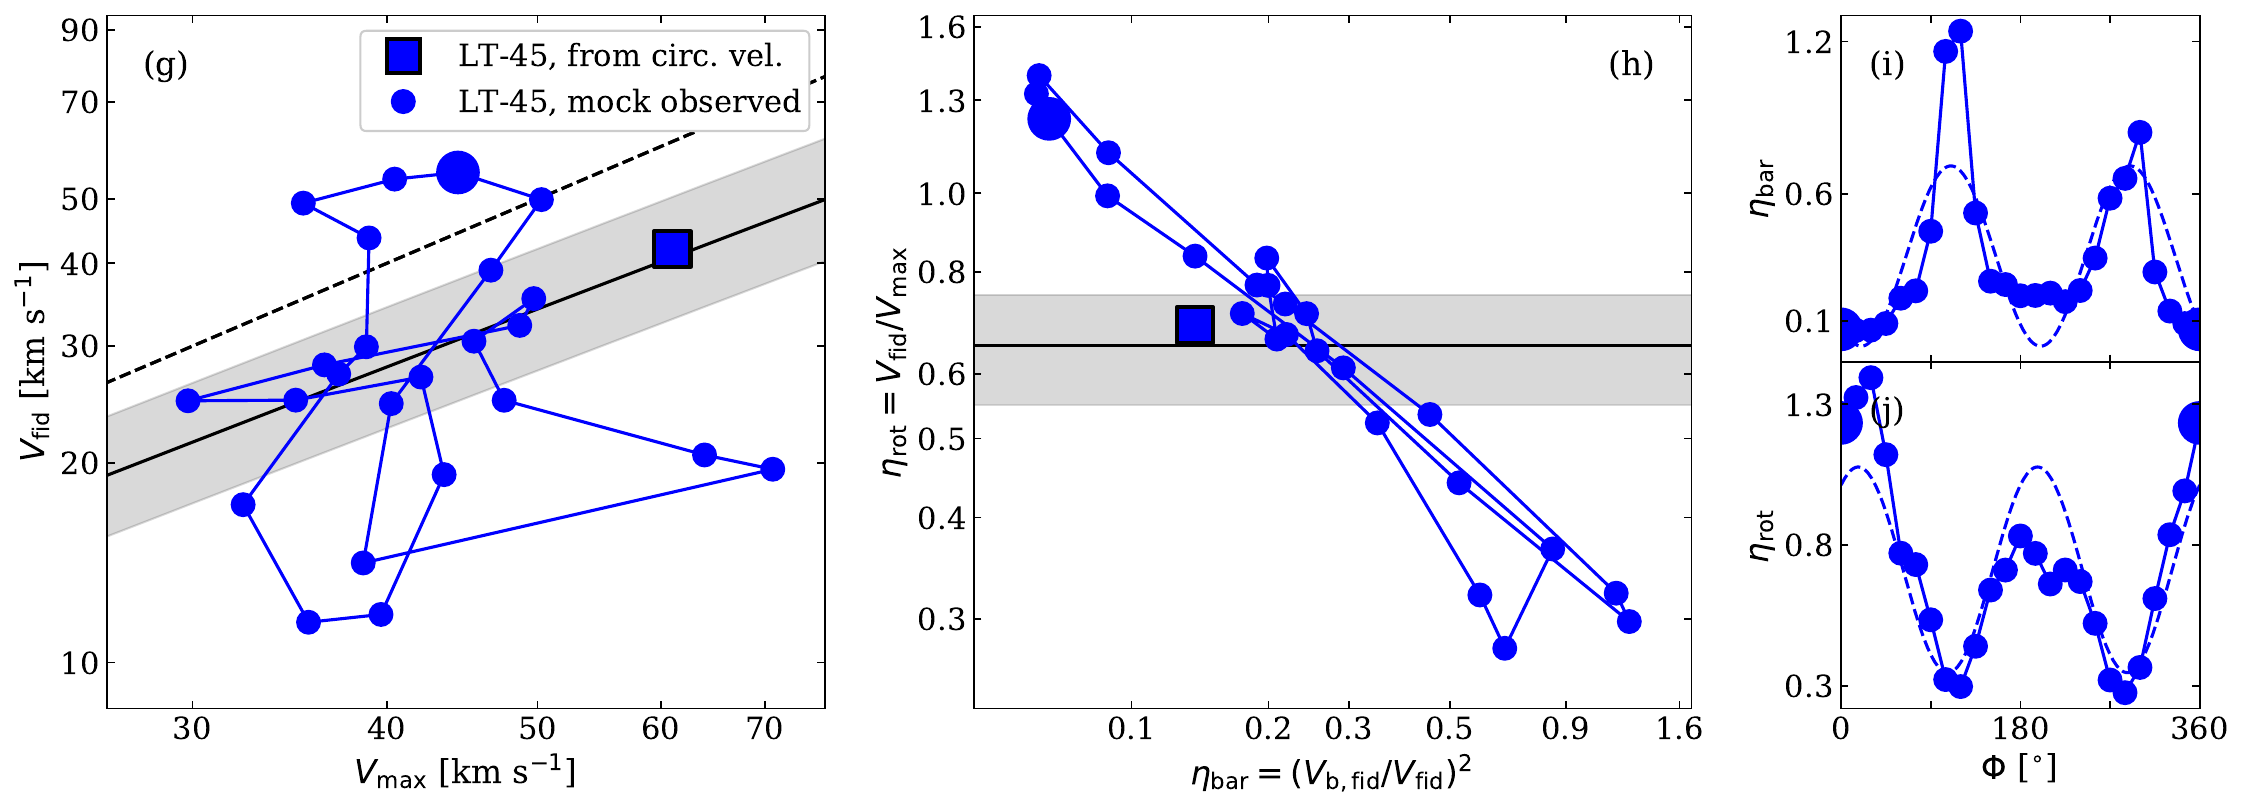}
\end{minipage}
\begin{minipage}{.4\textwidth}
\includegraphics[width=\textwidth]{../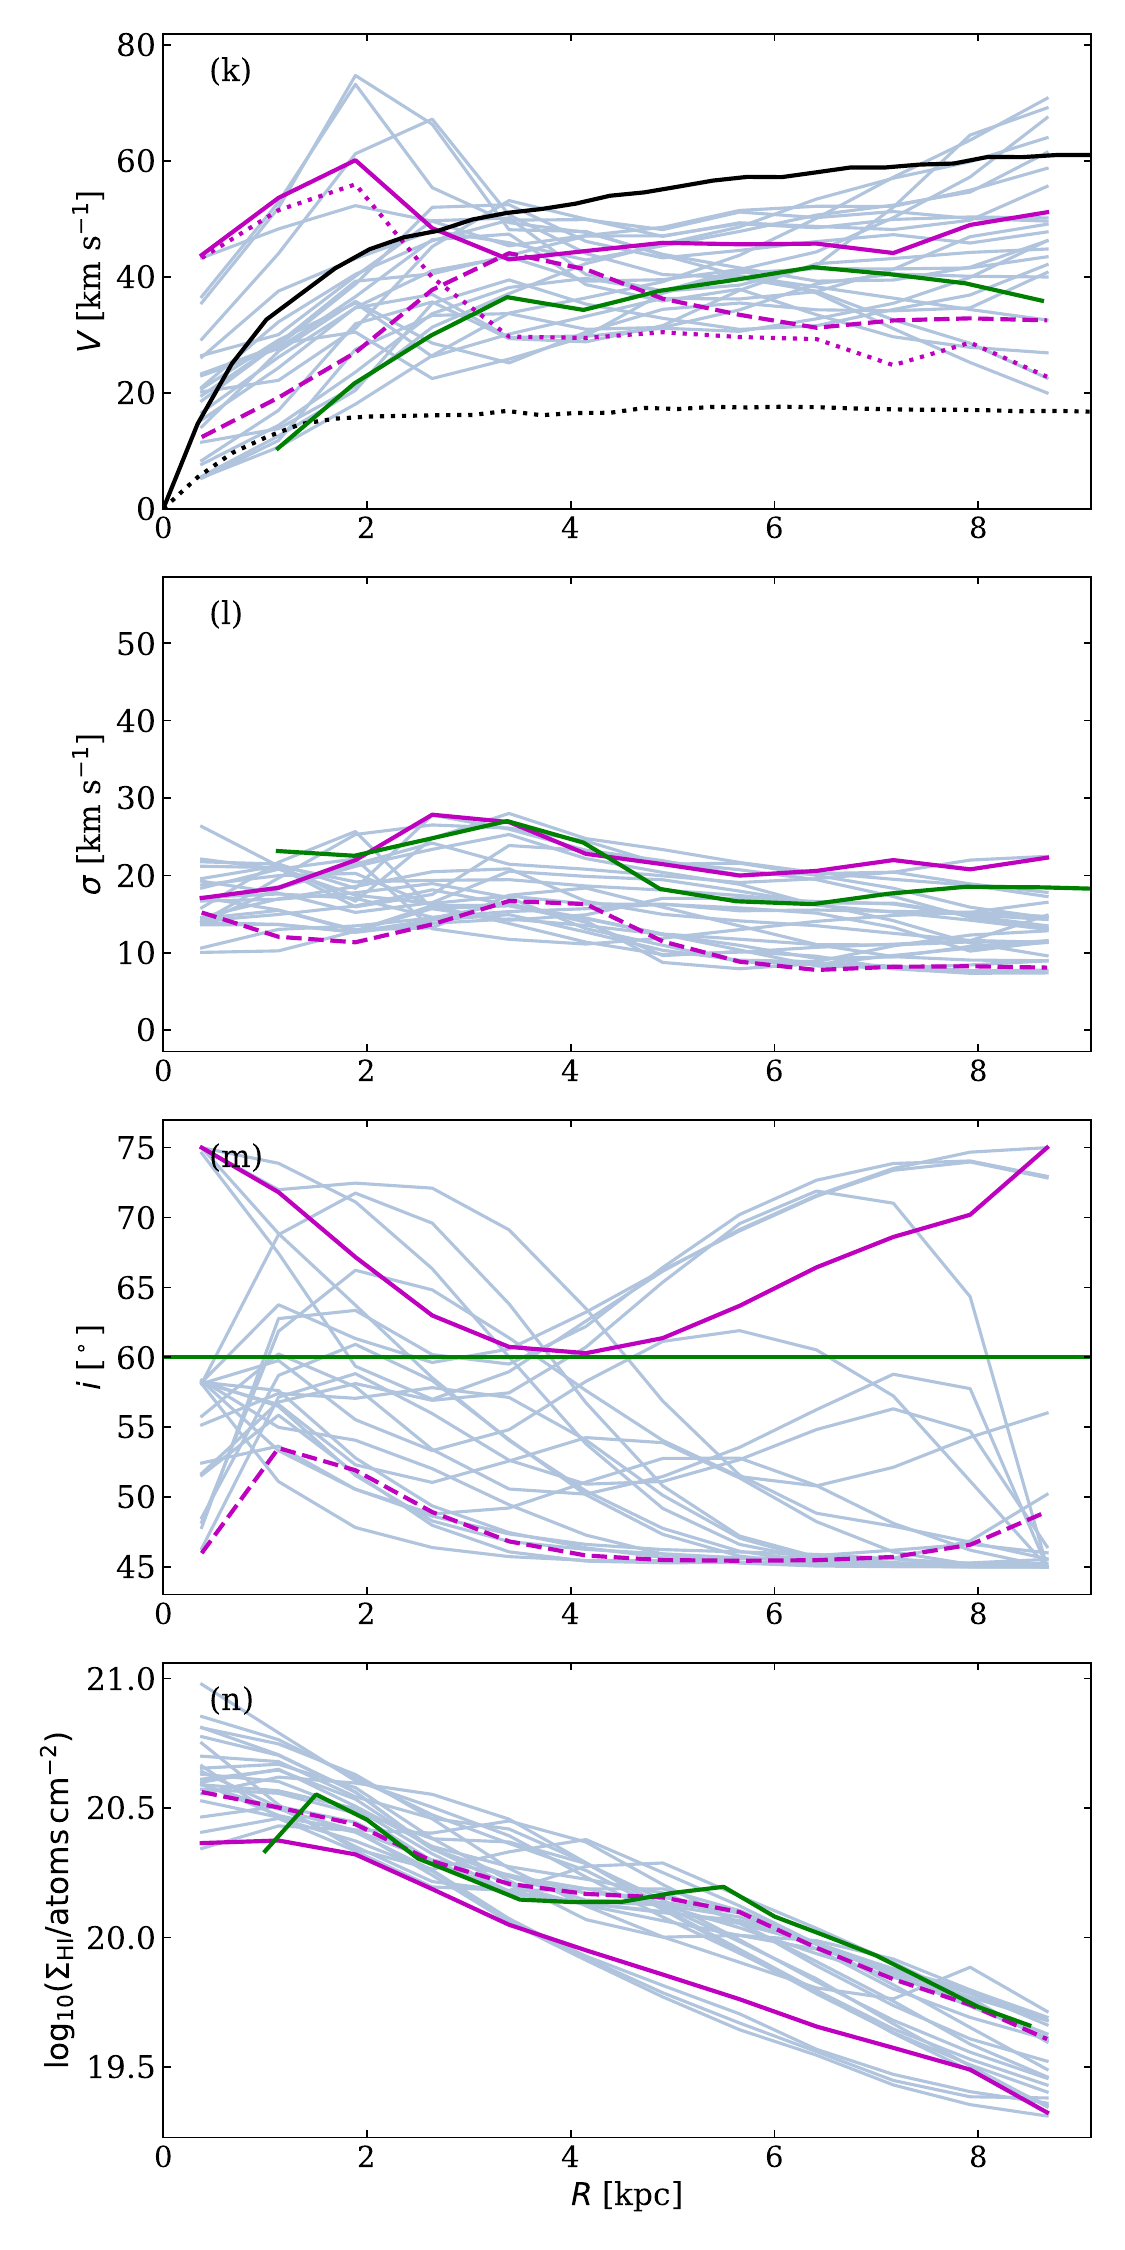}
\end{minipage}
\caption{A set of summary figures for galaxy LT-45, excluded from kinematic analysis. These include example moment maps for two orientations (panels (a)--(f); similar to Fig.~\ref{fig:visualisations}), a summary of the parameters $V_\mathrm{fid}$, $V_\mathrm{max}$, $\eta_\mathrm{rot}$, and $\eta_\mathrm{bar}$ (panels (g)--(j); similar to Fig.~\ref{fig:loops}), and a summary of the rotation curve analysis from $24$ viewing angles (panels (k)--(n); similar to Fig.~\ref{fig:rot_curves}). See description of Appendix~\ref{app:supplementary} for details.}
\label{fig:S40}
\end{figure}
\clearpage

\begin{figure}
\begin{minipage}{.9\textwidth}
\includegraphics[width=\textwidth]{../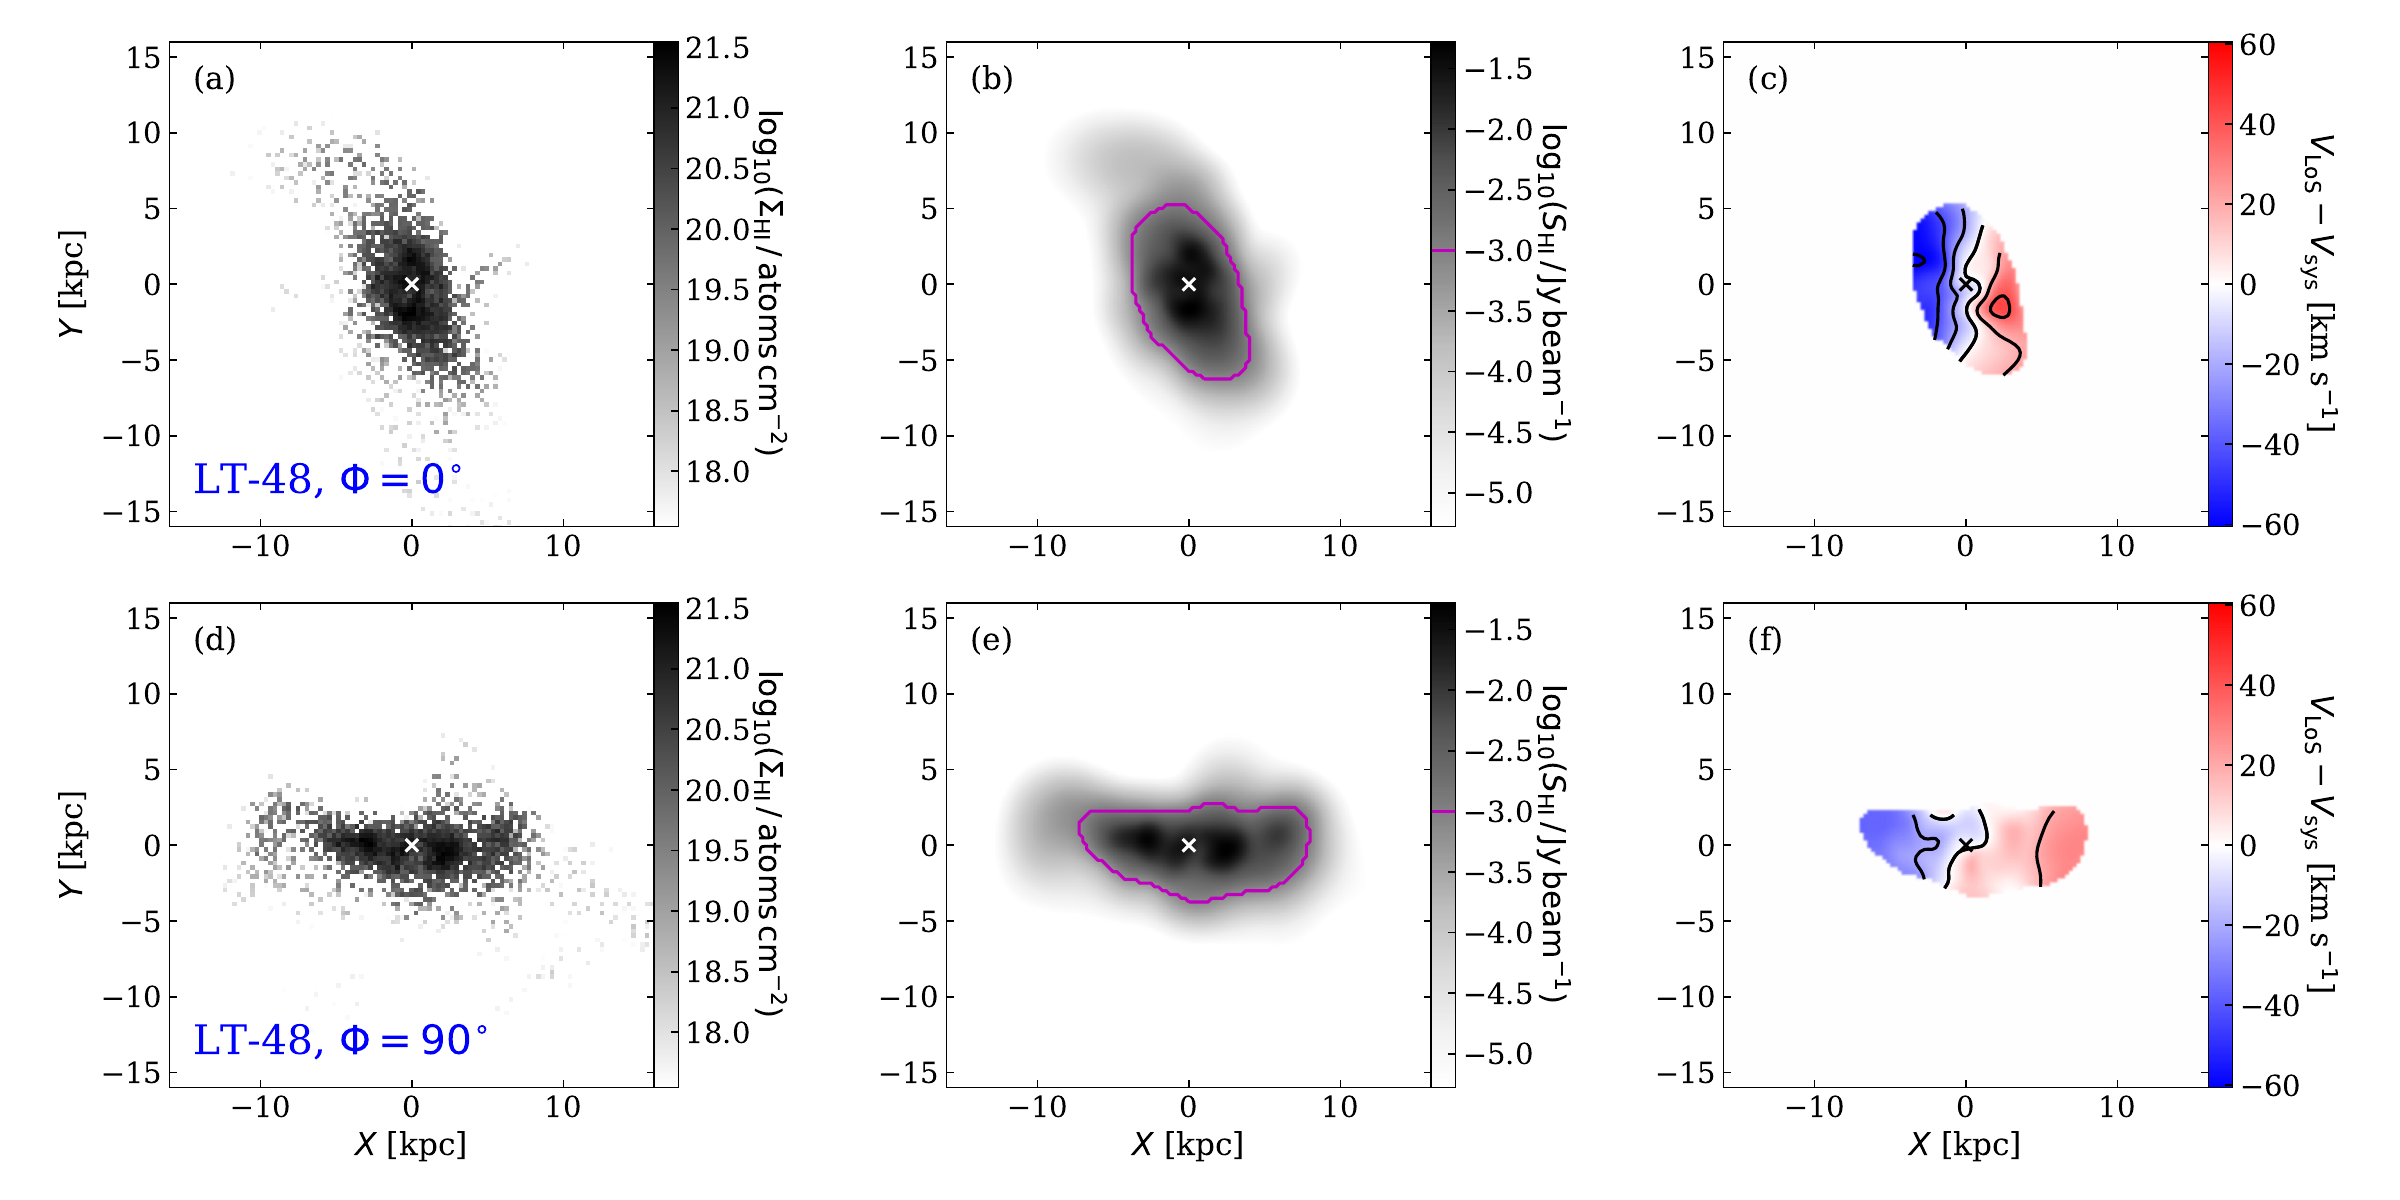}
\includegraphics[width=\textwidth]{../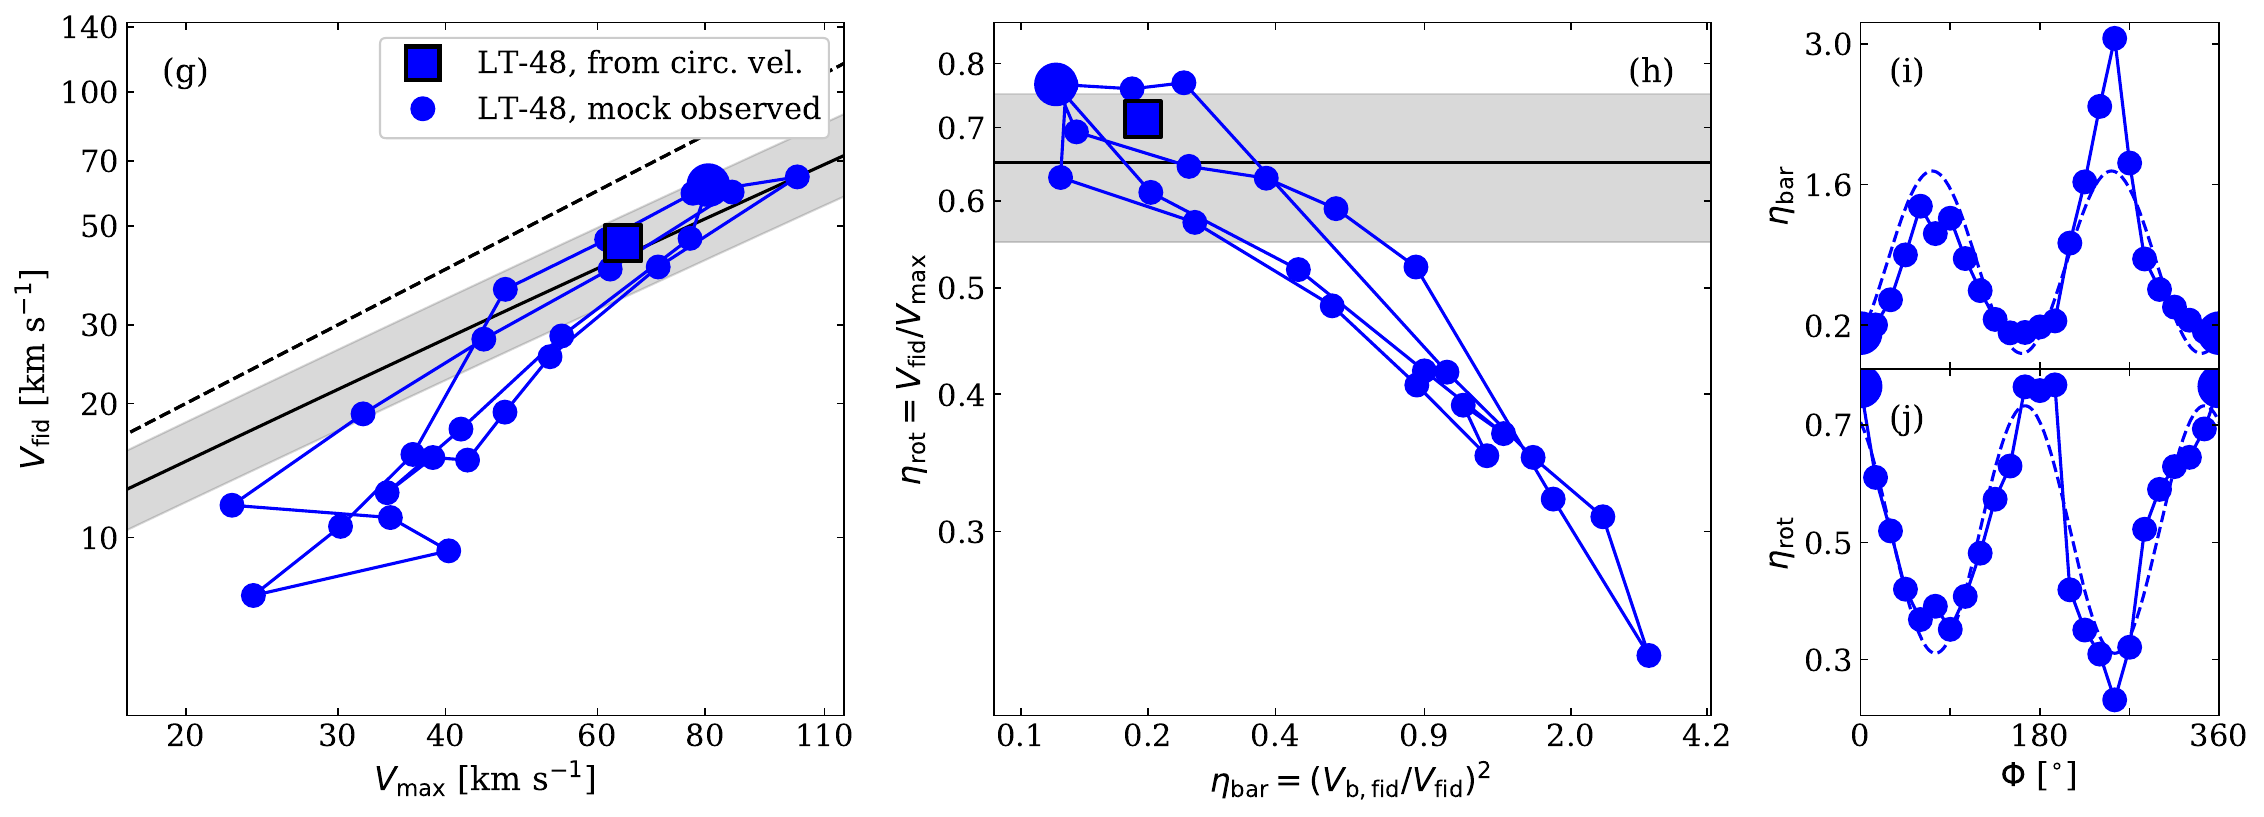}
\end{minipage}
\begin{minipage}{.4\textwidth}
\includegraphics[width=\textwidth]{../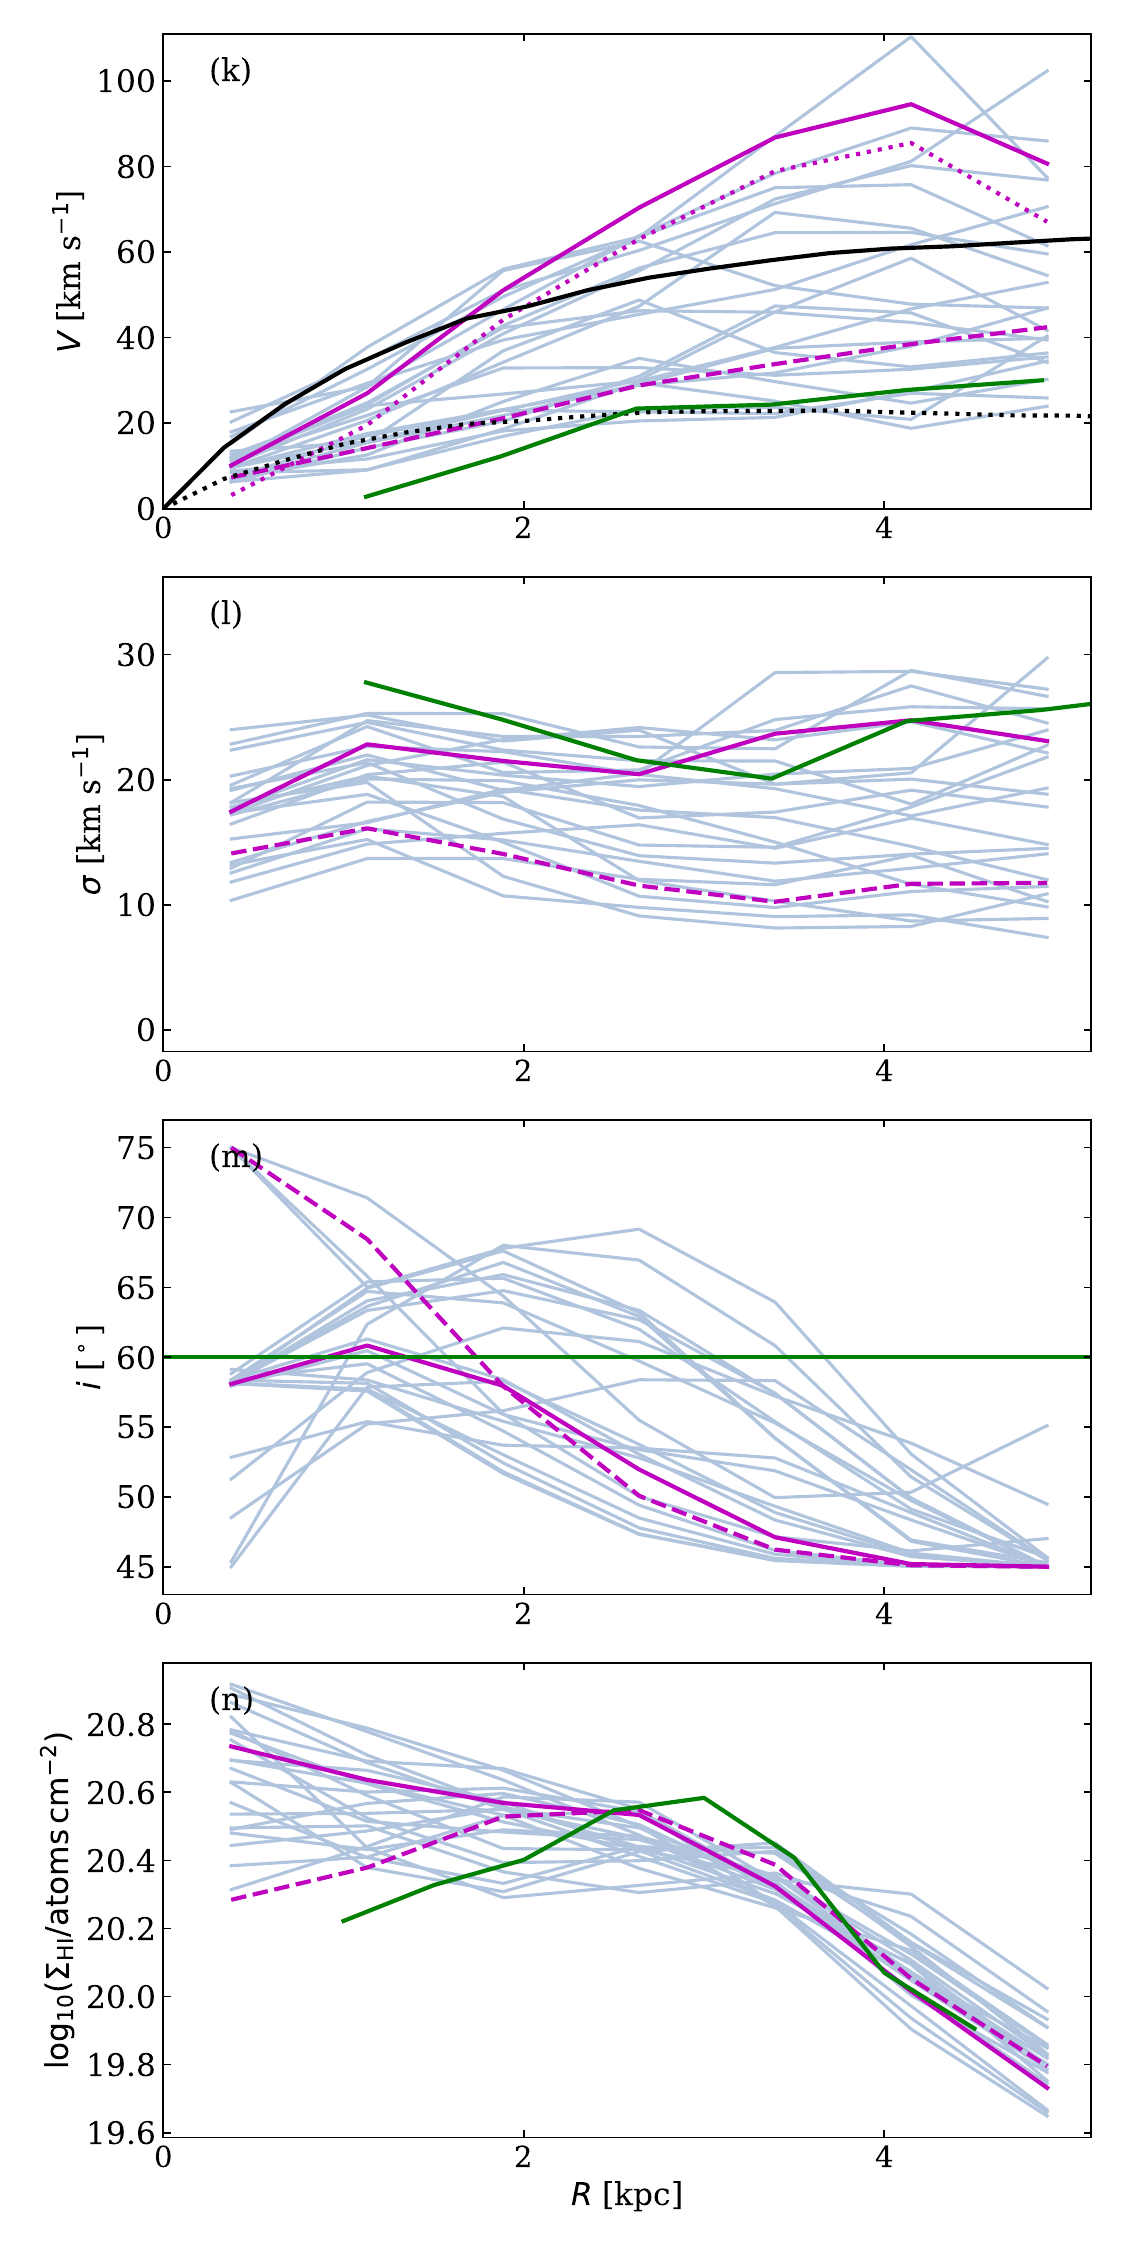}
\end{minipage}
\caption{A set of summary figures for galaxy LT-48, excluded from kinematic analysis. These include example moment maps for two orientations (panels (a)--(f); similar to Fig.~\ref{fig:visualisations}), a summary of the parameters $V_\mathrm{fid}$, $V_\mathrm{max}$, $\eta_\mathrm{rot}$, and $\eta_\mathrm{bar}$ (panels (g)--(j); similar to Fig.~\ref{fig:loops}), and a summary of the rotation curve analysis from $24$ viewing angles (panels (k)--(n); similar to Fig.~\ref{fig:rot_curves}). See description of Appendix~\ref{app:supplementary} for details.}
\label{fig:S41}
\end{figure}
\clearpage

\begin{figure}
\begin{minipage}{.9\textwidth}
\includegraphics[width=\textwidth]{../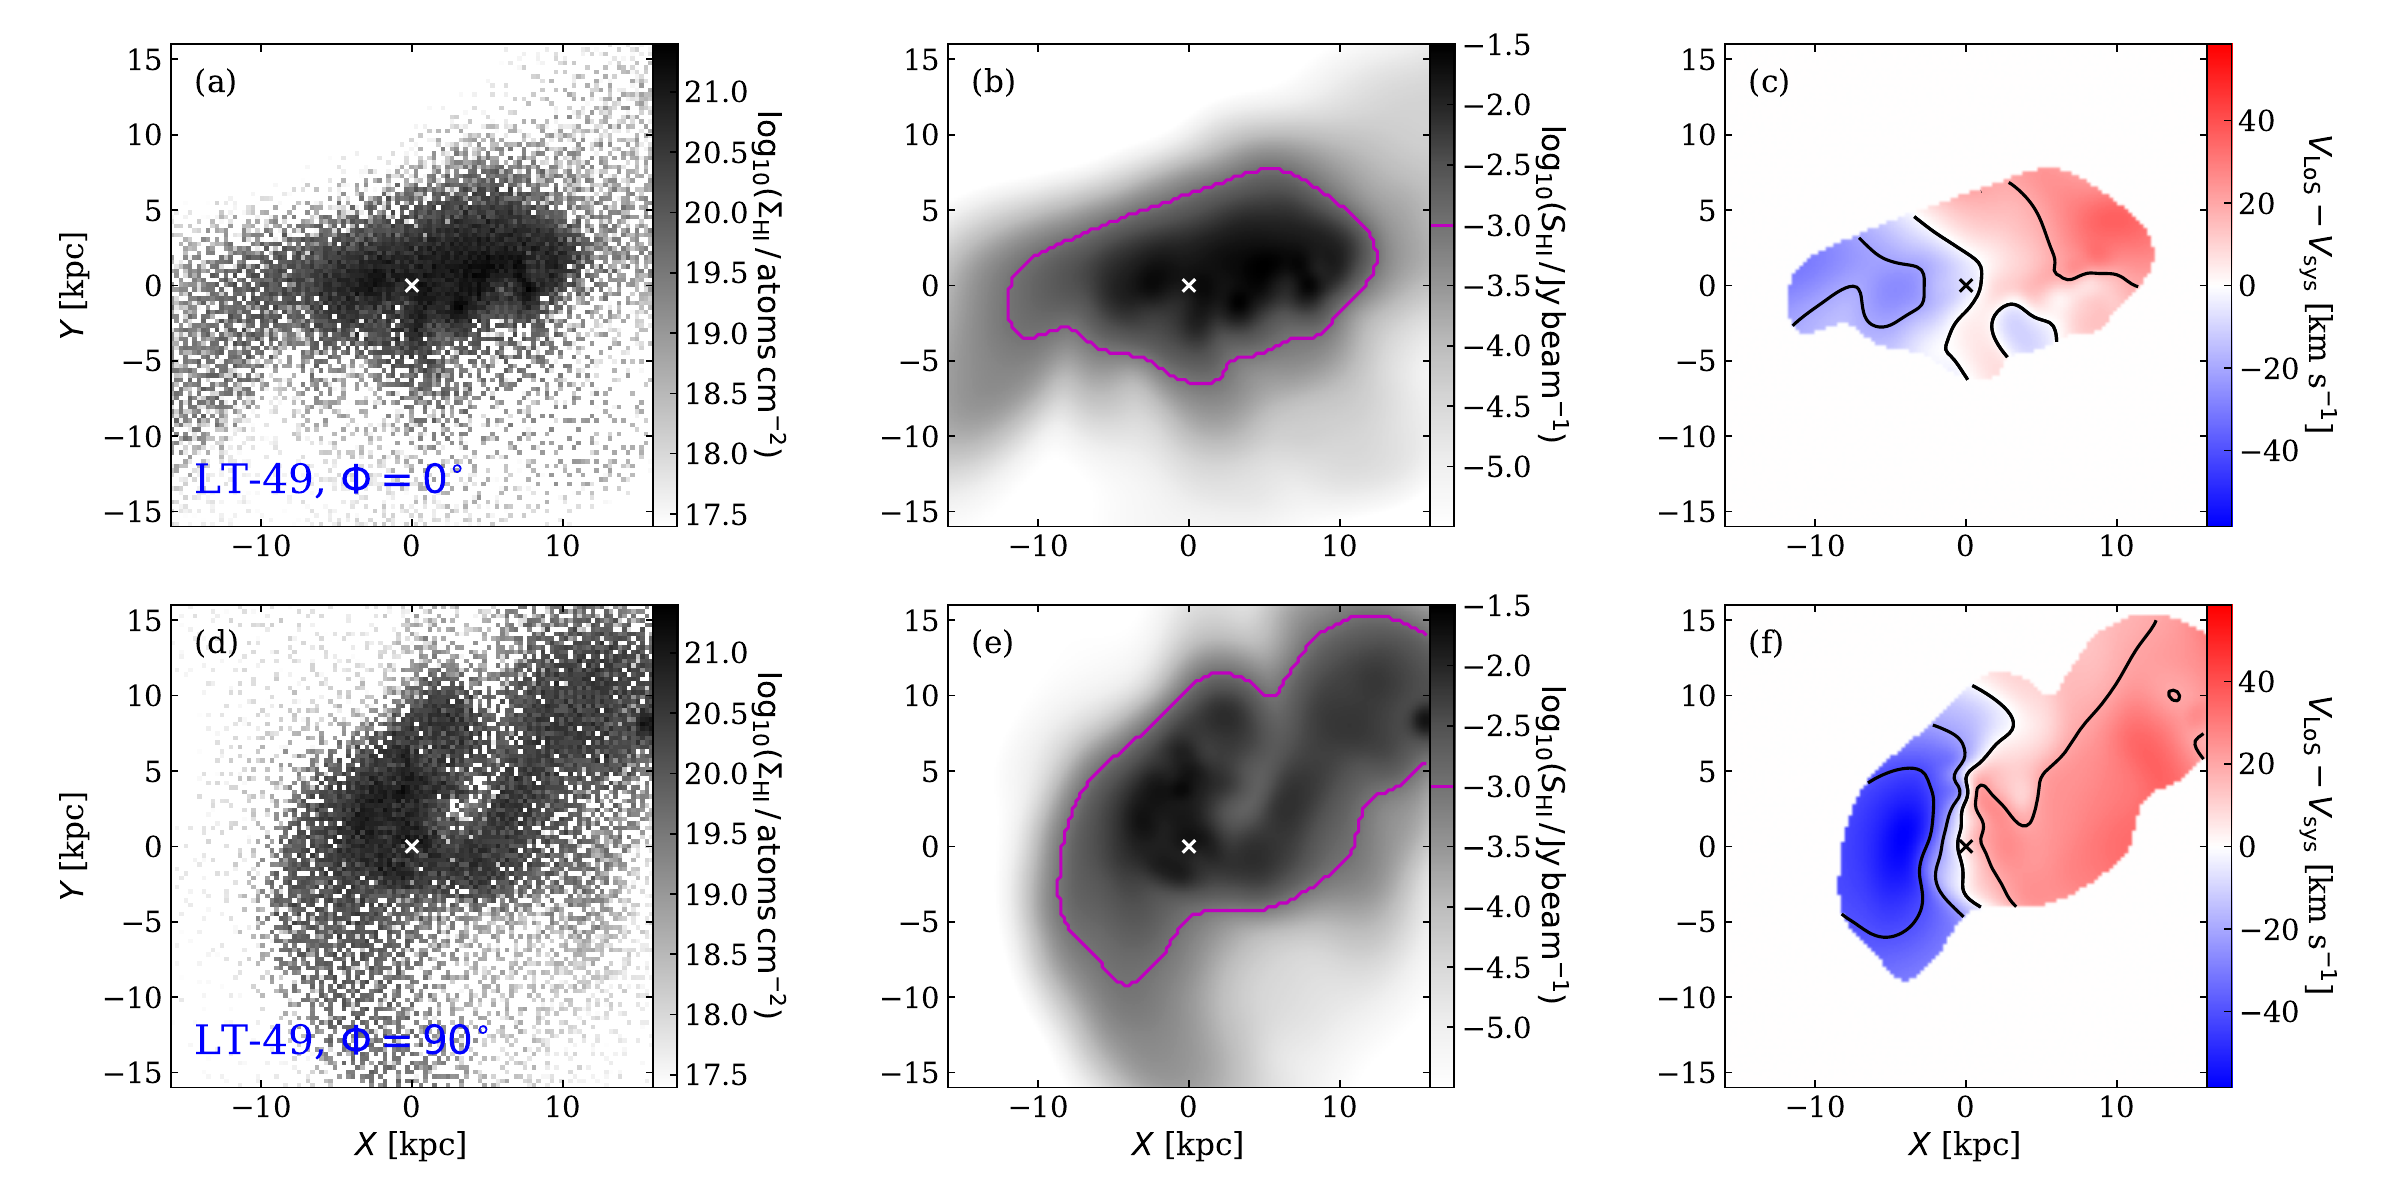}
\includegraphics[width=\textwidth]{../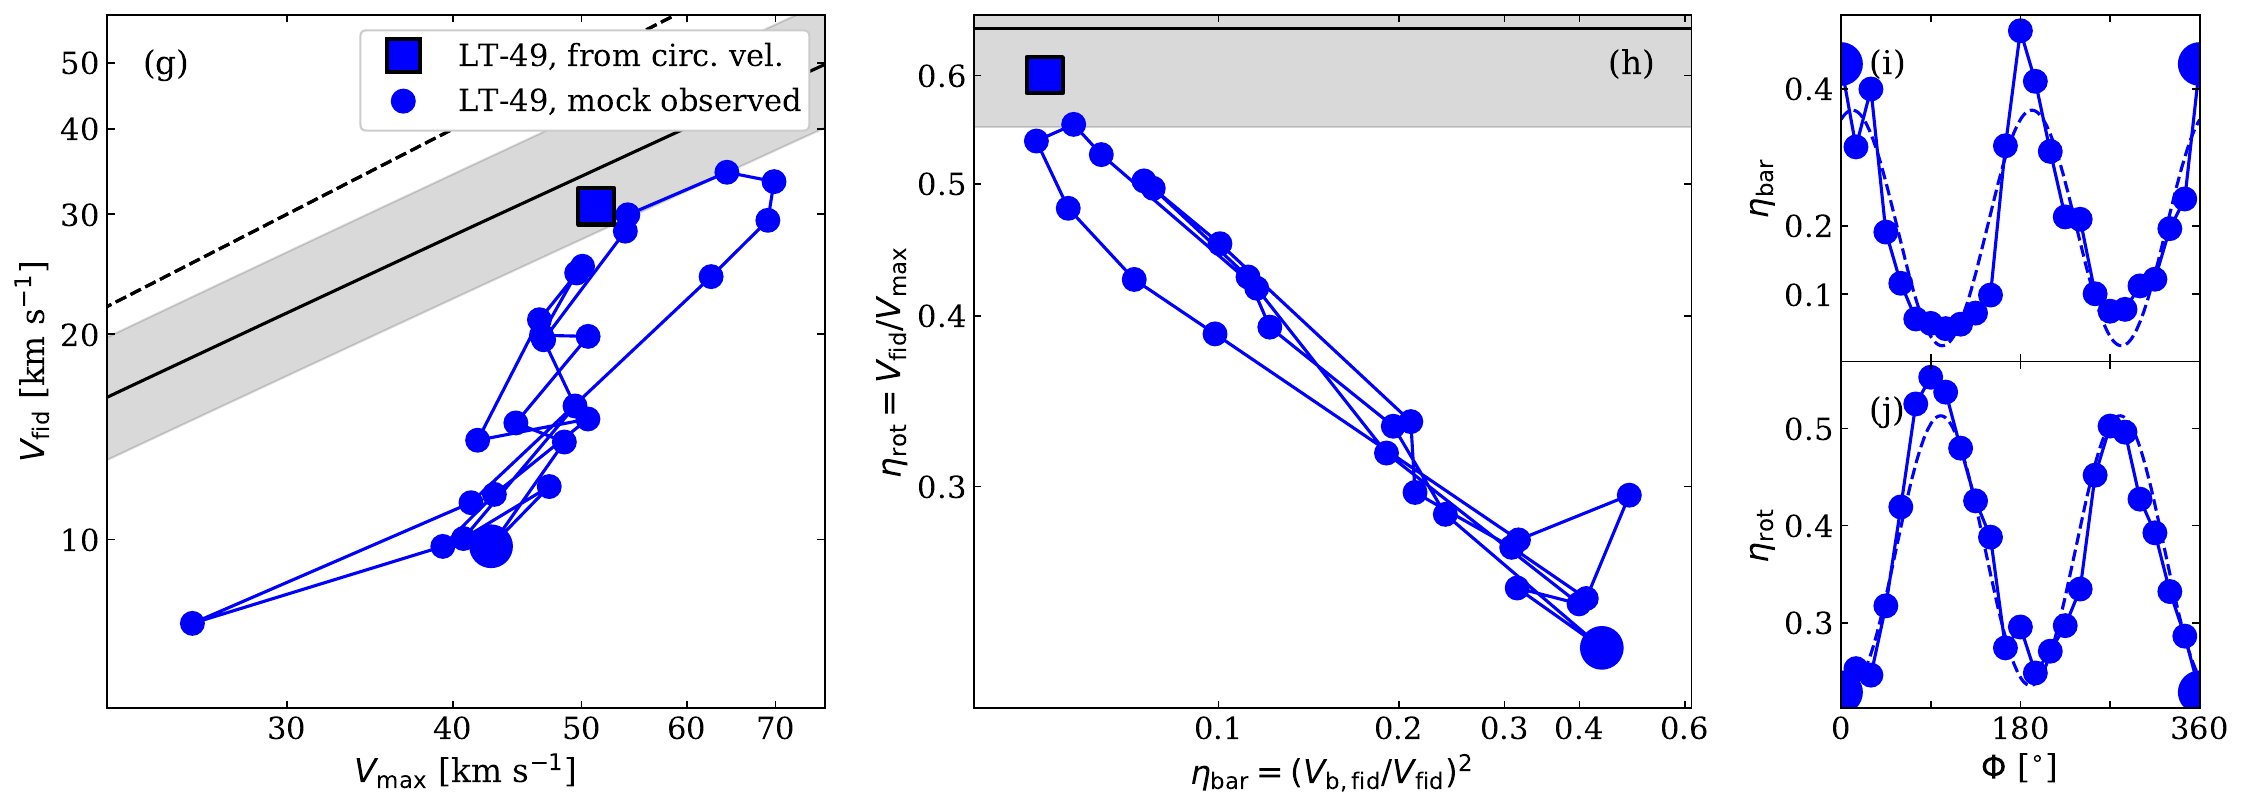}
\end{minipage}
\begin{minipage}{.4\textwidth}
\includegraphics[width=\textwidth]{../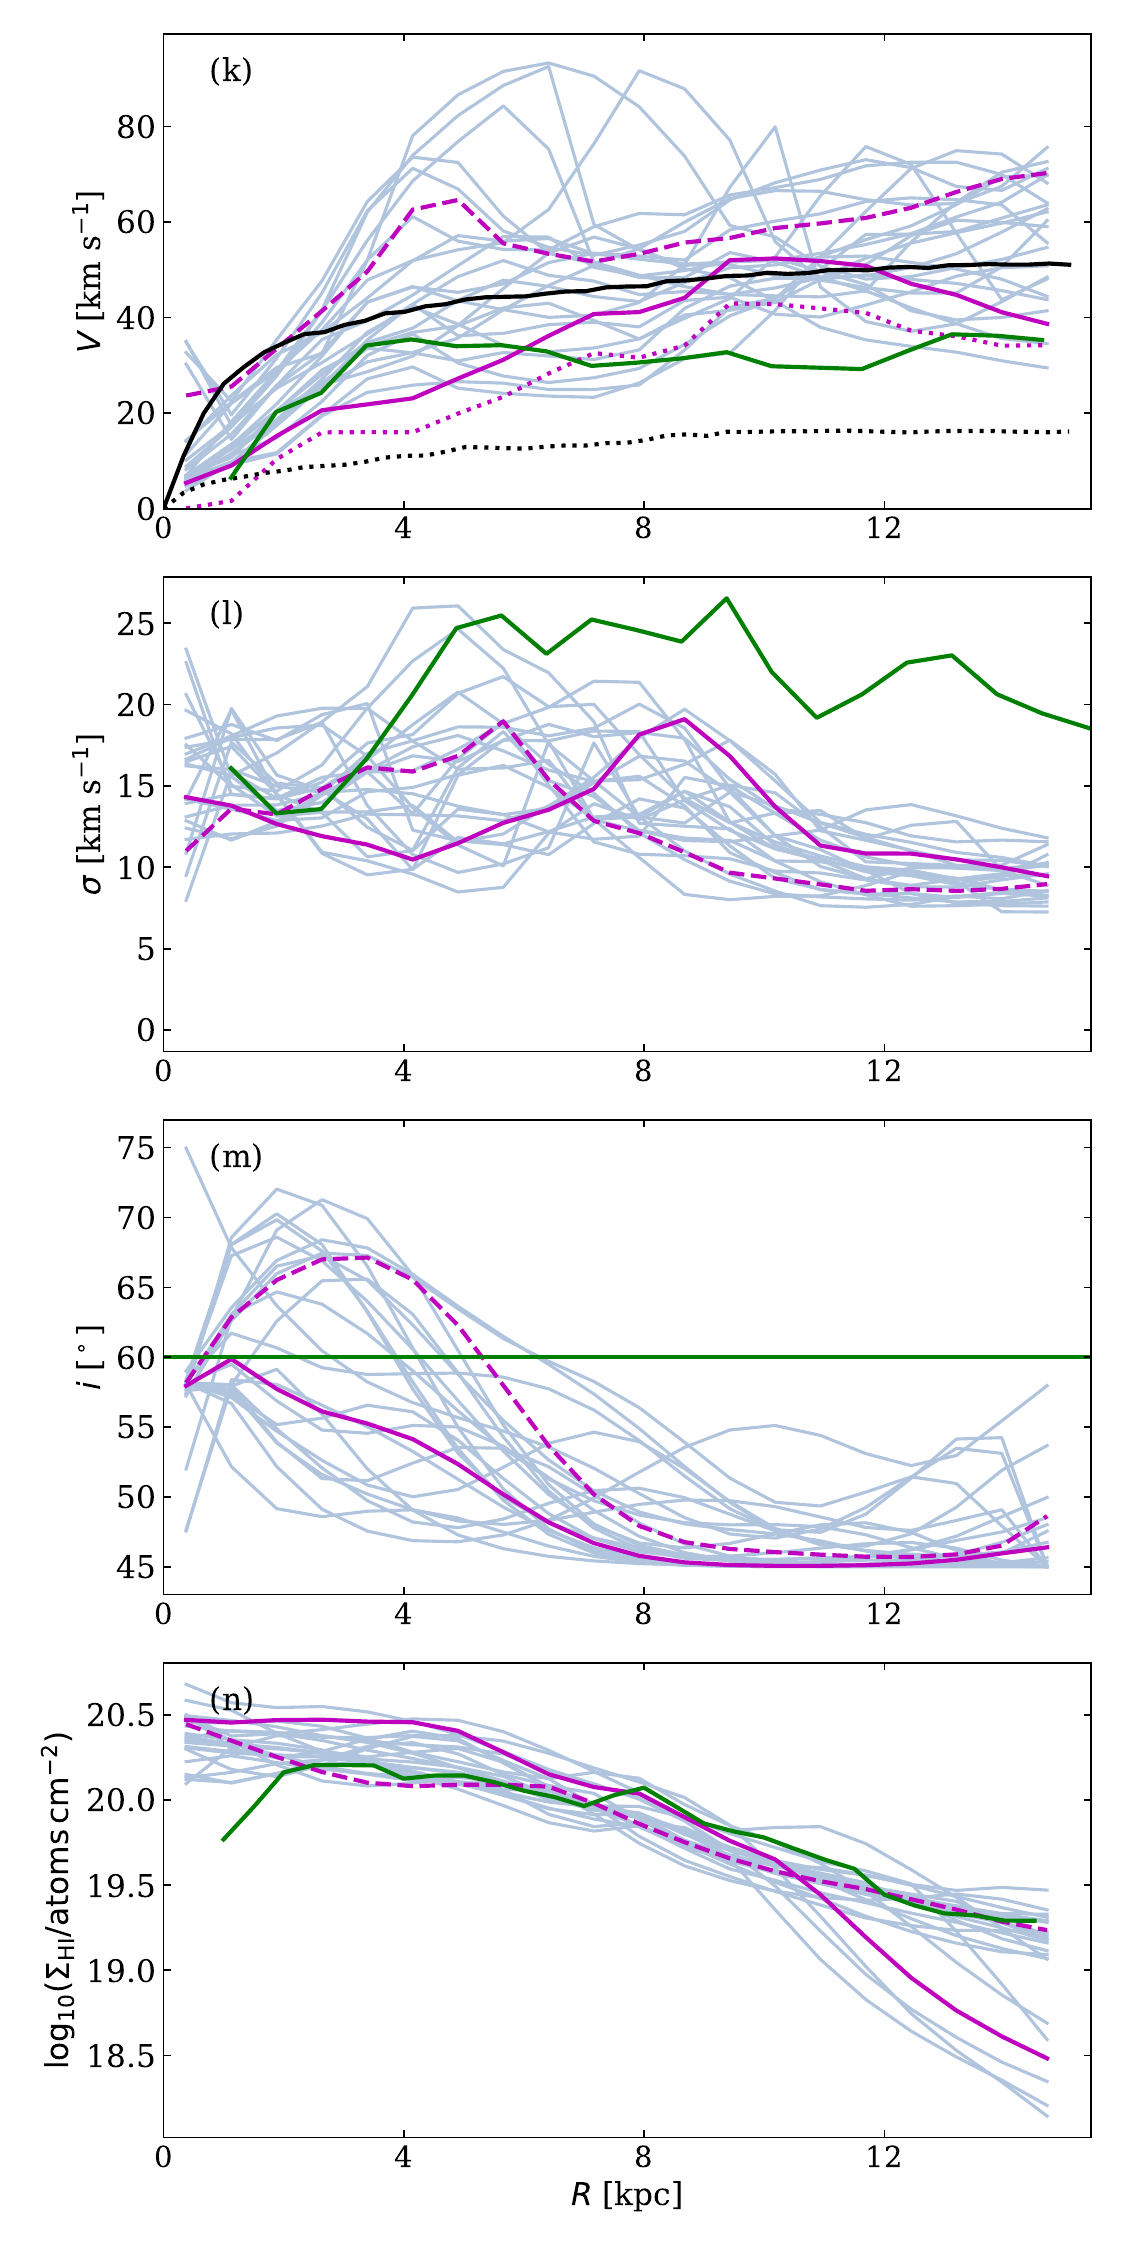}
\end{minipage}
\caption{A set of summary figures for galaxy LT-49, excluded from kinematic analysis. These include example moment maps for two orientations (panels (a)--(f); similar to Fig.~\ref{fig:visualisations}), a summary of the parameters $V_\mathrm{fid}$, $V_\mathrm{max}$, $\eta_\mathrm{rot}$, and $\eta_\mathrm{bar}$ (panels (g)--(j); similar to Fig.~\ref{fig:loops}), and a summary of the rotation curve analysis from $24$ viewing angles (panels (k)--(n); similar to Fig.~\ref{fig:rot_curves}). See description of Appendix~\ref{app:supplementary} for details.}
\label{fig:S42}
\end{figure}
\clearpage

\begin{figure}
\begin{minipage}{.9\textwidth}
\includegraphics[width=\textwidth]{../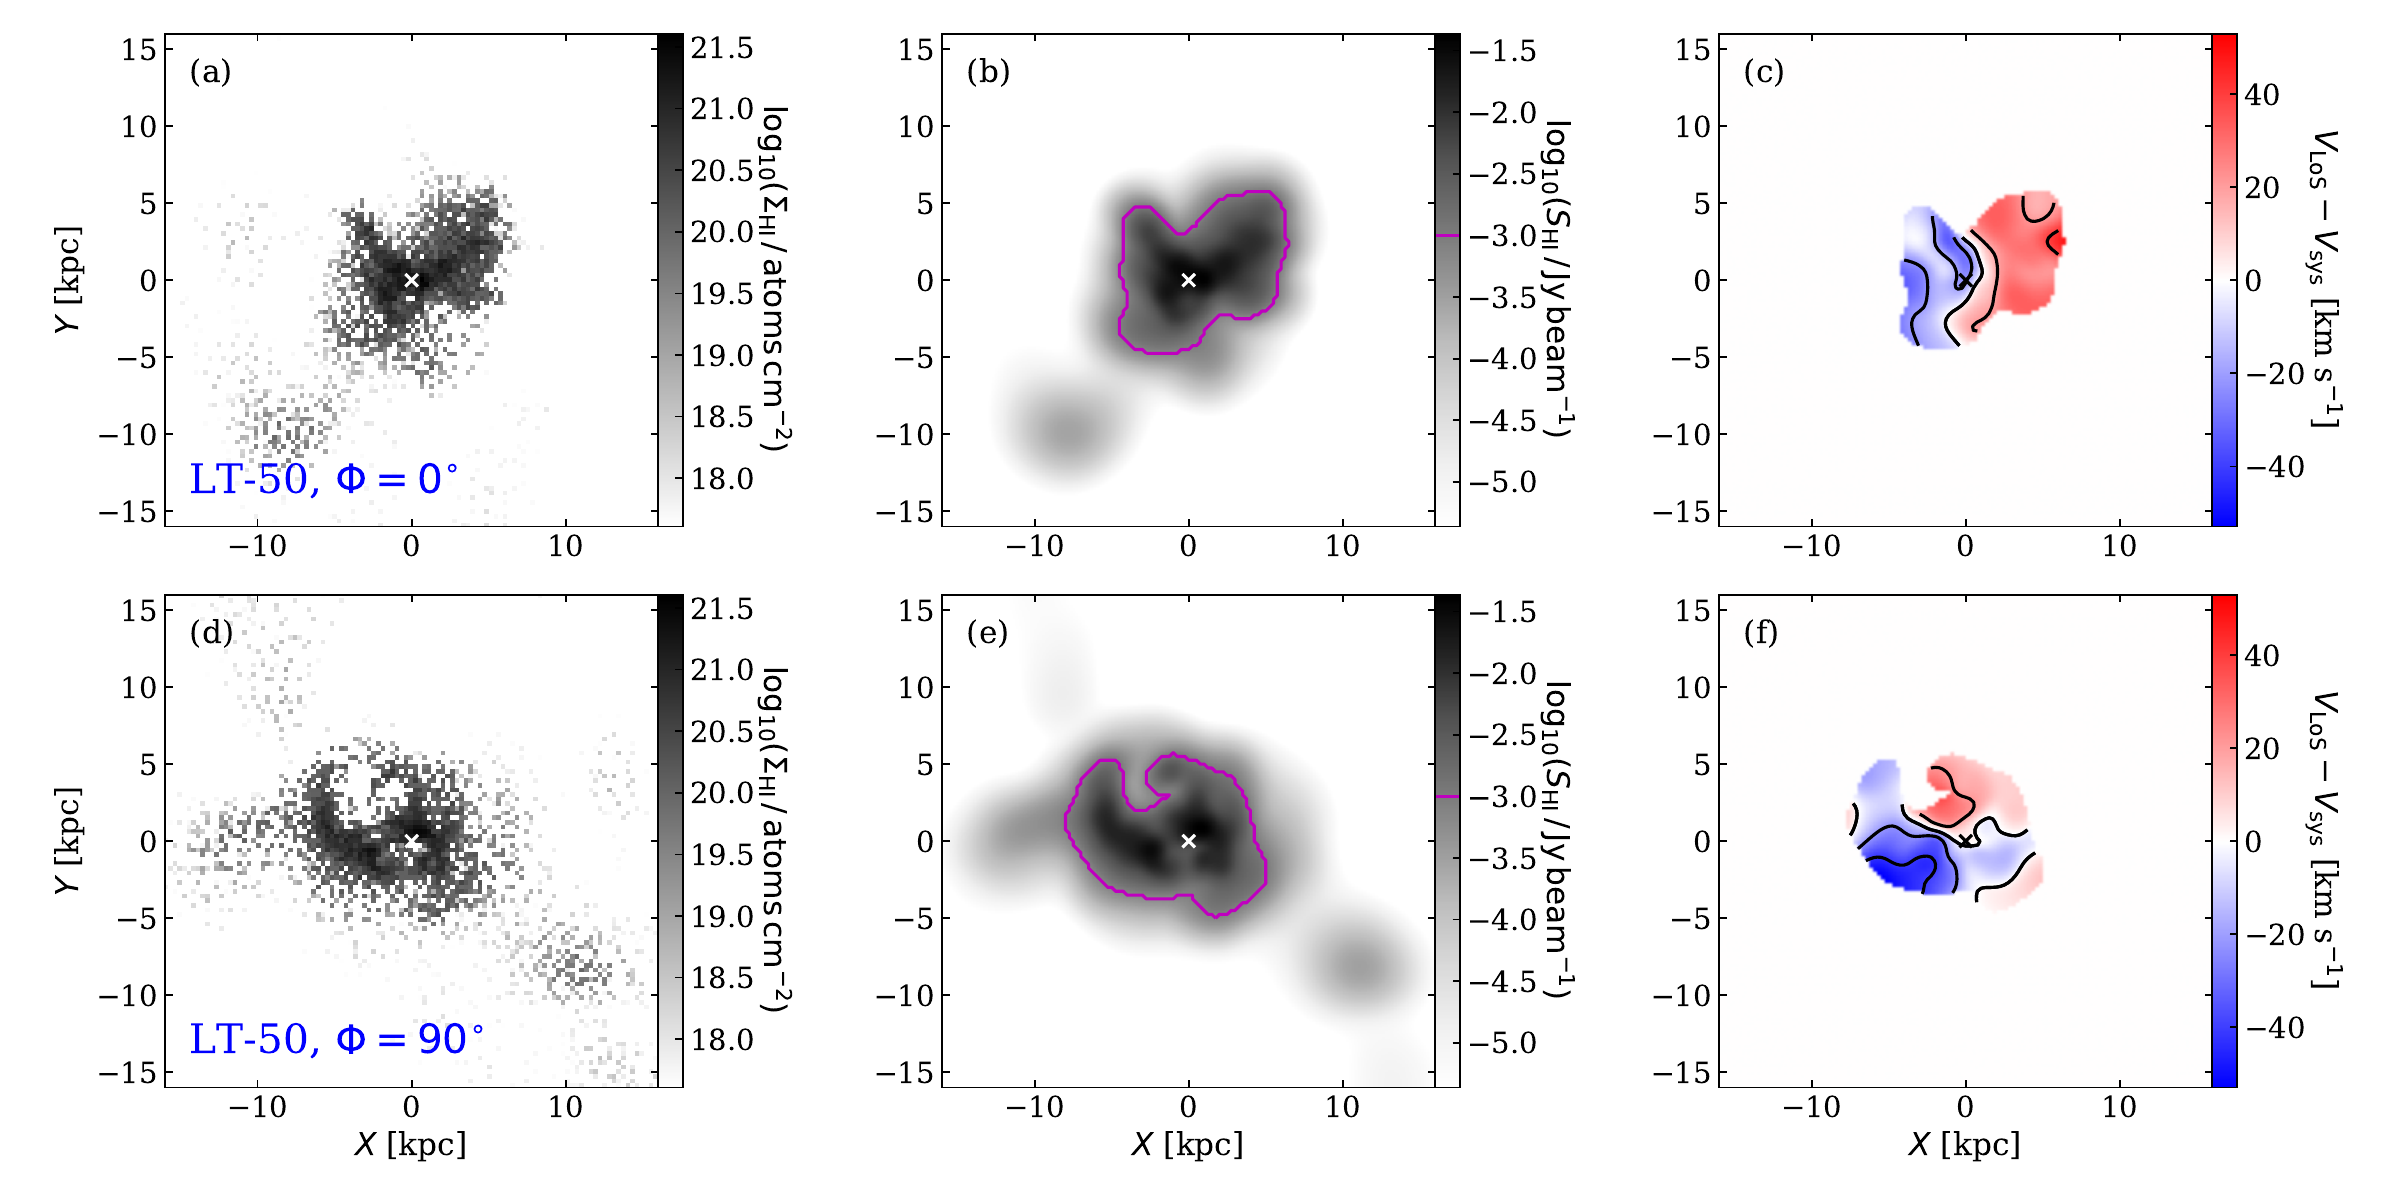}
\includegraphics[width=\textwidth]{../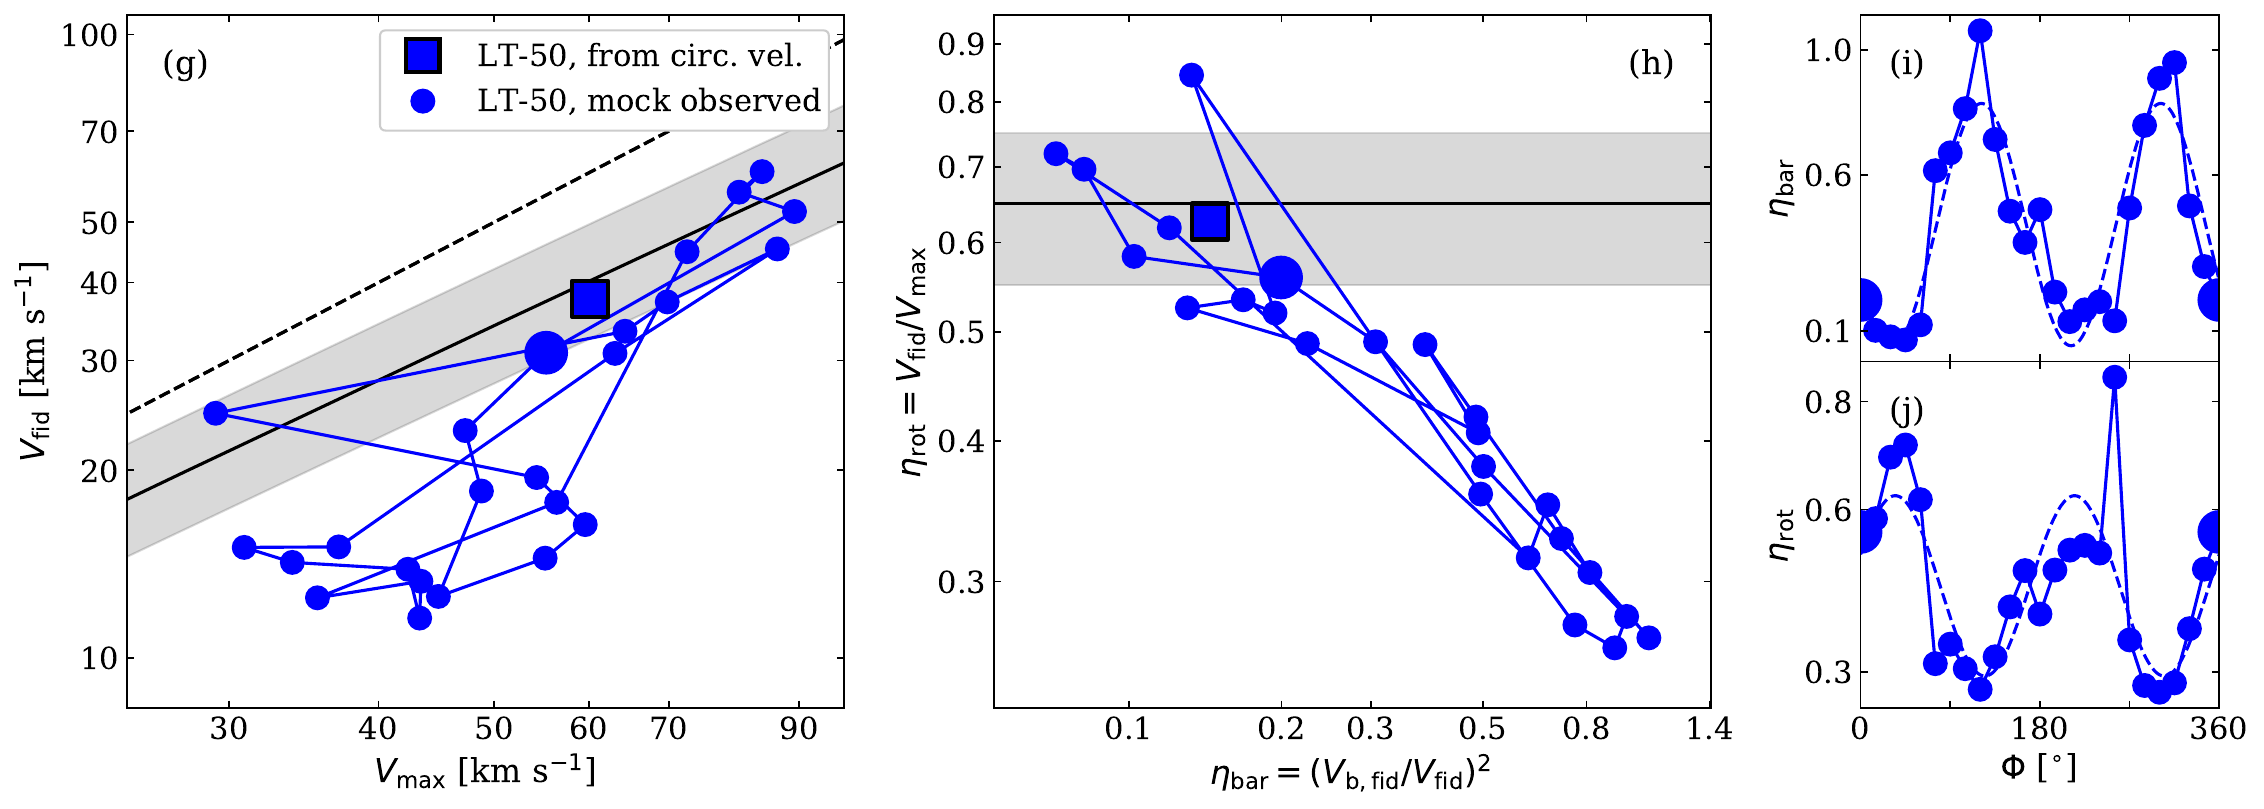}
\end{minipage}
\begin{minipage}{.4\textwidth}
\includegraphics[width=\textwidth]{../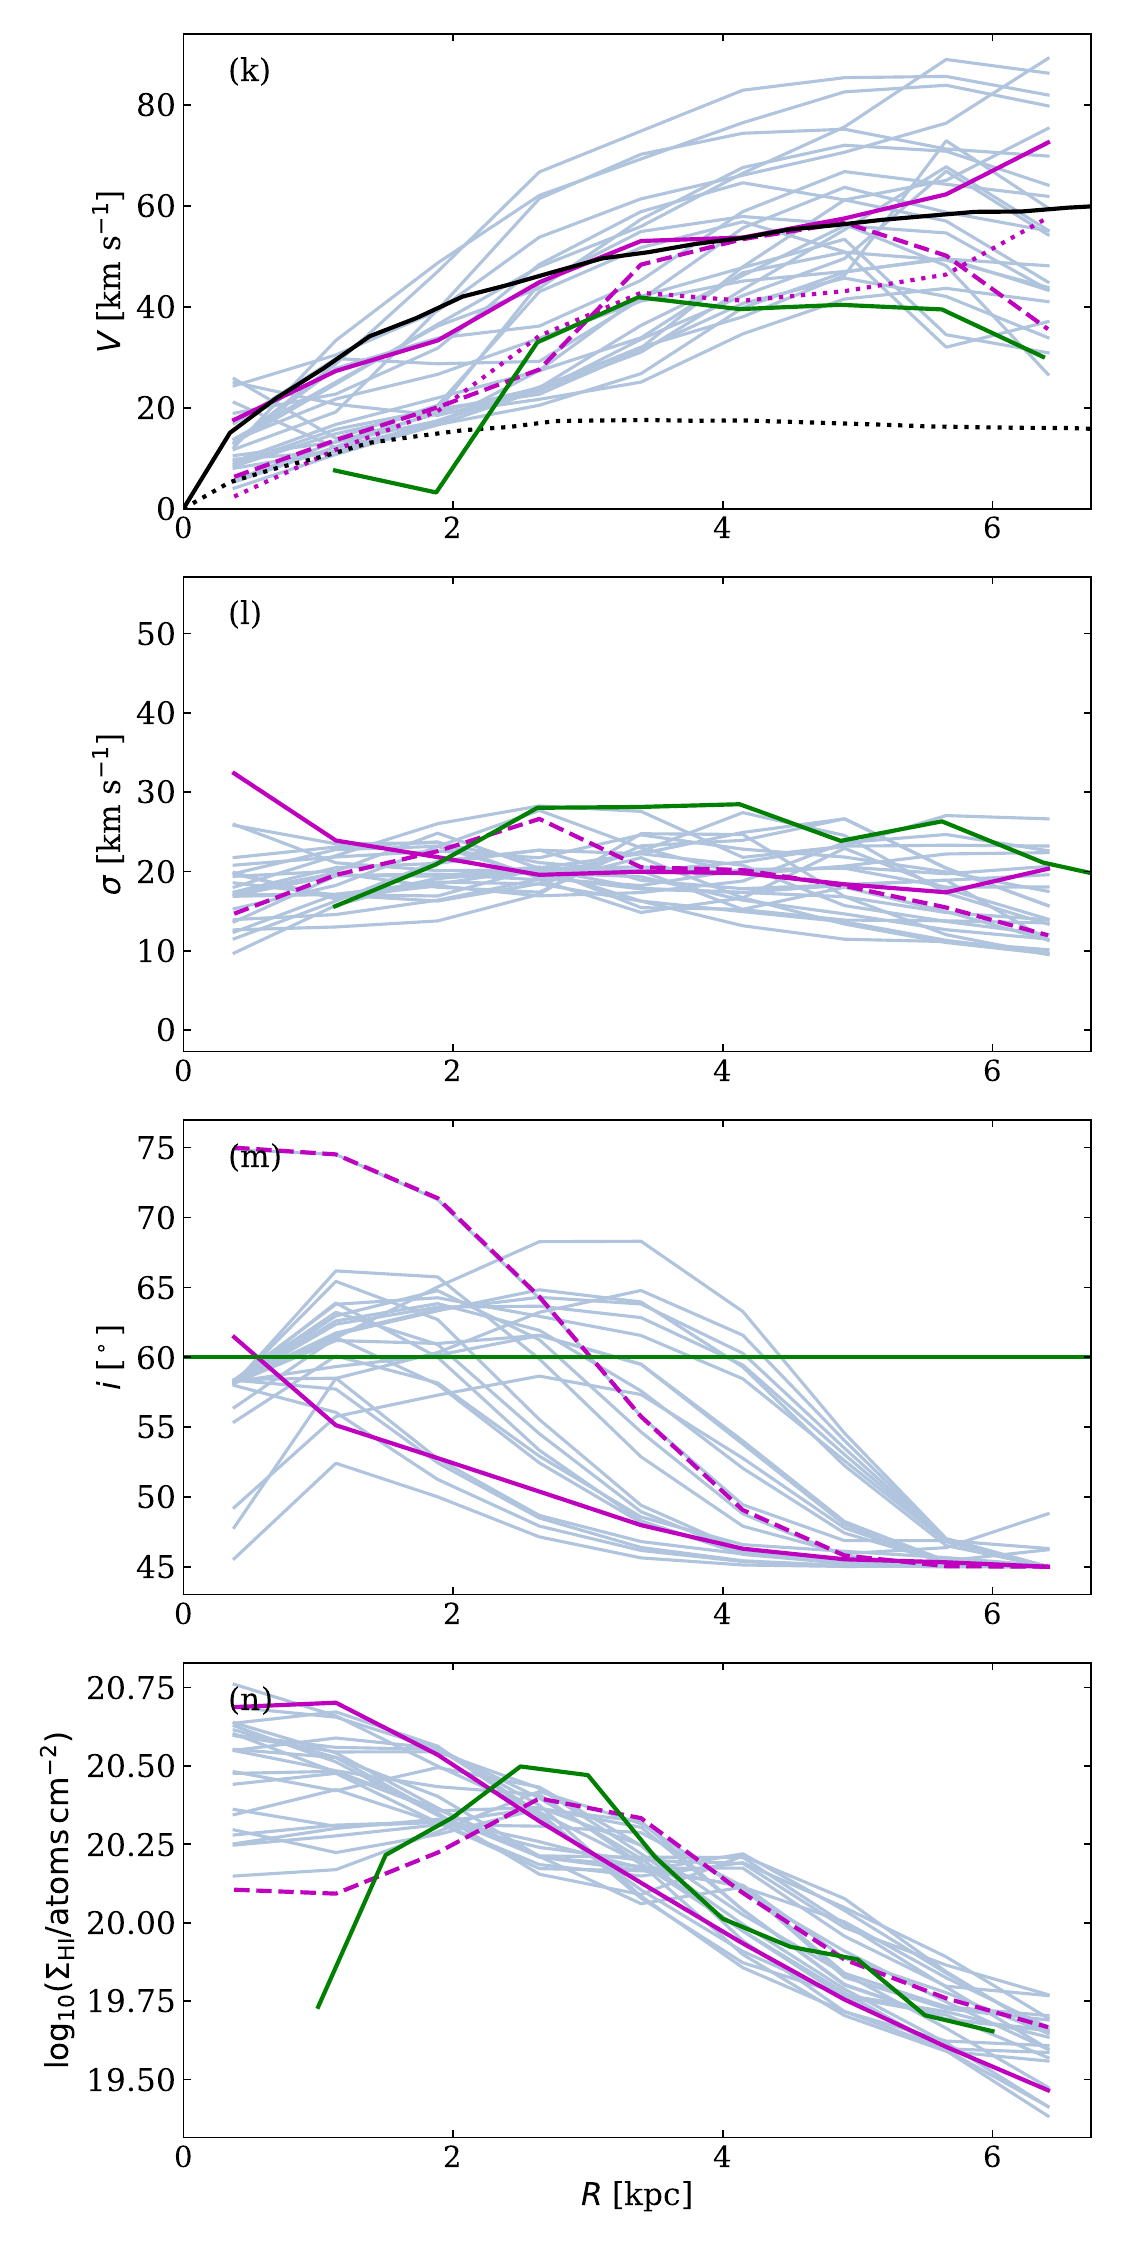}
\end{minipage}
\caption{A set of summary figures for galaxy LT-50, excluded from kinematic analysis. These include example moment maps for two orientations (panels (a)--(f); similar to Fig.~\ref{fig:visualisations}), a summary of the parameters $V_\mathrm{fid}$, $V_\mathrm{max}$, $\eta_\mathrm{rot}$, and $\eta_\mathrm{bar}$ (panels (g)--(j); similar to Fig.~\ref{fig:loops}), and a summary of the rotation curve analysis from $24$ viewing angles (panels (k)--(n); similar to Fig.~\ref{fig:rot_curves}). See description of Appendix~\ref{app:supplementary} for details.}
\label{fig:S43}
\end{figure}
\clearpage

\begin{figure}
\begin{minipage}{.9\textwidth}
\includegraphics[width=\textwidth]{../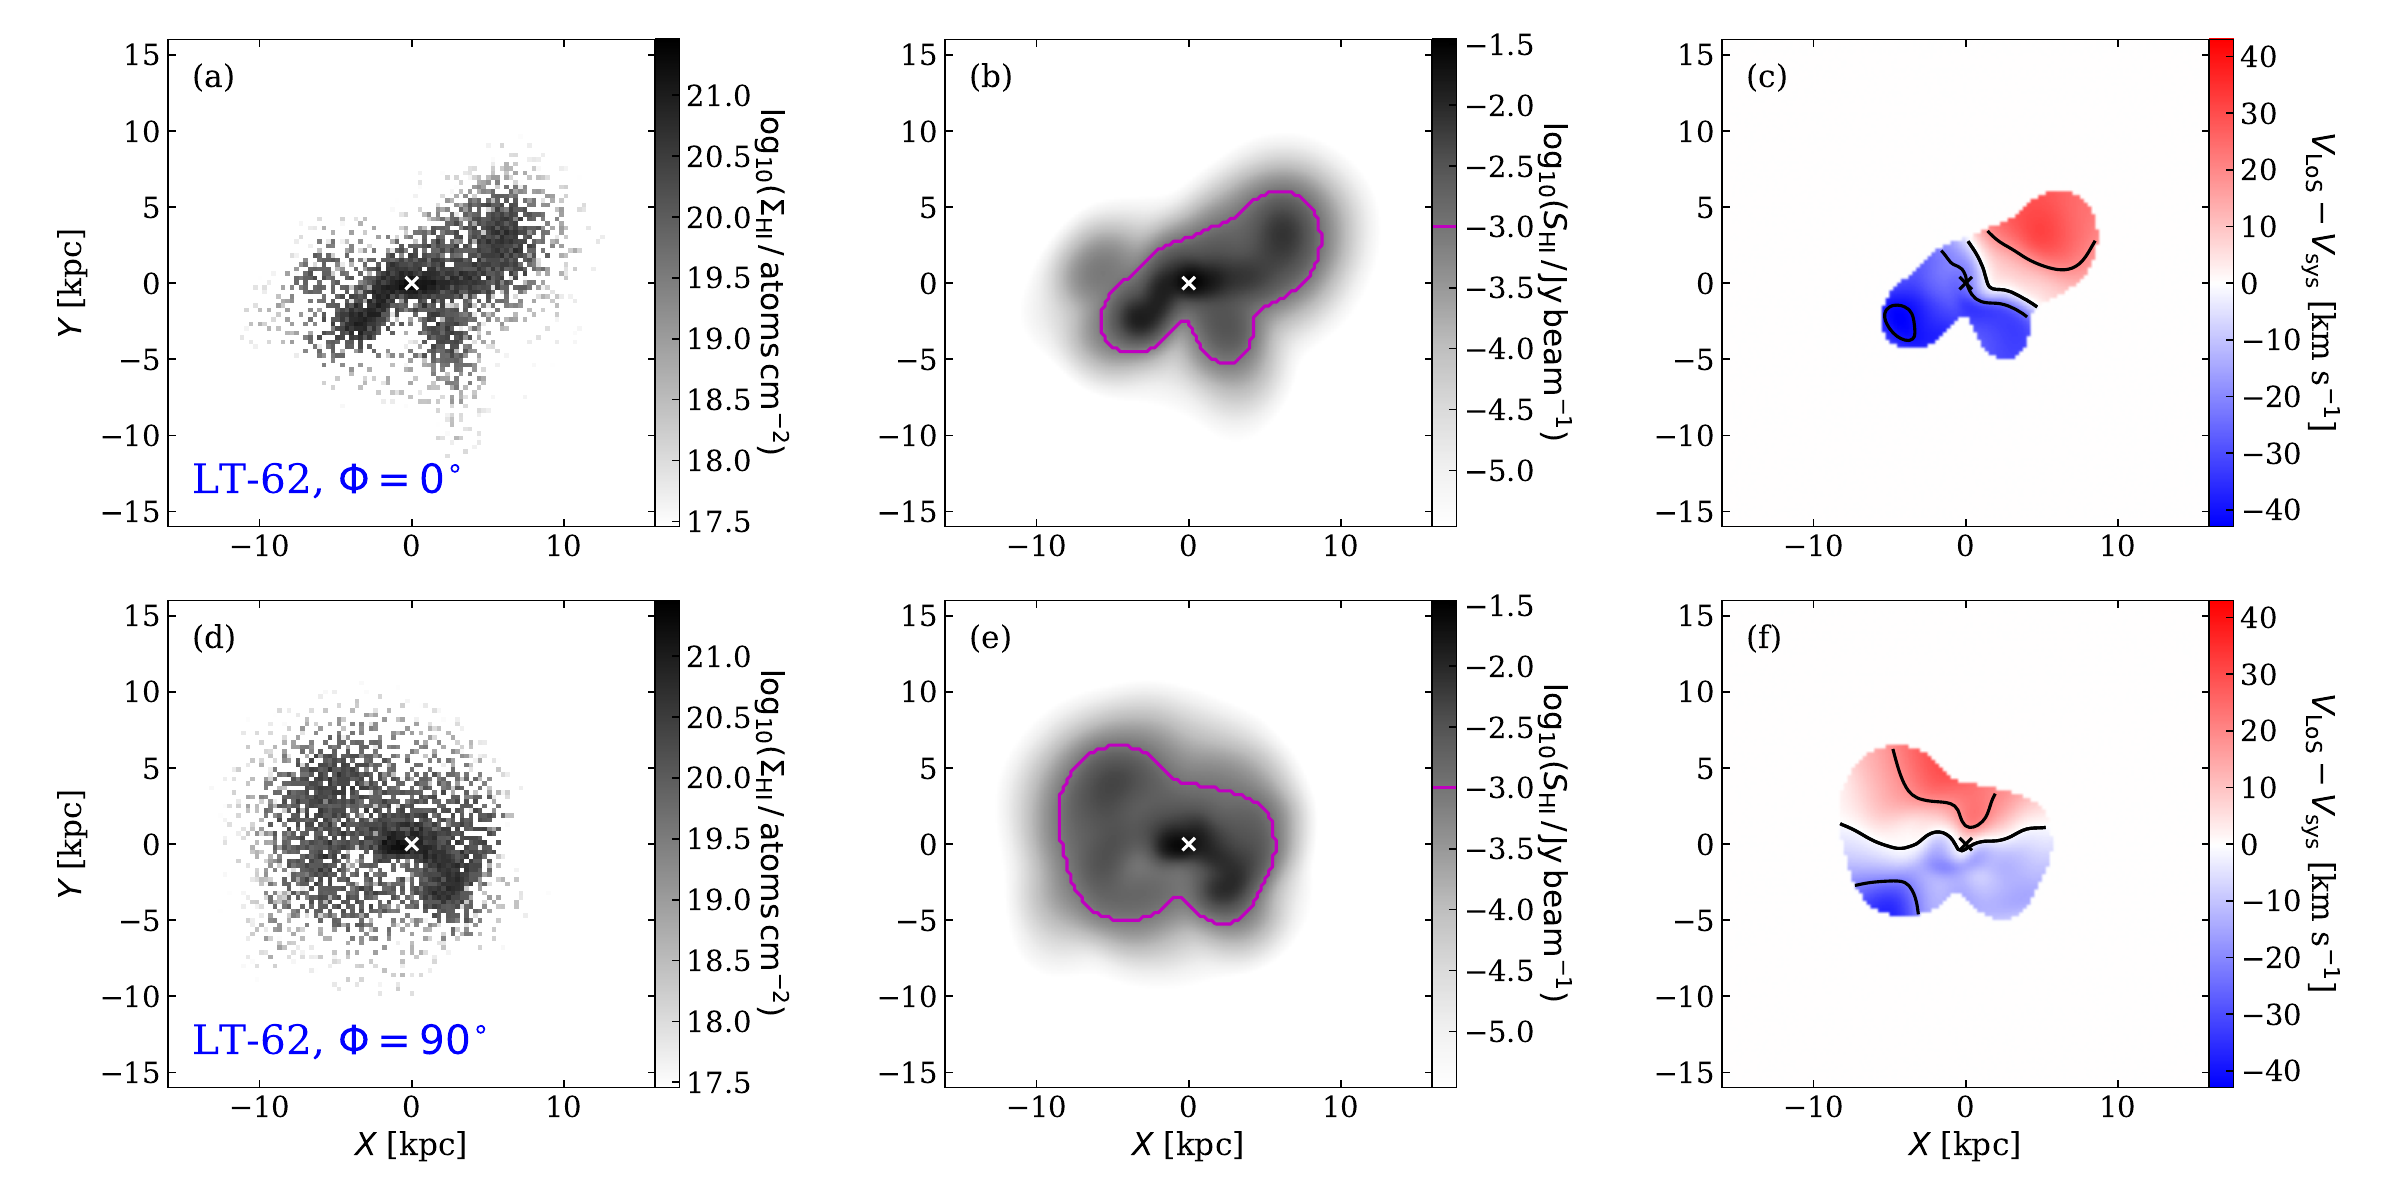}
\includegraphics[width=\textwidth]{../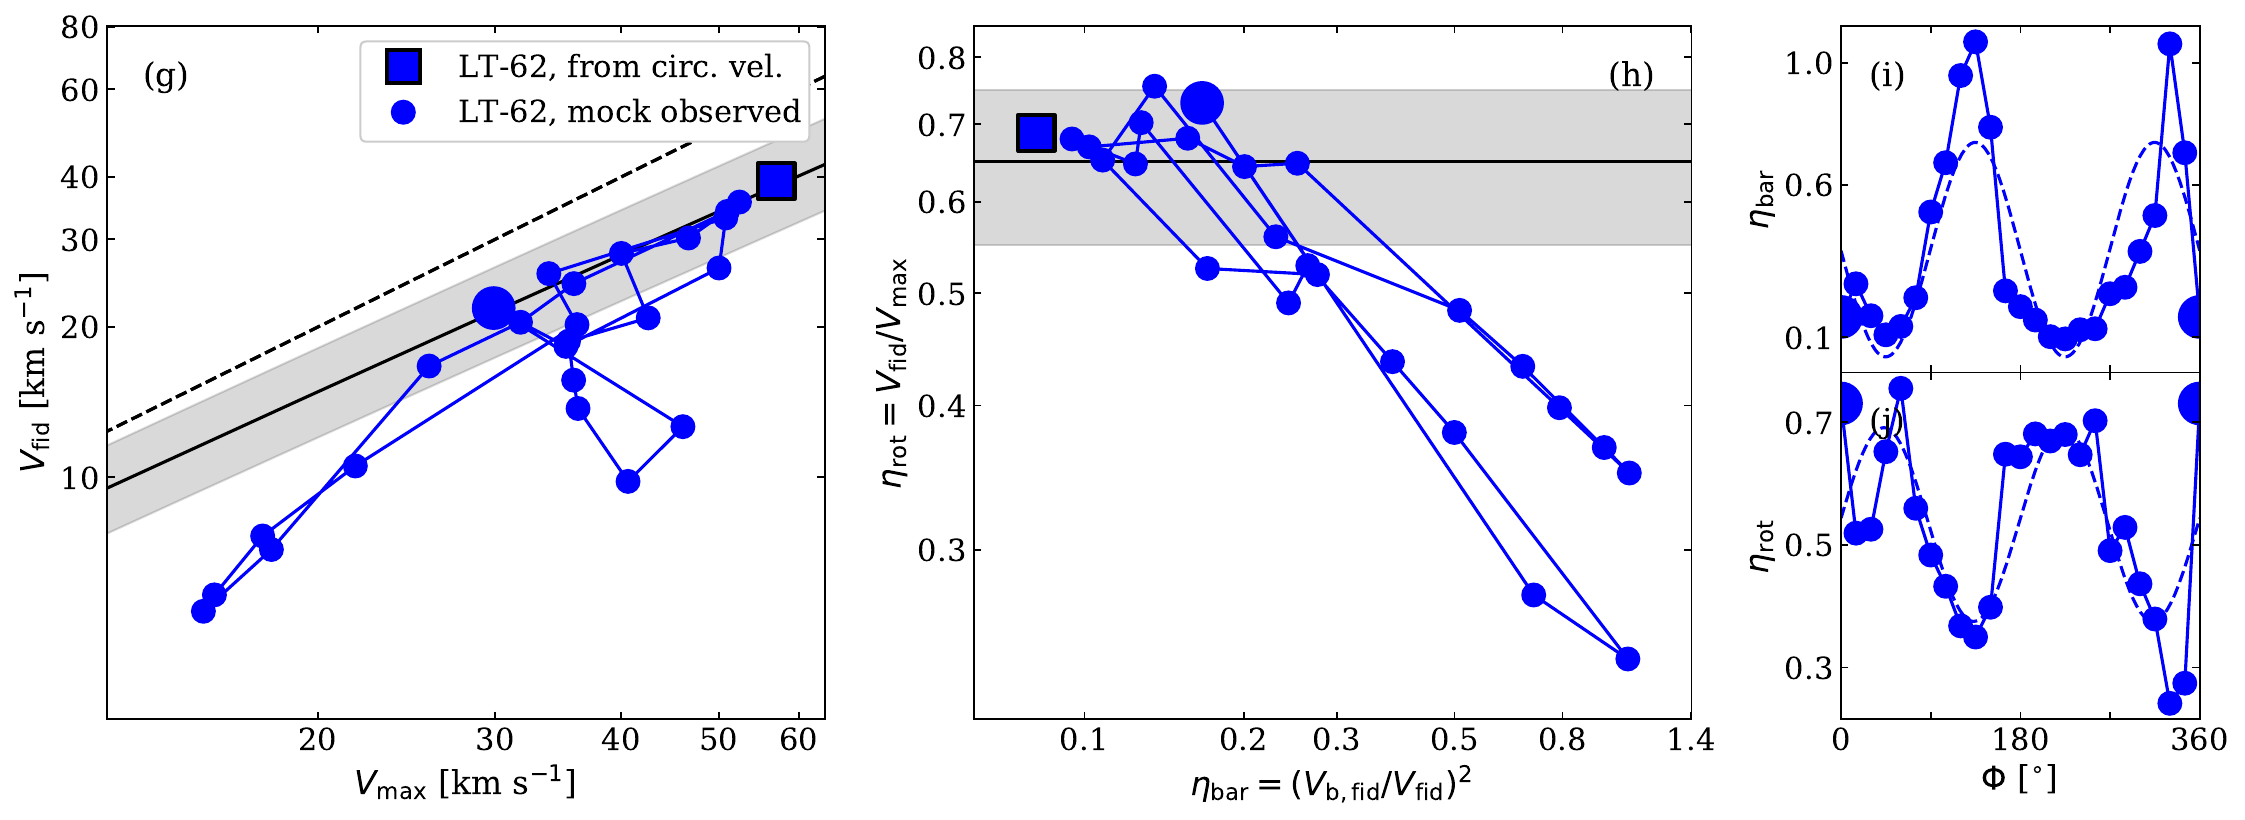}
\end{minipage}
\begin{minipage}{.4\textwidth}
\includegraphics[width=\textwidth]{../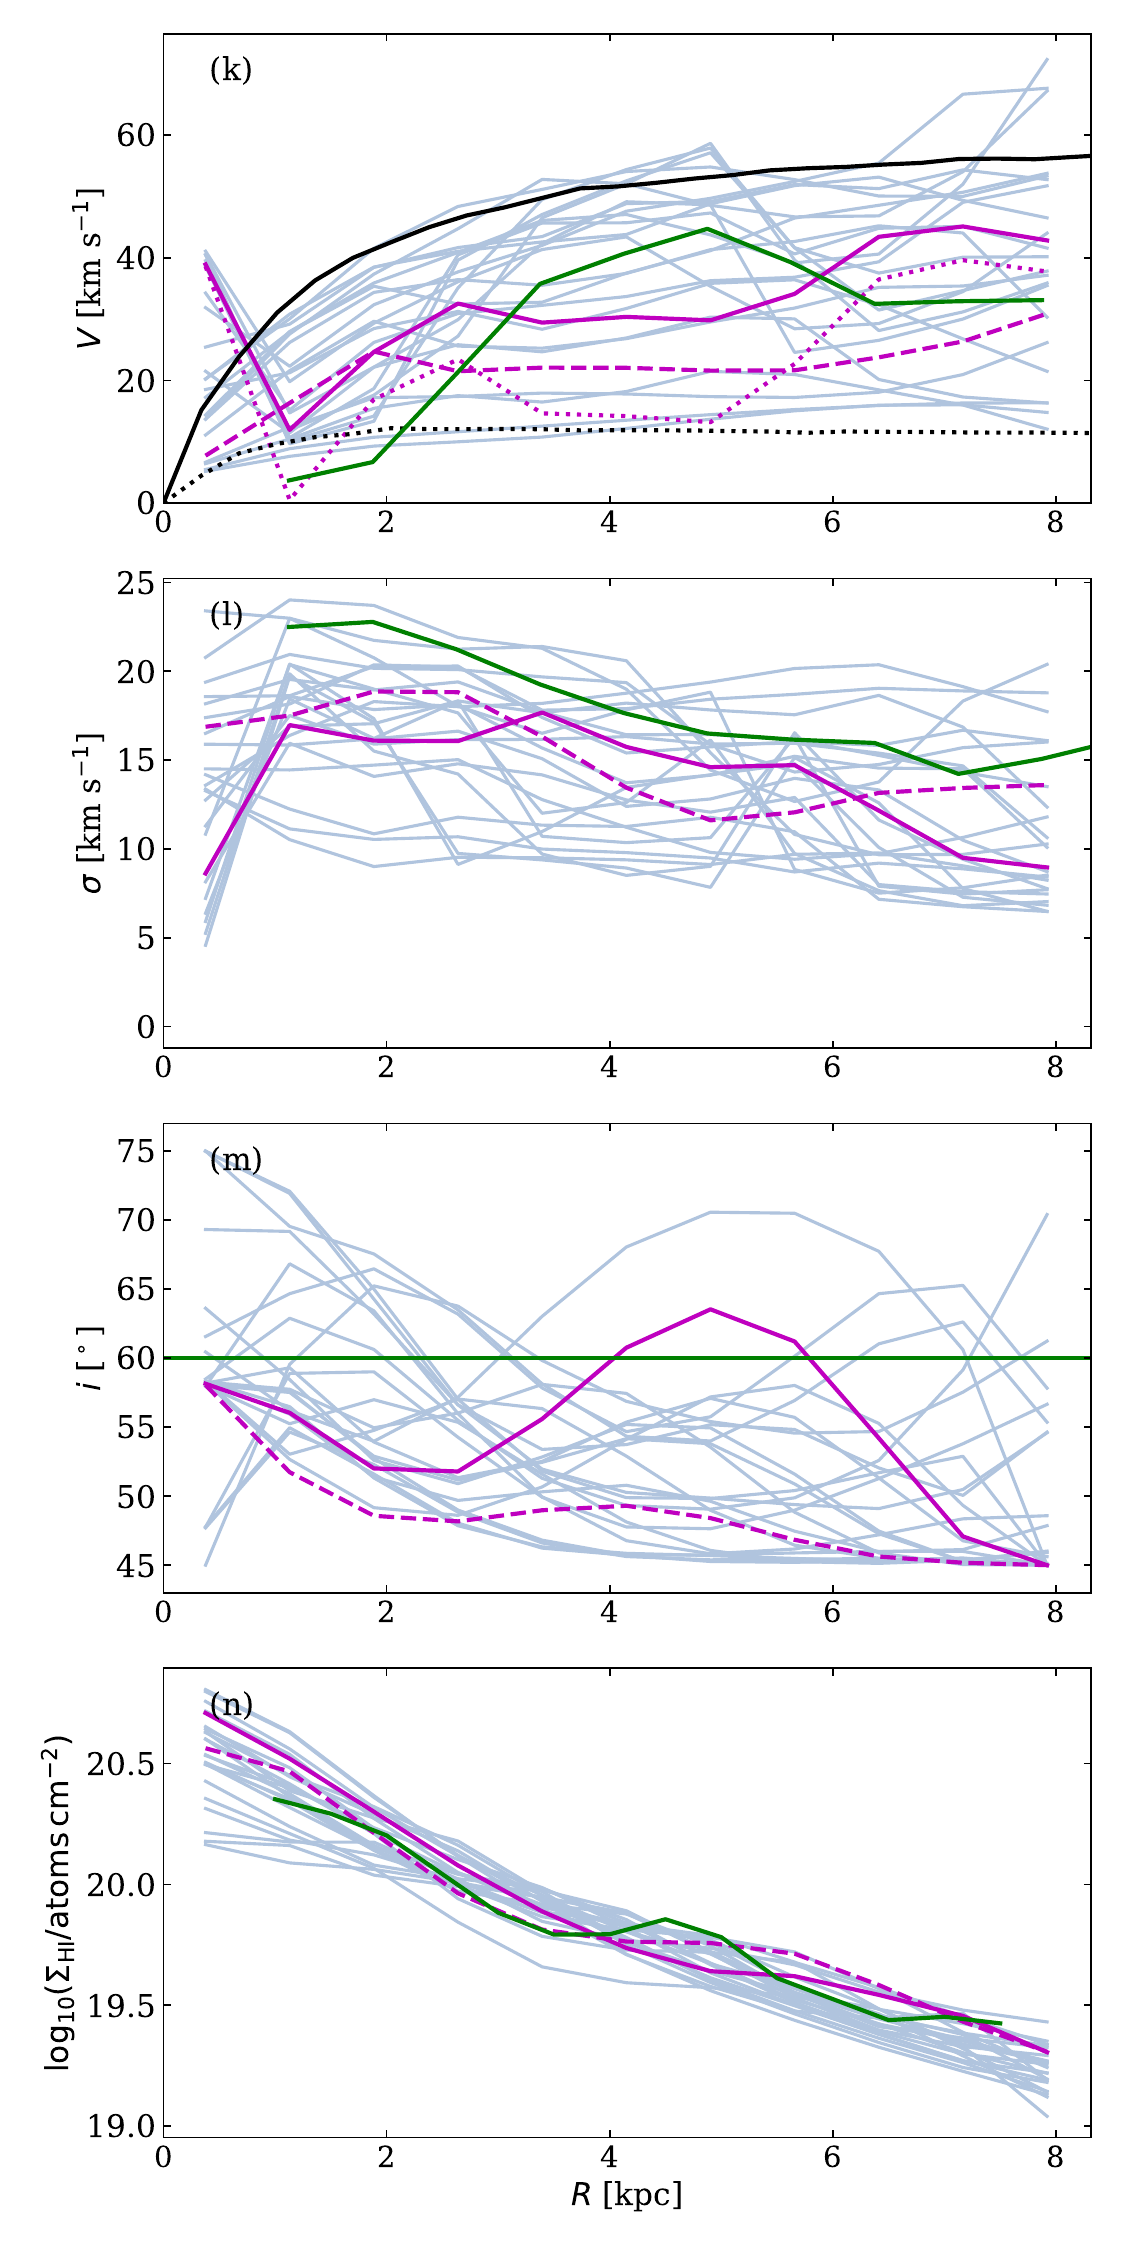}
\end{minipage}
\caption{A set of summary figures for galaxy LT-62, excluded from kinematic analysis. These include example moment maps for two orientations (panels (a)--(f); similar to Fig.~\ref{fig:visualisations}), a summary of the parameters $V_\mathrm{fid}$, $V_\mathrm{max}$, $\eta_\mathrm{rot}$, and $\eta_\mathrm{bar}$ (panels (g)--(j); similar to Fig.~\ref{fig:loops}), and a summary of the rotation curve analysis from $24$ viewing angles (panels (k)--(n); similar to Fig.~\ref{fig:rot_curves}). See description of Appendix~\ref{app:supplementary} for details.}
\label{fig:S44}
\end{figure}
\clearpage

\begin{figure}
\begin{minipage}{.9\textwidth}
\includegraphics[width=\textwidth]{../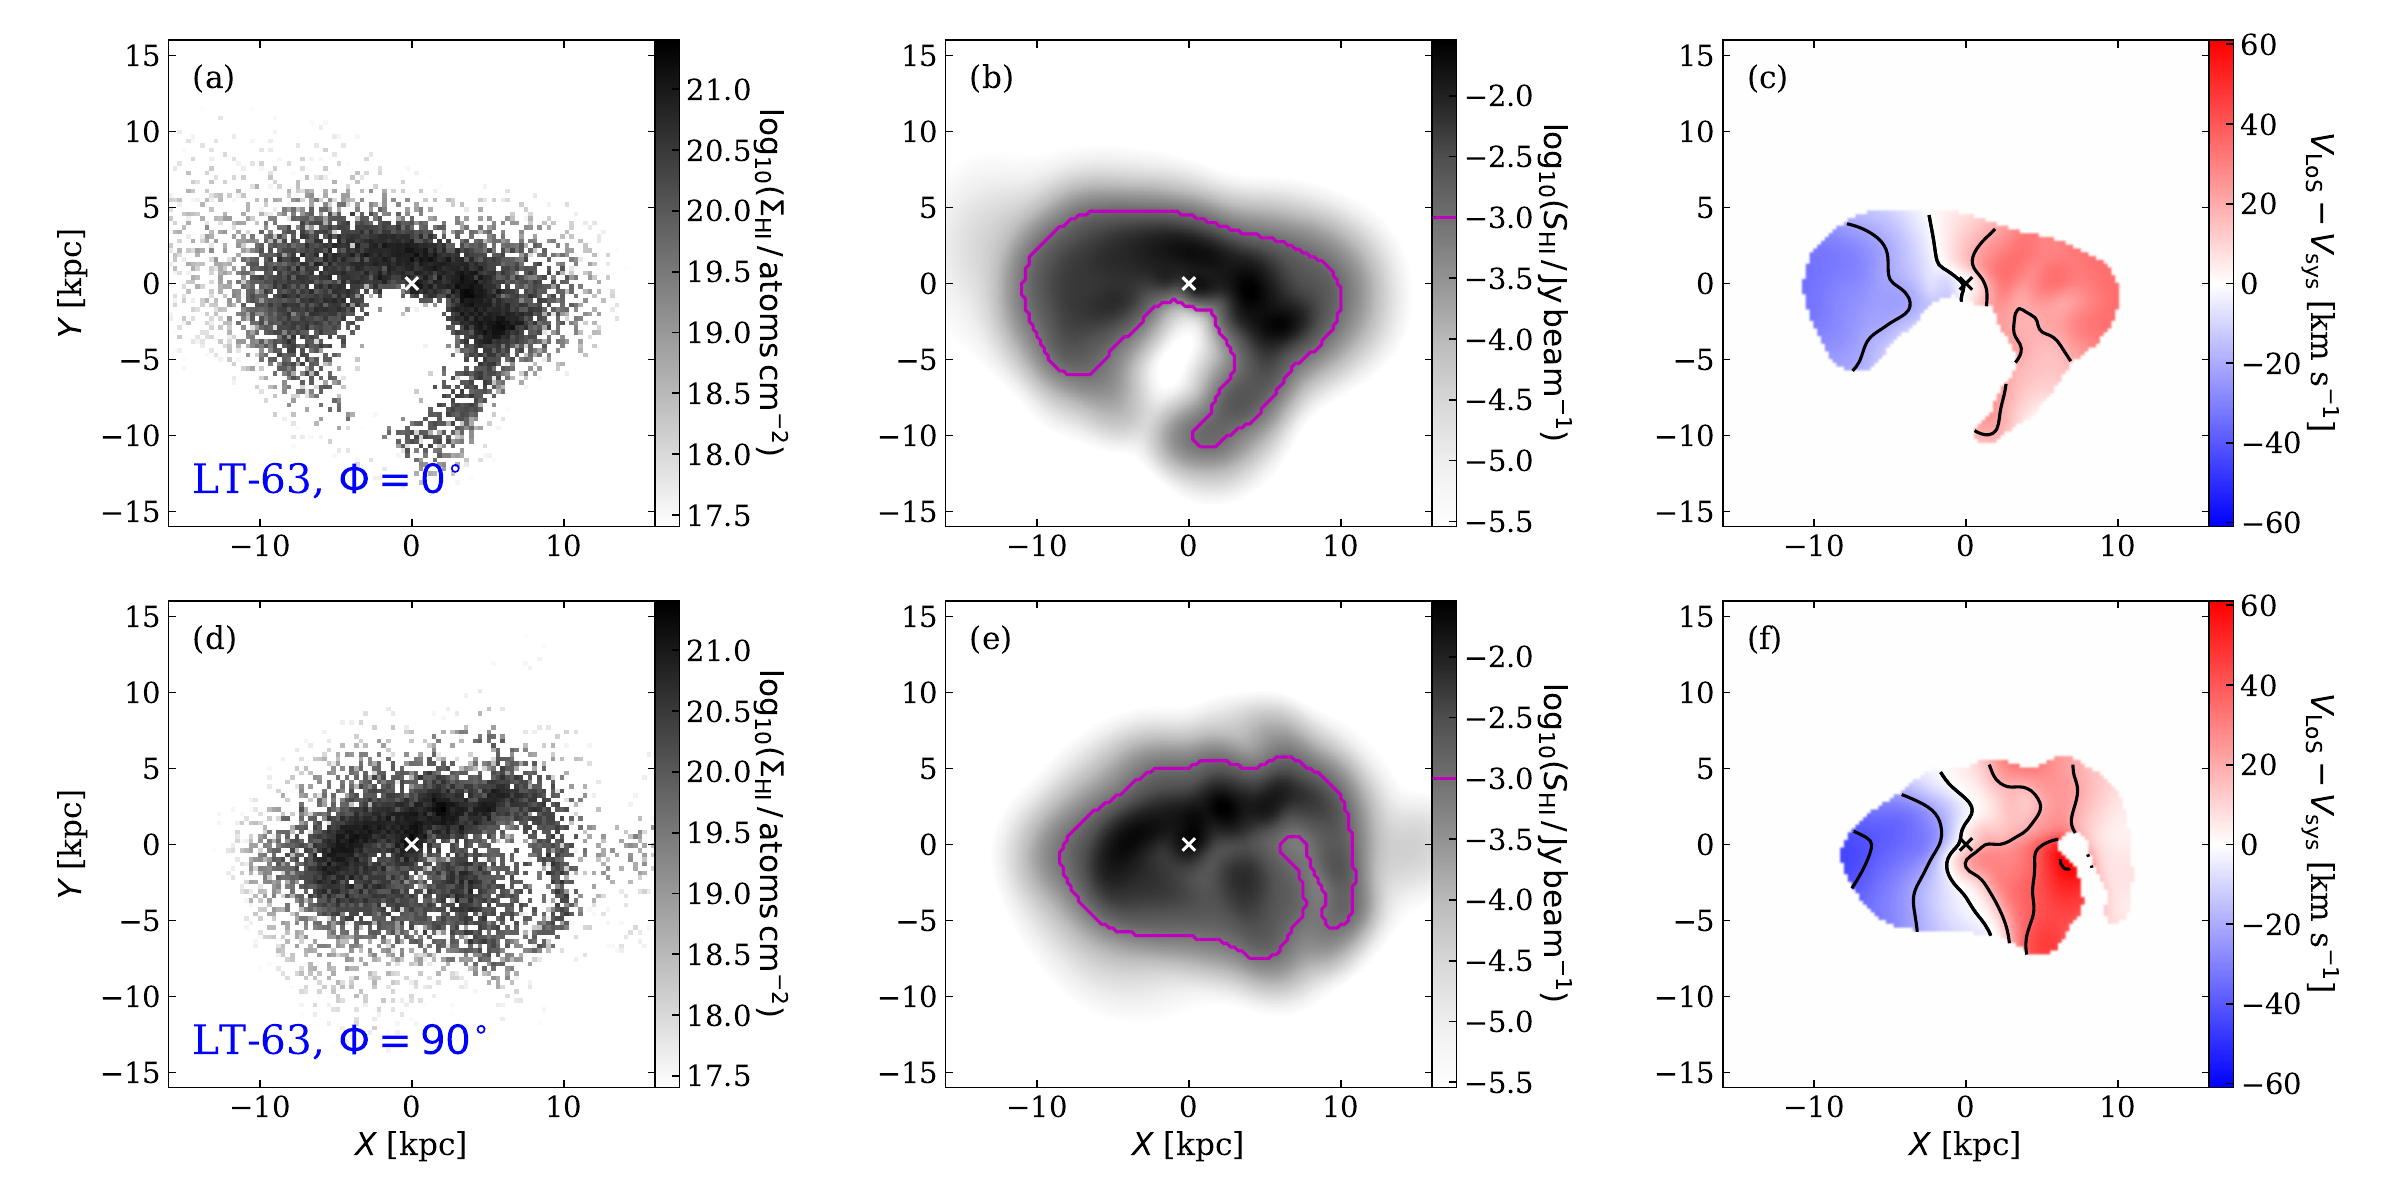}
\includegraphics[width=\textwidth]{../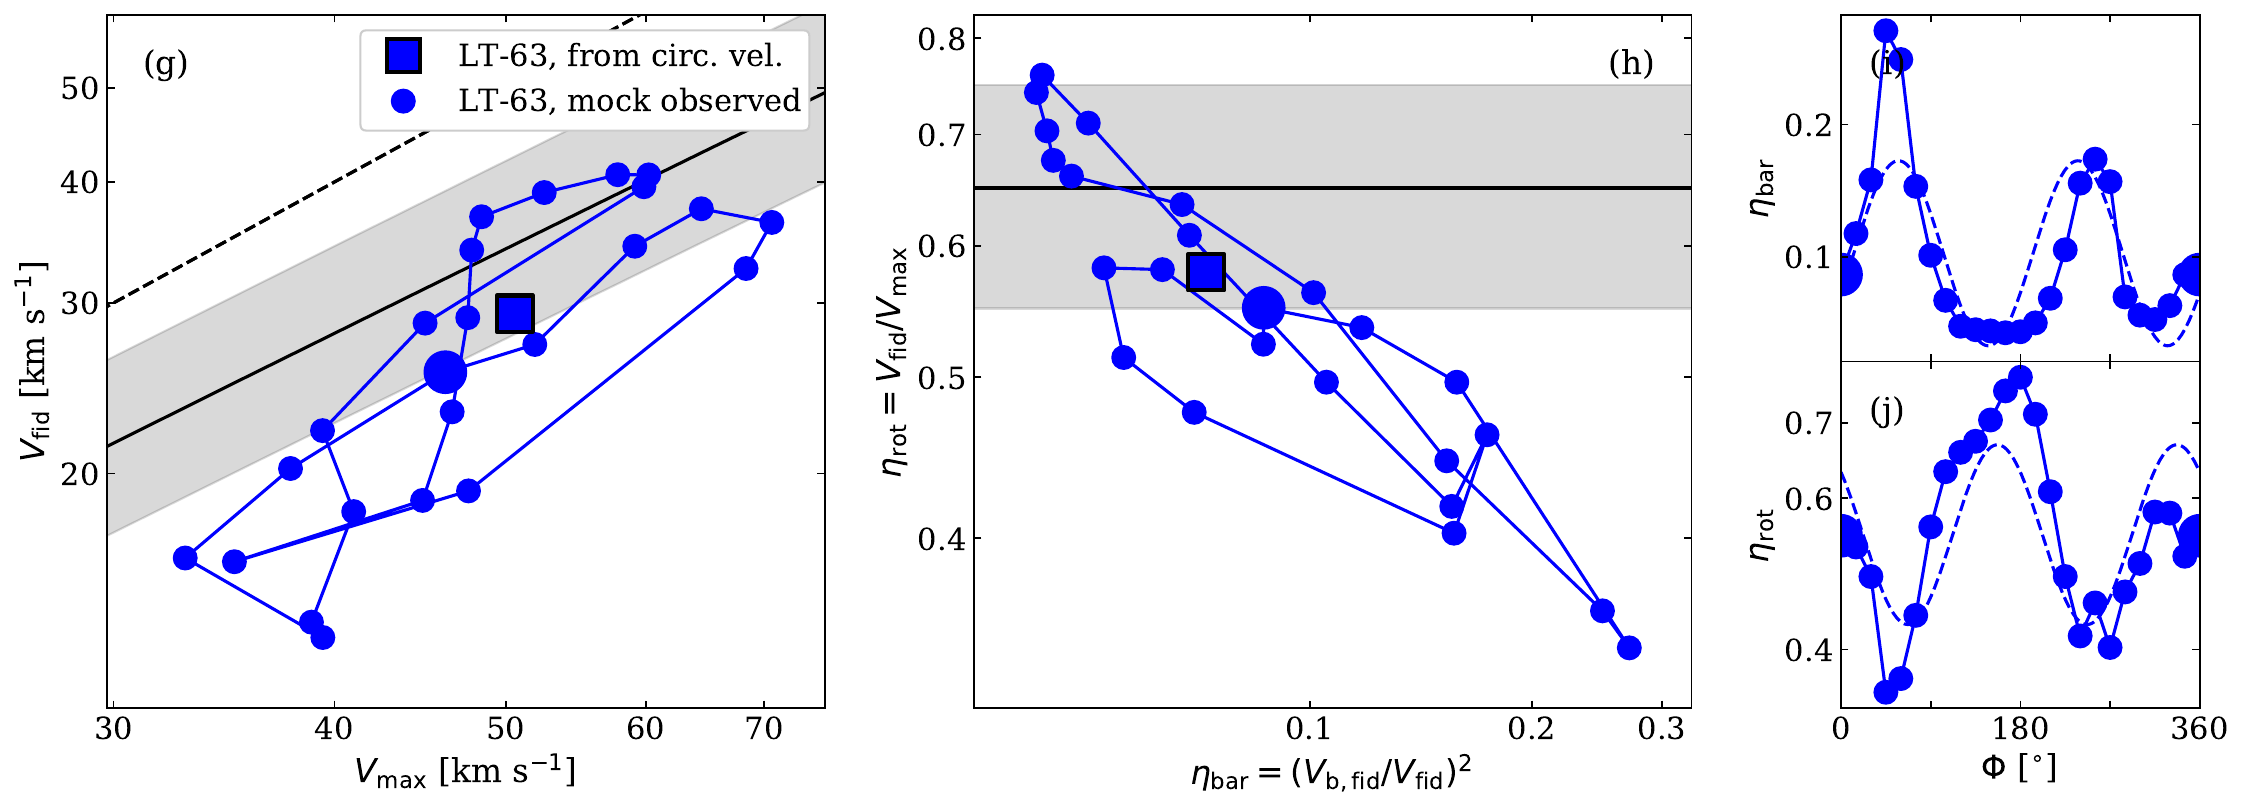}
\end{minipage}
\begin{minipage}{.4\textwidth}
\includegraphics[width=\textwidth]{../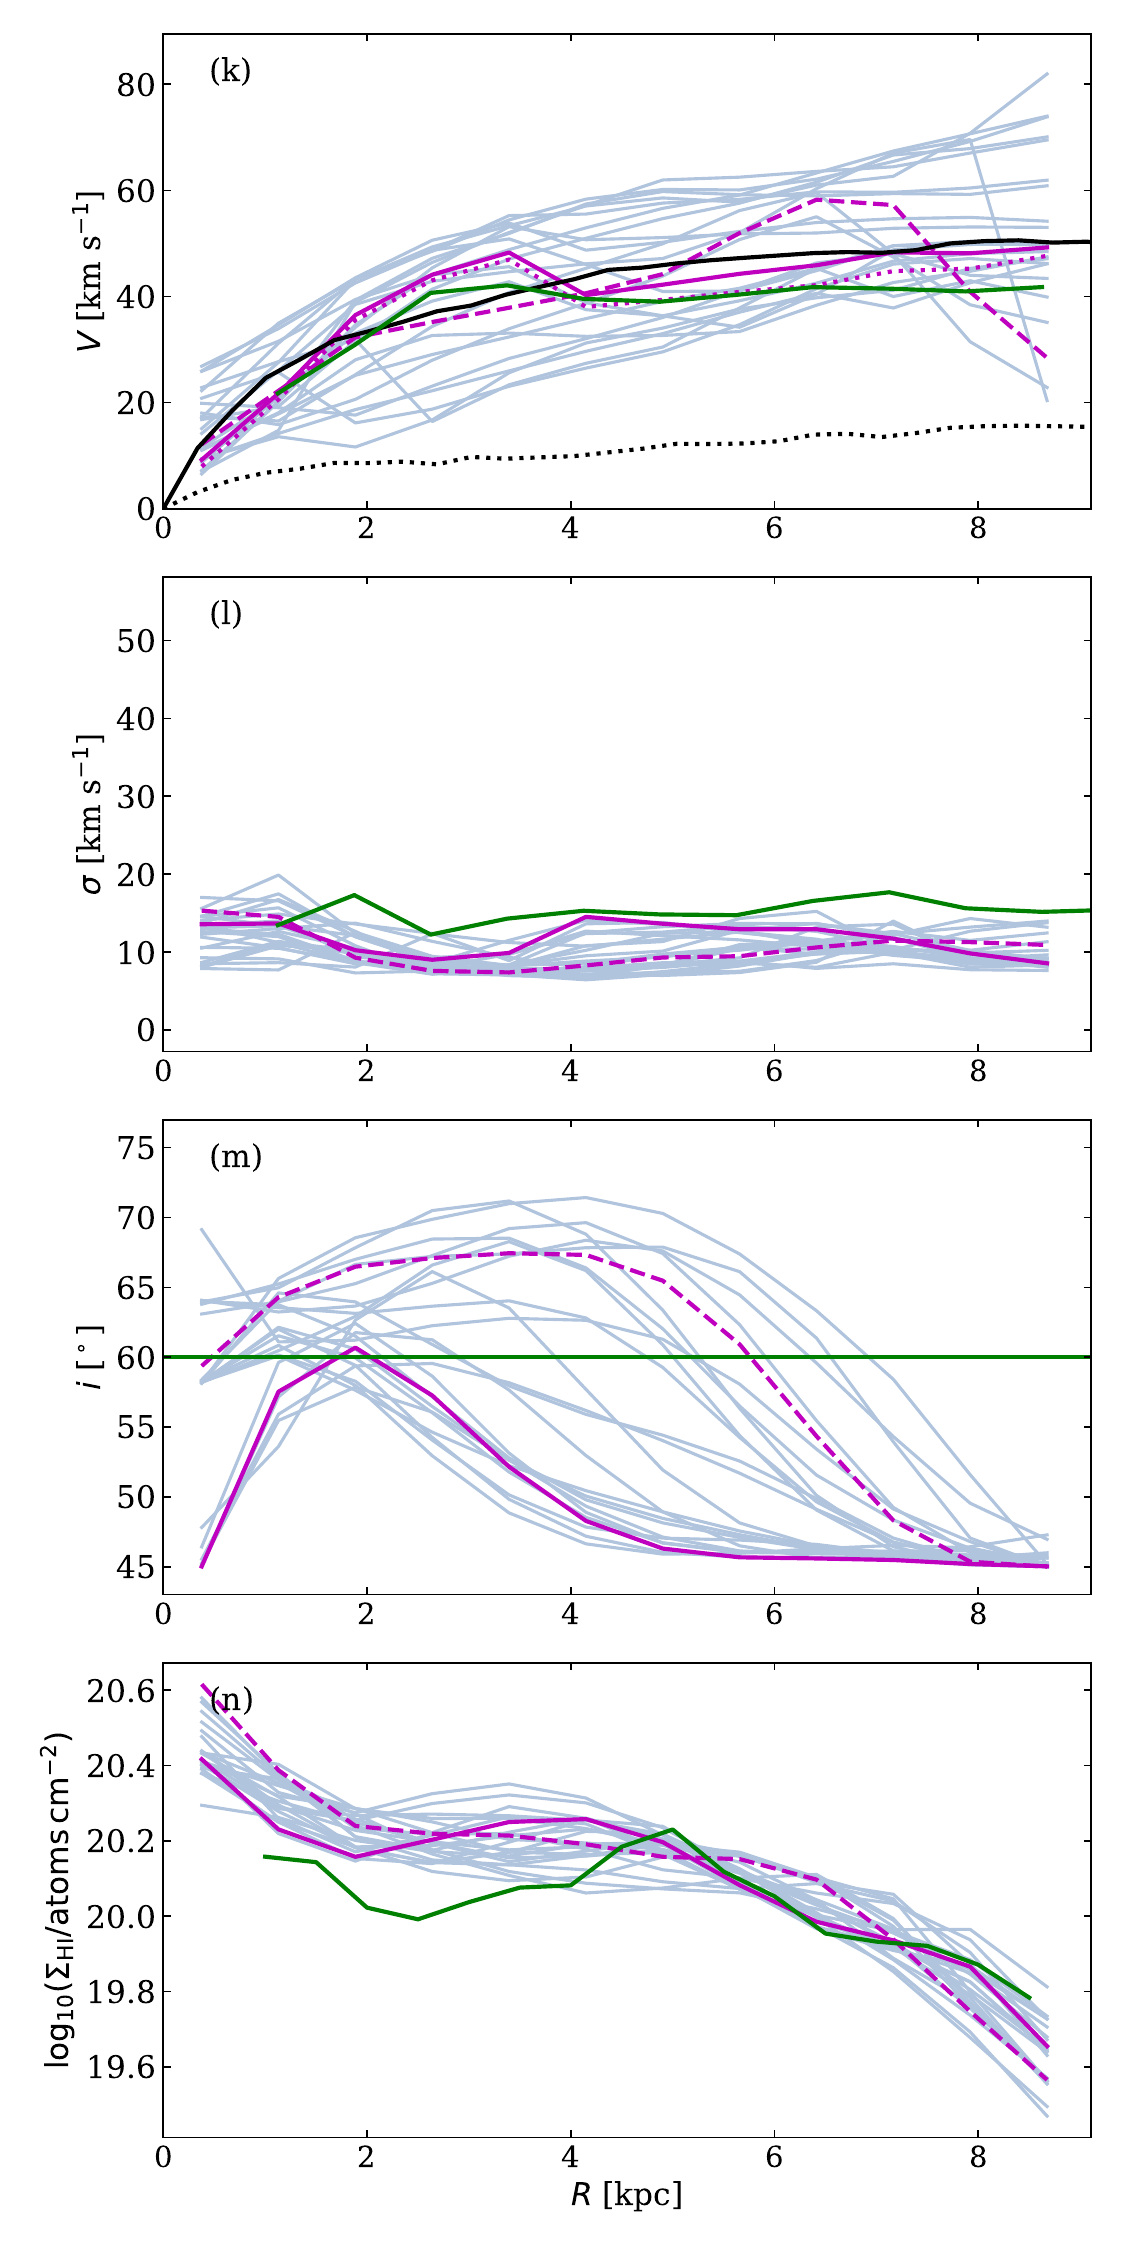}
\end{minipage}
\caption{A set of summary figures for galaxy LT-63, excluded from kinematic analysis. These include example moment maps for two orientations (panels (a)--(f); similar to Fig.~\ref{fig:visualisations}), a summary of the parameters $V_\mathrm{fid}$, $V_\mathrm{max}$, $\eta_\mathrm{rot}$, and $\eta_\mathrm{bar}$ (panels (g)--(j); similar to Fig.~\ref{fig:loops}), and a summary of the rotation curve analysis from $24$ viewing angles (panels (k)--(n); similar to Fig.~\ref{fig:rot_curves}). See description of Appendix~\ref{app:supplementary} for details.}
\label{fig:S45}
\end{figure}
\clearpage

\begin{figure}
\begin{minipage}{.9\textwidth}
\includegraphics[width=\textwidth]{../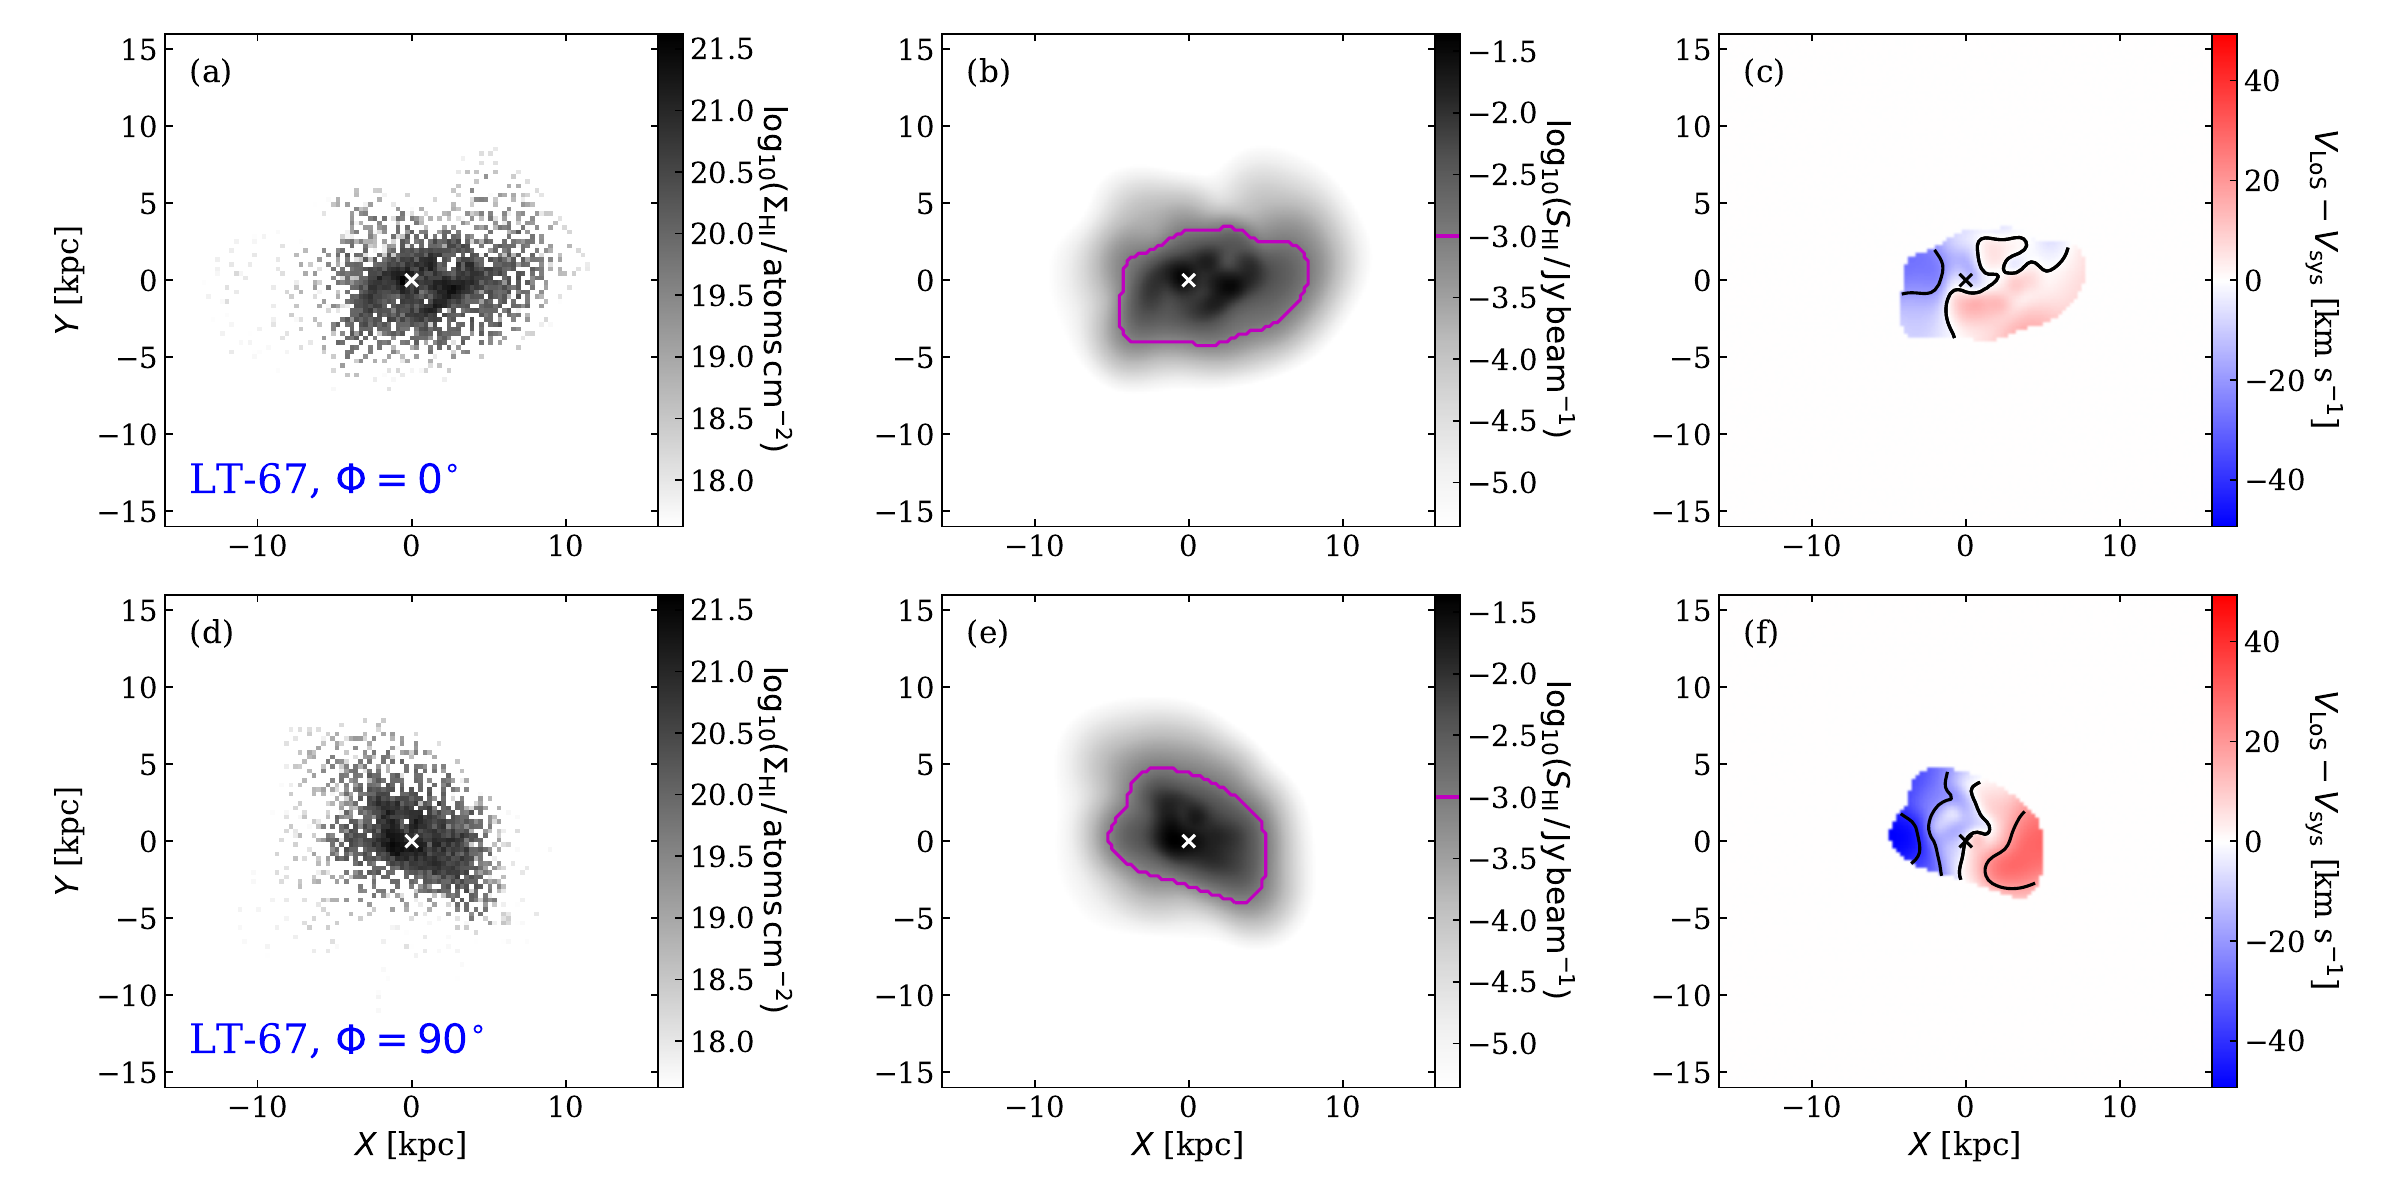}
\includegraphics[width=\textwidth]{../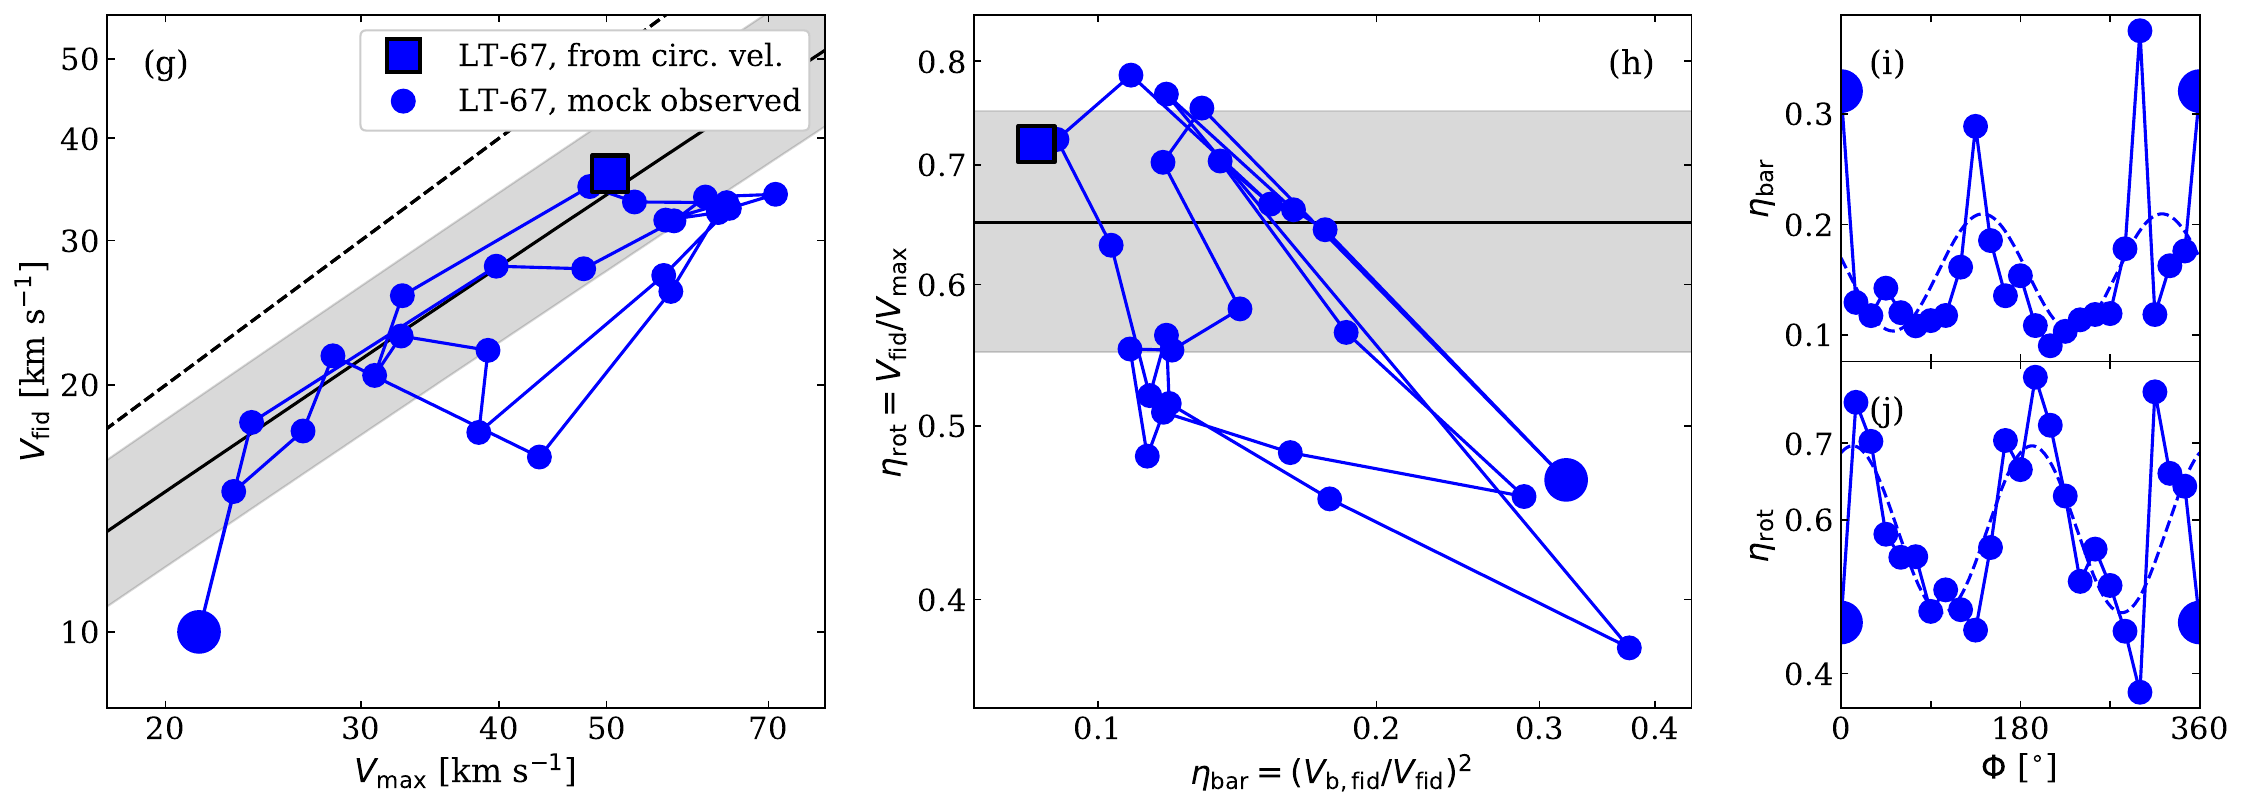}
\end{minipage}
\begin{minipage}{.4\textwidth}
\includegraphics[width=\textwidth]{../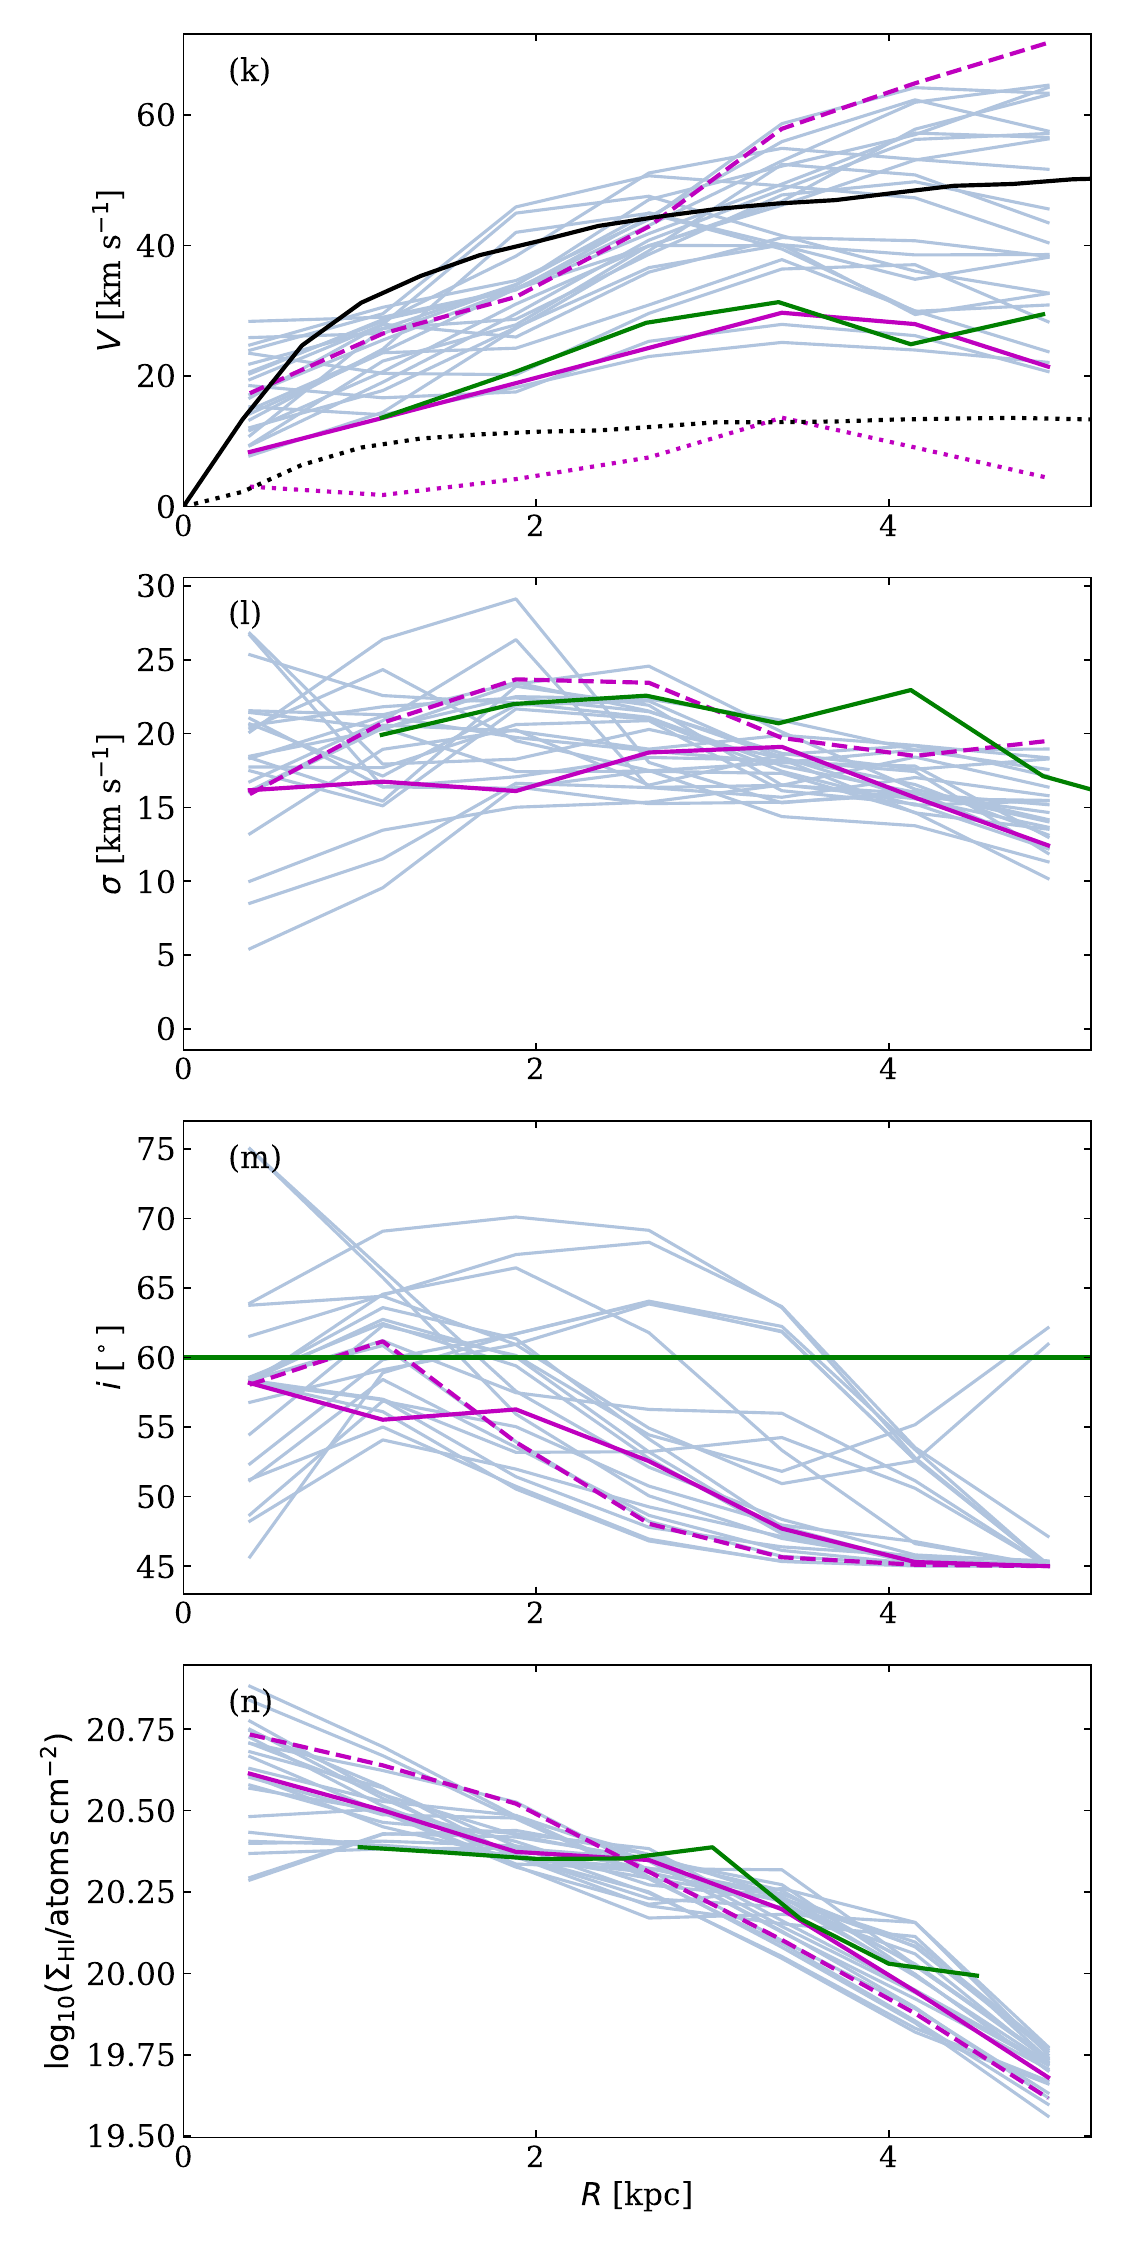}
\end{minipage}
\caption{A set of summary figures for galaxy LT-67, excluded from kinematic analysis. These include example moment maps for two orientations (panels (a)--(f); similar to Fig.~\ref{fig:visualisations}), a summary of the parameters $V_\mathrm{fid}$, $V_\mathrm{max}$, $\eta_\mathrm{rot}$, and $\eta_\mathrm{bar}$ (panels (g)--(j); similar to Fig.~\ref{fig:loops}), and a summary of the rotation curve analysis from $24$ viewing angles (panels (k)--(n); similar to Fig.~\ref{fig:rot_curves}). See description of Appendix~\ref{app:supplementary} for details.}
\label{fig:S46}
\end{figure}
\clearpage

\begin{figure}
\begin{minipage}{.9\textwidth}
\includegraphics[width=\textwidth]{../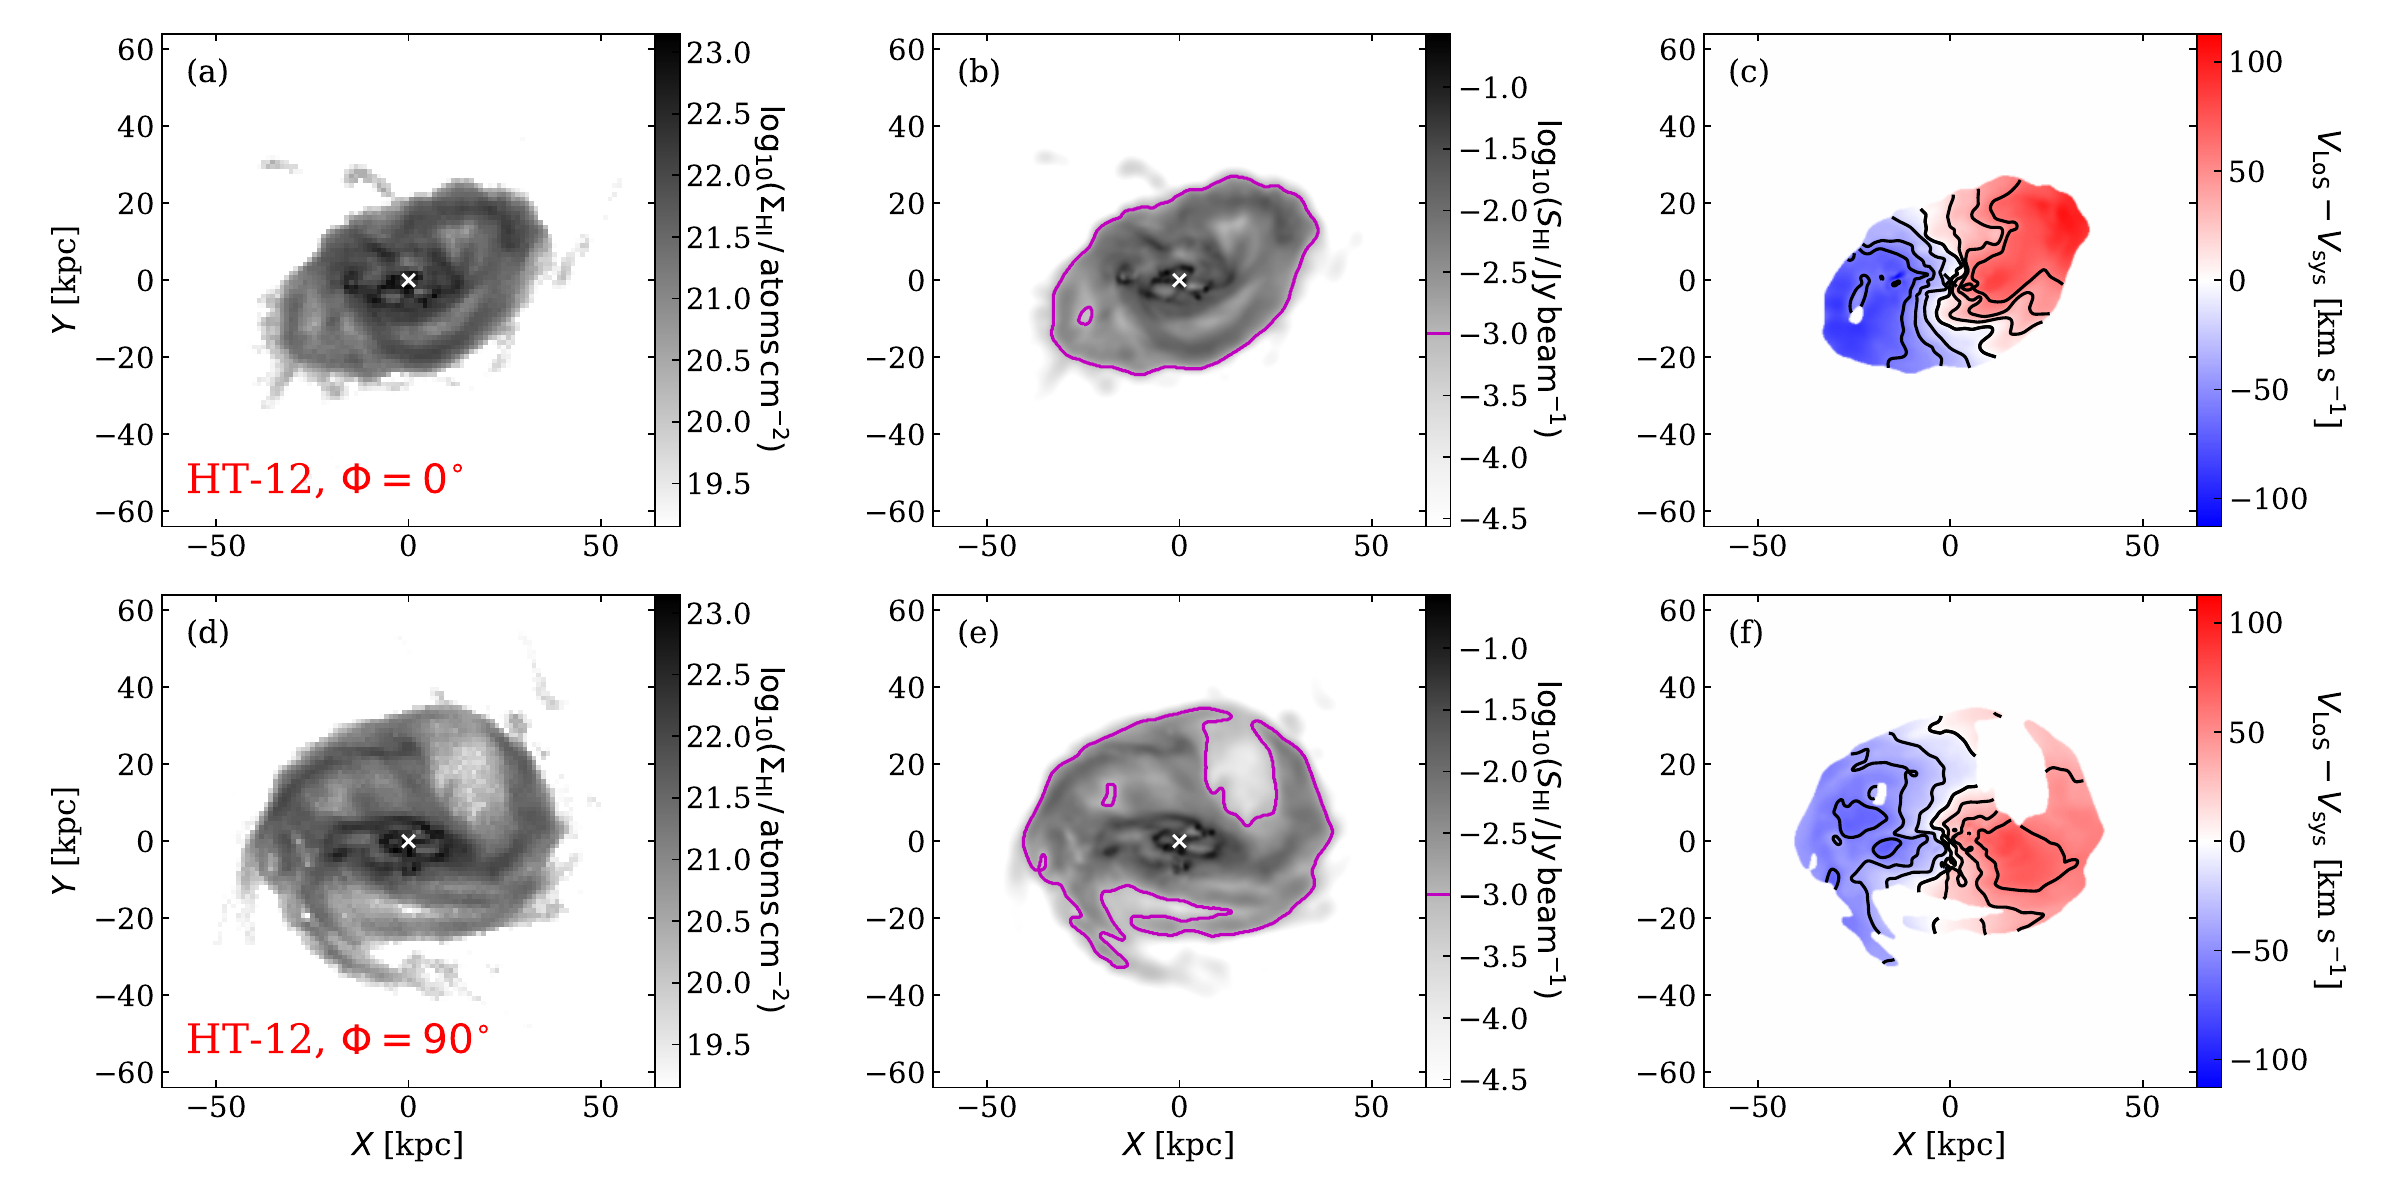}
\includegraphics[width=\textwidth]{../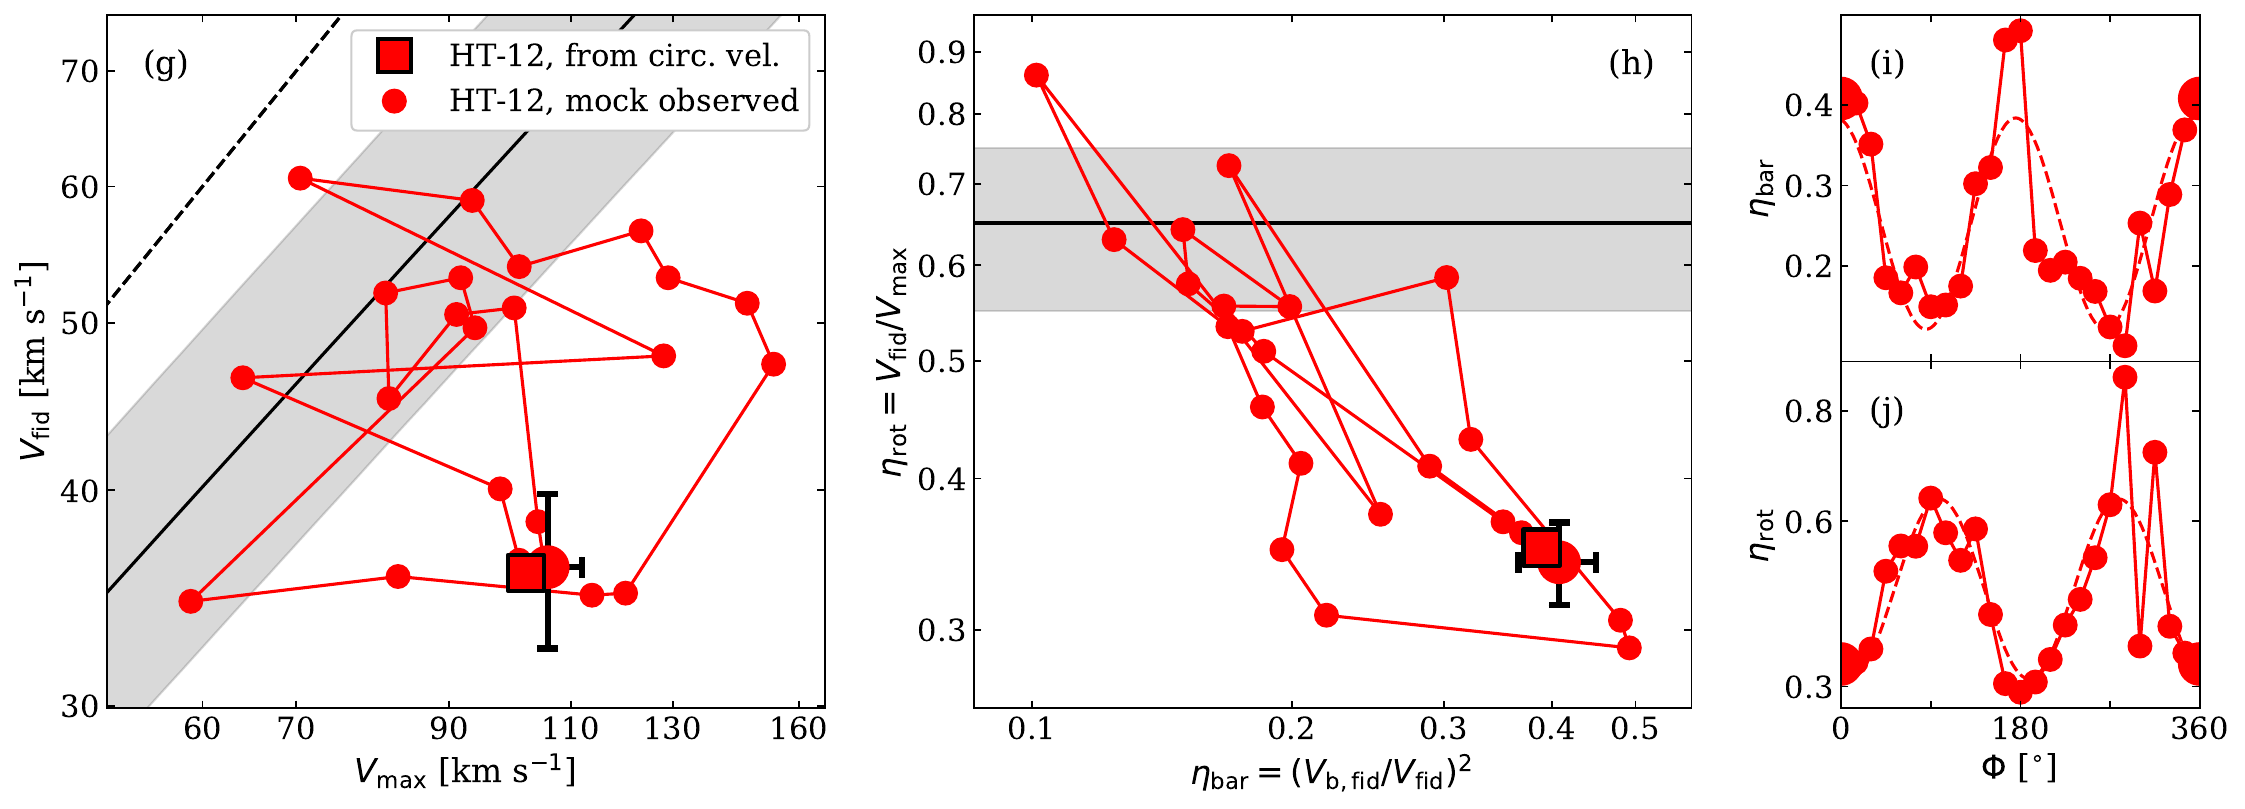}
\end{minipage}
\begin{minipage}{.4\textwidth}
\includegraphics[width=\textwidth]{../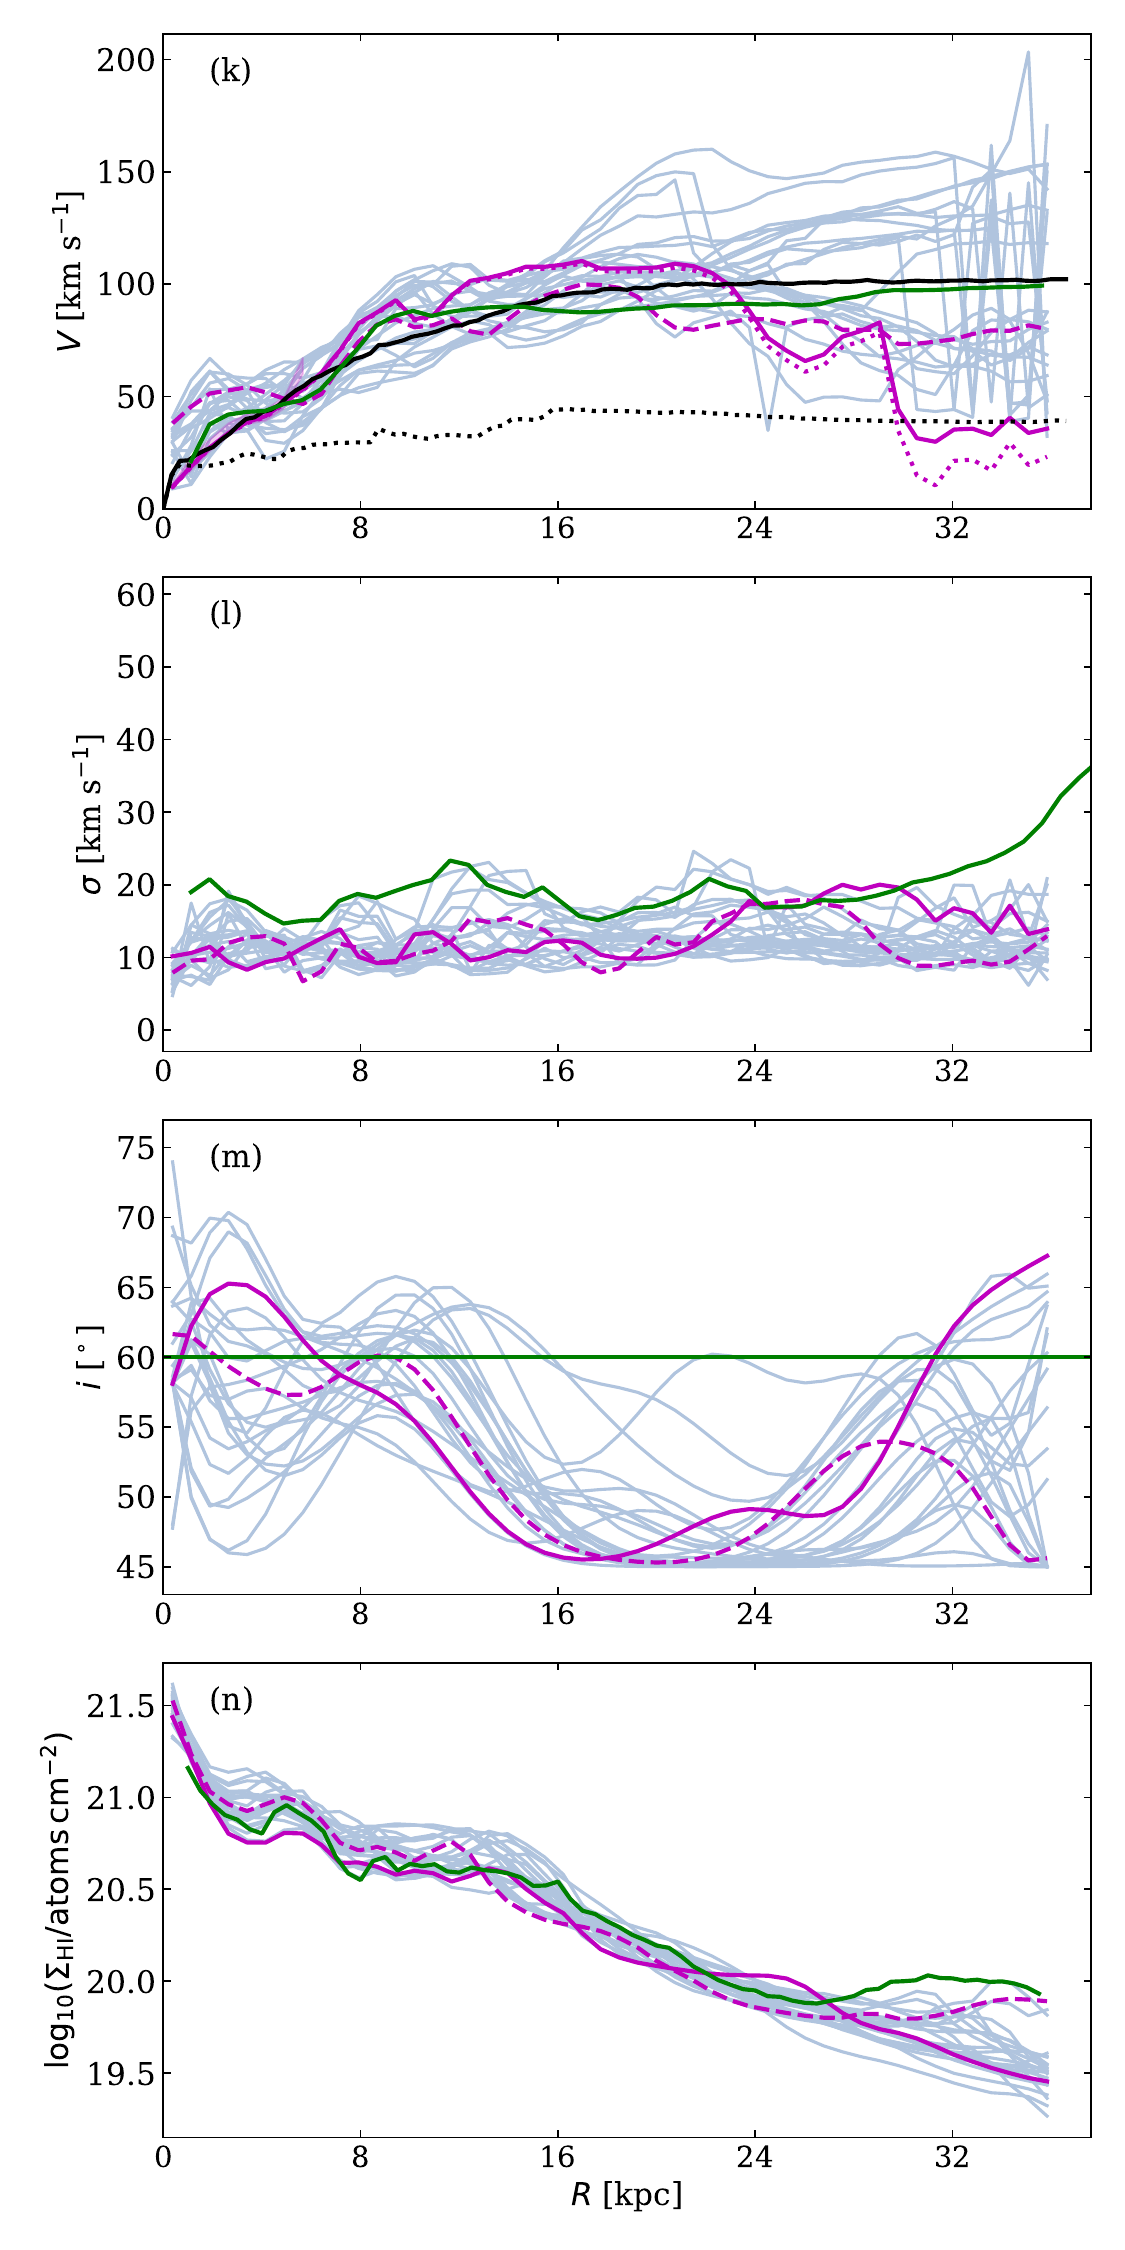}
\end{minipage}
\caption{A set of summary figures for galaxy HT-12, selected for kinematic analysis. These include example moment maps for two orientations (panels (a)--(f); similar to Fig.~\ref{fig:visualisations}), a summary of the parameters $V_\mathrm{fid}$, $V_\mathrm{max}$, $\eta_\mathrm{rot}$, and $\eta_\mathrm{bar}$ (panels (g)--(j); similar to Fig.~\ref{fig:loops}), and a summary of the rotation curve analysis from $24$ viewing angles (panels (k)--(n); similar to Fig.~\ref{fig:rot_curves}). See description of Appendix~\ref{app:supplementary} for details.}
\label{fig:S47}
\end{figure}
\clearpage

\begin{figure}
\begin{minipage}{.9\textwidth}
\includegraphics[width=\textwidth]{../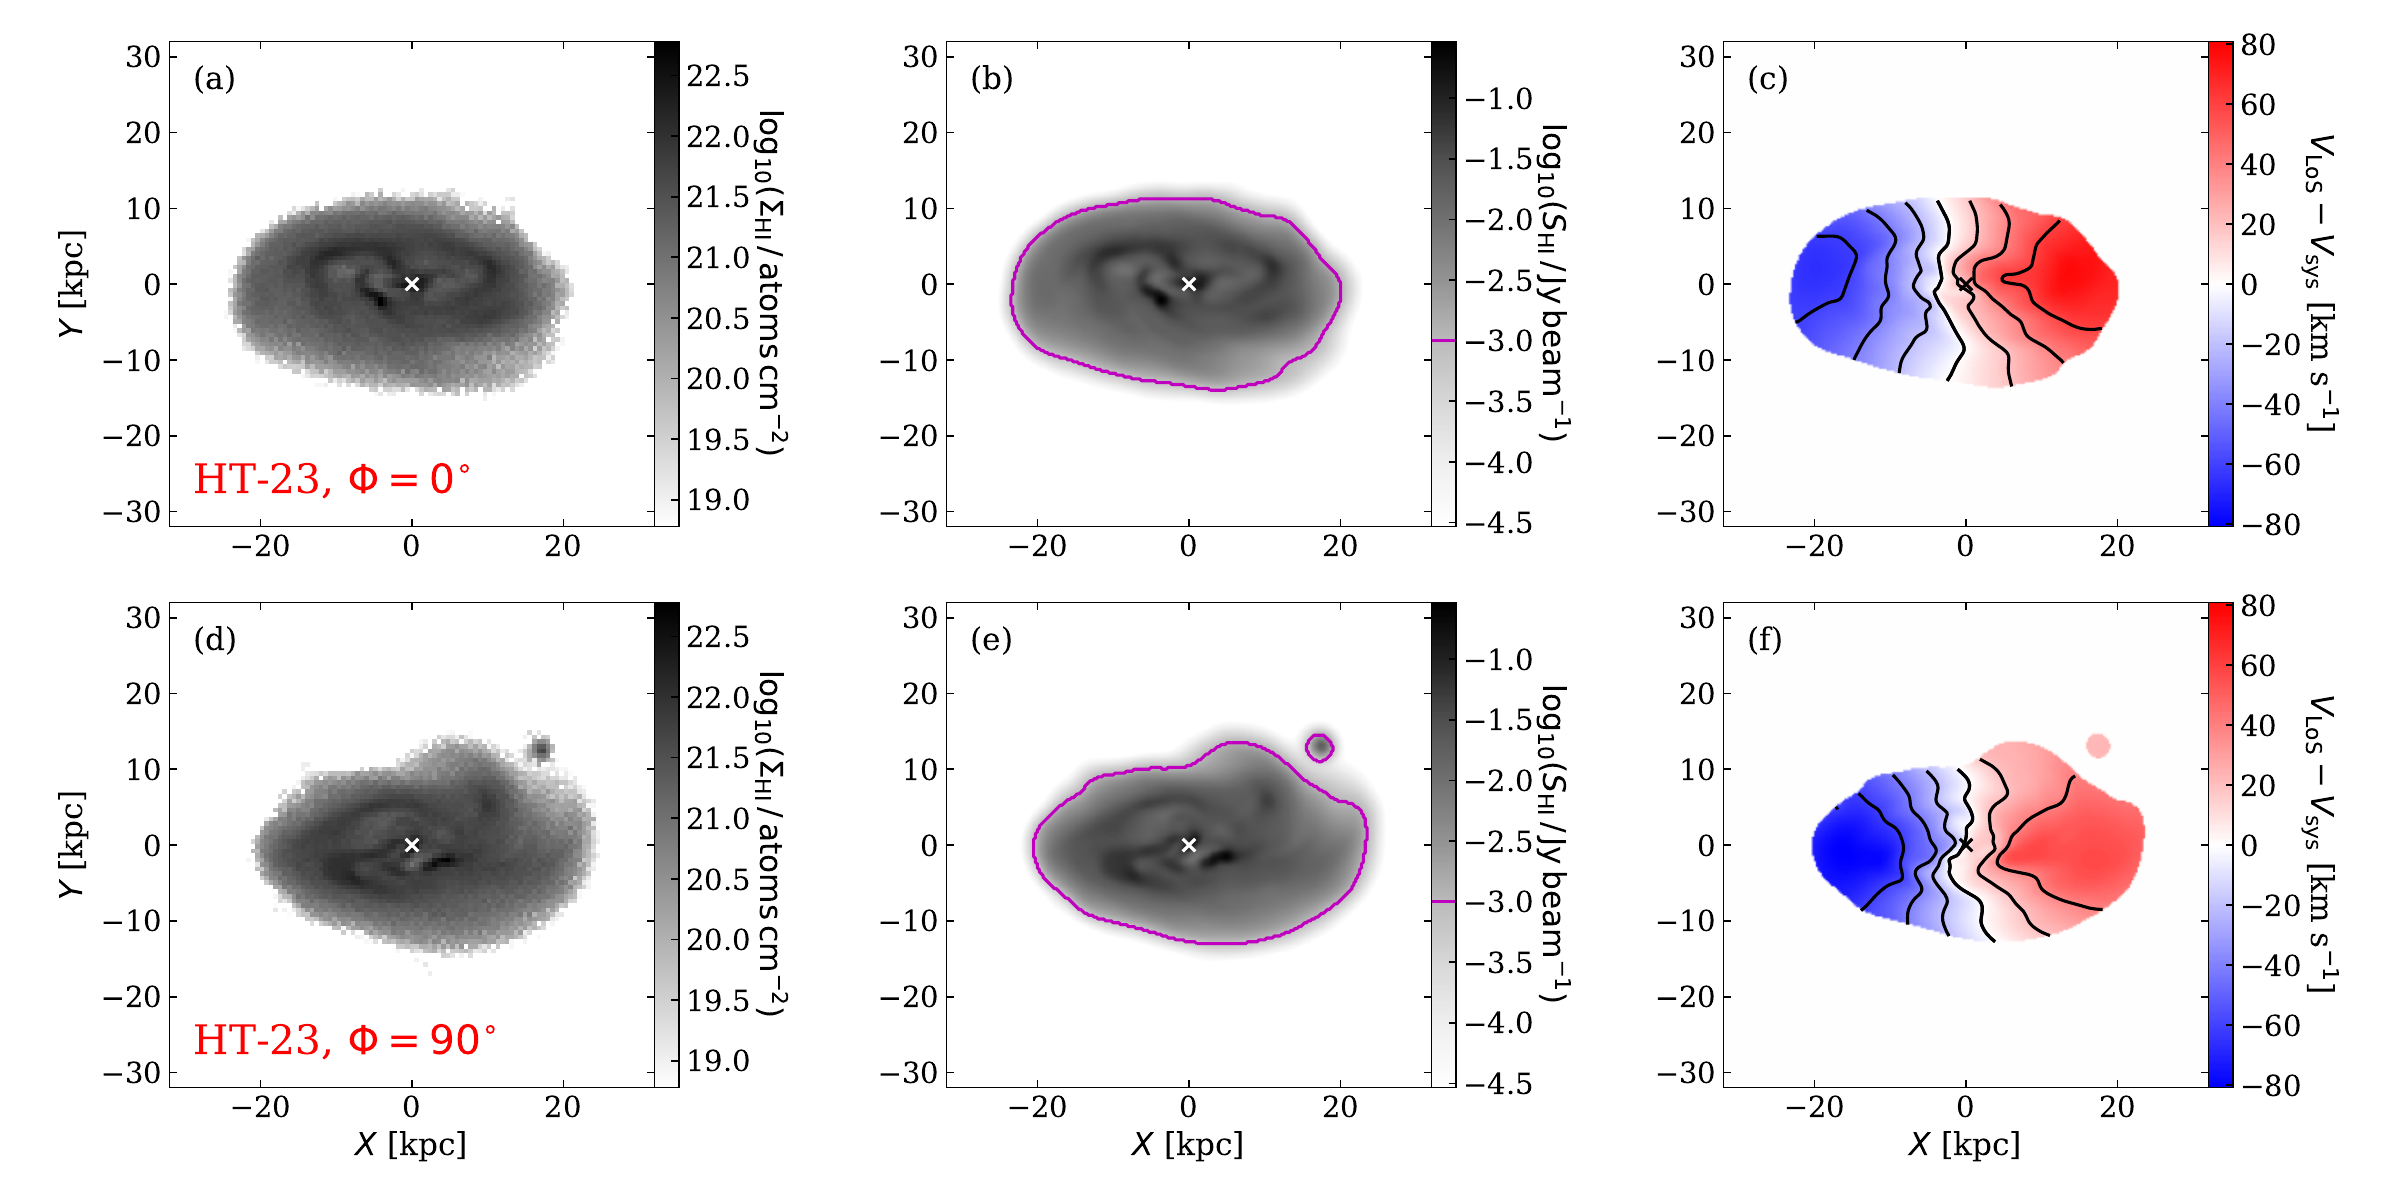}
\includegraphics[width=\textwidth]{../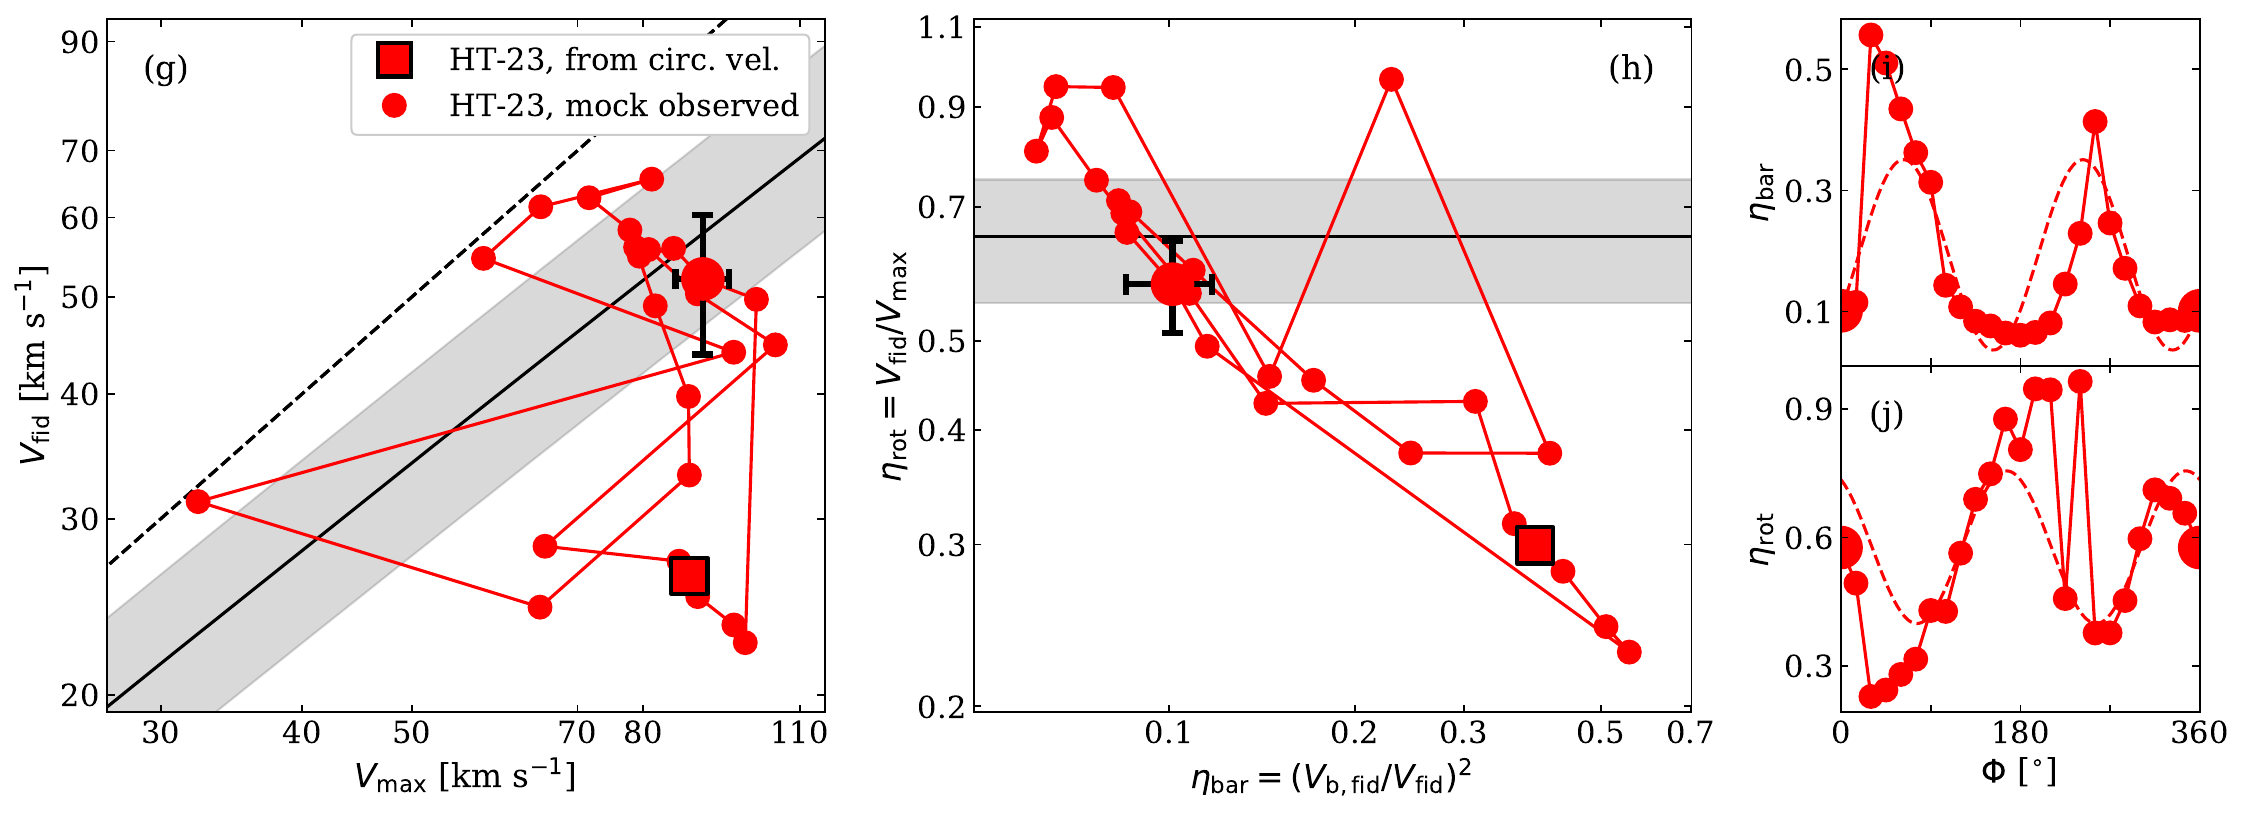}
\end{minipage}
\begin{minipage}{.4\textwidth}
\includegraphics[width=\textwidth]{../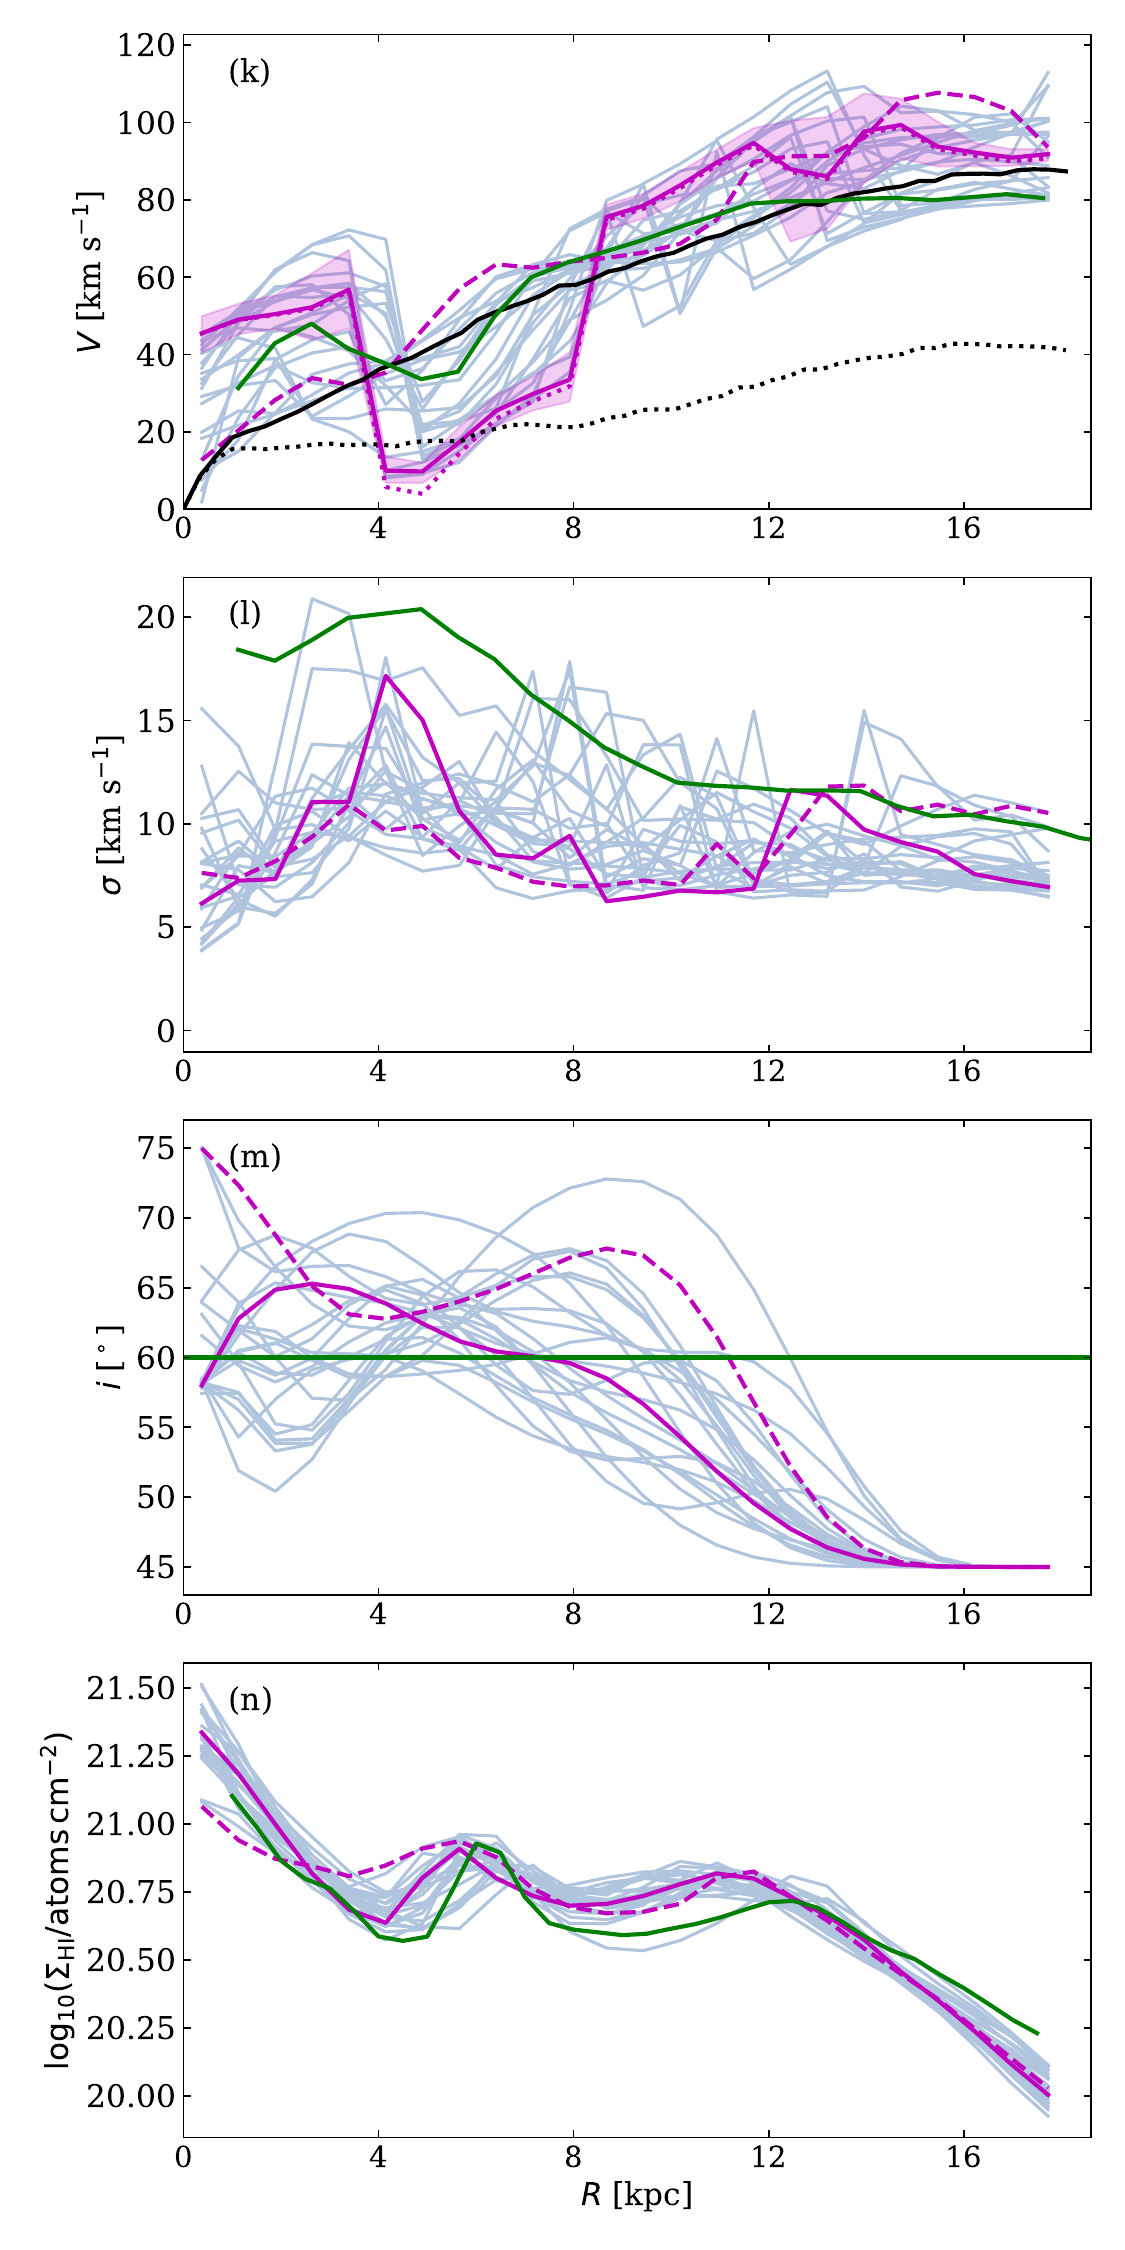}
\end{minipage}
\caption{A set of summary figures for galaxy HT-23, selected for kinematic analysis. These include example moment maps for two orientations (panels (a)--(f); similar to Fig.~\ref{fig:visualisations}), a summary of the parameters $V_\mathrm{fid}$, $V_\mathrm{max}$, $\eta_\mathrm{rot}$, and $\eta_\mathrm{bar}$ (panels (g)--(j); similar to Fig.~\ref{fig:loops}), and a summary of the rotation curve analysis from $24$ viewing angles (panels (k)--(n); similar to Fig.~\ref{fig:rot_curves}). See description of Appendix~\ref{app:supplementary} for details.}
\label{fig:S48}
\end{figure}
\clearpage

\begin{figure}
\begin{minipage}{.9\textwidth}
\includegraphics[width=\textwidth]{../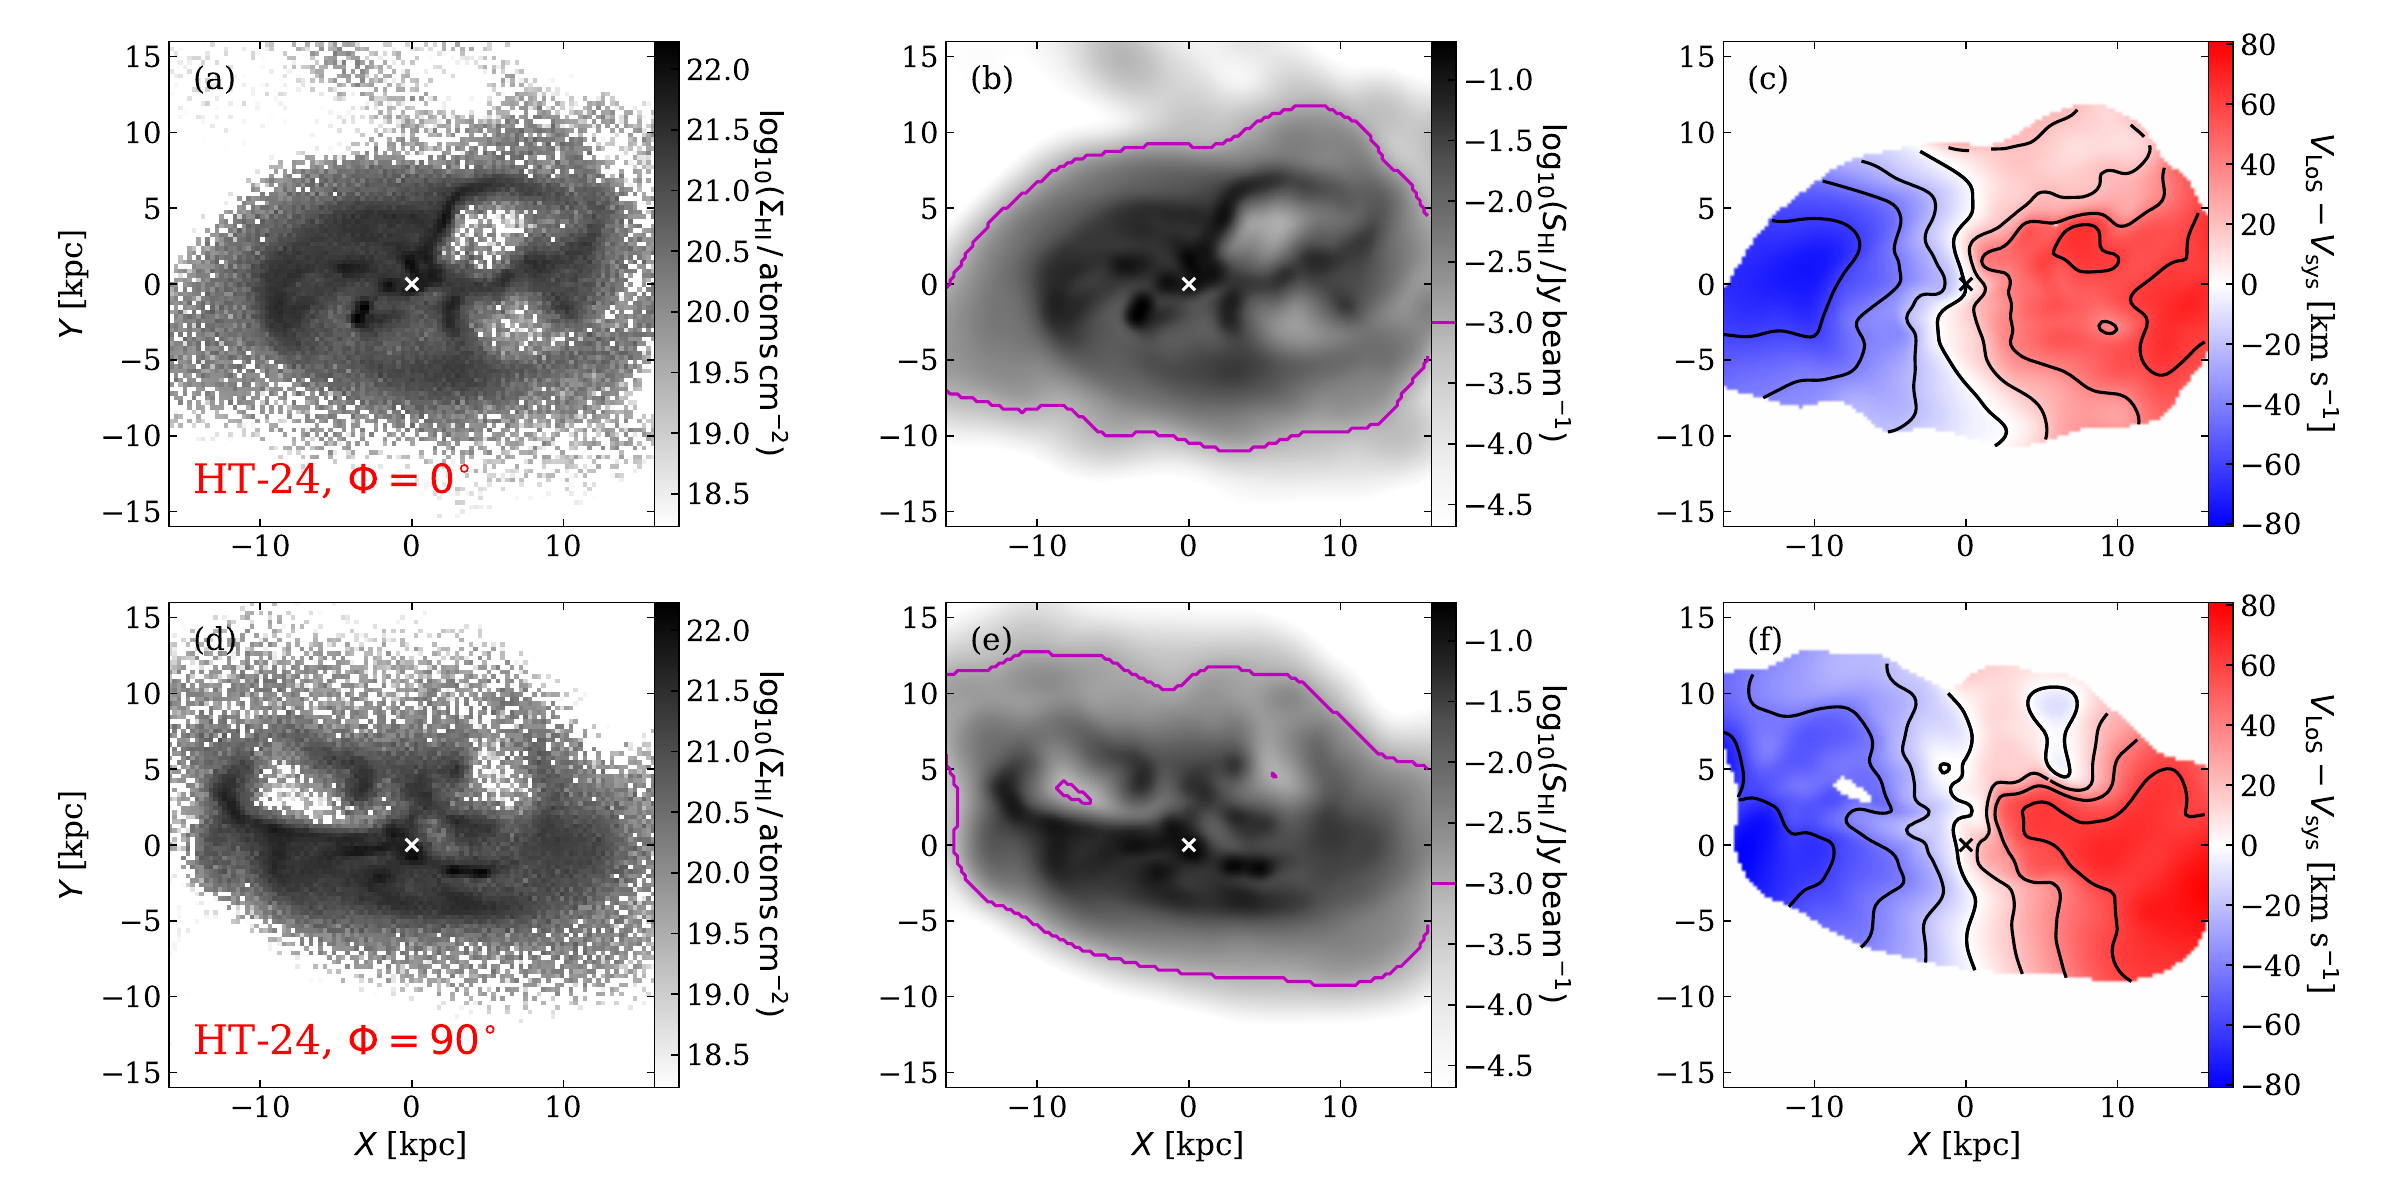}
\includegraphics[width=\textwidth]{../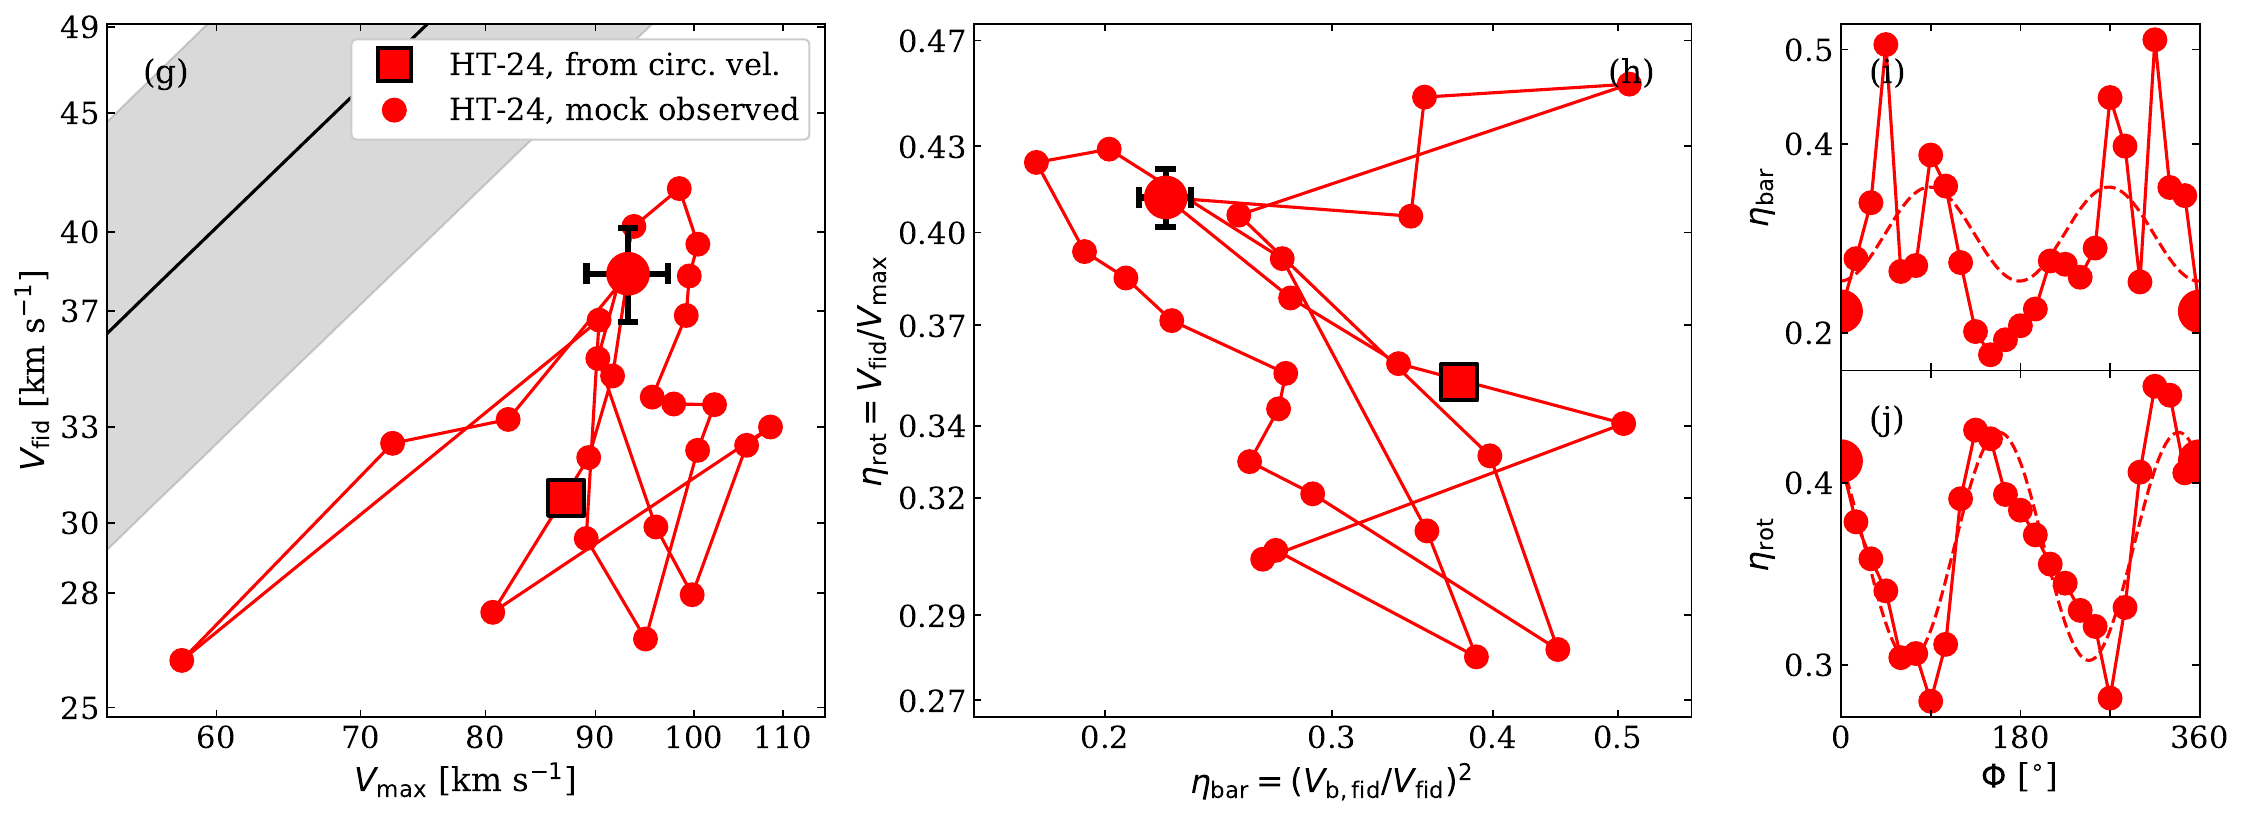}
\end{minipage}
\begin{minipage}{.4\textwidth}
\includegraphics[width=\textwidth]{../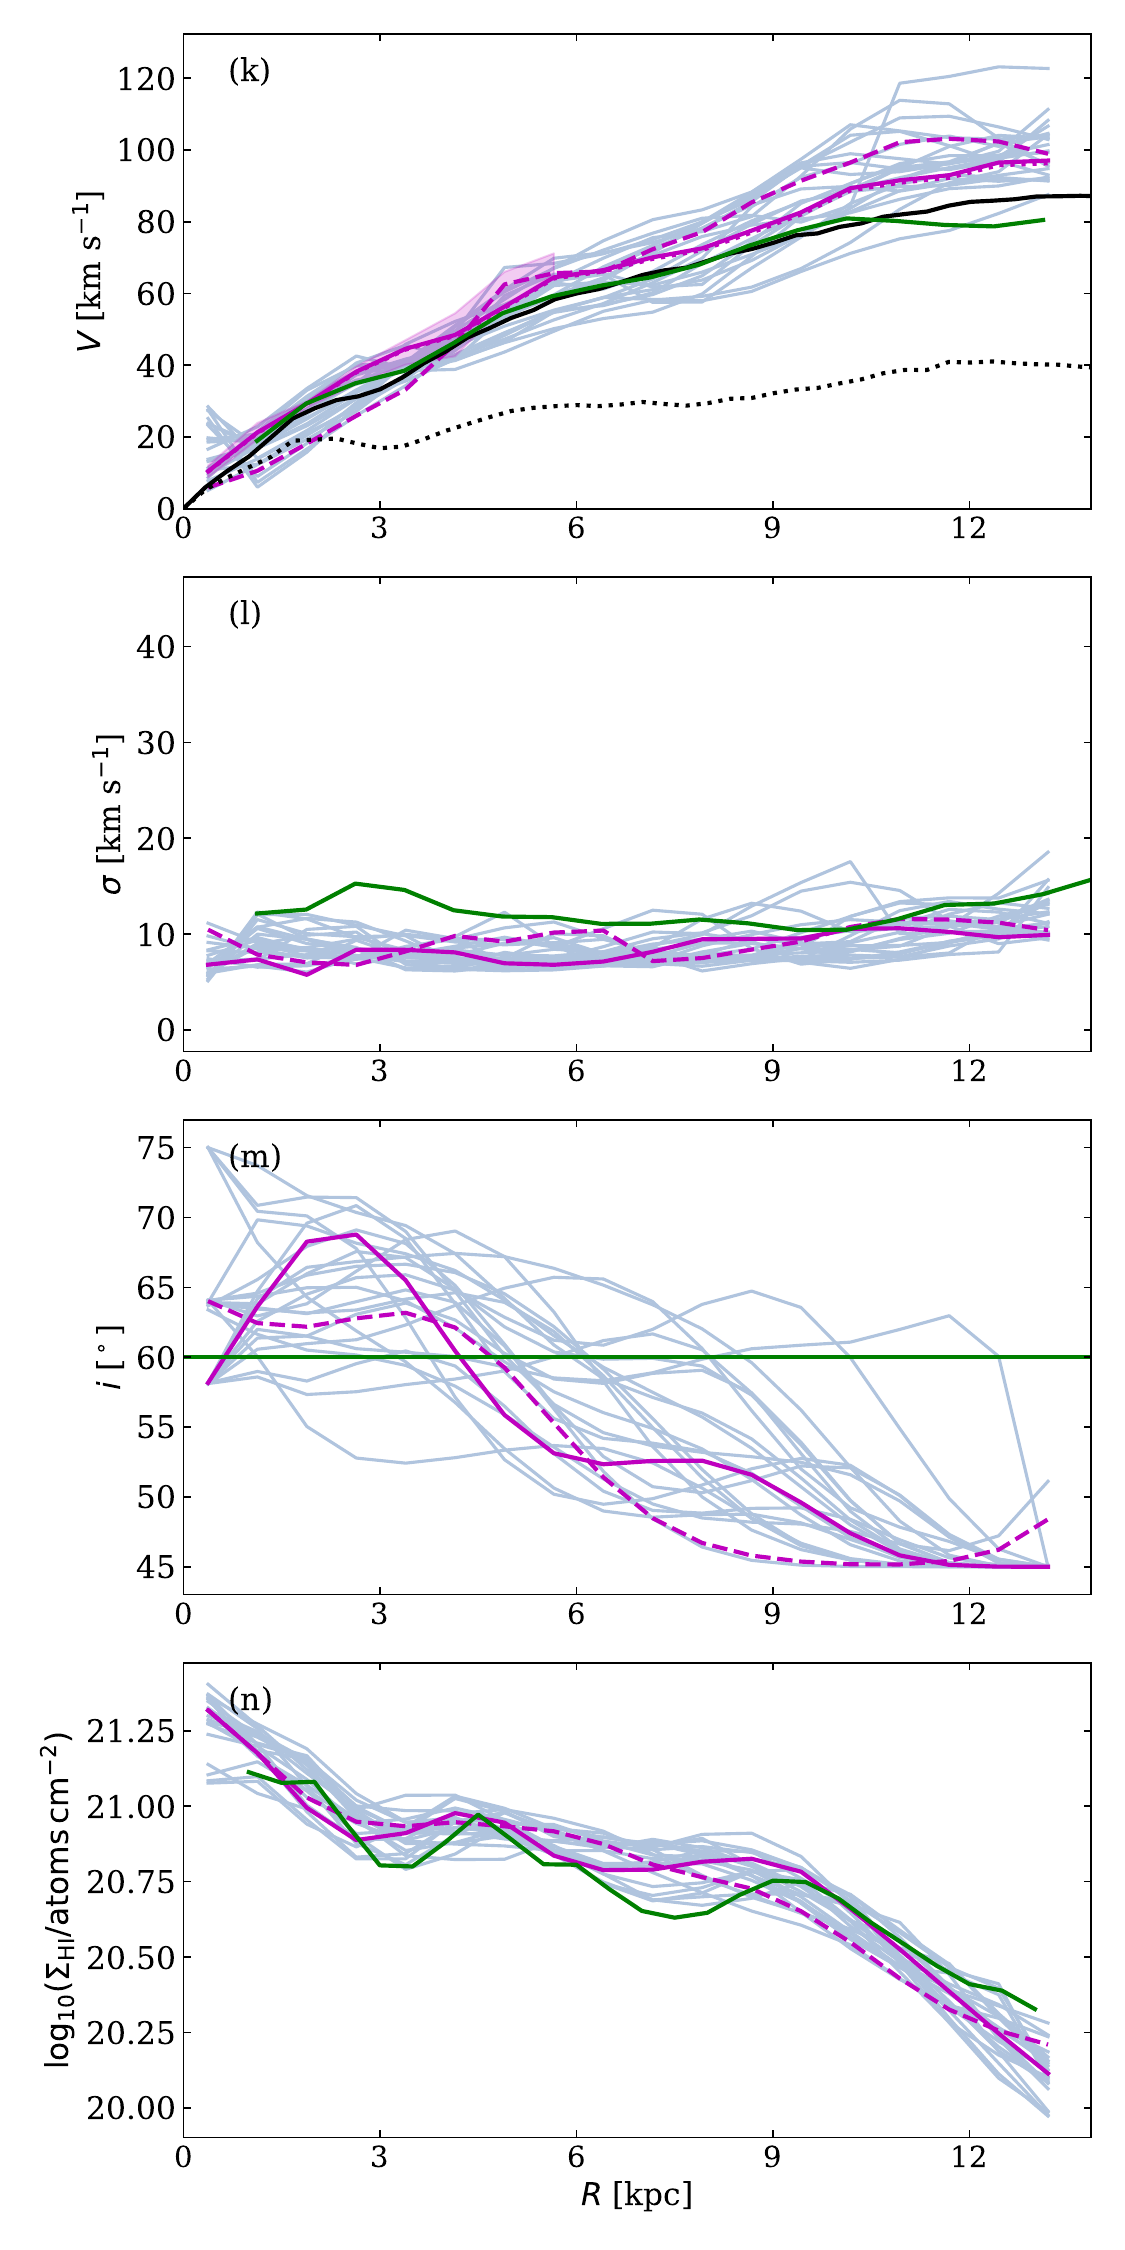}
\end{minipage}
\caption{A set of summary figures for galaxy HT-24, selected for kinematic analysis. These include example moment maps for two orientations (panels (a)--(f); similar to Fig.~\ref{fig:visualisations}), a summary of the parameters $V_\mathrm{fid}$, $V_\mathrm{max}$, $\eta_\mathrm{rot}$, and $\eta_\mathrm{bar}$ (panels (g)--(j); similar to Fig.~\ref{fig:loops}), and a summary of the rotation curve analysis from $24$ viewing angles (panels (k)--(n); similar to Fig.~\ref{fig:rot_curves}). See description of Appendix~\ref{app:supplementary} for details.}
\label{fig:S49}
\end{figure}
\clearpage

\begin{figure}
\begin{minipage}{.9\textwidth}
\includegraphics[width=\textwidth]{../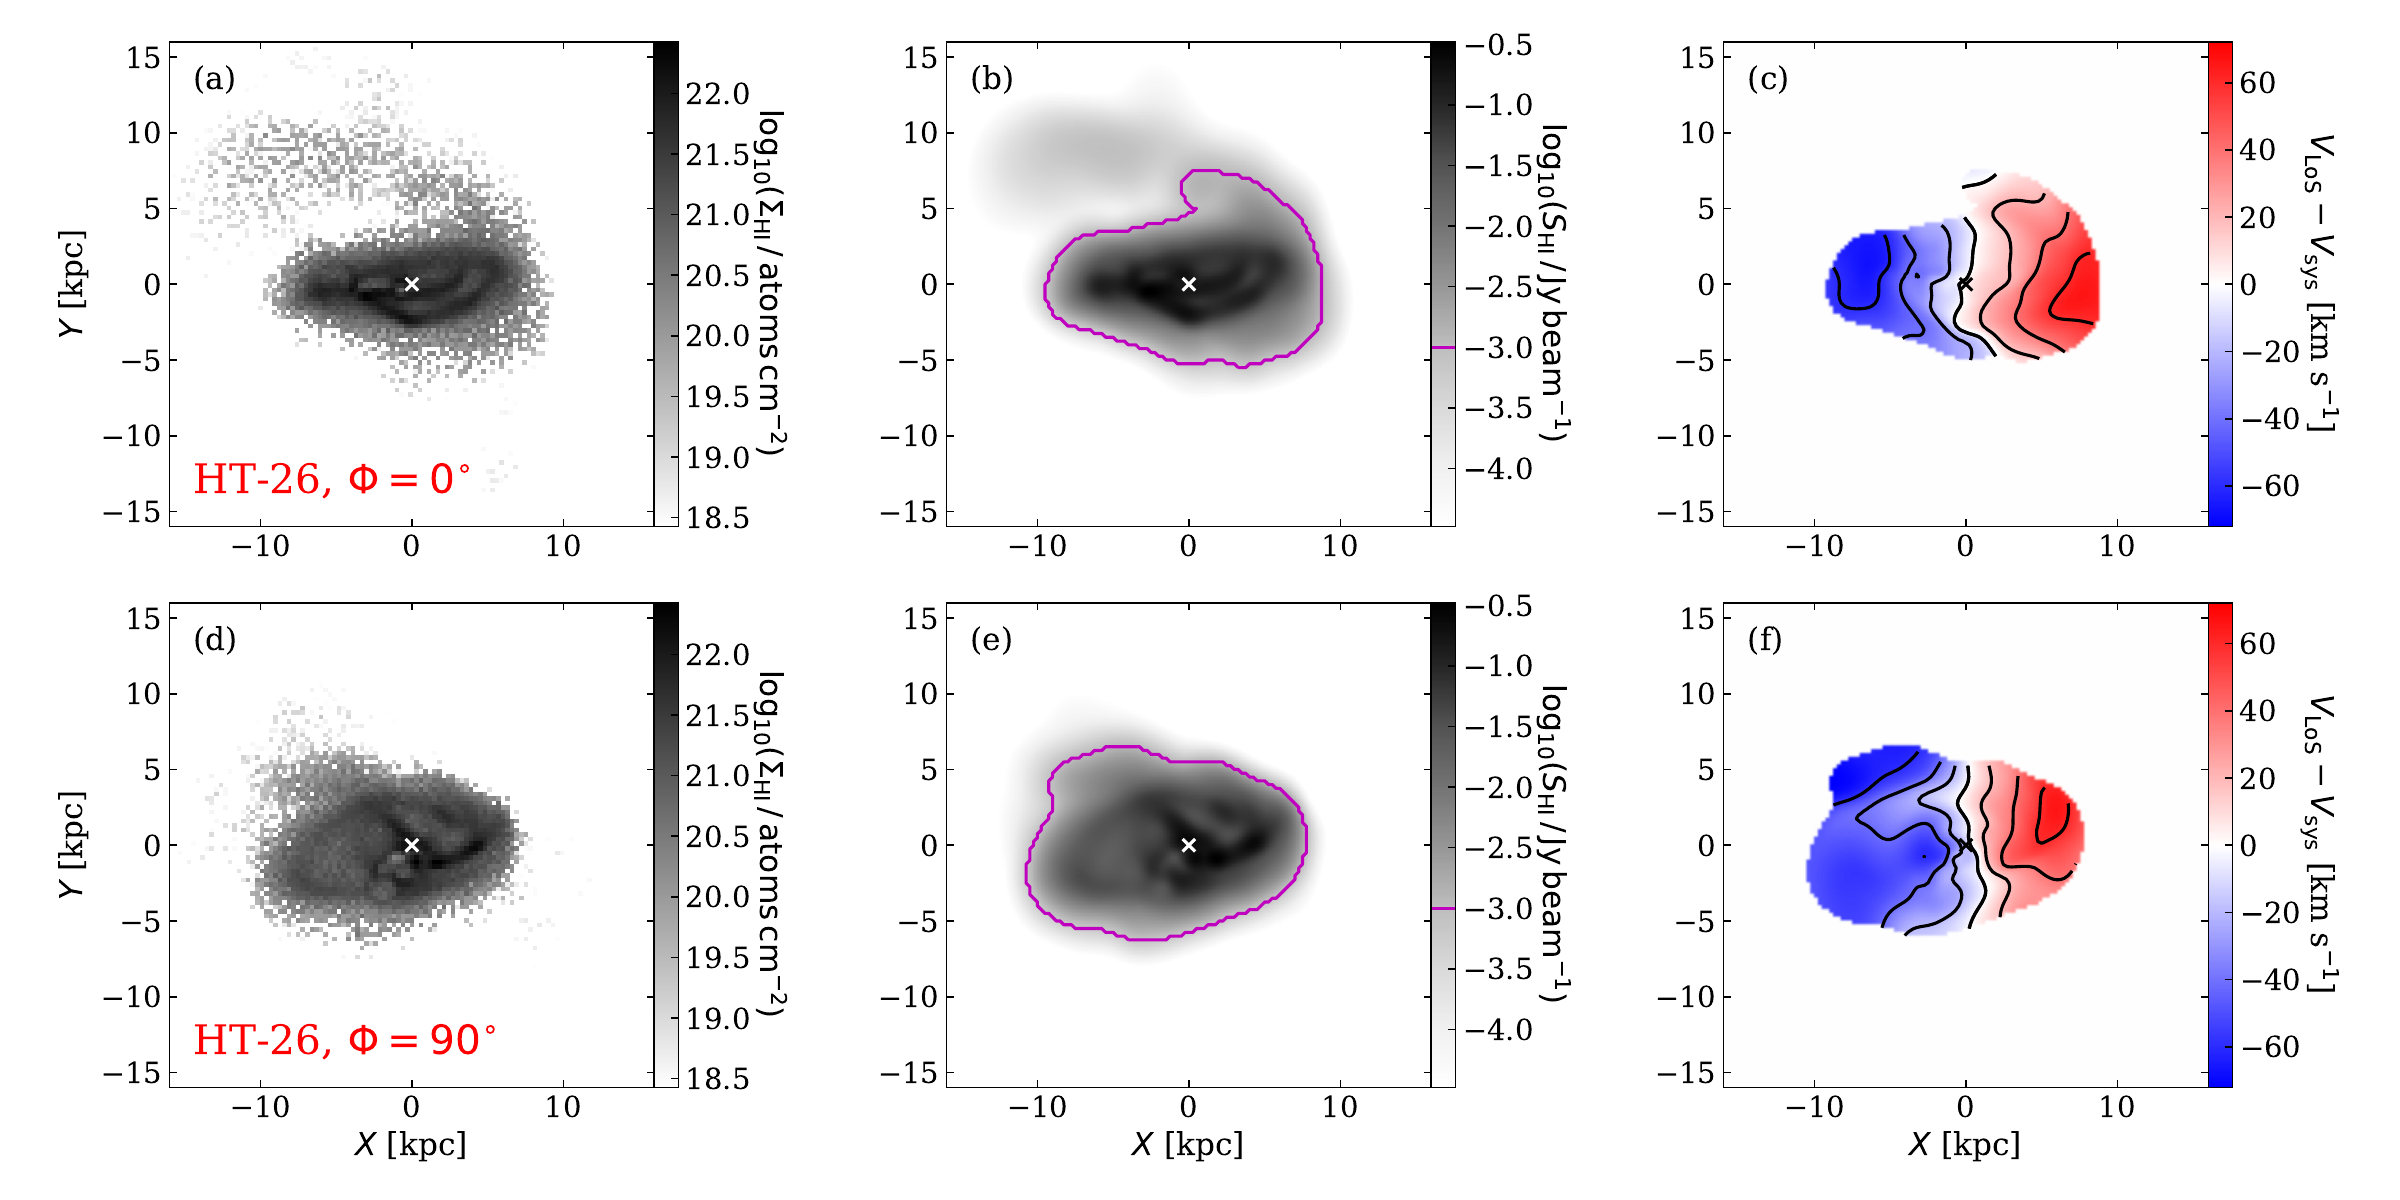}
\includegraphics[width=\textwidth]{../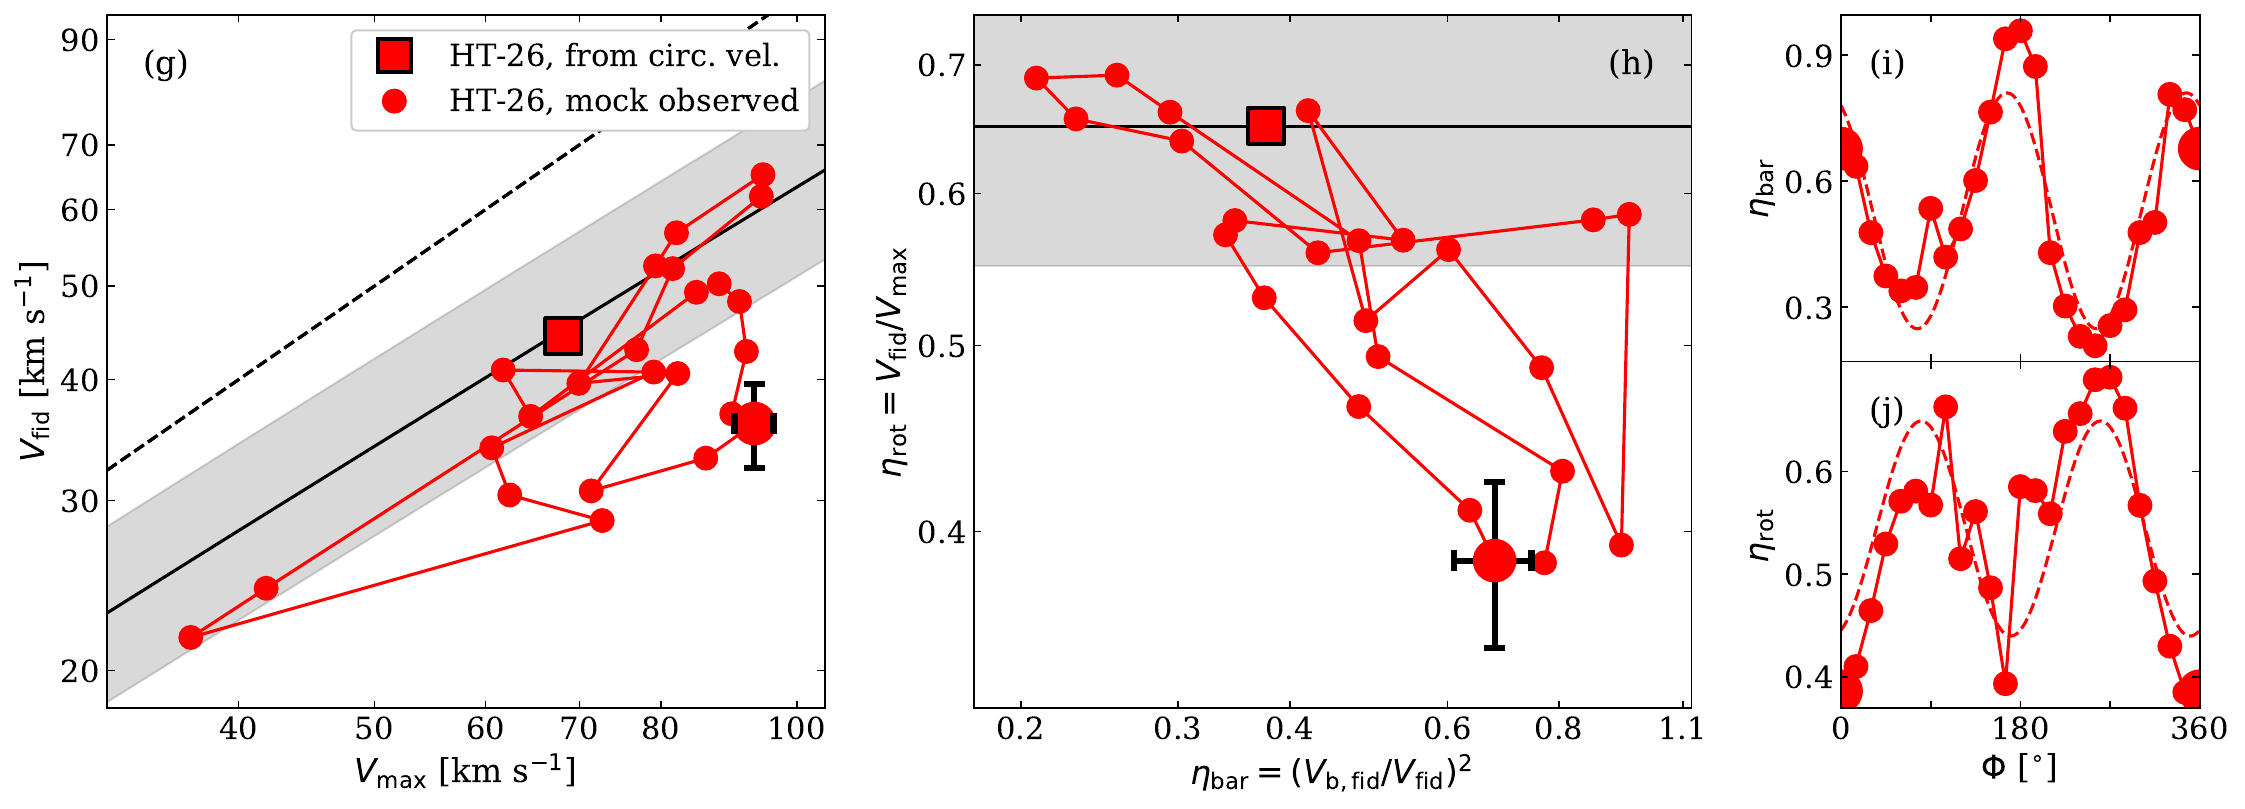}
\end{minipage}
\begin{minipage}{.4\textwidth}
\includegraphics[width=\textwidth]{../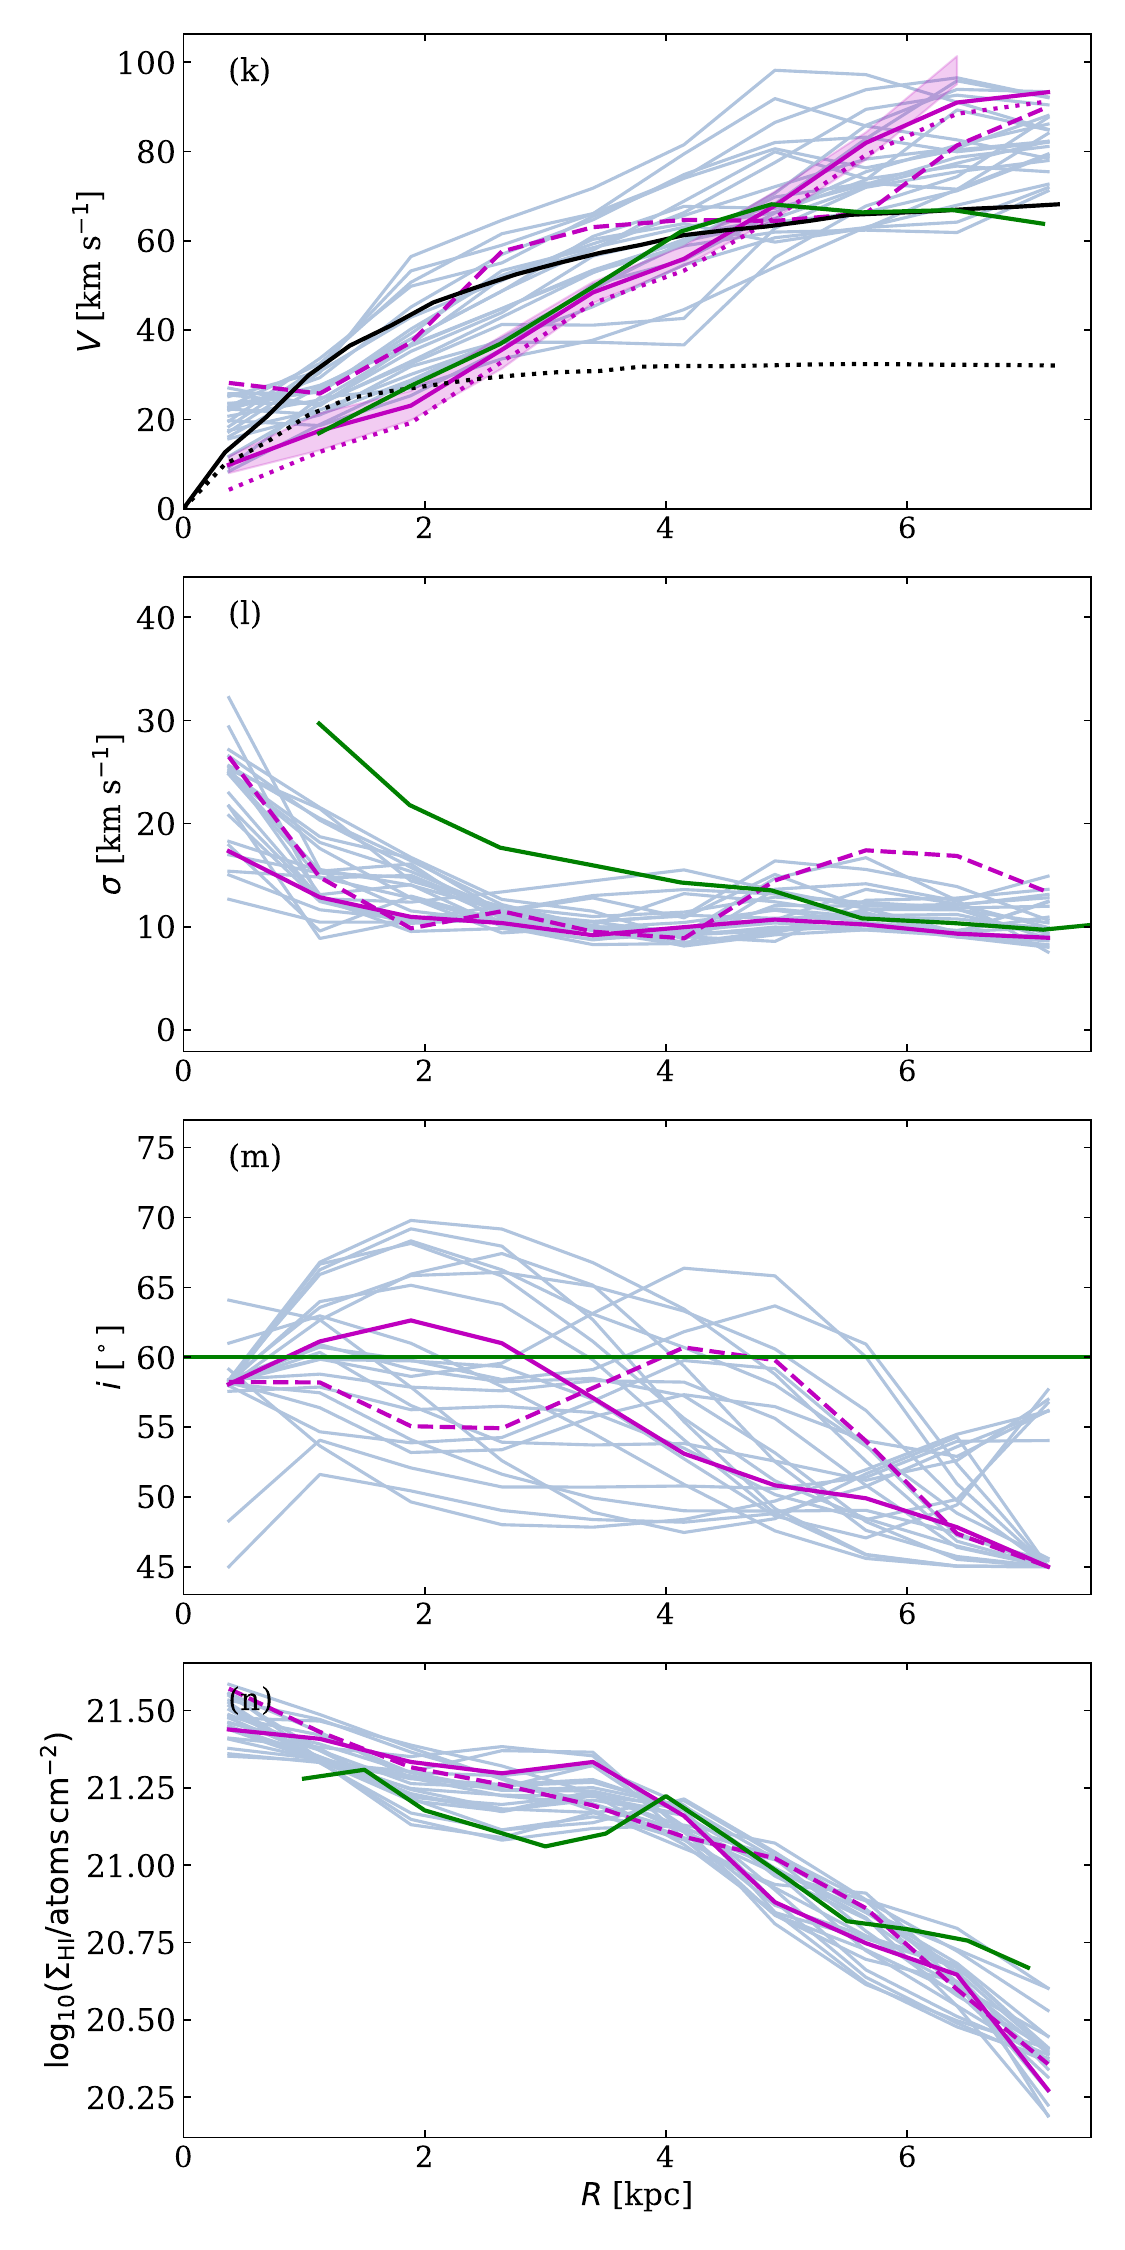}
\end{minipage}
\caption{A set of summary figures for galaxy HT-26, selected for kinematic analysis. These include example moment maps for two orientations (panels (a)--(f); similar to Fig.~\ref{fig:visualisations}), a summary of the parameters $V_\mathrm{fid}$, $V_\mathrm{max}$, $\eta_\mathrm{rot}$, and $\eta_\mathrm{bar}$ (panels (g)--(j); similar to Fig.~\ref{fig:loops}), and a summary of the rotation curve analysis from $24$ viewing angles (panels (k)--(n); similar to Fig.~\ref{fig:rot_curves}). See description of Appendix~\ref{app:supplementary} for details.}
\label{fig:S50}
\end{figure}
\clearpage

\begin{figure}
\begin{minipage}{.9\textwidth}
\includegraphics[width=\textwidth]{../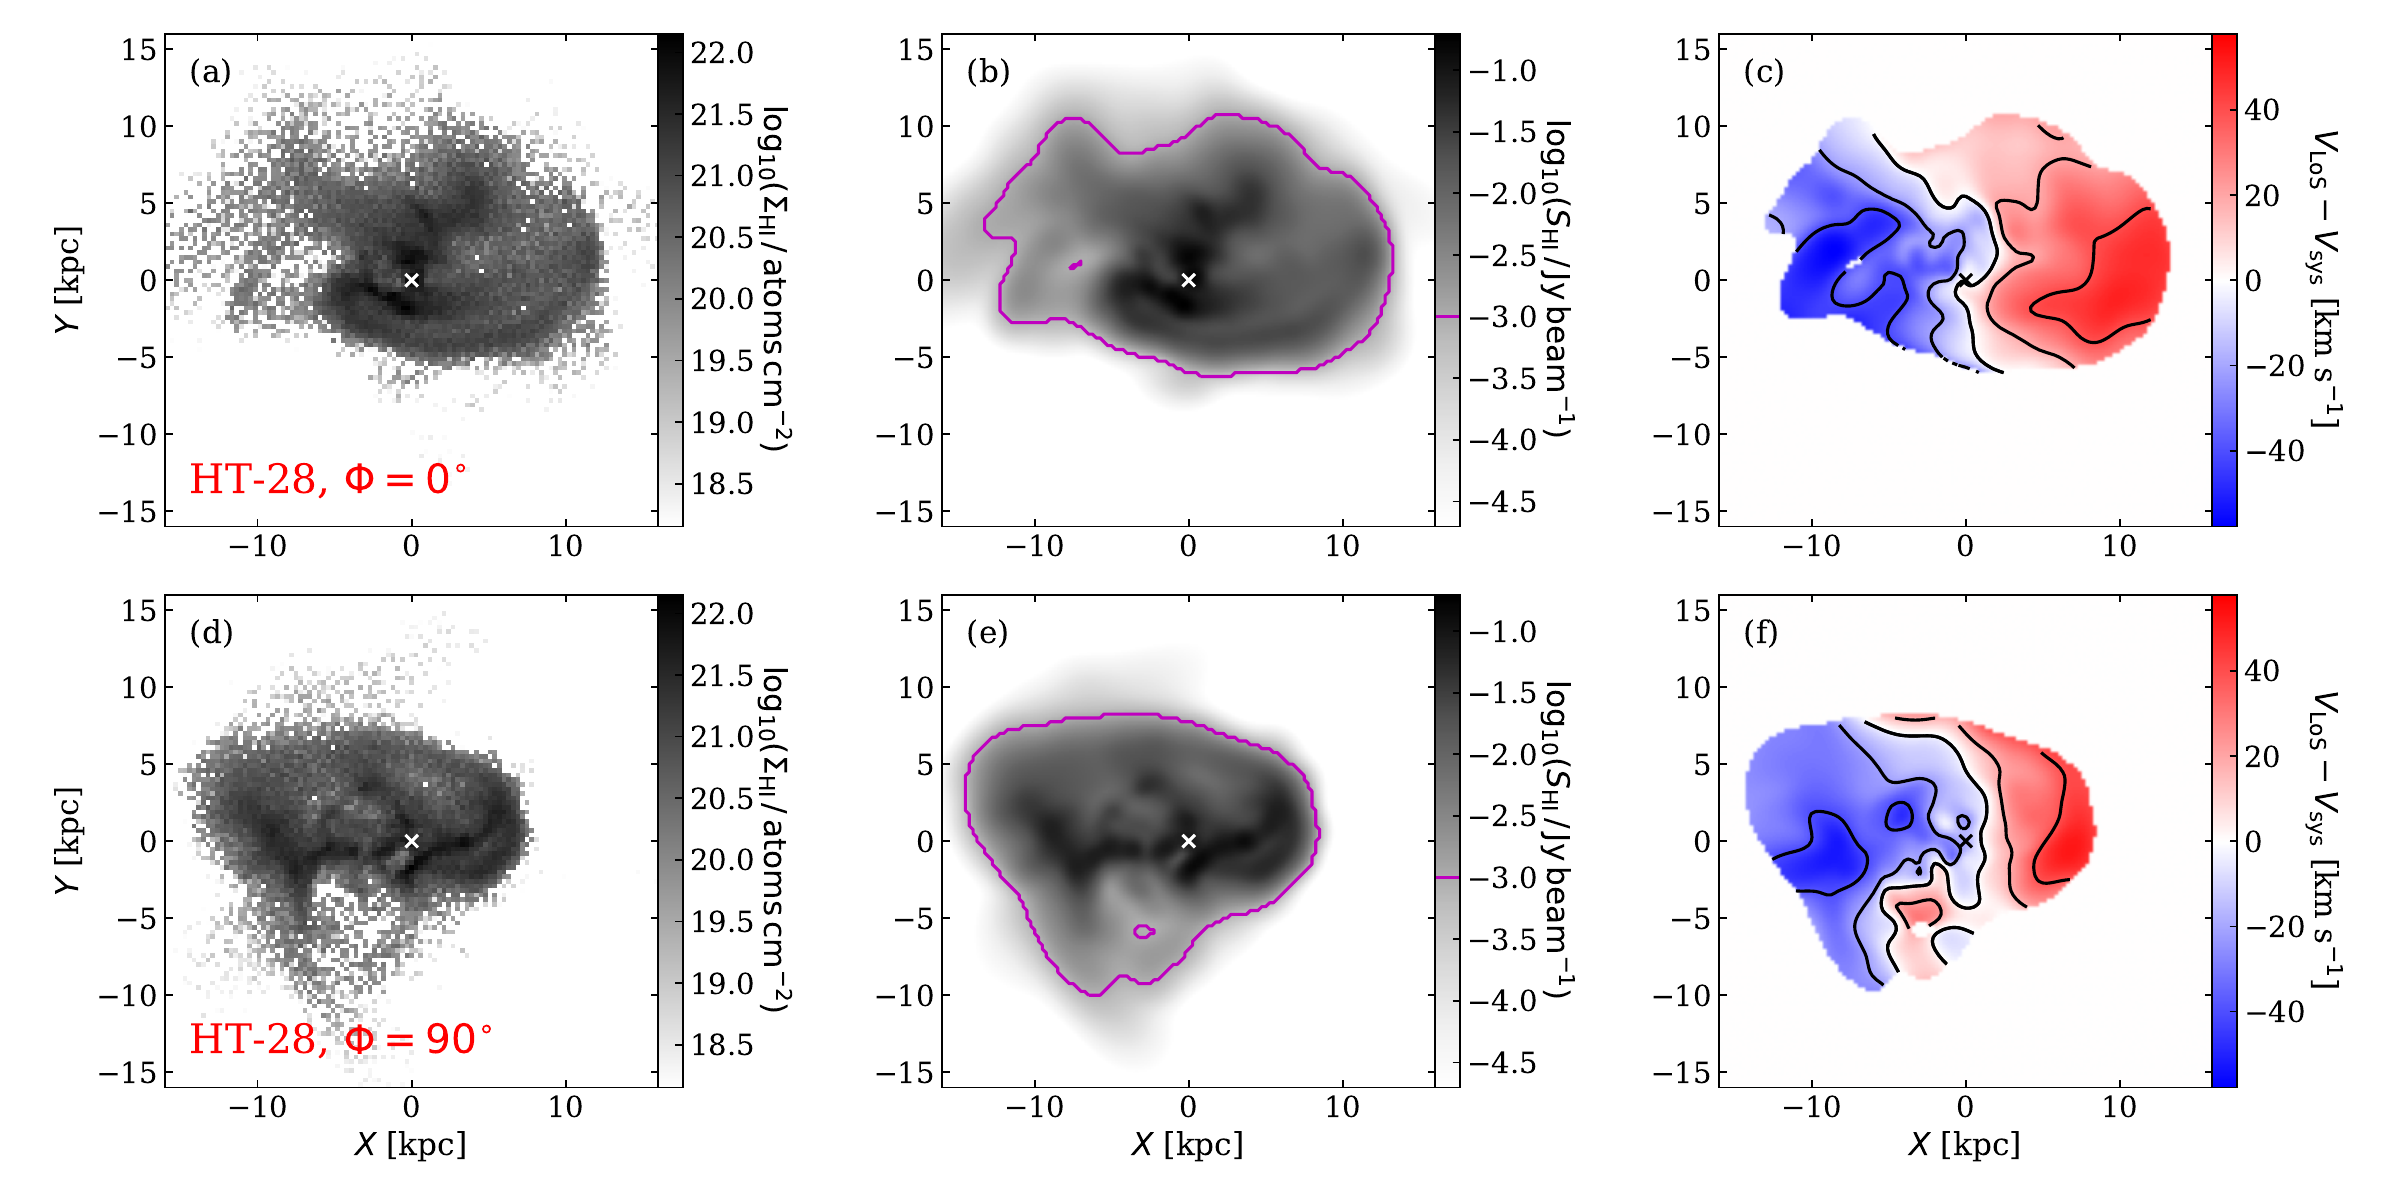}
\includegraphics[width=\textwidth]{../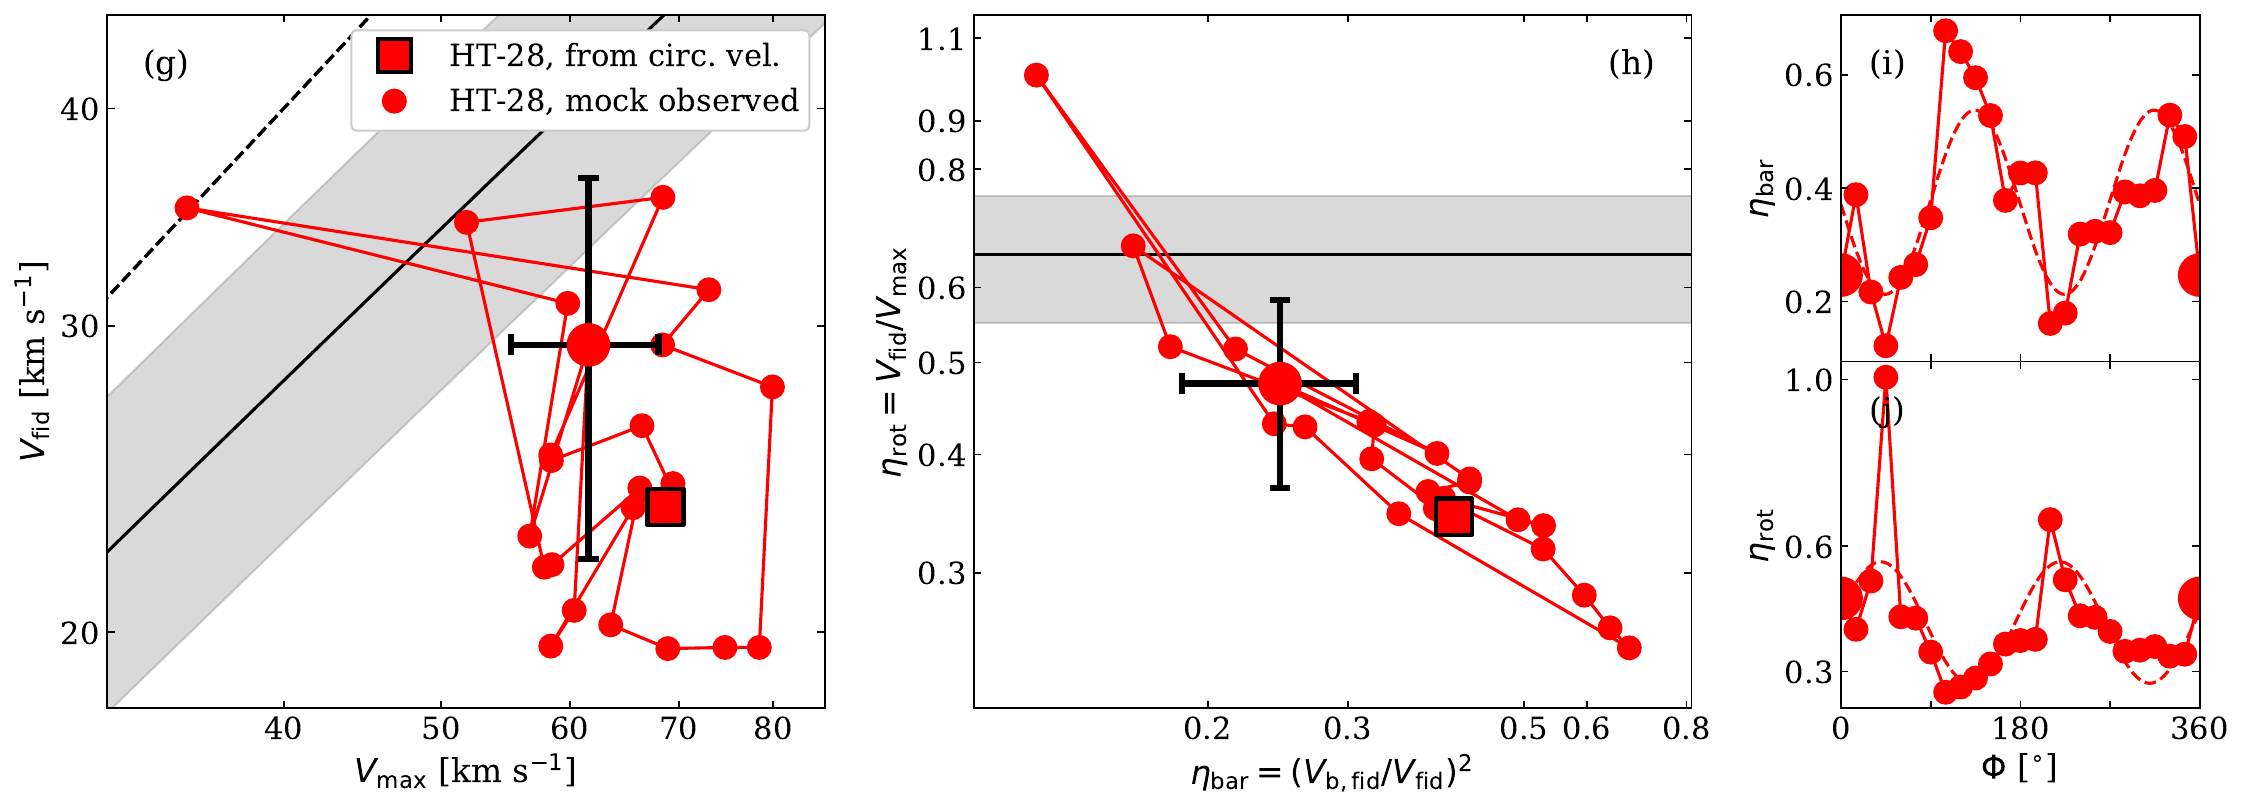}
\end{minipage}
\begin{minipage}{.4\textwidth}
\includegraphics[width=\textwidth]{../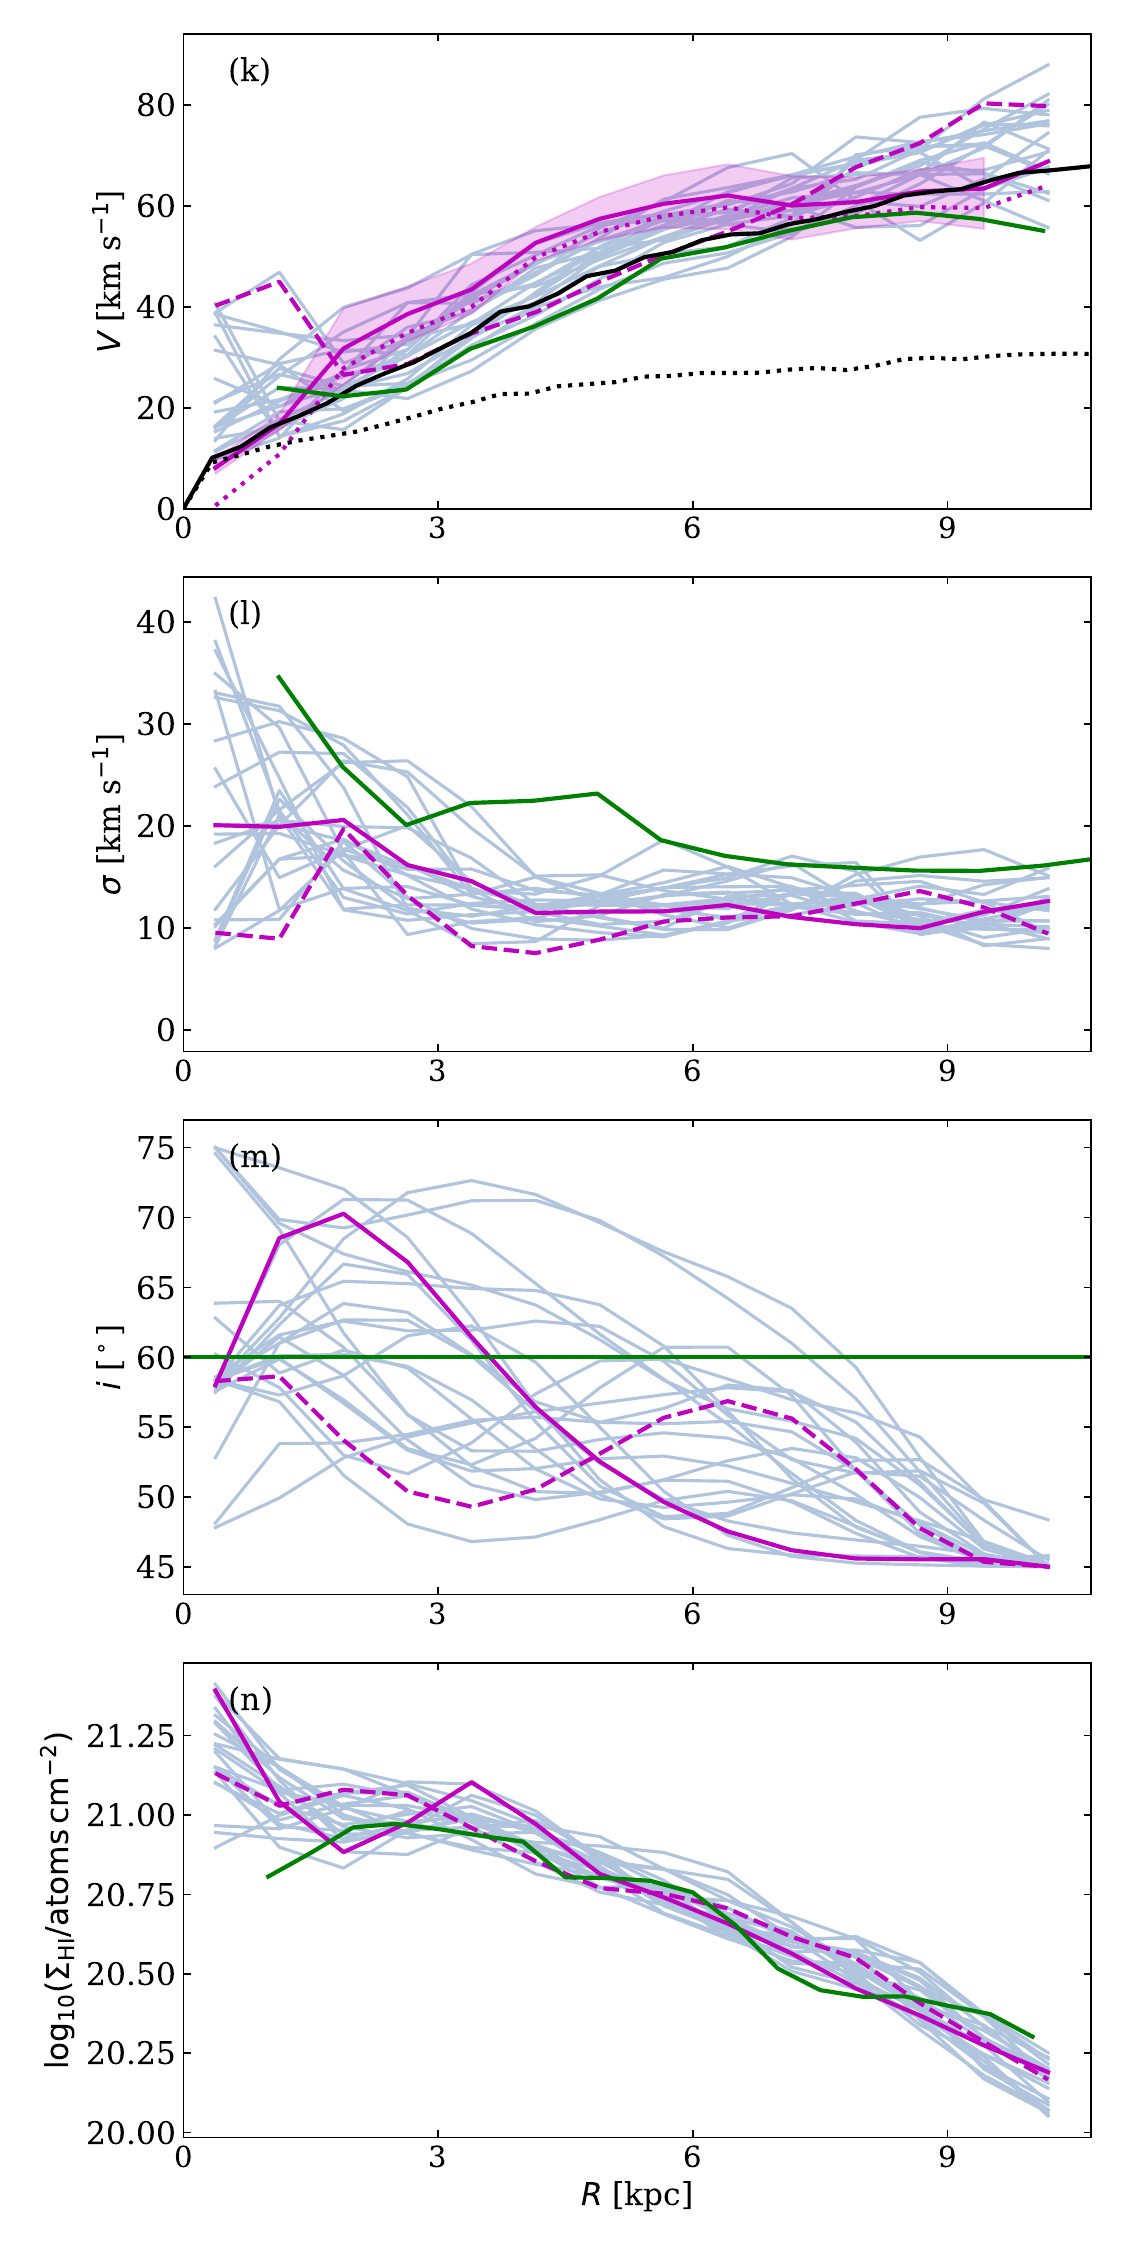}
\end{minipage}
\caption{A set of summary figures for galaxy HT-28, selected for kinematic analysis. These include example moment maps for two orientations (panels (a)--(f); similar to Fig.~\ref{fig:visualisations}), a summary of the parameters $V_\mathrm{fid}$, $V_\mathrm{max}$, $\eta_\mathrm{rot}$, and $\eta_\mathrm{bar}$ (panels (g)--(j); similar to Fig.~\ref{fig:loops}), and a summary of the rotation curve analysis from $24$ viewing angles (panels (k)--(n); similar to Fig.~\ref{fig:rot_curves}). See description of Appendix~\ref{app:supplementary} for details.}
\label{fig:S51}
\end{figure}
\clearpage

\begin{figure}
\begin{minipage}{.9\textwidth}
\includegraphics[width=\textwidth]{../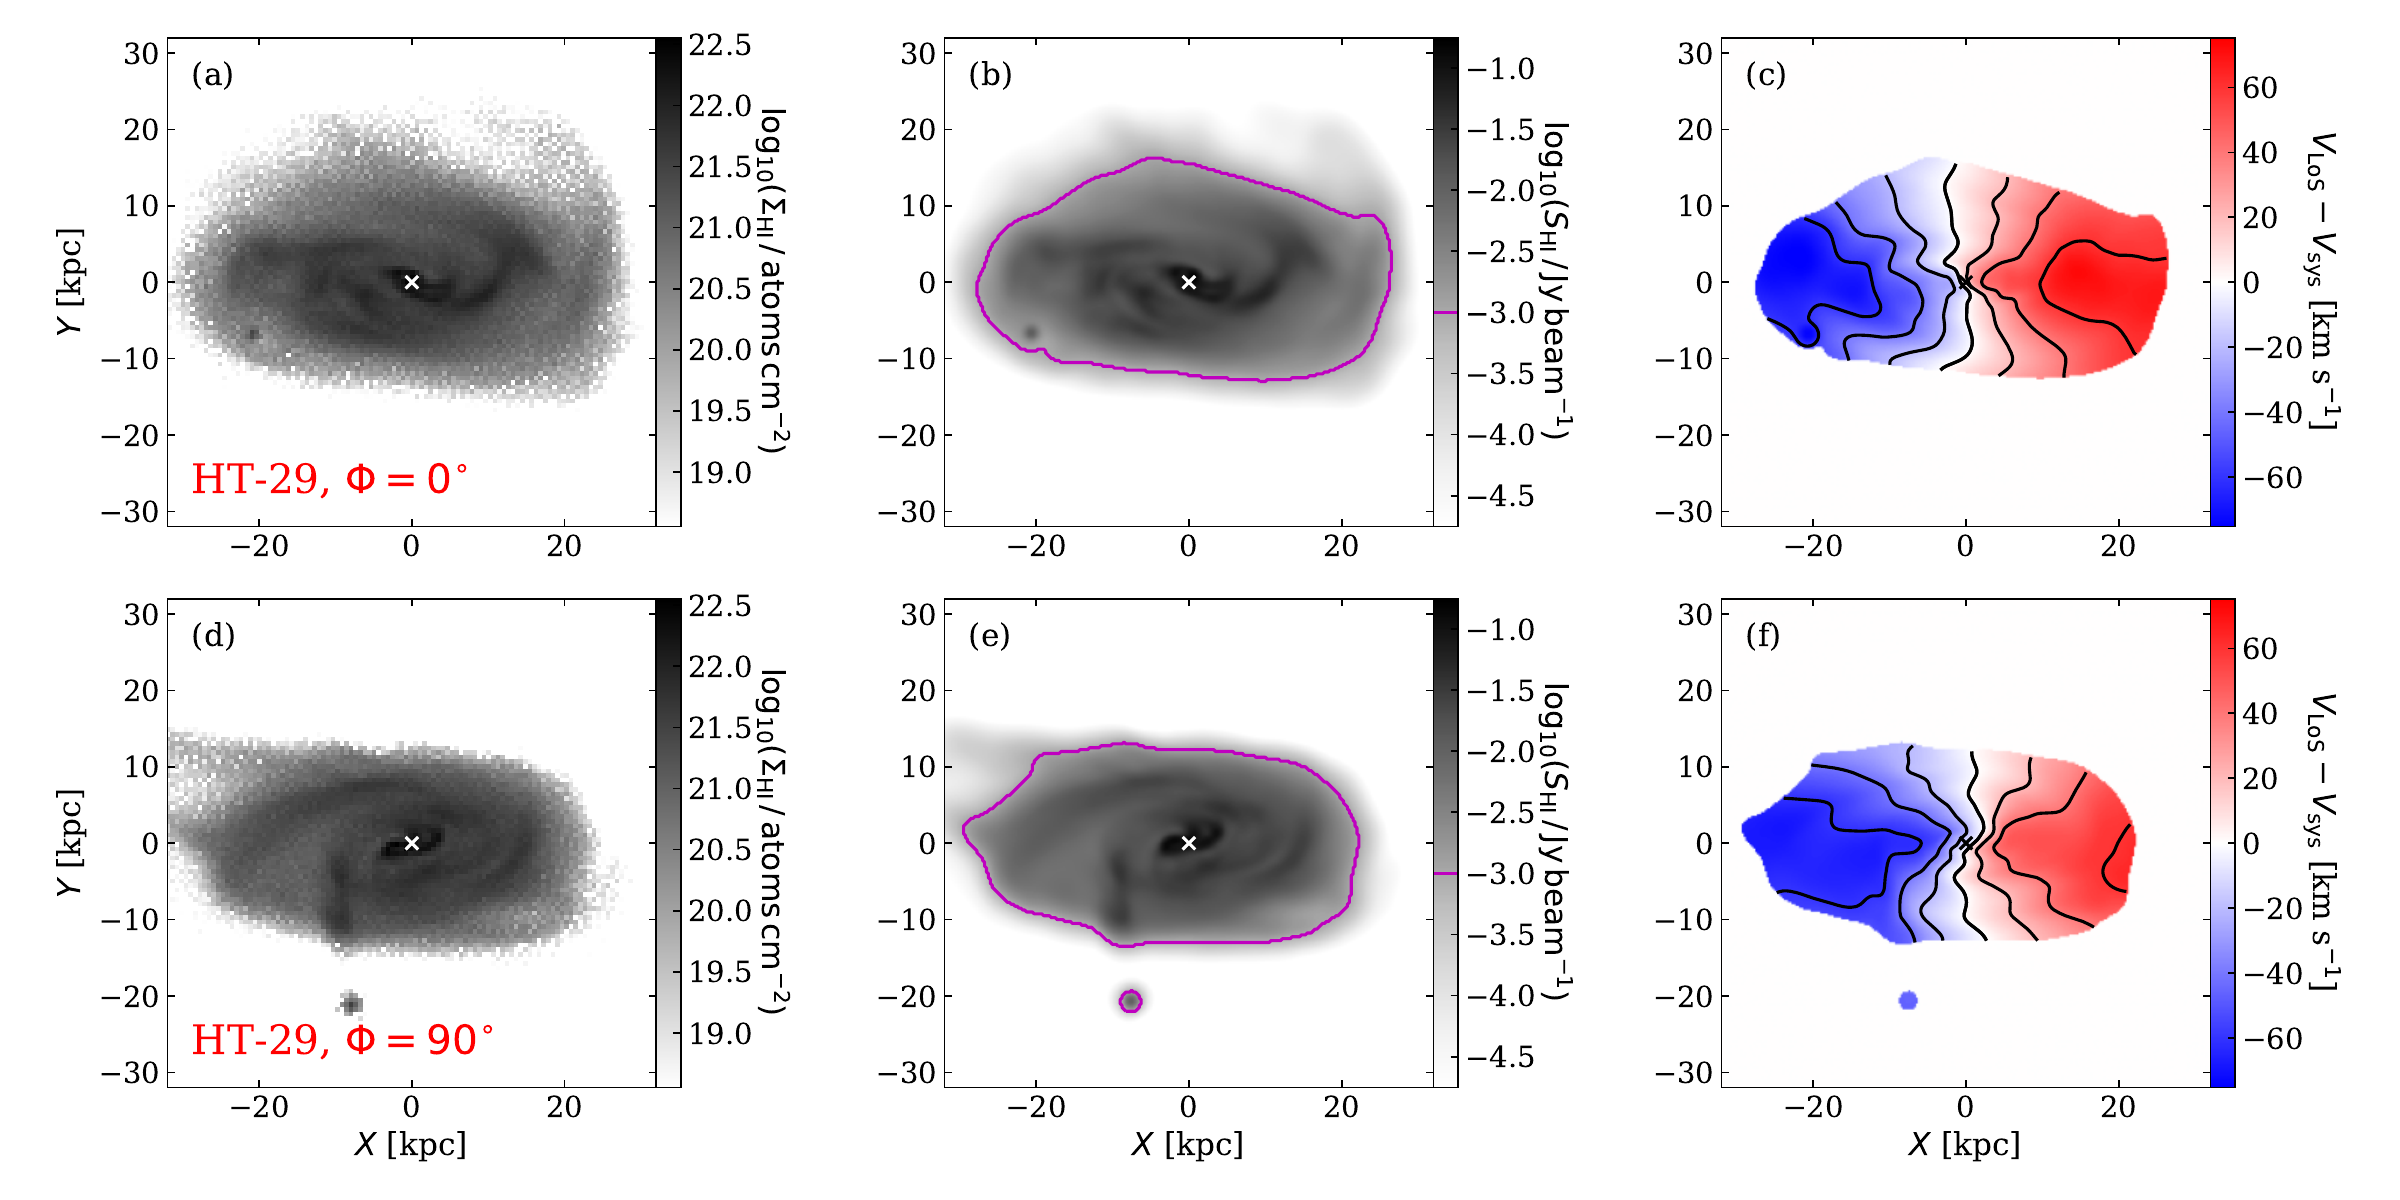}
\includegraphics[width=\textwidth]{../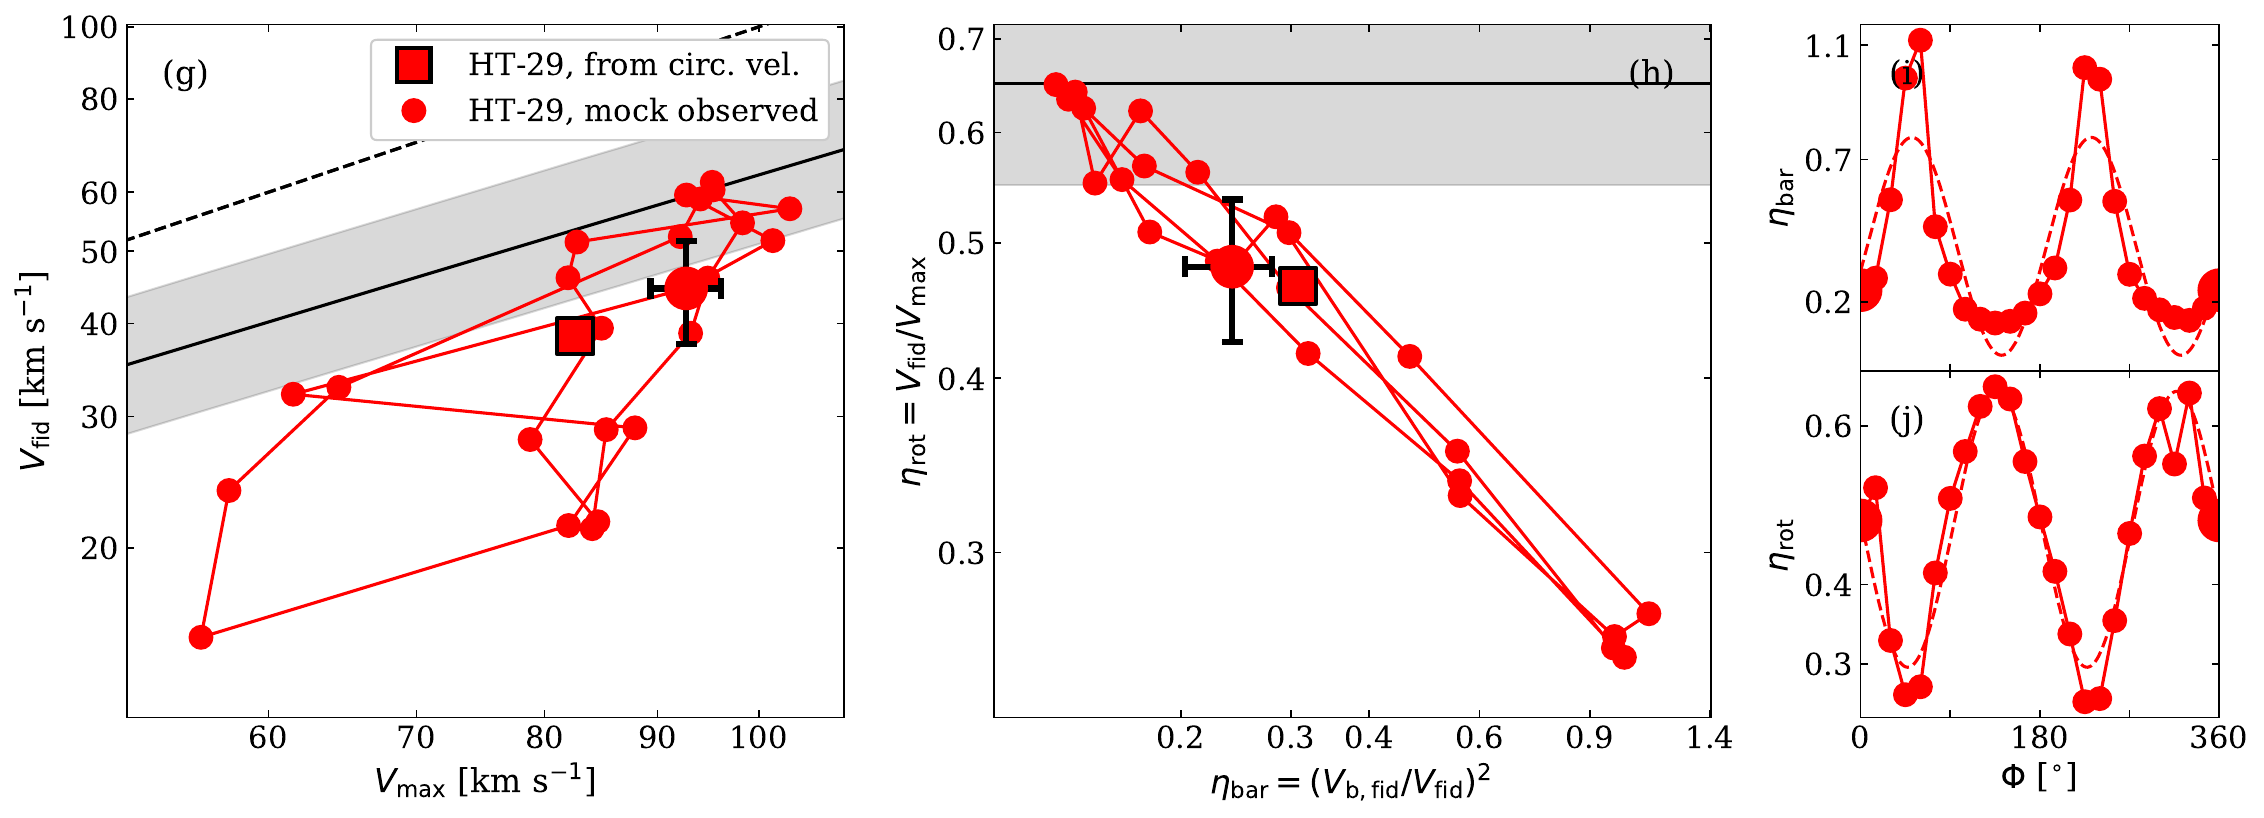}
\end{minipage}
\begin{minipage}{.4\textwidth}
\includegraphics[width=\textwidth]{../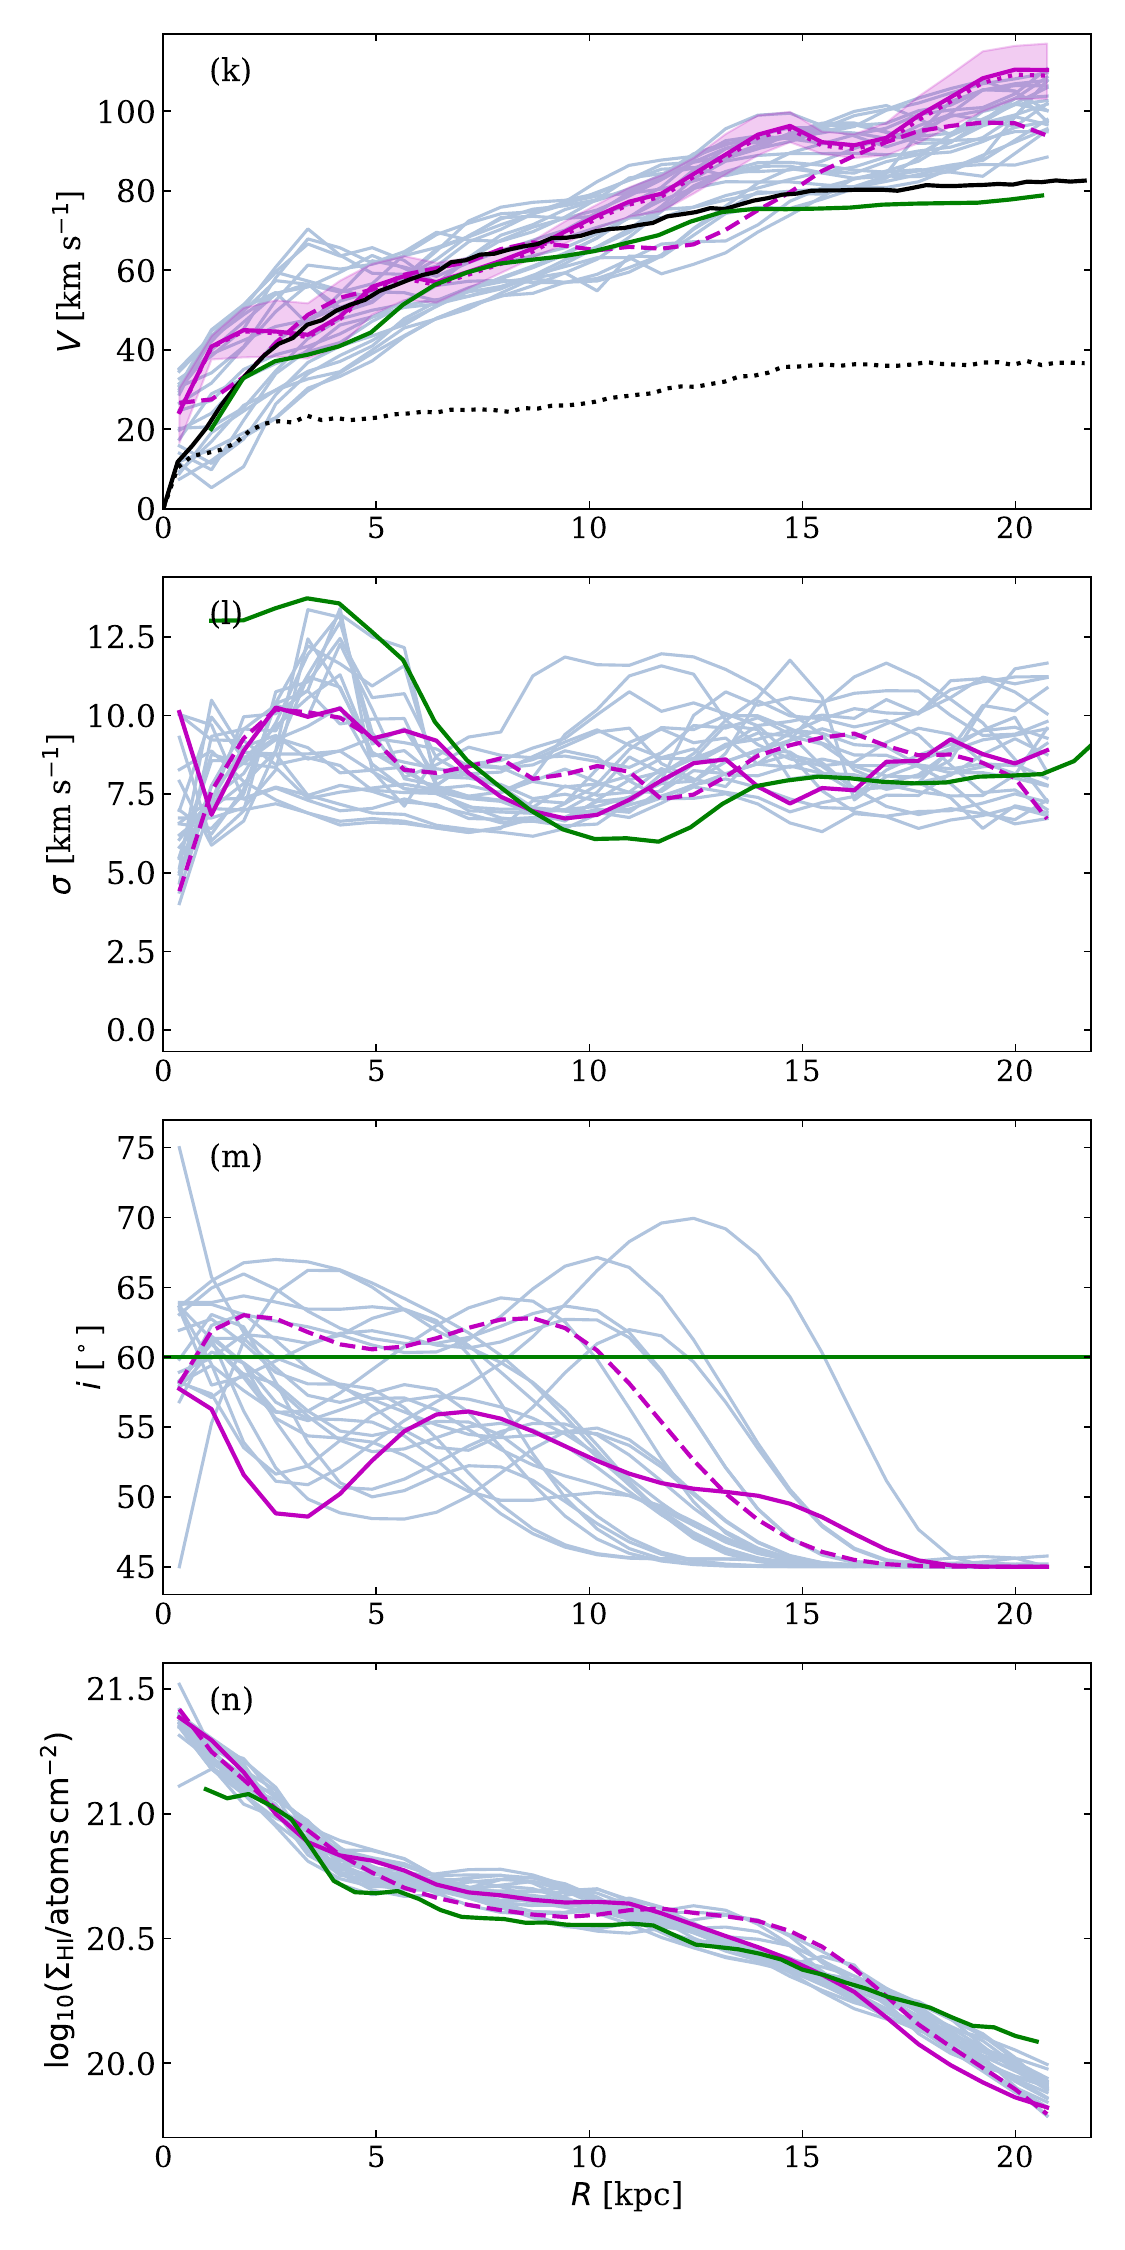}
\end{minipage}
\caption{A set of summary figures for galaxy HT-29, selected for kinematic analysis. These include example moment maps for two orientations (panels (a)--(f); similar to Fig.~\ref{fig:visualisations}), a summary of the parameters $V_\mathrm{fid}$, $V_\mathrm{max}$, $\eta_\mathrm{rot}$, and $\eta_\mathrm{bar}$ (panels (g)--(j); similar to Fig.~\ref{fig:loops}), and a summary of the rotation curve analysis from $24$ viewing angles (panels (k)--(n); similar to Fig.~\ref{fig:rot_curves}). See description of Appendix~\ref{app:supplementary} for details.}
\label{fig:S52}
\end{figure}
\clearpage

\begin{figure}
\begin{minipage}{.9\textwidth}
\includegraphics[width=\textwidth]{../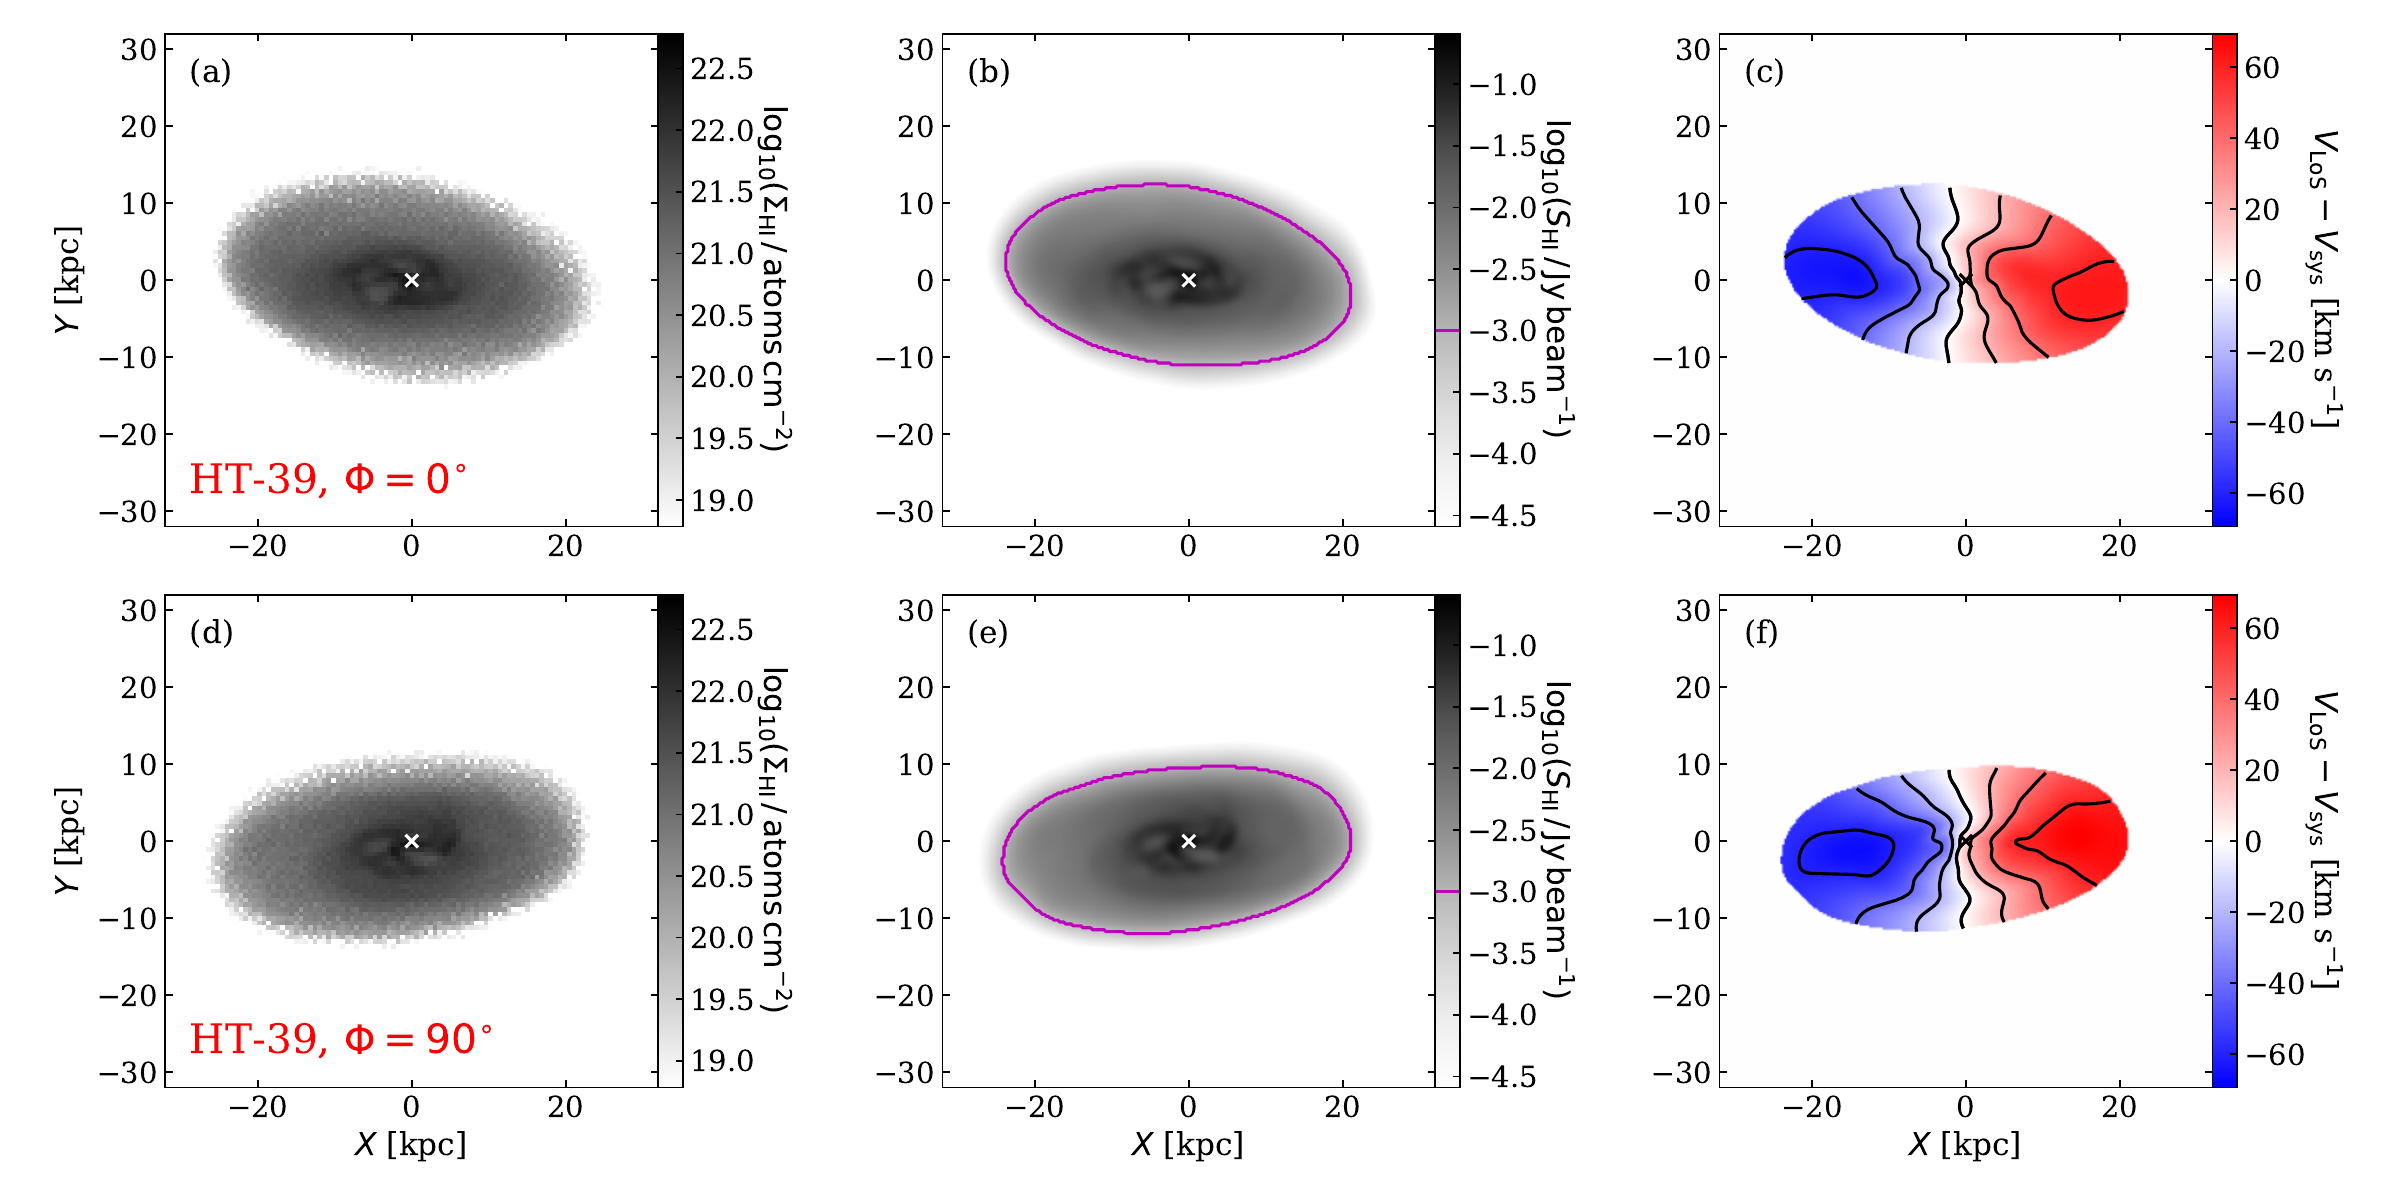}
\includegraphics[width=\textwidth]{../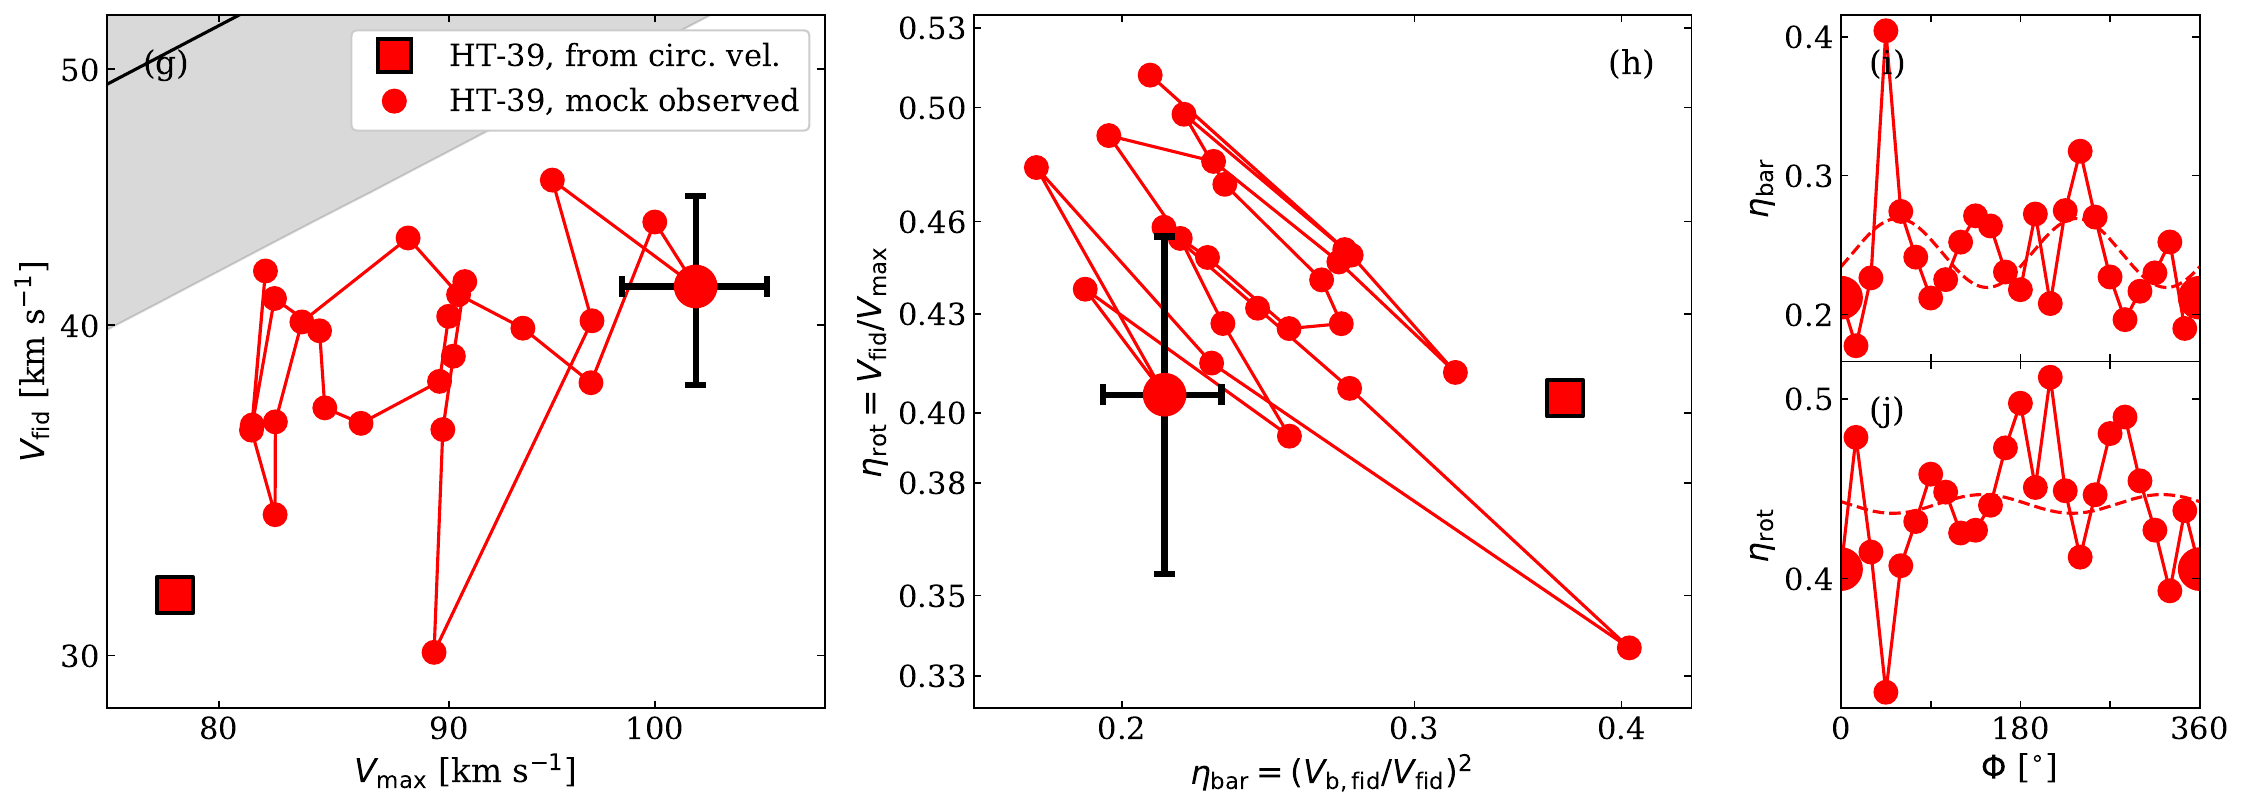}
\end{minipage}
\begin{minipage}{.4\textwidth}
\includegraphics[width=\textwidth]{../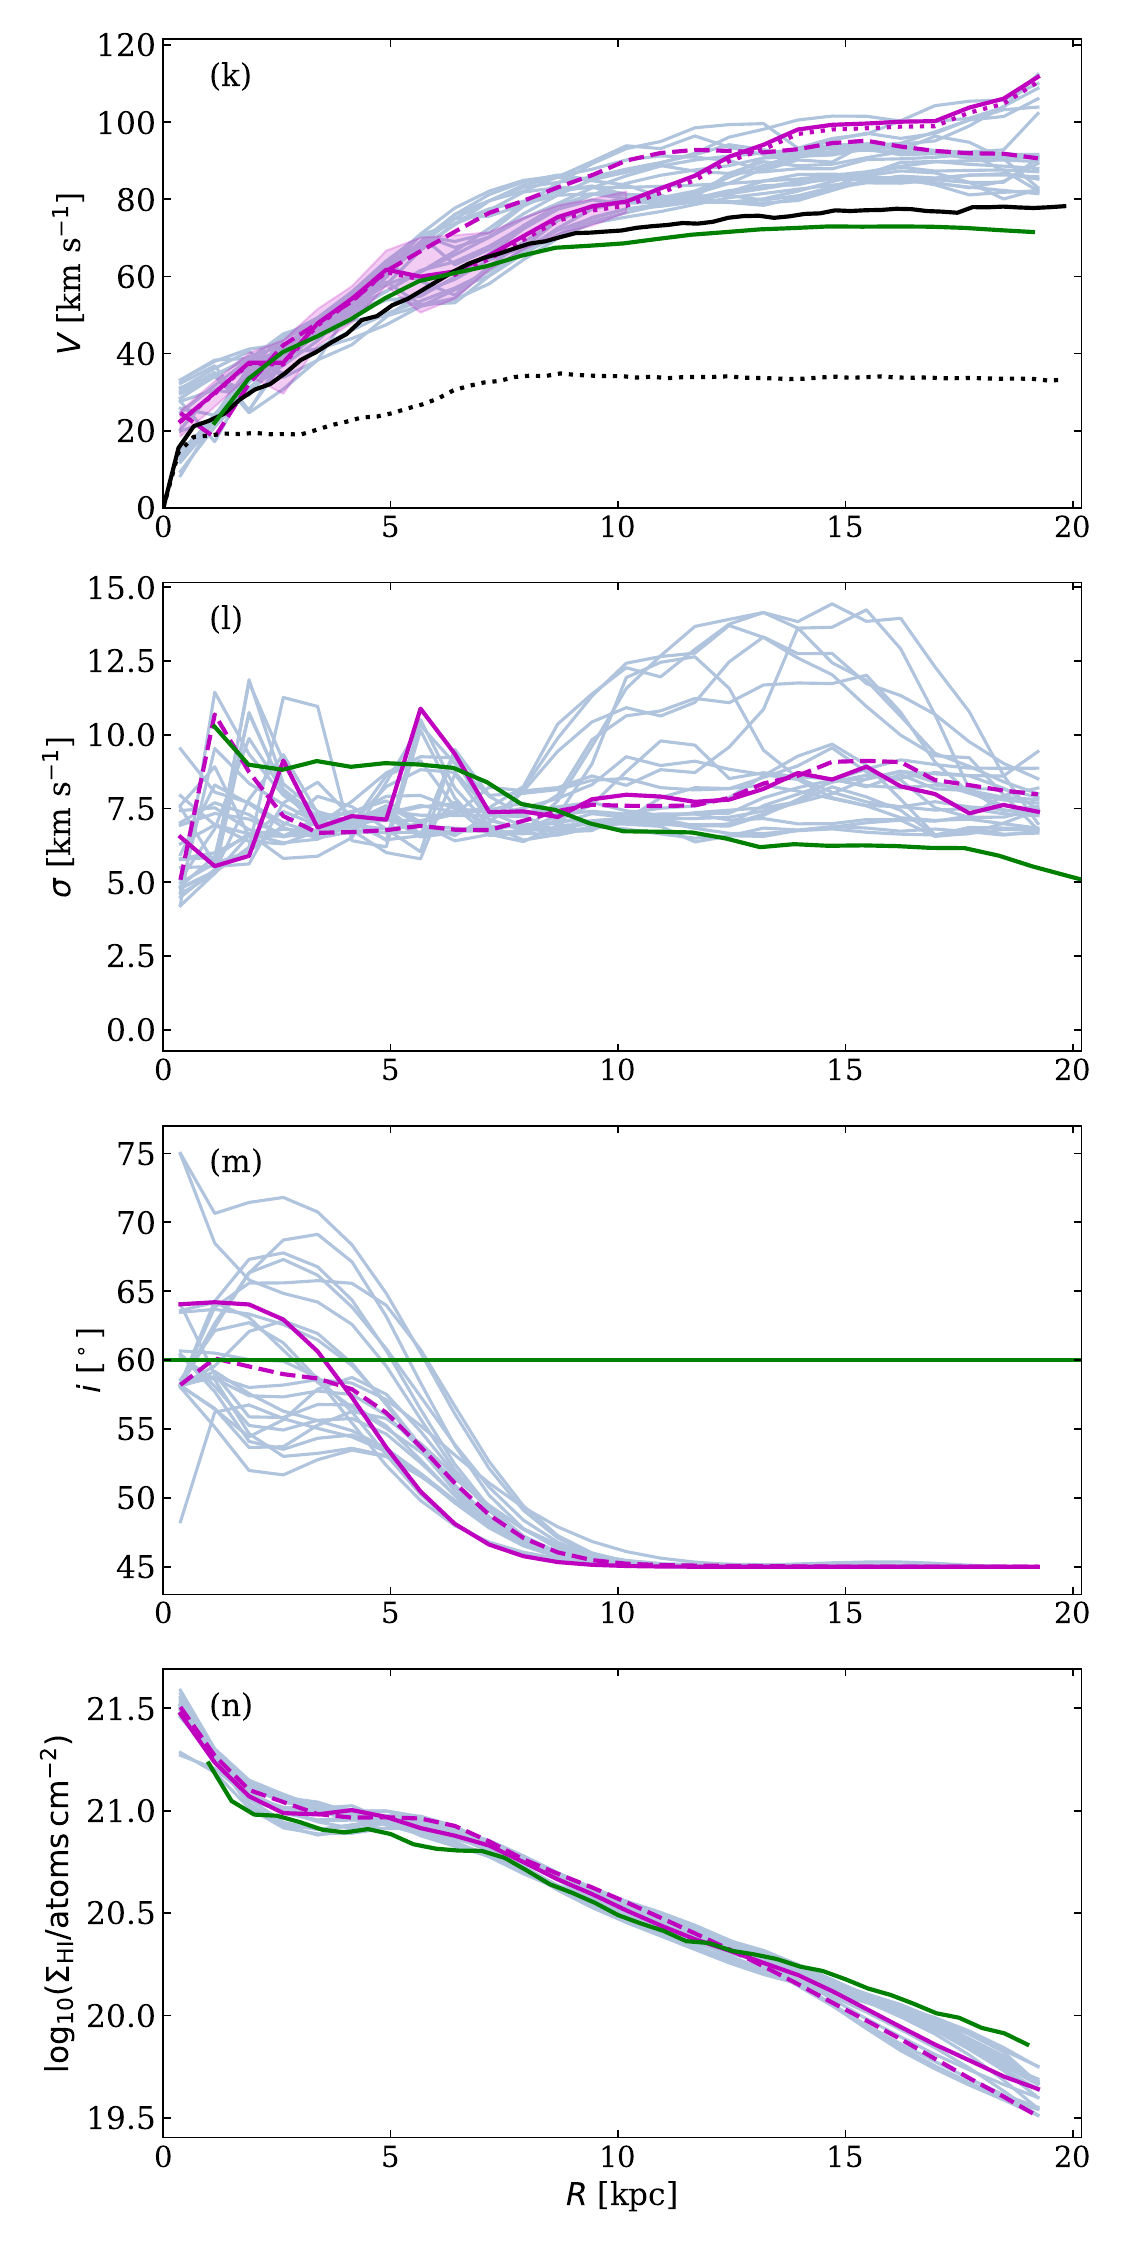}
\end{minipage}
\caption{A set of summary figures for galaxy HT-39, selected for kinematic analysis. These include example moment maps for two orientations (panels (a)--(f); similar to Fig.~\ref{fig:visualisations}), a summary of the parameters $V_\mathrm{fid}$, $V_\mathrm{max}$, $\eta_\mathrm{rot}$, and $\eta_\mathrm{bar}$ (panels (g)--(j); similar to Fig.~\ref{fig:loops}), and a summary of the rotation curve analysis from $24$ viewing angles (panels (k)--(n); similar to Fig.~\ref{fig:rot_curves}). See description of Appendix~\ref{app:supplementary} for details.}
\label{fig:S53}
\end{figure}
\clearpage

\begin{figure}
\begin{minipage}{.9\textwidth}
\includegraphics[width=\textwidth]{../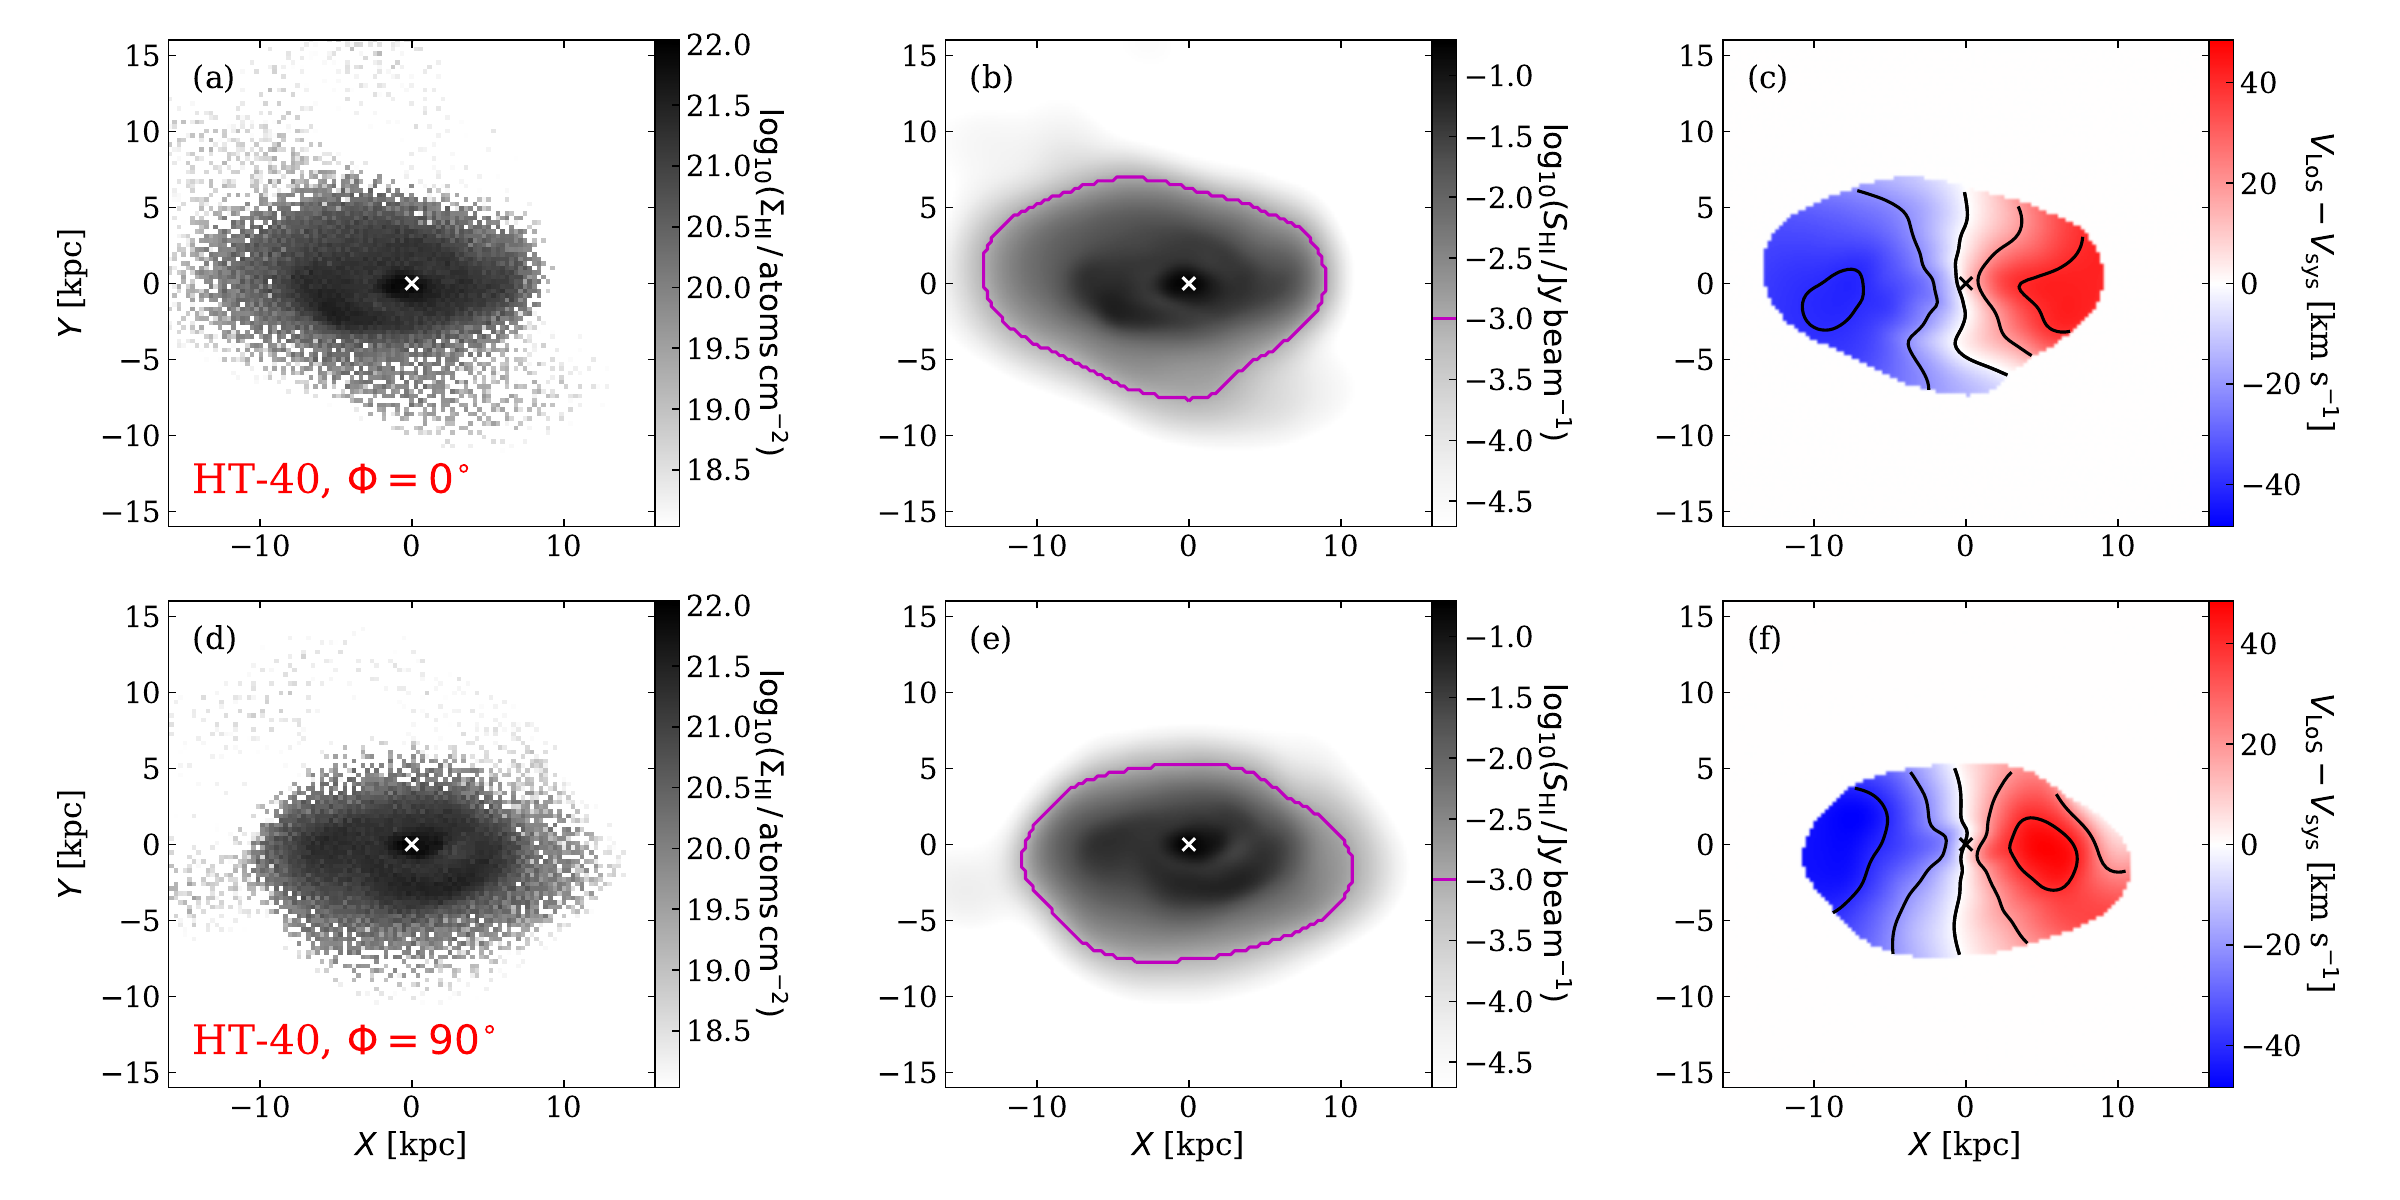}
\includegraphics[width=\textwidth]{../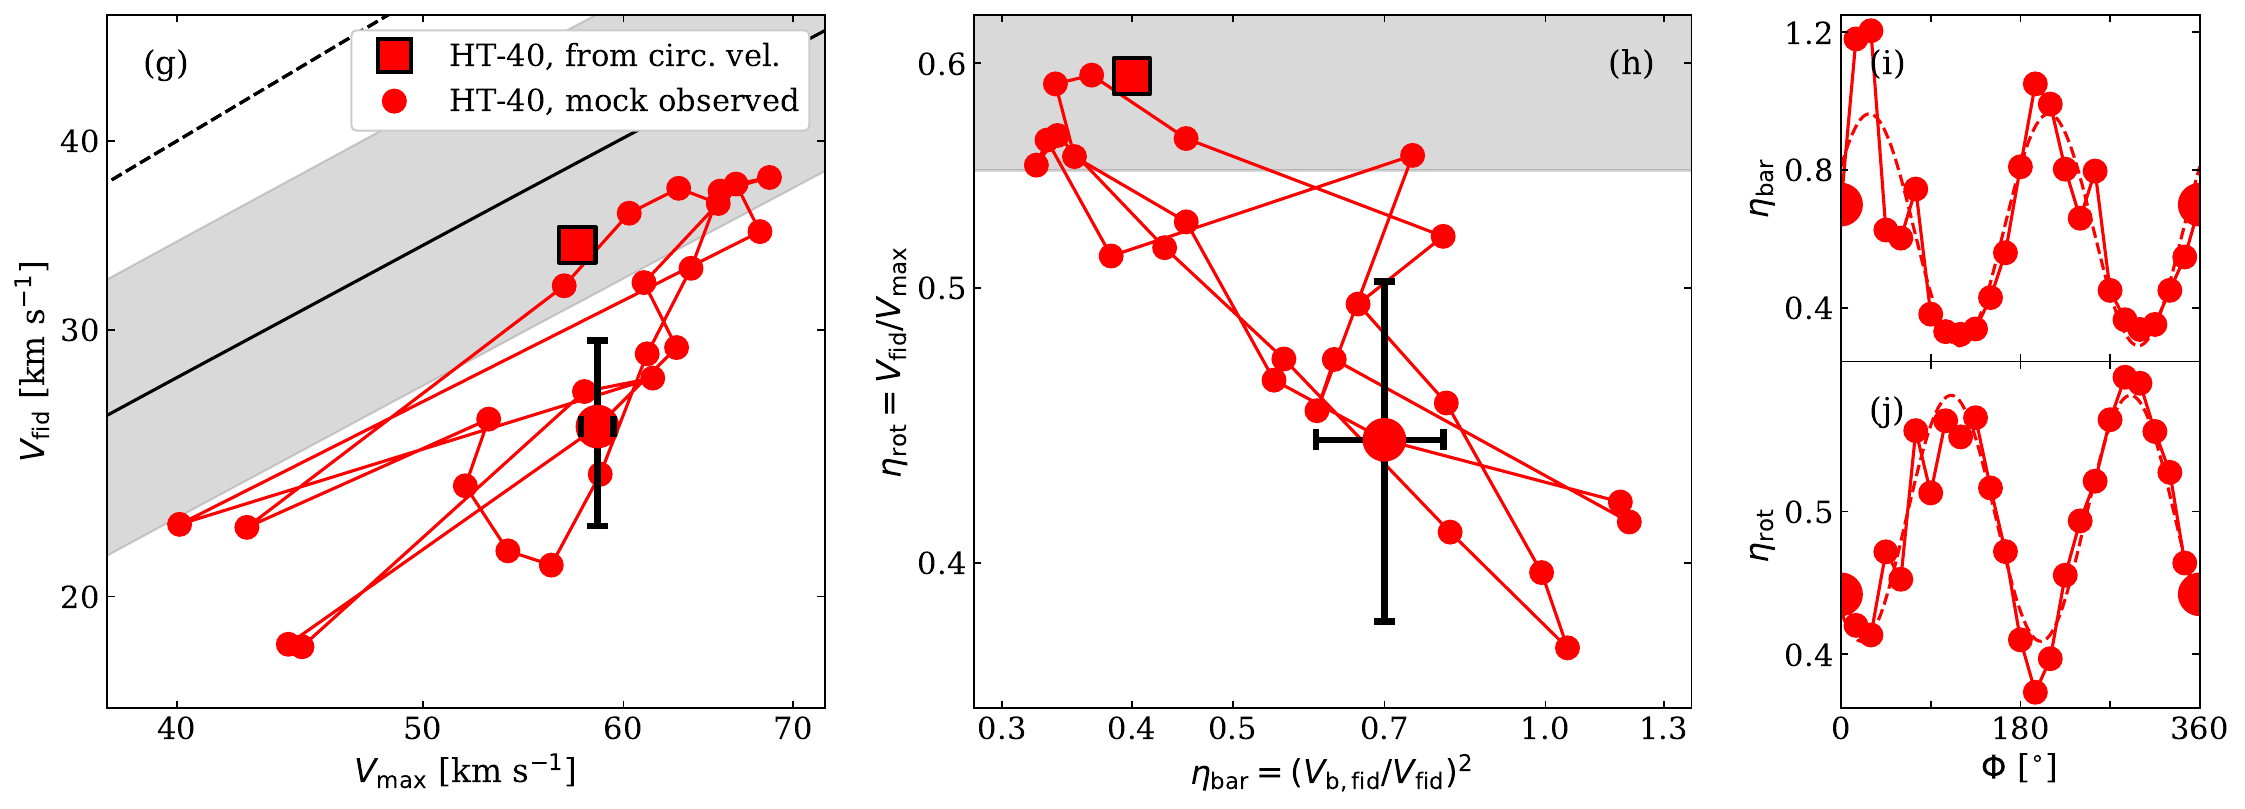}
\end{minipage}
\begin{minipage}{.4\textwidth}
\includegraphics[width=\textwidth]{../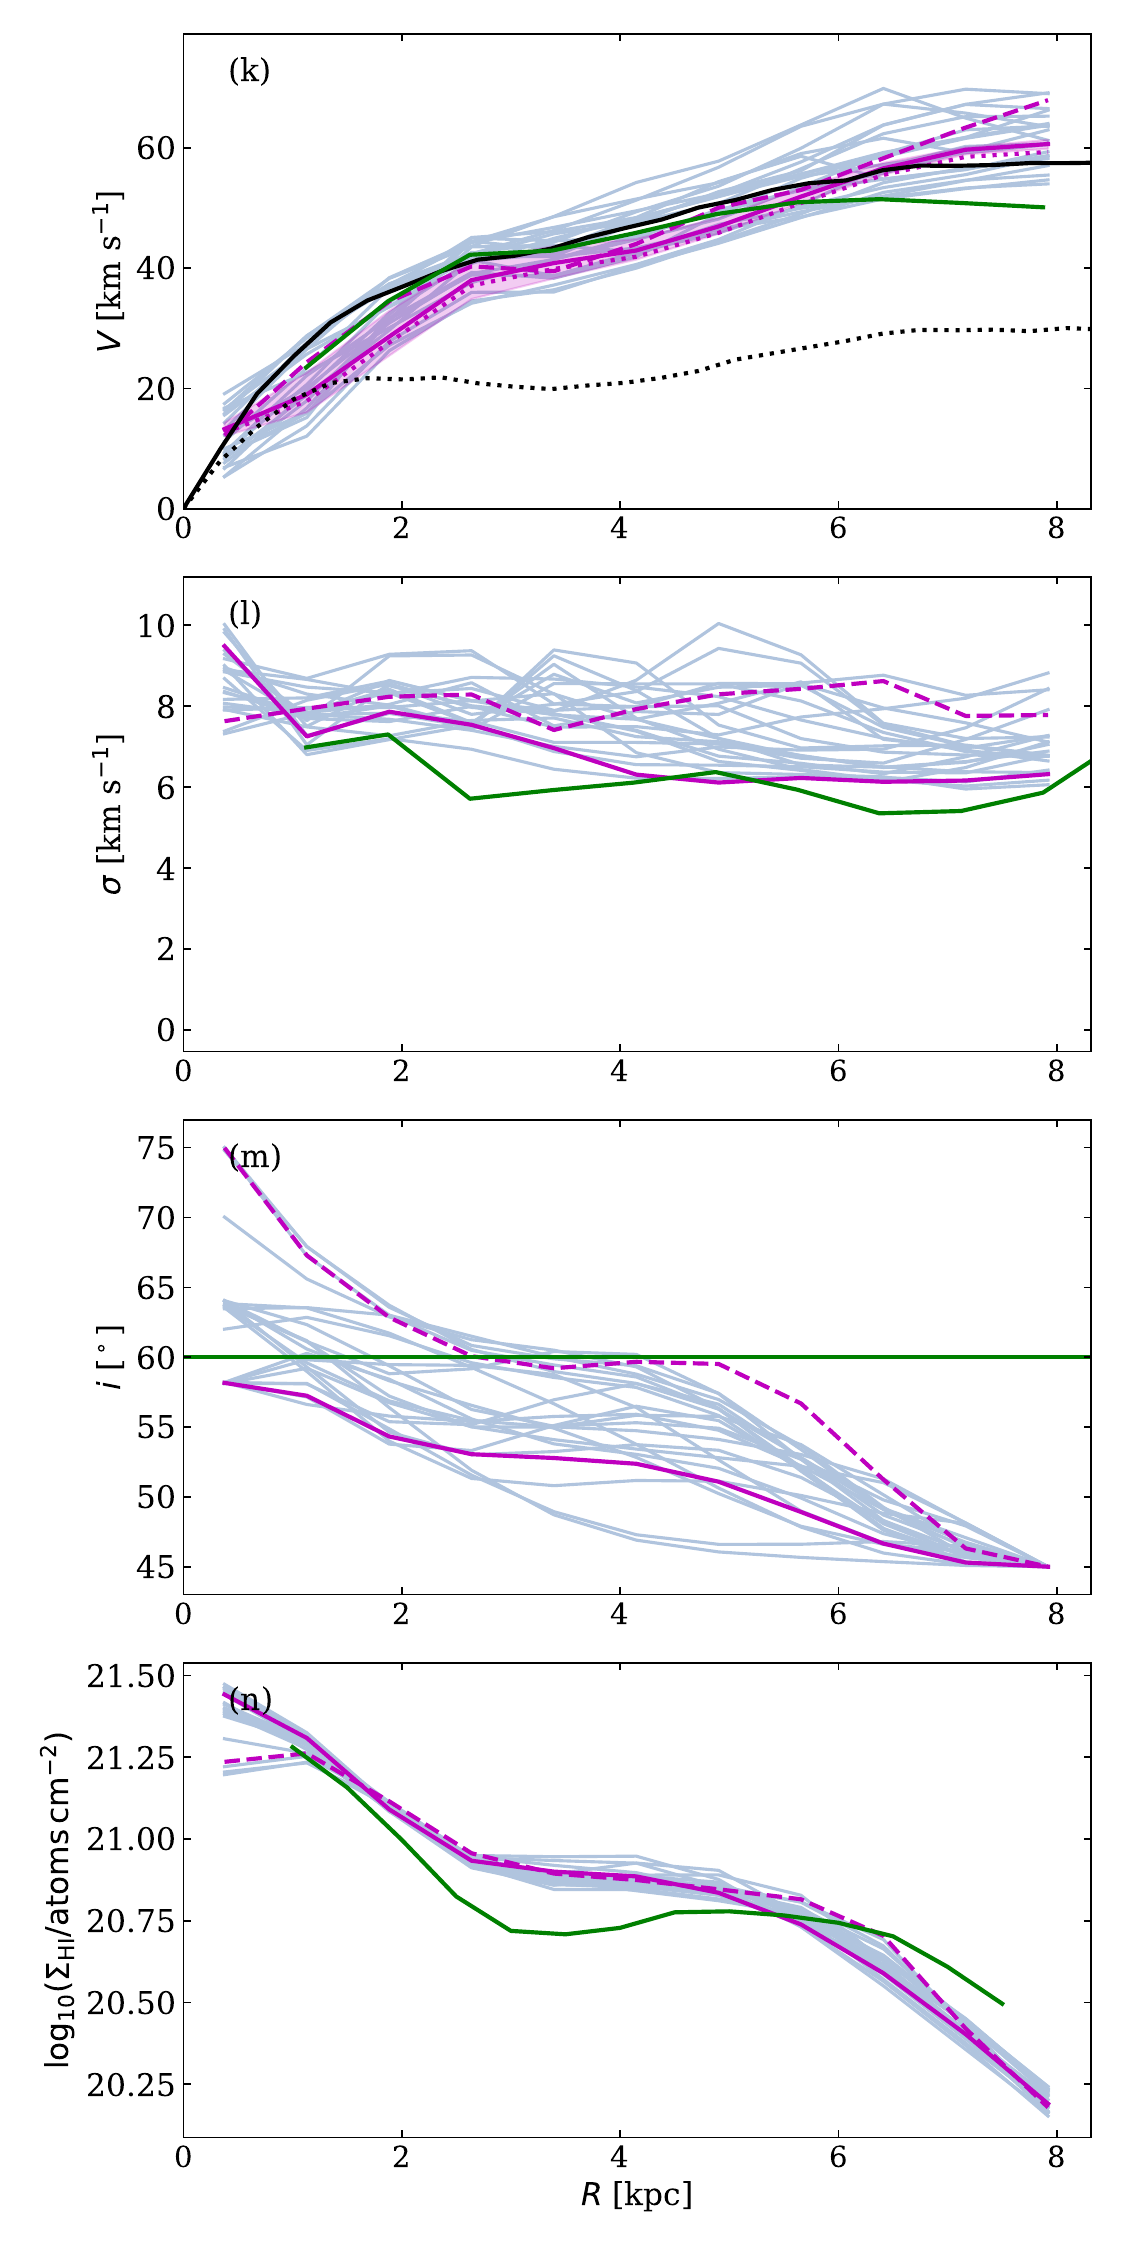}
\end{minipage}
\caption{A set of summary figures for galaxy HT-40, selected for kinematic analysis. These include example moment maps for two orientations (panels (a)--(f); similar to Fig.~\ref{fig:visualisations}), a summary of the parameters $V_\mathrm{fid}$, $V_\mathrm{max}$, $\eta_\mathrm{rot}$, and $\eta_\mathrm{bar}$ (panels (g)--(j); similar to Fig.~\ref{fig:loops}), and a summary of the rotation curve analysis from $24$ viewing angles (panels (k)--(n); similar to Fig.~\ref{fig:rot_curves}). See description of Appendix~\ref{app:supplementary} for details.}
\label{fig:S54}
\end{figure}
\clearpage

\begin{figure}
\begin{minipage}{.9\textwidth}
\includegraphics[width=\textwidth]{../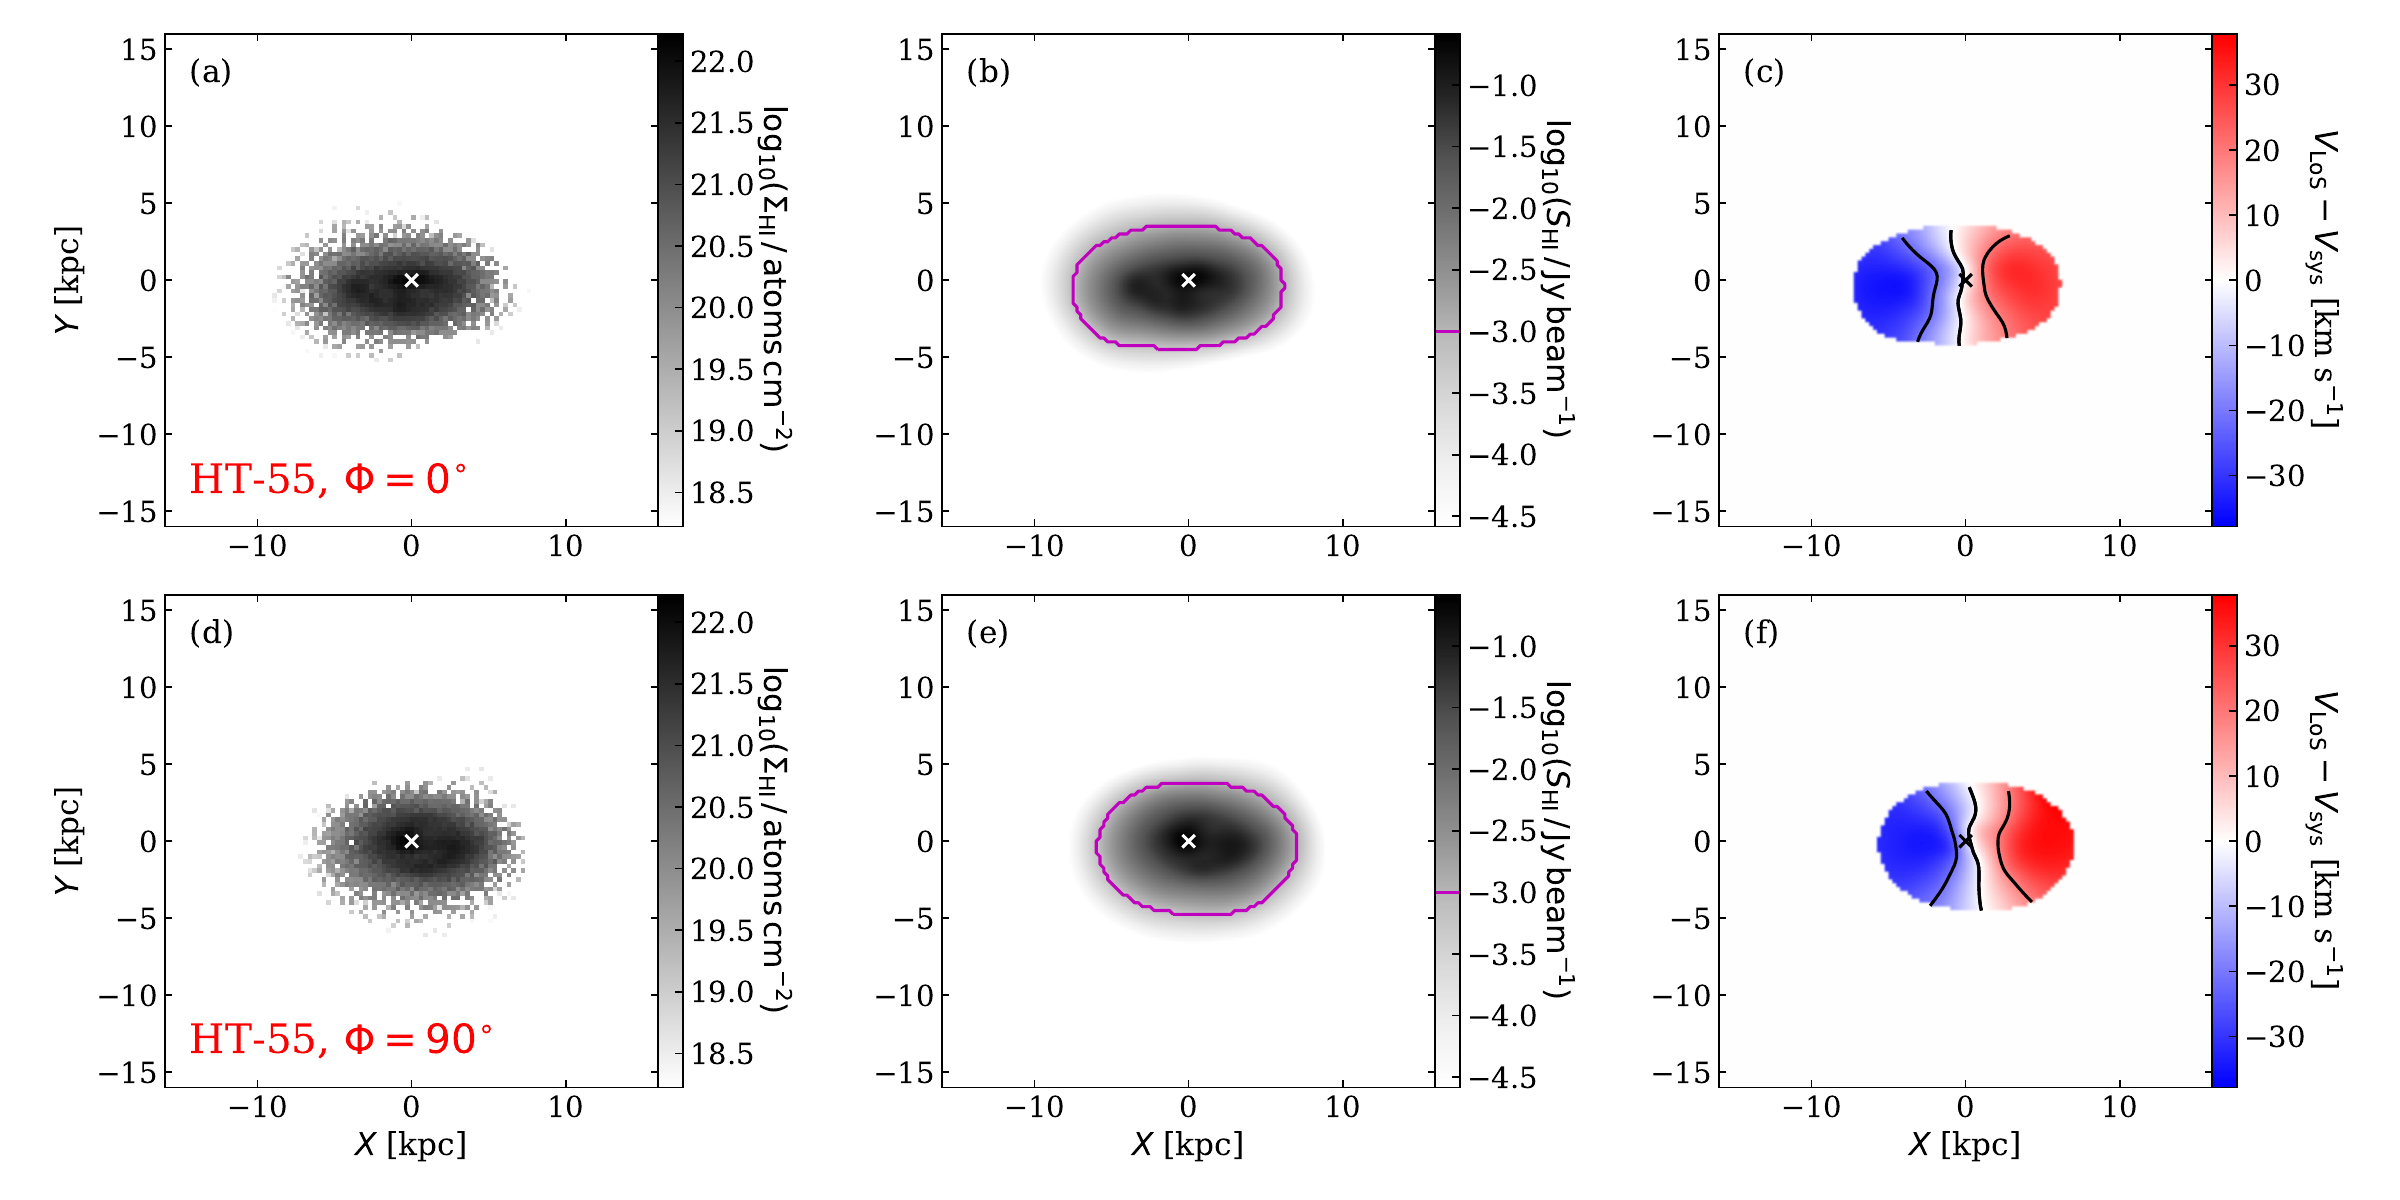}
\includegraphics[width=\textwidth]{../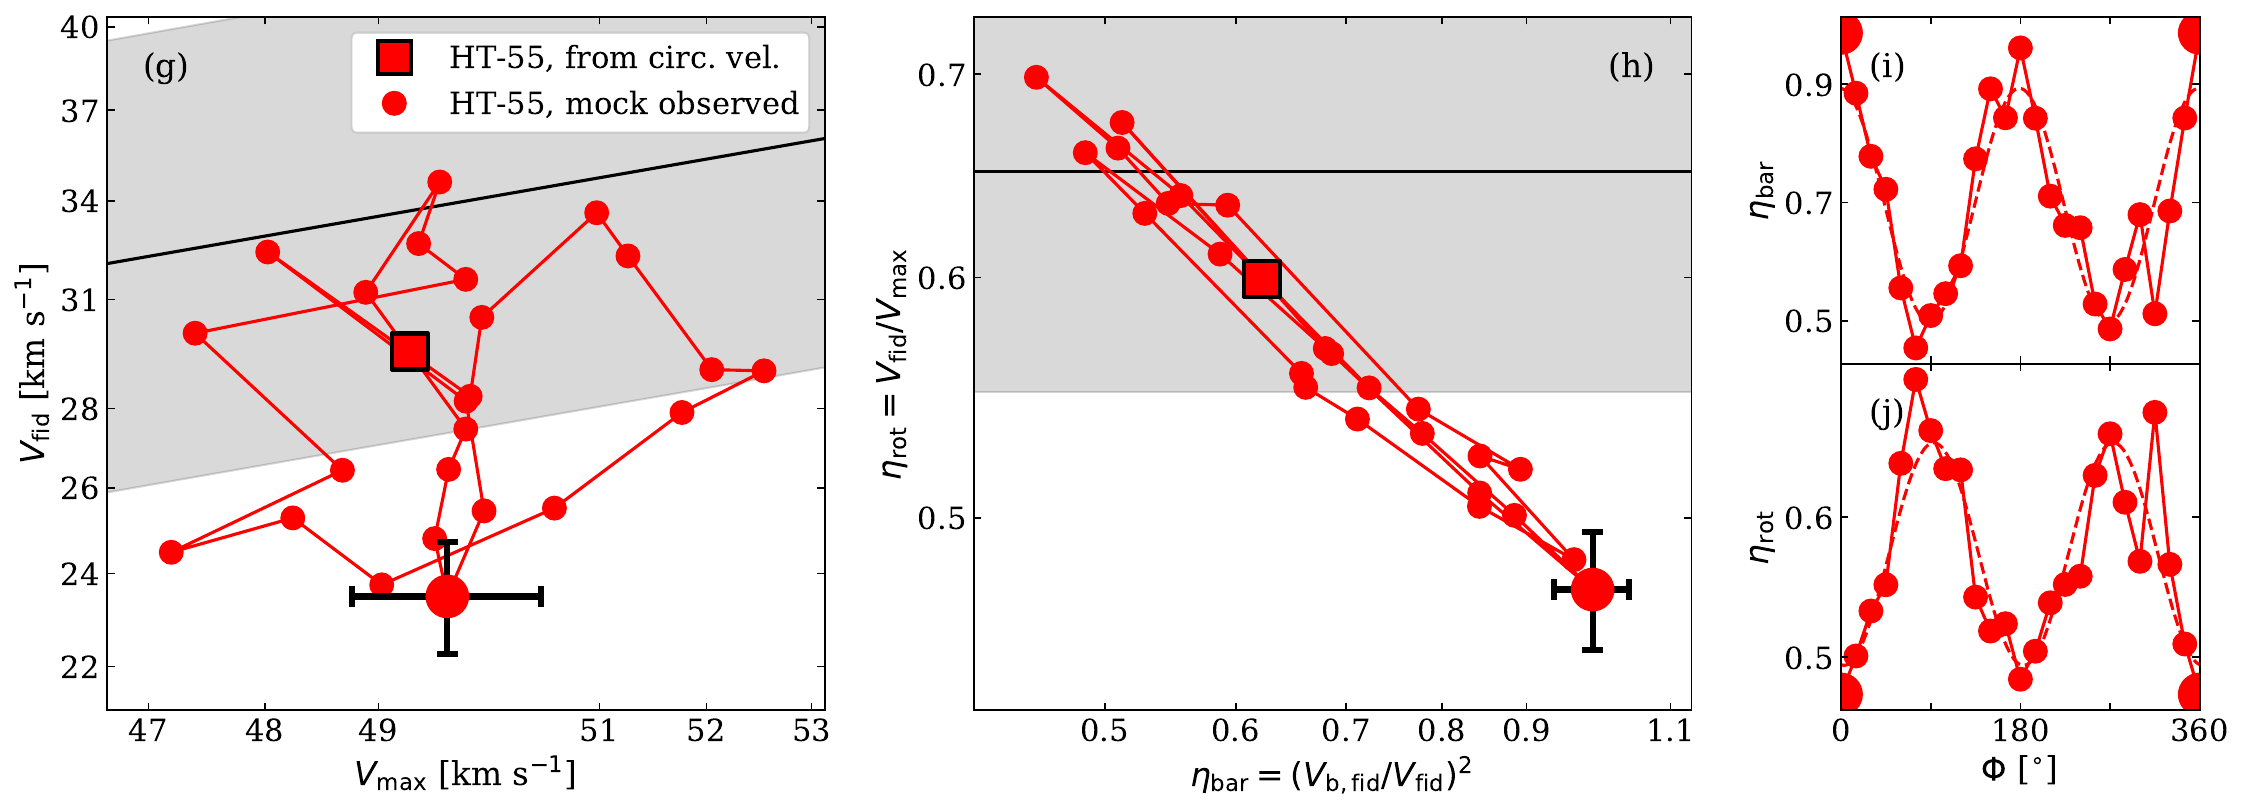}
\end{minipage}
\begin{minipage}{.4\textwidth}
\includegraphics[width=\textwidth]{../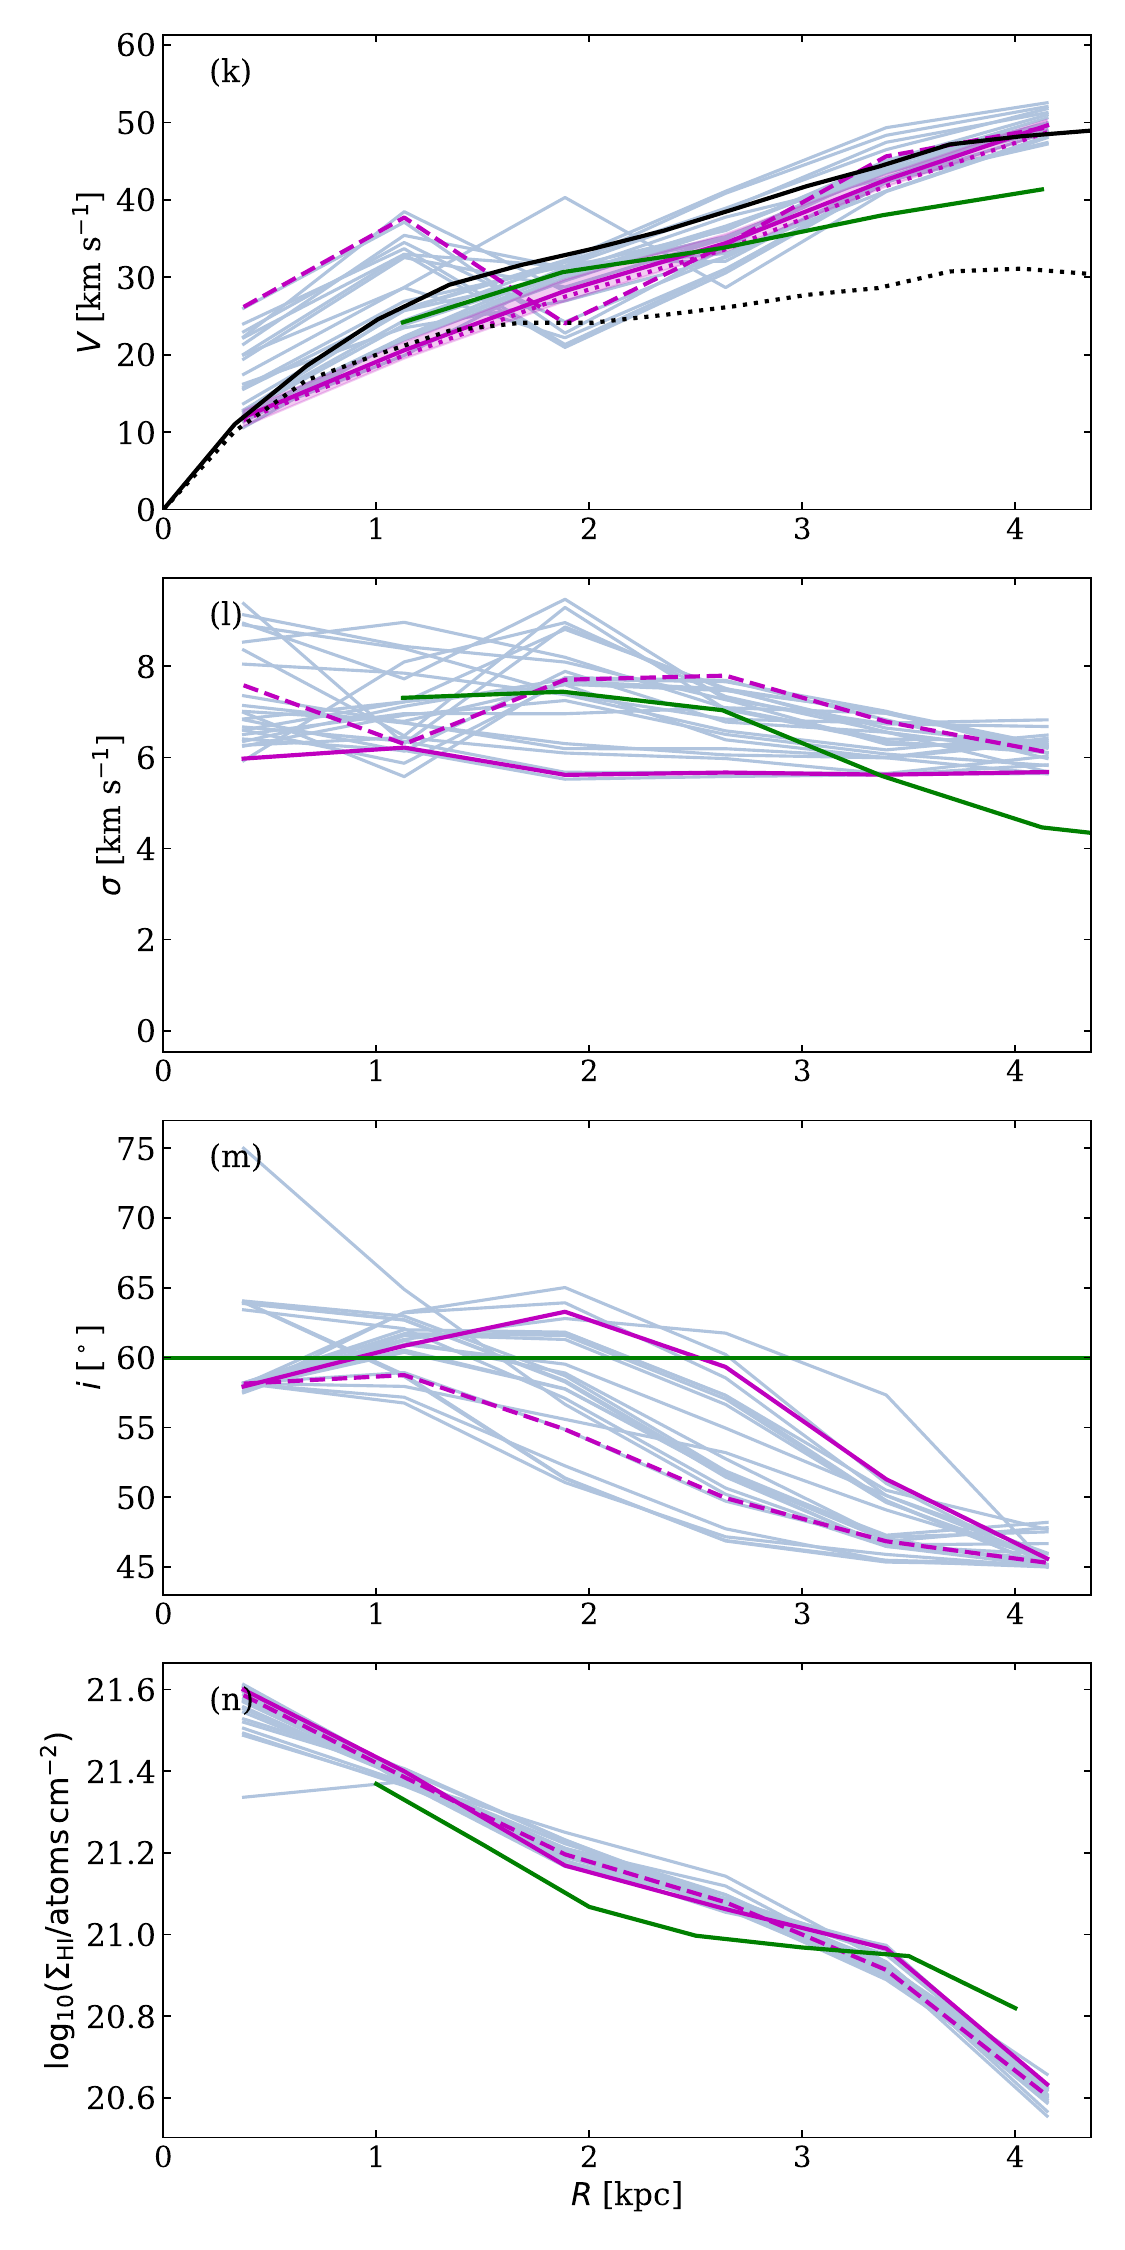}
\end{minipage}
\caption{A set of summary figures for galaxy HT-55, selected for kinematic analysis. These include example moment maps for two orientations (panels (a)--(f); similar to Fig.~\ref{fig:visualisations}), a summary of the parameters $V_\mathrm{fid}$, $V_\mathrm{max}$, $\eta_\mathrm{rot}$, and $\eta_\mathrm{bar}$ (panels (g)--(j); similar to Fig.~\ref{fig:loops}), and a summary of the rotation curve analysis from $24$ viewing angles (panels (k)--(n); similar to Fig.~\ref{fig:rot_curves}). See description of Appendix~\ref{app:supplementary} for details.}
\label{fig:S55}
\end{figure}
\clearpage

\begin{figure}
\begin{minipage}{.9\textwidth}
\includegraphics[width=\textwidth]{../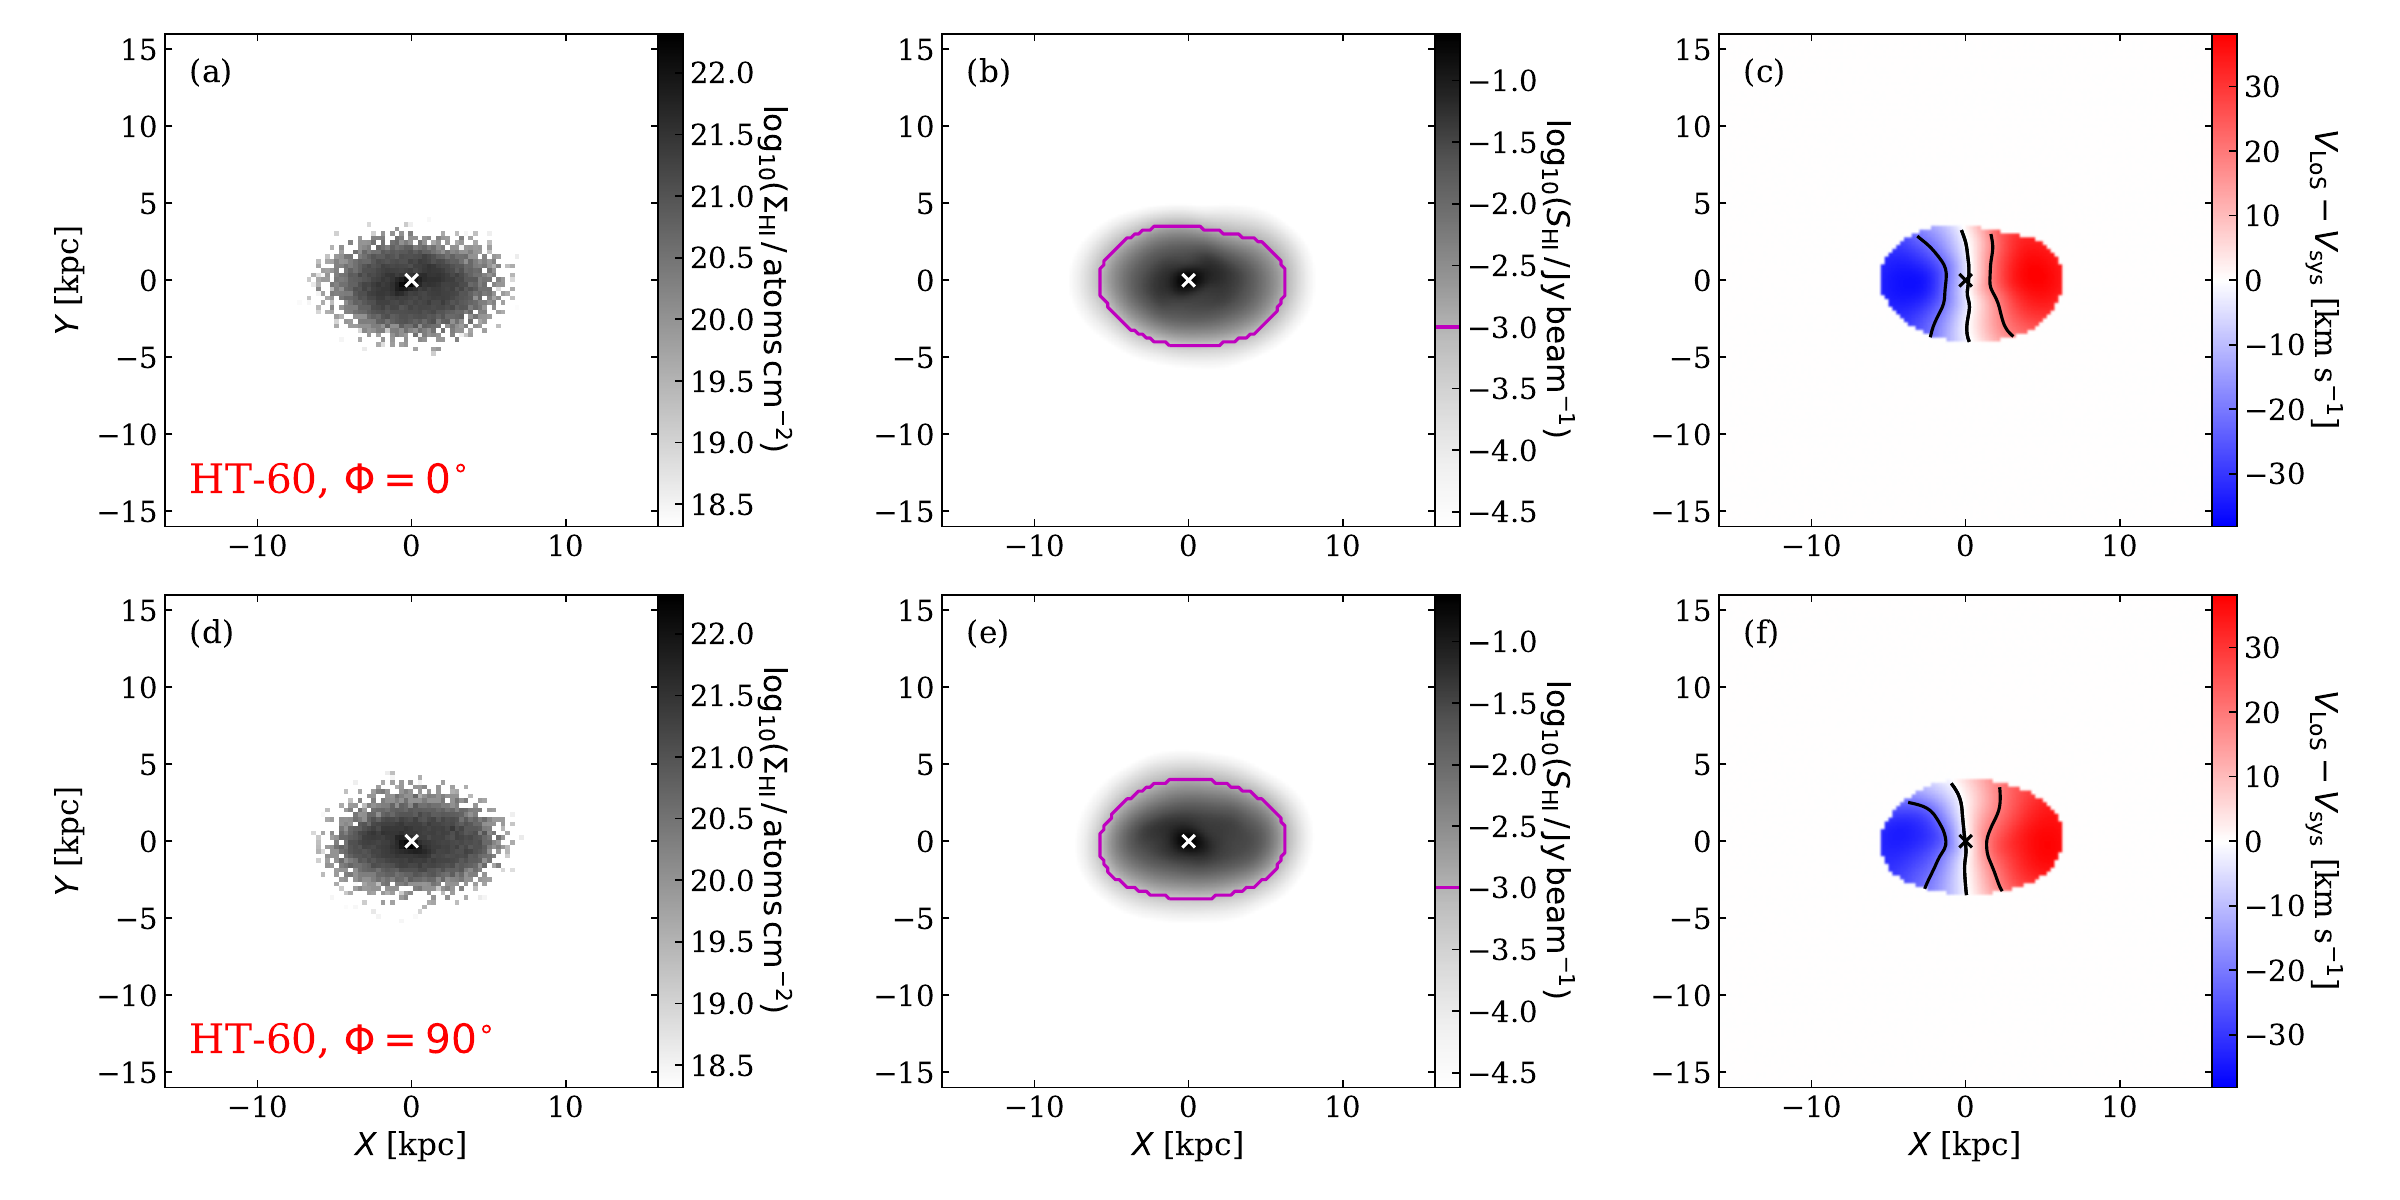}
\includegraphics[width=\textwidth]{../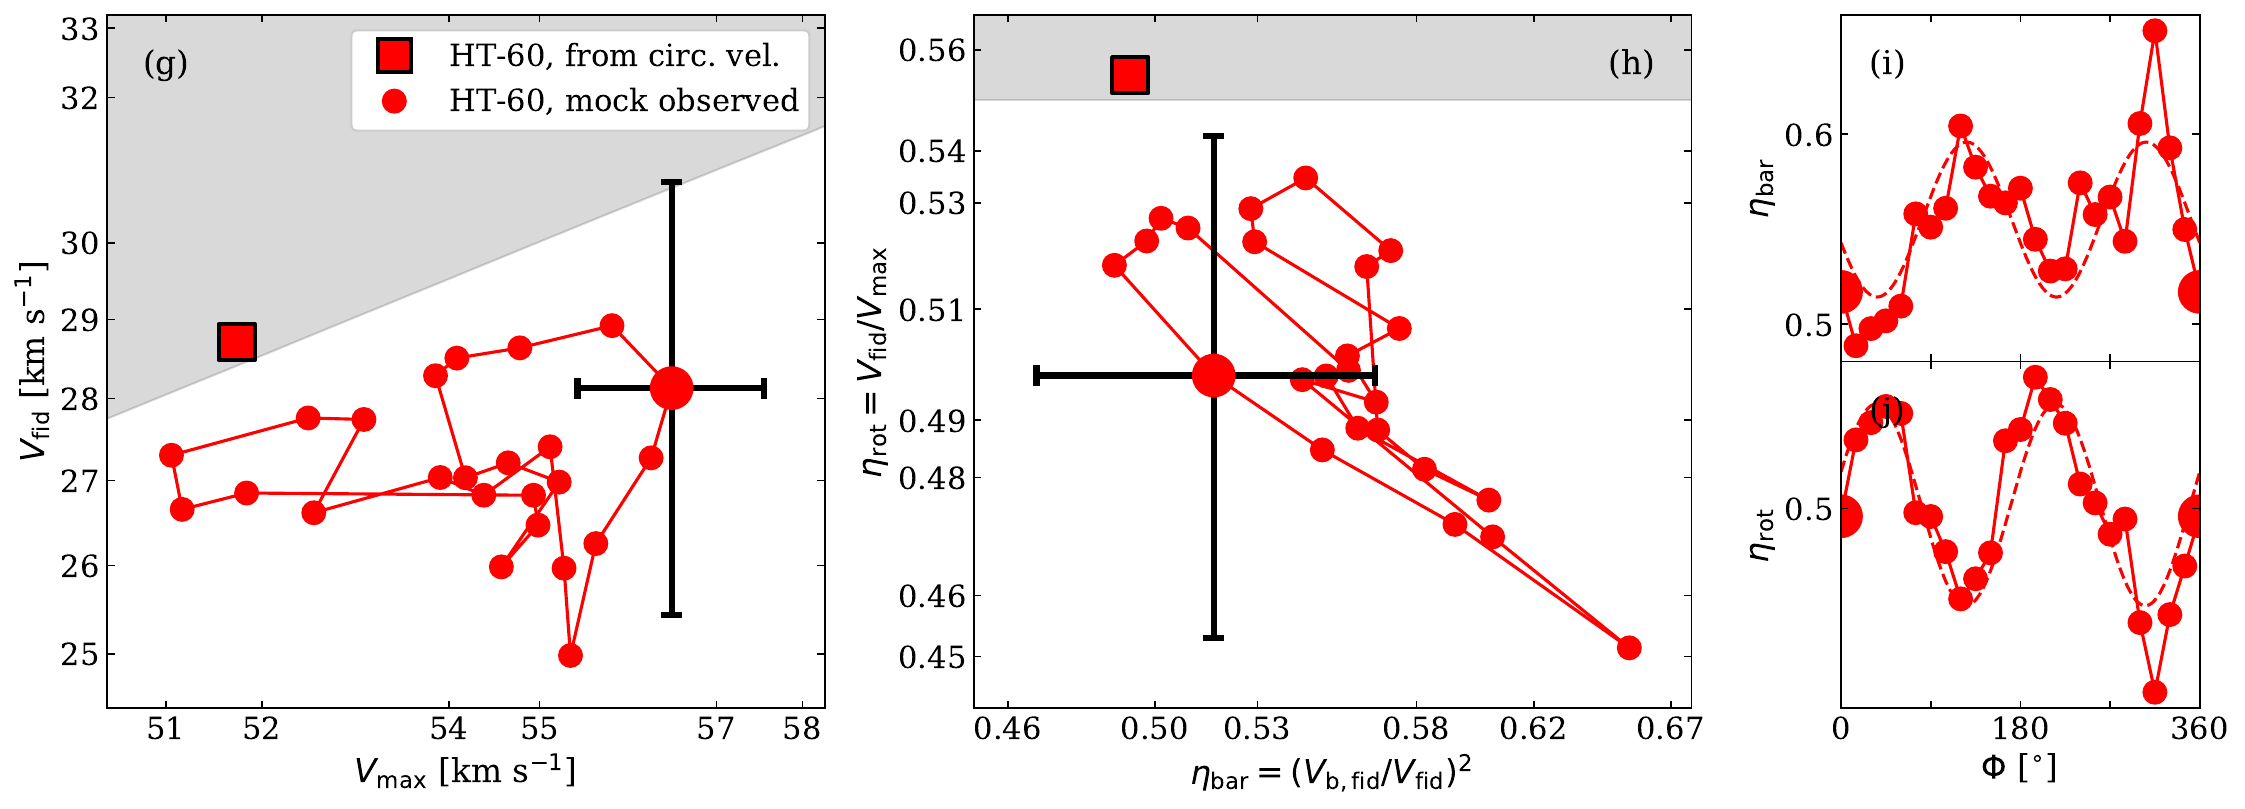}
\end{minipage}
\begin{minipage}{.4\textwidth}
\includegraphics[width=\textwidth]{../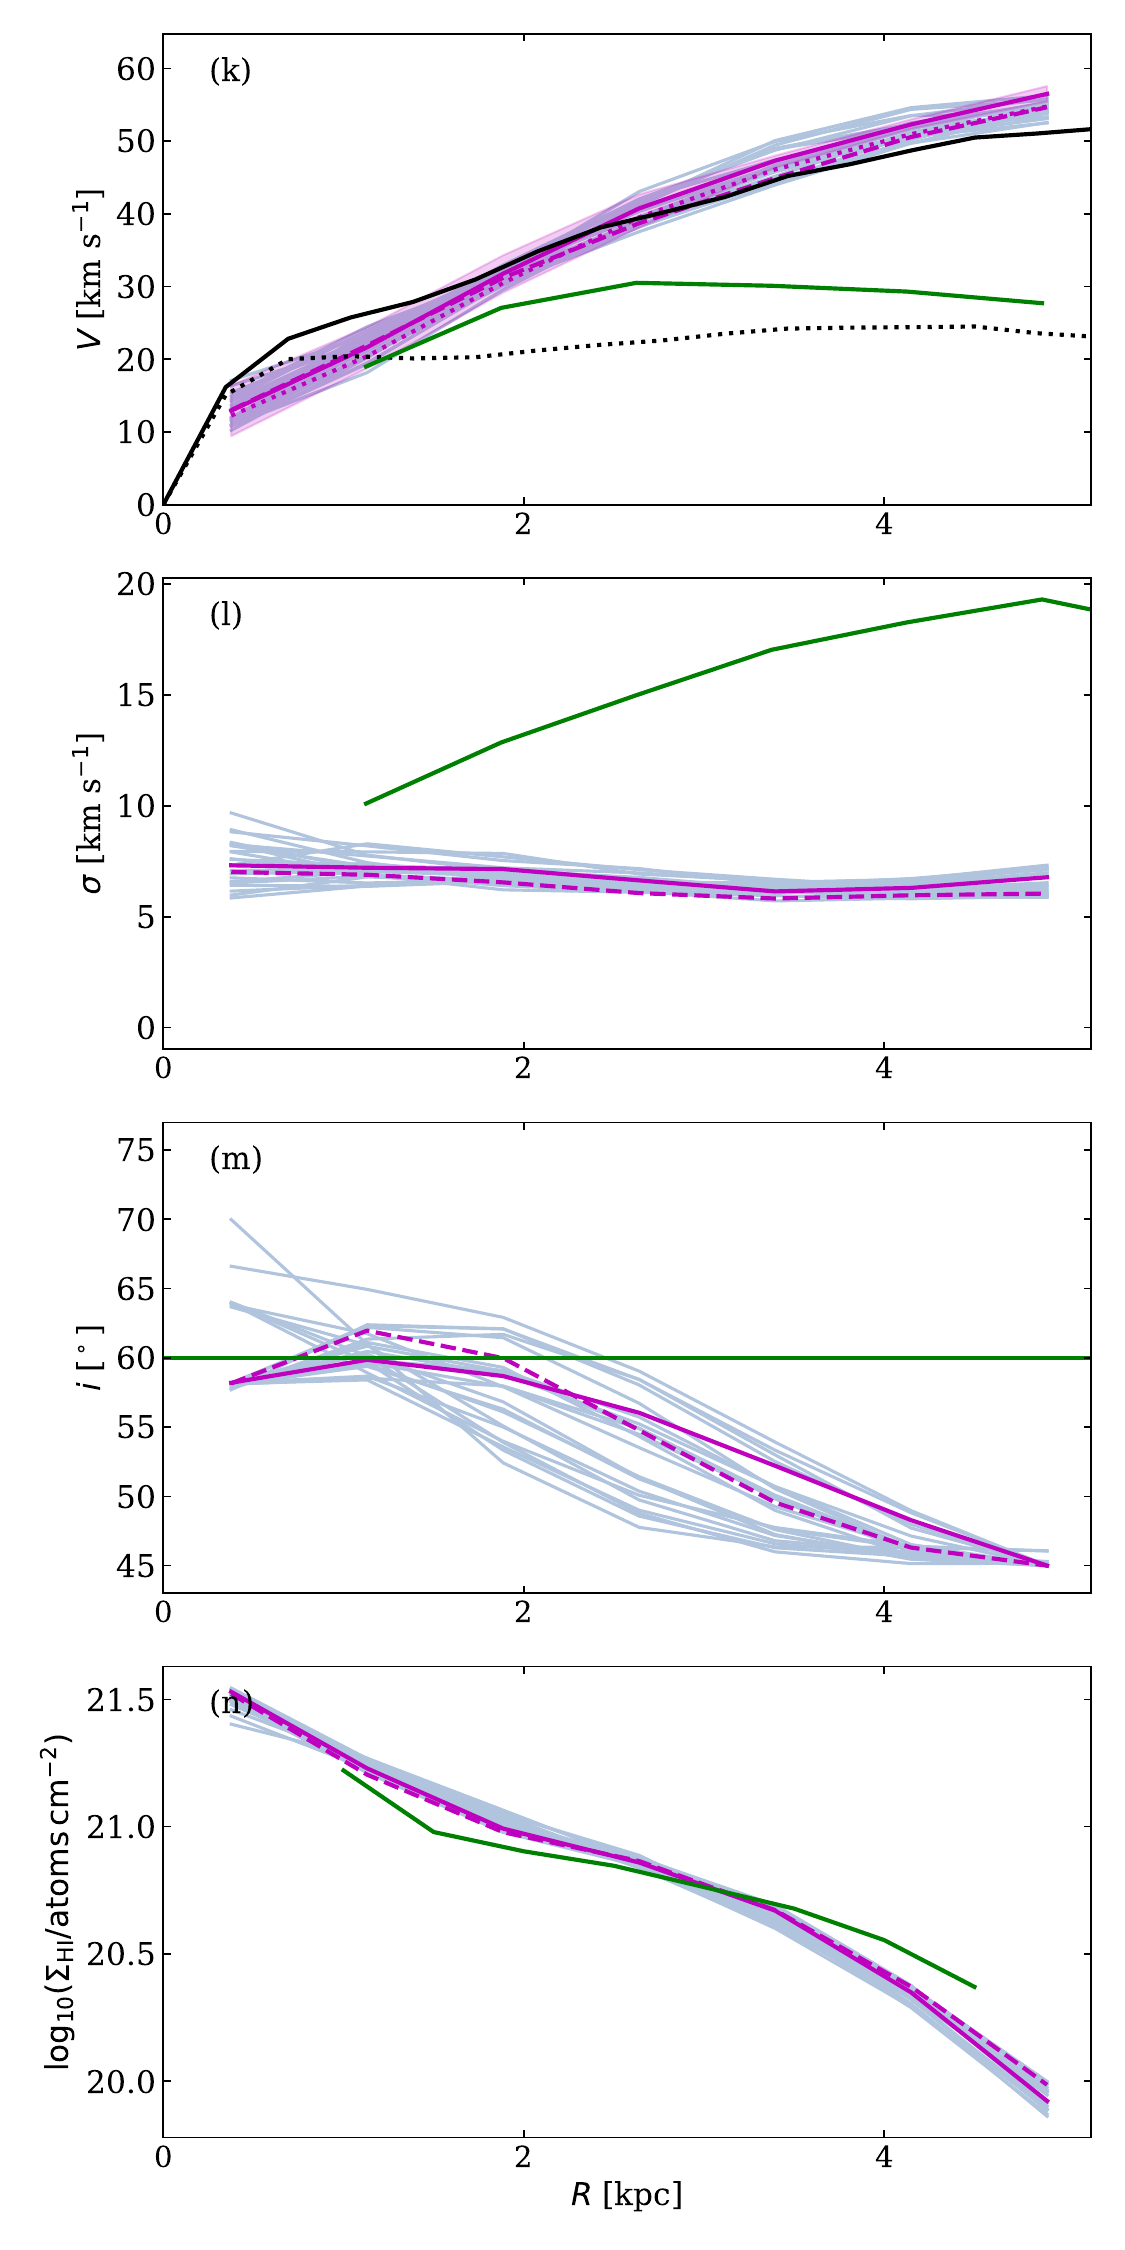}
\end{minipage}
\caption{A set of summary figures for galaxy HT-60, selected for kinematic analysis. These include example moment maps for two orientations (panels (a)--(f); similar to Fig.~\ref{fig:visualisations}), a summary of the parameters $V_\mathrm{fid}$, $V_\mathrm{max}$, $\eta_\mathrm{rot}$, and $\eta_\mathrm{bar}$ (panels (g)--(j); similar to Fig.~\ref{fig:loops}), and a summary of the rotation curve analysis from $24$ viewing angles (panels (k)--(n); similar to Fig.~\ref{fig:rot_curves}). See description of Appendix~\ref{app:supplementary} for details.}
\label{fig:S56}
\end{figure}
\clearpage

\begin{figure}
\begin{minipage}{.9\textwidth}
\includegraphics[width=\textwidth]{../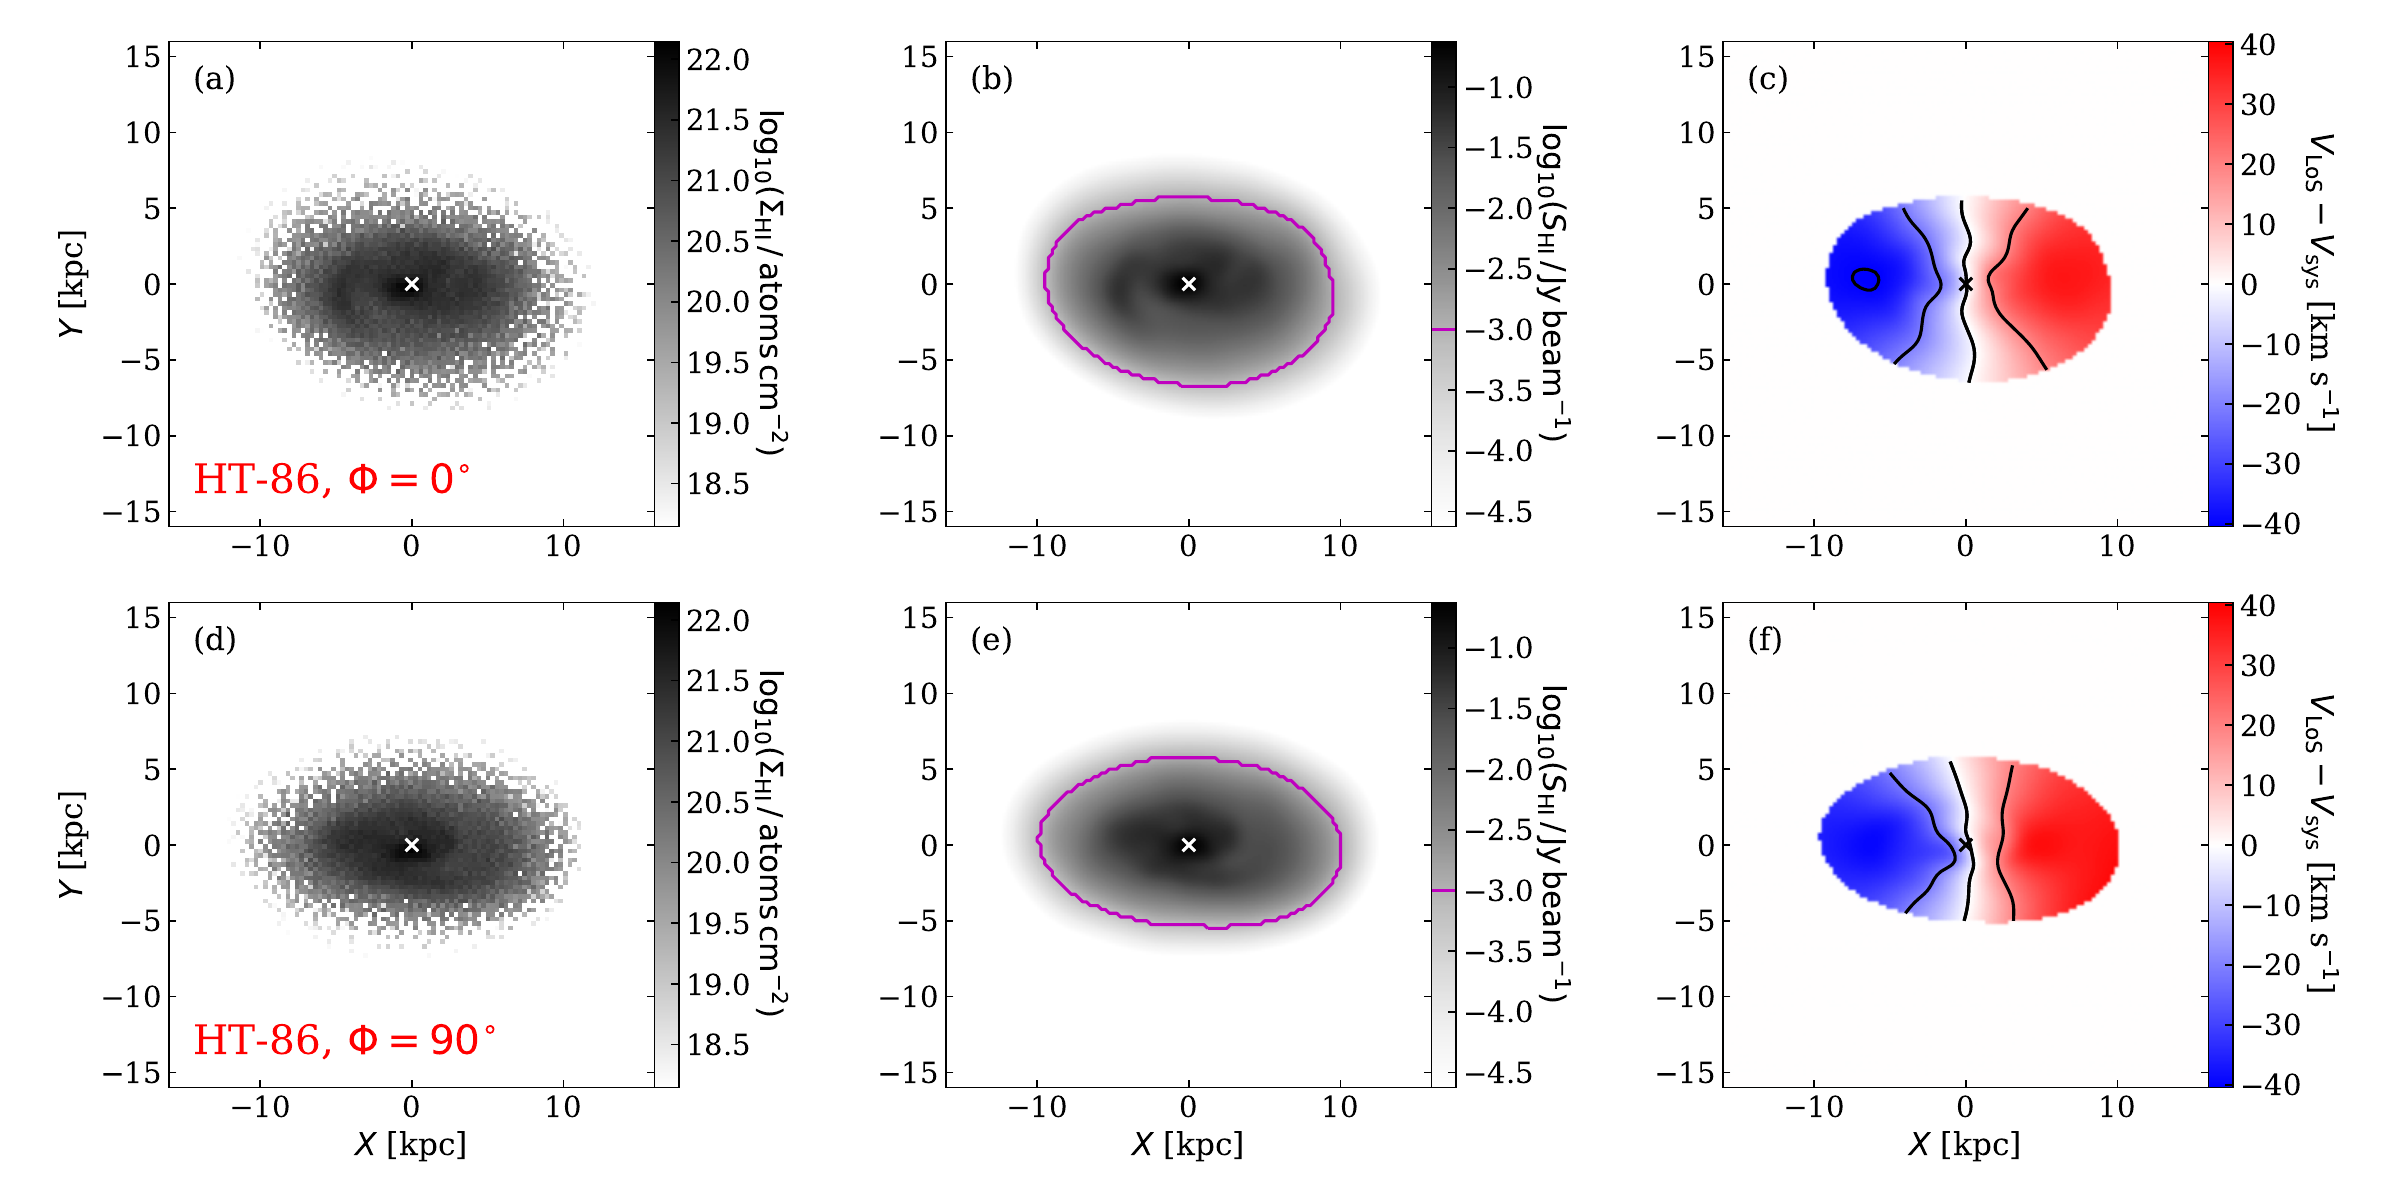}
\includegraphics[width=\textwidth]{../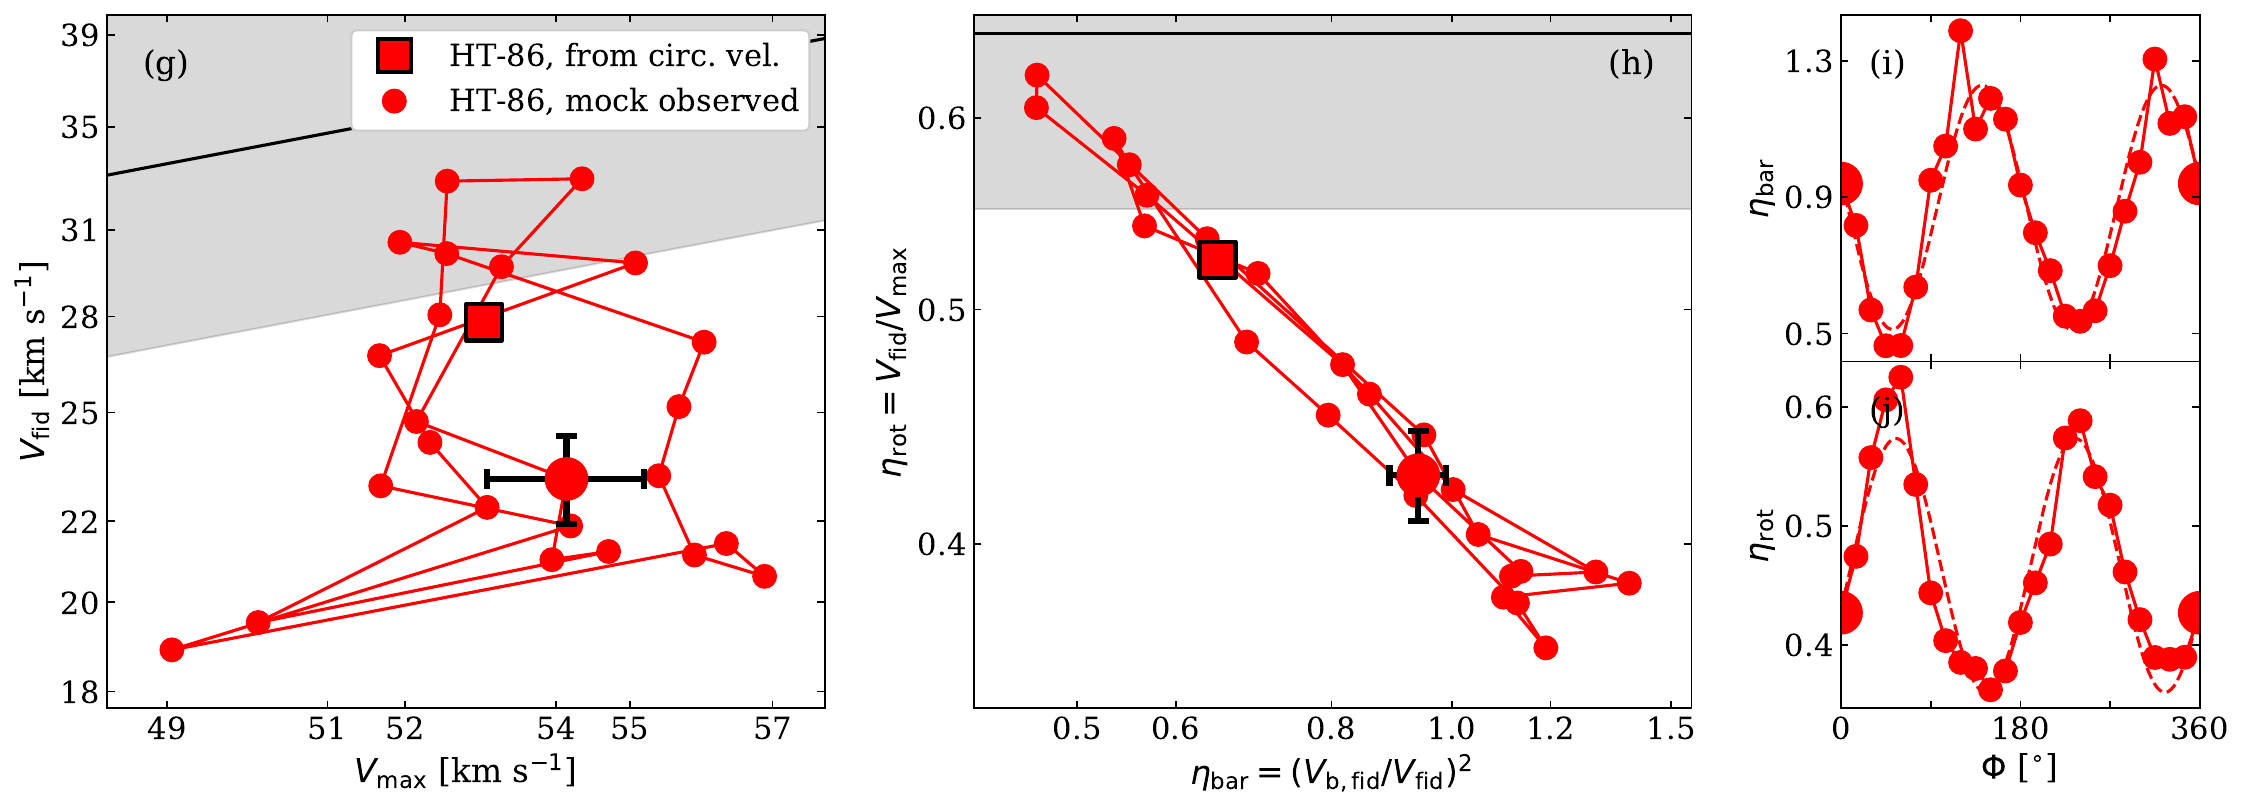}
\end{minipage}
\begin{minipage}{.4\textwidth}
\includegraphics[width=\textwidth]{../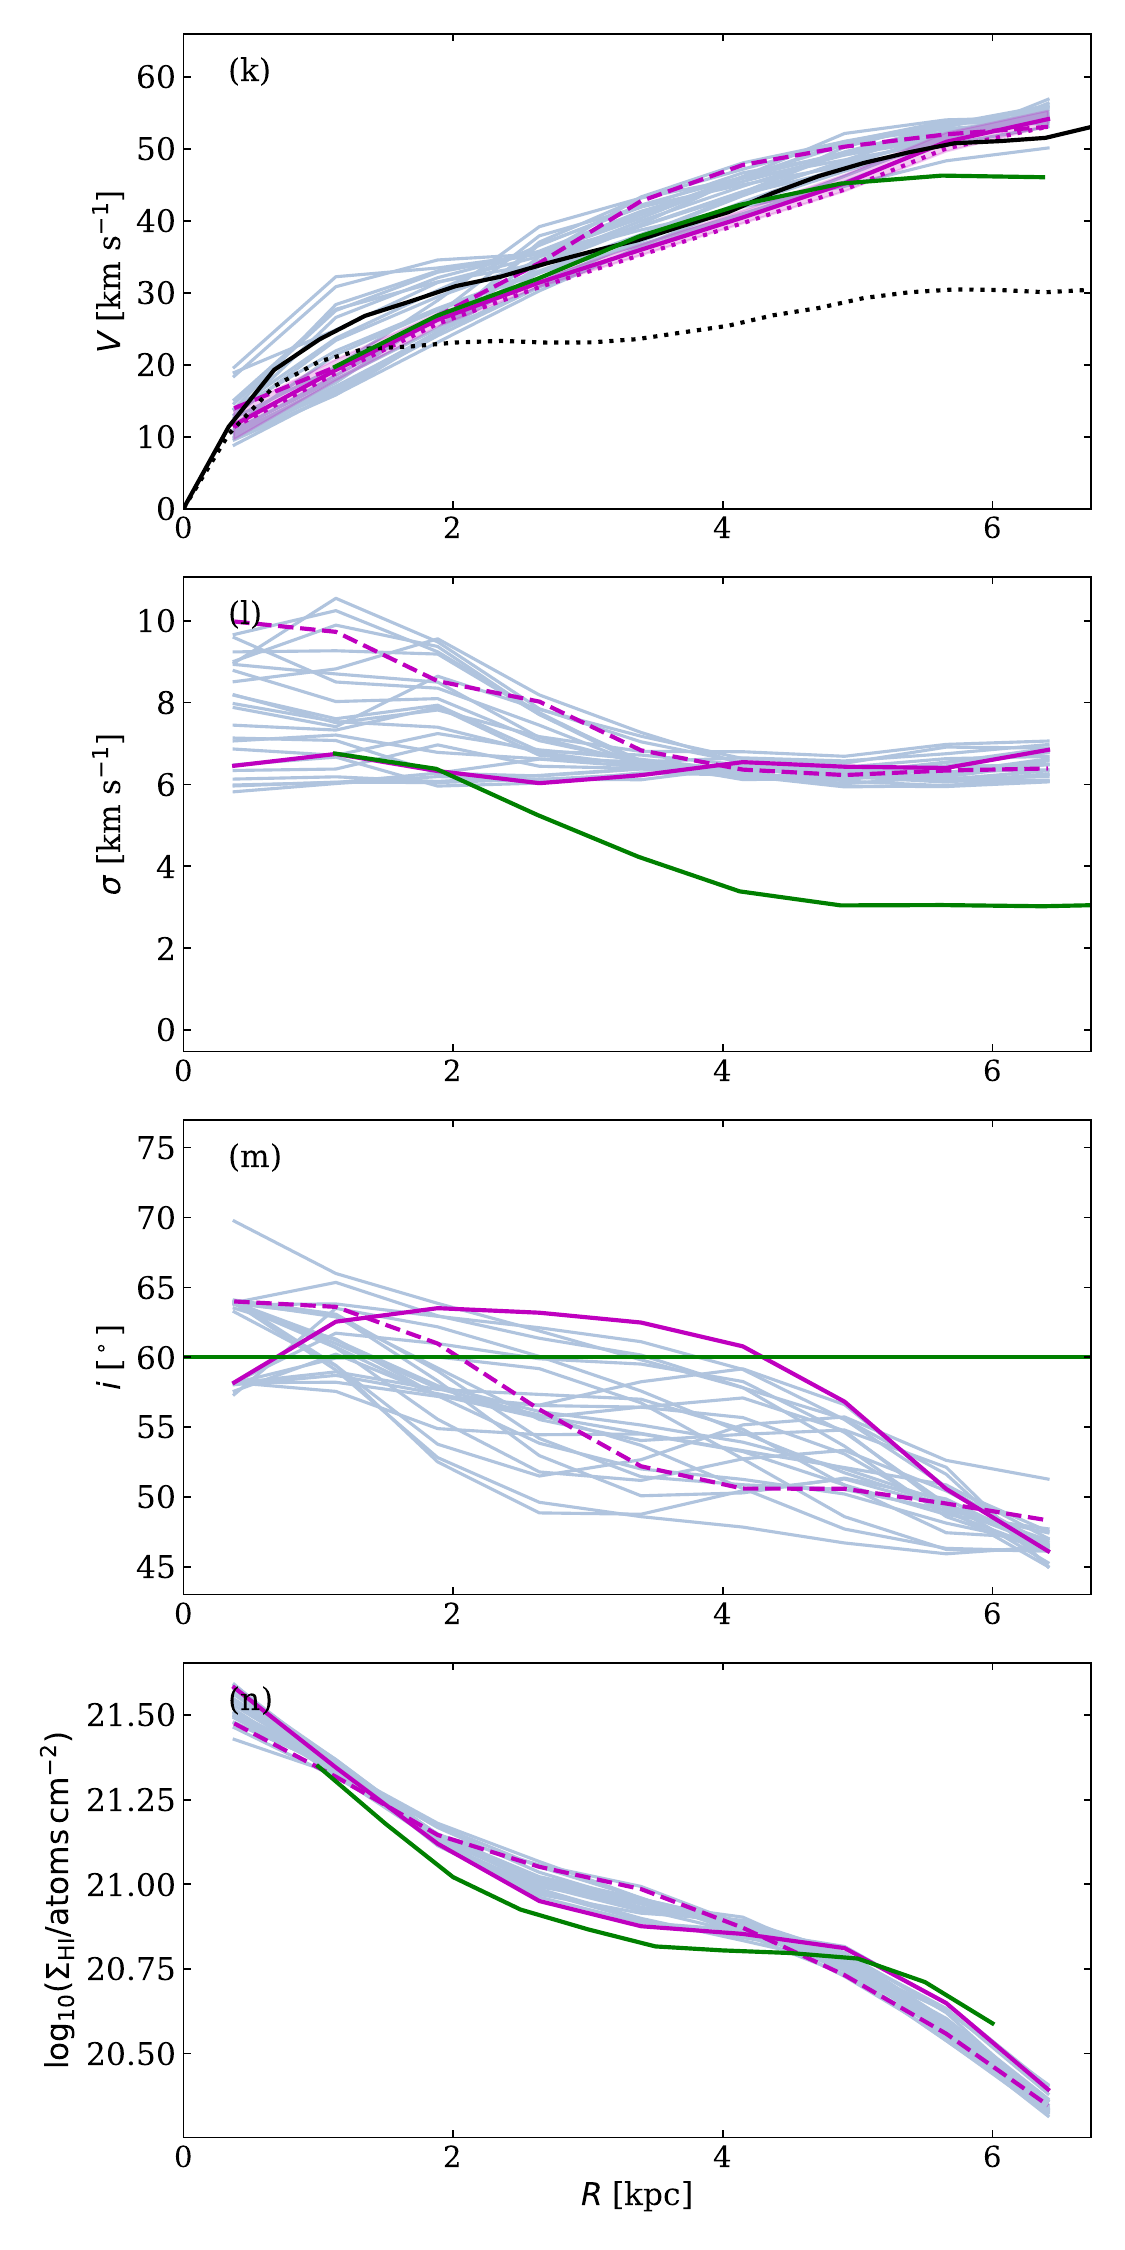}
\end{minipage}
\caption{A set of summary figures for galaxy HT-86, selected for kinematic analysis. These include example moment maps for two orientations (panels (a)--(f); similar to Fig.~\ref{fig:visualisations}), a summary of the parameters $V_\mathrm{fid}$, $V_\mathrm{max}$, $\eta_\mathrm{rot}$, and $\eta_\mathrm{bar}$ (panels (g)--(j); similar to Fig.~\ref{fig:loops}), and a summary of the rotation curve analysis from $24$ viewing angles (panels (k)--(n); similar to Fig.~\ref{fig:rot_curves}). See description of Appendix~\ref{app:supplementary} for details.}
\label{fig:S57}
\end{figure}
\clearpage

\begin{figure}
\begin{minipage}{.9\textwidth}
\includegraphics[width=\textwidth]{../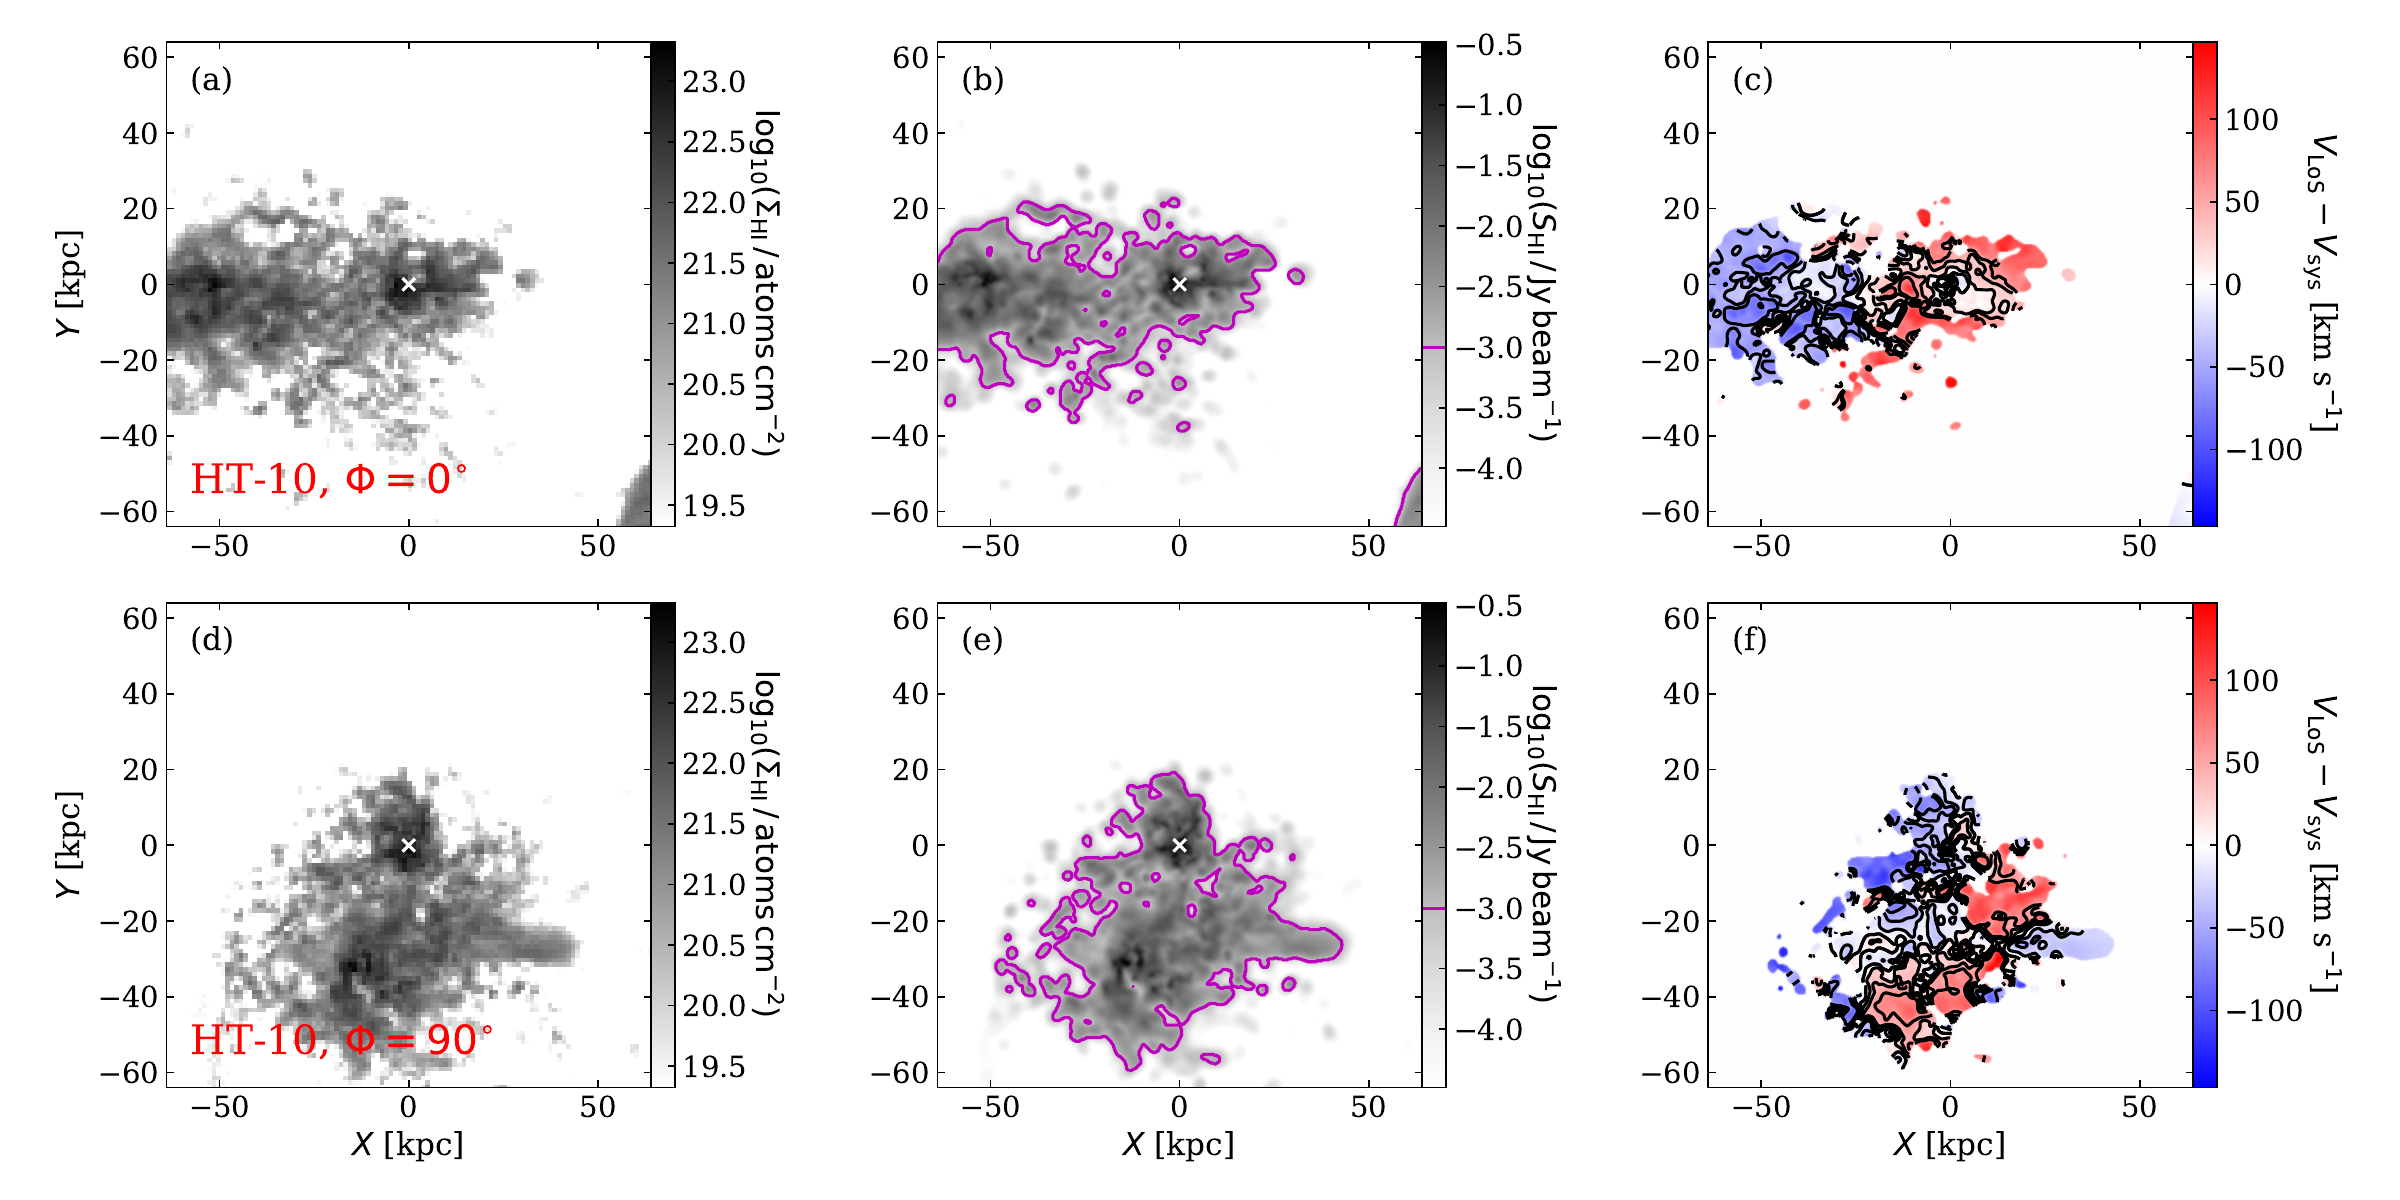}
\includegraphics[width=\textwidth]{../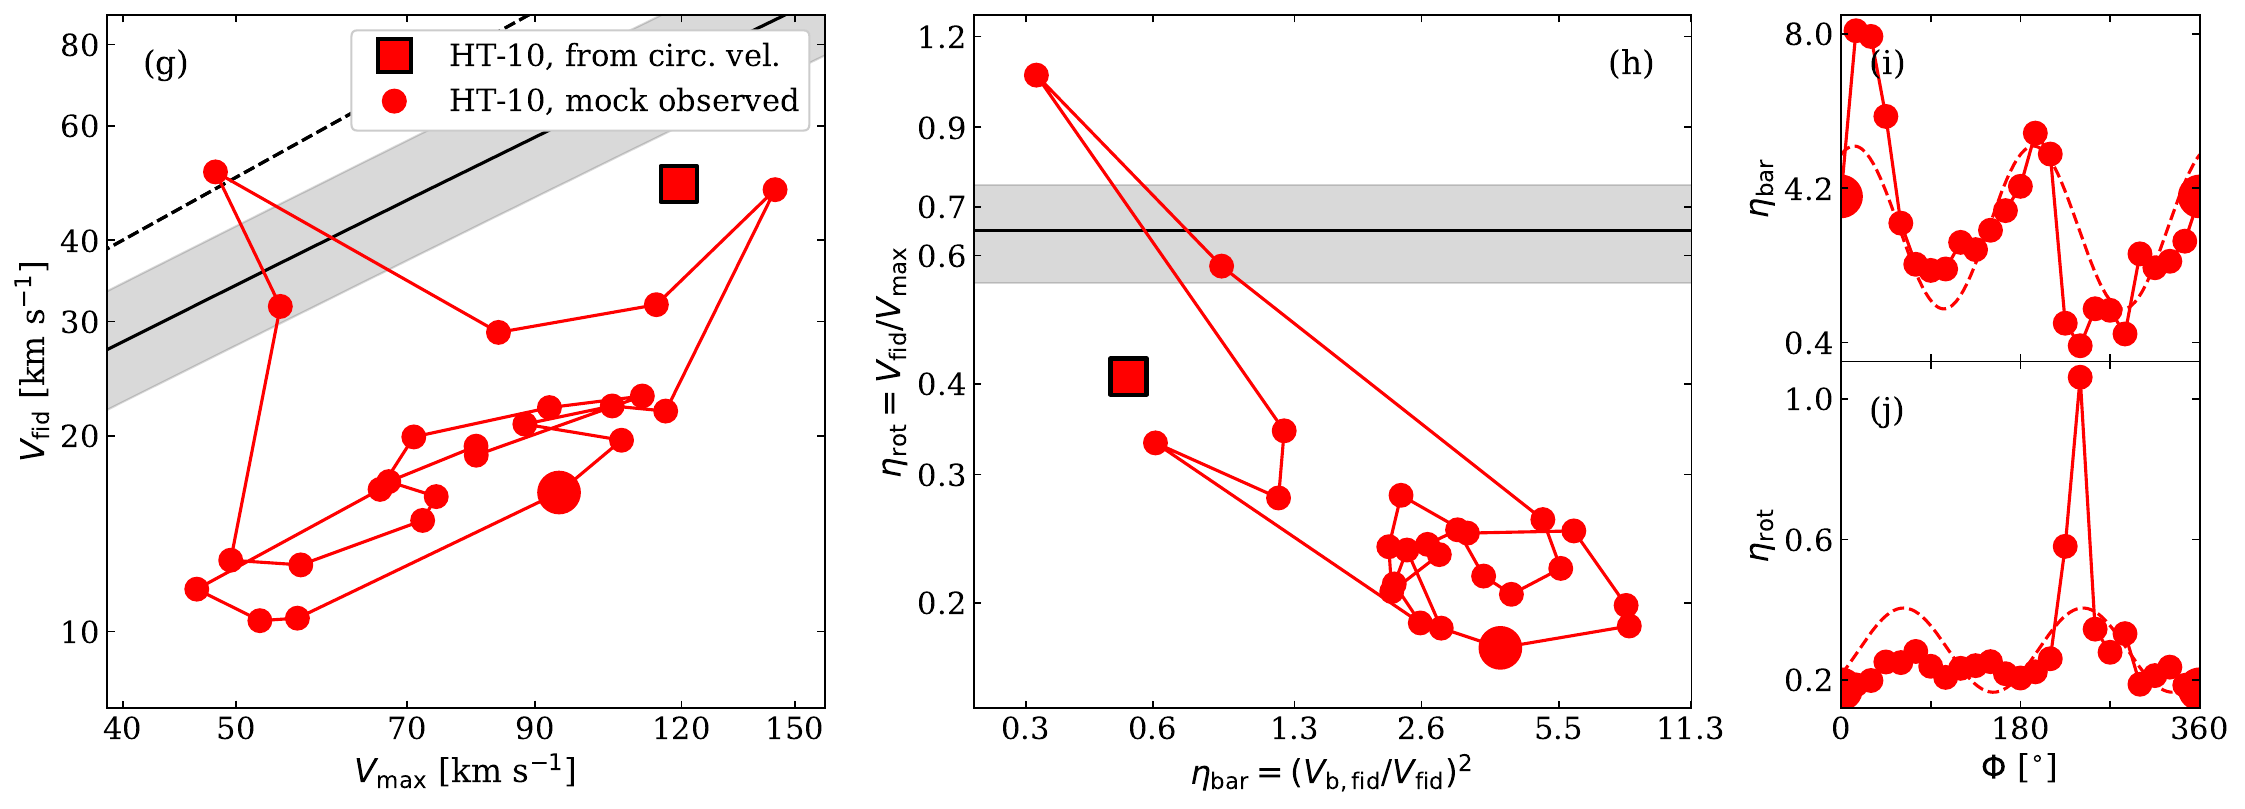}
\end{minipage}
\begin{minipage}{.4\textwidth}
\includegraphics[width=\textwidth]{../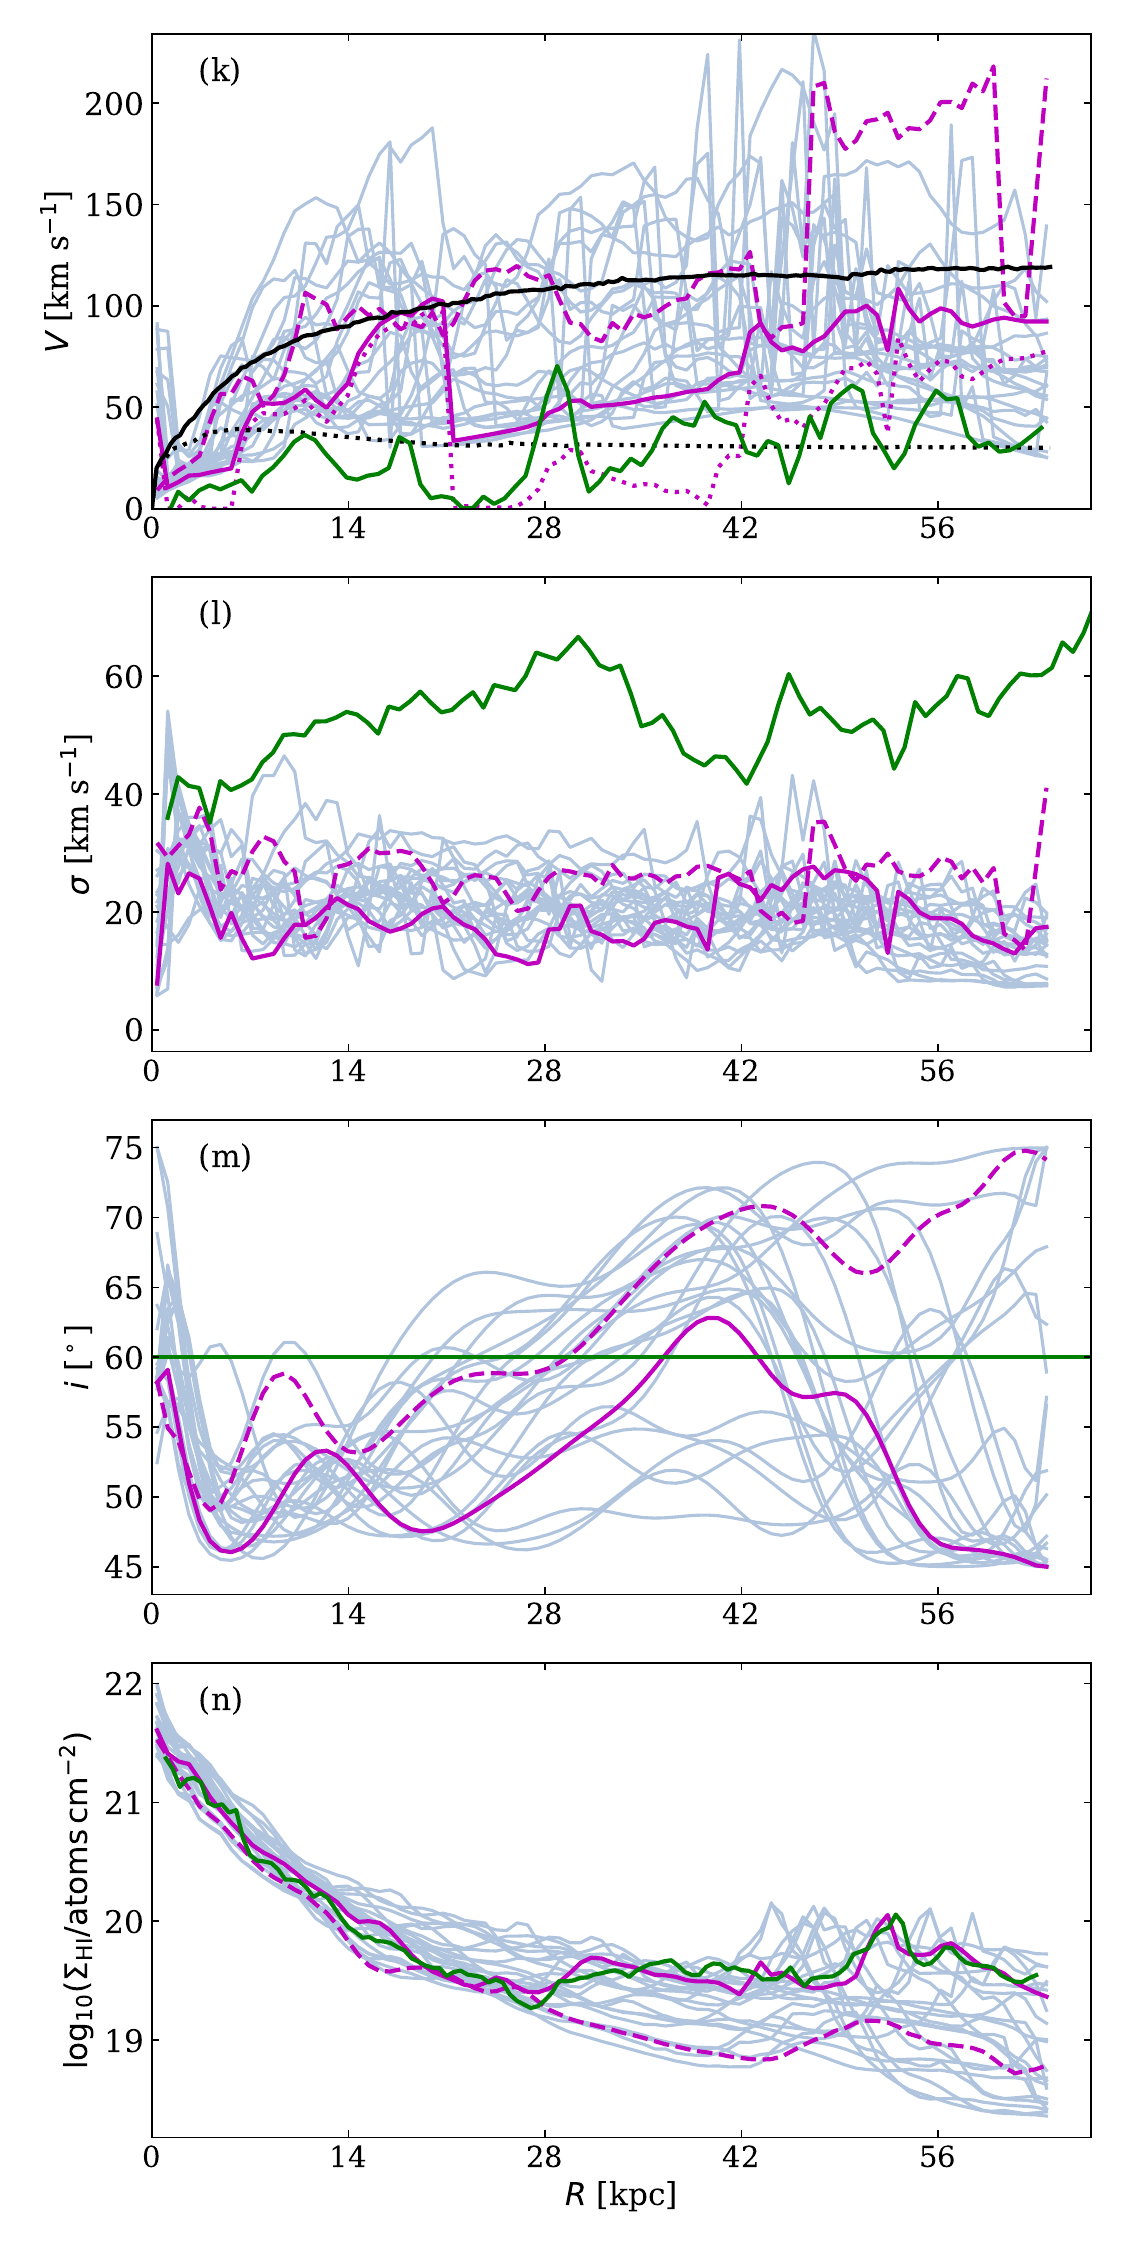}
\end{minipage}
\caption{A set of summary figures for galaxy HT-10, excluded from kinematic analysis. These include example moment maps for two orientations (panels (a)--(f); similar to Fig.~\ref{fig:visualisations}), a summary of the parameters $V_\mathrm{fid}$, $V_\mathrm{max}$, $\eta_\mathrm{rot}$, and $\eta_\mathrm{bar}$ (panels (g)--(j); similar to Fig.~\ref{fig:loops}), and a summary of the rotation curve analysis from $24$ viewing angles (panels (k)--(n); similar to Fig.~\ref{fig:rot_curves}). See description of Appendix~\ref{app:supplementary} for details.}
\label{fig:S58}
\end{figure}
\clearpage

\begin{figure}
\begin{minipage}{.9\textwidth}
\includegraphics[width=\textwidth]{../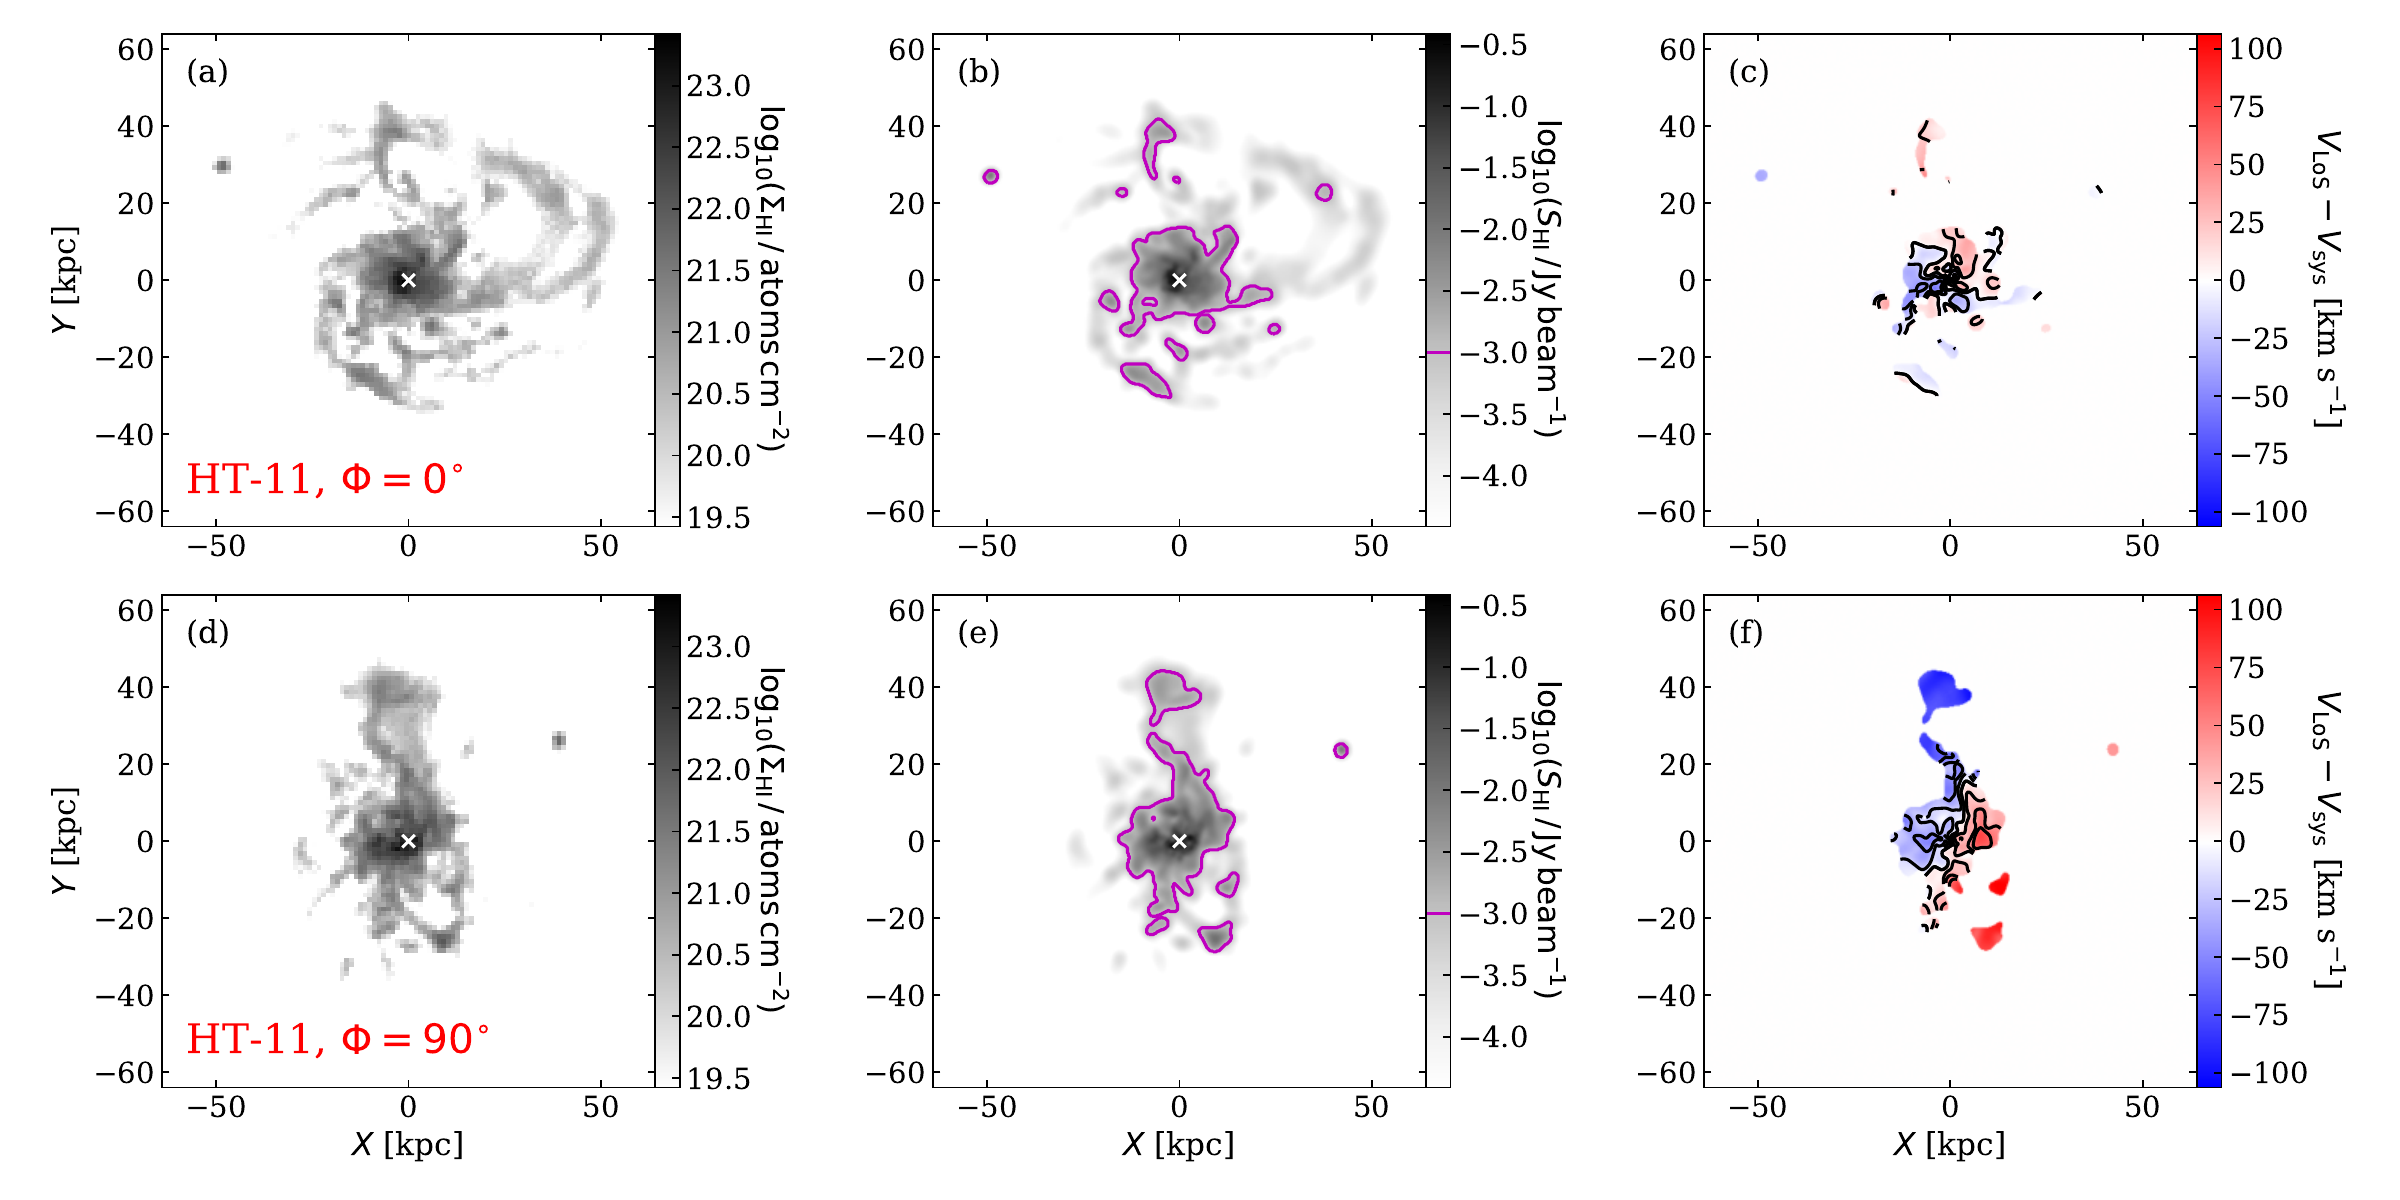}
\includegraphics[width=\textwidth]{../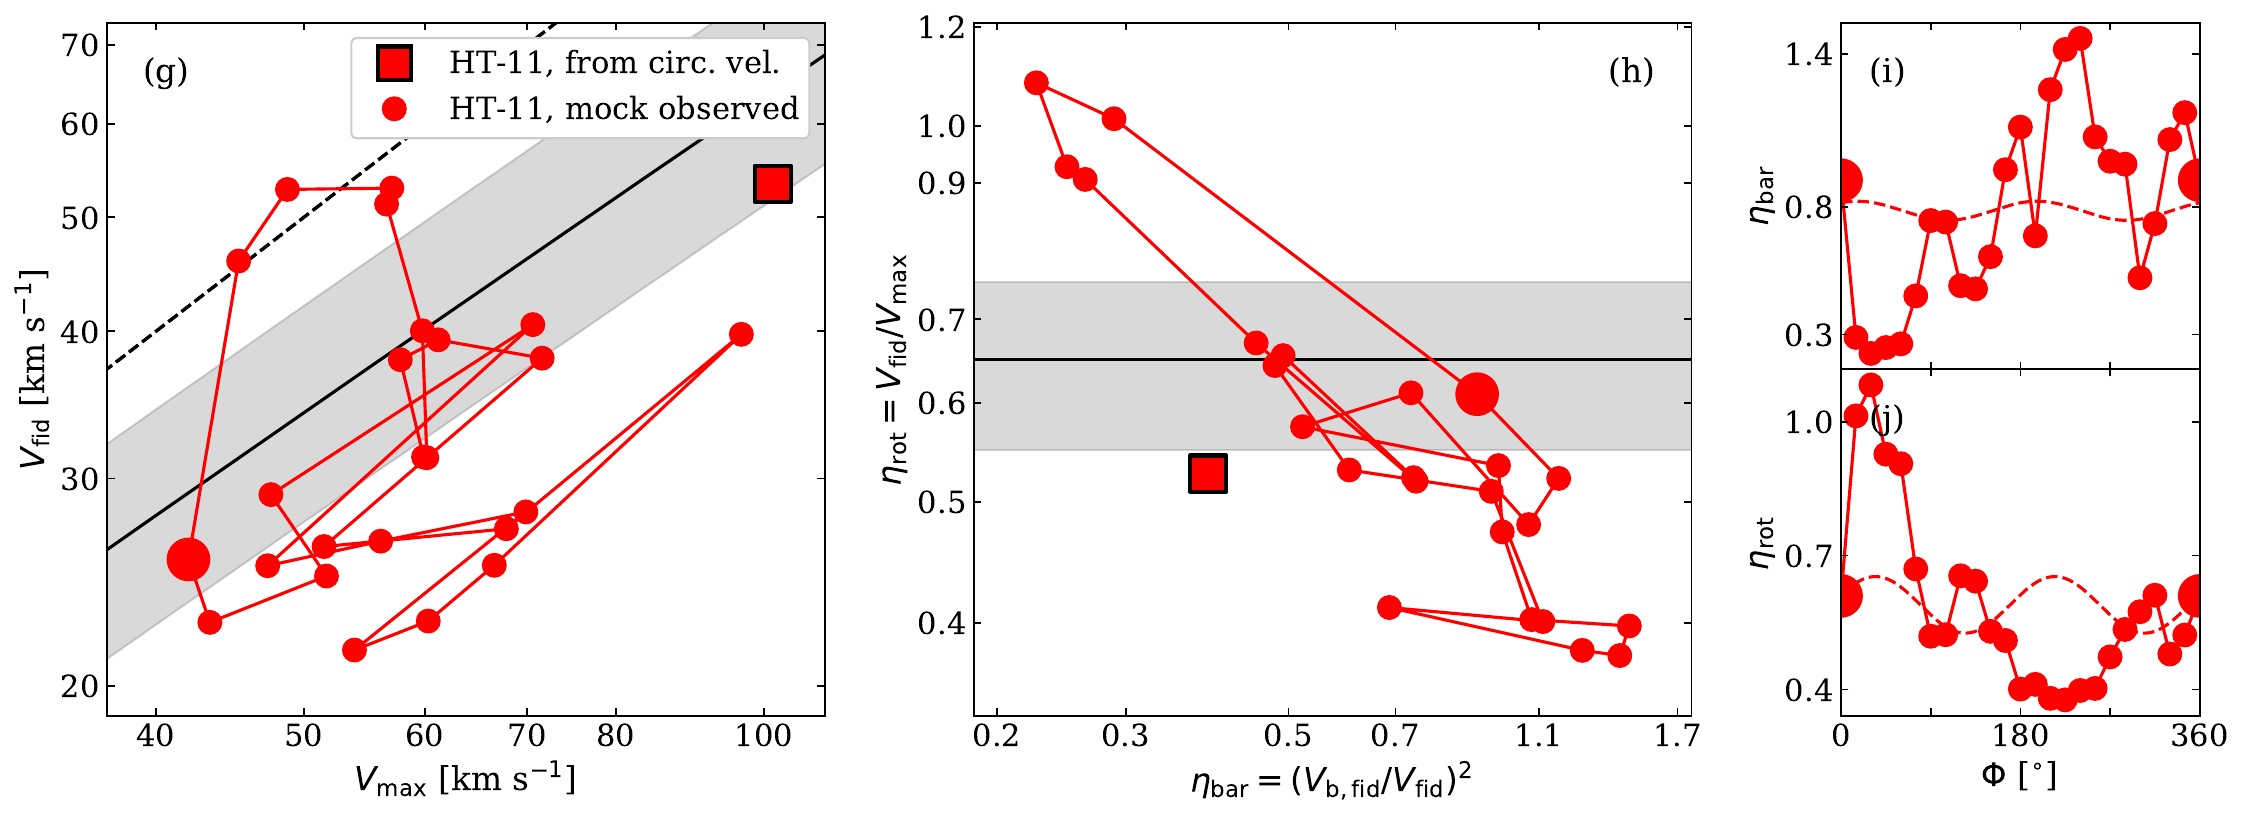}
\end{minipage}
\begin{minipage}{.4\textwidth}
\includegraphics[width=\textwidth]{../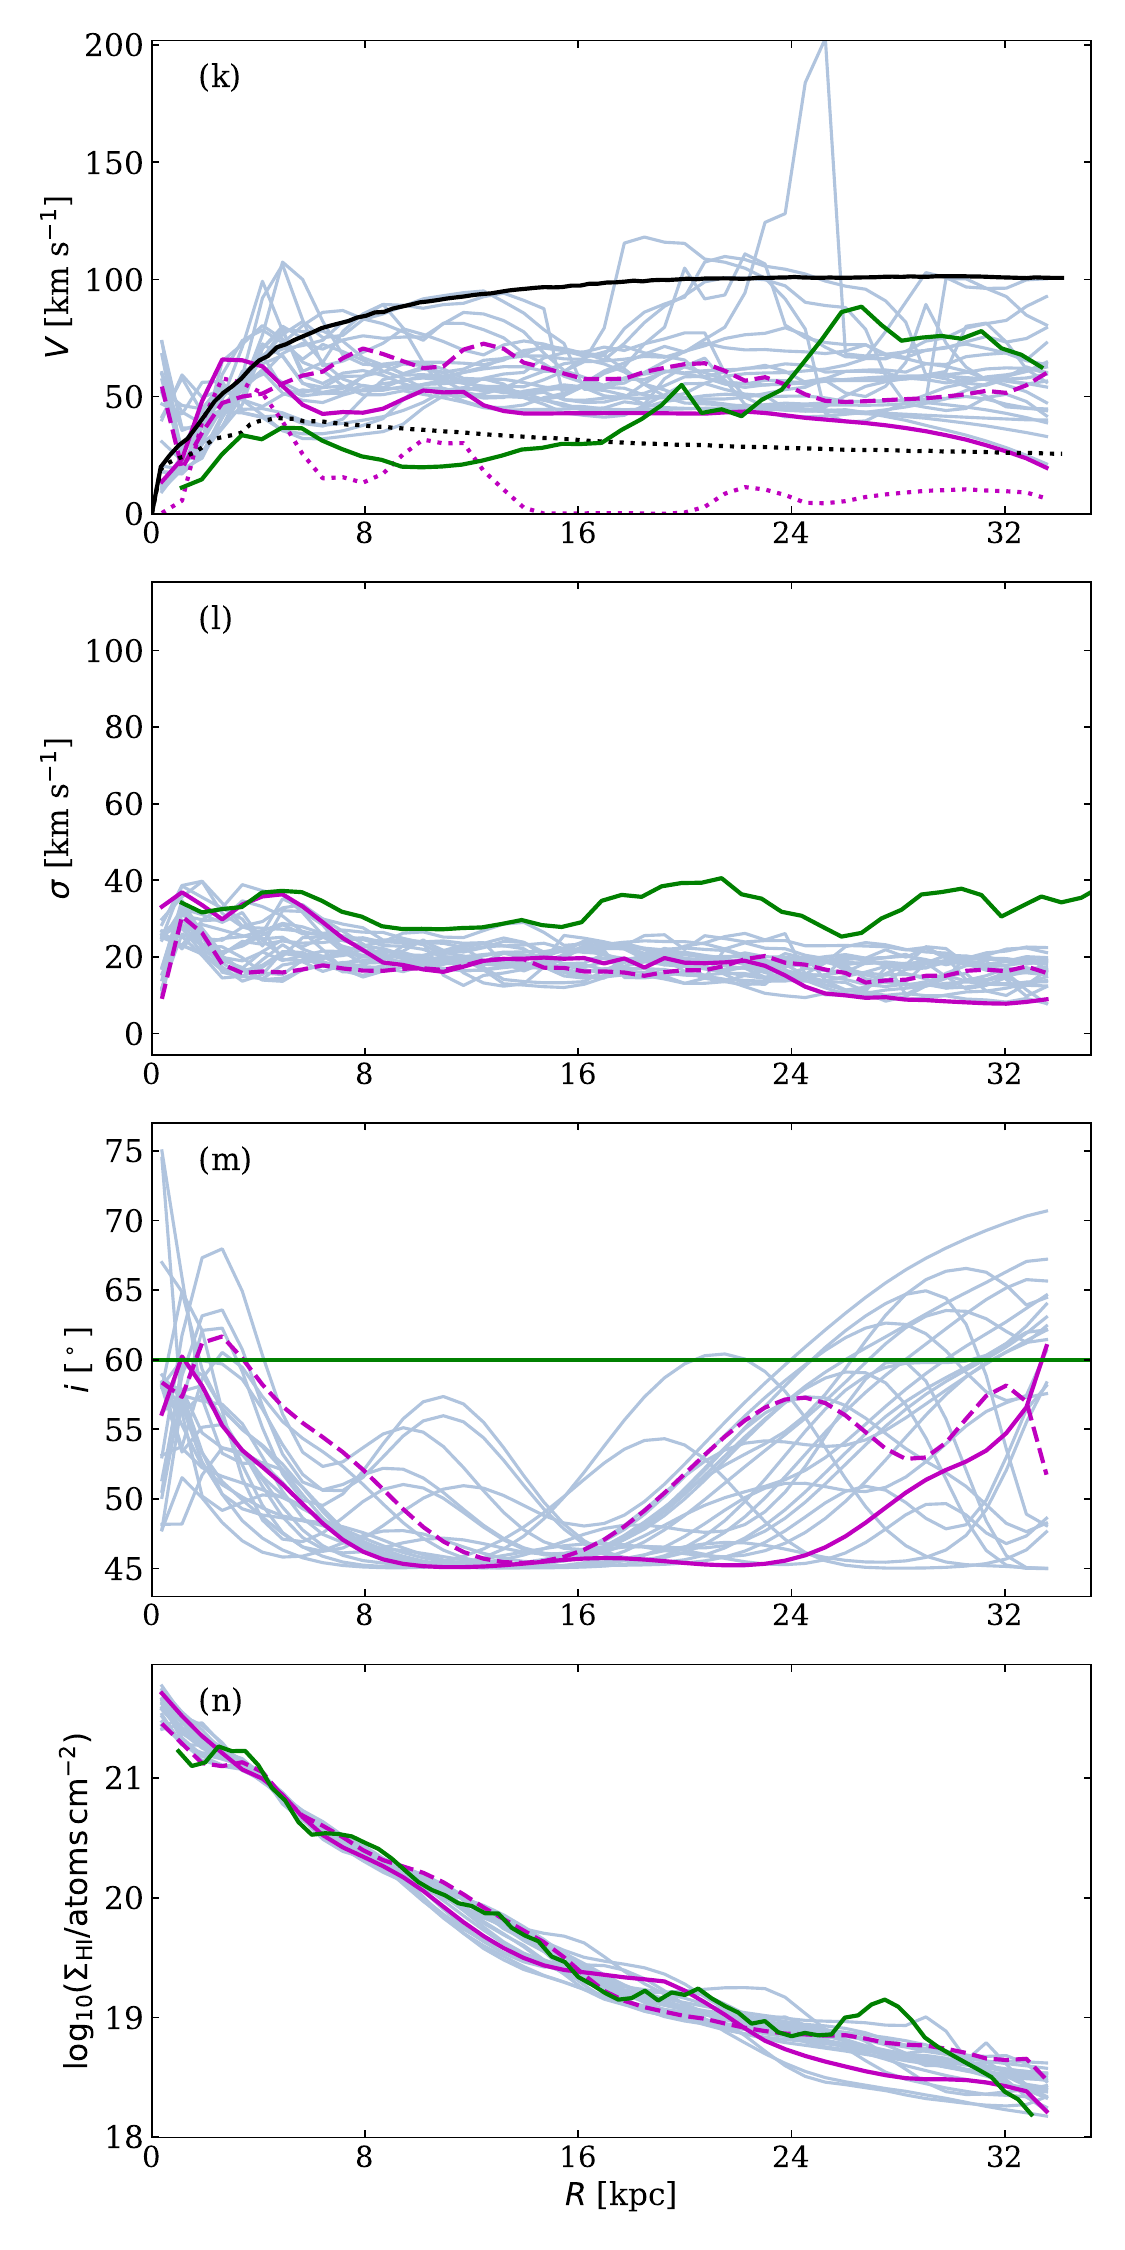}
\end{minipage}
\caption{A set of summary figures for galaxy HT-11, excluded from kinematic analysis. These include example moment maps for two orientations (panels (a)--(f); similar to Fig.~\ref{fig:visualisations}), a summary of the parameters $V_\mathrm{fid}$, $V_\mathrm{max}$, $\eta_\mathrm{rot}$, and $\eta_\mathrm{bar}$ (panels (g)--(j); similar to Fig.~\ref{fig:loops}), and a summary of the rotation curve analysis from $24$ viewing angles (panels (k)--(n); similar to Fig.~\ref{fig:rot_curves}). See description of Appendix~\ref{app:supplementary} for details.}
\label{fig:S59}
\end{figure}
\clearpage

\begin{figure}
\begin{minipage}{.9\textwidth}
\includegraphics[width=\textwidth]{../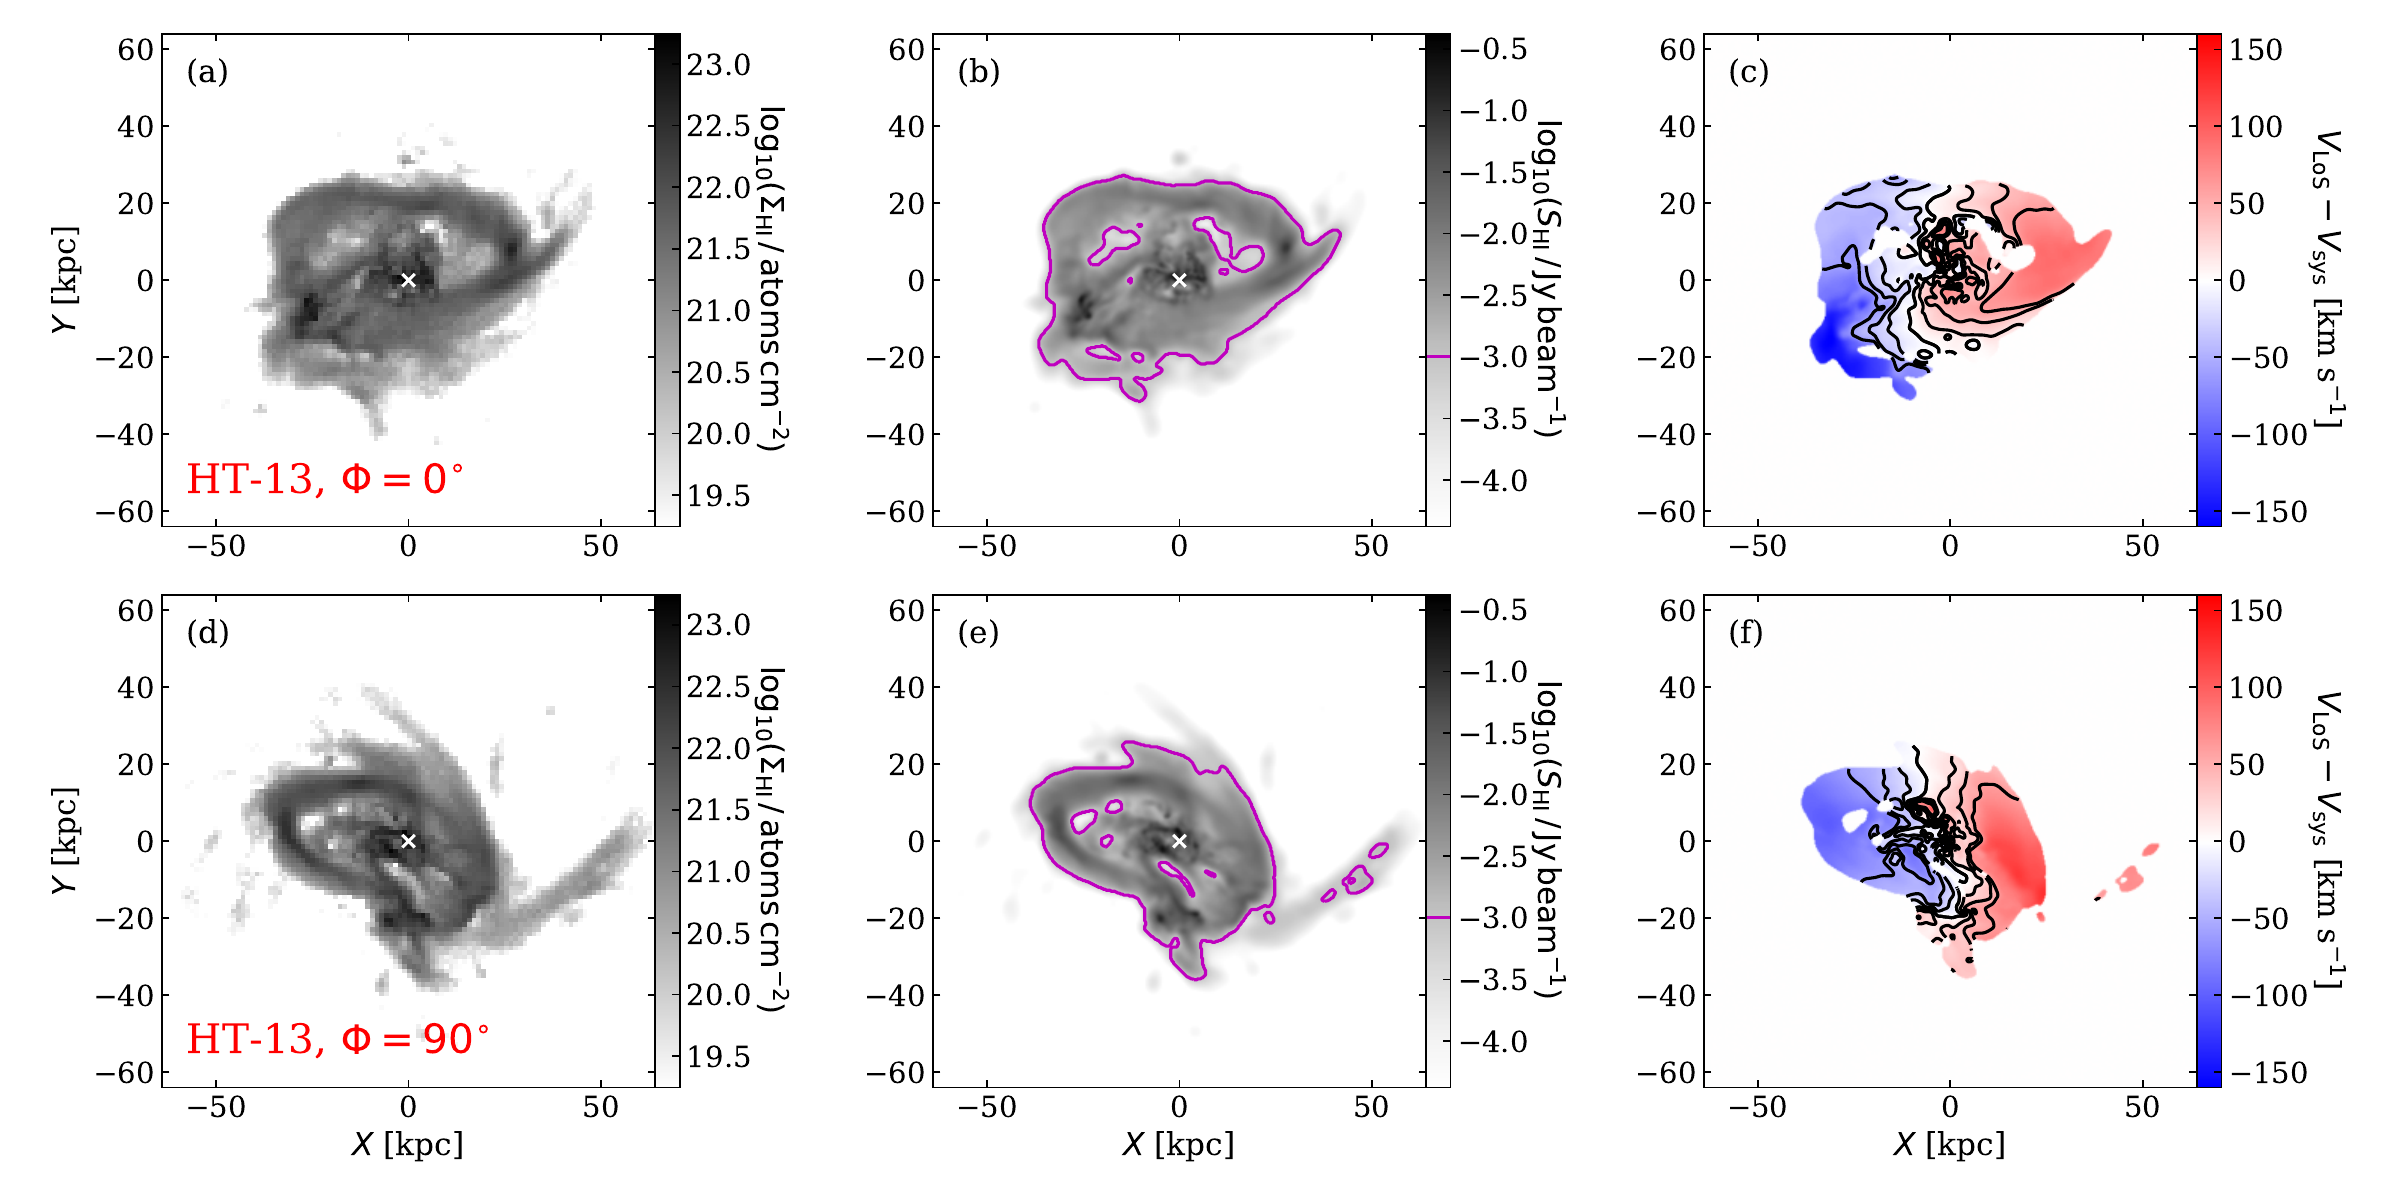}
\includegraphics[width=\textwidth]{../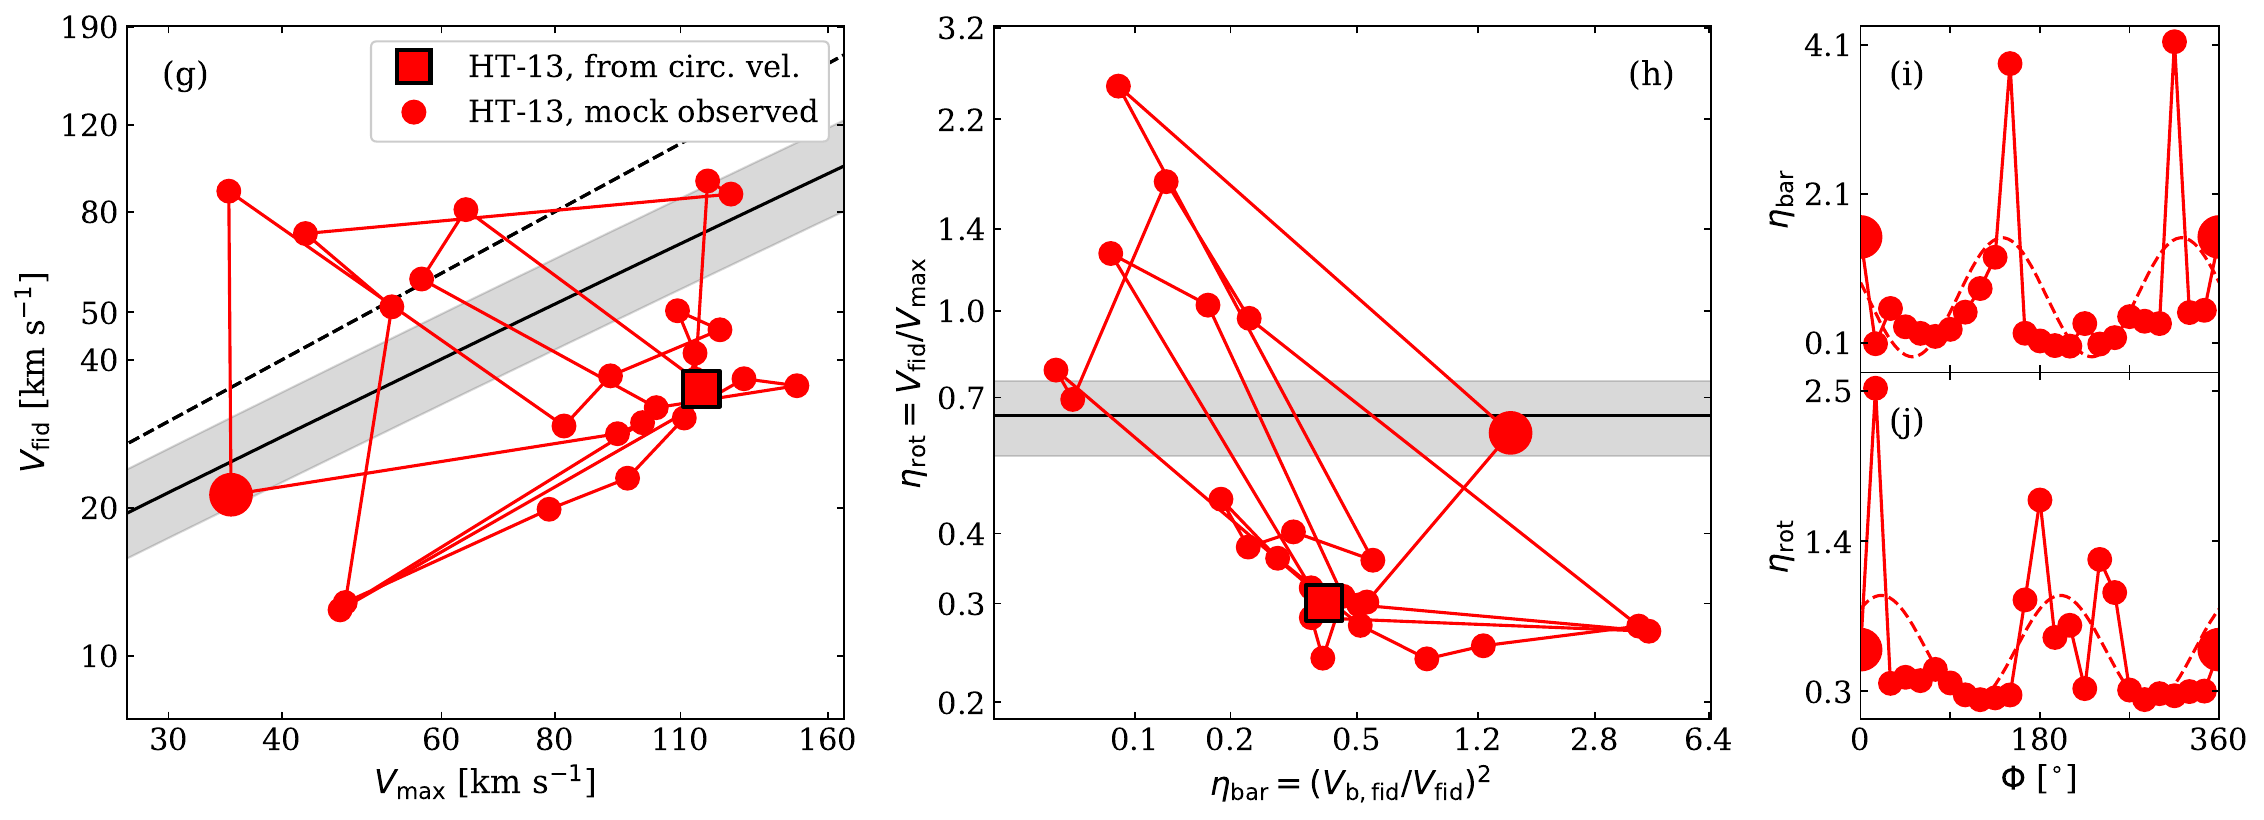}
\end{minipage}
\begin{minipage}{.4\textwidth}
\includegraphics[width=\textwidth]{../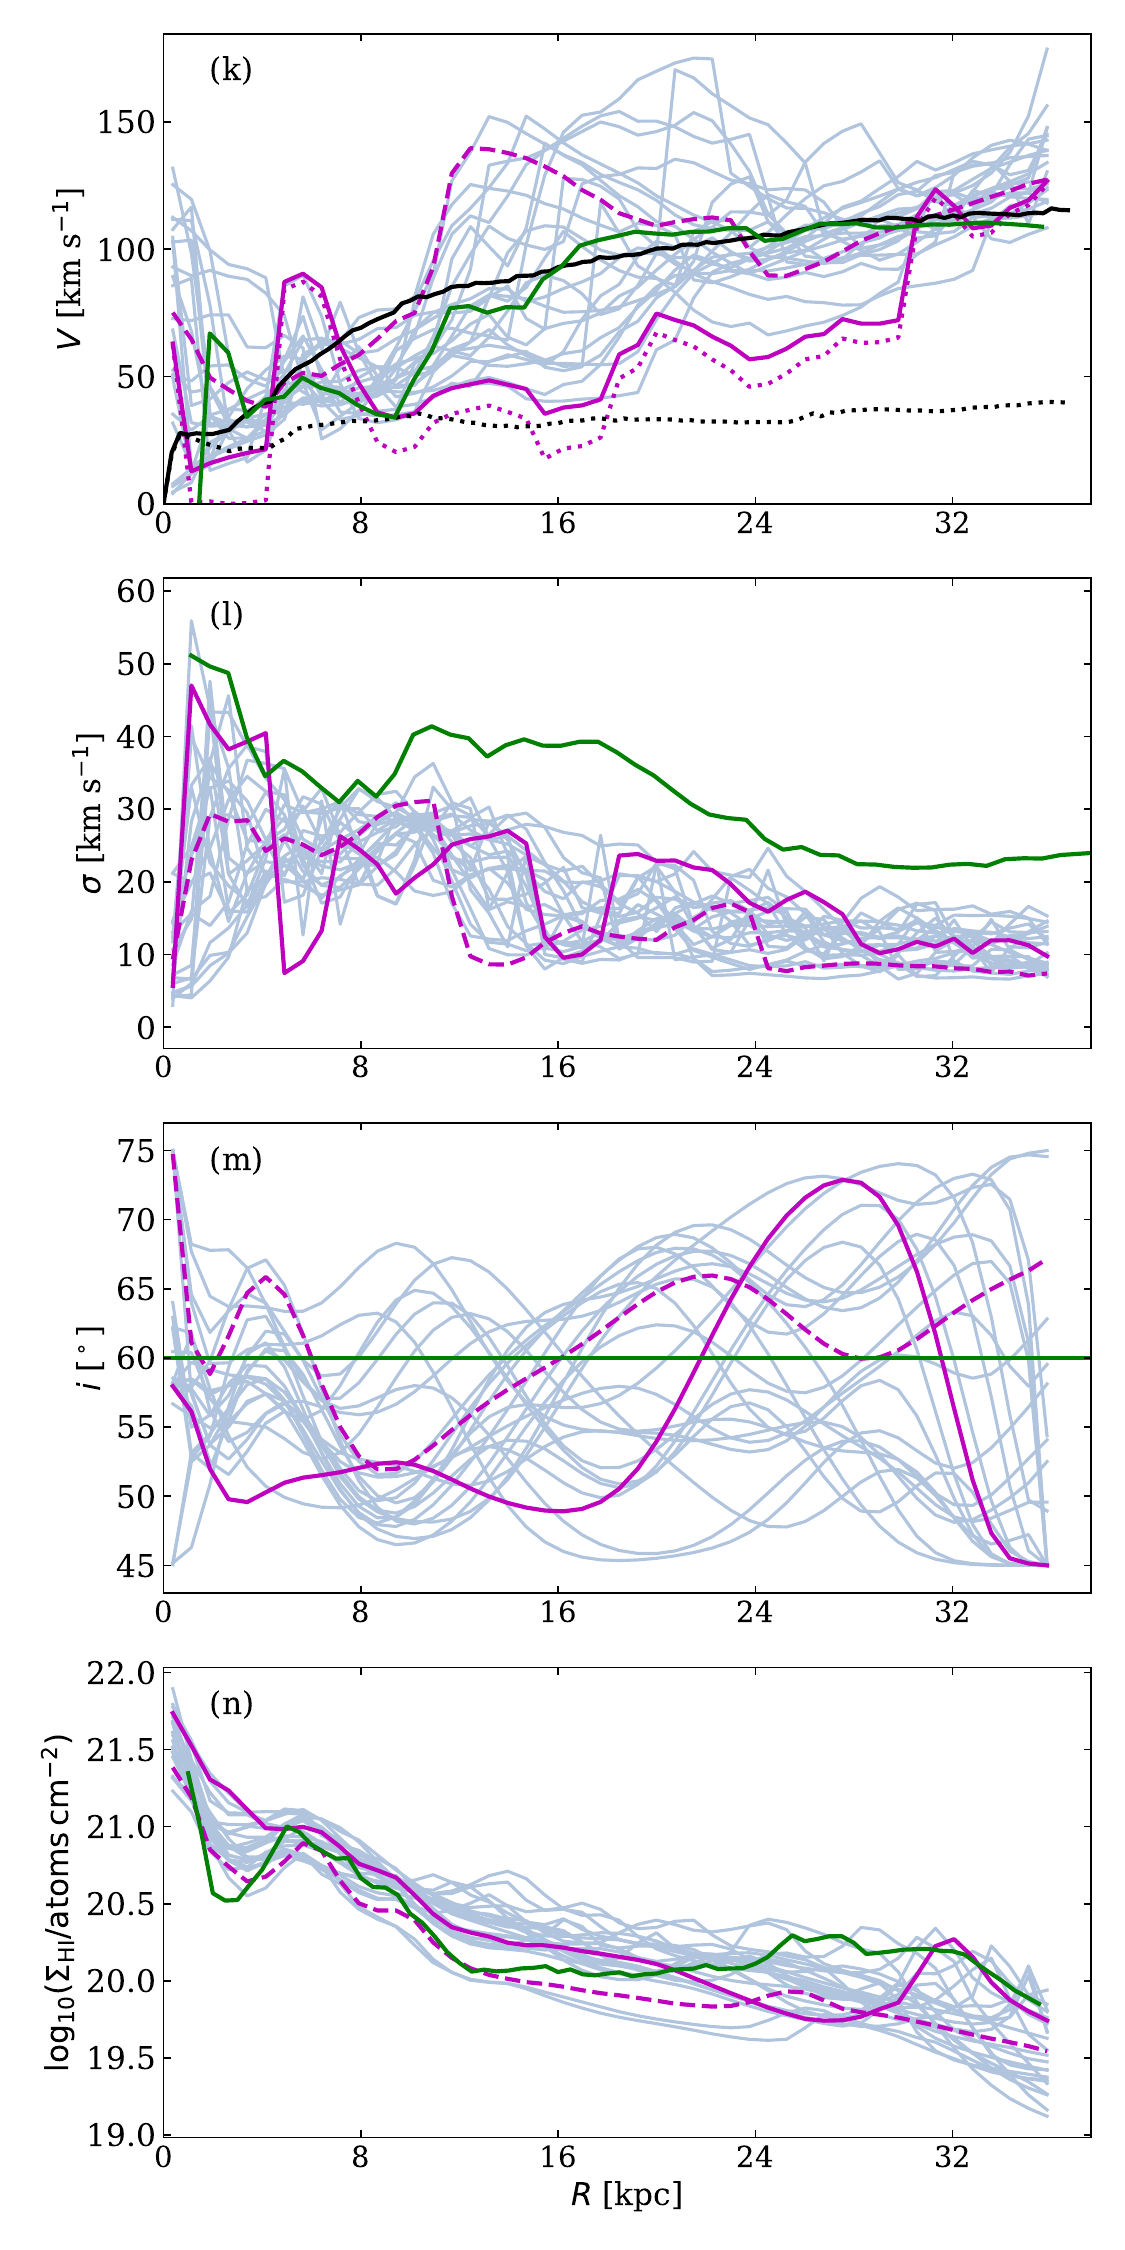}
\end{minipage}
\caption{A set of summary figures for galaxy HT-13, excluded from kinematic analysis. These include example moment maps for two orientations (panels (a)--(f); similar to Fig.~\ref{fig:visualisations}), a summary of the parameters $V_\mathrm{fid}$, $V_\mathrm{max}$, $\eta_\mathrm{rot}$, and $\eta_\mathrm{bar}$ (panels (g)--(j); similar to Fig.~\ref{fig:loops}), and a summary of the rotation curve analysis from $24$ viewing angles (panels (k)--(n); similar to Fig.~\ref{fig:rot_curves}). See description of Appendix~\ref{app:supplementary} for details.}
\label{fig:S60}
\end{figure}
\clearpage

\begin{figure}
\begin{minipage}{.9\textwidth}
\includegraphics[width=\textwidth]{../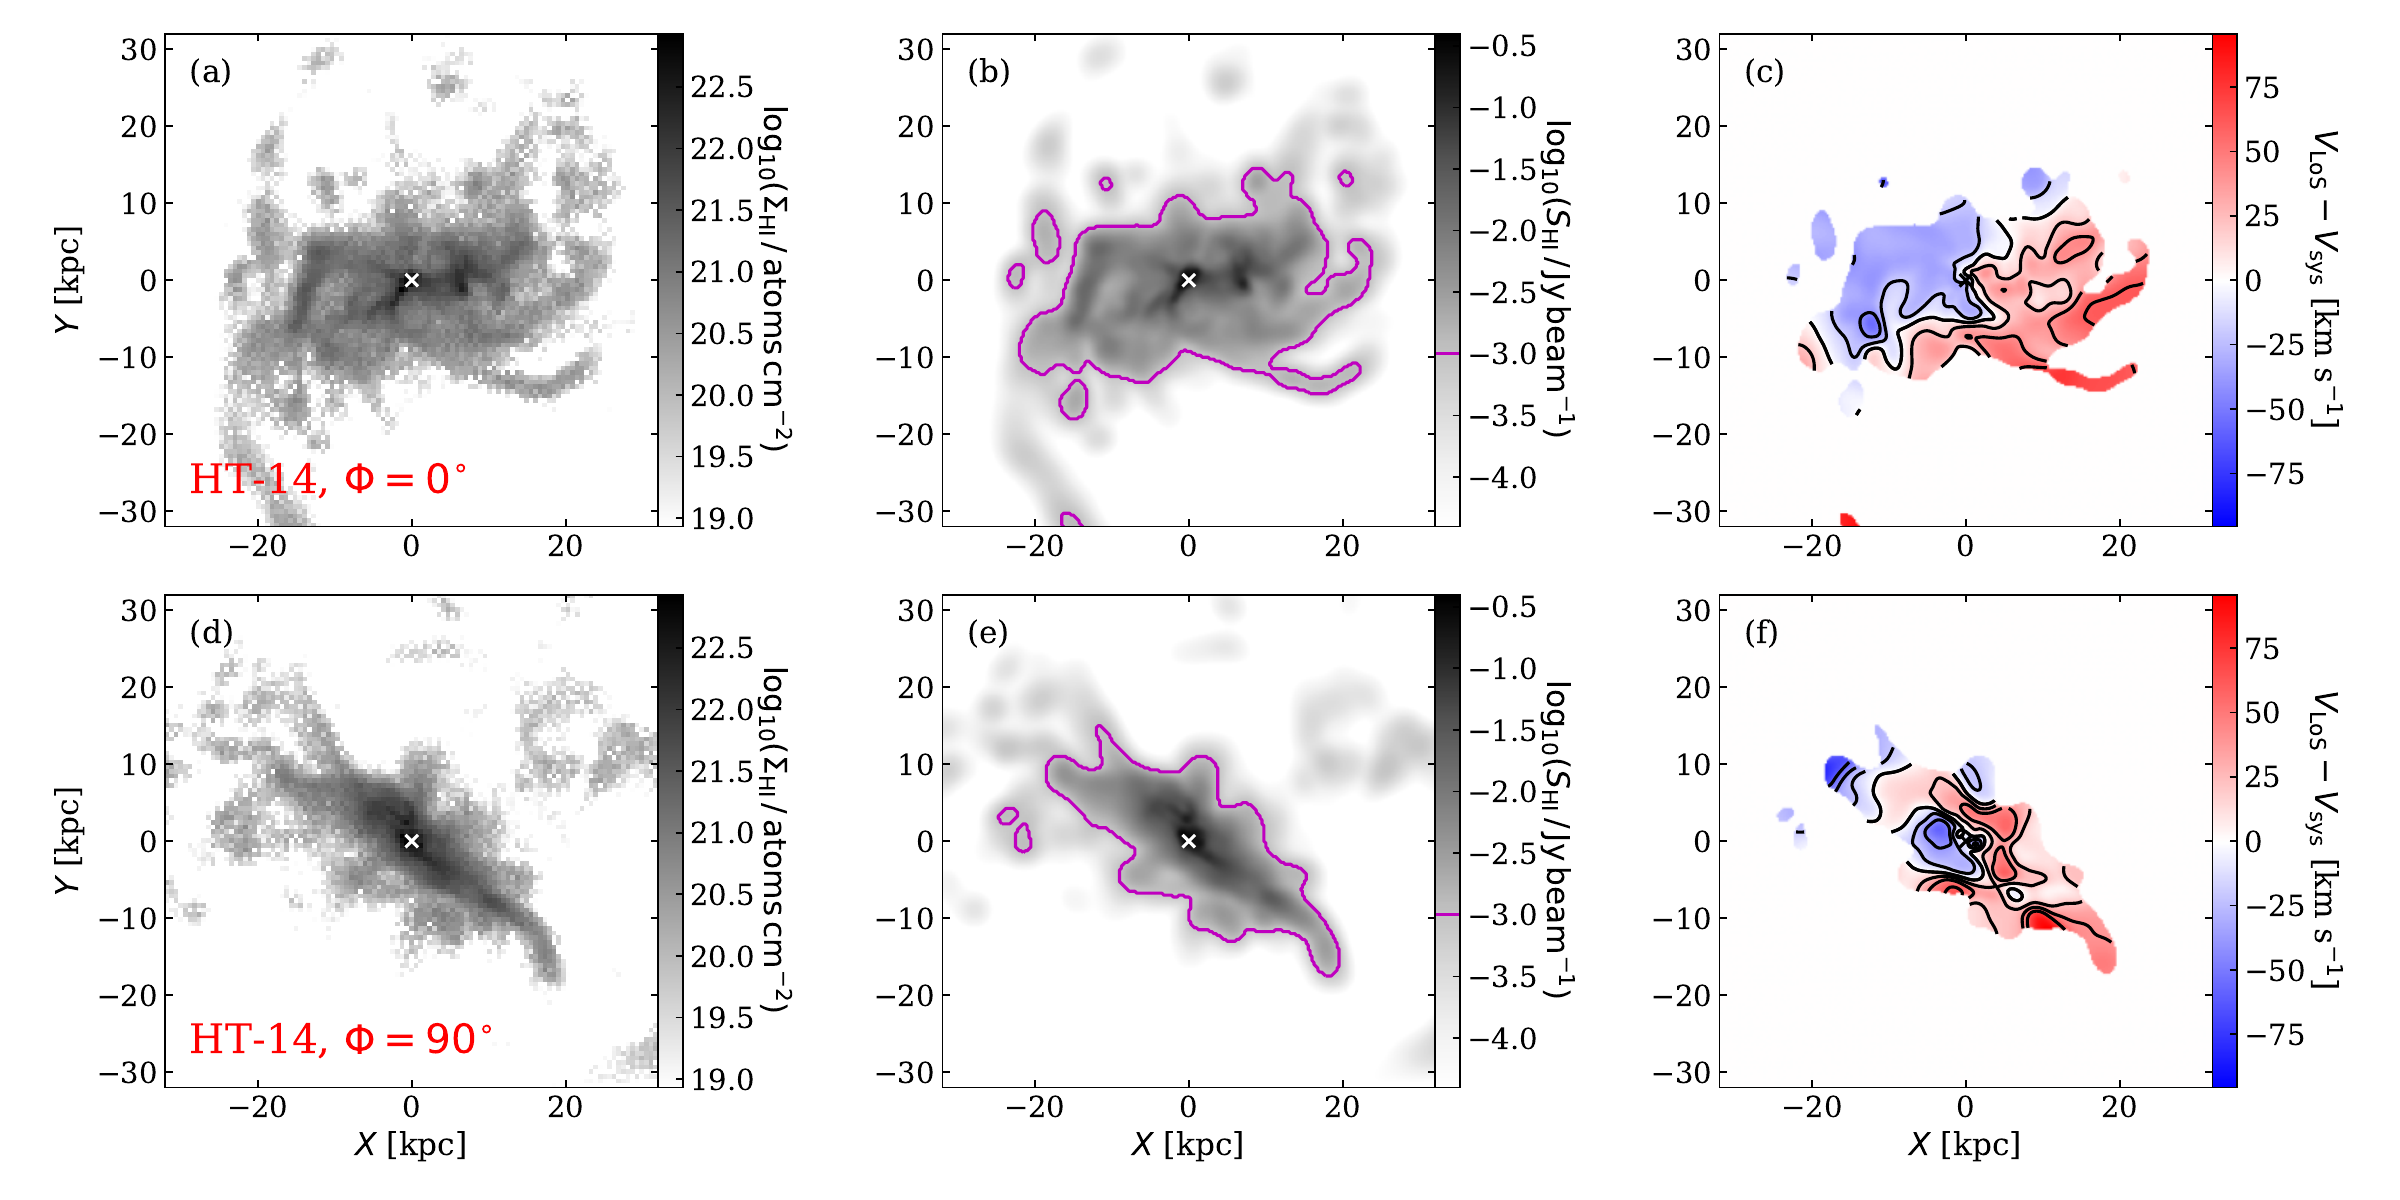}
\includegraphics[width=\textwidth]{../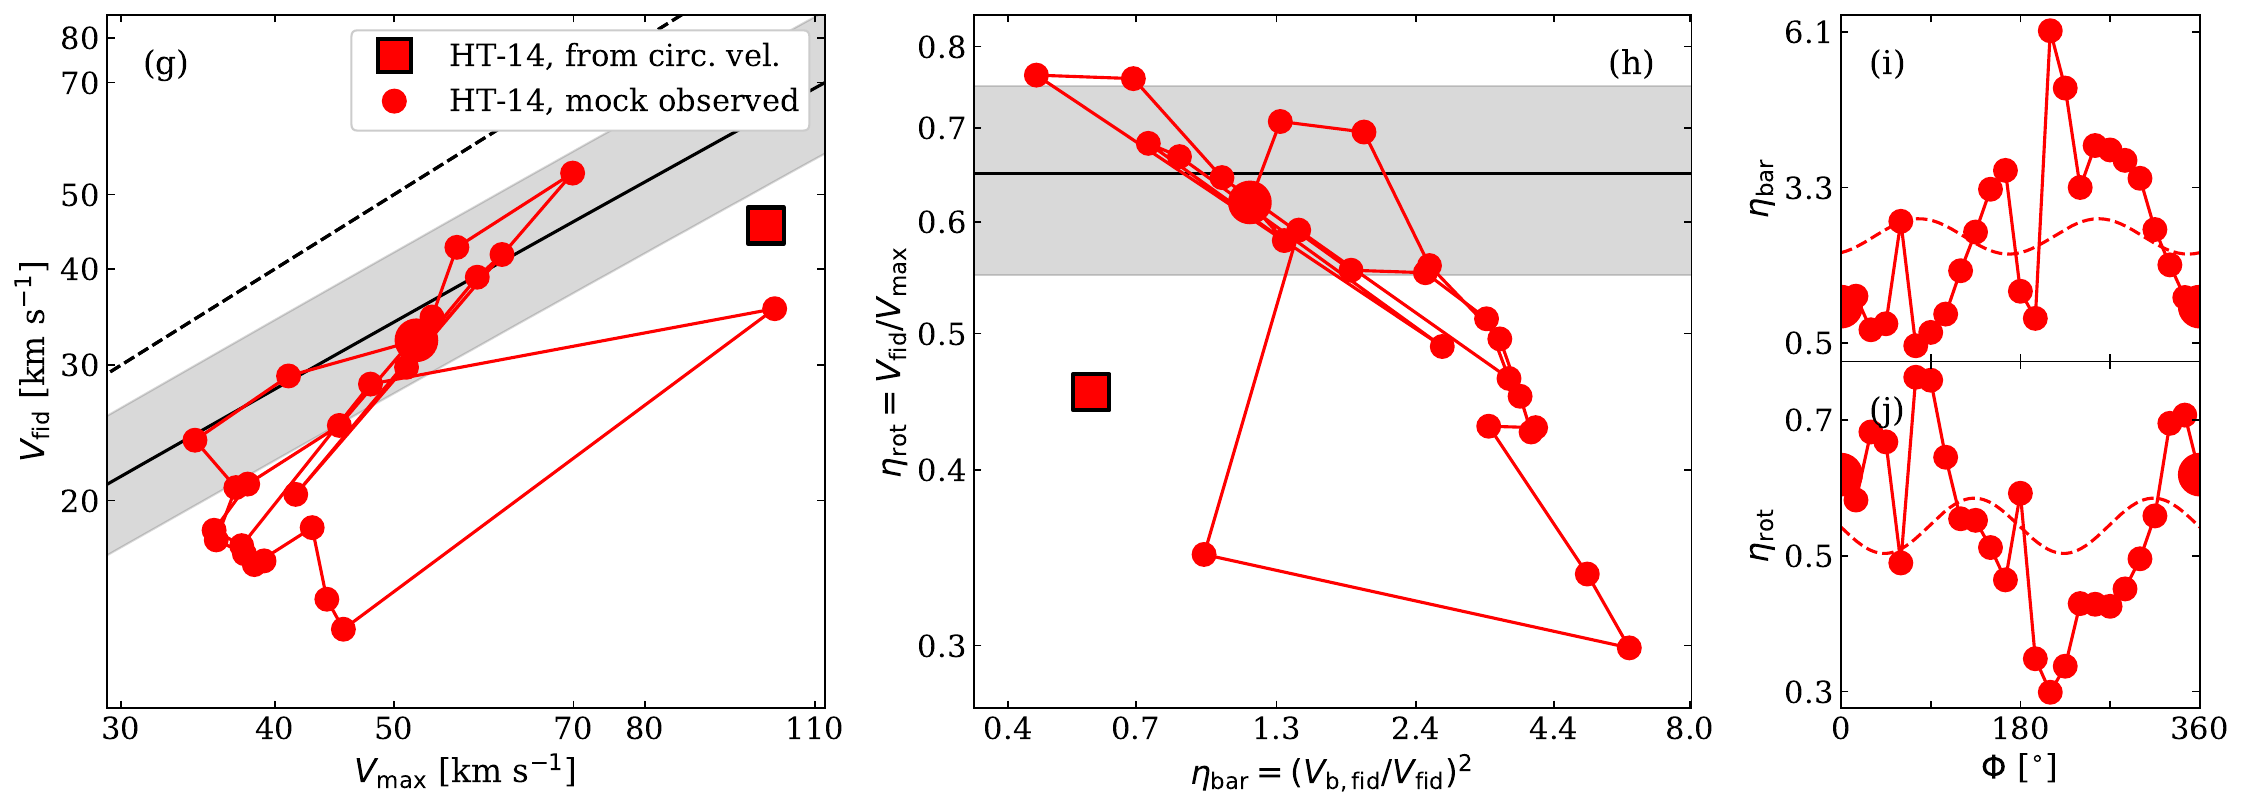}
\end{minipage}
\begin{minipage}{.4\textwidth}
\includegraphics[width=\textwidth]{../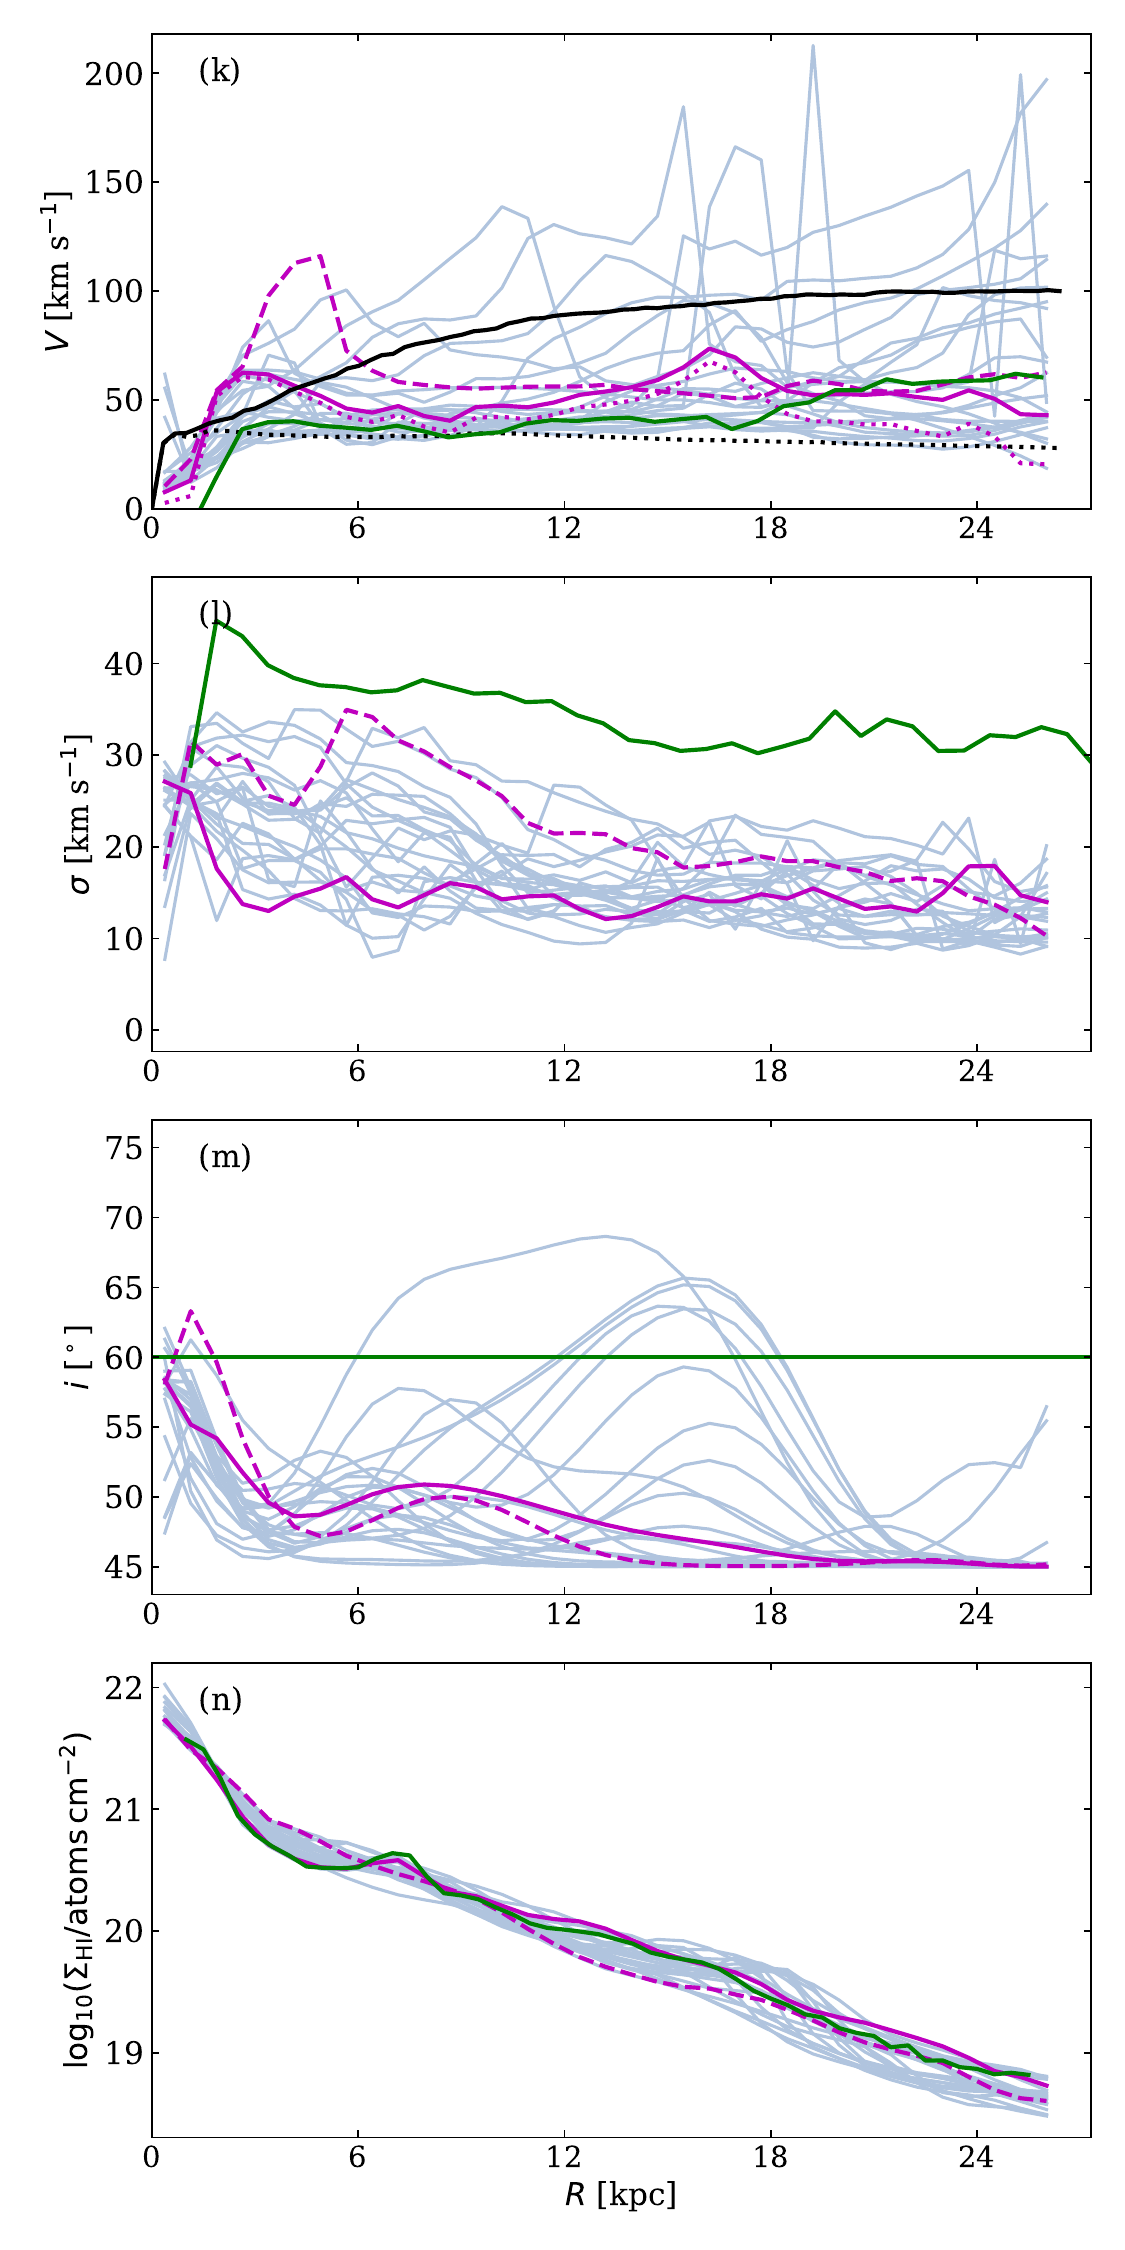}
\end{minipage}
\caption{A set of summary figures for galaxy HT-14, excluded from kinematic analysis. These include example moment maps for two orientations (panels (a)--(f); similar to Fig.~\ref{fig:visualisations}), a summary of the parameters $V_\mathrm{fid}$, $V_\mathrm{max}$, $\eta_\mathrm{rot}$, and $\eta_\mathrm{bar}$ (panels (g)--(j); similar to Fig.~\ref{fig:loops}), and a summary of the rotation curve analysis from $24$ viewing angles (panels (k)--(n); similar to Fig.~\ref{fig:rot_curves}). See description of Appendix~\ref{app:supplementary} for details.}
\label{fig:S61}
\end{figure}
\clearpage

\begin{figure}
\begin{minipage}{.9\textwidth}
\includegraphics[width=\textwidth]{../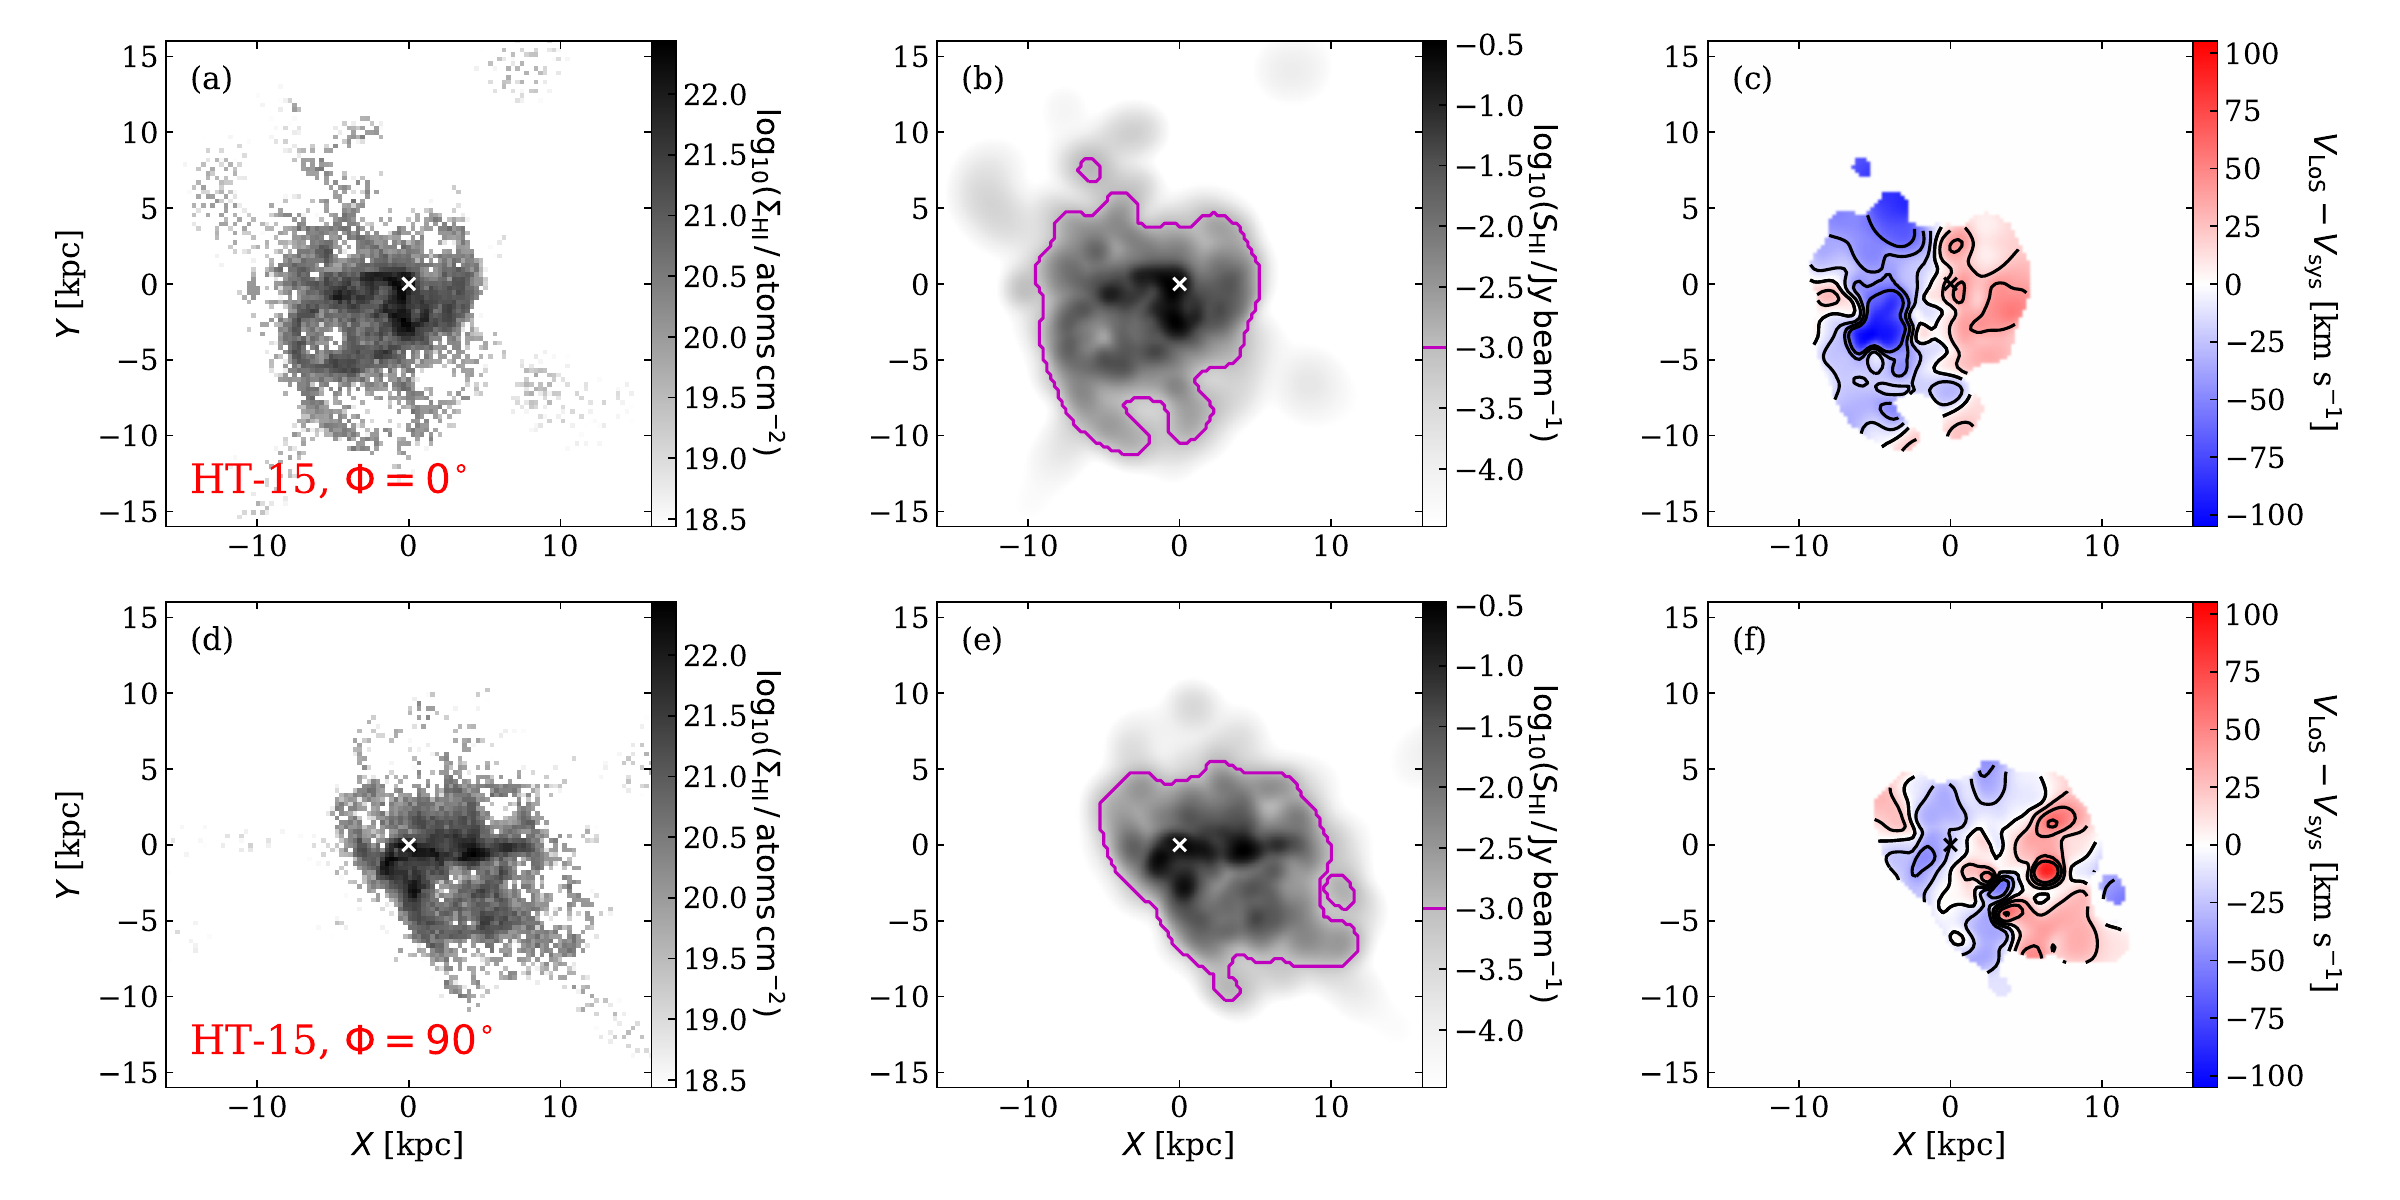}
\includegraphics[width=\textwidth]{../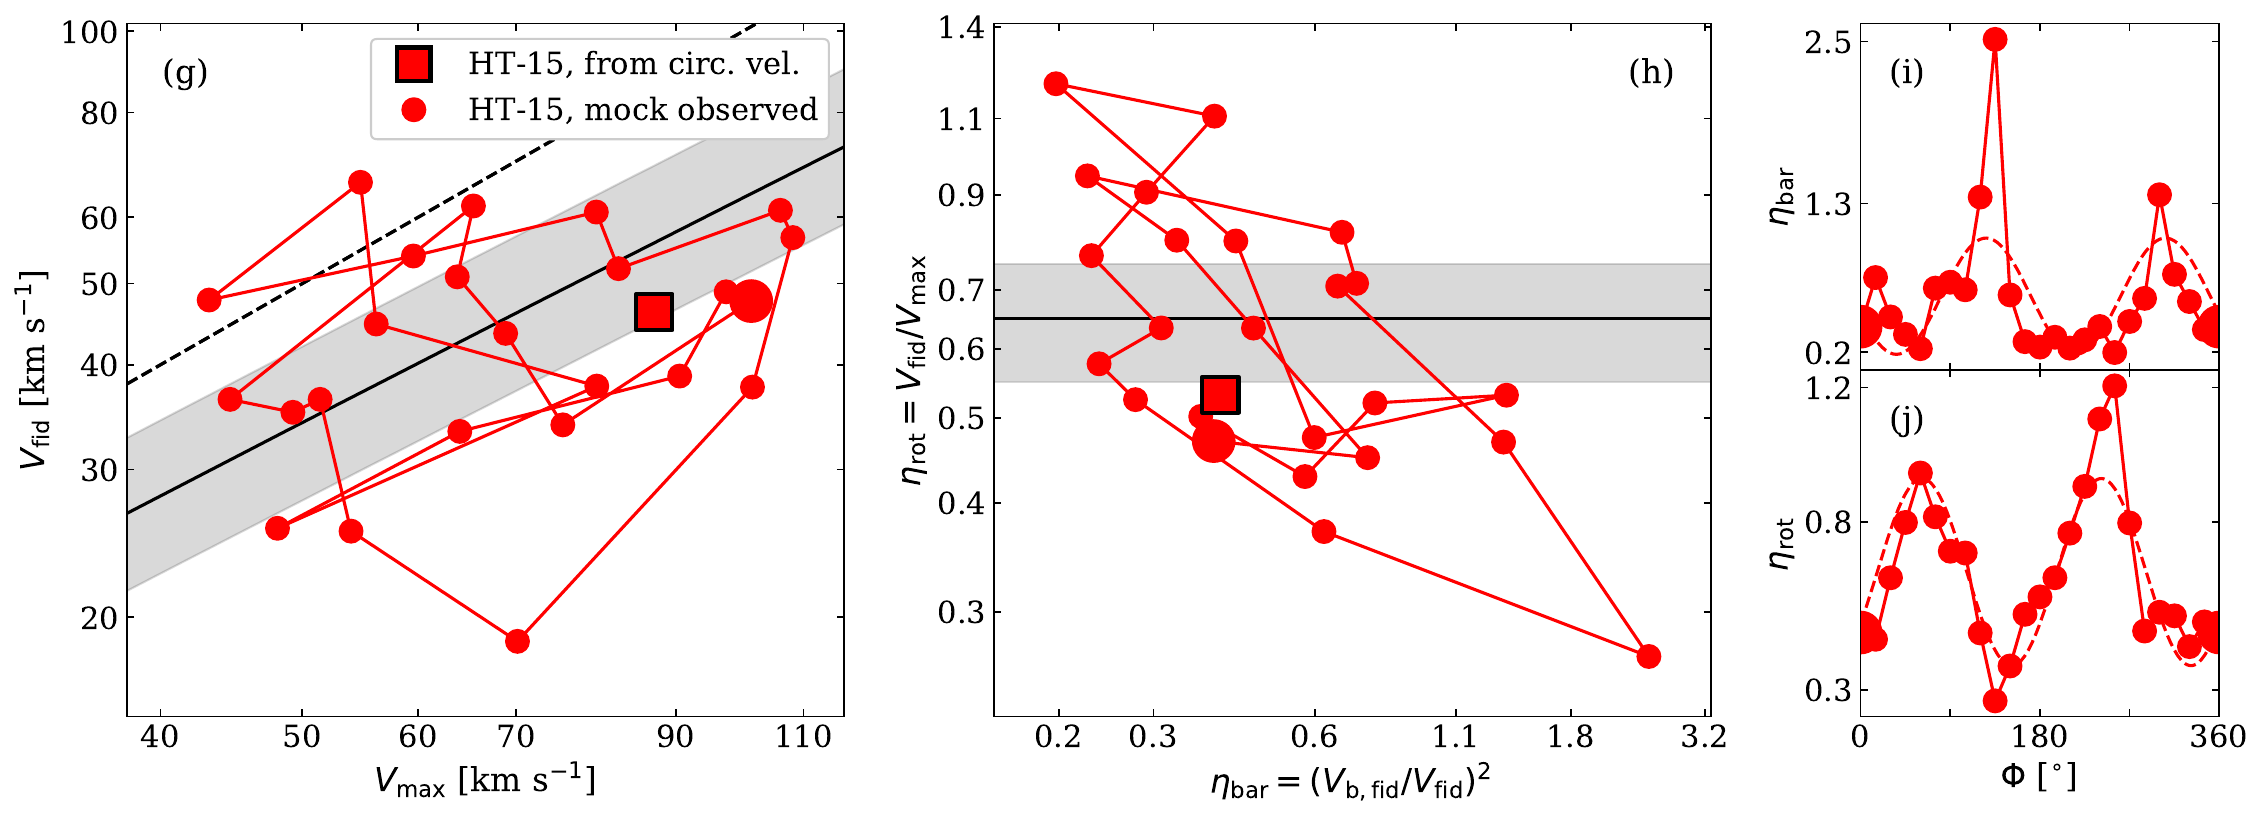}
\end{minipage}
\begin{minipage}{.4\textwidth}
\includegraphics[width=\textwidth]{../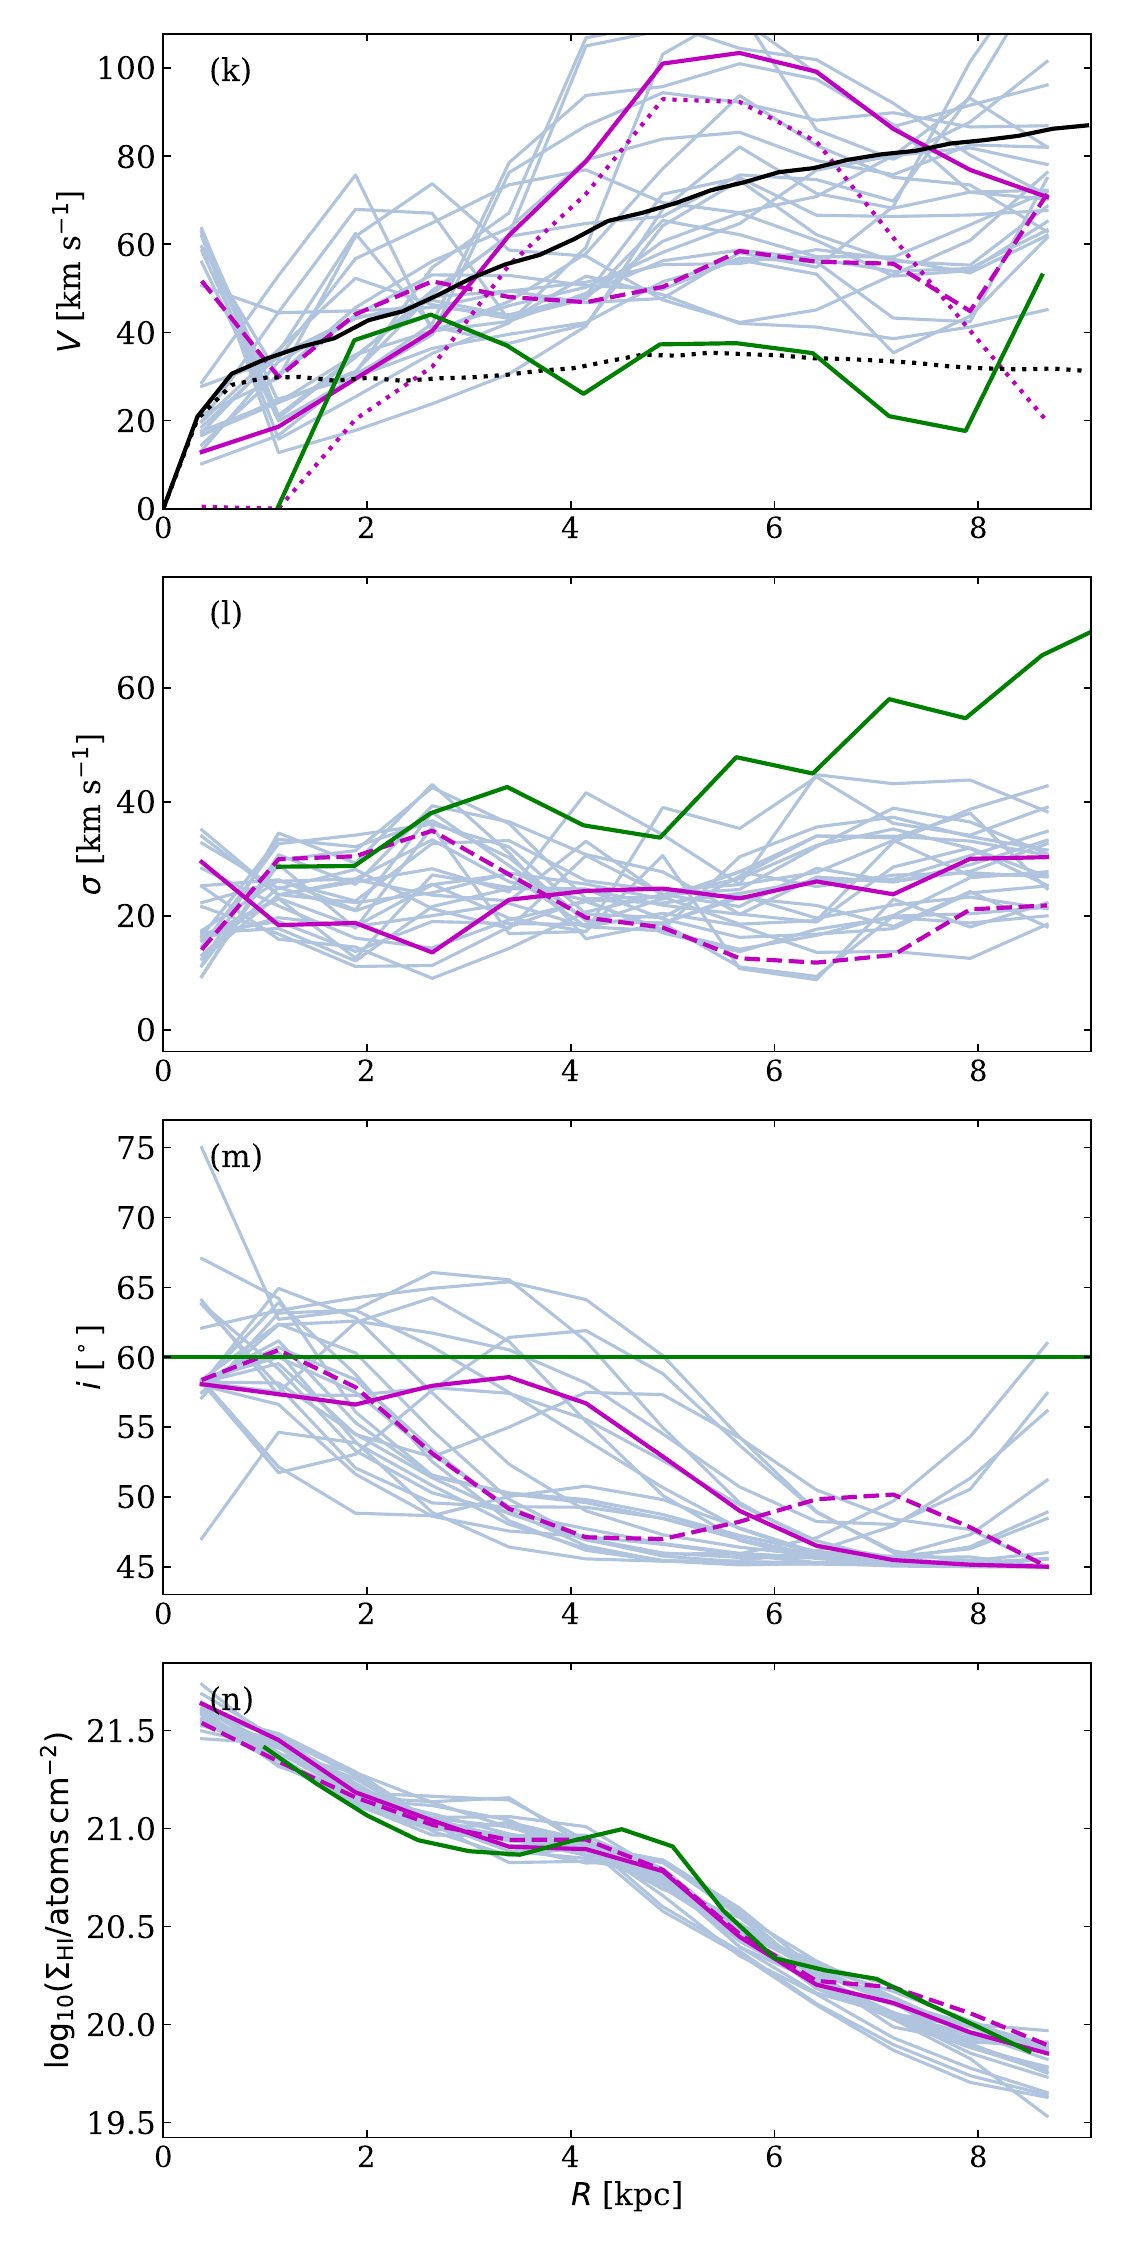}
\end{minipage}
\caption{A set of summary figures for galaxy HT-15, excluded from kinematic analysis. These include example moment maps for two orientations (panels (a)--(f); similar to Fig.~\ref{fig:visualisations}), a summary of the parameters $V_\mathrm{fid}$, $V_\mathrm{max}$, $\eta_\mathrm{rot}$, and $\eta_\mathrm{bar}$ (panels (g)--(j); similar to Fig.~\ref{fig:loops}), and a summary of the rotation curve analysis from $24$ viewing angles (panels (k)--(n); similar to Fig.~\ref{fig:rot_curves}). See description of Appendix~\ref{app:supplementary} for details.}
\label{fig:S62}
\end{figure}
\clearpage

\begin{figure}
\begin{minipage}{.9\textwidth}
\includegraphics[width=\textwidth]{../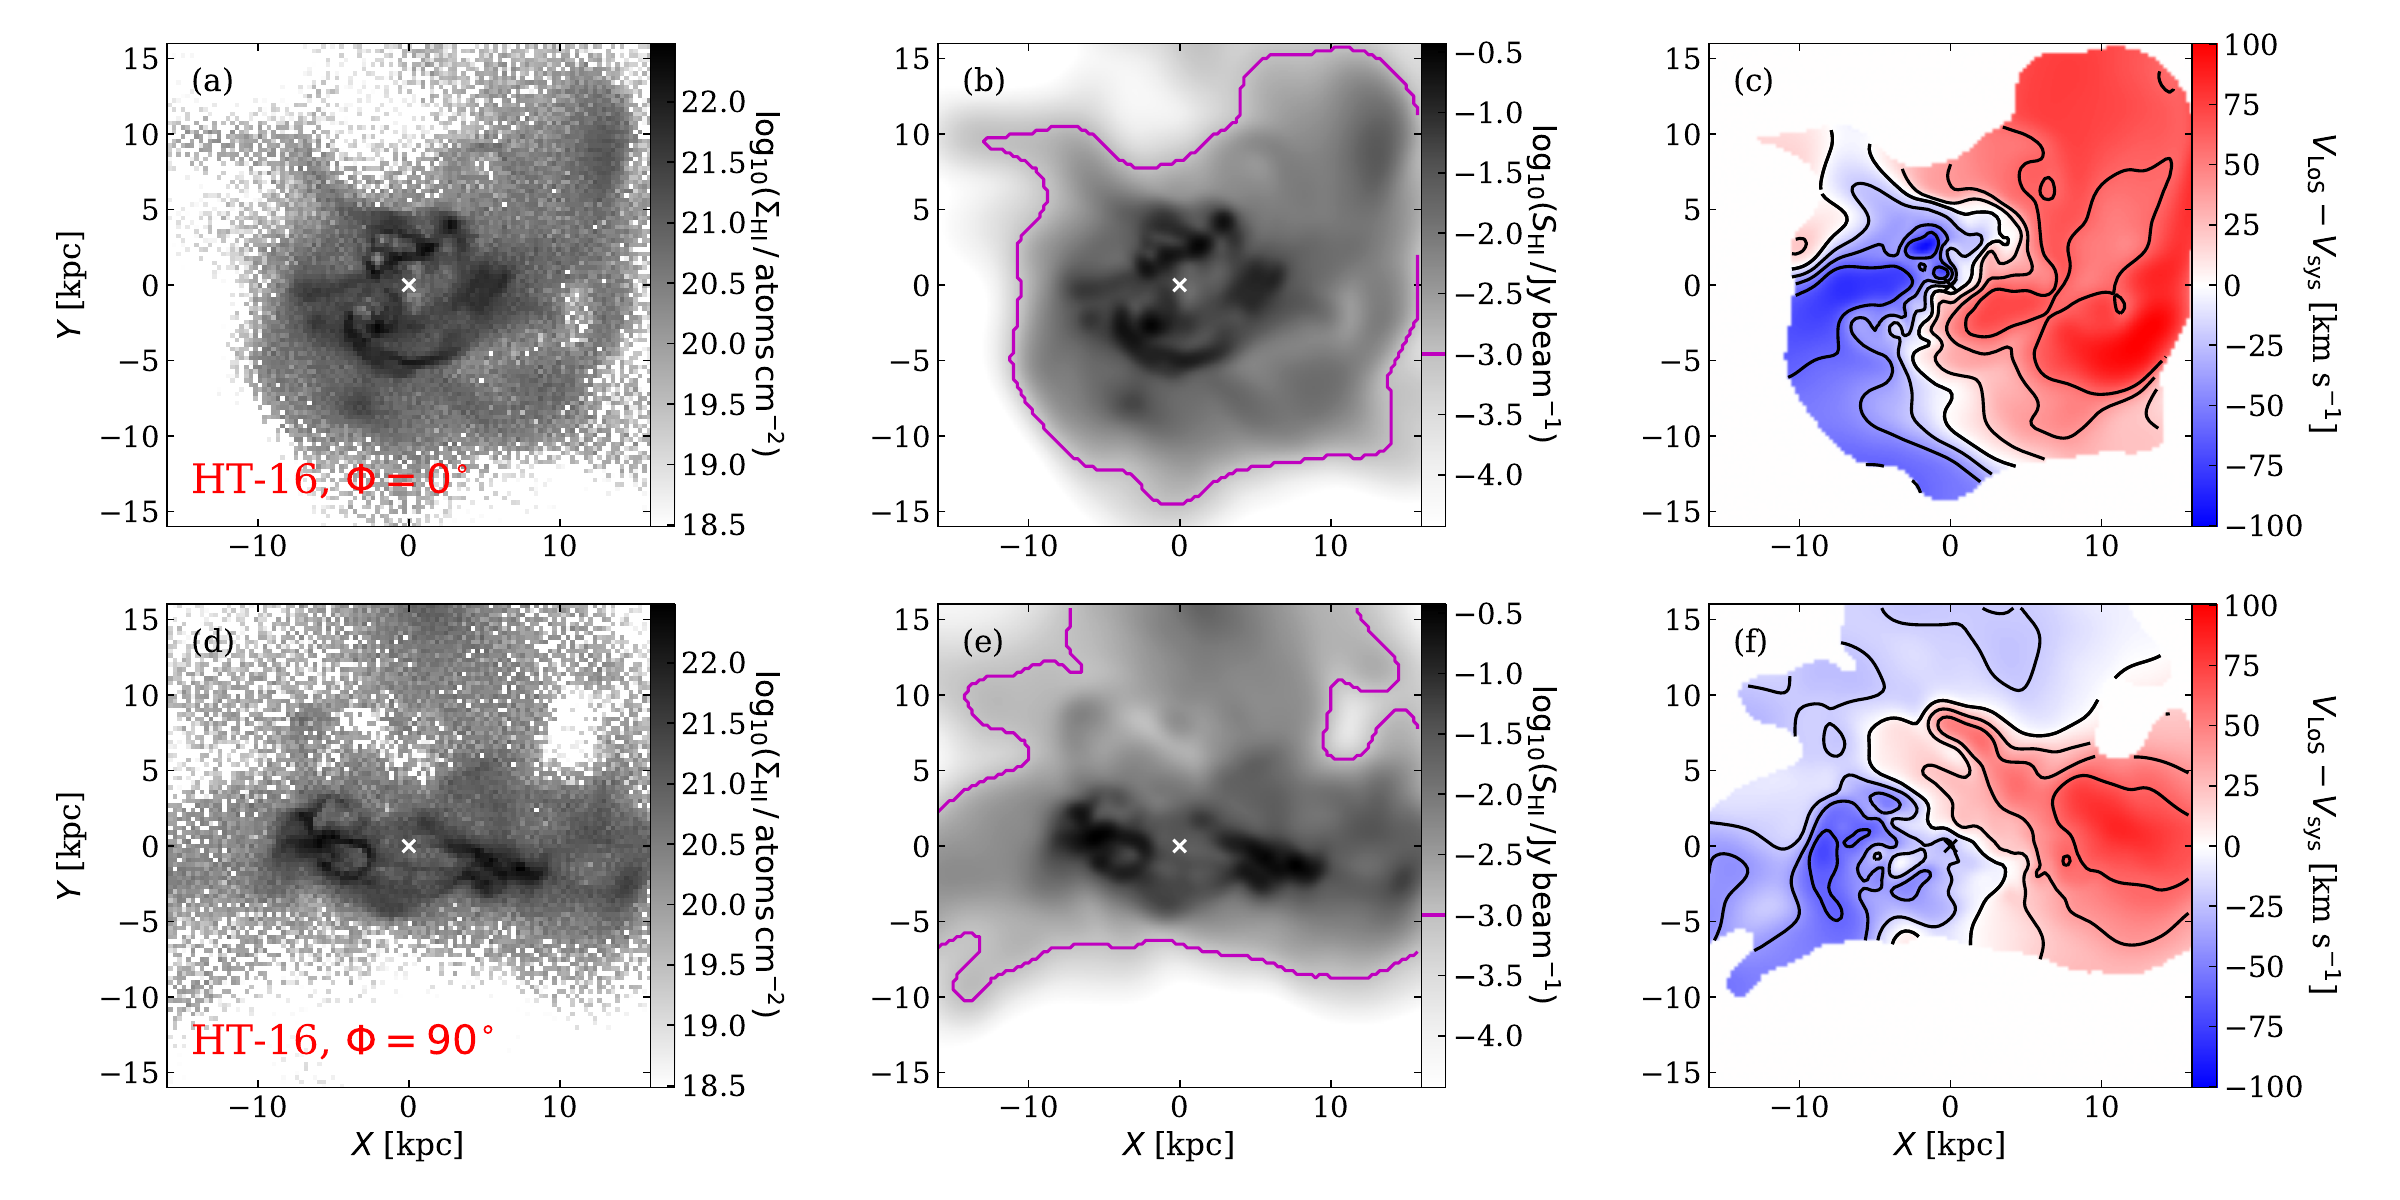}
\end{minipage}
\begin{minipage}{.4\textwidth}
\includegraphics[width=\textwidth]{../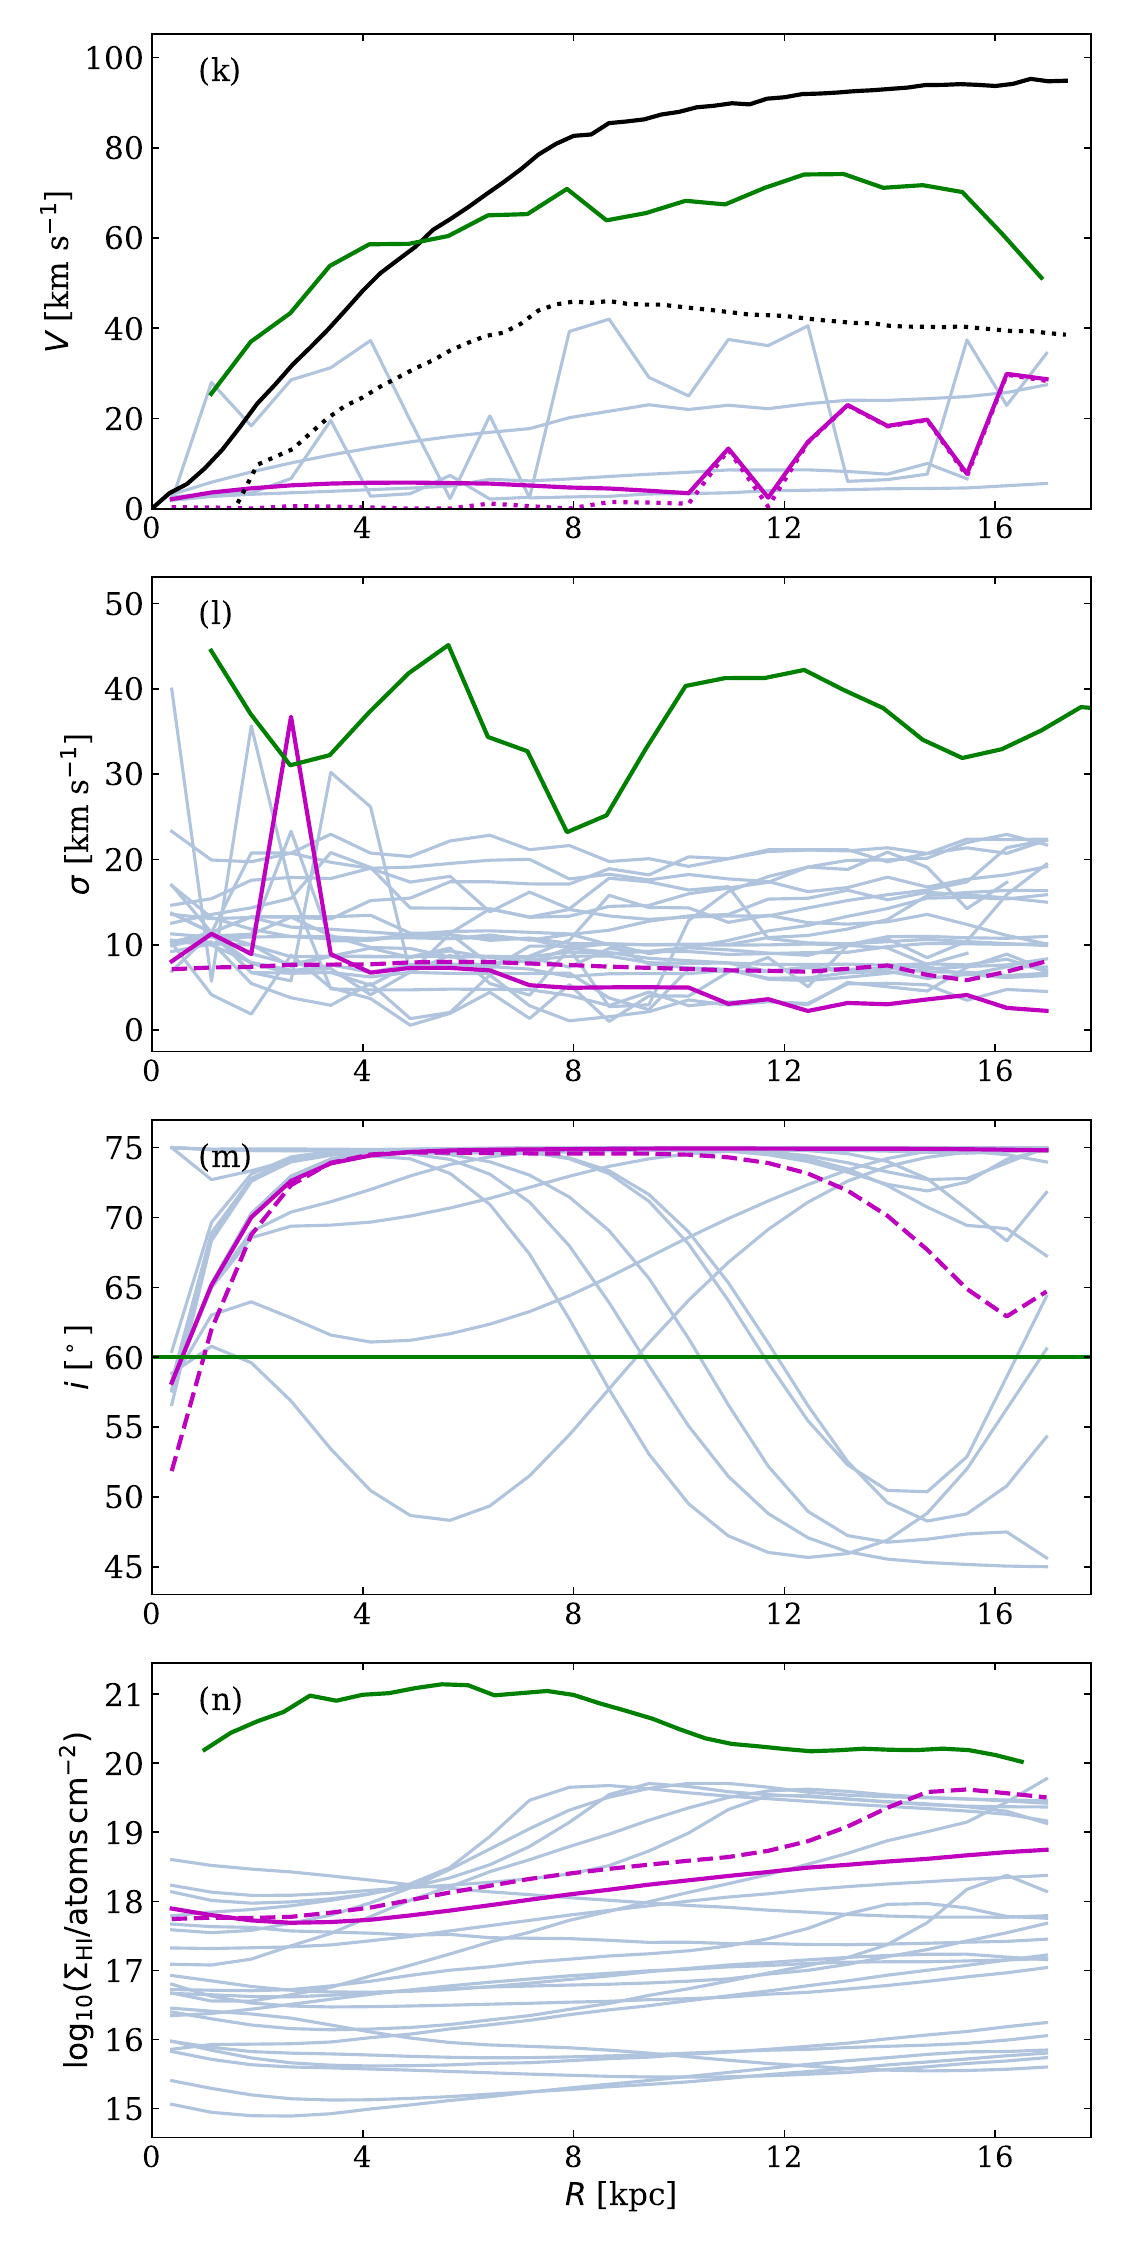}
\end{minipage}
\caption{A set of summary figures for galaxy HT-16, excluded from kinematic analysis. These include example moment maps for two orientations (panels (a)--(f); similar to Fig.~\ref{fig:visualisations}) and a summary of the rotation curve analysis from $24$ viewing angles (panels (k)--(n); similar to Fig.~\ref{fig:rot_curves}). See description of Appendix~\ref{app:supplementary} for details.}
\label{fig:S63}
\end{figure}
\clearpage

\begin{figure}
\begin{minipage}{.9\textwidth}
\includegraphics[width=\textwidth]{../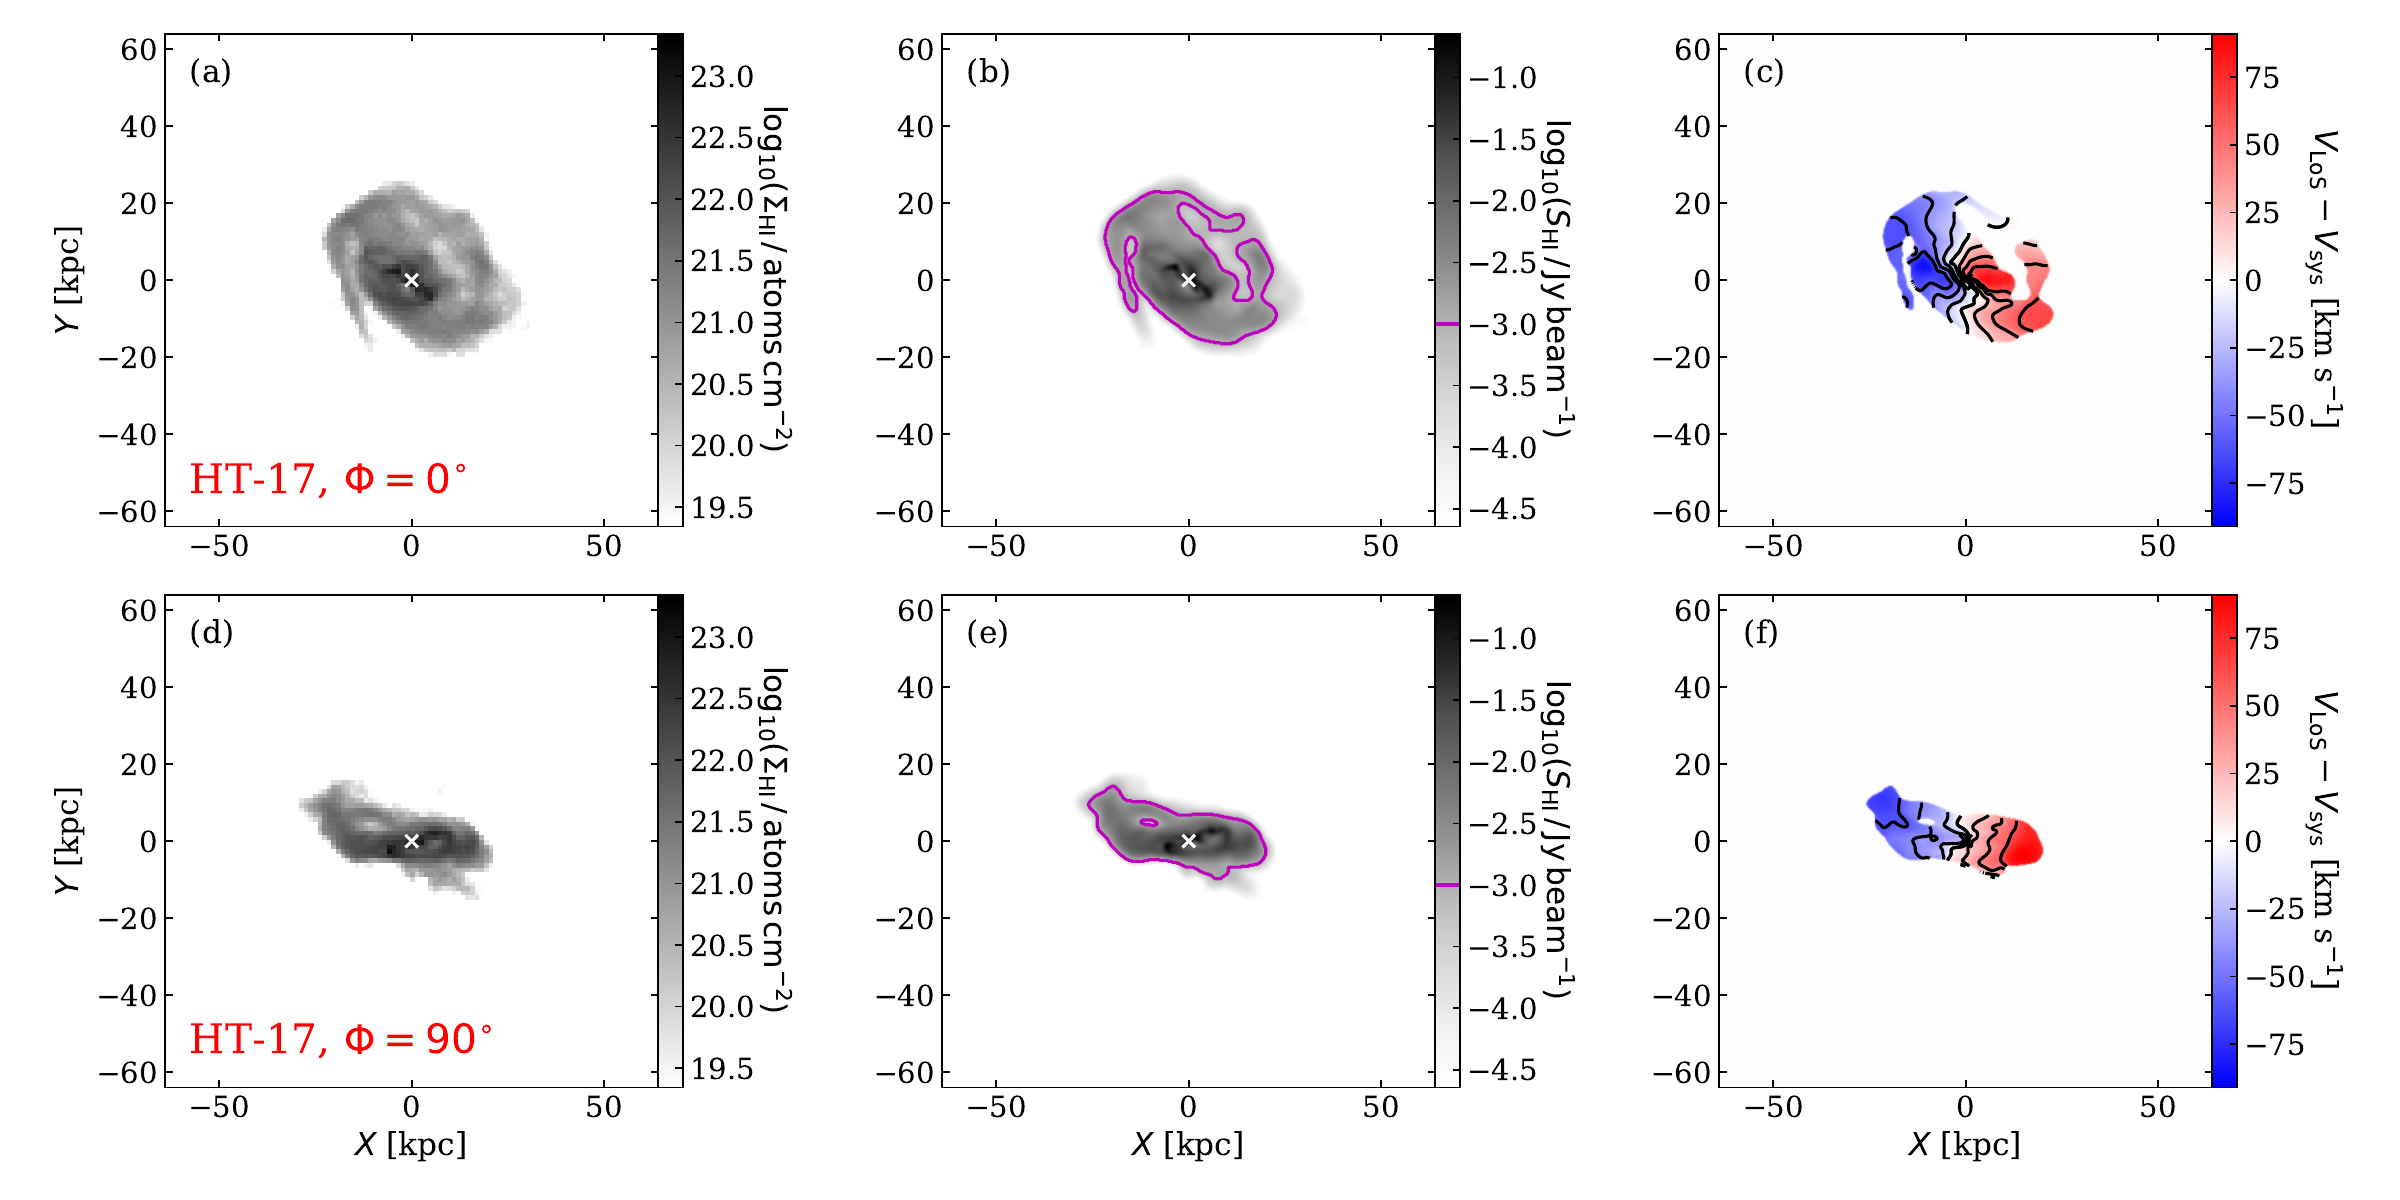}
\includegraphics[width=\textwidth]{../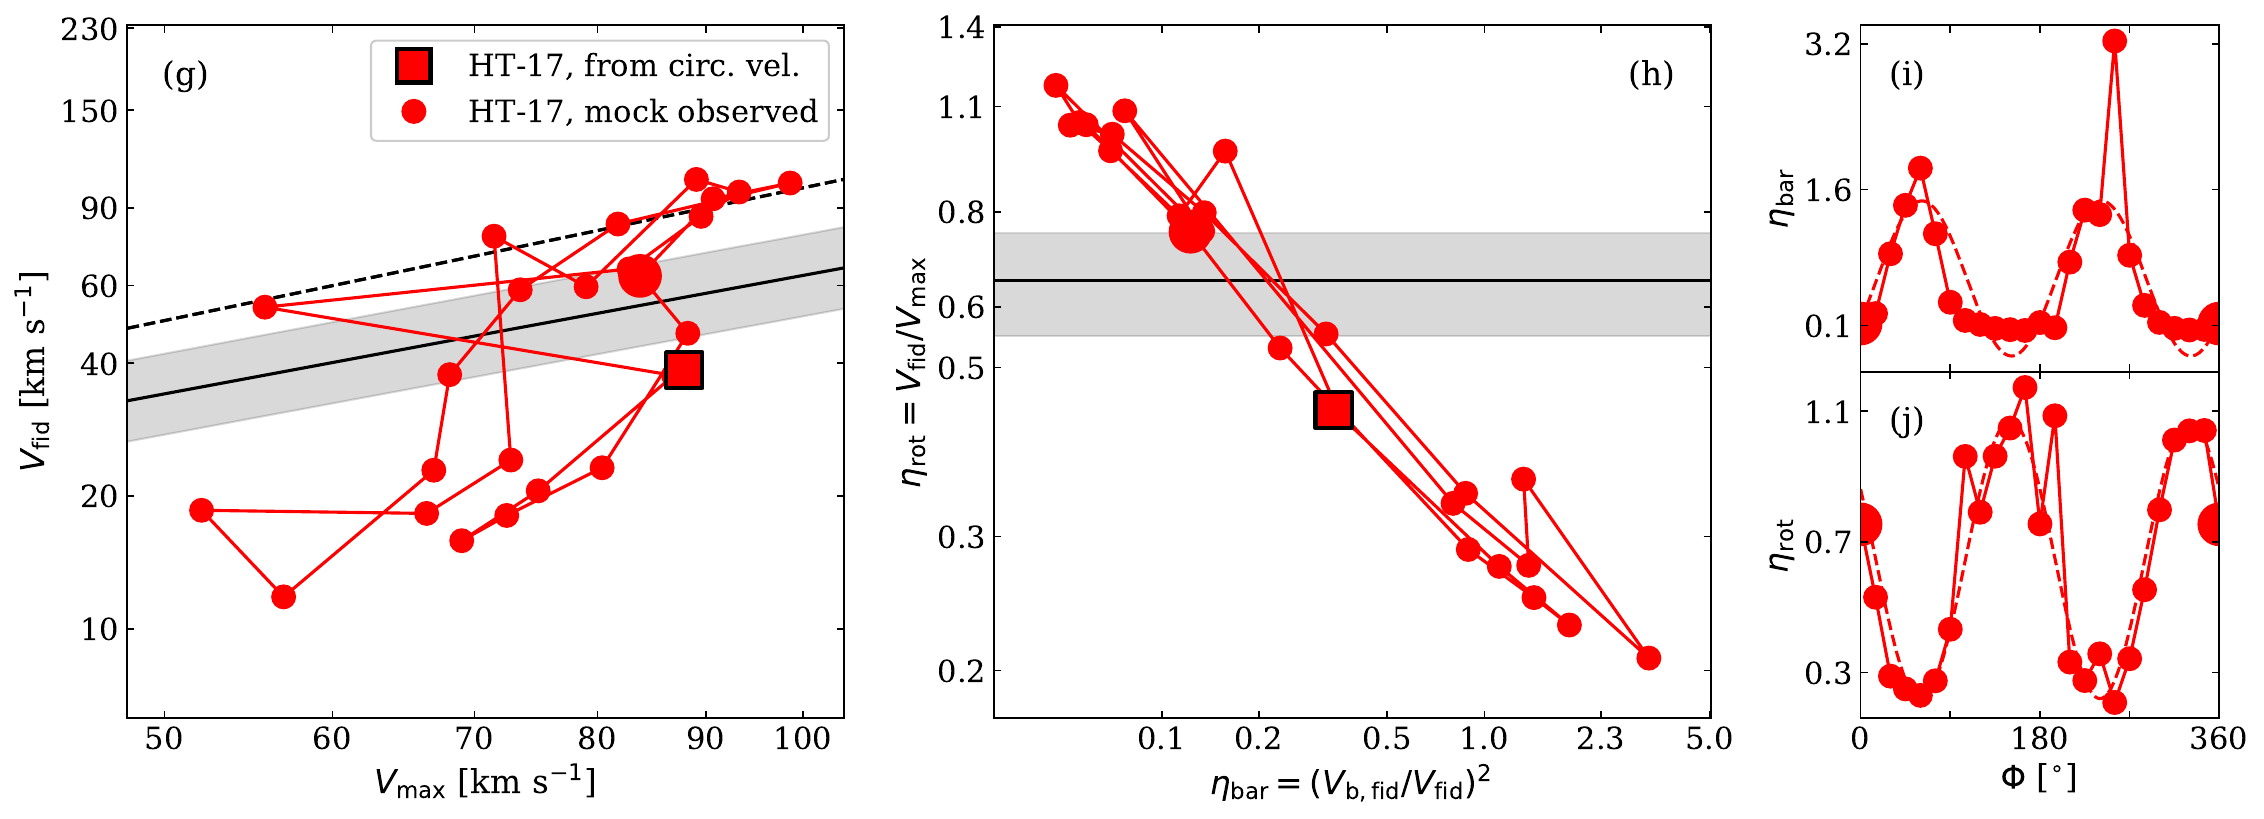}
\end{minipage}
\begin{minipage}{.4\textwidth}
\includegraphics[width=\textwidth]{../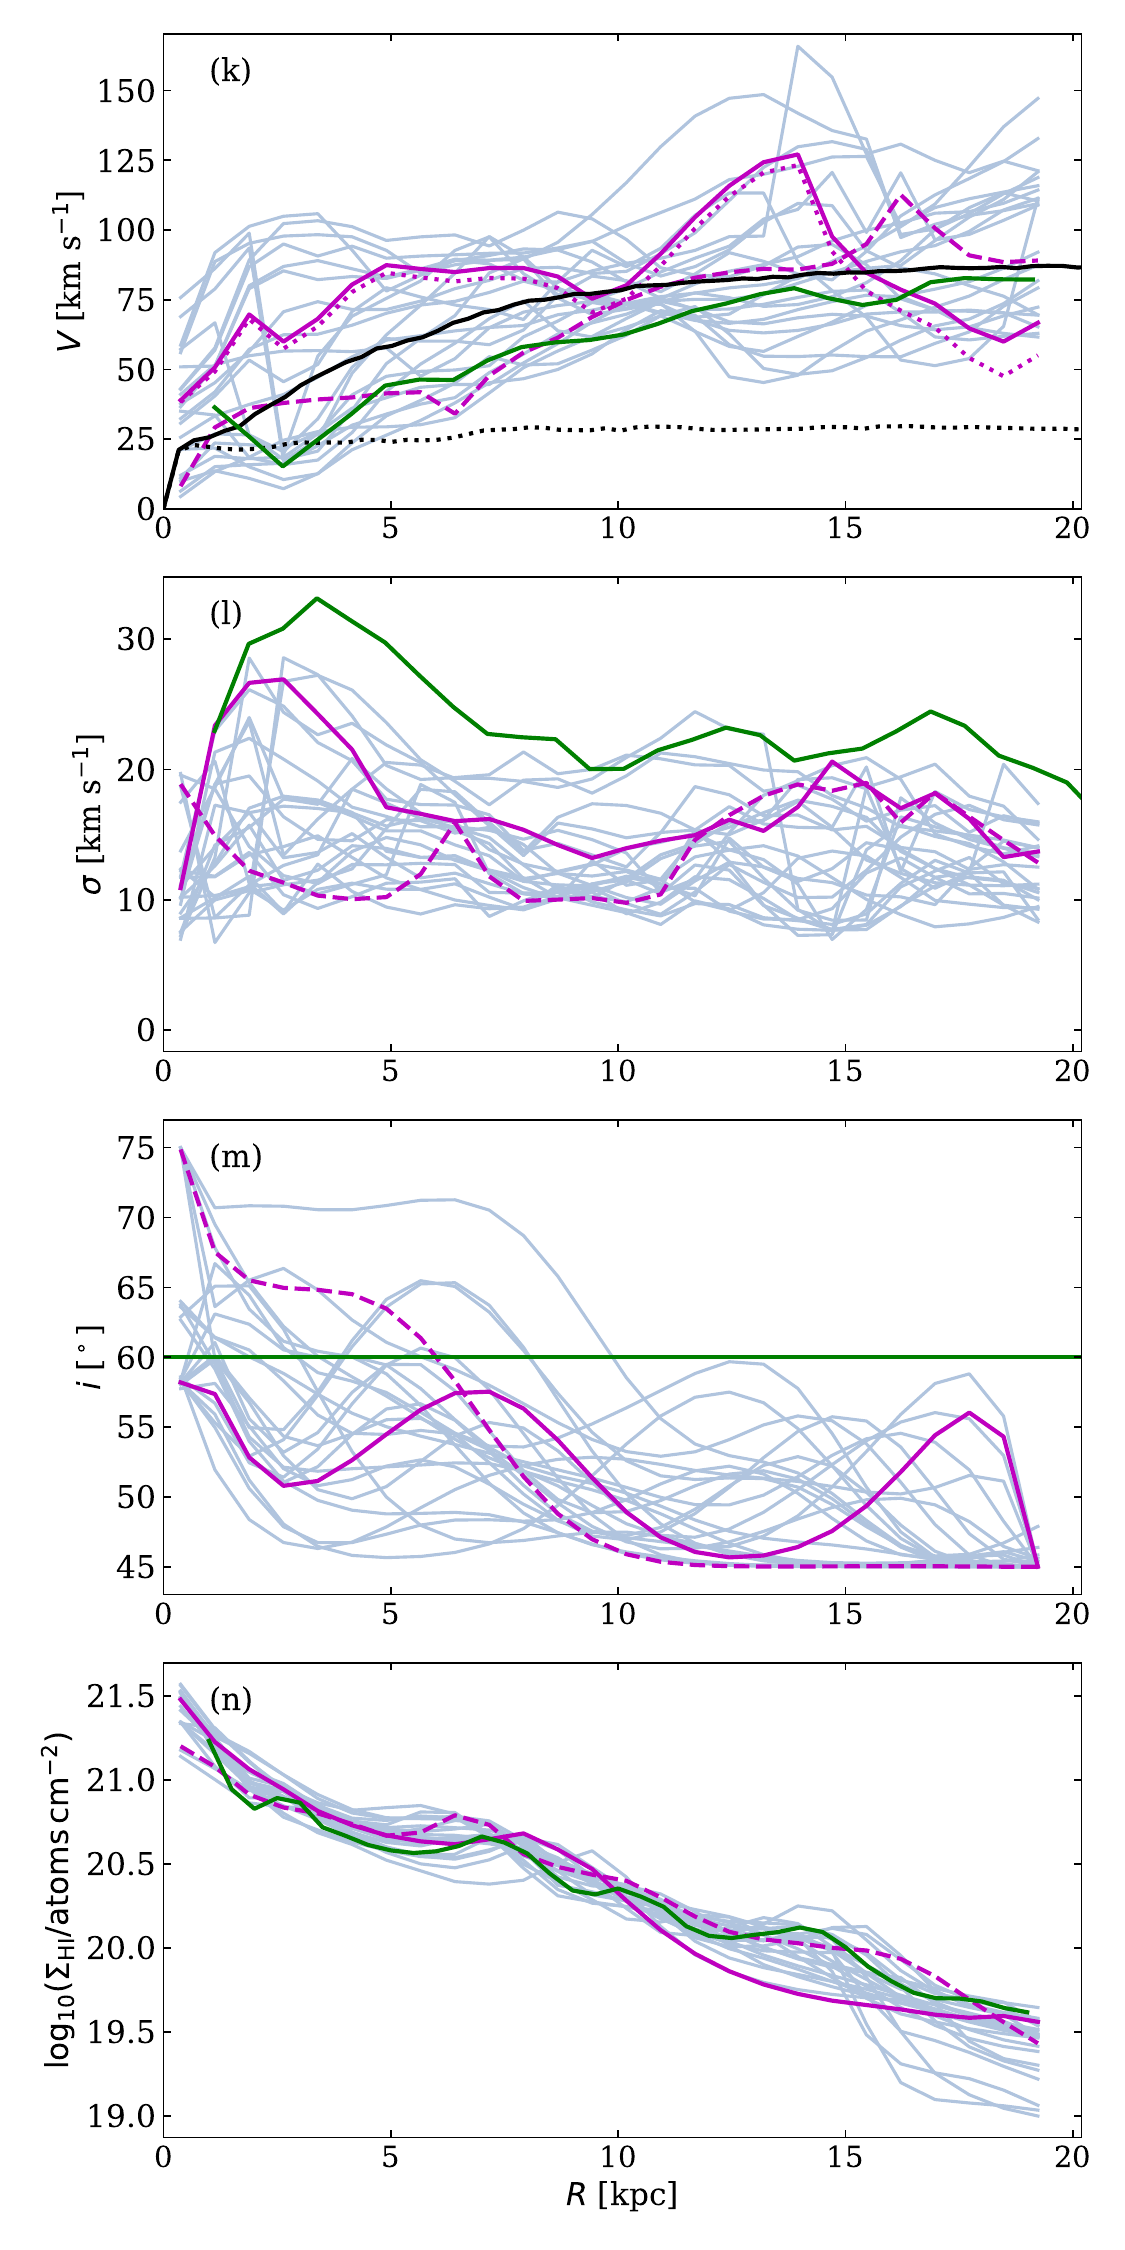}
\end{minipage}
\caption{A set of summary figures for galaxy HT-17, excluded from kinematic analysis. These include example moment maps for two orientations (panels (a)--(f); similar to Fig.~\ref{fig:visualisations}), a summary of the parameters $V_\mathrm{fid}$, $V_\mathrm{max}$, $\eta_\mathrm{rot}$, and $\eta_\mathrm{bar}$ (panels (g)--(j); similar to Fig.~\ref{fig:loops}), and a summary of the rotation curve analysis from $24$ viewing angles (panels (k)--(n); similar to Fig.~\ref{fig:rot_curves}). See description of Appendix~\ref{app:supplementary} for details.}
\label{fig:S64}
\end{figure}
\clearpage

\begin{figure}
\begin{minipage}{.9\textwidth}
\includegraphics[width=\textwidth]{../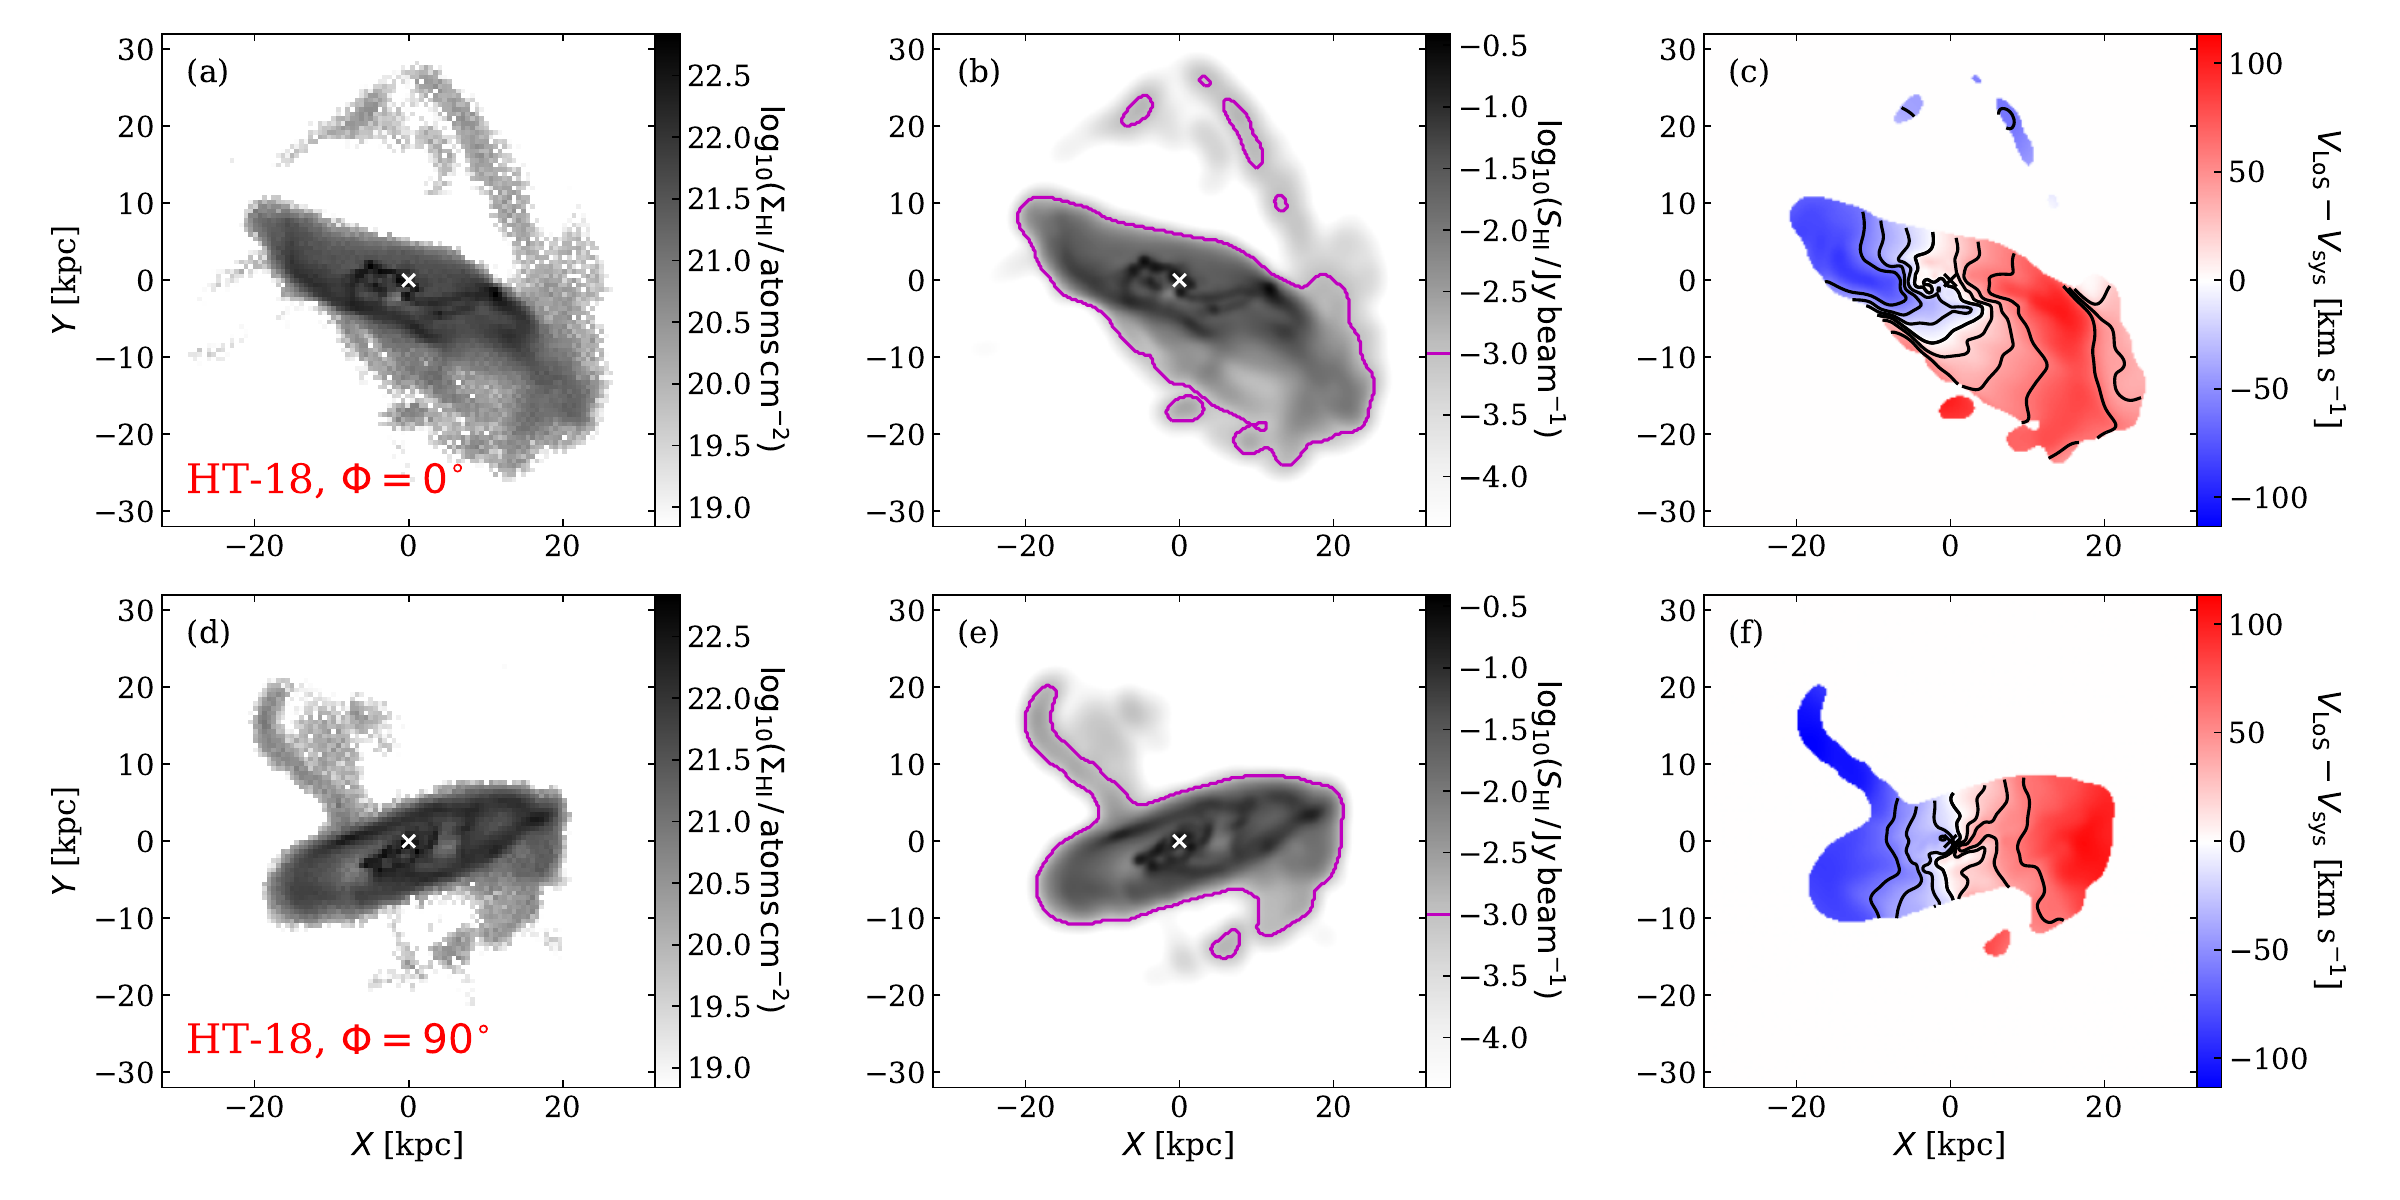}
\includegraphics[width=\textwidth]{../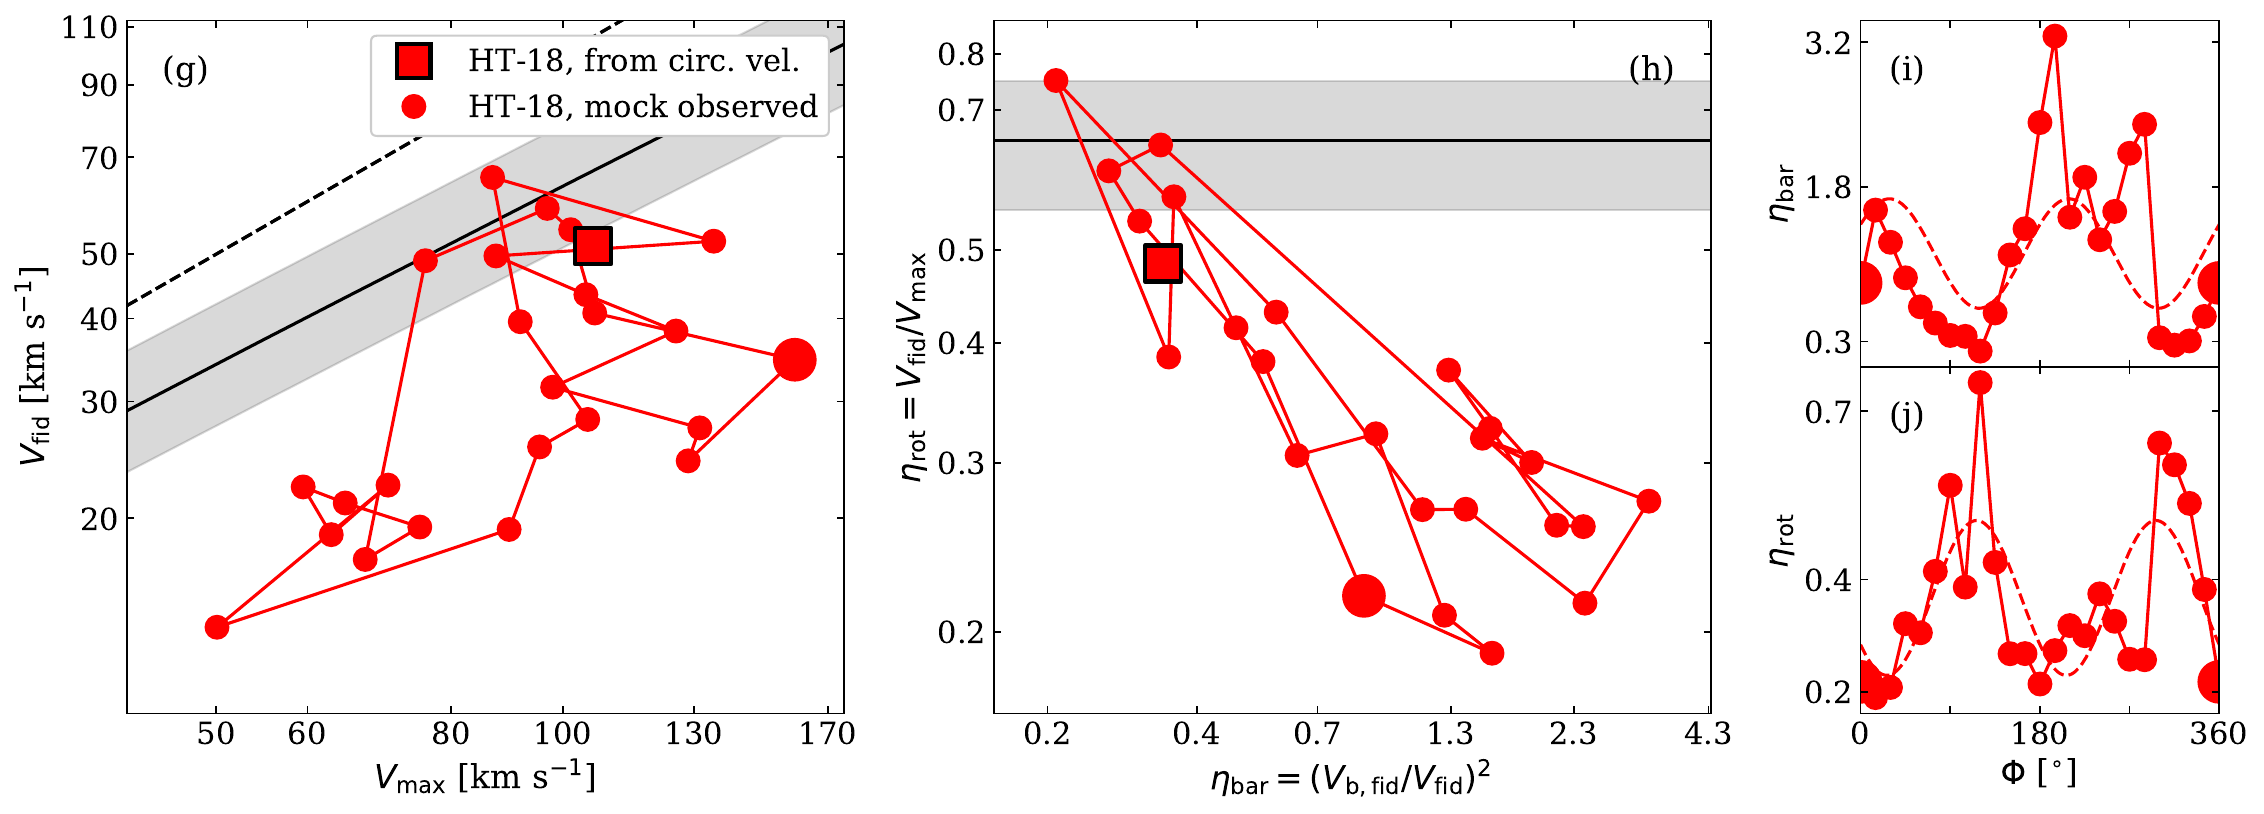}
\end{minipage}
\begin{minipage}{.4\textwidth}
\includegraphics[width=\textwidth]{../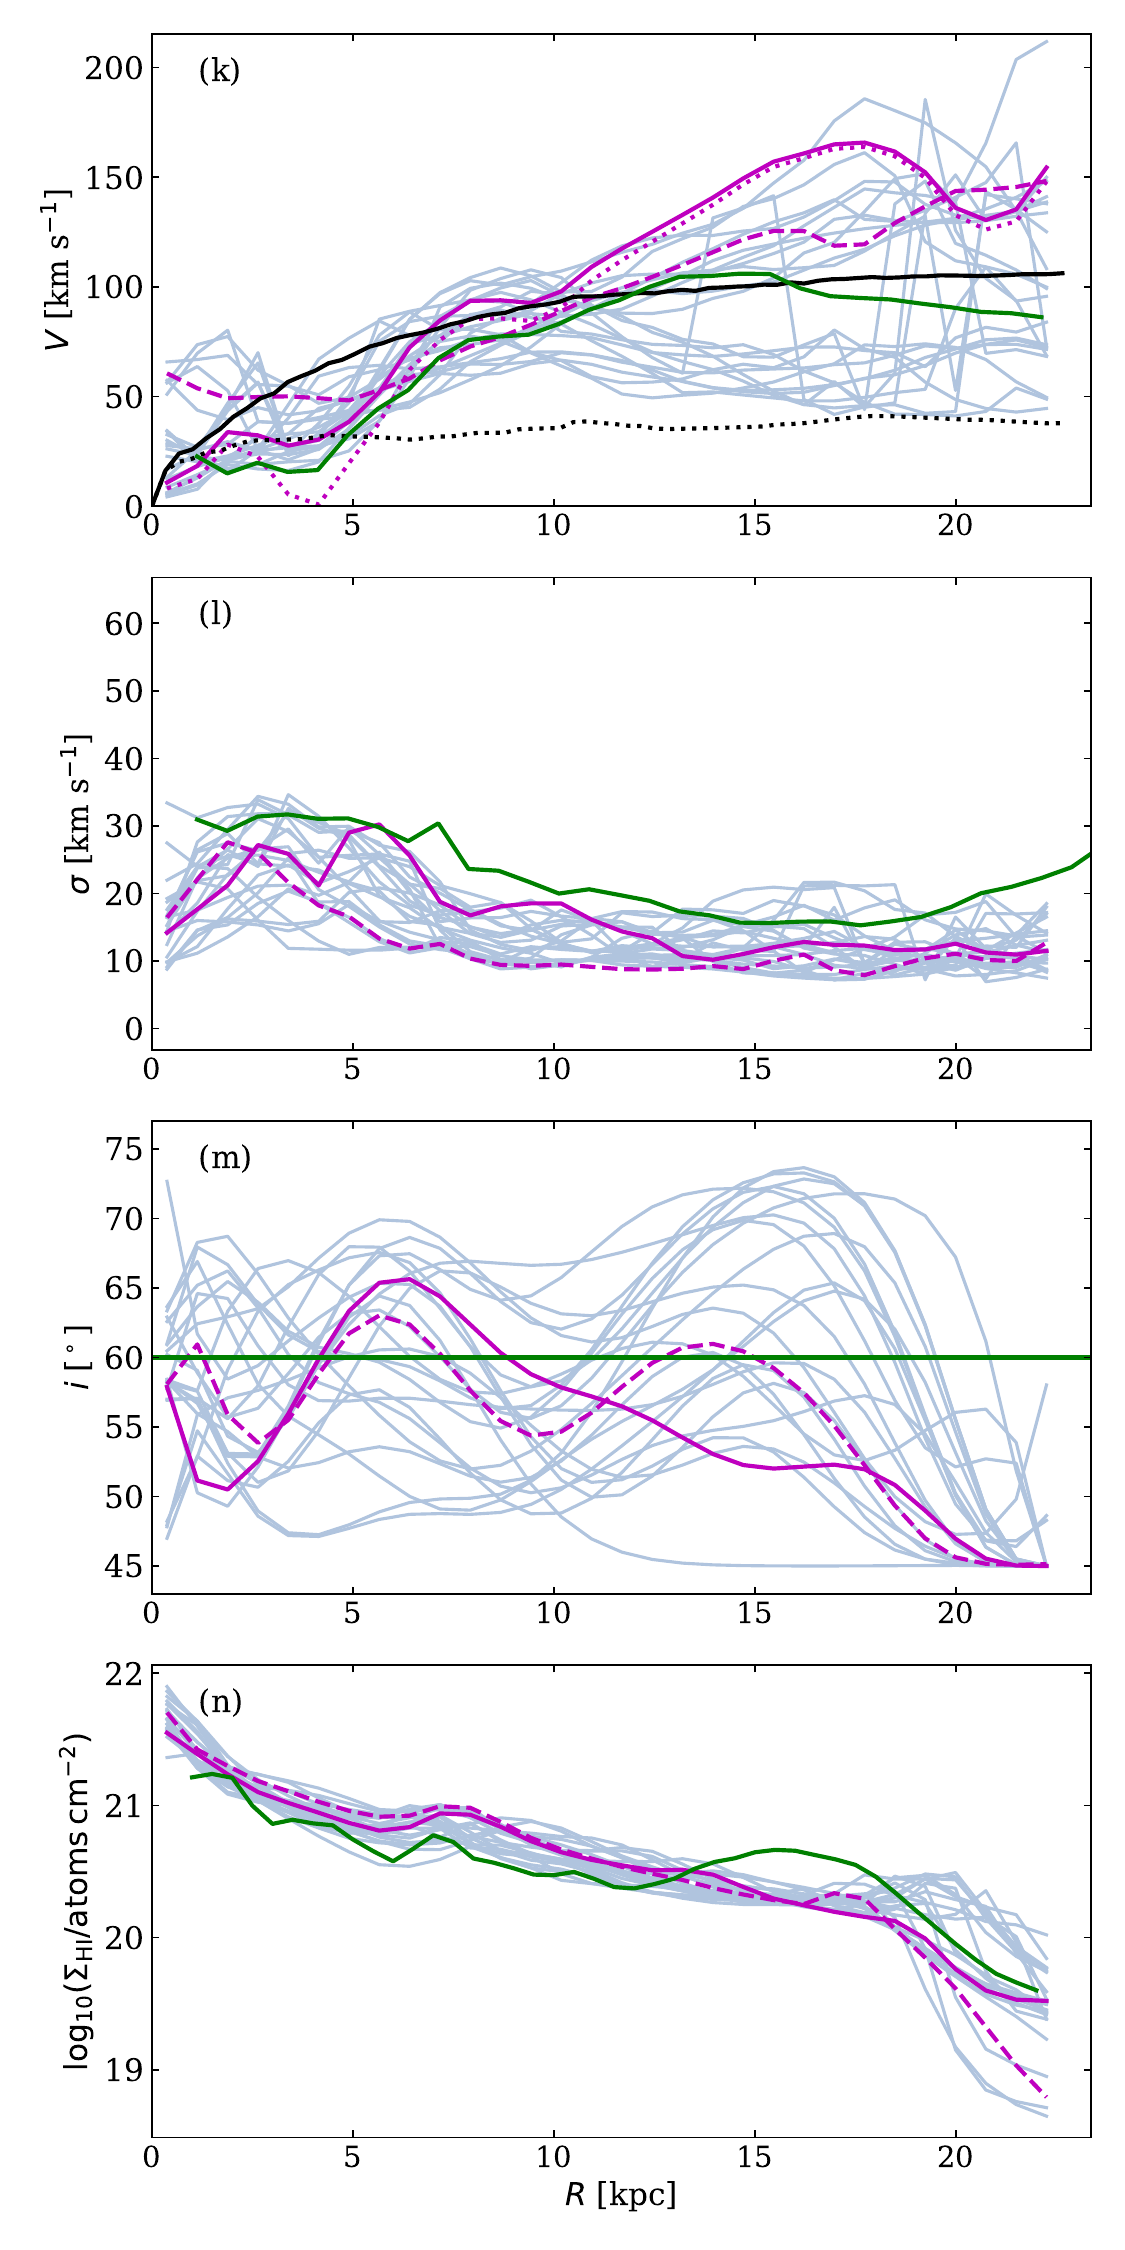}
\end{minipage}
\caption{A set of summary figures for galaxy HT-18, excluded from kinematic analysis. These include example moment maps for two orientations (panels (a)--(f); similar to Fig.~\ref{fig:visualisations}), a summary of the parameters $V_\mathrm{fid}$, $V_\mathrm{max}$, $\eta_\mathrm{rot}$, and $\eta_\mathrm{bar}$ (panels (g)--(j); similar to Fig.~\ref{fig:loops}), and a summary of the rotation curve analysis from $24$ viewing angles (panels (k)--(n); similar to Fig.~\ref{fig:rot_curves}). See description of Appendix~\ref{app:supplementary} for details.}
\label{fig:S65}
\end{figure}
\clearpage

\begin{figure}
\begin{minipage}{.9\textwidth}
\includegraphics[width=\textwidth]{../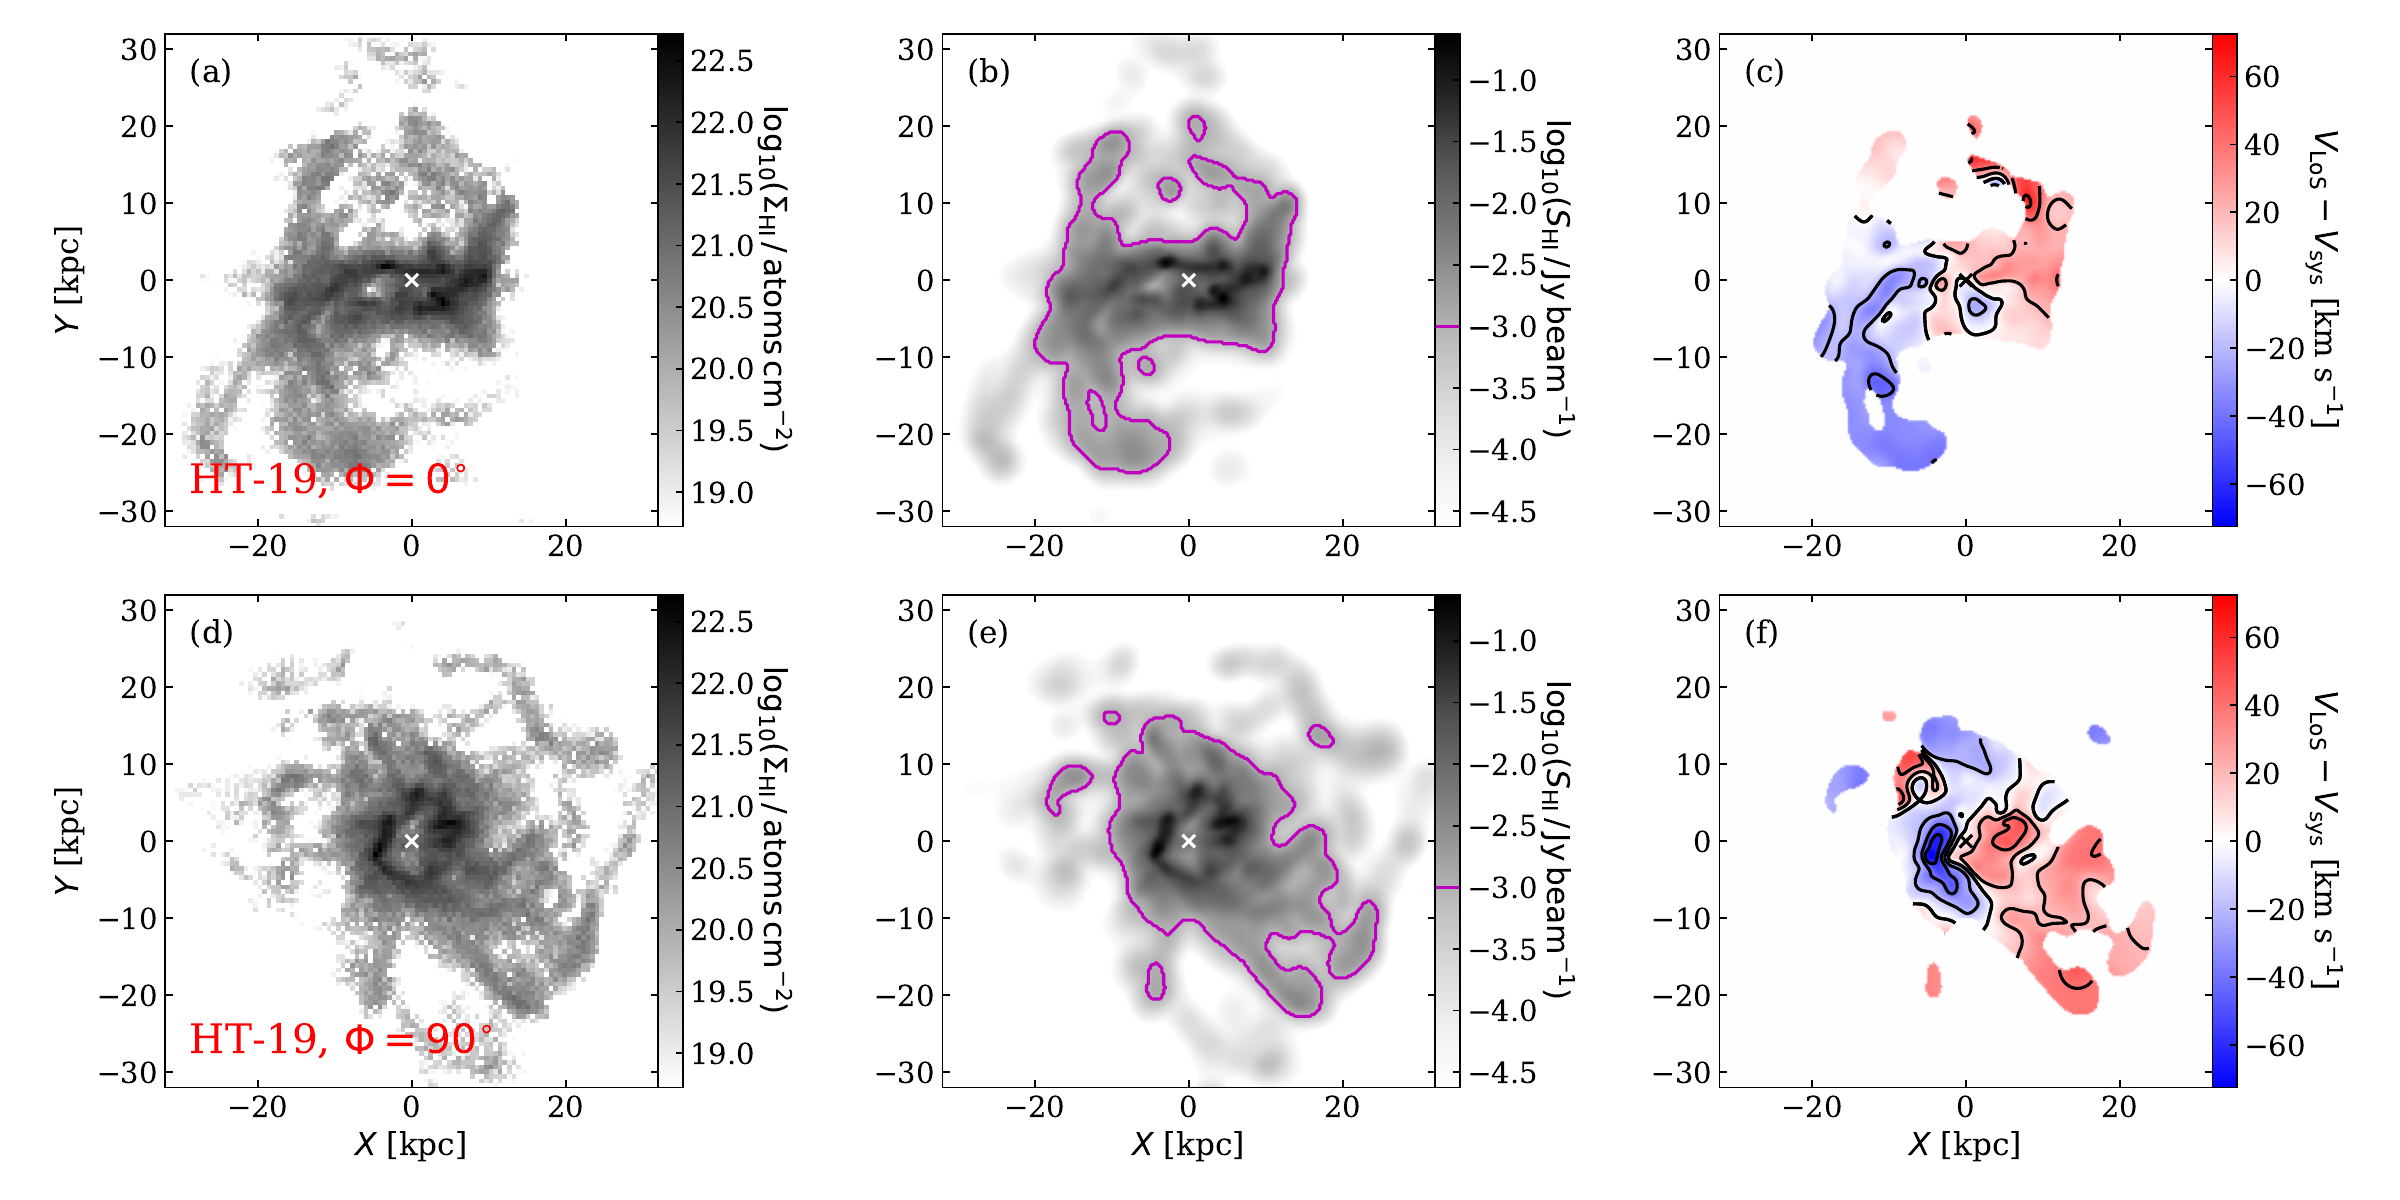}
\includegraphics[width=\textwidth]{../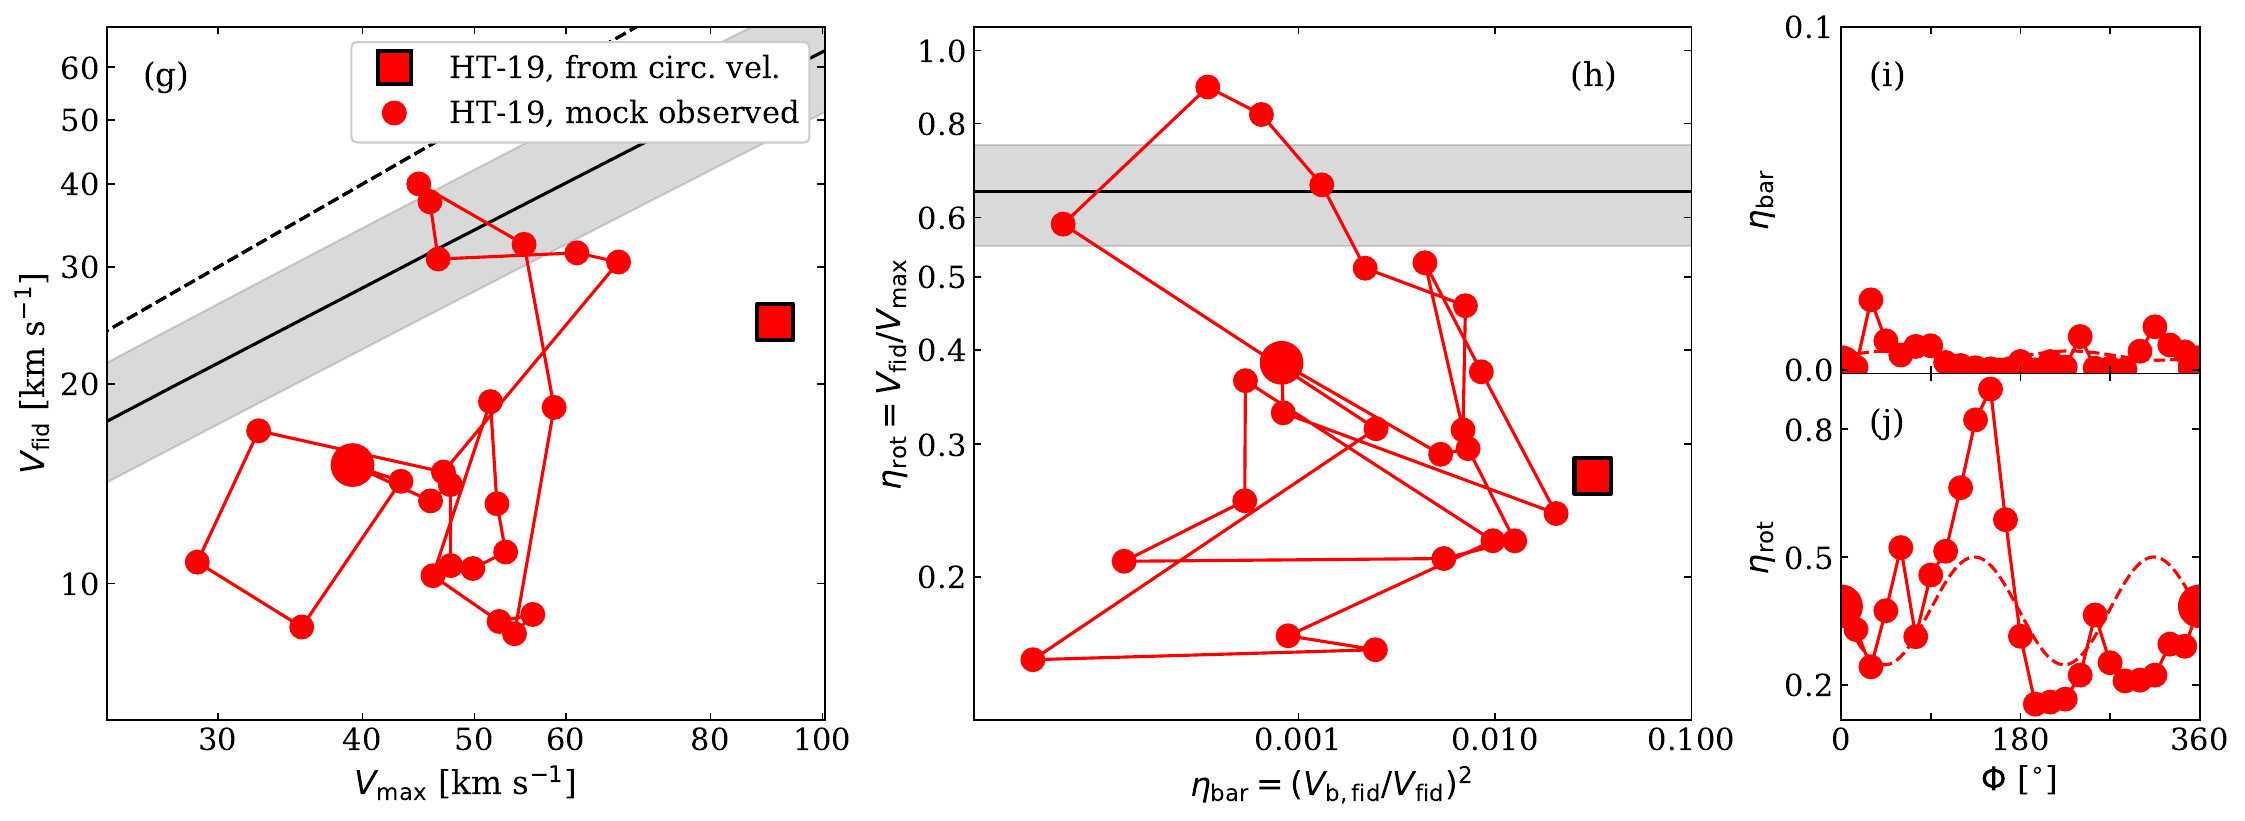}
\end{minipage}
\begin{minipage}{.4\textwidth}
\includegraphics[width=\textwidth]{../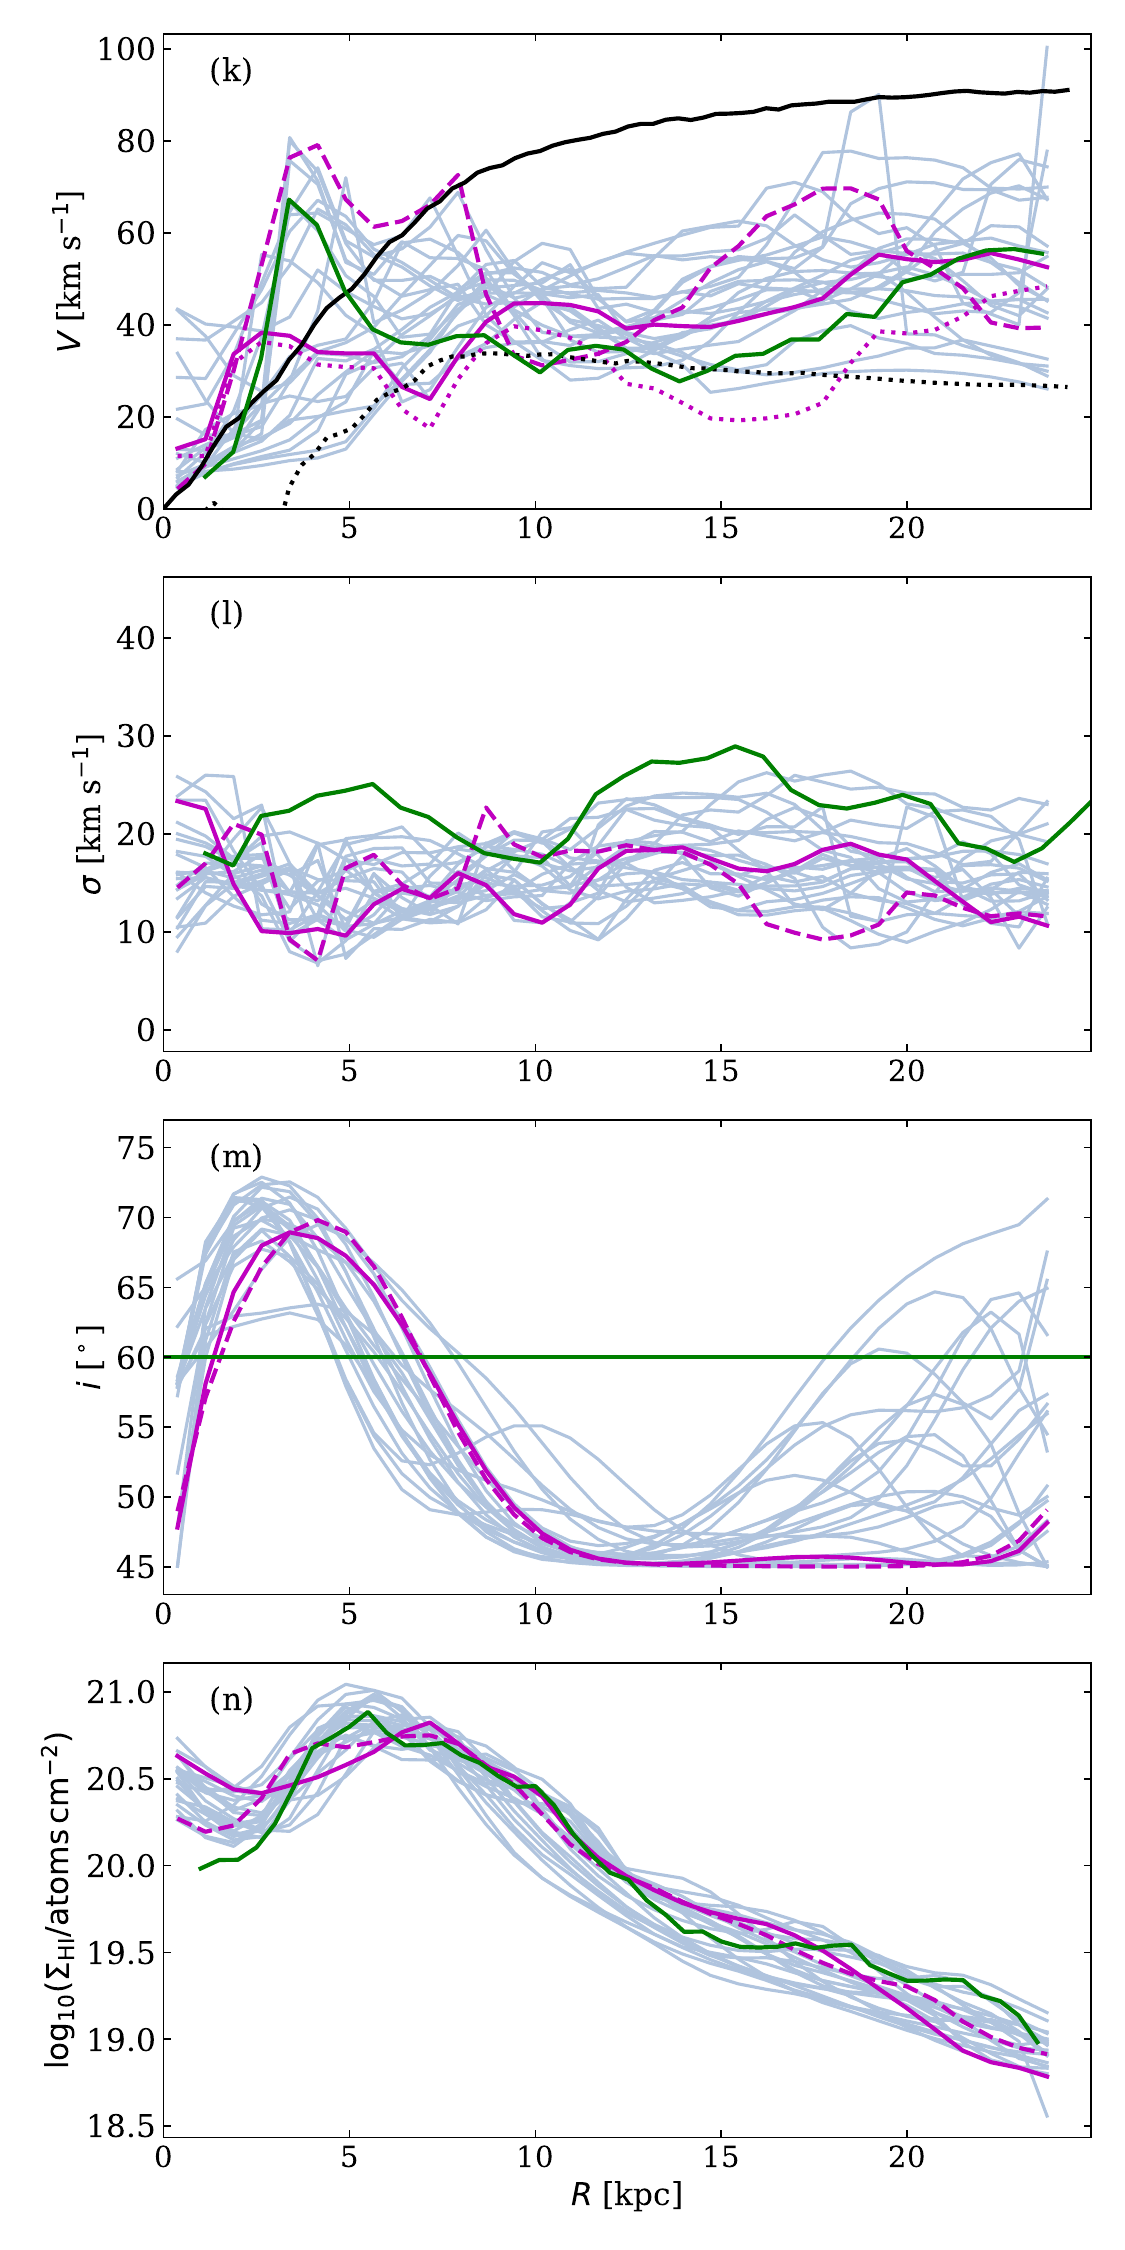}
\end{minipage}
\caption{A set of summary figures for galaxy HT-19, excluded from kinematic analysis. These include example moment maps for two orientations (panels (a)--(f); similar to Fig.~\ref{fig:visualisations}), a summary of the parameters $V_\mathrm{fid}$, $V_\mathrm{max}$, $\eta_\mathrm{rot}$, and $\eta_\mathrm{bar}$ (panels (g)--(j); similar to Fig.~\ref{fig:loops}), and a summary of the rotation curve analysis from $24$ viewing angles (panels (k)--(n); similar to Fig.~\ref{fig:rot_curves}). See description of Appendix~\ref{app:supplementary} for details.}
\label{fig:S66}
\end{figure}
\clearpage

\begin{figure}
\begin{minipage}{.9\textwidth}
\includegraphics[width=\textwidth]{../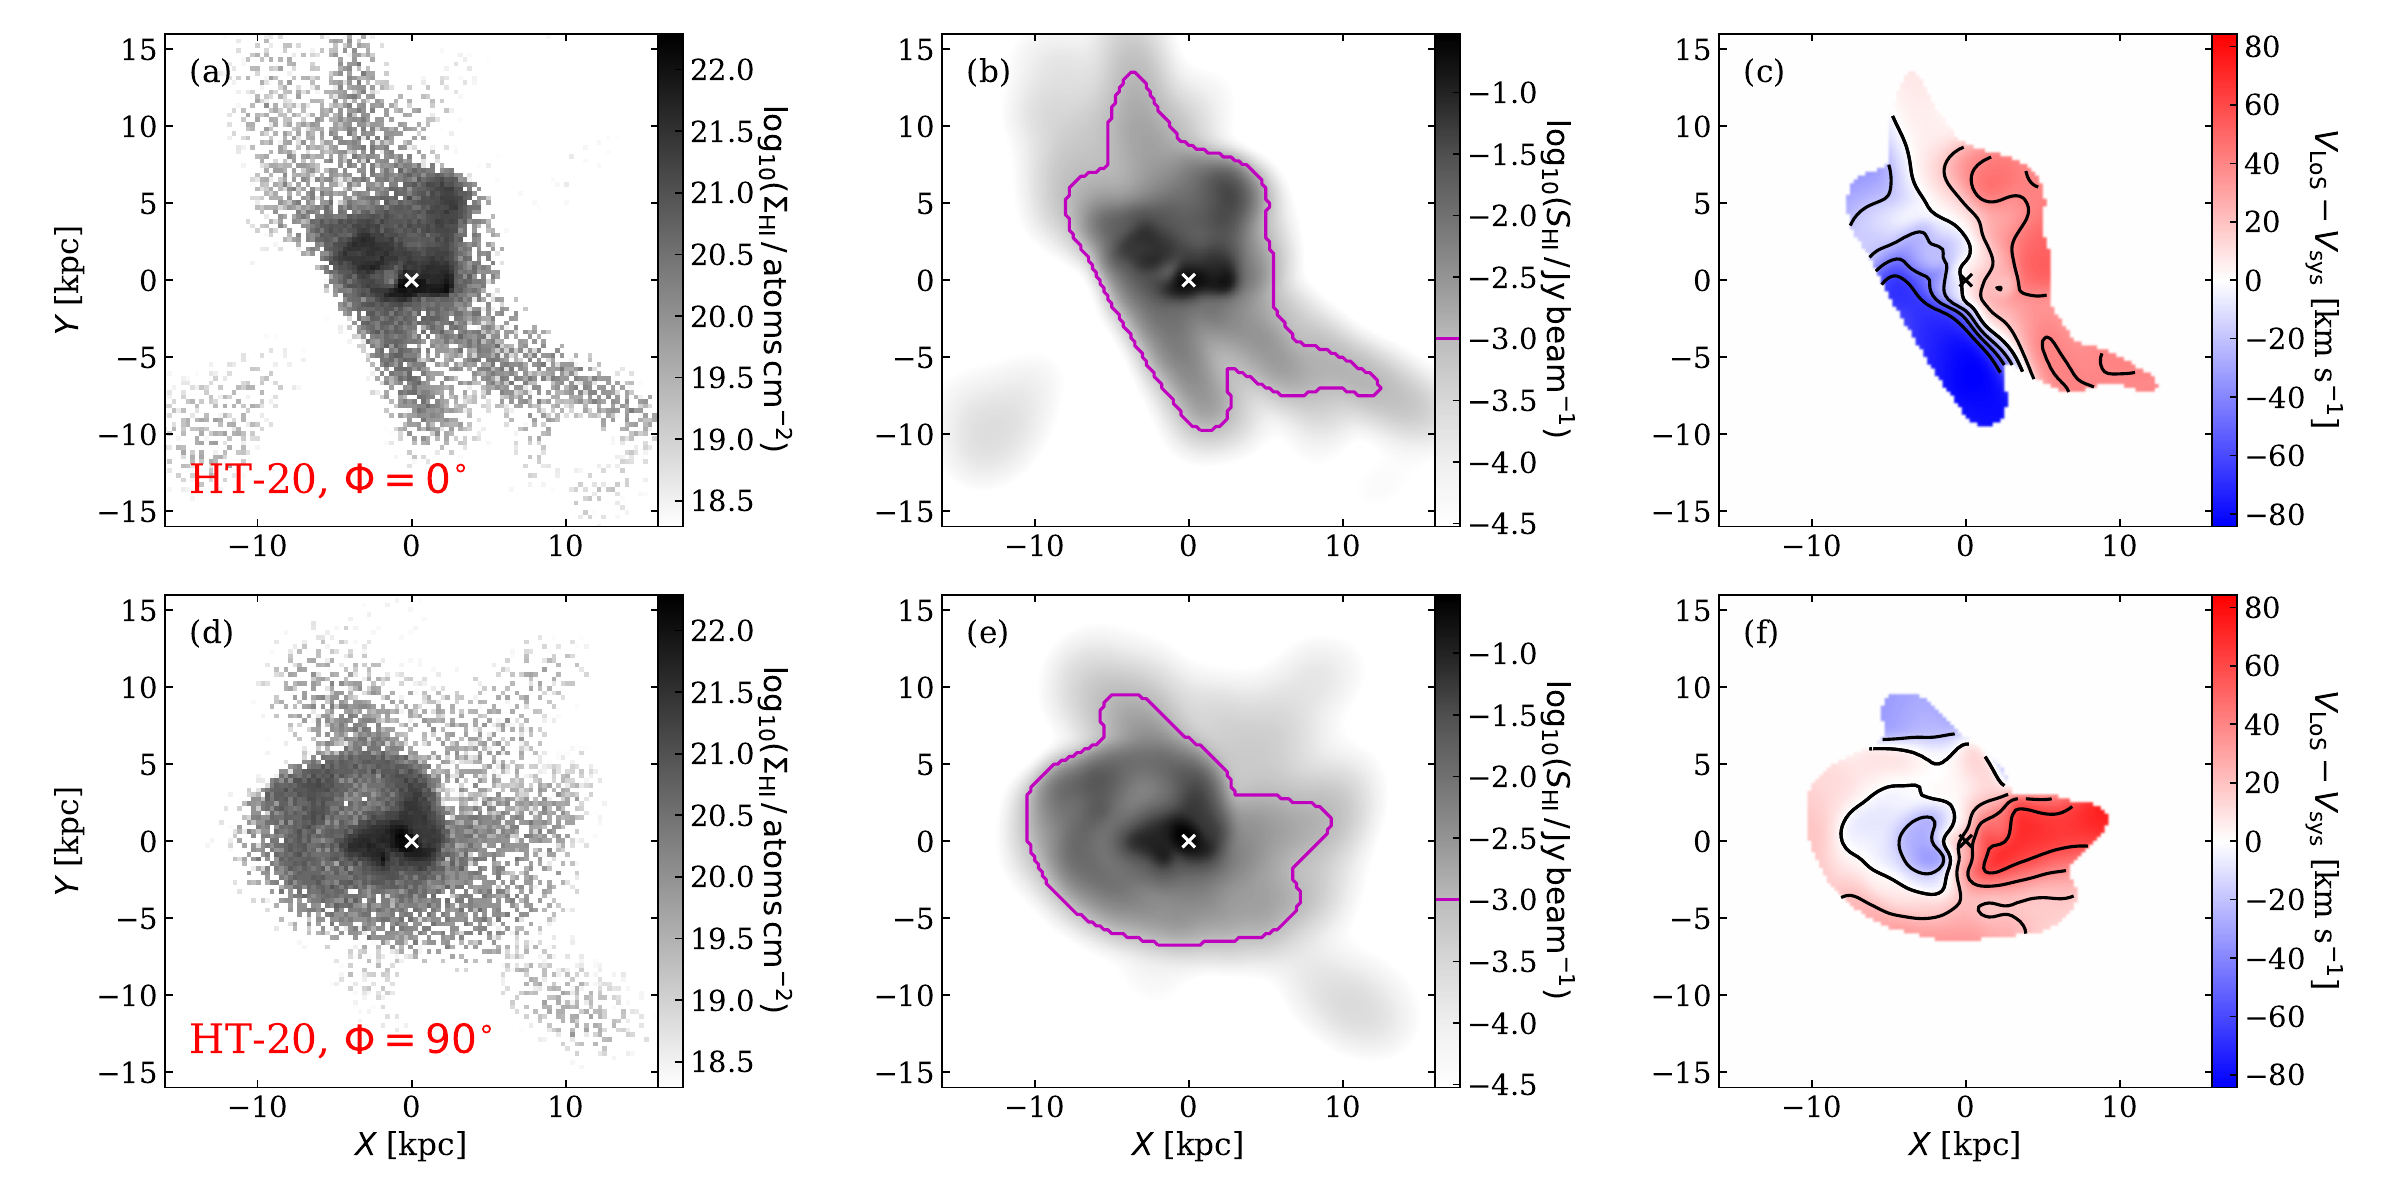}
\includegraphics[width=\textwidth]{../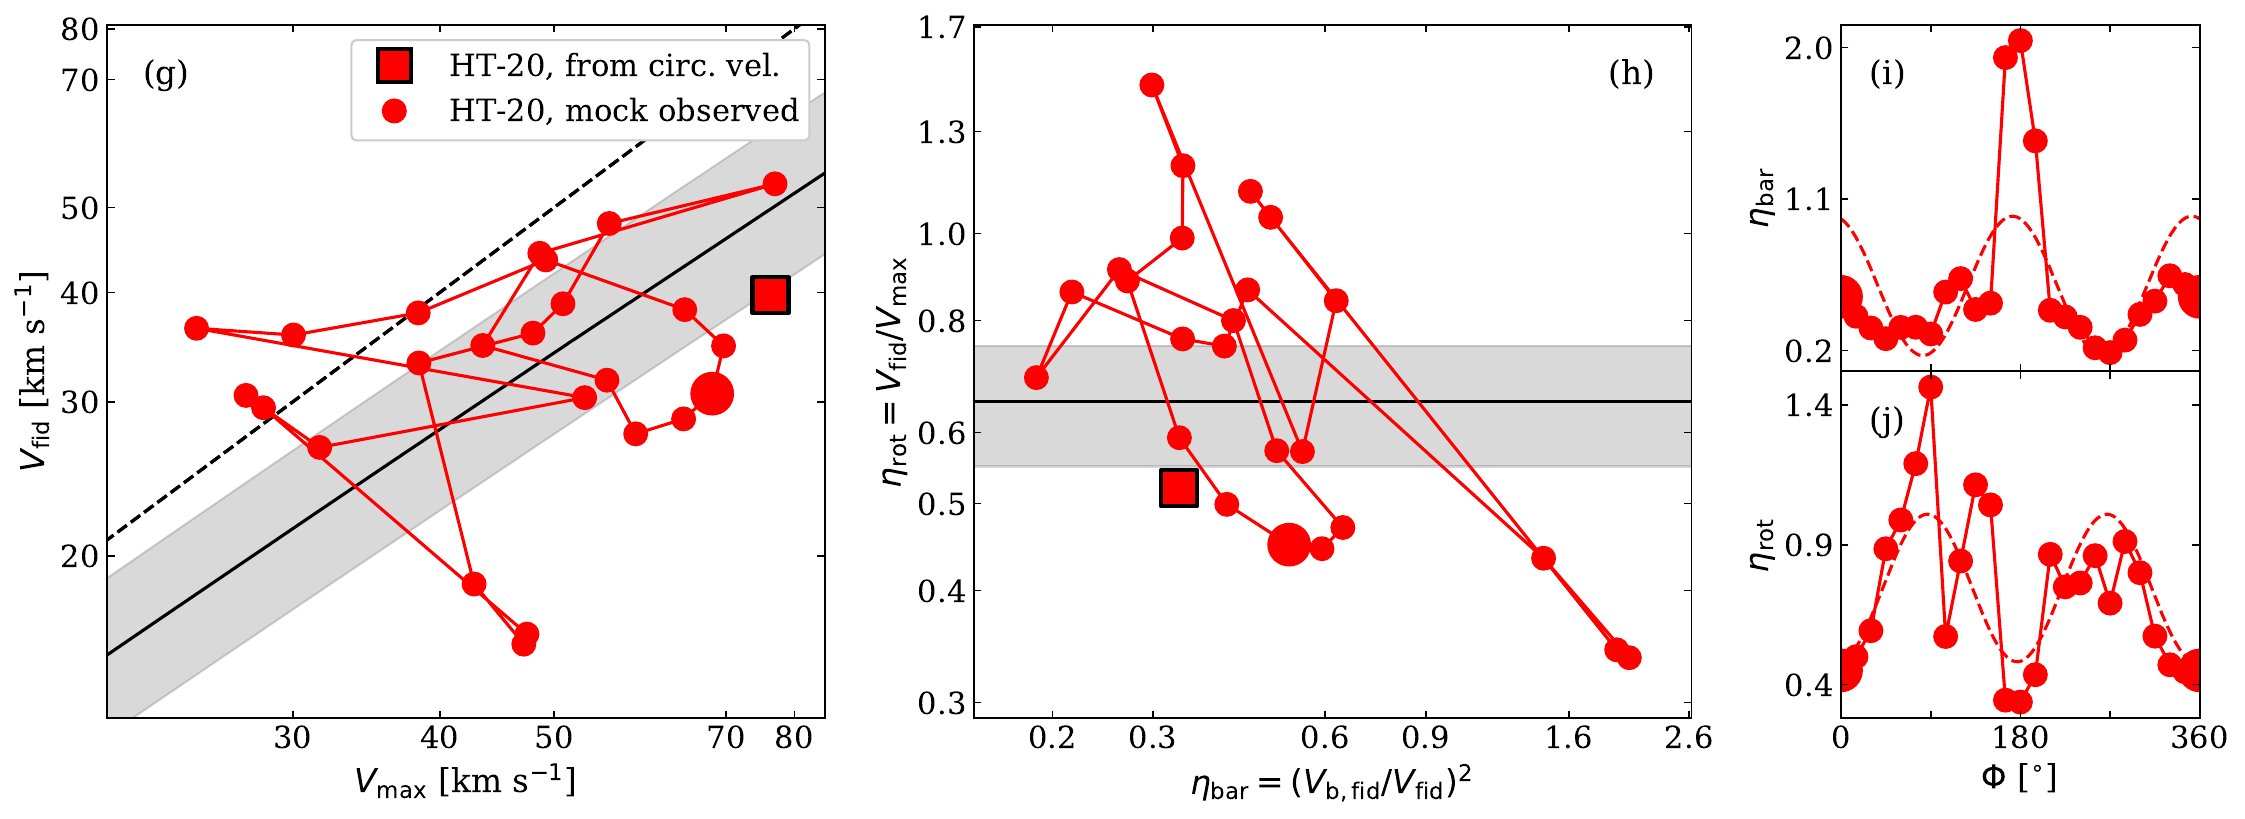}
\end{minipage}
\begin{minipage}{.4\textwidth}
\includegraphics[width=\textwidth]{../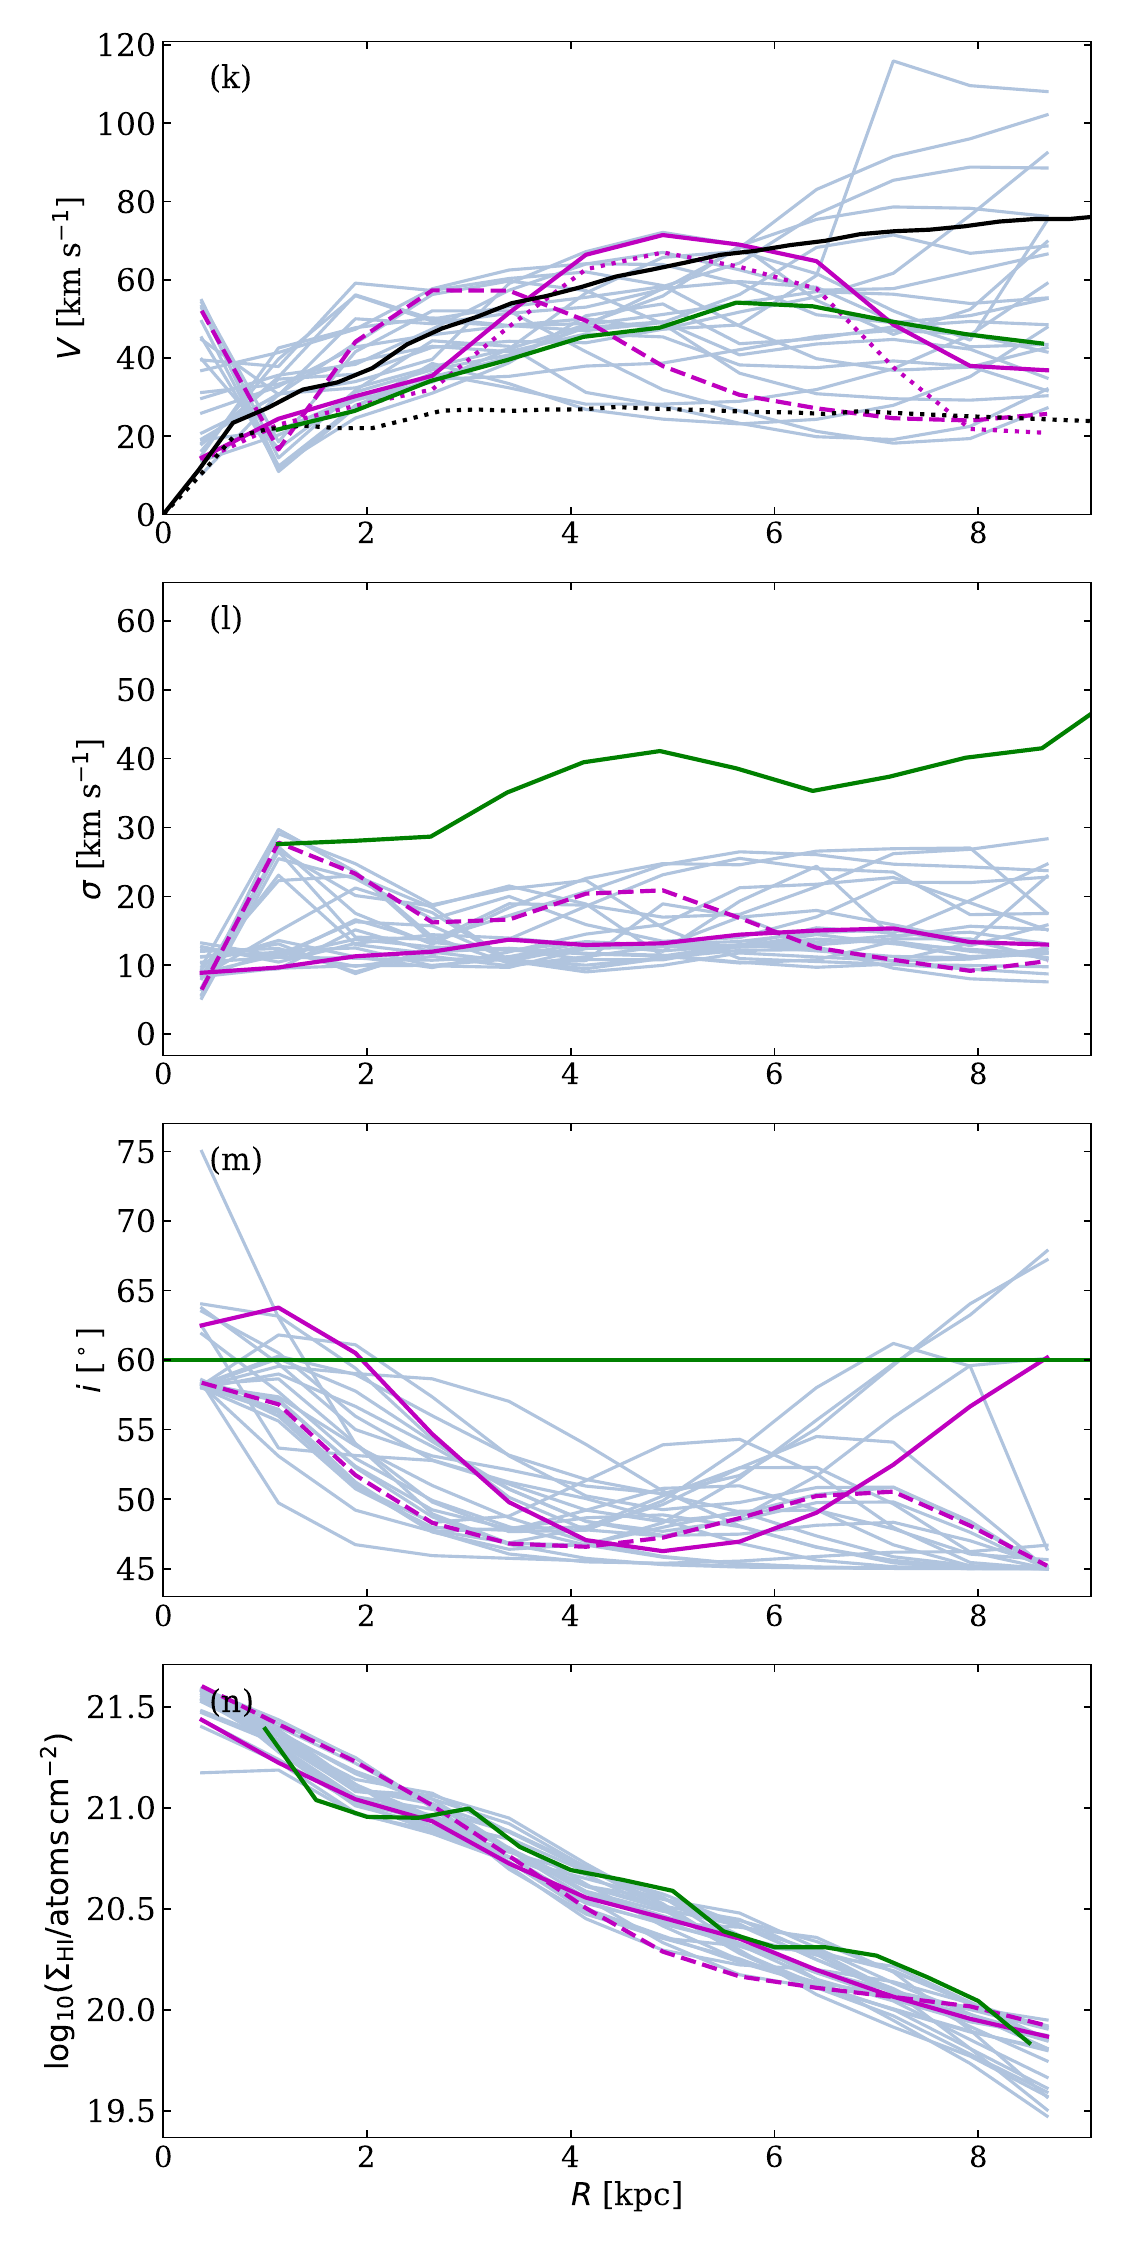}
\end{minipage}
\caption{A set of summary figures for galaxy HT-20, excluded from kinematic analysis. These include example moment maps for two orientations (panels (a)--(f); similar to Fig.~\ref{fig:visualisations}), a summary of the parameters $V_\mathrm{fid}$, $V_\mathrm{max}$, $\eta_\mathrm{rot}$, and $\eta_\mathrm{bar}$ (panels (g)--(j); similar to Fig.~\ref{fig:loops}), and a summary of the rotation curve analysis from $24$ viewing angles (panels (k)--(n); similar to Fig.~\ref{fig:rot_curves}). See description of Appendix~\ref{app:supplementary} for details.}
\label{fig:S67}
\end{figure}
\clearpage

\begin{figure}
\begin{minipage}{.9\textwidth}
\includegraphics[width=\textwidth]{../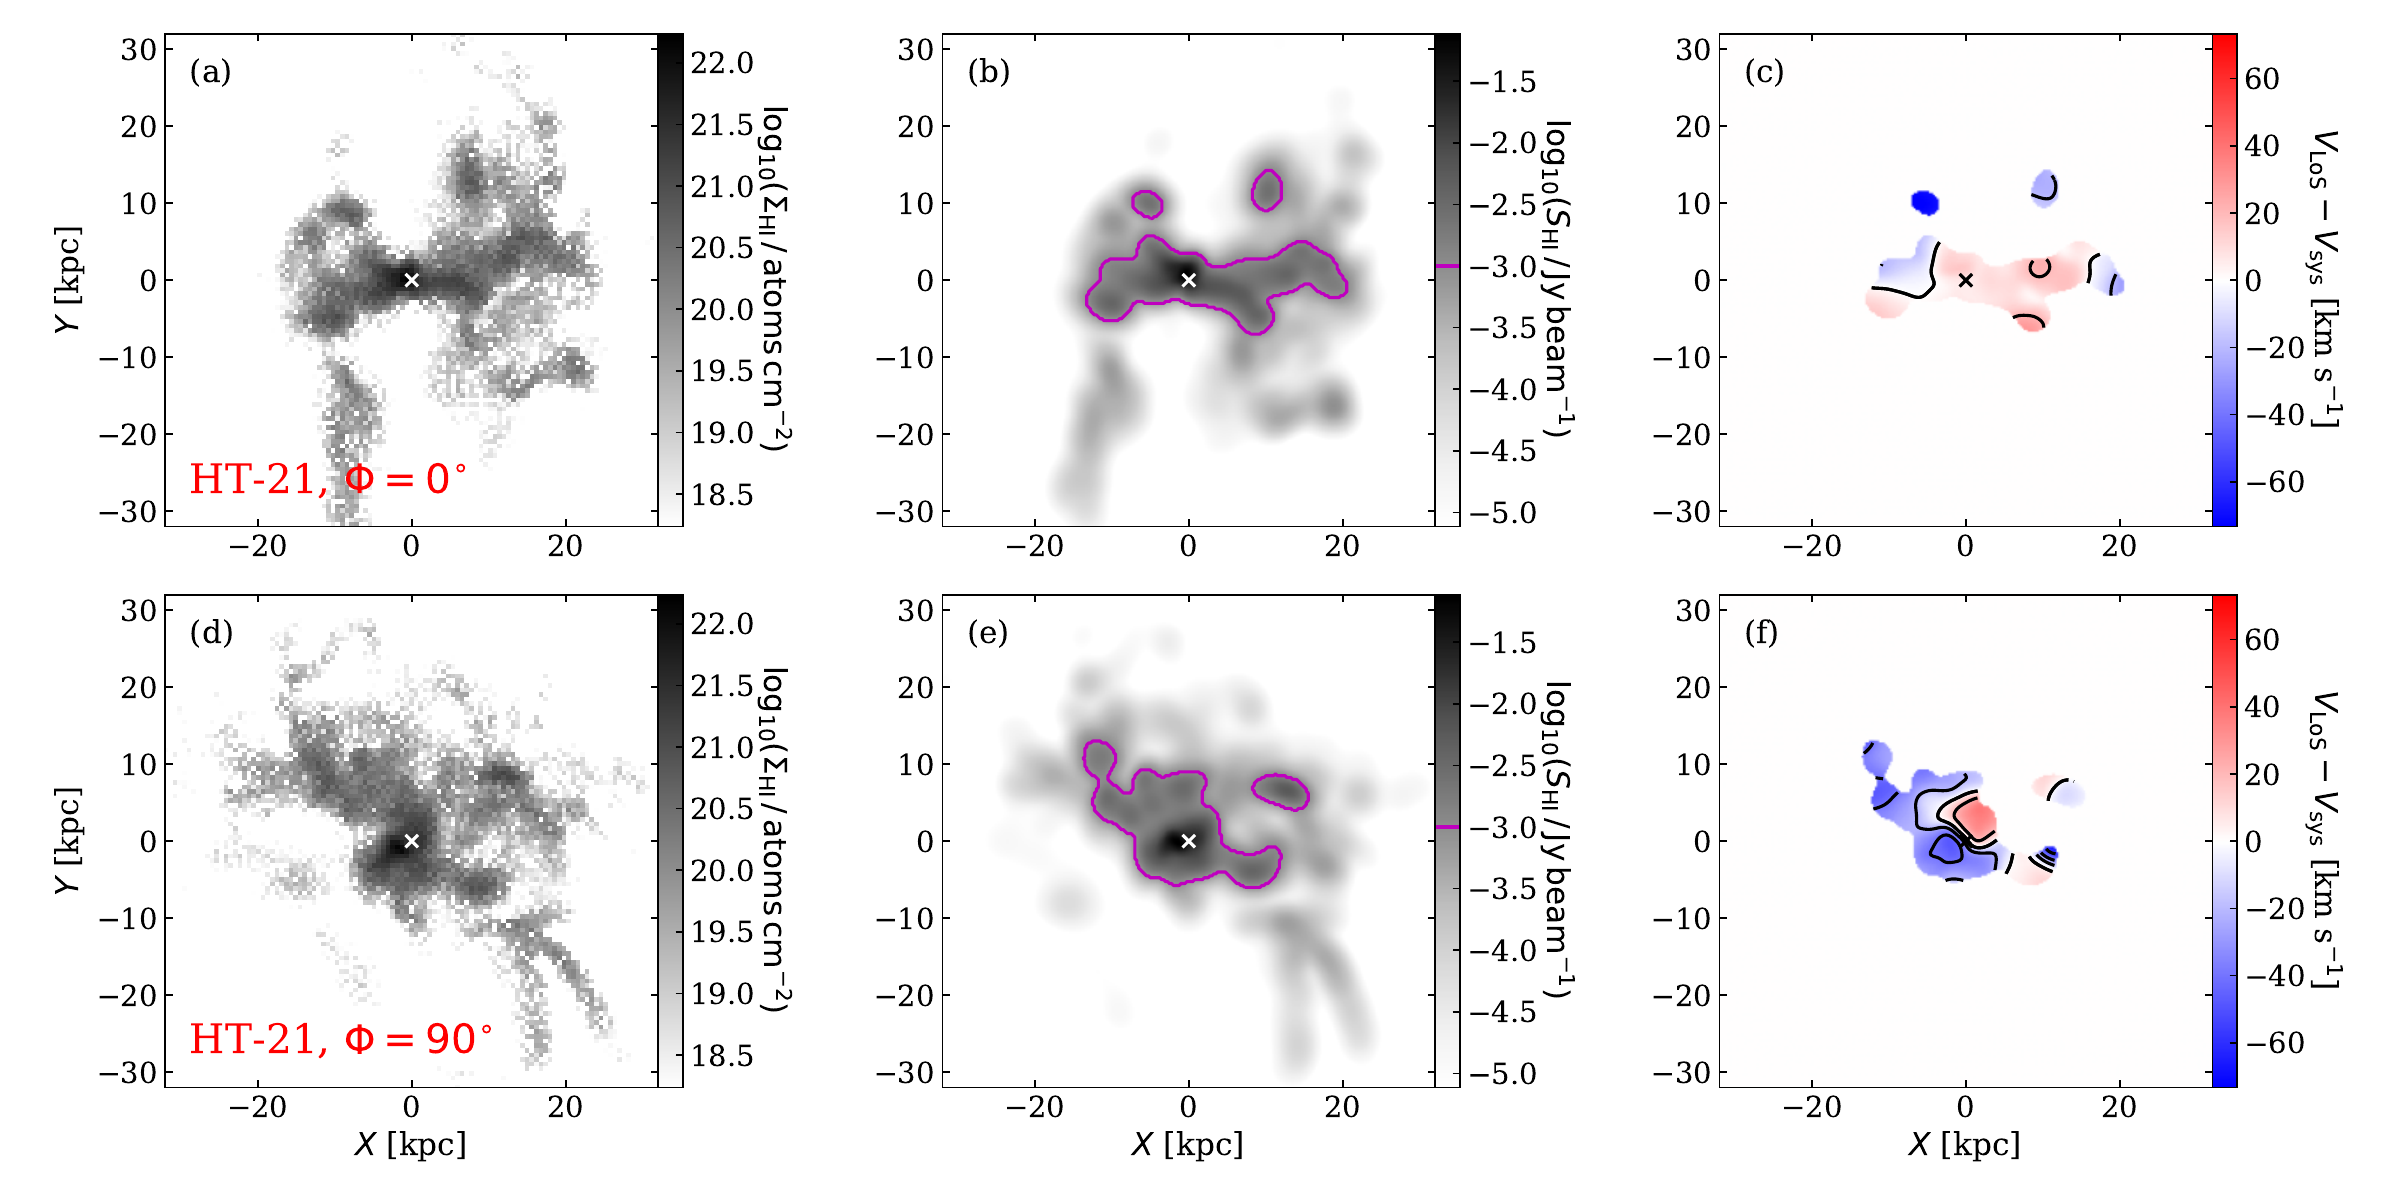}
\end{minipage}
\begin{minipage}{.4\textwidth}
\includegraphics[width=\textwidth]{../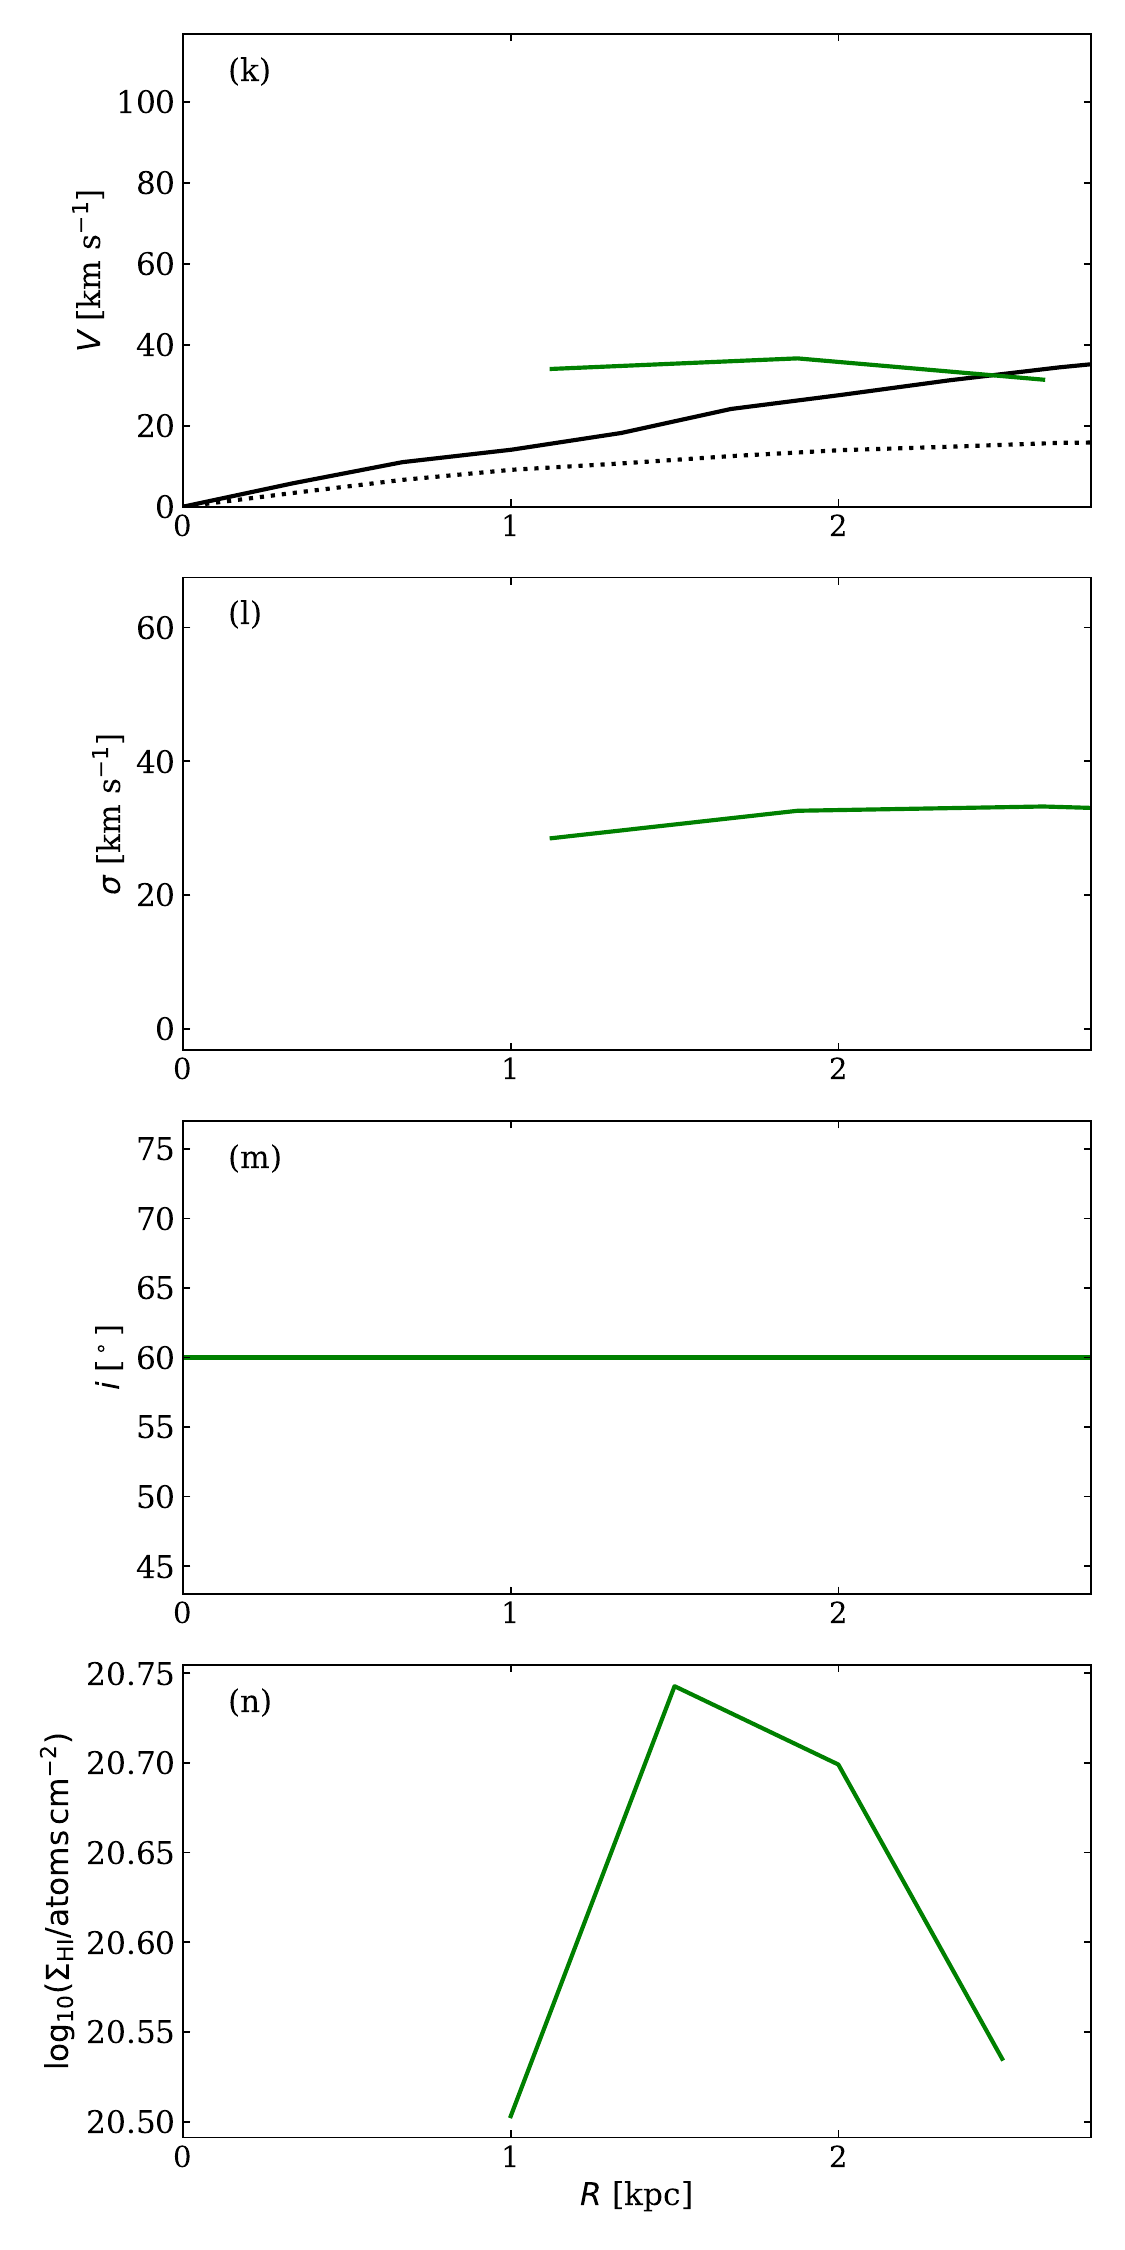}
\end{minipage}
\caption{A set of summary figures for galaxy HT-21, excluded from kinematic analysis. These include example moment maps for two orientations (panels (a)--(f); similar to Fig.~\ref{fig:visualisations}) and a summary of the rotation curve analysis from $24$ viewing angles (panels (k)--(n); similar to Fig.~\ref{fig:rot_curves}). See description of Appendix~\ref{app:supplementary} for details.}
\label{fig:S68}
\end{figure}
\clearpage

\begin{figure}
\begin{minipage}{.9\textwidth}
\includegraphics[width=\textwidth]{../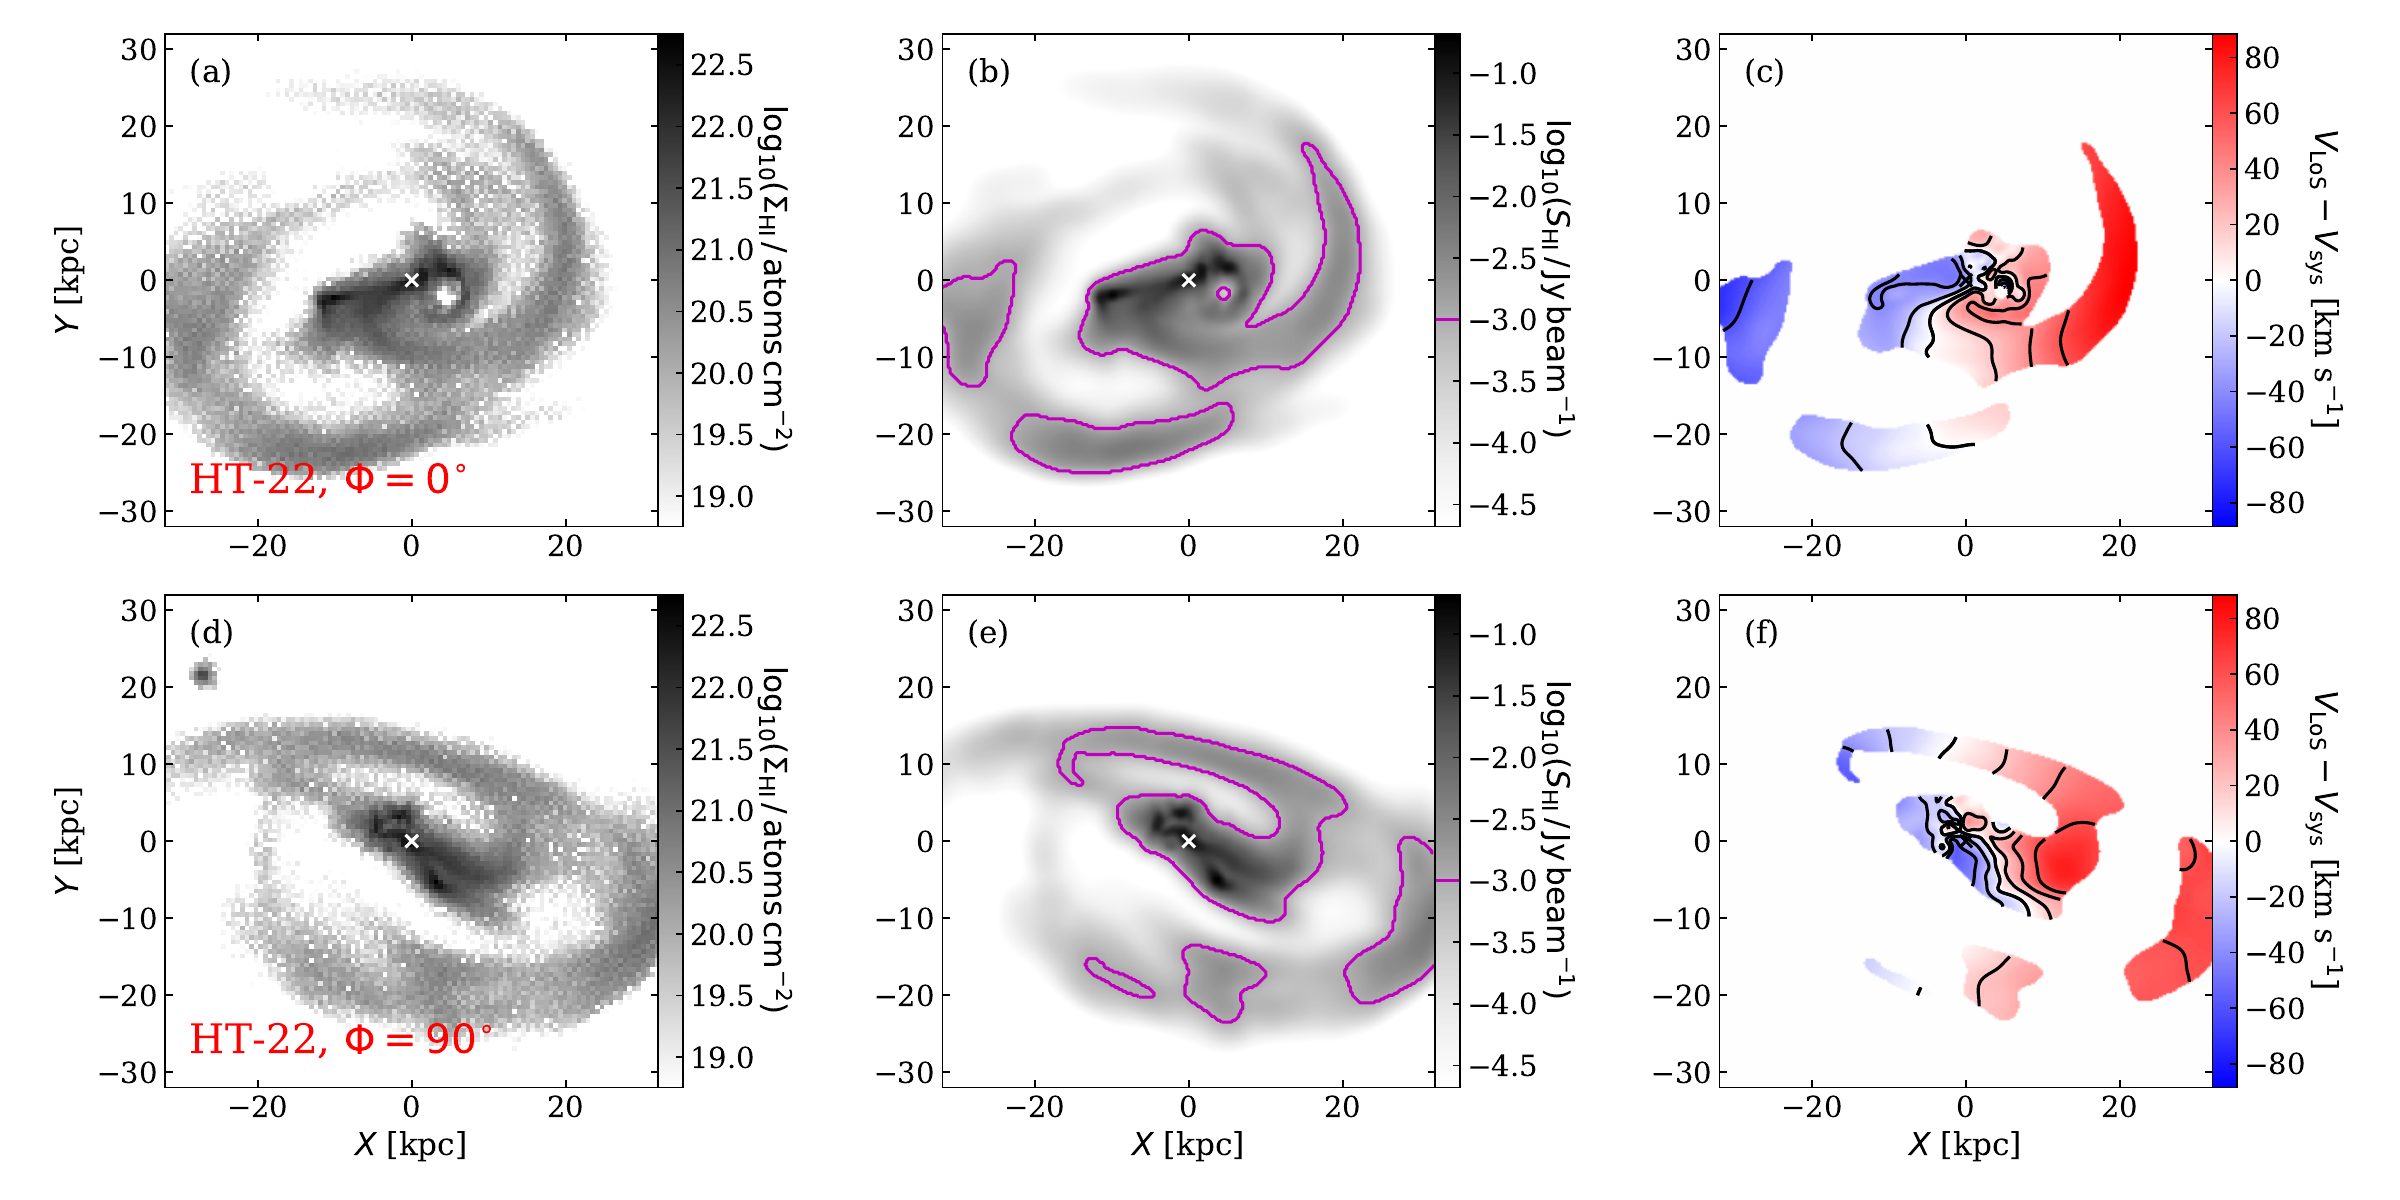}
\includegraphics[width=\textwidth]{../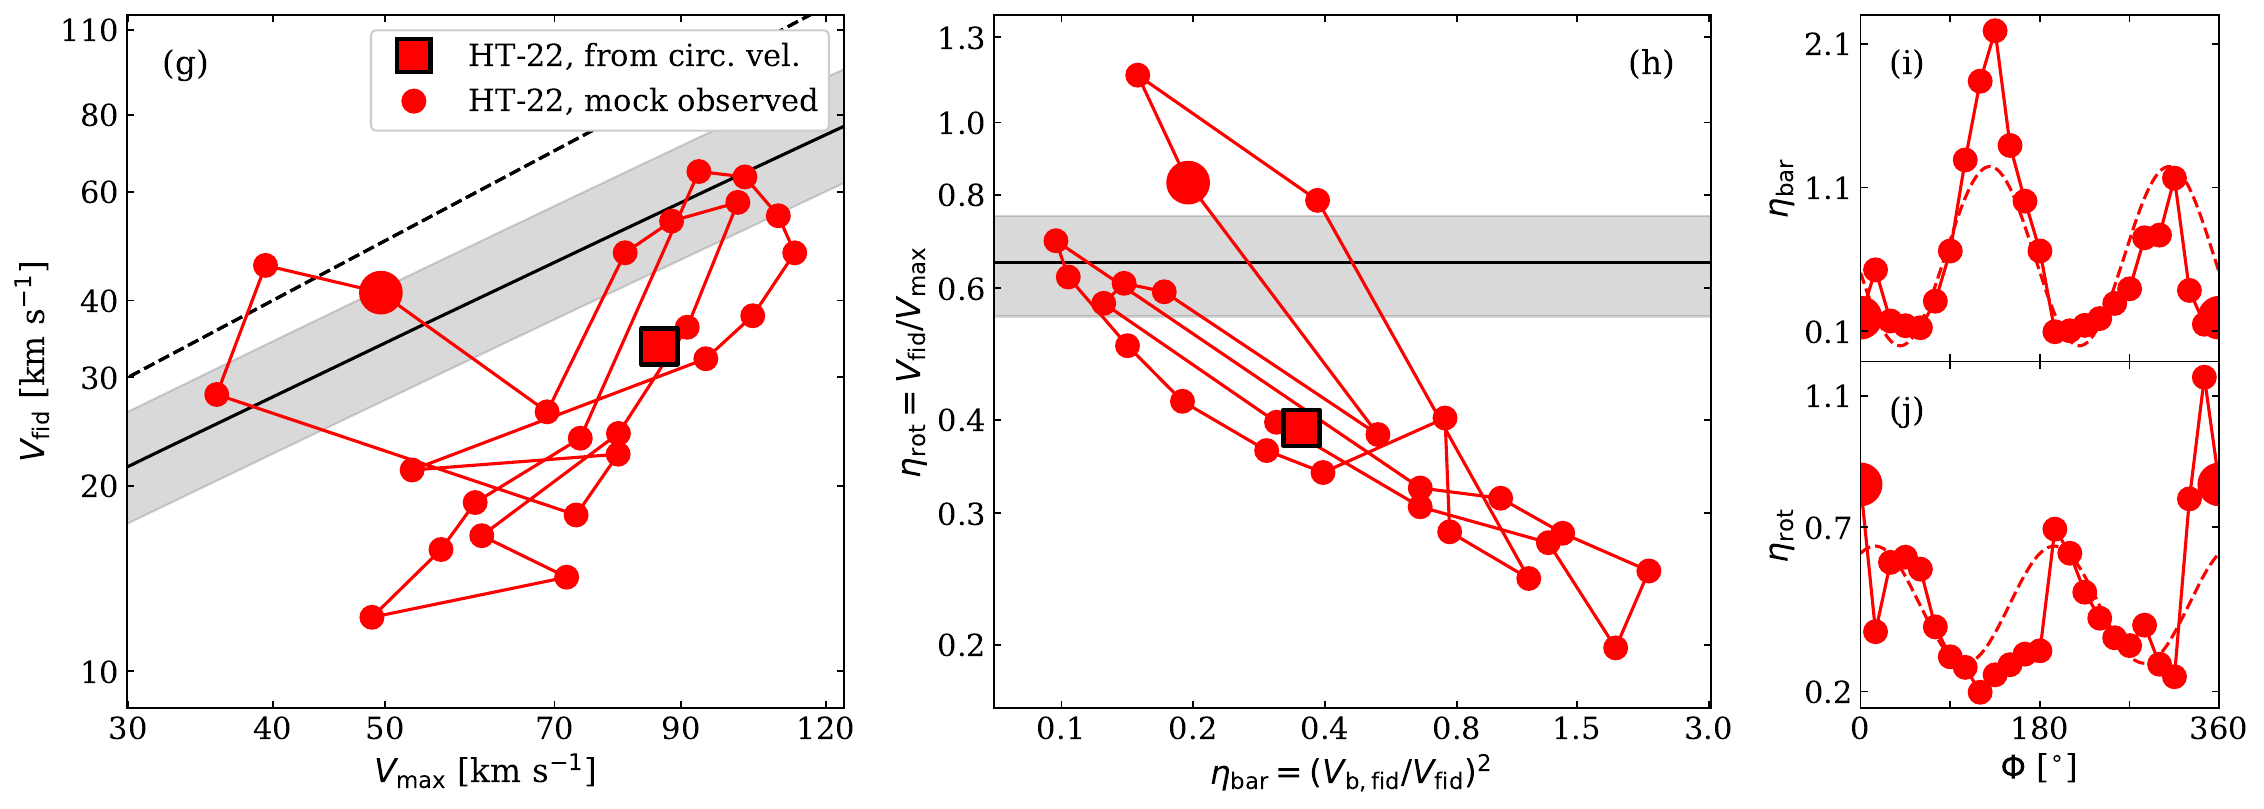}
\end{minipage}
\begin{minipage}{.4\textwidth}
\includegraphics[width=\textwidth]{../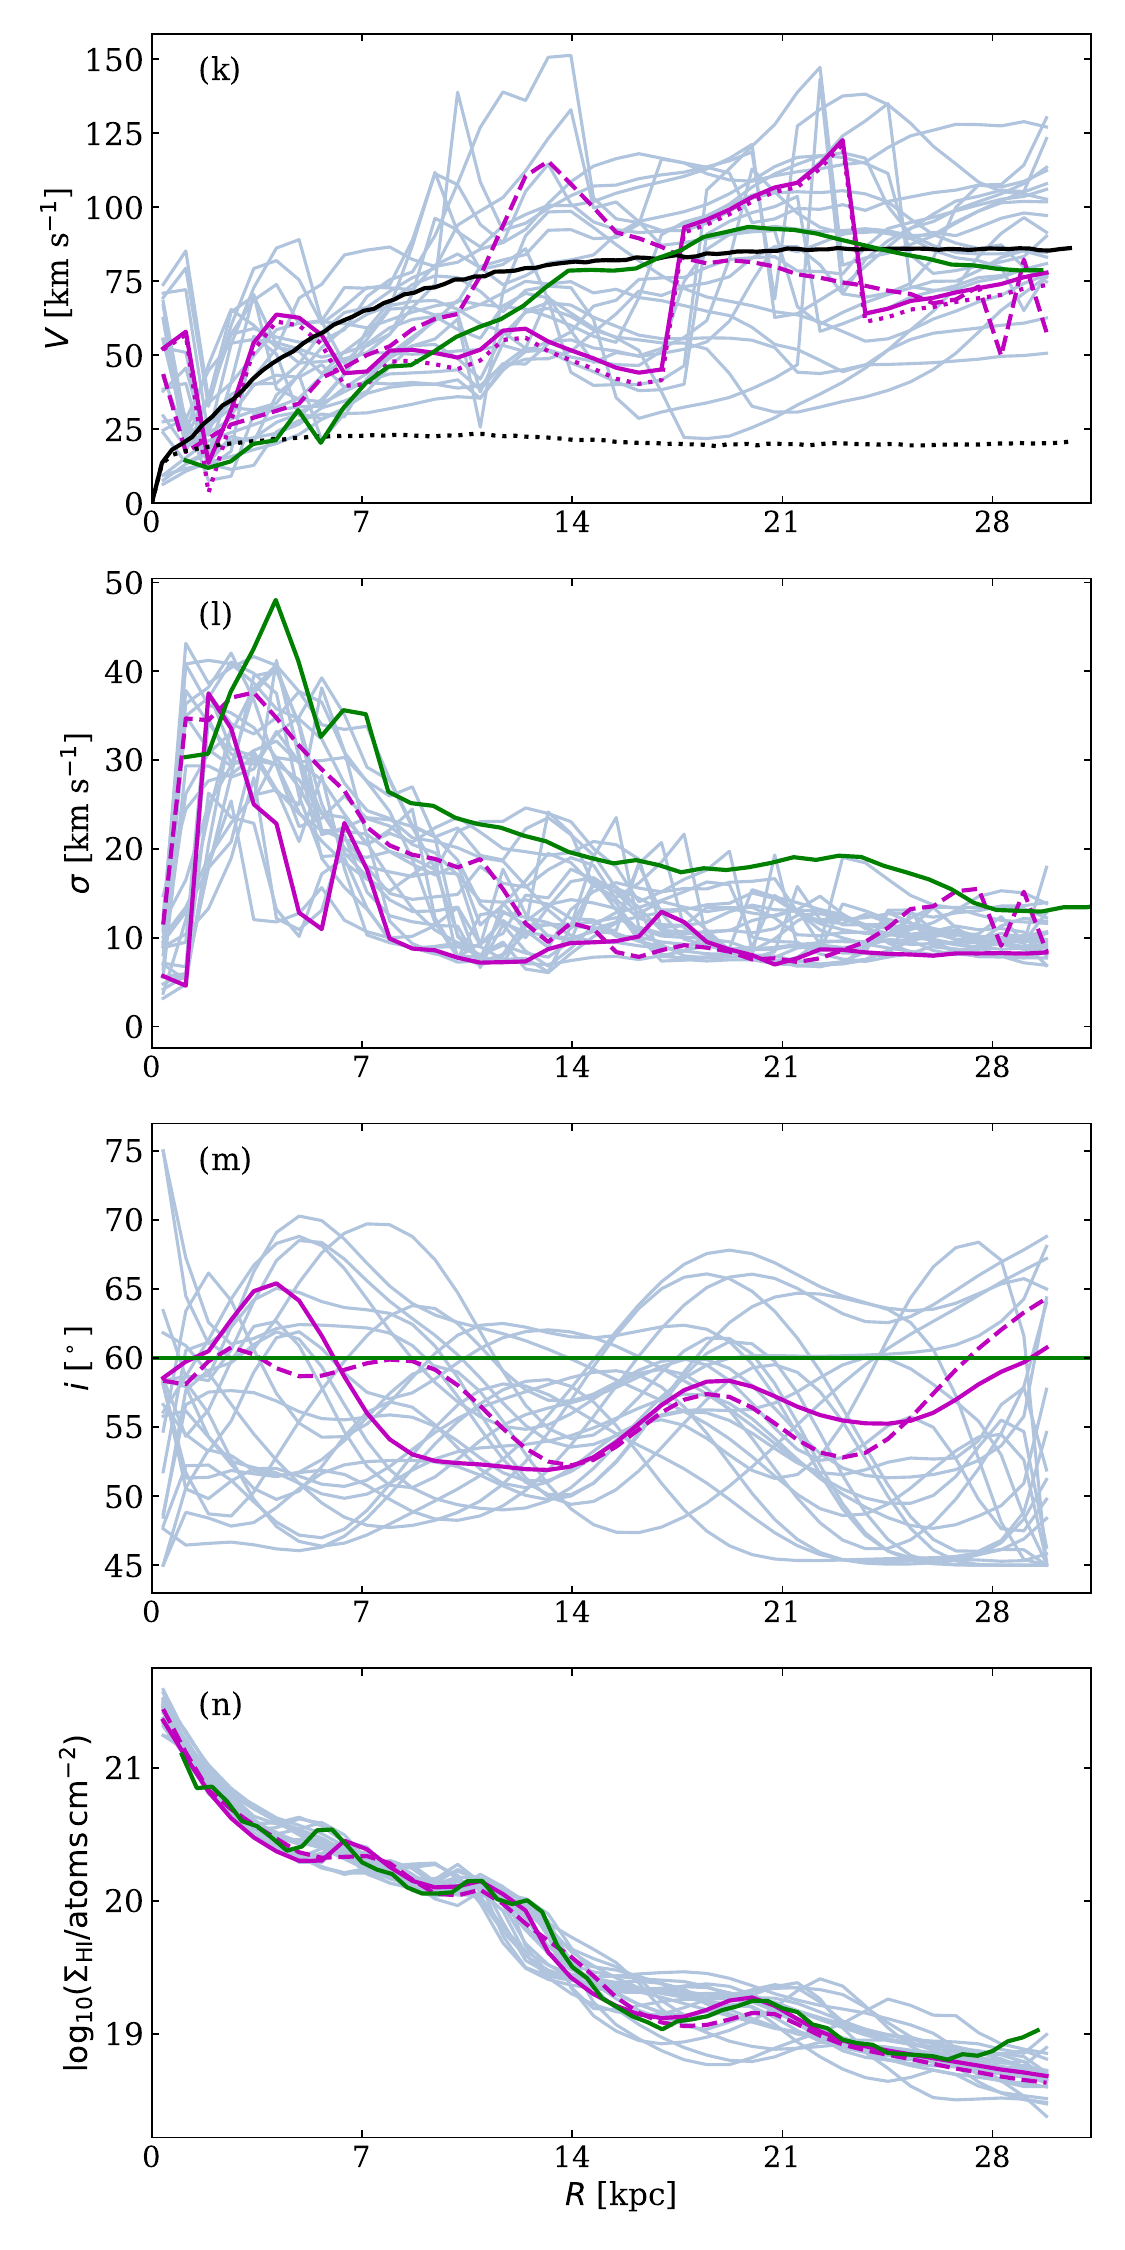}
\end{minipage}
\caption{A set of summary figures for galaxy HT-22, excluded from kinematic analysis. These include example moment maps for two orientations (panels (a)--(f); similar to Fig.~\ref{fig:visualisations}), a summary of the parameters $V_\mathrm{fid}$, $V_\mathrm{max}$, $\eta_\mathrm{rot}$, and $\eta_\mathrm{bar}$ (panels (g)--(j); similar to Fig.~\ref{fig:loops}), and a summary of the rotation curve analysis from $24$ viewing angles (panels (k)--(n); similar to Fig.~\ref{fig:rot_curves}). See description of Appendix~\ref{app:supplementary} for details.}
\label{fig:S69}
\end{figure}
\clearpage

\begin{figure}
\begin{minipage}{.9\textwidth}
\includegraphics[width=\textwidth]{../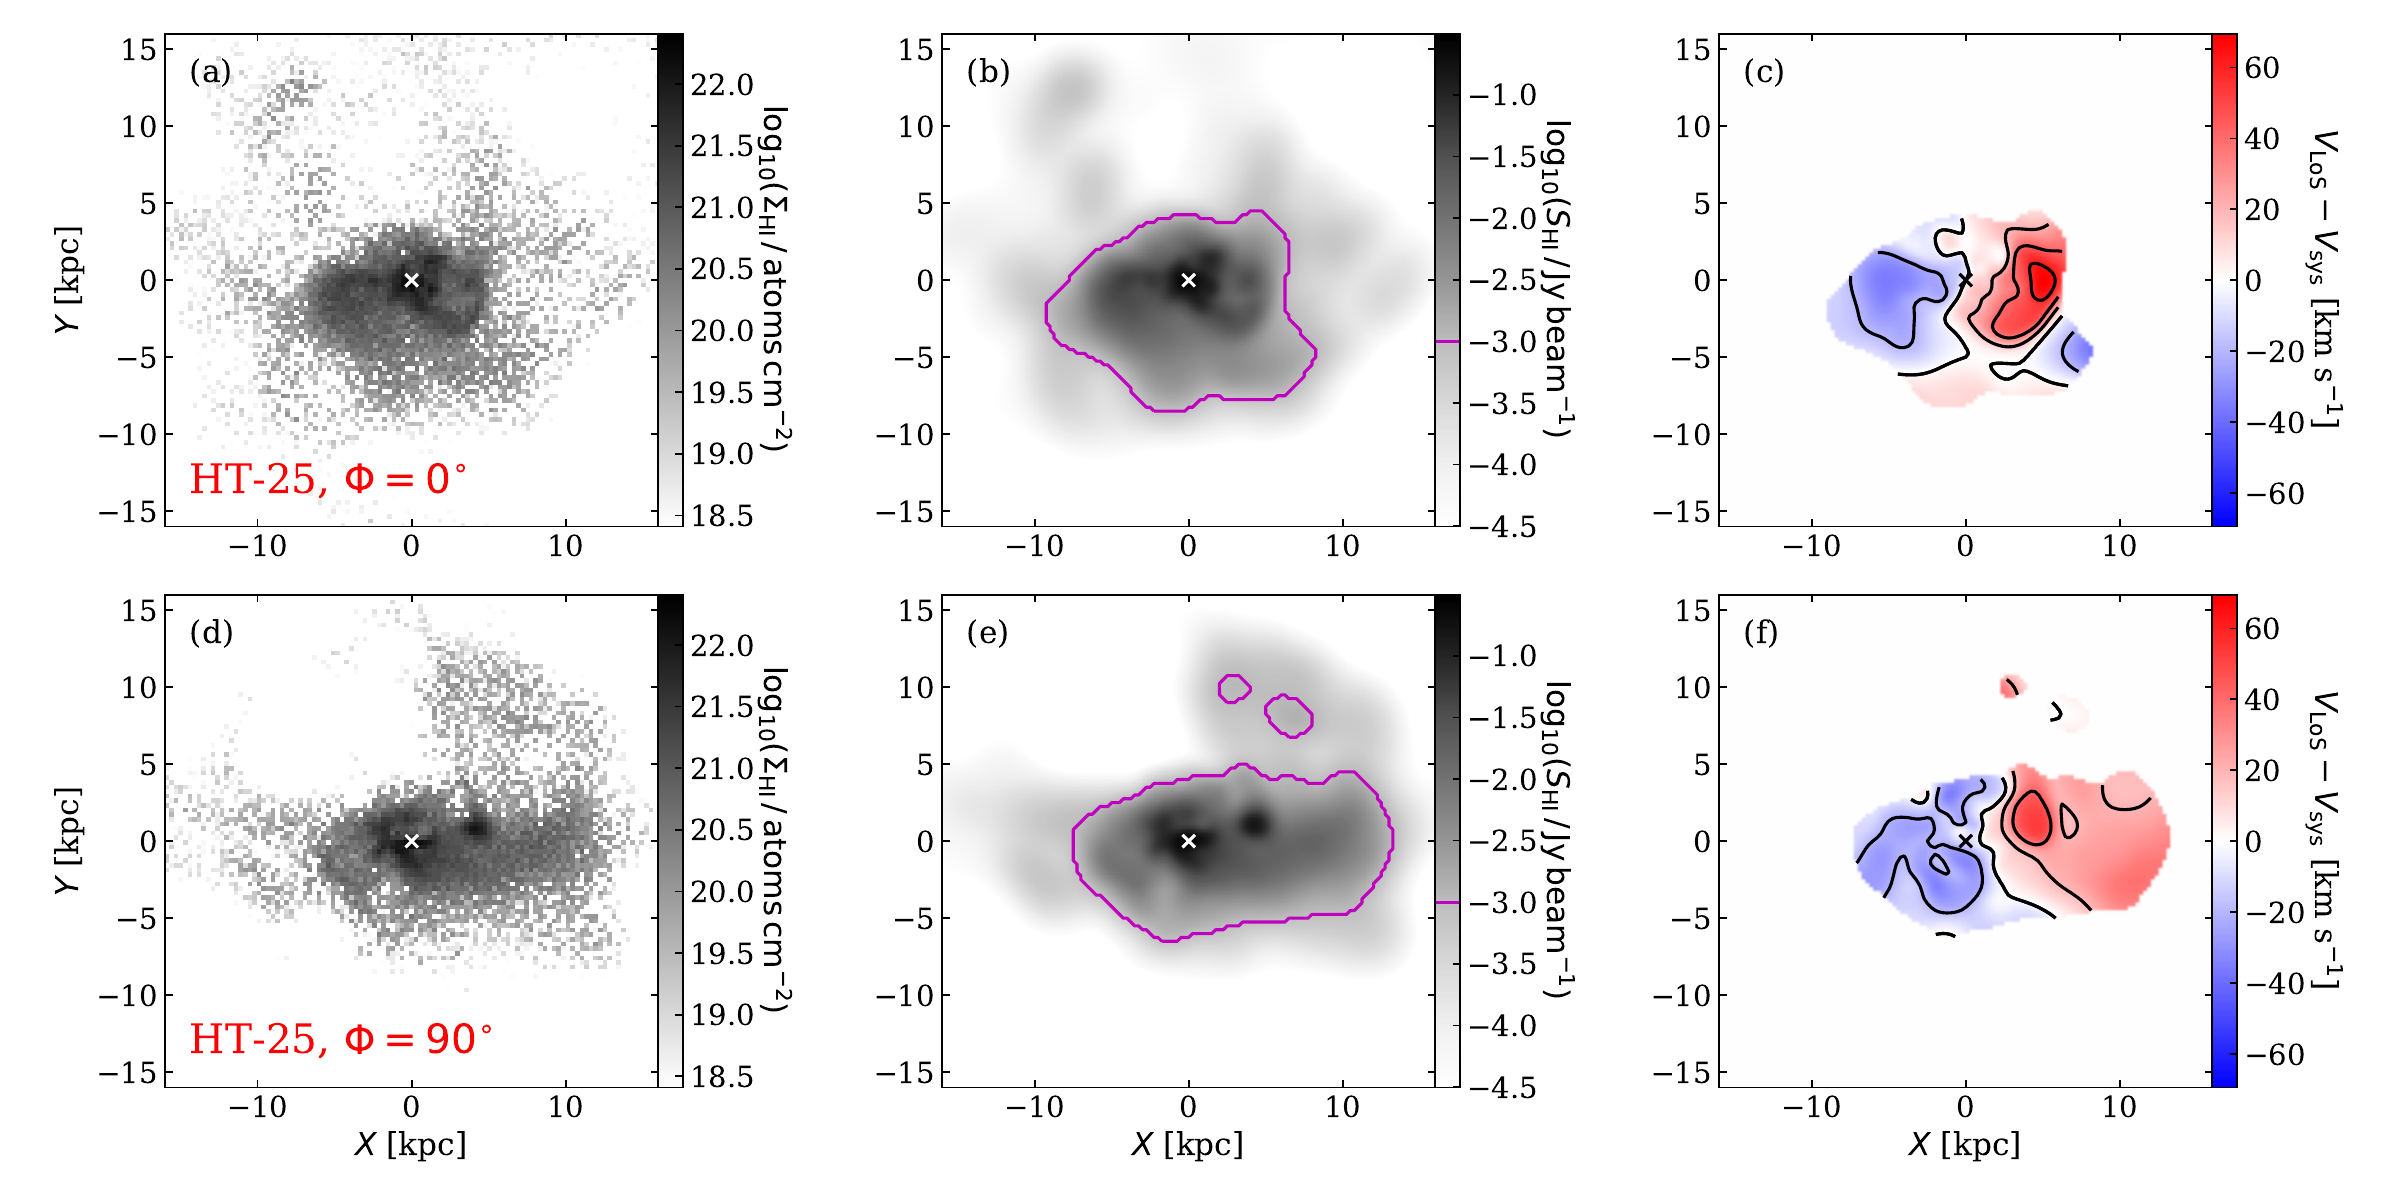}
\includegraphics[width=\textwidth]{../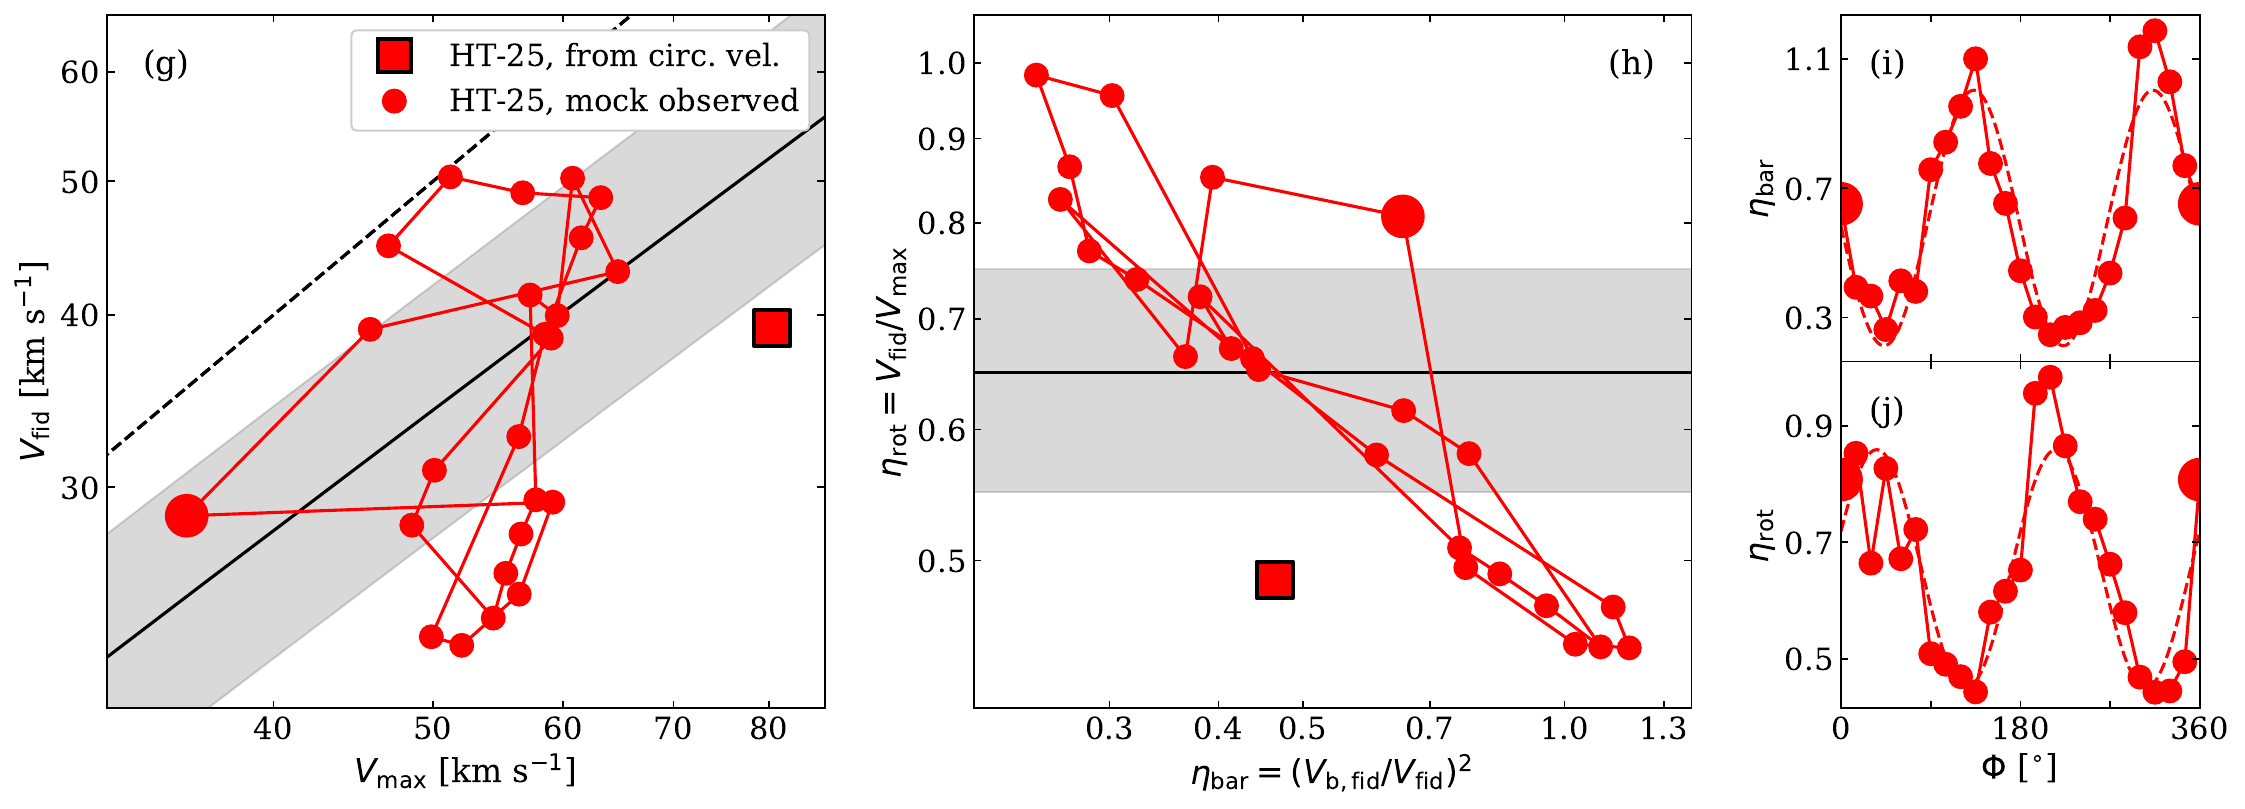}
\end{minipage}
\begin{minipage}{.4\textwidth}
\includegraphics[width=\textwidth]{../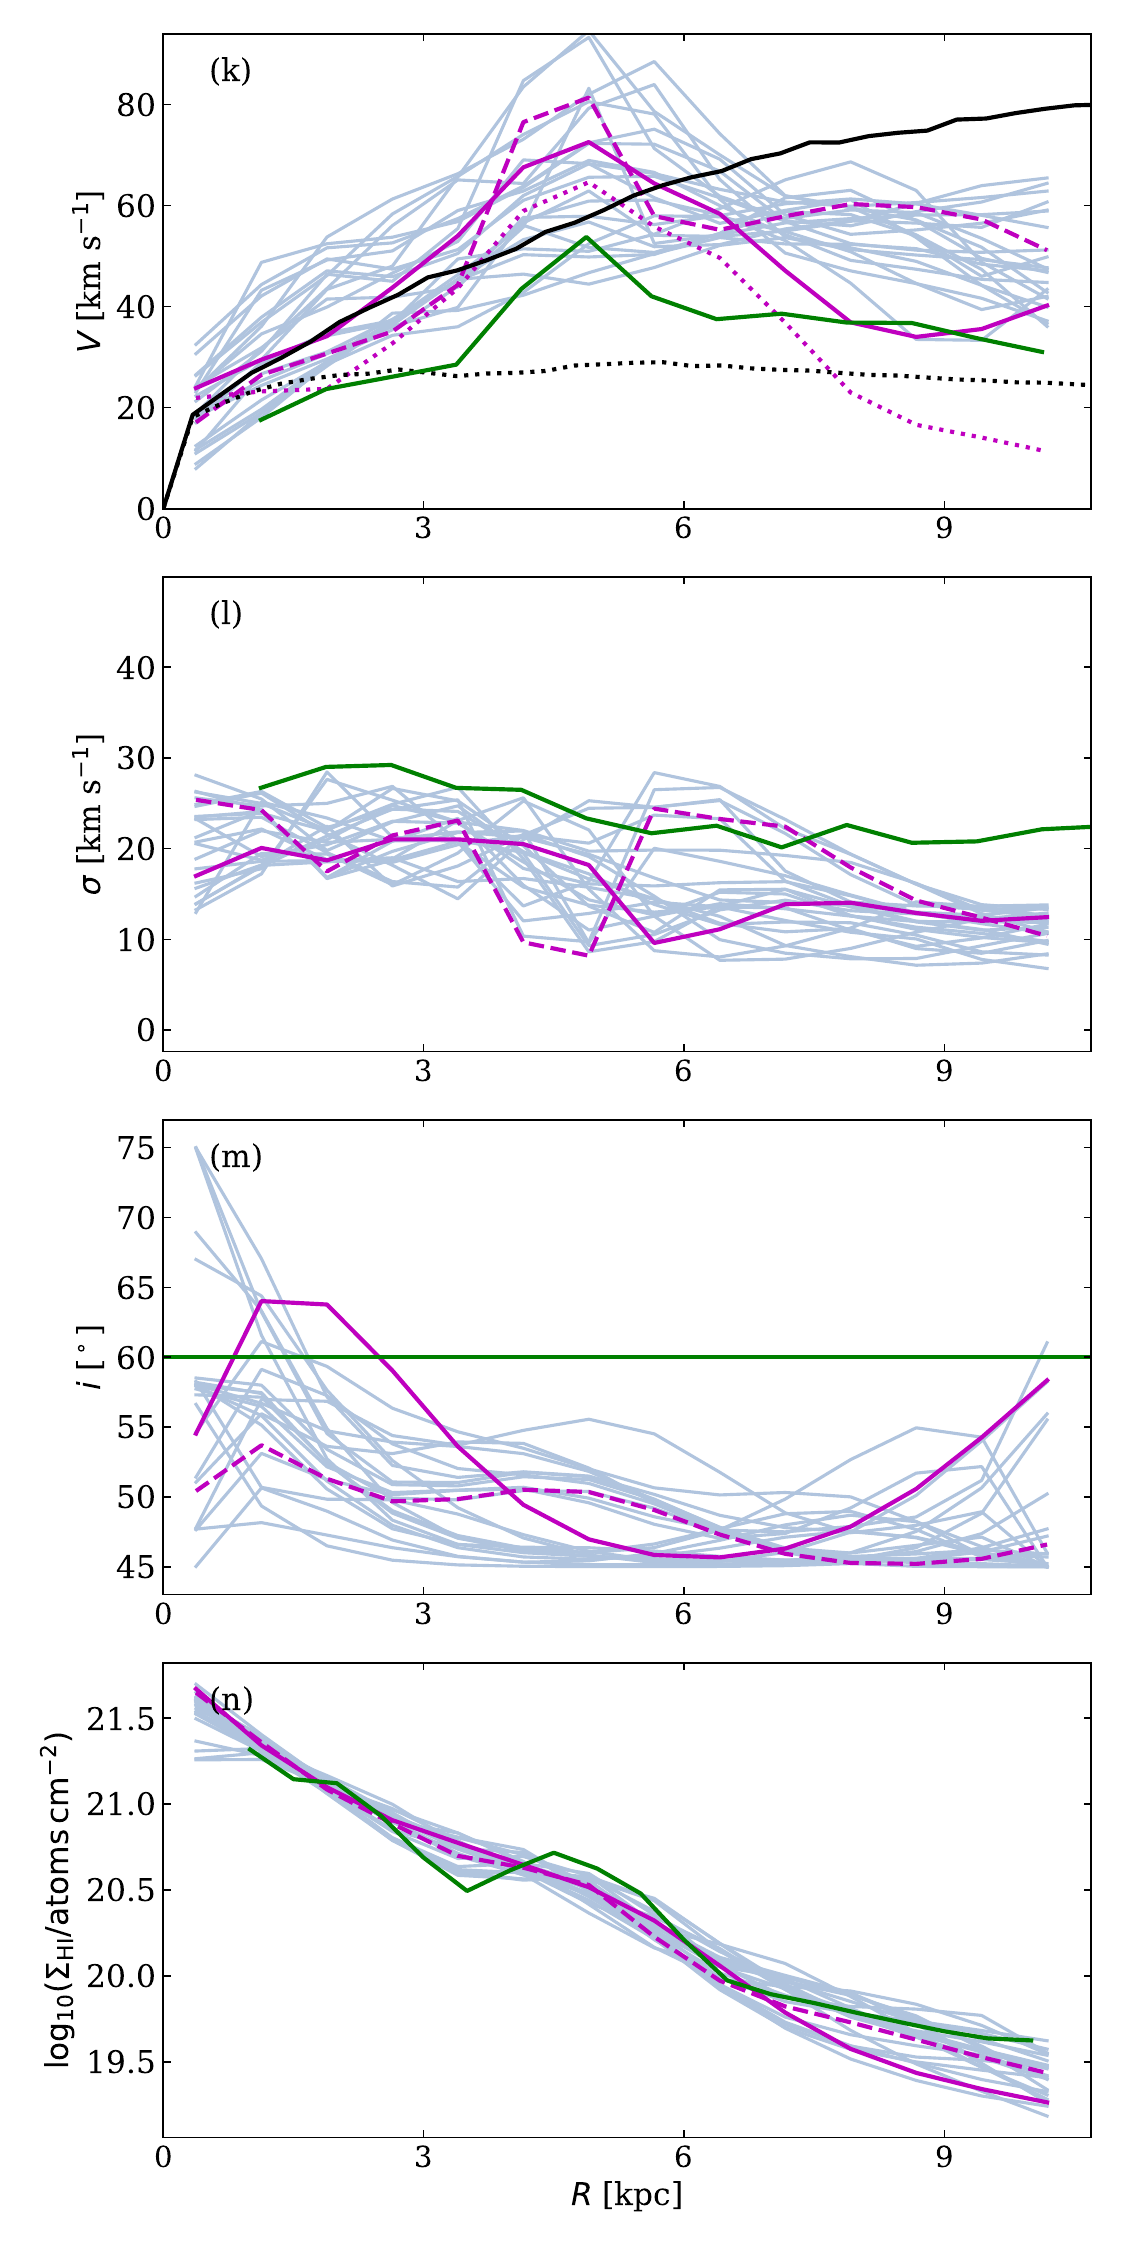}
\end{minipage}
\caption{A set of summary figures for galaxy HT-25, excluded from kinematic analysis. These include example moment maps for two orientations (panels (a)--(f); similar to Fig.~\ref{fig:visualisations}), a summary of the parameters $V_\mathrm{fid}$, $V_\mathrm{max}$, $\eta_\mathrm{rot}$, and $\eta_\mathrm{bar}$ (panels (g)--(j); similar to Fig.~\ref{fig:loops}), and a summary of the rotation curve analysis from $24$ viewing angles (panels (k)--(n); similar to Fig.~\ref{fig:rot_curves}). See description of Appendix~\ref{app:supplementary} for details.}
\label{fig:S70}
\end{figure}
\clearpage

\begin{figure}
\begin{minipage}{.9\textwidth}
\includegraphics[width=\textwidth]{../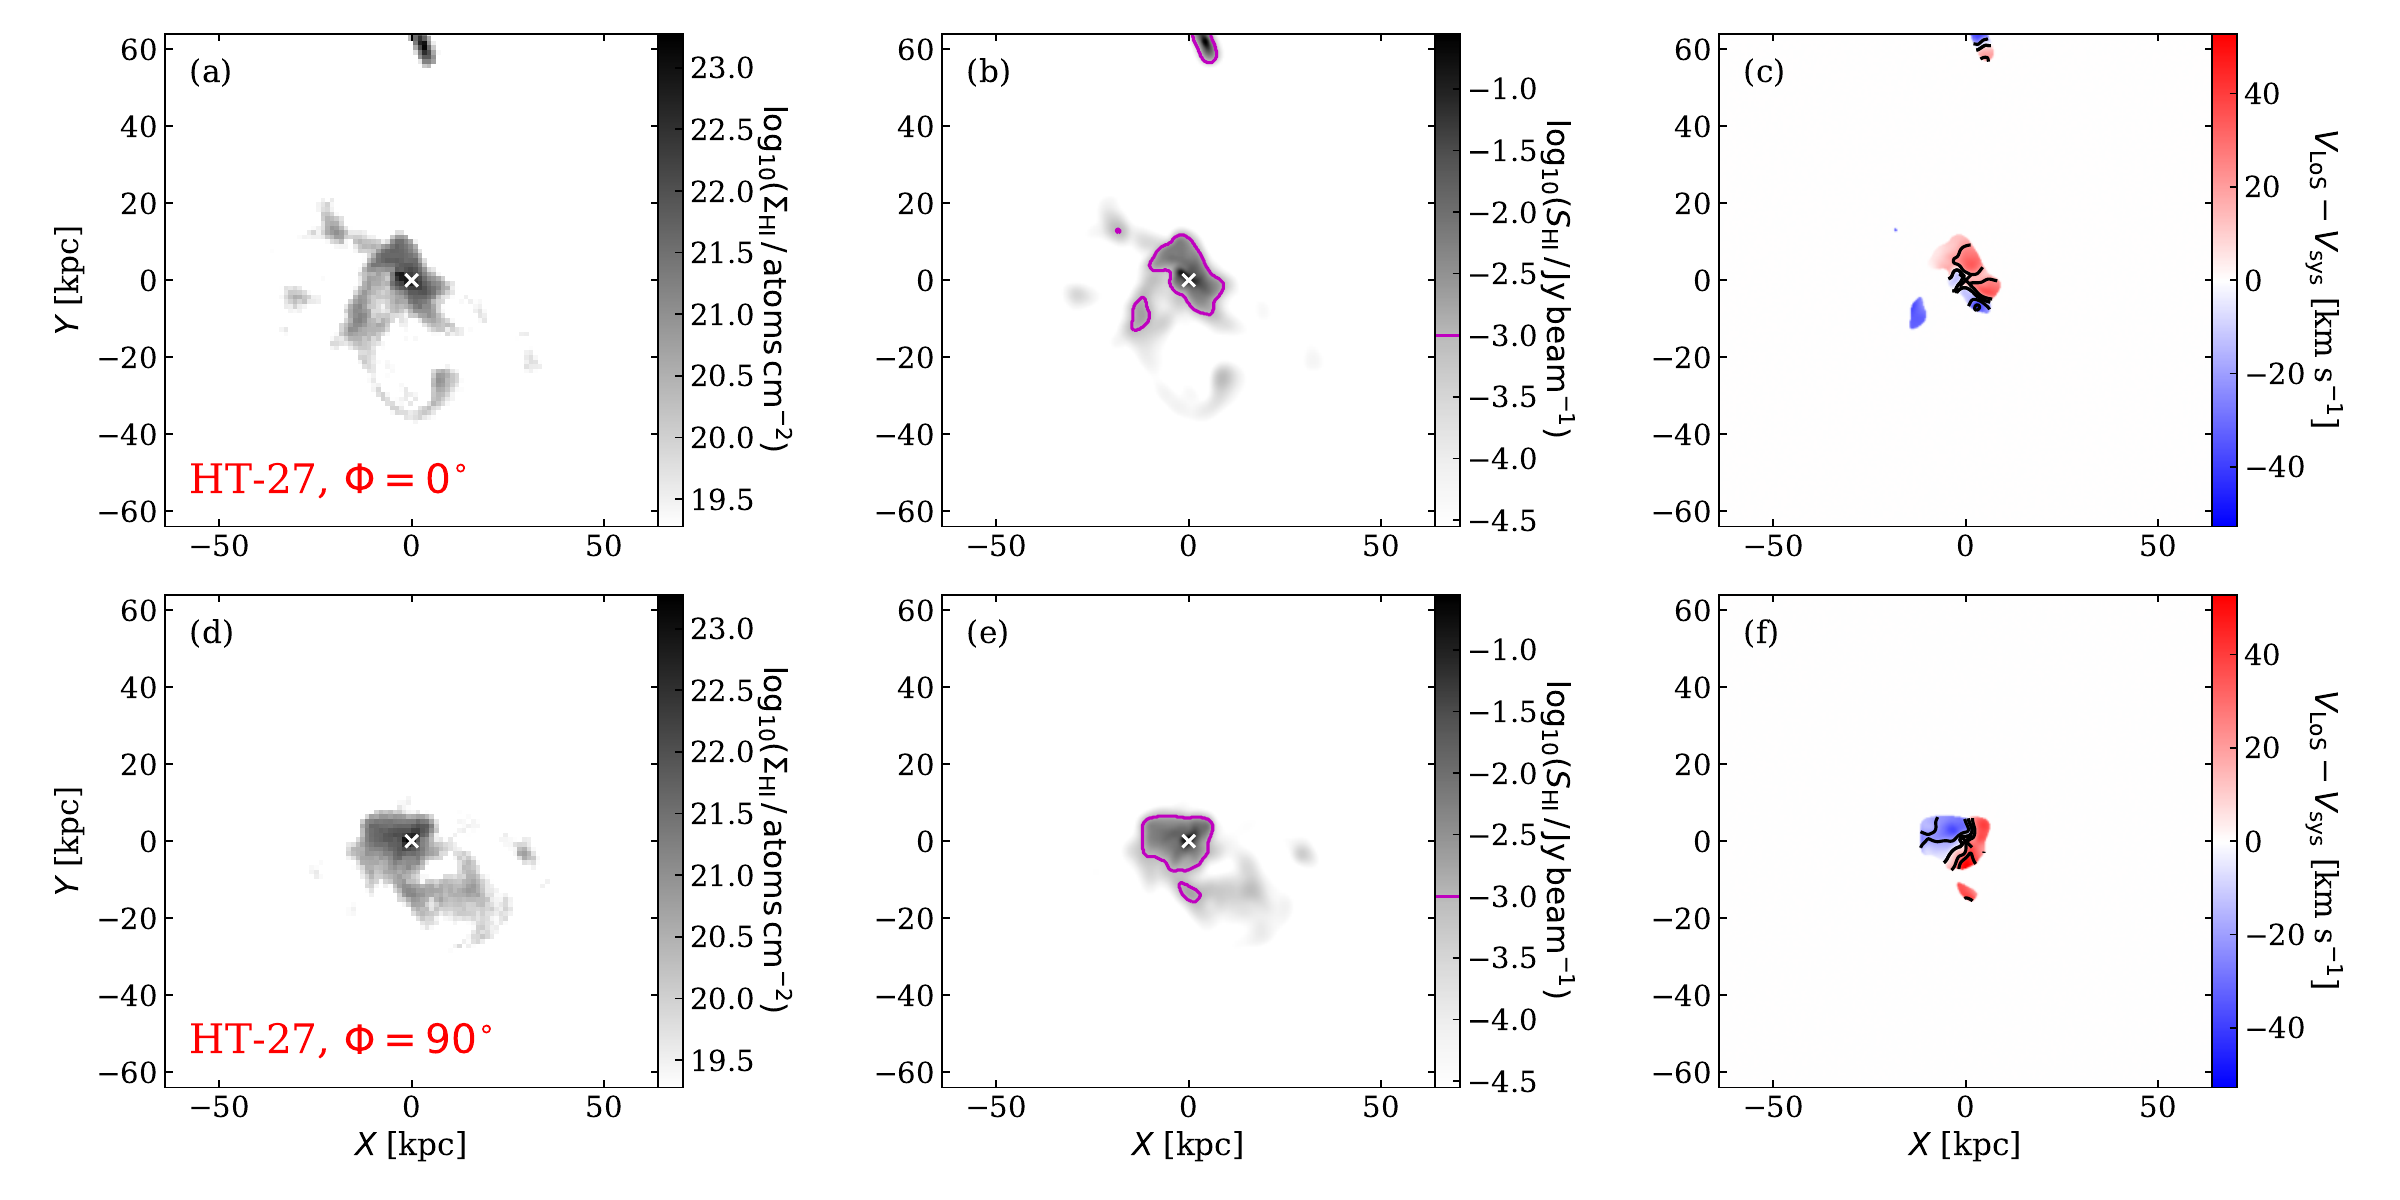}
\includegraphics[width=\textwidth]{../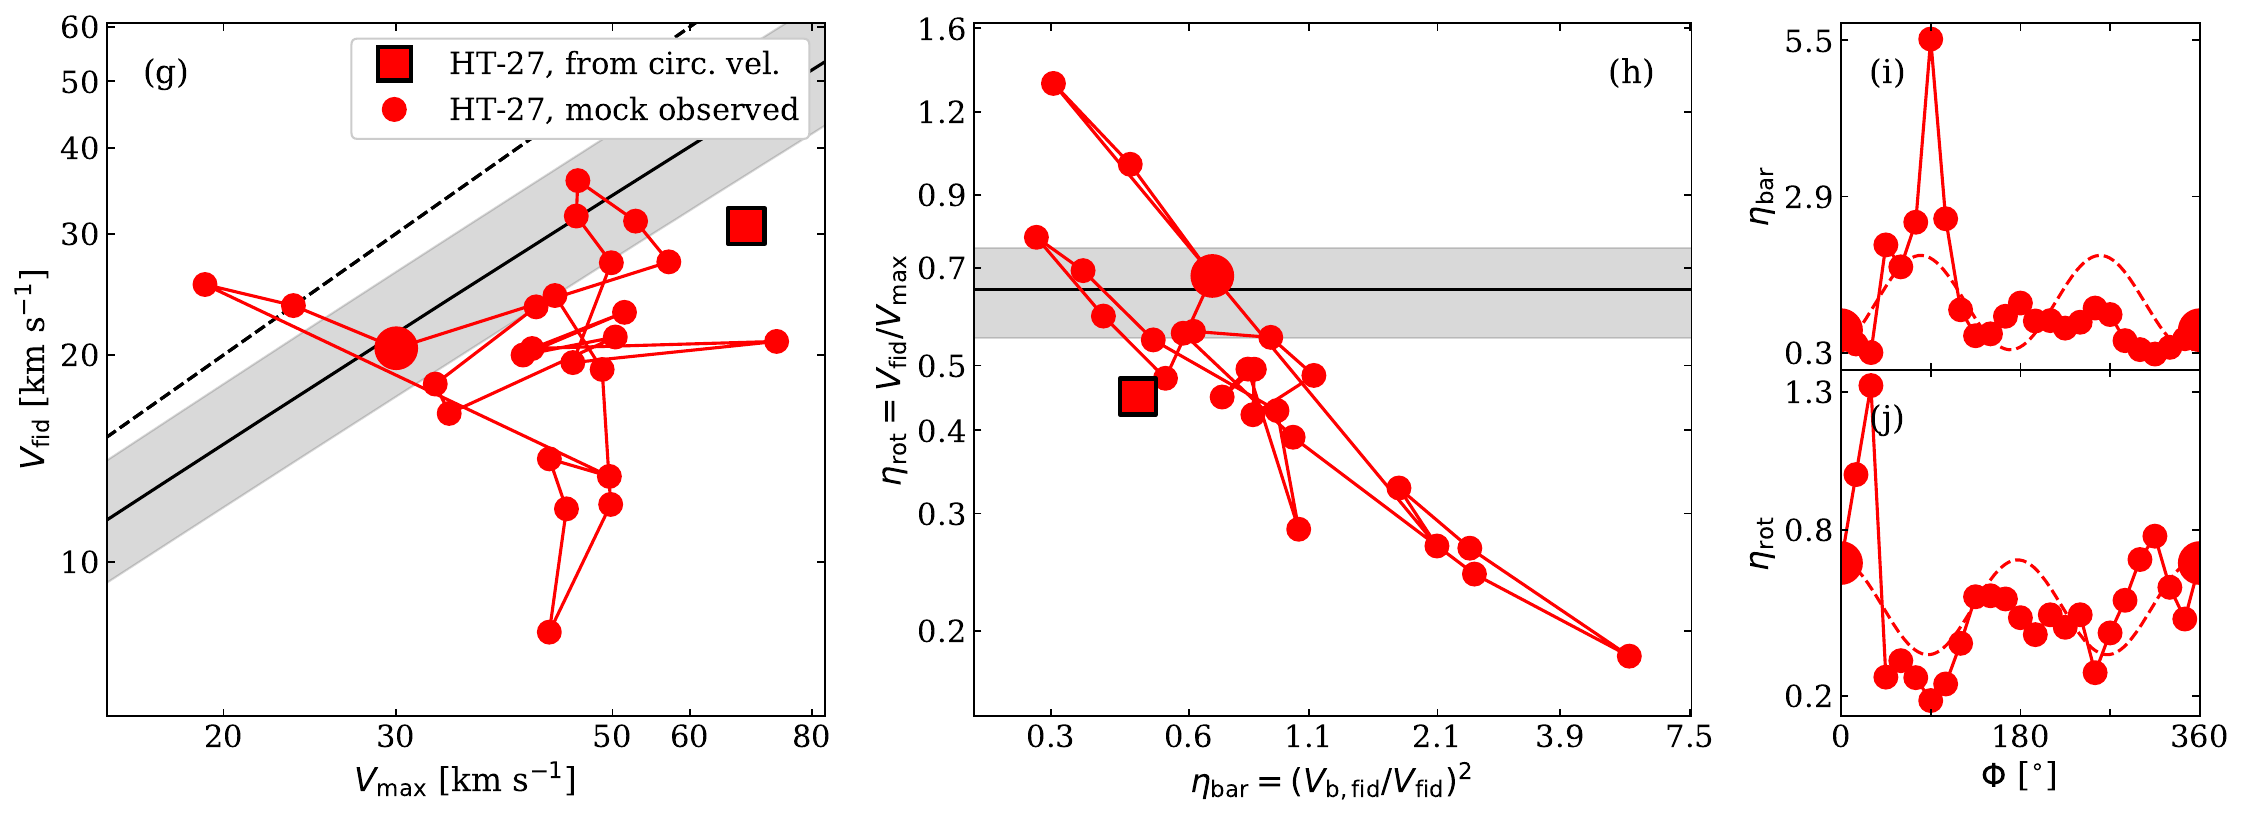}
\end{minipage}
\begin{minipage}{.4\textwidth}
\includegraphics[width=\textwidth]{../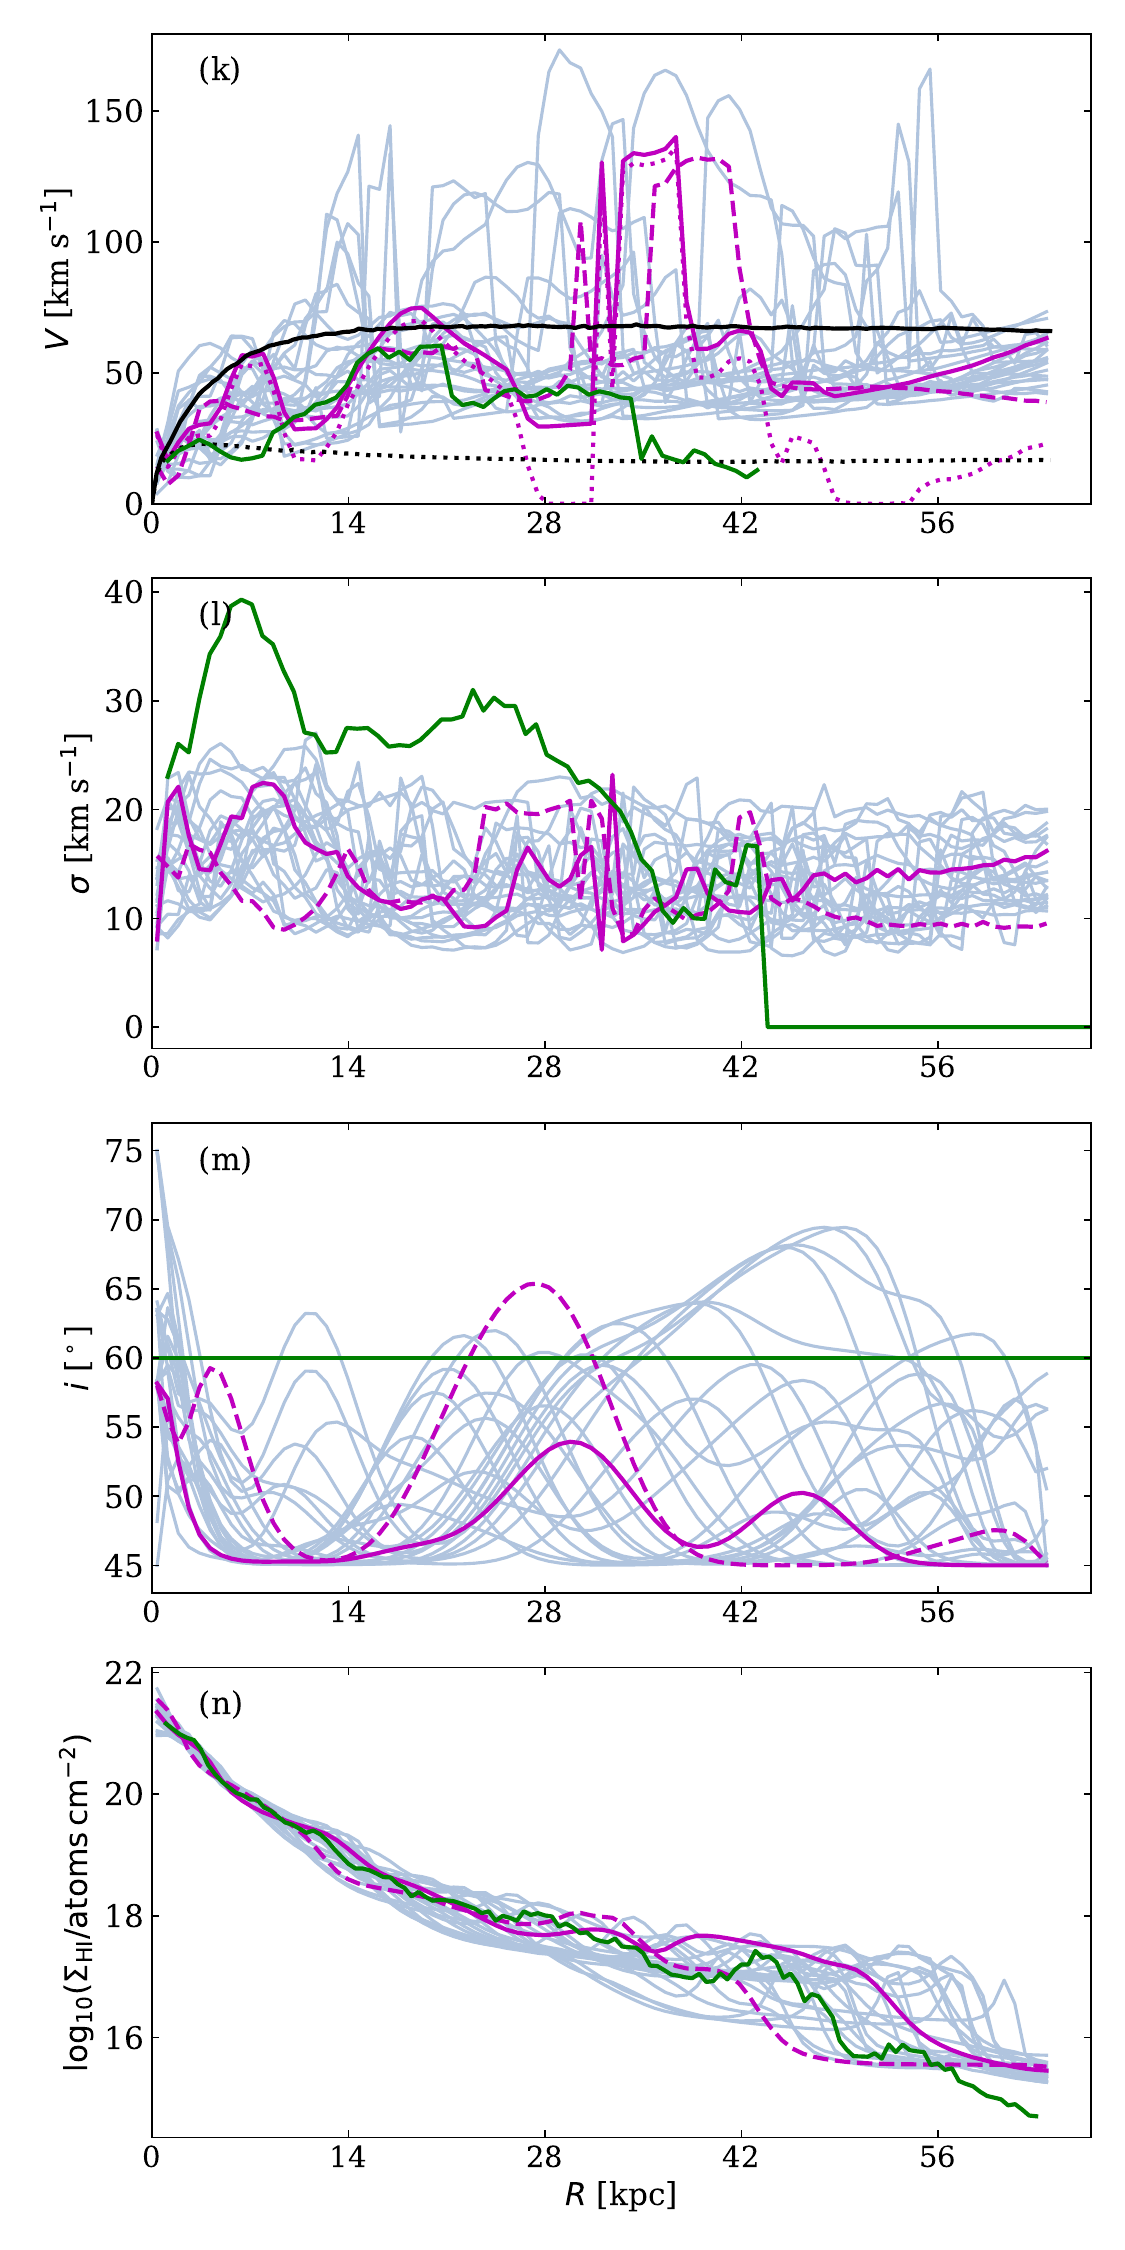}
\end{minipage}
\caption{A set of summary figures for galaxy HT-27, excluded from kinematic analysis. These include example moment maps for two orientations (panels (a)--(f); similar to Fig.~\ref{fig:visualisations}), a summary of the parameters $V_\mathrm{fid}$, $V_\mathrm{max}$, $\eta_\mathrm{rot}$, and $\eta_\mathrm{bar}$ (panels (g)--(j); similar to Fig.~\ref{fig:loops}), and a summary of the rotation curve analysis from $24$ viewing angles (panels (k)--(n); similar to Fig.~\ref{fig:rot_curves}). See description of Appendix~\ref{app:supplementary} for details.}
\label{fig:S71}
\end{figure}
\clearpage

\begin{figure}
\begin{minipage}{.9\textwidth}
\includegraphics[width=\textwidth]{../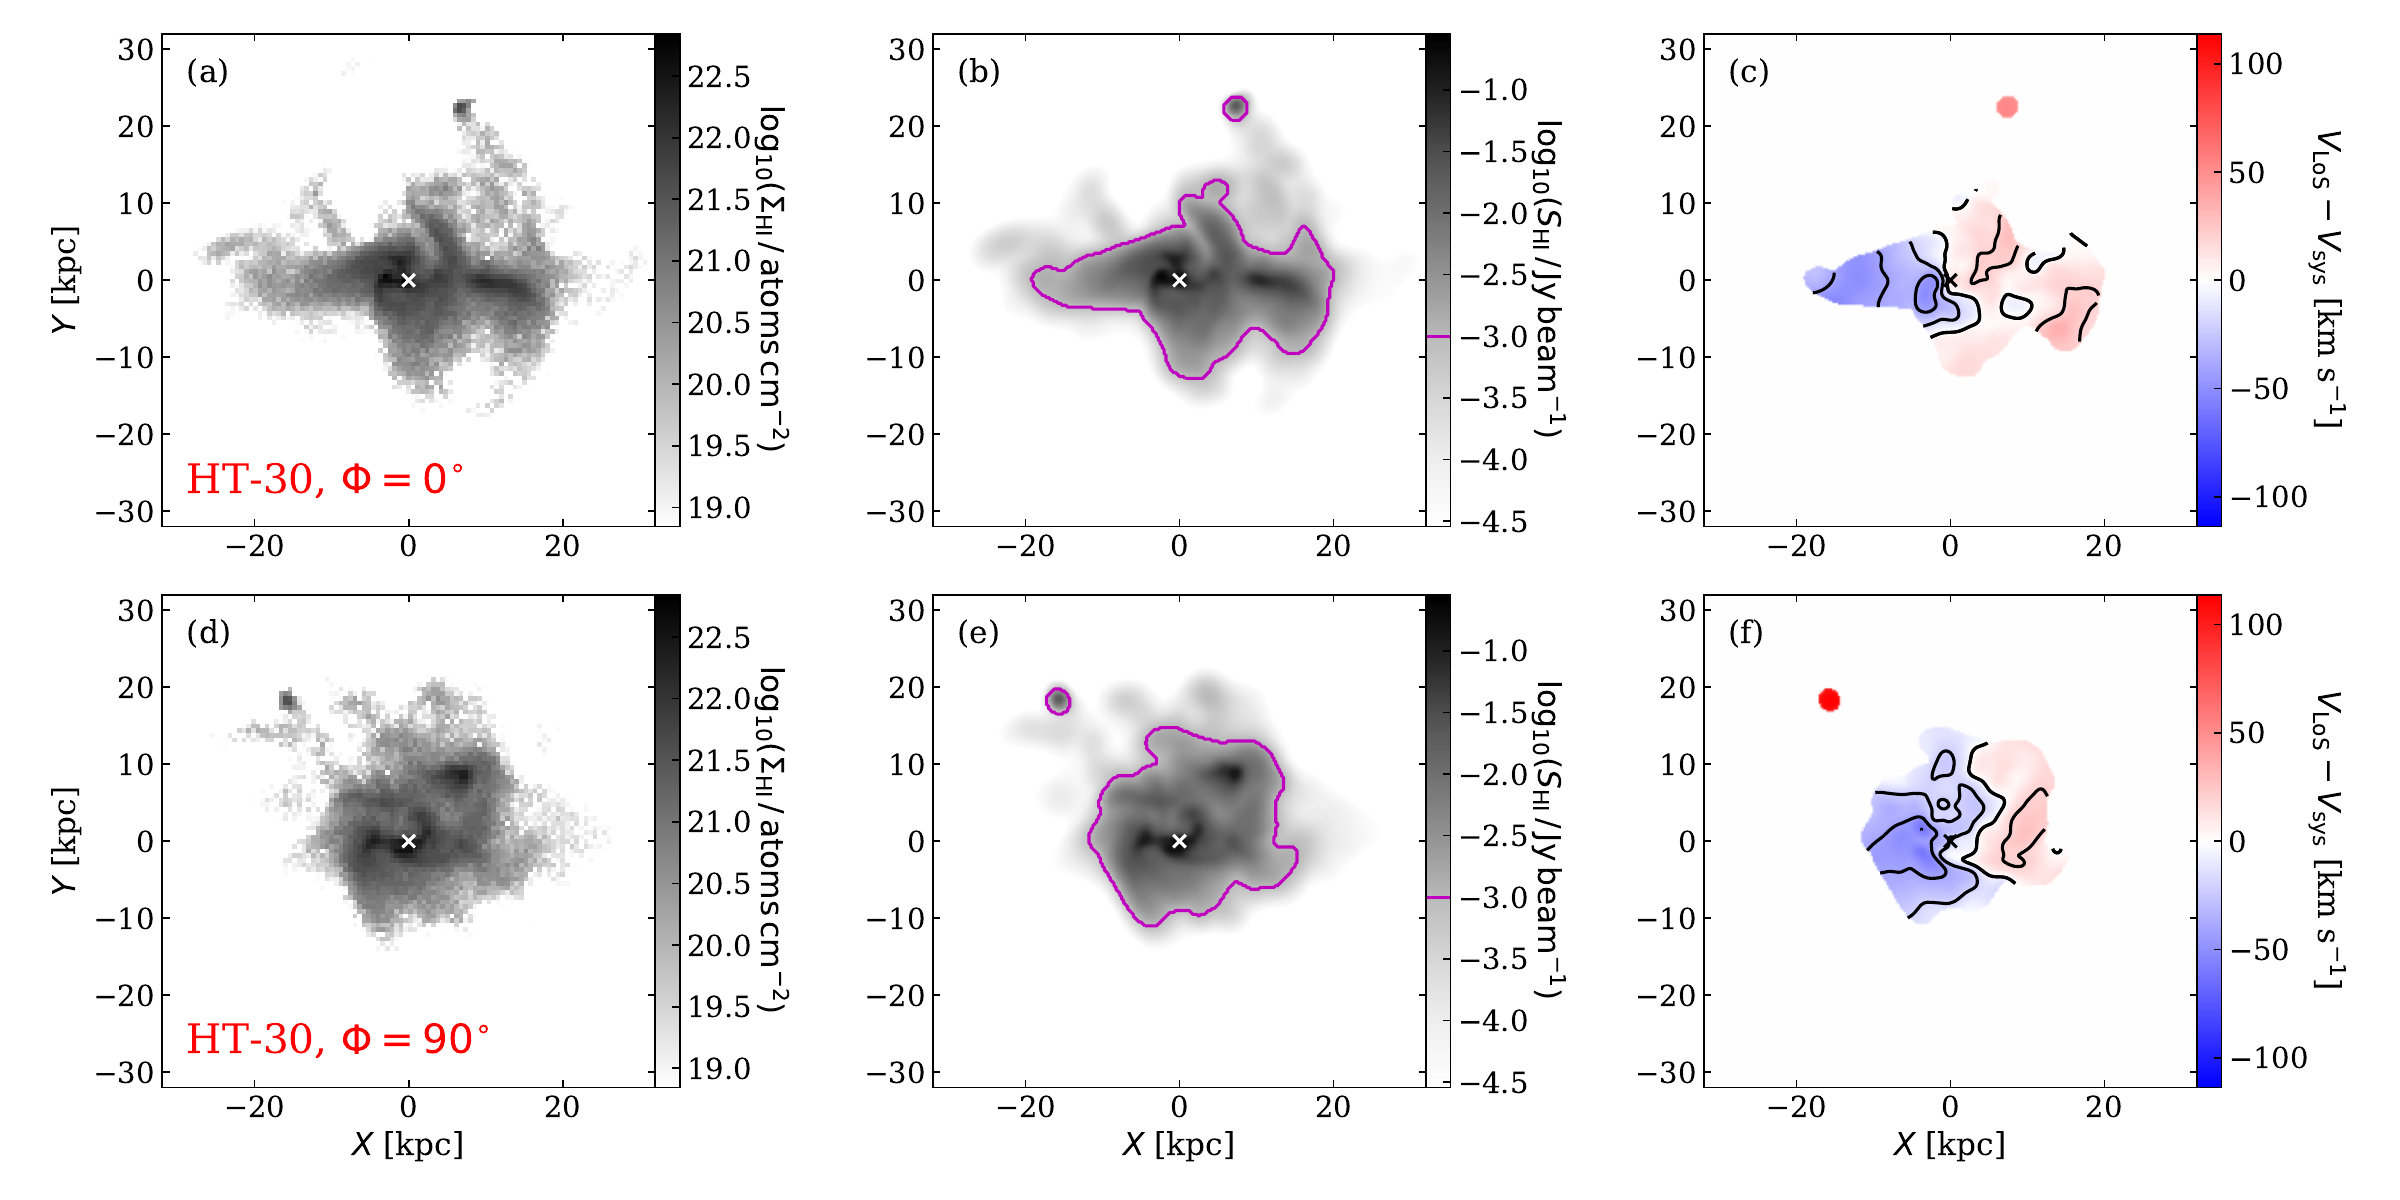}
\includegraphics[width=\textwidth]{../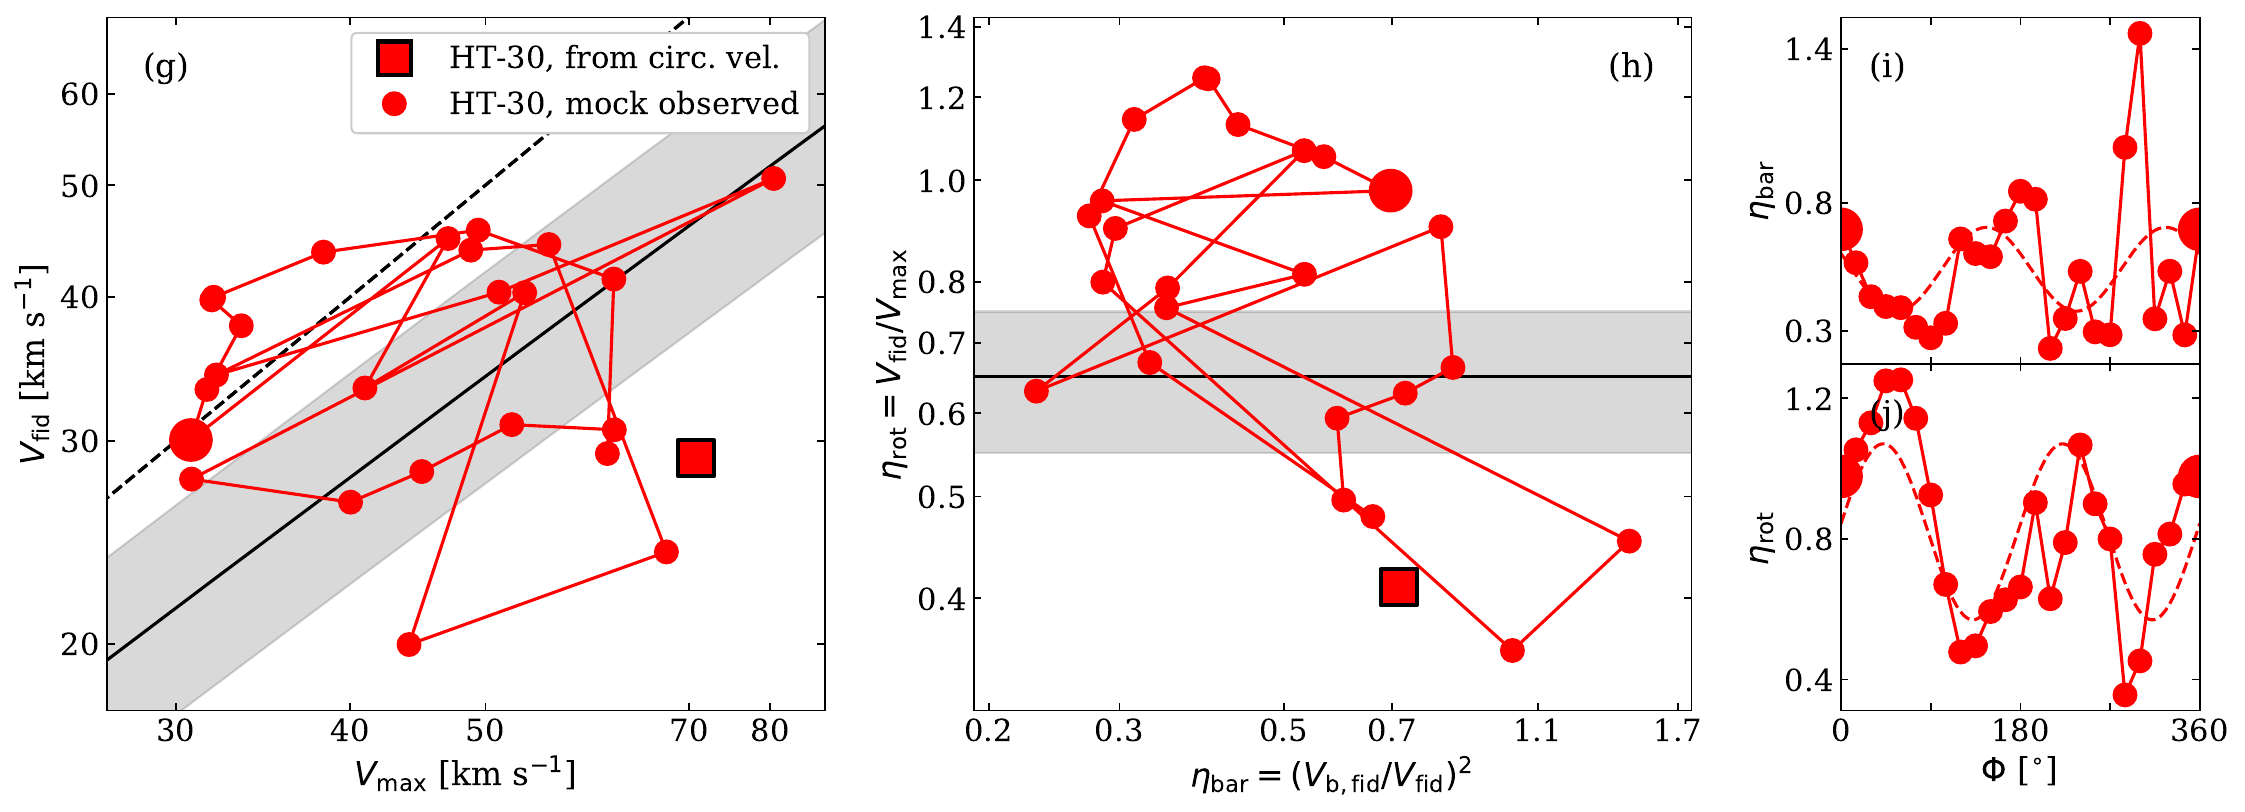}
\end{minipage}
\begin{minipage}{.4\textwidth}
\includegraphics[width=\textwidth]{../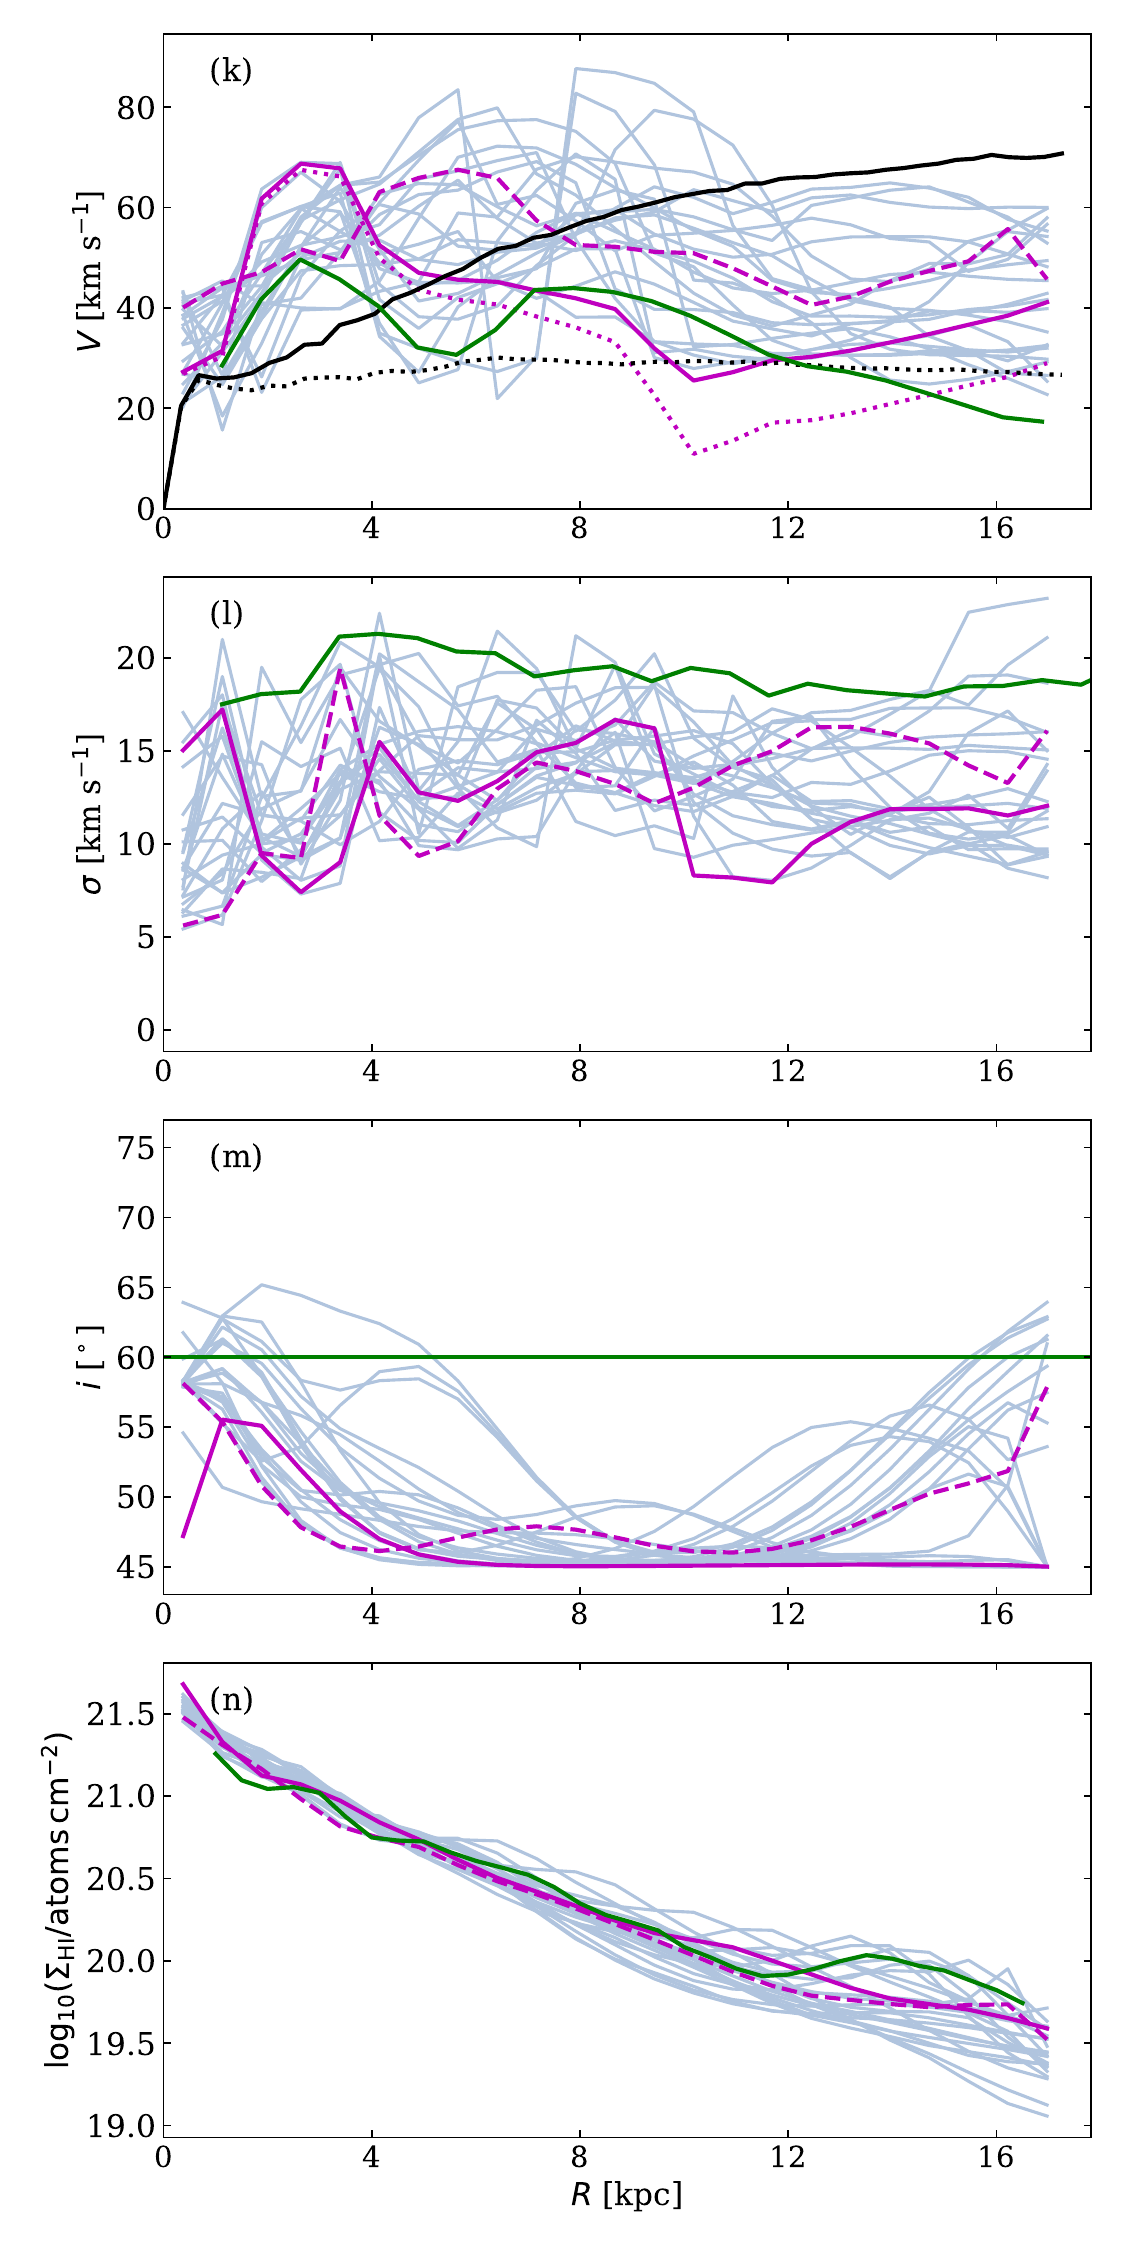}
\end{minipage}
\caption{A set of summary figures for galaxy HT-30, excluded from kinematic analysis. These include example moment maps for two orientations (panels (a)--(f); similar to Fig.~\ref{fig:visualisations}), a summary of the parameters $V_\mathrm{fid}$, $V_\mathrm{max}$, $\eta_\mathrm{rot}$, and $\eta_\mathrm{bar}$ (panels (g)--(j); similar to Fig.~\ref{fig:loops}), and a summary of the rotation curve analysis from $24$ viewing angles (panels (k)--(n); similar to Fig.~\ref{fig:rot_curves}). See description of Appendix~\ref{app:supplementary} for details.}
\label{fig:S72}
\end{figure}
\clearpage

\begin{figure}
\begin{minipage}{.9\textwidth}
\includegraphics[width=\textwidth]{../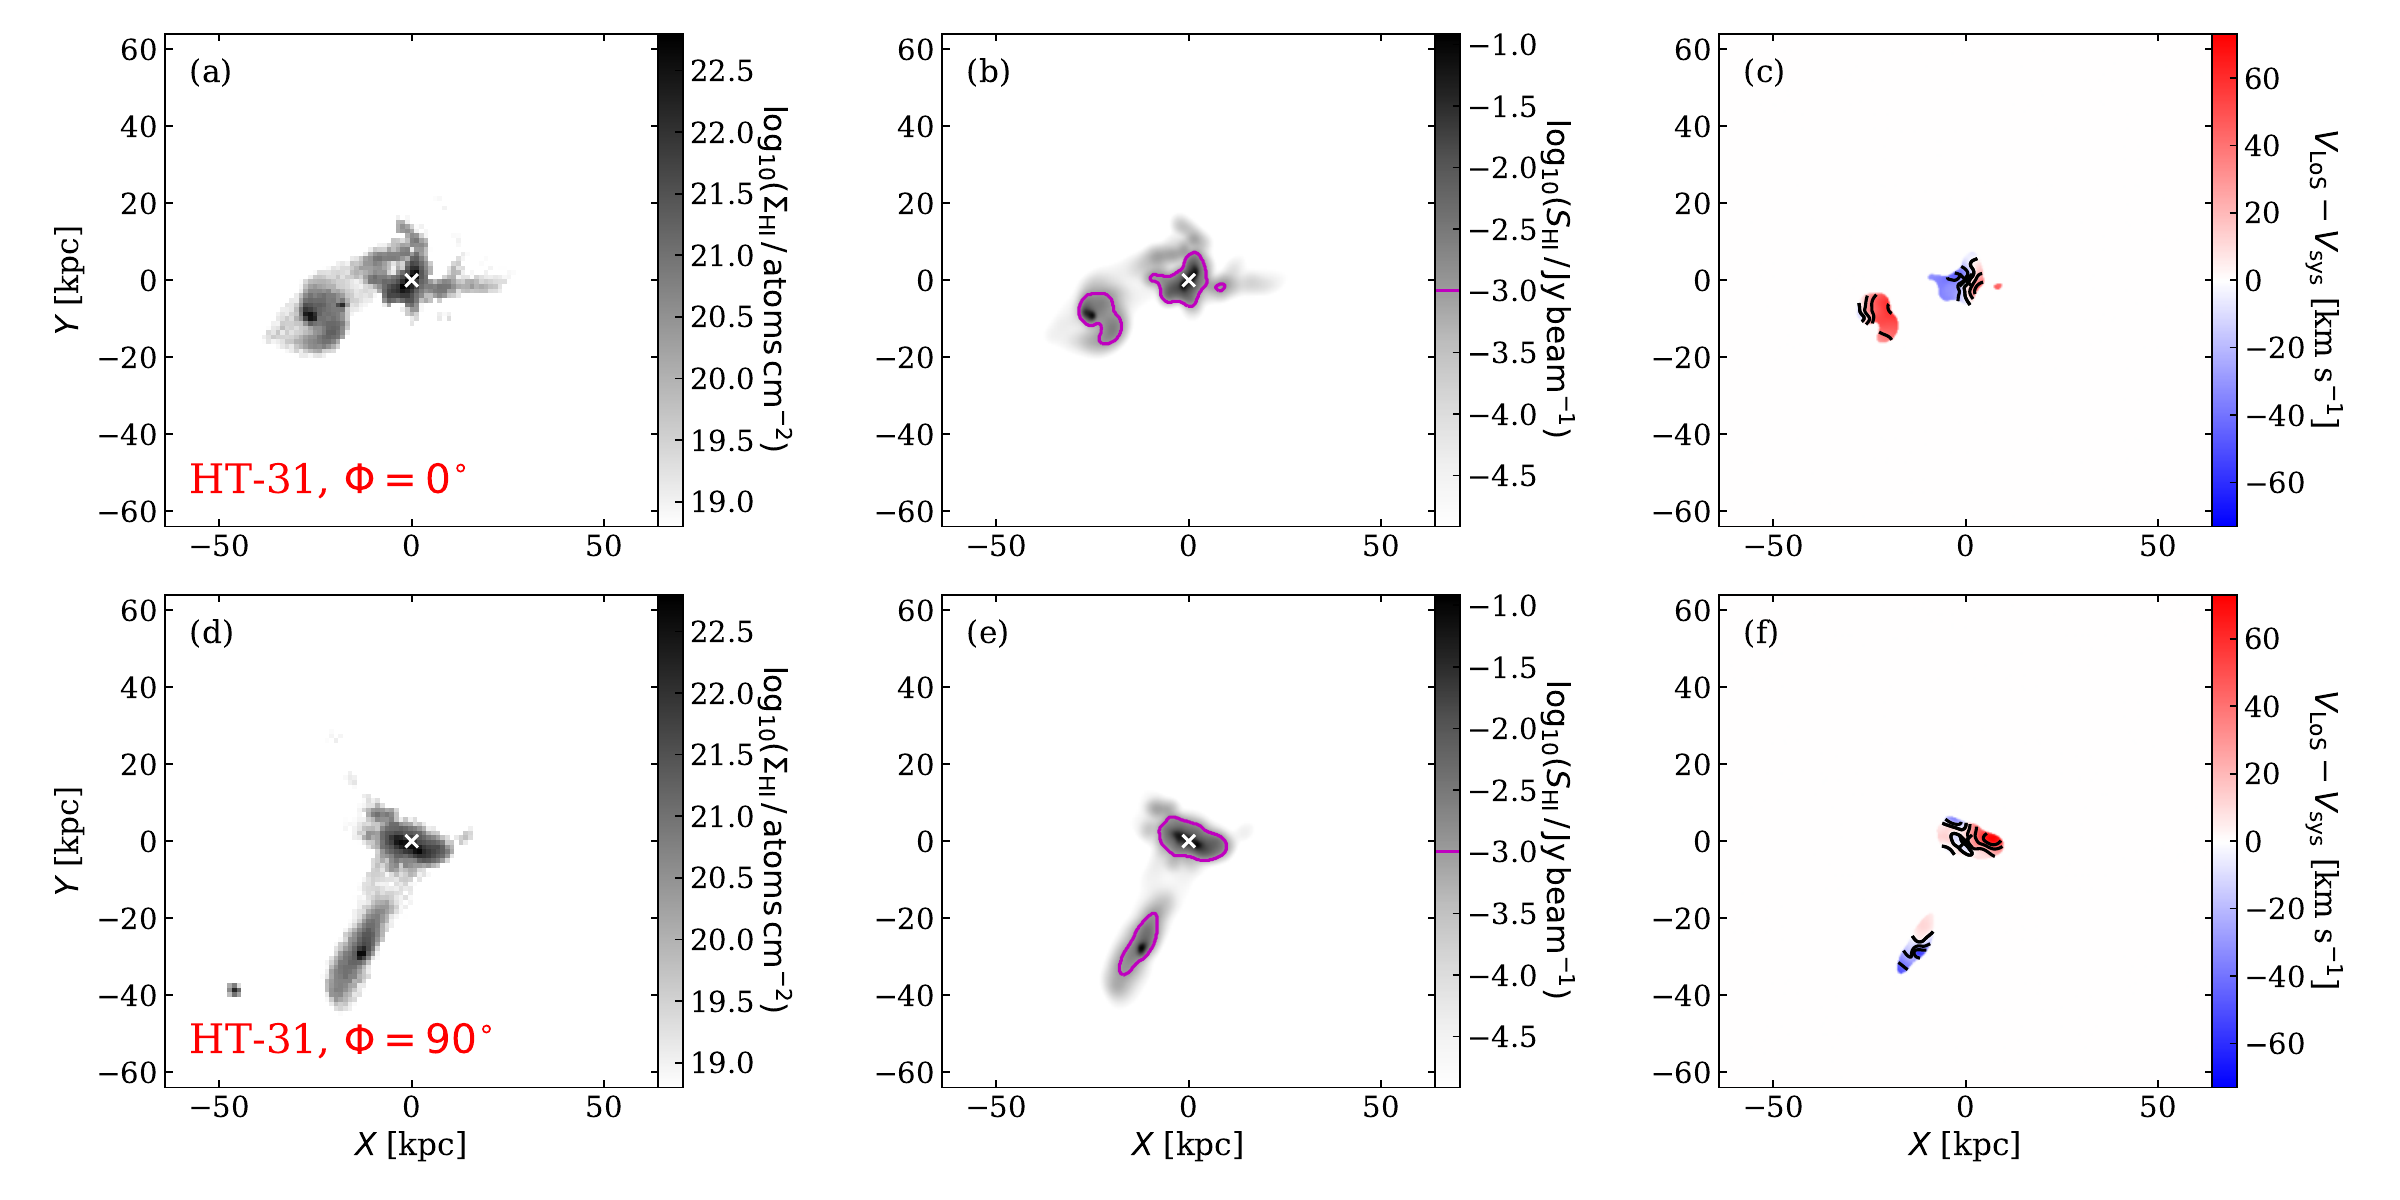}
\includegraphics[width=\textwidth]{../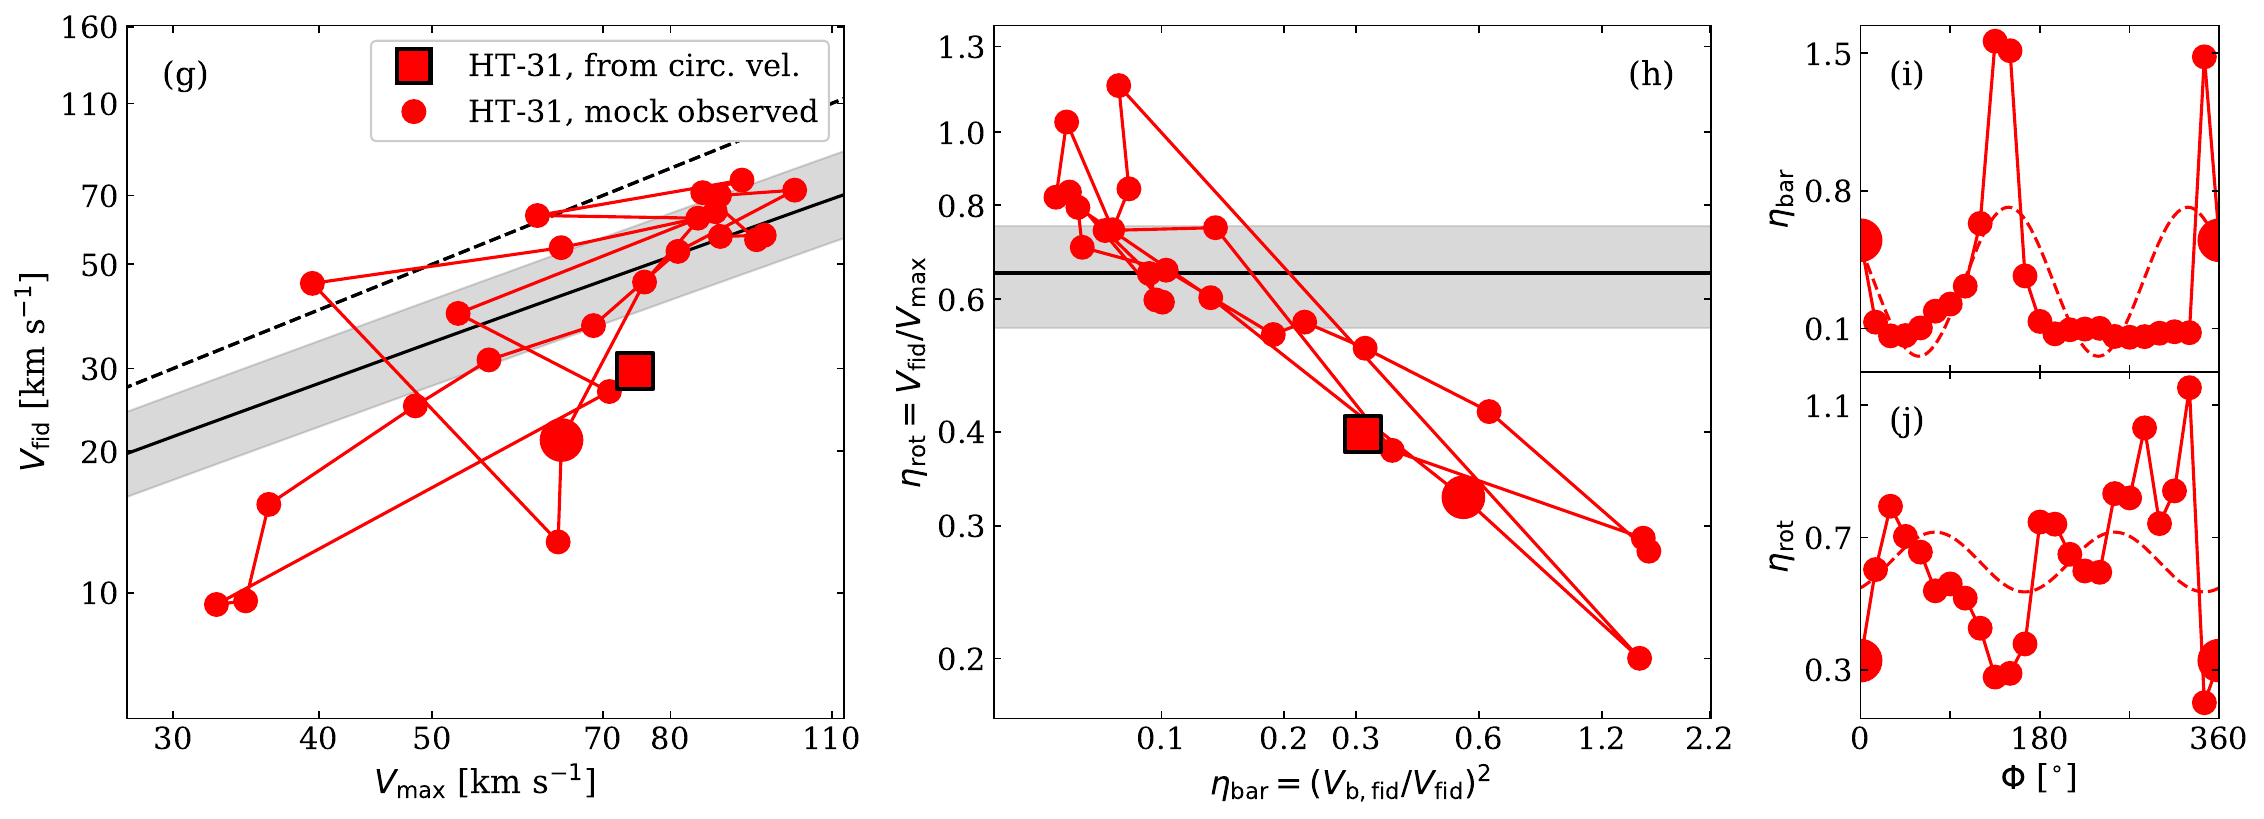}
\end{minipage}
\begin{minipage}{.4\textwidth}
\includegraphics[width=\textwidth]{../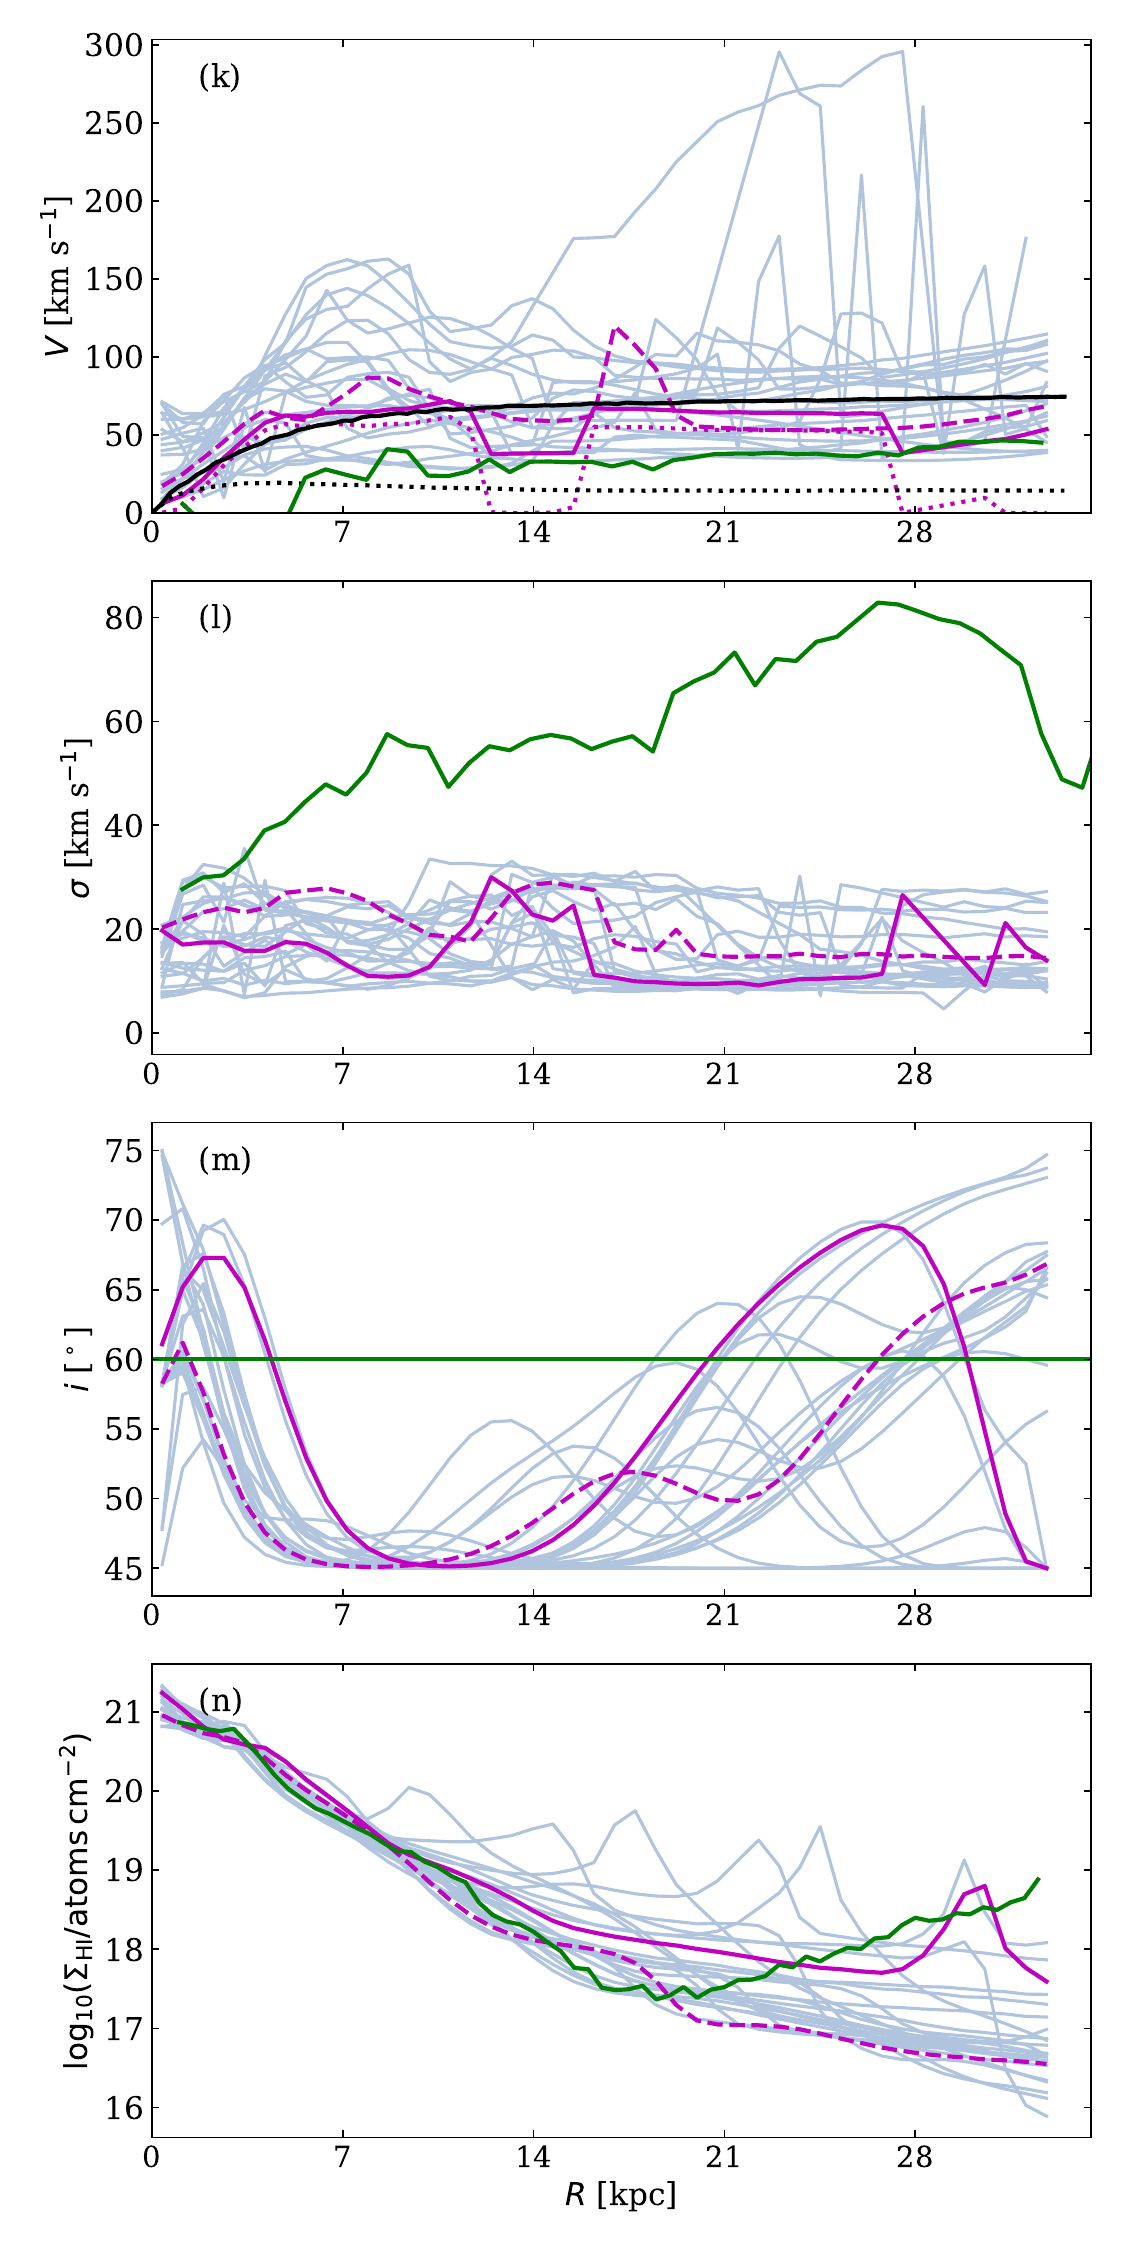}
\end{minipage}
\caption{A set of summary figures for galaxy HT-31, excluded from kinematic analysis. These include example moment maps for two orientations (panels (a)--(f); similar to Fig.~\ref{fig:visualisations}), a summary of the parameters $V_\mathrm{fid}$, $V_\mathrm{max}$, $\eta_\mathrm{rot}$, and $\eta_\mathrm{bar}$ (panels (g)--(j); similar to Fig.~\ref{fig:loops}), and a summary of the rotation curve analysis from $24$ viewing angles (panels (k)--(n); similar to Fig.~\ref{fig:rot_curves}). See description of Appendix~\ref{app:supplementary} for details.}
\label{fig:S73}
\end{figure}
\clearpage

\begin{figure}
\begin{minipage}{.9\textwidth}
\includegraphics[width=\textwidth]{../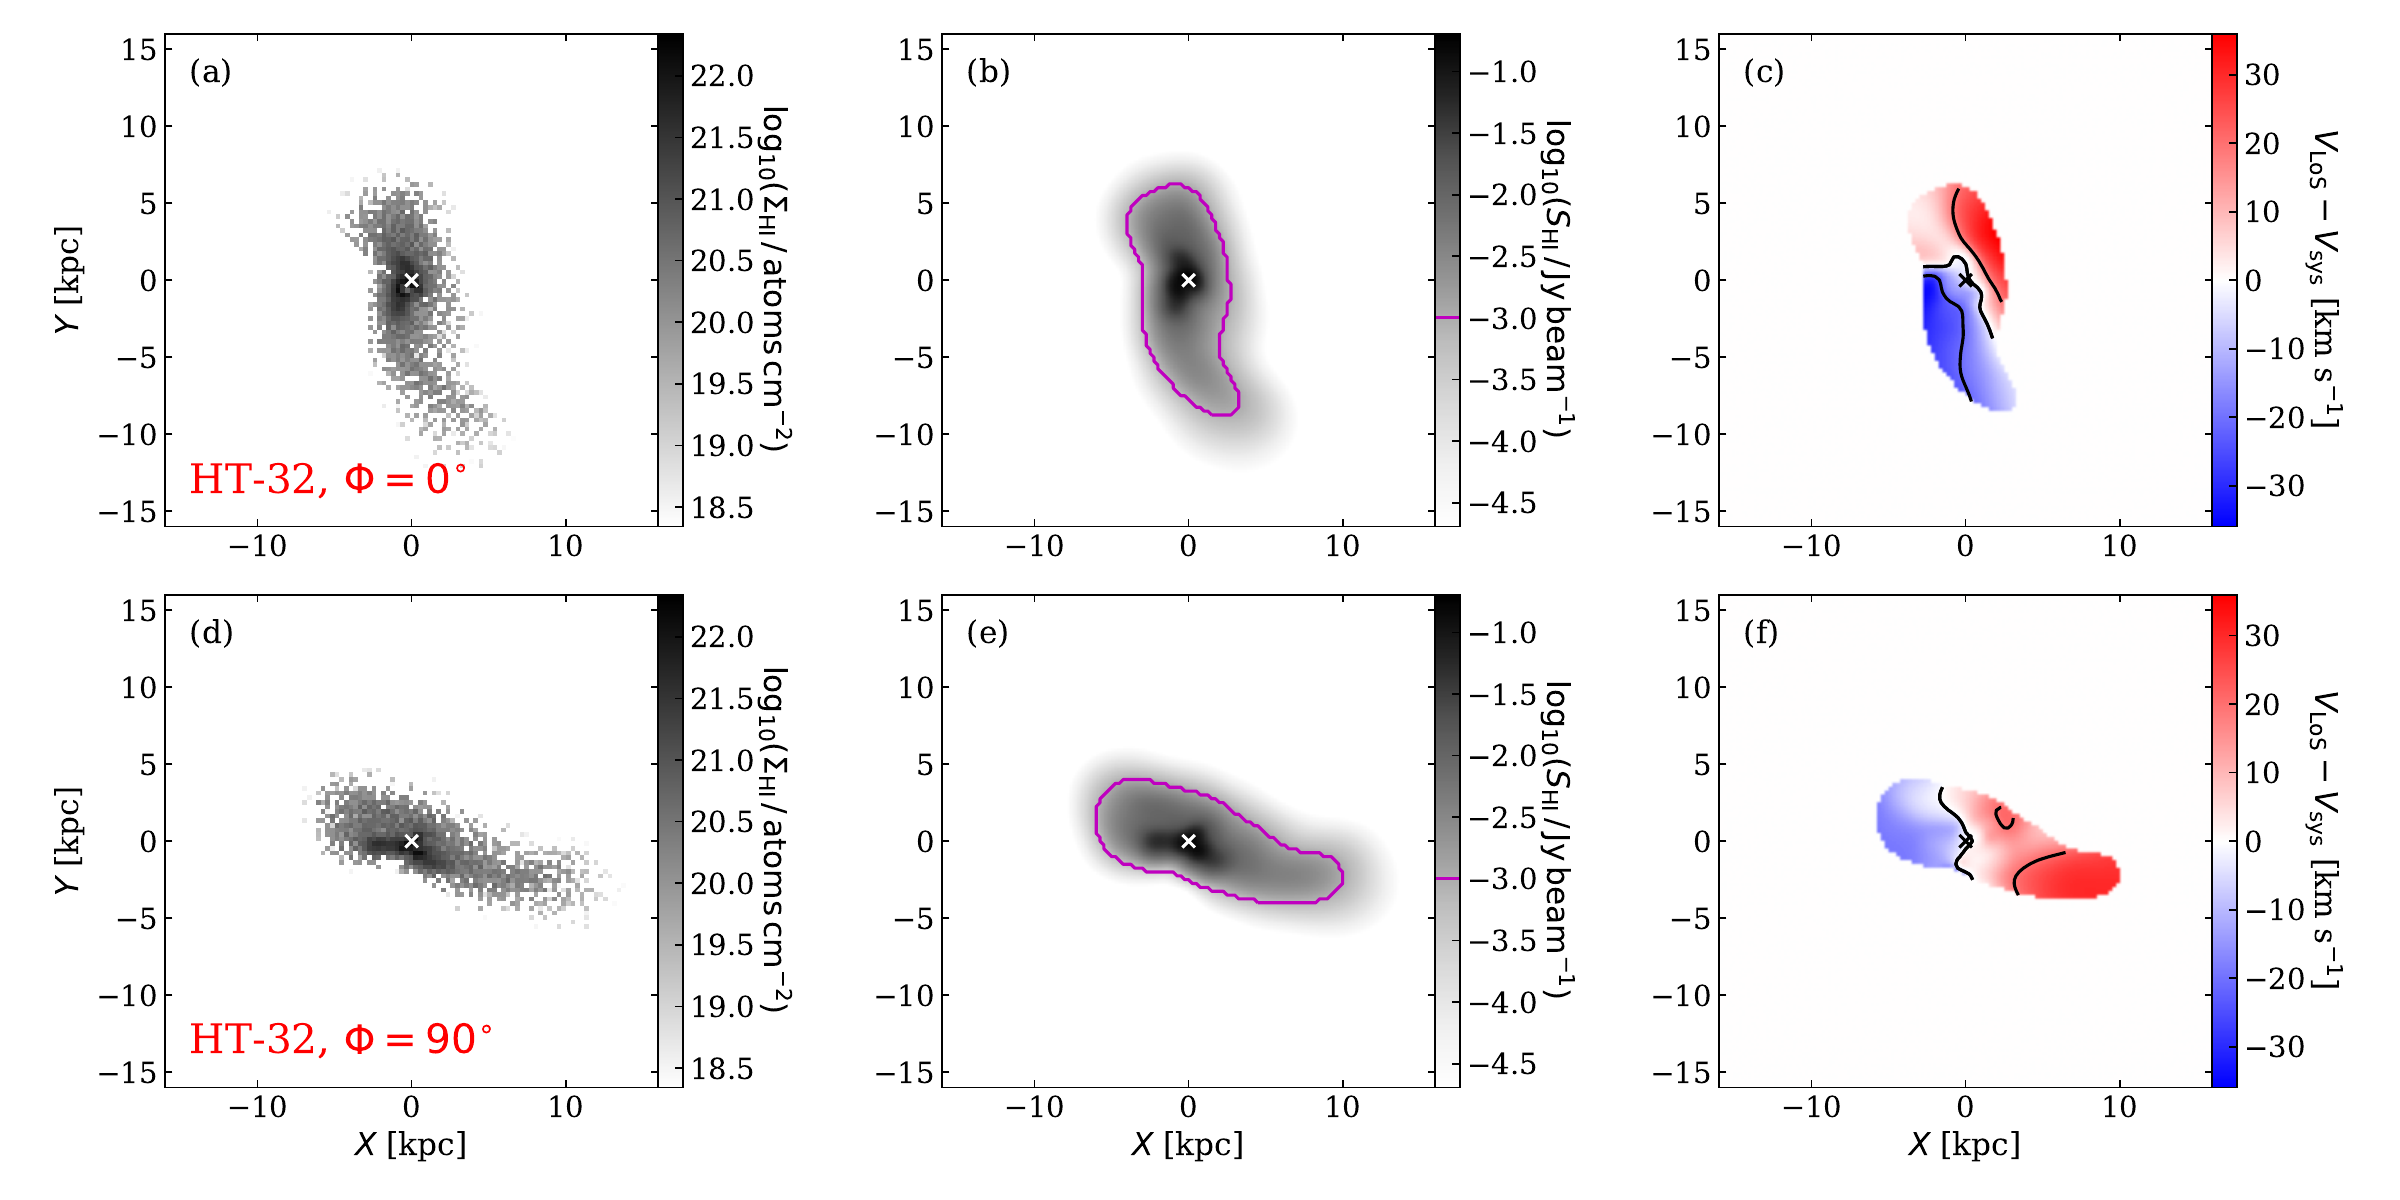}
\includegraphics[width=\textwidth]{../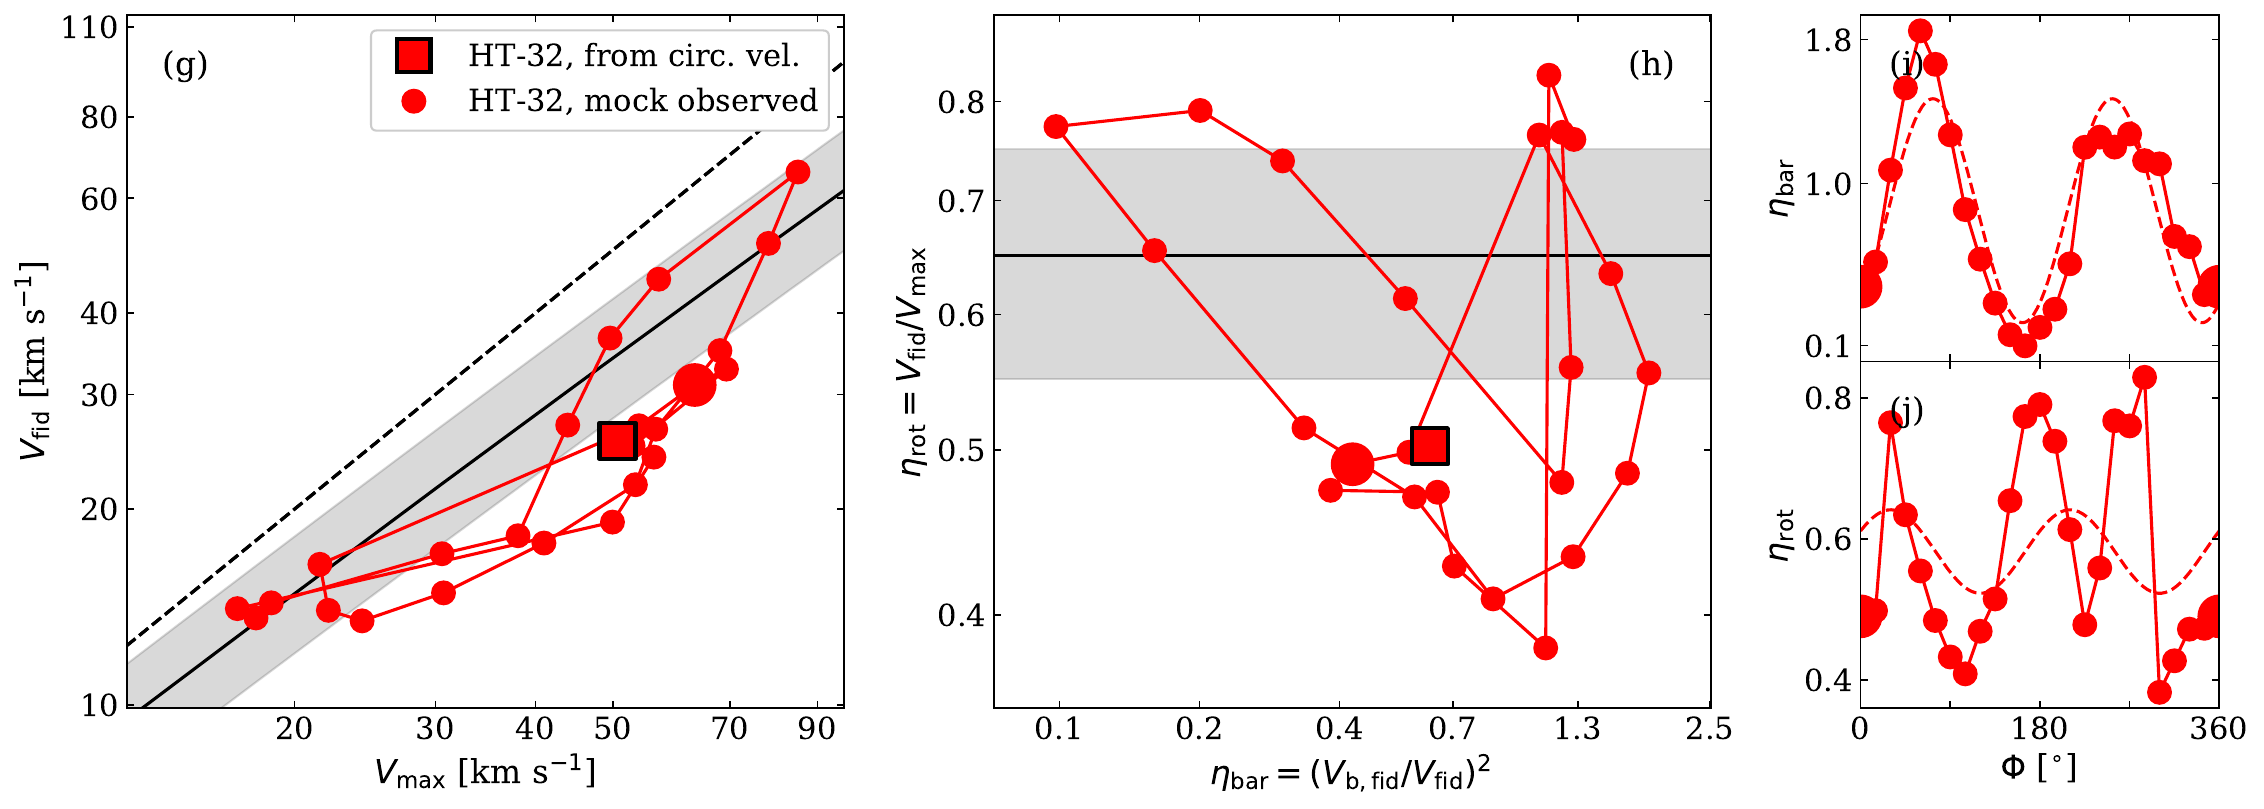}
\end{minipage}
\begin{minipage}{.4\textwidth}
\includegraphics[width=\textwidth]{../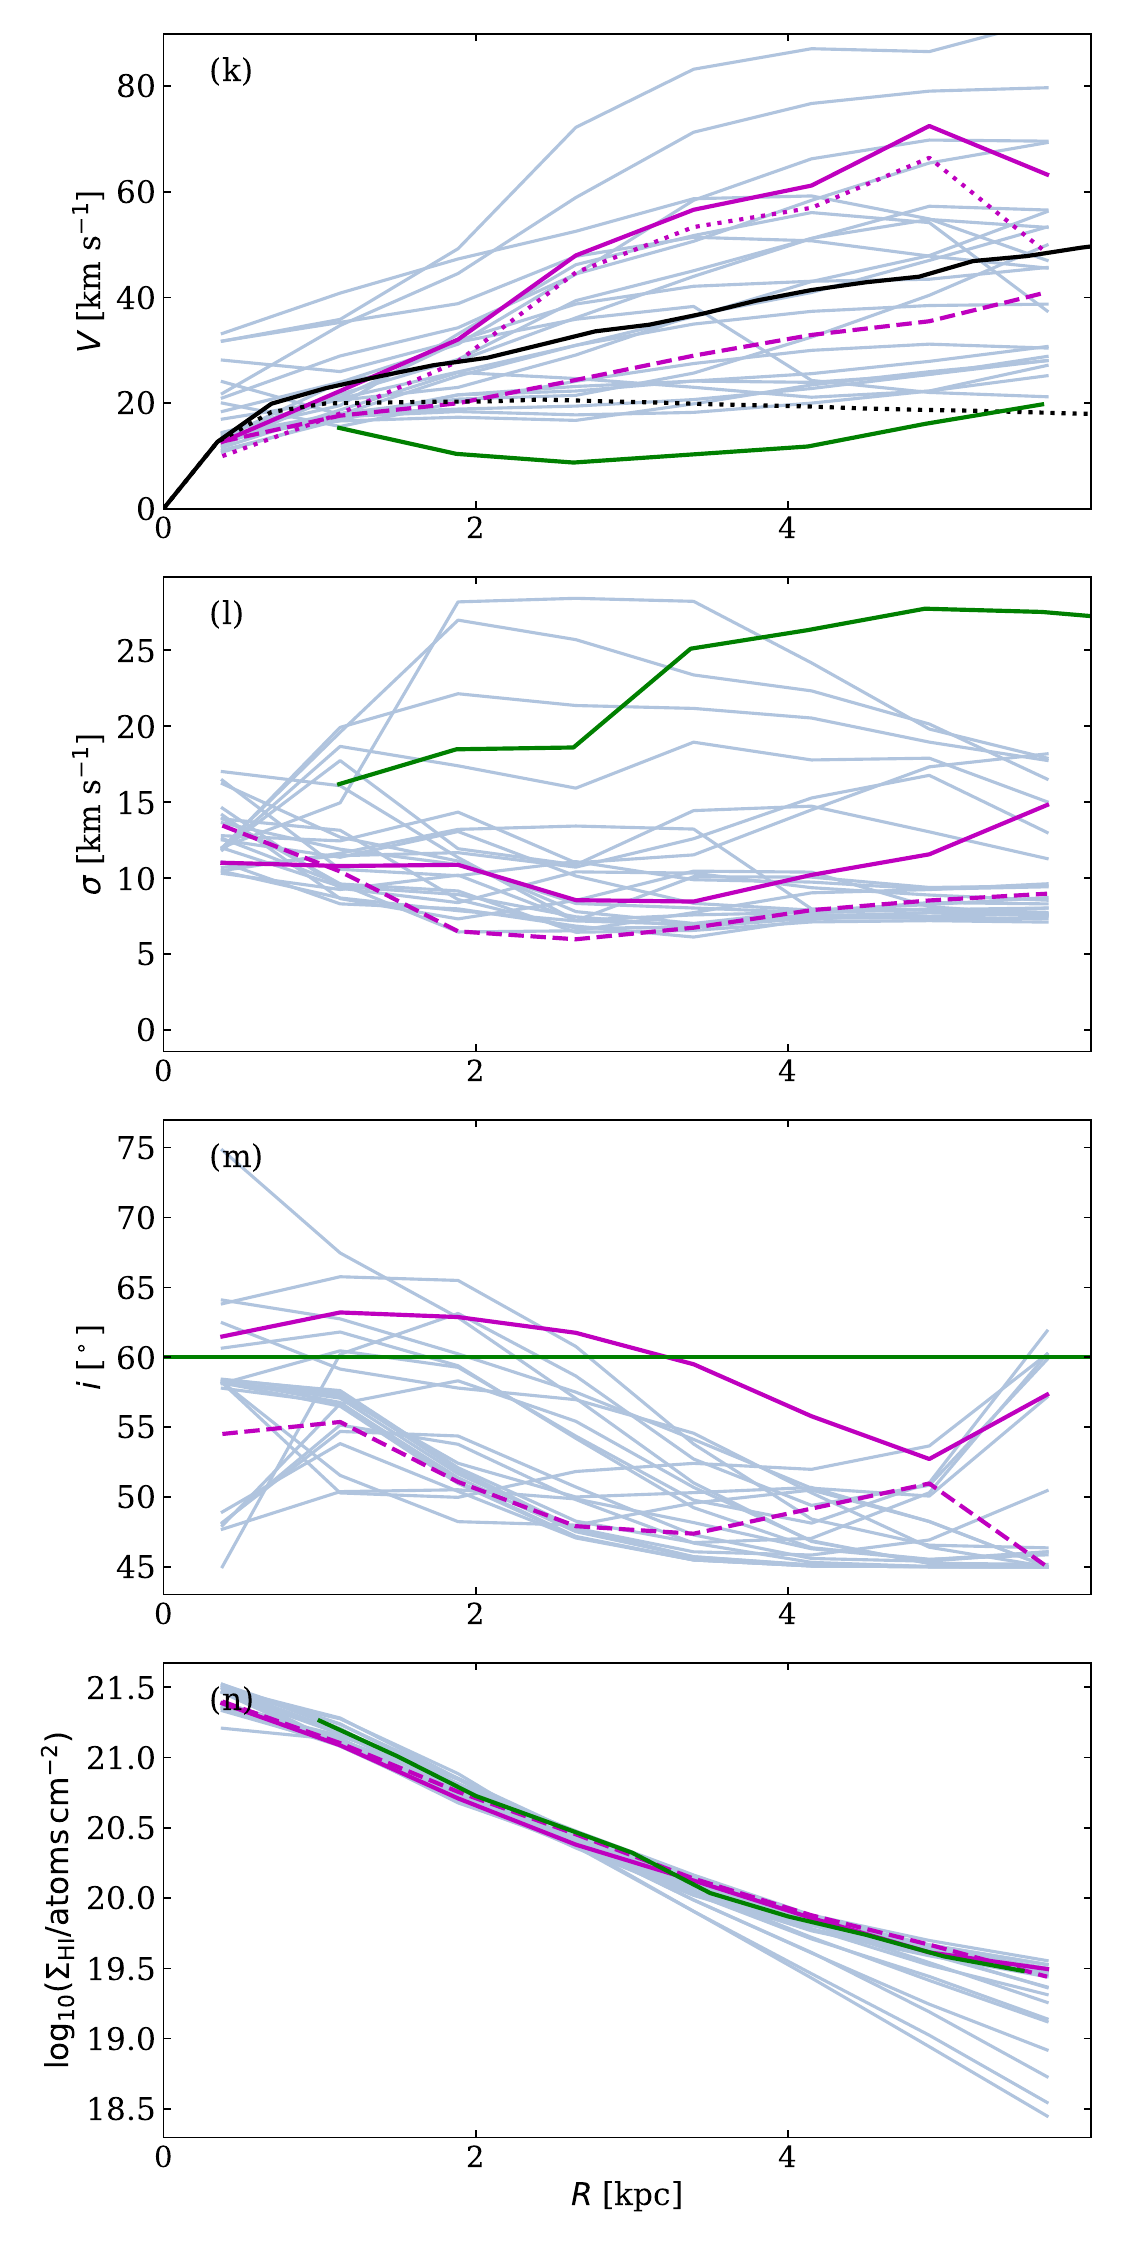}
\end{minipage}
\caption{A set of summary figures for galaxy HT-32, excluded from kinematic analysis. These include example moment maps for two orientations (panels (a)--(f); similar to Fig.~\ref{fig:visualisations}), a summary of the parameters $V_\mathrm{fid}$, $V_\mathrm{max}$, $\eta_\mathrm{rot}$, and $\eta_\mathrm{bar}$ (panels (g)--(j); similar to Fig.~\ref{fig:loops}), and a summary of the rotation curve analysis from $24$ viewing angles (panels (k)--(n); similar to Fig.~\ref{fig:rot_curves}). See description of Appendix~\ref{app:supplementary} for details.}
\label{fig:S74}
\end{figure}
\clearpage

\begin{figure}
\begin{minipage}{.9\textwidth}
\includegraphics[width=\textwidth]{../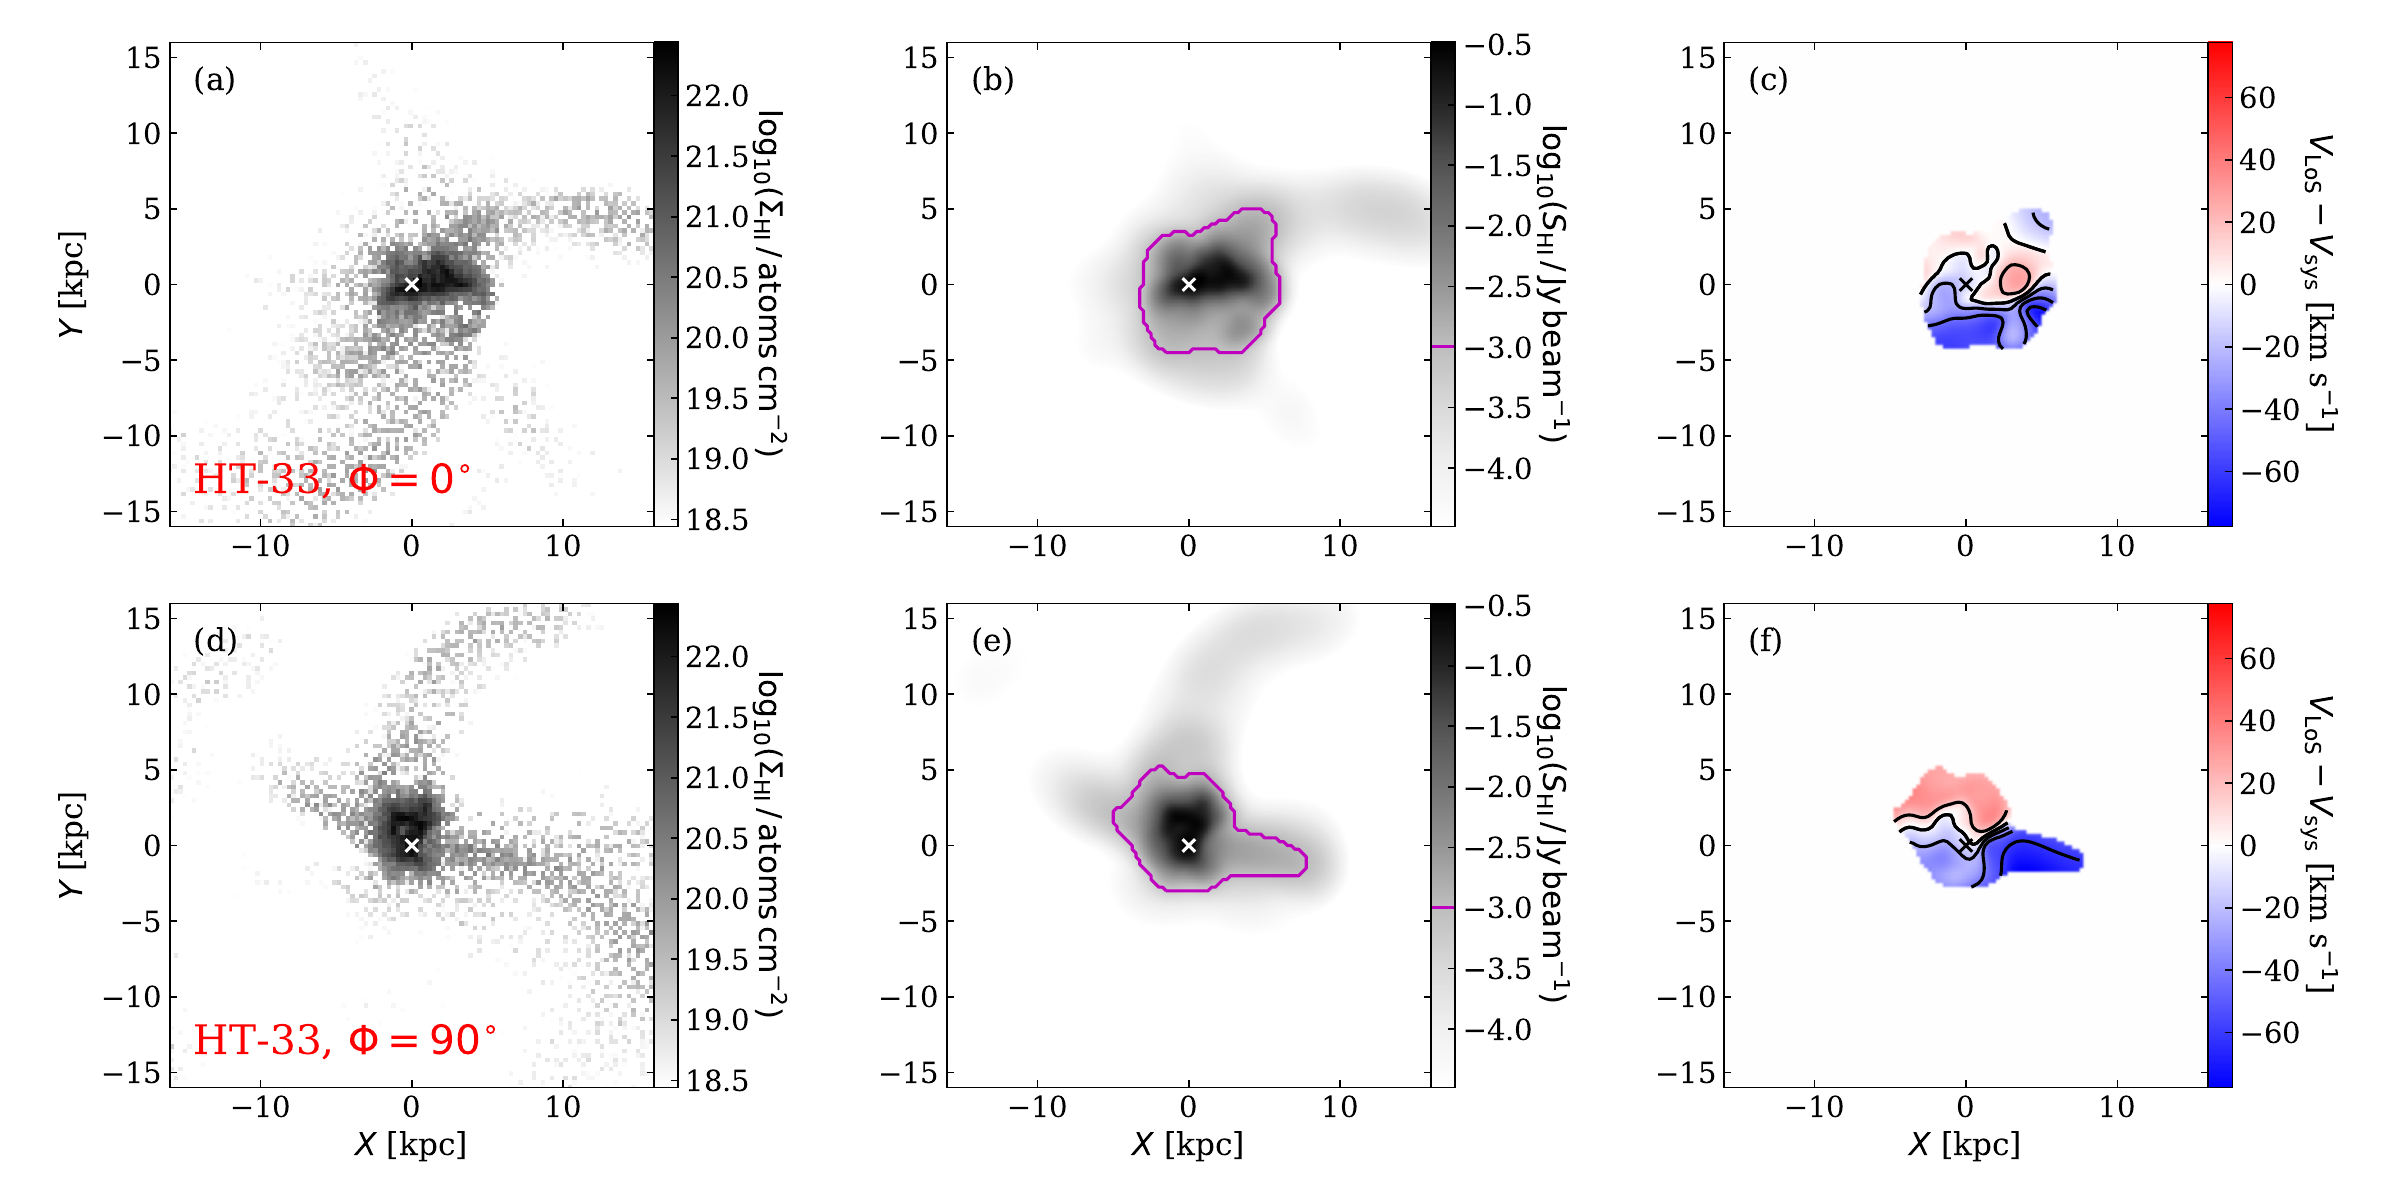}
\includegraphics[width=\textwidth]{../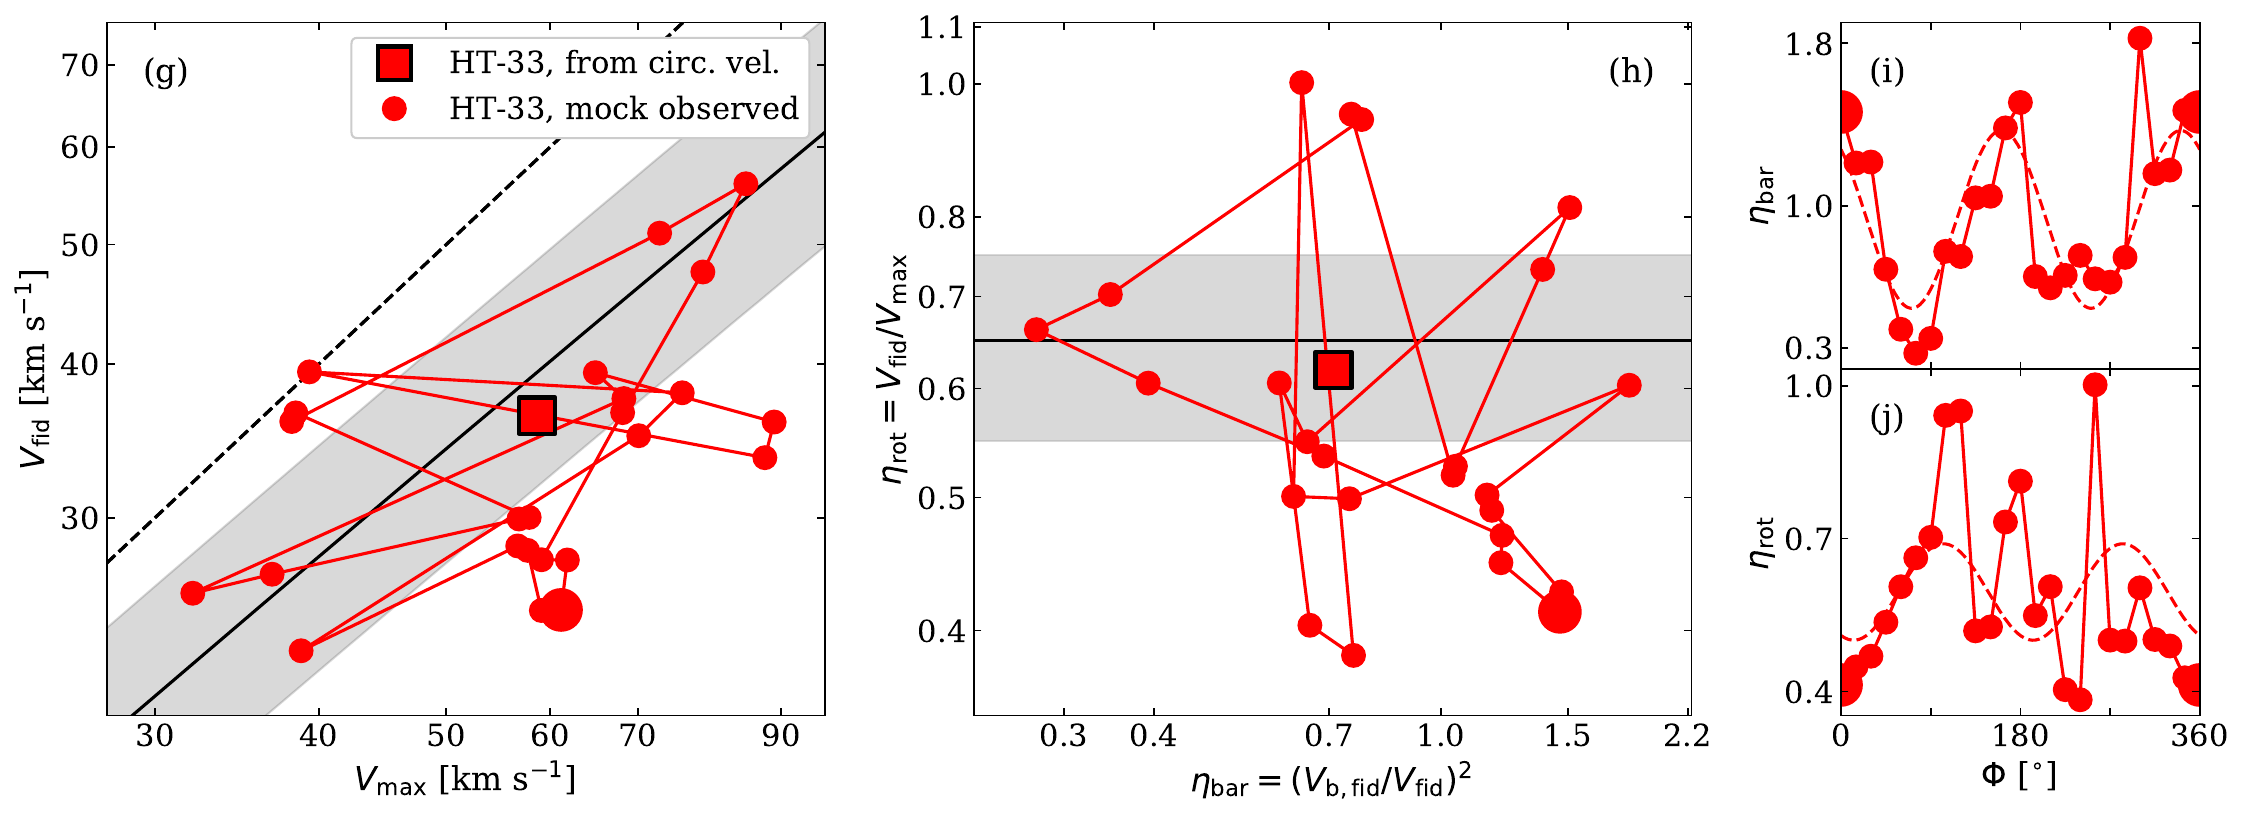}
\end{minipage}
\begin{minipage}{.4\textwidth}
\includegraphics[width=\textwidth]{../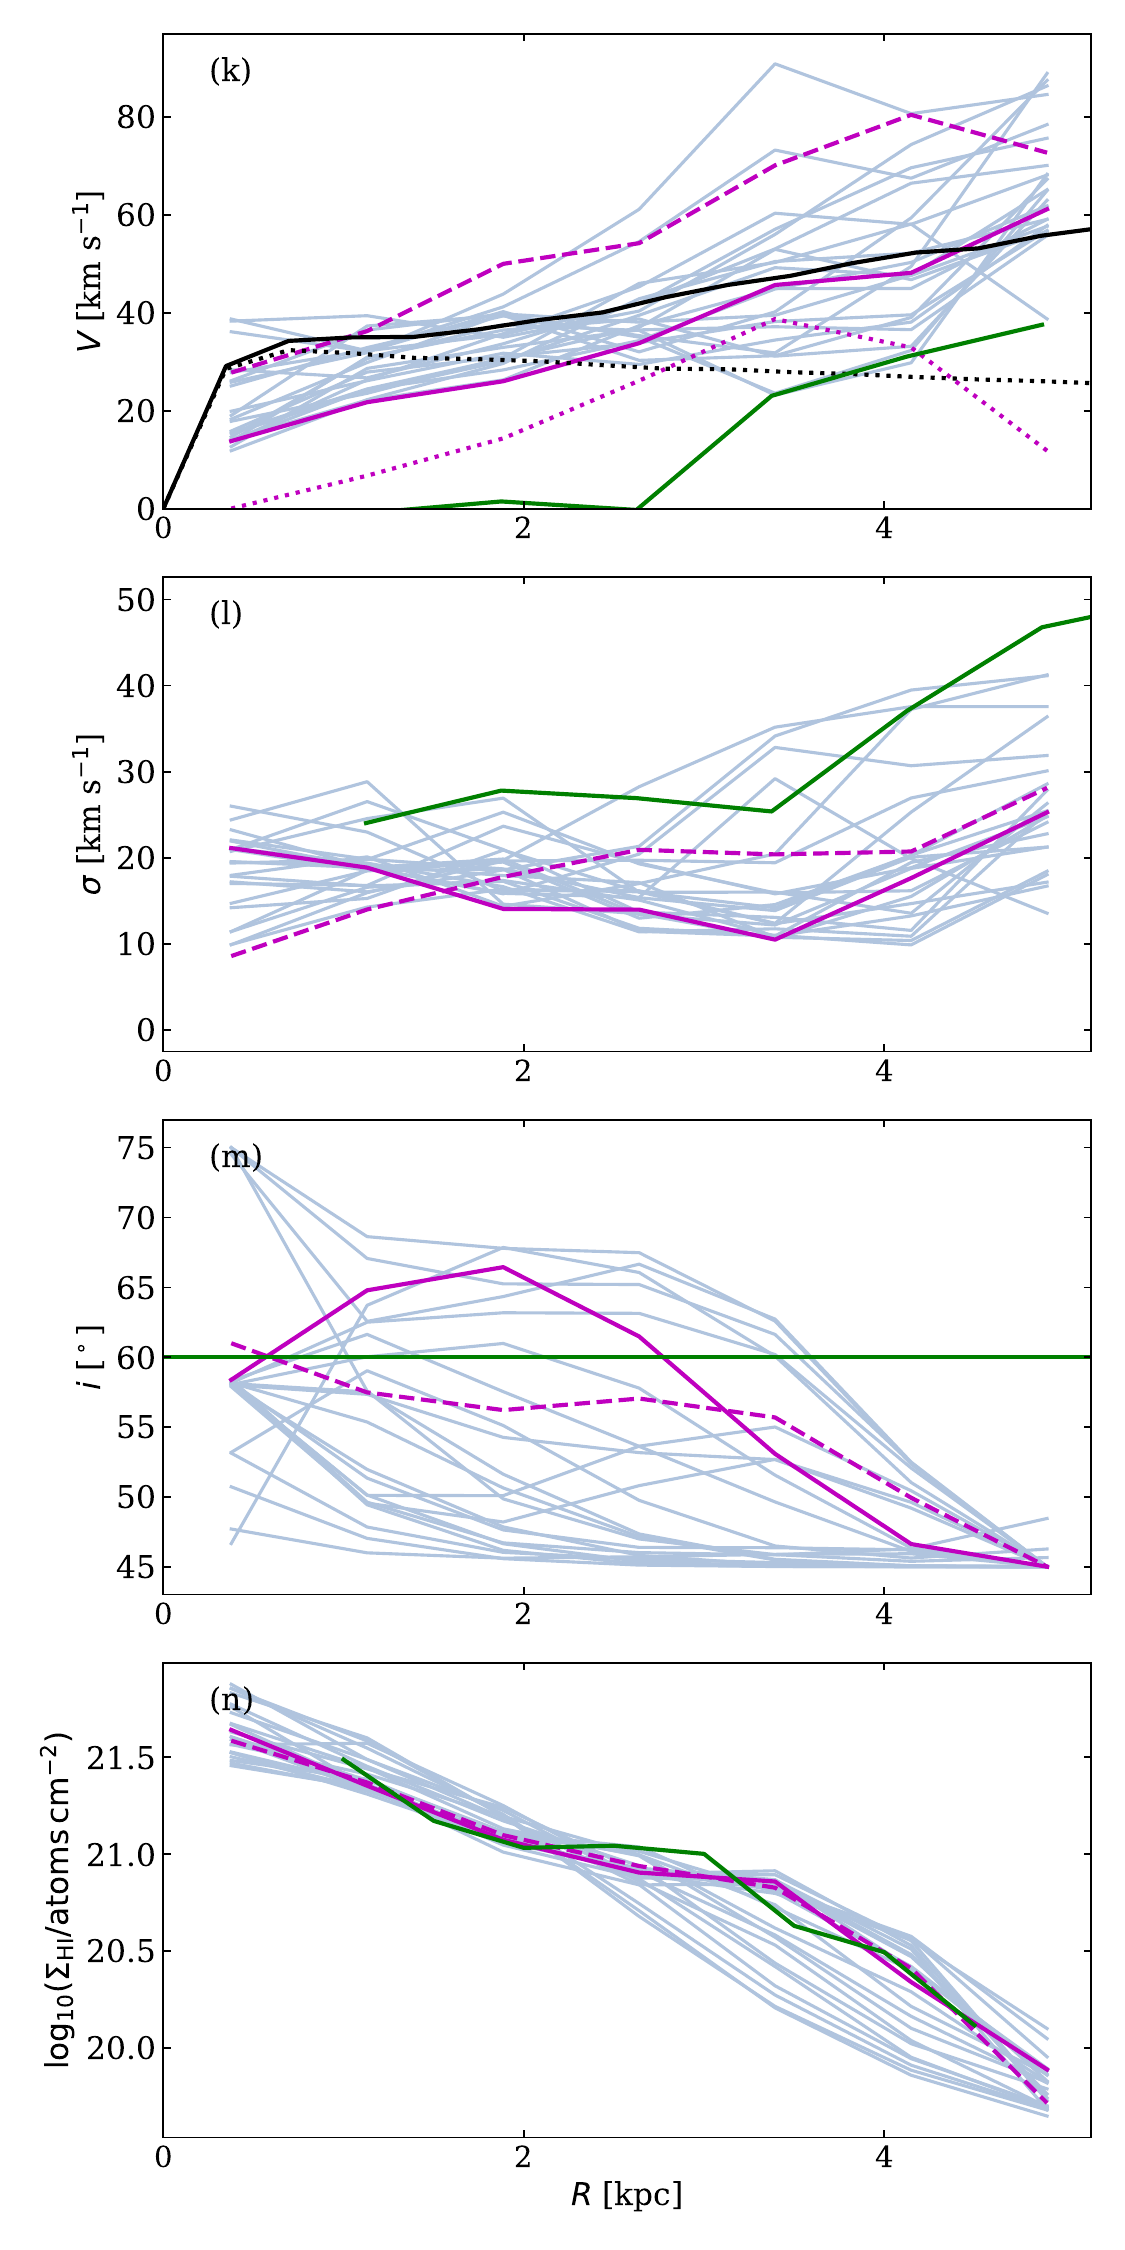}
\end{minipage}
\caption{A set of summary figures for galaxy HT-33, excluded from kinematic analysis. These include example moment maps for two orientations (panels (a)--(f); similar to Fig.~\ref{fig:visualisations}), a summary of the parameters $V_\mathrm{fid}$, $V_\mathrm{max}$, $\eta_\mathrm{rot}$, and $\eta_\mathrm{bar}$ (panels (g)--(j); similar to Fig.~\ref{fig:loops}), and a summary of the rotation curve analysis from $24$ viewing angles (panels (k)--(n); similar to Fig.~\ref{fig:rot_curves}). See description of Appendix~\ref{app:supplementary} for details.}
\label{fig:S75}
\end{figure}
\clearpage

\begin{figure}
\begin{minipage}{.9\textwidth}
\includegraphics[width=\textwidth]{../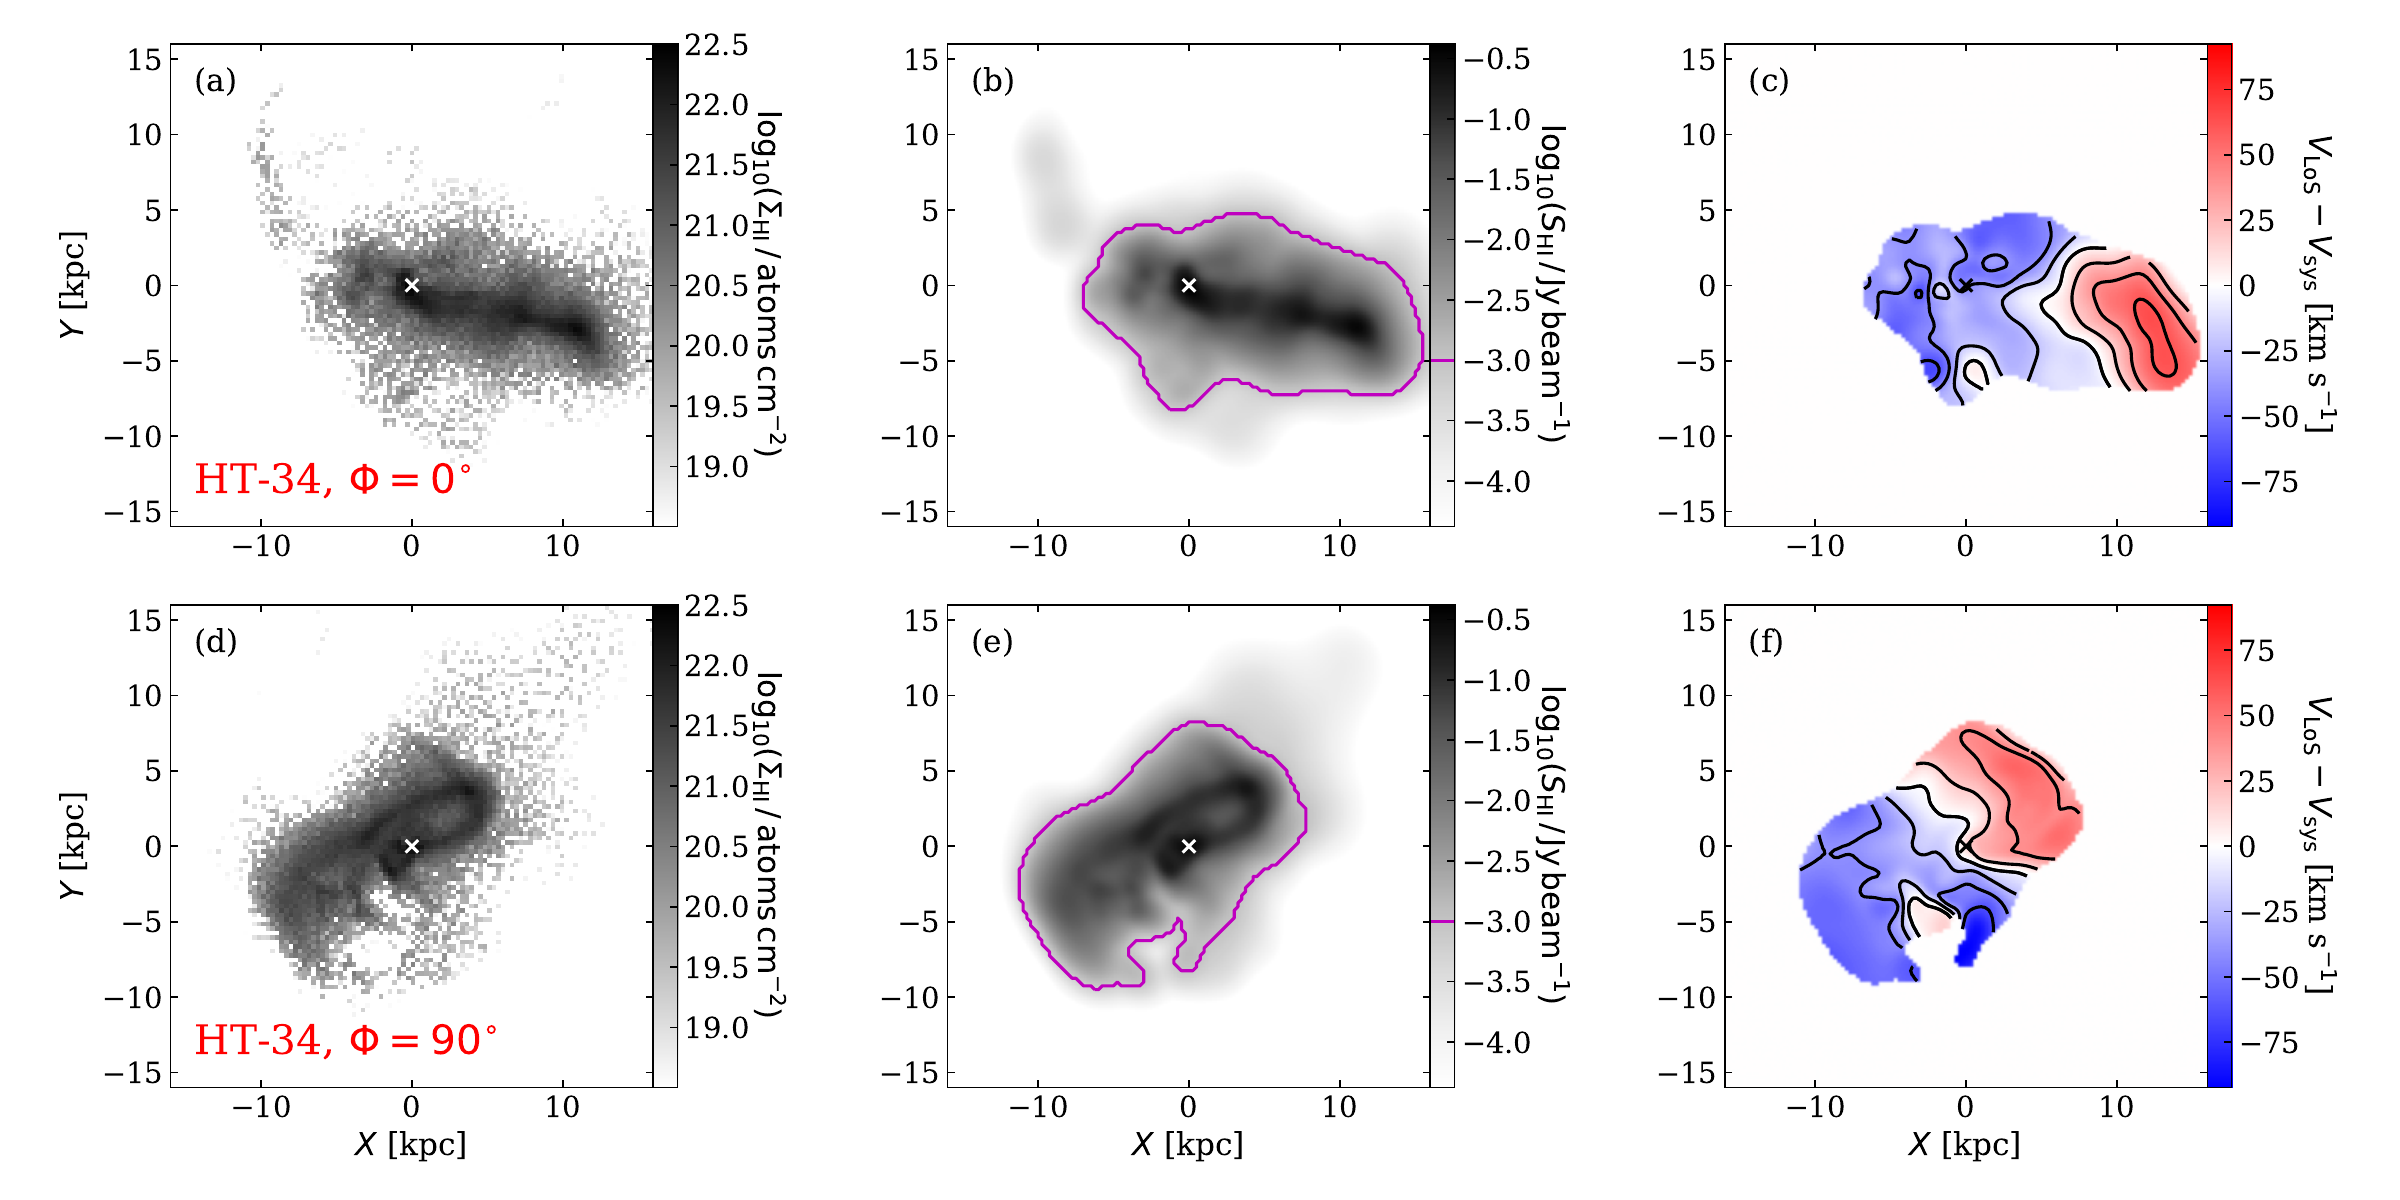}
\includegraphics[width=\textwidth]{../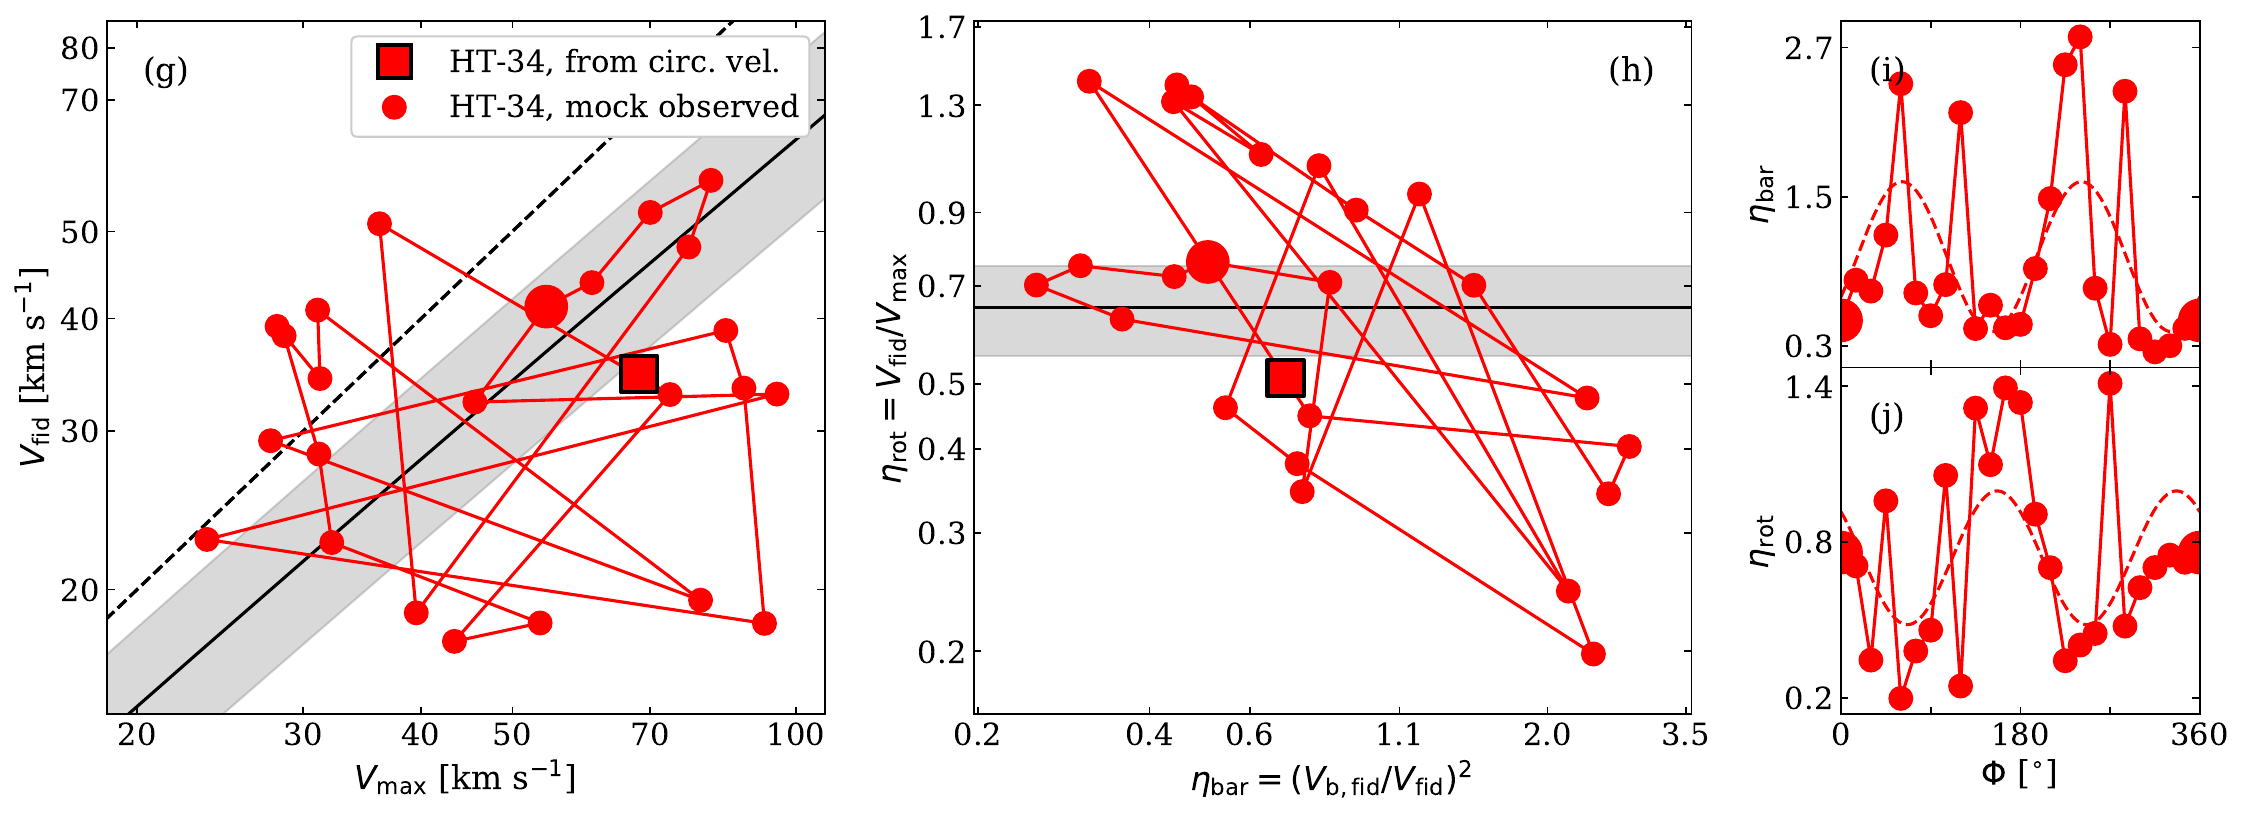}
\end{minipage}
\begin{minipage}{.4\textwidth}
\includegraphics[width=\textwidth]{../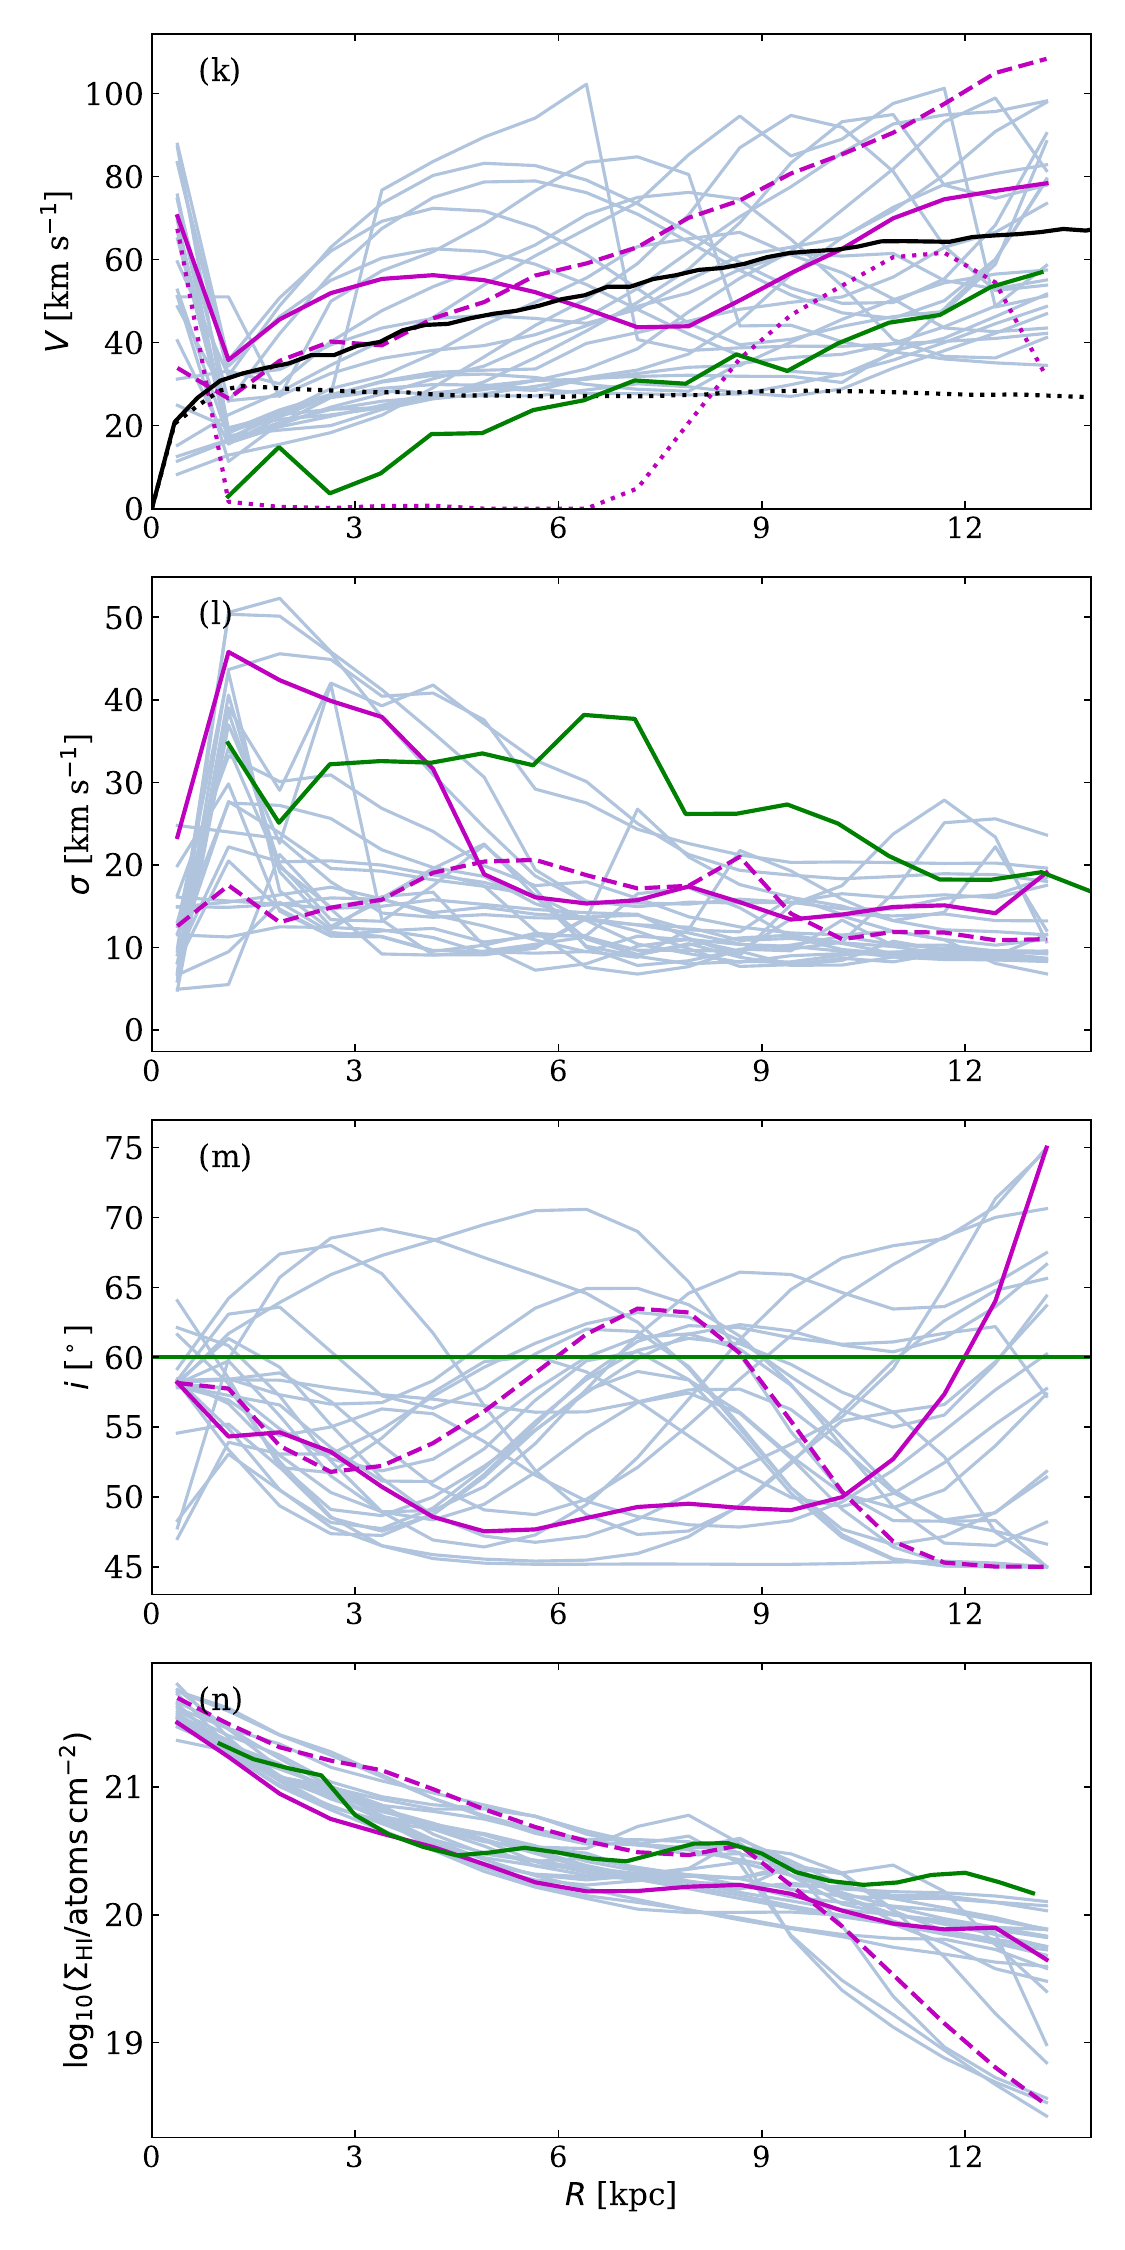}
\end{minipage}
\caption{A set of summary figures for galaxy HT-34, excluded from kinematic analysis. These include example moment maps for two orientations (panels (a)--(f); similar to Fig.~\ref{fig:visualisations}), a summary of the parameters $V_\mathrm{fid}$, $V_\mathrm{max}$, $\eta_\mathrm{rot}$, and $\eta_\mathrm{bar}$ (panels (g)--(j); similar to Fig.~\ref{fig:loops}), and a summary of the rotation curve analysis from $24$ viewing angles (panels (k)--(n); similar to Fig.~\ref{fig:rot_curves}). See description of Appendix~\ref{app:supplementary} for details.}
\label{fig:S76}
\end{figure}
\clearpage

\begin{figure}
\begin{minipage}{.9\textwidth}
\includegraphics[width=\textwidth]{../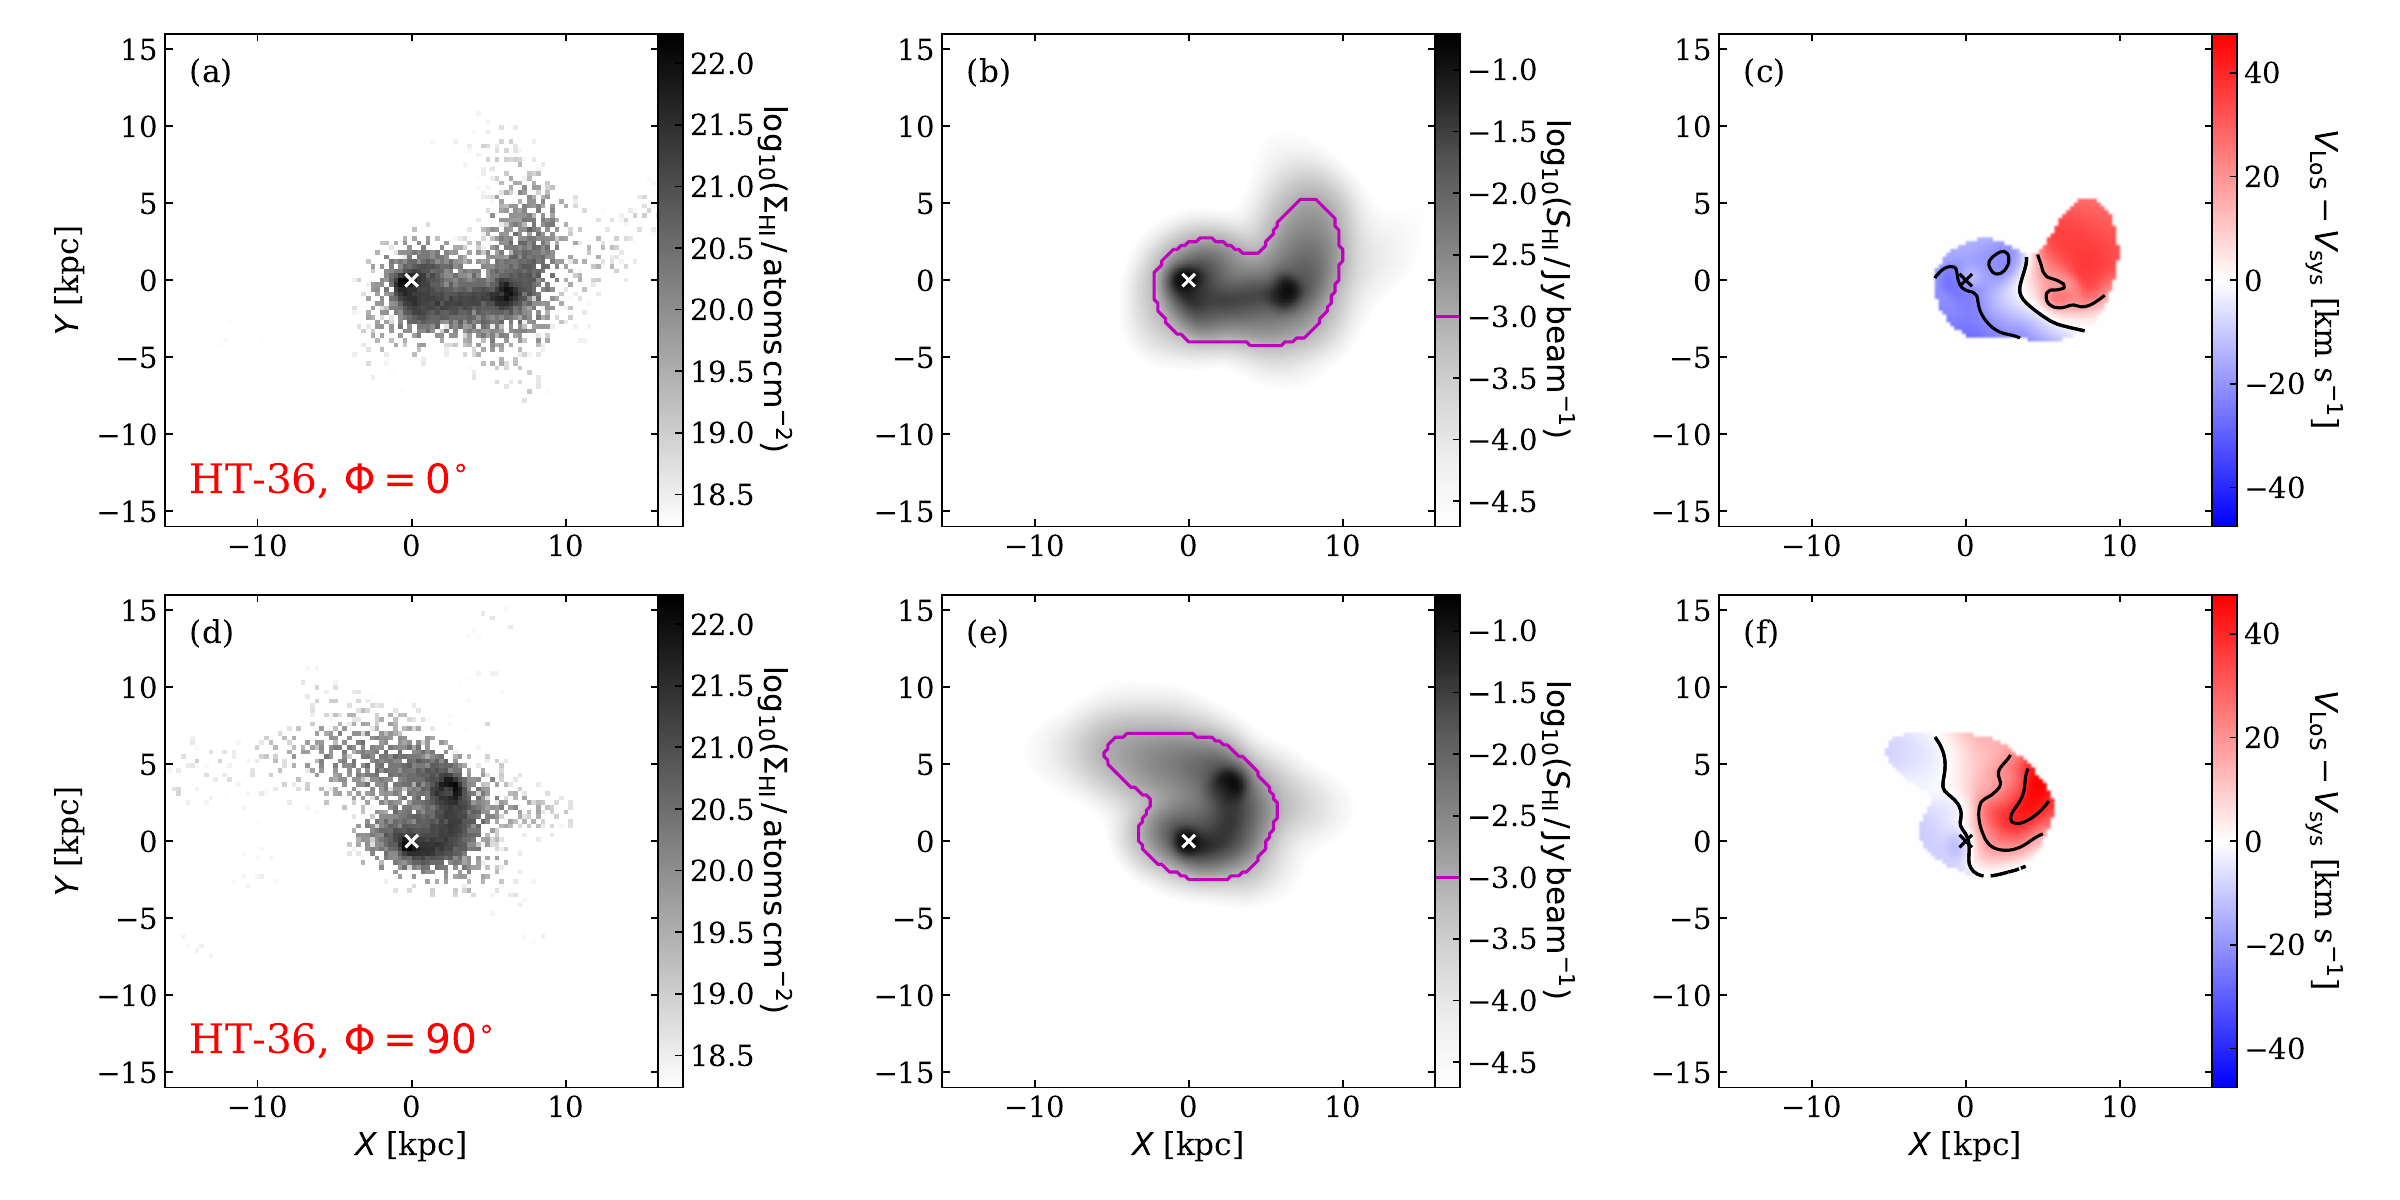}
\includegraphics[width=\textwidth]{../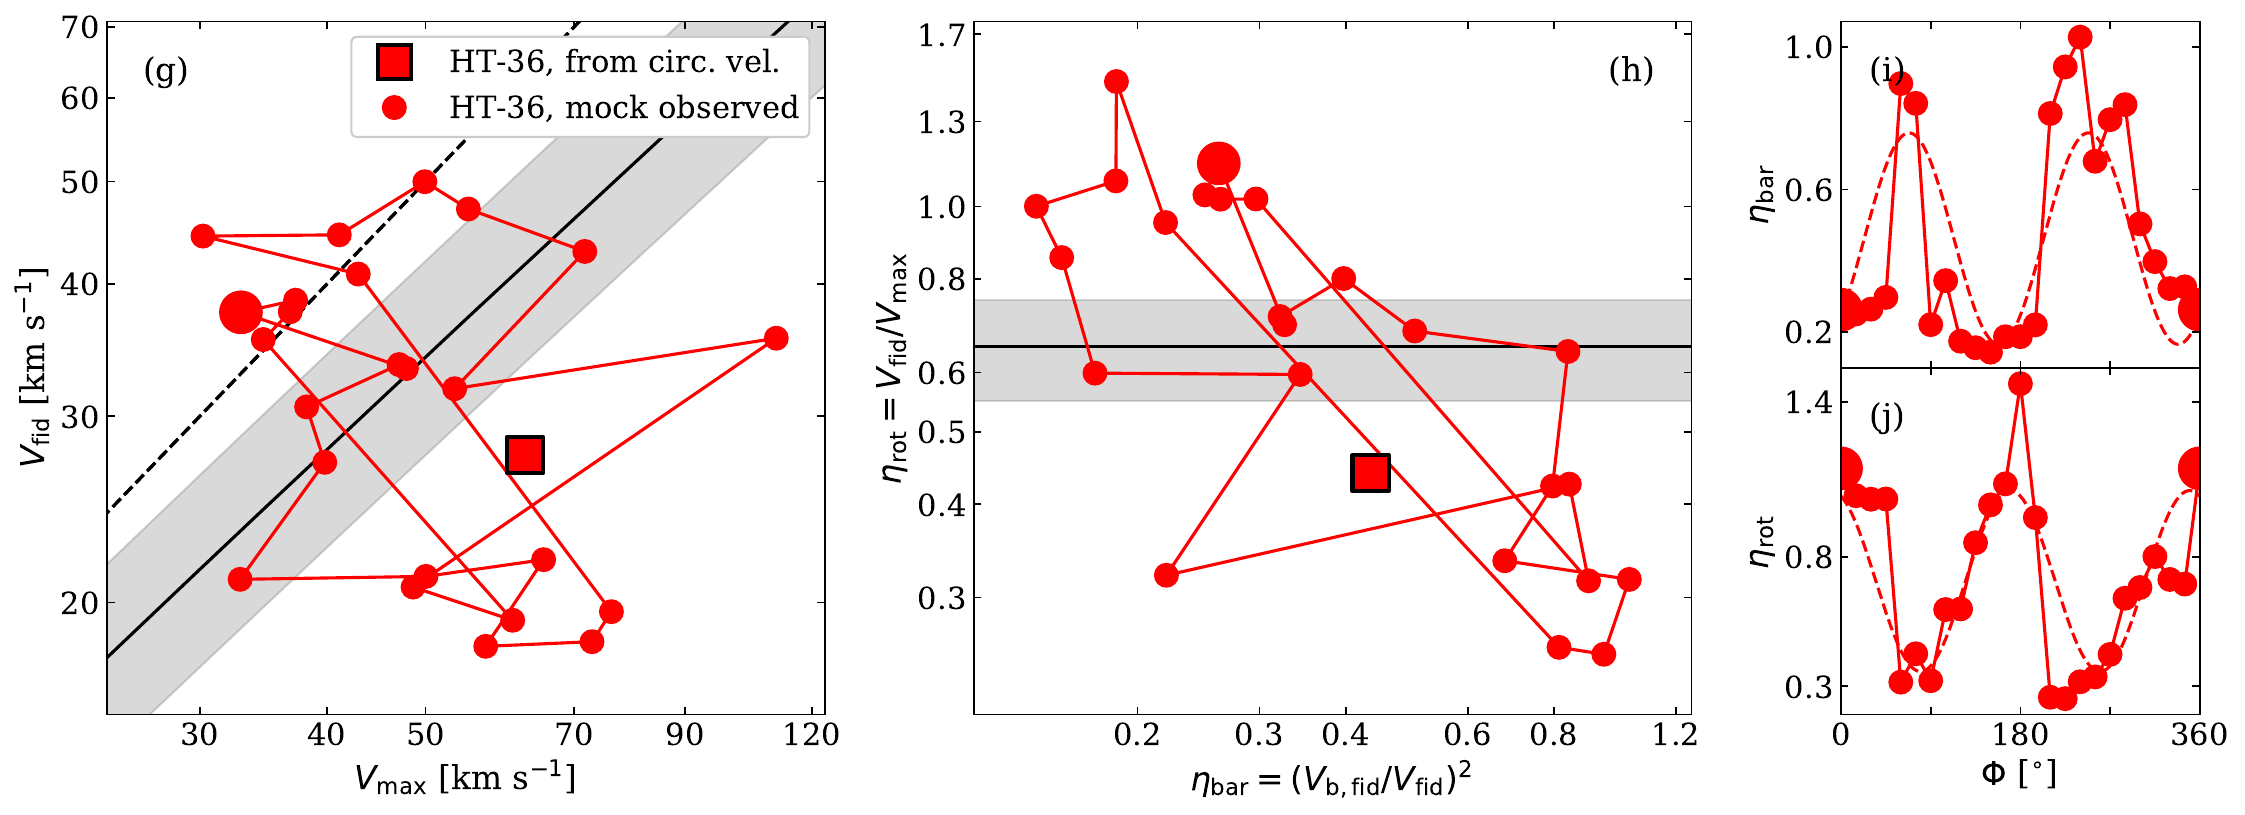}
\end{minipage}
\begin{minipage}{.4\textwidth}
\includegraphics[width=\textwidth]{../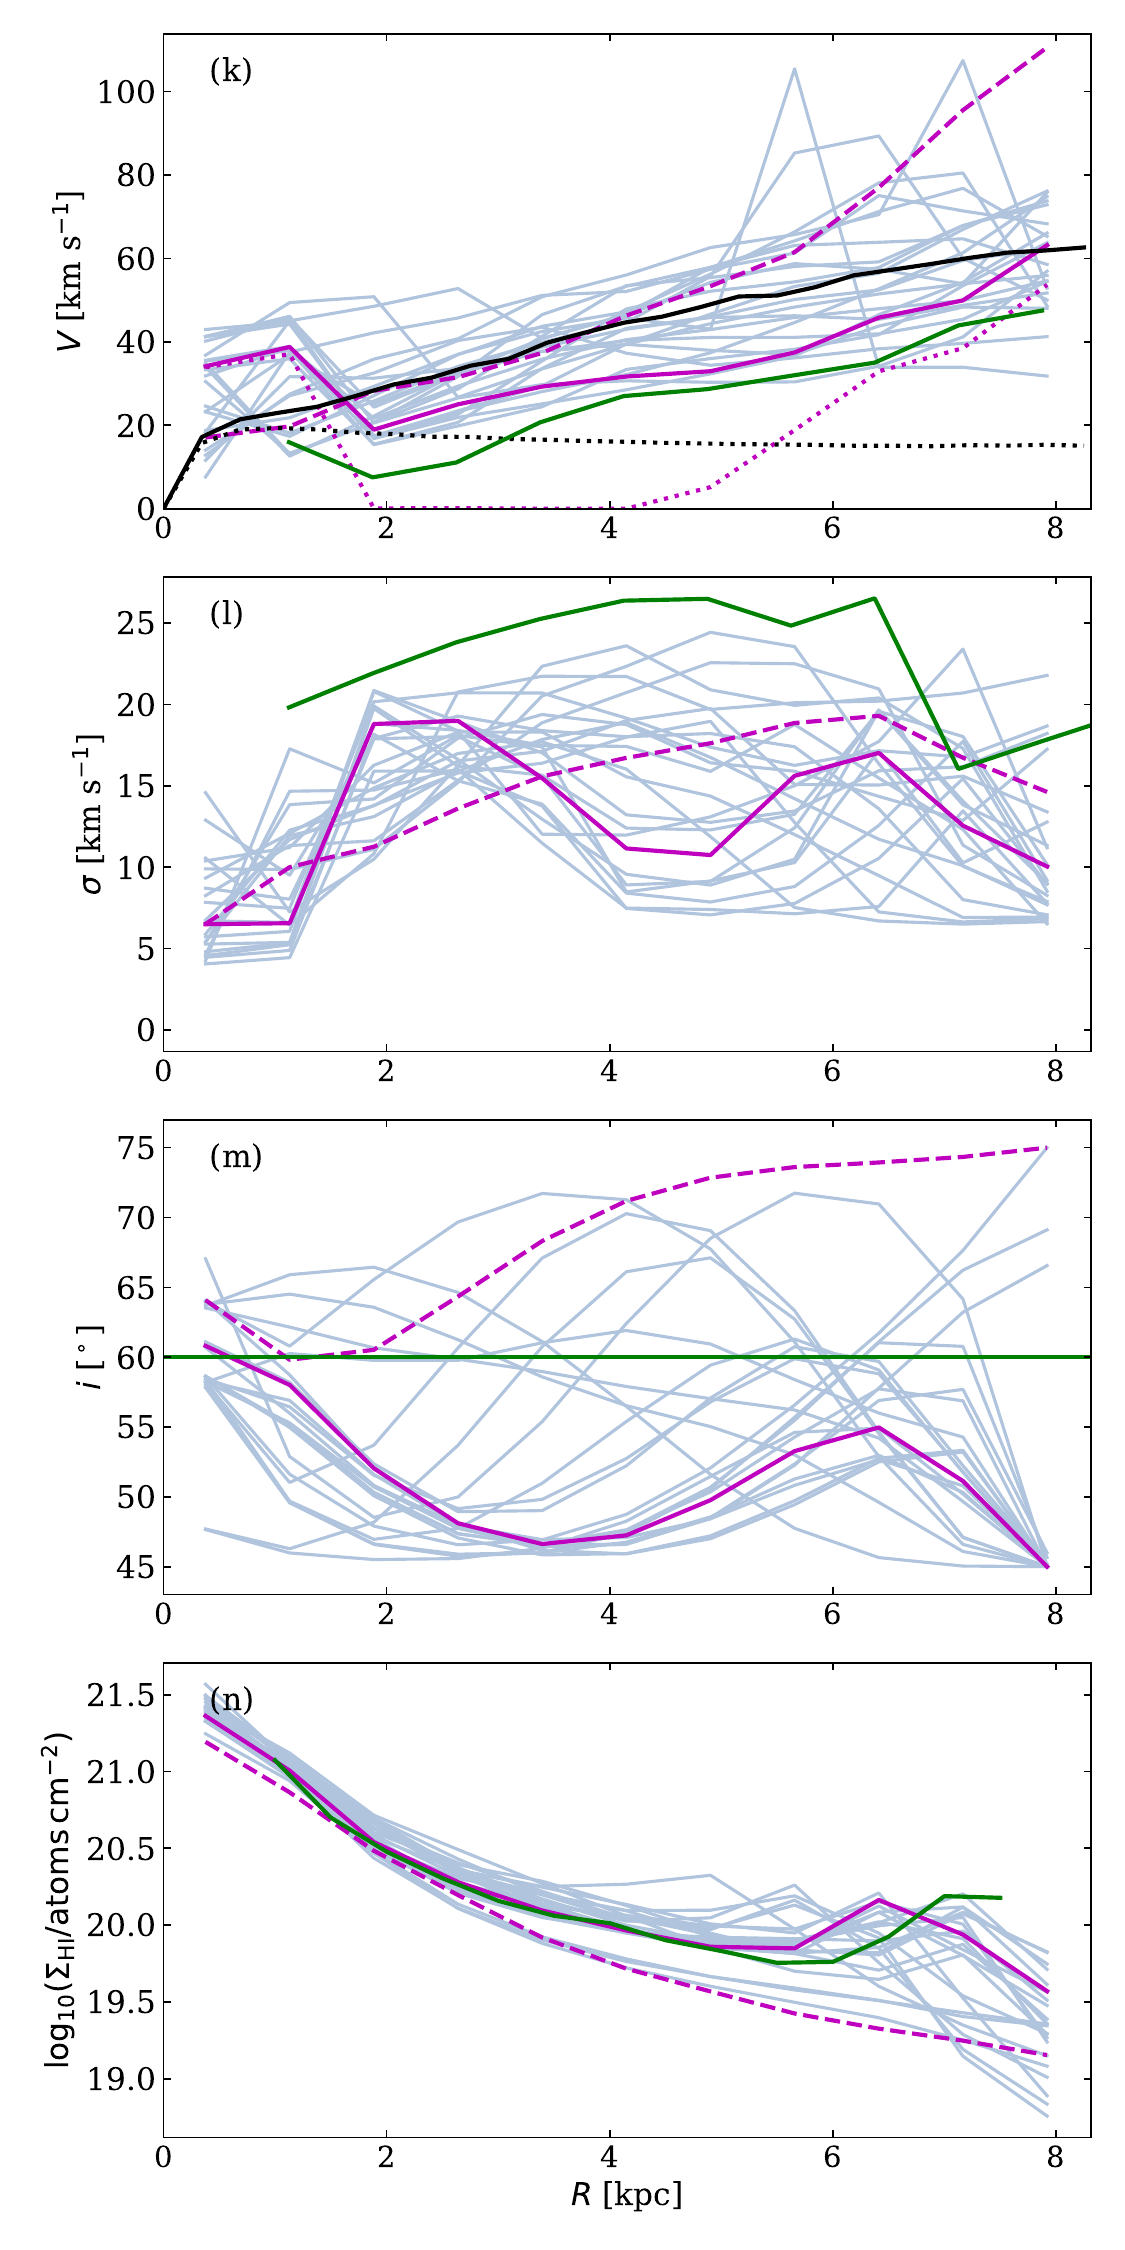}
\end{minipage}
\caption{A set of summary figures for galaxy HT-36, excluded from kinematic analysis. These include example moment maps for two orientations (panels (a)--(f); similar to Fig.~\ref{fig:visualisations}), a summary of the parameters $V_\mathrm{fid}$, $V_\mathrm{max}$, $\eta_\mathrm{rot}$, and $\eta_\mathrm{bar}$ (panels (g)--(j); similar to Fig.~\ref{fig:loops}), and a summary of the rotation curve analysis from $24$ viewing angles (panels (k)--(n); similar to Fig.~\ref{fig:rot_curves}). See description of Appendix~\ref{app:supplementary} for details.}
\label{fig:S77}
\end{figure}
\clearpage

\begin{figure}
\begin{minipage}{.9\textwidth}
\includegraphics[width=\textwidth]{../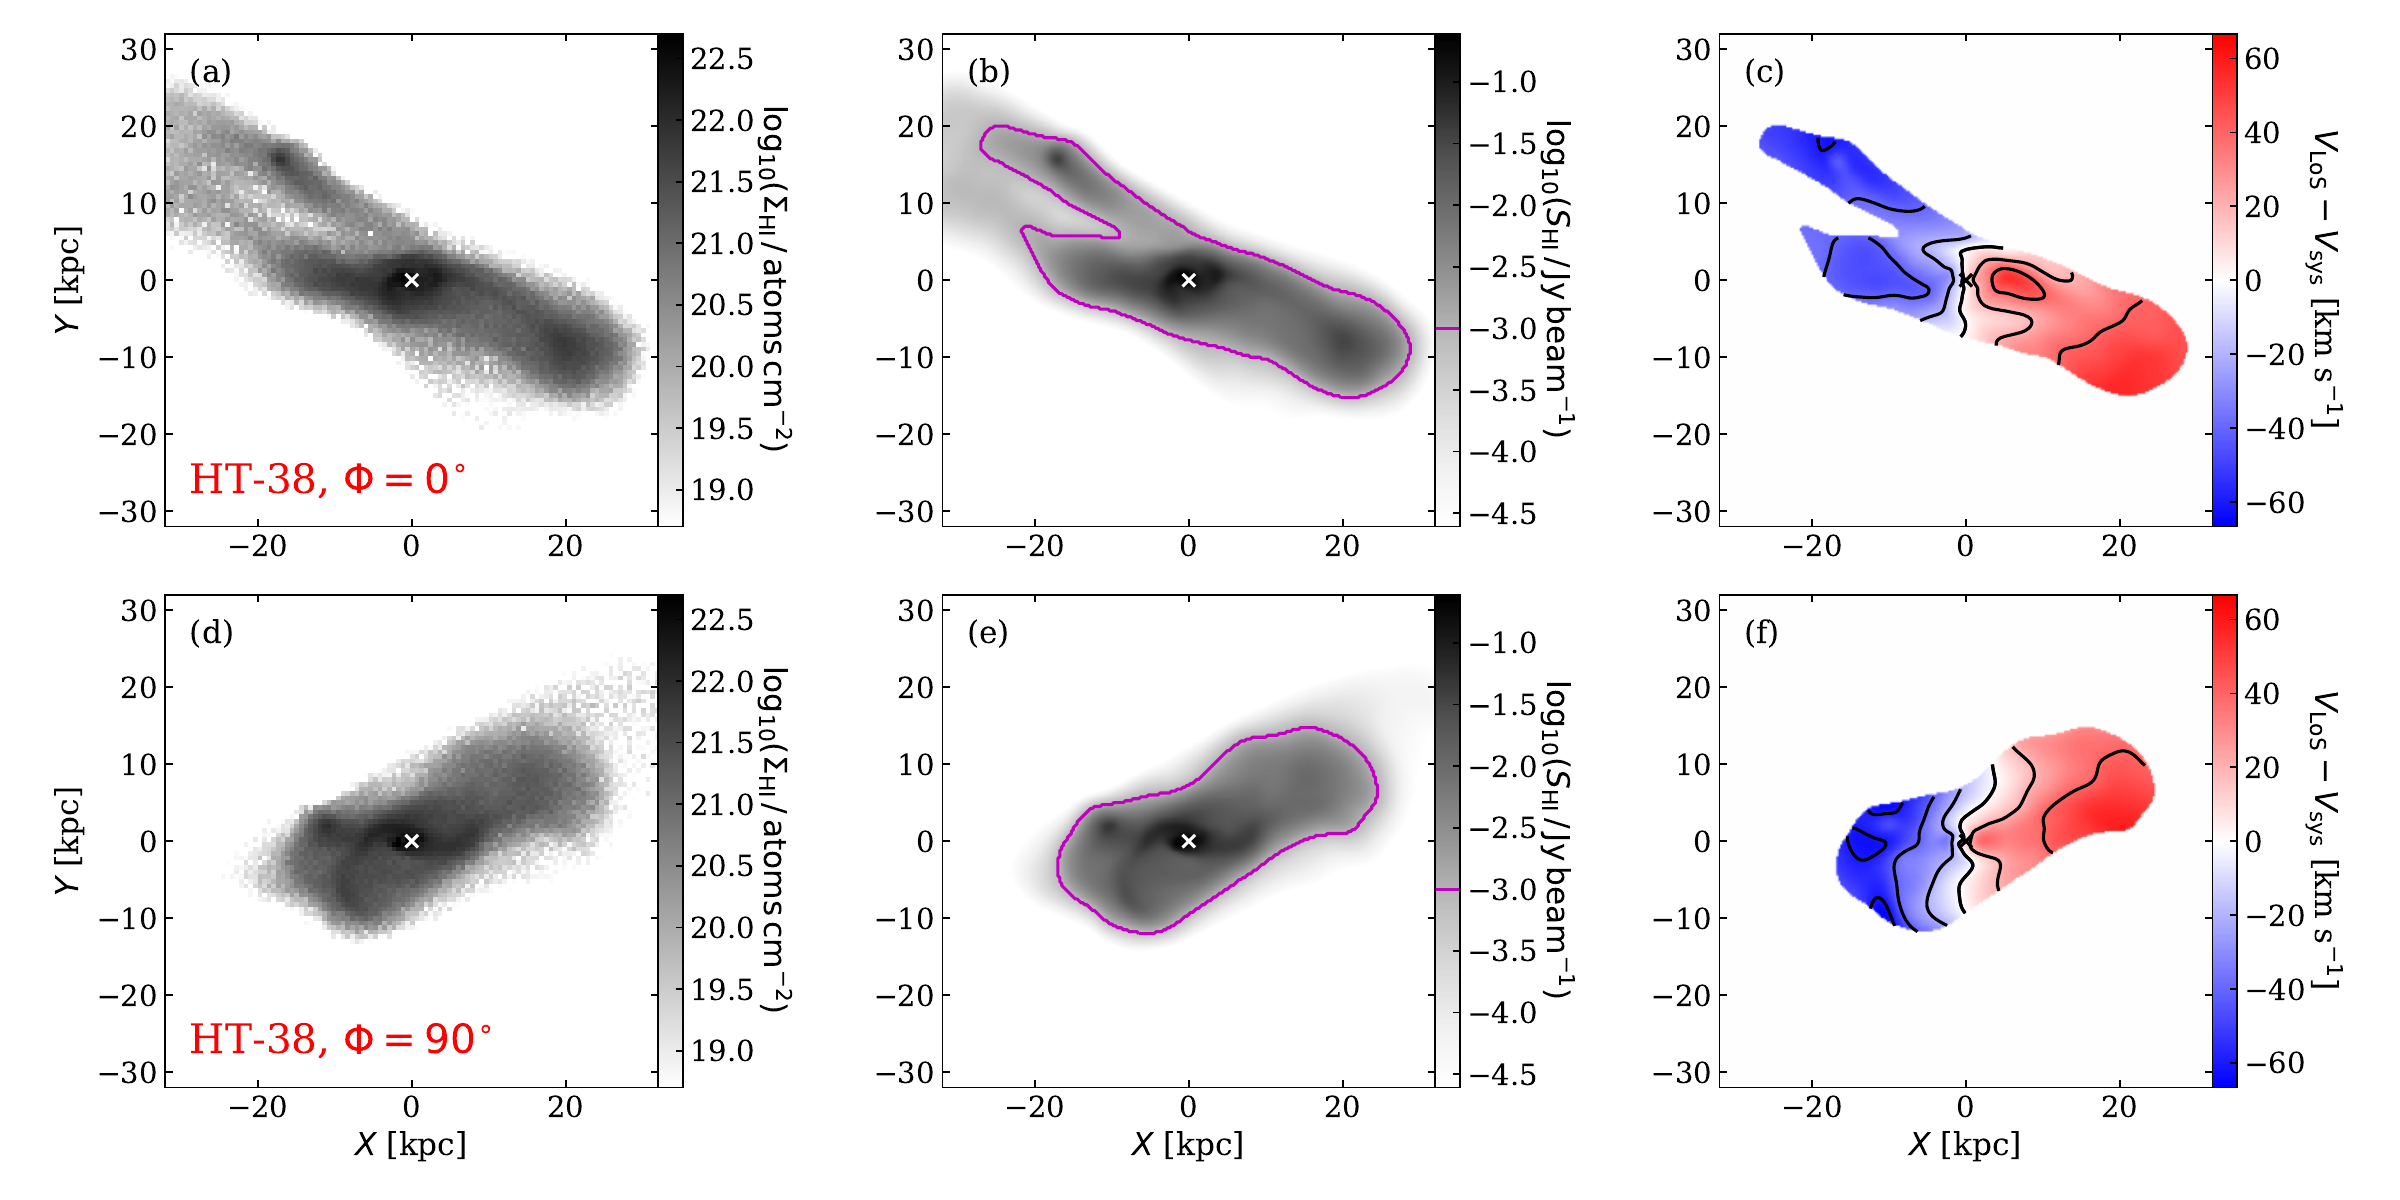}
\includegraphics[width=\textwidth]{../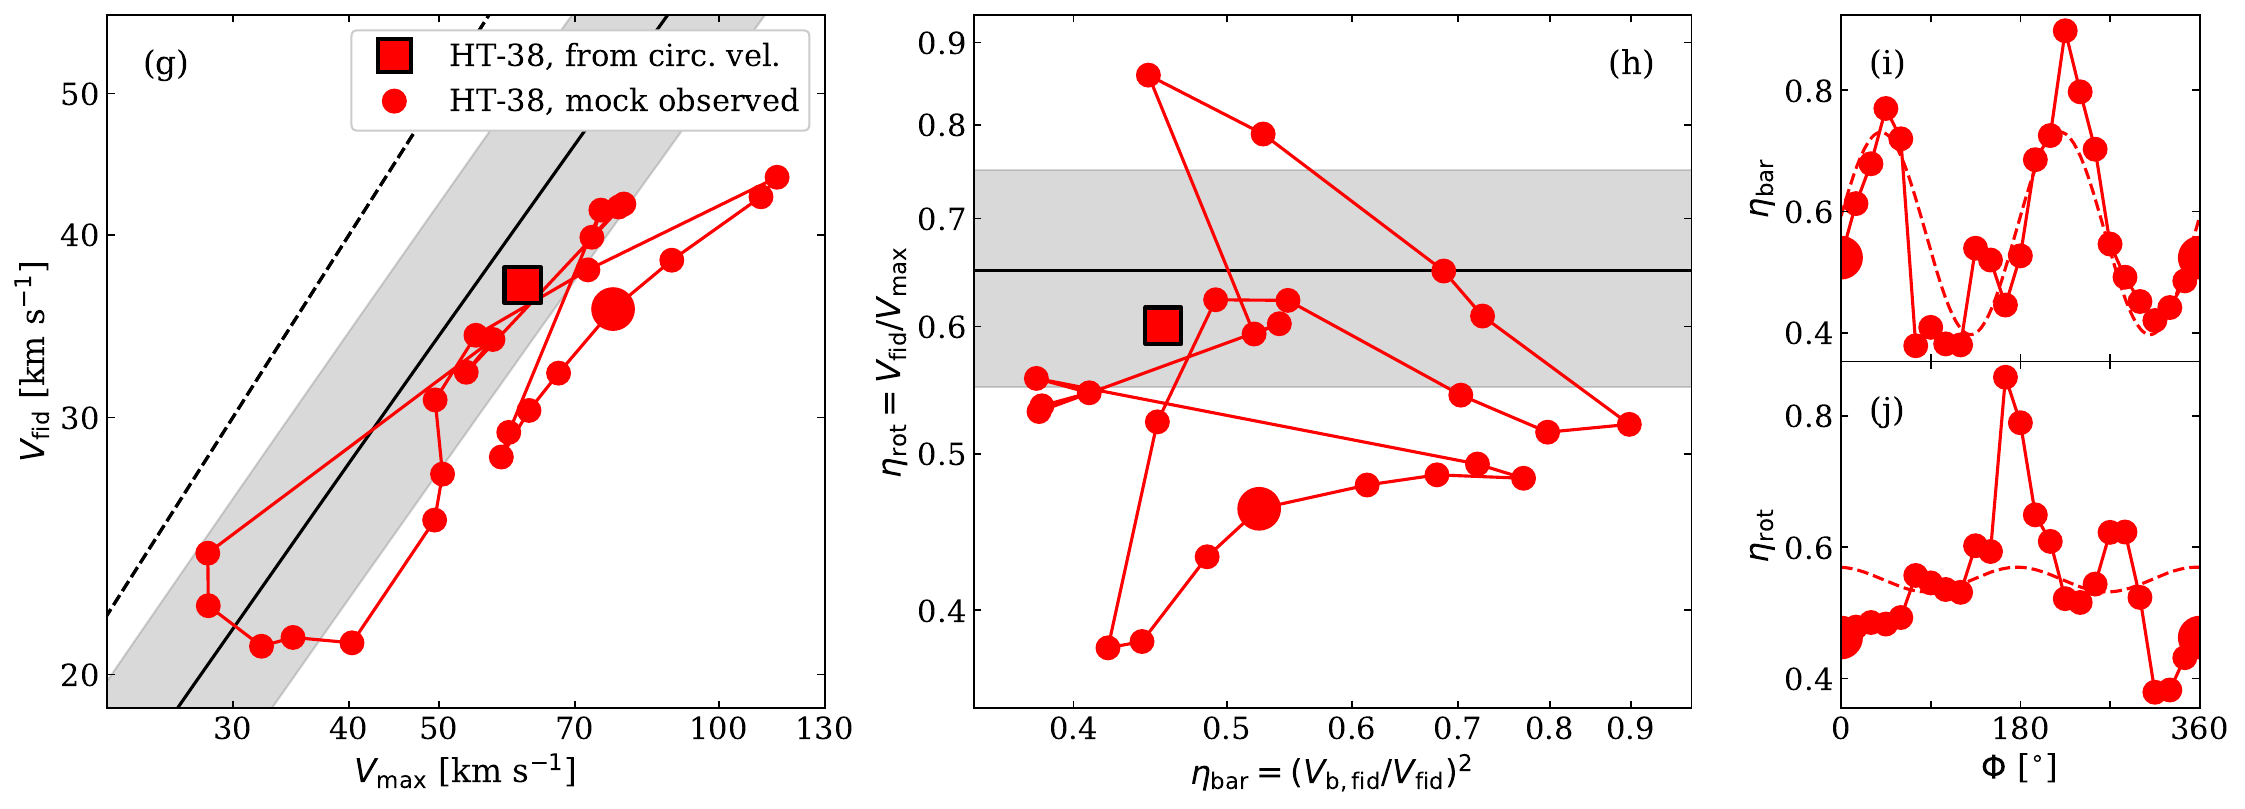}
\end{minipage}
\begin{minipage}{.4\textwidth}
\includegraphics[width=\textwidth]{../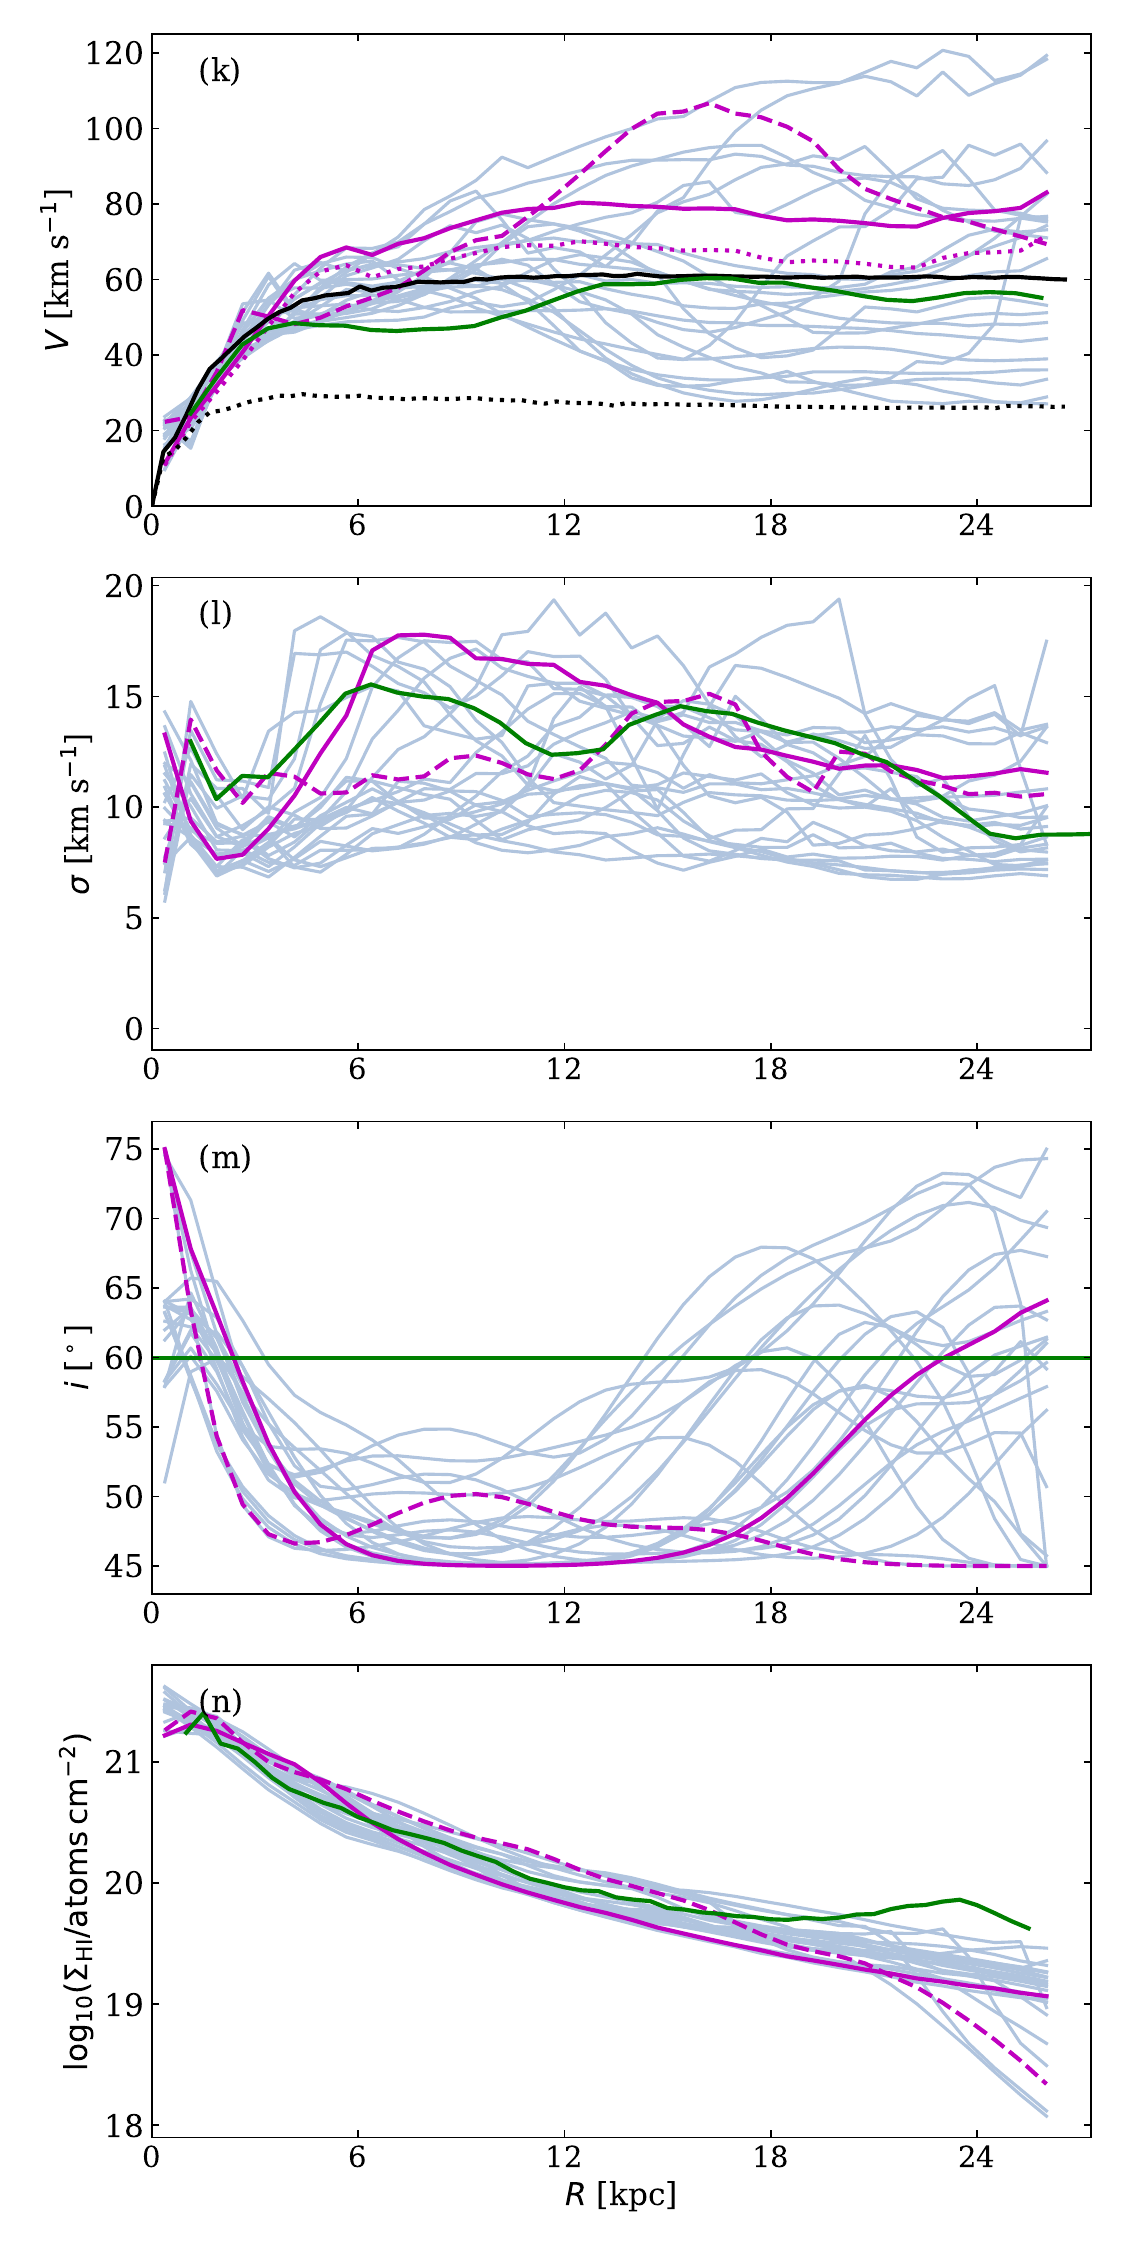}
\end{minipage}
\caption{A set of summary figures for galaxy HT-38, excluded from kinematic analysis. These include example moment maps for two orientations (panels (a)--(f); similar to Fig.~\ref{fig:visualisations}), a summary of the parameters $V_\mathrm{fid}$, $V_\mathrm{max}$, $\eta_\mathrm{rot}$, and $\eta_\mathrm{bar}$ (panels (g)--(j); similar to Fig.~\ref{fig:loops}), and a summary of the rotation curve analysis from $24$ viewing angles (panels (k)--(n); similar to Fig.~\ref{fig:rot_curves}). See description of Appendix~\ref{app:supplementary} for details.}
\label{fig:S78}
\end{figure}
\clearpage

\begin{figure}
\begin{minipage}{.9\textwidth}
\includegraphics[width=\textwidth]{../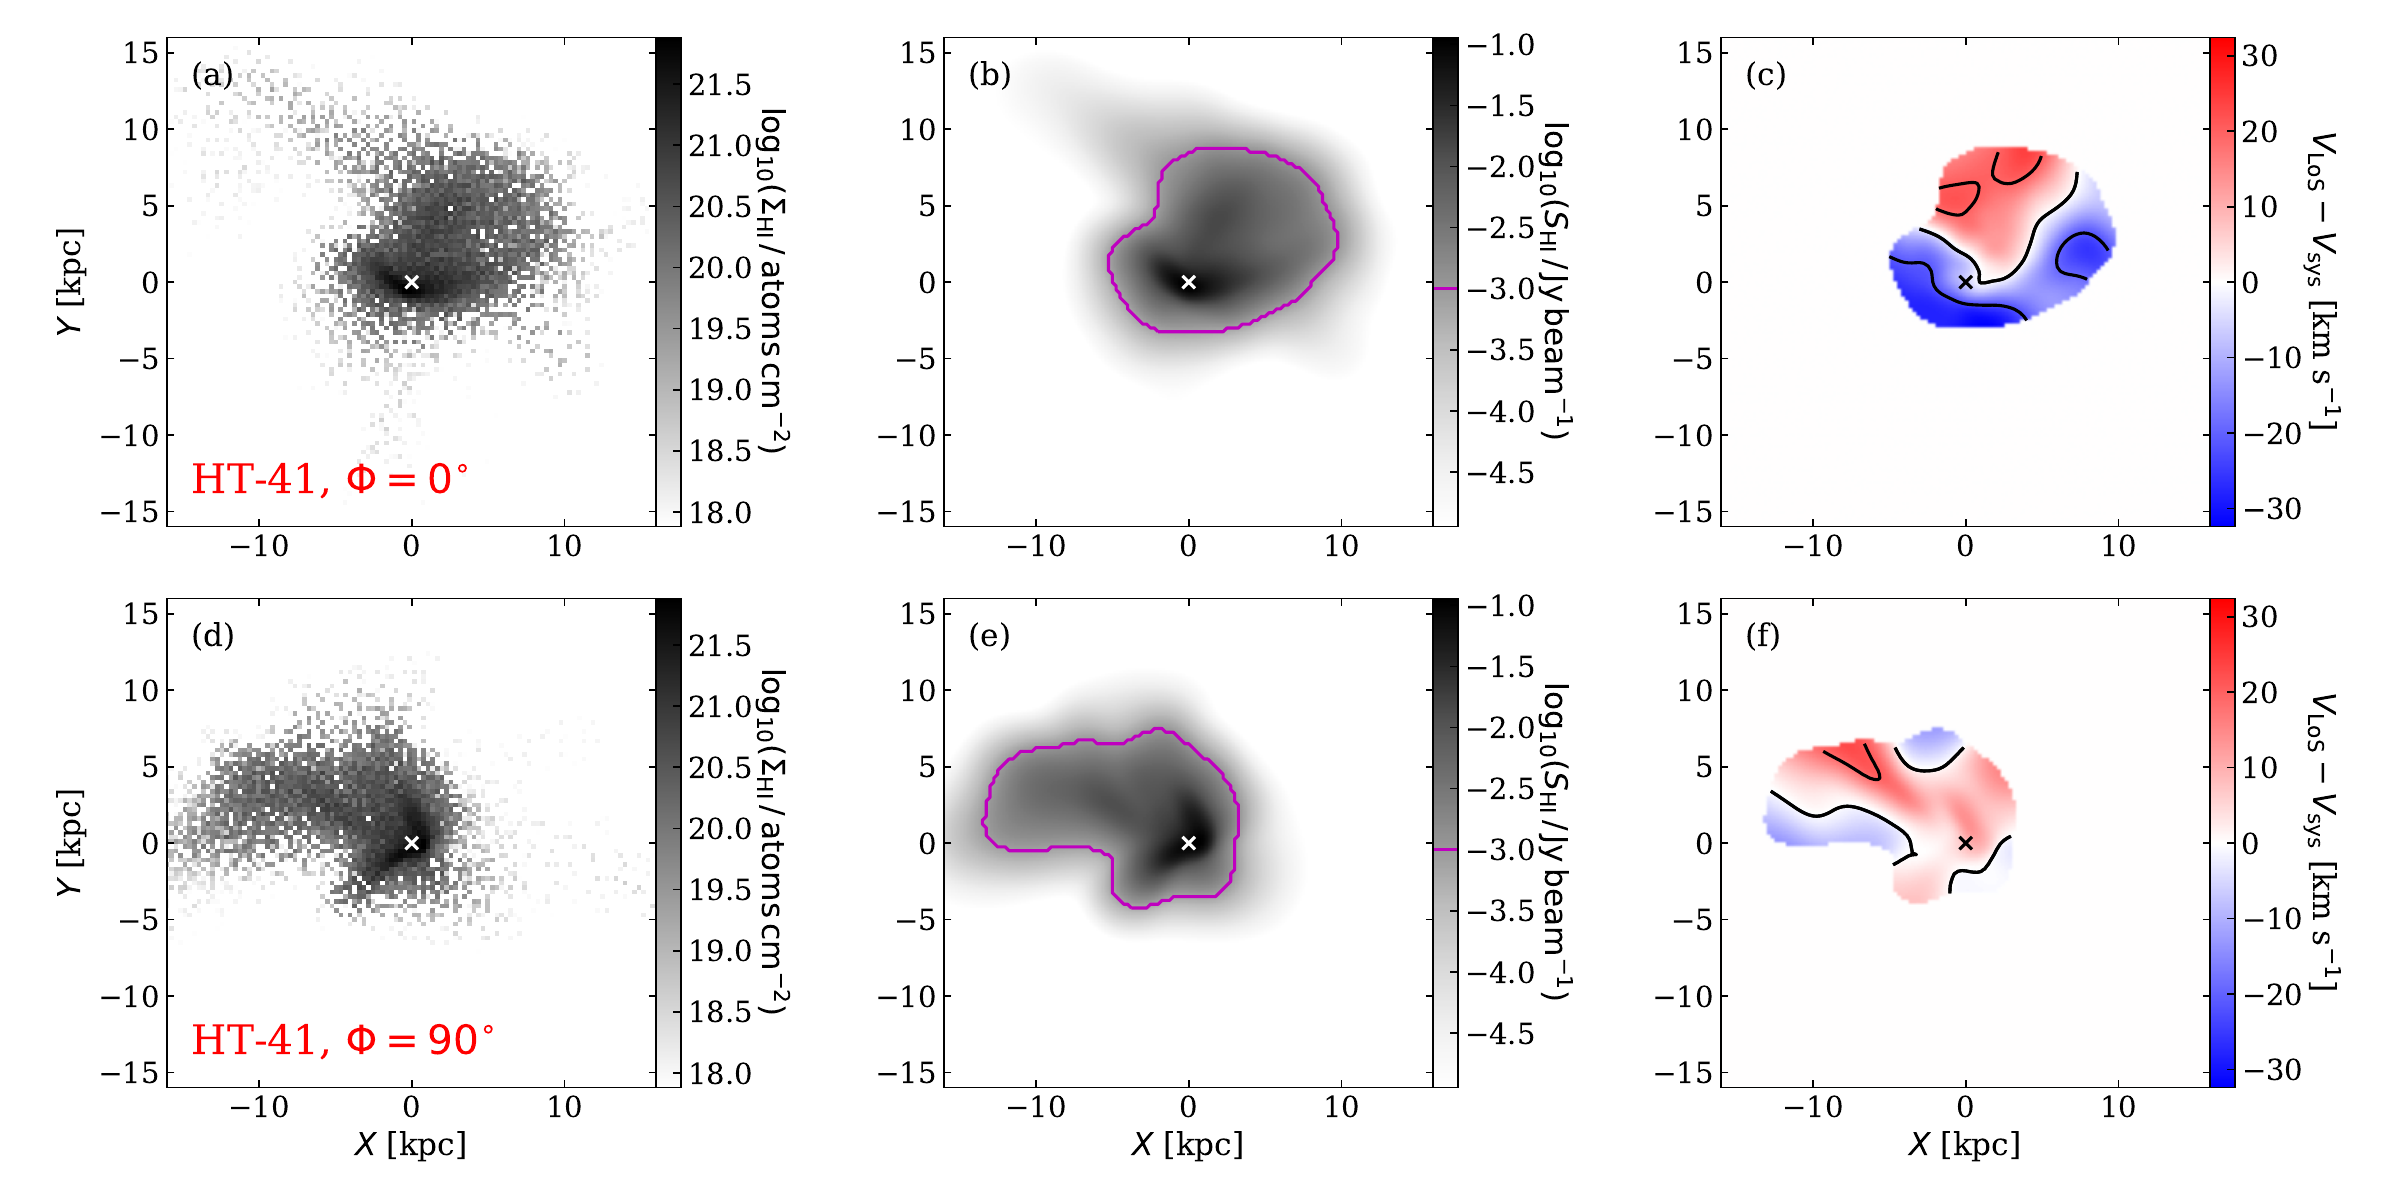}
\includegraphics[width=\textwidth]{../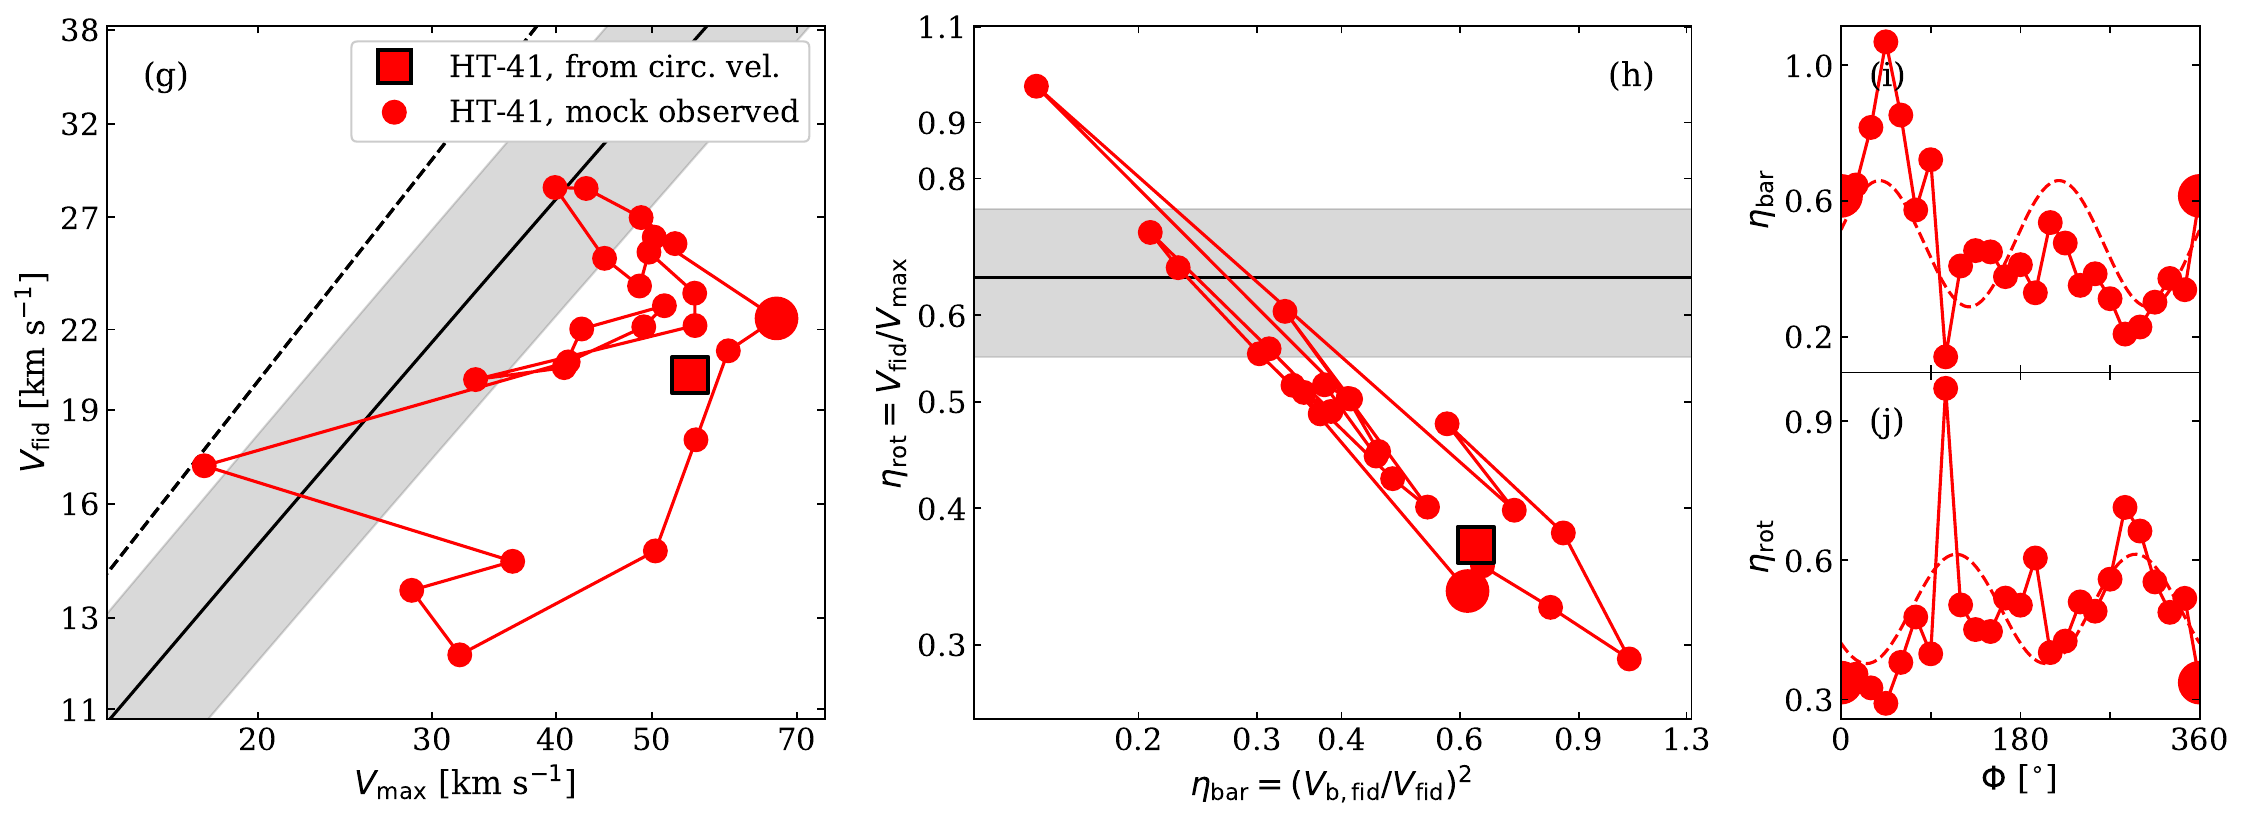}
\end{minipage}
\begin{minipage}{.4\textwidth}
\includegraphics[width=\textwidth]{../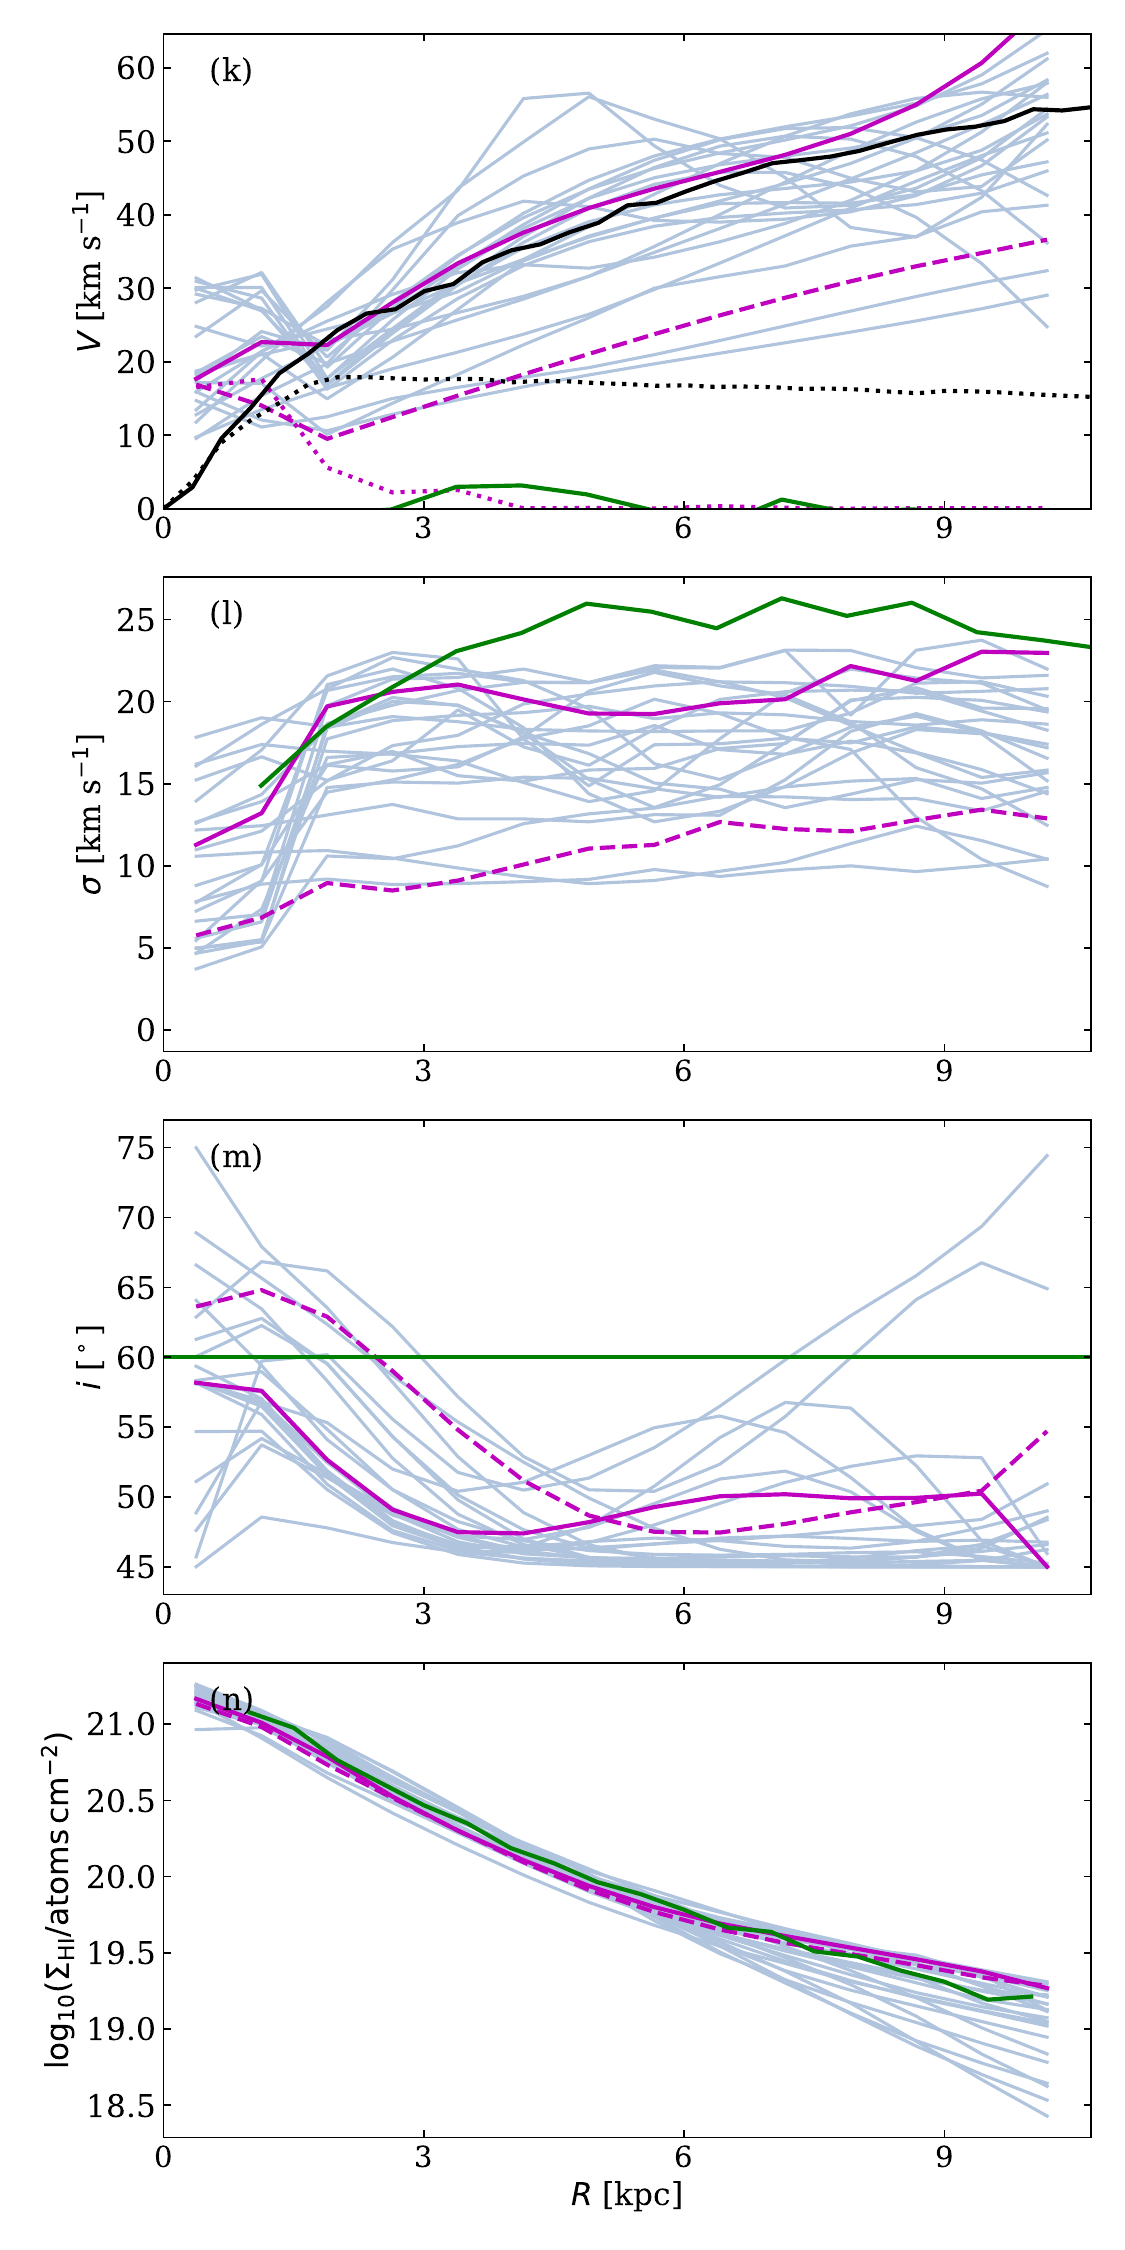}
\end{minipage}
\caption{A set of summary figures for galaxy HT-41, excluded from kinematic analysis. These include example moment maps for two orientations (panels (a)--(f); similar to Fig.~\ref{fig:visualisations}), a summary of the parameters $V_\mathrm{fid}$, $V_\mathrm{max}$, $\eta_\mathrm{rot}$, and $\eta_\mathrm{bar}$ (panels (g)--(j); similar to Fig.~\ref{fig:loops}), and a summary of the rotation curve analysis from $24$ viewing angles (panels (k)--(n); similar to Fig.~\ref{fig:rot_curves}). See description of Appendix~\ref{app:supplementary} for details.}
\label{fig:S79}
\end{figure}
\clearpage

\begin{figure}
\begin{minipage}{.9\textwidth}
\includegraphics[width=\textwidth]{../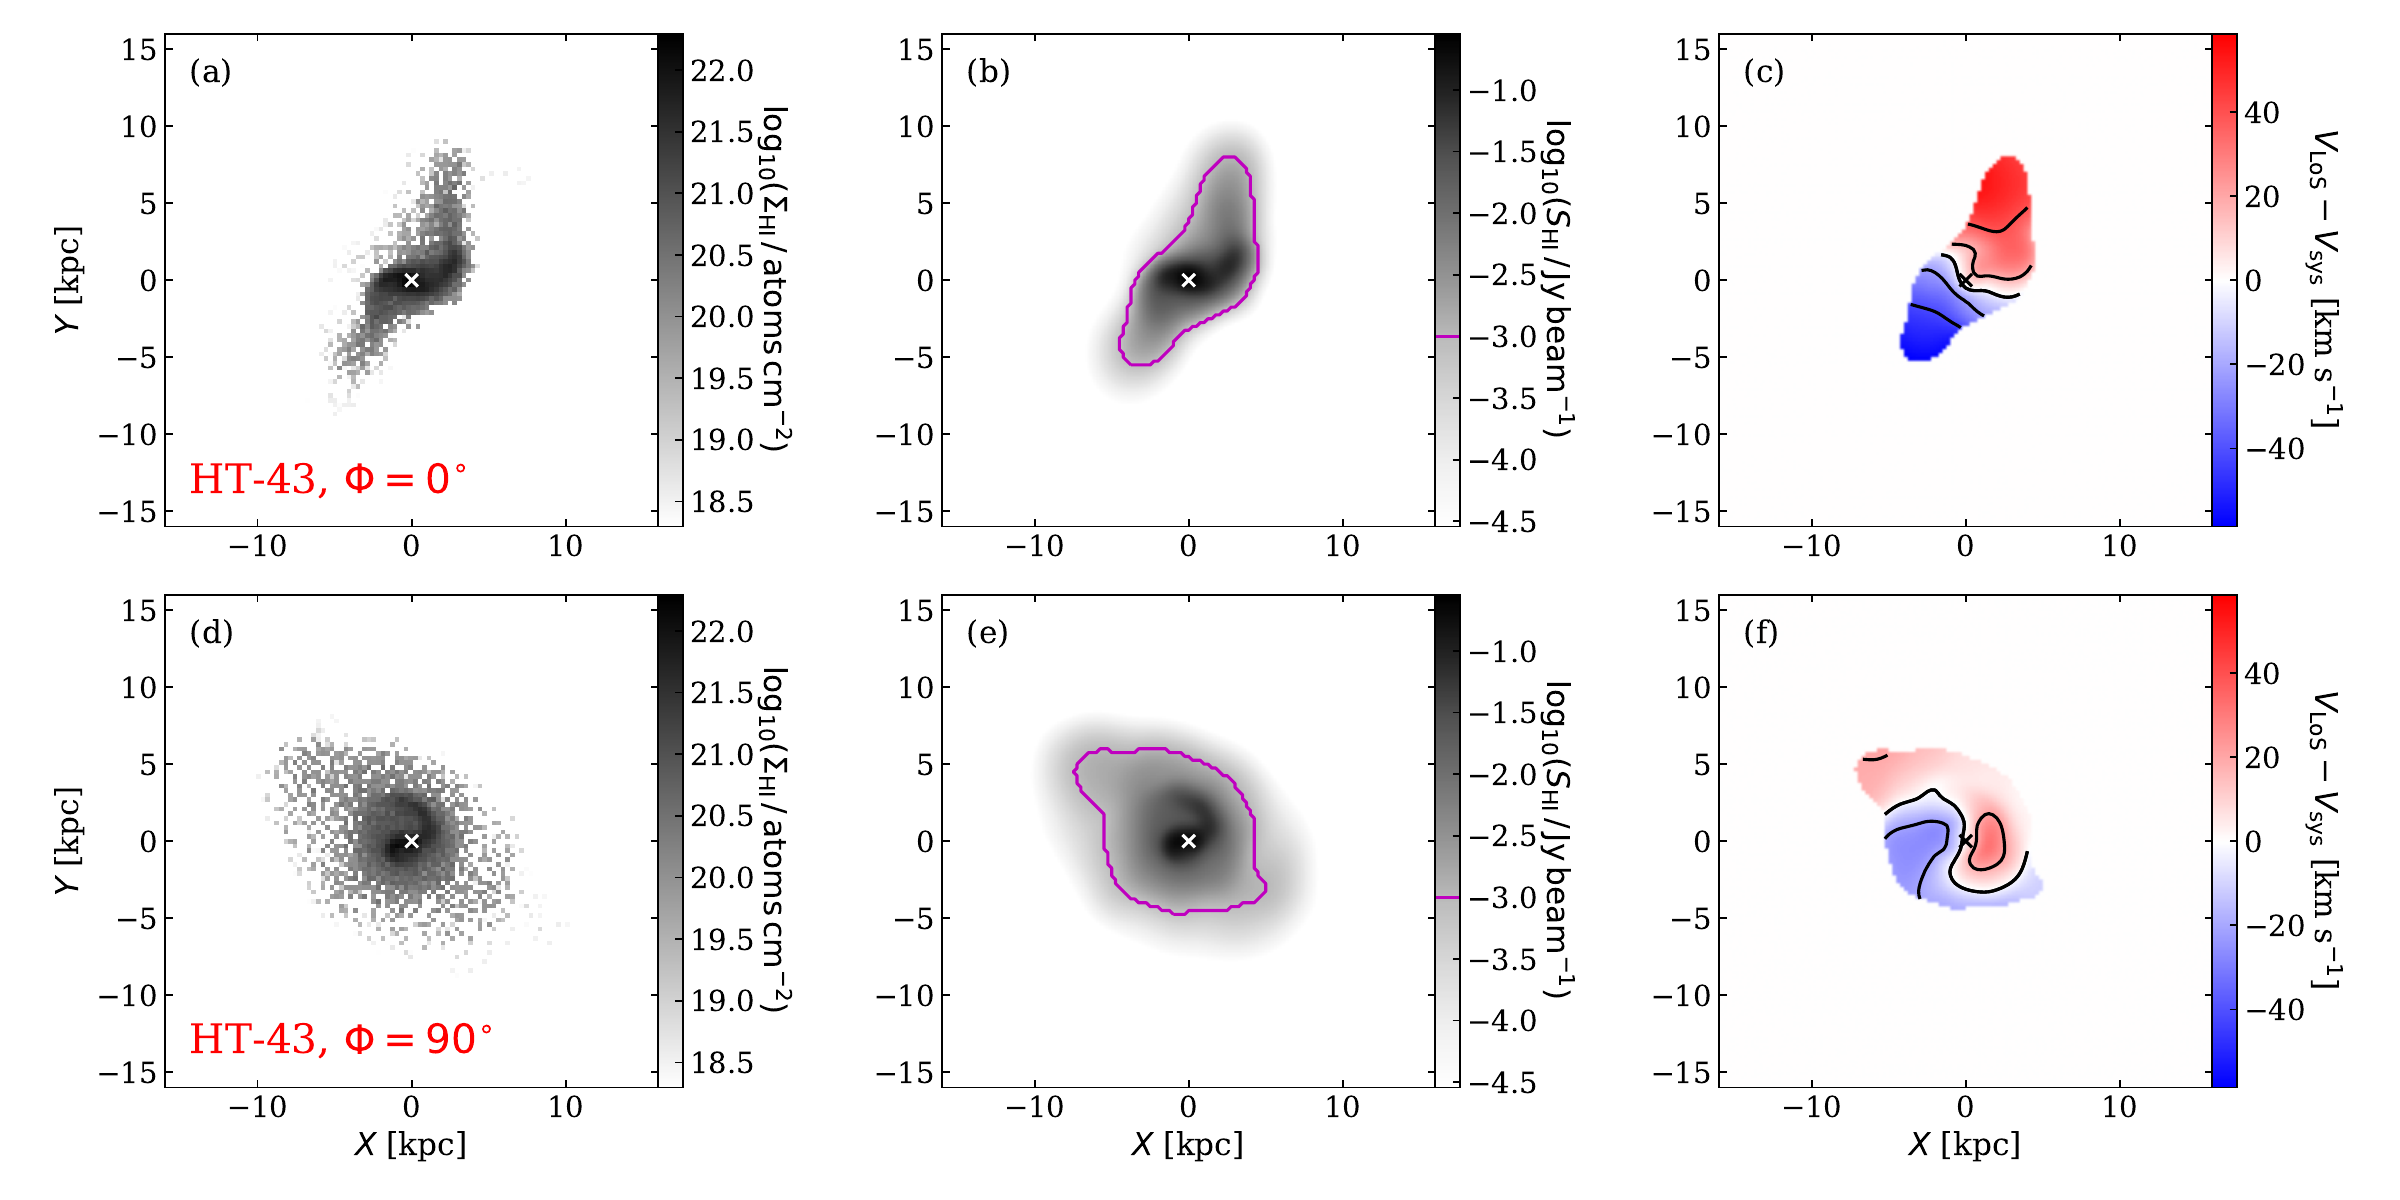}
\includegraphics[width=\textwidth]{../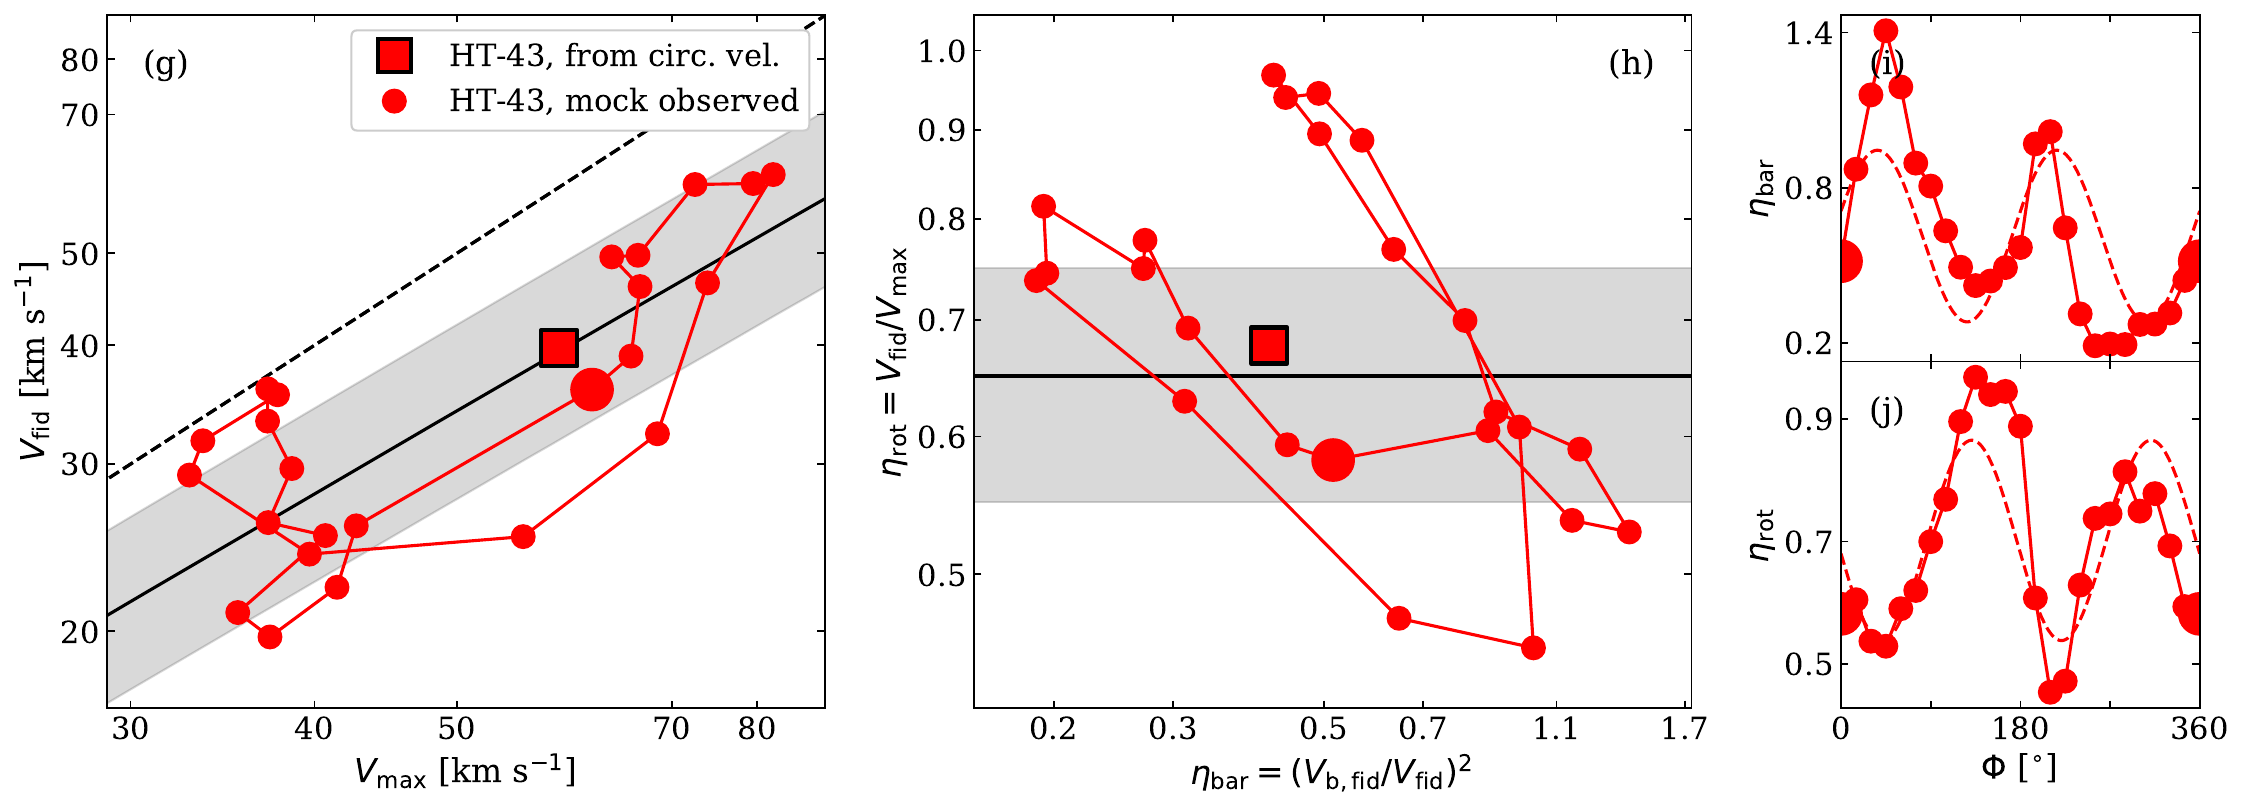}
\end{minipage}
\begin{minipage}{.4\textwidth}
\includegraphics[width=\textwidth]{../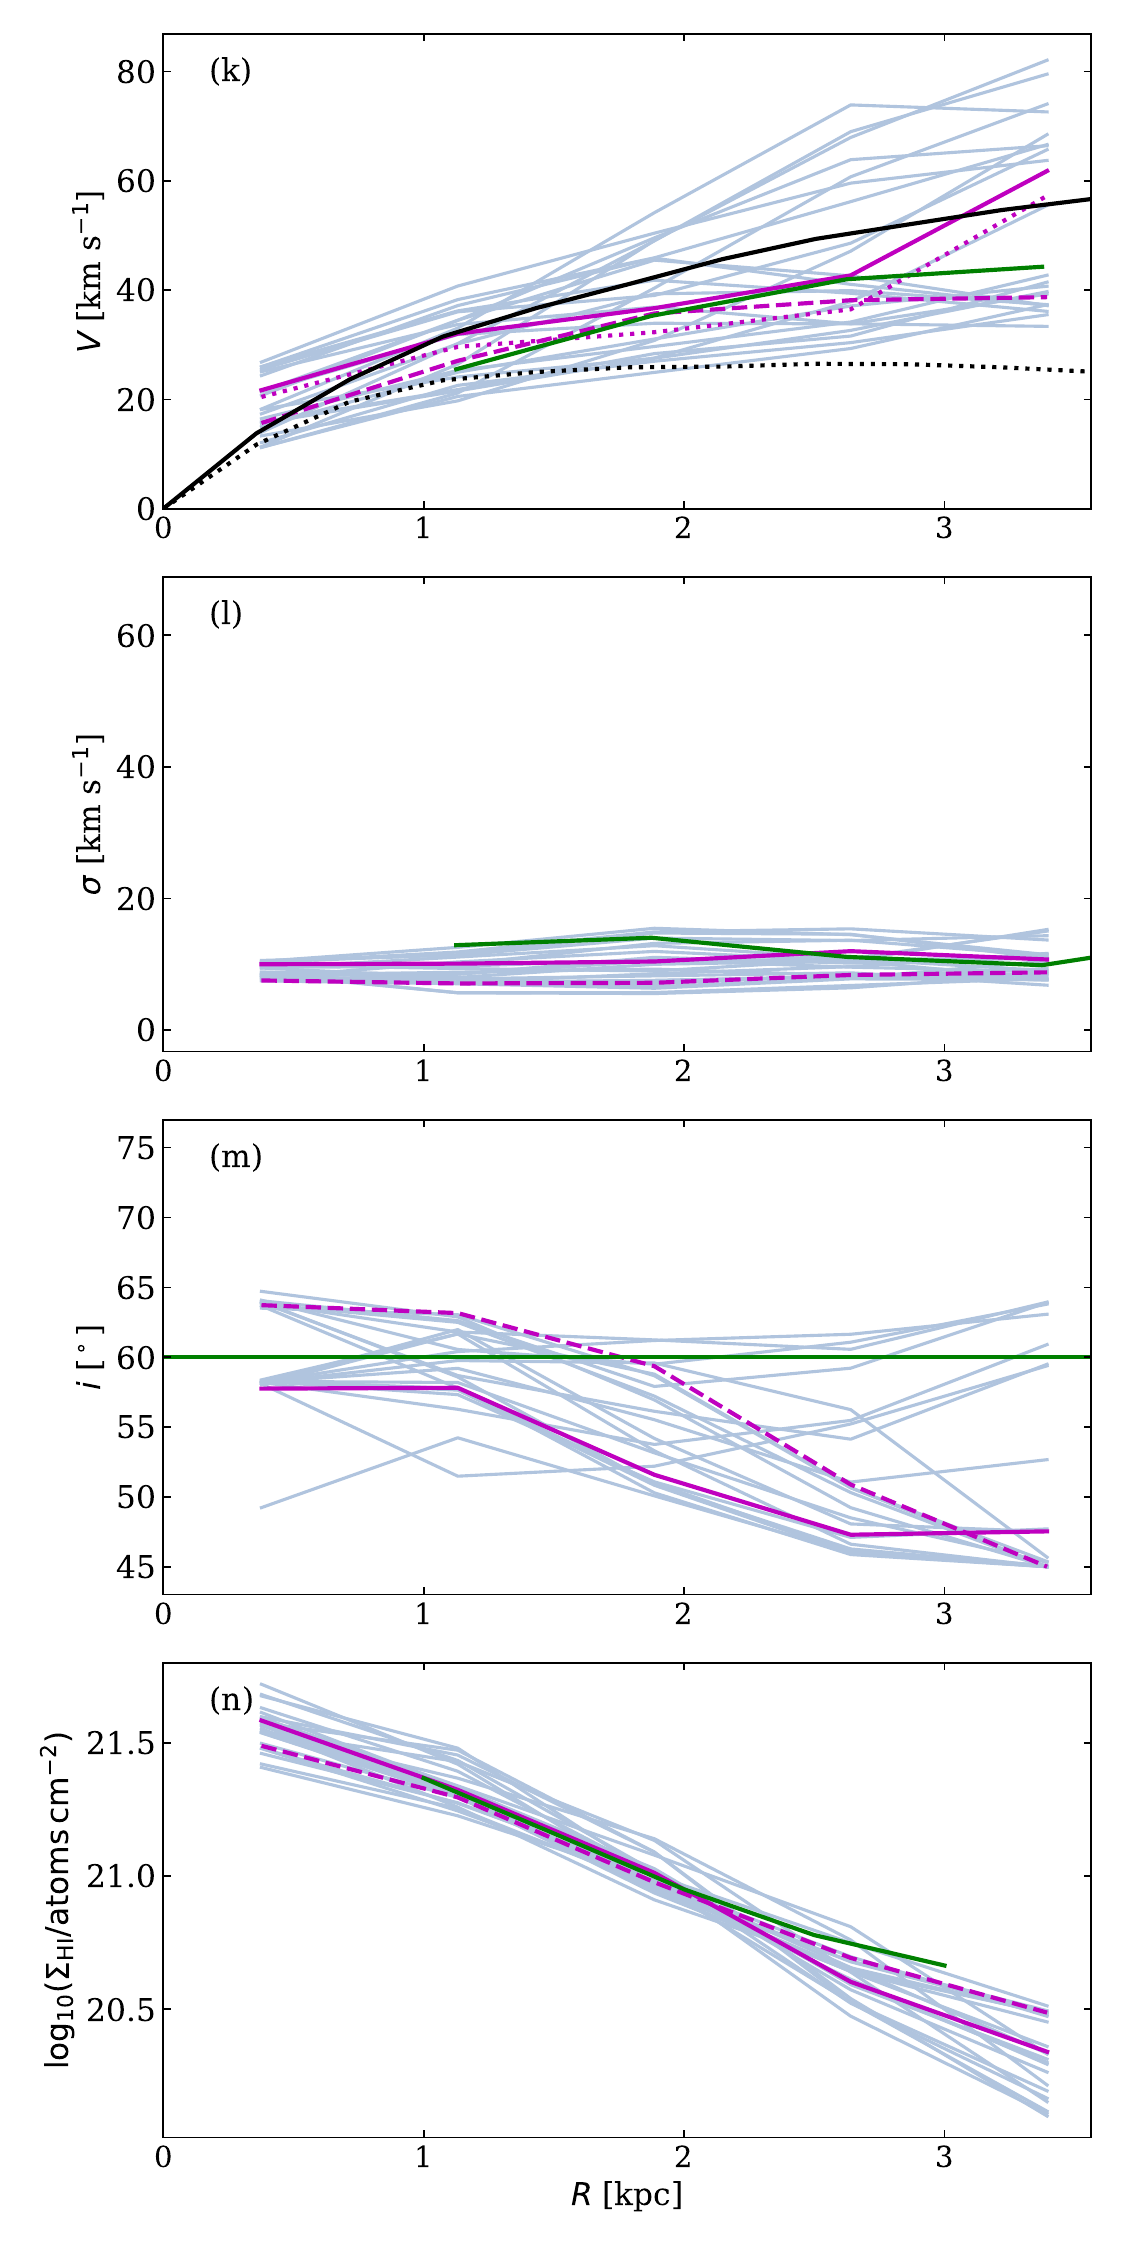}
\end{minipage}
\caption{A set of summary figures for galaxy HT-43, excluded from kinematic analysis. These include example moment maps for two orientations (panels (a)--(f); similar to Fig.~\ref{fig:visualisations}), a summary of the parameters $V_\mathrm{fid}$, $V_\mathrm{max}$, $\eta_\mathrm{rot}$, and $\eta_\mathrm{bar}$ (panels (g)--(j); similar to Fig.~\ref{fig:loops}), and a summary of the rotation curve analysis from $24$ viewing angles (panels (k)--(n); similar to Fig.~\ref{fig:rot_curves}). See description of Appendix~\ref{app:supplementary} for details.}
\label{fig:S80}
\end{figure}
\clearpage

\begin{figure}
\begin{minipage}{.9\textwidth}
\includegraphics[width=\textwidth]{../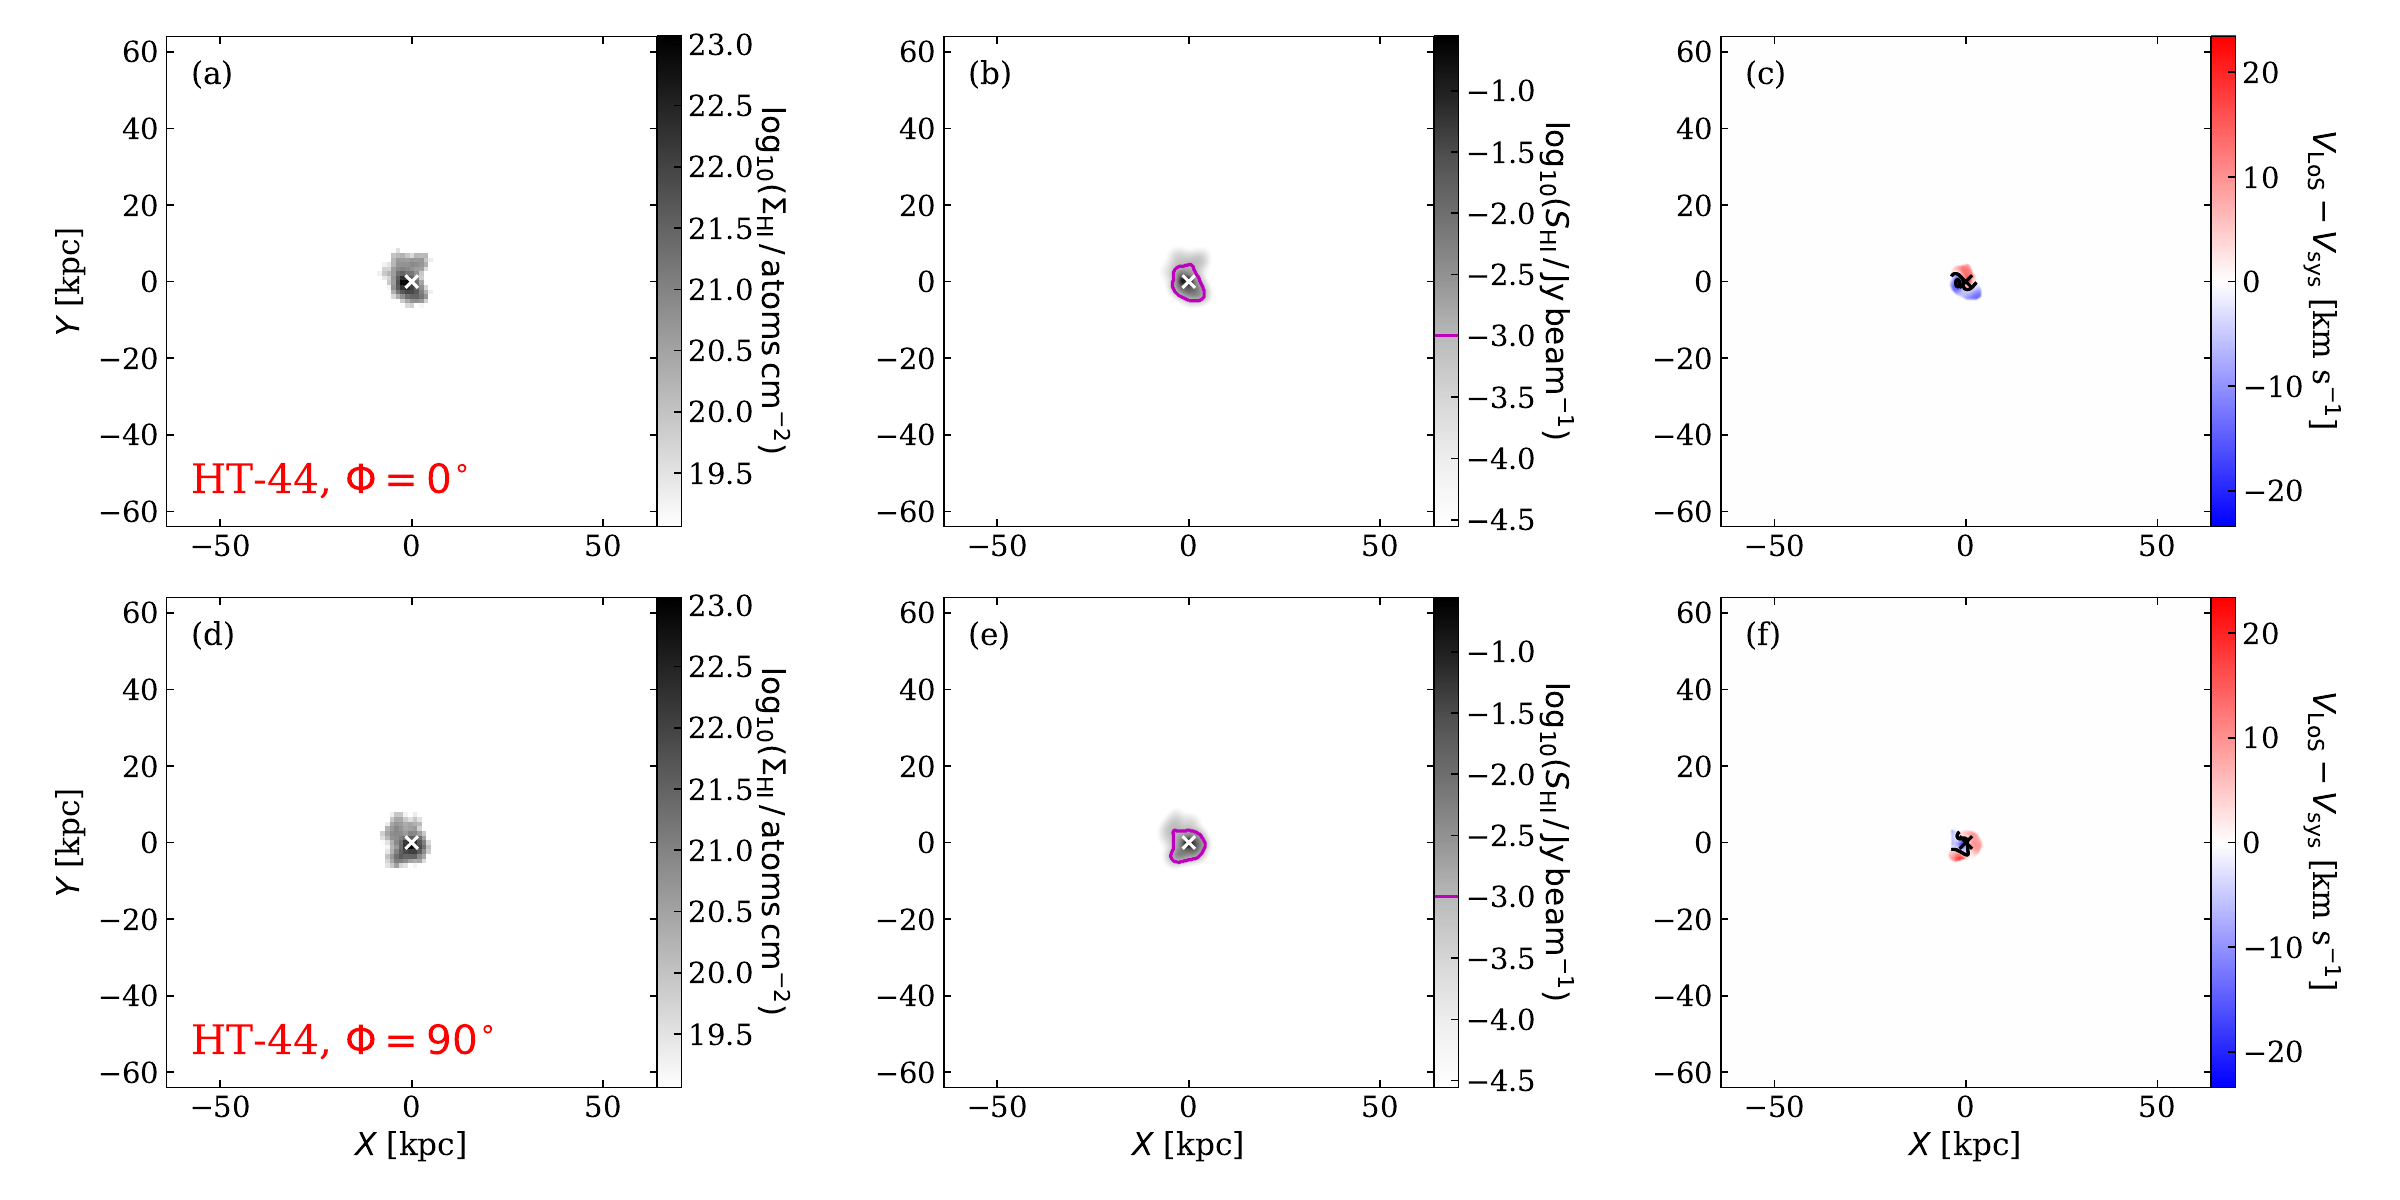}
\includegraphics[width=\textwidth]{../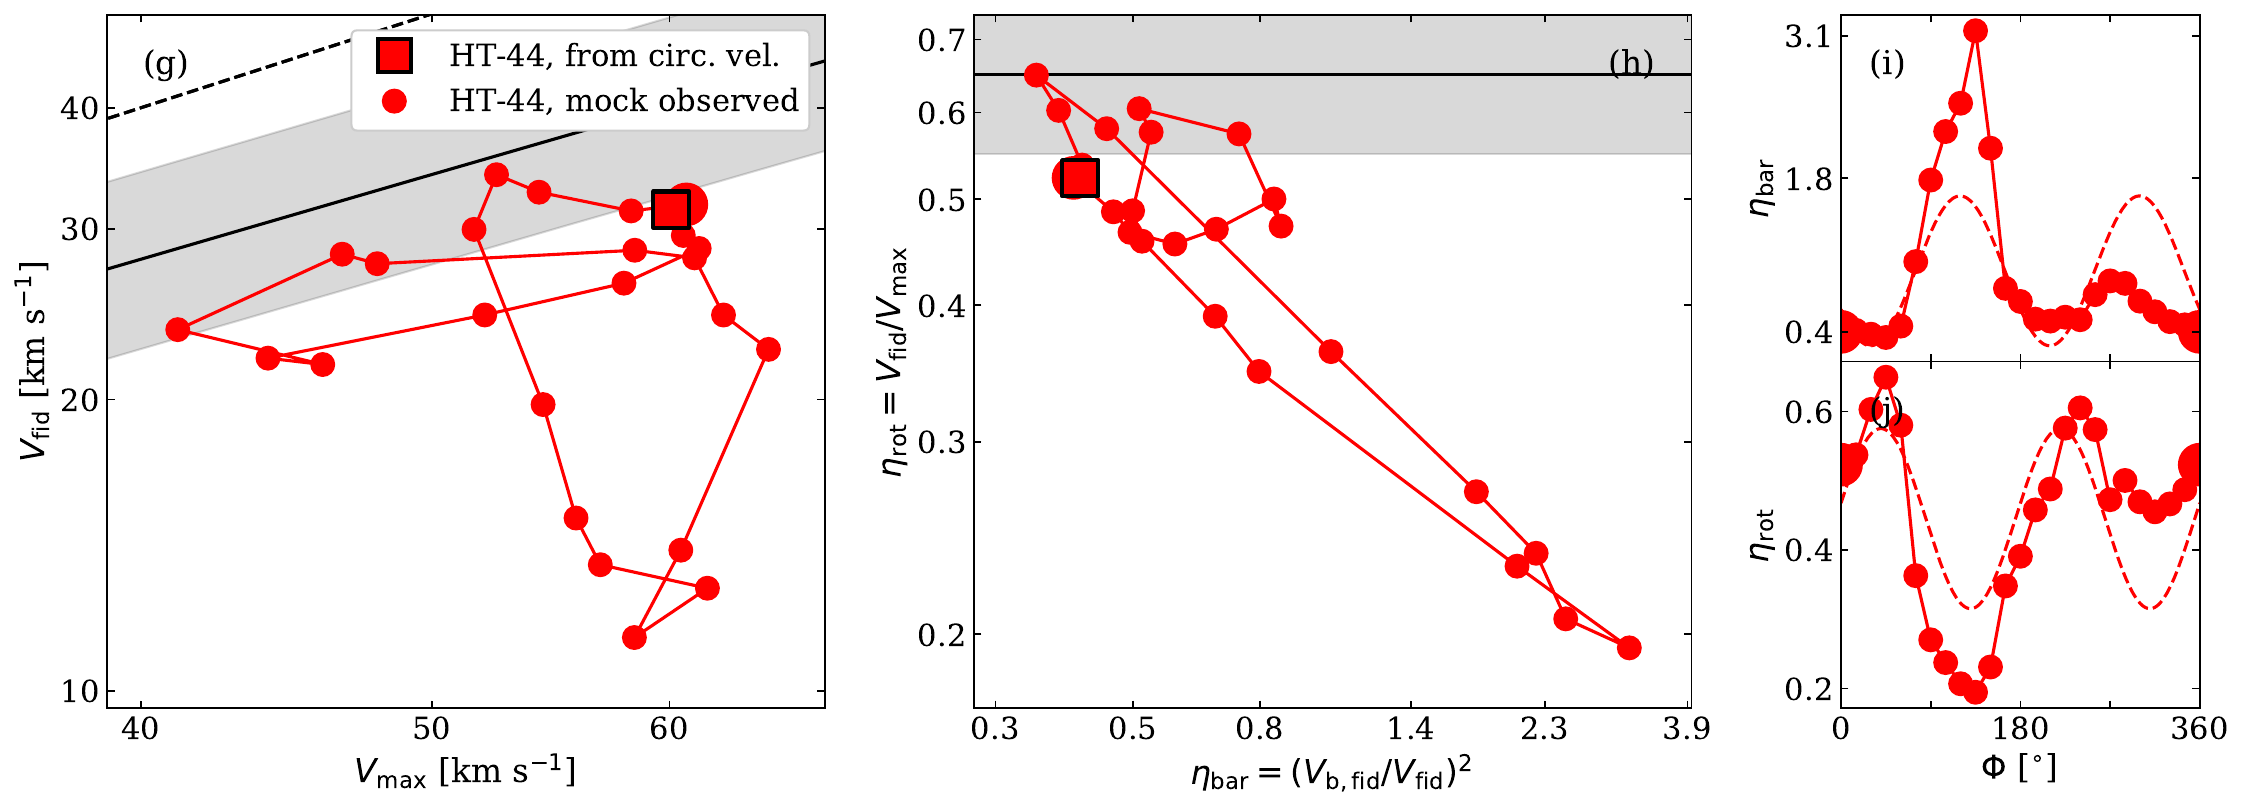}
\end{minipage}
\begin{minipage}{.4\textwidth}
\includegraphics[width=\textwidth]{../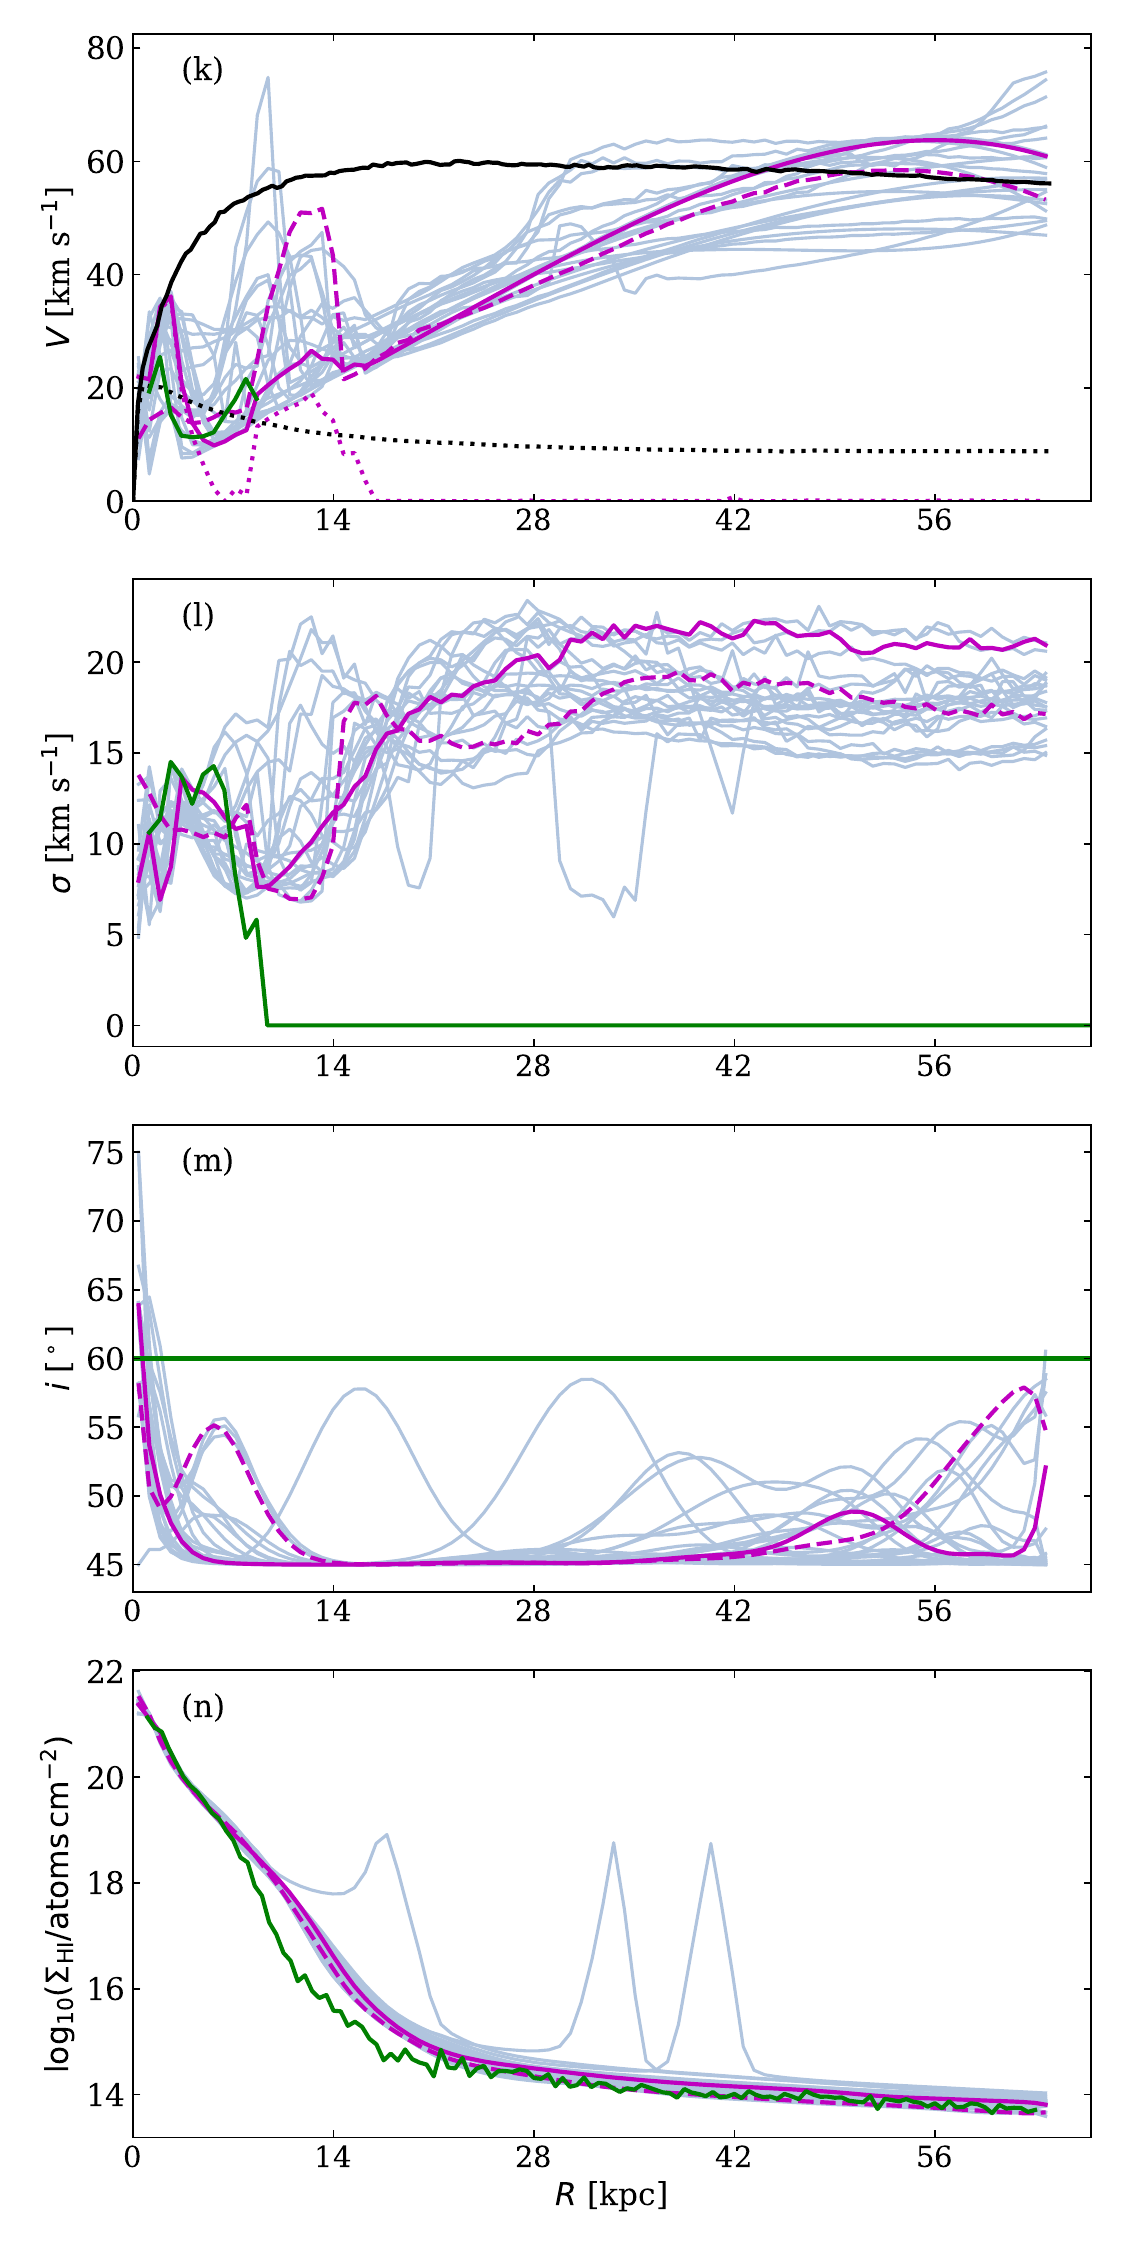}
\end{minipage}
\caption{A set of summary figures for galaxy HT-44, excluded from kinematic analysis. These include example moment maps for two orientations (panels (a)--(f); similar to Fig.~\ref{fig:visualisations}), a summary of the parameters $V_\mathrm{fid}$, $V_\mathrm{max}$, $\eta_\mathrm{rot}$, and $\eta_\mathrm{bar}$ (panels (g)--(j); similar to Fig.~\ref{fig:loops}), and a summary of the rotation curve analysis from $24$ viewing angles (panels (k)--(n); similar to Fig.~\ref{fig:rot_curves}). See description of Appendix~\ref{app:supplementary} for details.}
\label{fig:S81}
\end{figure}
\clearpage

\begin{figure}
\begin{minipage}{.9\textwidth}
\includegraphics[width=\textwidth]{../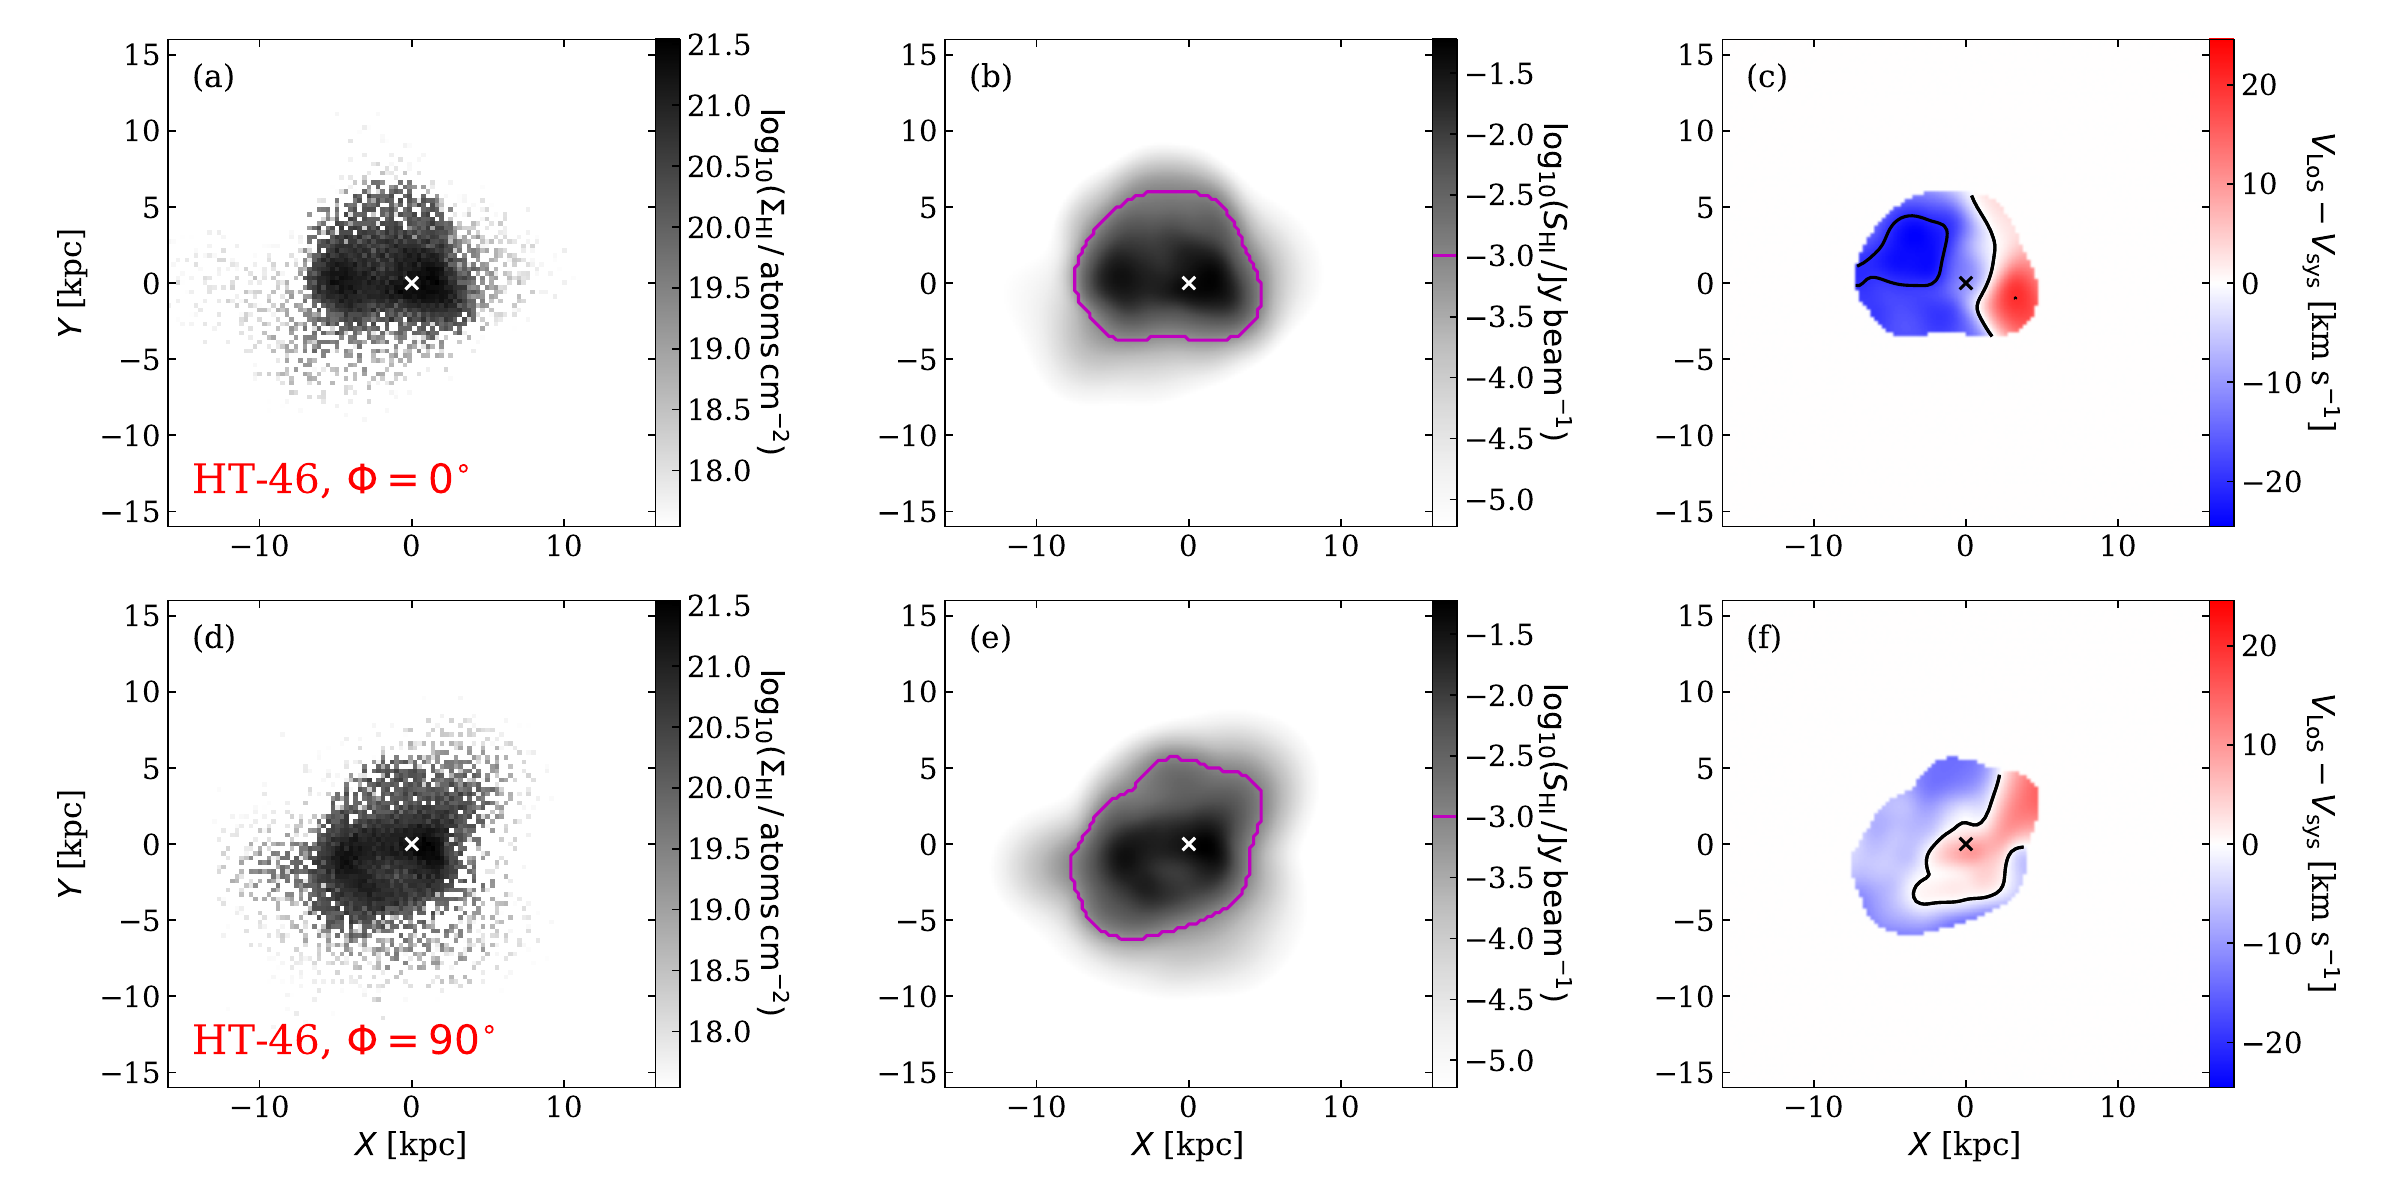}
\includegraphics[width=\textwidth]{../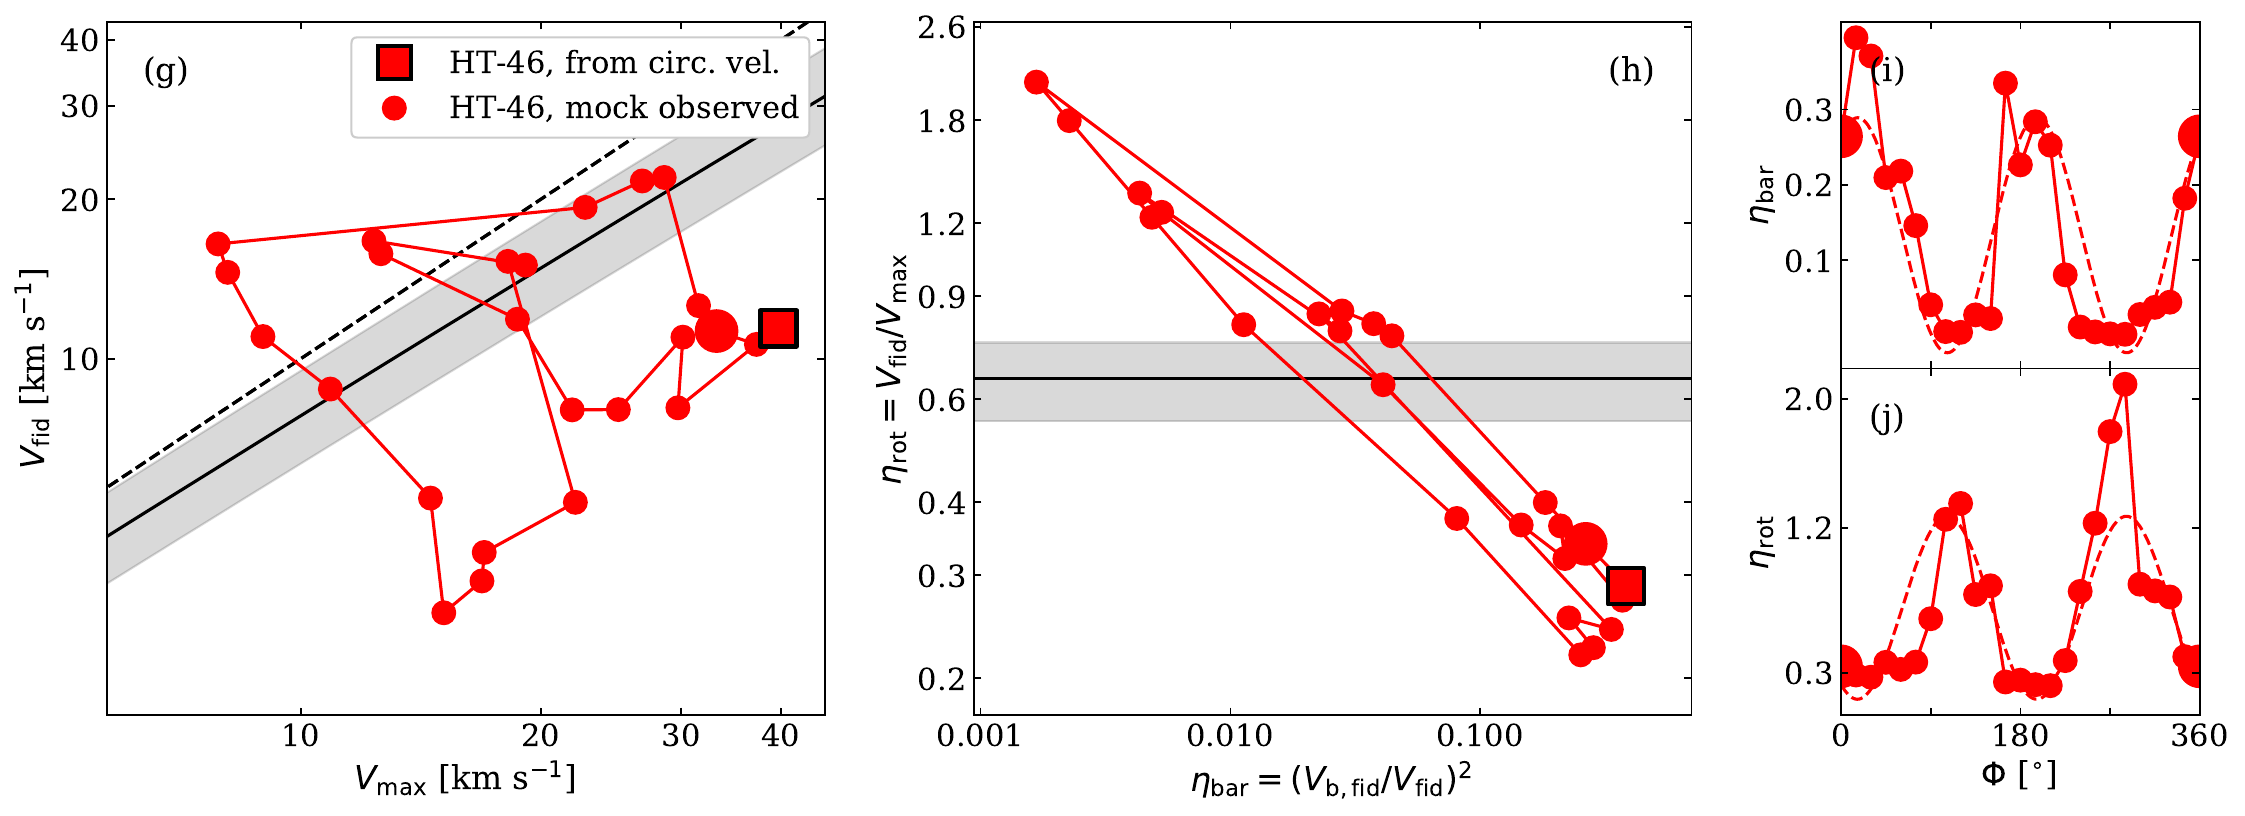}
\end{minipage}
\begin{minipage}{.4\textwidth}
\includegraphics[width=\textwidth]{../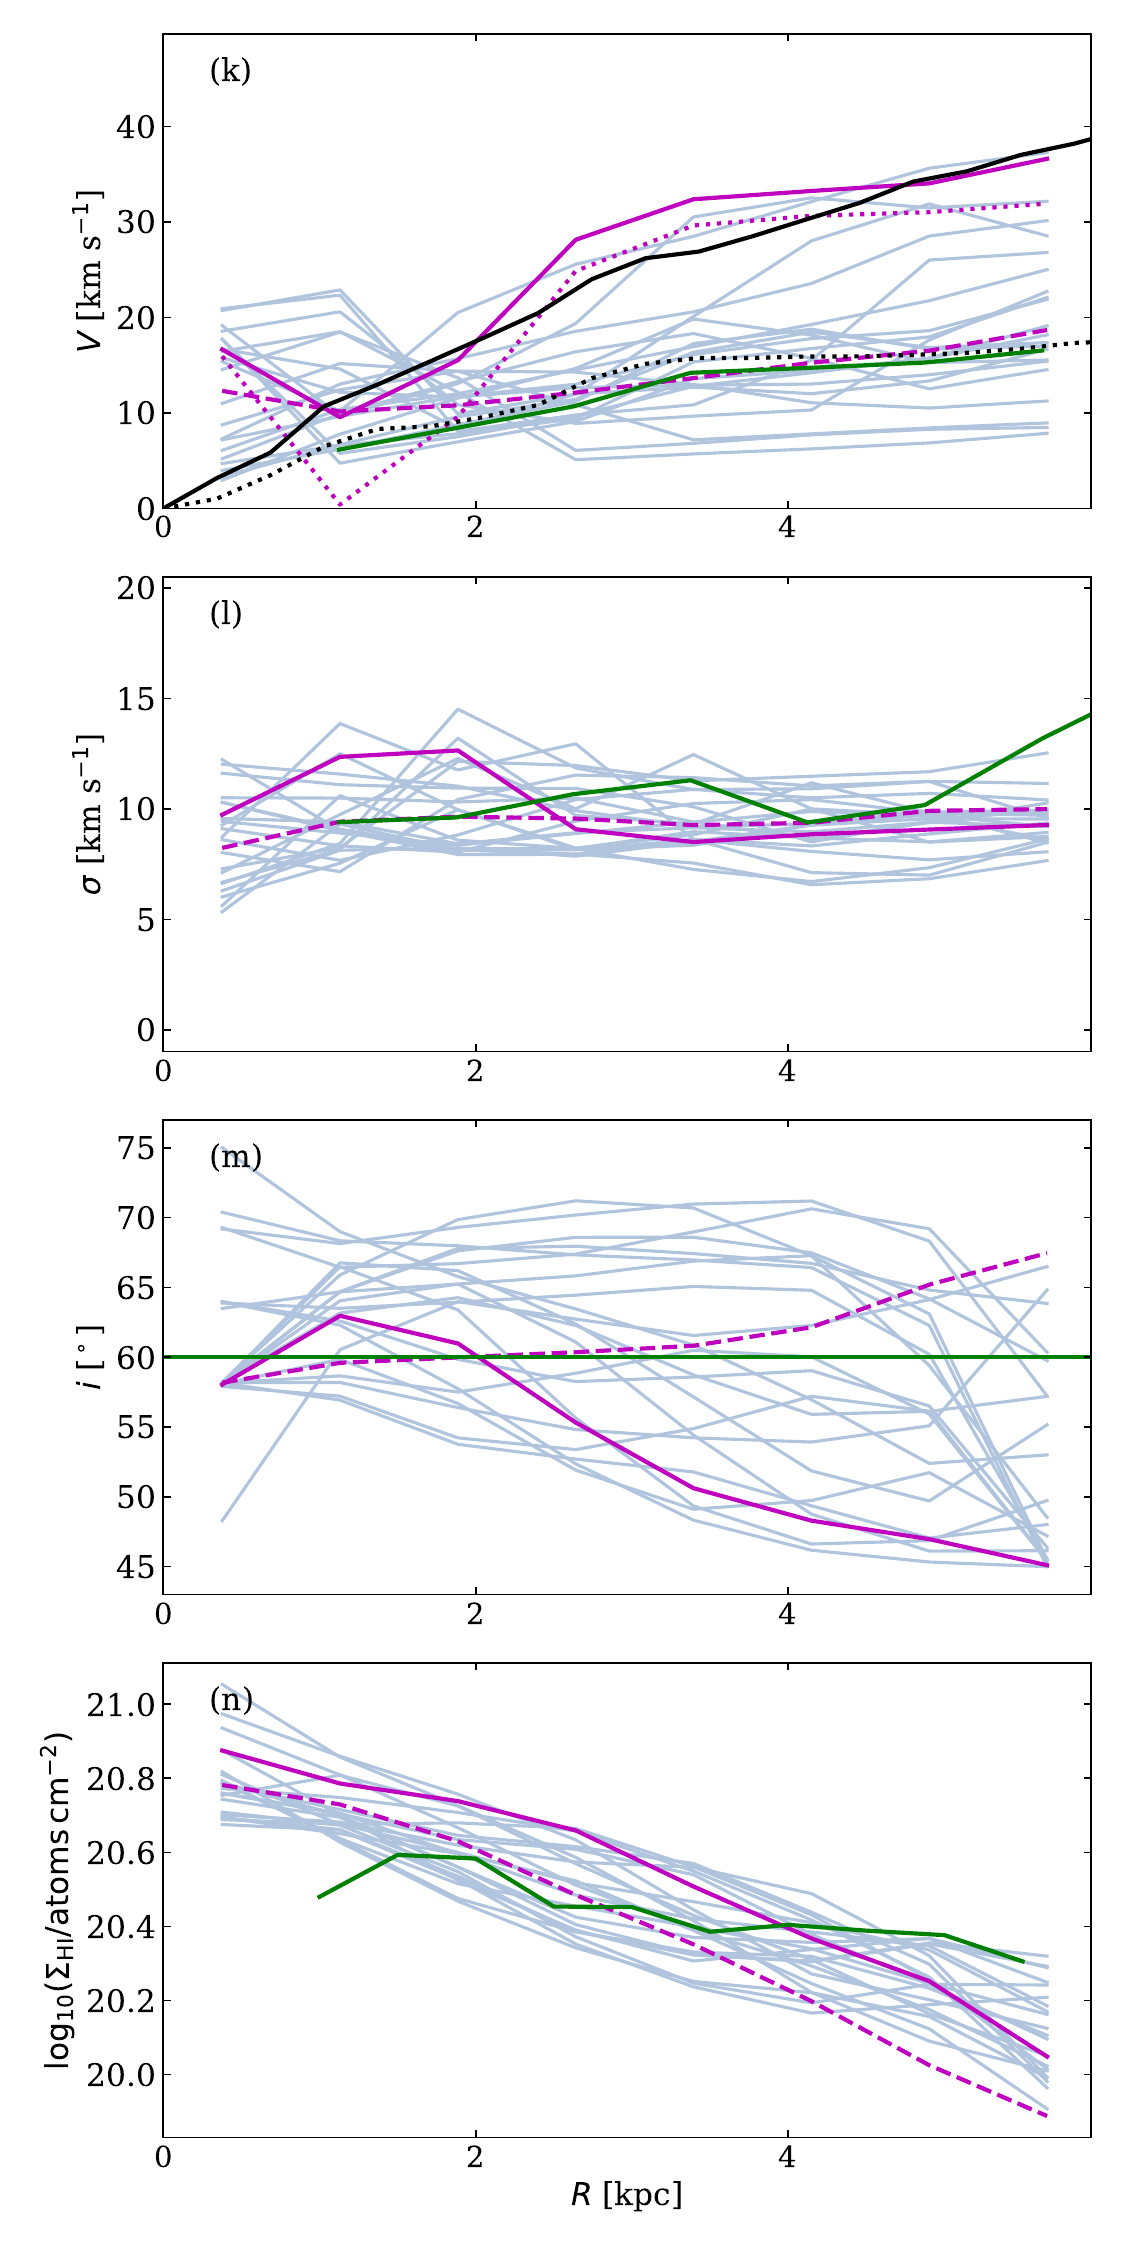}
\end{minipage}
\caption{A set of summary figures for galaxy HT-46, excluded from kinematic analysis. These include example moment maps for two orientations (panels (a)--(f); similar to Fig.~\ref{fig:visualisations}), a summary of the parameters $V_\mathrm{fid}$, $V_\mathrm{max}$, $\eta_\mathrm{rot}$, and $\eta_\mathrm{bar}$ (panels (g)--(j); similar to Fig.~\ref{fig:loops}), and a summary of the rotation curve analysis from $24$ viewing angles (panels (k)--(n); similar to Fig.~\ref{fig:rot_curves}). See description of Appendix~\ref{app:supplementary} for details.}
\label{fig:S82}
\end{figure}
\clearpage

\begin{figure}
\begin{minipage}{.9\textwidth}
\includegraphics[width=\textwidth]{../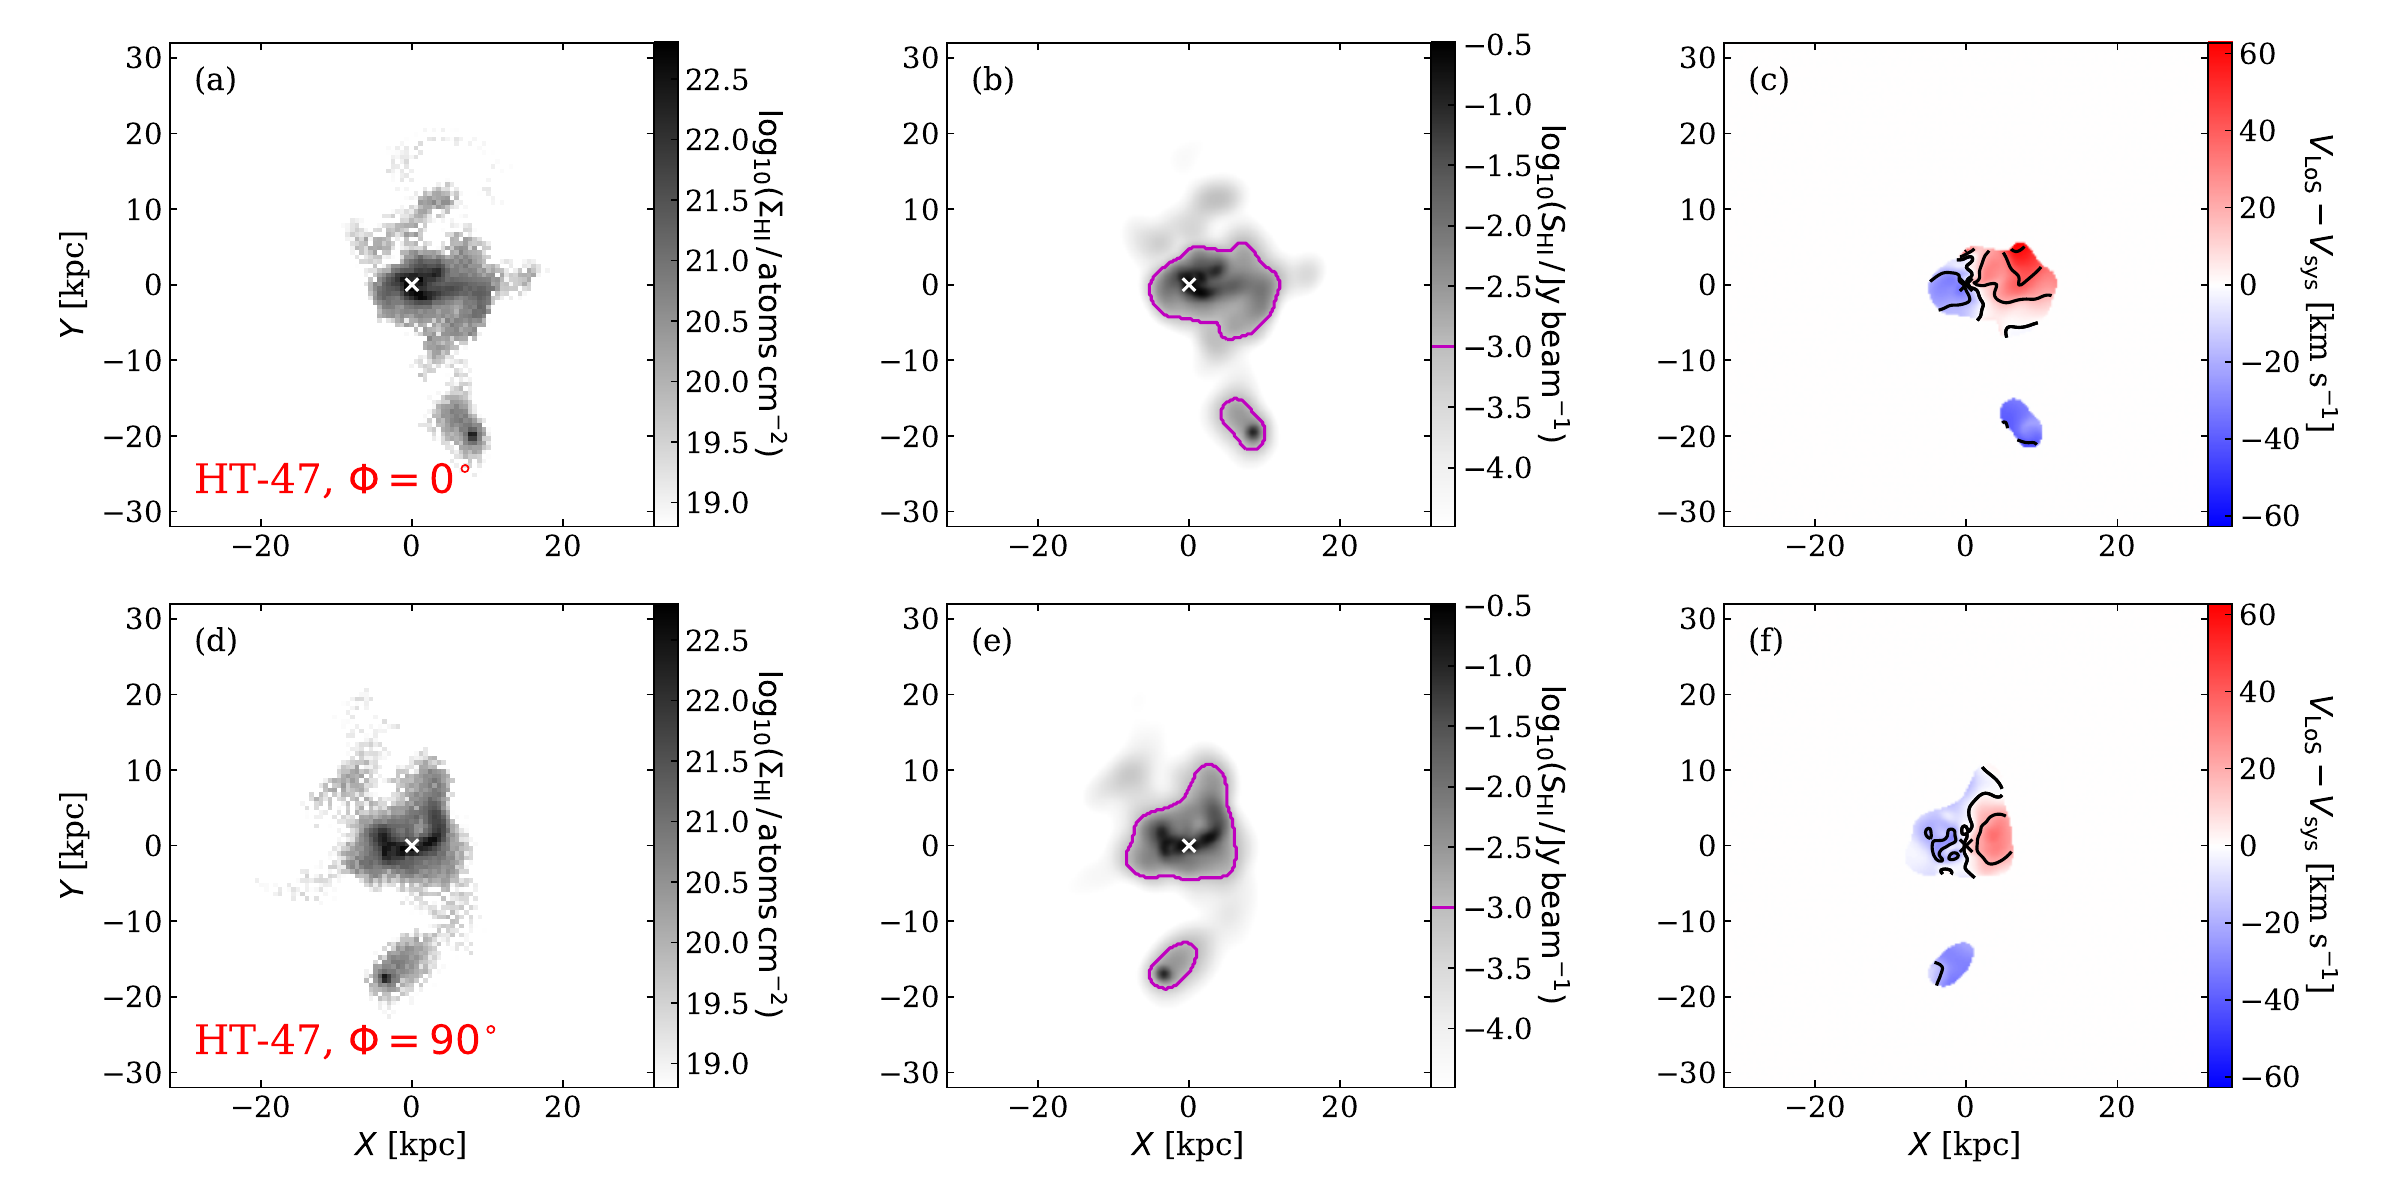}
\includegraphics[width=\textwidth]{../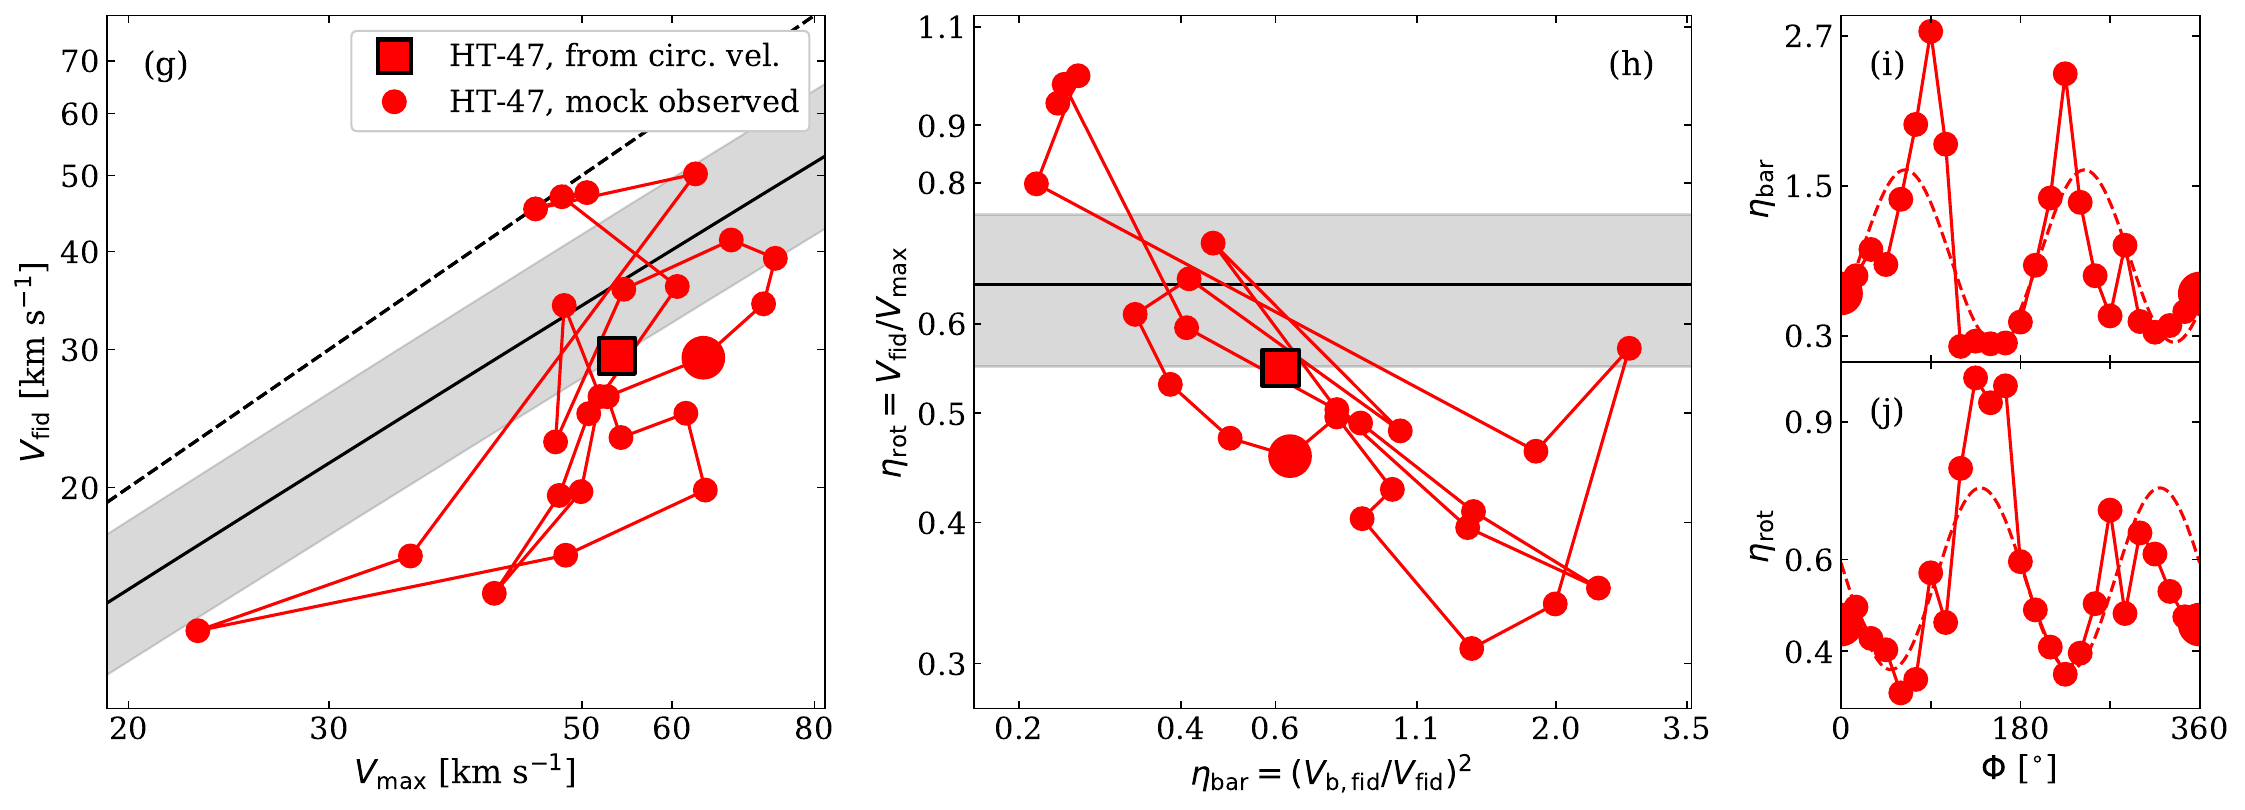}
\end{minipage}
\begin{minipage}{.4\textwidth}
\includegraphics[width=\textwidth]{../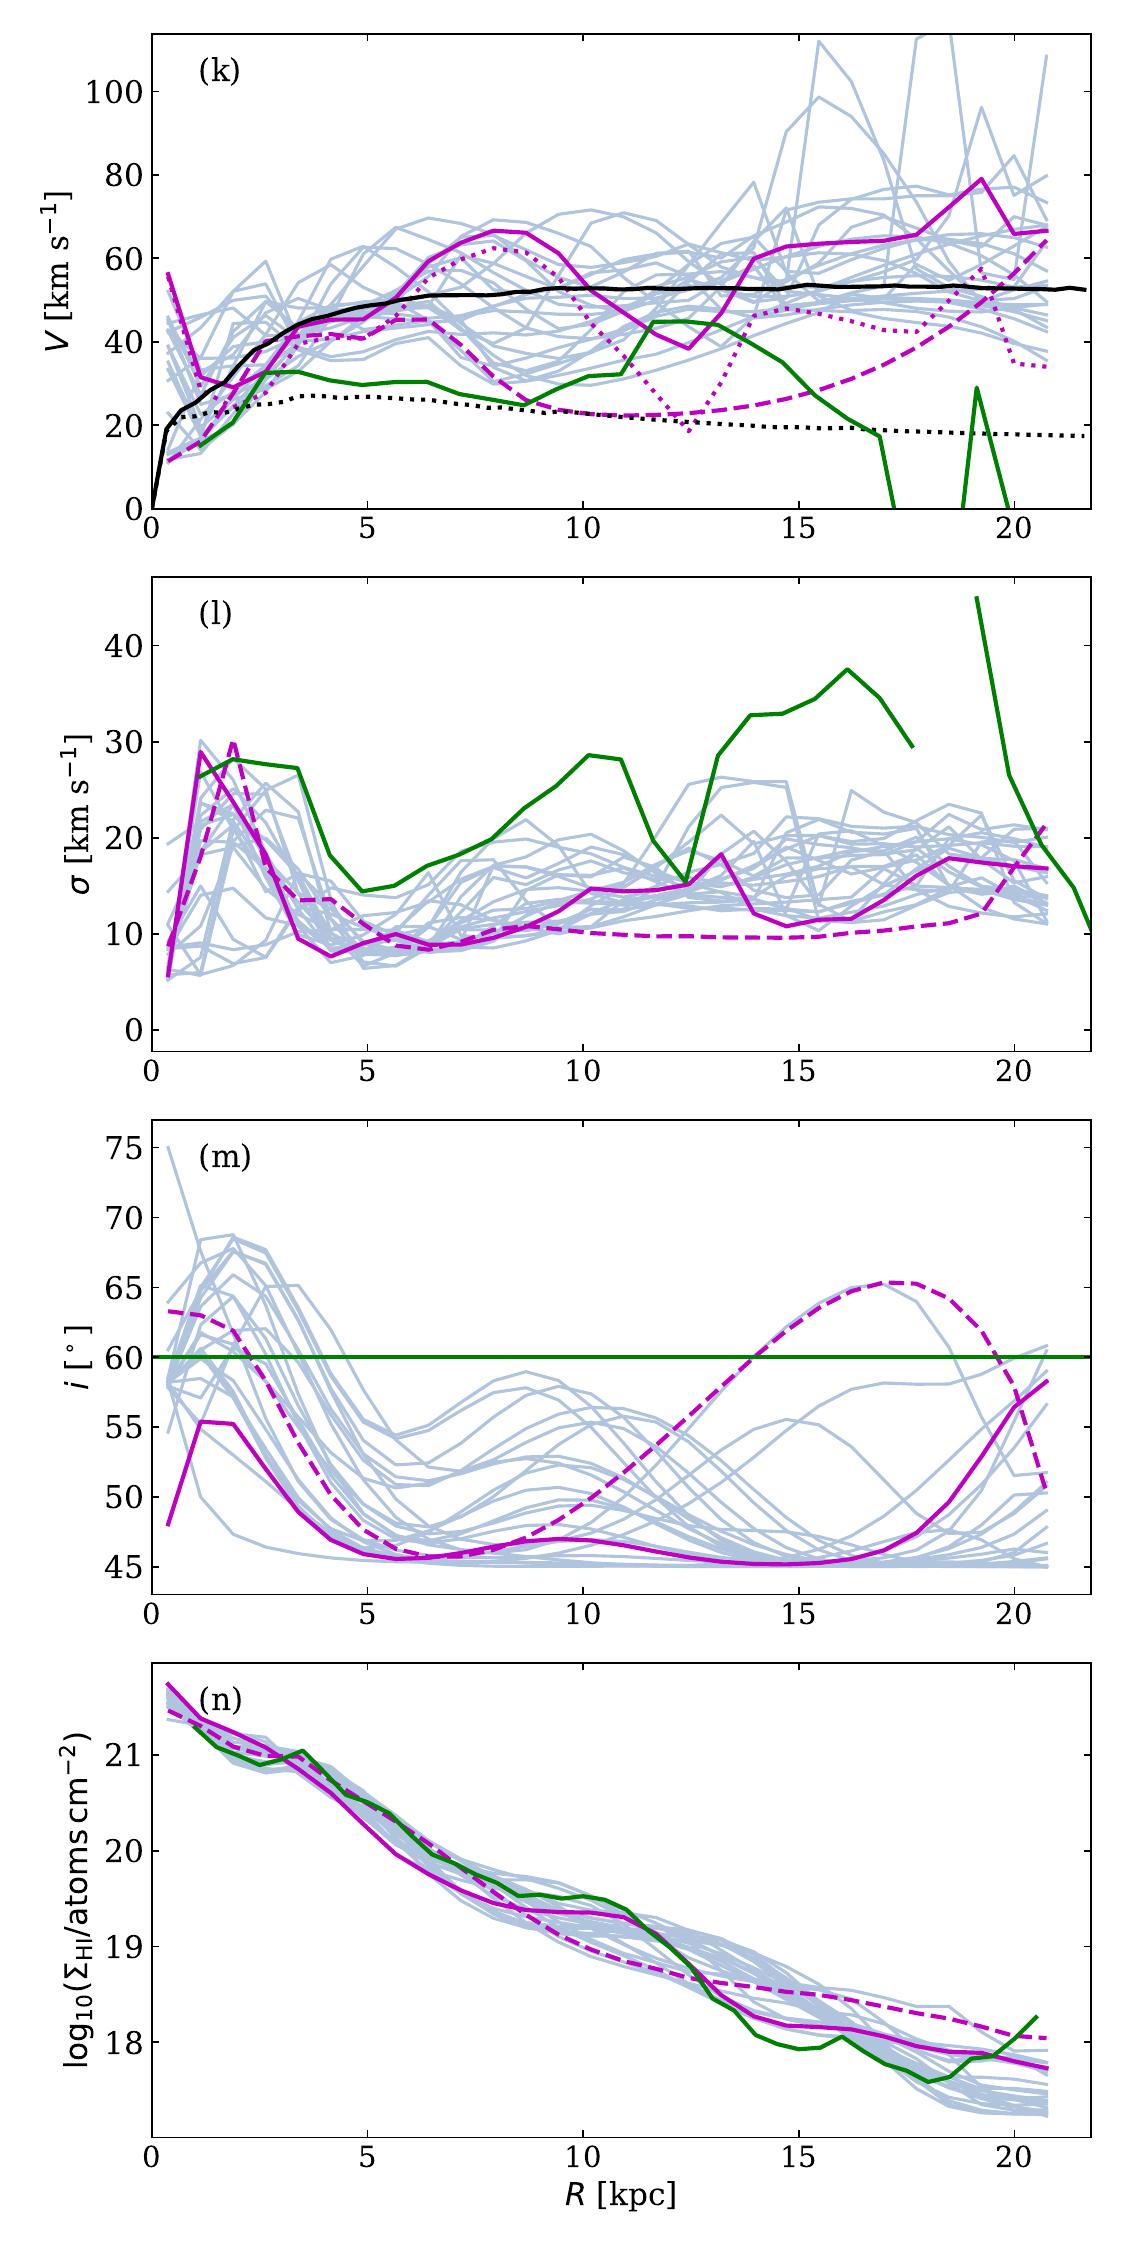}
\end{minipage}
\caption{A set of summary figures for galaxy HT-47, excluded from kinematic analysis. These include example moment maps for two orientations (panels (a)--(f); similar to Fig.~\ref{fig:visualisations}), a summary of the parameters $V_\mathrm{fid}$, $V_\mathrm{max}$, $\eta_\mathrm{rot}$, and $\eta_\mathrm{bar}$ (panels (g)--(j); similar to Fig.~\ref{fig:loops}), and a summary of the rotation curve analysis from $24$ viewing angles (panels (k)--(n); similar to Fig.~\ref{fig:rot_curves}). See description of Appendix~\ref{app:supplementary} for details.}
\label{fig:S83}
\end{figure}
\clearpage

\begin{figure}
\begin{minipage}{.9\textwidth}
\includegraphics[width=\textwidth]{../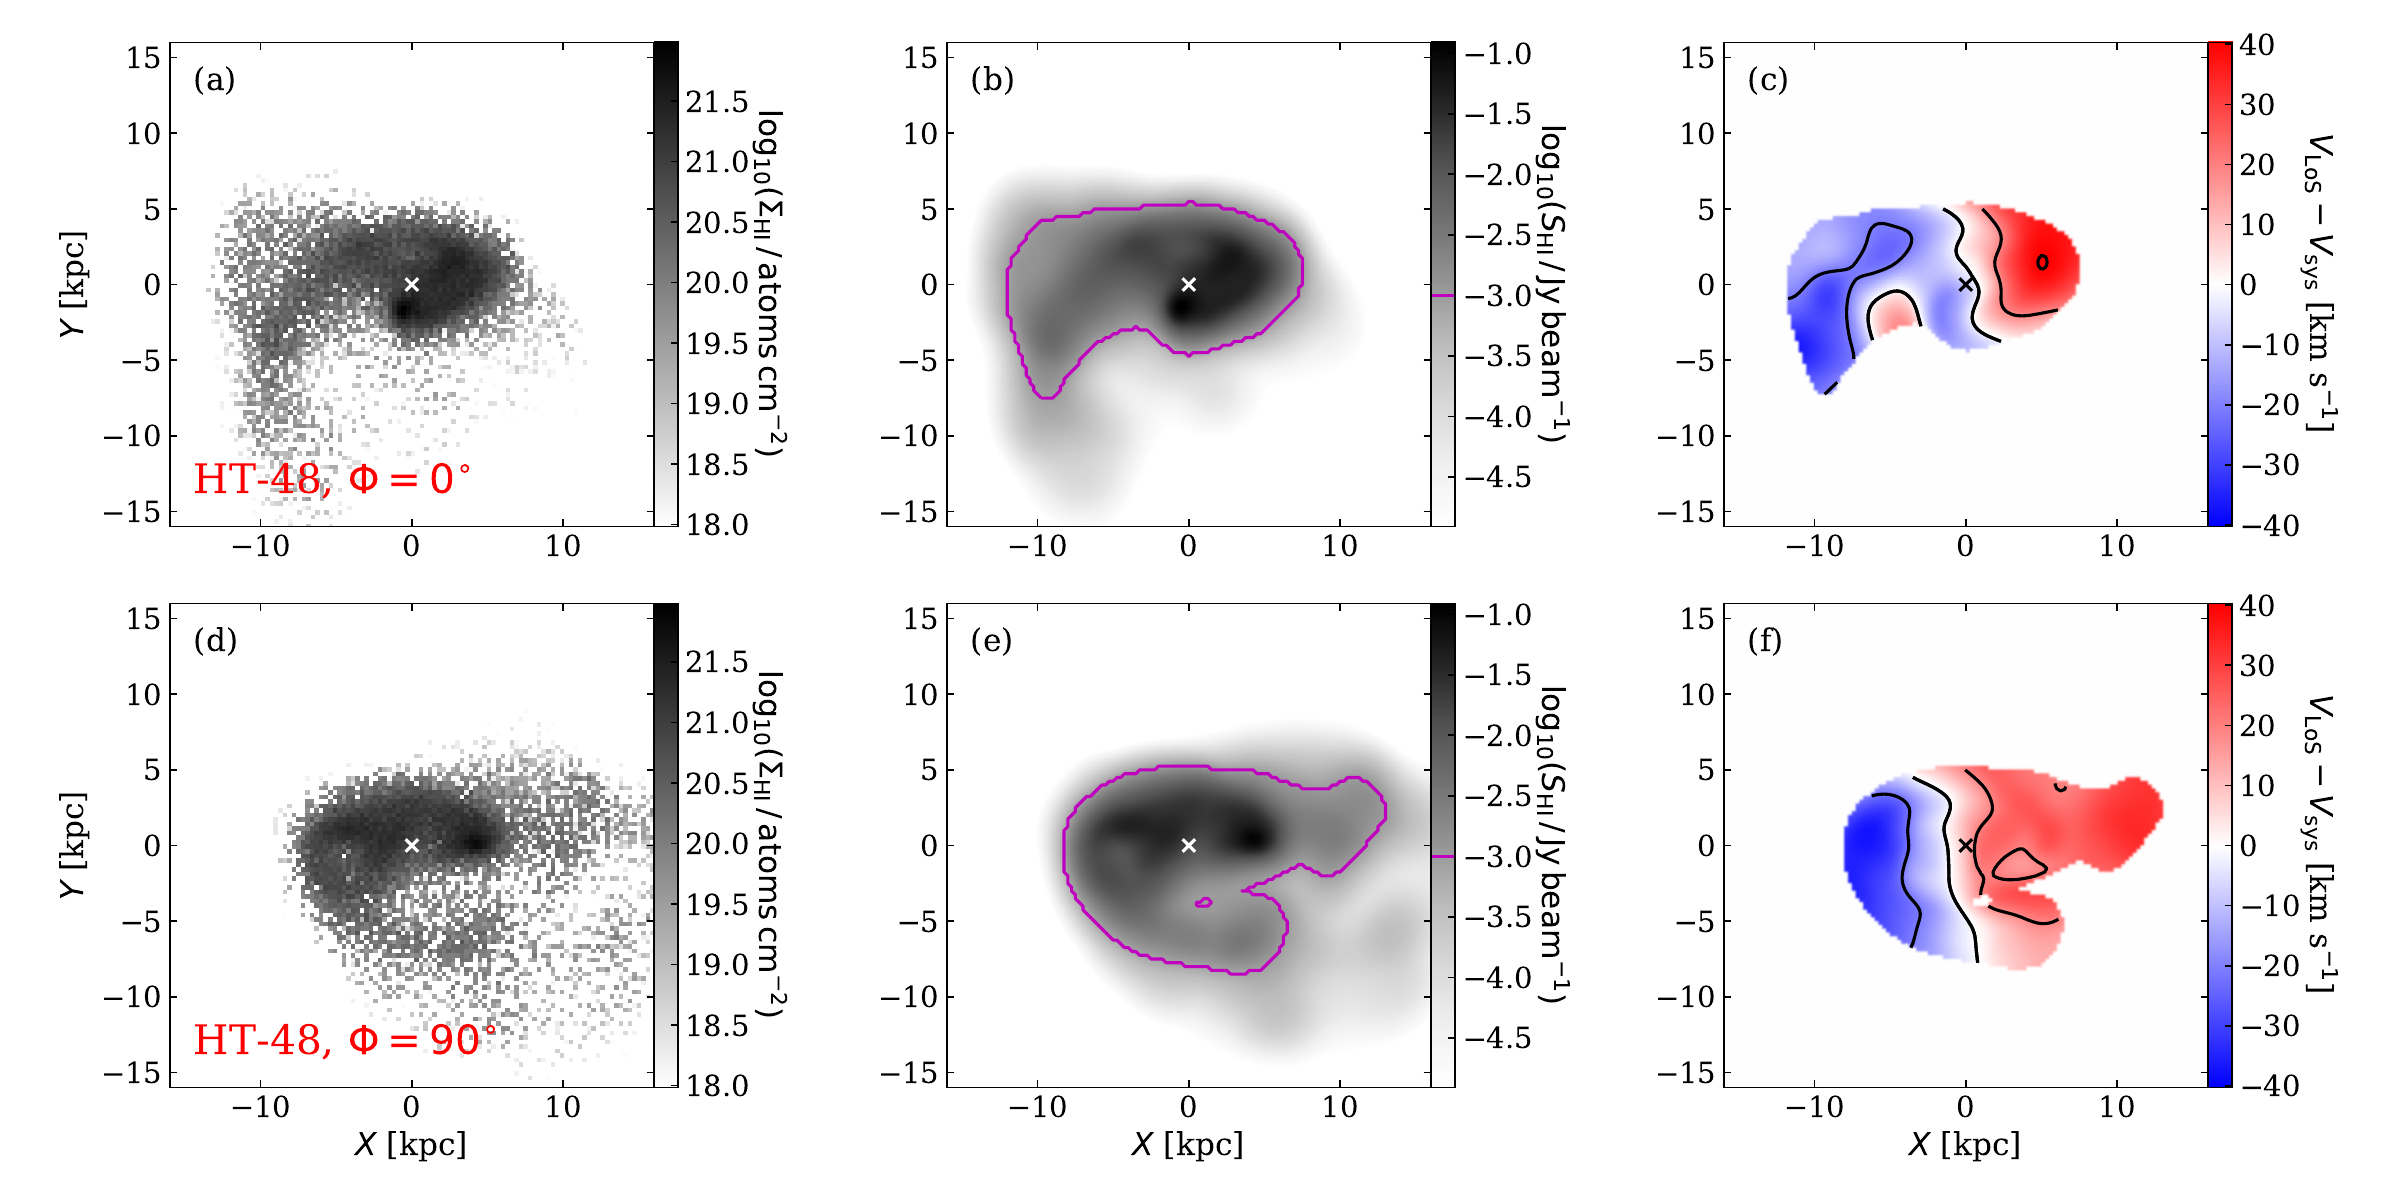}
\includegraphics[width=\textwidth]{../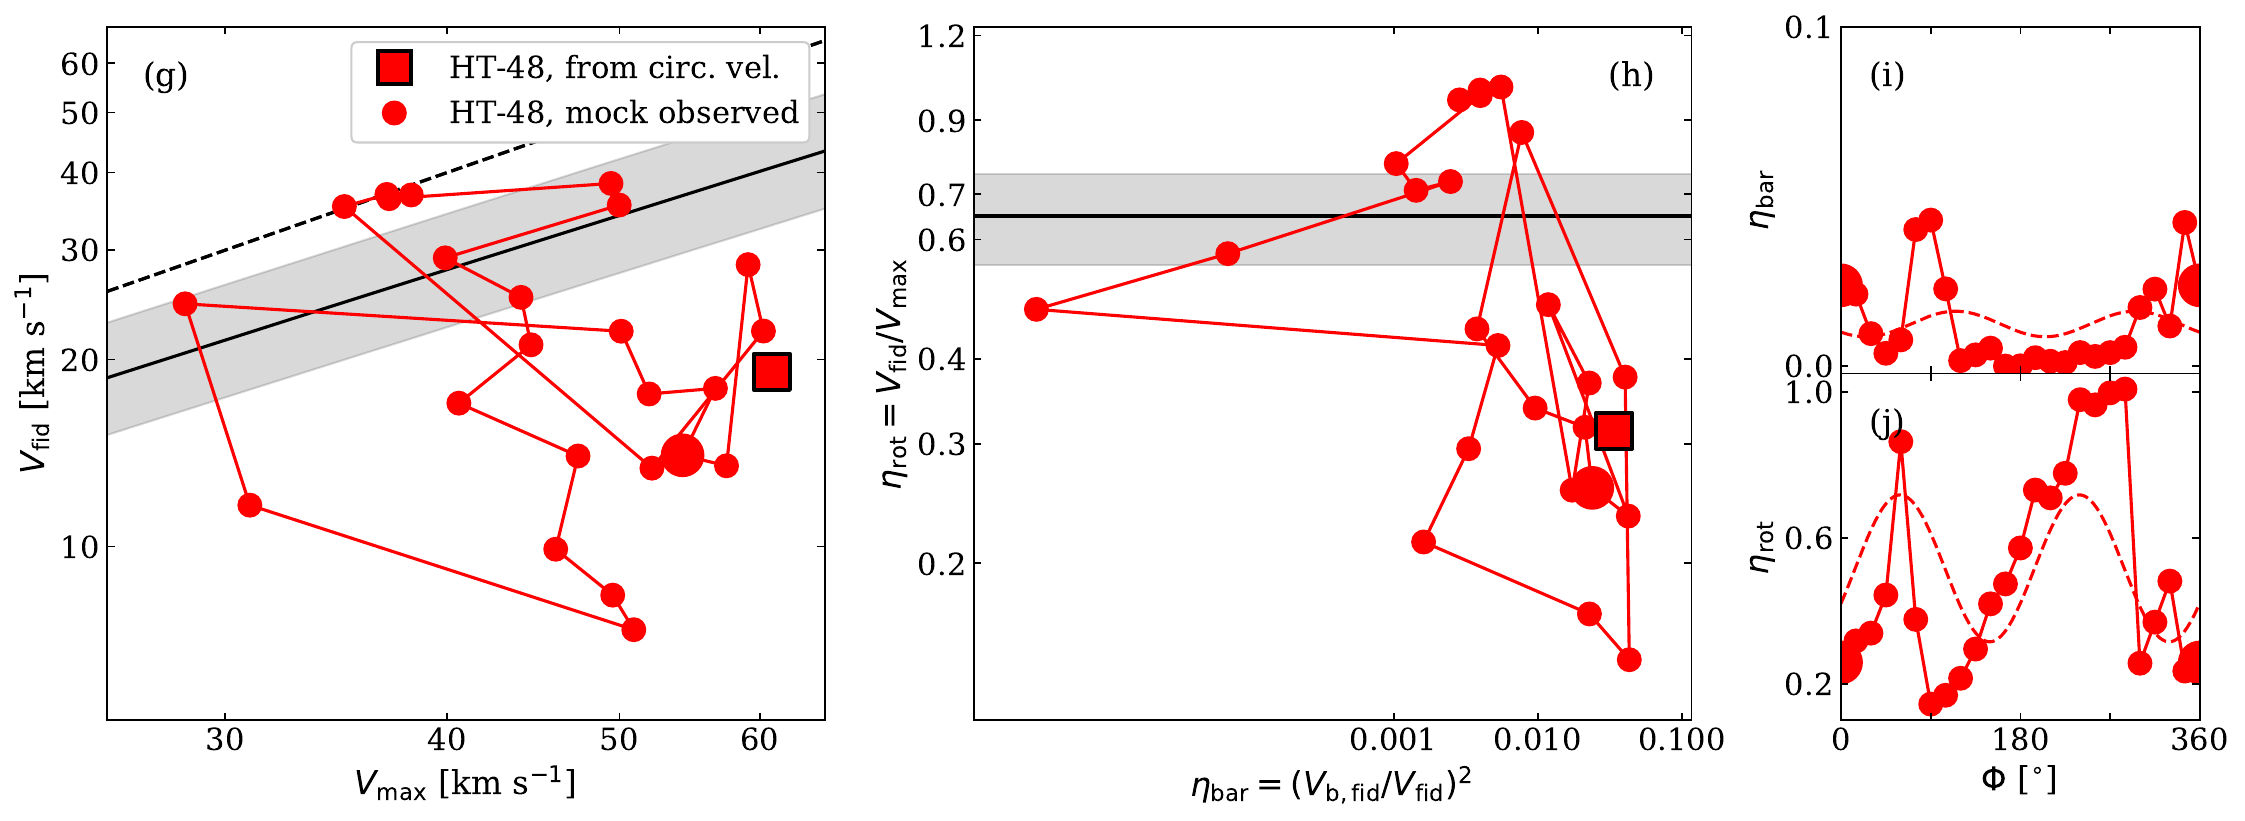}
\end{minipage}
\begin{minipage}{.4\textwidth}
\includegraphics[width=\textwidth]{../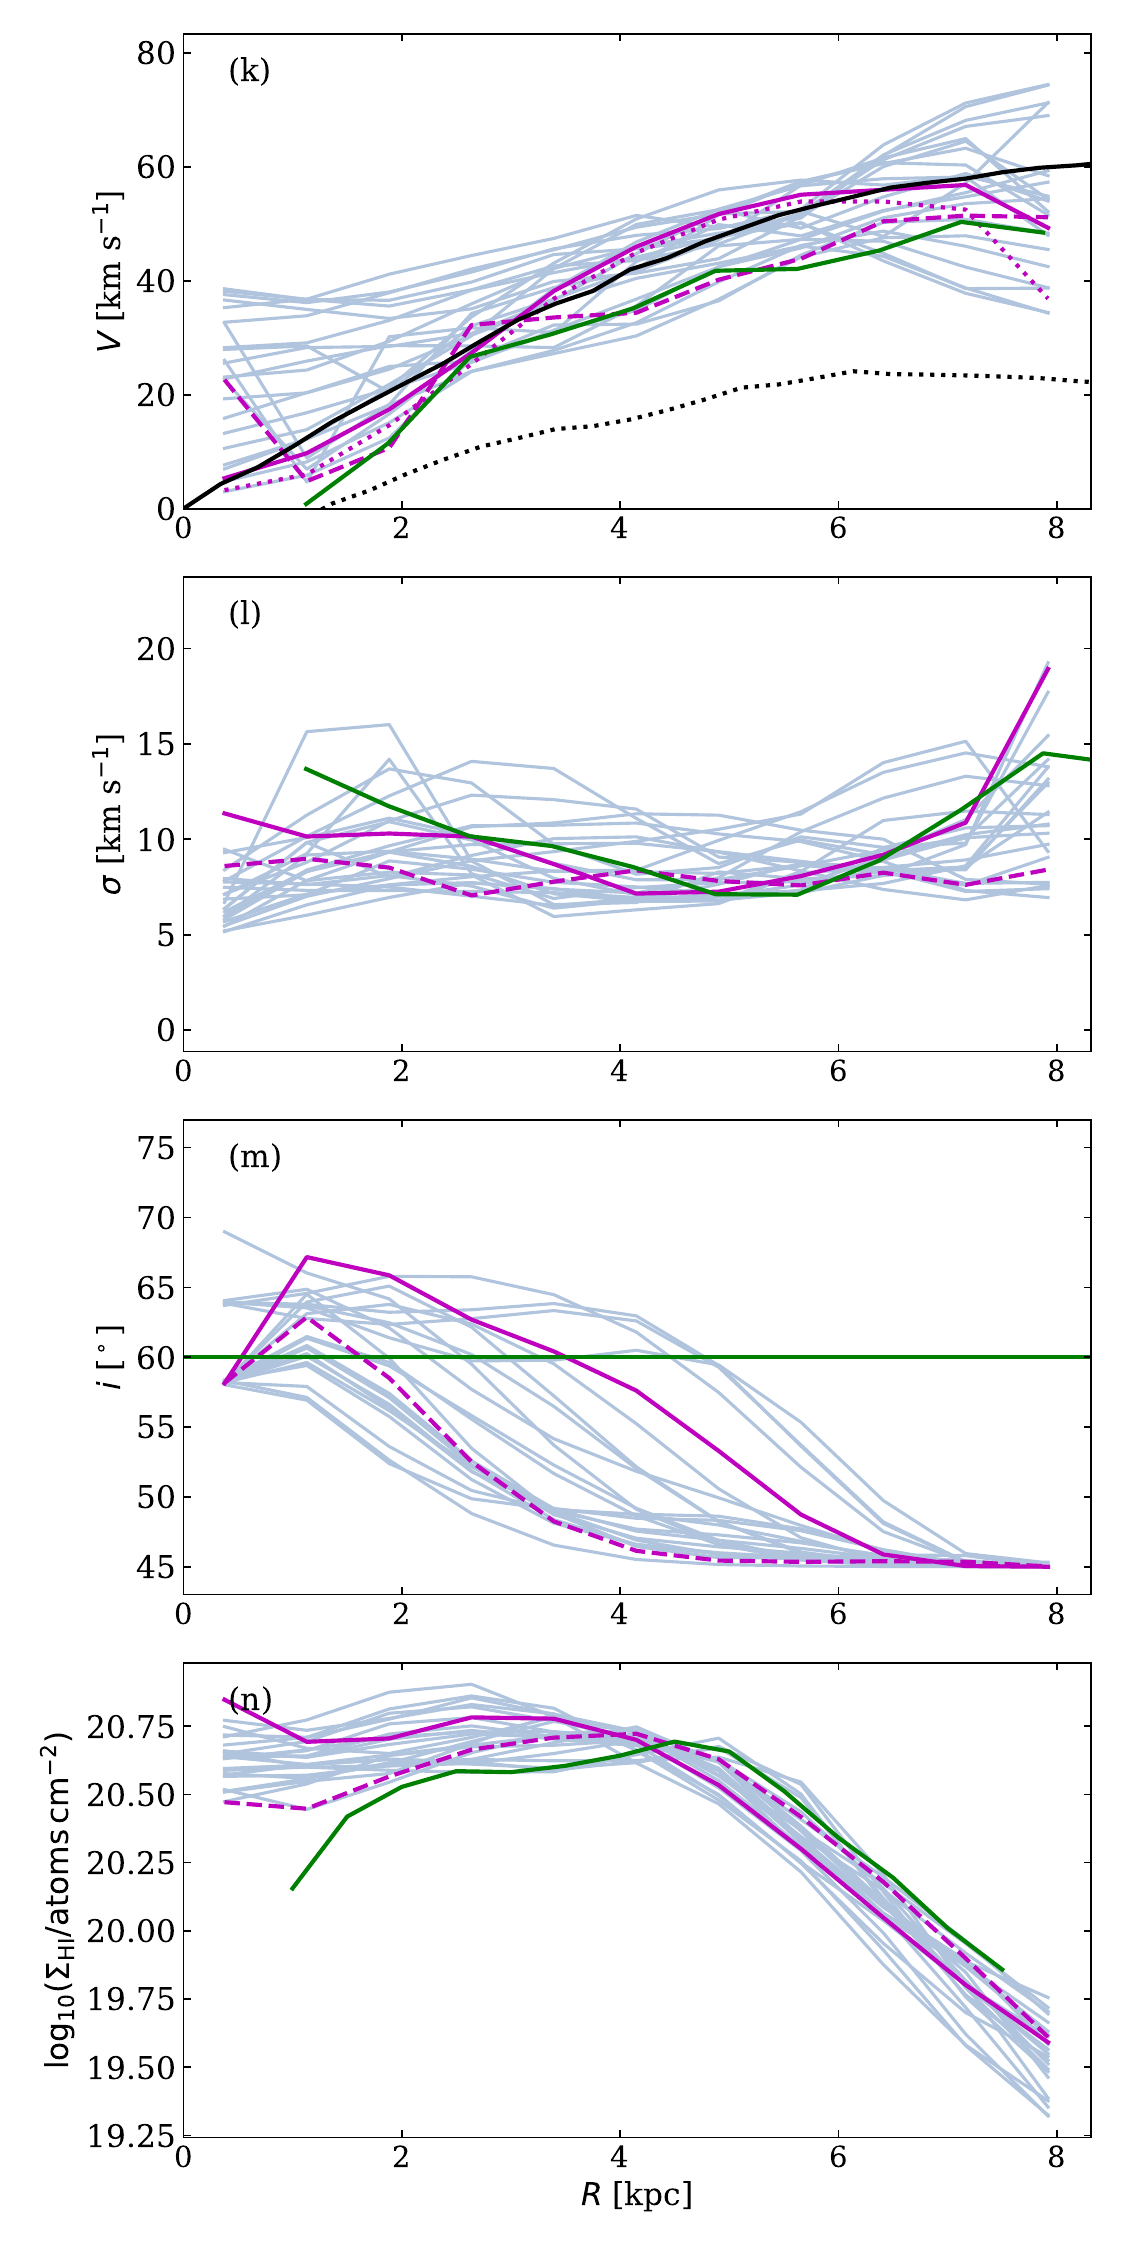}
\end{minipage}
\caption{A set of summary figures for galaxy HT-48, excluded from kinematic analysis. These include example moment maps for two orientations (panels (a)--(f); similar to Fig.~\ref{fig:visualisations}), a summary of the parameters $V_\mathrm{fid}$, $V_\mathrm{max}$, $\eta_\mathrm{rot}$, and $\eta_\mathrm{bar}$ (panels (g)--(j); similar to Fig.~\ref{fig:loops}), and a summary of the rotation curve analysis from $24$ viewing angles (panels (k)--(n); similar to Fig.~\ref{fig:rot_curves}). See description of Appendix~\ref{app:supplementary} for details.}
\label{fig:S84}
\end{figure}
\clearpage

\begin{figure}
\begin{minipage}{.9\textwidth}
\includegraphics[width=\textwidth]{../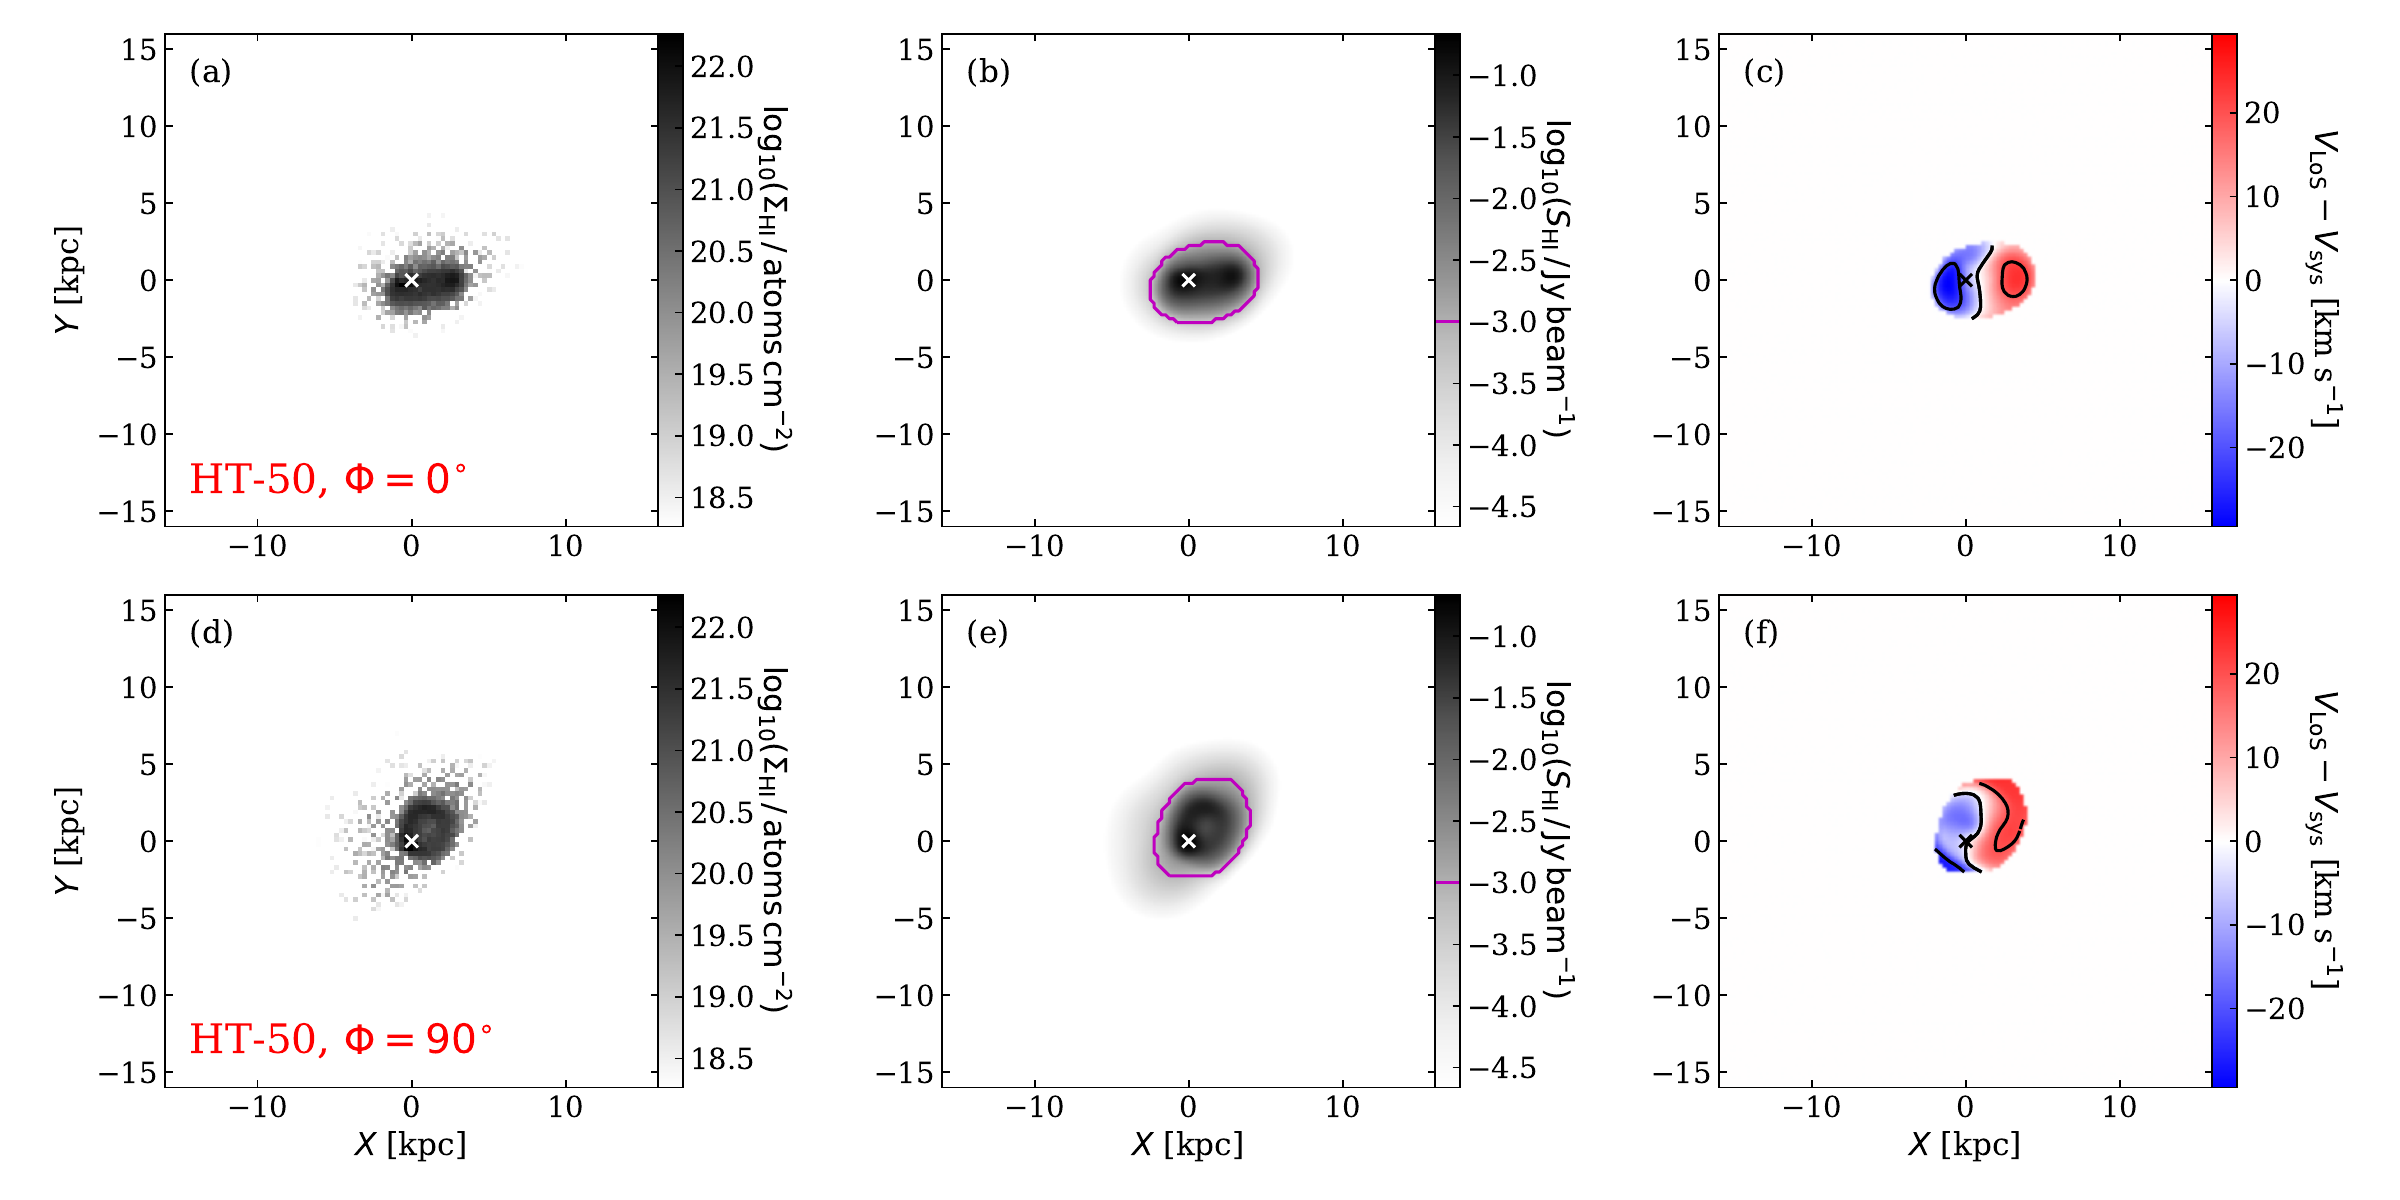}
\includegraphics[width=\textwidth]{../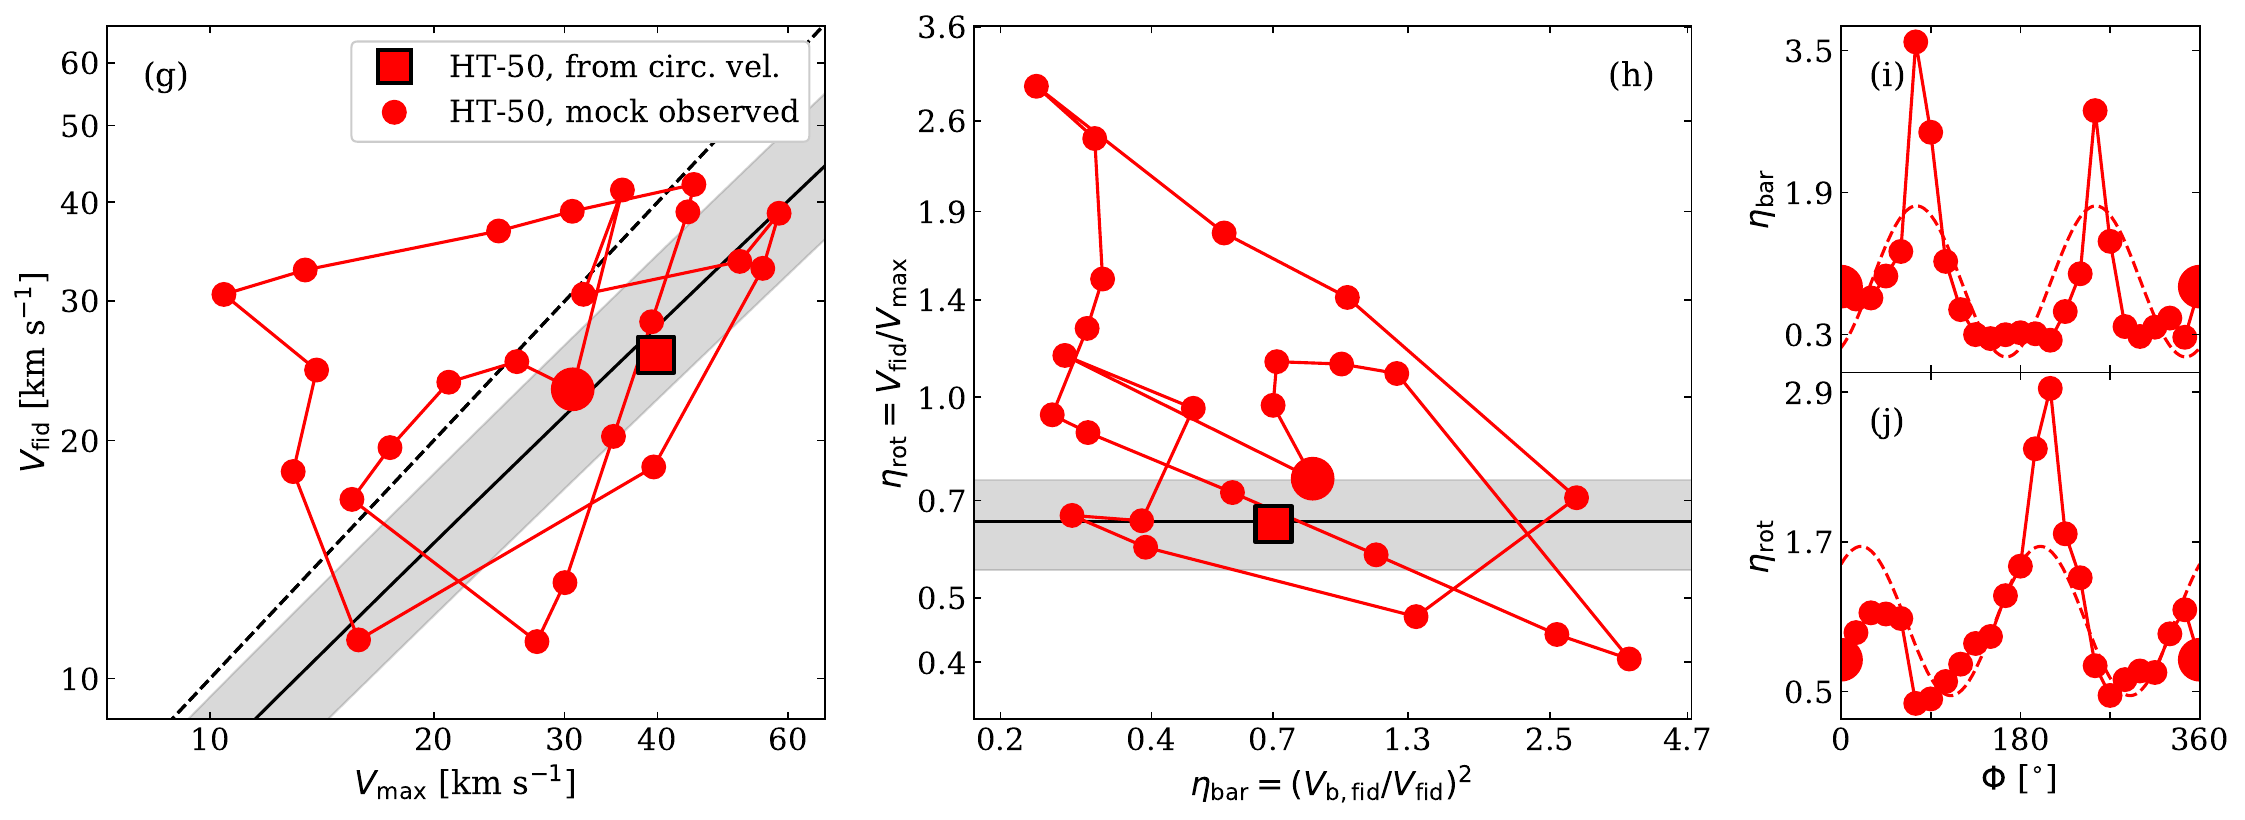}
\end{minipage}
\begin{minipage}{.4\textwidth}
\includegraphics[width=\textwidth]{../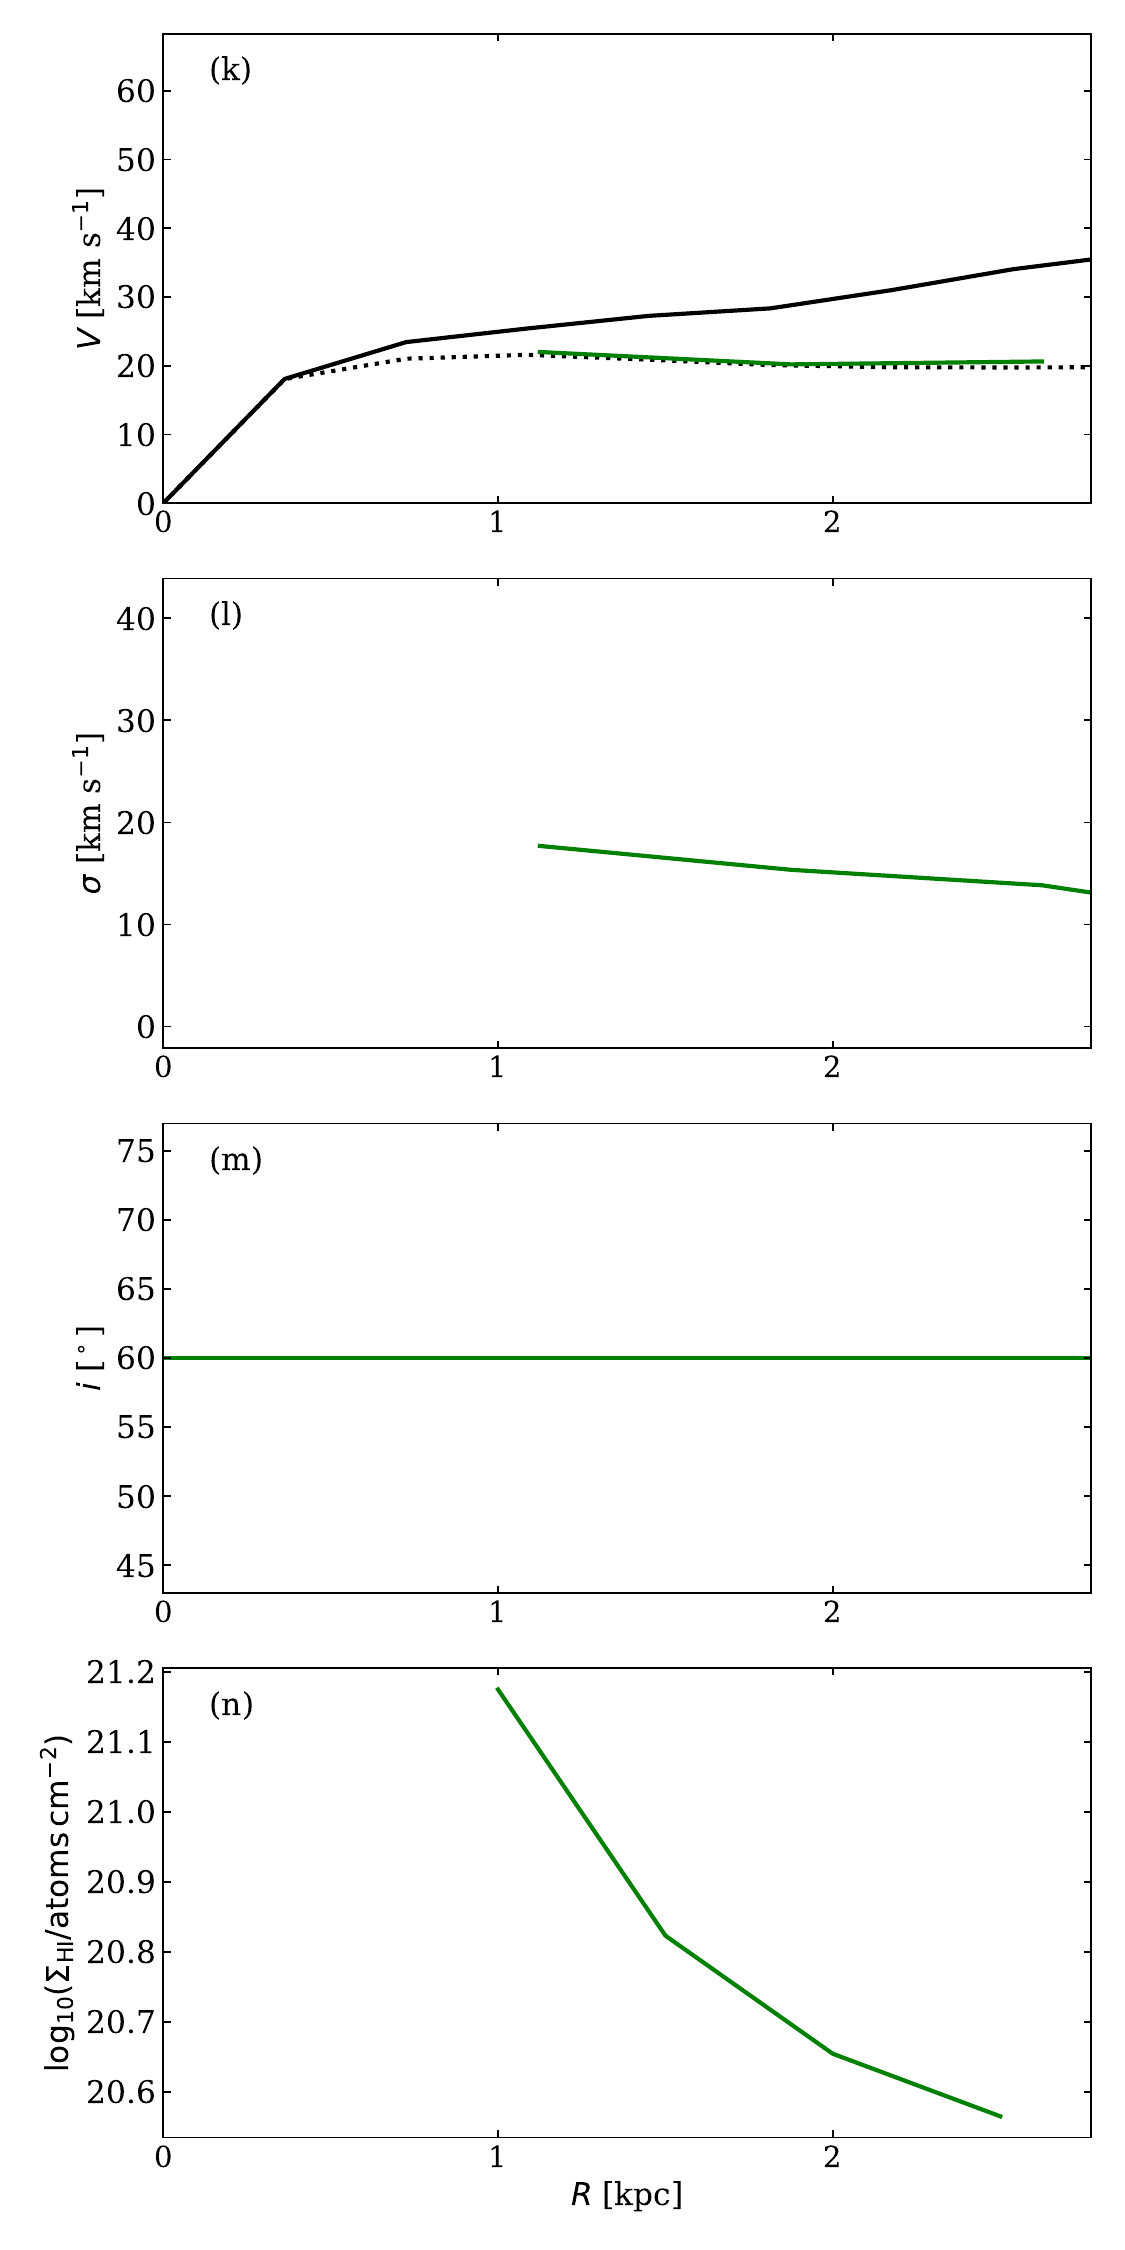}
\end{minipage}
\caption{A set of summary figures for galaxy HT-50, excluded from kinematic analysis. These include example moment maps for two orientations (panels (a)--(f); similar to Fig.~\ref{fig:visualisations}), a summary of the parameters $V_\mathrm{fid}$, $V_\mathrm{max}$, $\eta_\mathrm{rot}$, and $\eta_\mathrm{bar}$ (panels (g)--(j); similar to Fig.~\ref{fig:loops}), and a summary of the rotation curve analysis from $24$ viewing angles (panels (k)--(n); similar to Fig.~\ref{fig:rot_curves}). See description of Appendix~\ref{app:supplementary} for details.}
\label{fig:S85}
\end{figure}
\clearpage

\begin{figure}
\begin{minipage}{.9\textwidth}
\includegraphics[width=\textwidth]{../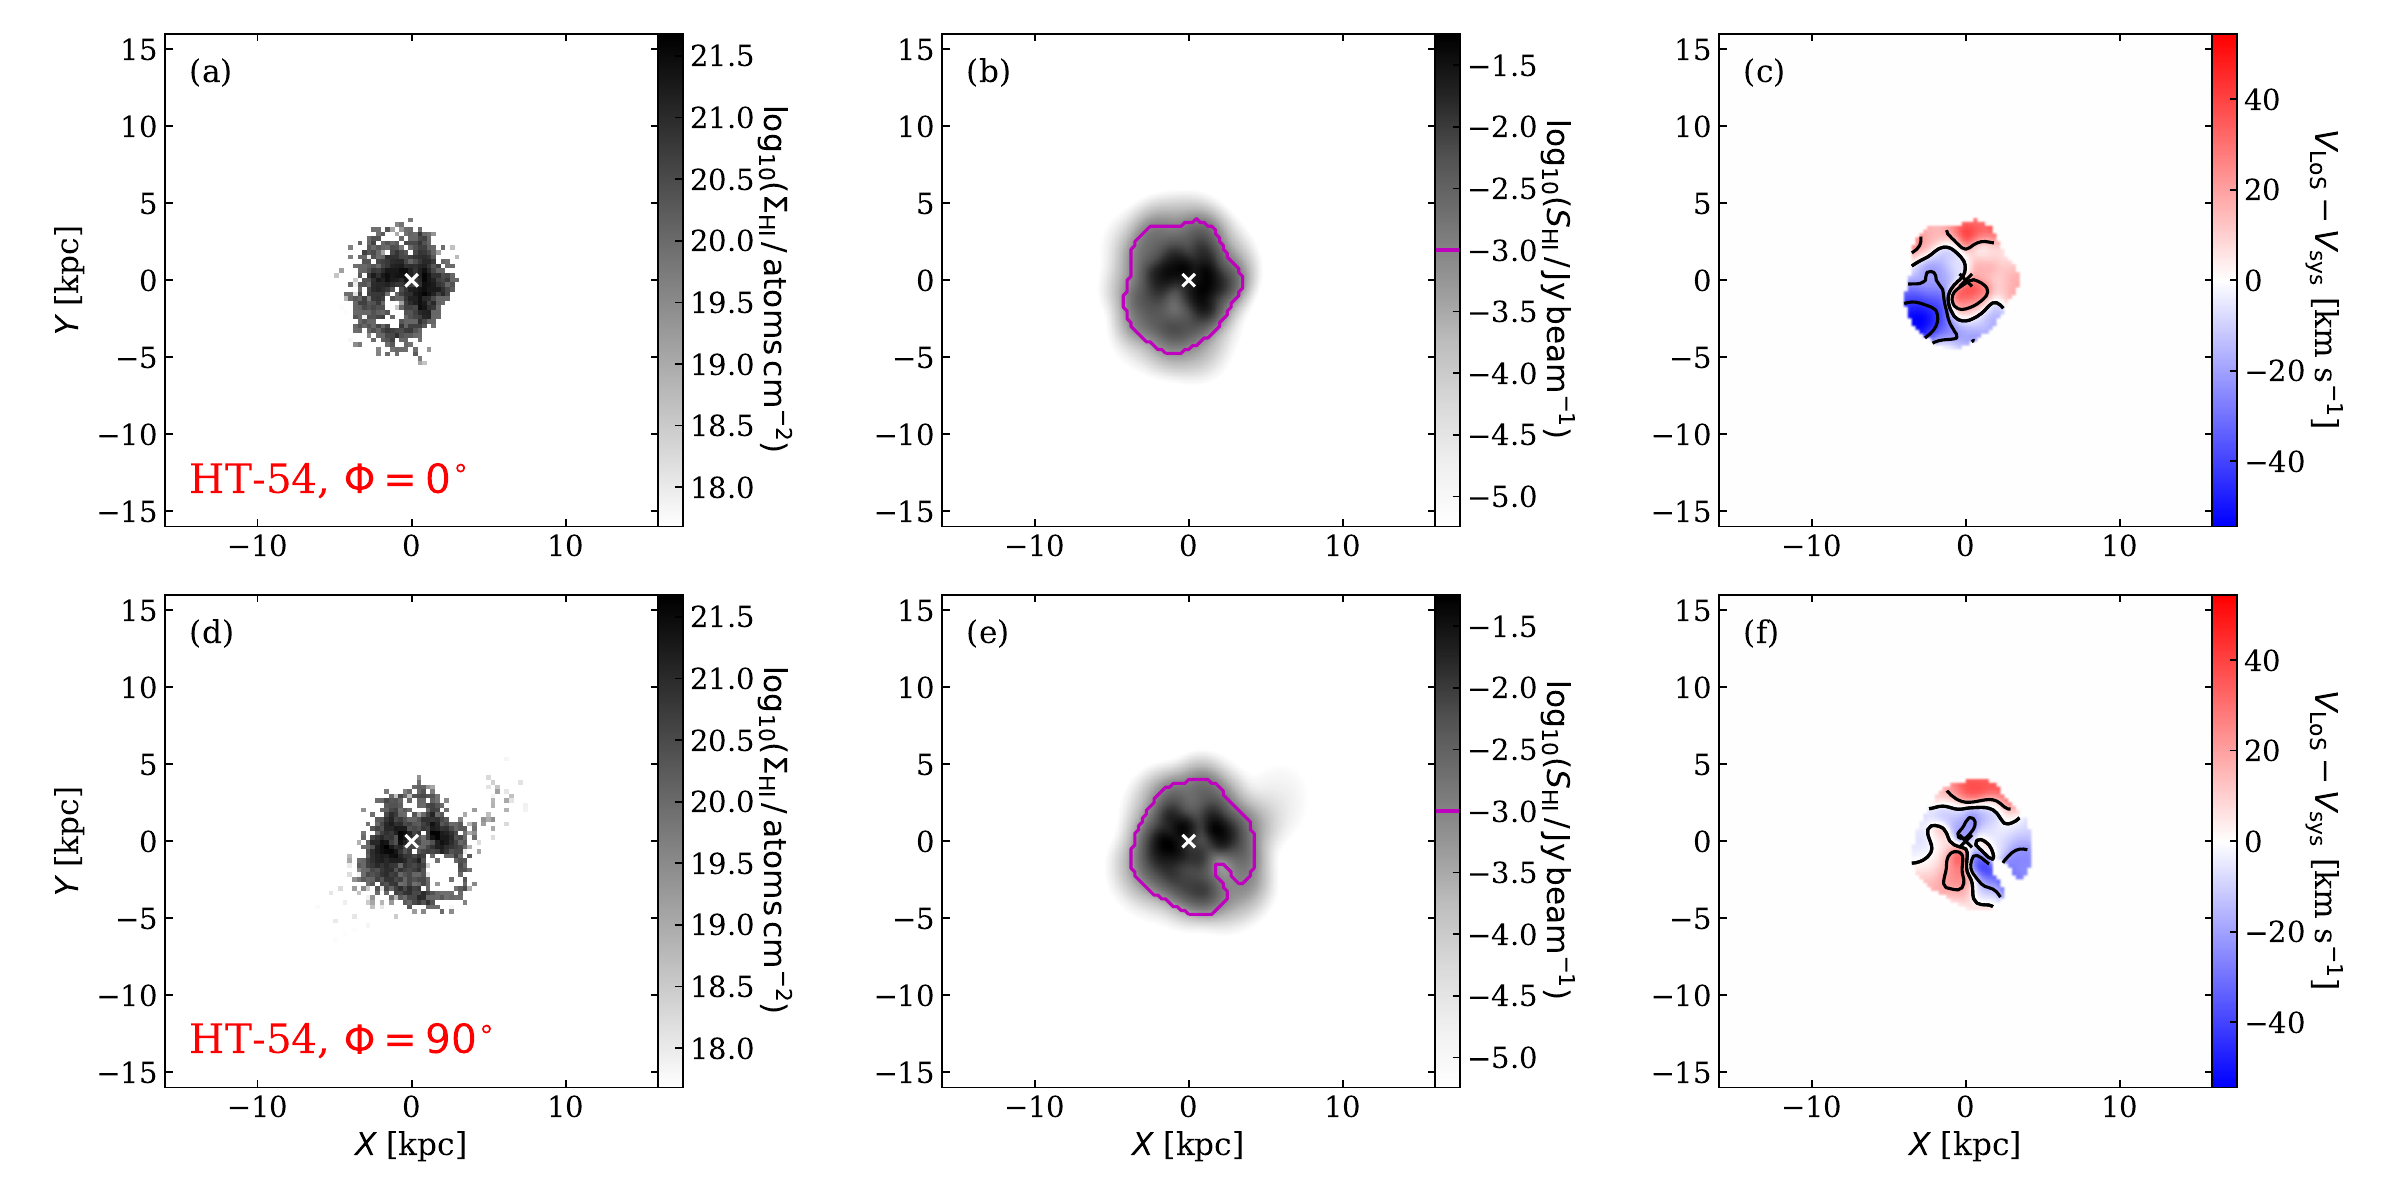}
\end{minipage}
\begin{minipage}{.4\textwidth}
\includegraphics[width=\textwidth]{../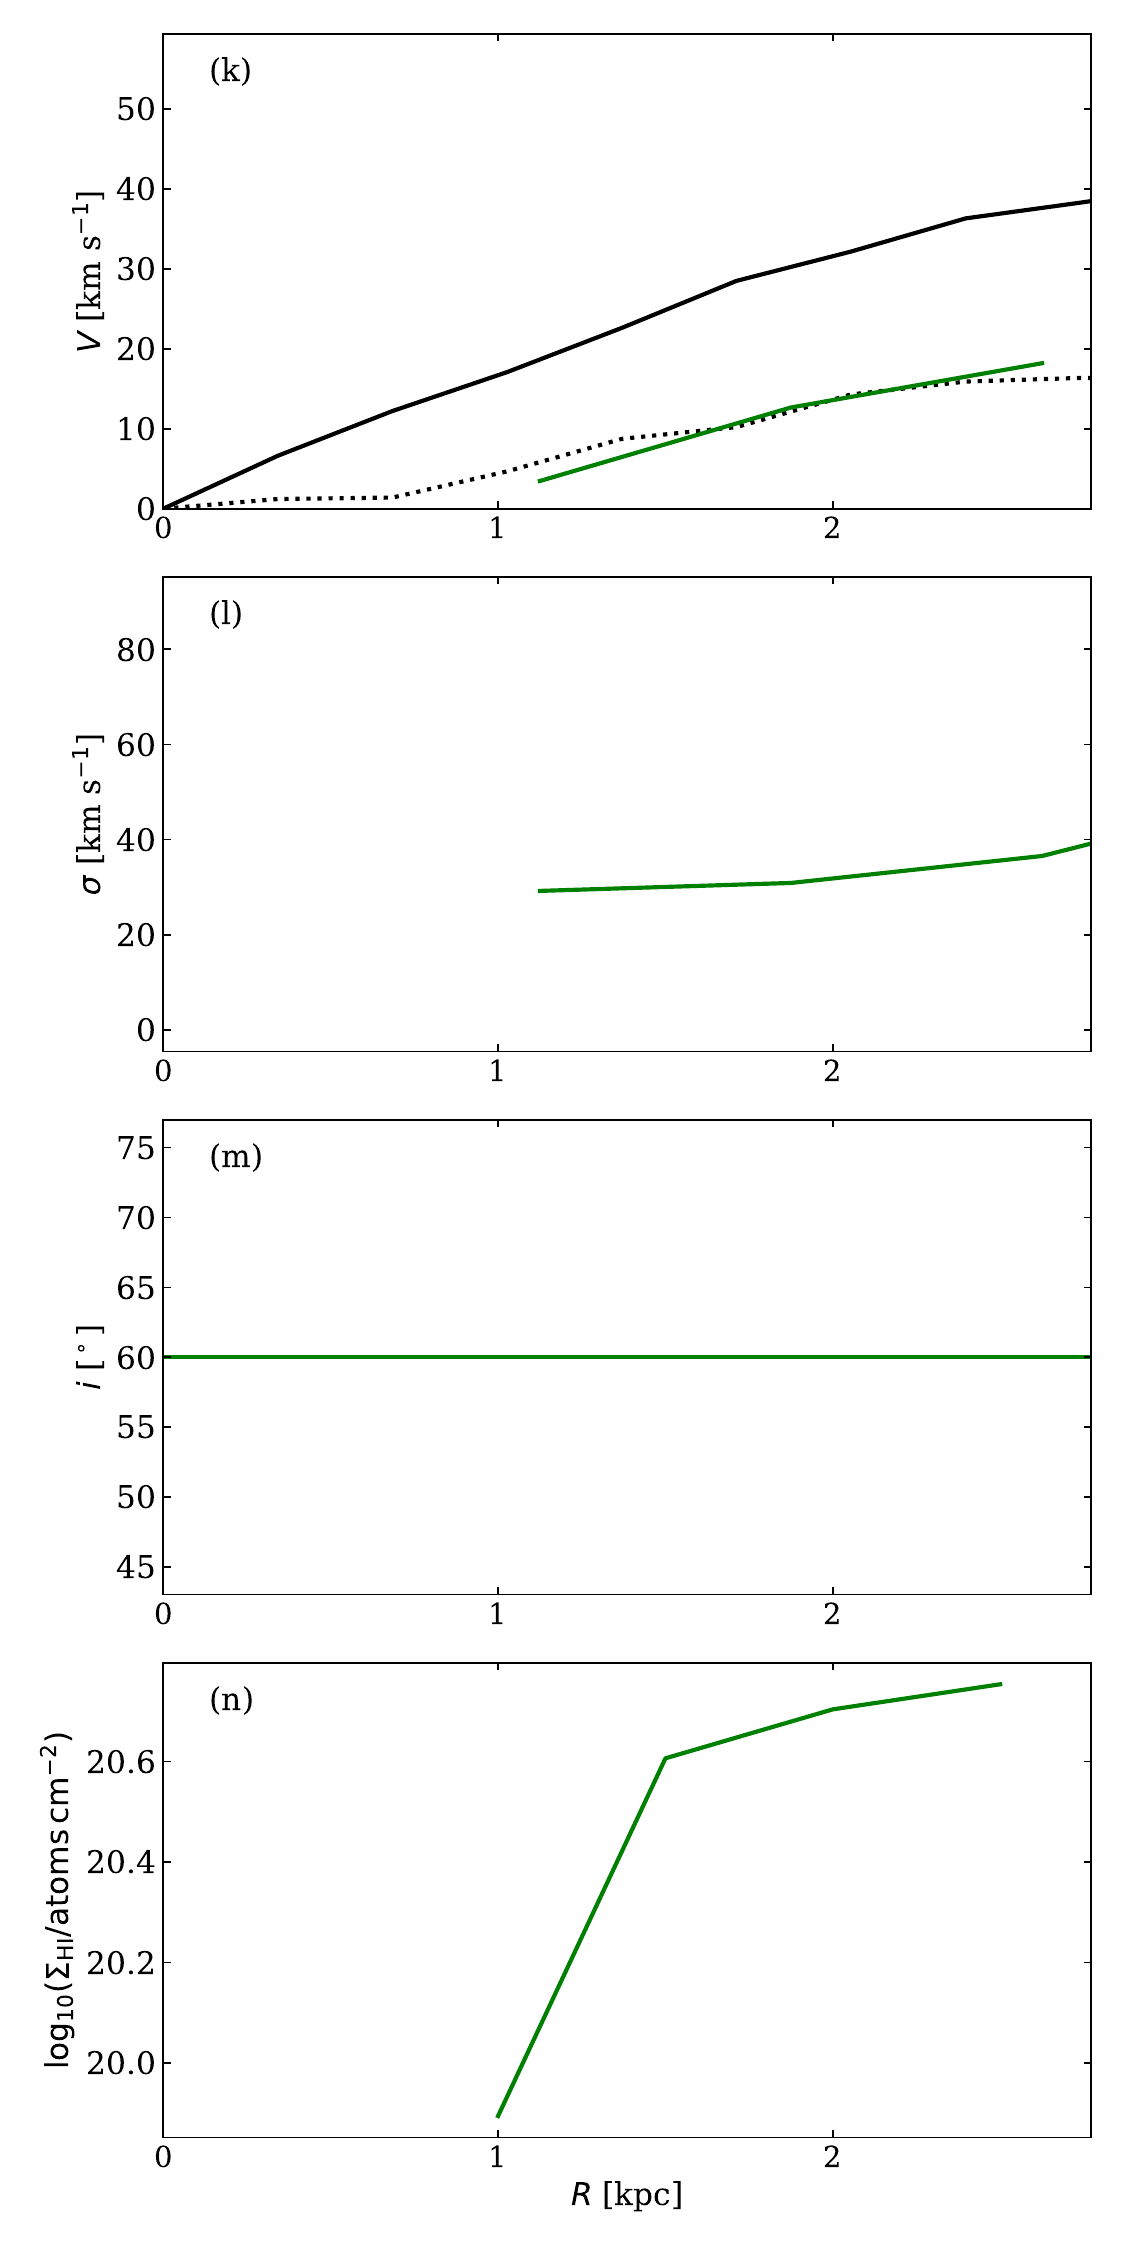}
\end{minipage}
\caption{A set of summary figures for galaxy HT-54, excluded from kinematic analysis. These include example moment maps for two orientations (panels (a)--(f); similar to Fig.~\ref{fig:visualisations}) and a summary of the rotation curve analysis from $24$ viewing angles (panels (k)--(n); similar to Fig.~\ref{fig:rot_curves}). See description of Appendix~\ref{app:supplementary} for details.}
\label{fig:S86}
\end{figure}
\clearpage

\begin{figure}
\begin{minipage}{.9\textwidth}
\includegraphics[width=\textwidth]{../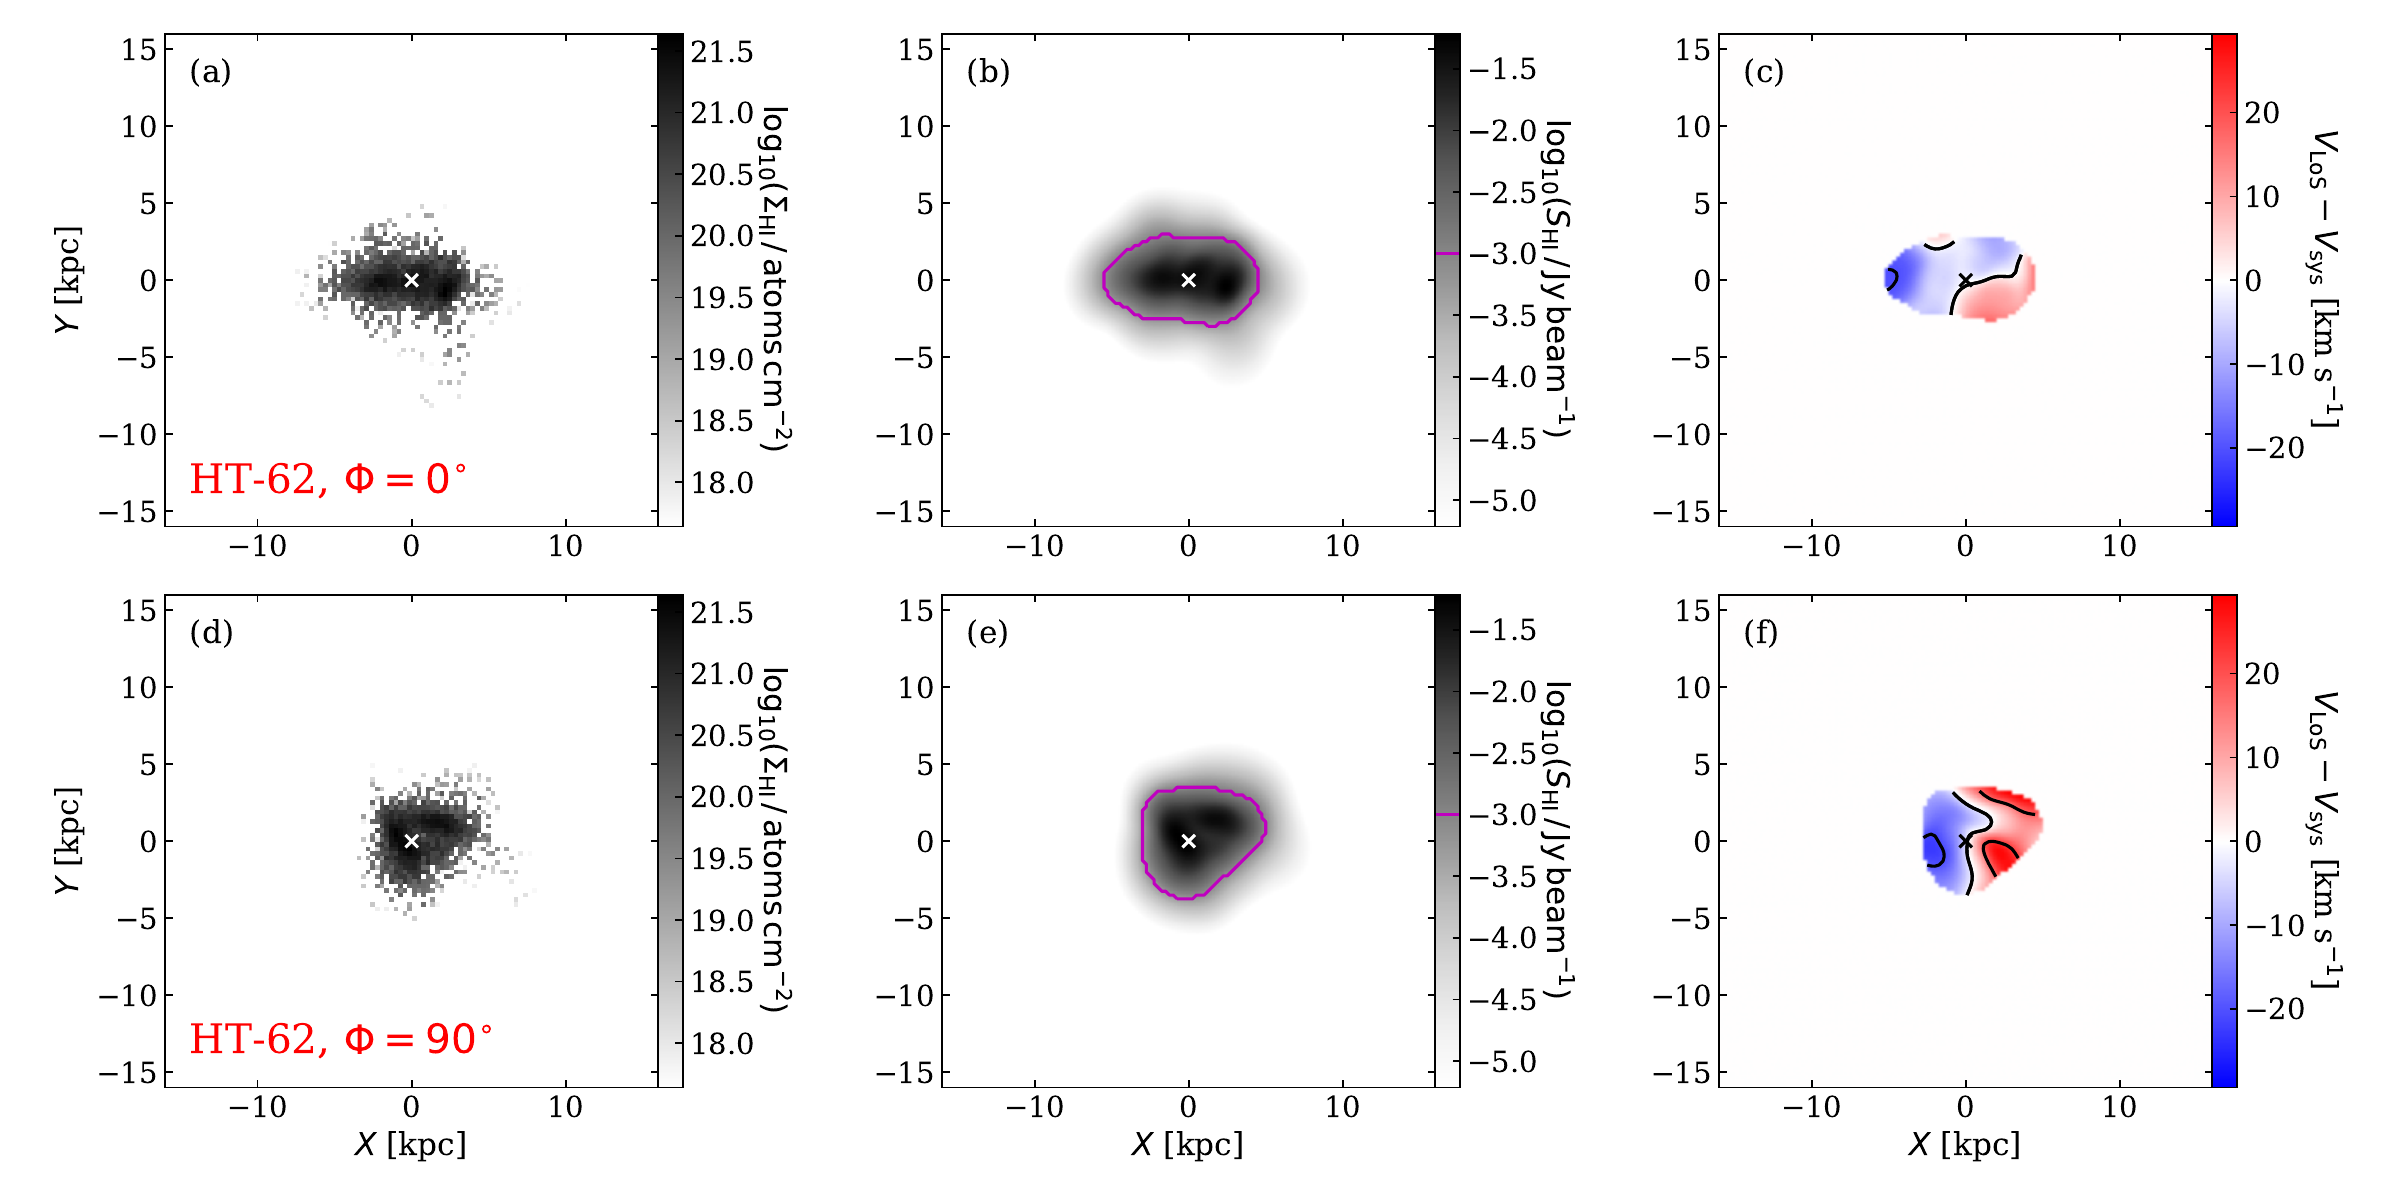}
\end{minipage}
\begin{minipage}{.4\textwidth}
\includegraphics[width=\textwidth]{../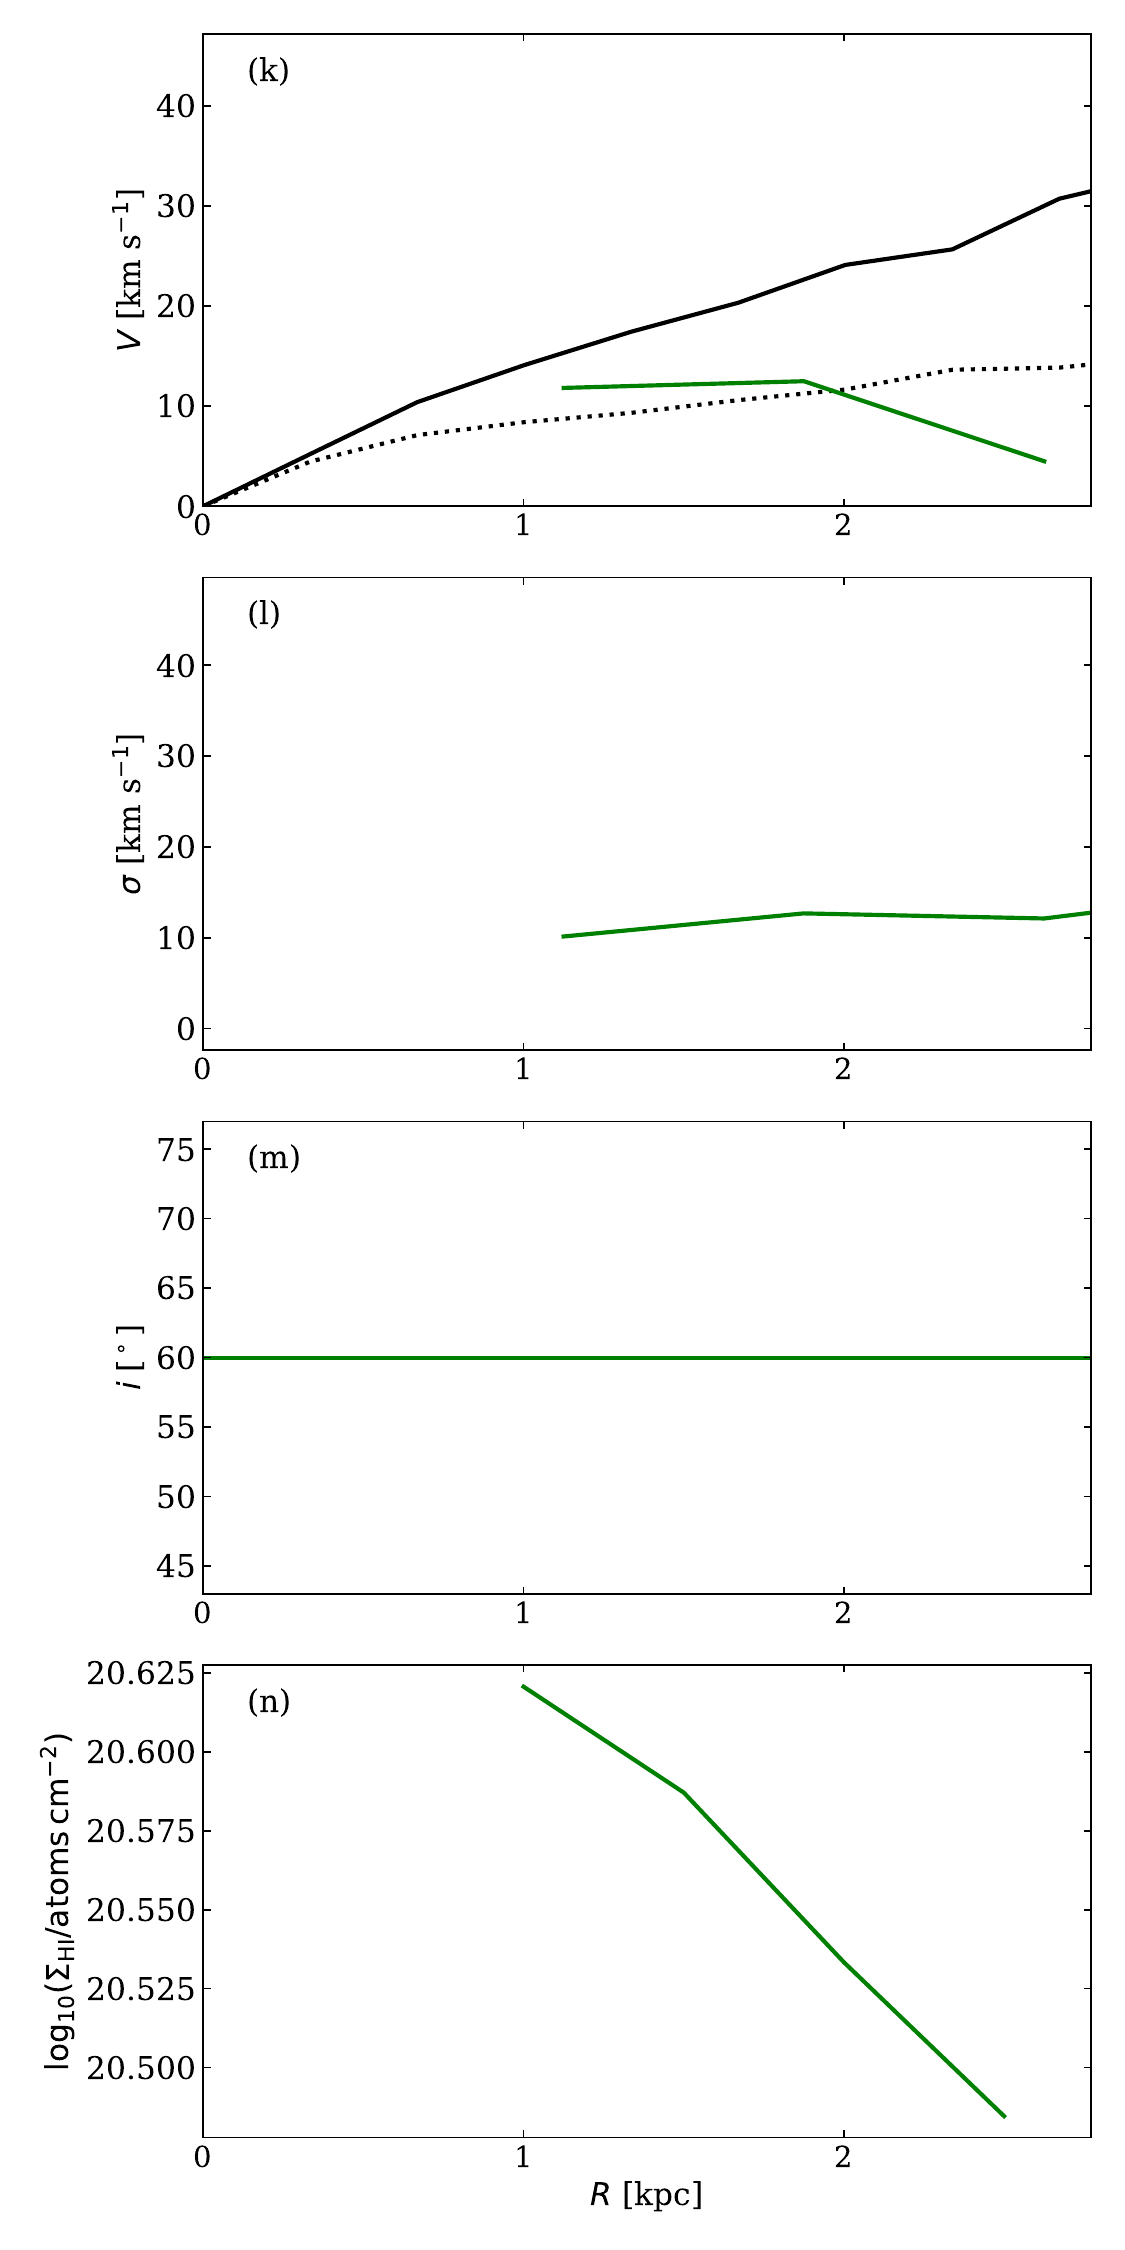}
\end{minipage}
\caption{A set of summary figures for galaxy HT-62, excluded from kinematic analysis. These include example moment maps for two orientations (panels (a)--(f); similar to Fig.~\ref{fig:visualisations}) and a summary of the rotation curve analysis from $24$ viewing angles (panels (k)--(n); similar to Fig.~\ref{fig:rot_curves}). See description of Appendix~\ref{app:supplementary} for details.}
\label{fig:S87}
\end{figure}
\clearpage

\begin{figure}
\begin{minipage}{.9\textwidth}
\includegraphics[width=\textwidth]{../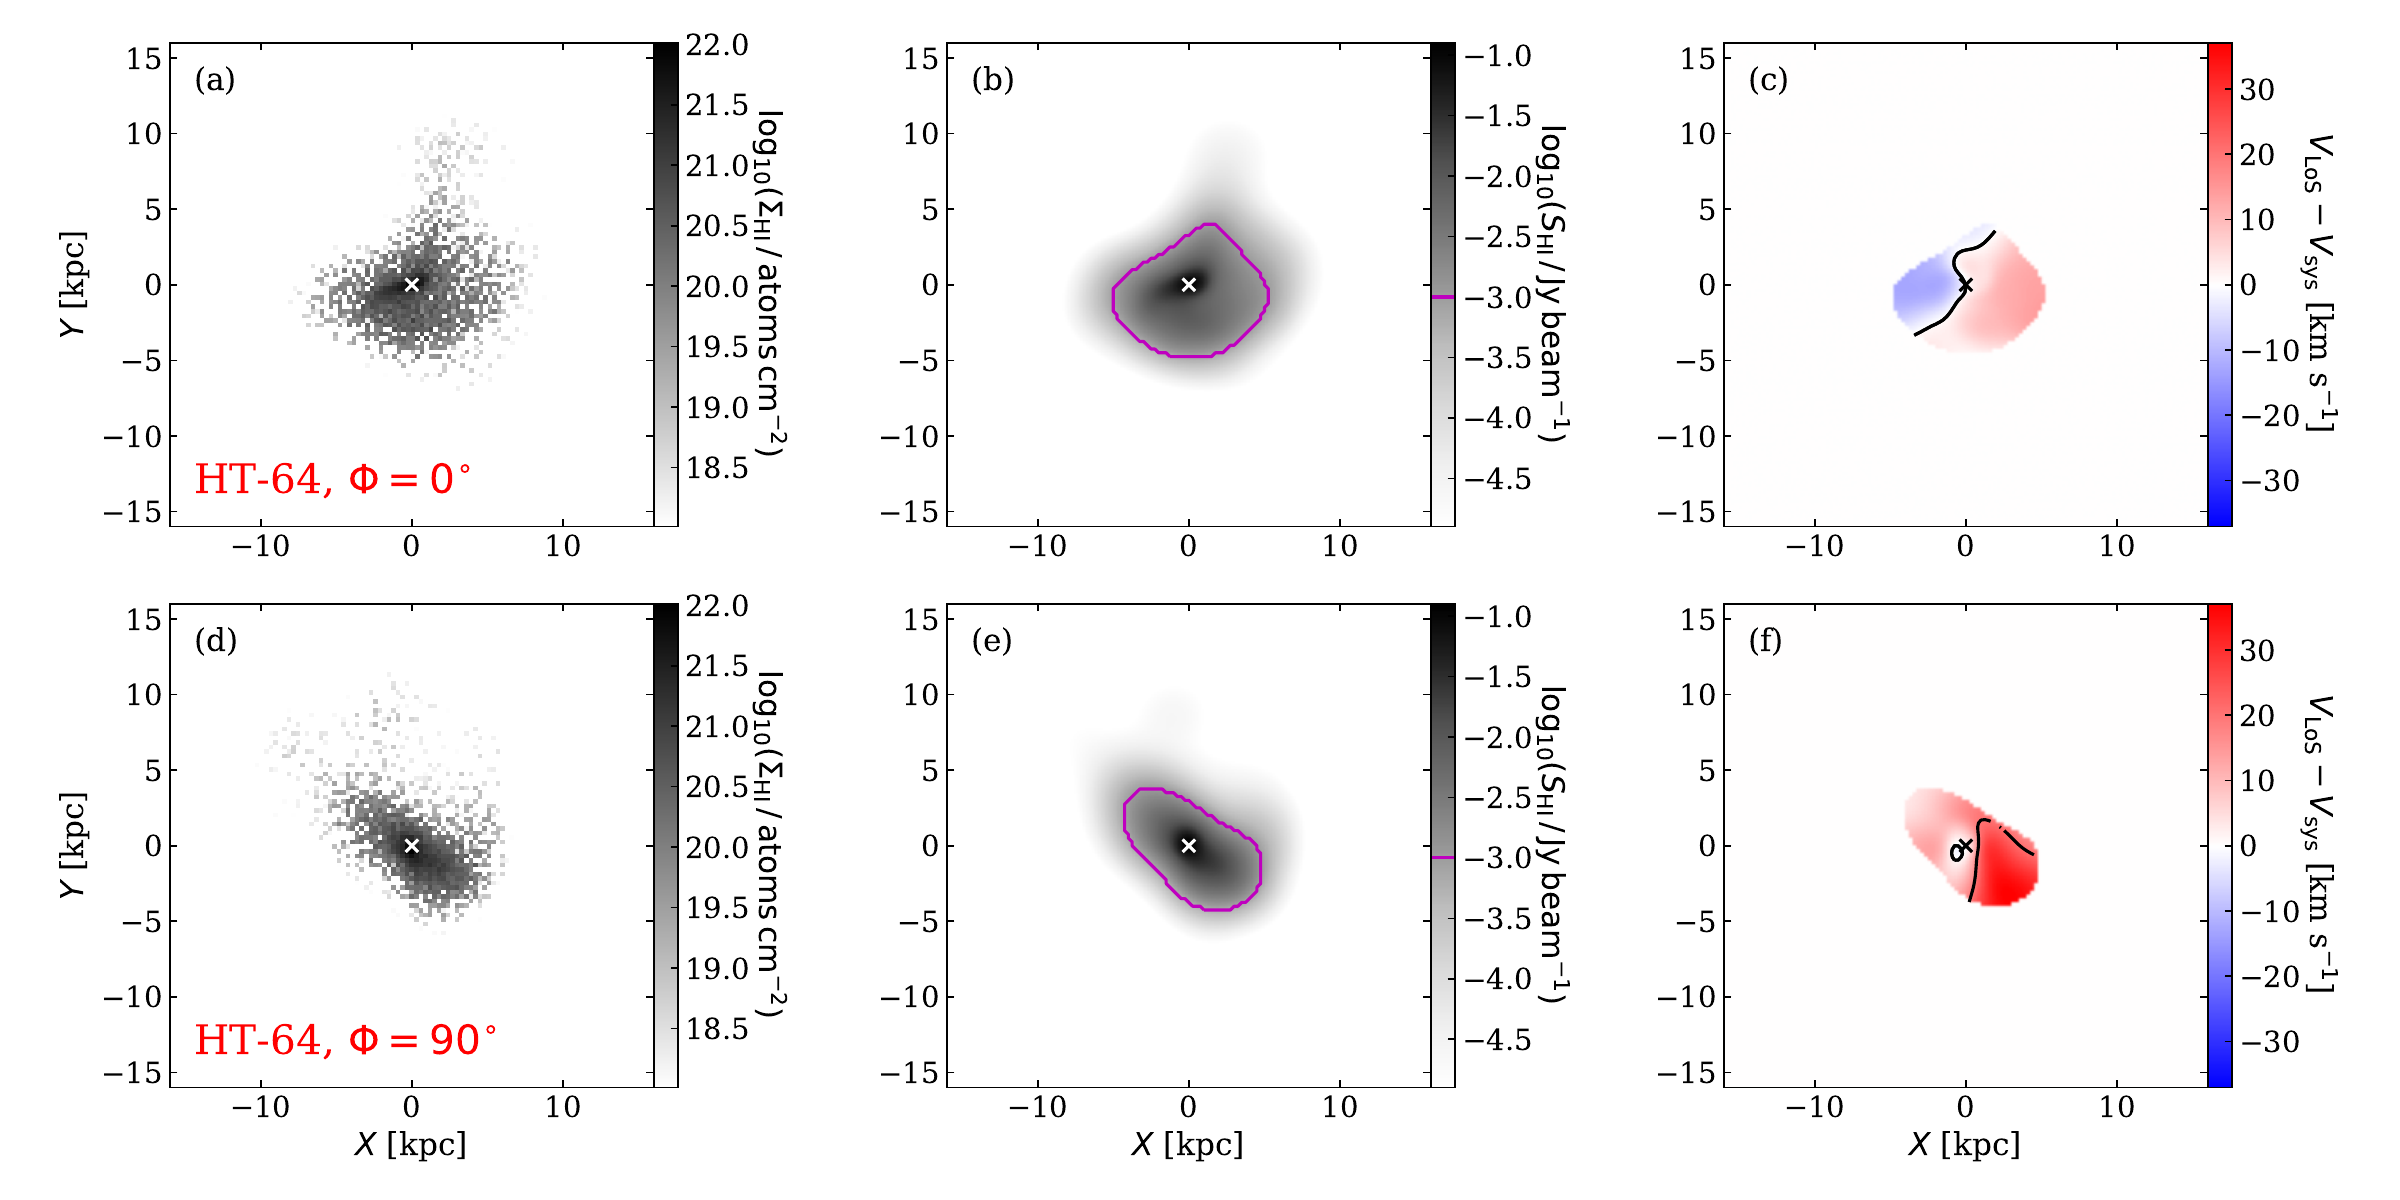}
\includegraphics[width=\textwidth]{../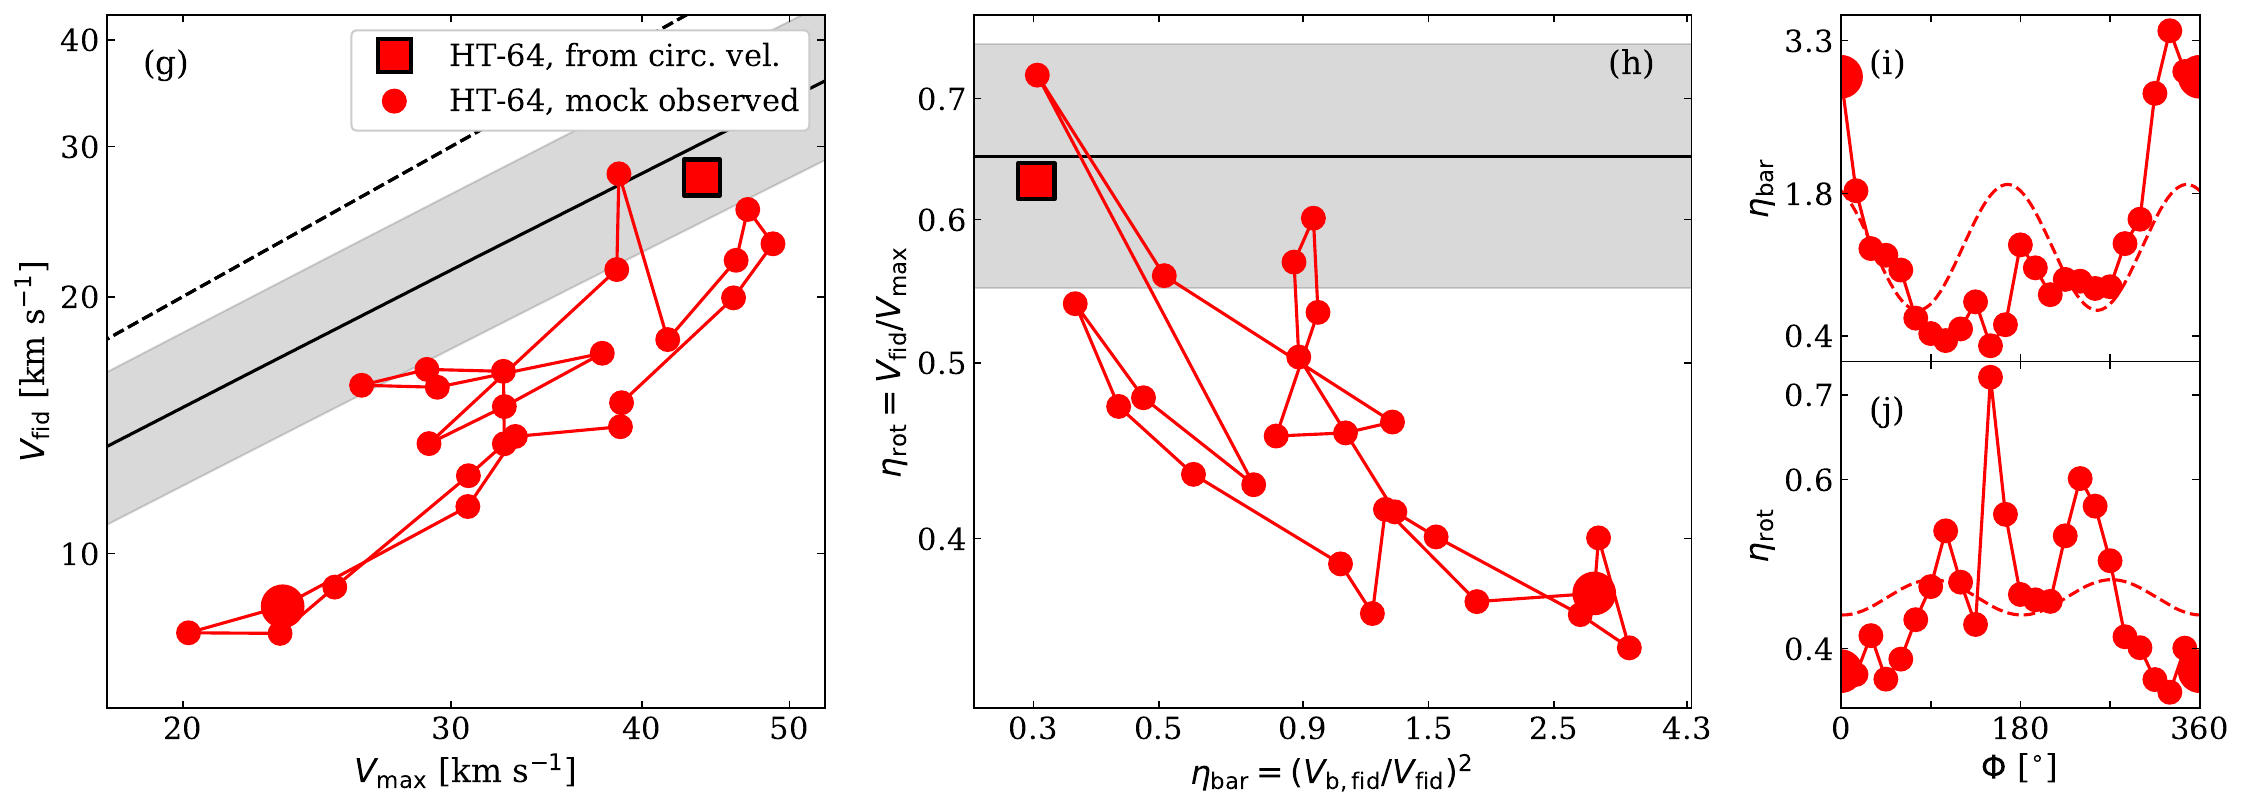}
\end{minipage}
\begin{minipage}{.4\textwidth}
\includegraphics[width=\textwidth]{../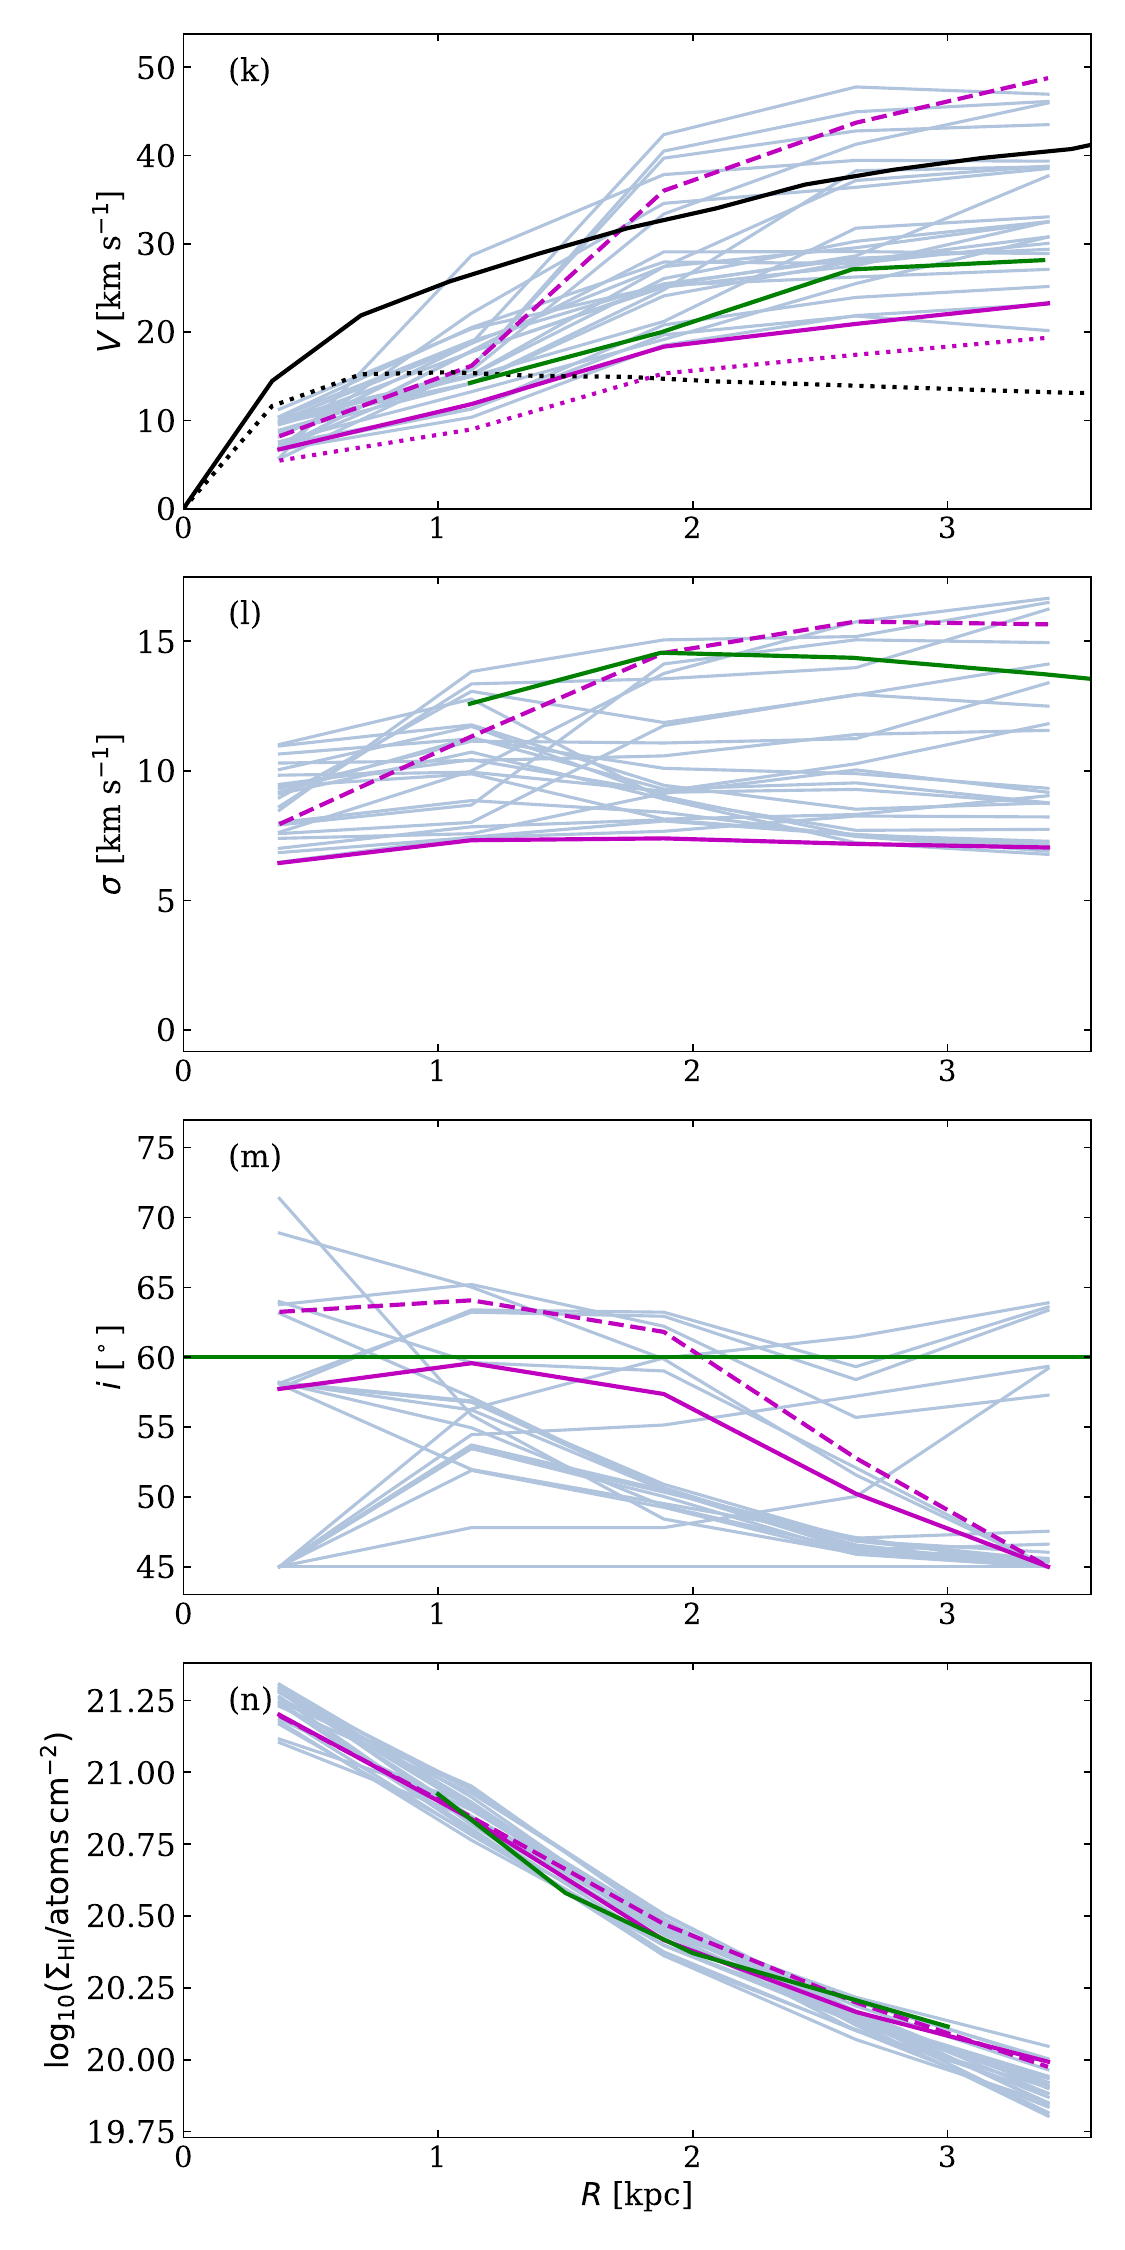}
\end{minipage}
\caption{A set of summary figures for galaxy HT-64, excluded from kinematic analysis. These include example moment maps for two orientations (panels (a)--(f); similar to Fig.~\ref{fig:visualisations}), a summary of the parameters $V_\mathrm{fid}$, $V_\mathrm{max}$, $\eta_\mathrm{rot}$, and $\eta_\mathrm{bar}$ (panels (g)--(j); similar to Fig.~\ref{fig:loops}), and a summary of the rotation curve analysis from $24$ viewing angles (panels (k)--(n); similar to Fig.~\ref{fig:rot_curves}). See description of Appendix~\ref{app:supplementary} for details.}
\label{fig:S88}
\end{figure}
\clearpage

\begin{figure}
\begin{minipage}{.9\textwidth}
\includegraphics[width=\textwidth]{../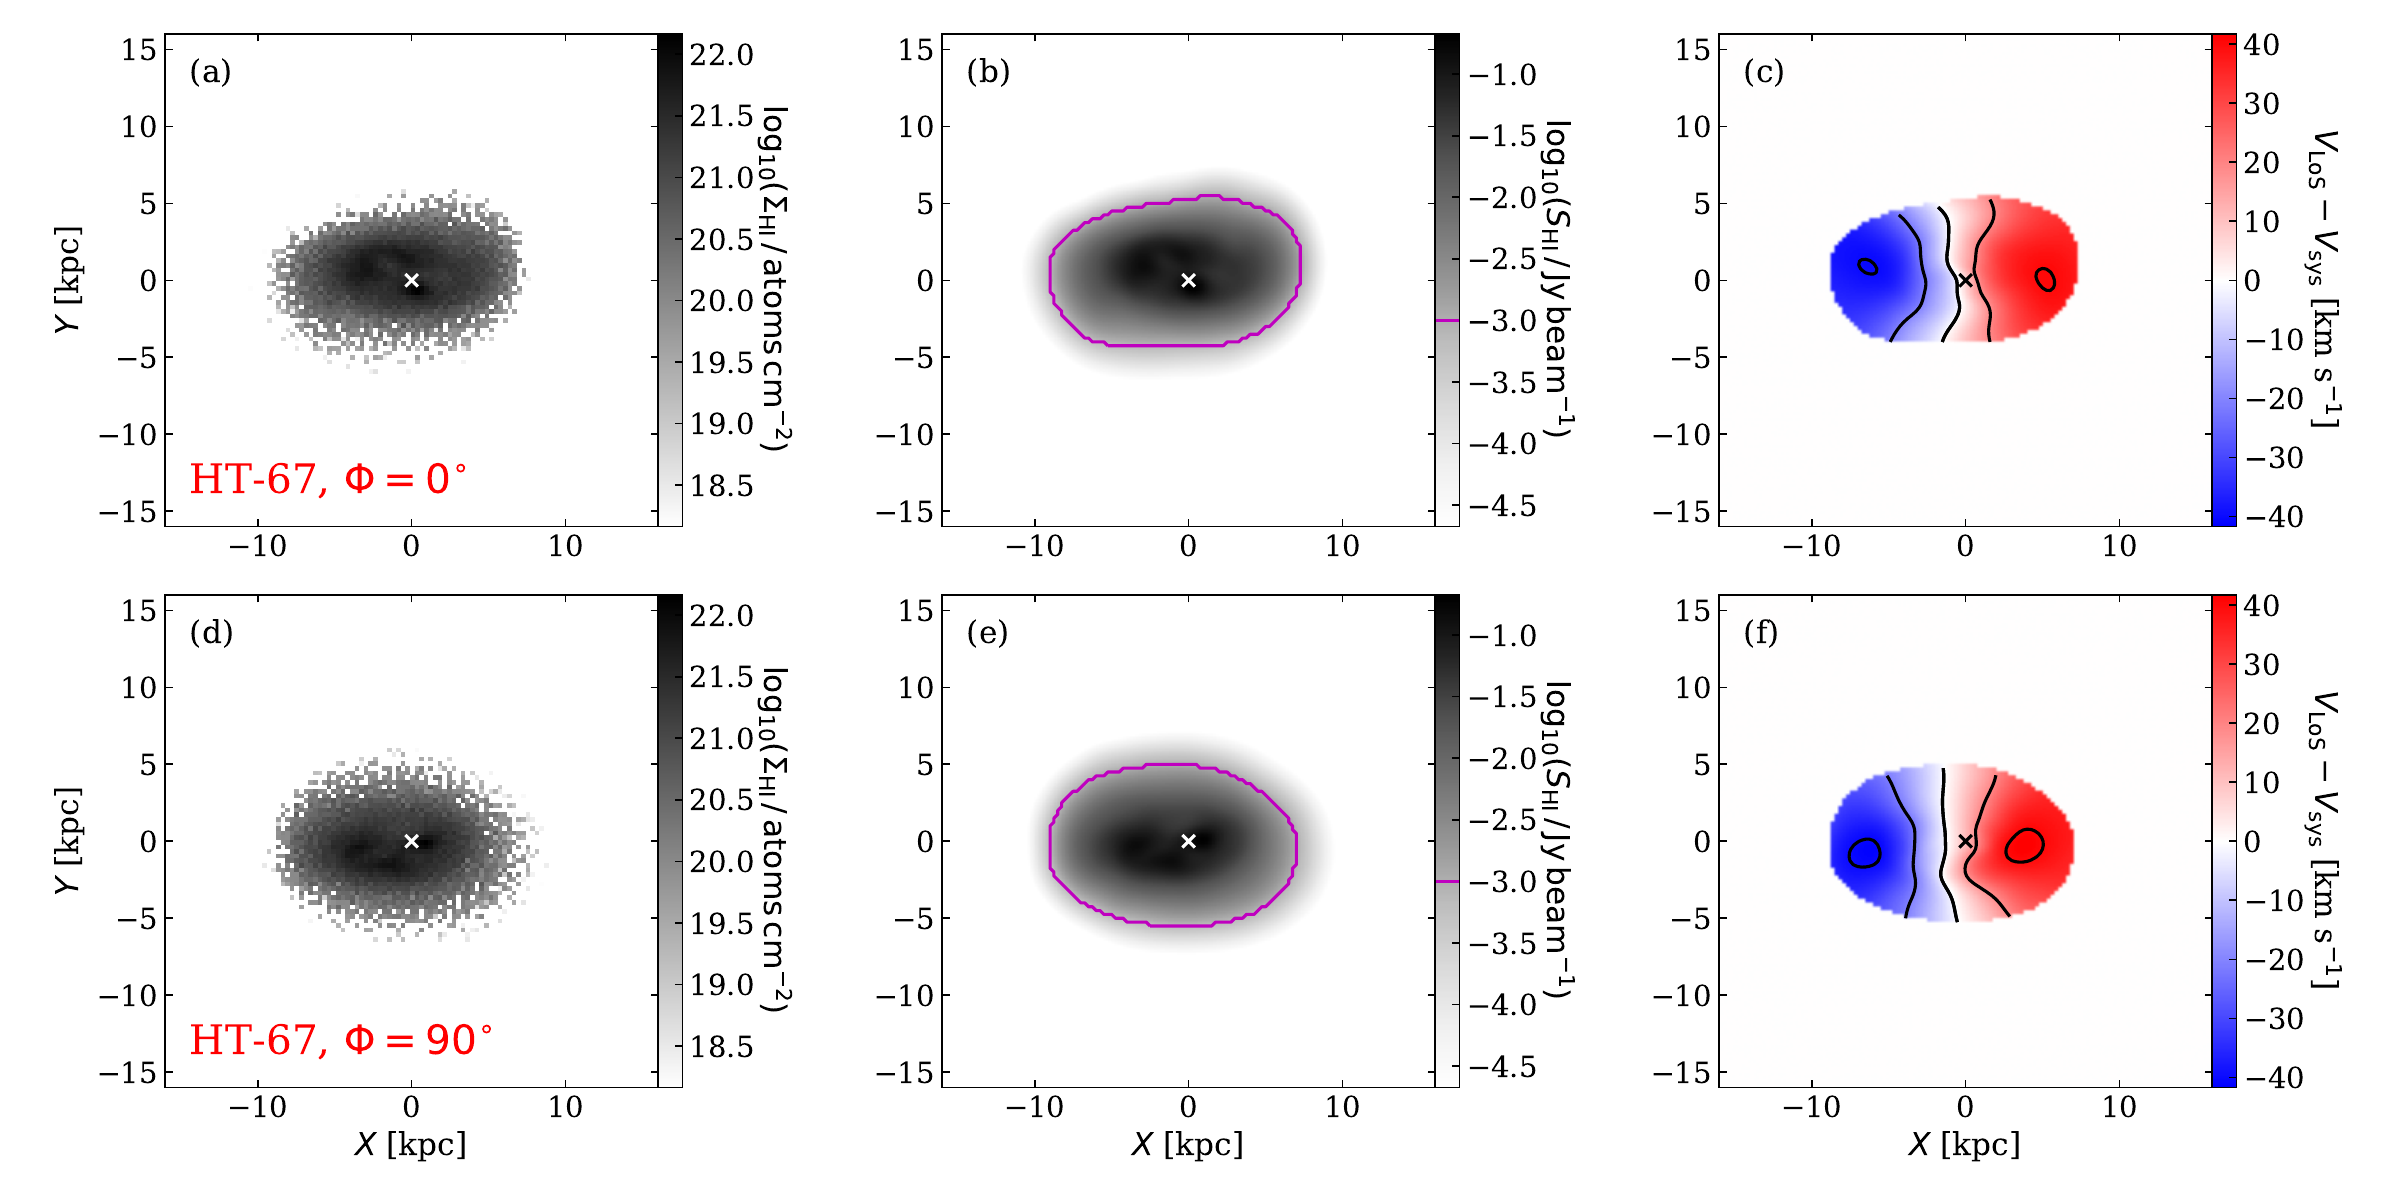}
\includegraphics[width=\textwidth]{../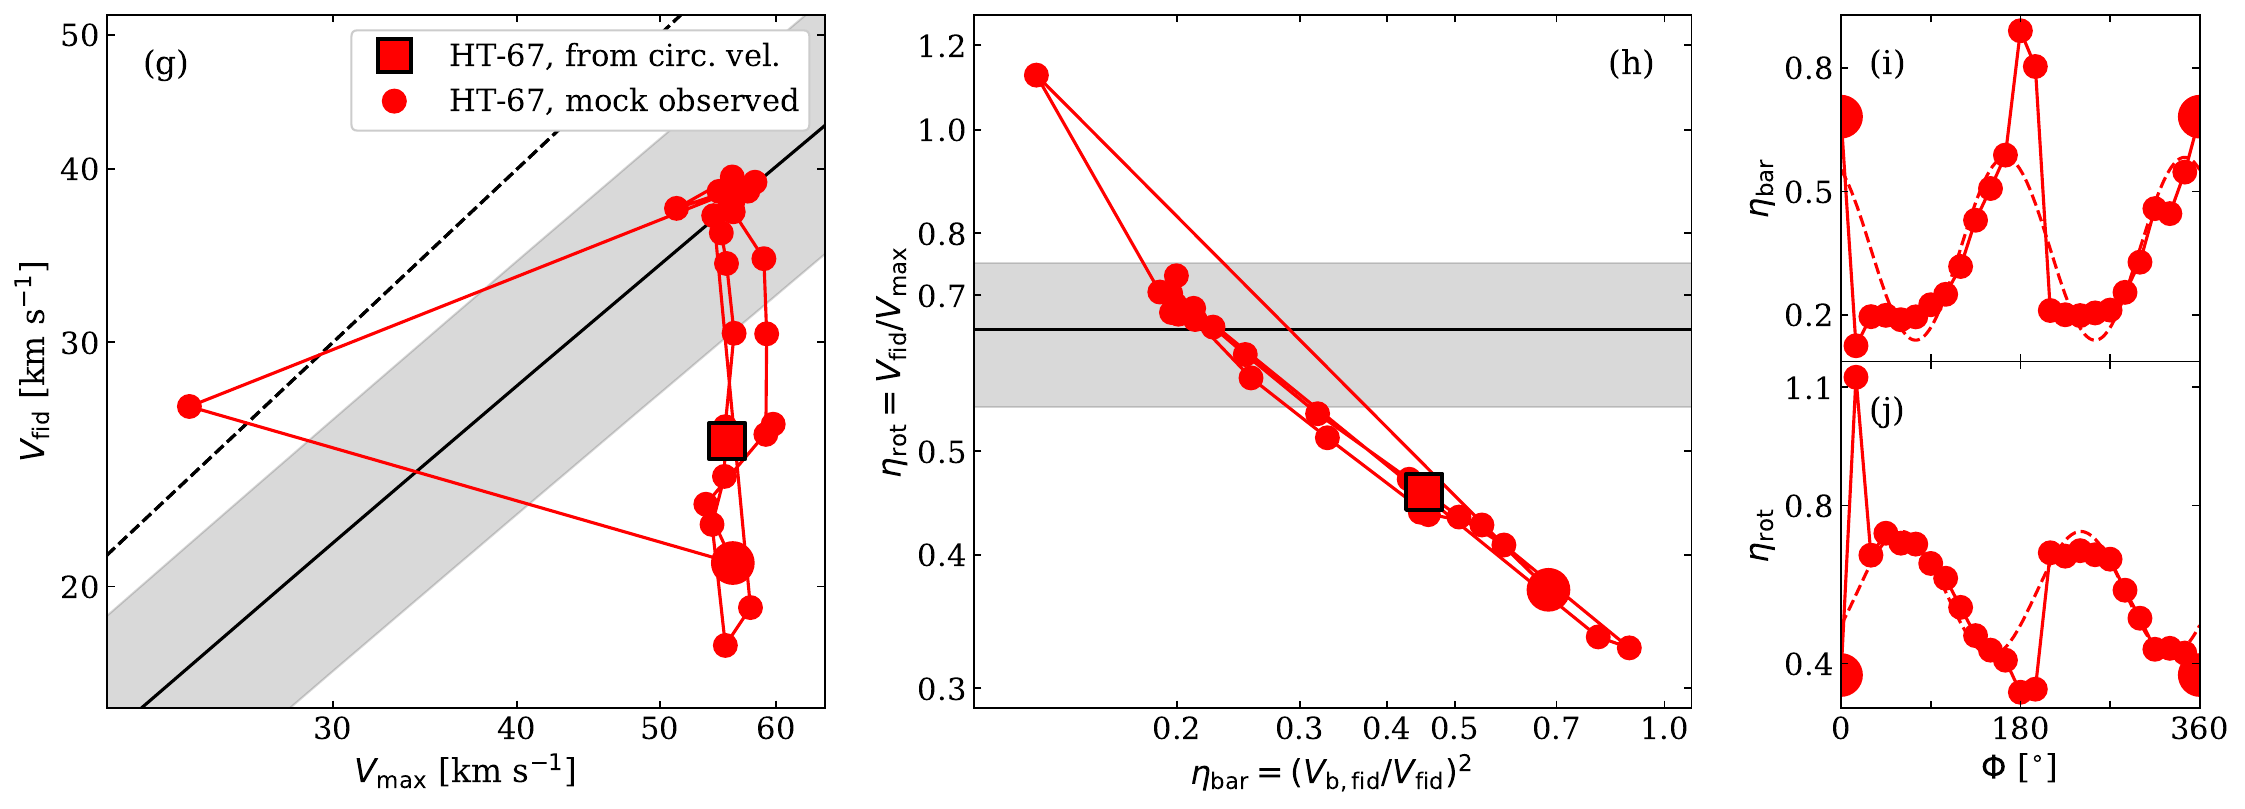}
\end{minipage}
\begin{minipage}{.4\textwidth}
\includegraphics[width=\textwidth]{../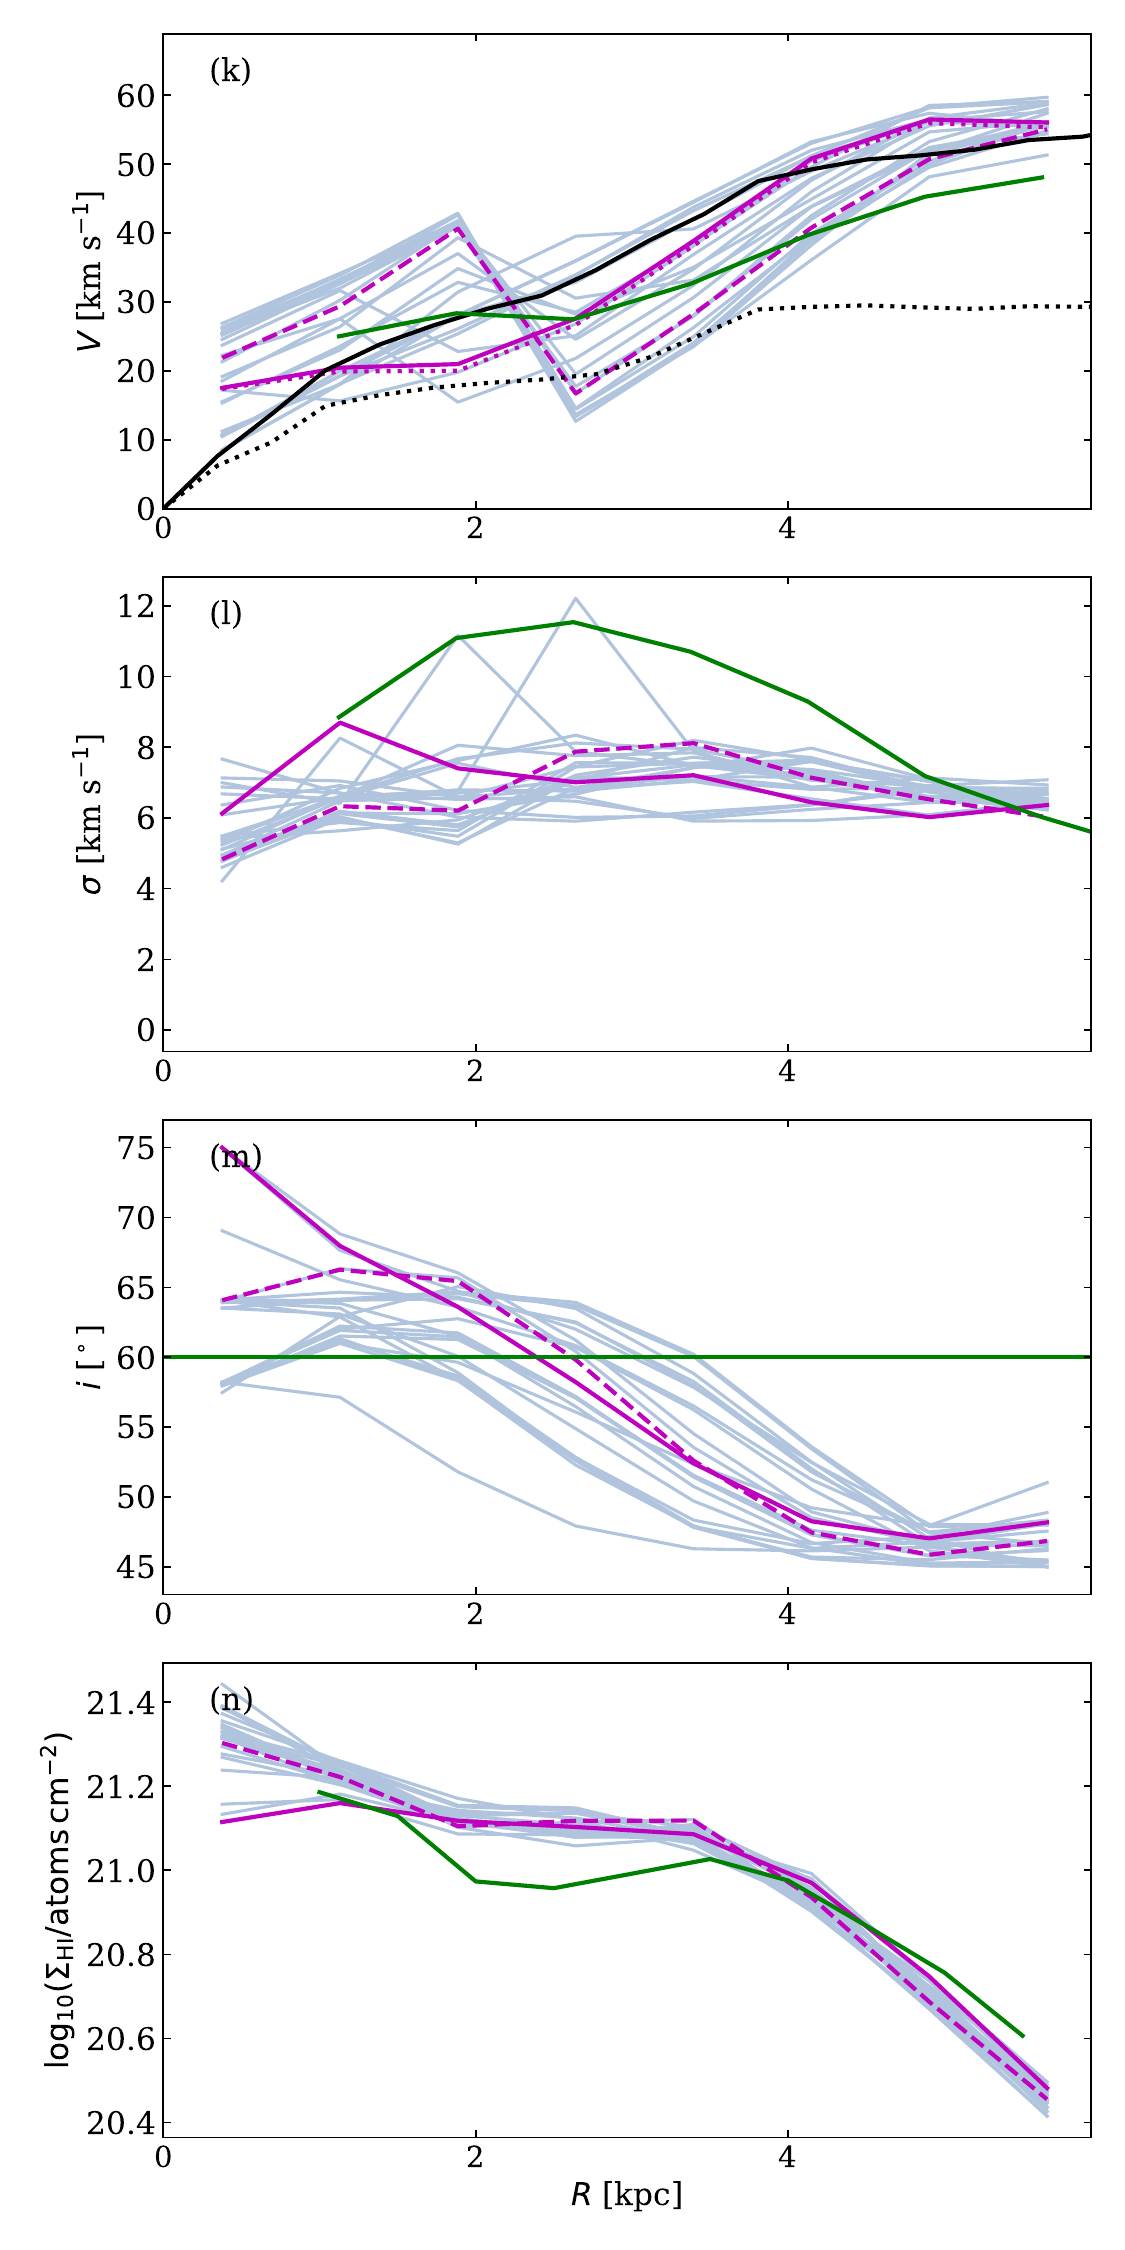}
\end{minipage}
\caption{A set of summary figures for galaxy HT-67, excluded from kinematic analysis. These include example moment maps for two orientations (panels (a)--(f); similar to Fig.~\ref{fig:visualisations}), a summary of the parameters $V_\mathrm{fid}$, $V_\mathrm{max}$, $\eta_\mathrm{rot}$, and $\eta_\mathrm{bar}$ (panels (g)--(j); similar to Fig.~\ref{fig:loops}), and a summary of the rotation curve analysis from $24$ viewing angles (panels (k)--(n); similar to Fig.~\ref{fig:rot_curves}). See description of Appendix~\ref{app:supplementary} for details.}
\label{fig:S89}
\end{figure}
\clearpage
\end{landscape}

\bsp
\label{lastpage-appendix}
\end{document}
